# Supplementary material for: A Bayesian approach to the global estimation of maternal mortality
Source: arXiv:1511.03330 source file (2015-11-10)
Supplement: Supplementary file 1 [file AOAS_suppl_fig1.pdf]

Afghanistan [AFG; B]  
(Southern Asia)

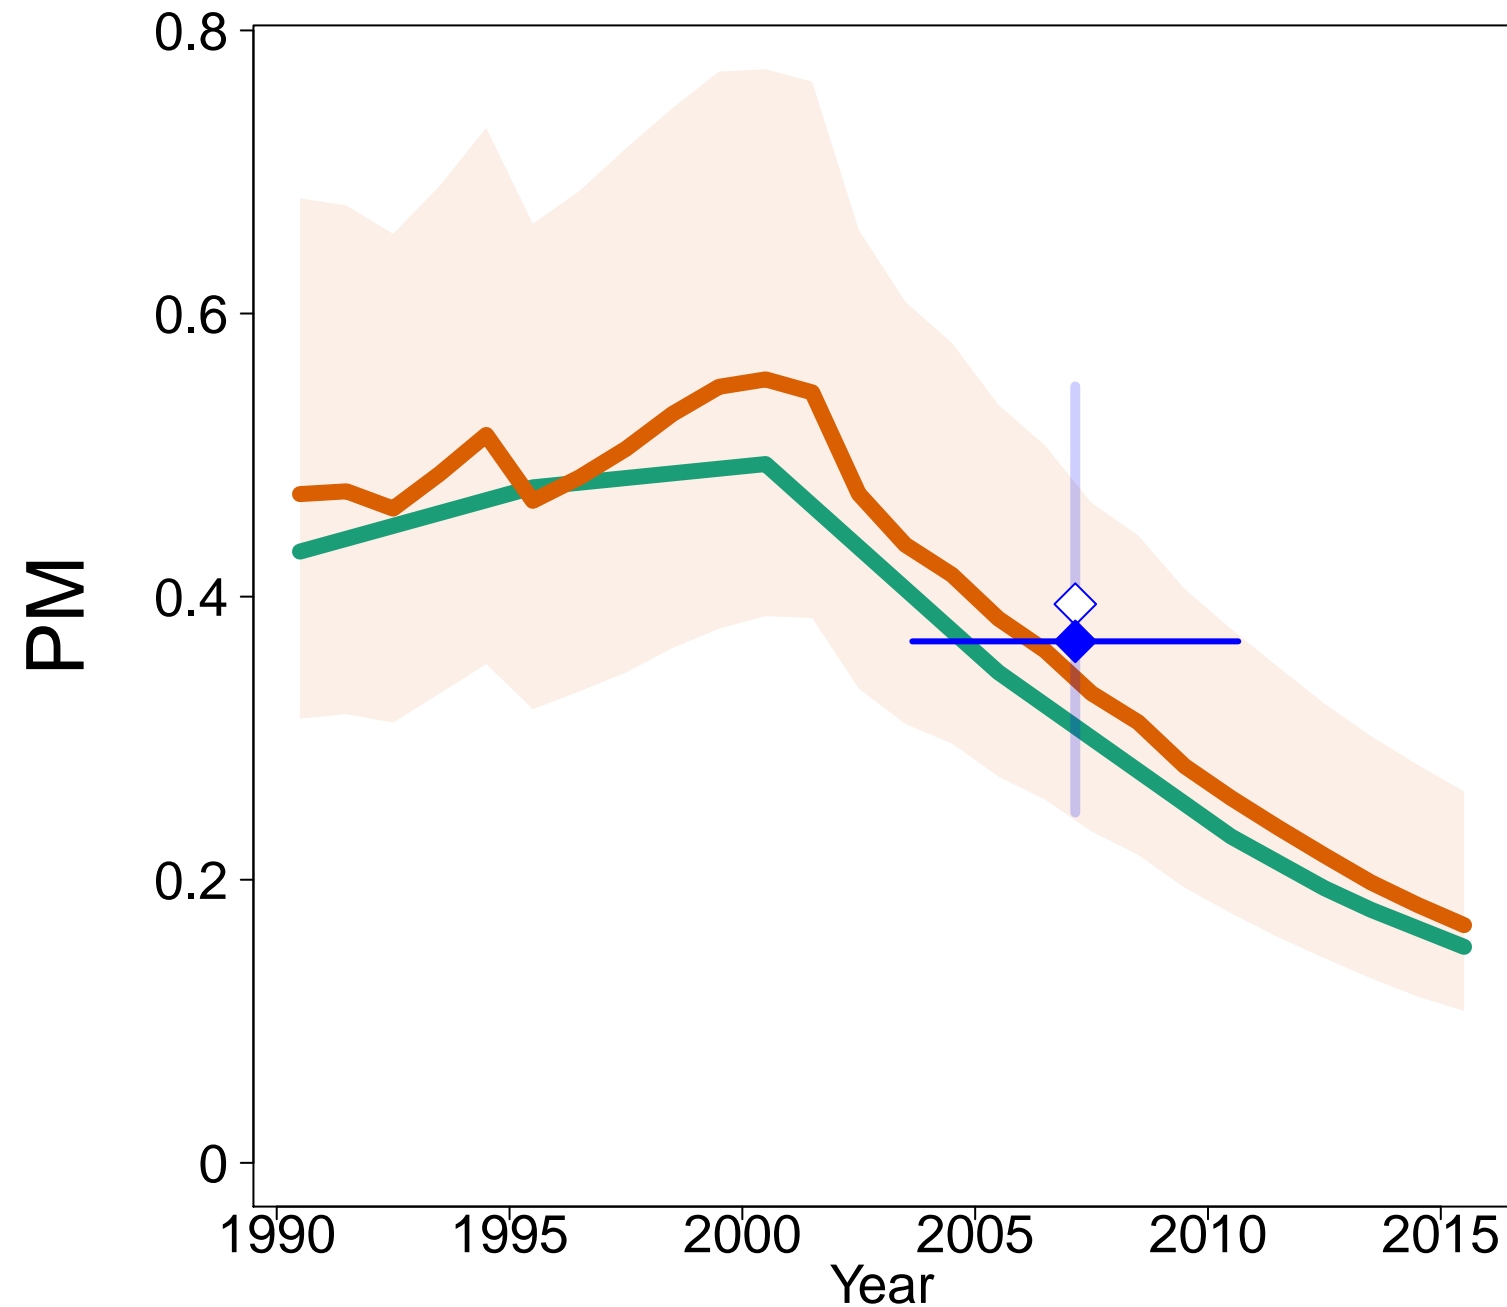

Afghanistan [AFG; B]  
(Southern Asia)

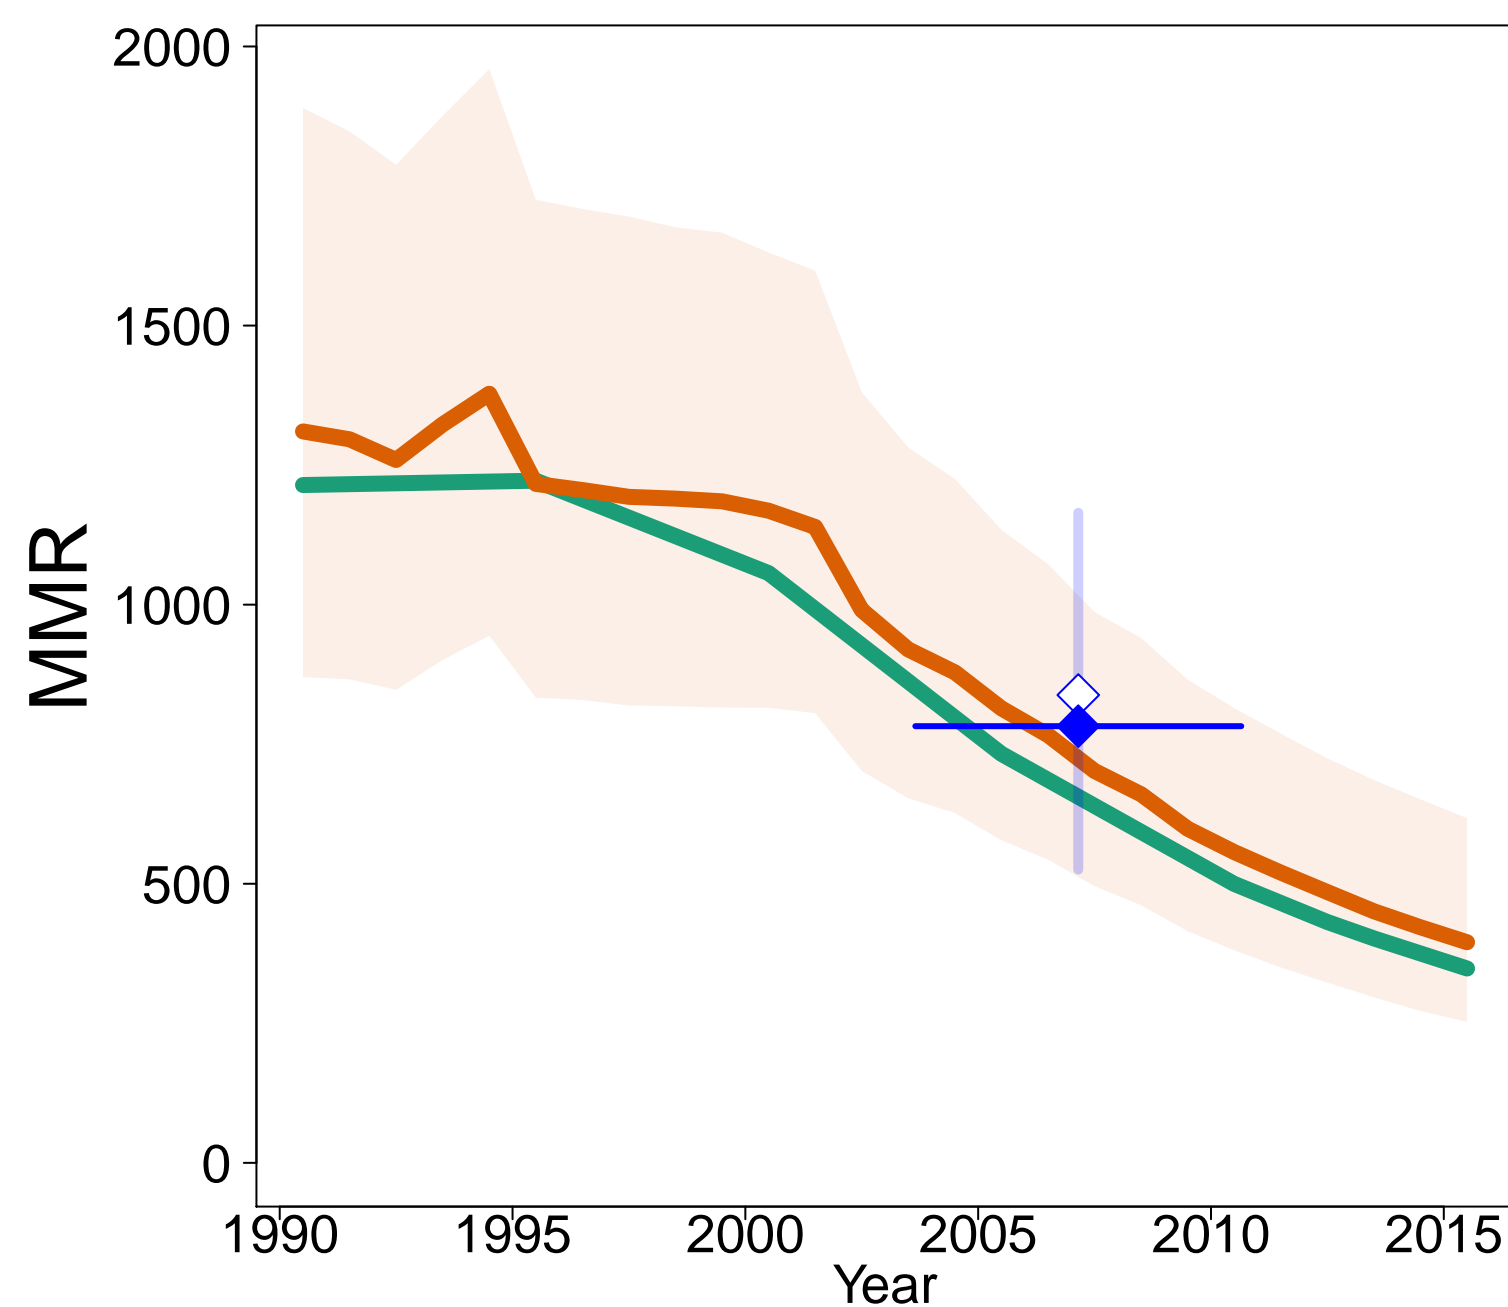

– Estimates –  
Bmat 2014  
MMEIG 2014  
– Data –  
Observed Data  
Adjusted Data  
– Data type –  
DHS

Albania [ALB; B]  
(Transition countries of South-Eastern Europe)

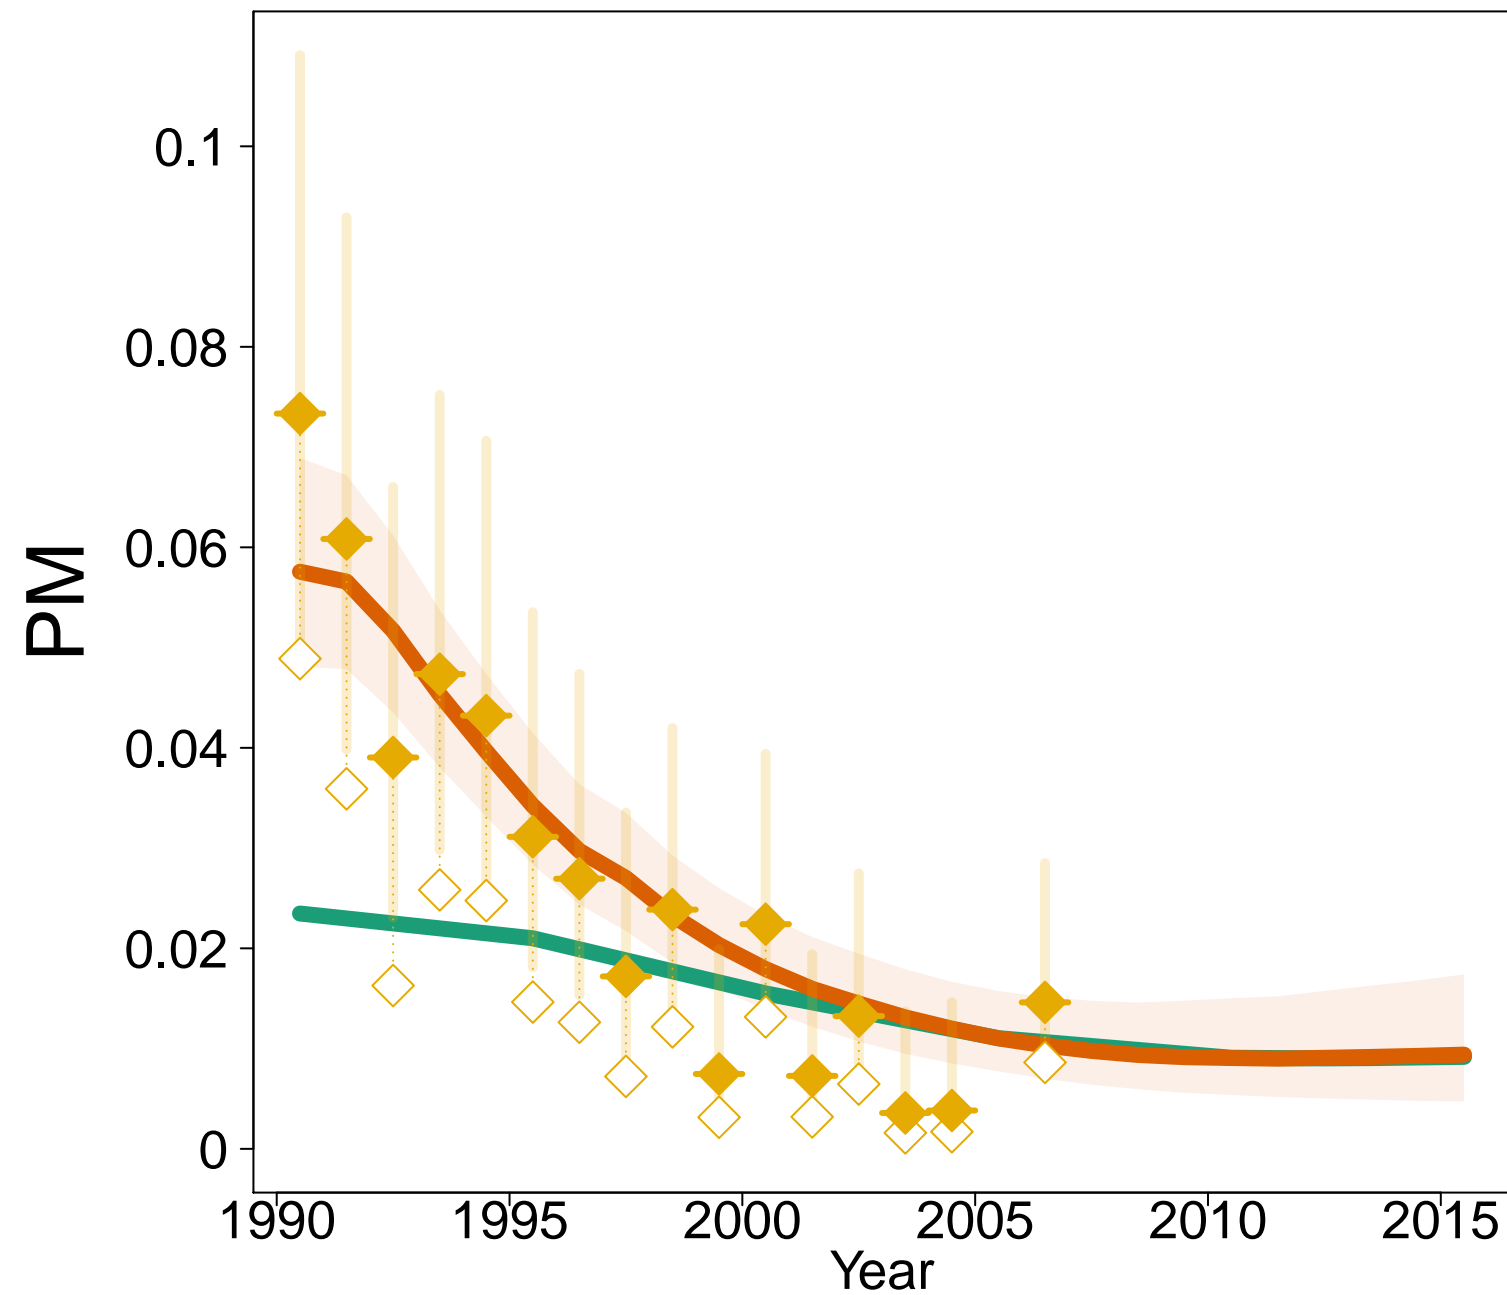

Albania [ALB; B]  
(Transition countries of South-Eastern Europe)

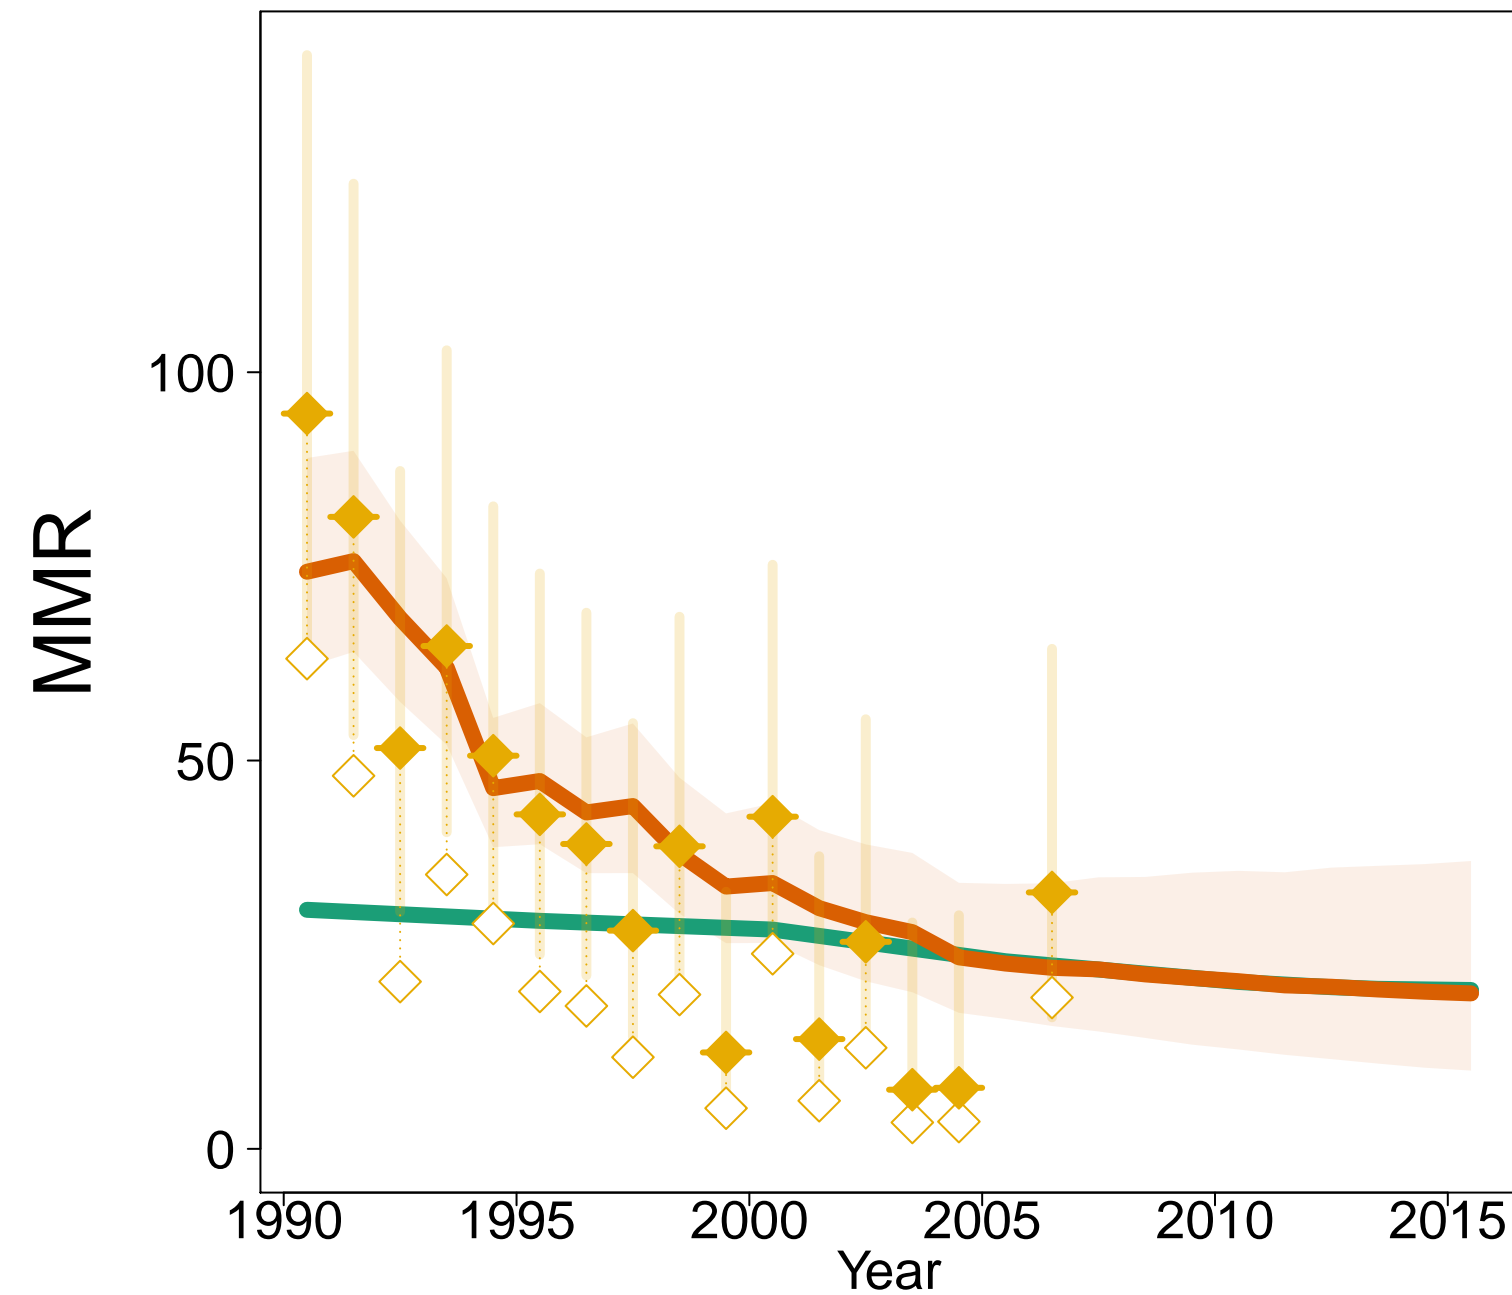

– Estimates –  
Bmat 2014  
MMEIG 2014  
– Data –  
Observed Data  
Adjusted Data  
– Data type –  
VR

Algeria [DZA; B]  
(Northern Africa)

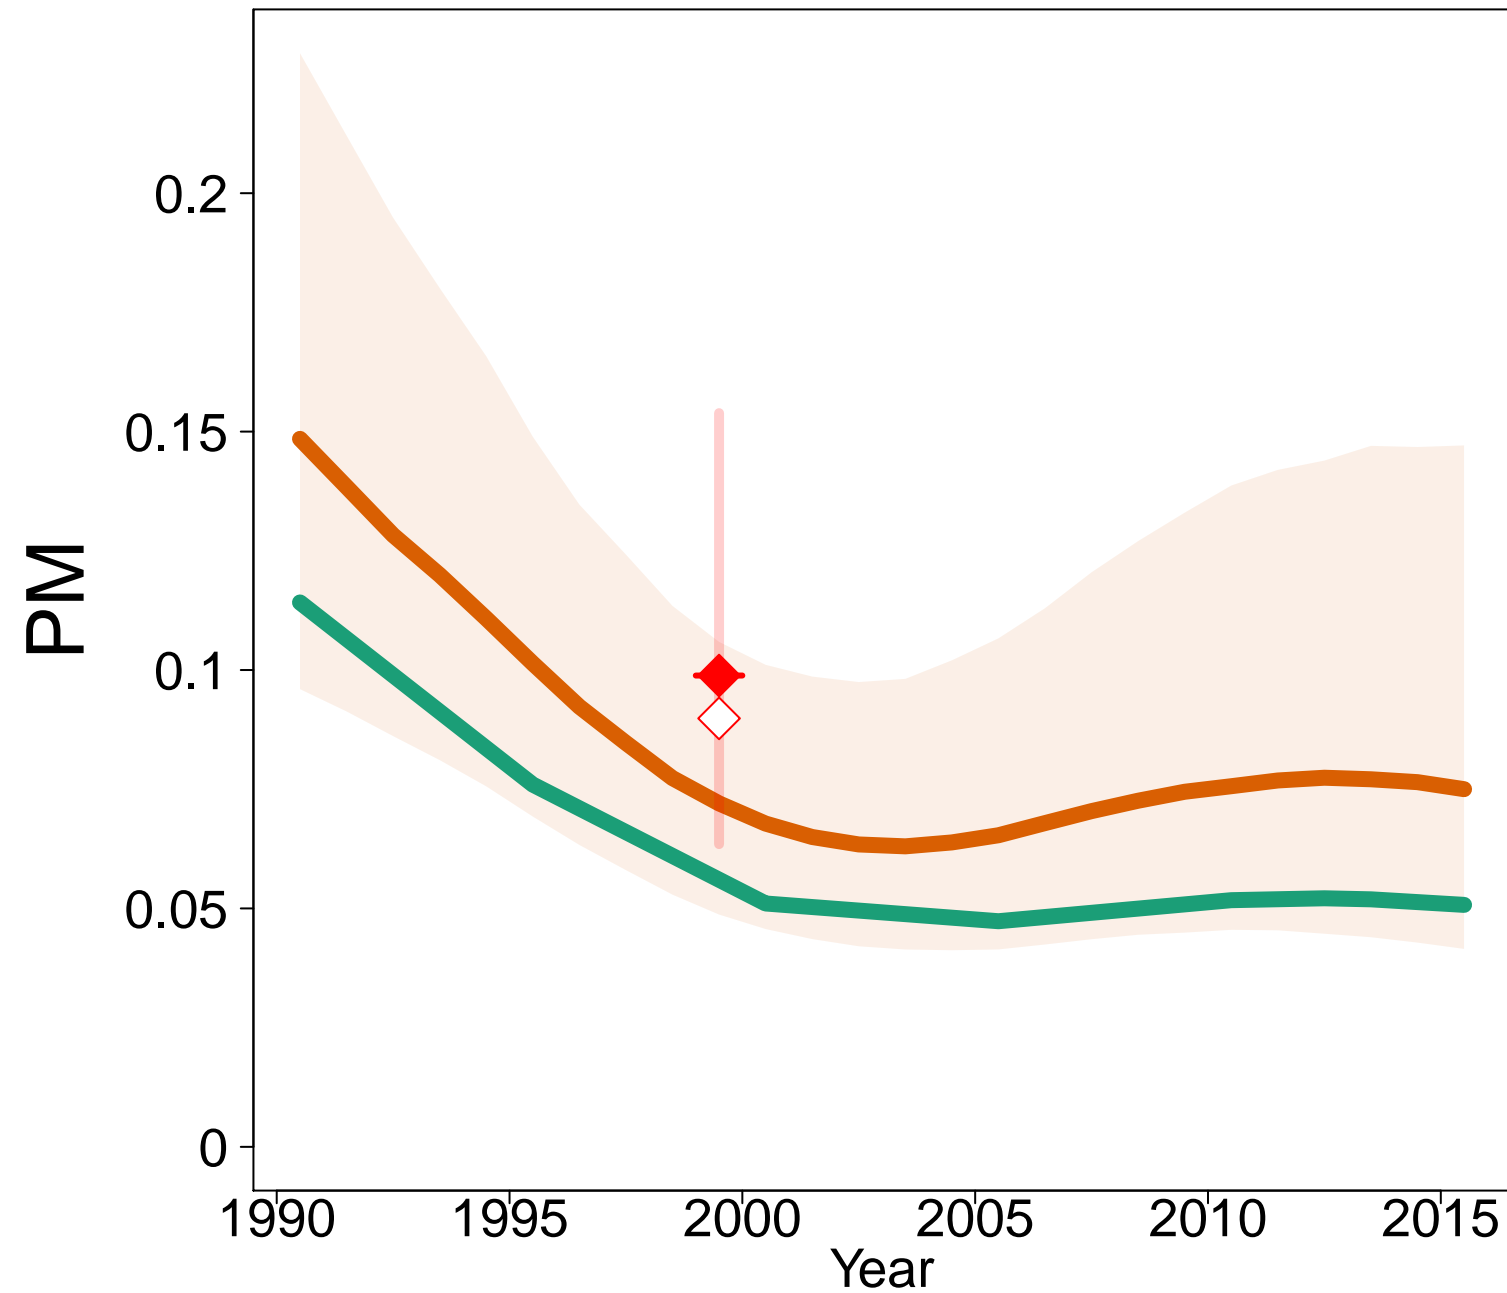

Algeria [DZA; B]  
(Northern Africa)

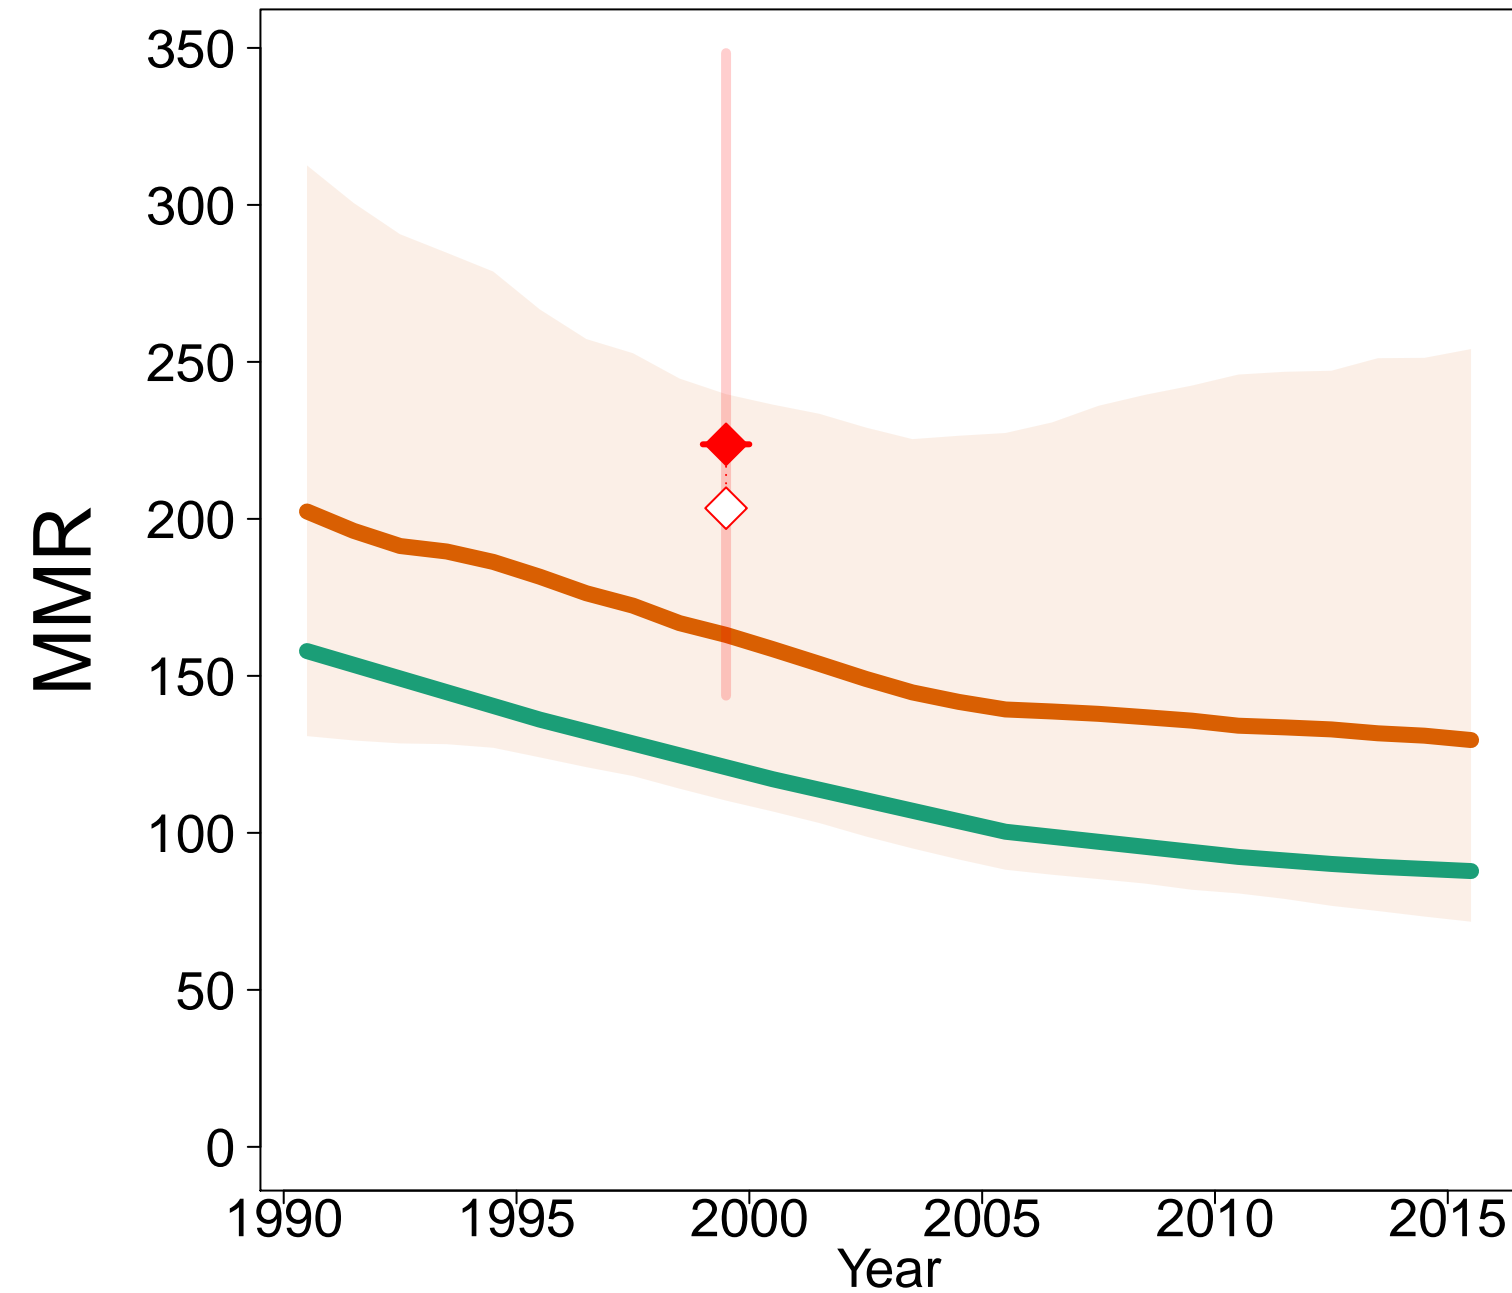

- Estimates –
- Bmat 2014
- MMEIG 2014
- Data –
- Observed Data
- Adjusted Data
- Data type –
- Misc. studies

Angola [AGO; C]  
(Middle Africa)

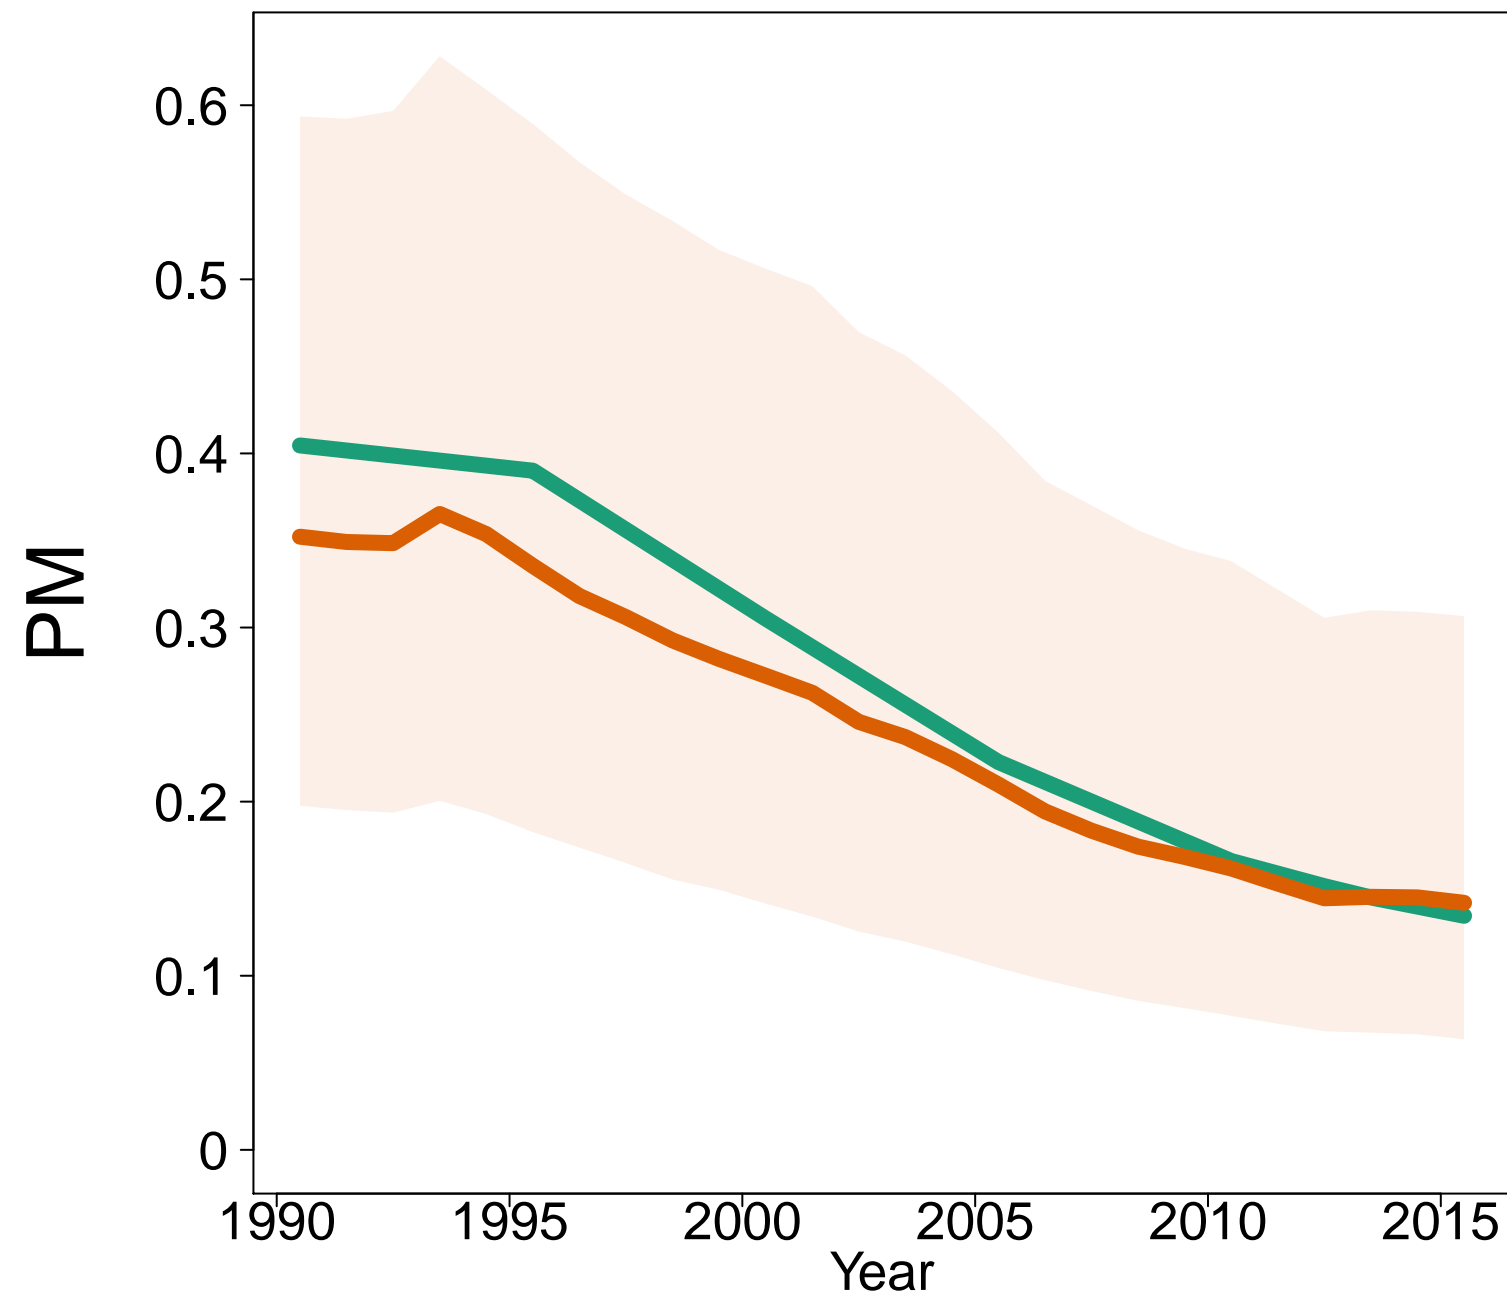

Angola [AGO; C]  
(Middle Africa)

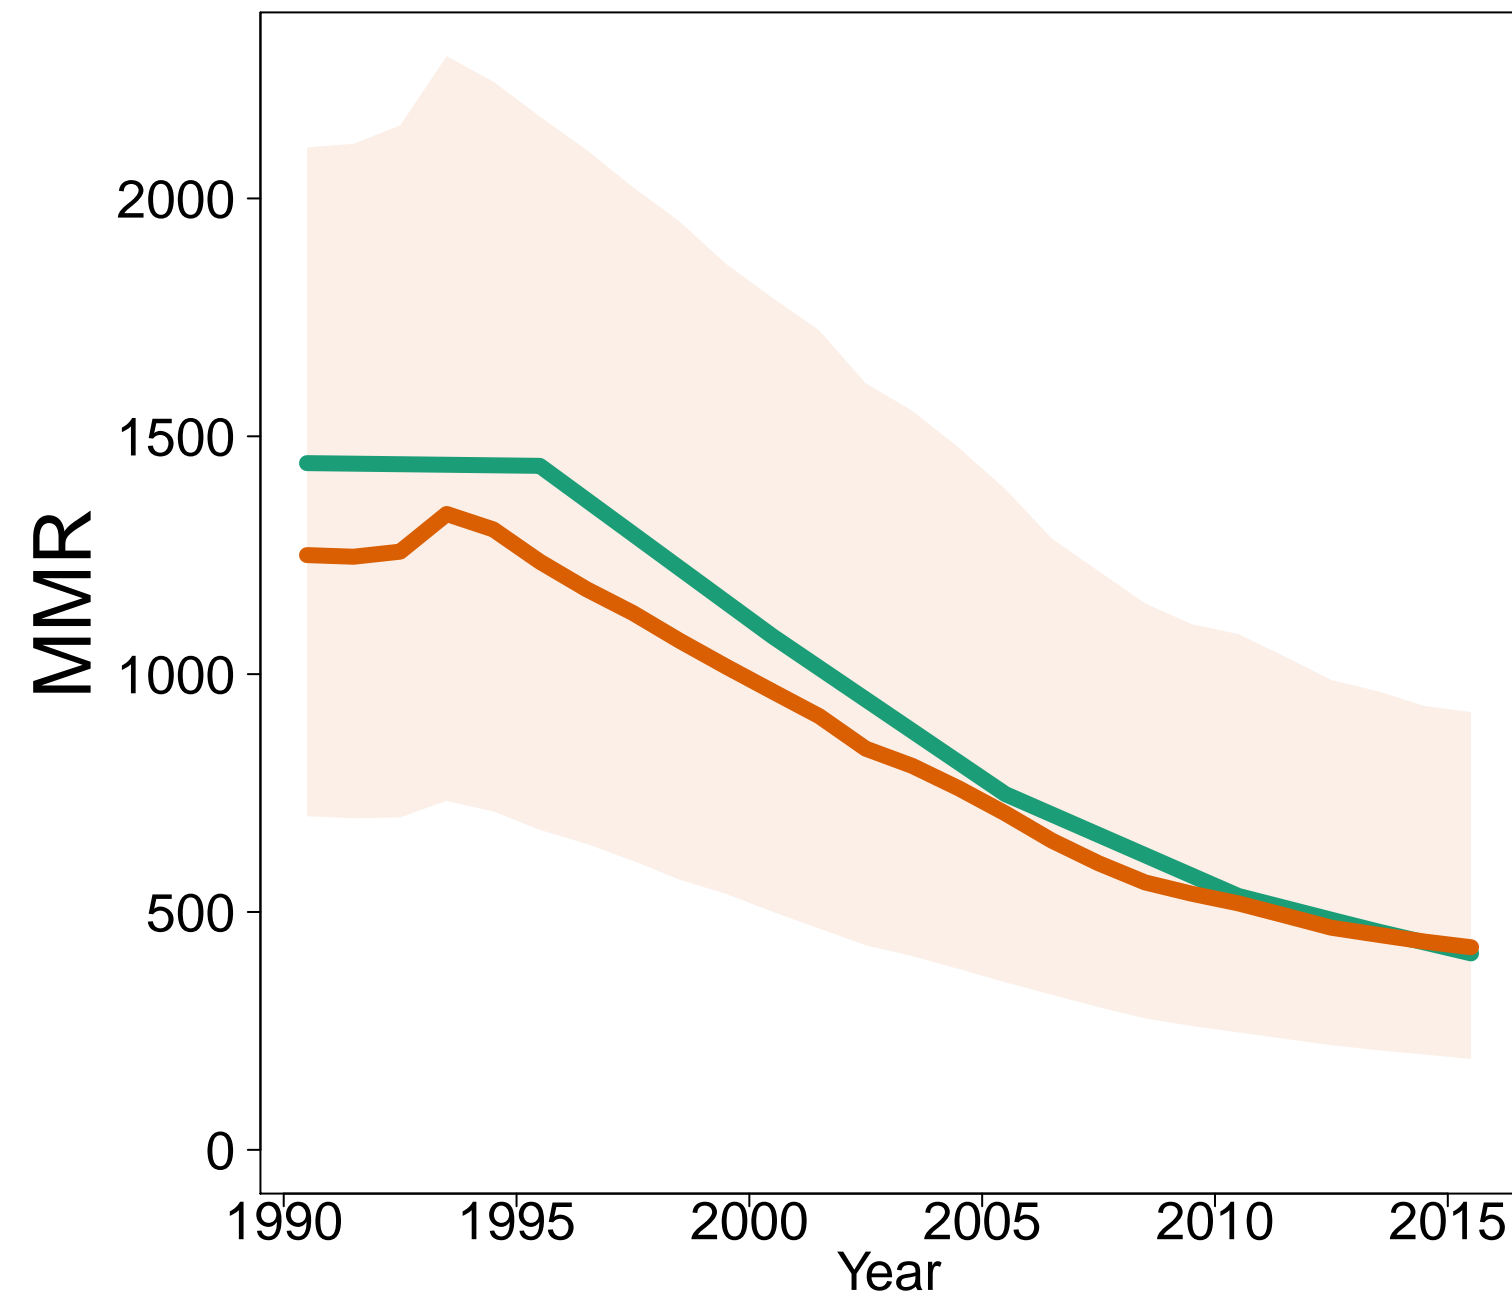

– Estimates –  
Bmat 2014  
MMEIG 2014  
– Data –

Argentina [ARG; A]  
(South America)

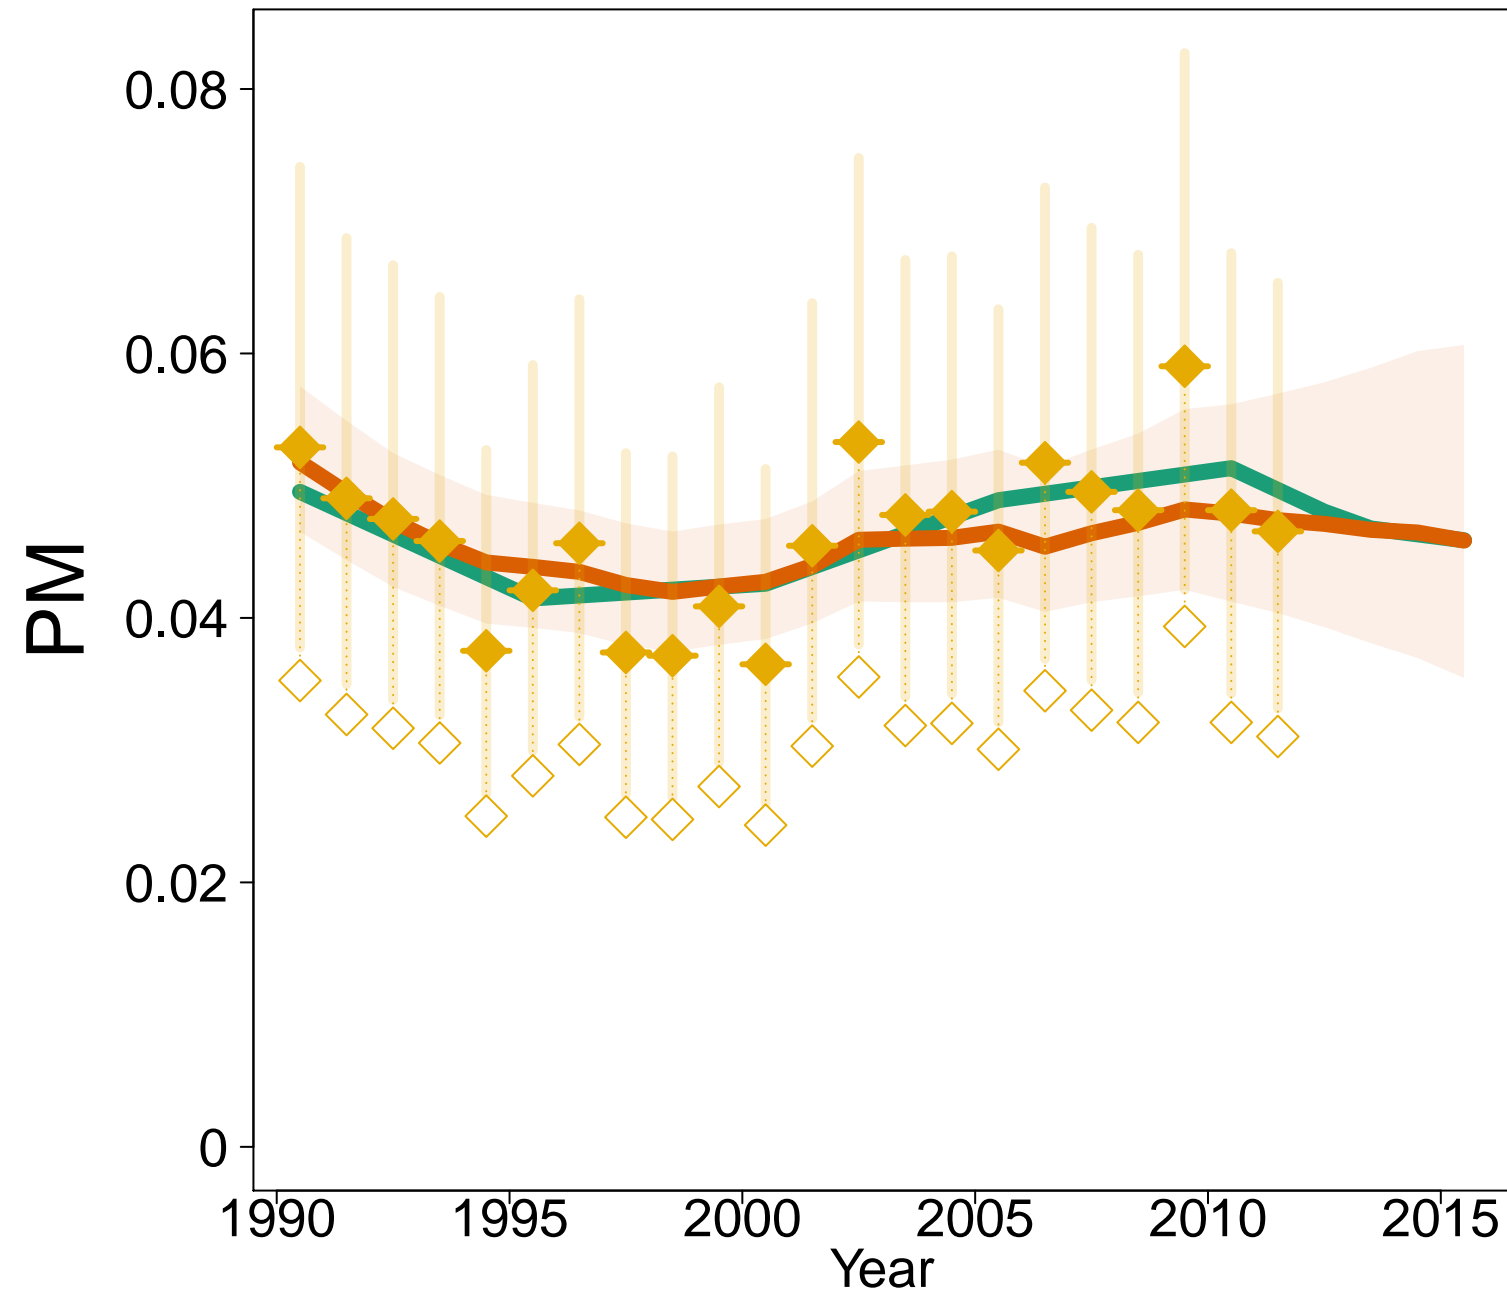

Argentina [ARG; A]  
(South America)

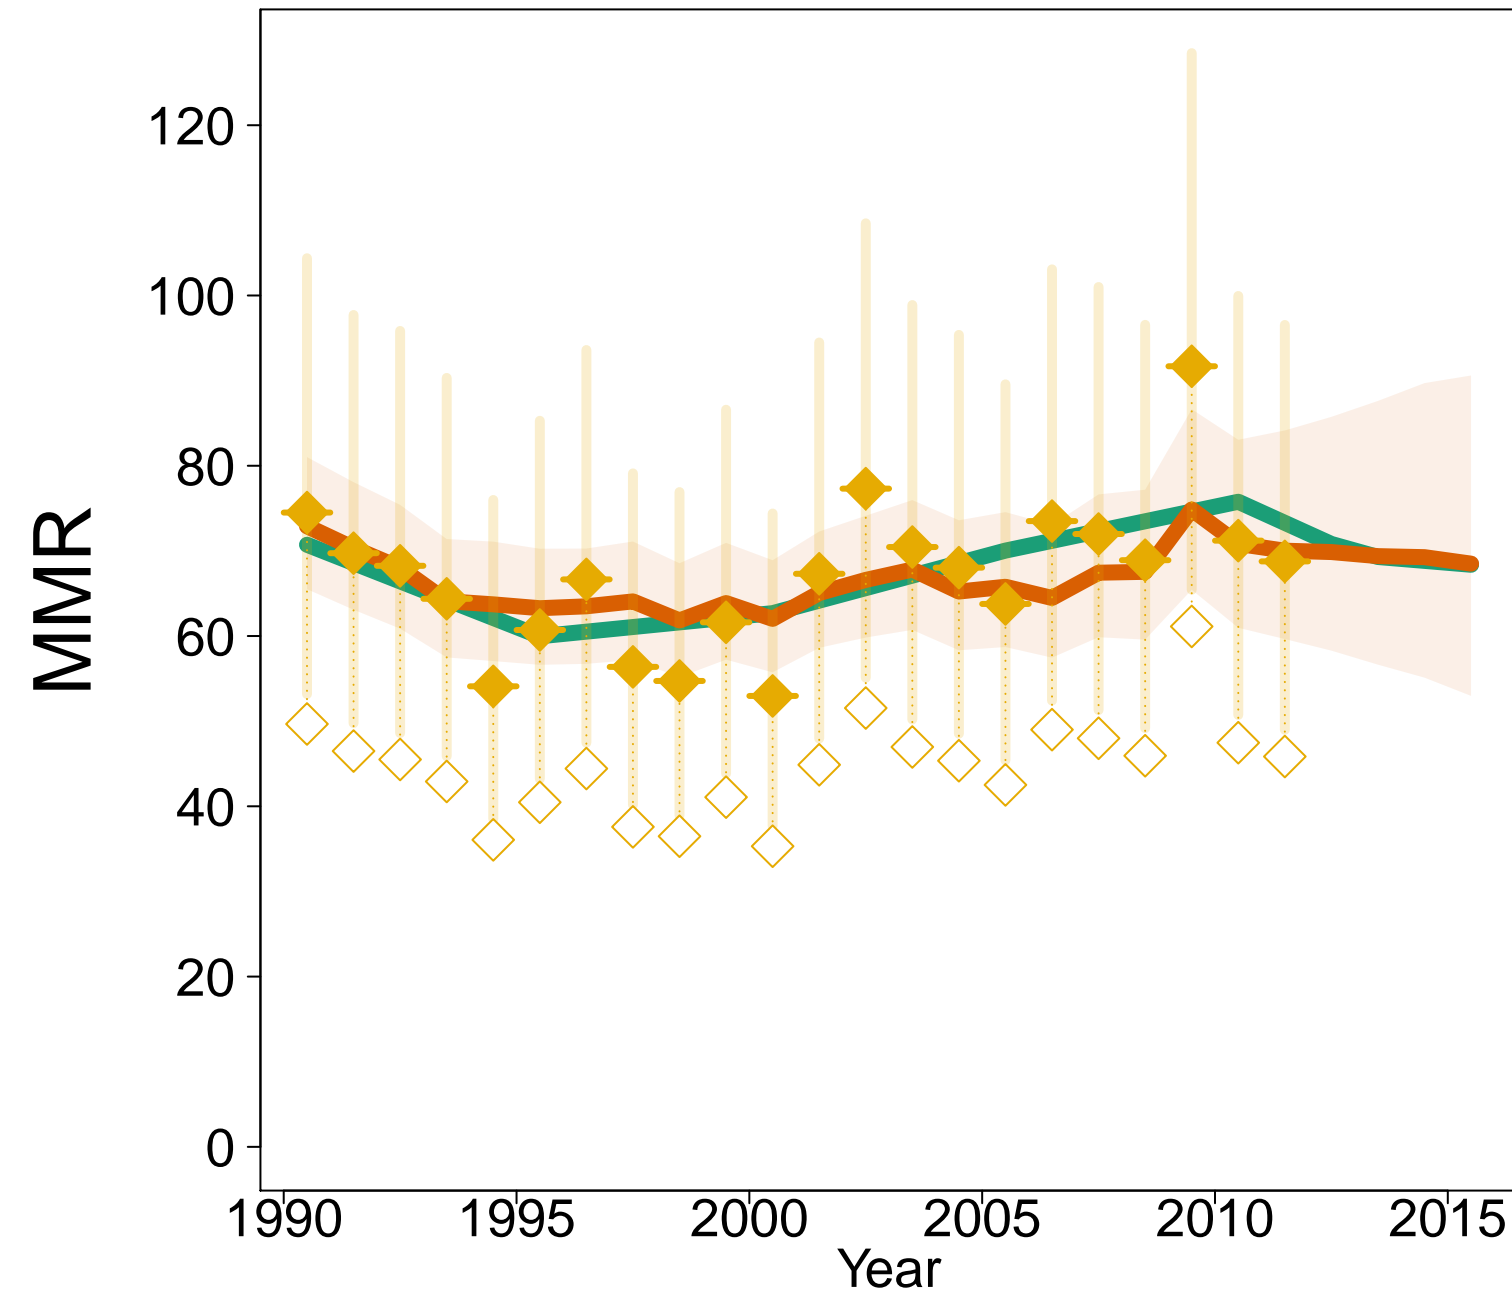

- Estimates –
- Bmat 2014
- MMEIG 2014
- Data –
- Observed Data
- Adjusted Data
- Data type –
- VR

Armenia [ARM; B]  
(Western Asia)

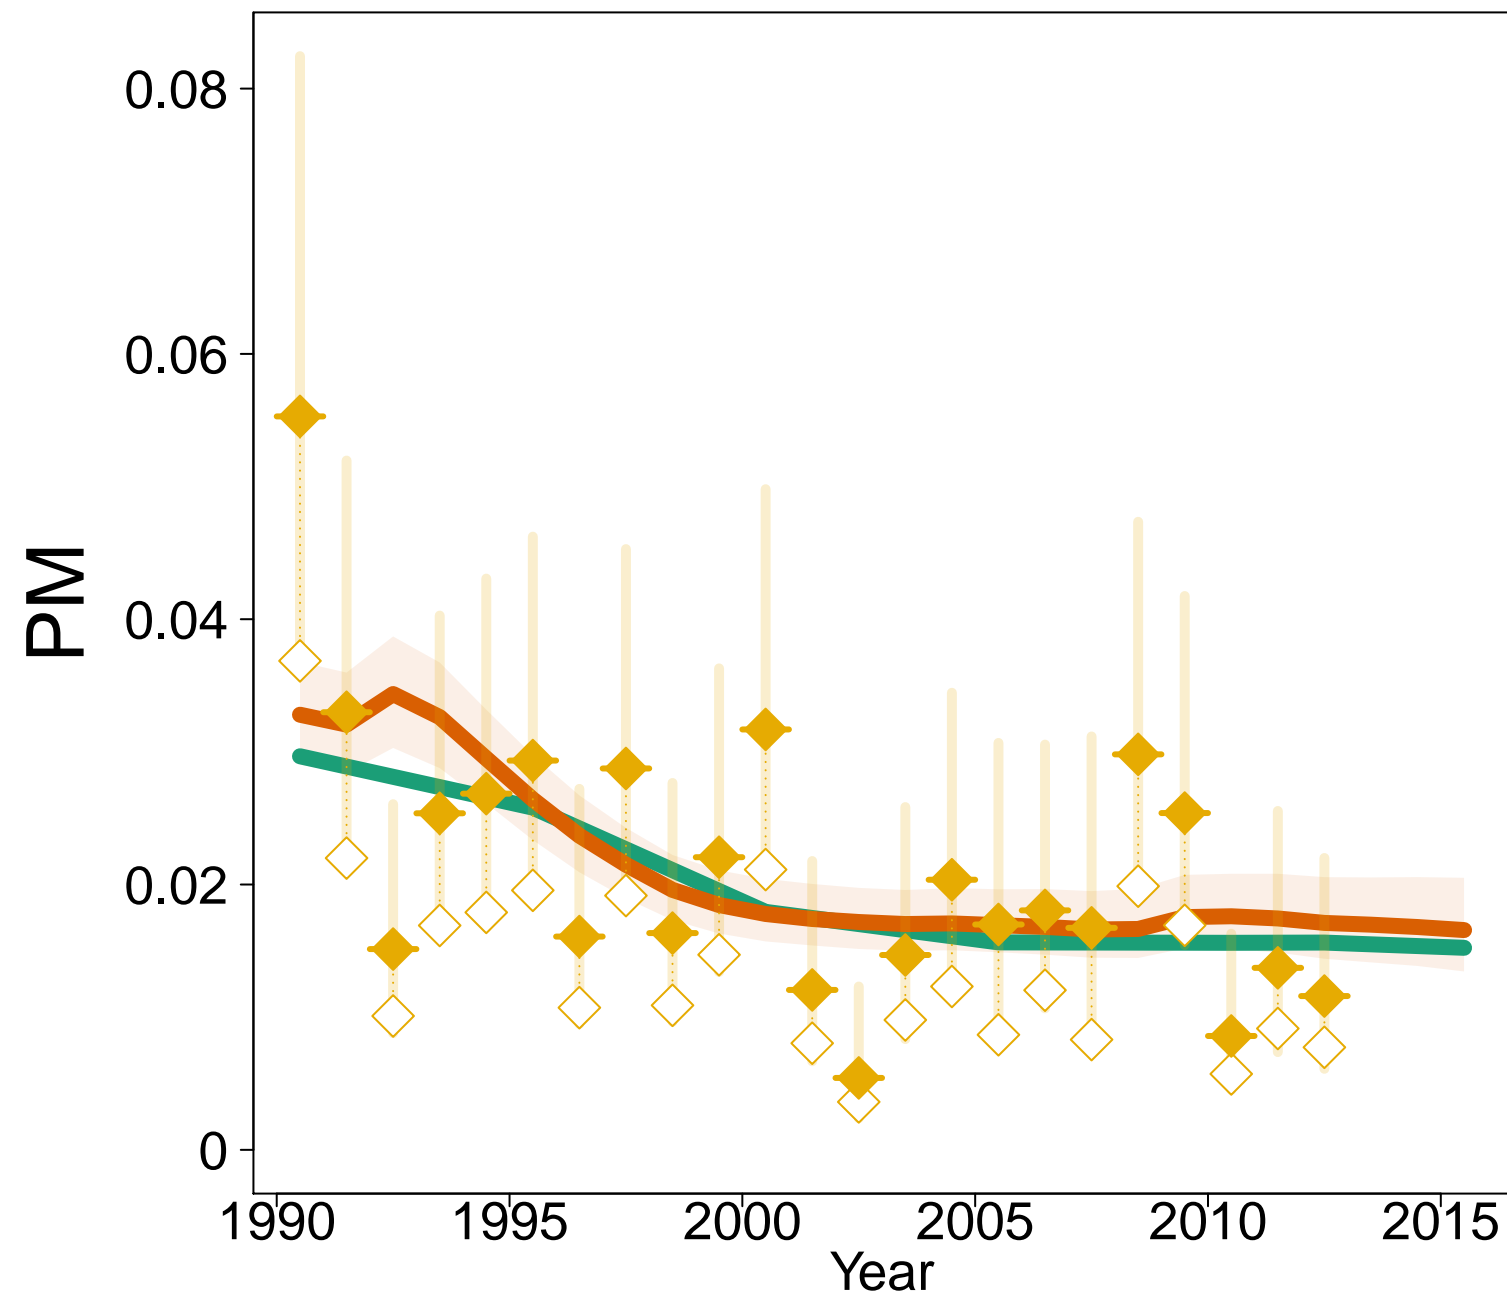

Armenia [ARM; B]  
(Western Asia)

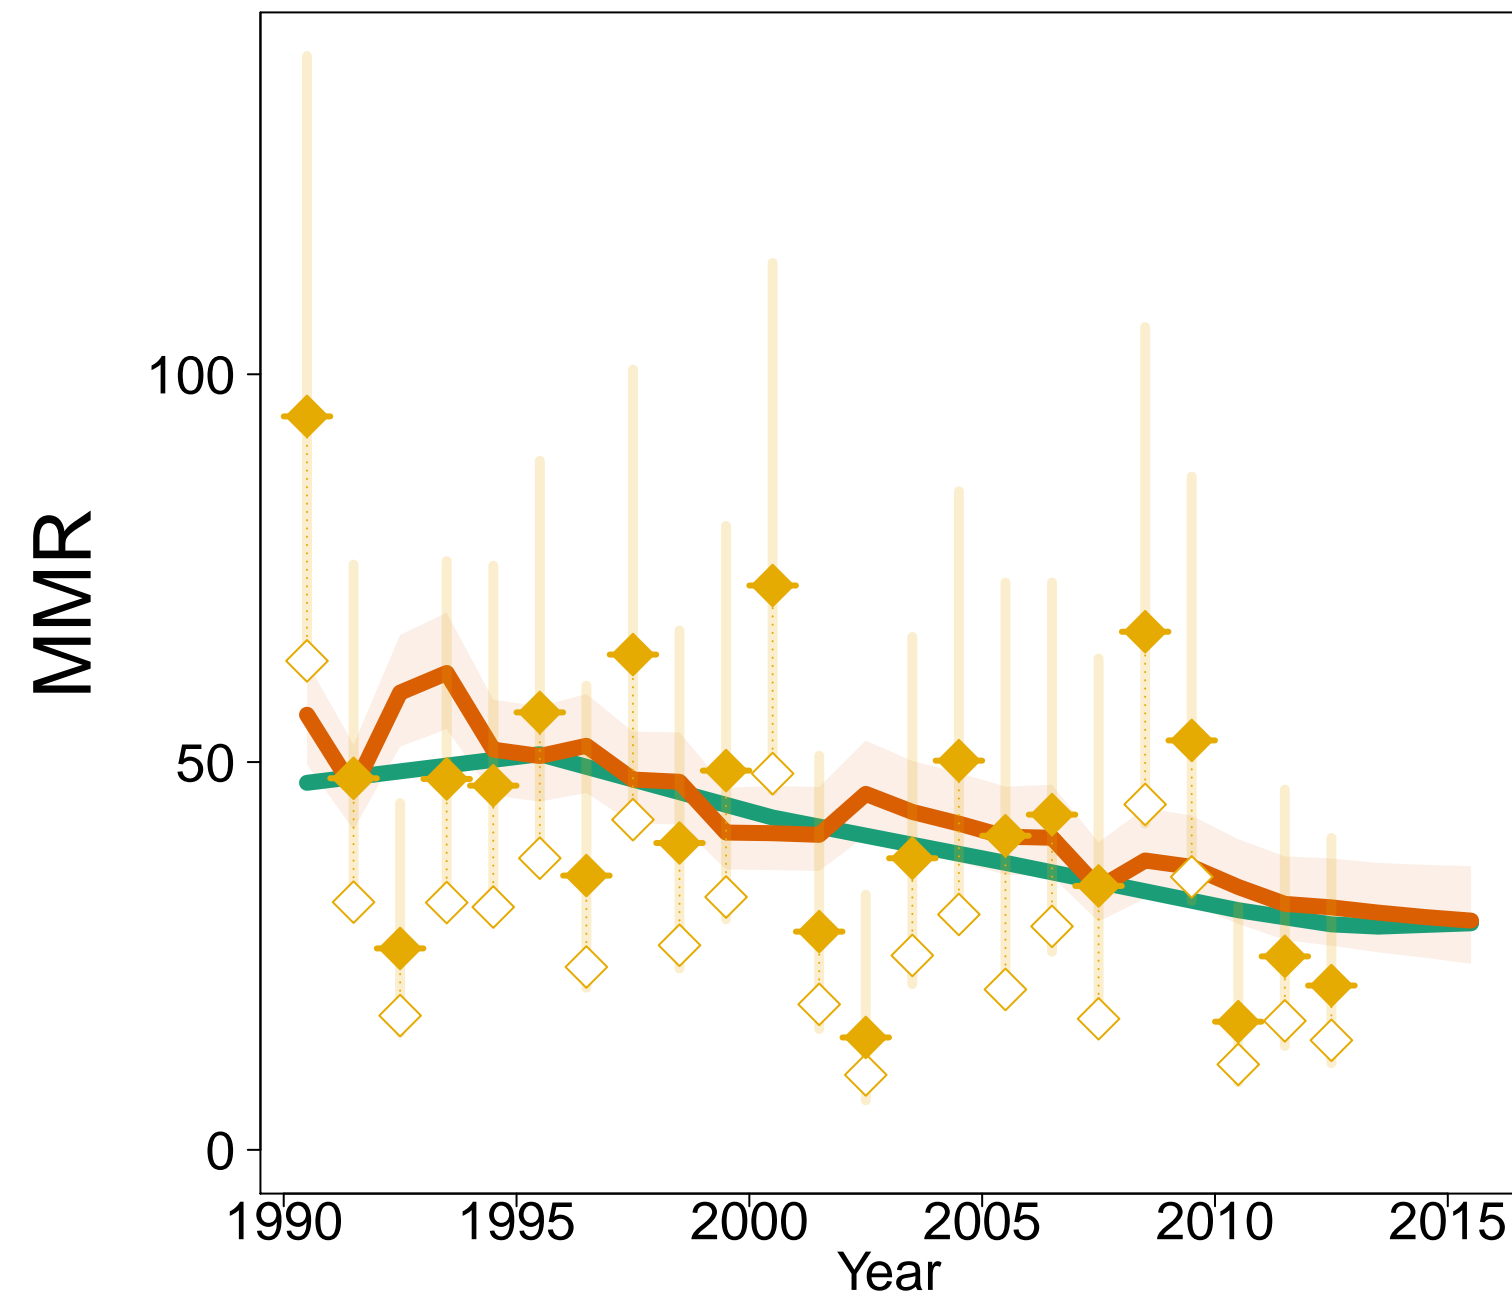

- Estimates –
- Bmat 2014
- MMEIG 2014
- Data –
- Observed Data
- Adjusted Data
- Data type –
- VR

Australia [AUS; A]  
(Developed regions)

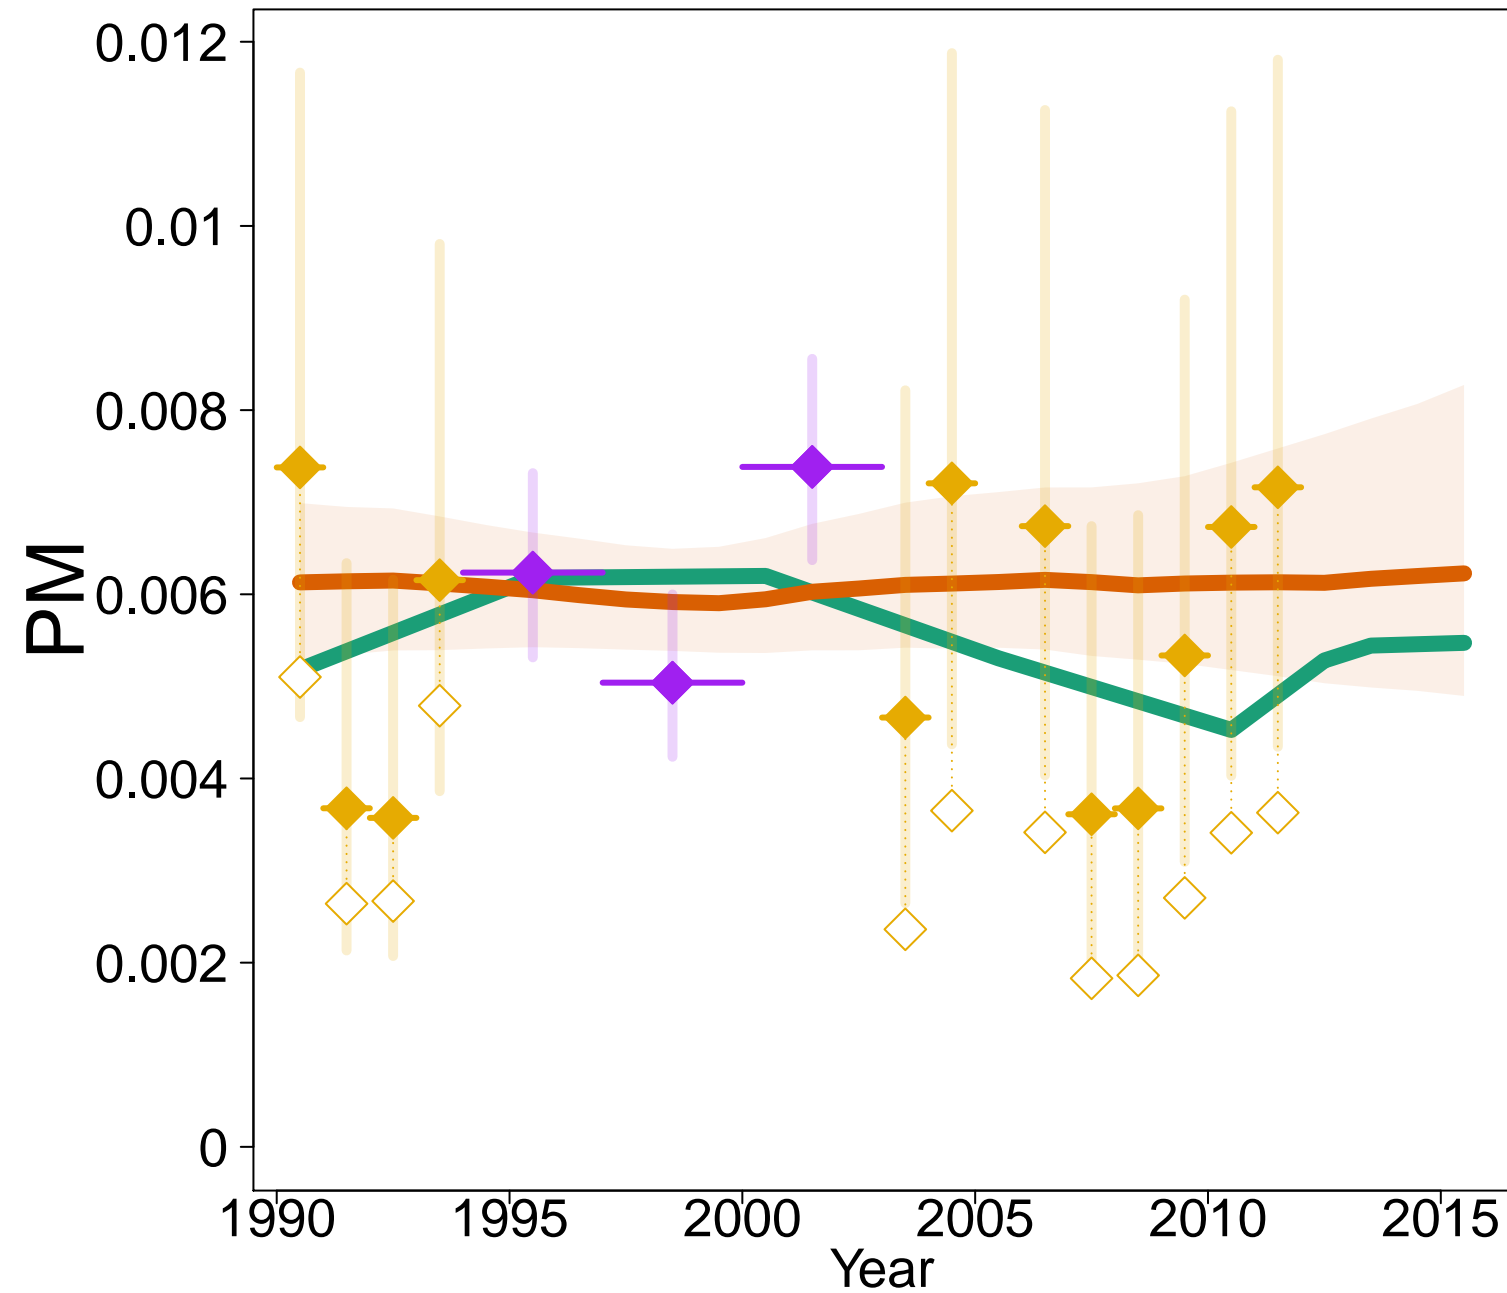

Australia [AUS; A]  
(Developed regions)

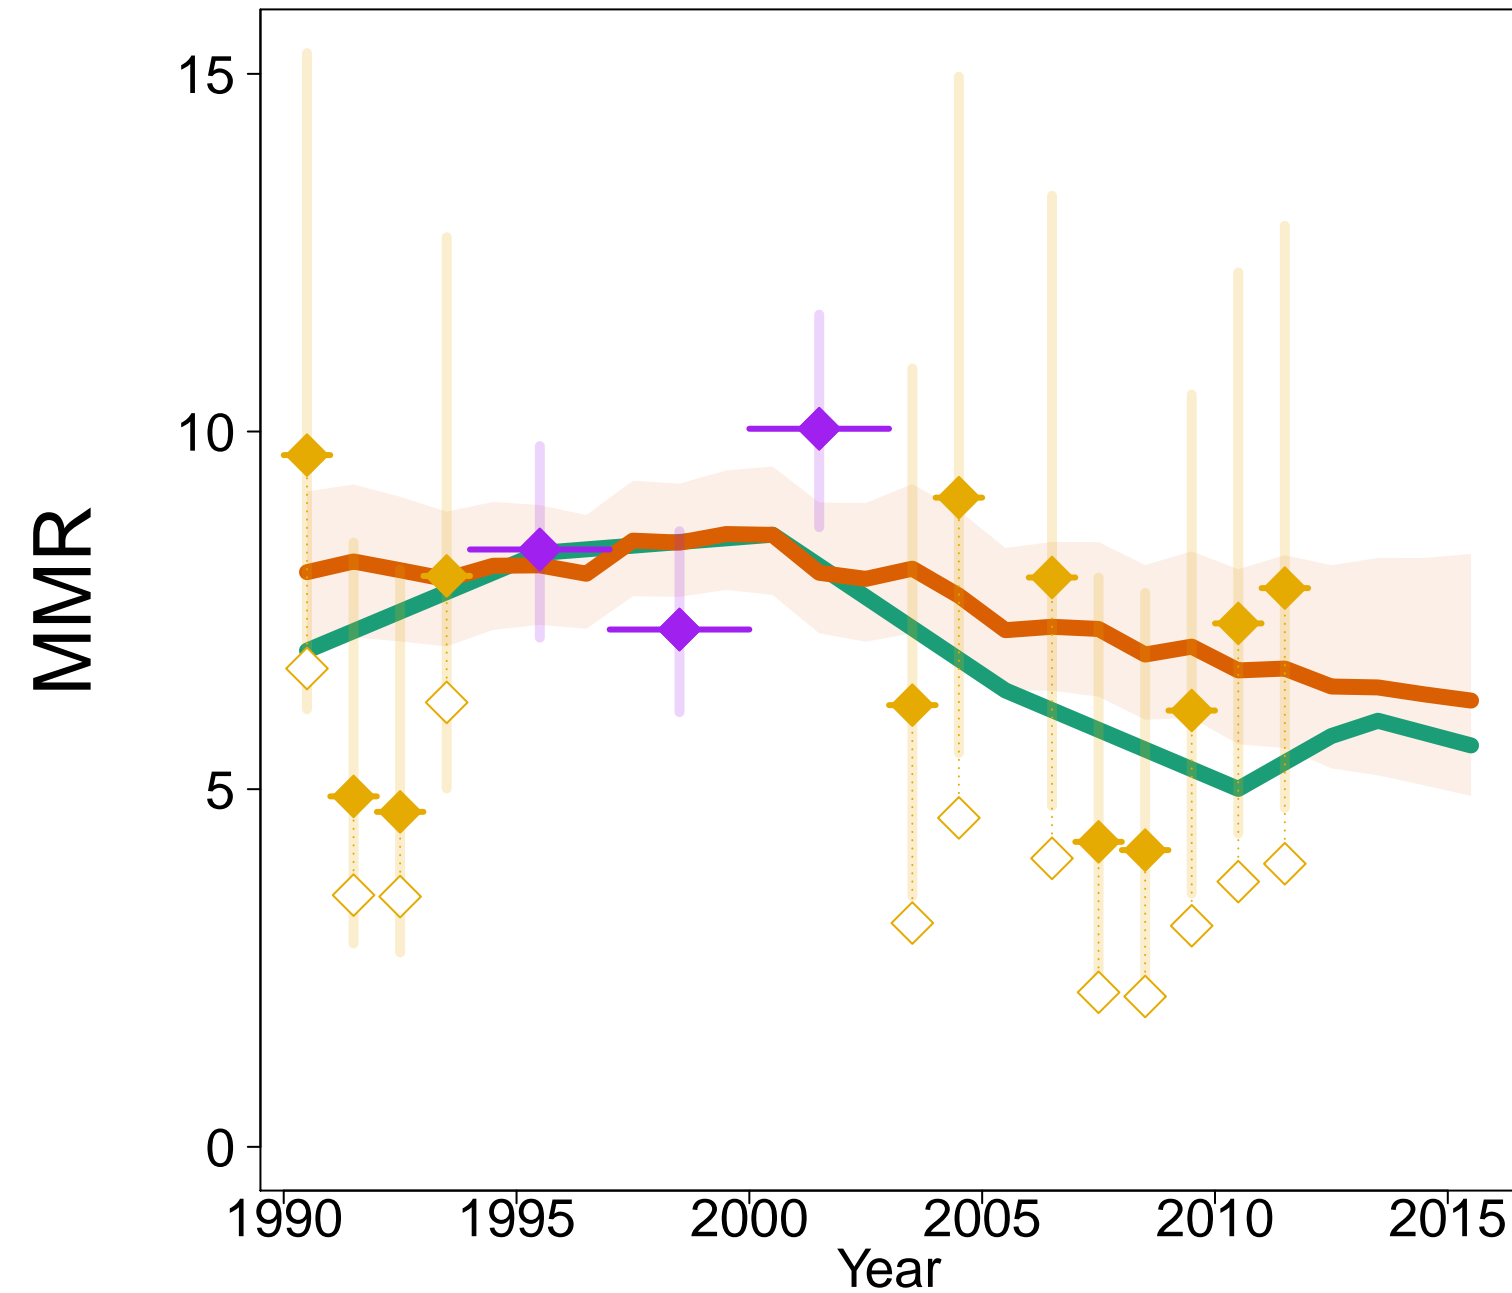

- Estimates –
- Bmat 2014
- MMEIG 2014
- Data –
- Observed Data
- Adjusted Data
- Data type –
- VR
- Spec. studies

Austria [AUT; A]  
(Developed regions)

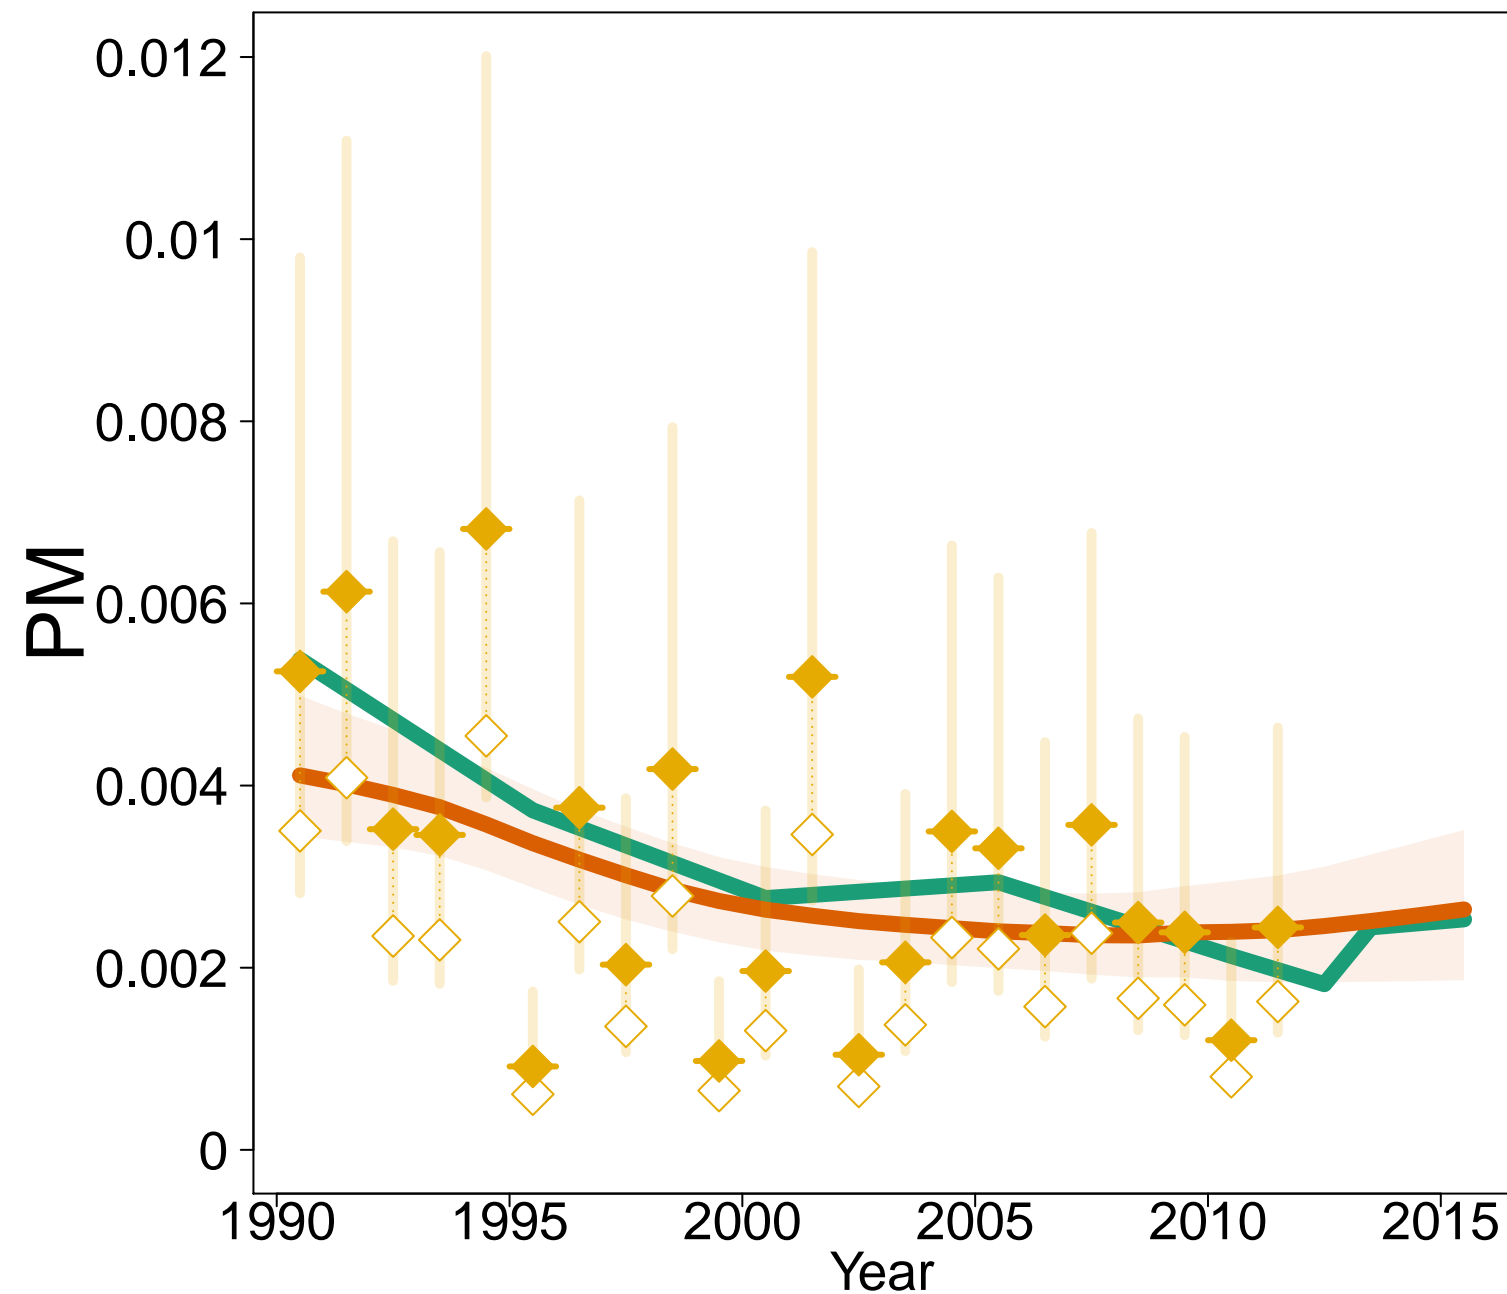

Austria [AUT; A]  
(Developed regions)

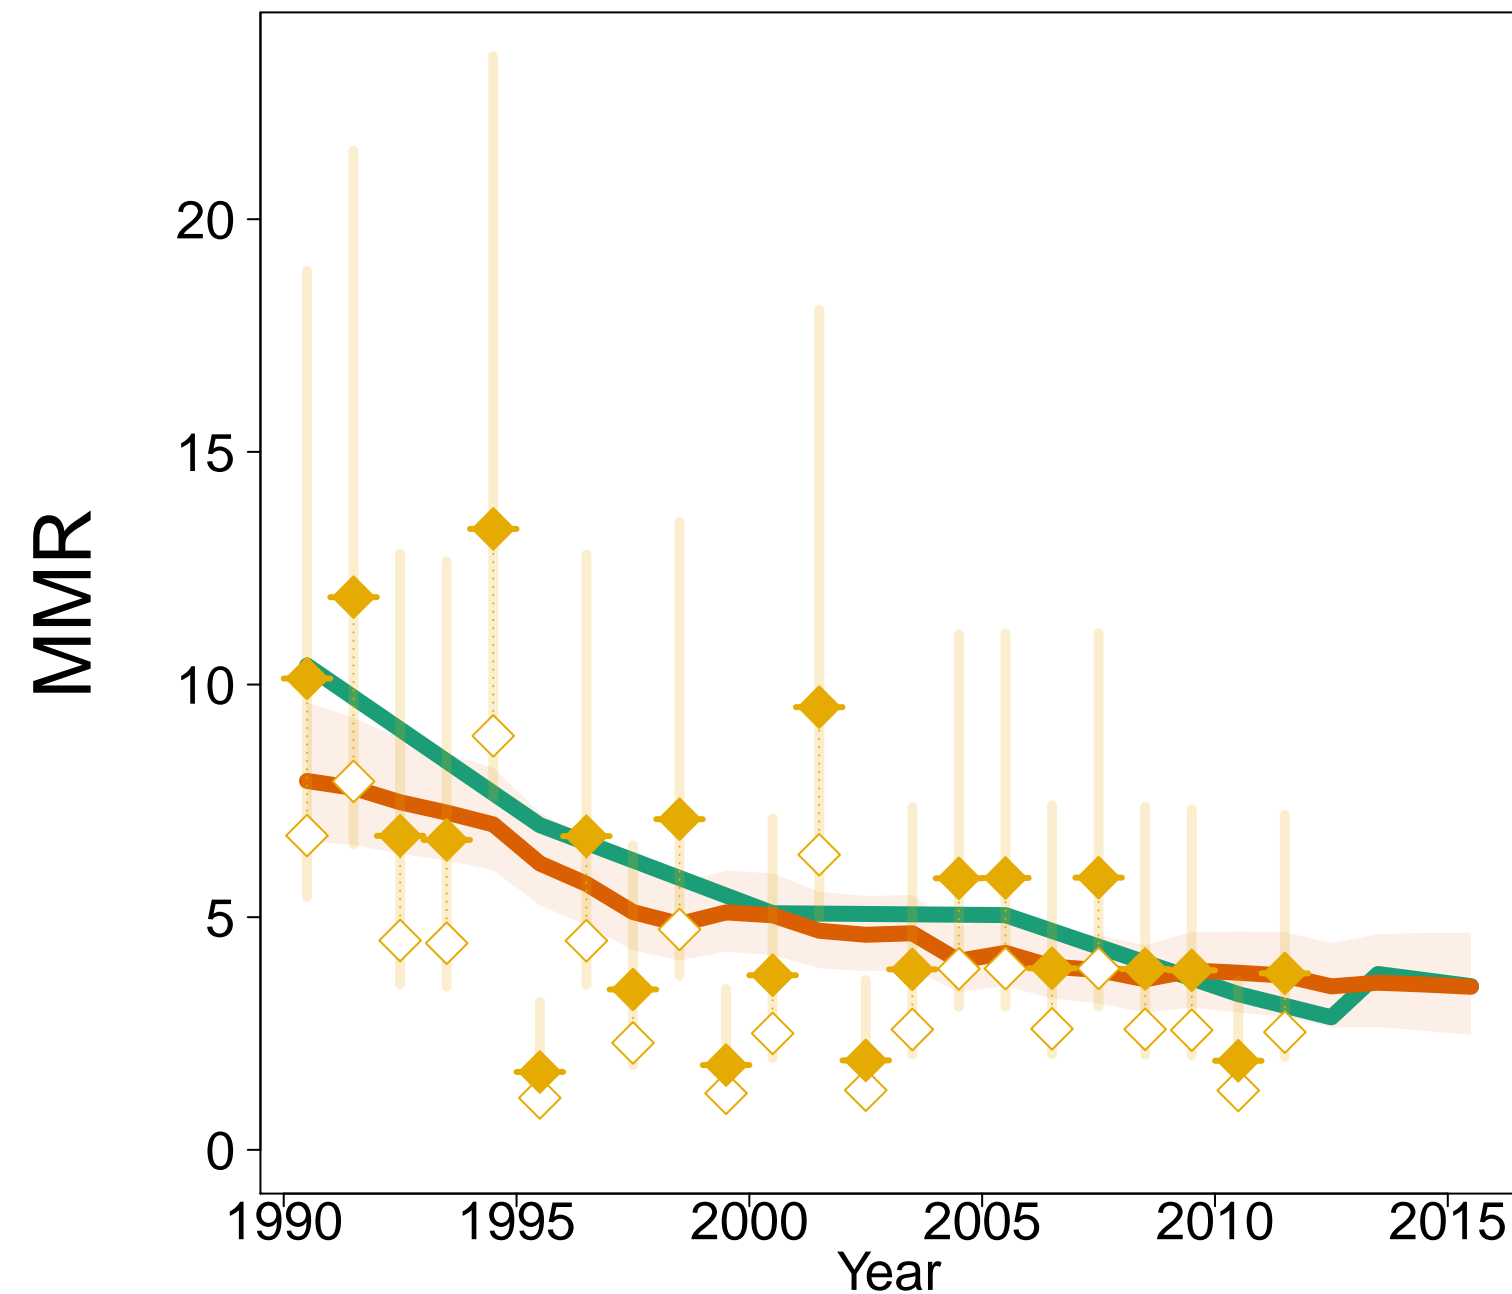

- Estimates –
- Bmat 2014
- MMEIG 2014
- Data –
- Observed Data
- Adjusted Data
- Data type –
- VR



Azerbaijan [AZE; B]  
(Western Asia)

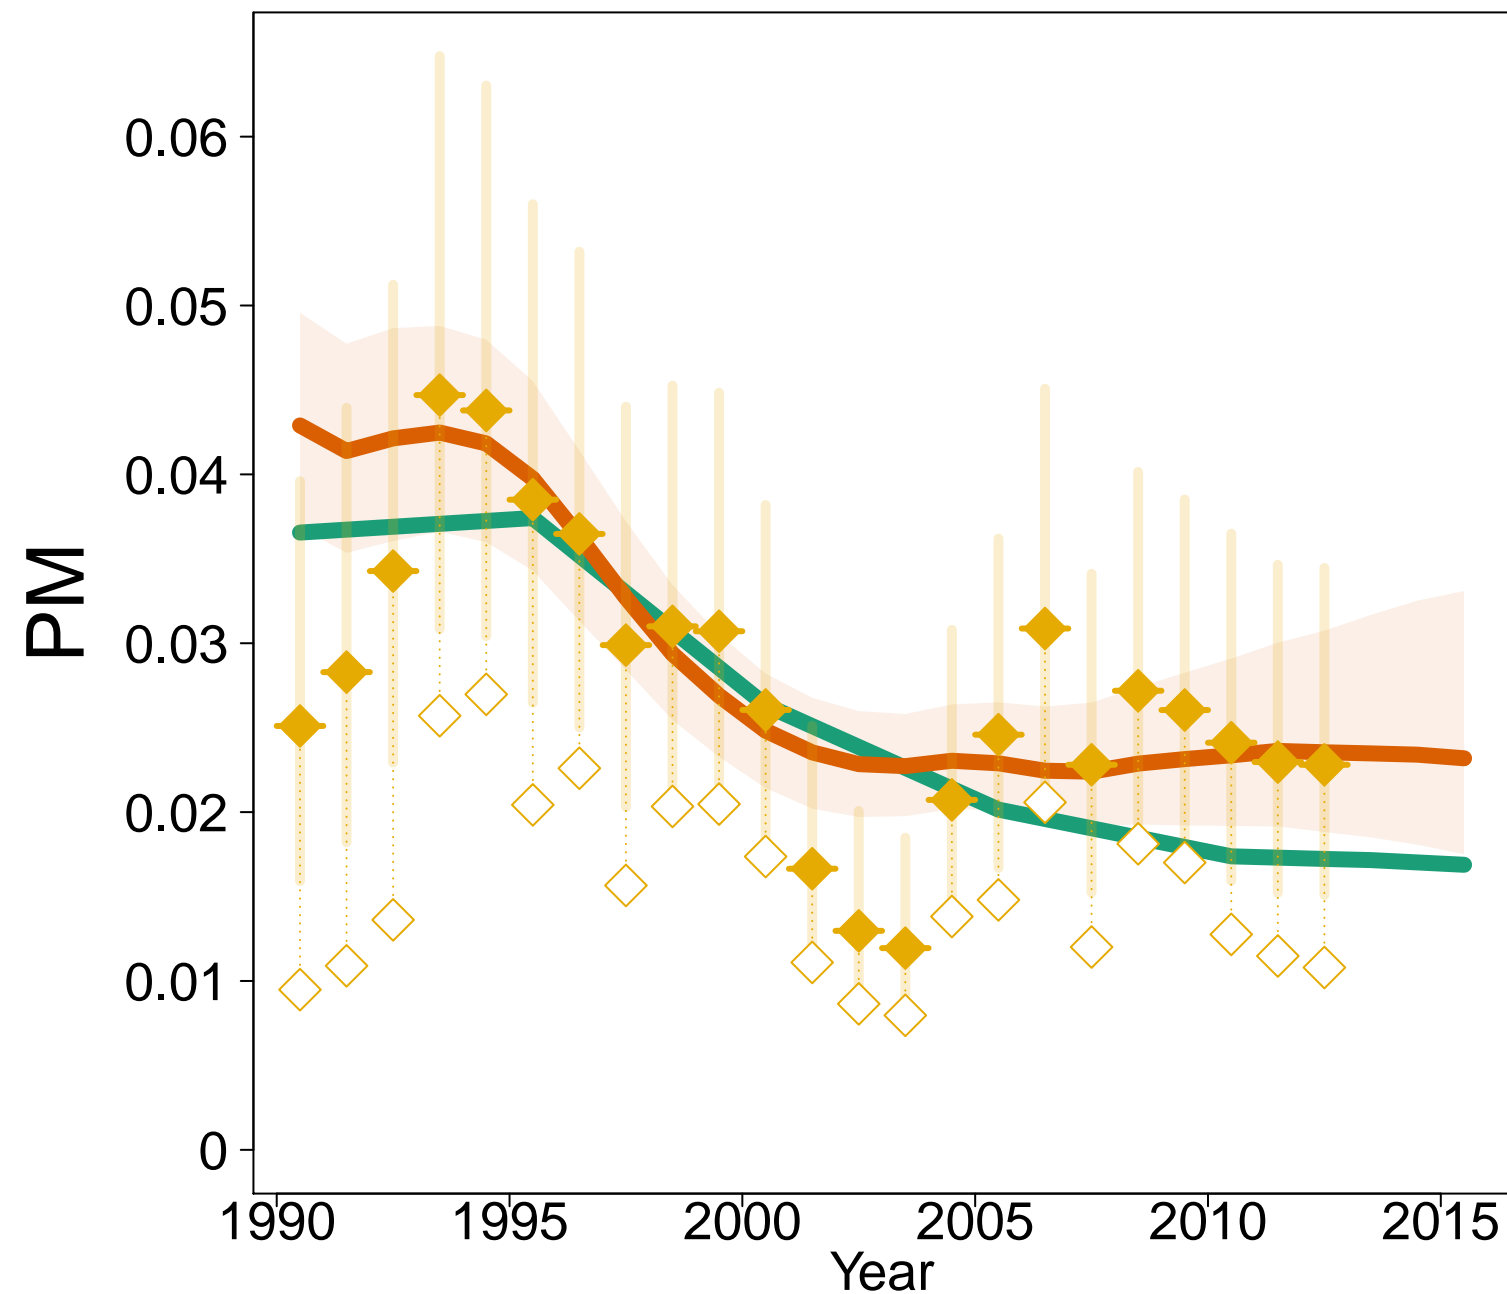

Azerbaijan [AZE; B]  
(Western Asia)

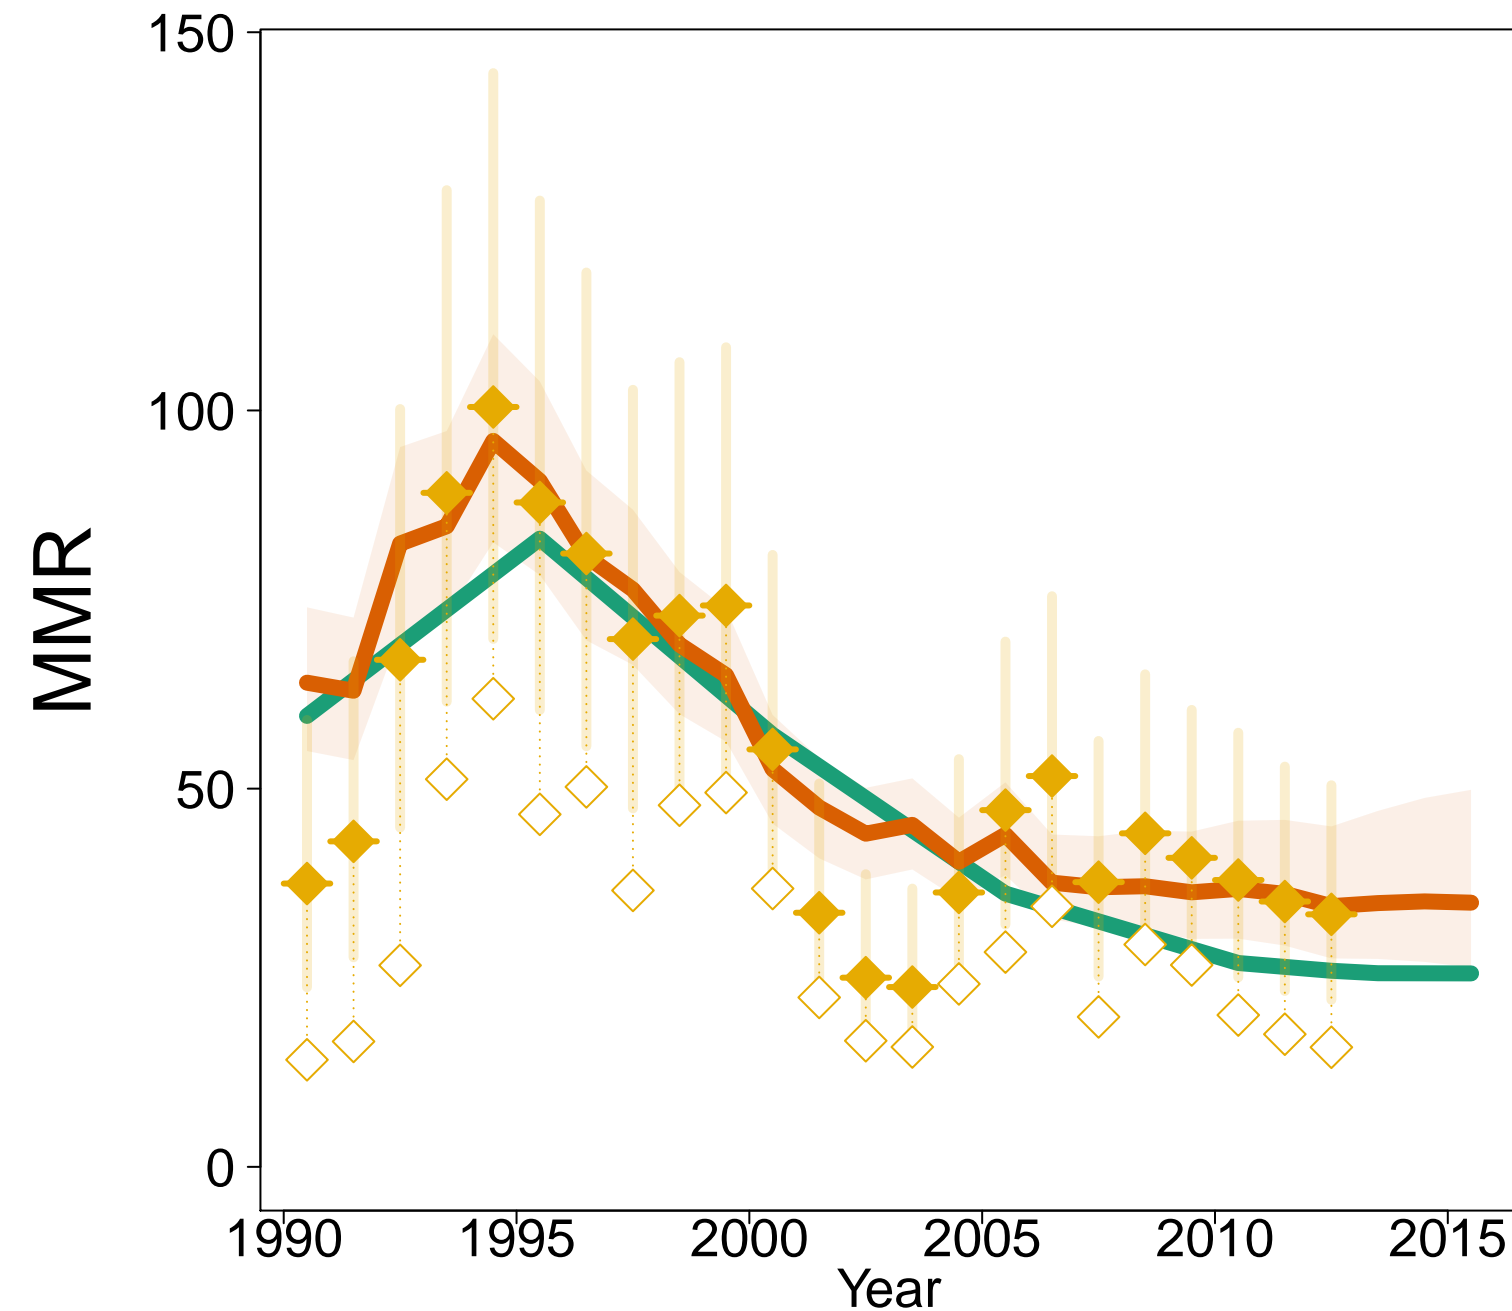

– Estimates –  
Bmat 2014  
MMEIG 2014  
– Data –  
Observed Data  
Adjusted Data  
– Data type –  
VR

Bahamas [BHS; A]  
(Caribbean)

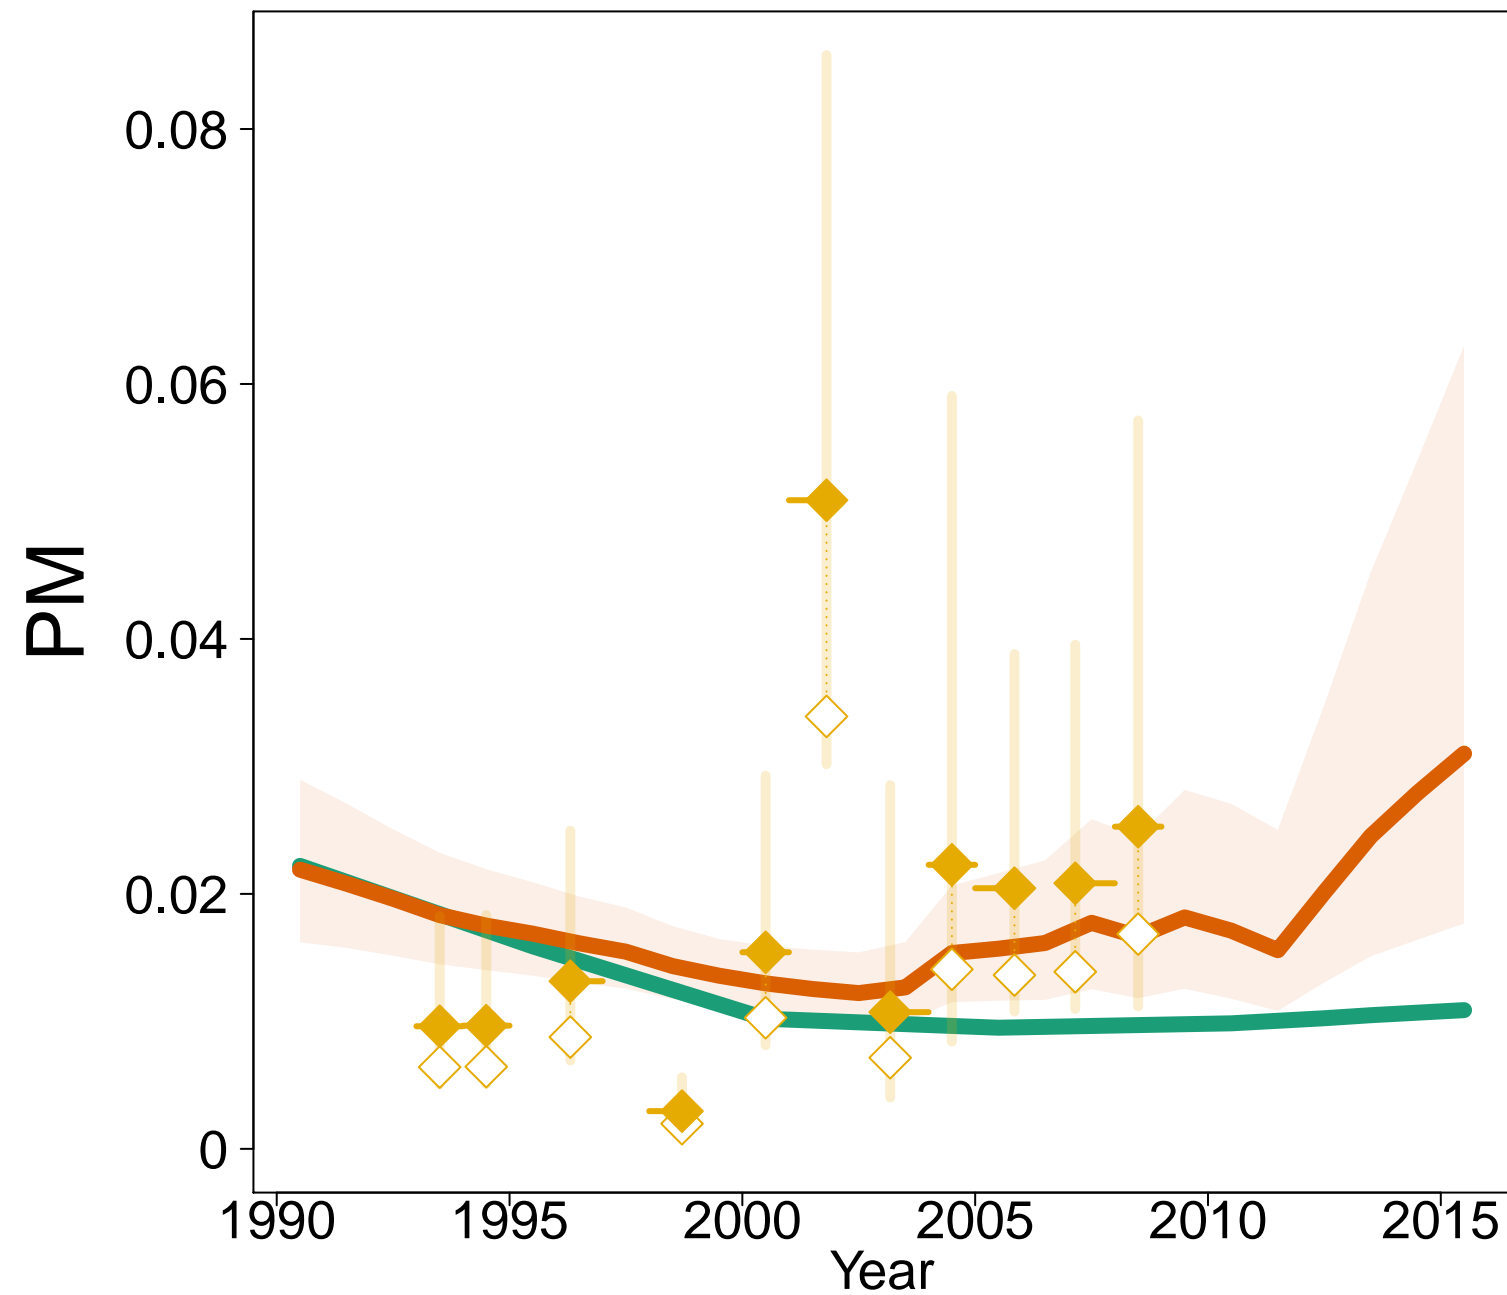

Bahamas [BHS; A]  
(Caribbean)

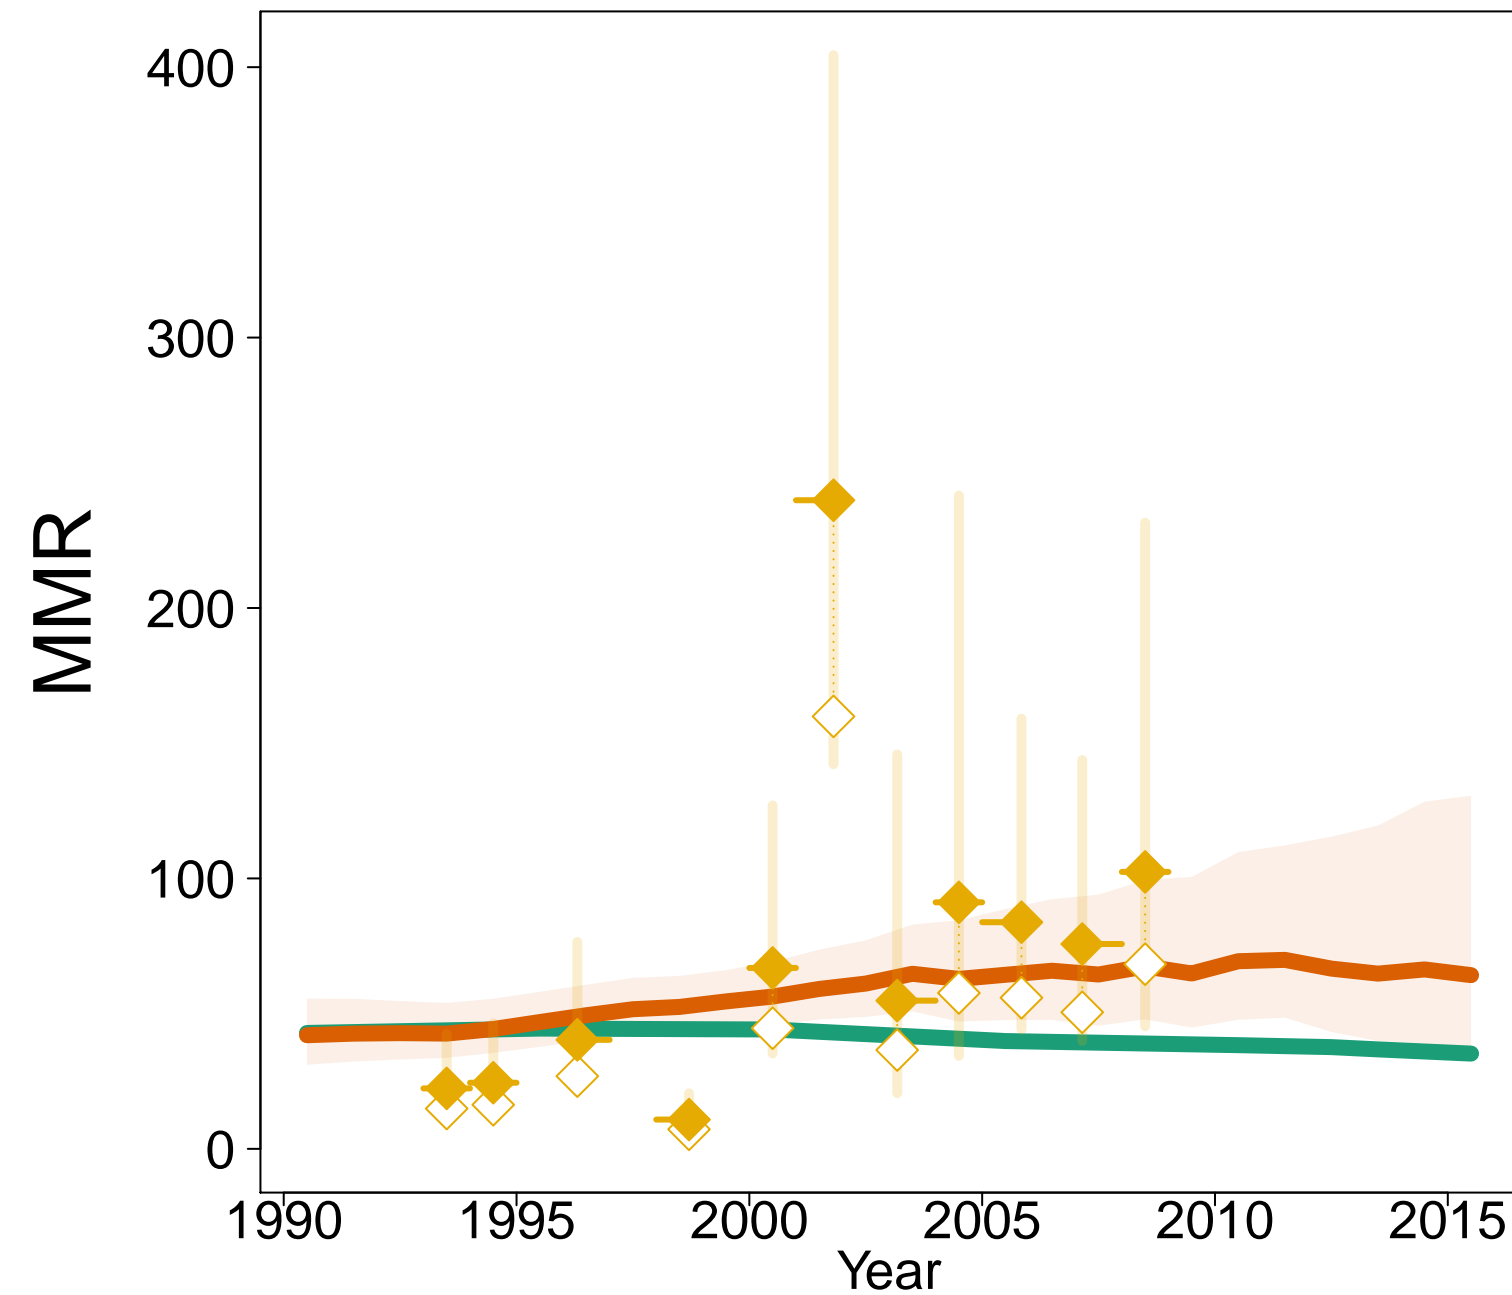

- Estimates –
- Bmat 2014
- MMEIG 2014
- Data –
- Observed Data
- Adjusted Data
- Data type –
- VR

Bahrain [BHR; A]  
(Western Asia)

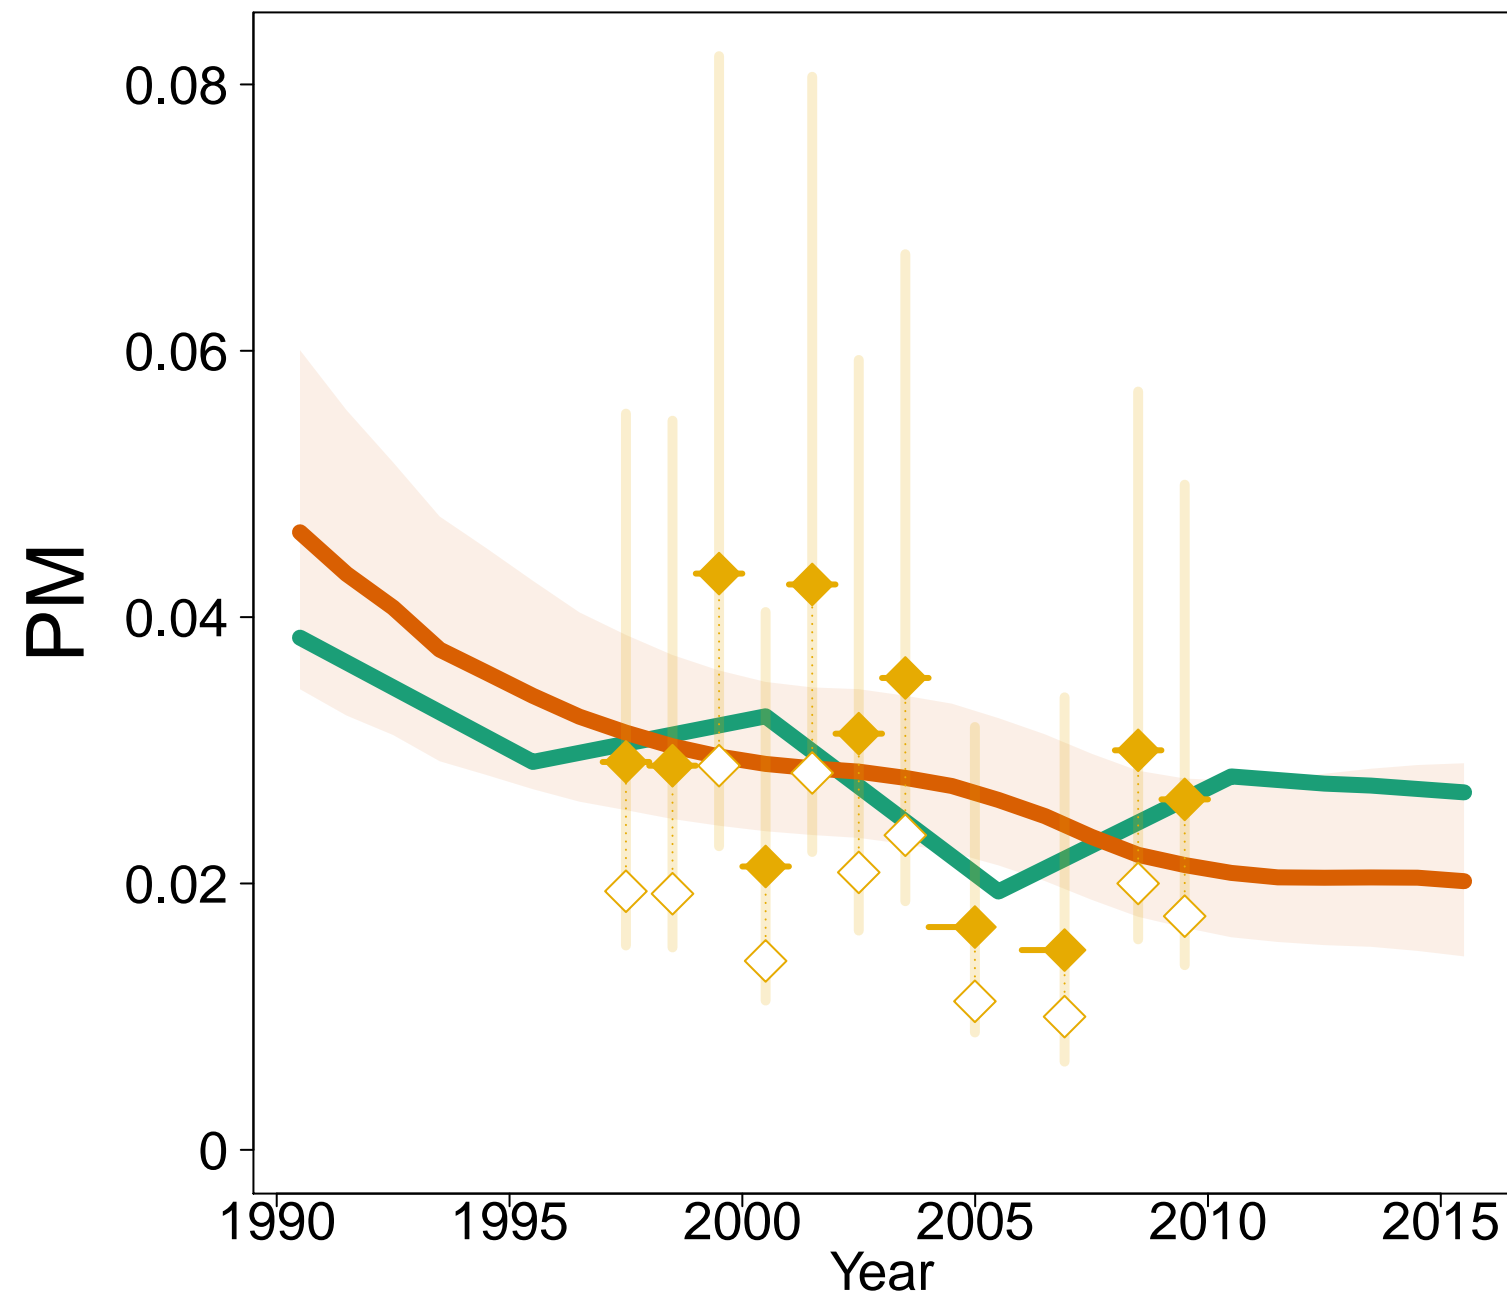

Bahrain [BHR; A]  
(Western Asia)

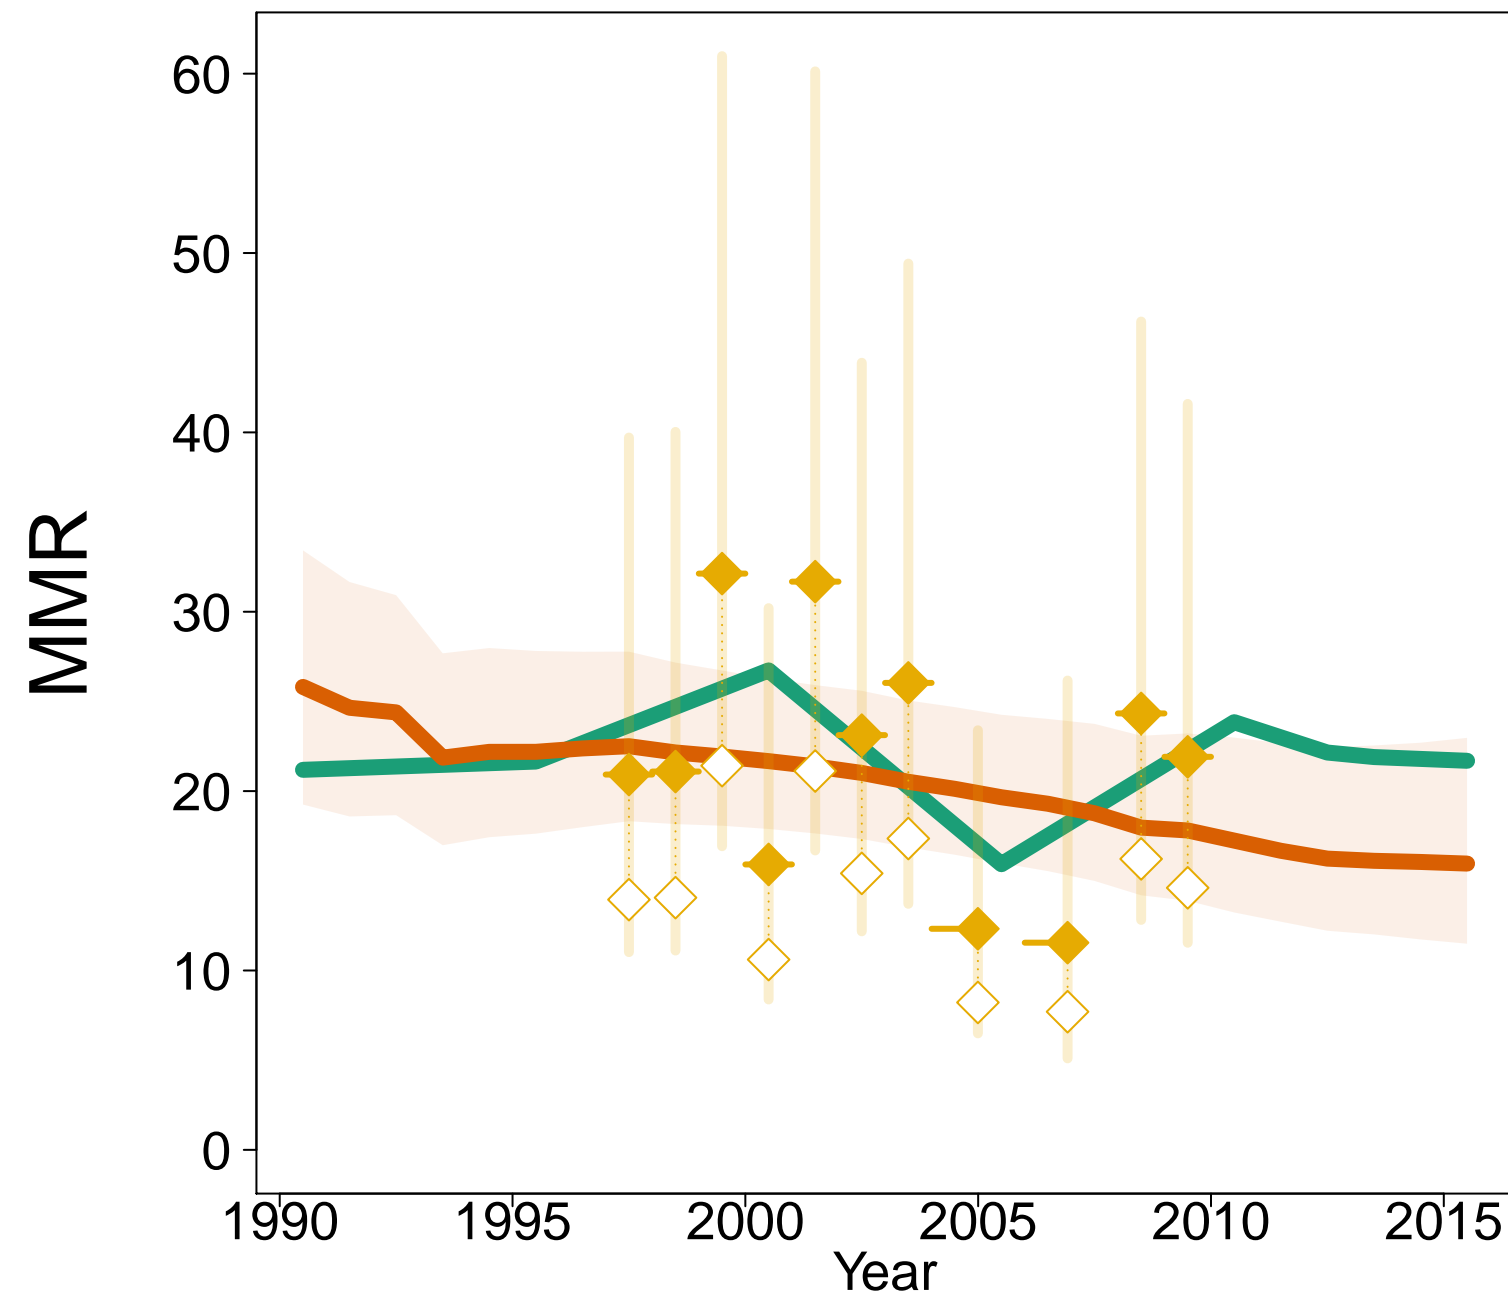

- Estimates –
- Bmat 2014
- MMEIG 2014
- Data –
- Observed Data
- Adjusted Data
- Data type –
- VR

Bangladesh [BGD; B]  
(Southern Asia)

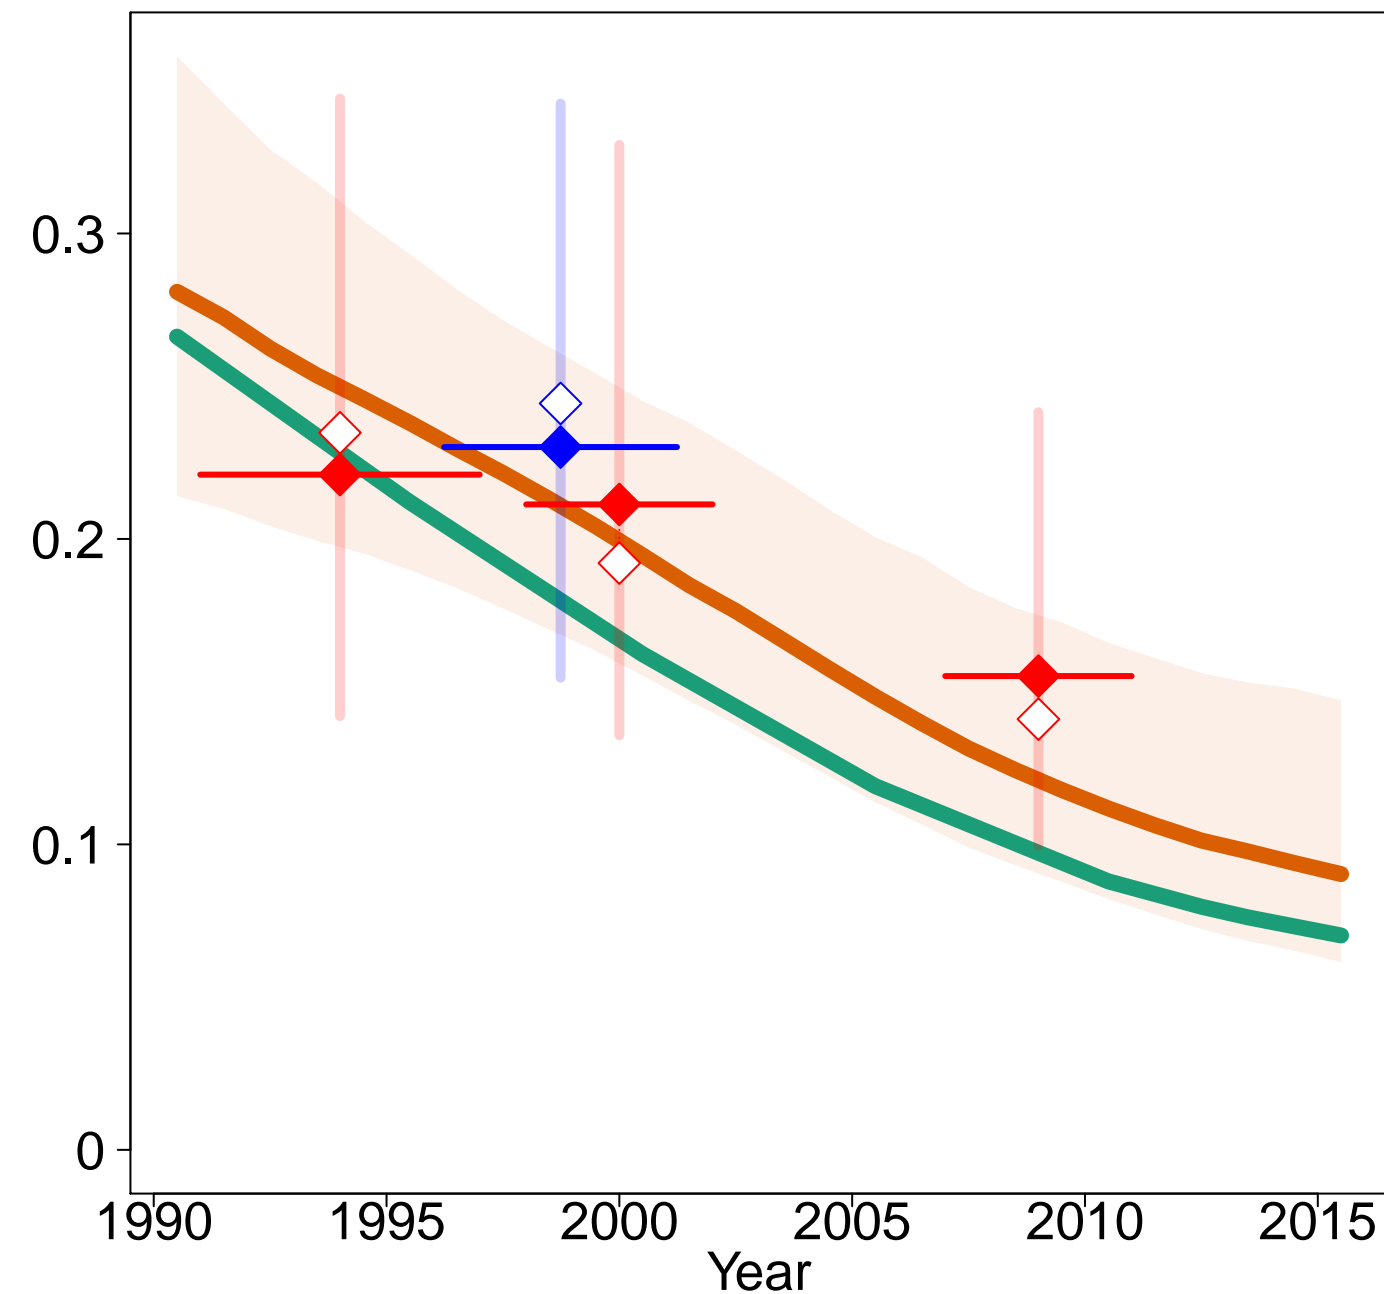

Bangladesh [BGD; B]  
(Southern Asia)

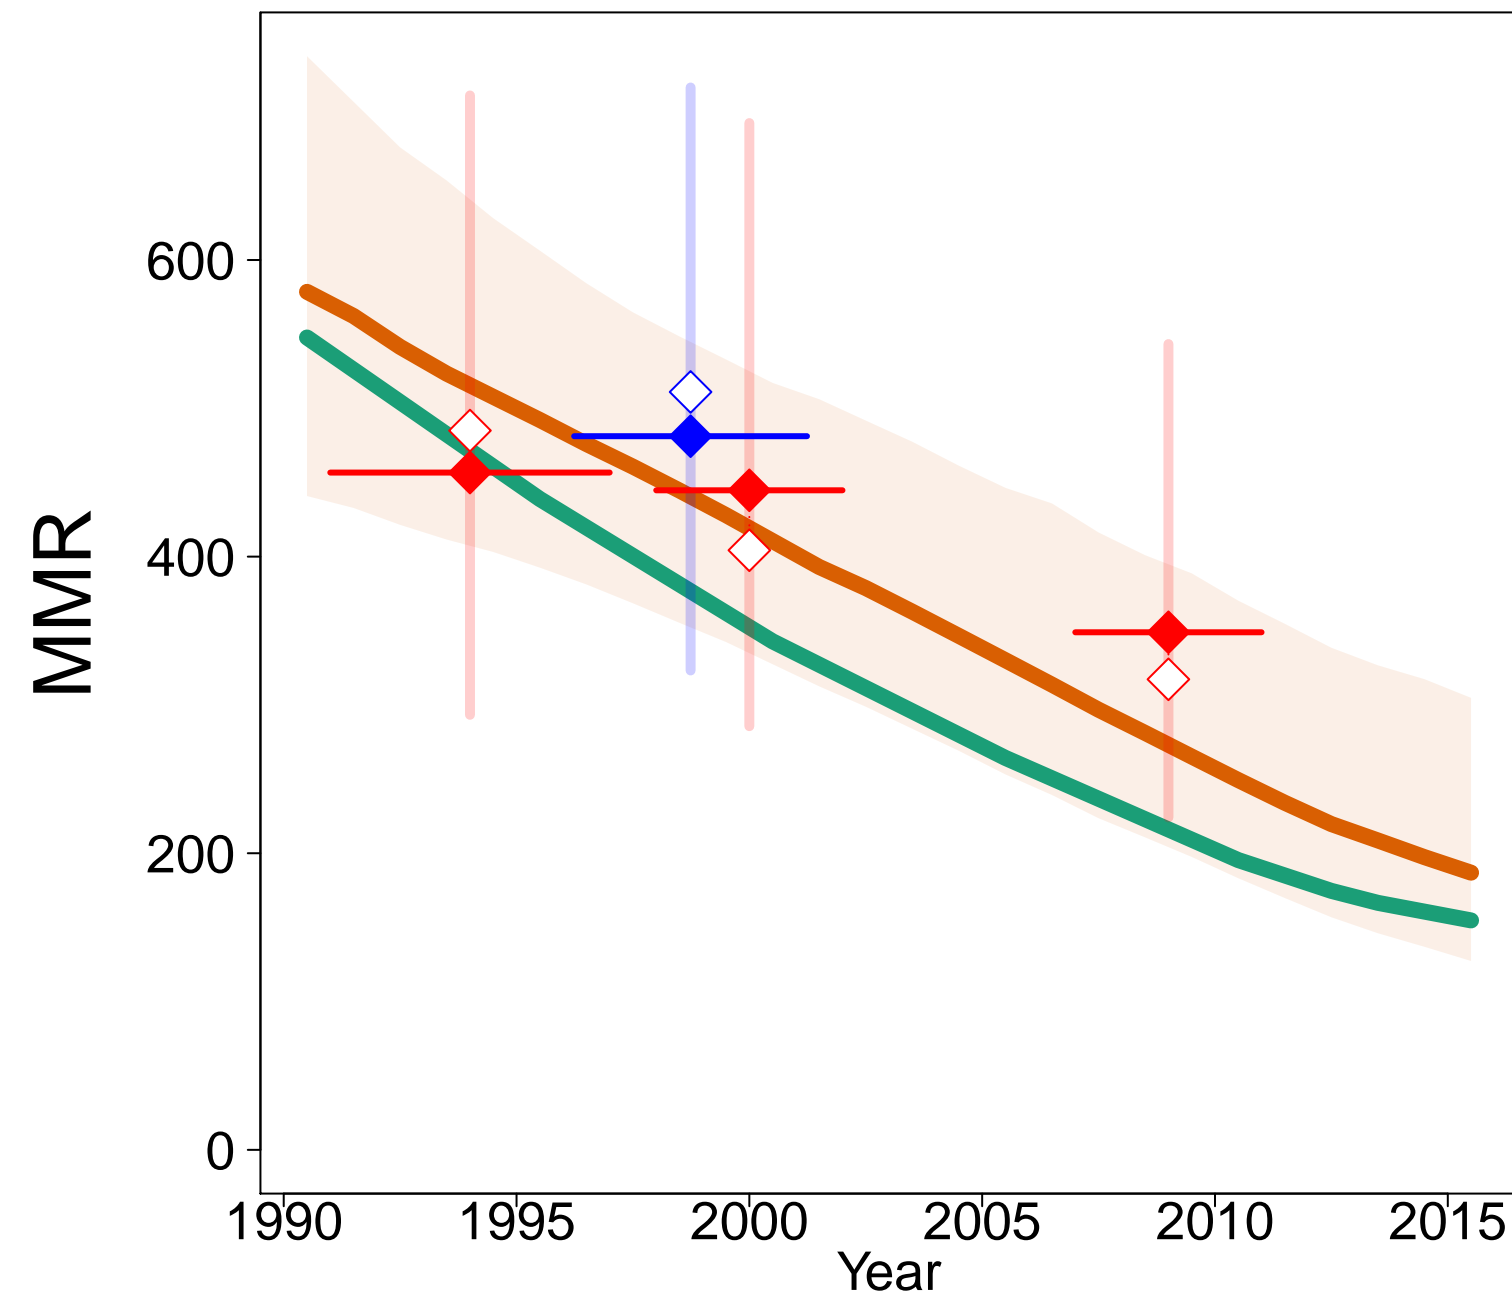

- Estimates –
- Bmat 2014
- MMEIG 2014
- Data –
- ◊ Observed Data
- ◆ Adjusted Data
- Data type –
- ◆ DHS
- ◆ Misc. studies

Barbados [BRB; A]  
(Caribbean)

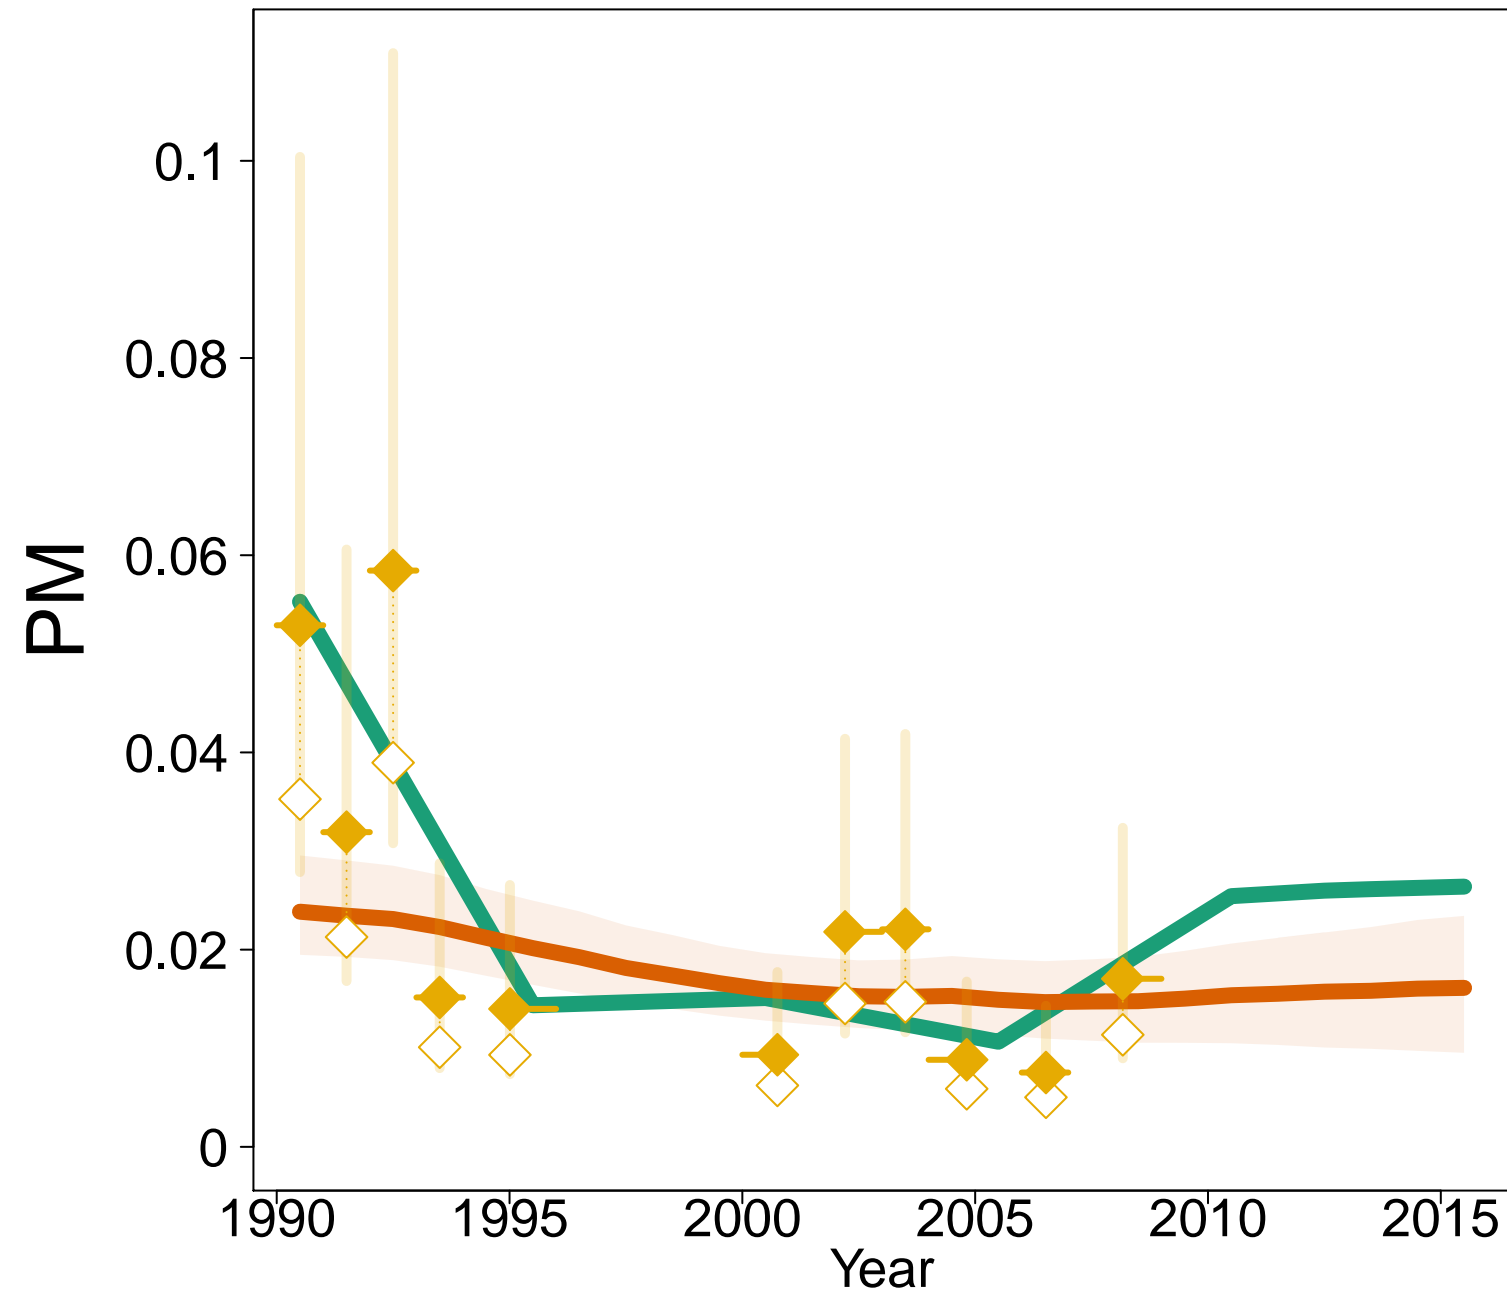

Barbados [BRB; A]  
(Caribbean)

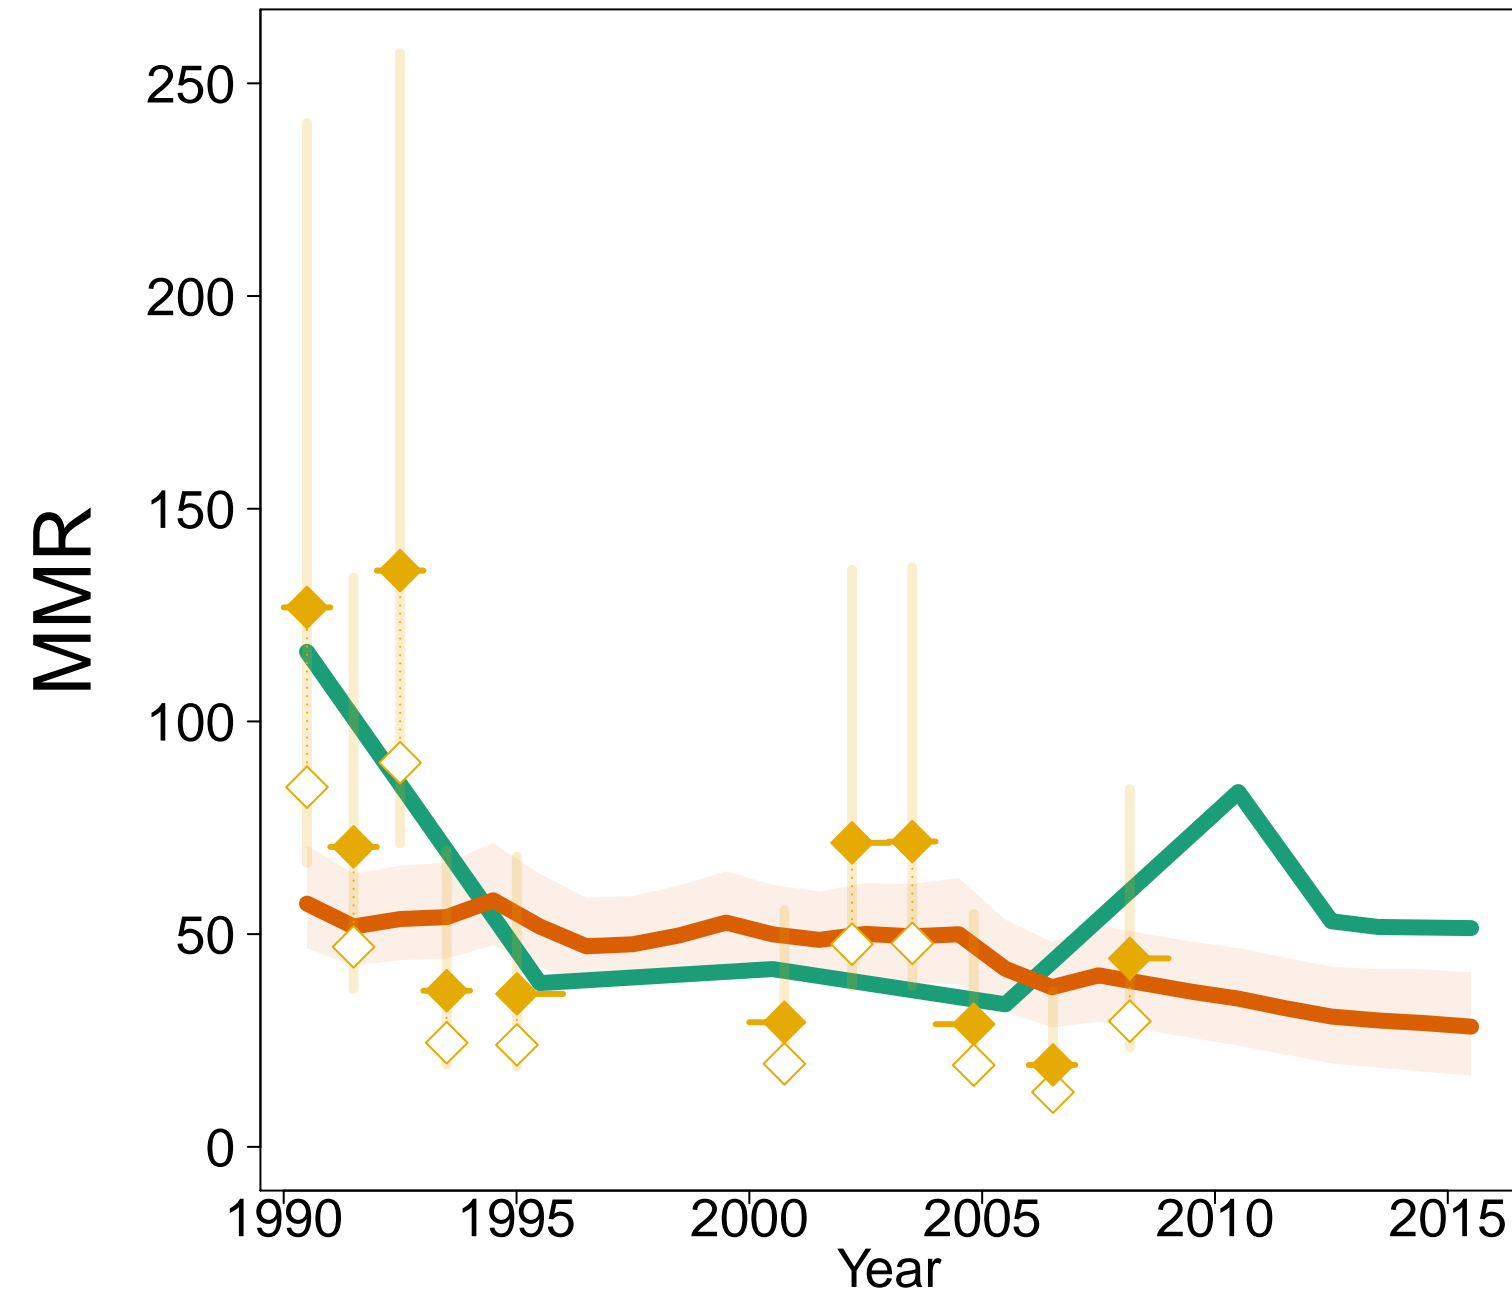

– Estimates –  
Bmat 2014  
MMEIG 2014  
– Data –  
Observed Data  
Adjusted Data  
– Data type –  
VR

Belarus [BLR; A]  
(Developed regions)

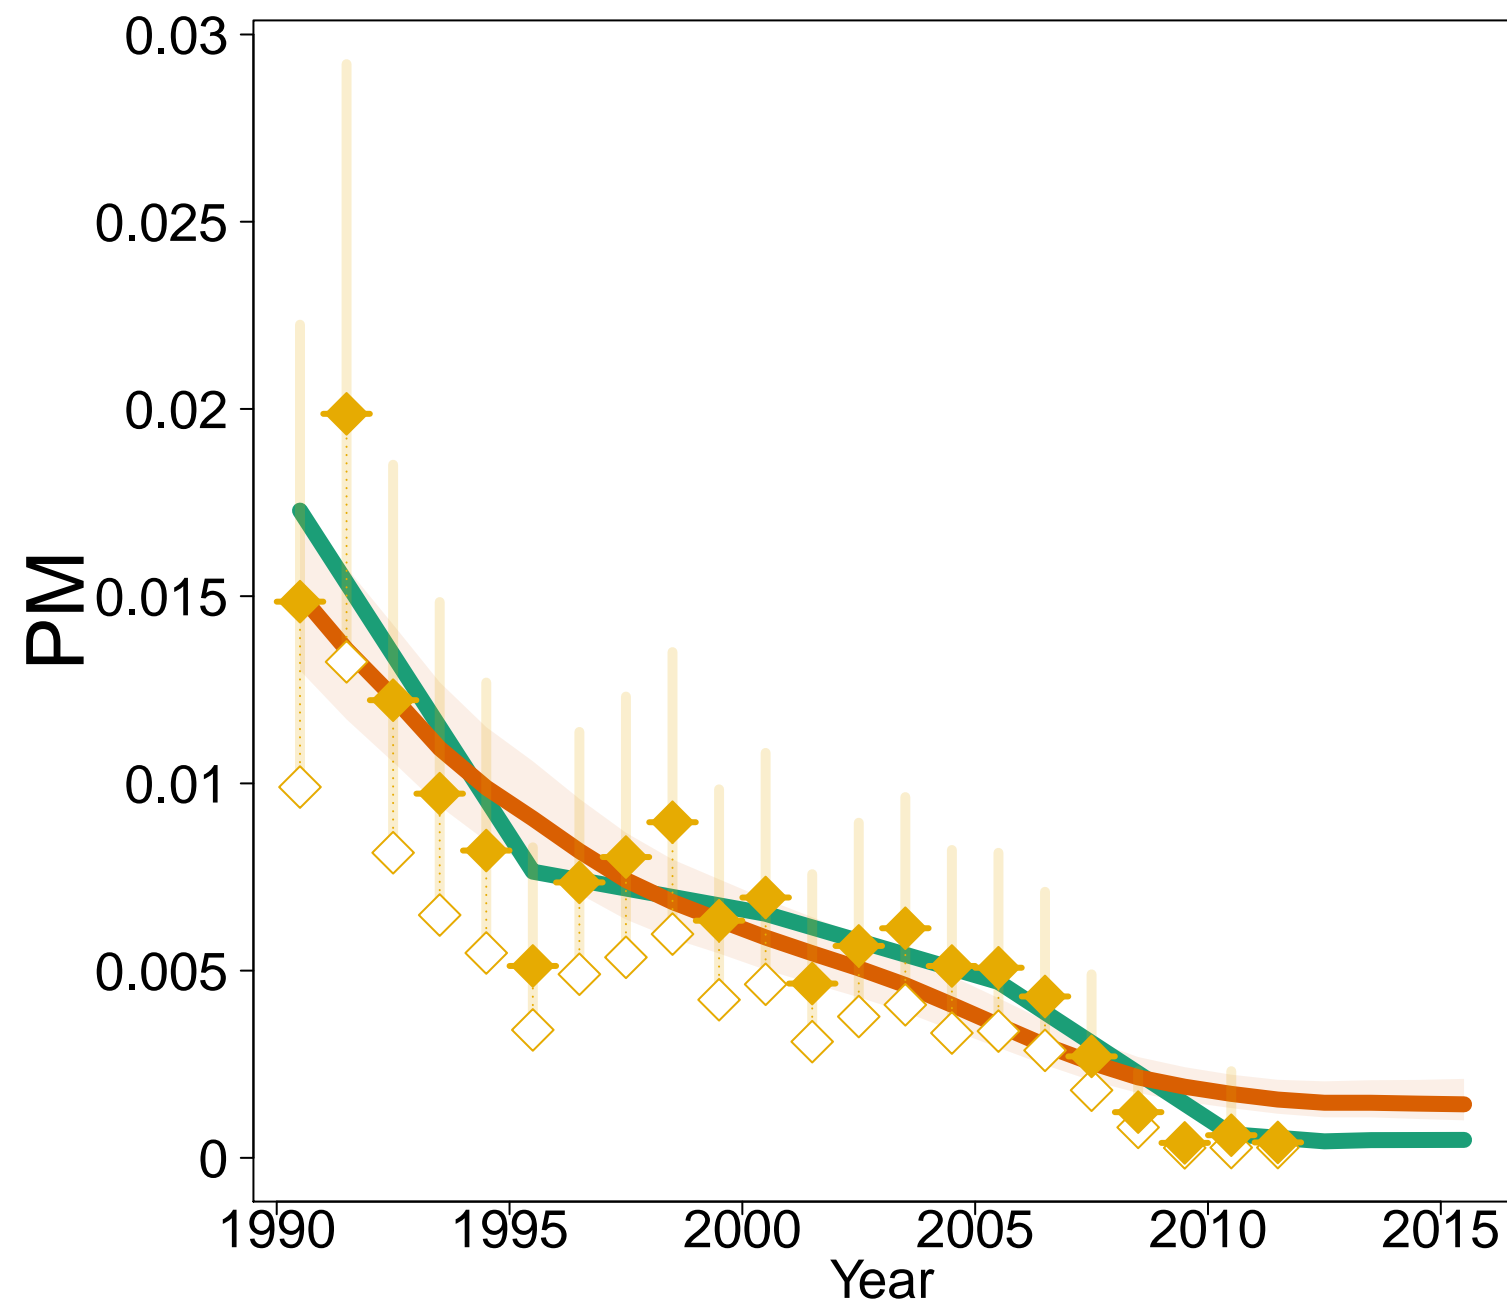

Belarus [BLR; A]  
(Developed regions)

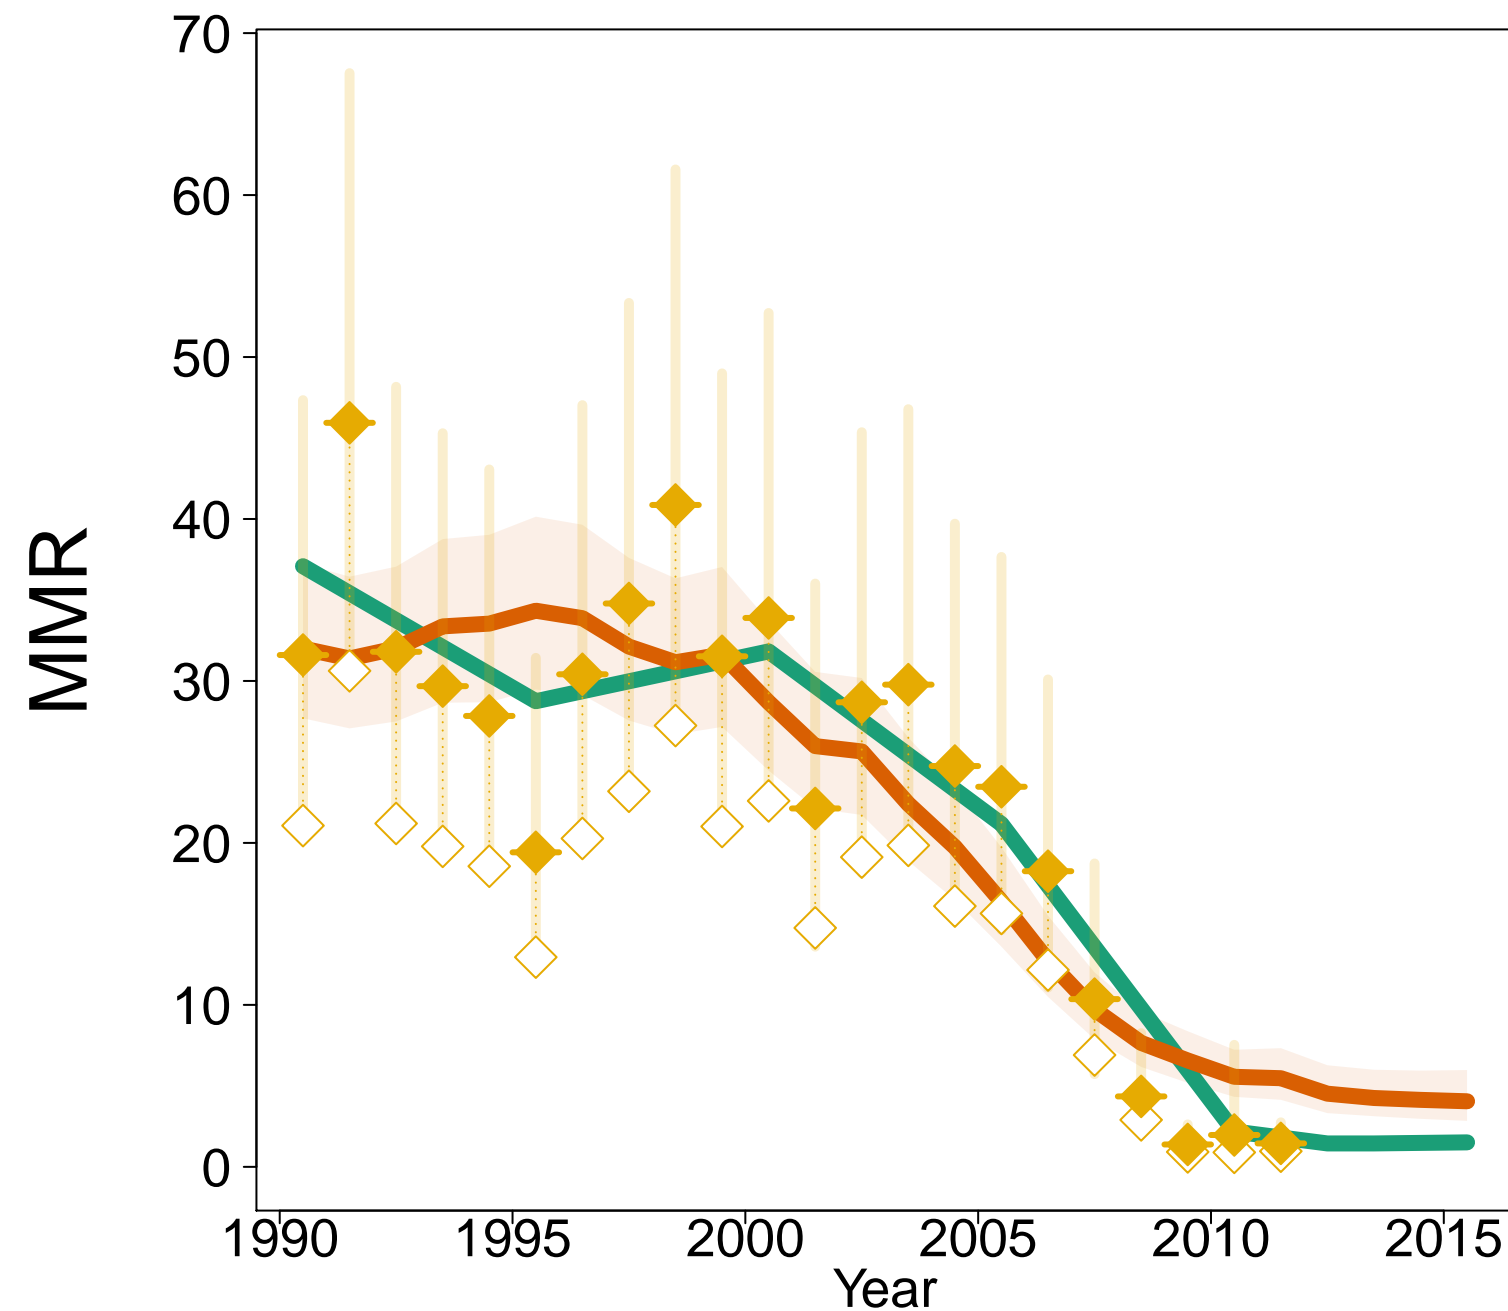

- Estimates –
- Bmat 2014
- MMEIG 2014
- Data –
- Observed Data
- Adjusted Data
- Data type –
- VR

Belgium [BEL; A]  
(Developed regions)

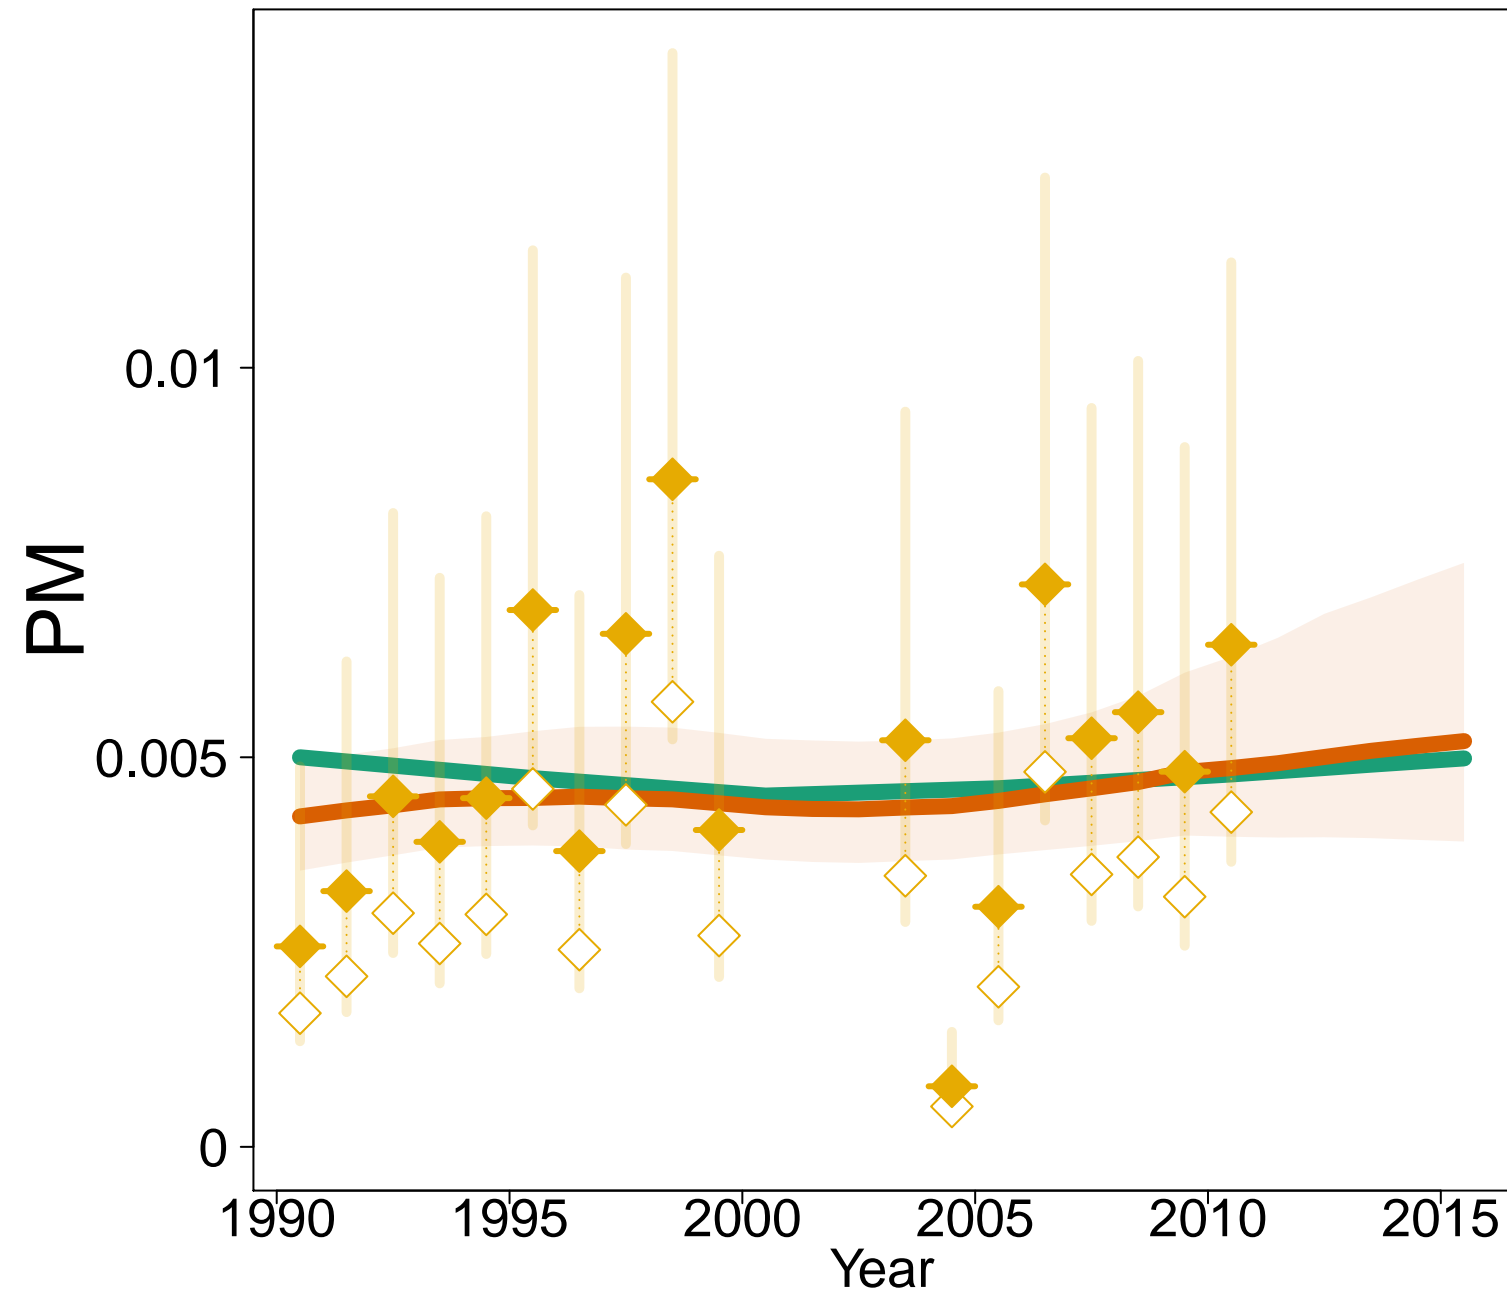

Belgium [BEL; A]  
(Developed regions)

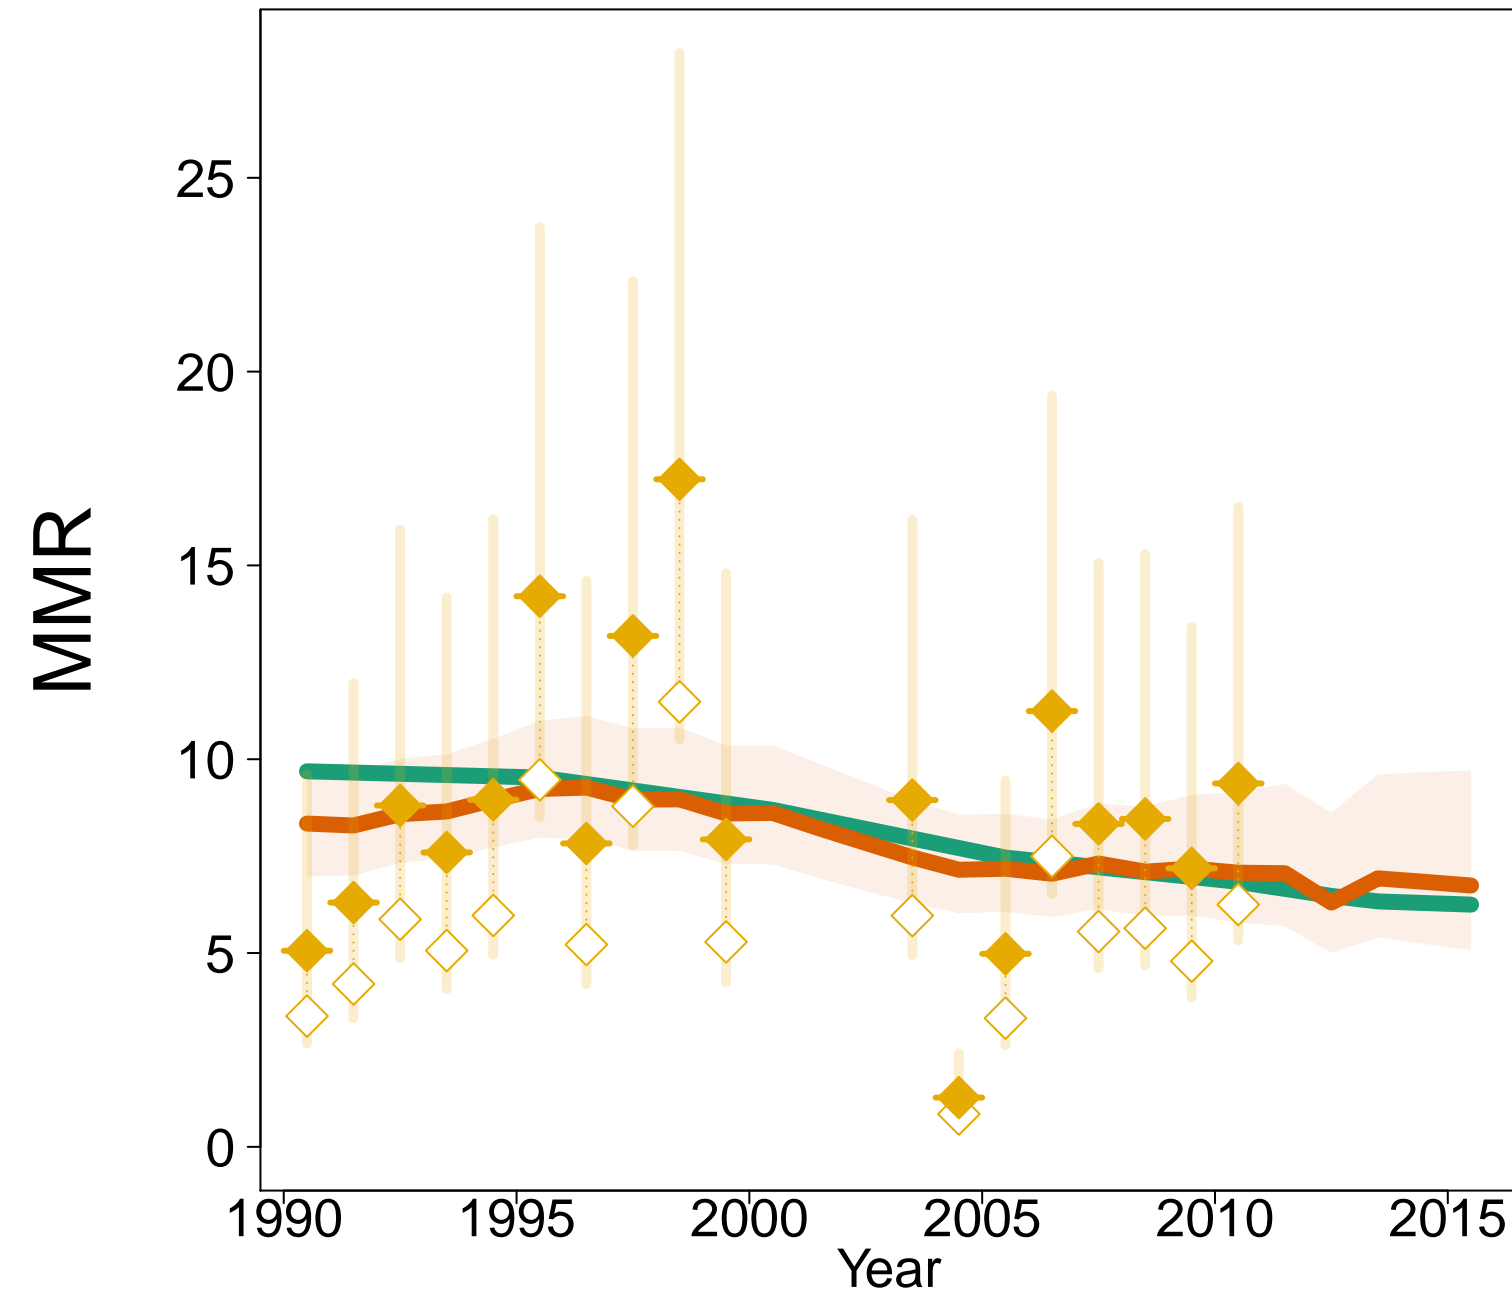

– Estimates –  
Bmat 2014  
MMEIG 2014  
– Data –  
Observed Data  
Adjusted Data  
– Data type –  
VR

Belize [BLZ; A]  
(Central America)

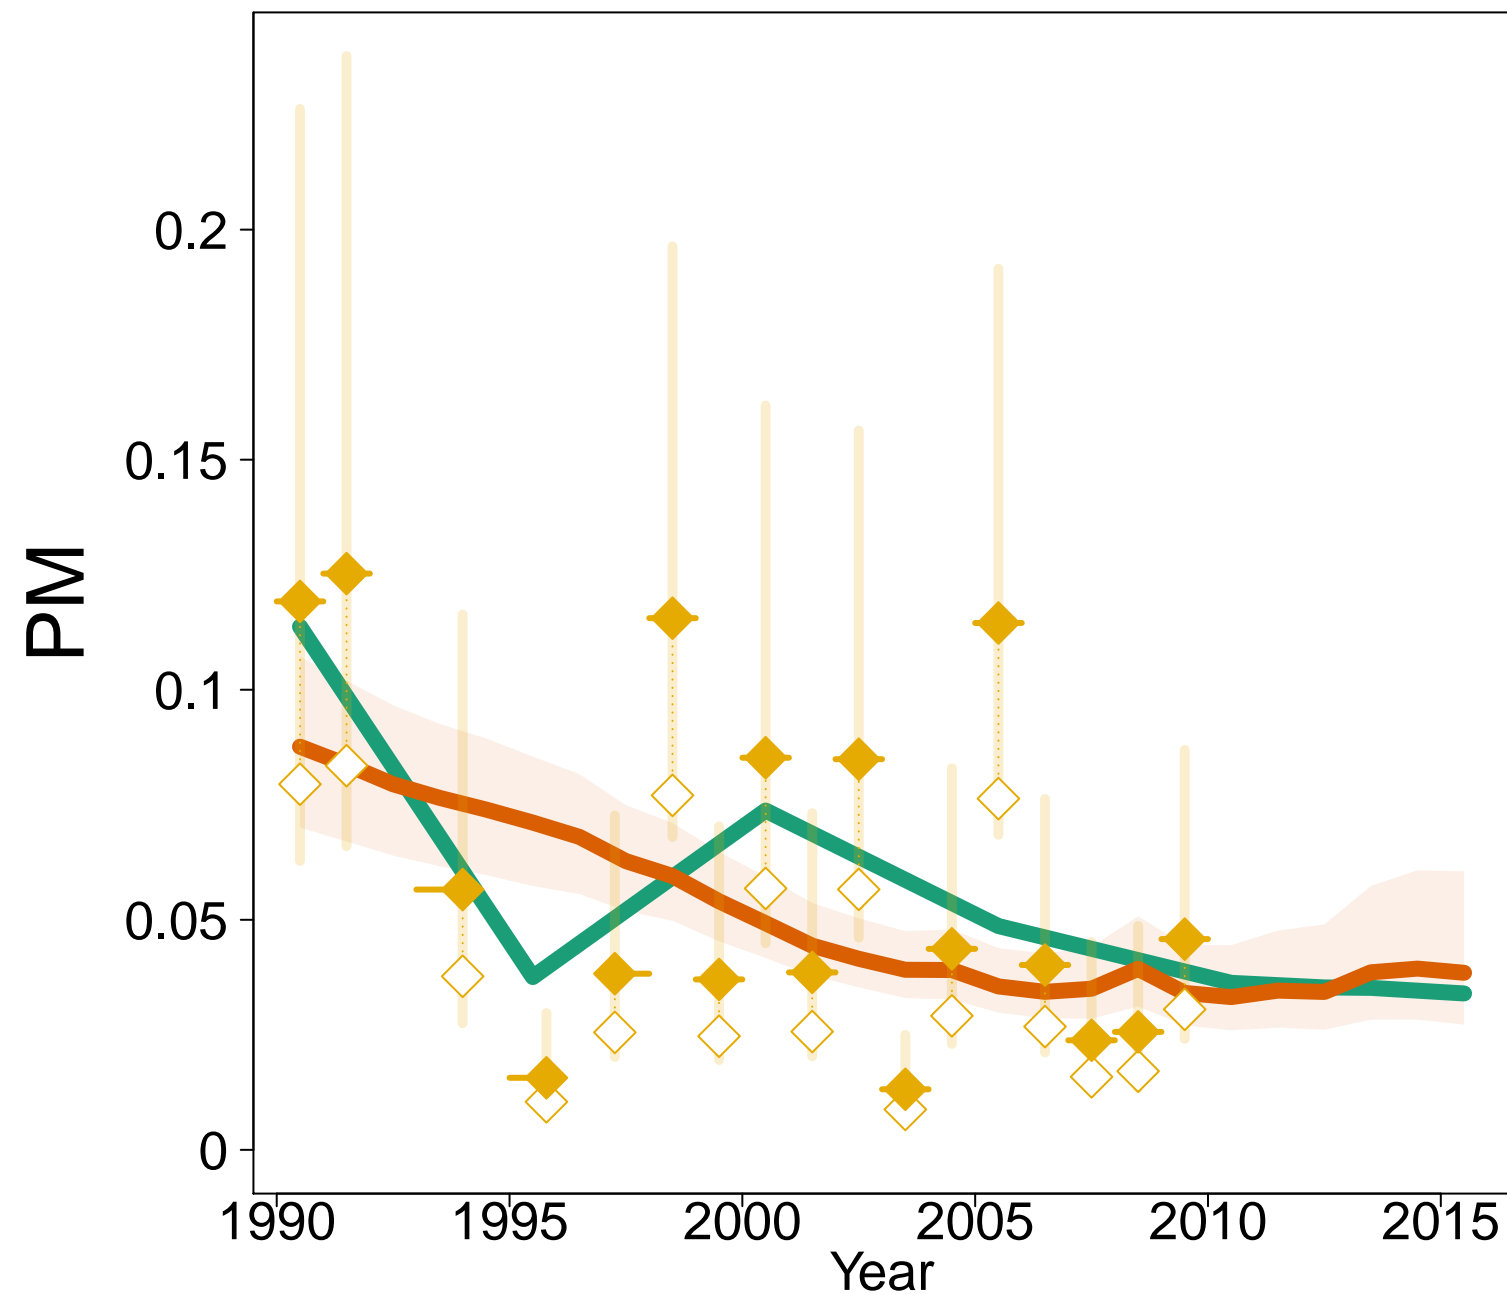

Belize [BLZ; A]  
(Central America)

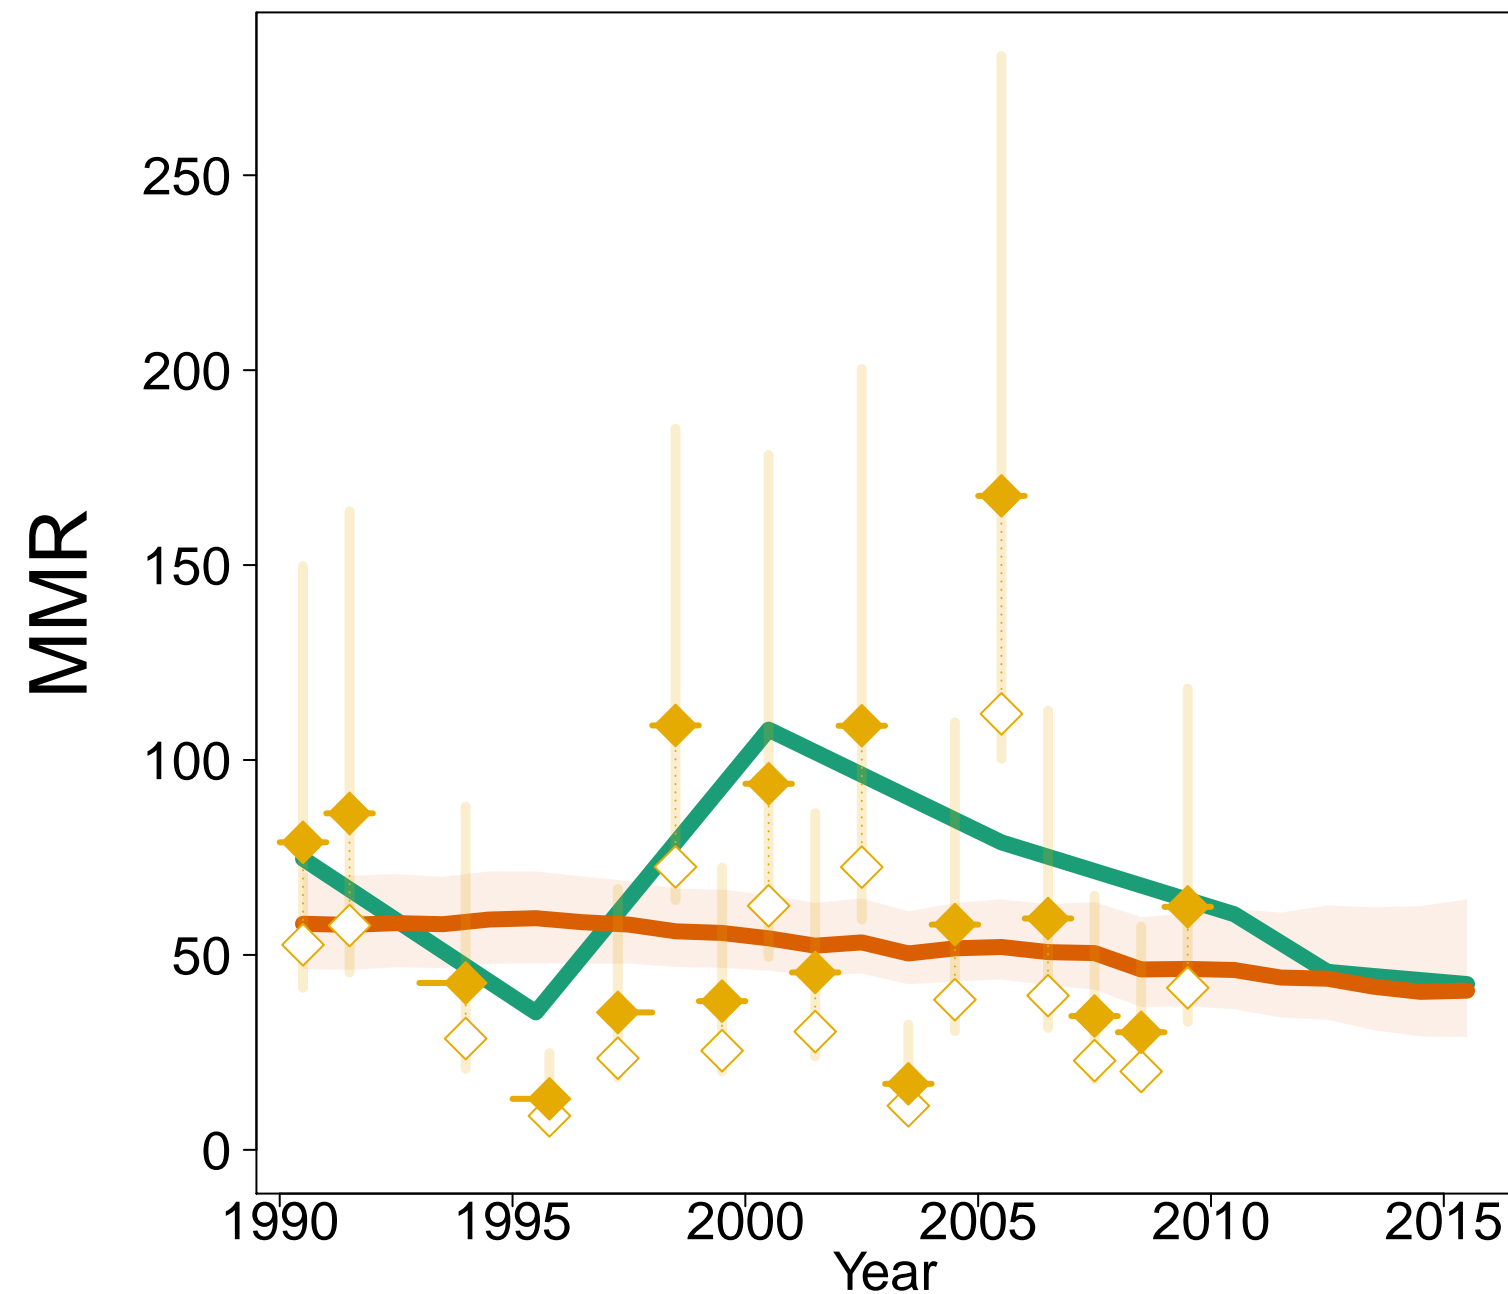

- Estimates –
- Bmat 2014
- MMEIG 2014
- Data –
- Observed Data
- Adjusted Data
- Data type –
- VR



Benin [BEN; B]  
(Western Africa)

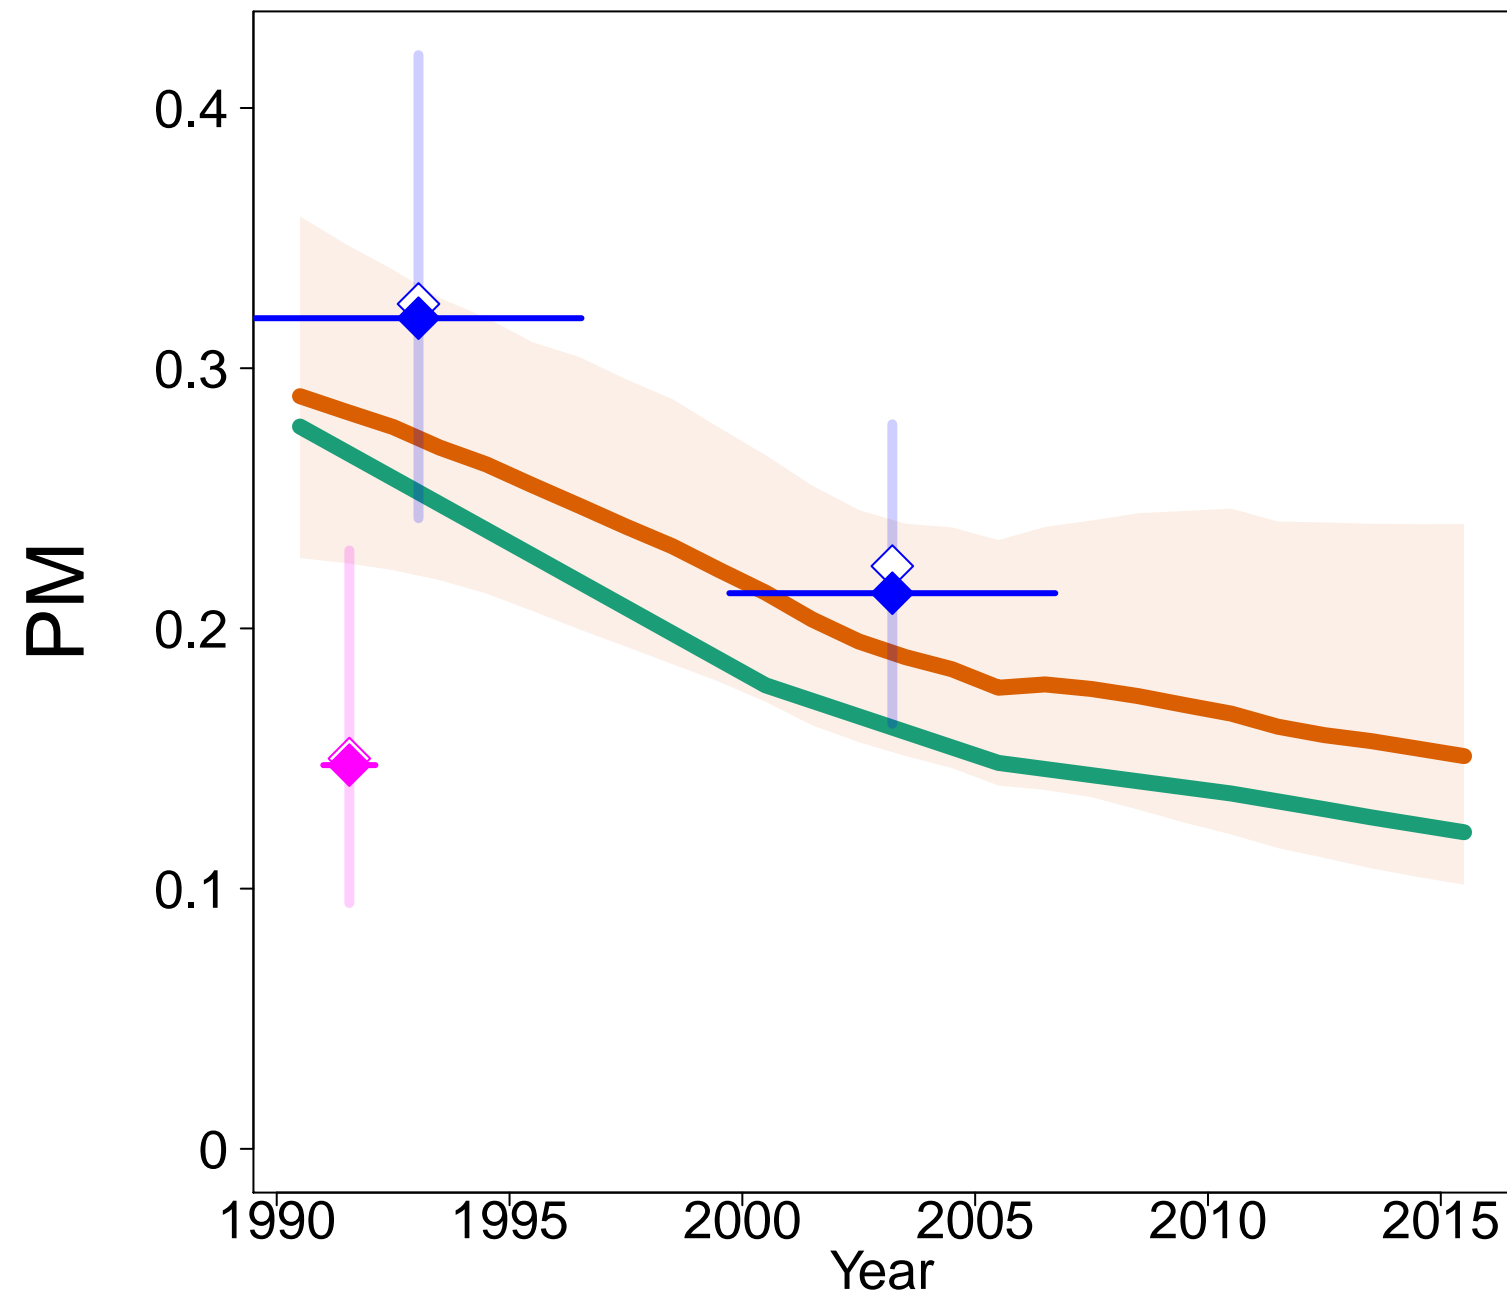

Benin [BEN; B]  
(Western Africa)

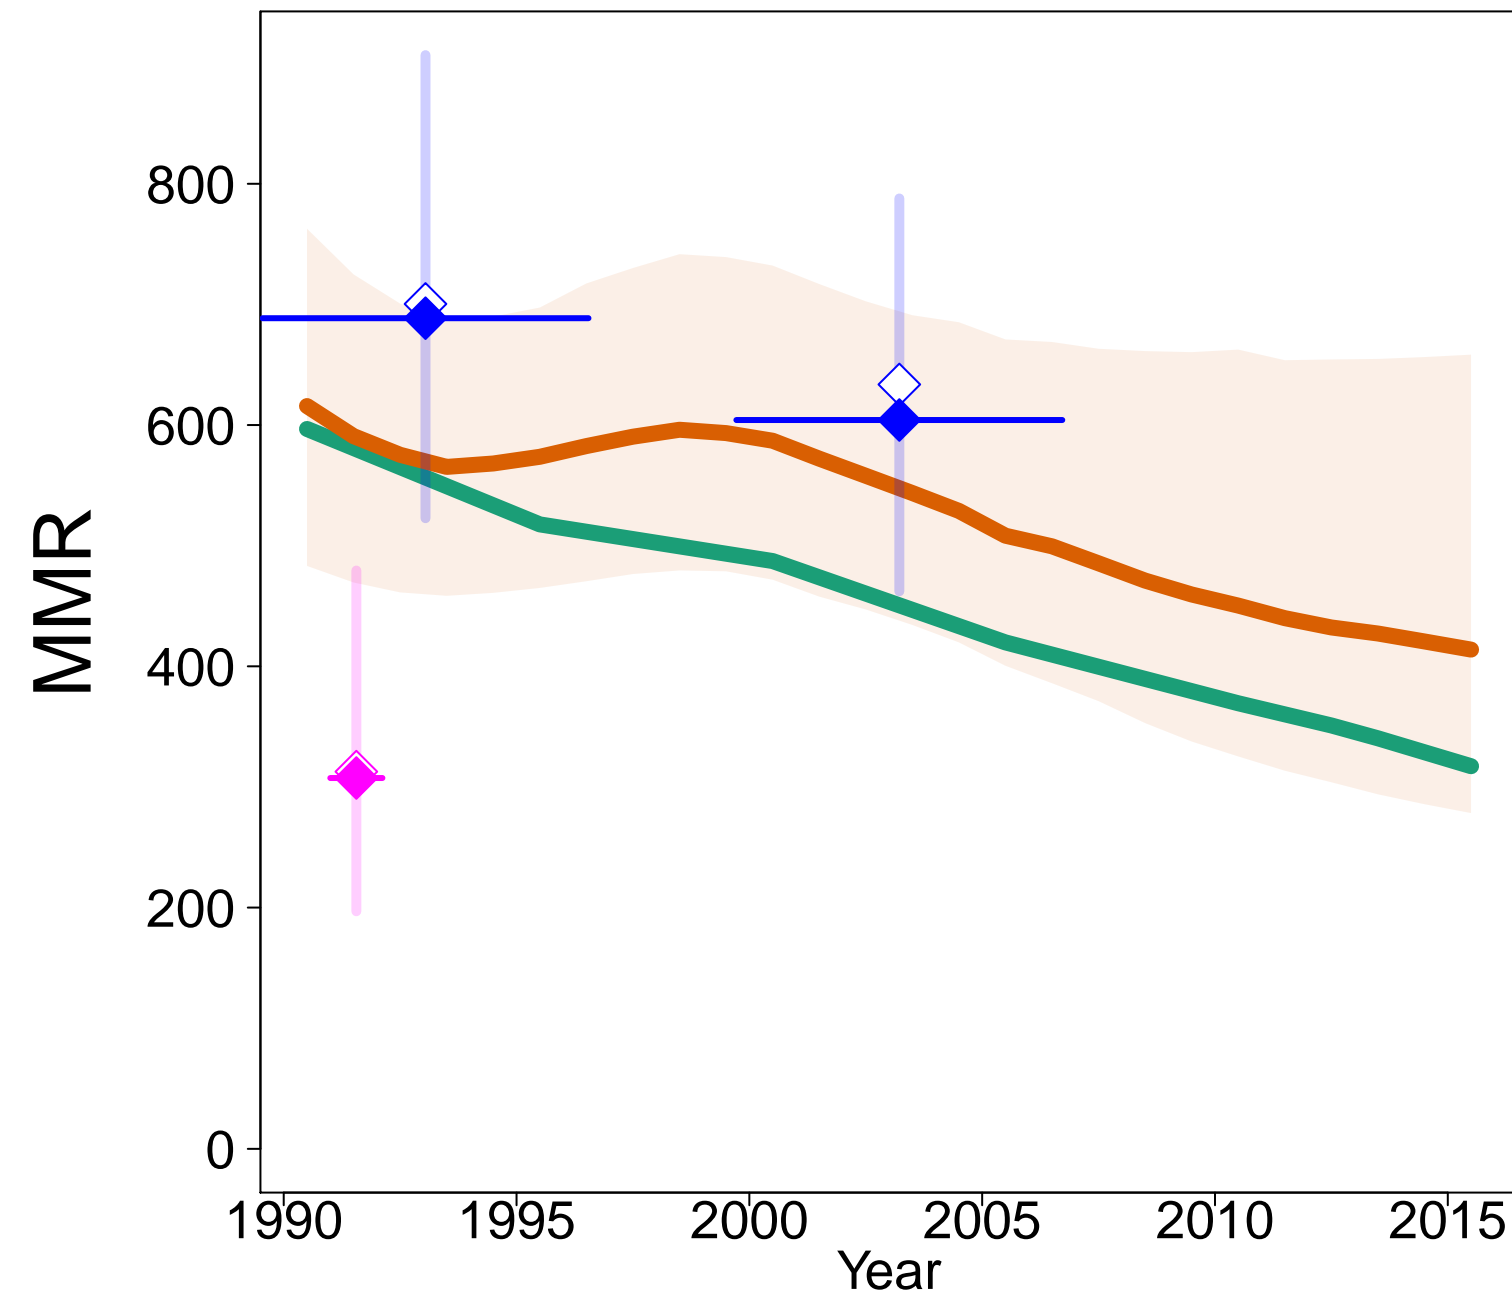

- Estimates –
- Bmat 2014
- MMEIG 2014
- Data –
- ◊ Observed Data
- ◼ Adjusted Data
- Data type –
- ◆ DHS
- ◆ Census

Bhutan [BTN; B]  
(Southern Asia)

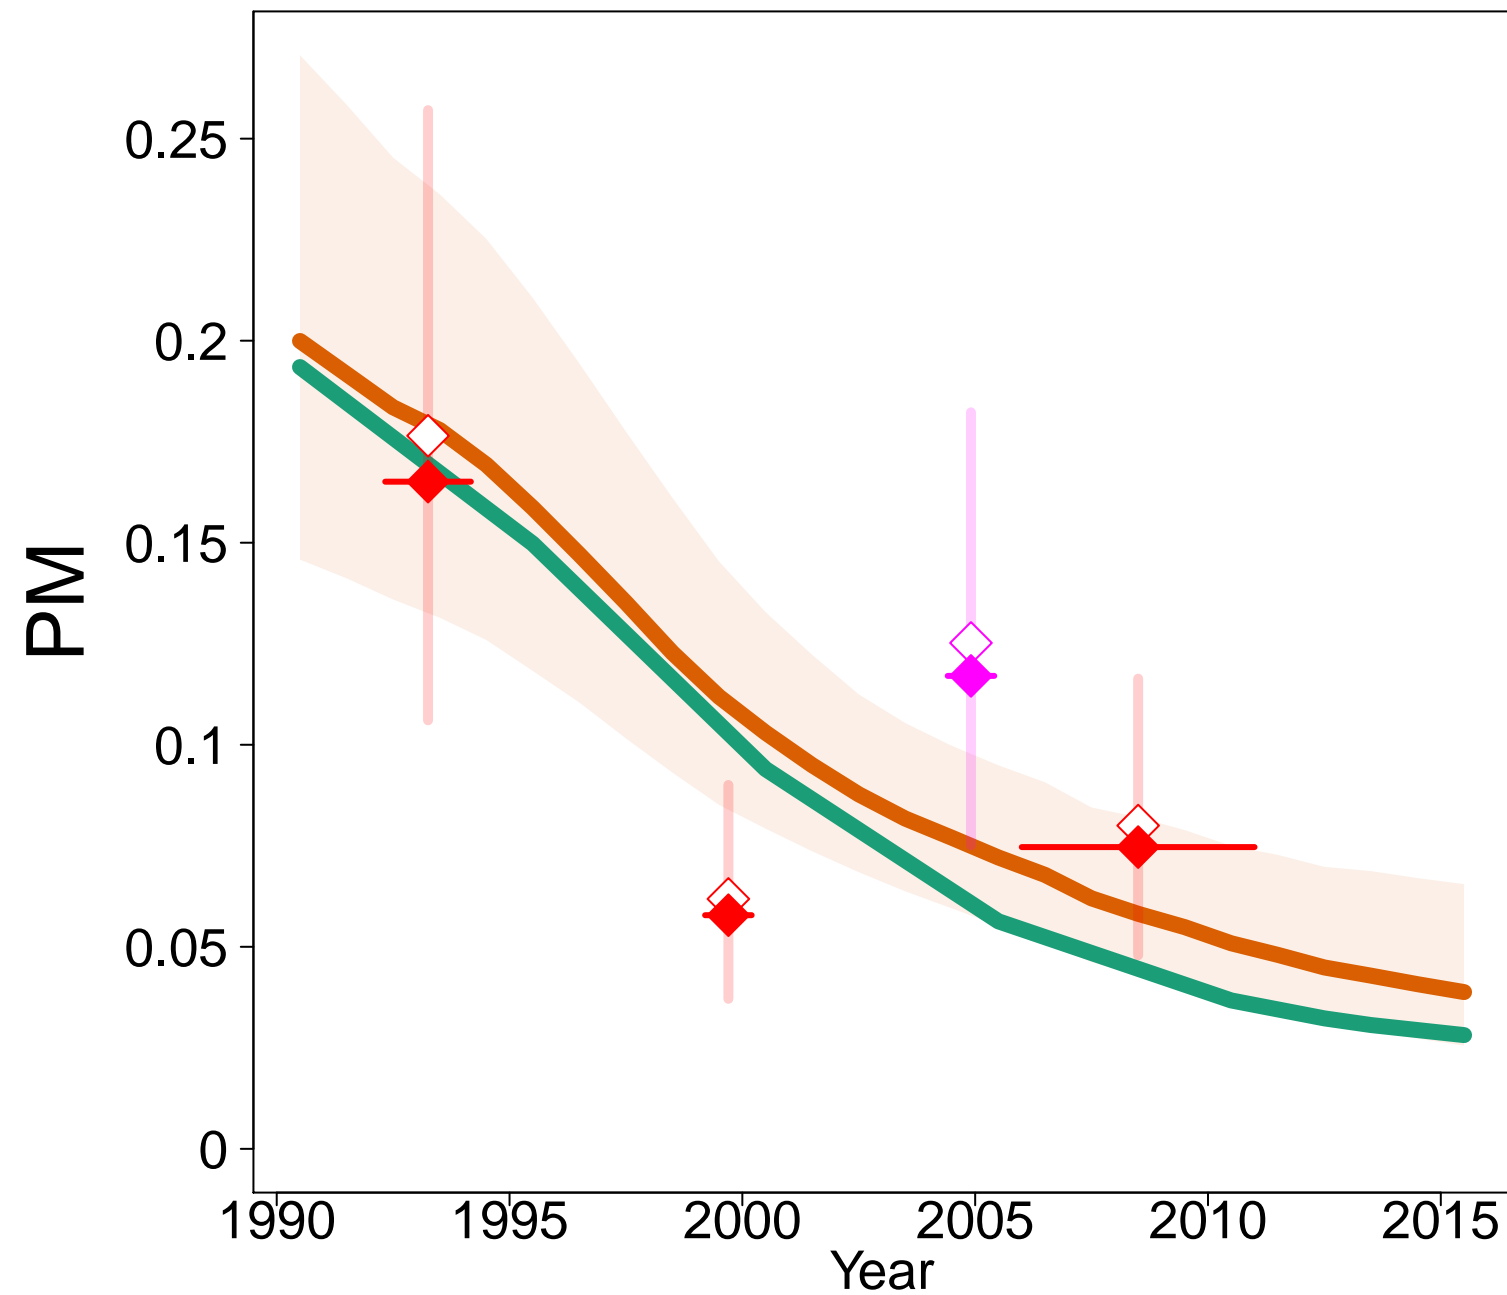

Bhutan [BTN; B]  
(Southern Asia)

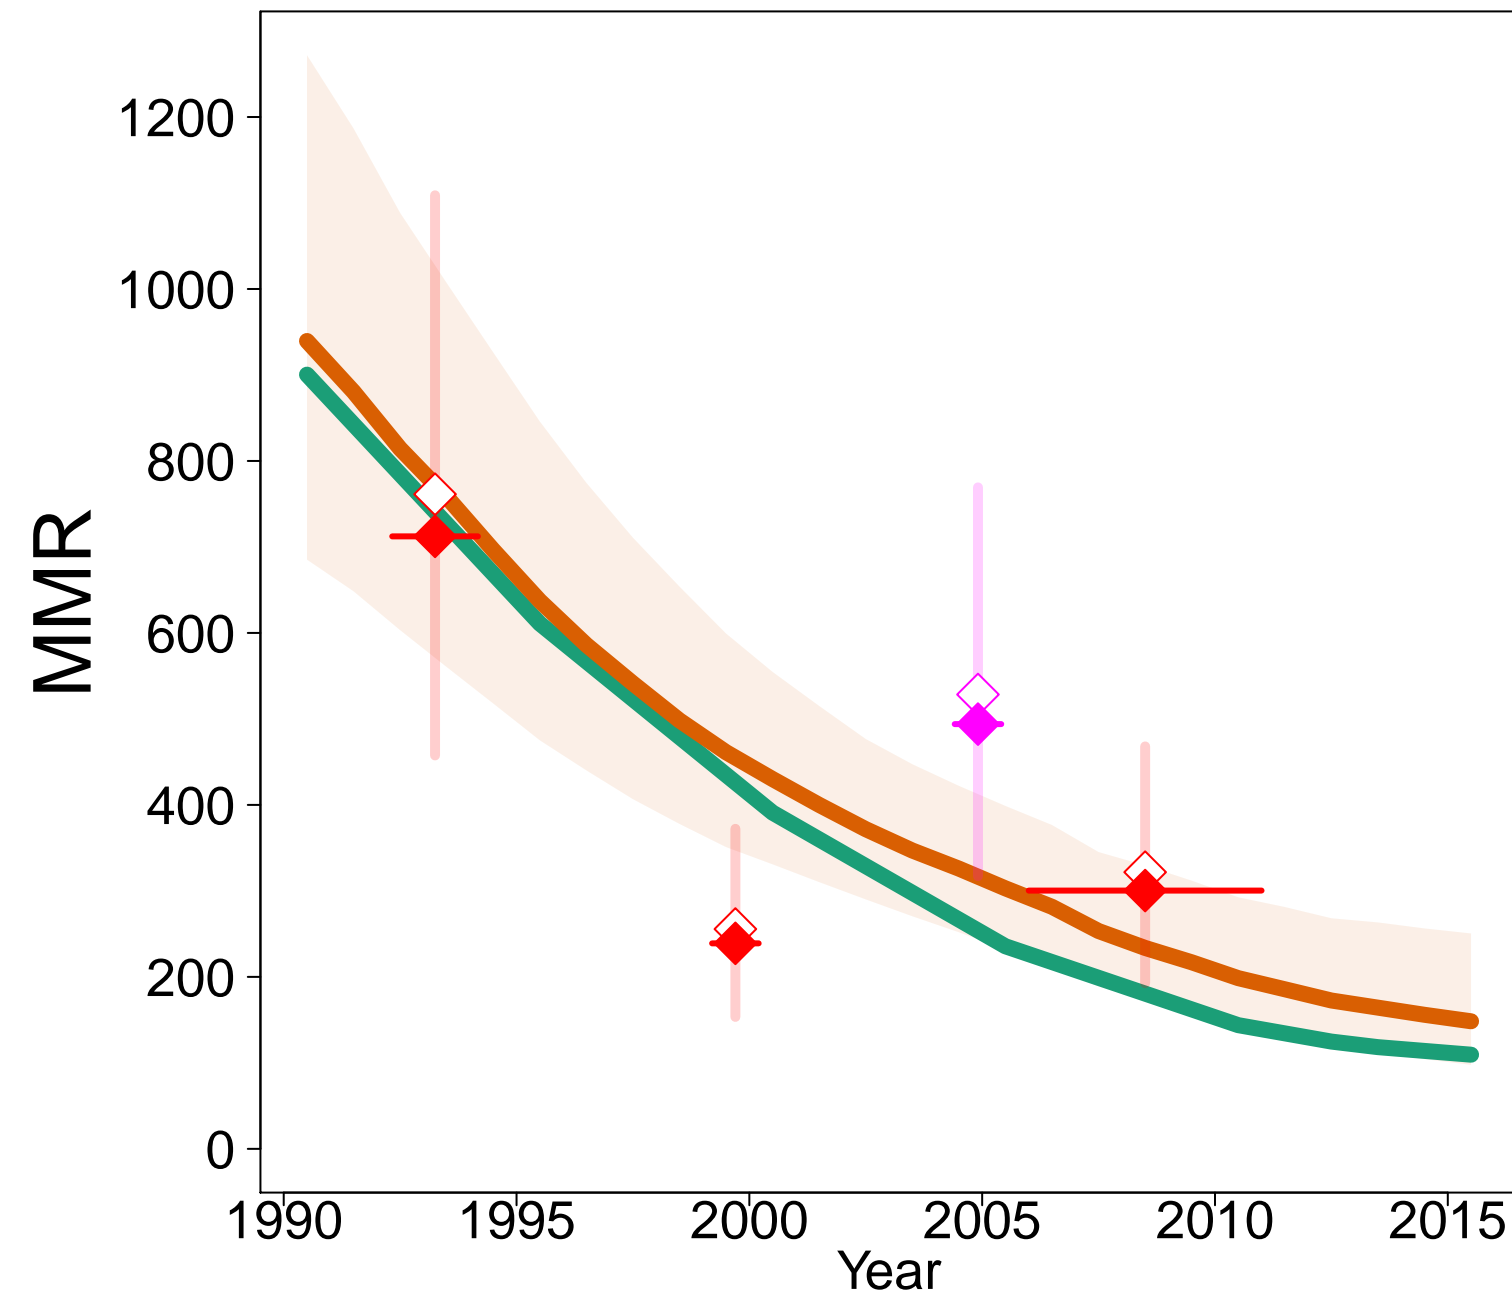

- Estimates –
- Bmat 2014
- MMEIG 2014
- Data –
- Observed Data
- Adjusted Data
- Data type –
- Census
- Misc. studies

Bolivia [BOL; B]  
(South America)

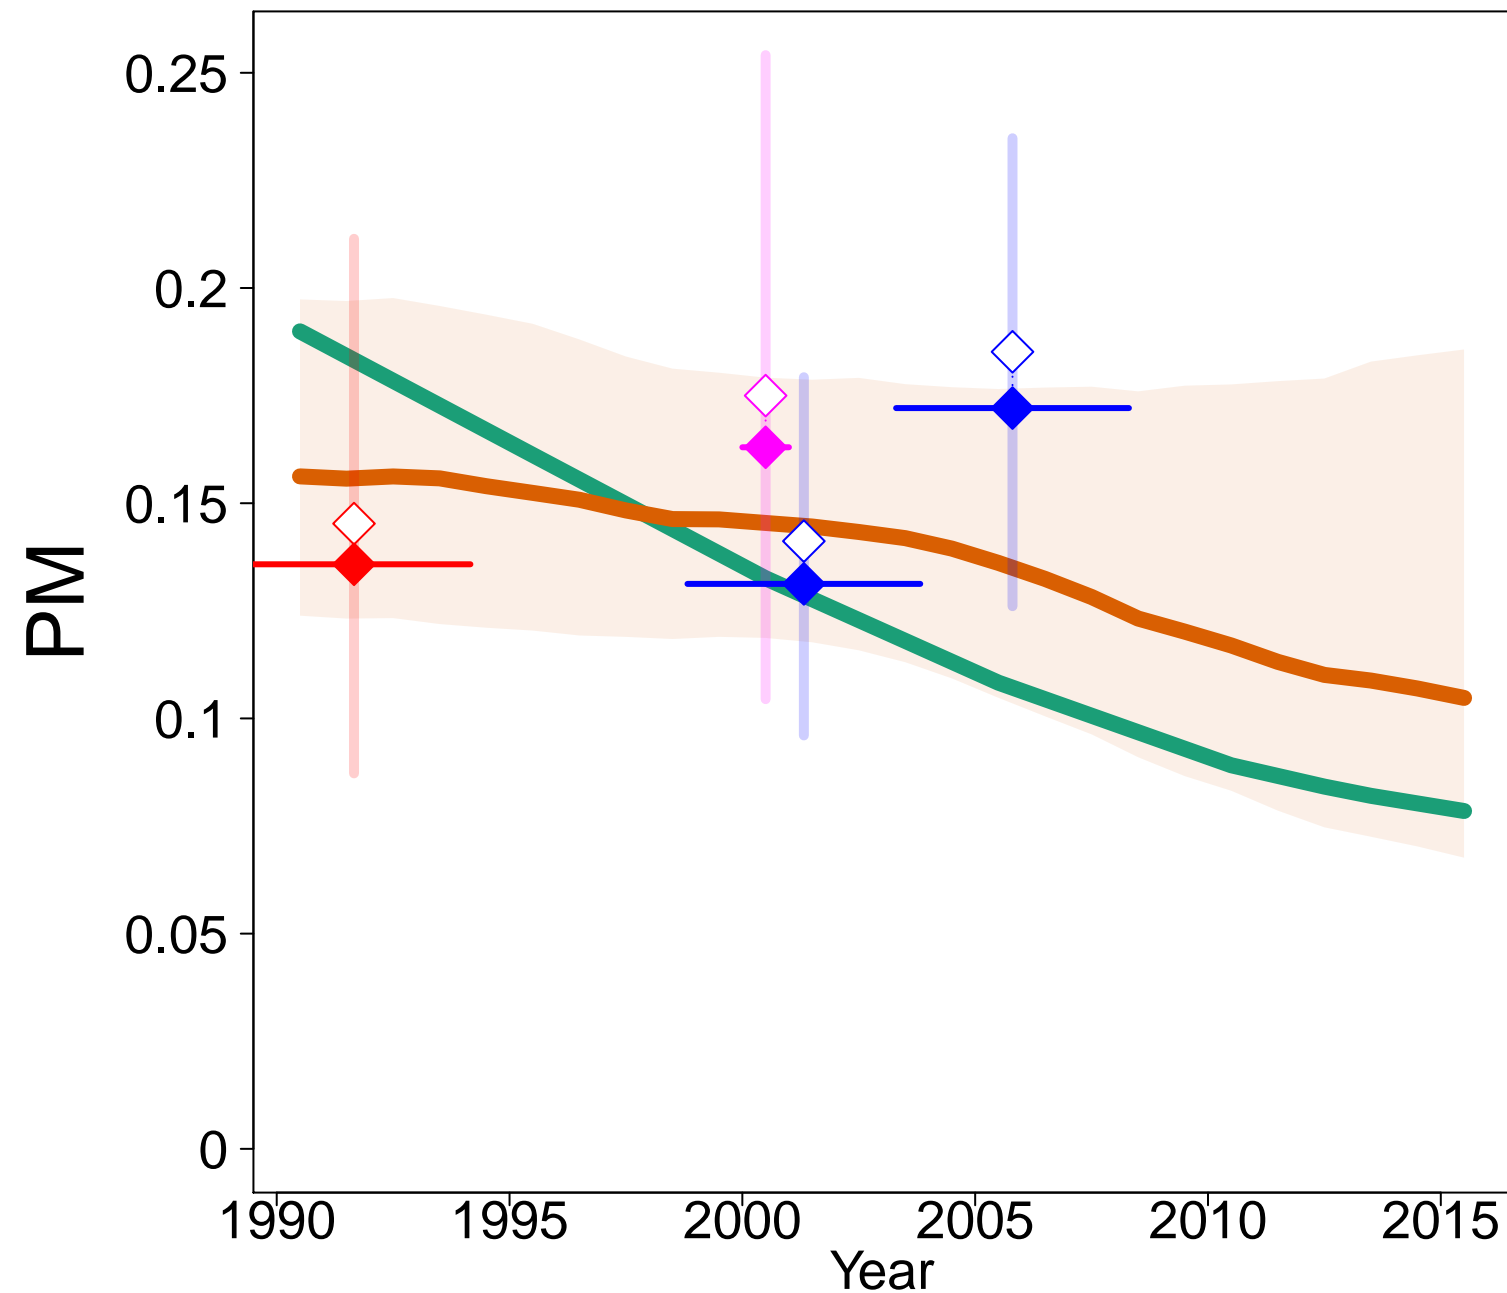

Bolivia [BOL; B]  
(South America)

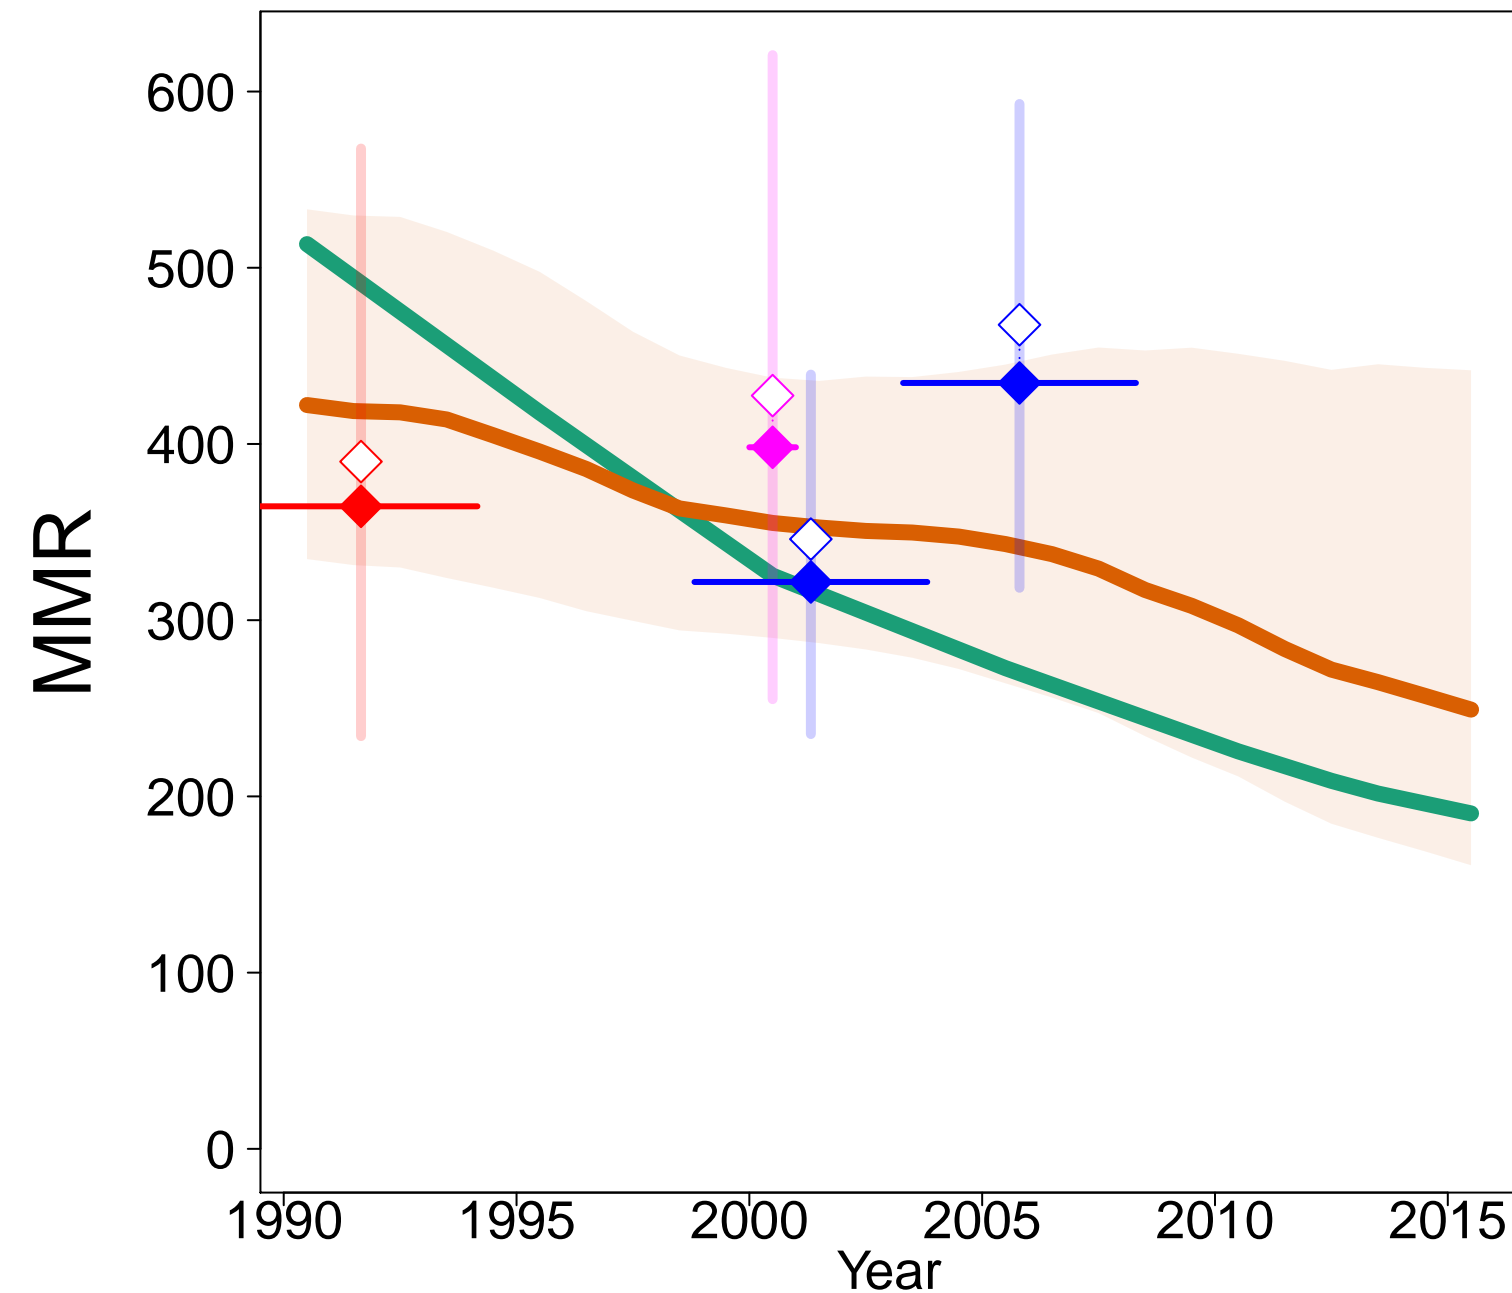

- Estimates –
- Bmat 2014
- MMEIG 2014
- Data –
- Observed Data
- Adjusted Data
- Data type –
- DHS
- Census
- Misc. studies

Bosnia and Herzegovina [BIH; B]  
(Transition countries of South-Eastern Europe)

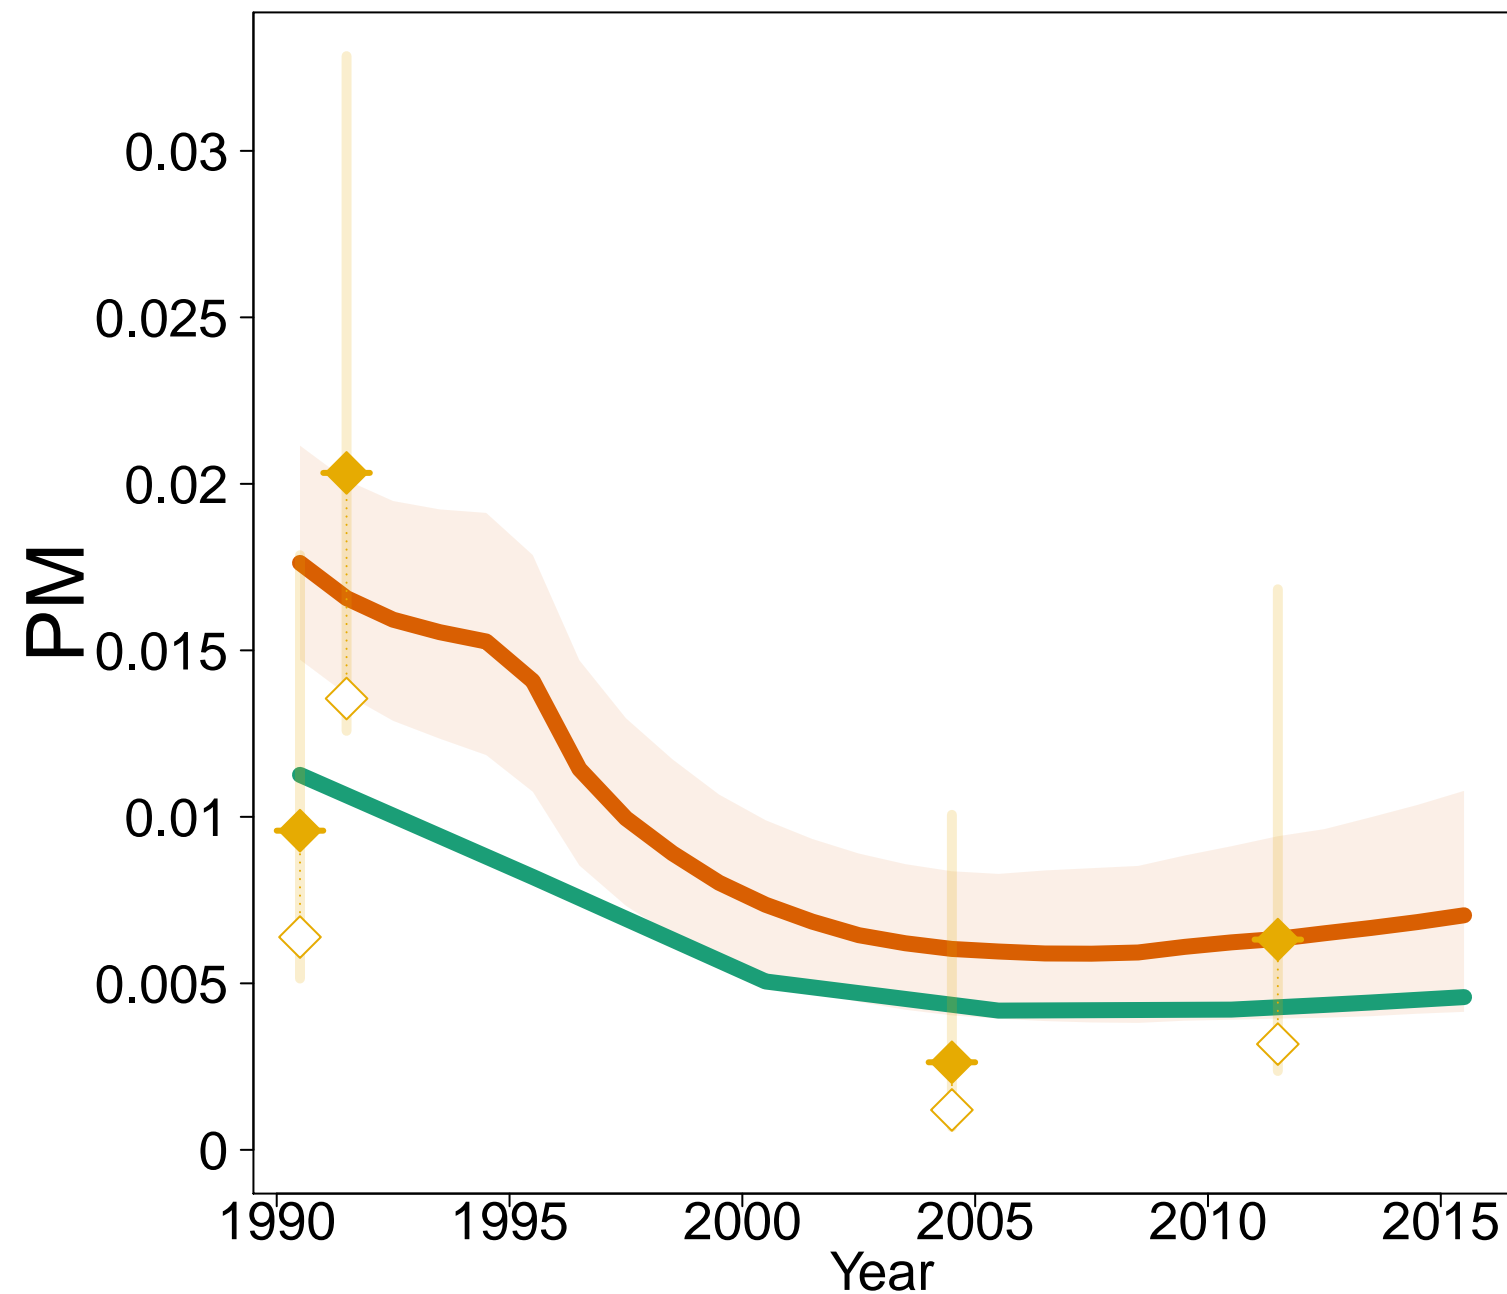

Bosnia and Herzegovina [BIH; B]  
(Transition countries of South-Eastern Europe)

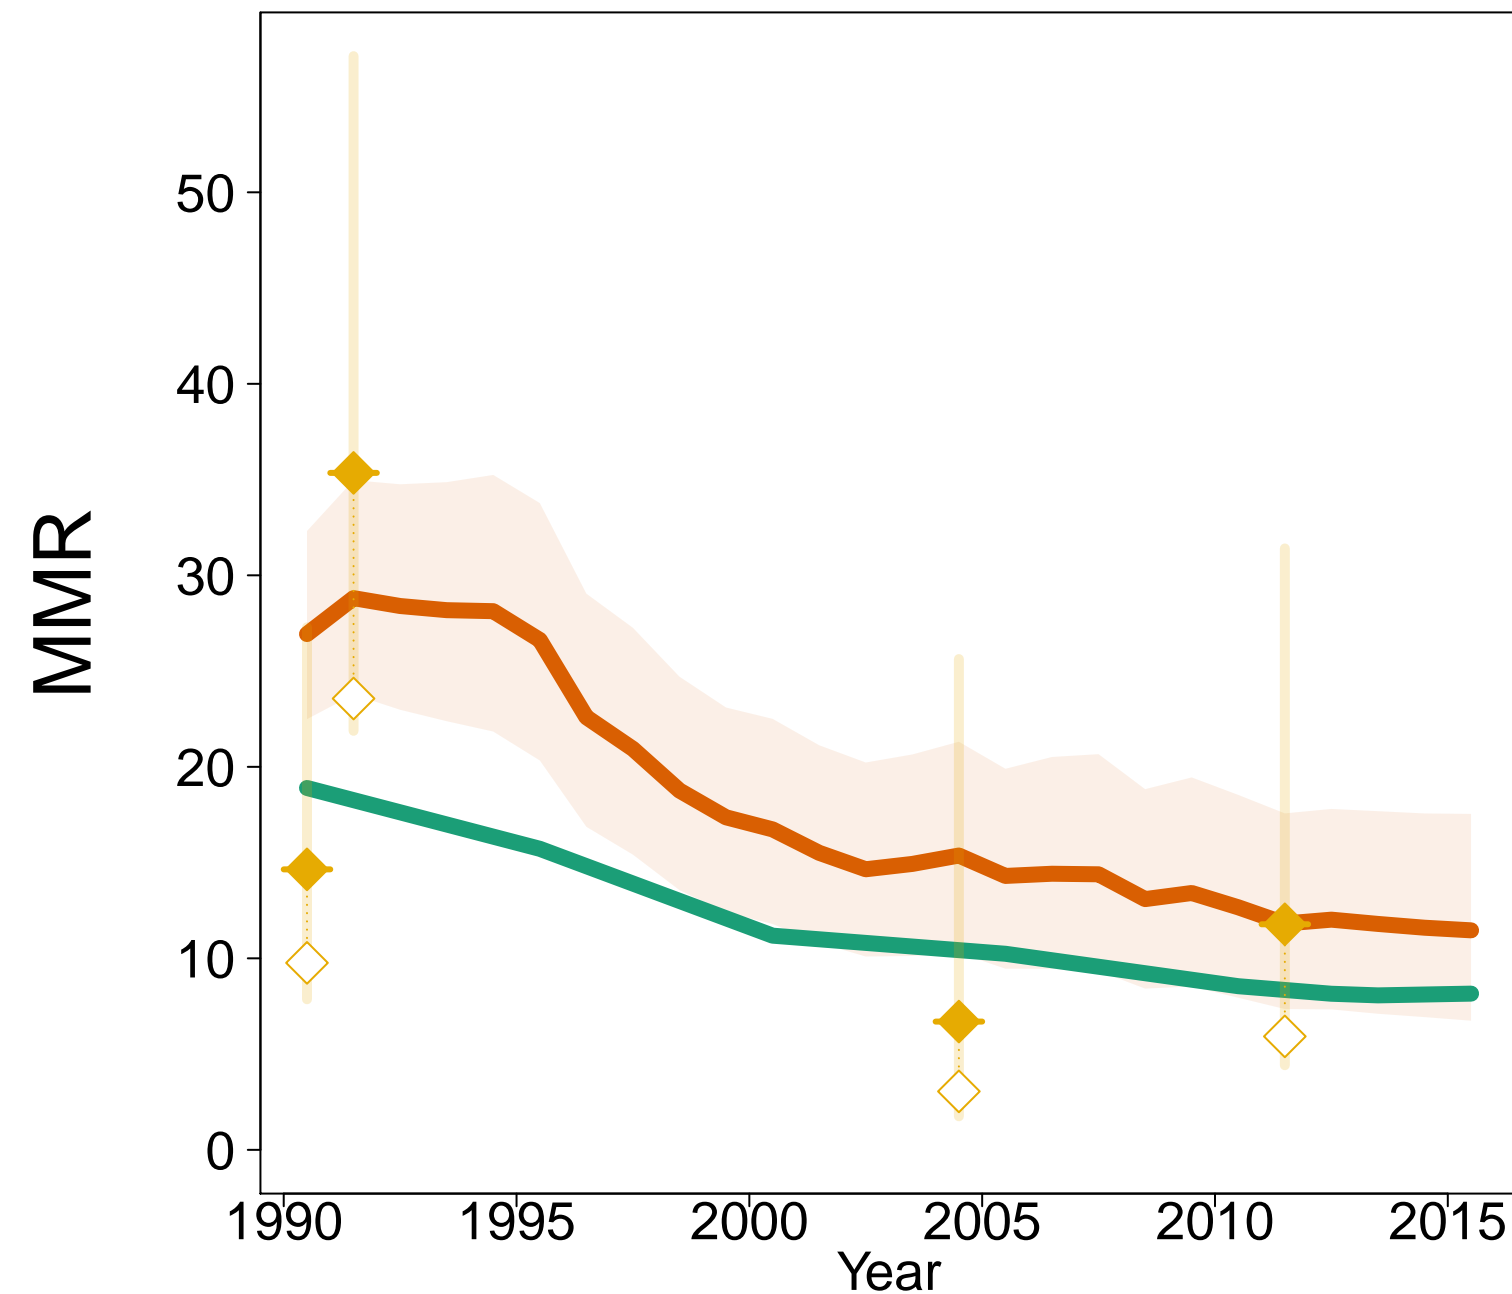

- Estimates –
- Bmat 2014
- MMEIG 2014
- Data –
- Observed Data
- Adjusted Data
- Data type –
- VR

Botswana [BWA; B]  
(Southern Africa)

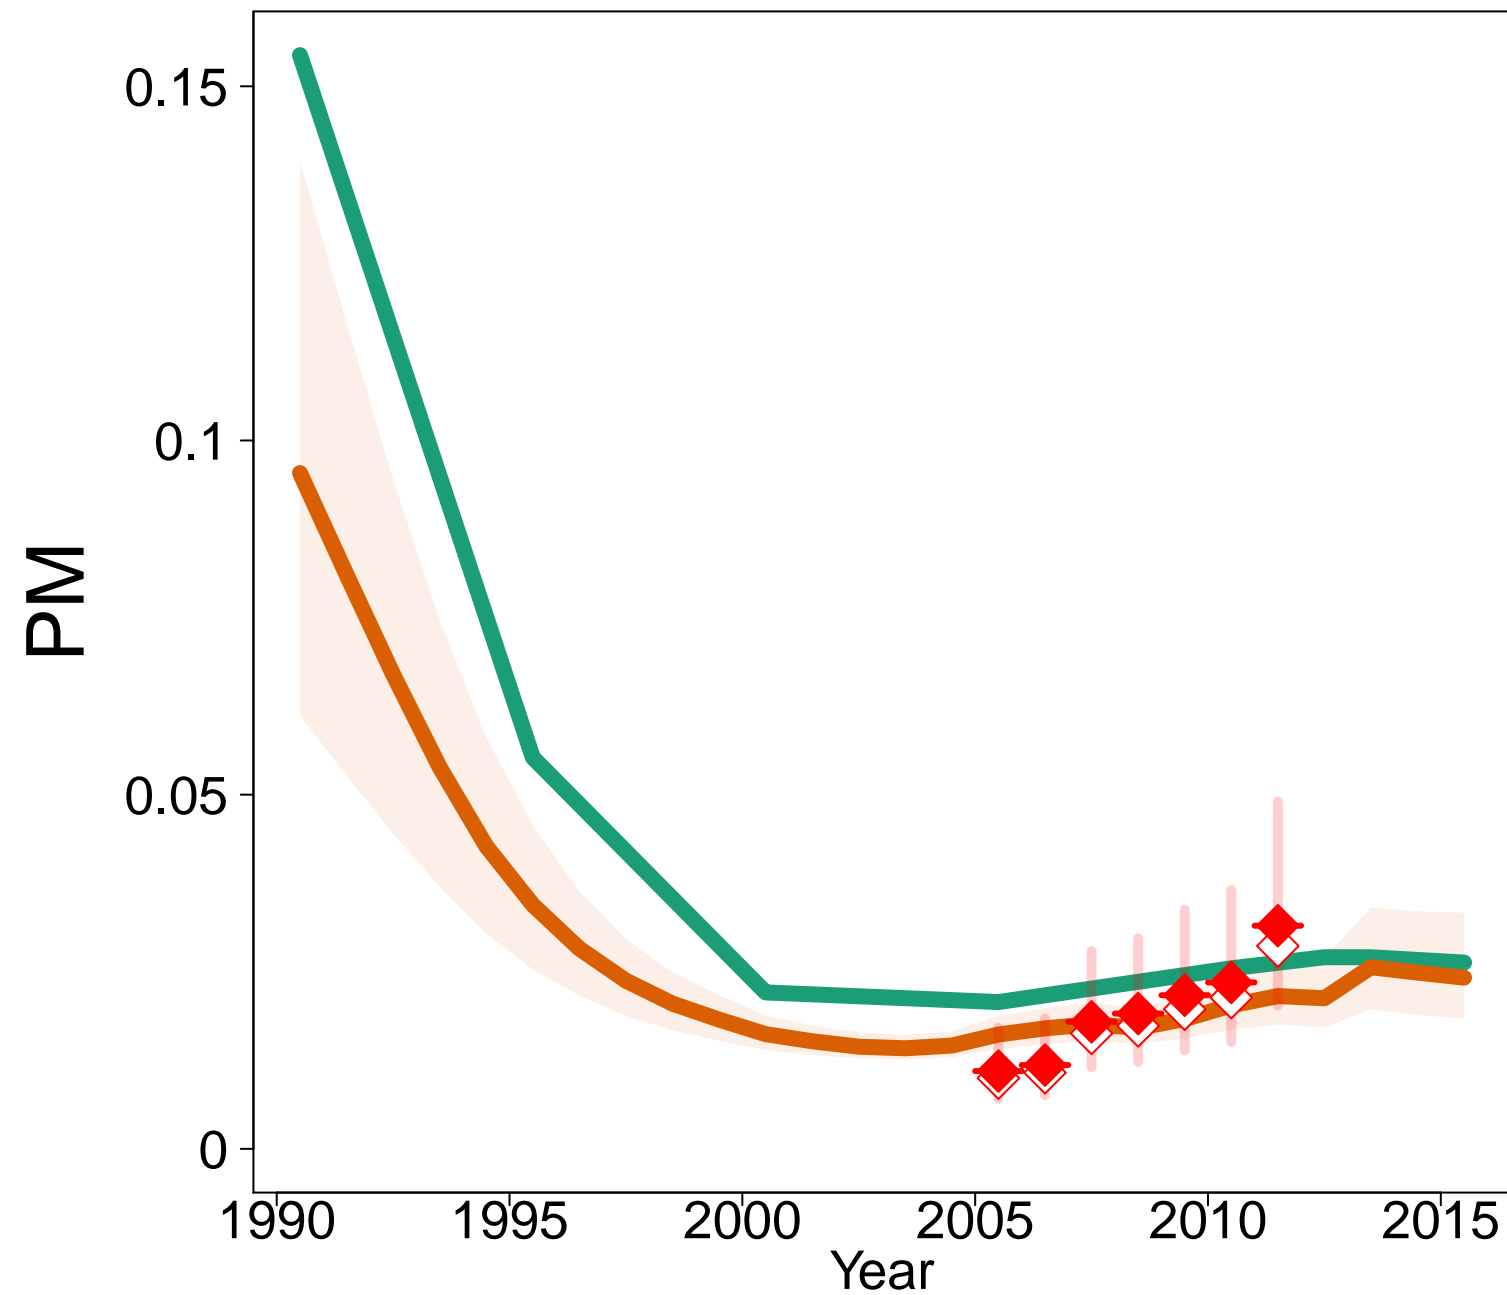

Botswana [BWA; B]  
(Southern Africa)

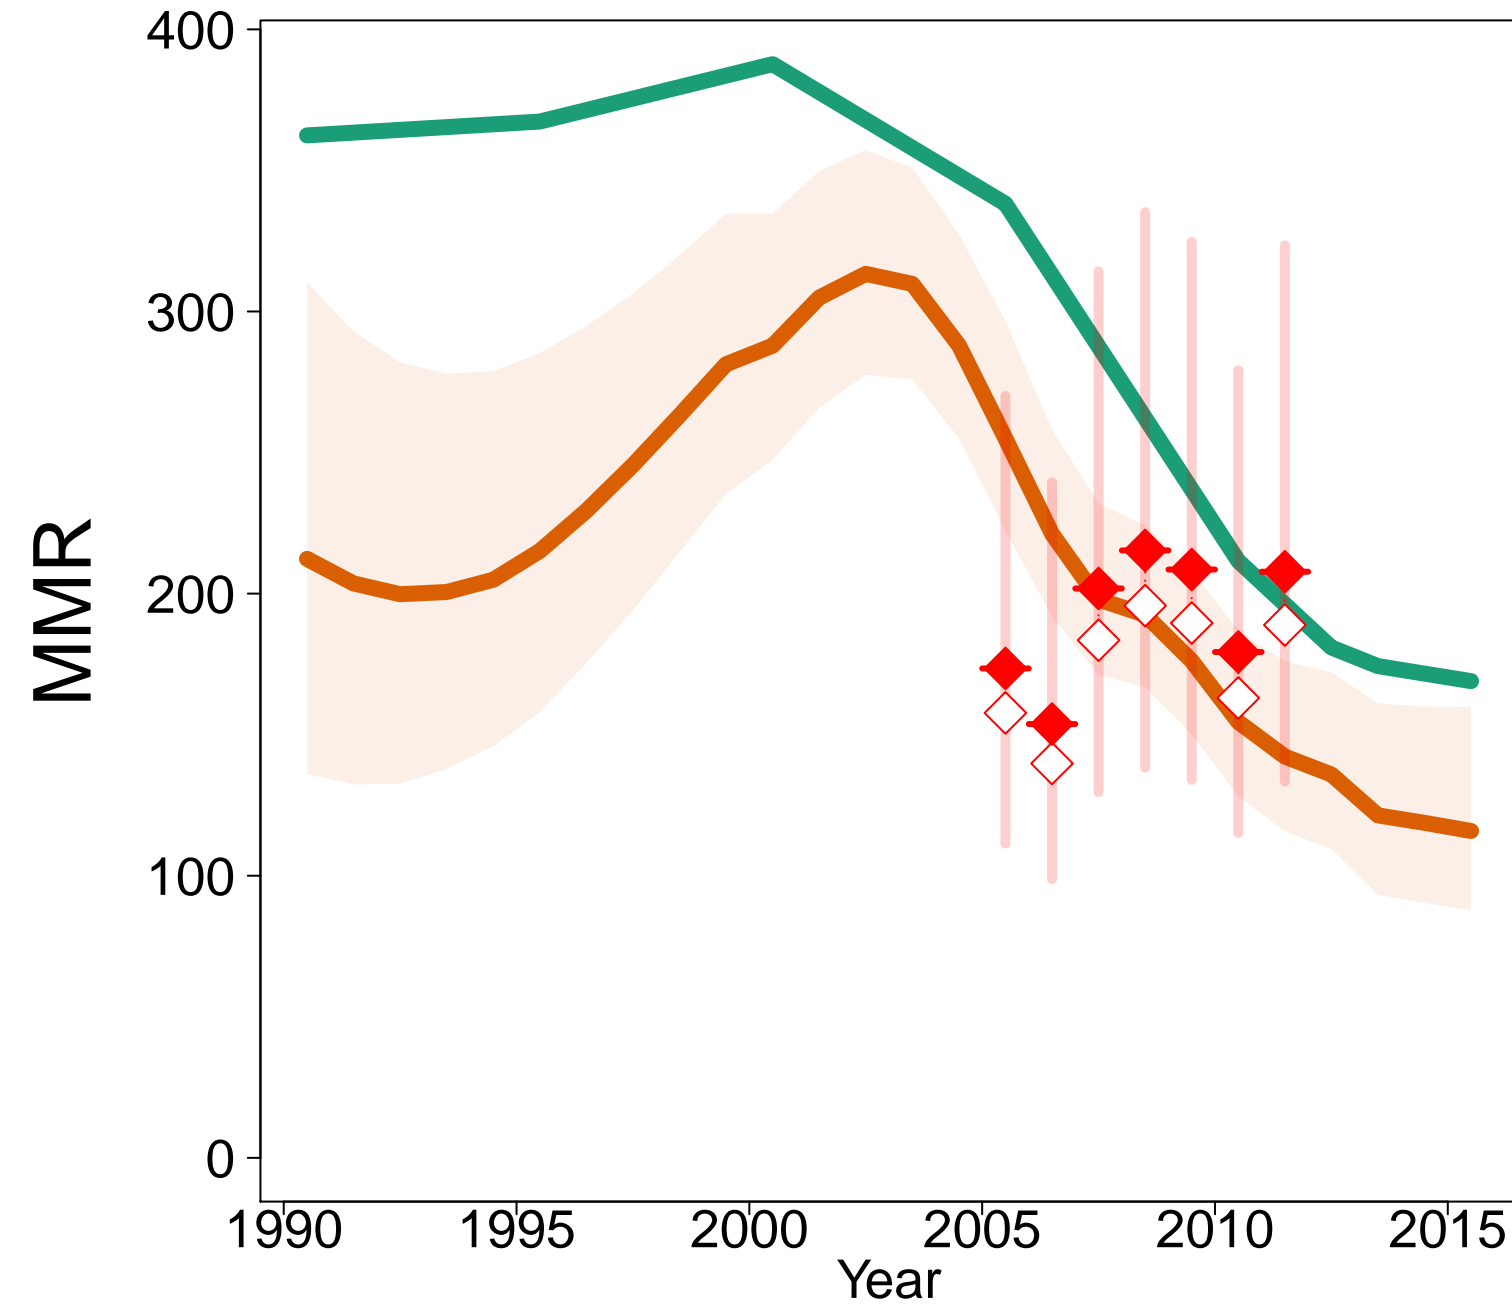

- Estimates –
- Bmat 2014
- MMEIG 2014
- Data –
- ◊ Observed Data
- ◆ Adjusted Data
- Data type –
- ◆ Misc. studies

Brazil [BRA; B]  
(South America)

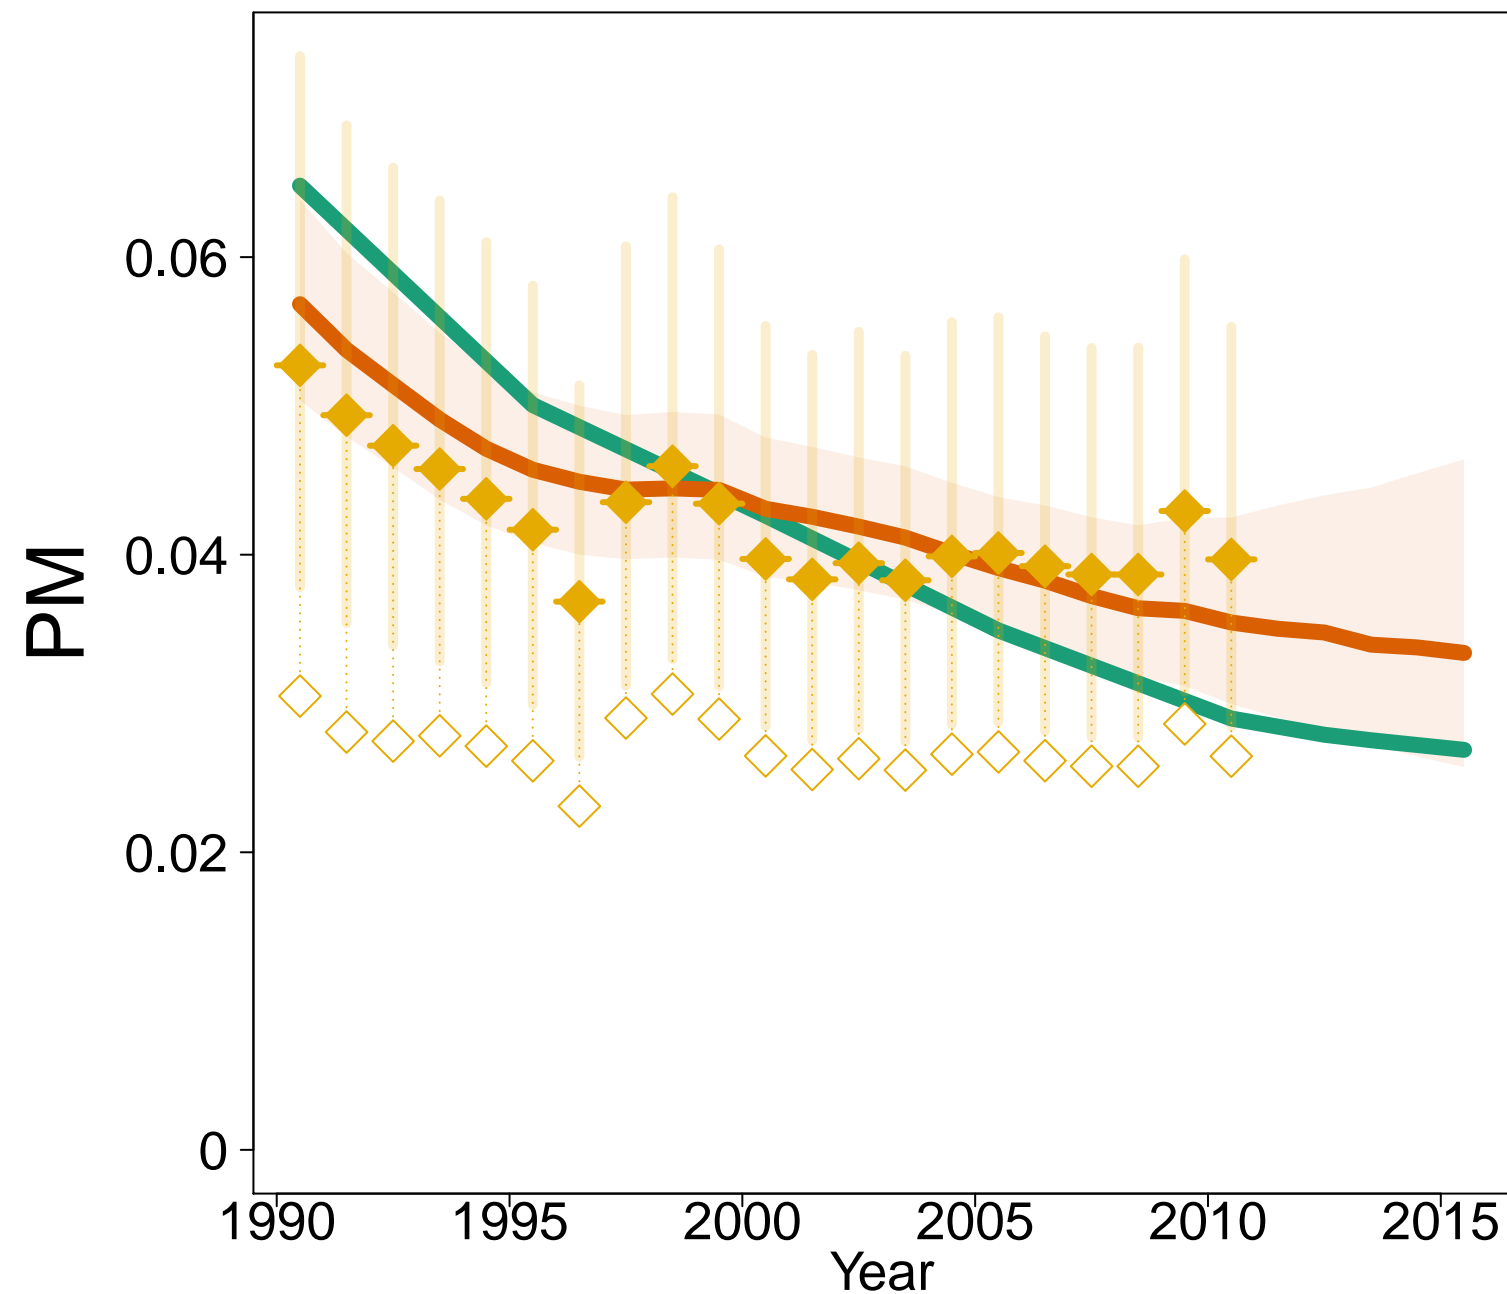

Brazil [BRA; B]  
(South America)

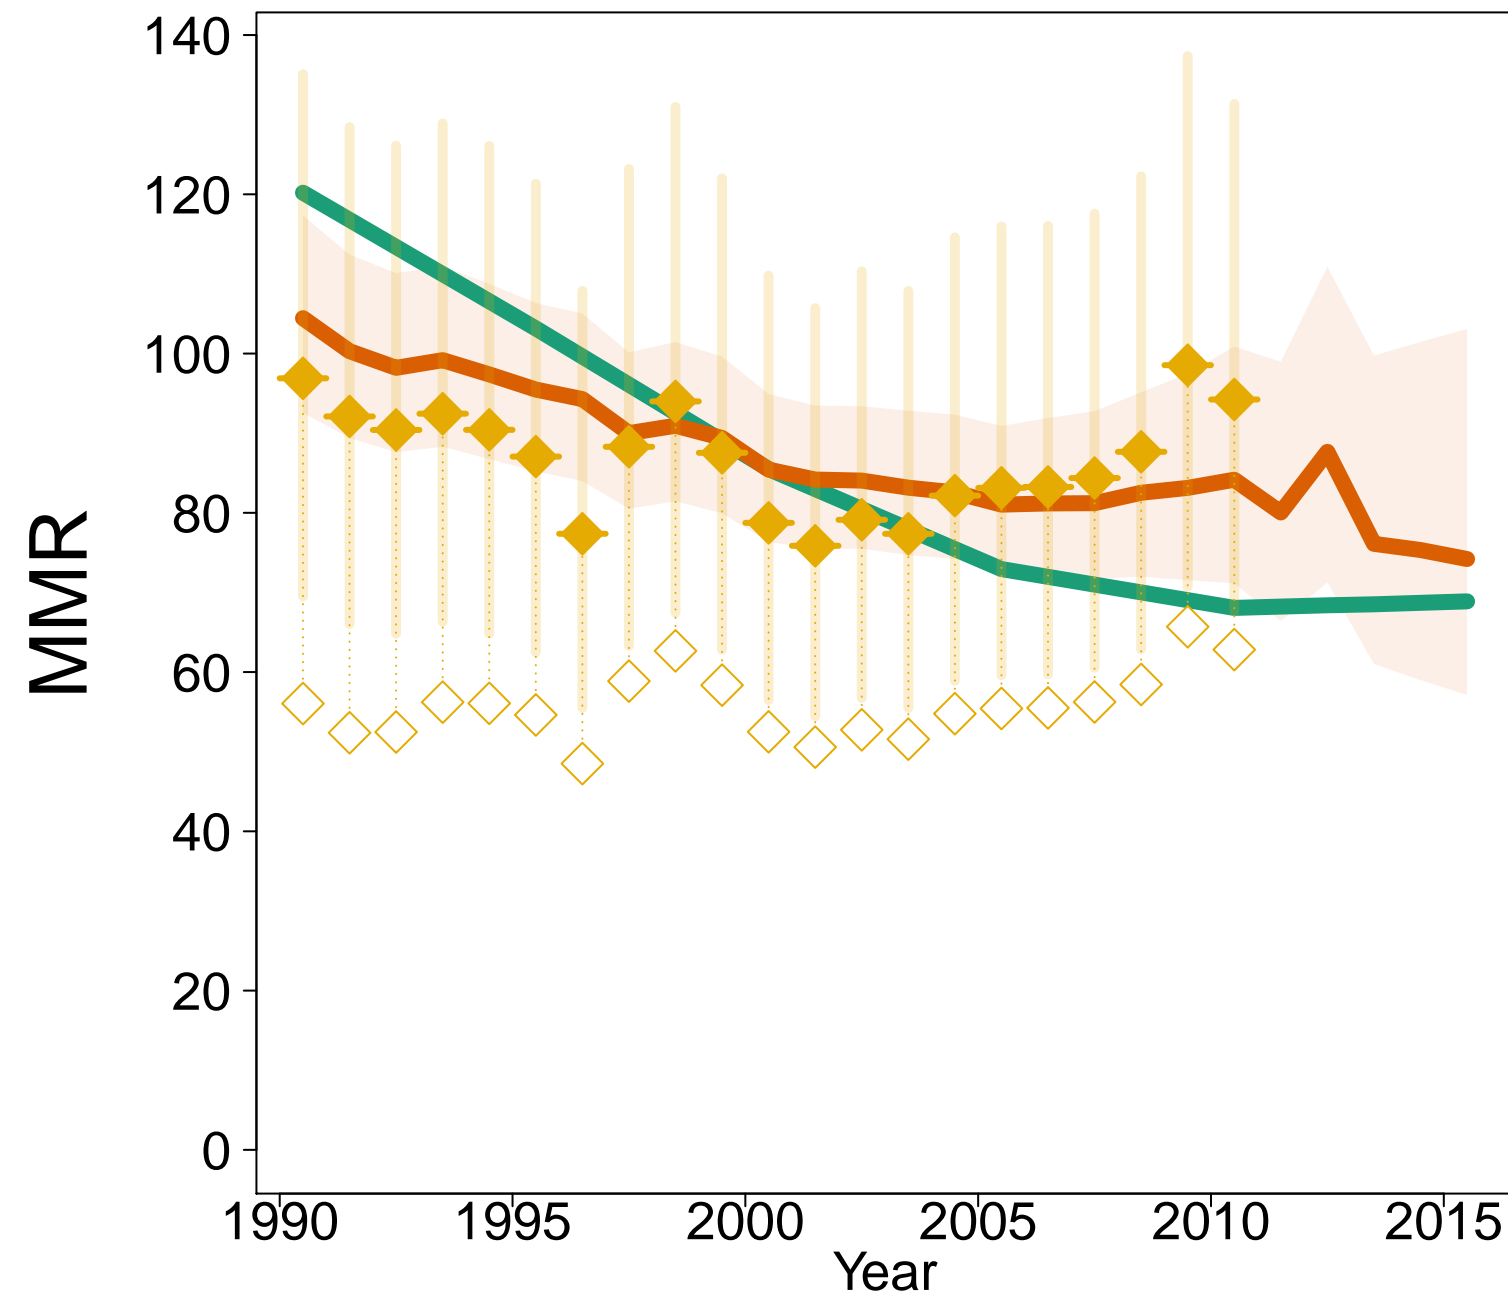

- Estimates –
- Bmat 2014
- MMEIG 2014
- Data –
- Observed Data
- Adjusted Data
- Data type –
- VR

Brunei Darussalam [BRN; B]  
(South-Eastern Asia / Oceania)

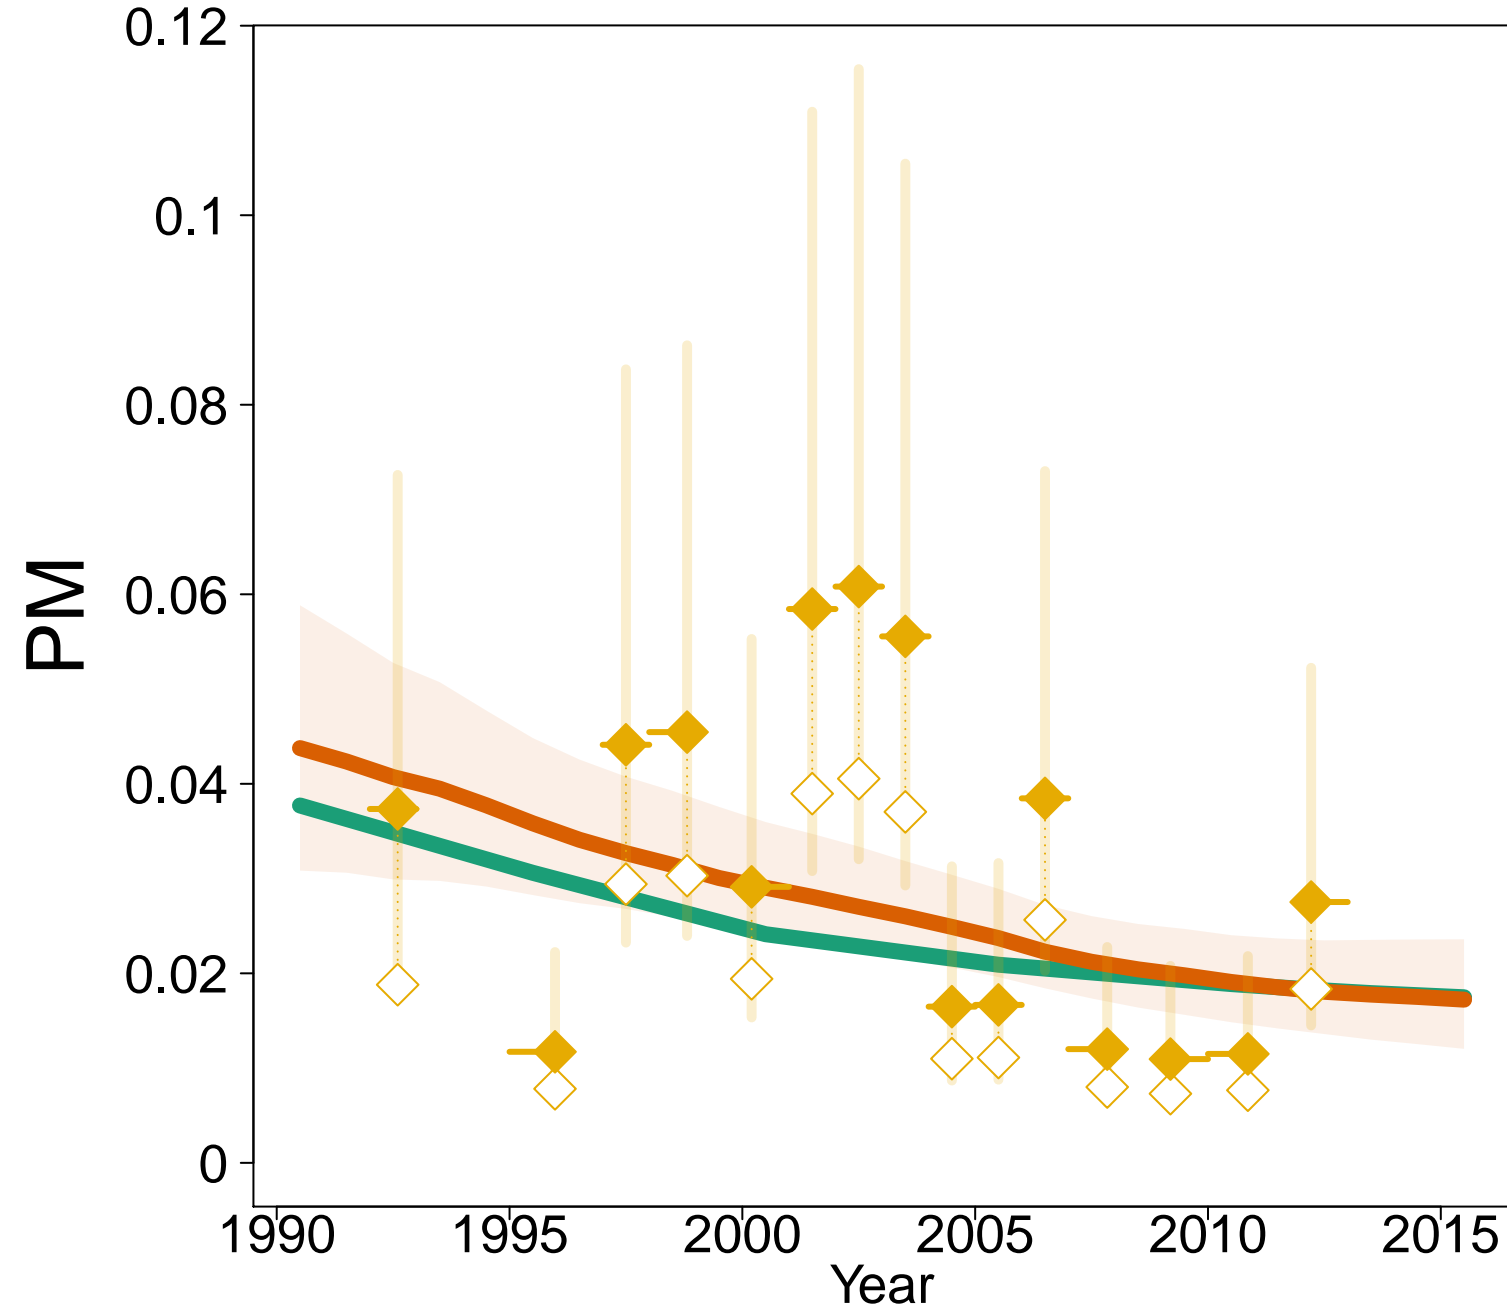

Brunei Darussalam [BRN; B]  
(South-Eastern Asia / Oceania)

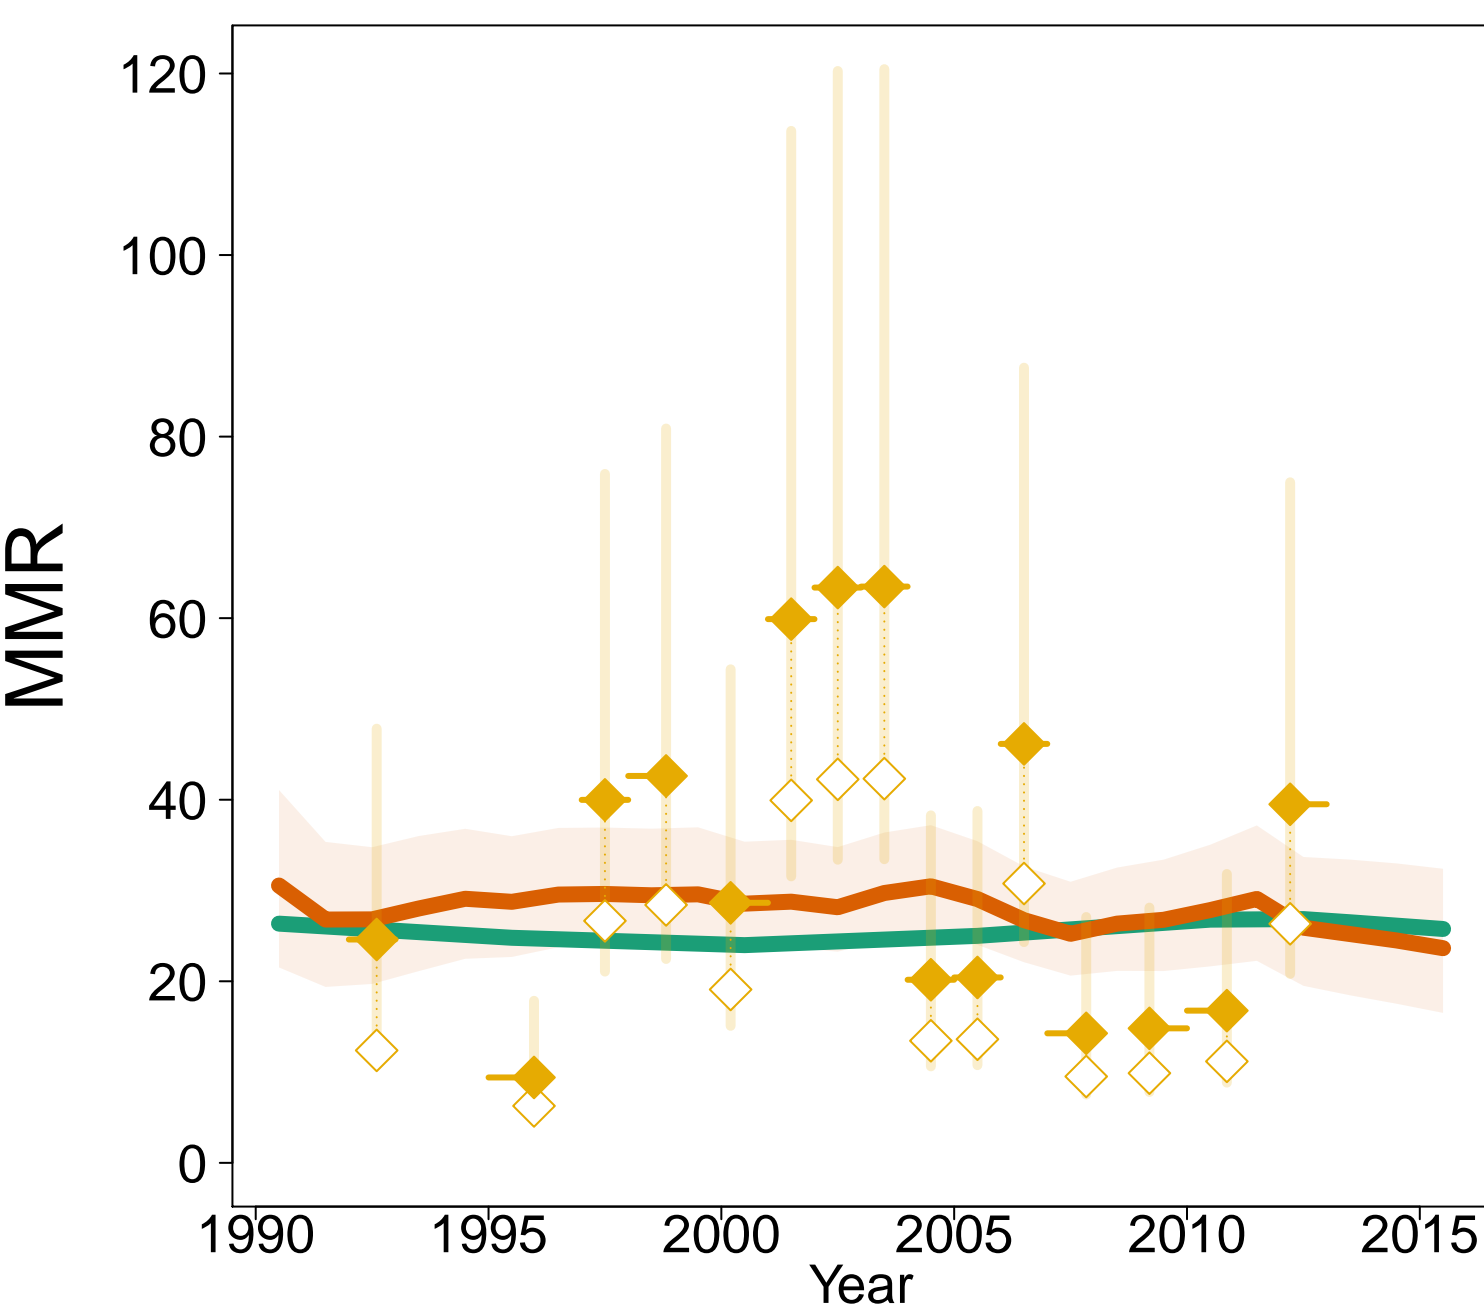

Bulgaria [BGR; A]  
(Developed regions)

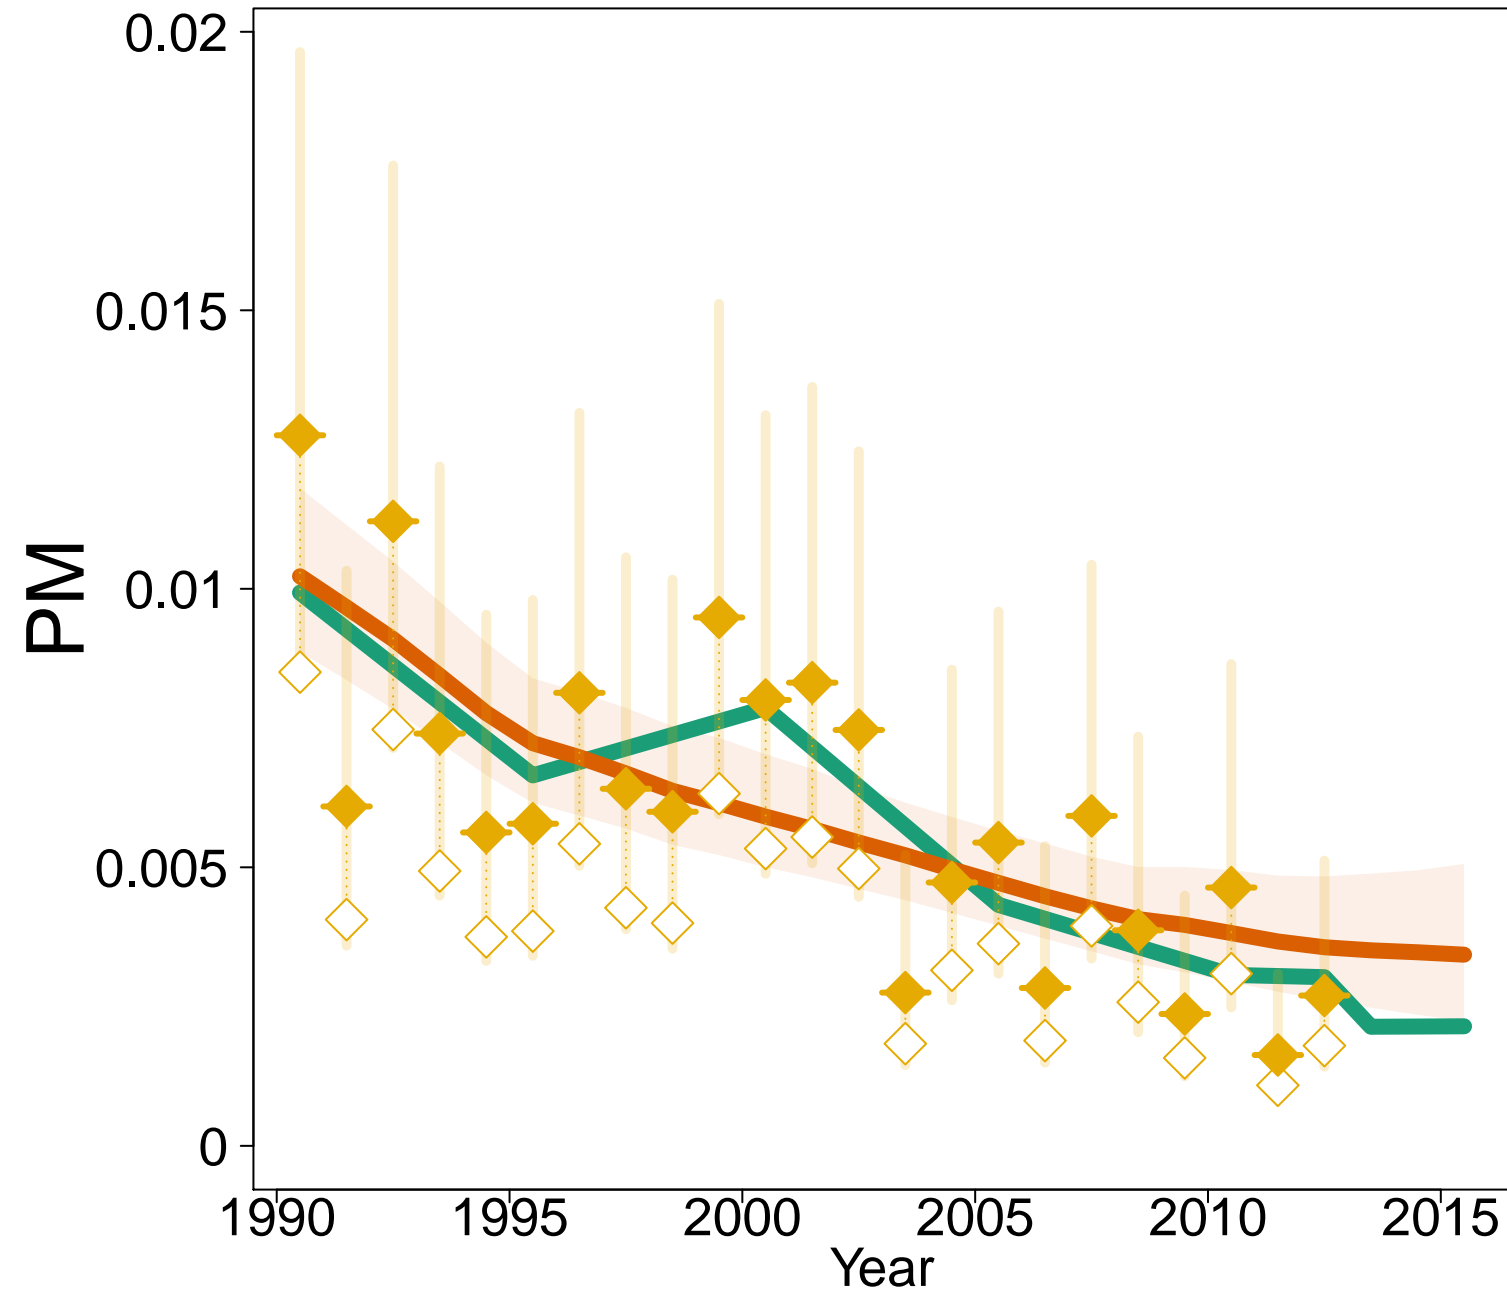

Bulgaria [BGR; A]  
(Developed regions)

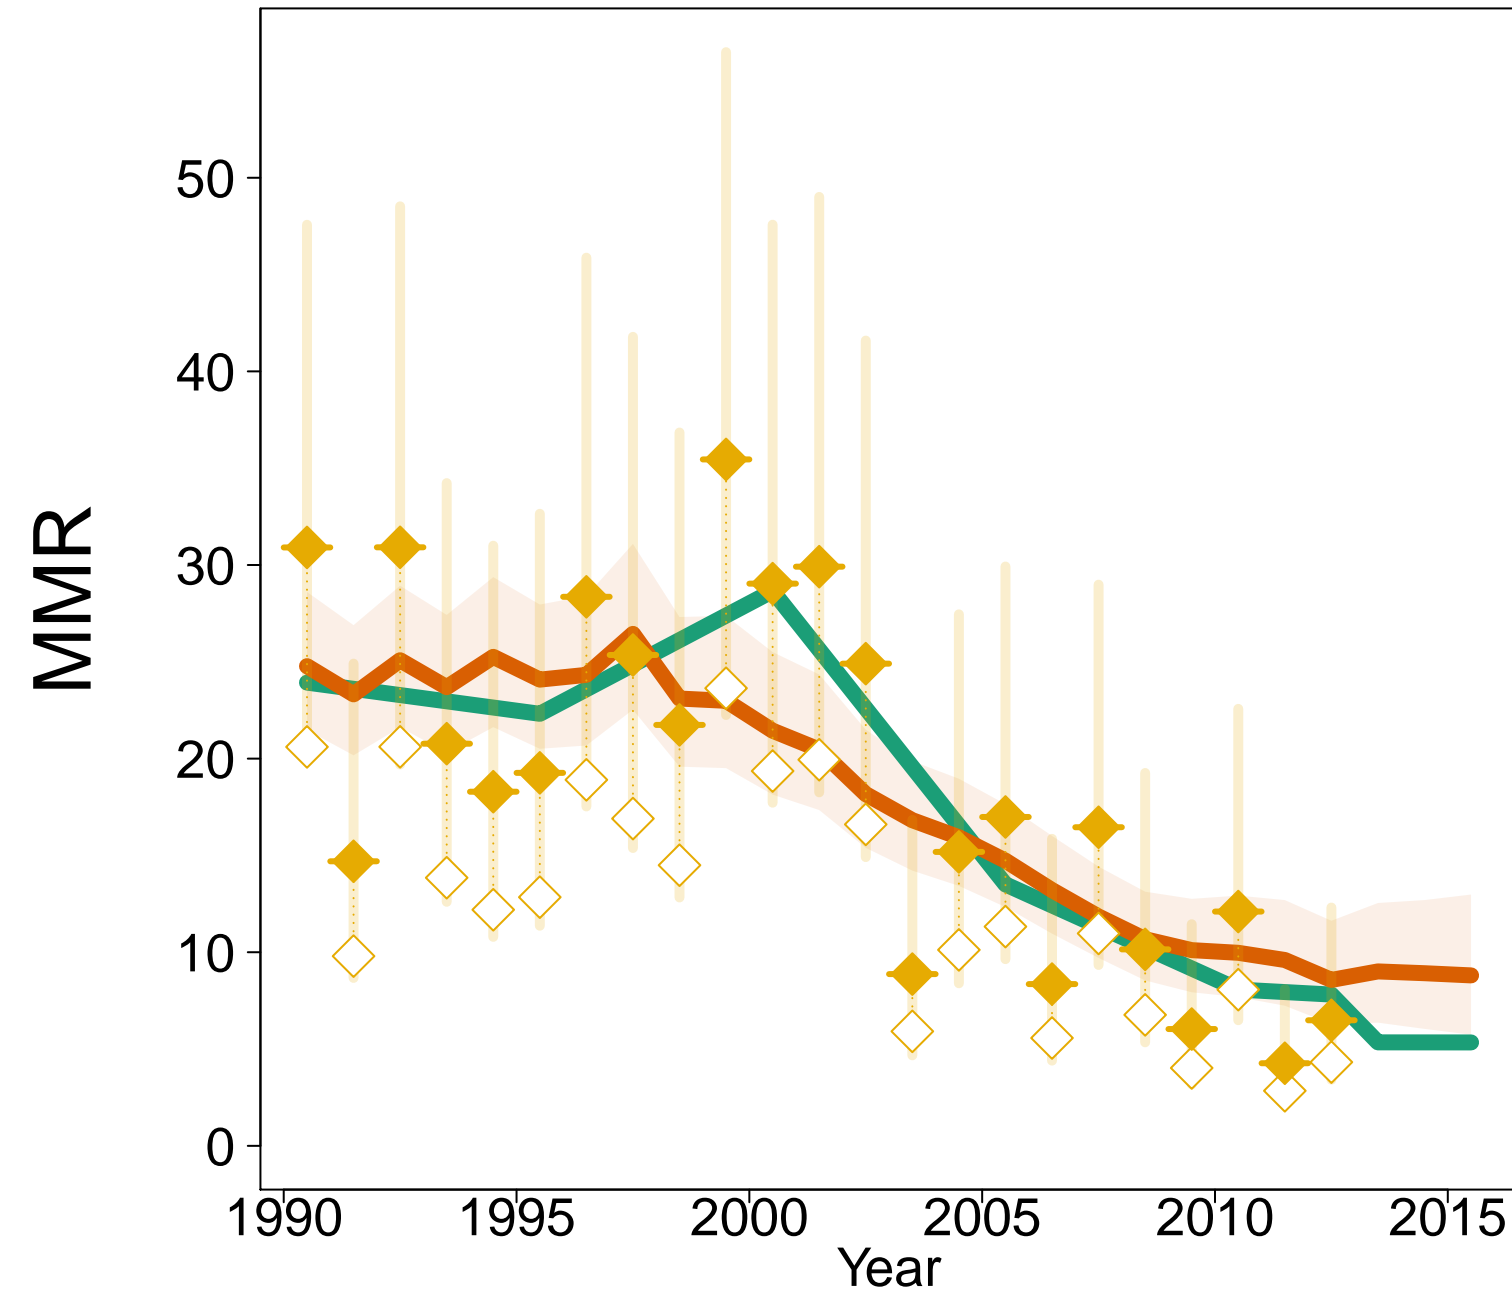

- Estimates –
- Bmat 2014
- MMEIG 2014
- Data –
- Observed Data
- Adjusted Data
- Data type –
- VR



Burkina Faso [BFA; B]  
(Western Africa)

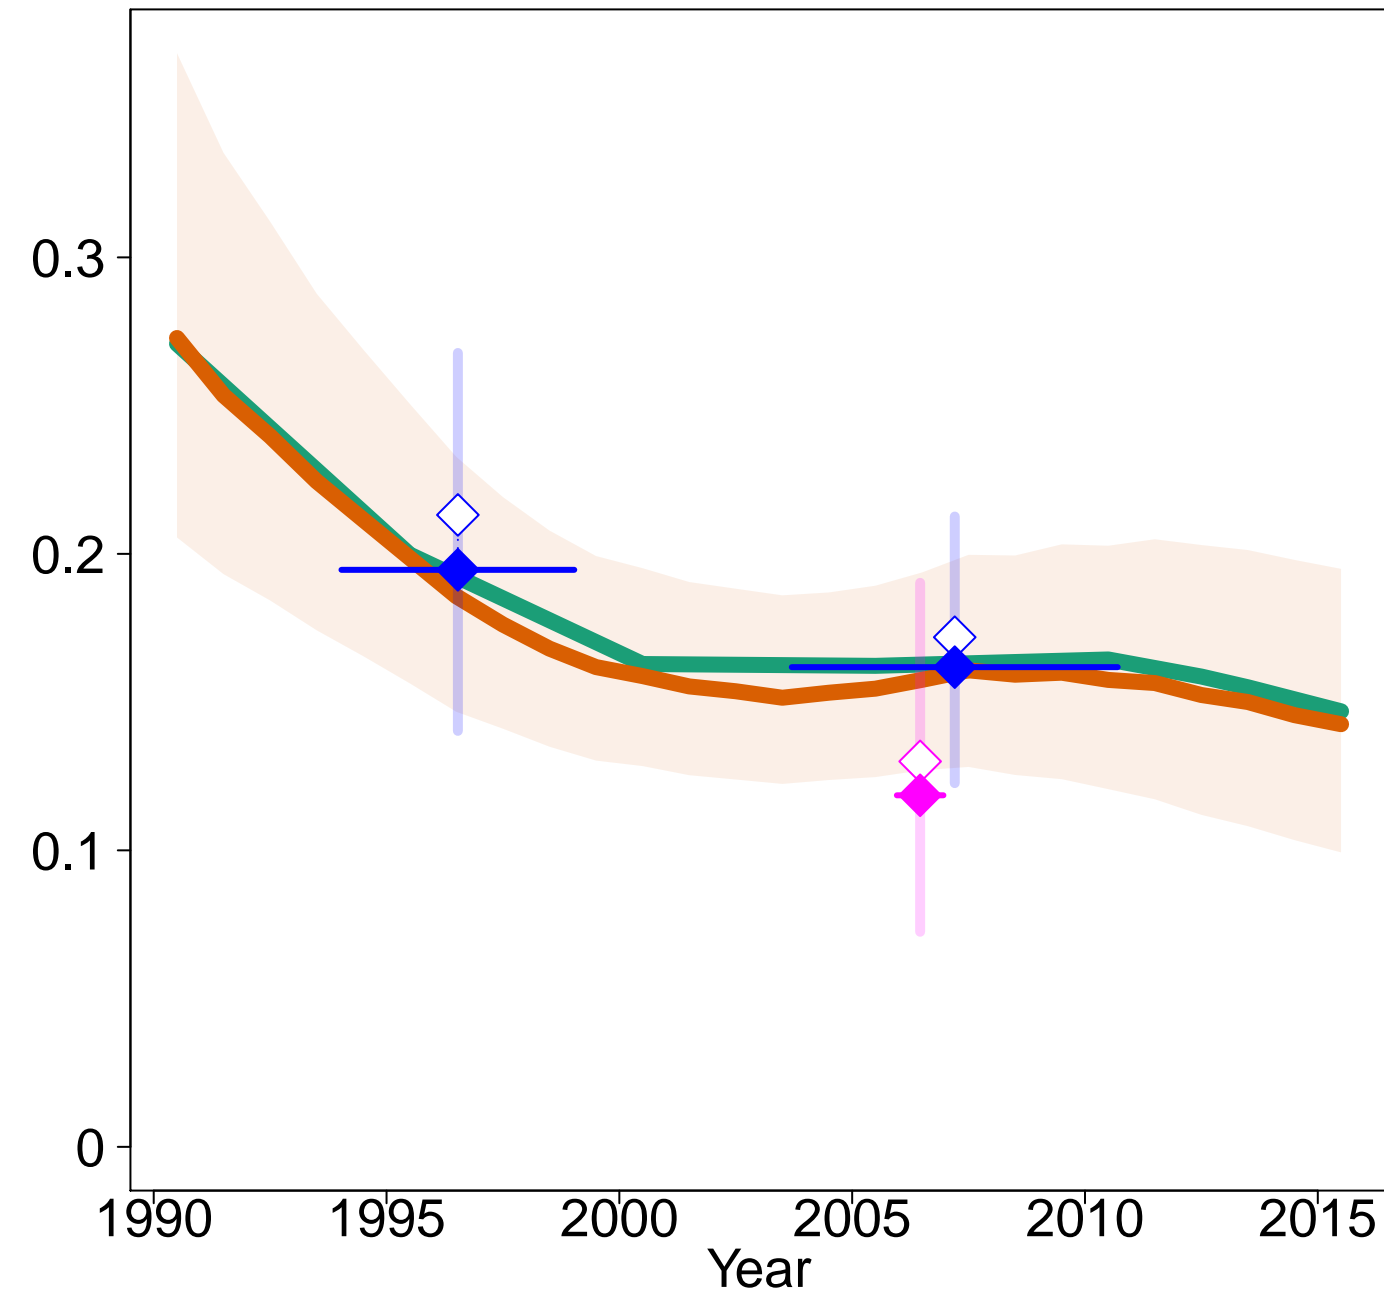

Burkina Faso [BFA; B]  
(Western Africa)

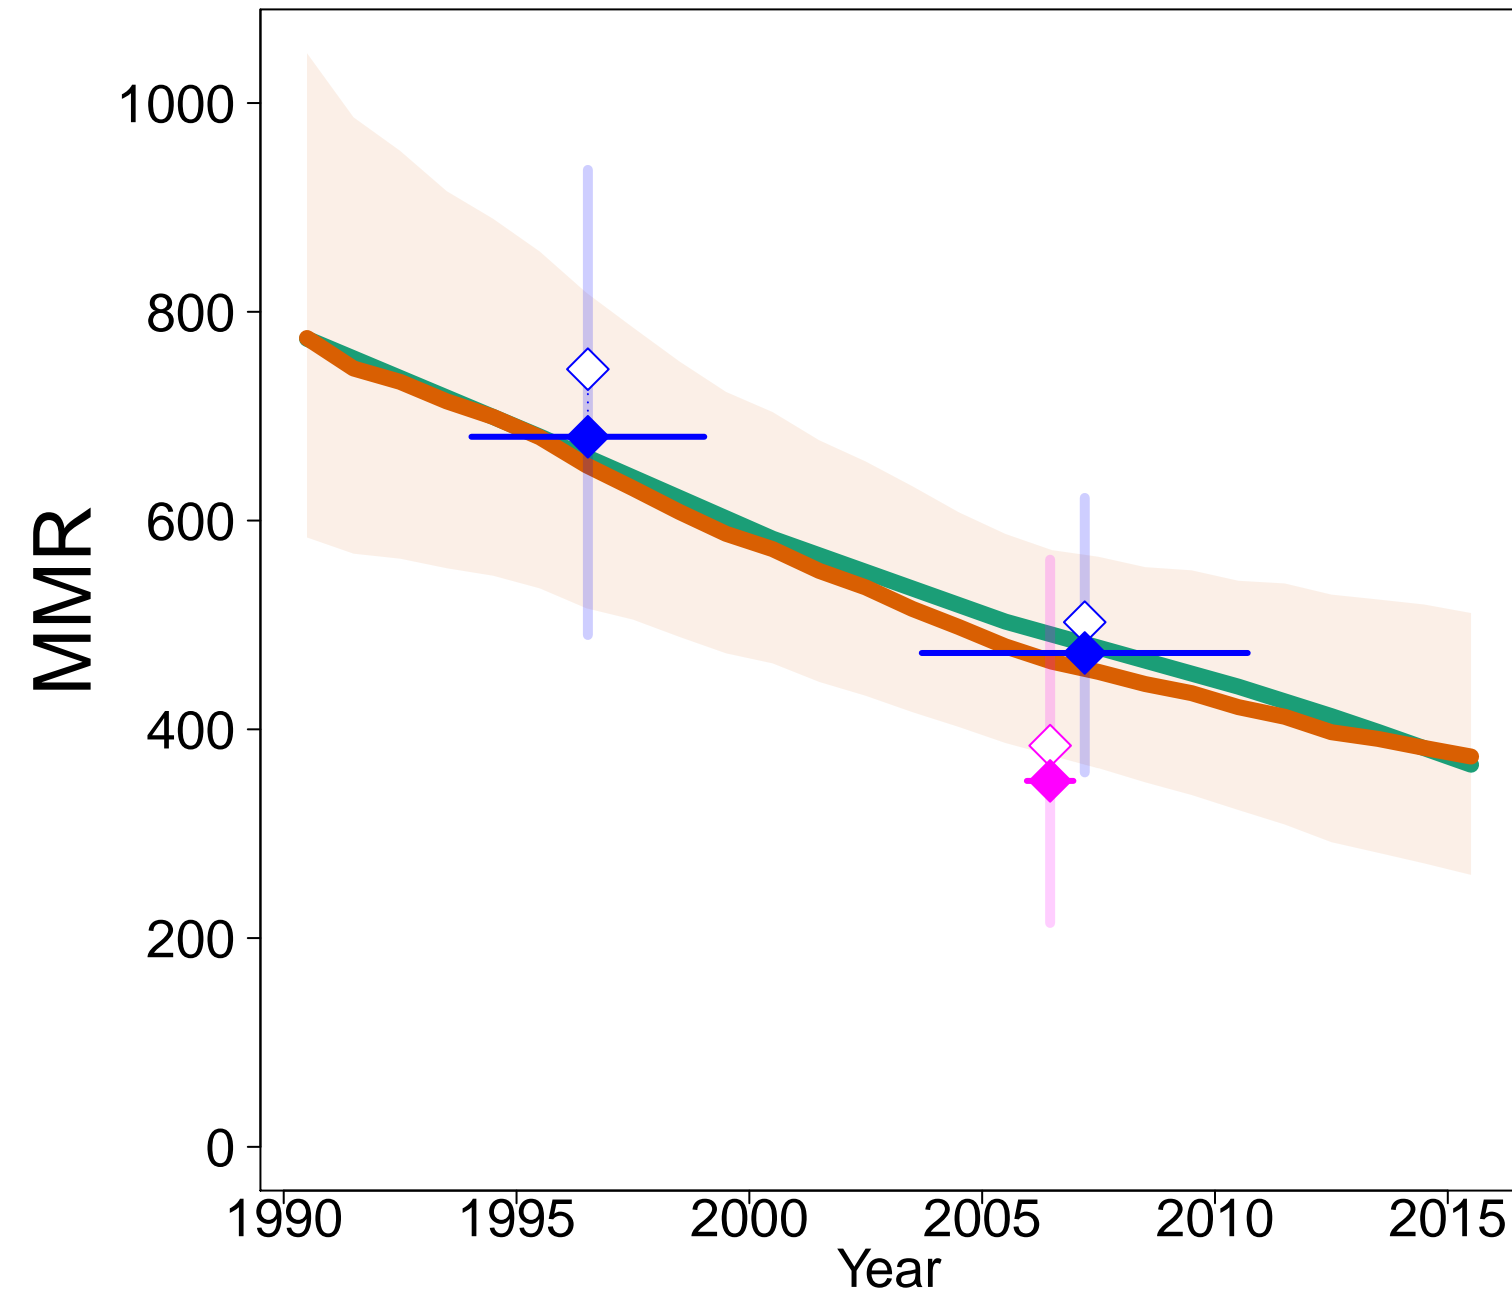

- Estimates –
- Bmat 2014
- MMEIG 2014
- Data –
- Observed Data
- Adjusted Data
- Data type –
- DHS
- Census

Burundi [BDI; B]  
(Eastern Africa)

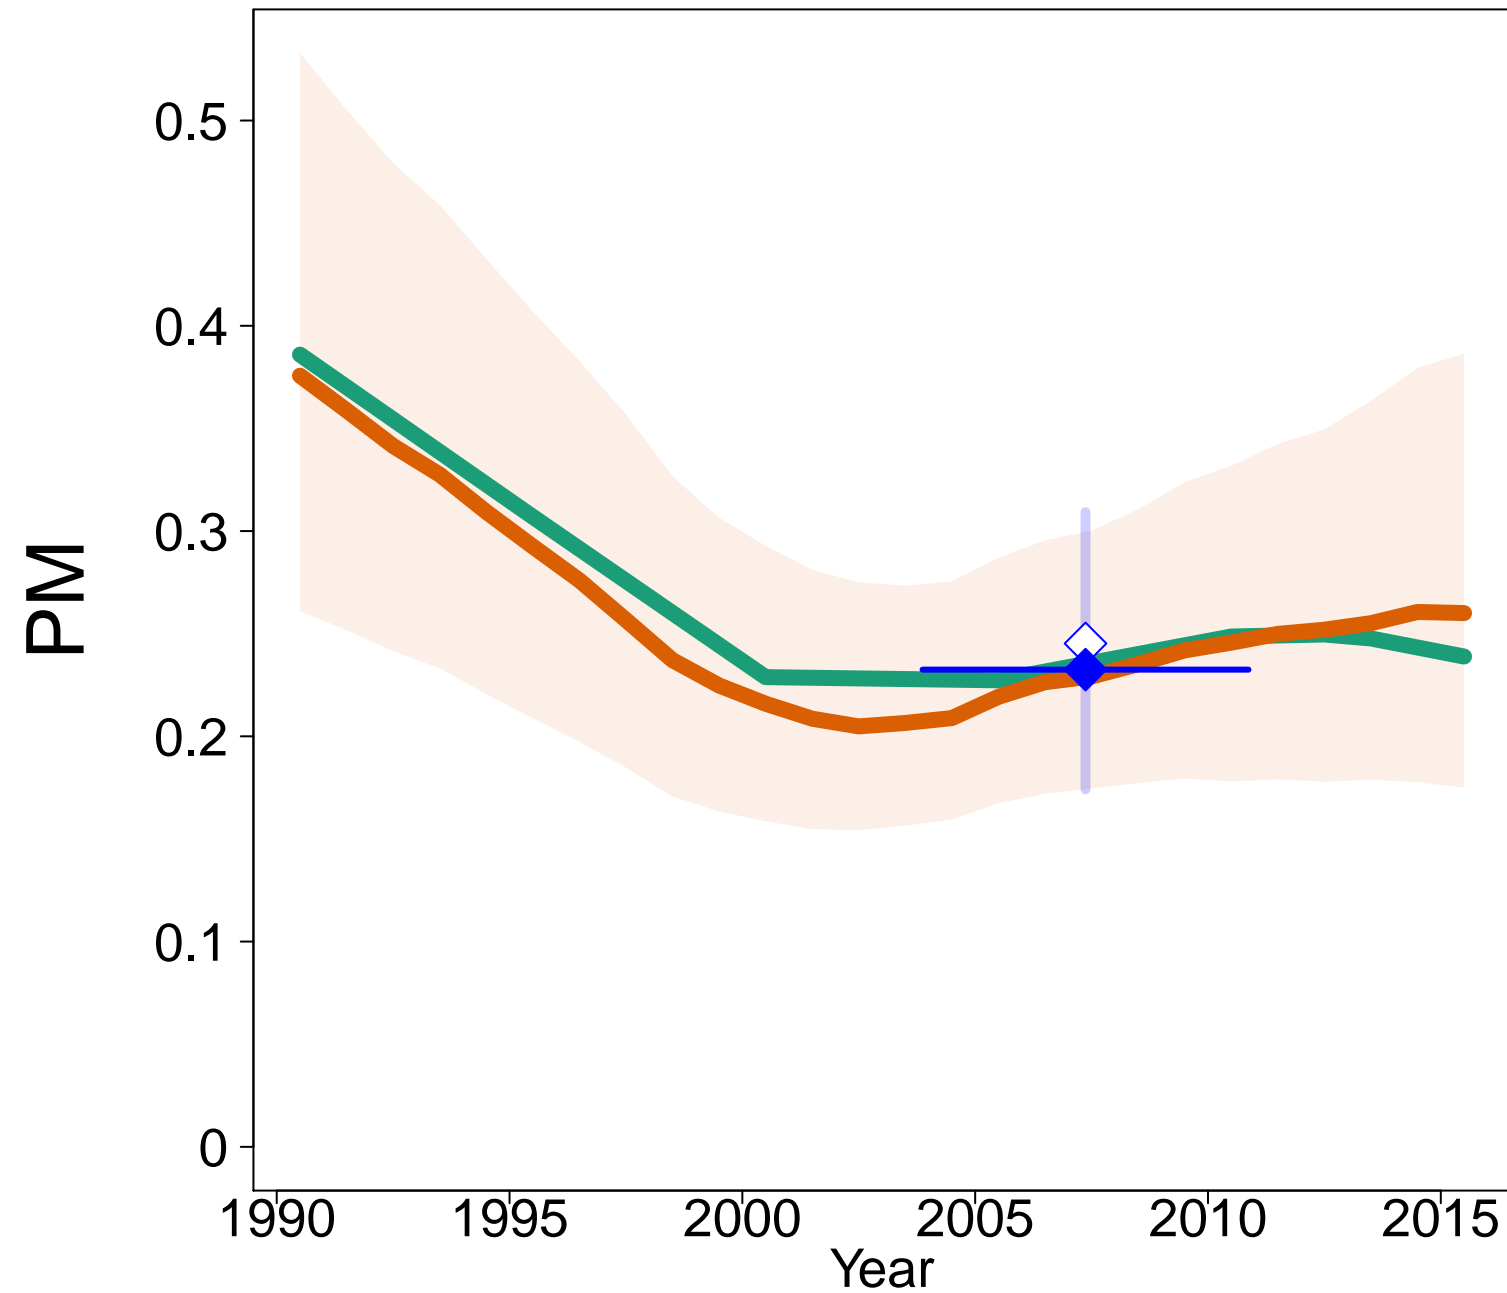

Burundi [BDI; B]  
(Eastern Africa)

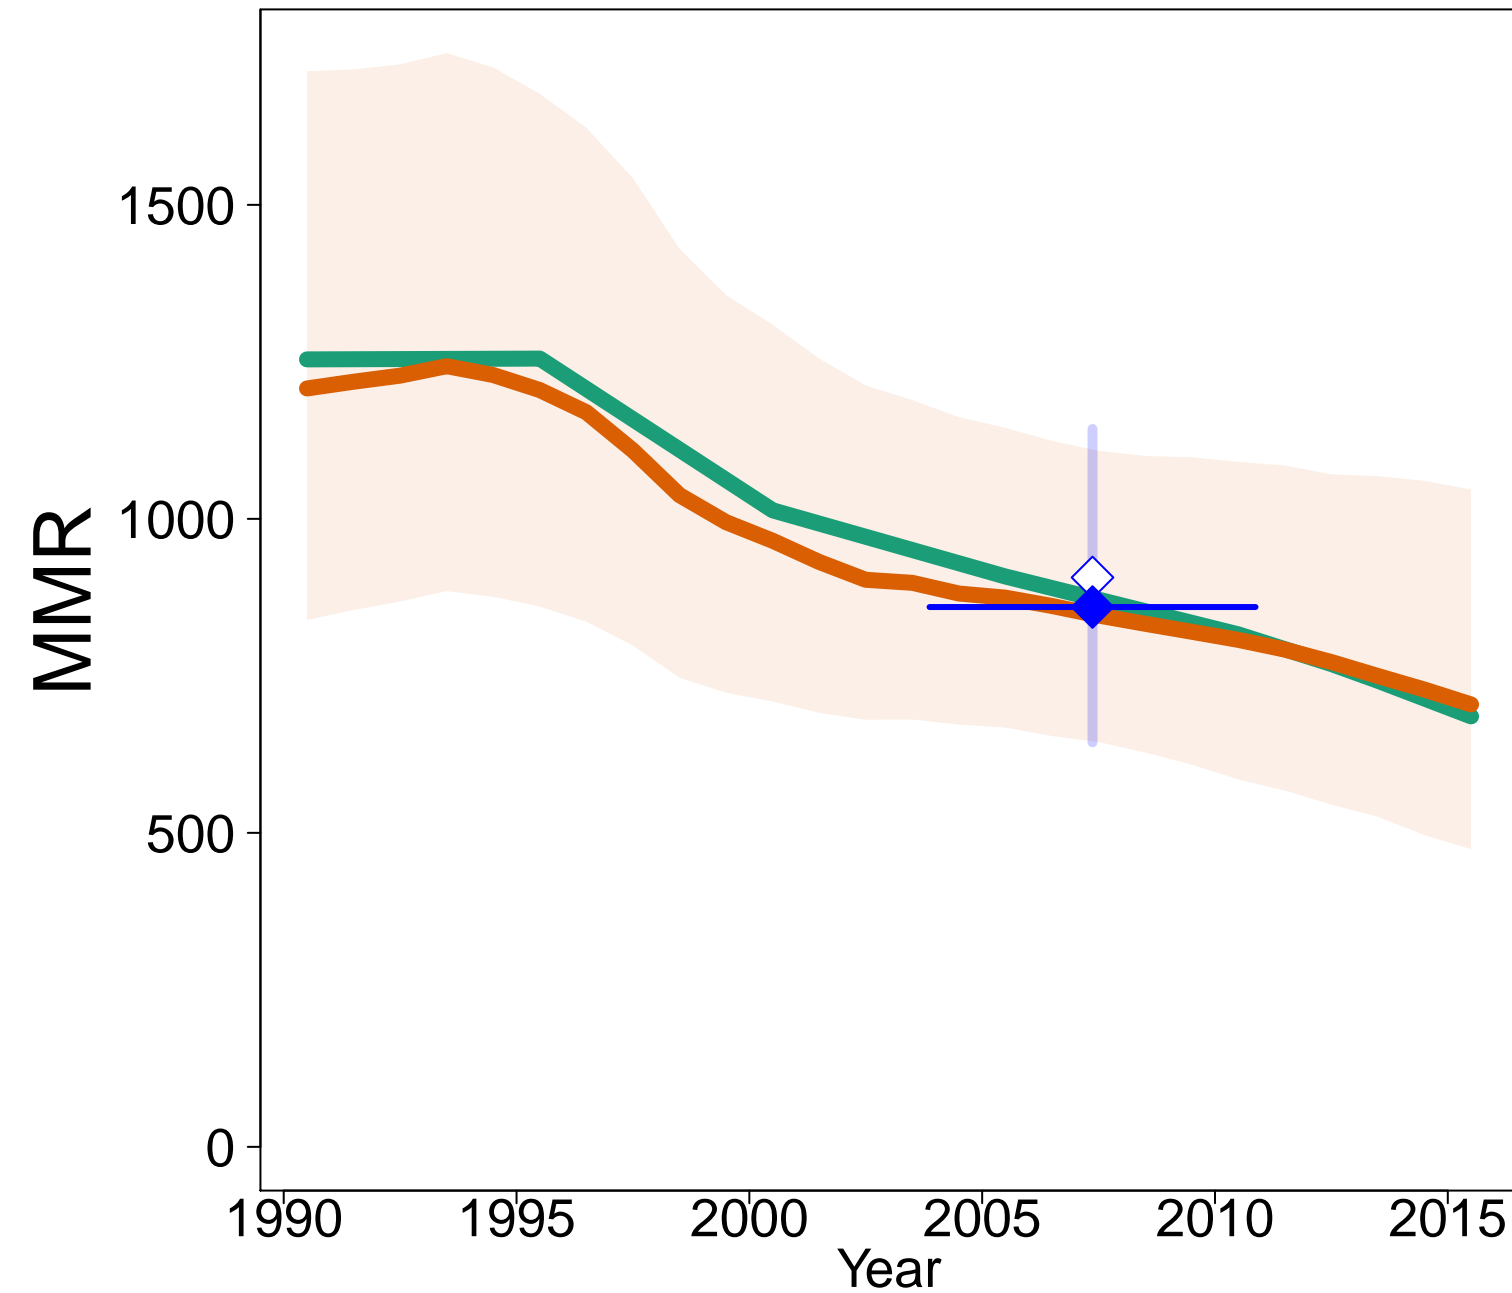

- Estimates –
- Bmat 2014
- MMEIG 2014
- Data –
- Observed Data
- Adjusted Data
- Data type –
- DHS

Cabo Verde [CPV; C]  
(Western Africa)

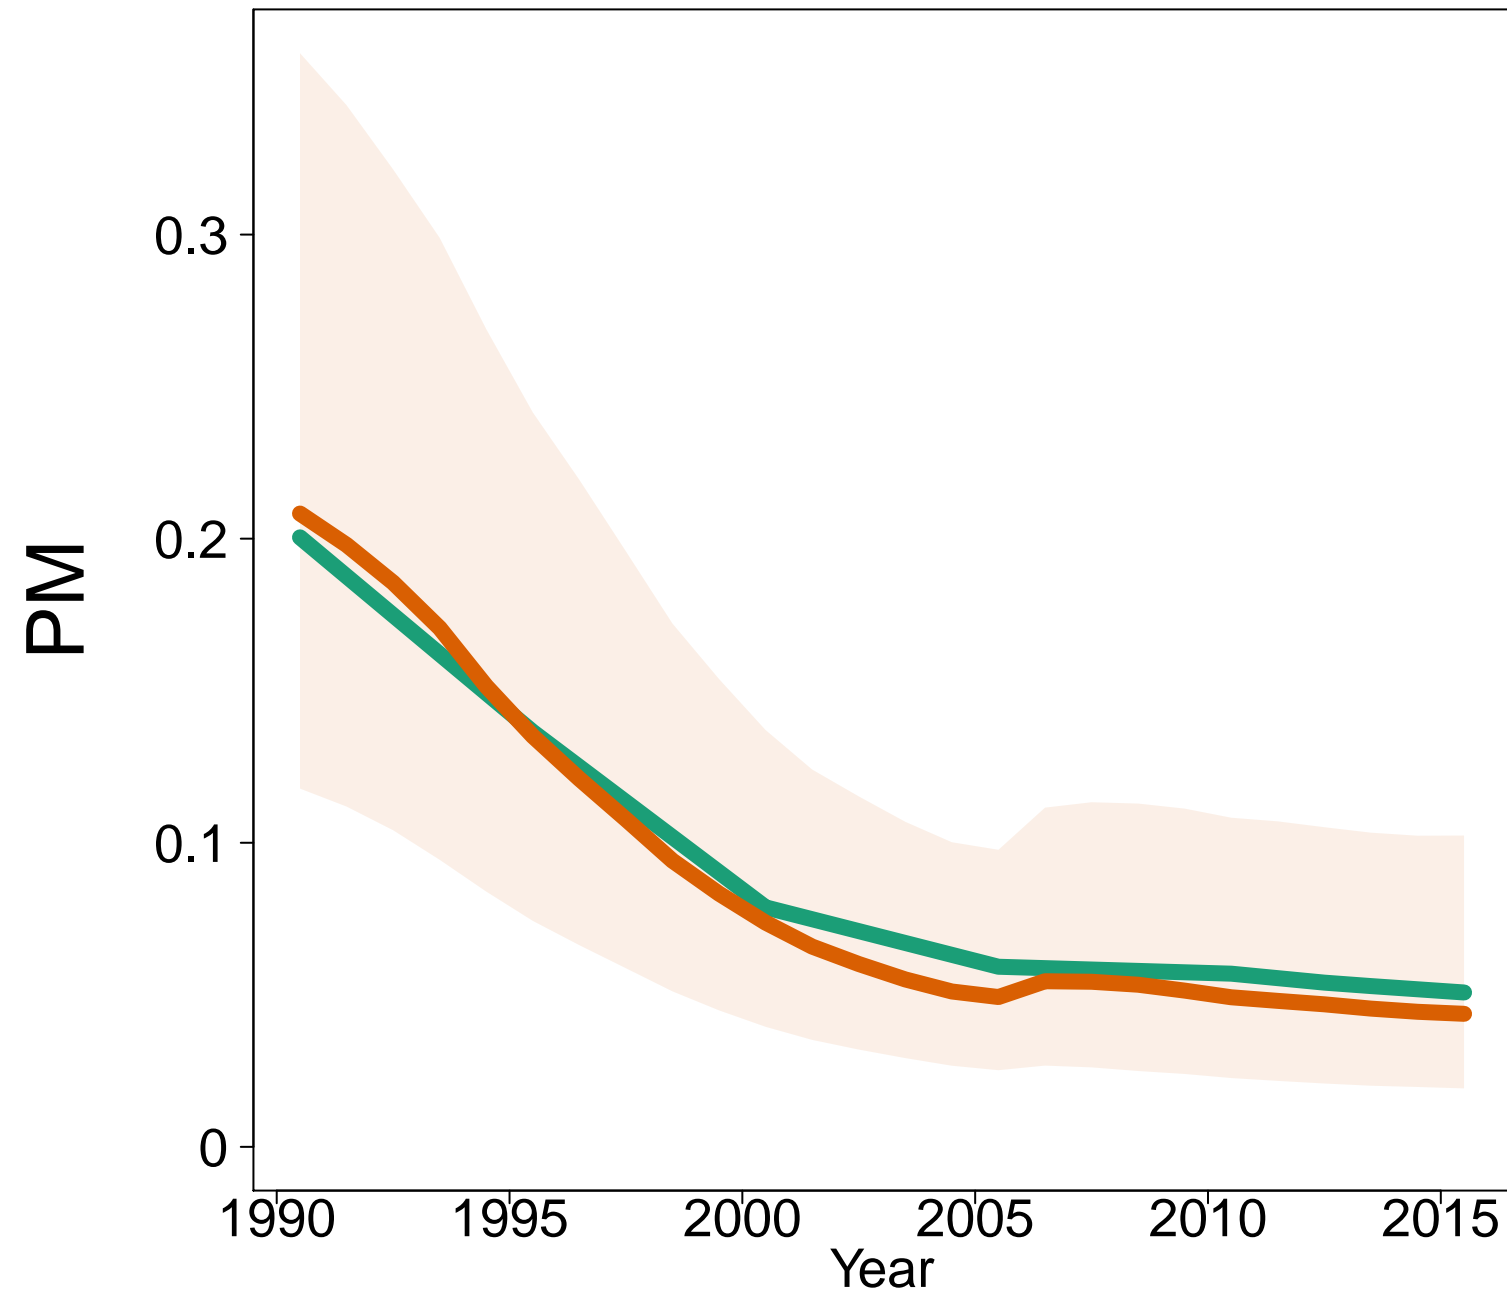

Cabo Verde [CPV; C]  
(Western Africa)

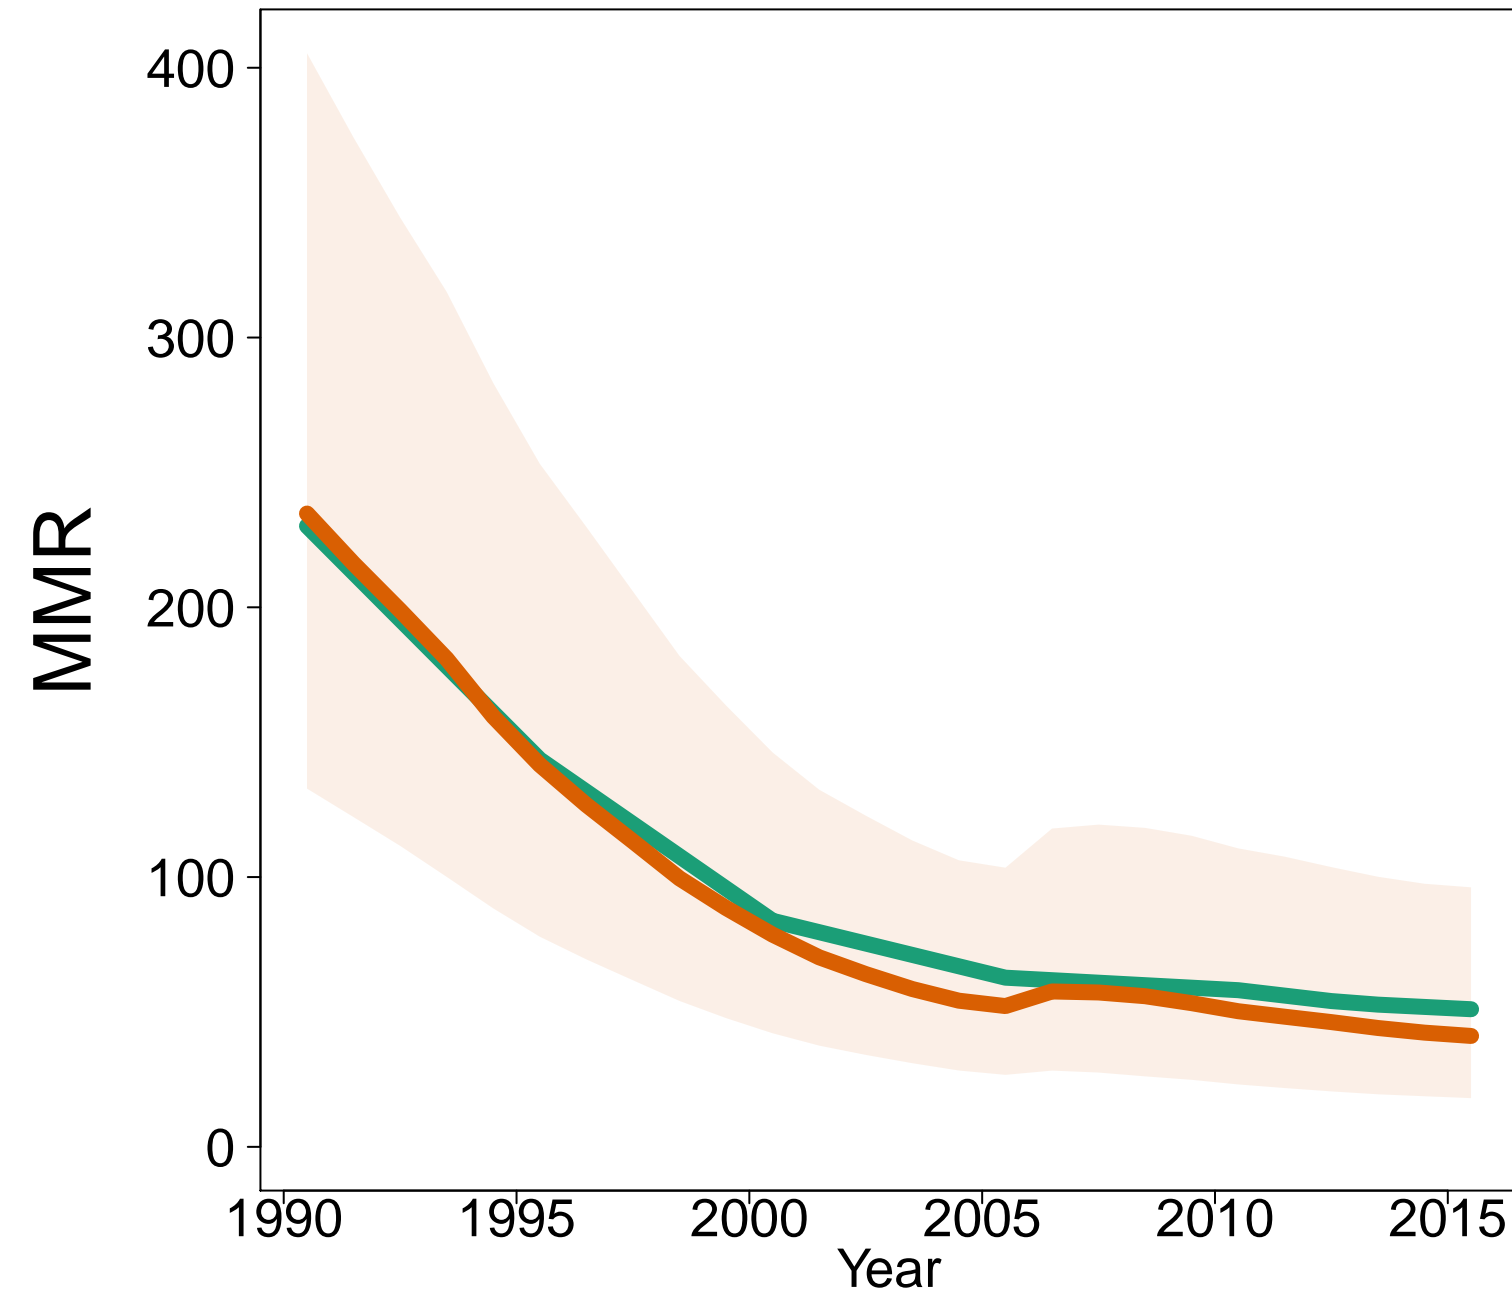

Cambodia [KHM; B]  
(South-Eastern Asia / Oceania)

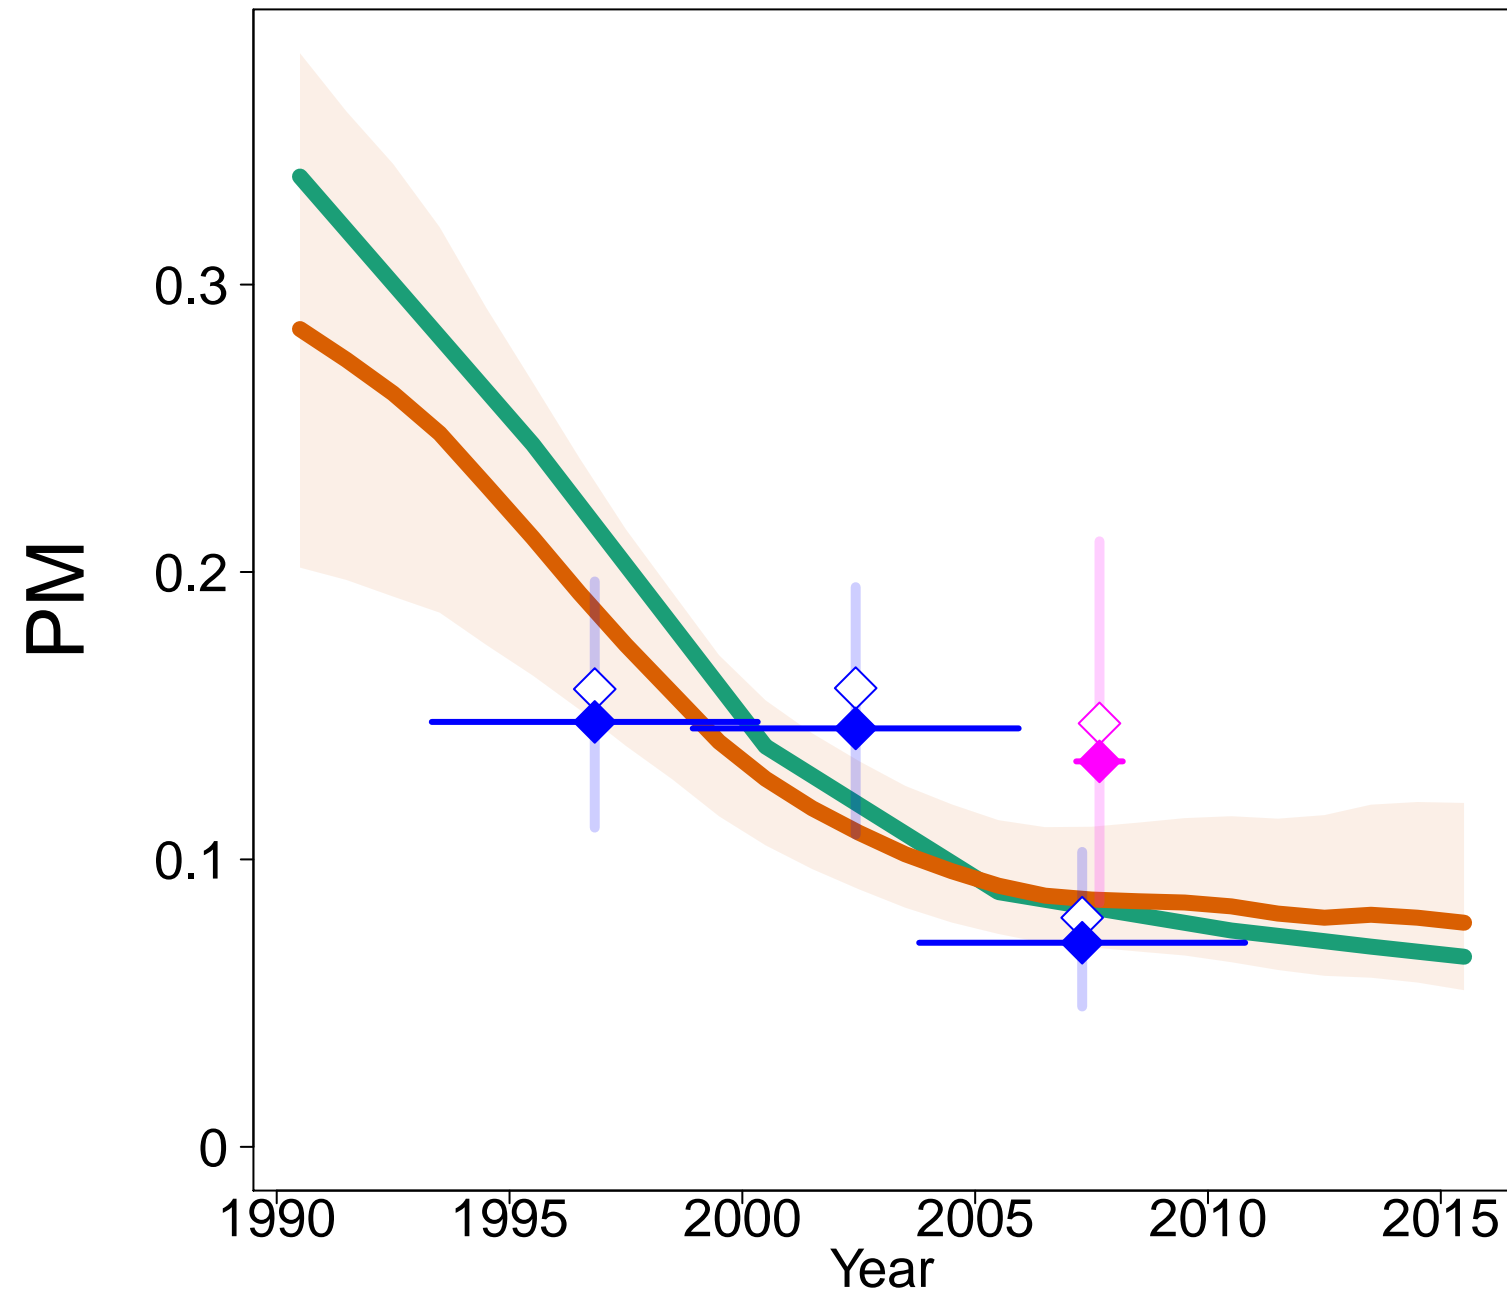

Cambodia [KHM; B]  
(South-Eastern Asia / Oceania)

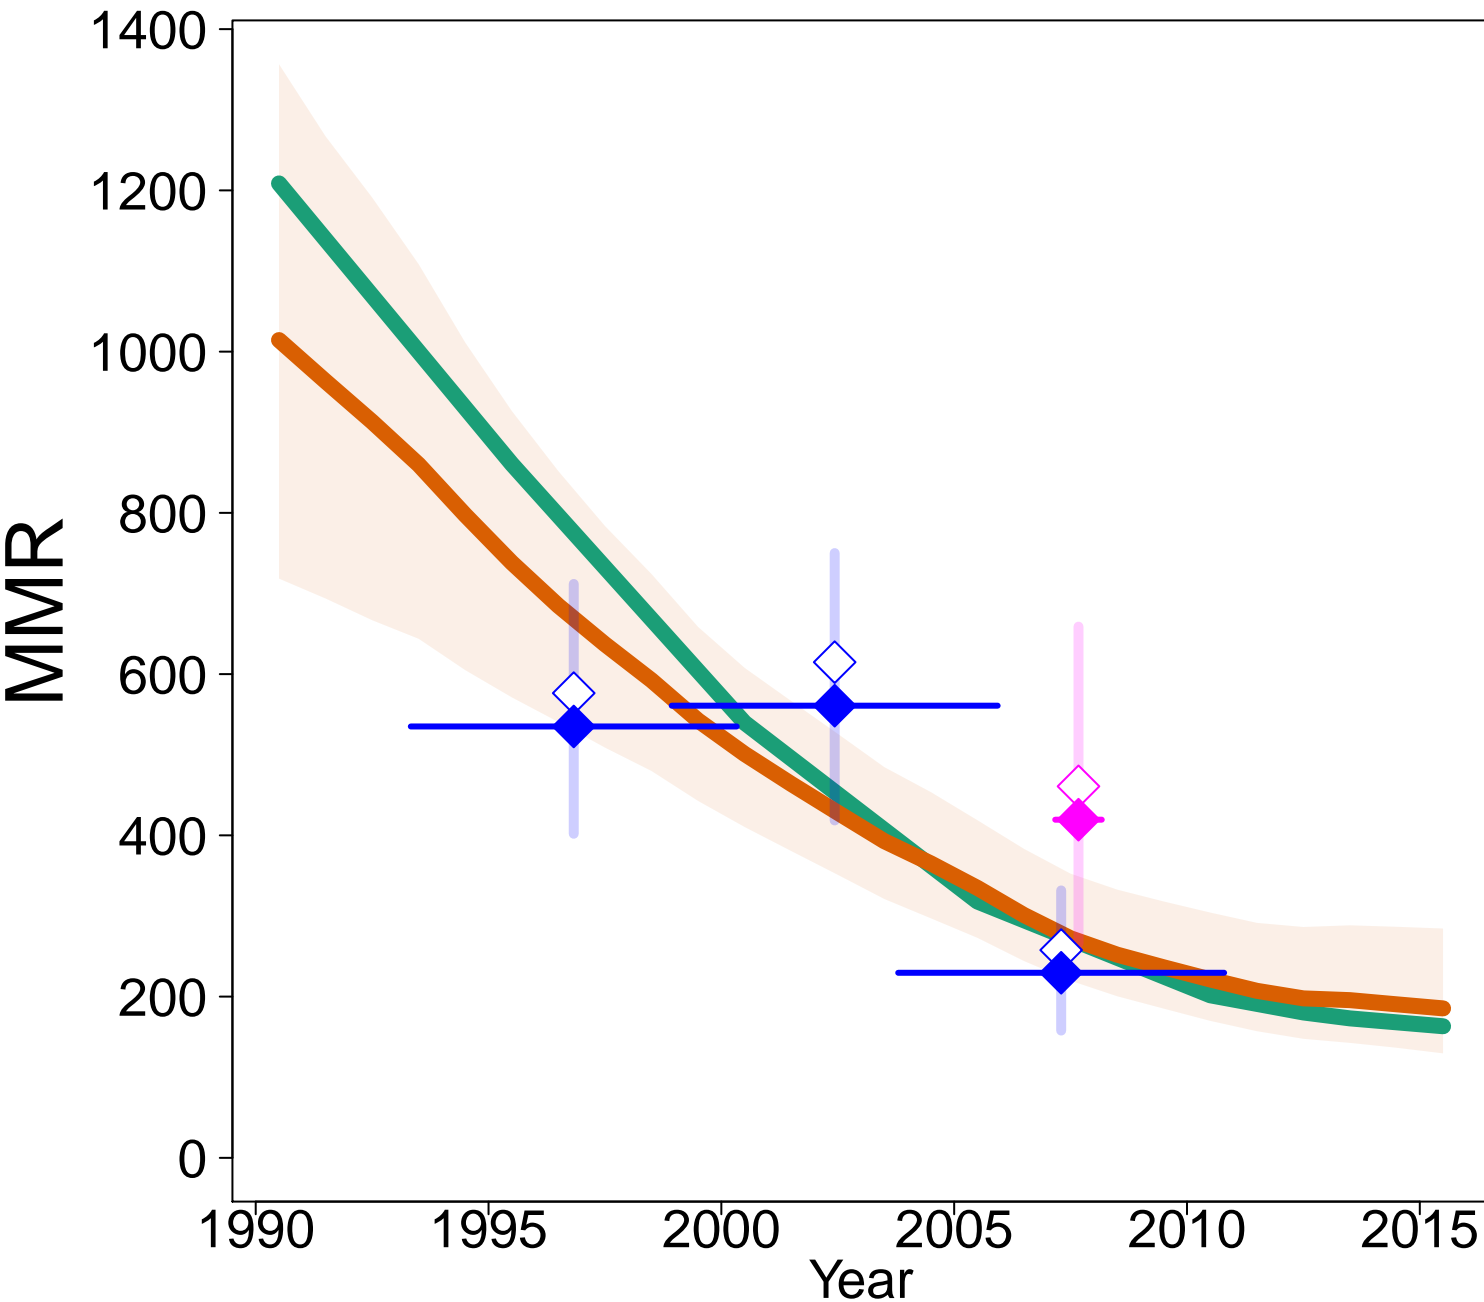

- Estimates –
- Bmat 2014
- MMEIG 2014
- Data –
- Observed Data
- Adjusted Data
- Data type –
- DHS
- Census

Cameroon [CMR; B]  
(Middle Africa)

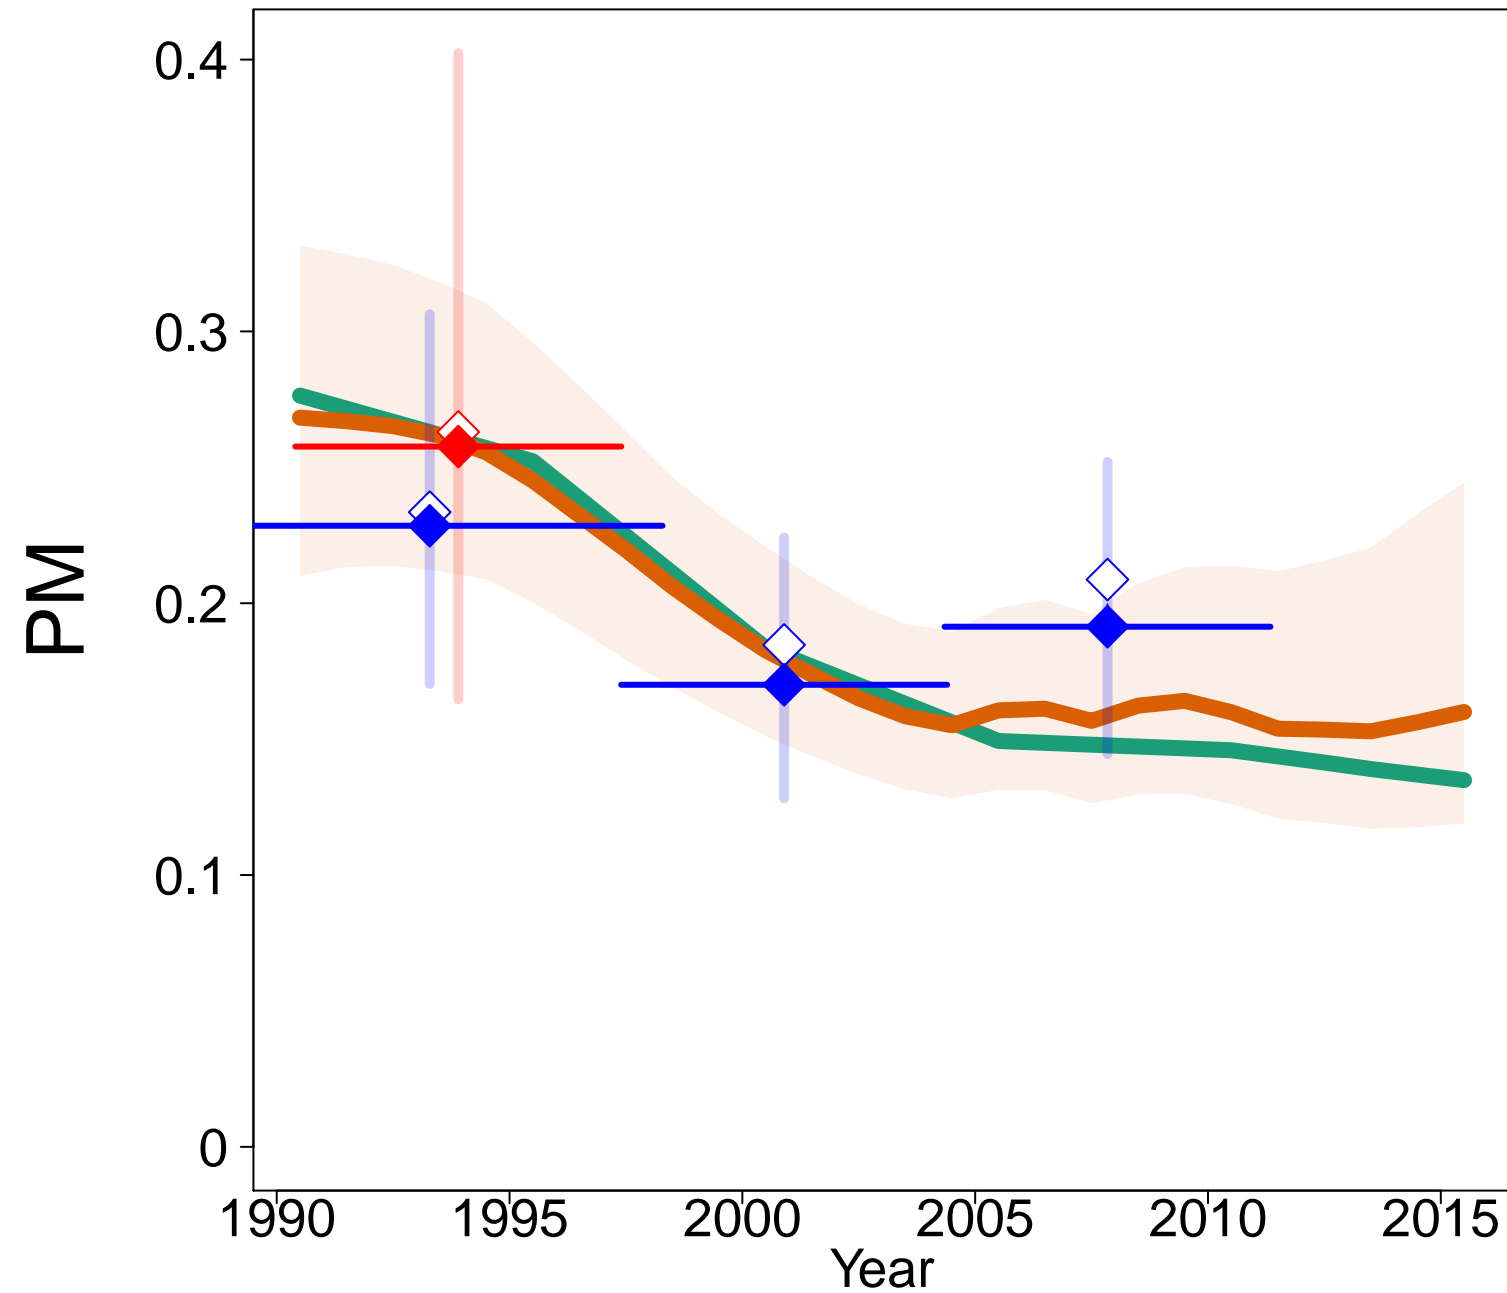

Cameroon [CMR; B]  
(Middle Africa)

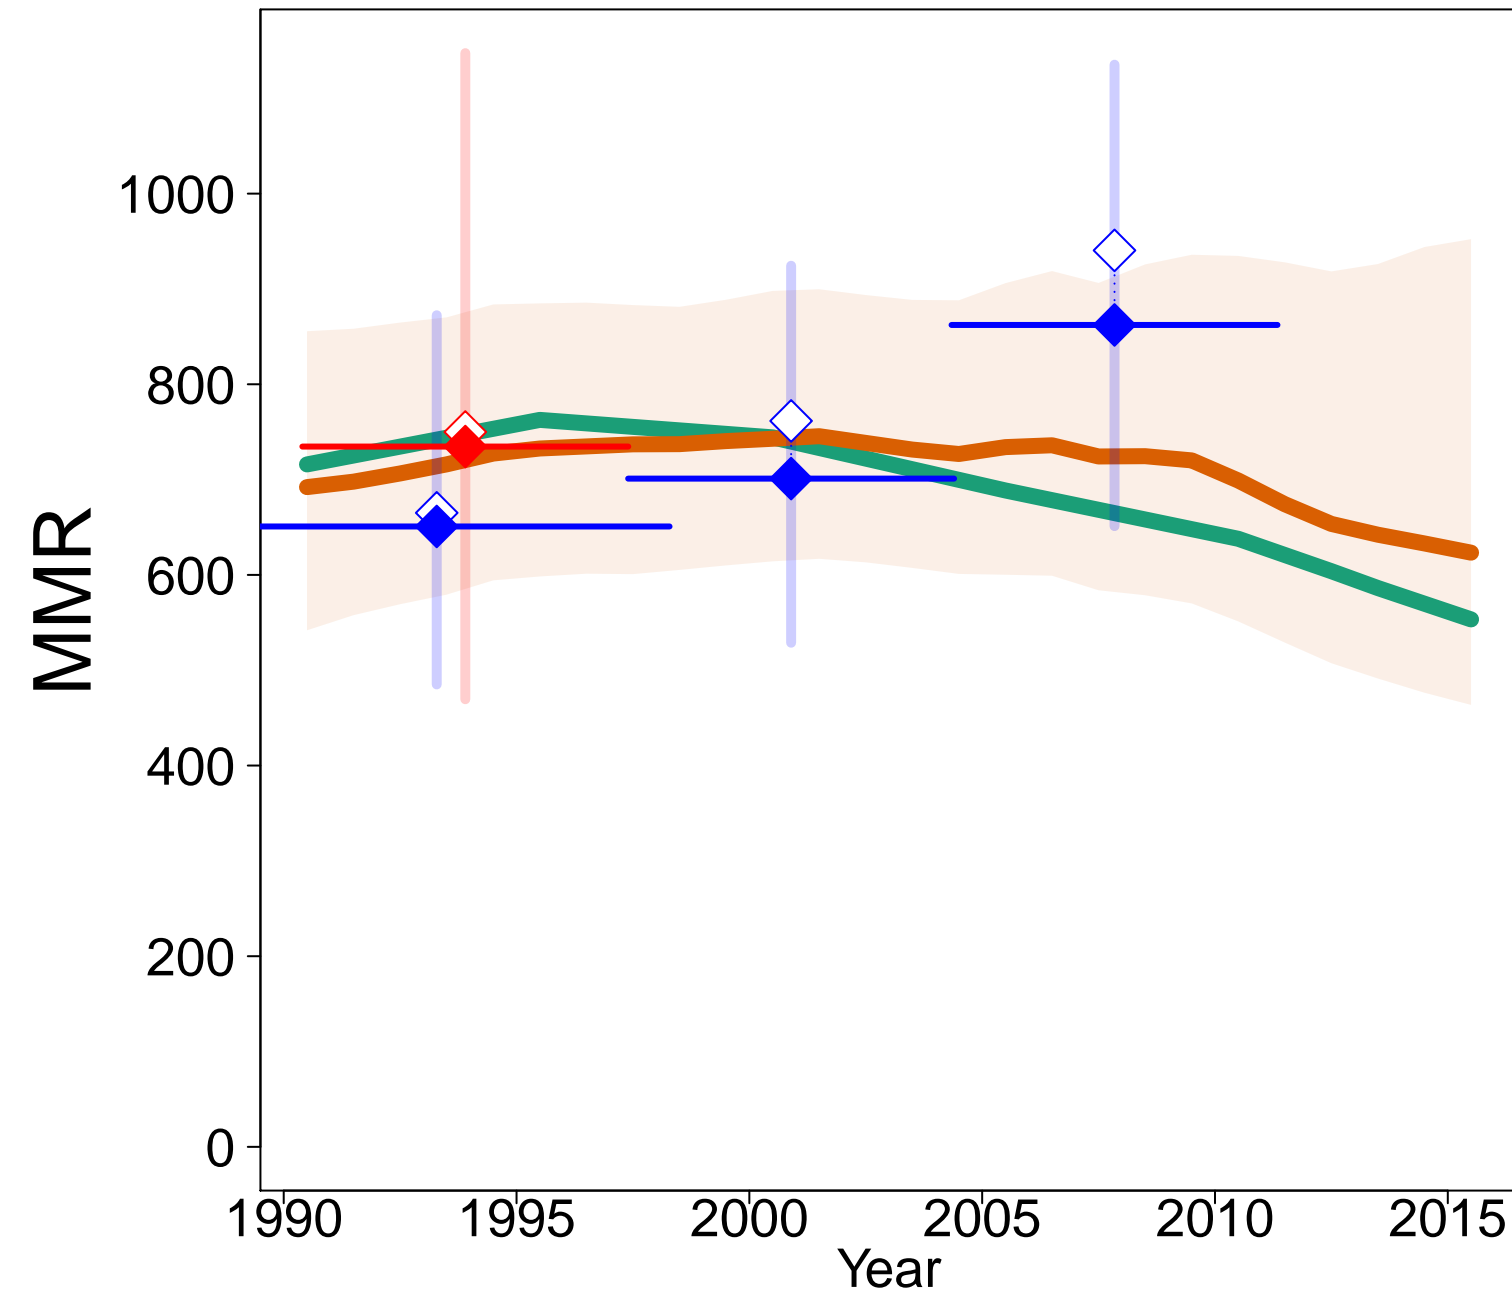

- Estimates –
- Bmat 2014
- MMEIG 2014
- Data –
- Observed Data
- Adjusted Data
- Data type –
- DHS
- Misc. studies

Canada [CAN; A]  
(Developed regions)

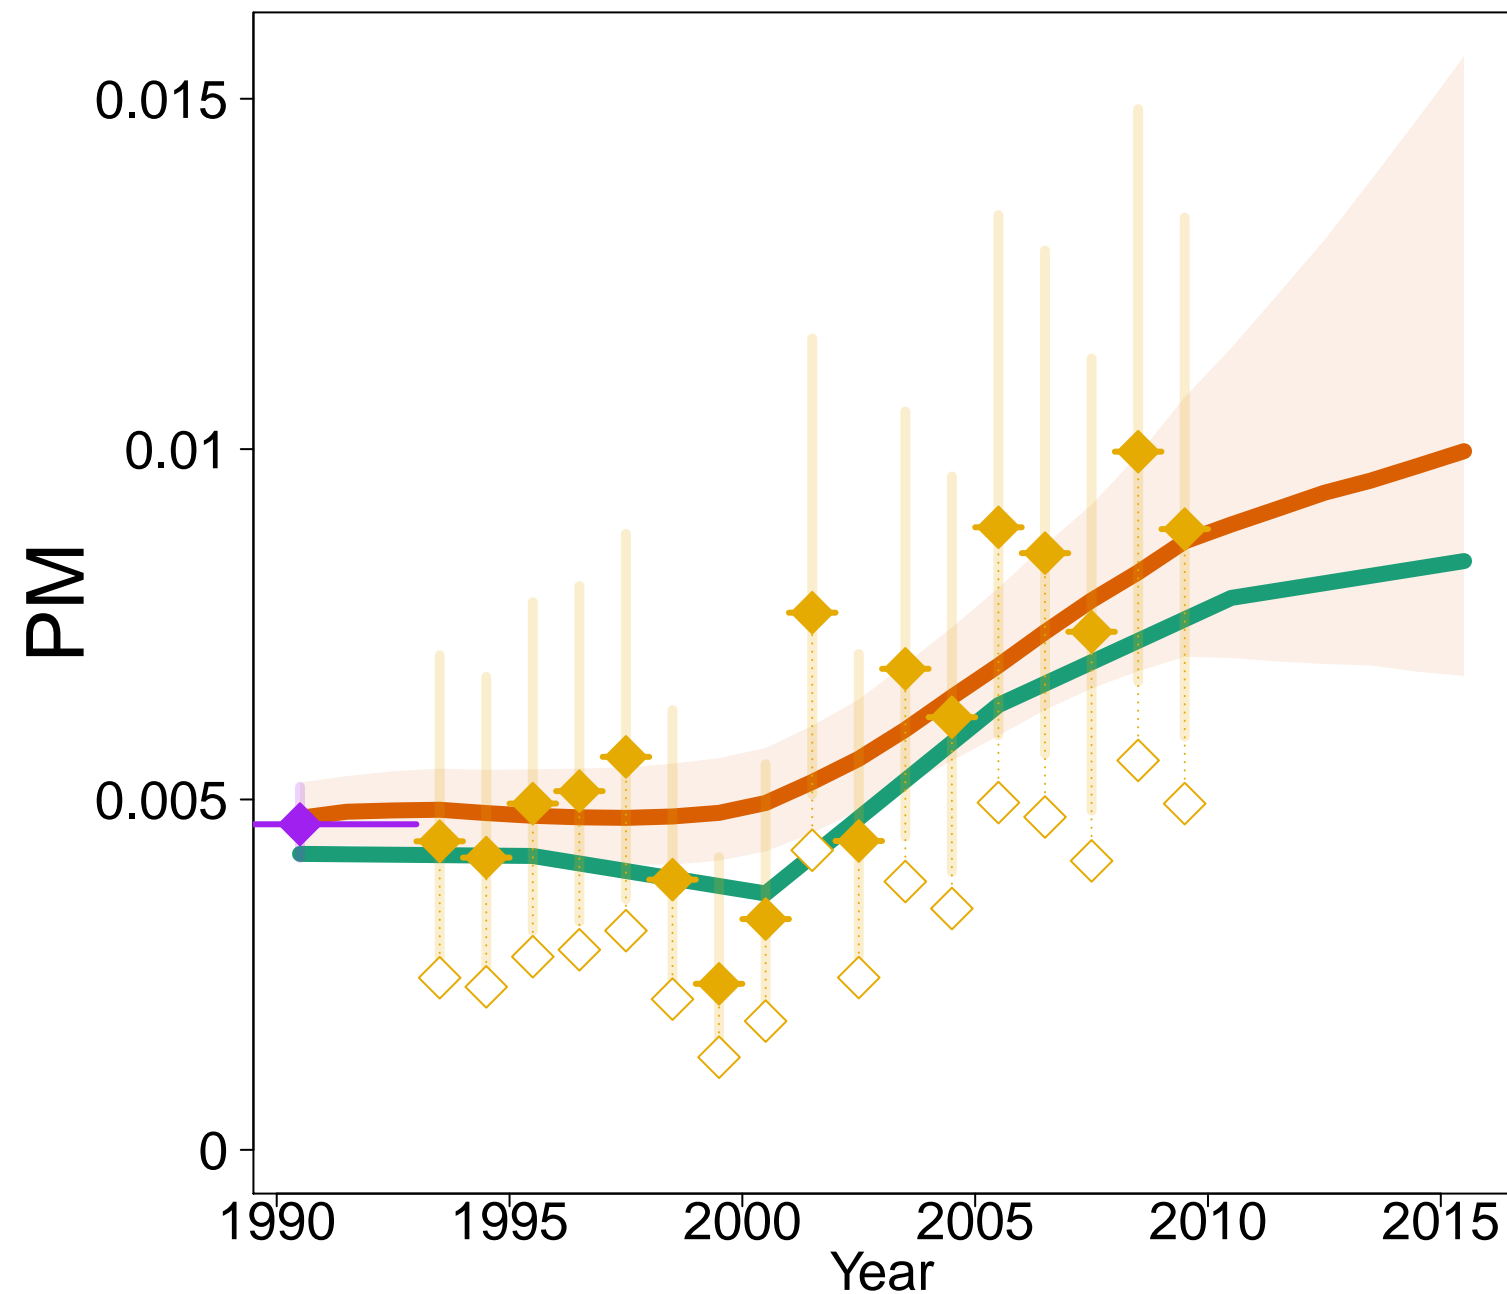

Canada [CAN; A]  
(Developed regions)

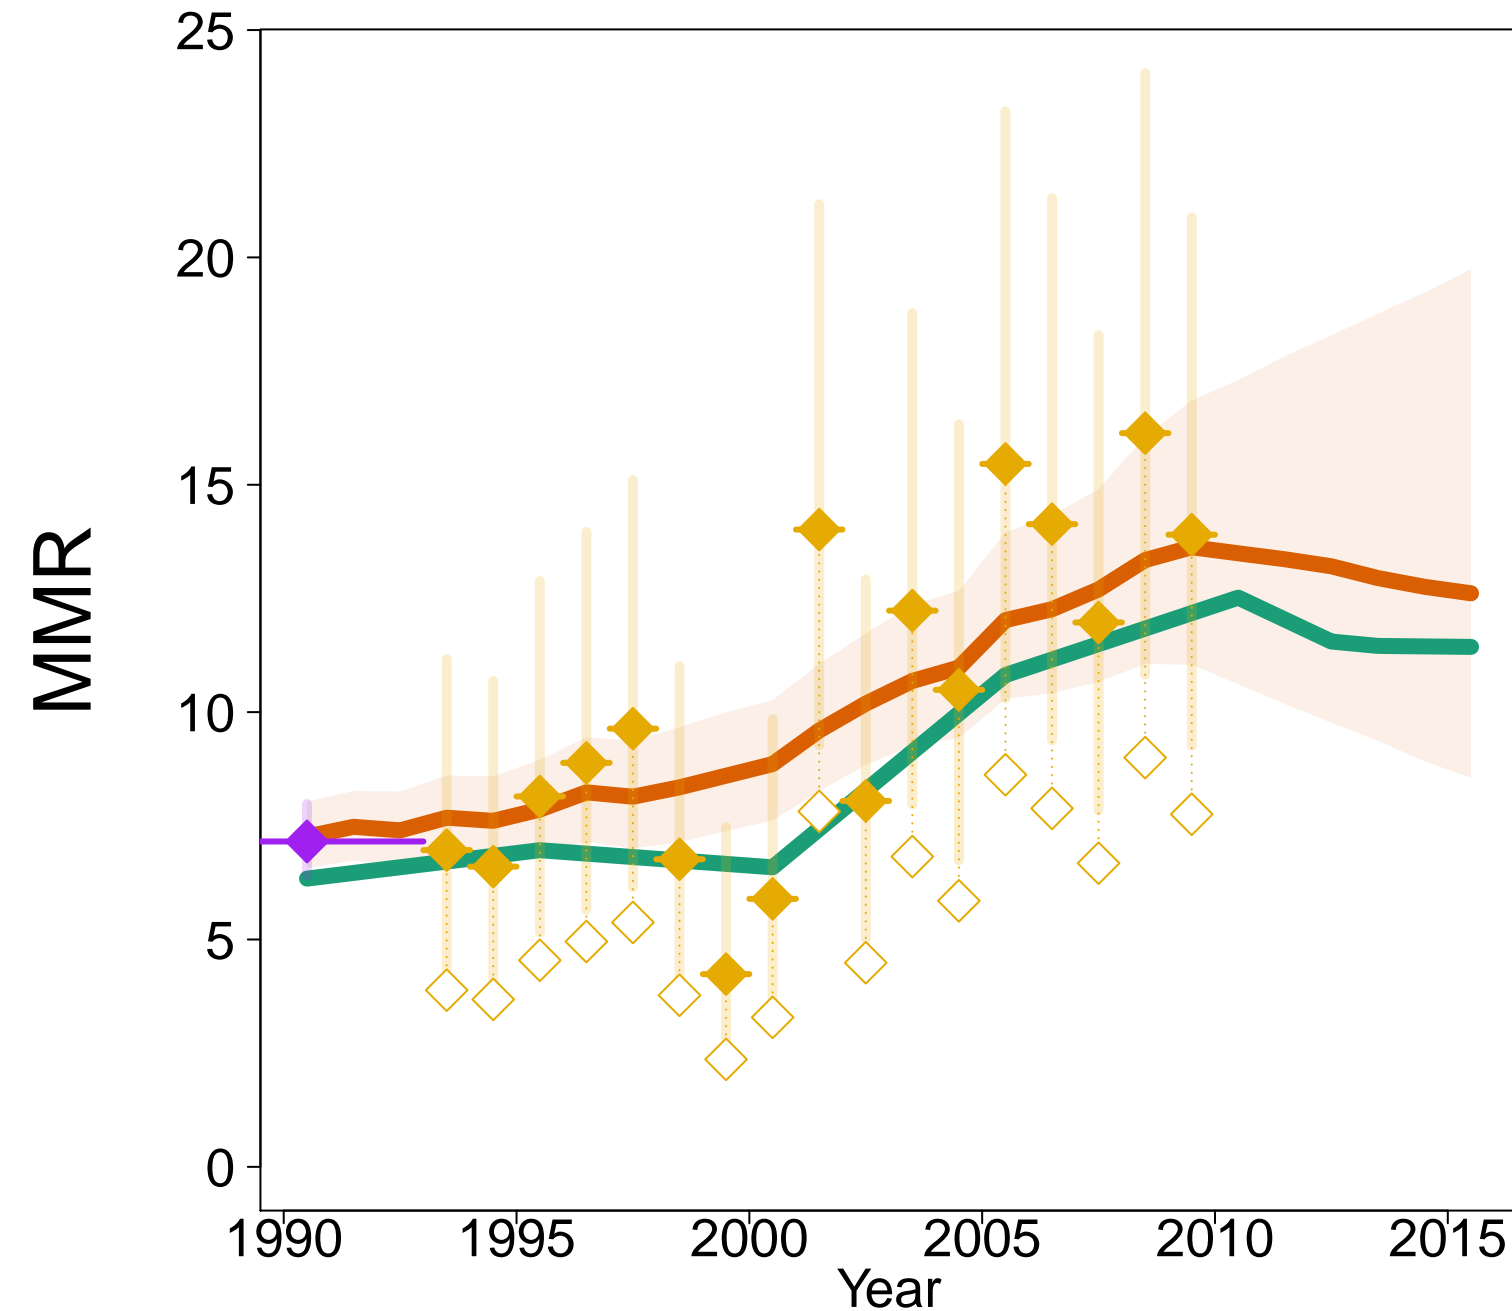

- Estimates –
- Bmat 2014
- MMEIG 2014
- Data –
- Observed Data
- Adjusted Data
- Data type –
- VR
- Spec. studies

Central African Republic [CAF; B]  
(Middle Africa)

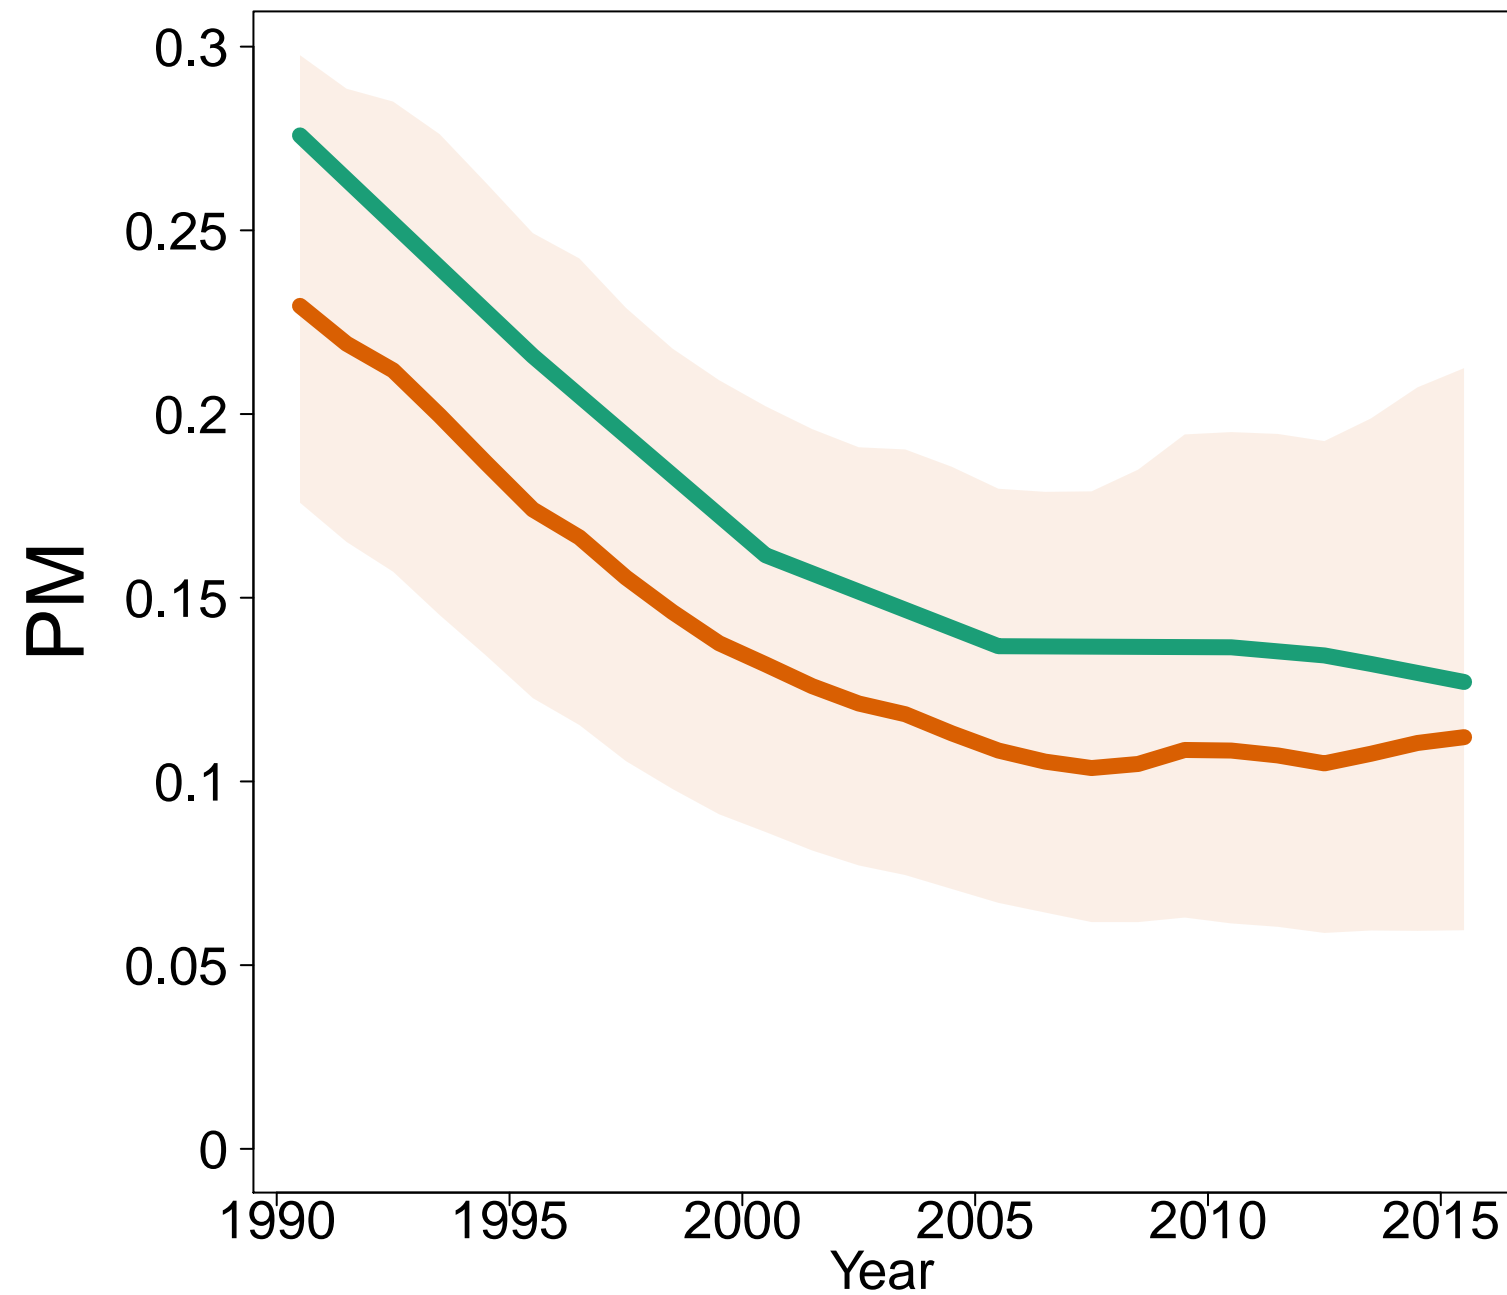

Central African Republic [CAF; B]  
(Middle Africa)

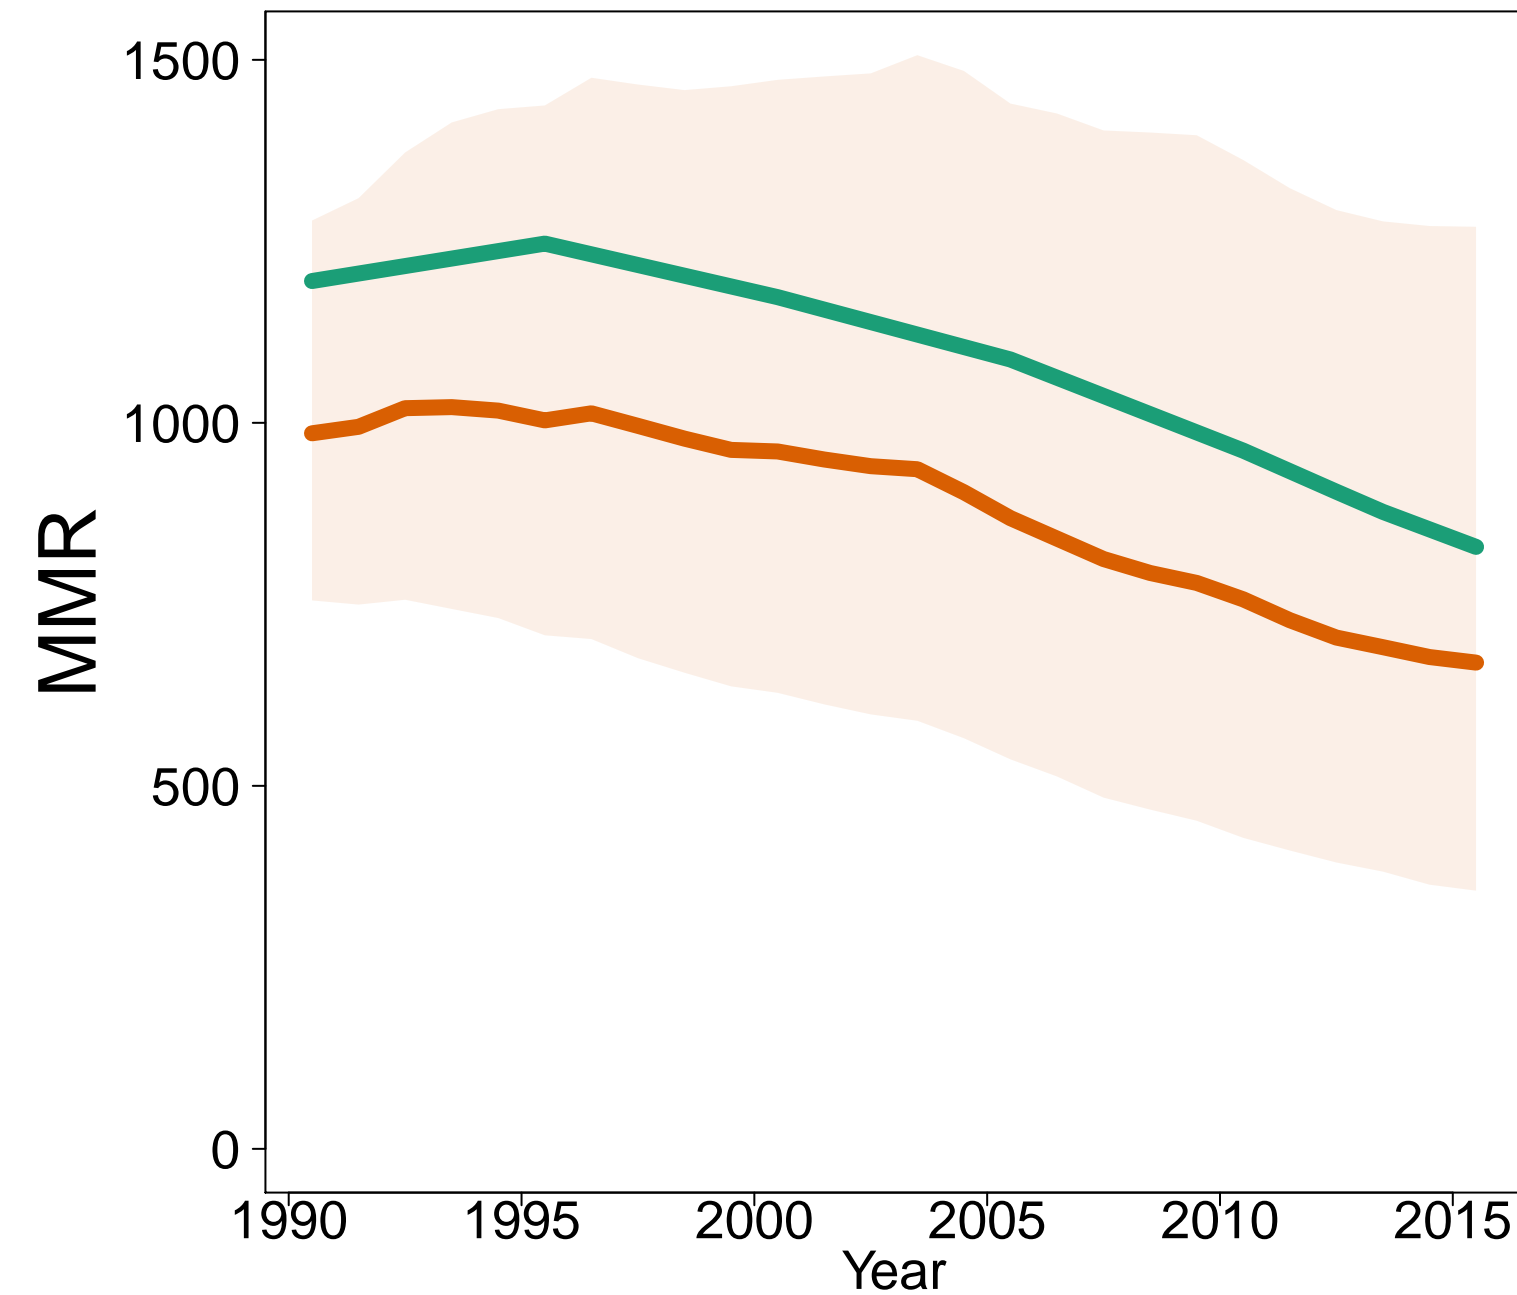

– Estimates –  
Bmat 2014  
MMEIG 2014  
– Data –

Chad [TCD; B]  
(Middle Africa)

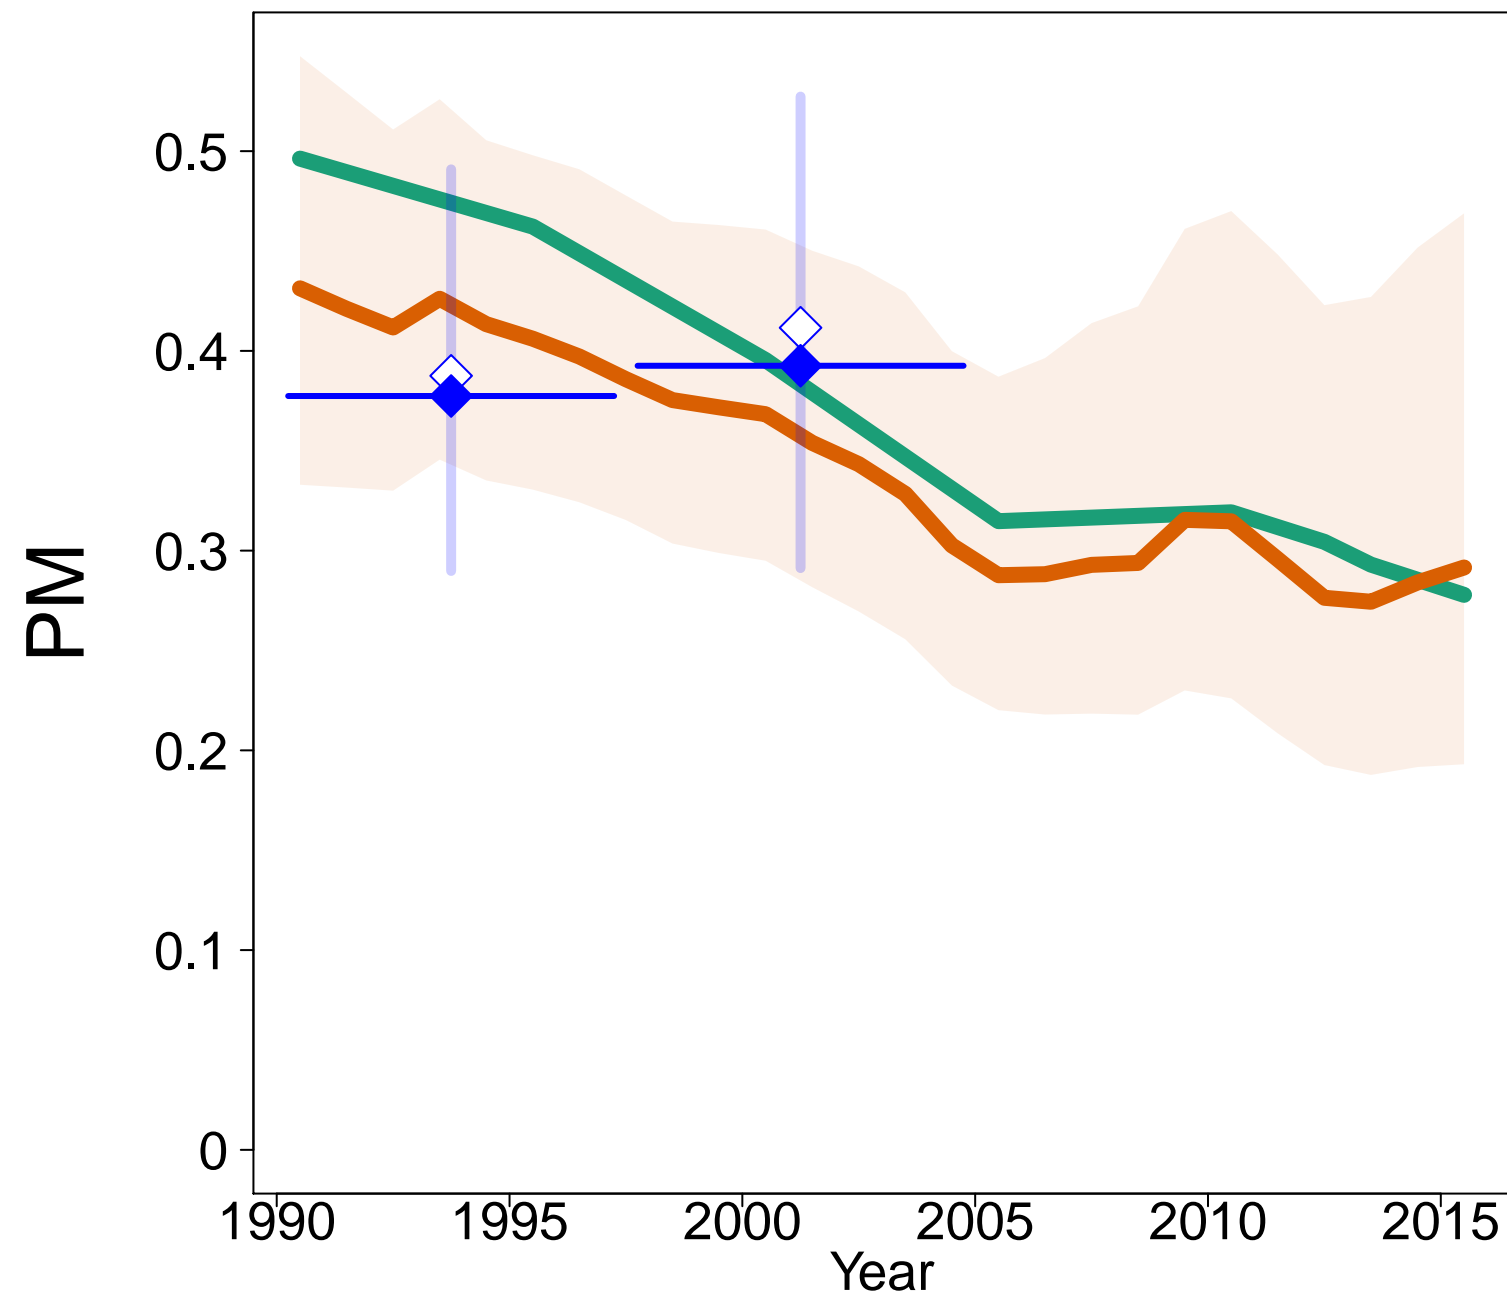

Chad [TCD; B]  
(Middle Africa)

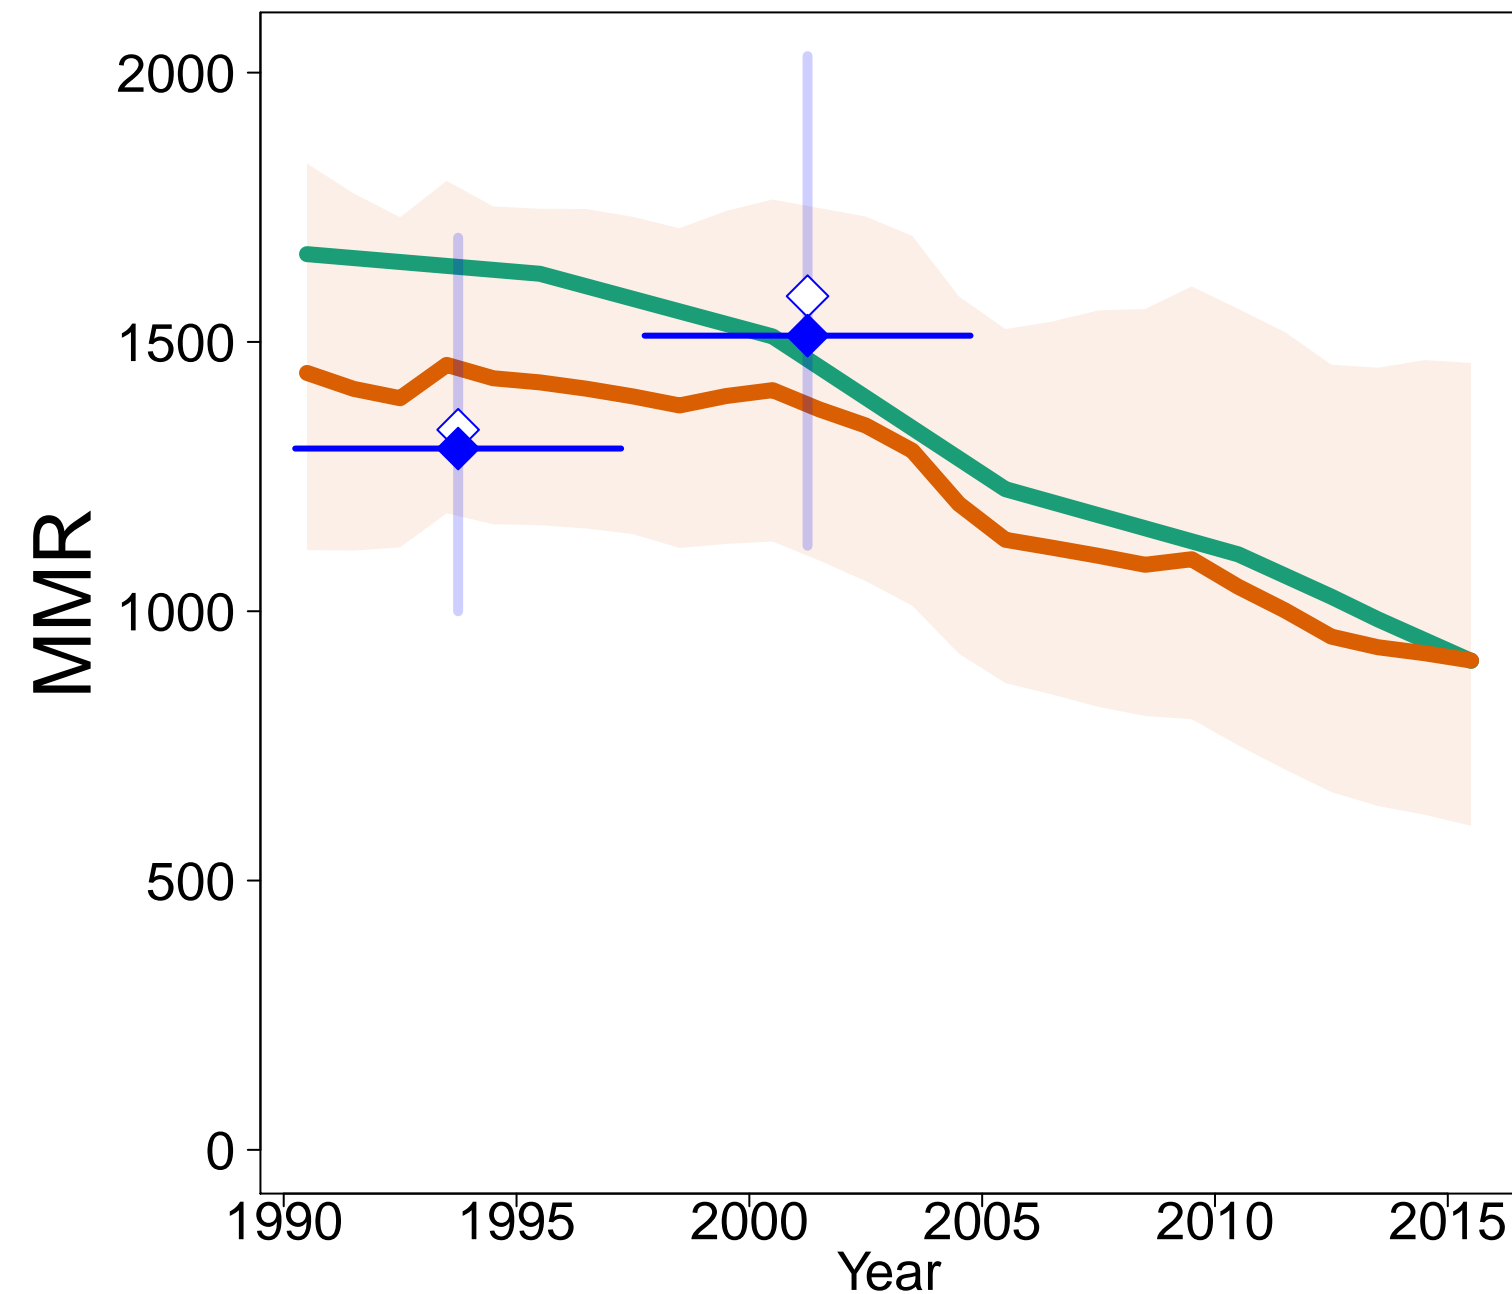

- Estimates –
- Bmat 2014
- MMEIG 2014
- Data –
- ◊ Observed Data
- ◆ Adjusted Data
- Data type –
- ◆ DHS



Chile [CHL; A]  
(South America)

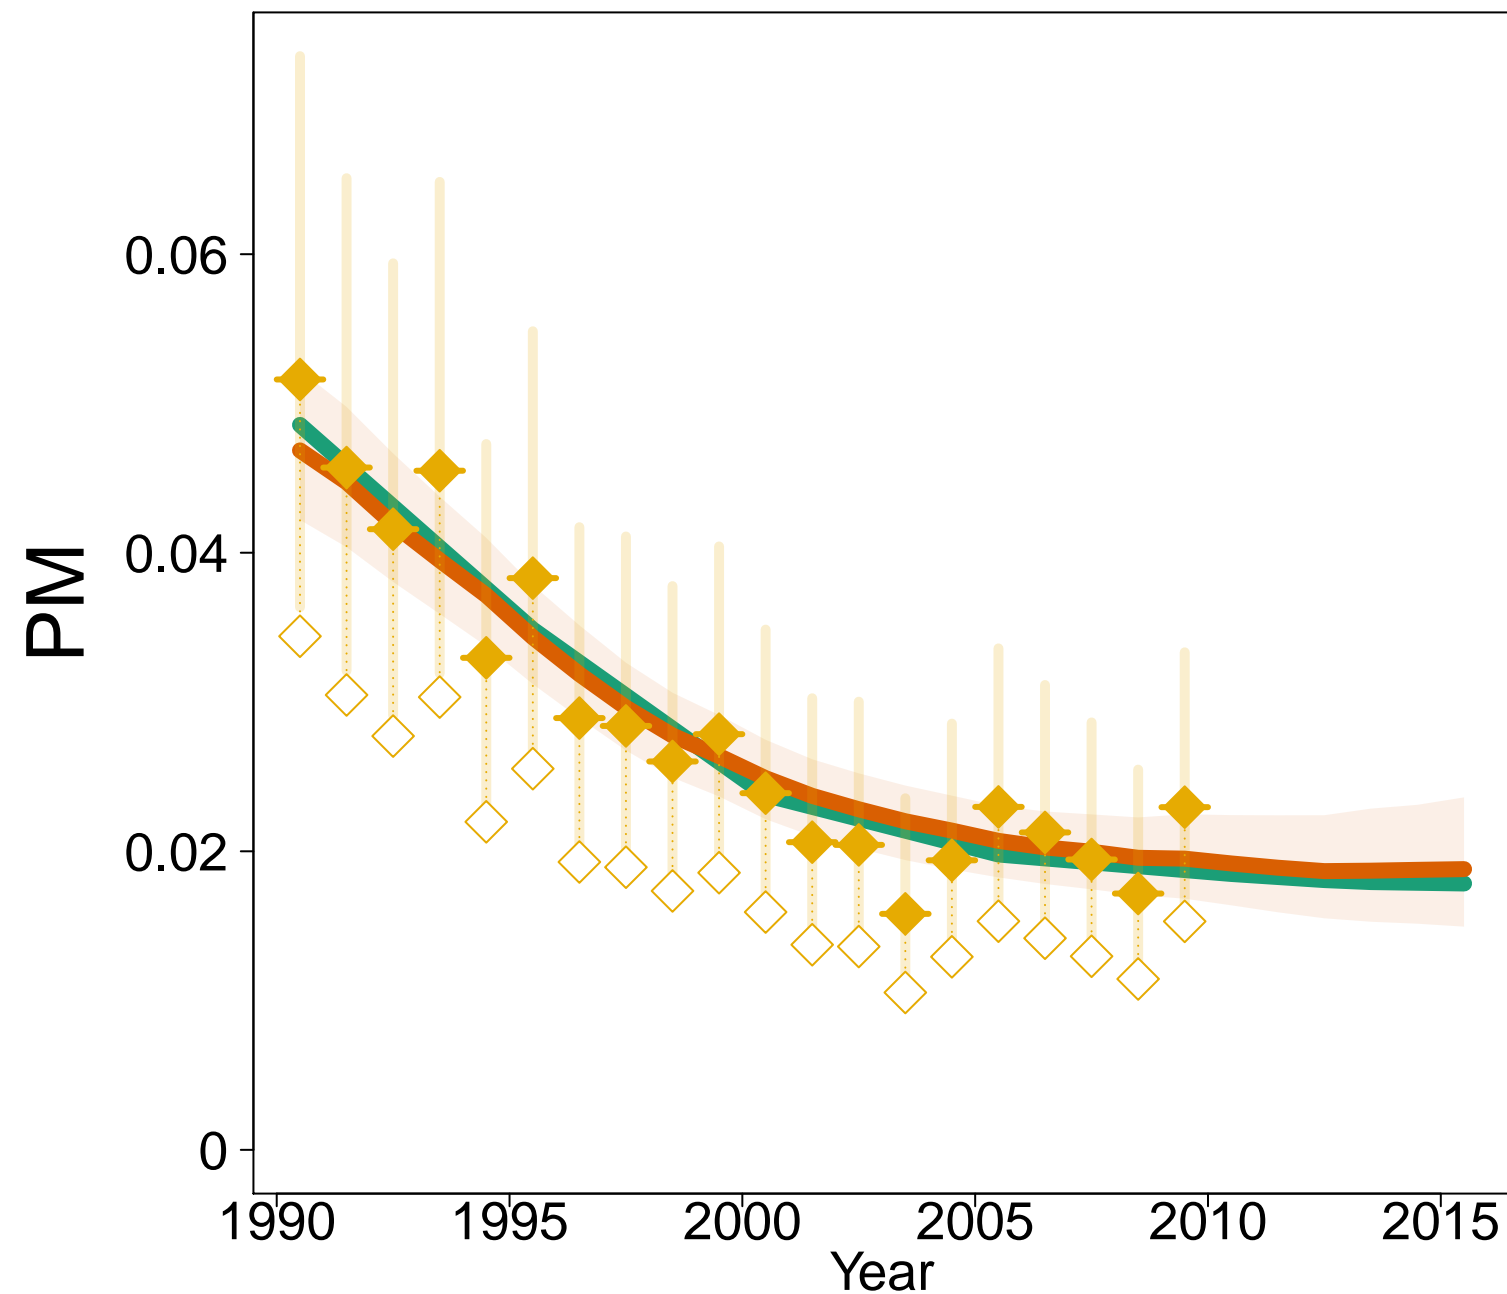

Chile [CHL; A]  
(South America)

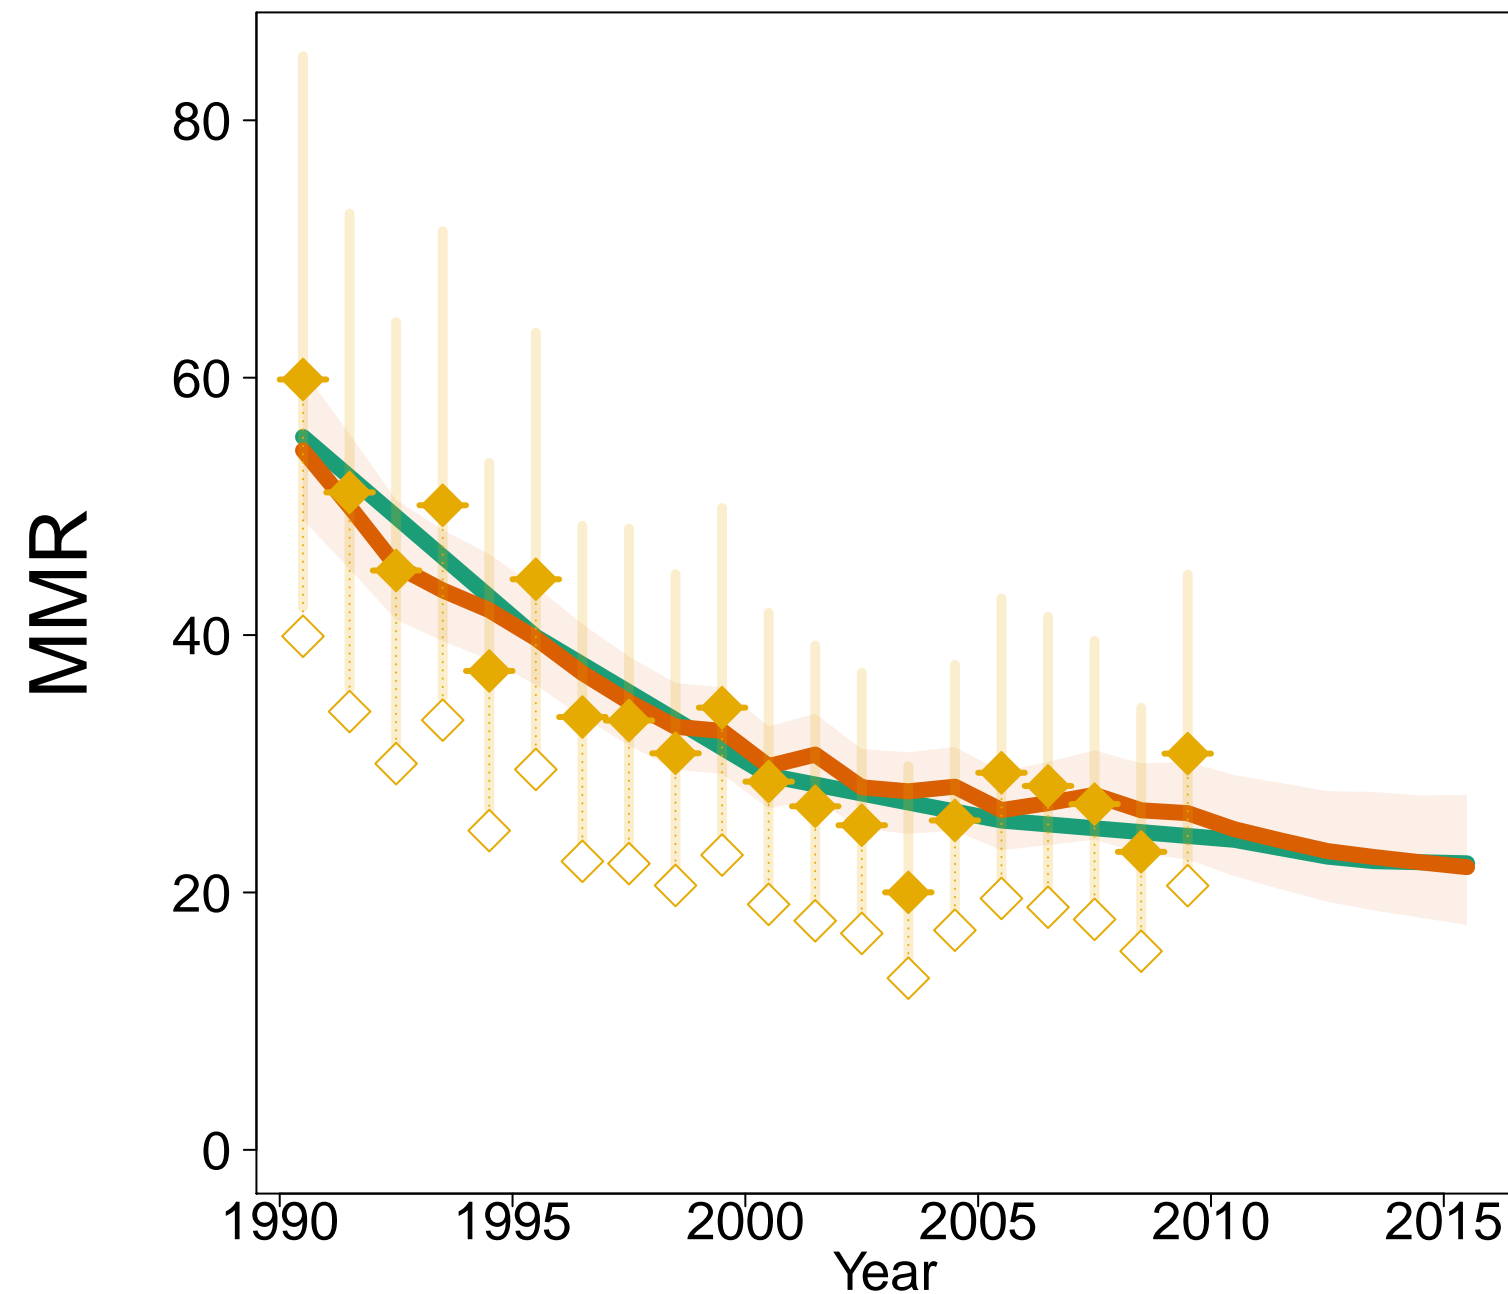

- Estimates –
- Bmat 2014
- MMEIG 2014
- Data –
- Observed Data
- Adjusted Data
- Data type –
- VR

China [CHN; B]  
(Eastern Asia)

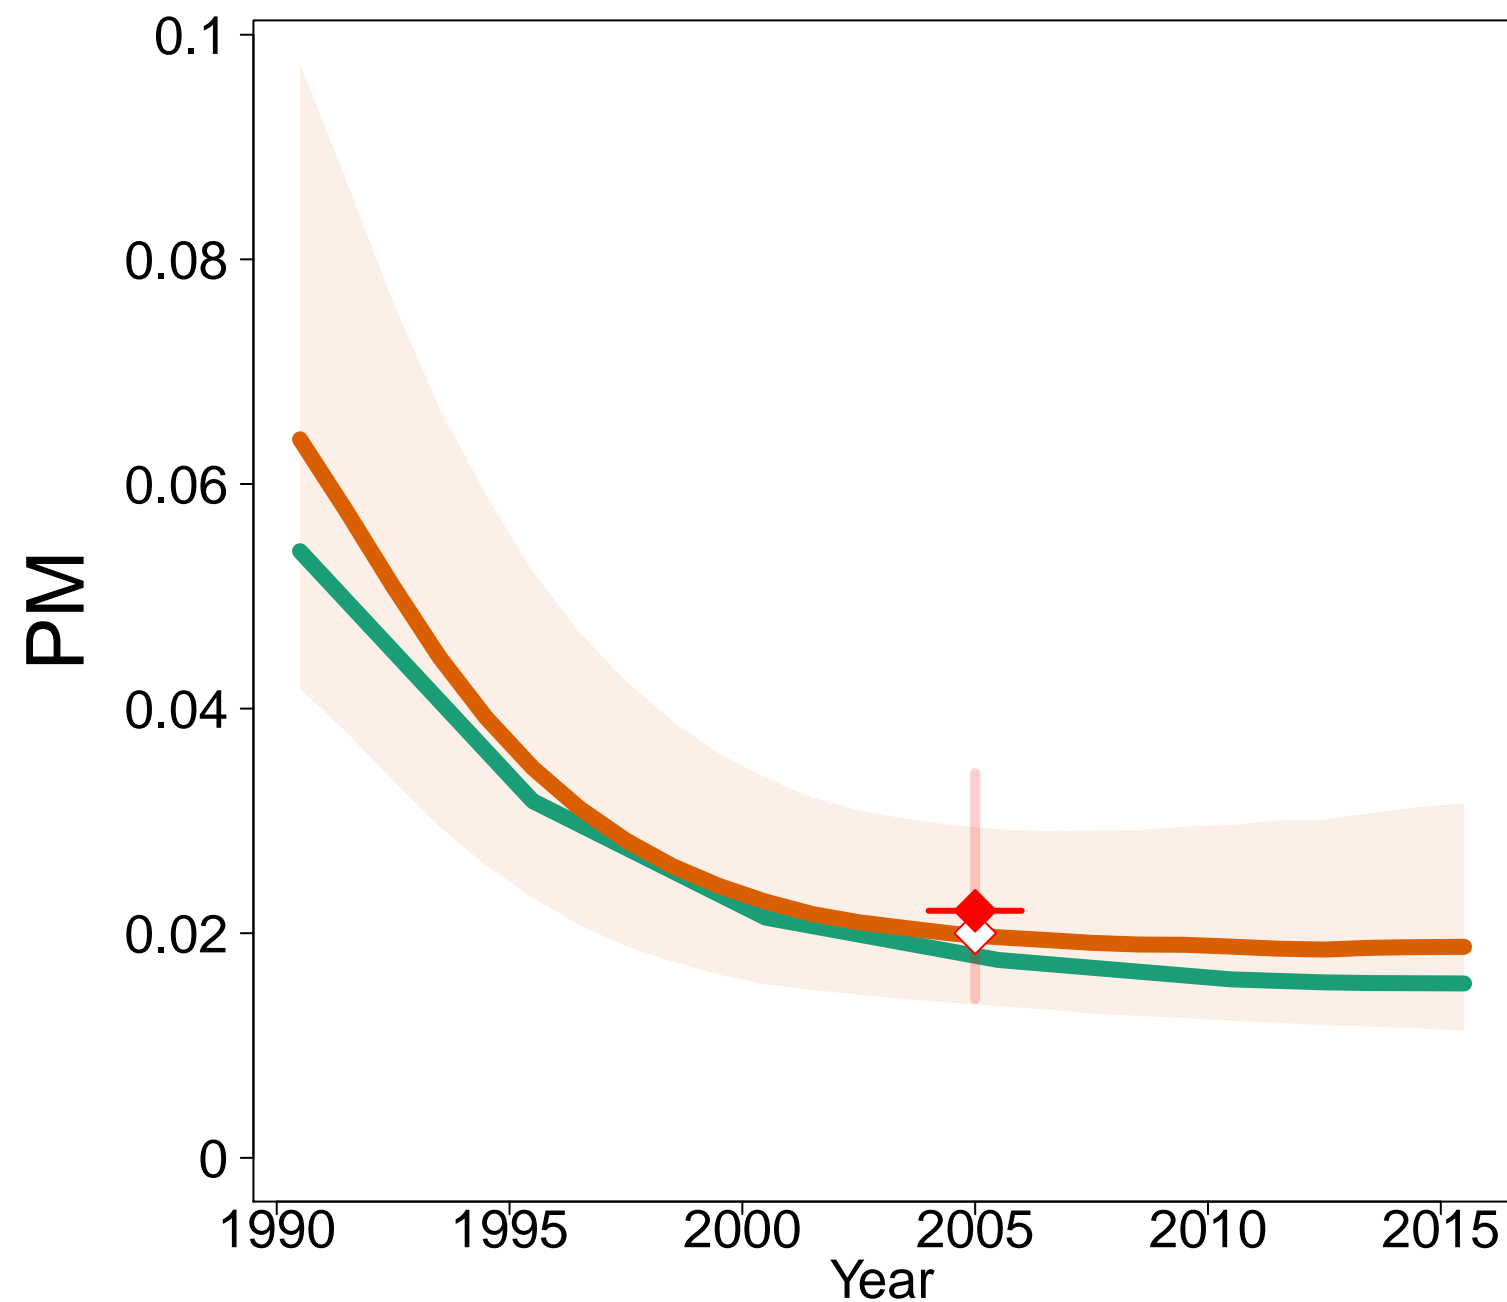

China [CHN; B]  
(Eastern Asia)

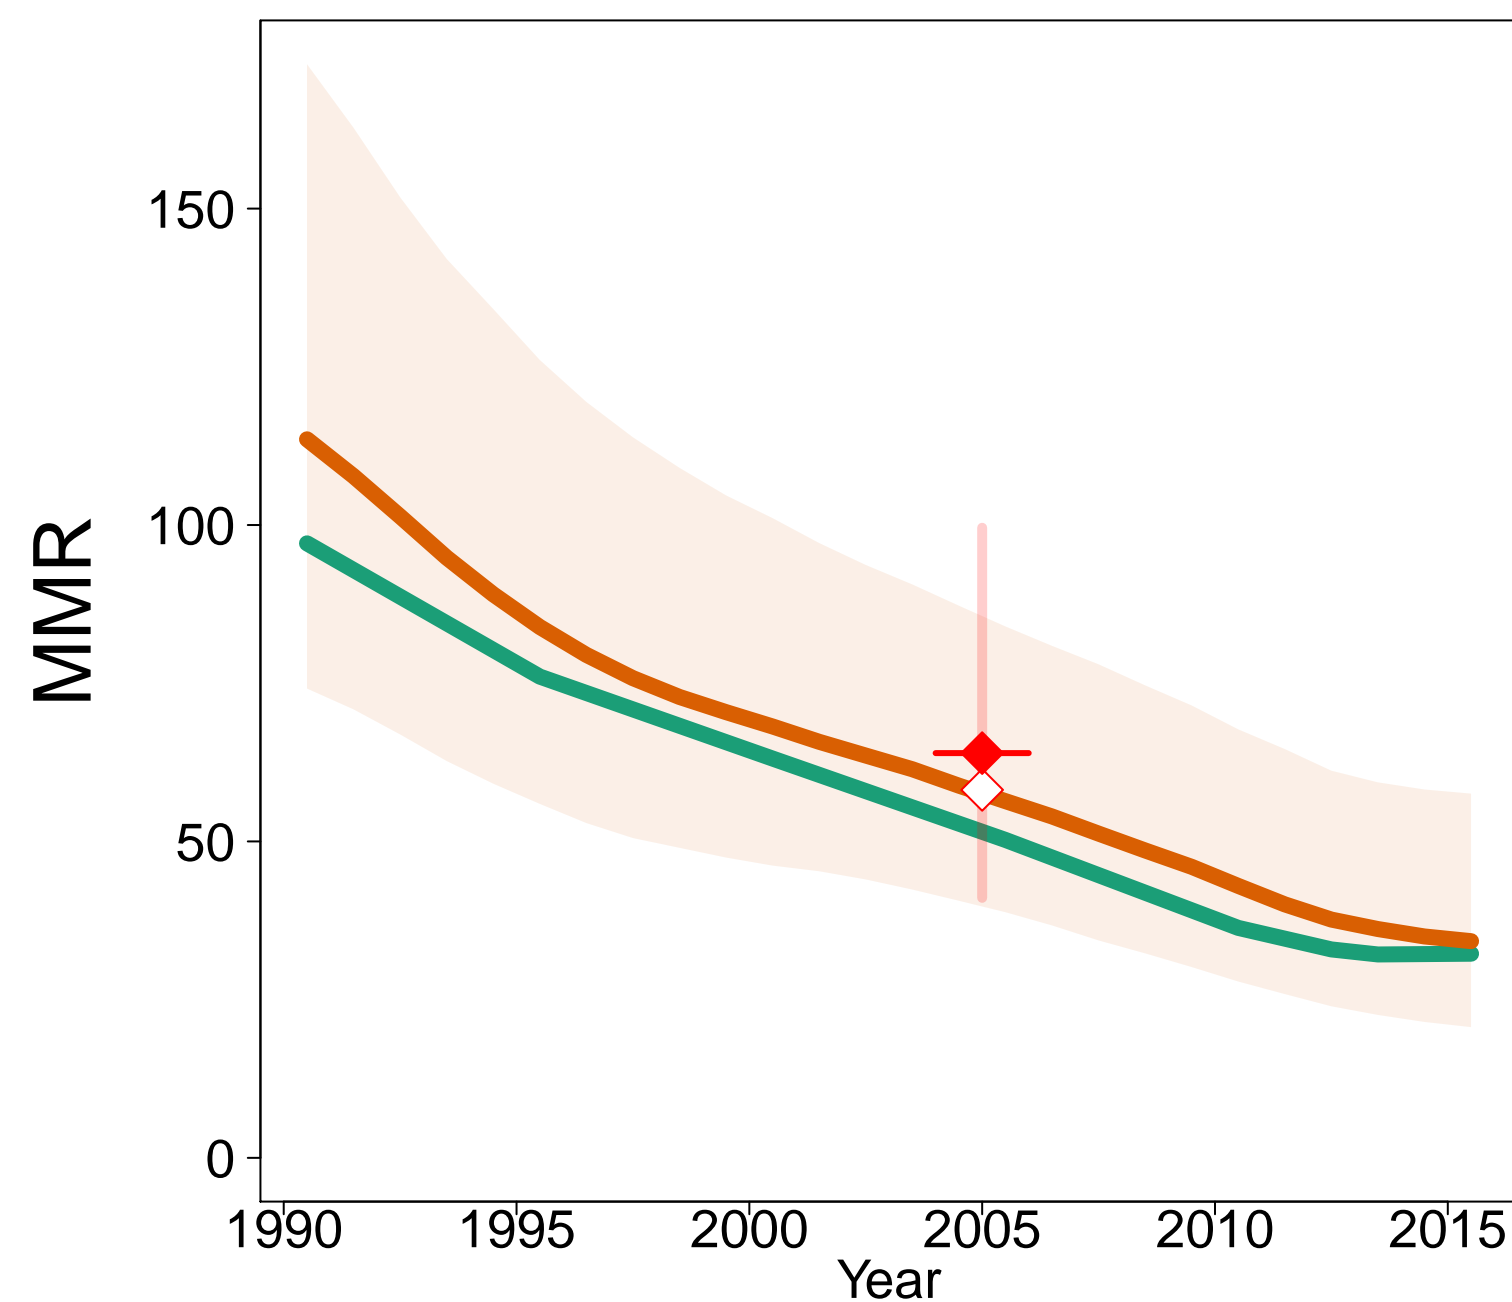

- Estimates –
- Bmat 2014
- MMEIG 2014
- Data –
- ◊ Observed Data
- ◆ Adjusted Data
- Data type –
- ◆ Misc. studies

Colombia [COL; A]  
(South America)

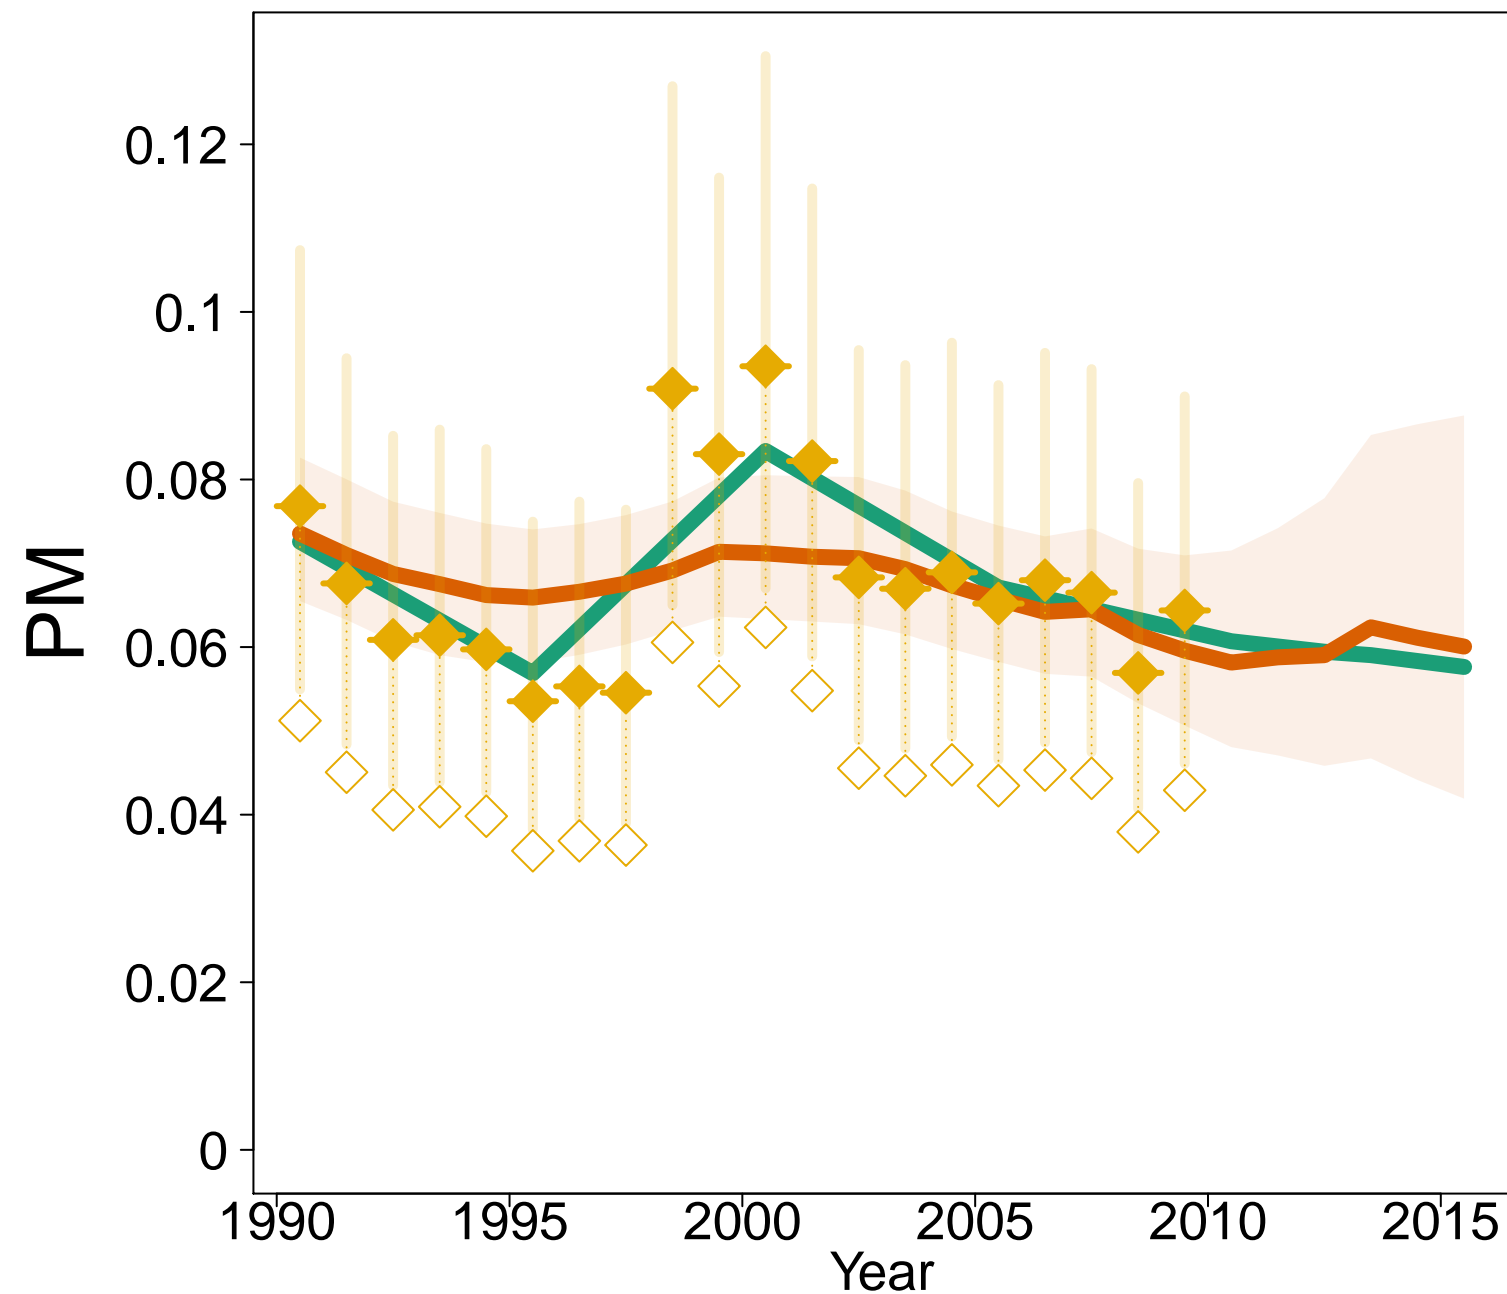

Colombia [COL; A]  
(South America)

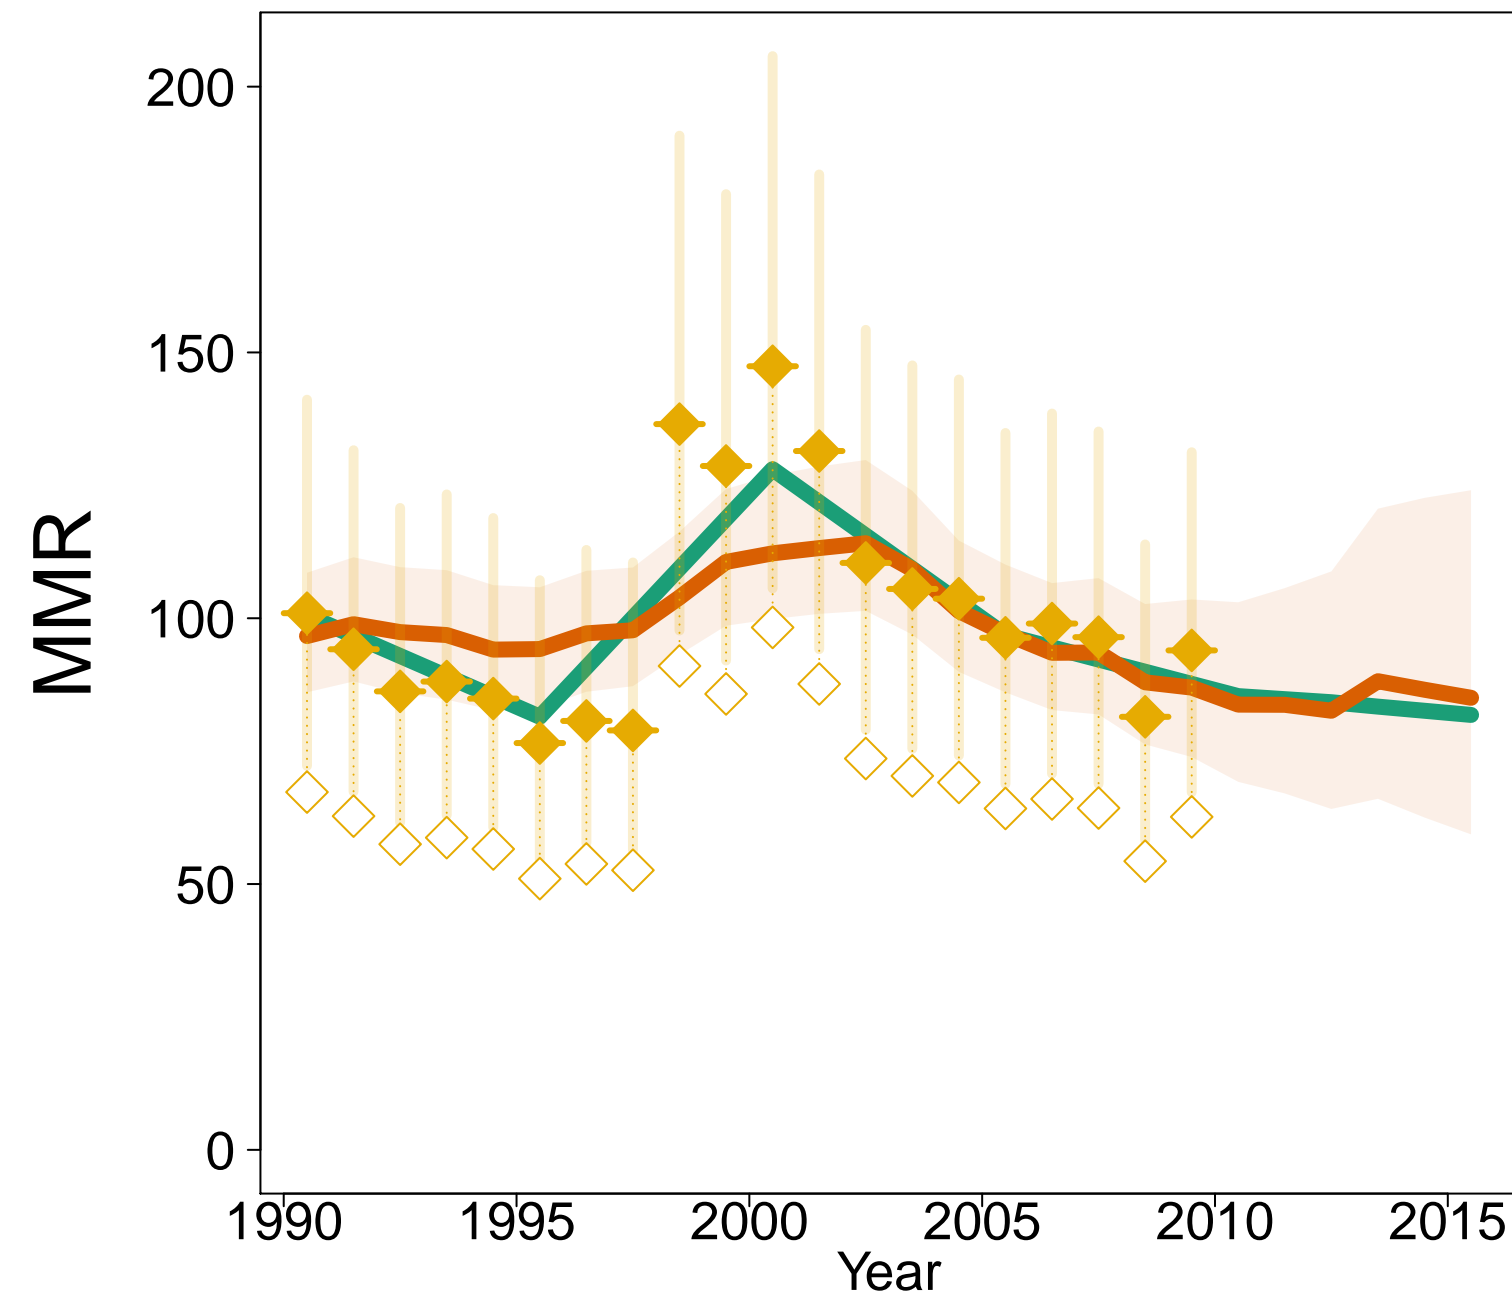

Comoros [COM; C]  
(Eastern Africa)

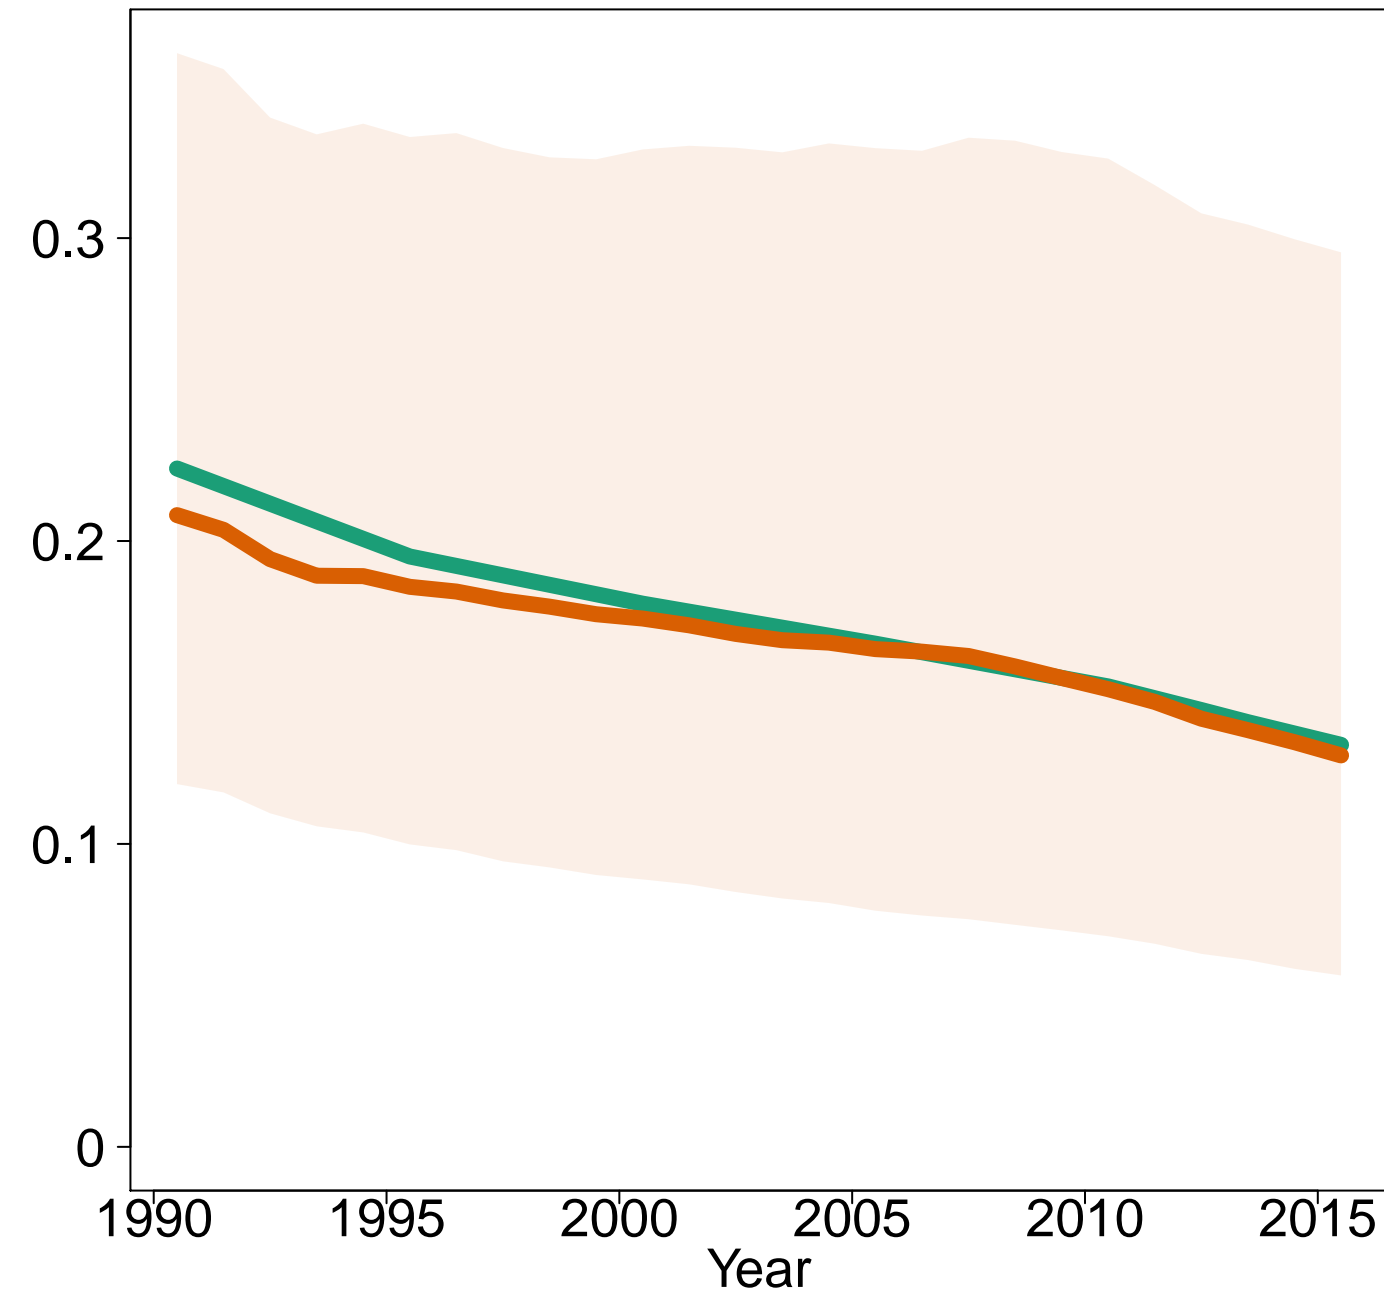

Comoros [COM; C]  
(Eastern Africa)

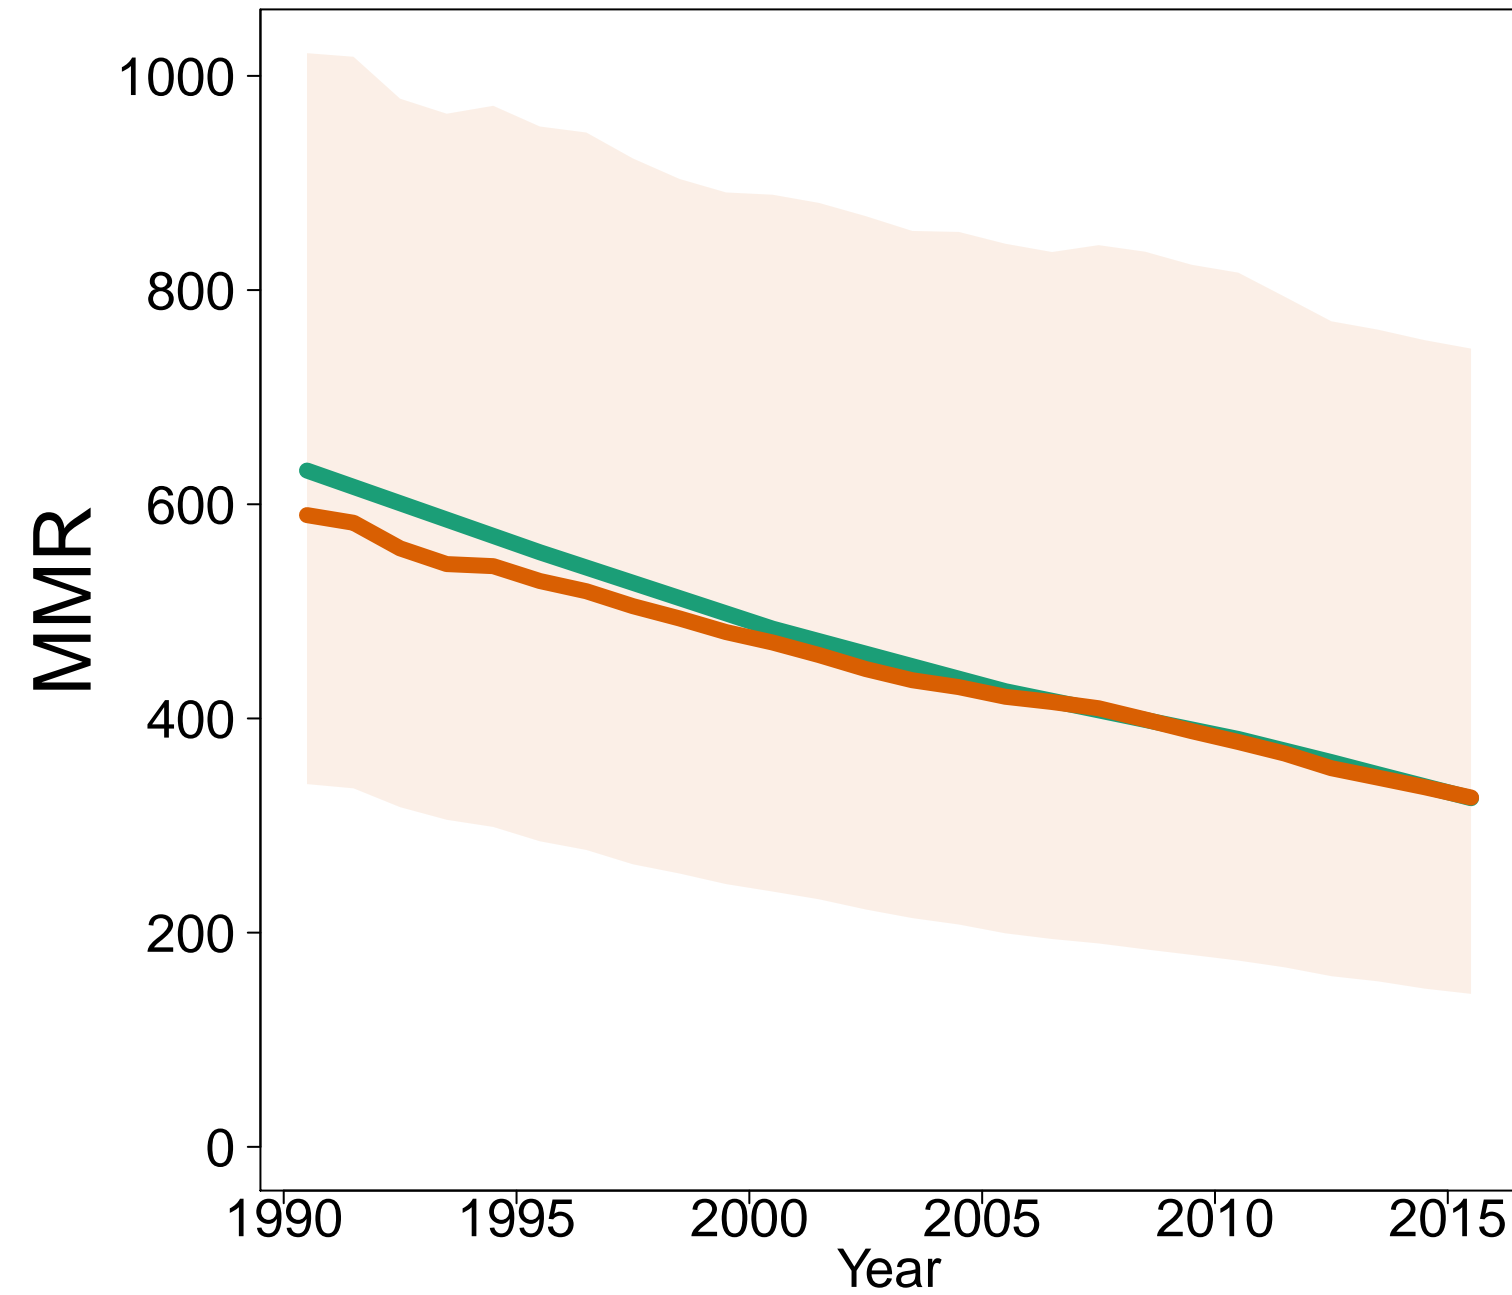

– Estimates –  
Bmat 2014  
MMEIG 2014  
– Data –

Congo [COG; B]  
(Middle Africa)

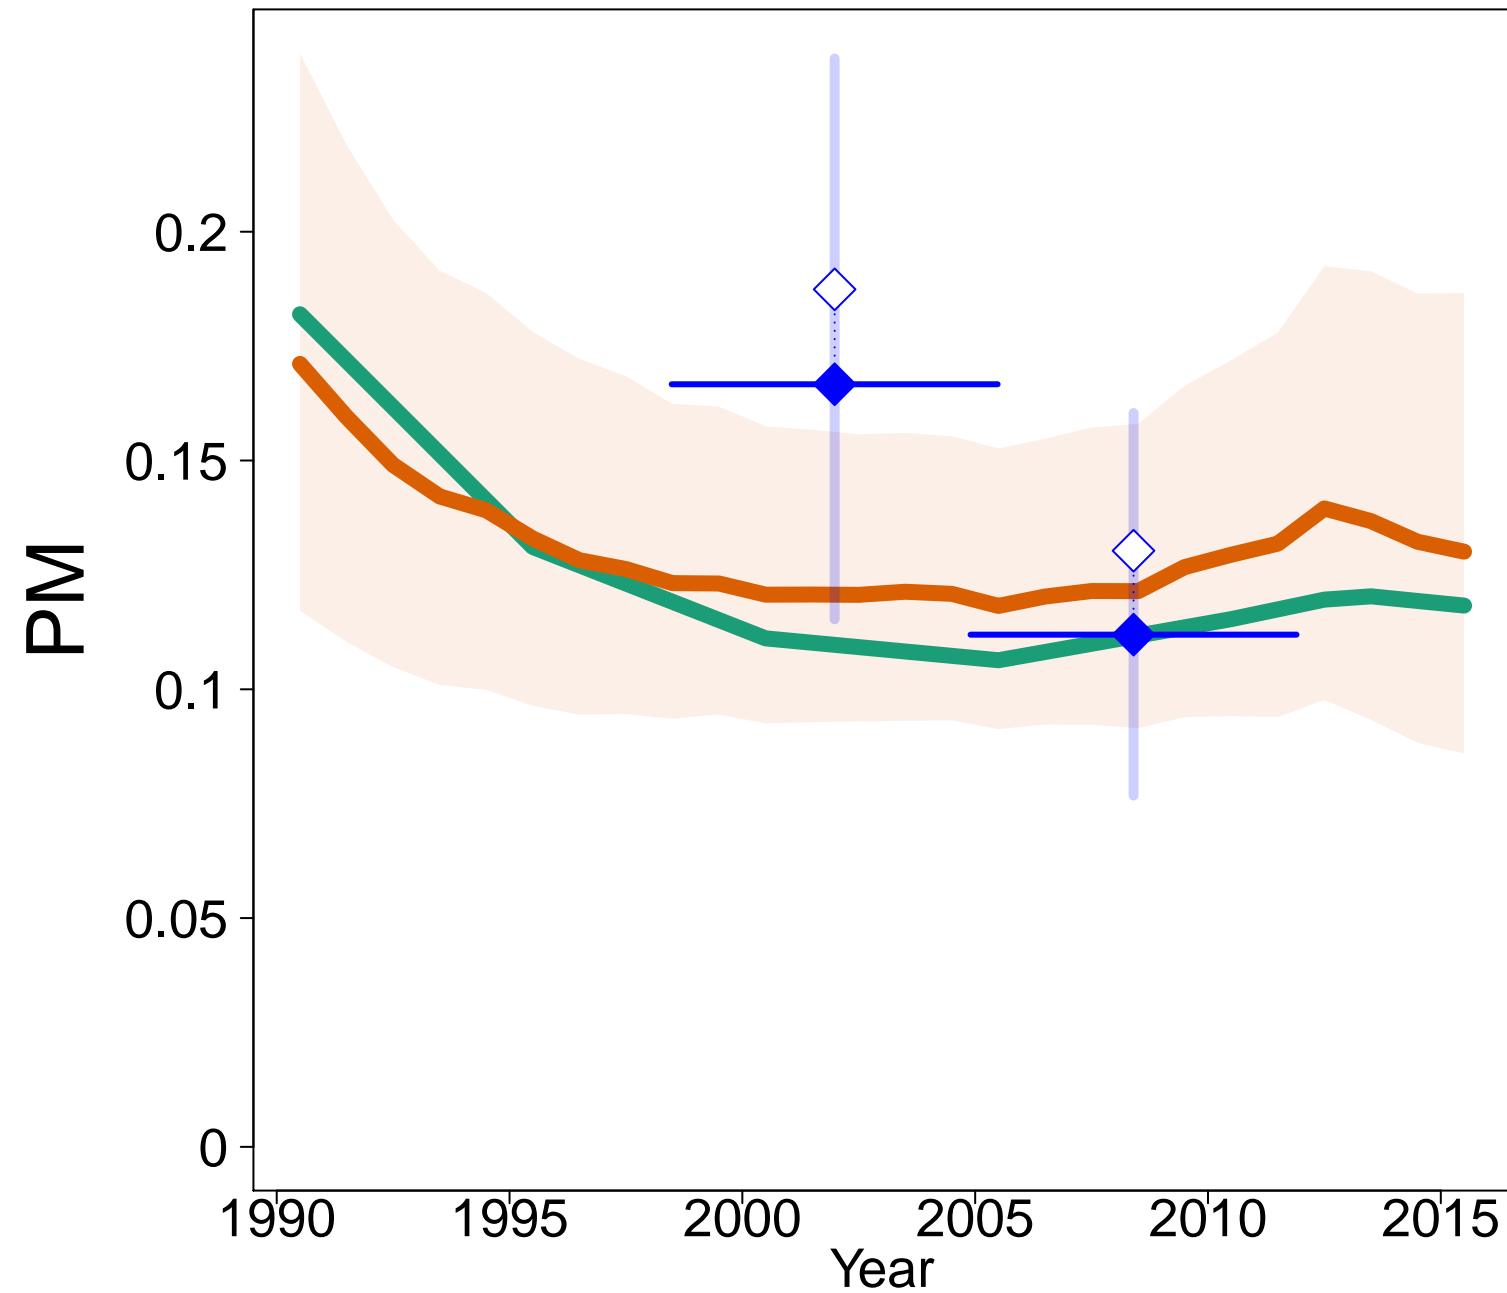

Congo [COG; B]  
(Middle Africa)

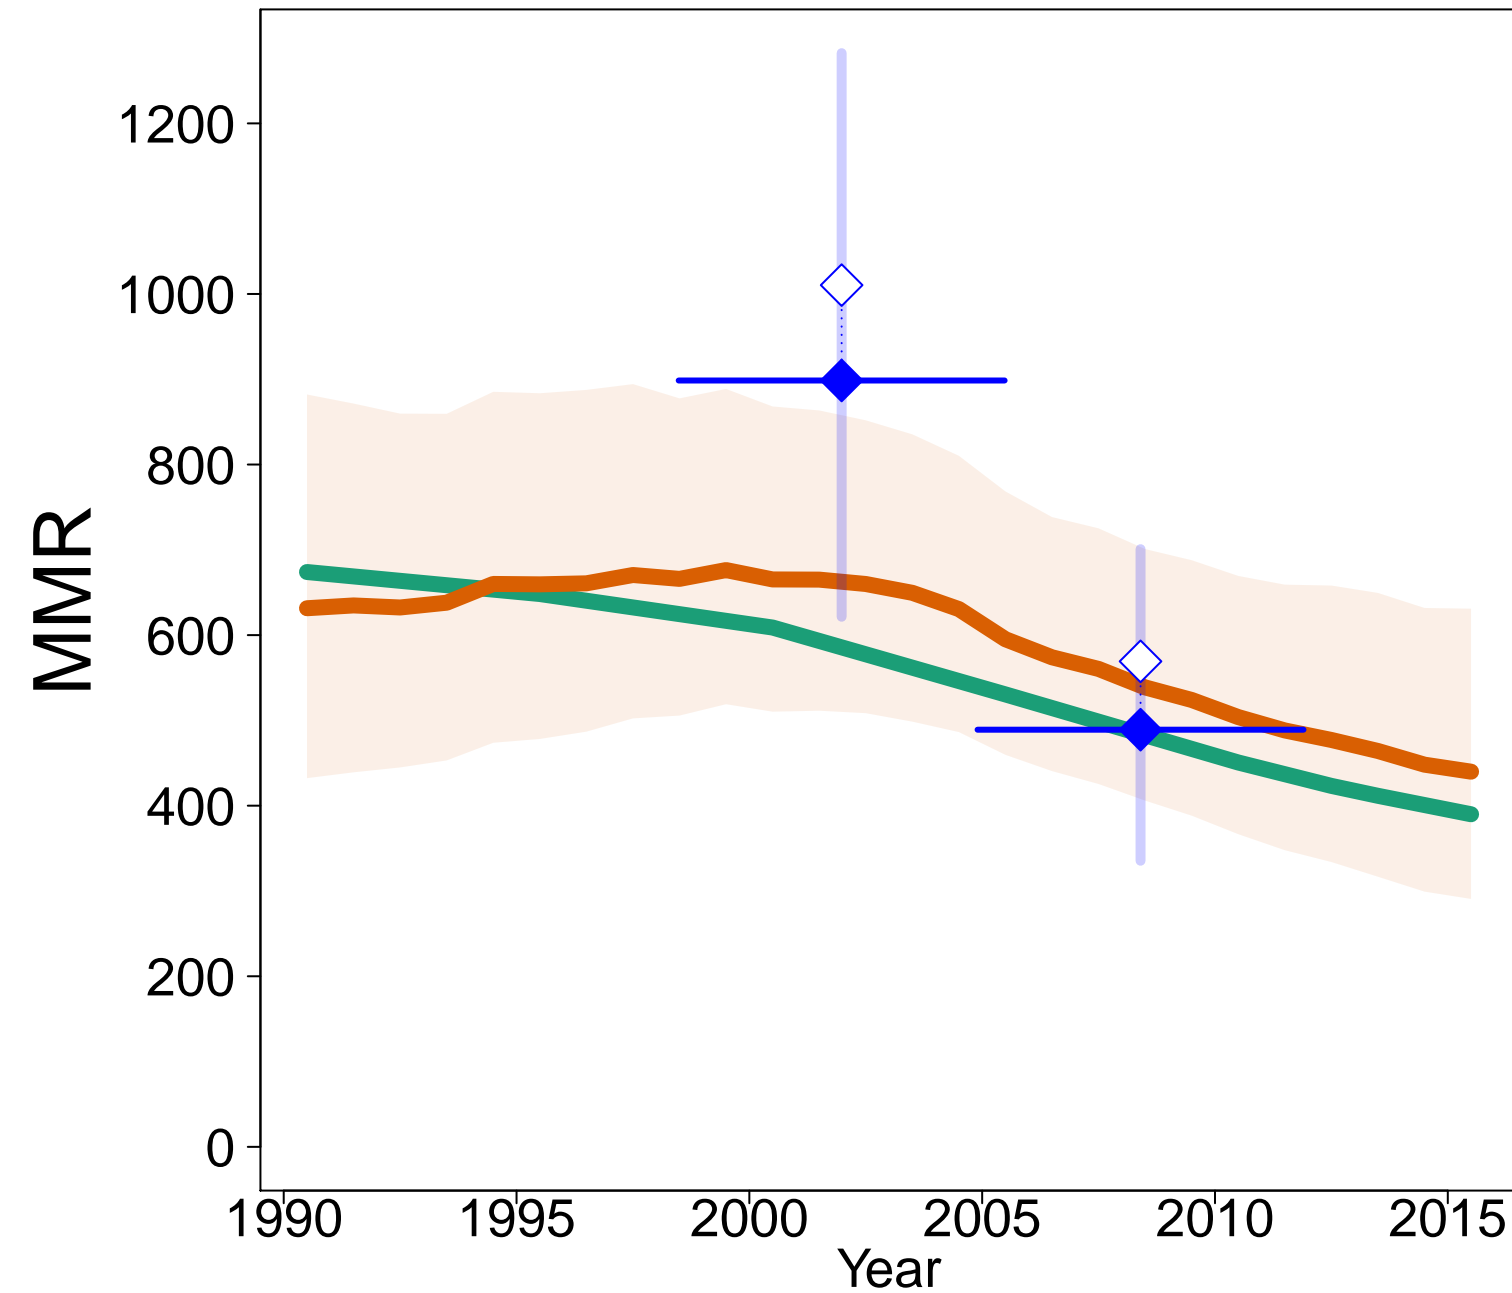

- Estimates –
- Bmat 2014
- MMEIG 2014
- Data –
- Observed Data
- Adjusted Data
- Data type –
- DHS

Costa Rica [CRI; A]  
(Central America)

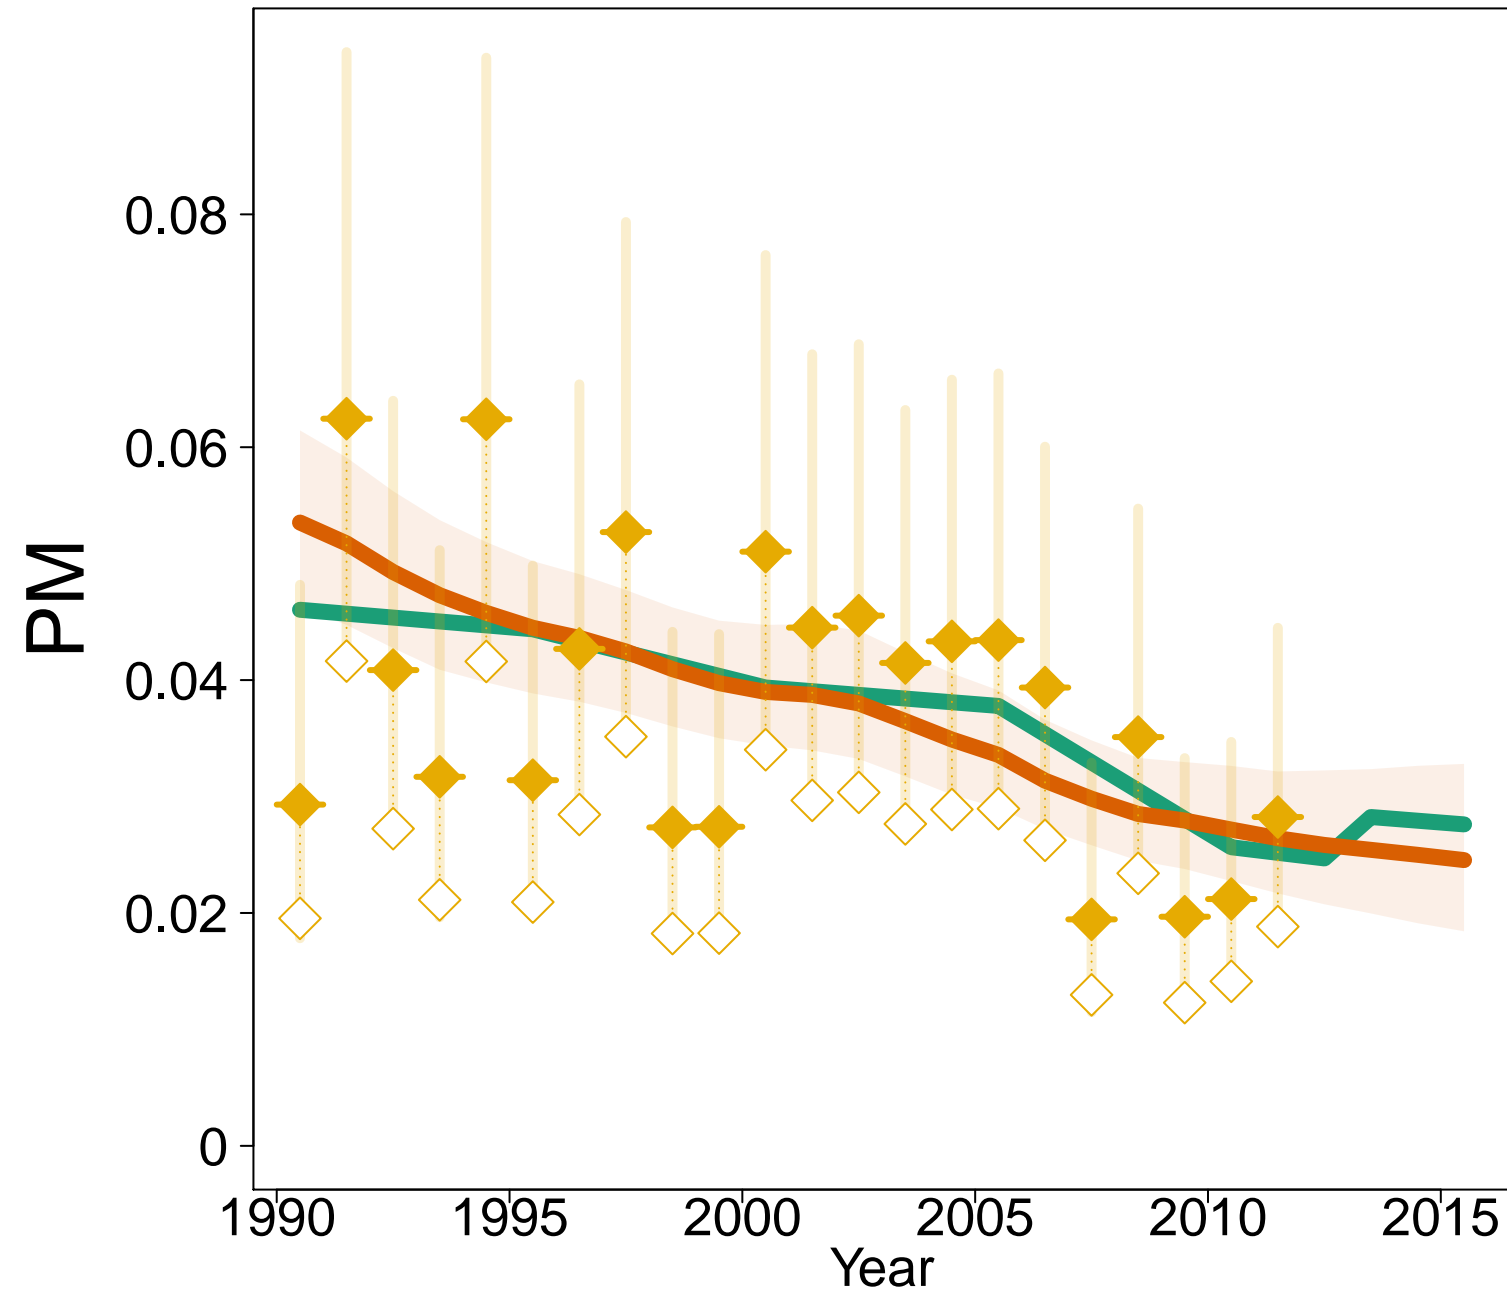

Costa Rica [CRI; A]  
(Central America)

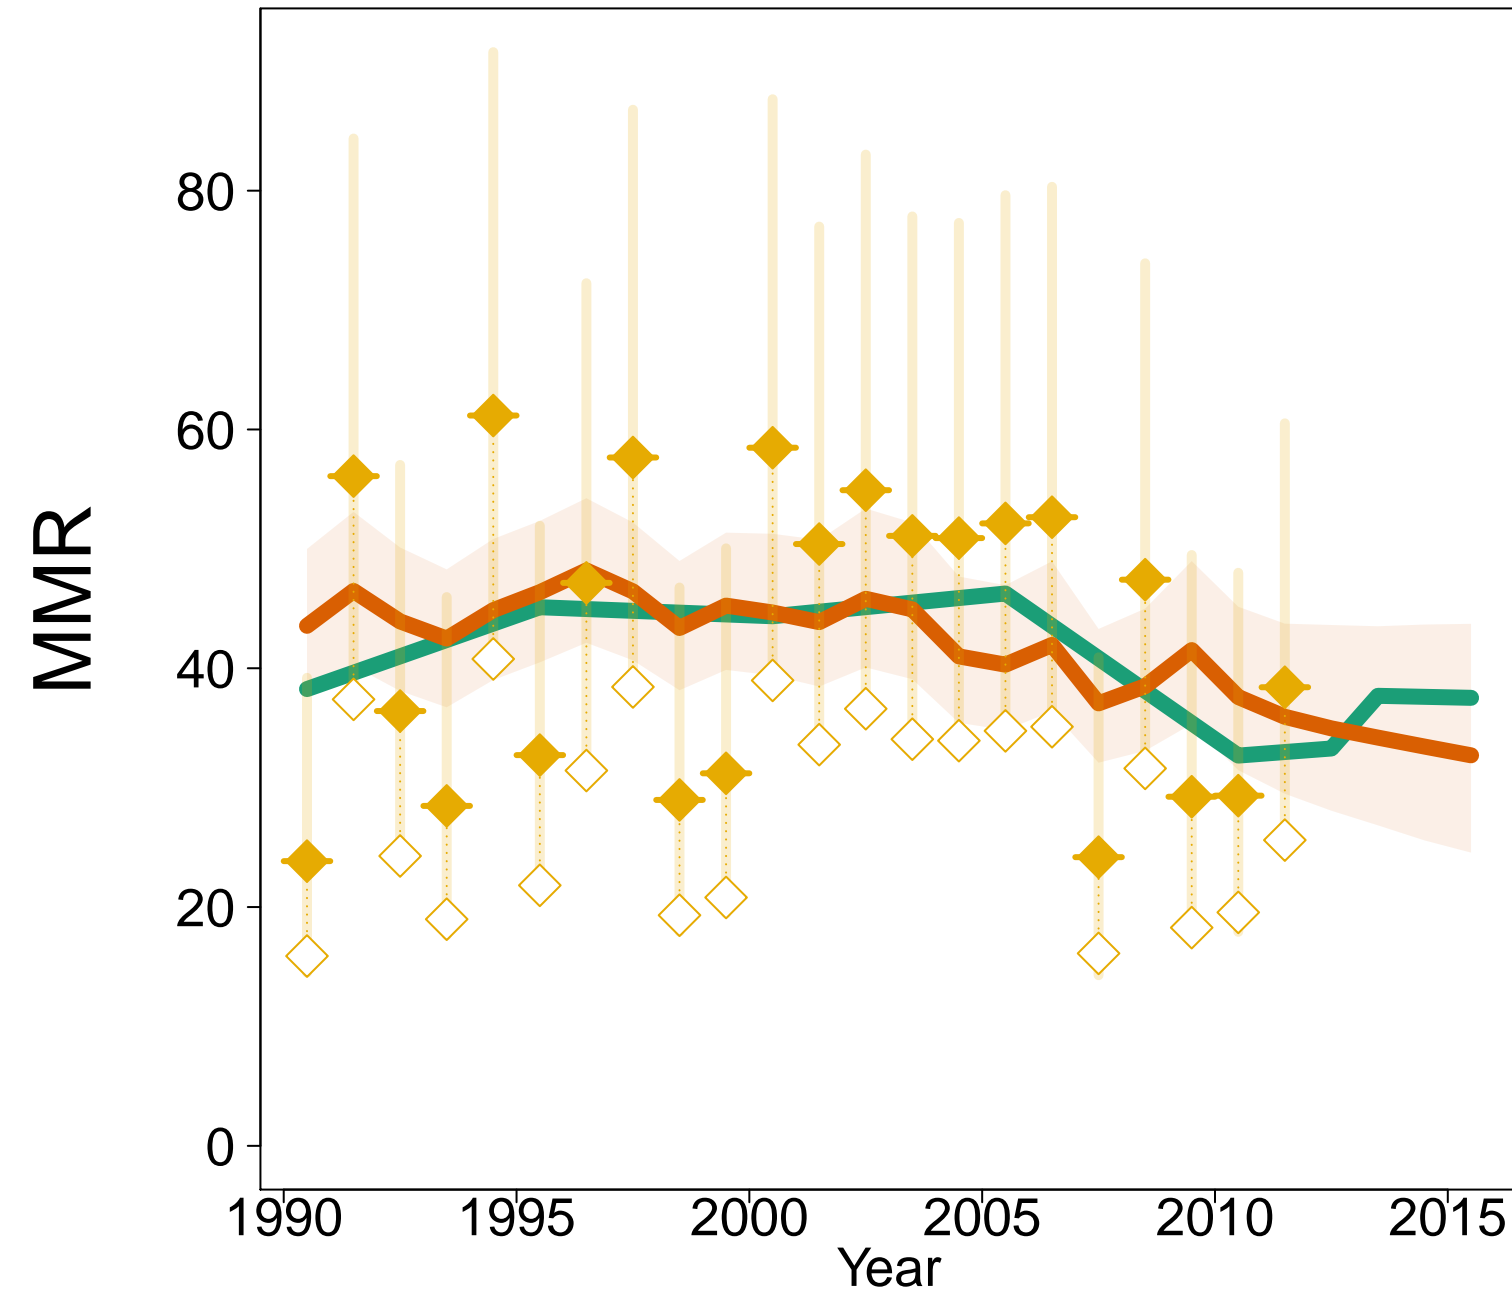

- Estimates –
- Bmat 2014
- MMEIG 2014
- Data –
- Observed Data
- Adjusted Data
- Data type –
- VR

Cote d'Ivoire [CIV; B]  
(Western Africa)

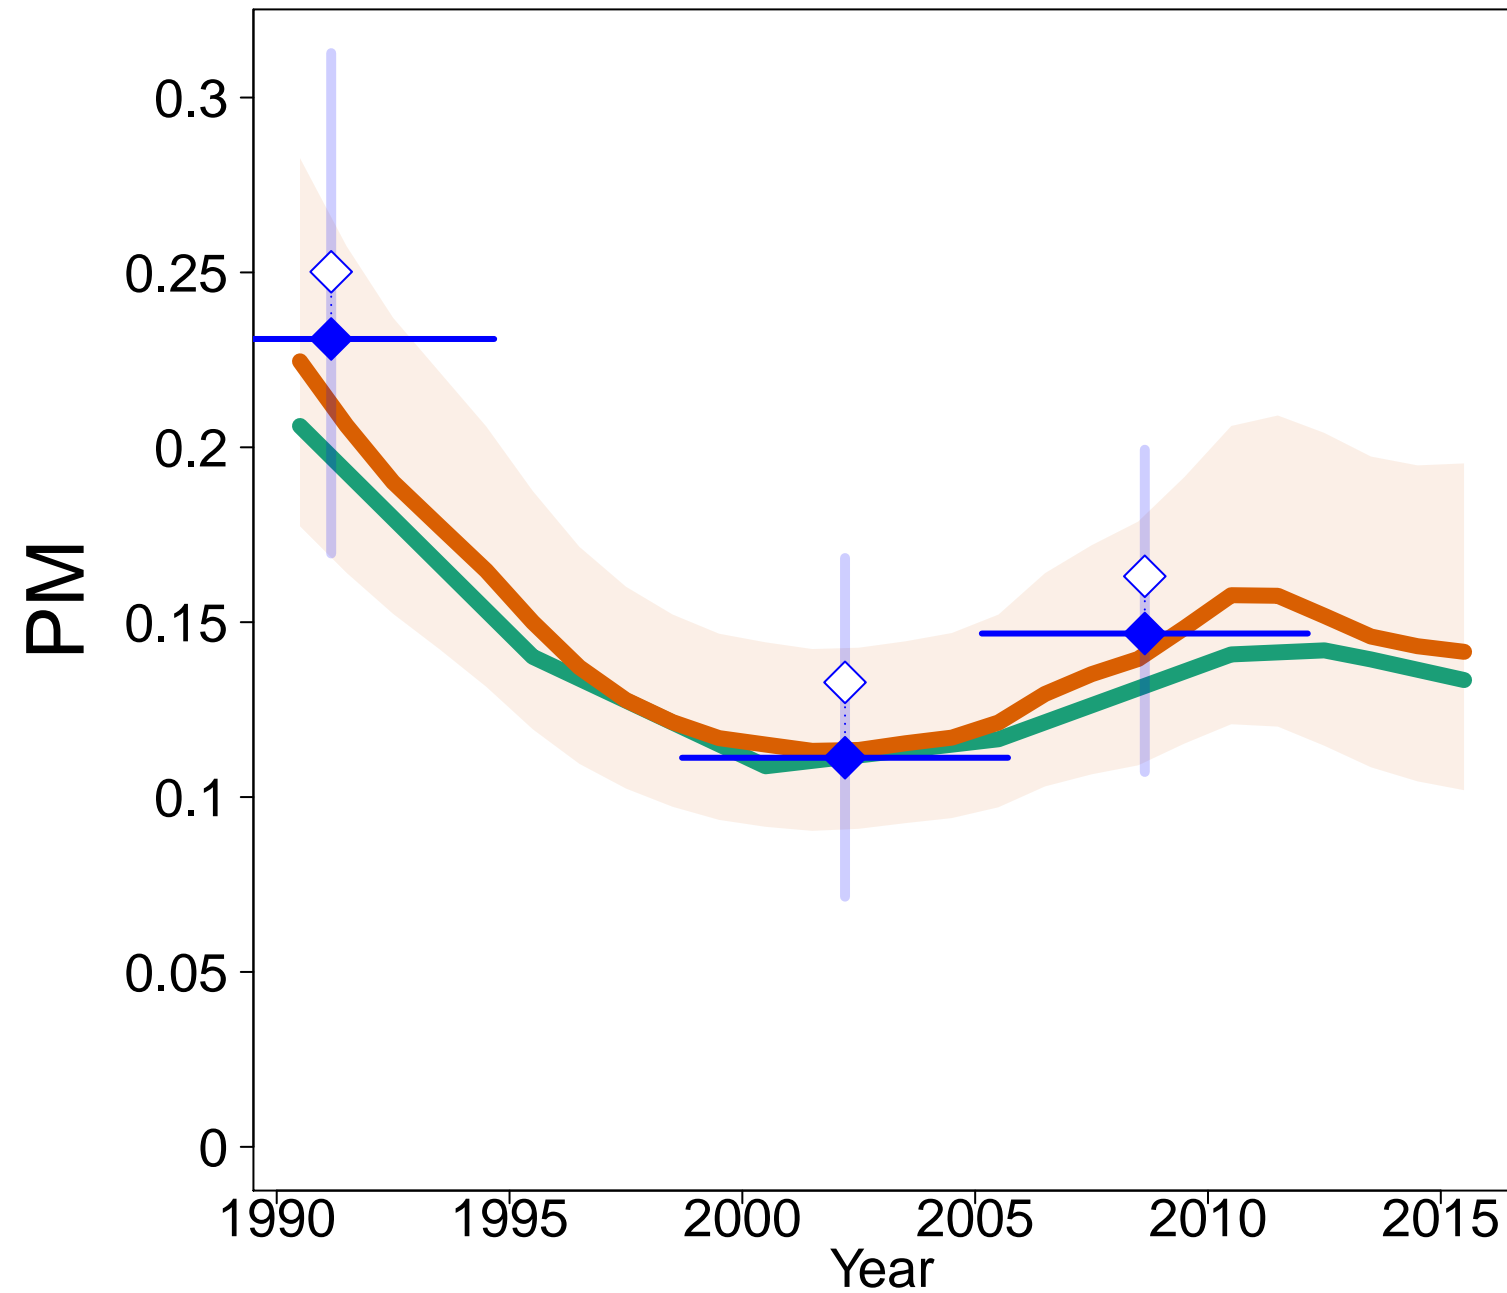

Cote d'Ivoire [CIV; B]  
(Western Africa)

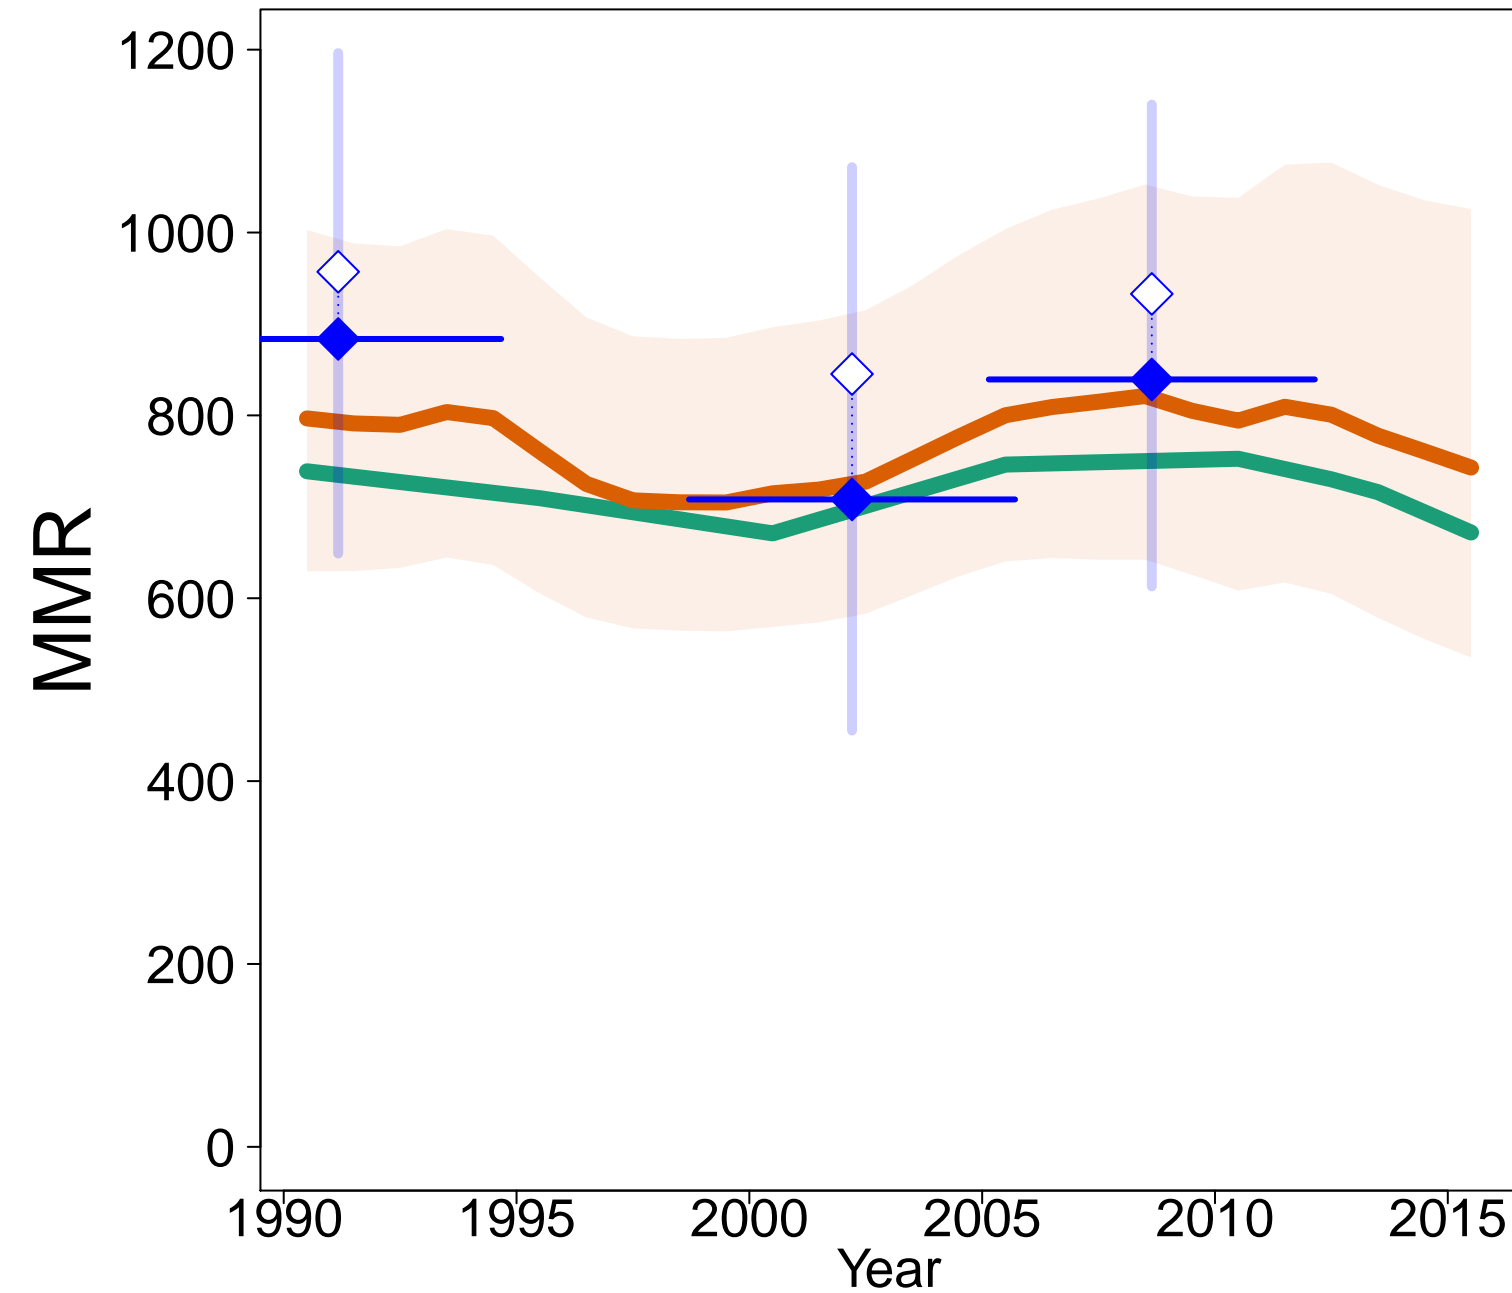

– Estimates –  
Bmat 2014  
MMEIG 2014  
– Data –  
Observed Data  
Adjusted Data  
– Data type –  
DHS

Croatia [HRV; A]  
(Transition countries of South-Eastern Europe)

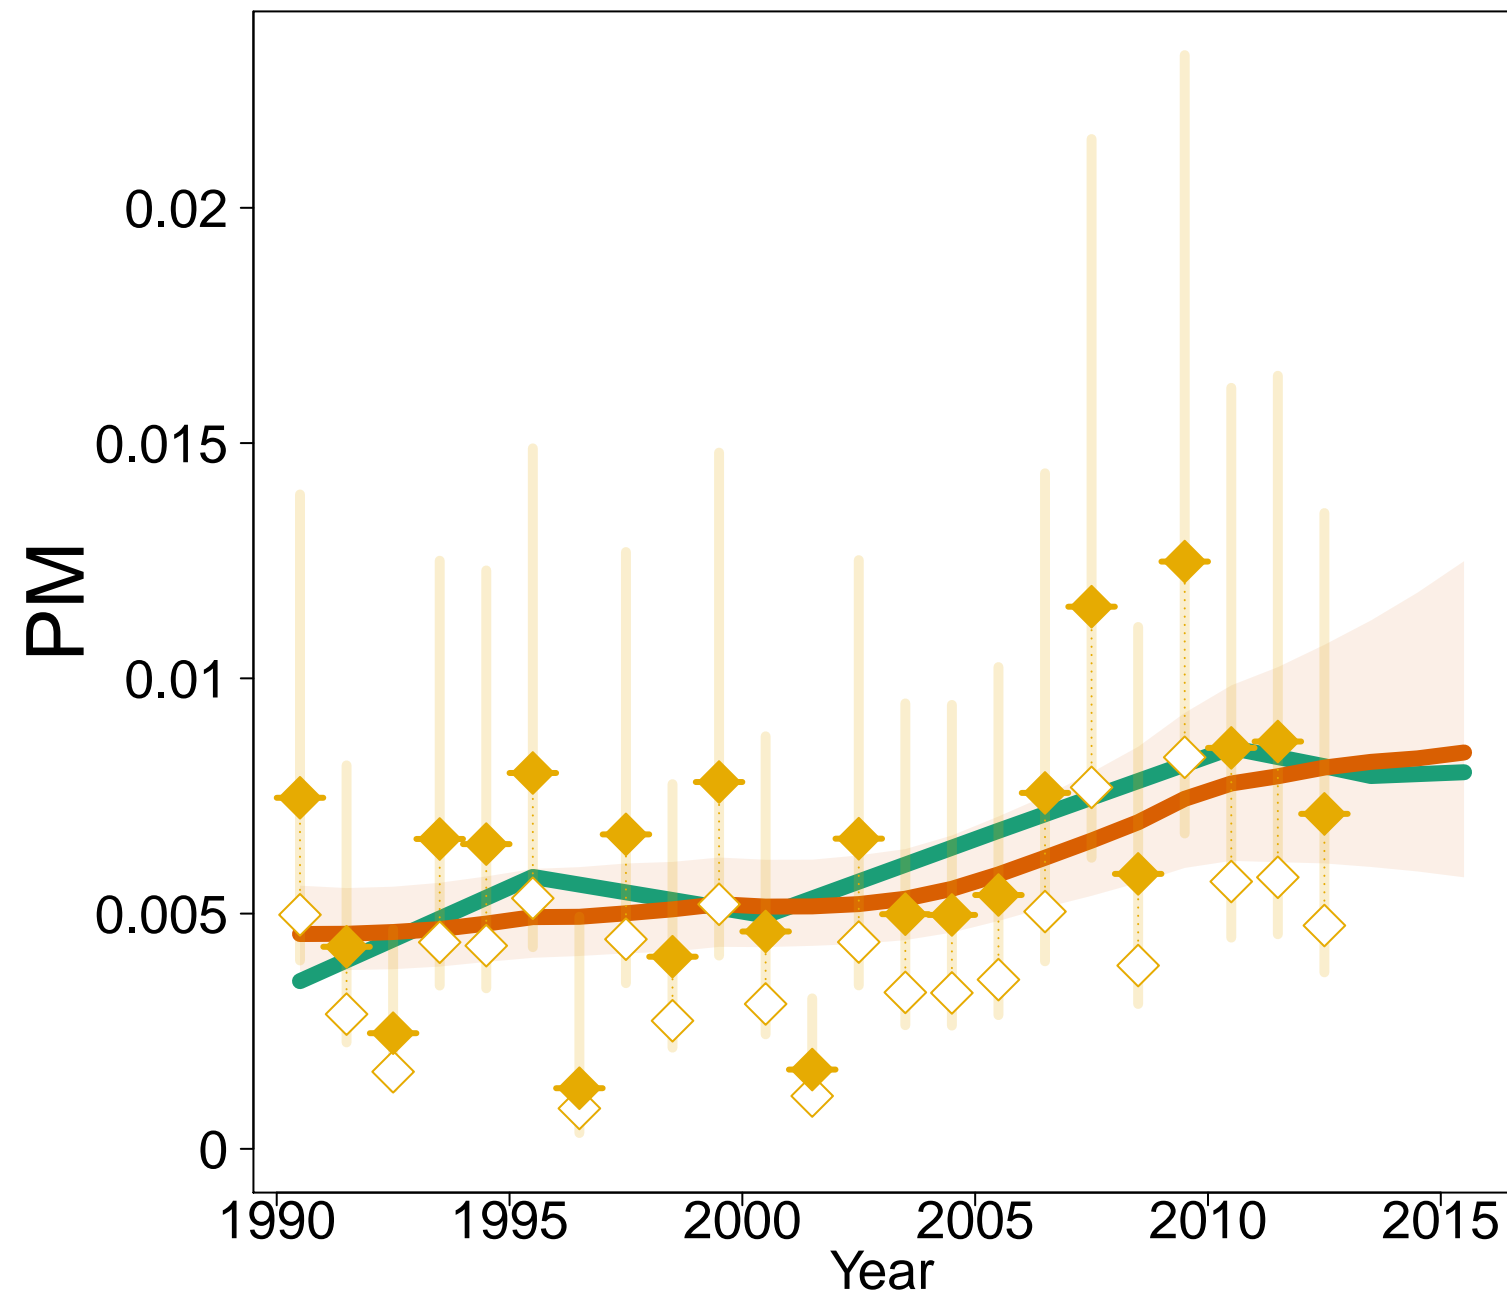

Croatia [HRV; A]  
(Transition countries of South-Eastern Europe)

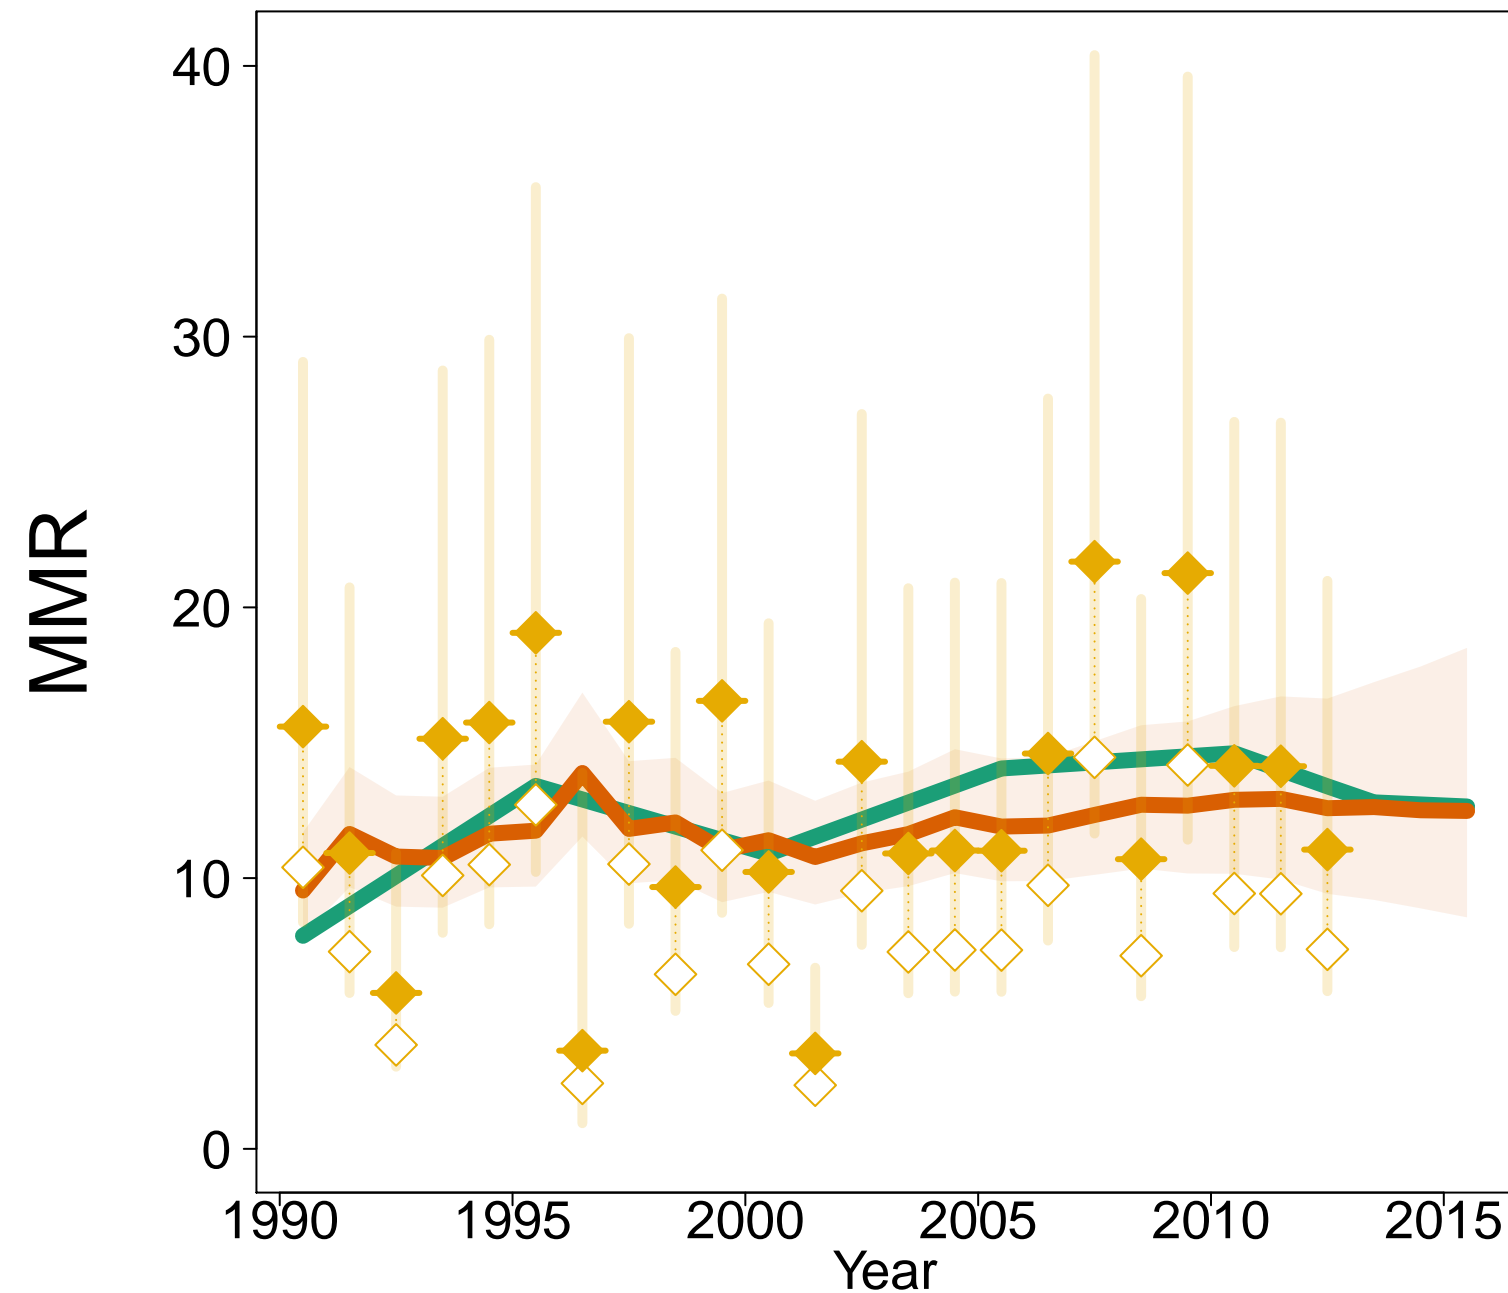

- Estimates –
- Bmat 2014
- MMEIG 2014
- Data –
- Observed Data
- Adjusted Data
- Data type –
- VR



Cuba [CUB; A]  
(Caribbean)

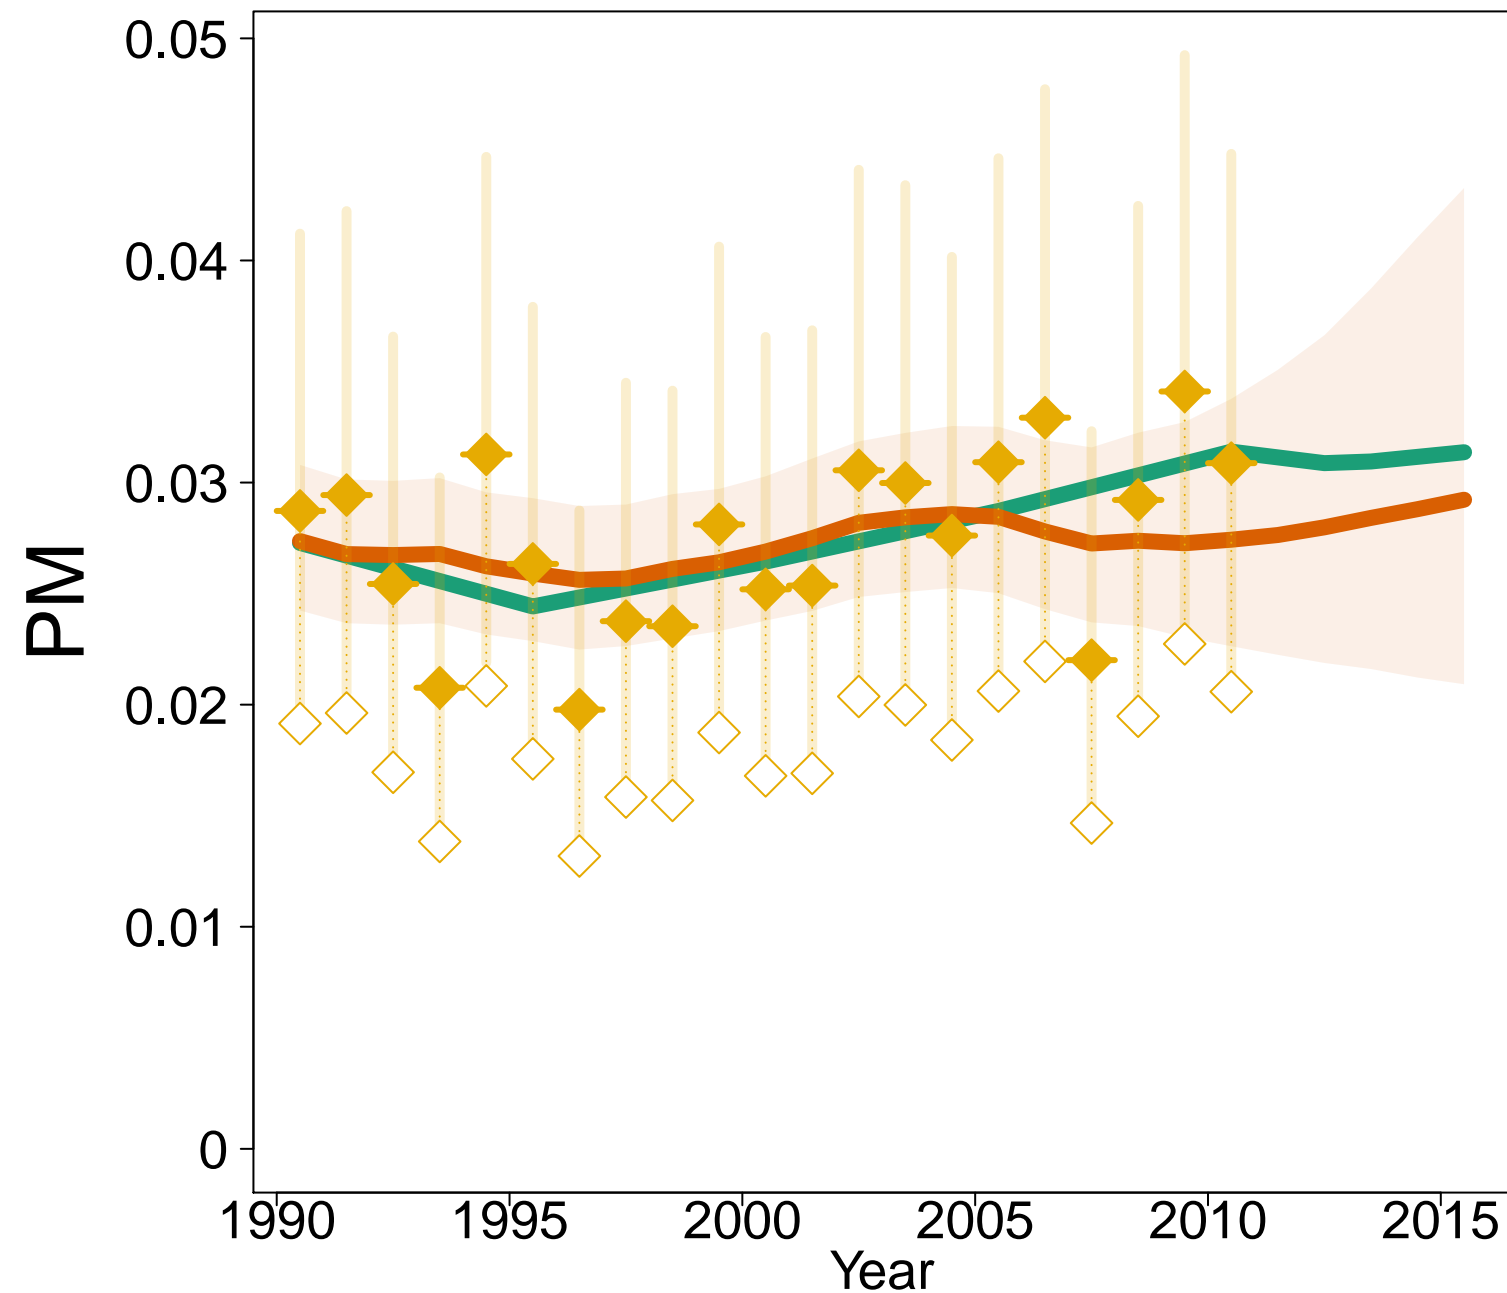

Cuba [CUB; A]  
(Caribbean)

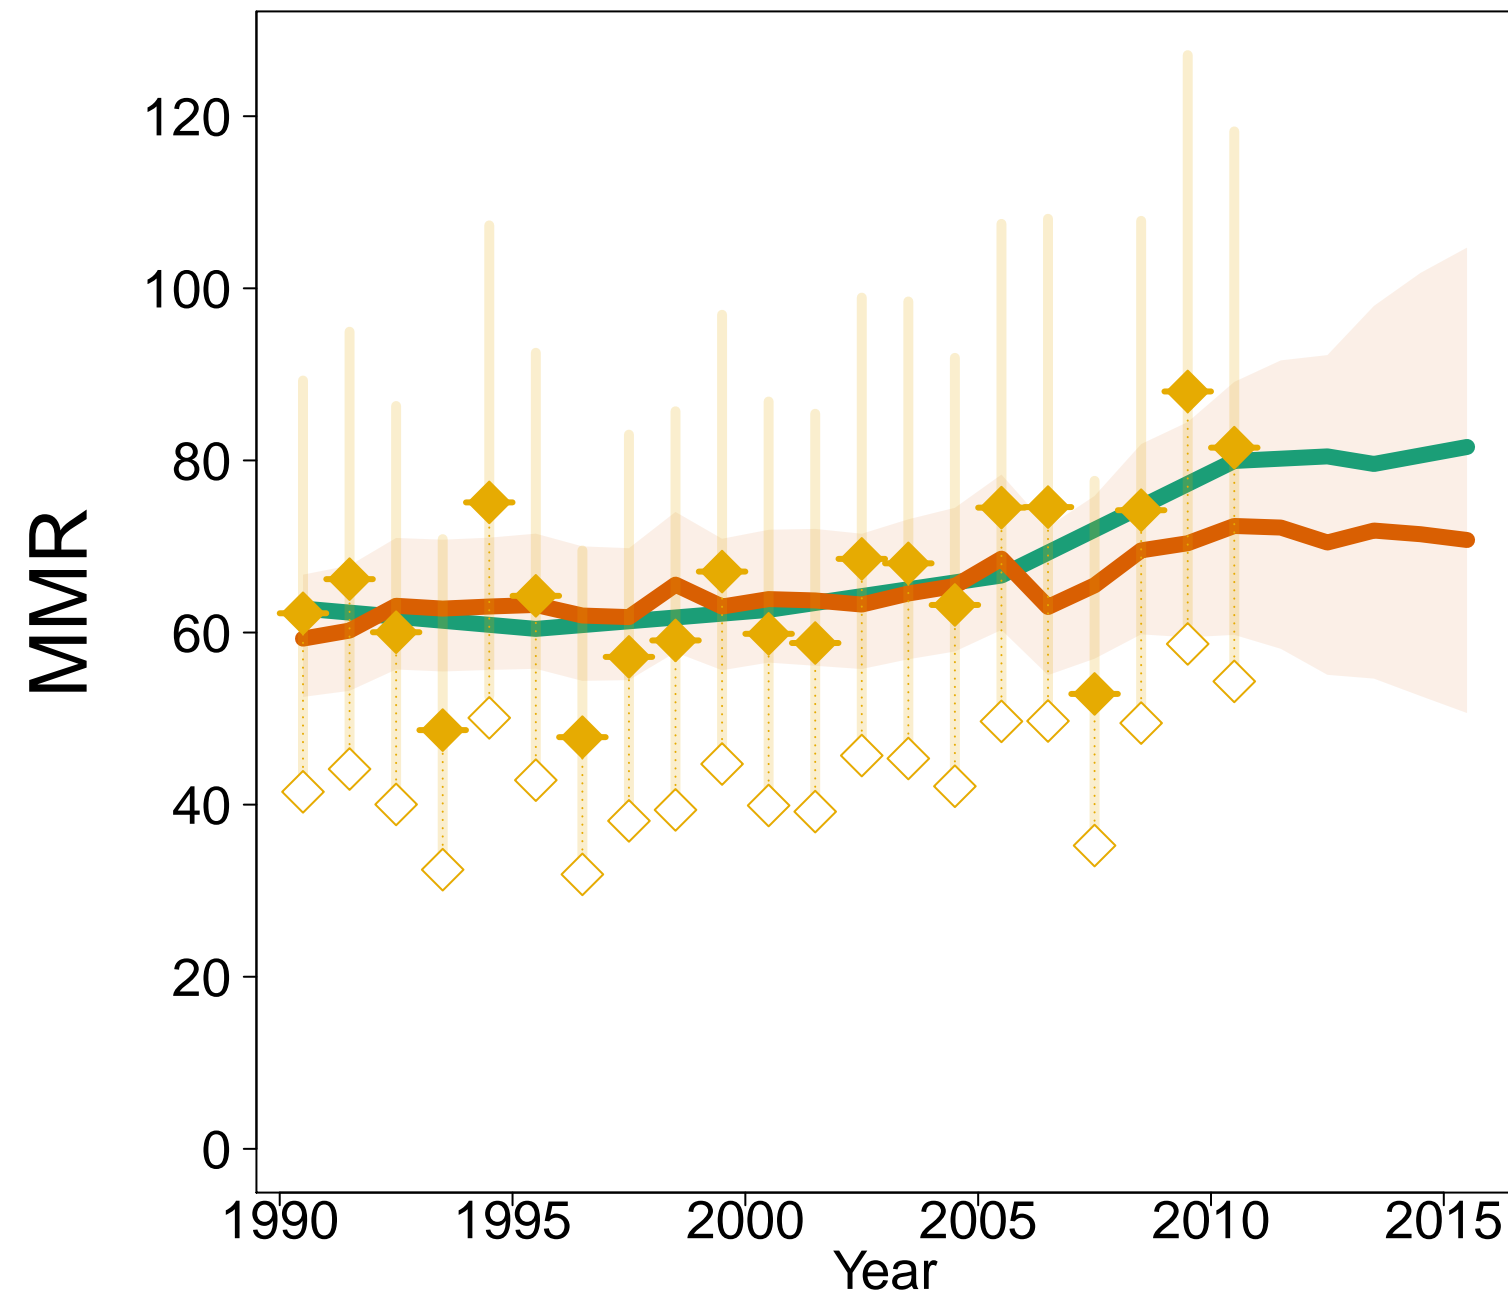

- Estimates –
- Bmat 2014
- MMEIG 2014
- Data –
- Observed Data
- Adjusted Data
- Data type –
- VR

Cyprus [CYP; C]  
(Western Asia)

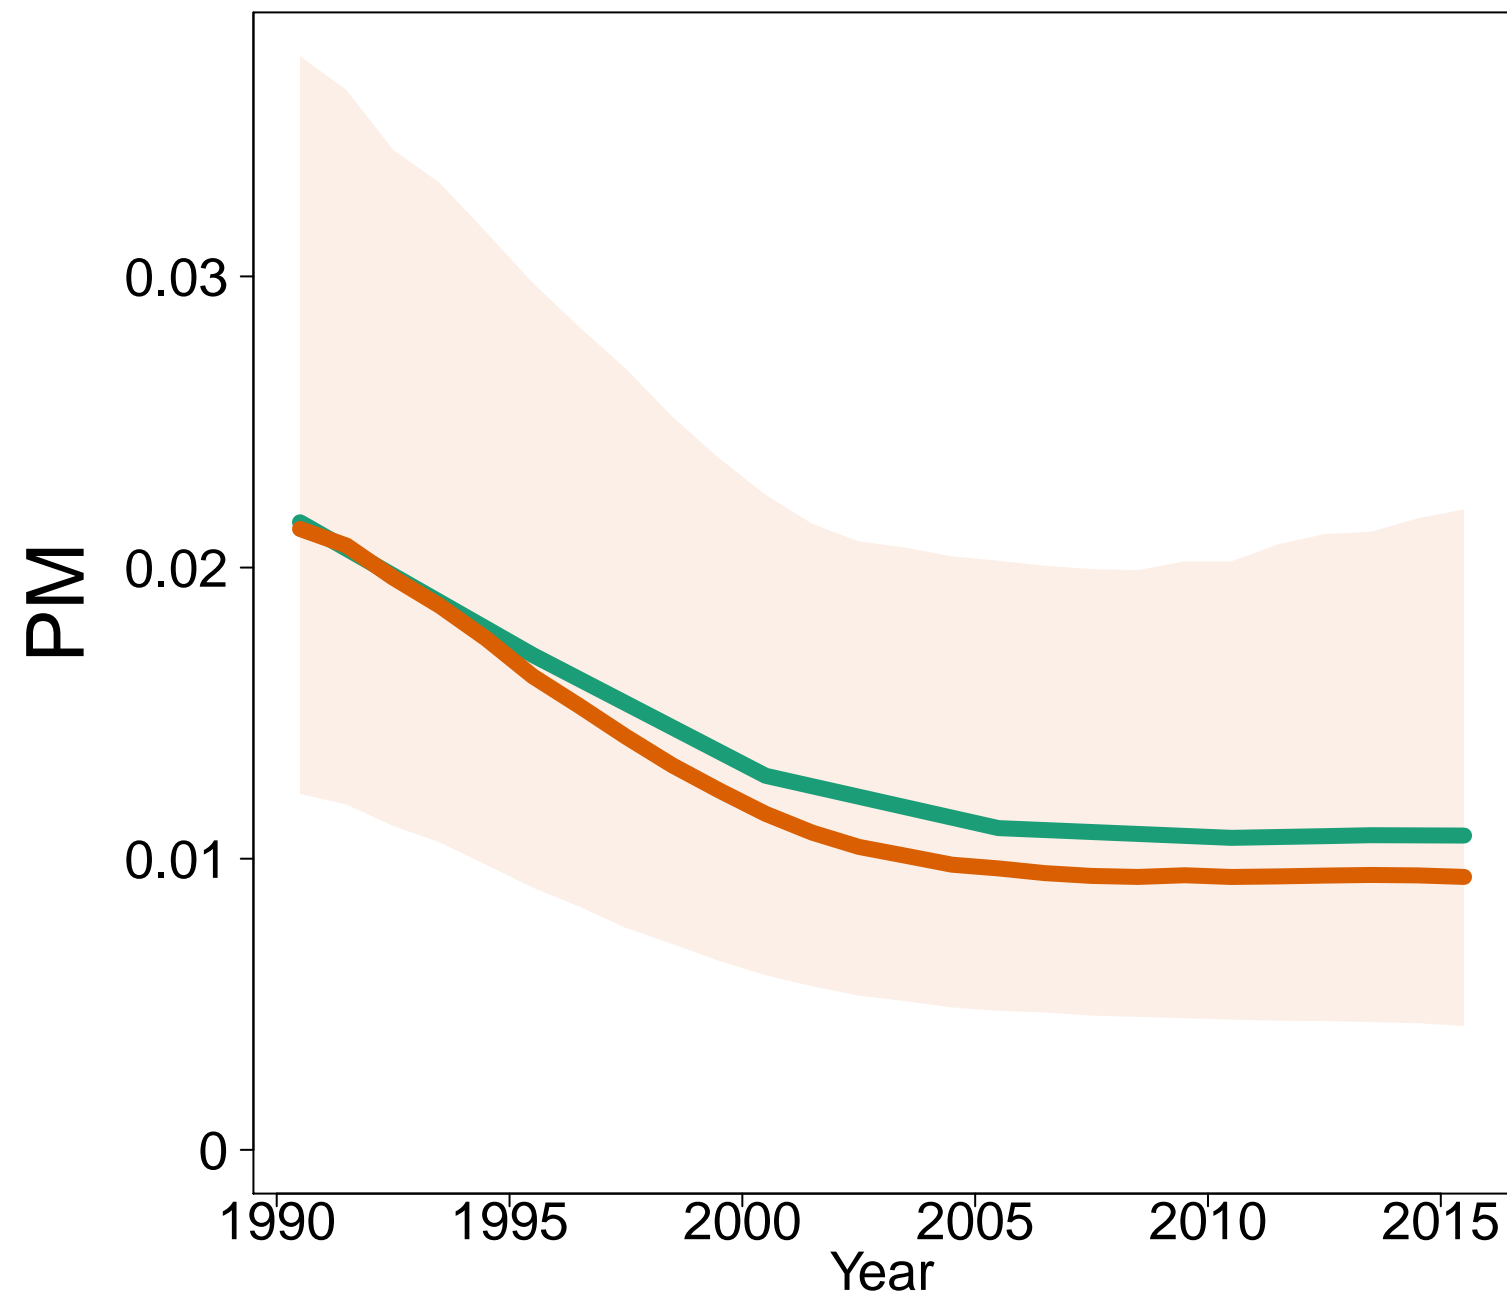

Cyprus [CYP; C]  
(Western Asia)

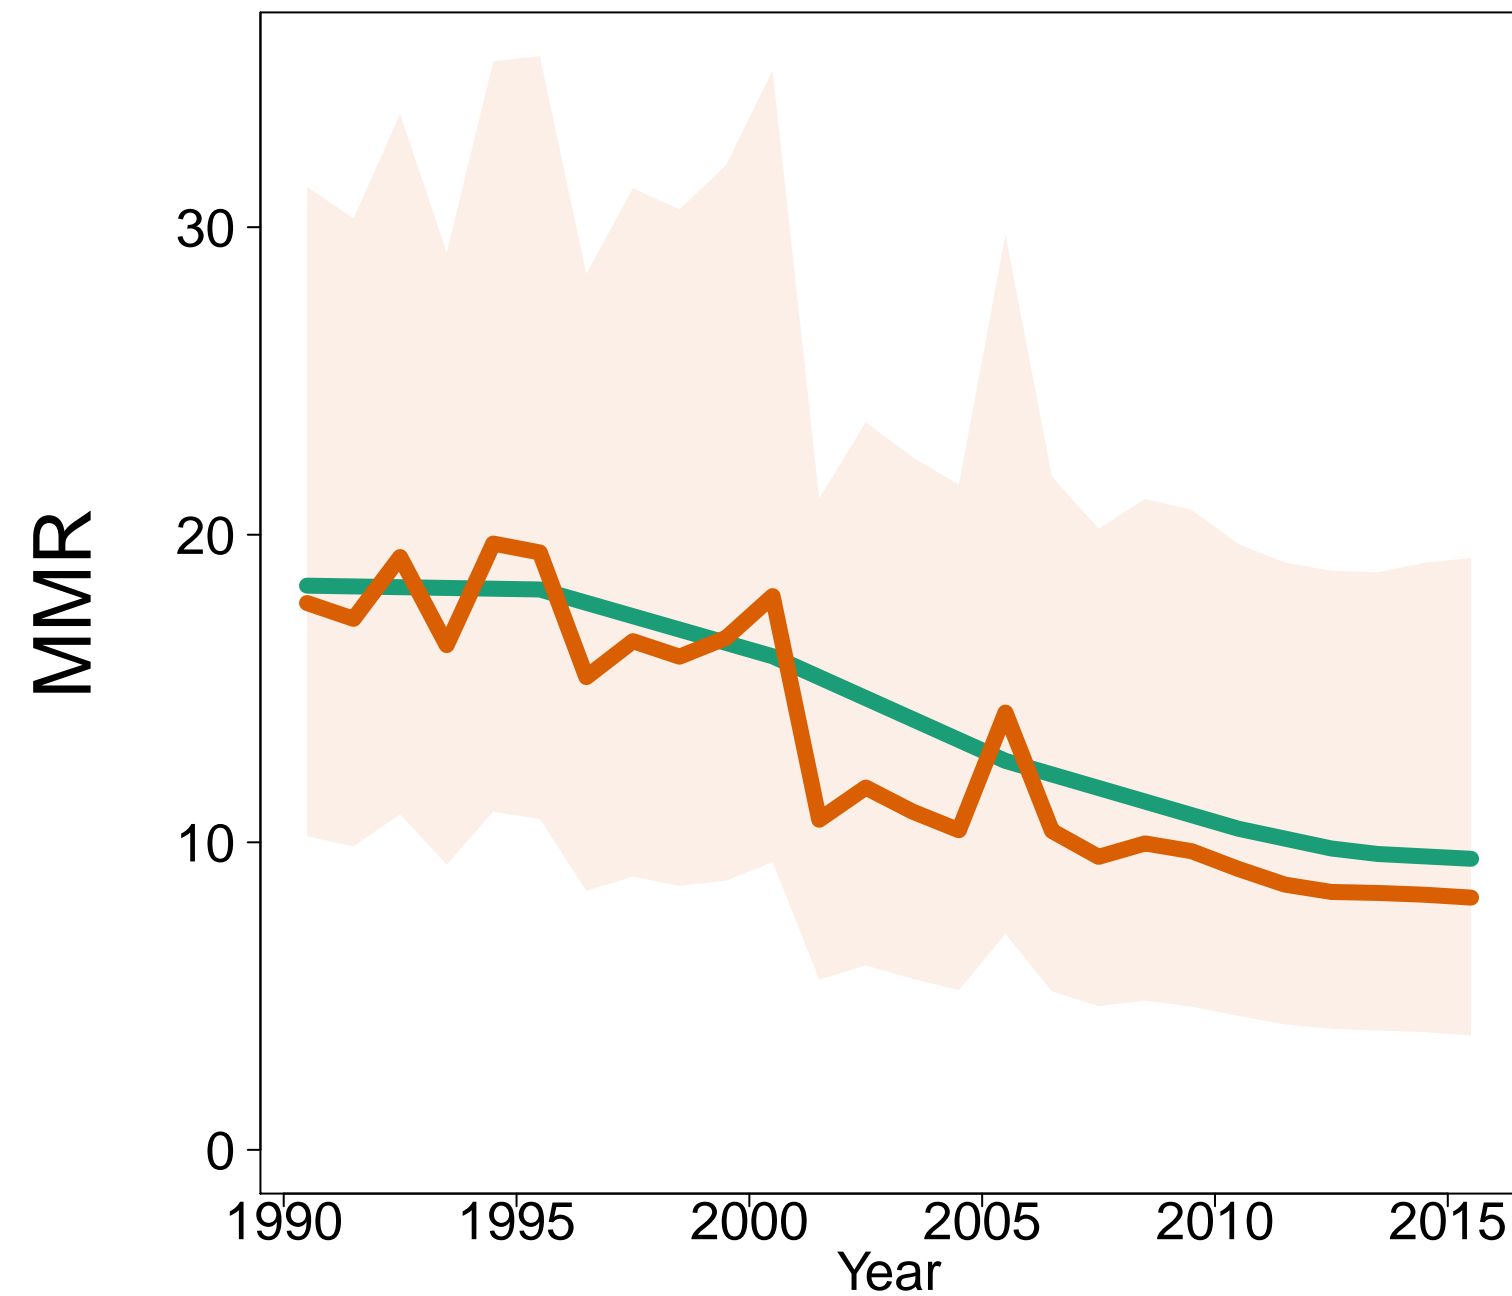

- Estimates –
- Bmat 2014
- MMEIG 2014
- Data –
- ◊ Observed Data
- ◆ Adjusted Data
- Data type –

Czech Republic [CZE; A]  
(Developed regions)

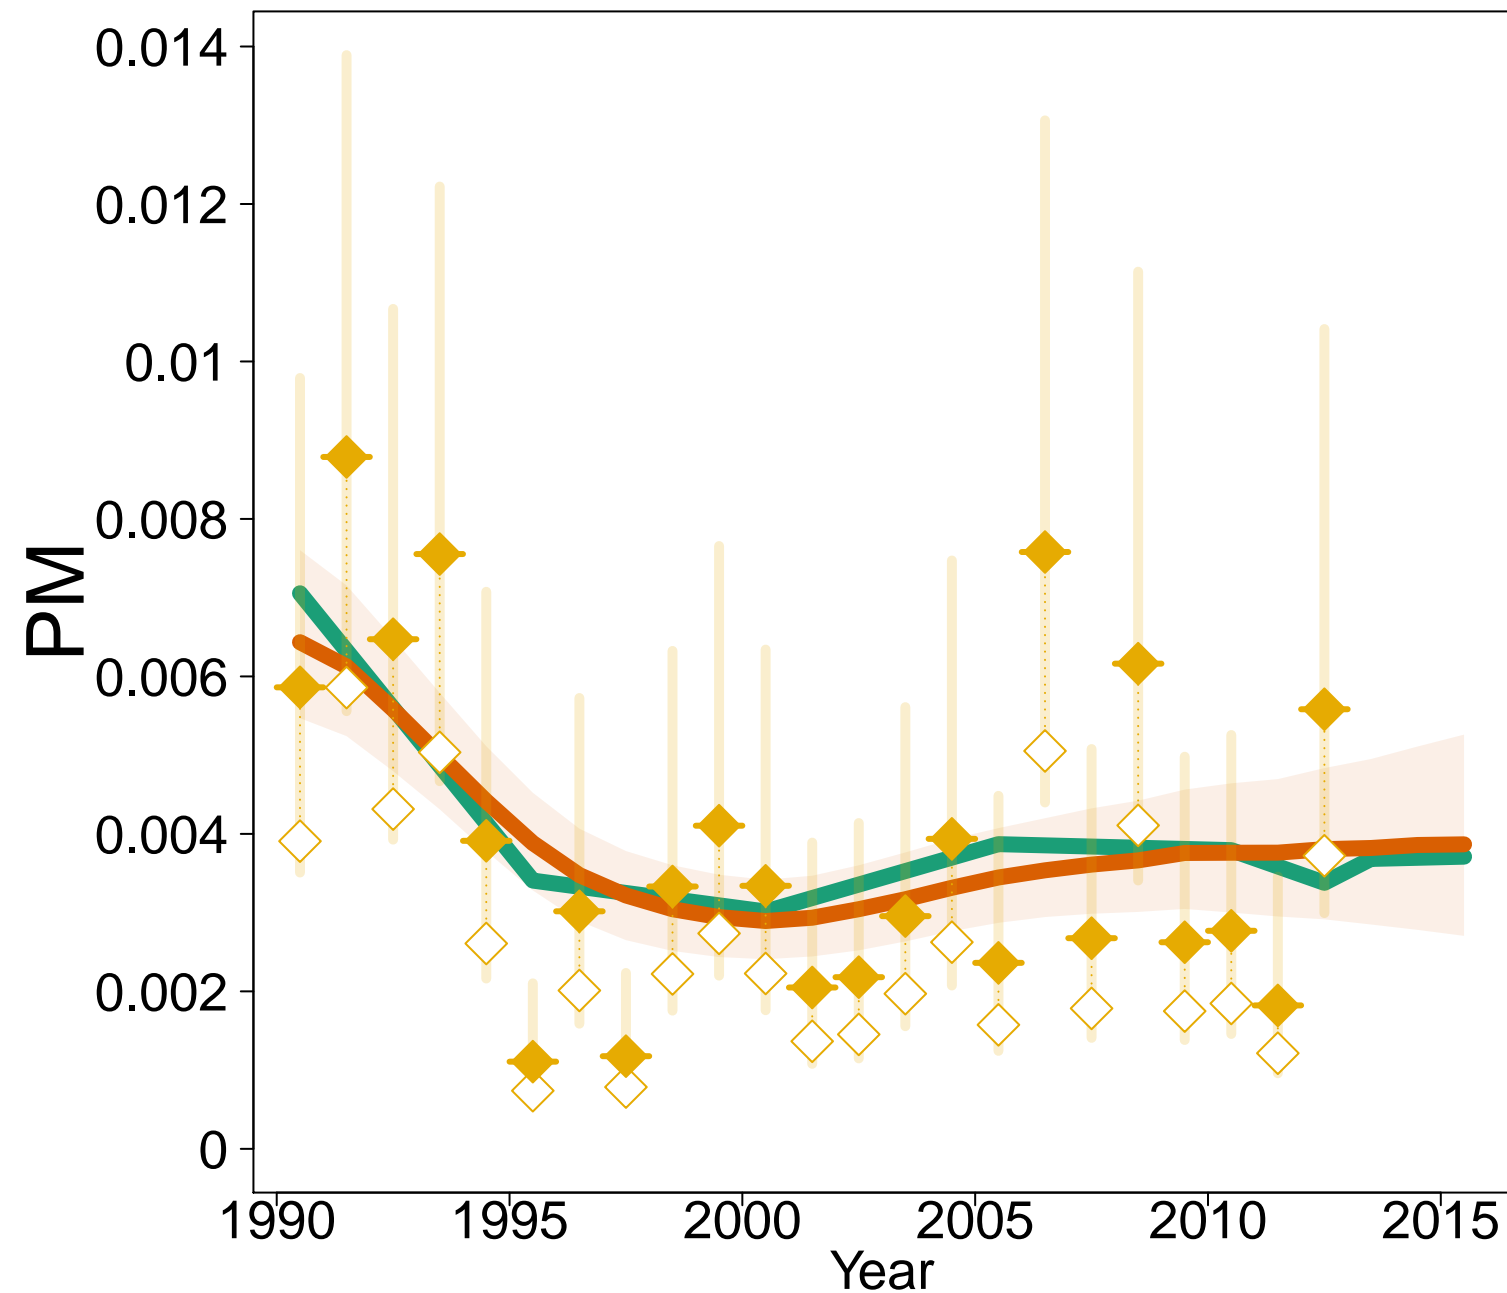

Czech Republic [CZE; A]  
(Developed regions)

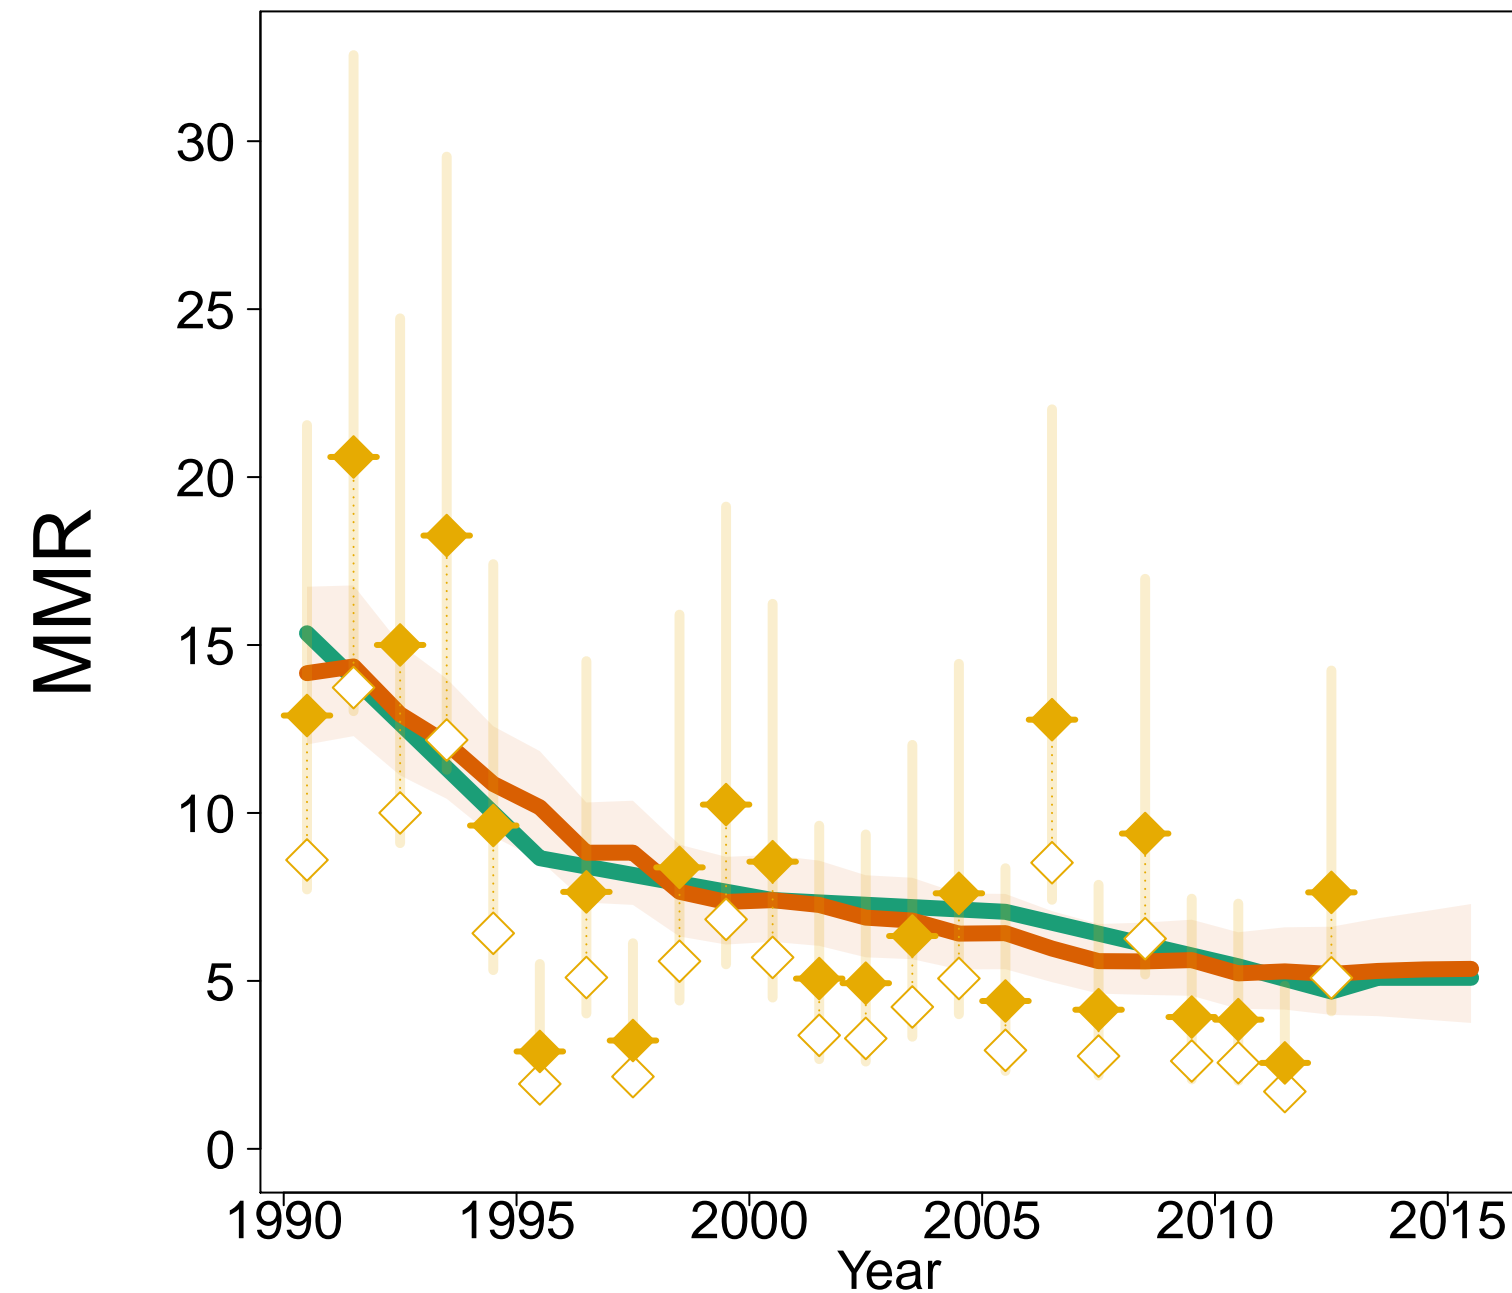

- Estimates –
- Bmat 2014
- MMEIG 2014
- Data –
- Observed Data
- Adjusted Data
- Data type –
- VR

Democratic People's Republic of Korea [PRK; C]  
(Eastern Asia)

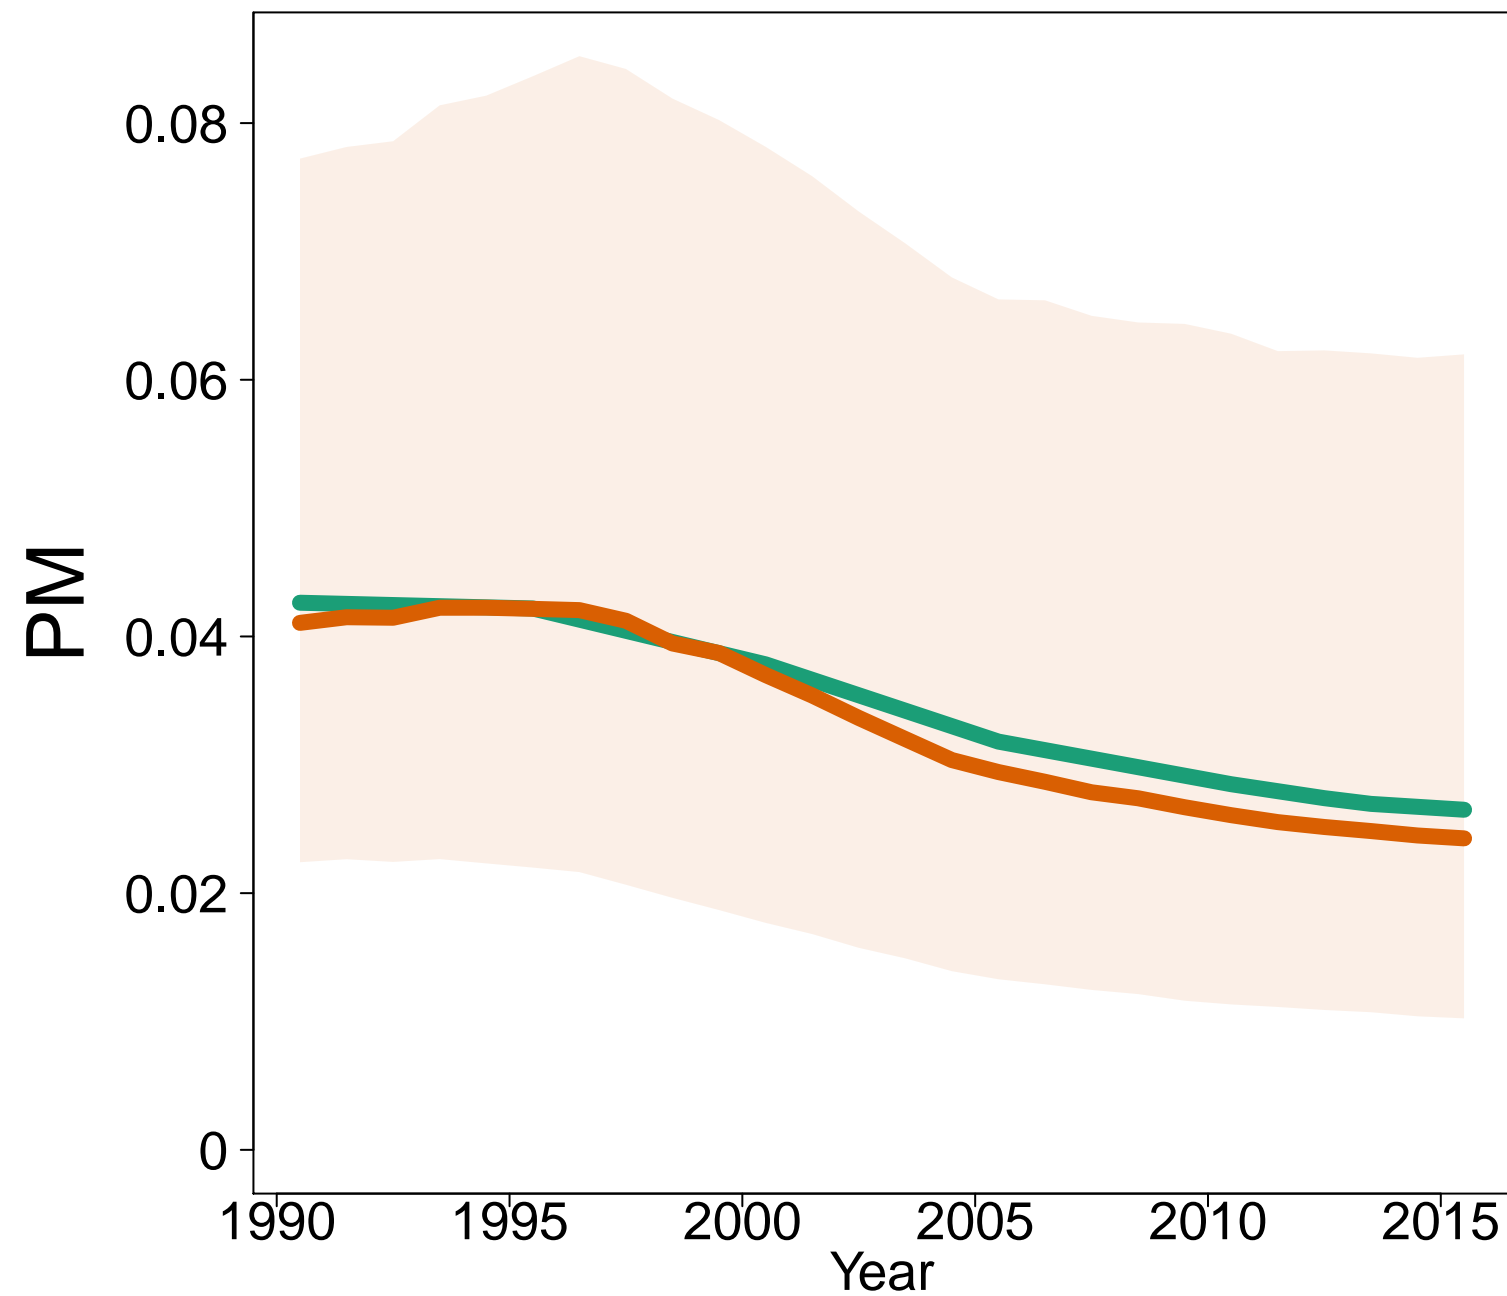

Democratic People's Republic of Korea [PRK; C]  
(Eastern Asia)

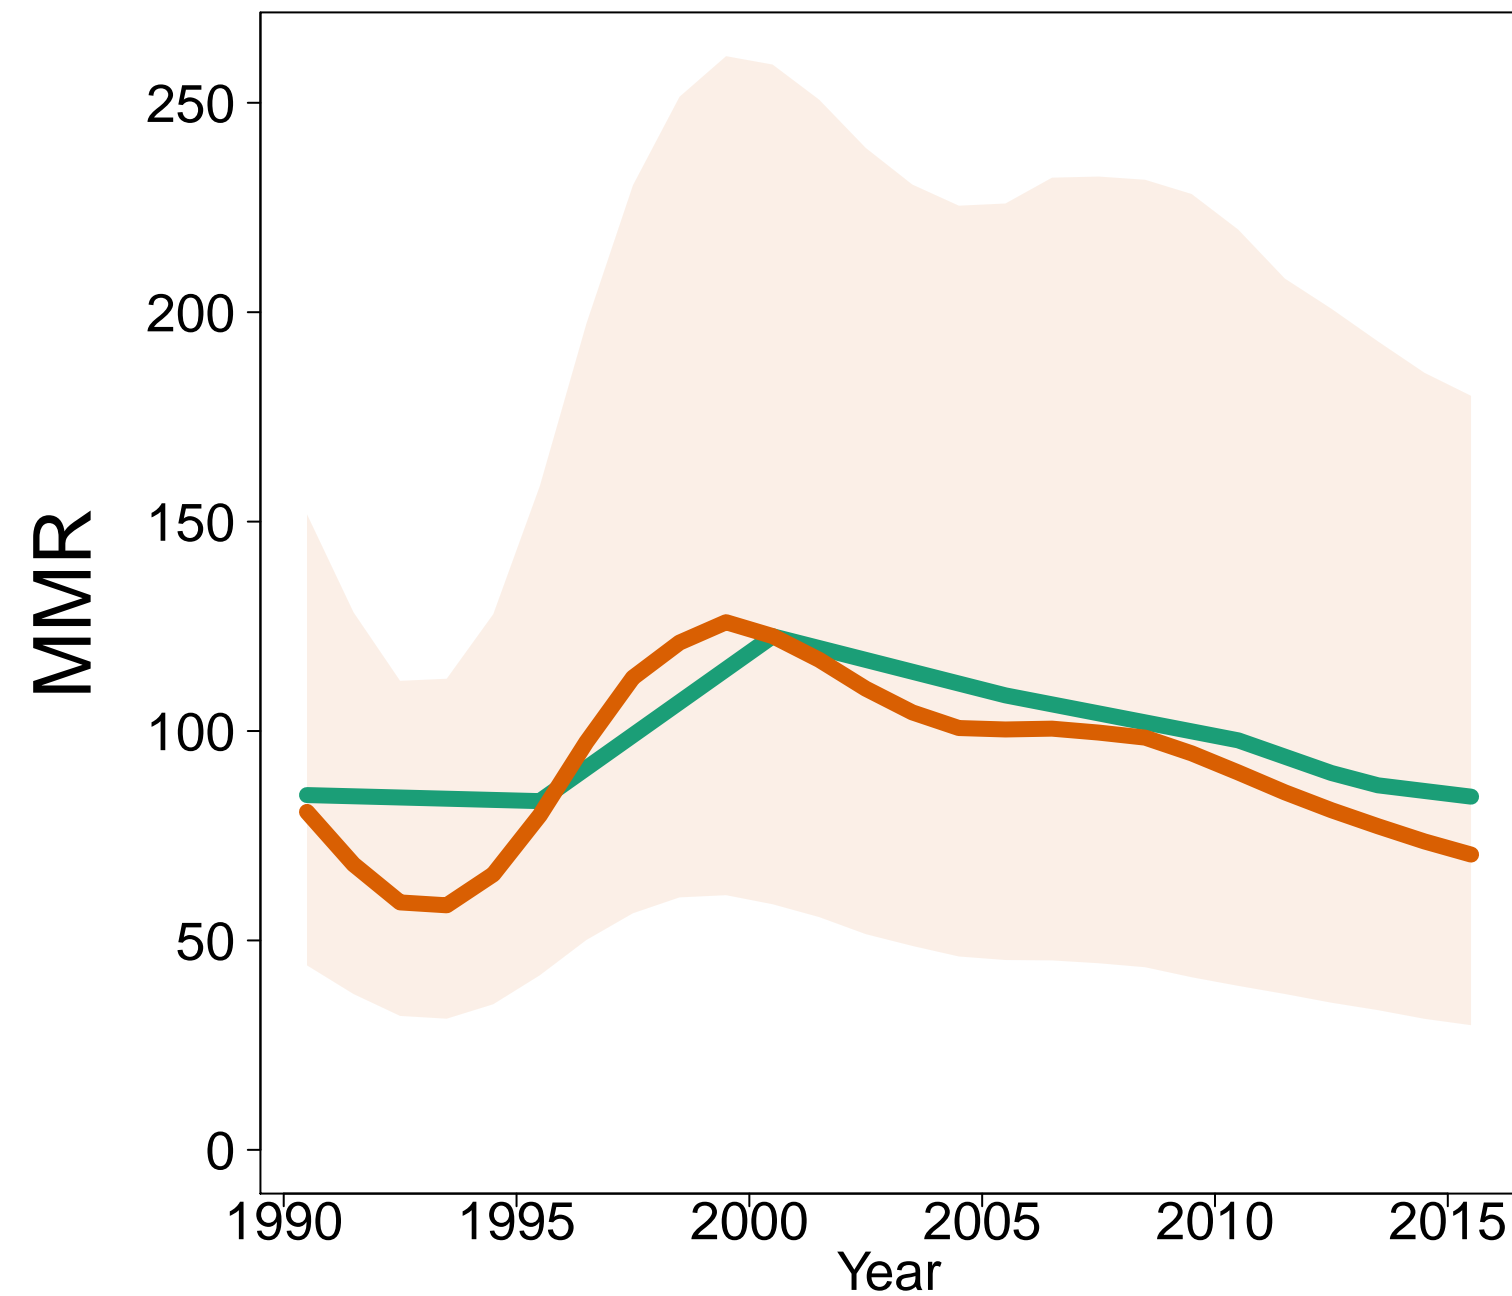

– Estimates –  
Bmat 2014  
MMEIG 2014  
– Data –

Democratic Republic of the Congo [COD; B]  
(Middle Africa)

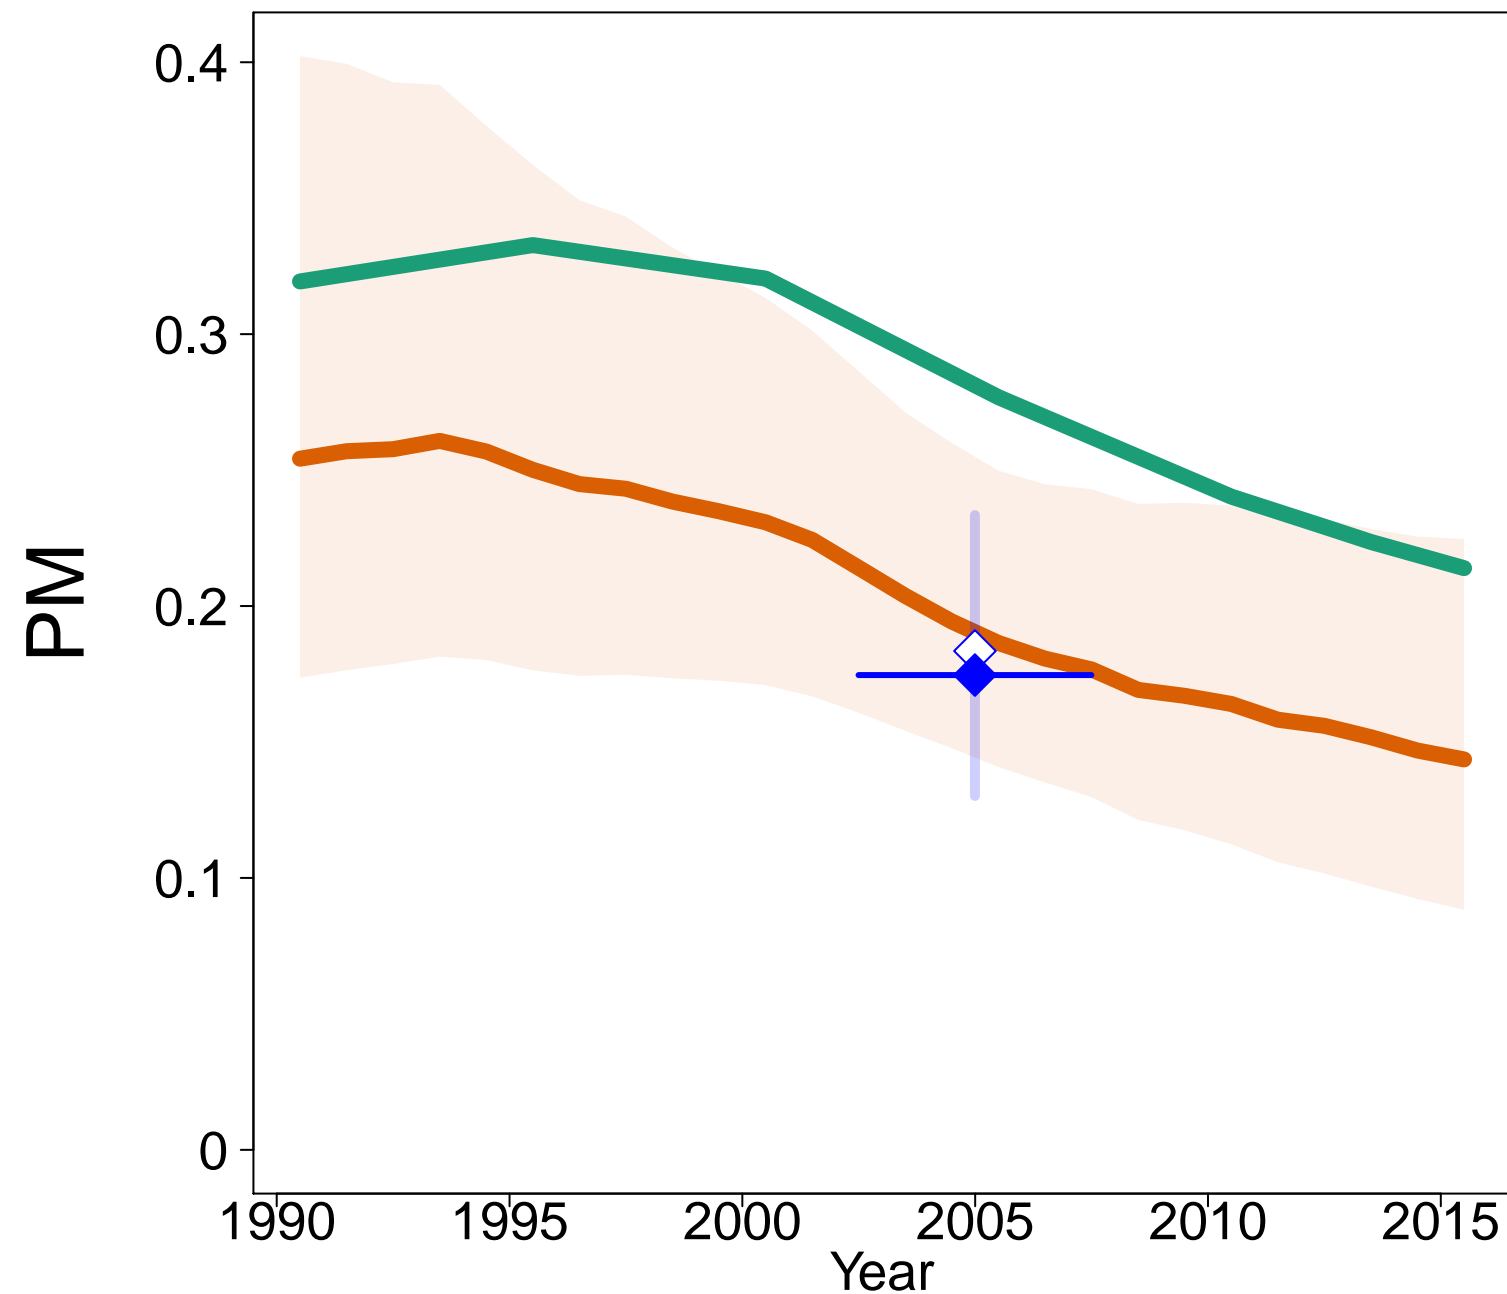

Democratic Republic of the Congo [COD; B]  
(Middle Africa)

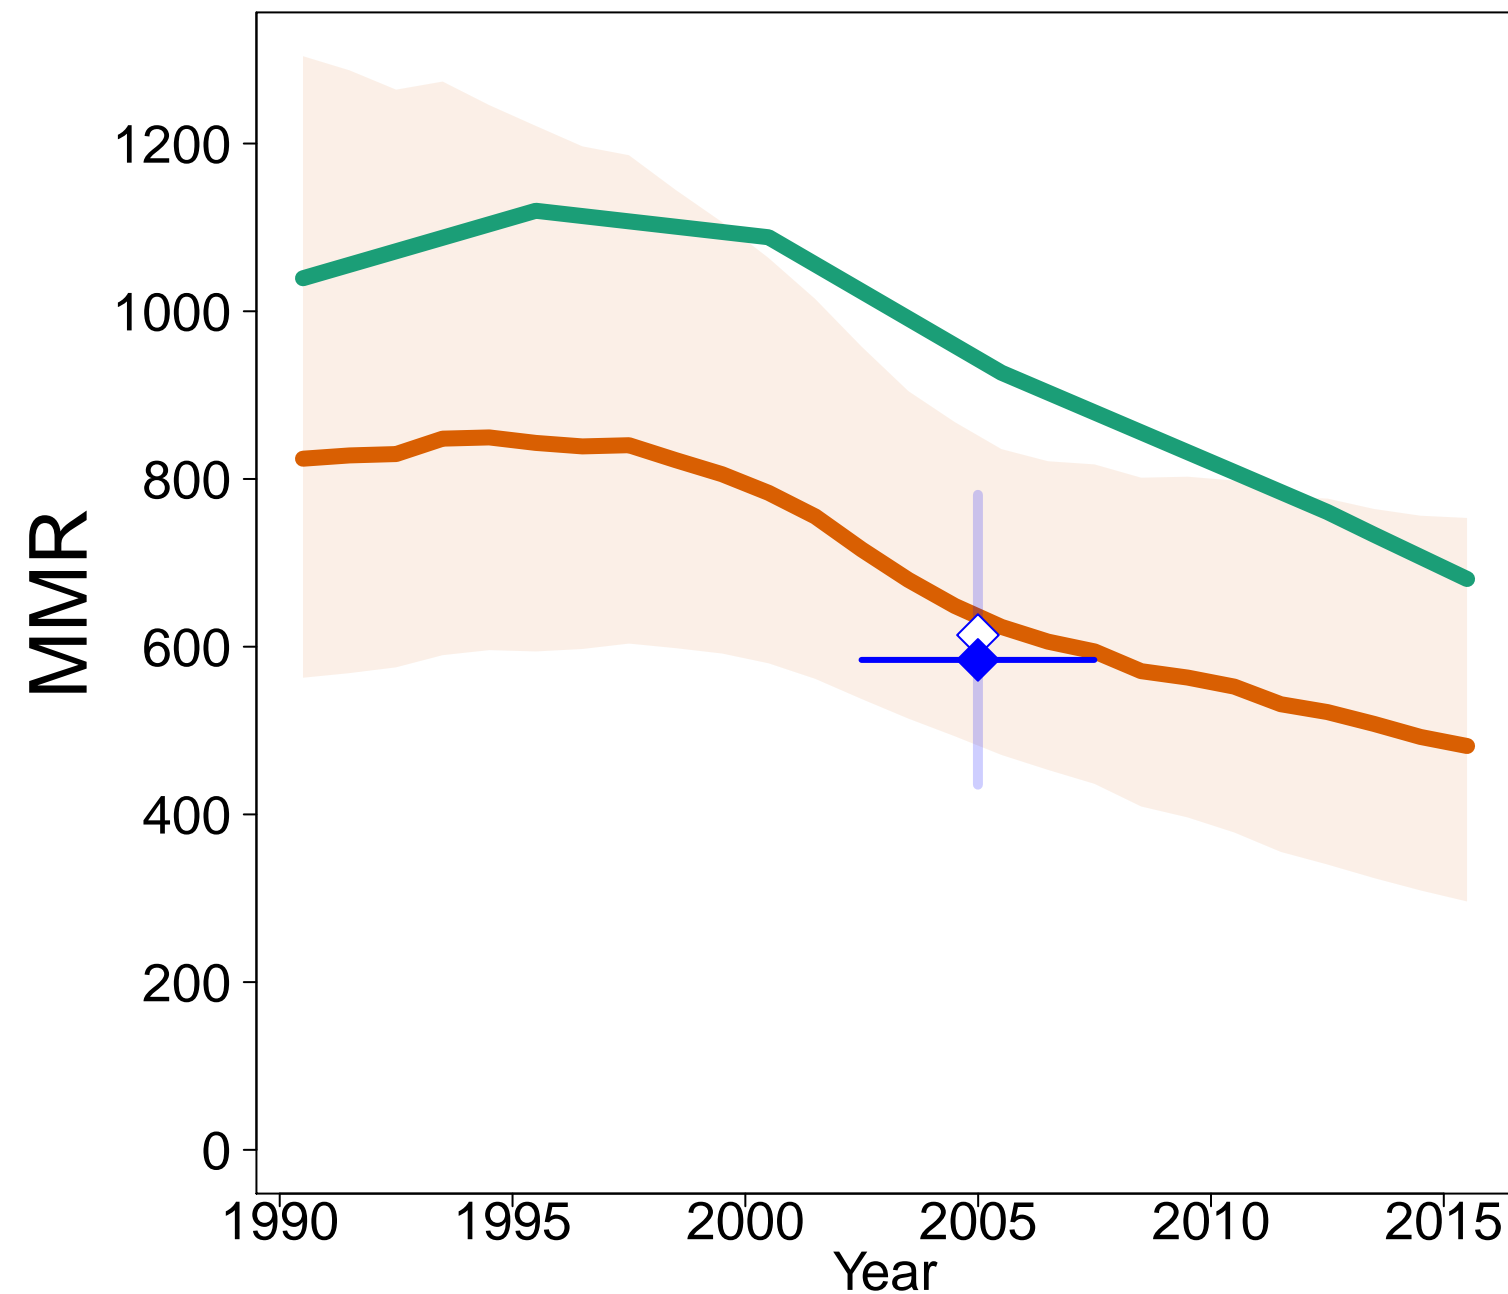

– Estimates –  
Bmat 2014  
MMEIG 2014  
– Data –  
Observed Data  
Adjusted Data  
– Data type –  
DHS

Denmark [DNK; A]  
(Developed regions)

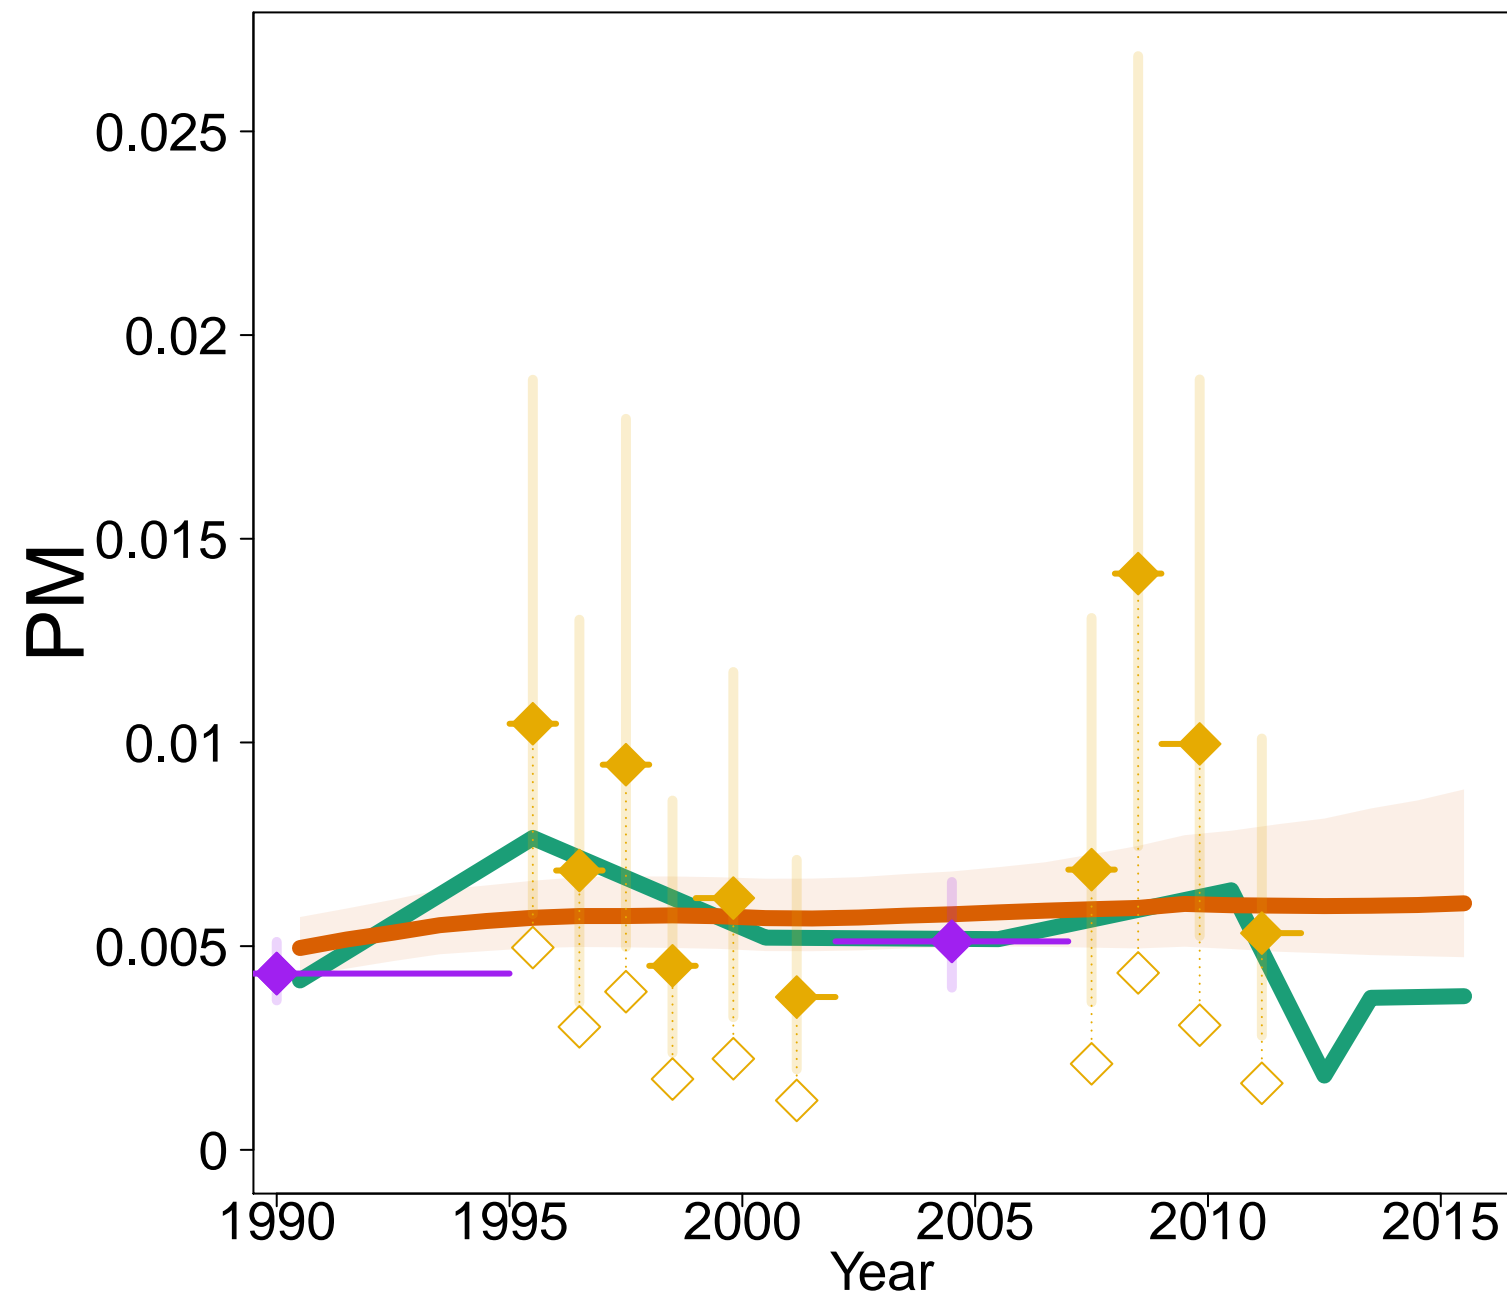

Denmark [DNK; A]  
(Developed regions)

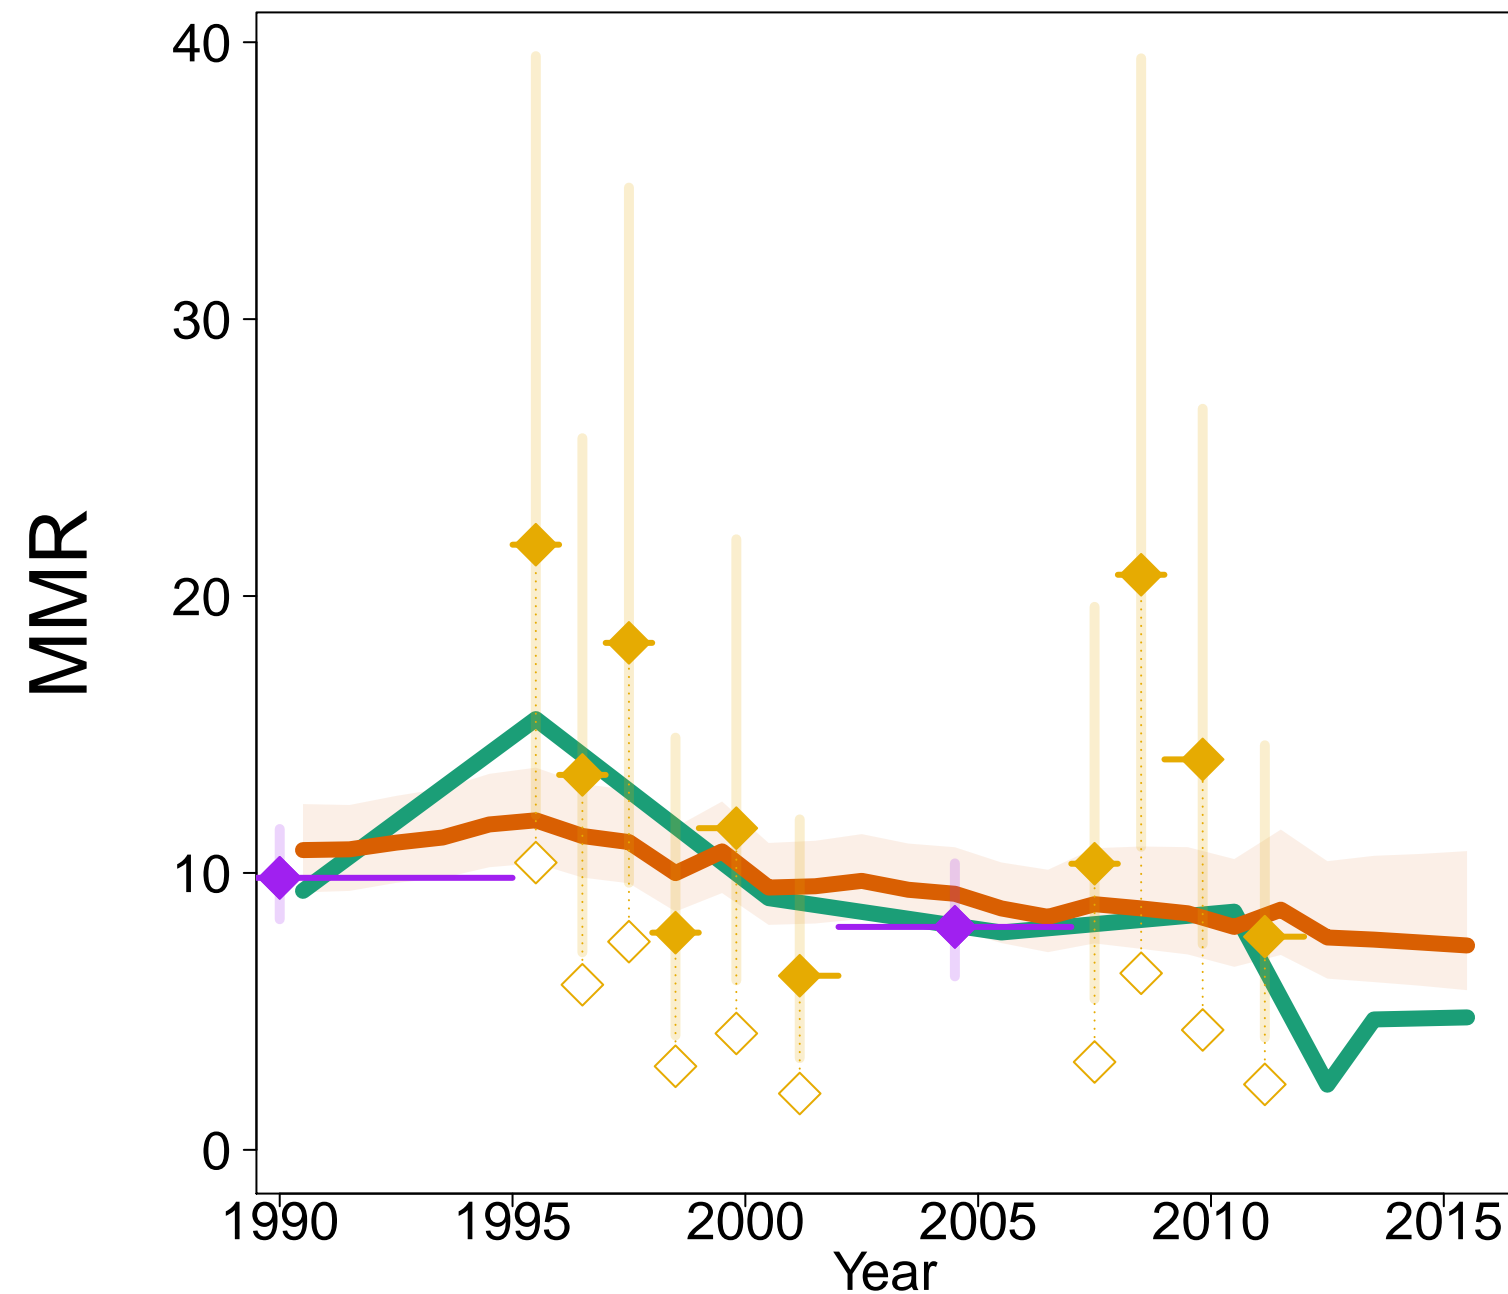

- Estimates –
- Bmat 2014
- MMEIG 2014
- Data –
- Observed Data
- Adjusted Data
- Data type –
- VR
- Spec. studies

Djibouti [DJI; C]  
(Eastern Africa)

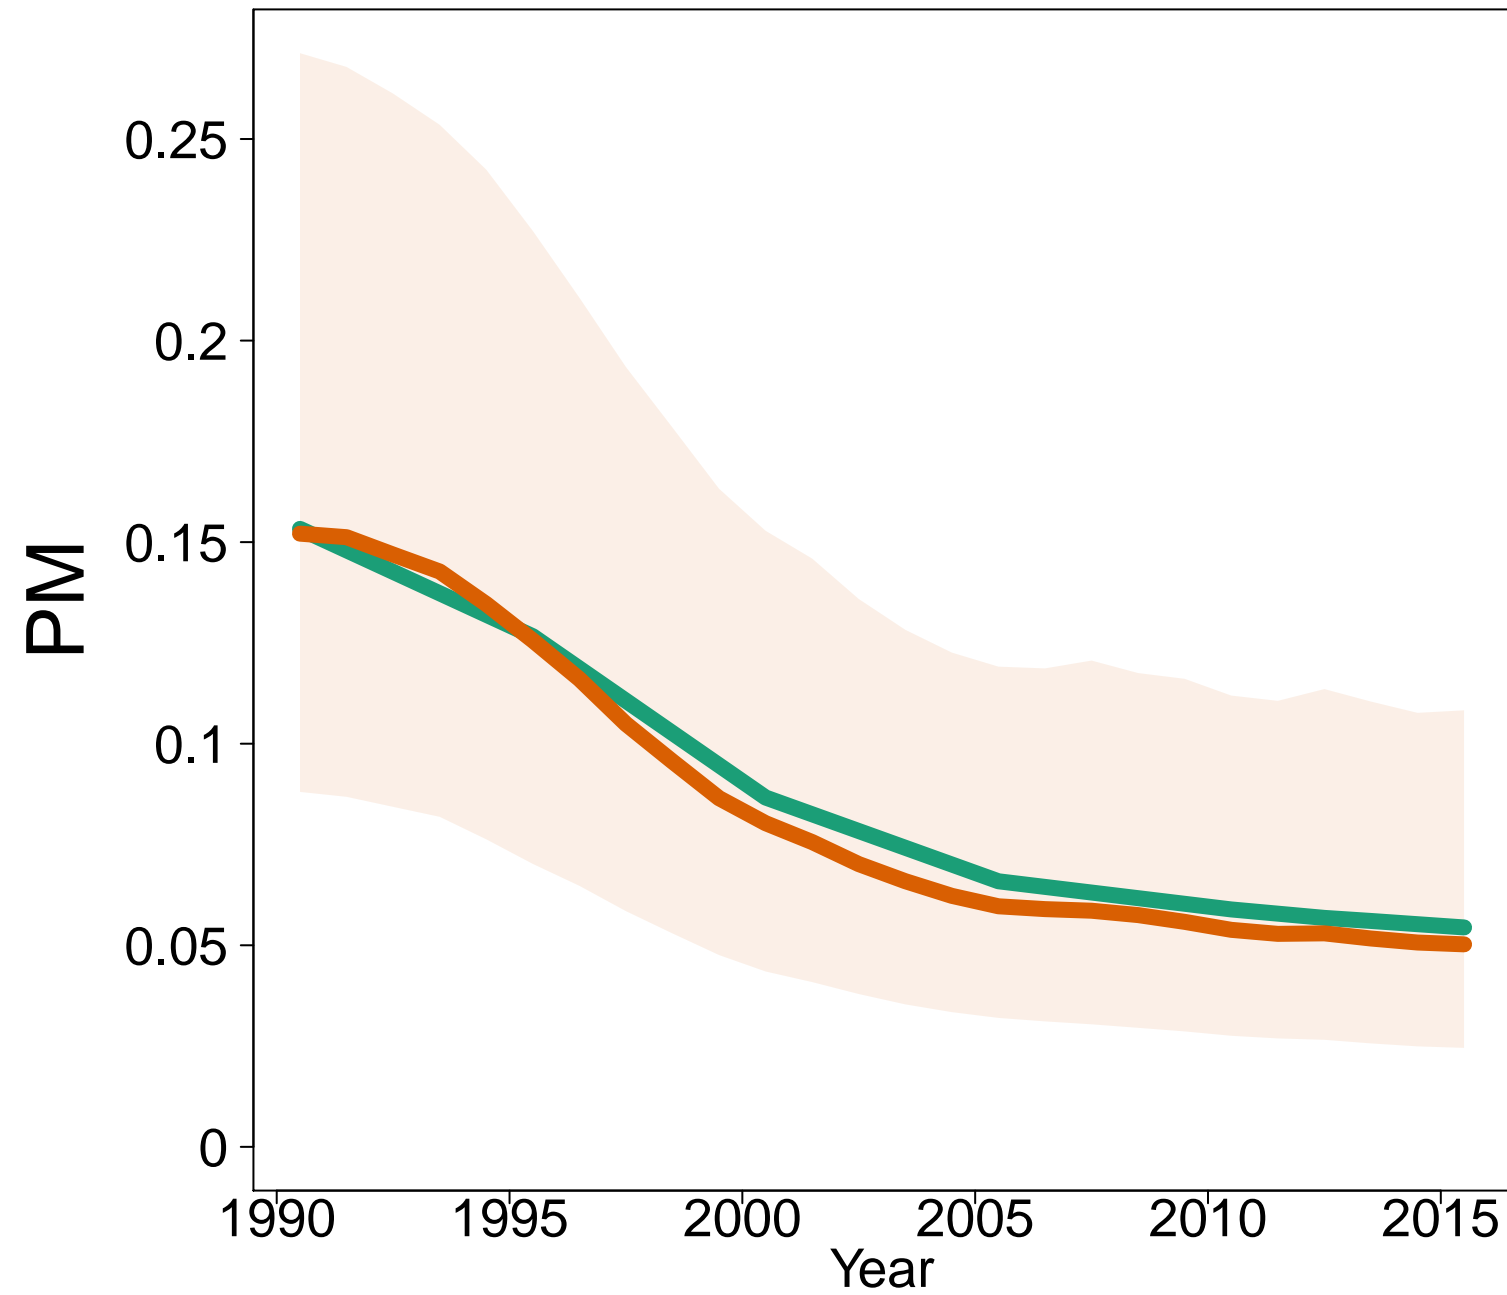

Djibouti [DJI; C]  
(Eastern Africa)

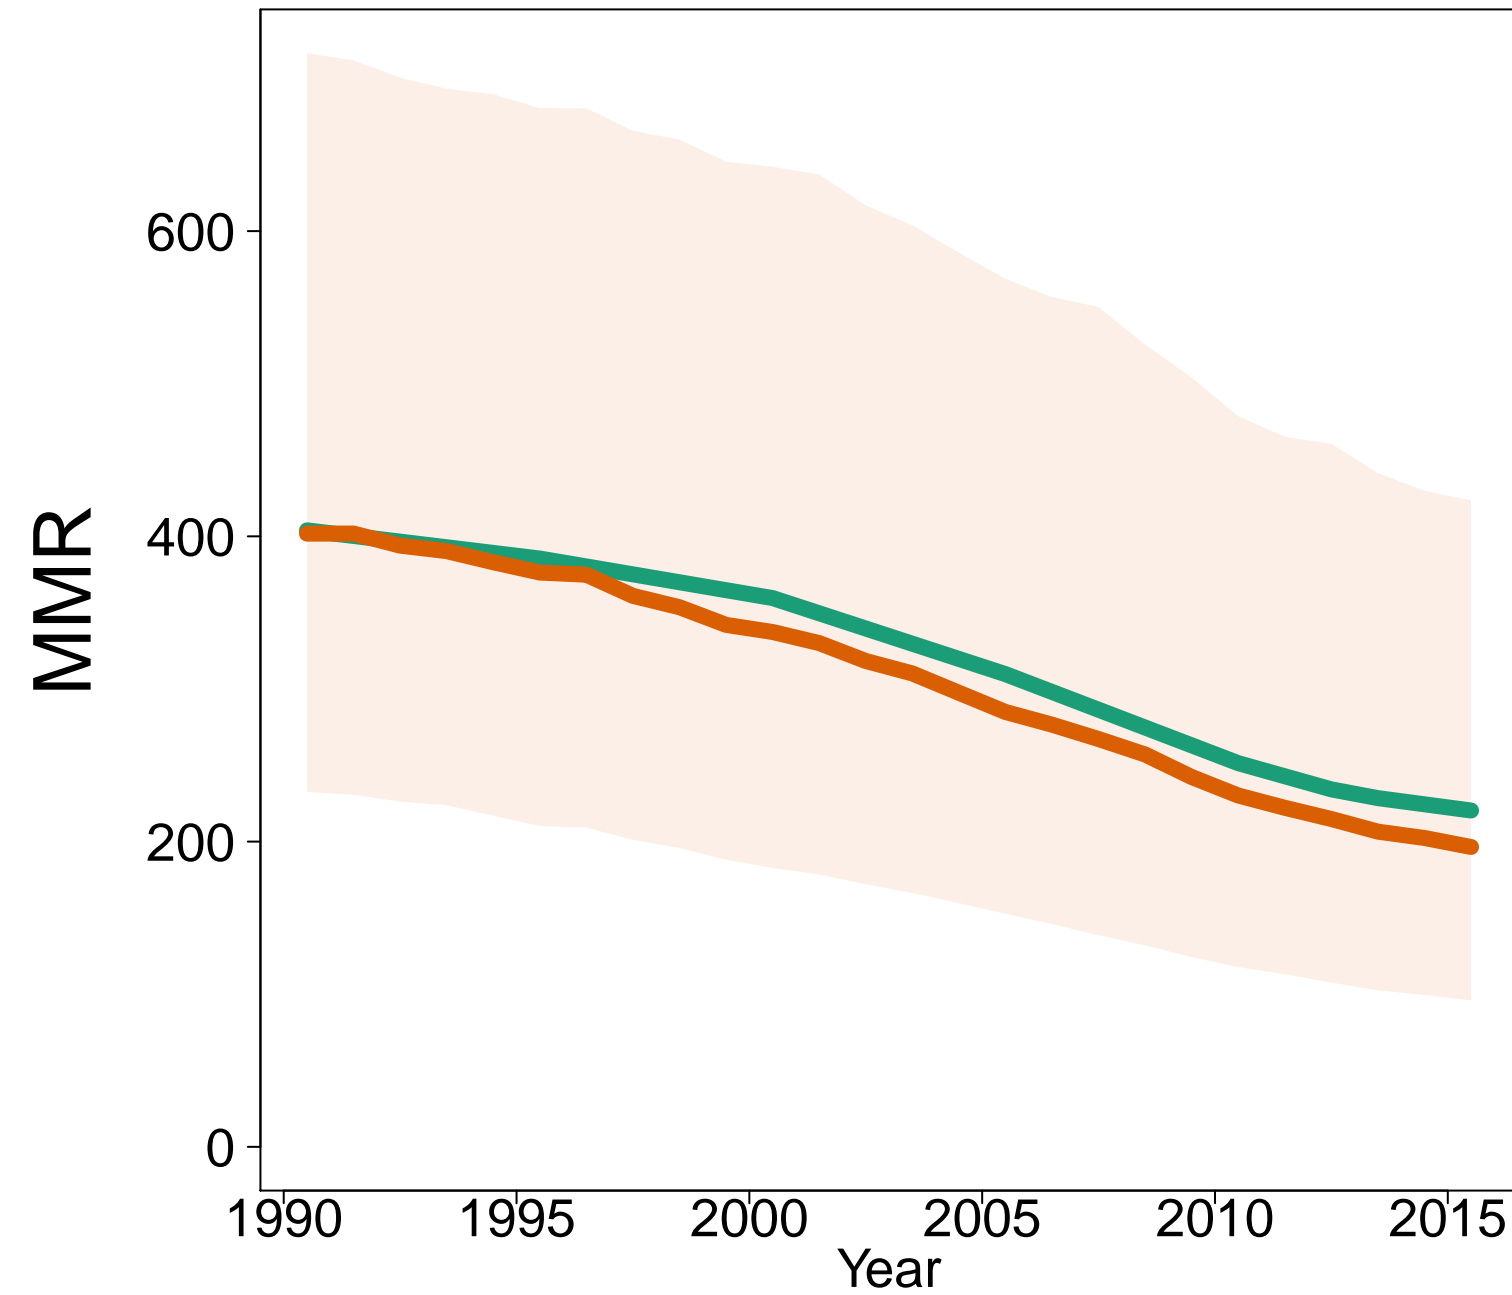

– Estimates –  
Bmat 2014  
MMEIG 2014  
– Data –

Dominican Republic [DOM; B]  
(Caribbean)

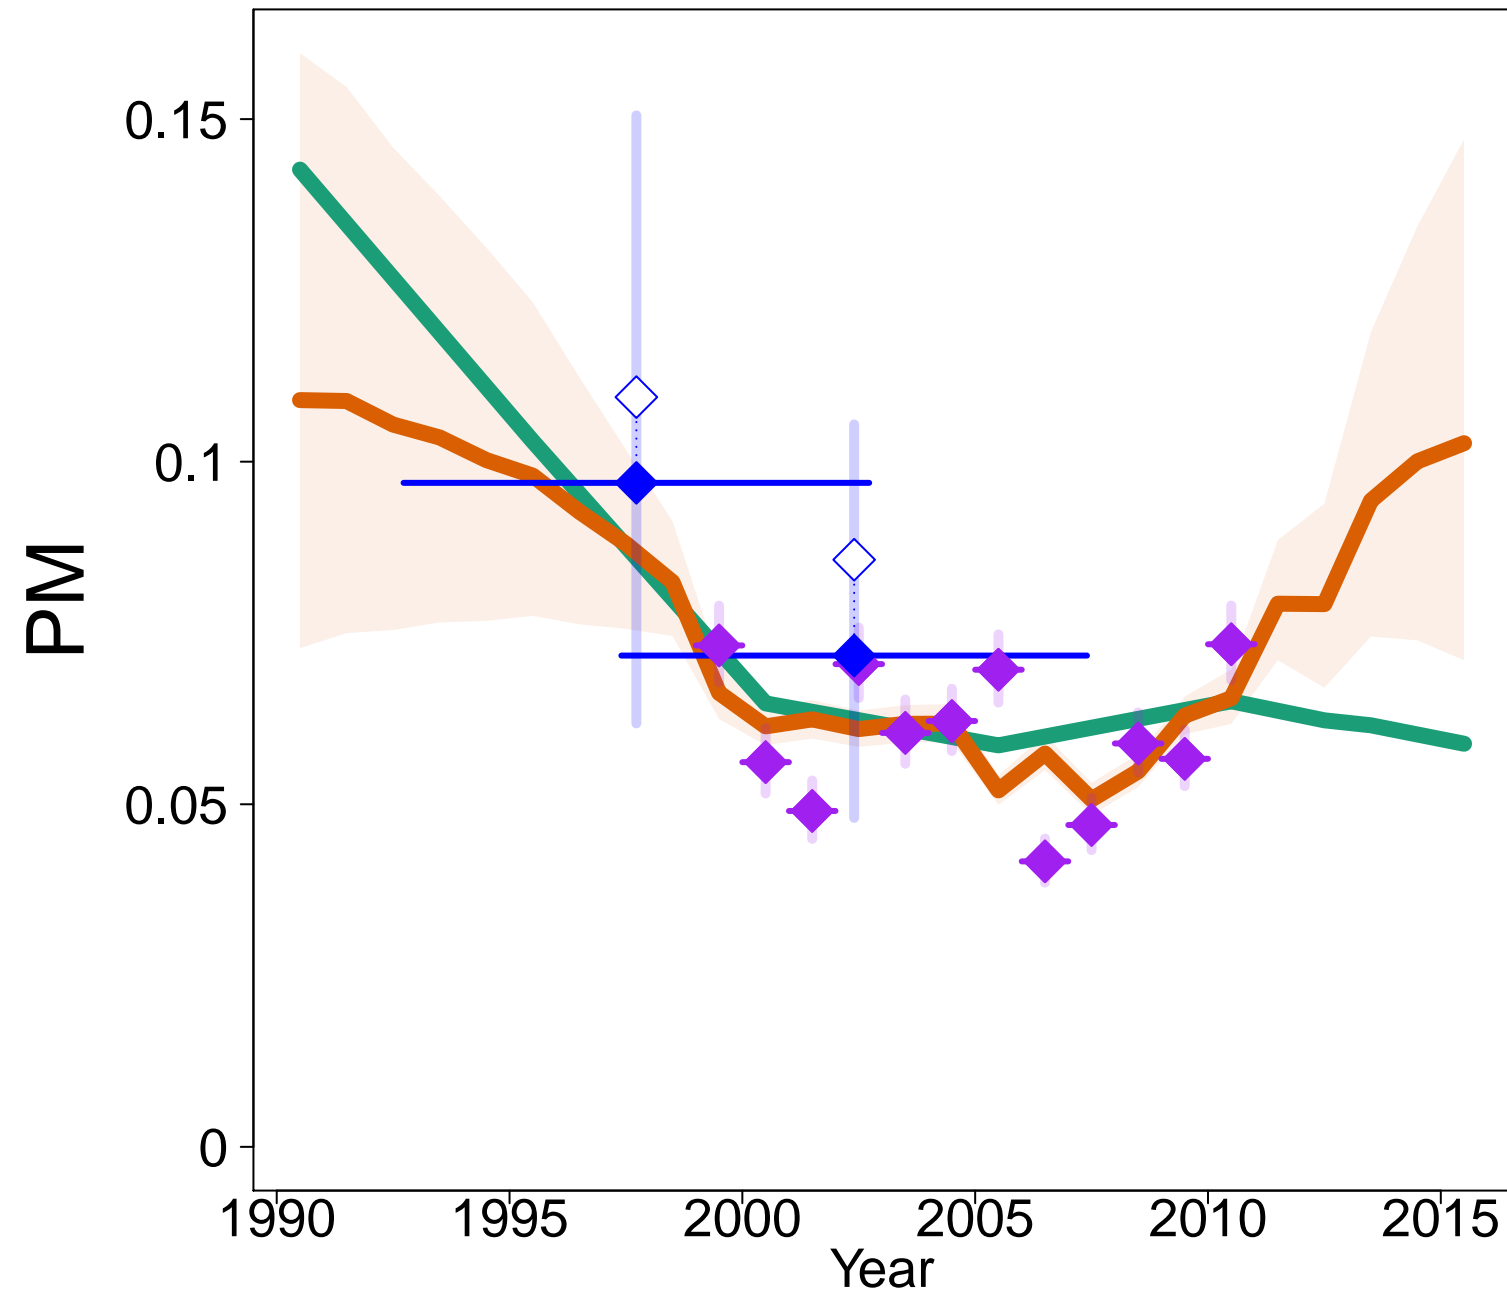

Dominican Republic [DOM; B]  
(Caribbean)

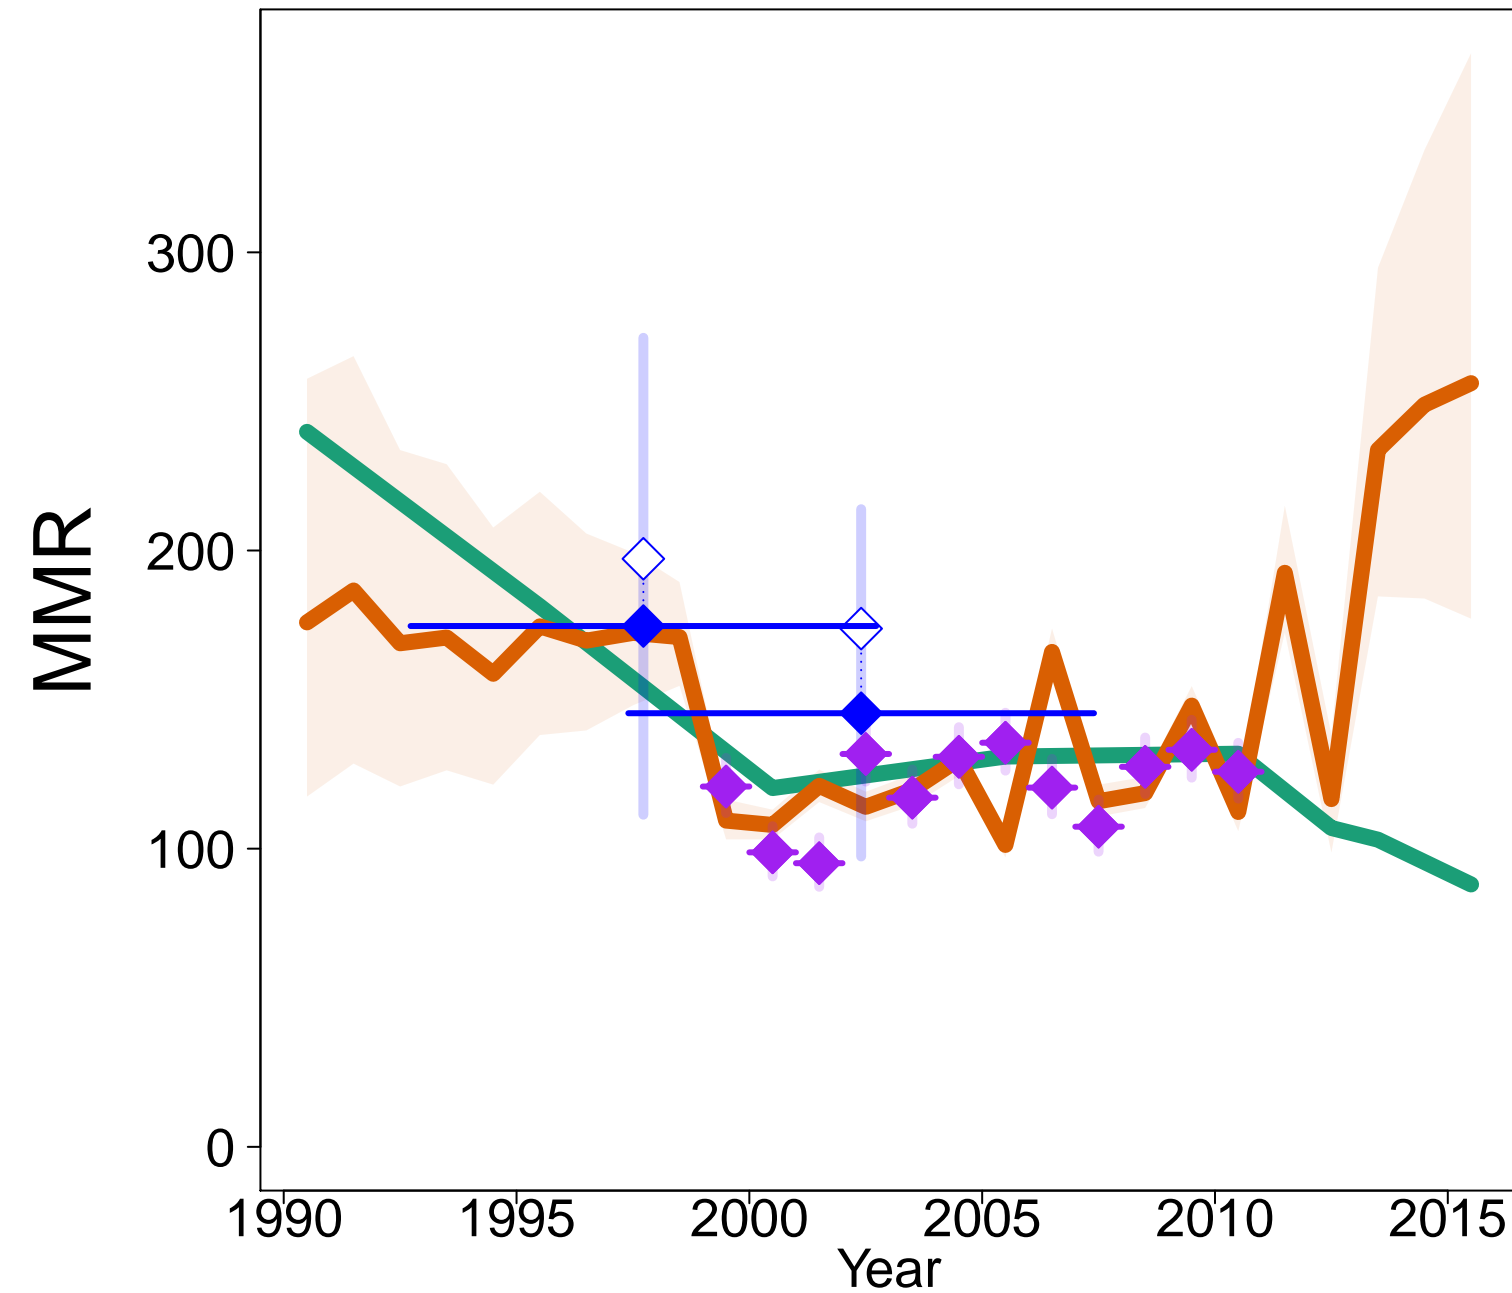

- Estimates –
- Bmat 2014
- MMEIG 2014
- Data –
- Observed Data
- Adjusted Data
- Data type –
- Spec. studies
- DHS



Ecuador [ECU; B]  
(South America)

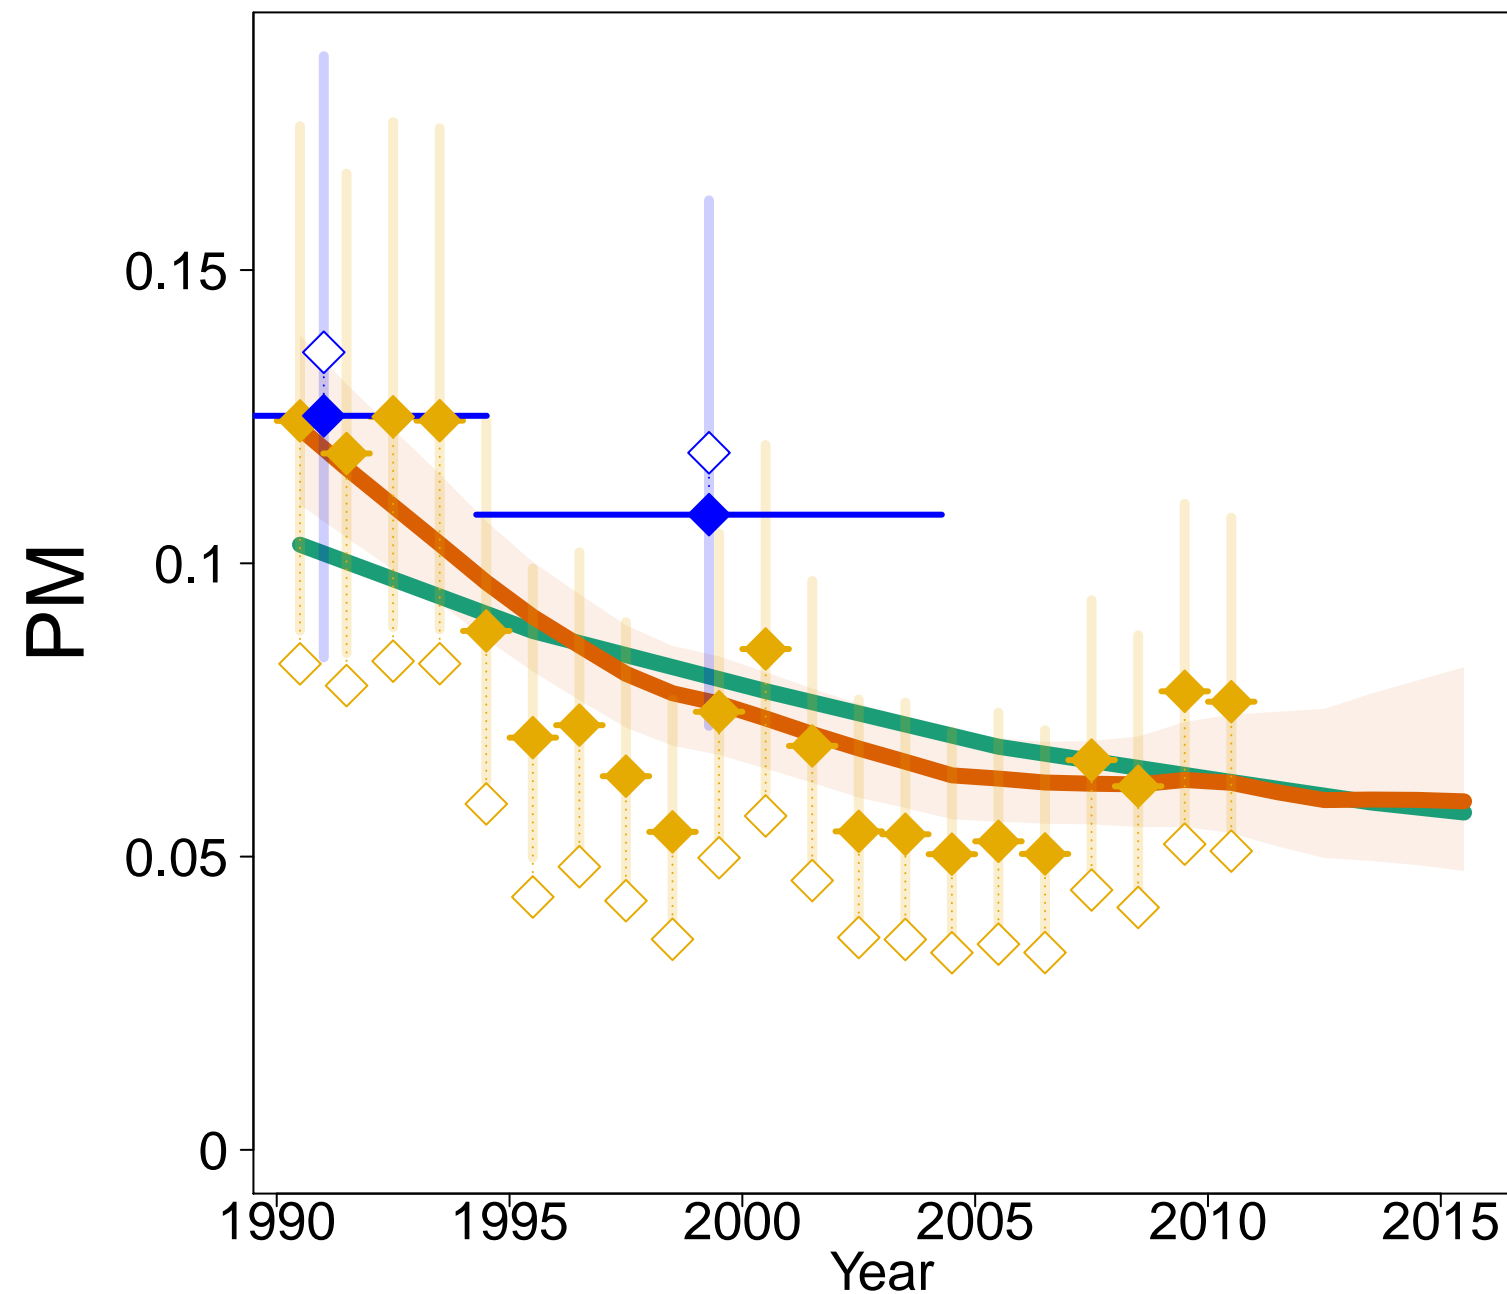

Ecuador [ECU; B]  
(South America)

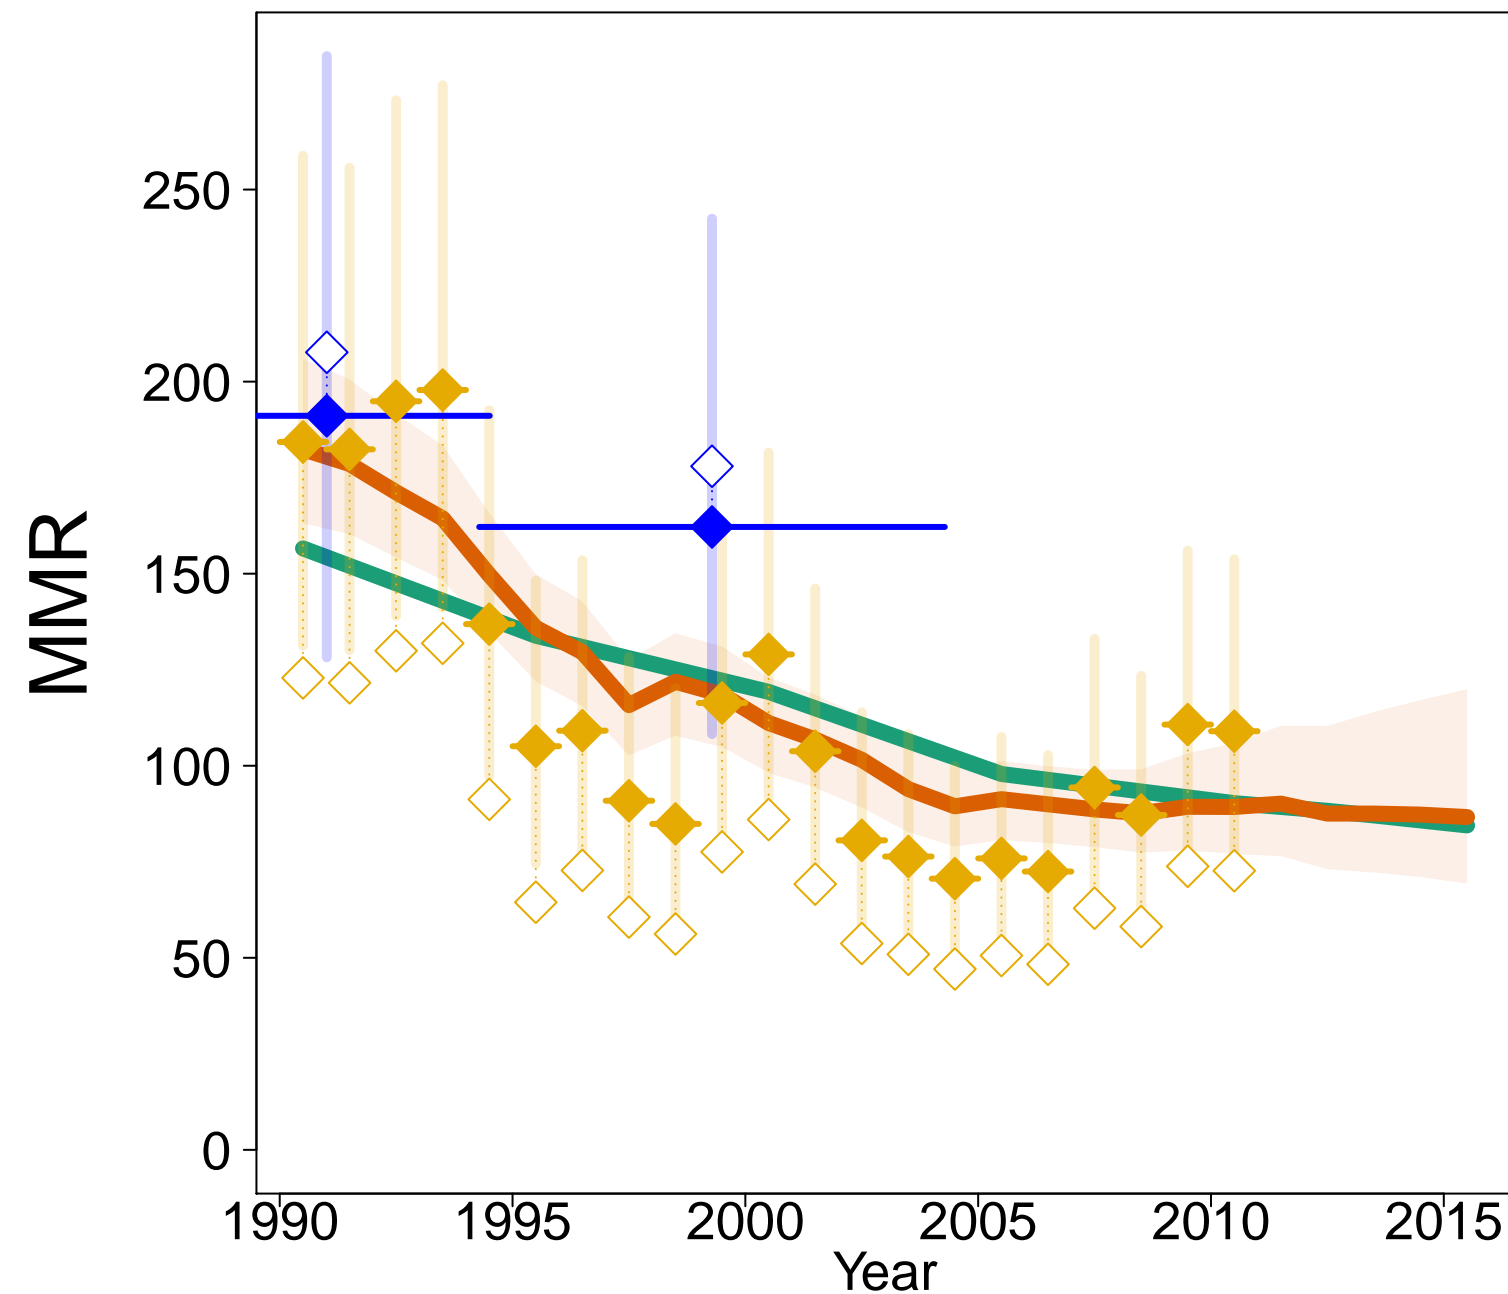

- Estimates –
- Bmat 2014
- MMEIG 2014
- Data –
- Observed Data
- Adjusted Data
- Data type –
- VR
- DHS

Egypt [EGY; B]  
(Northern Africa)

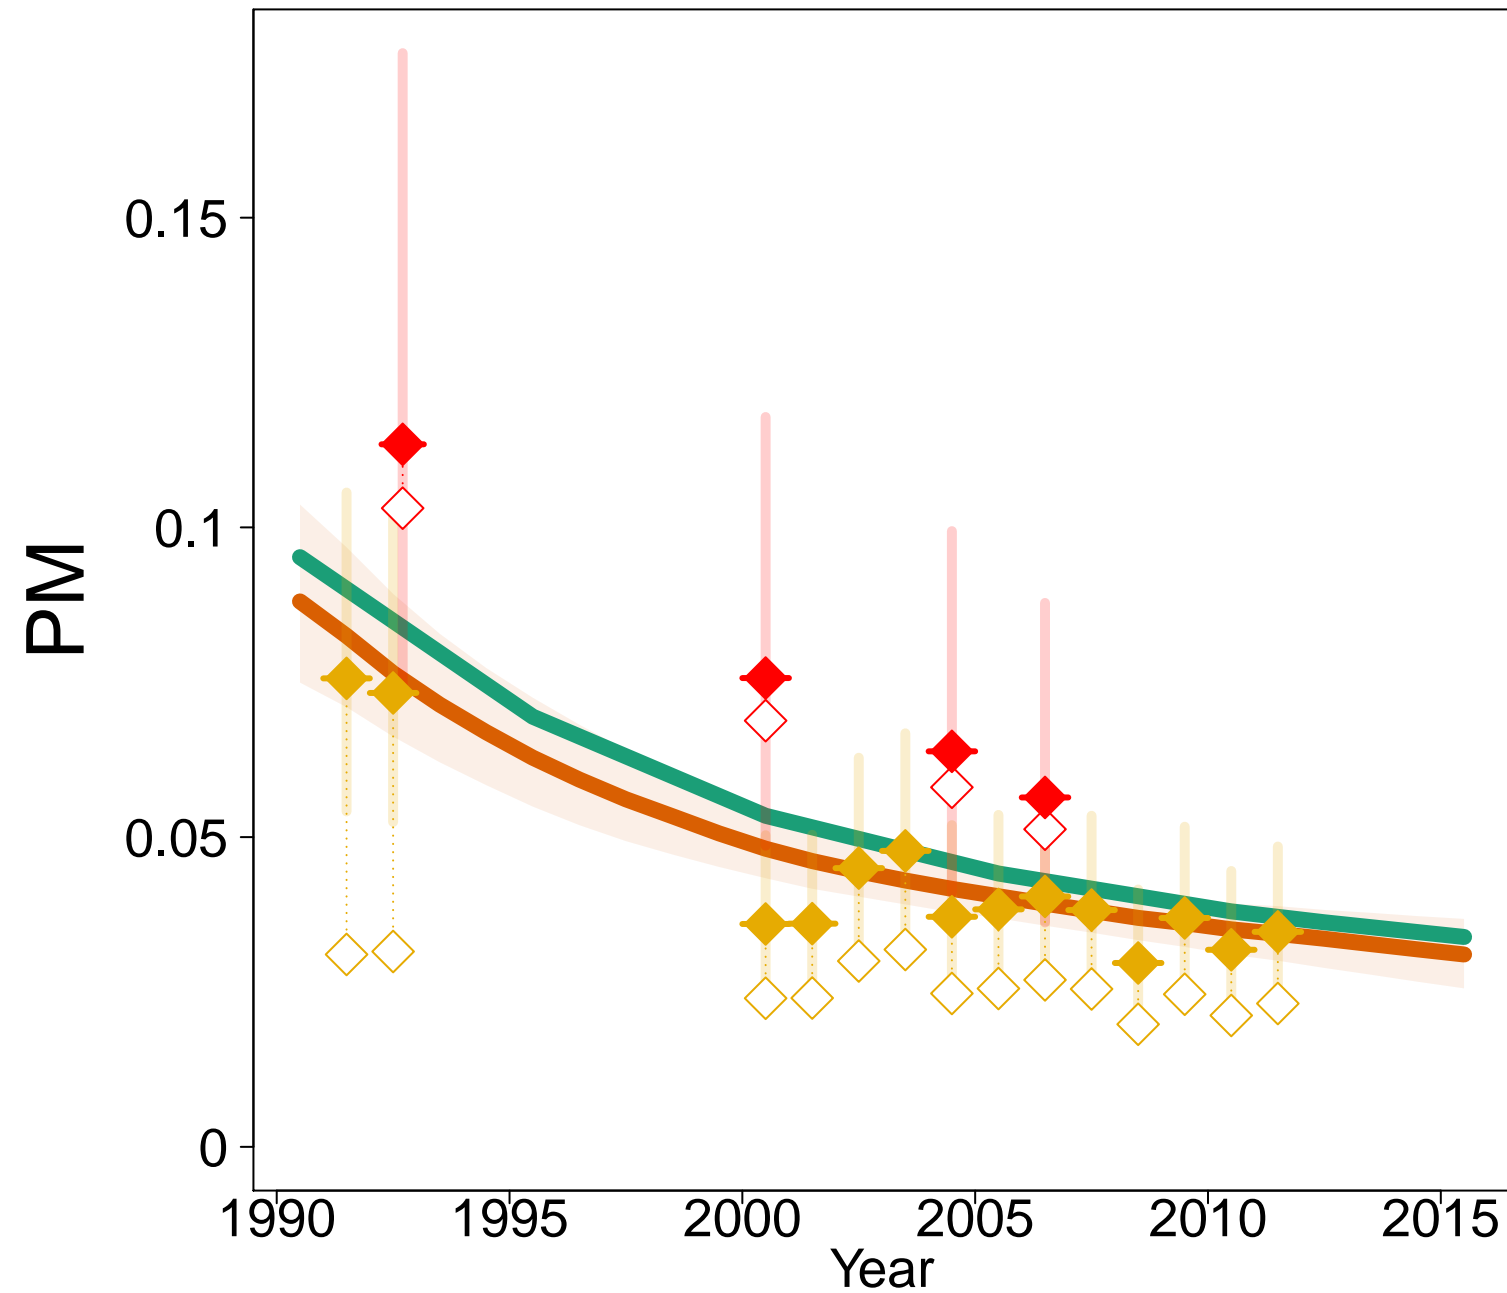

Egypt [EGY; B]  
(Northern Africa)

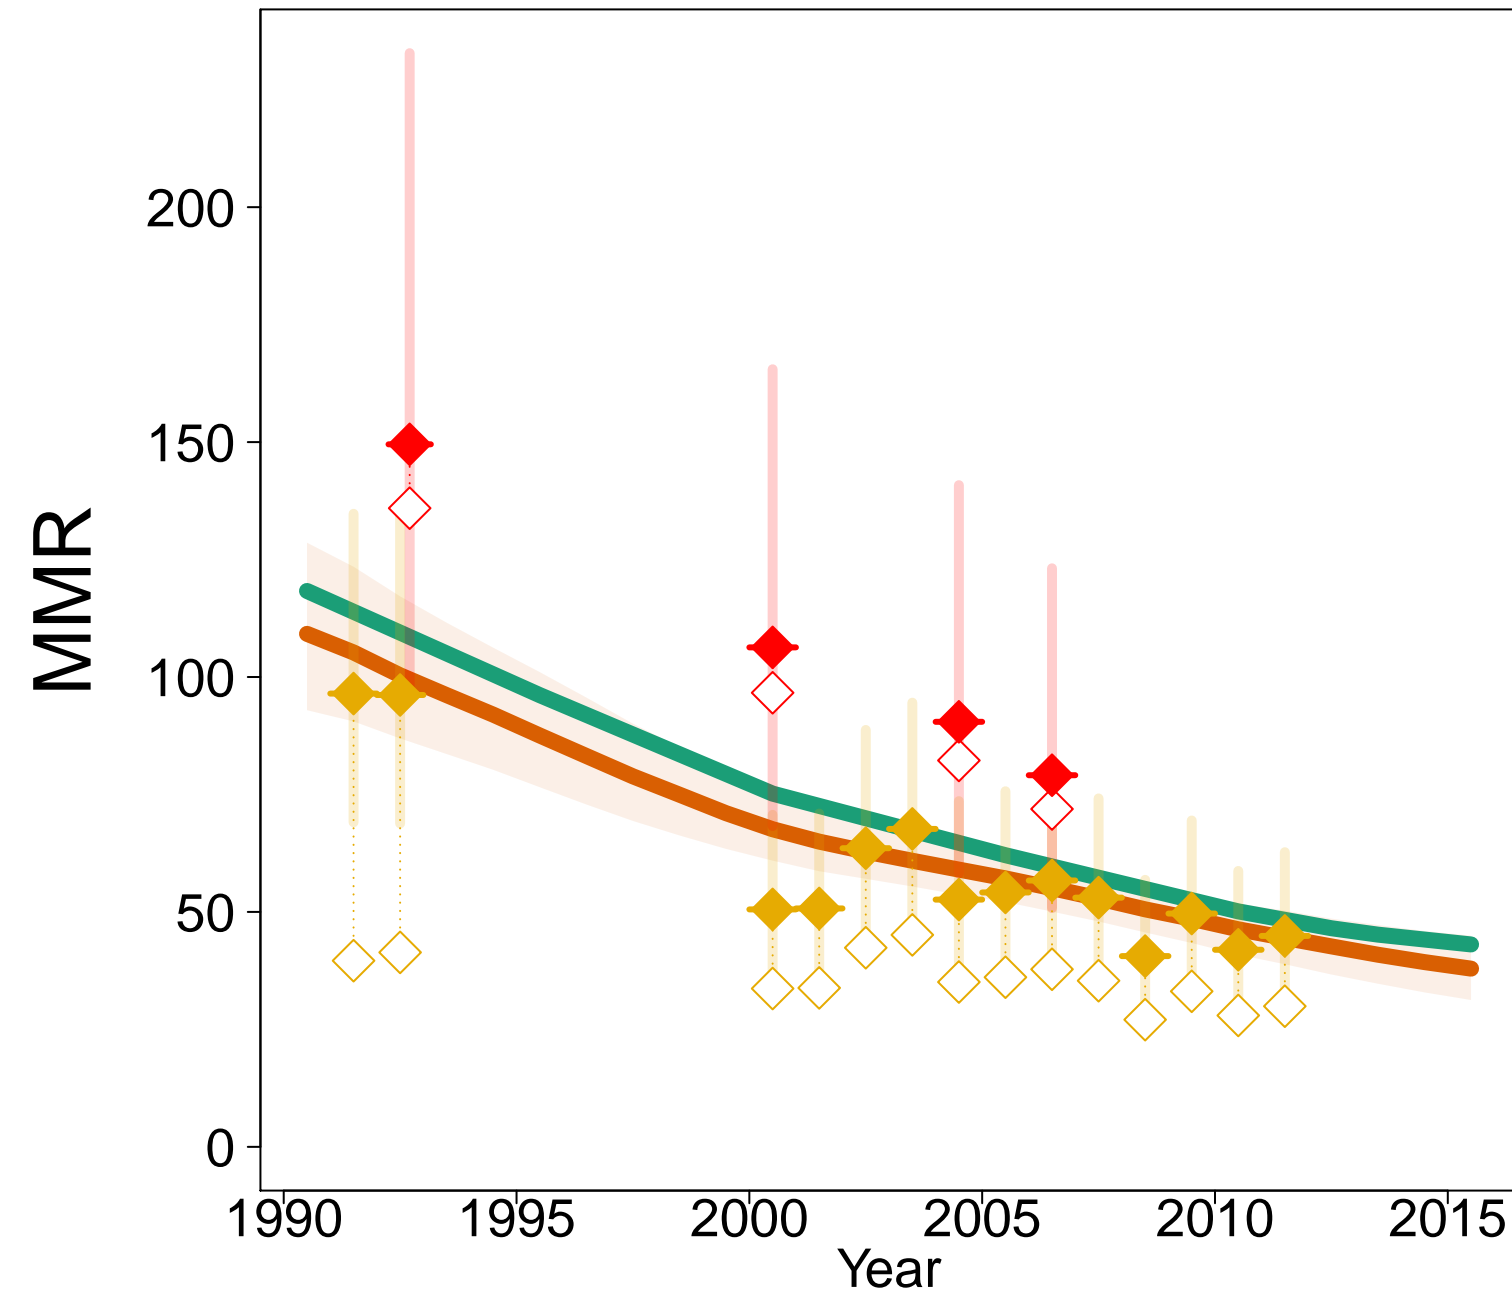

- Estimates –
- Bmat 2014
- MMEIG 2014
- Data –
- Observed Data
- Adjusted Data
- Data type –
- VR
- Misc. studies

El Salvador [SLV; B]  
(Central America)

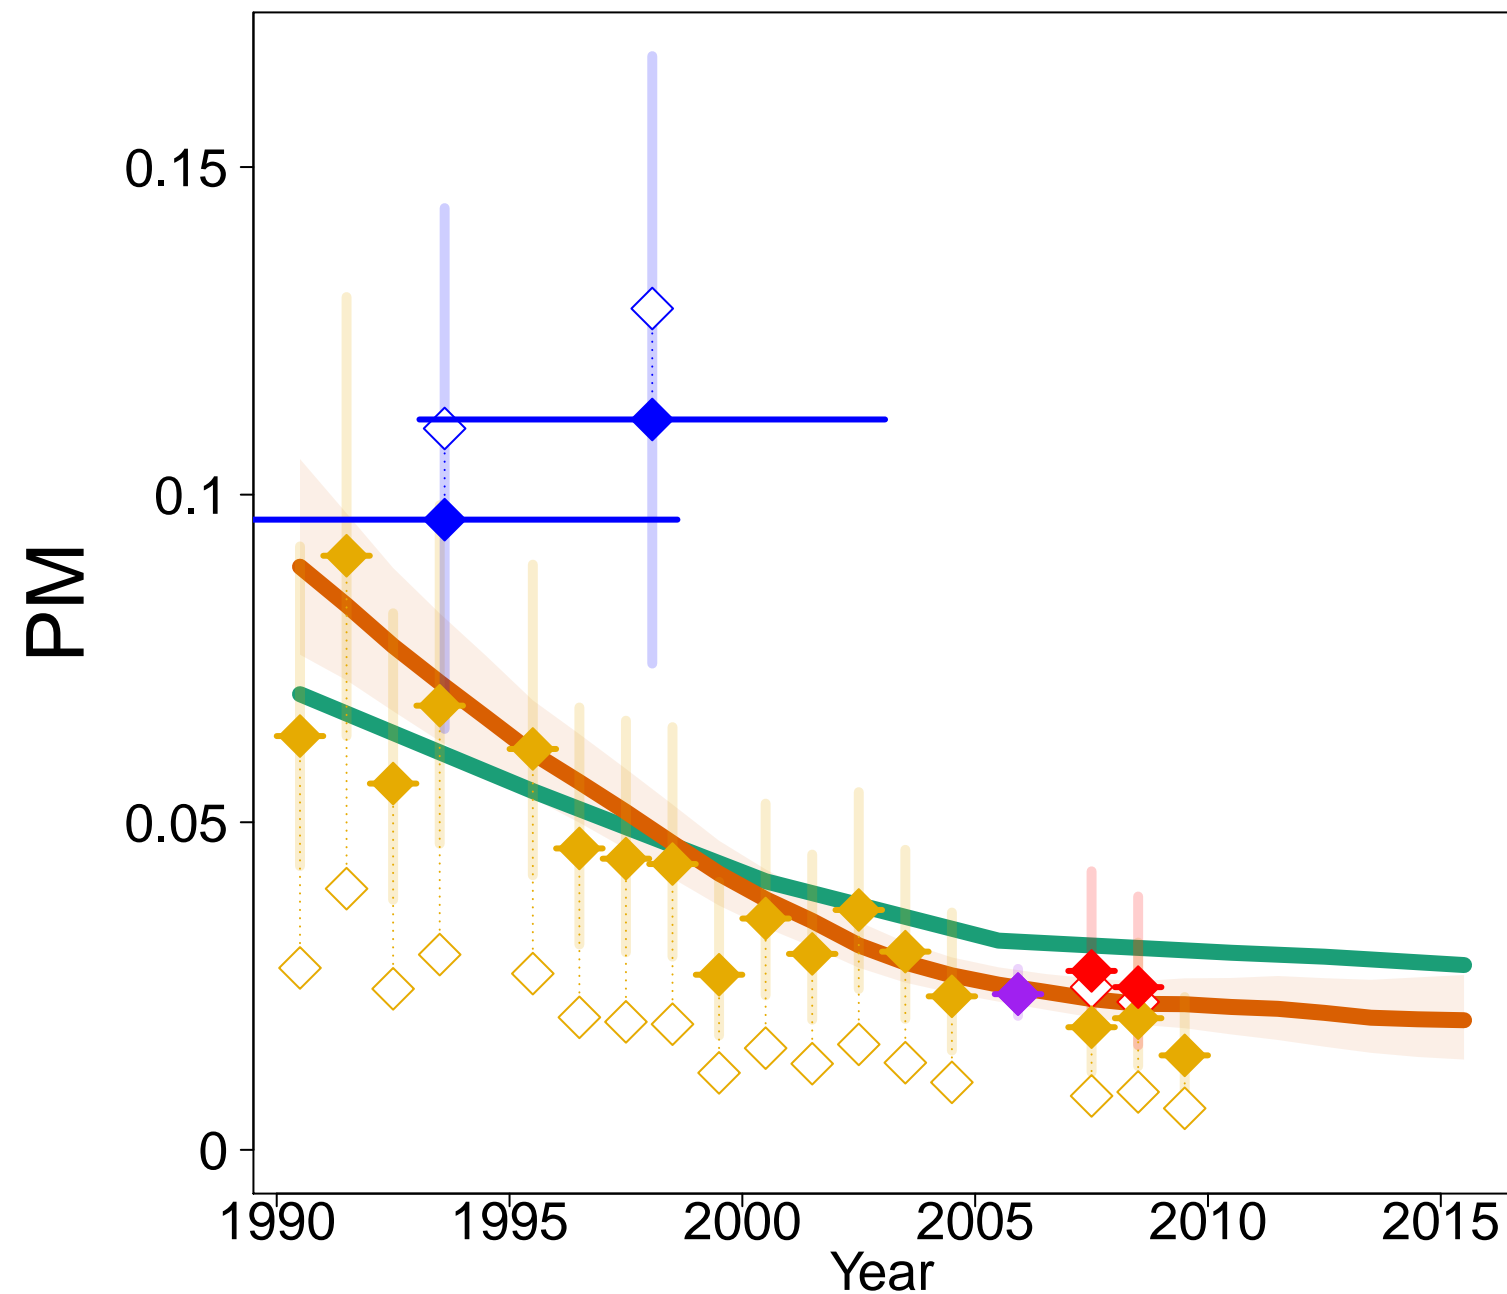

El Salvador [SLV; B]  
(Central America)

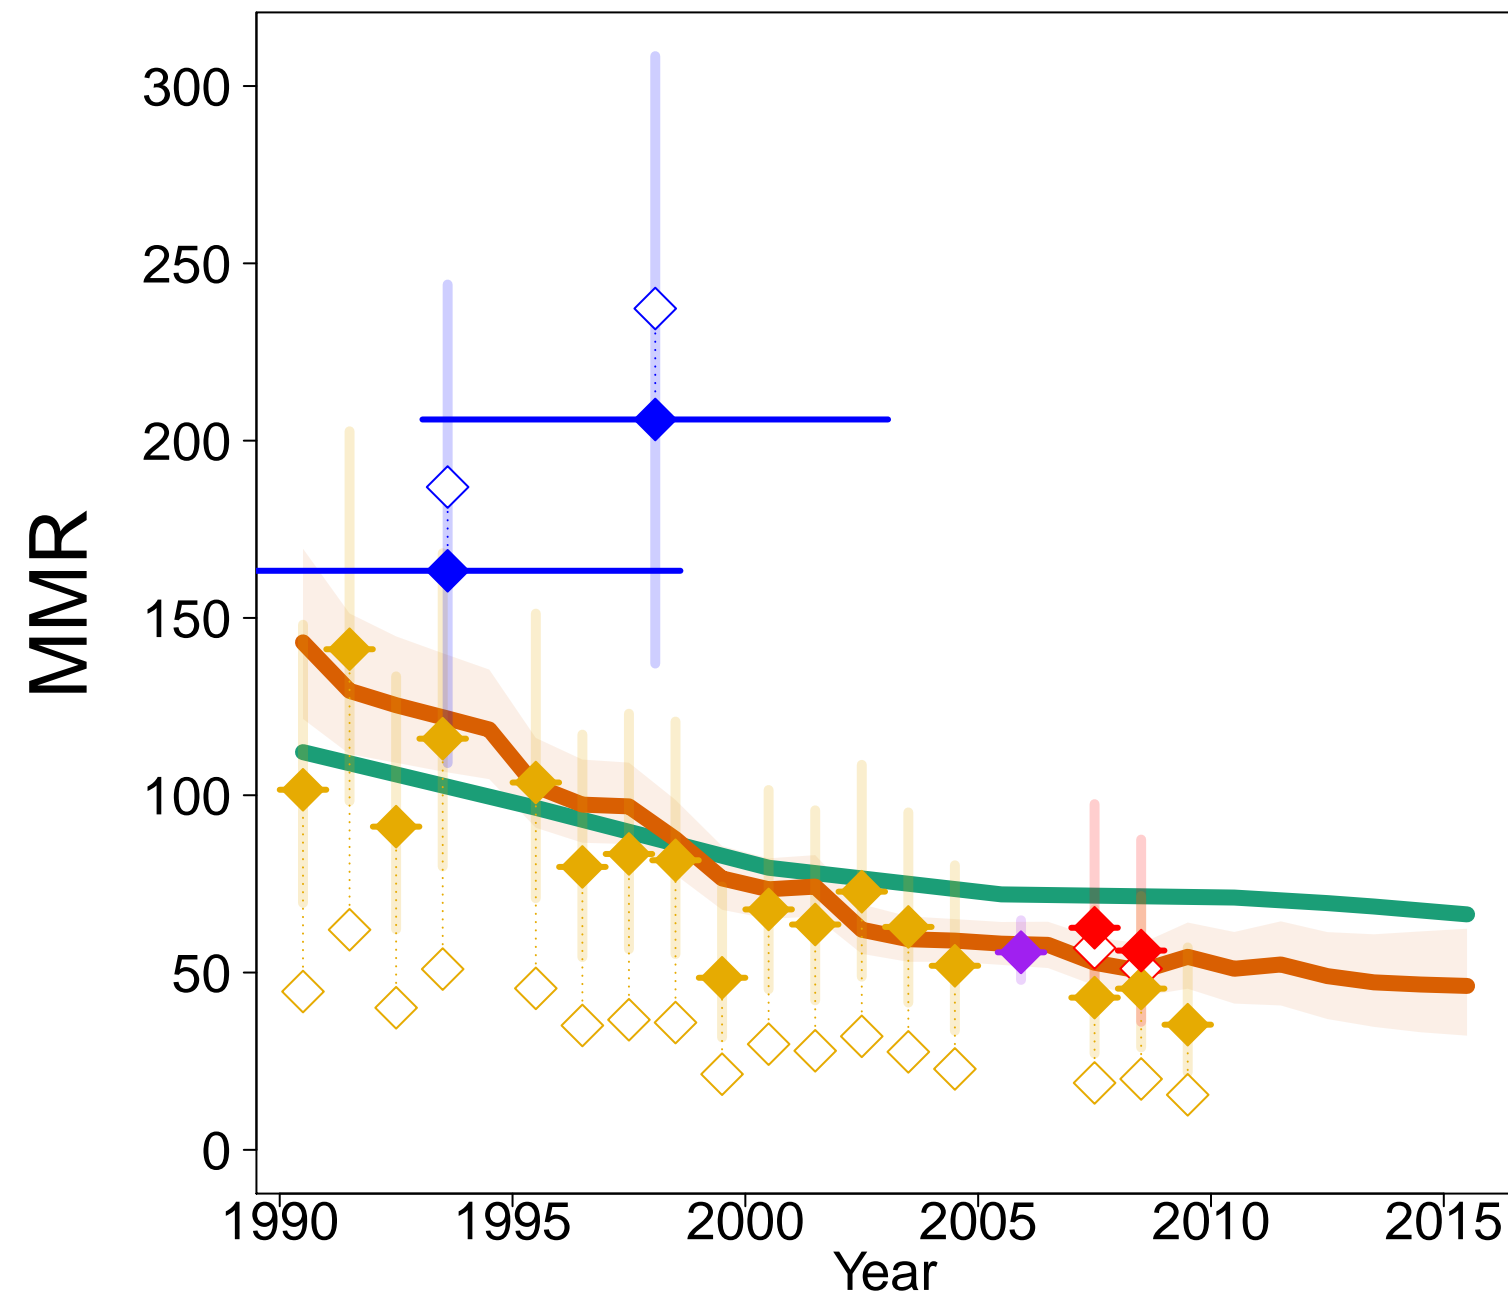

- Estimates –
- Bmat 2014
- MMEIG 2014
- Data –
- Observed Data
- Adjusted Data
- Data type –
- VR
- Spec. studies
- DHS
- Misc. studies

Equatorial Guinea [GNQ; B]  
(Middle Africa)

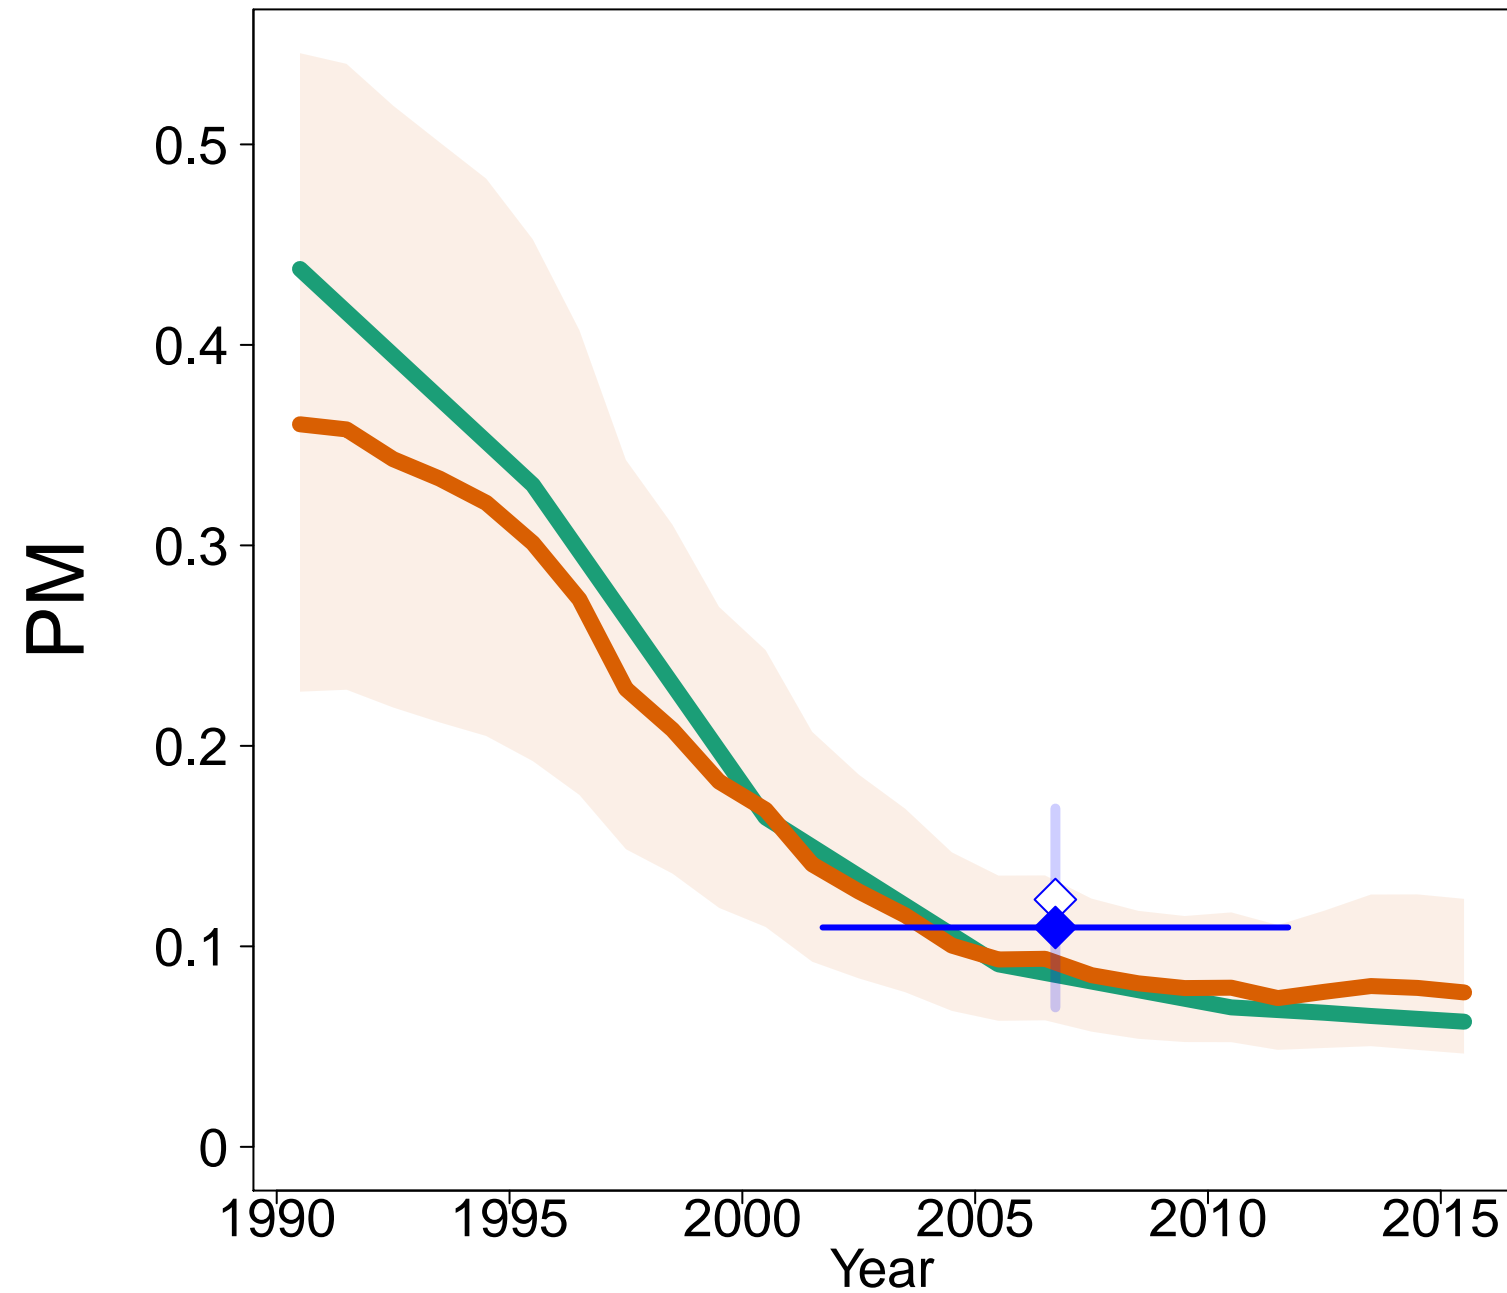

Equatorial Guinea [GNQ; B]  
(Middle Africa)

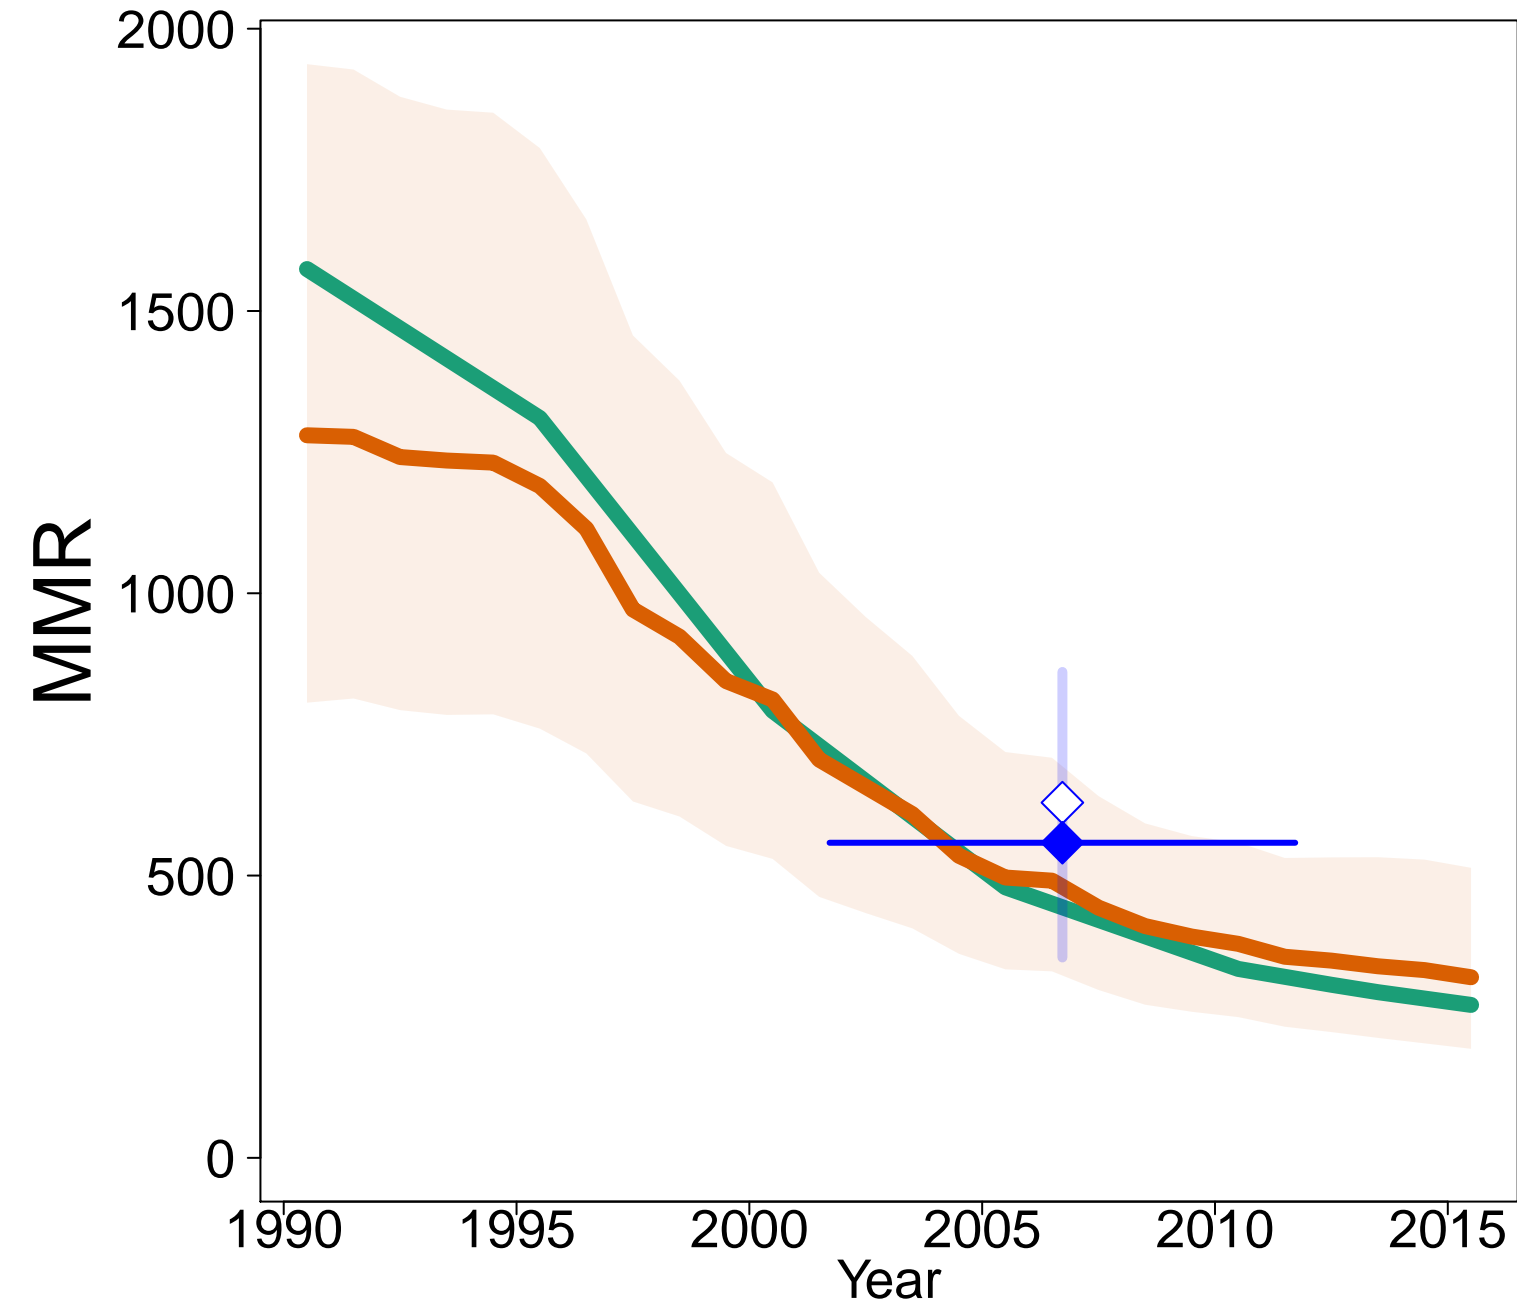

- Estimates –
- Bmat 2014
- MMEIG 2014
- Data –
- Observed Data
- Adjusted Data
- Data type –
- DHS

Eritrea [ERI; B]  
(Eastern Africa)

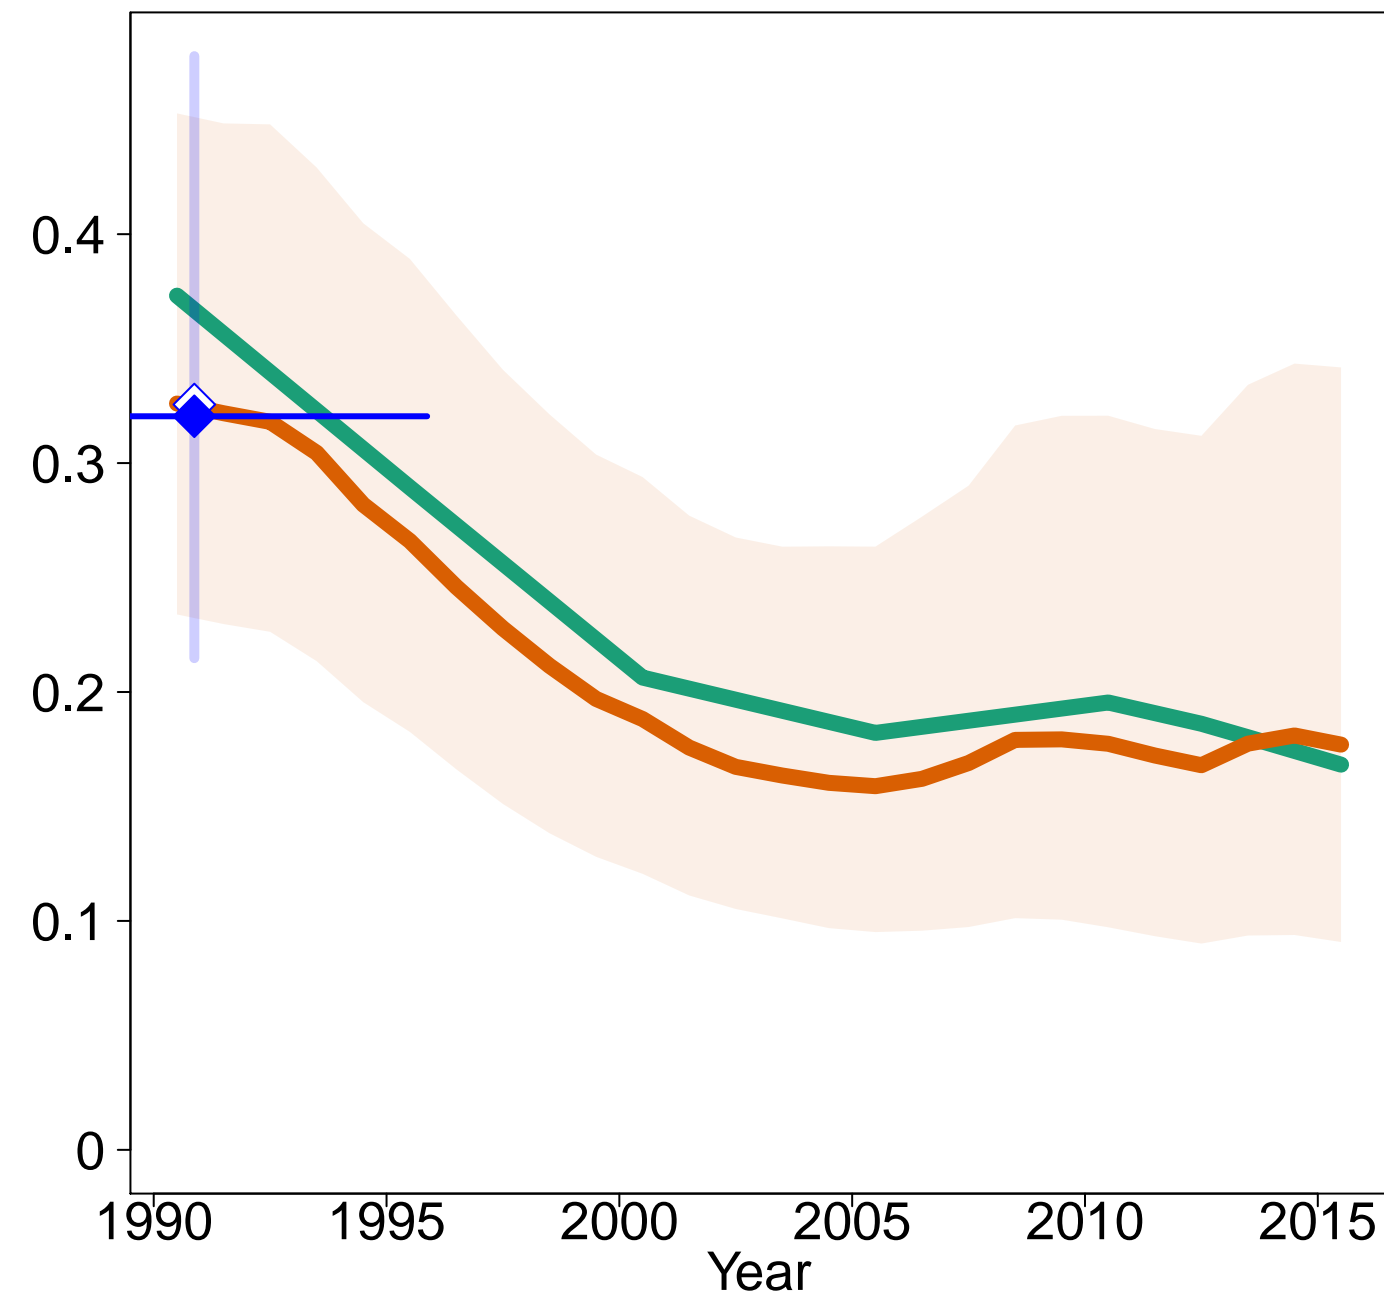

Eritrea [ERI; B]  
(Eastern Africa)

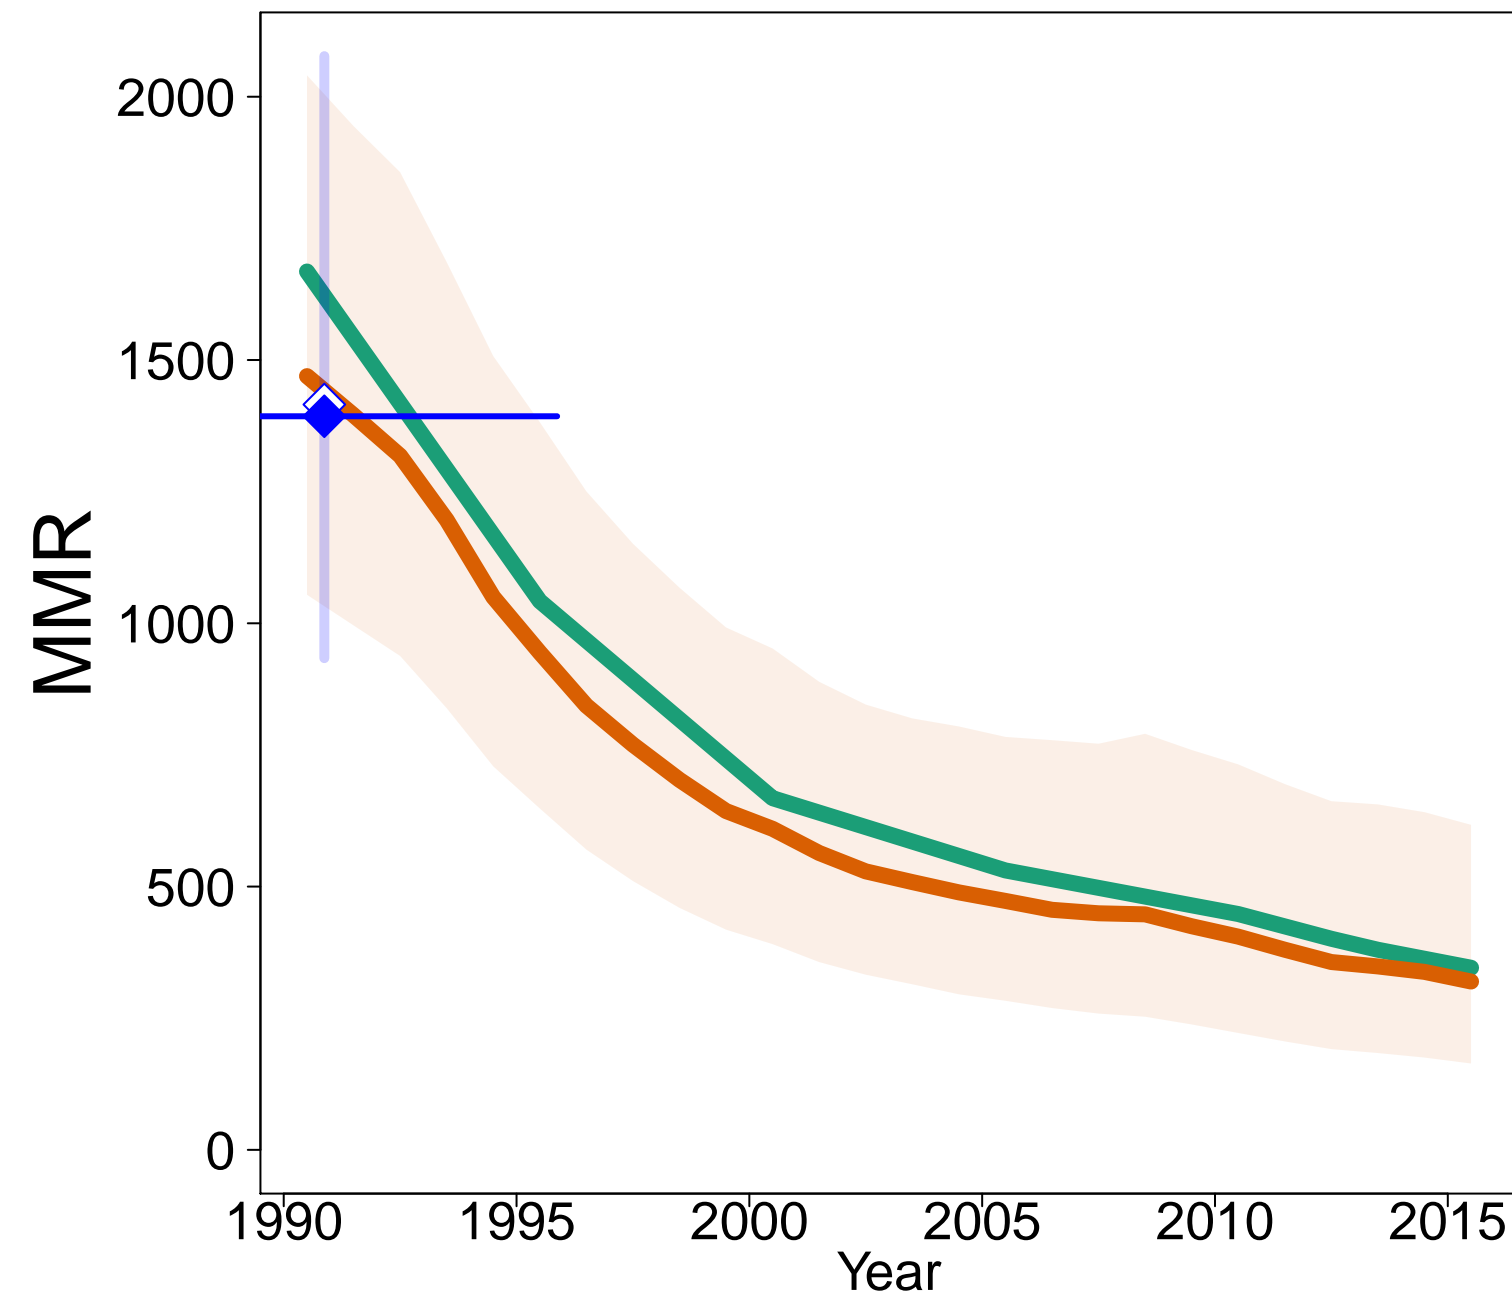

- Estimates –
- Bmat 2014
- MMEIG 2014
- Data –
- Observed Data
- Adjusted Data
- Data type –
- DHS

Estonia [EST; A]  
(Developed regions)

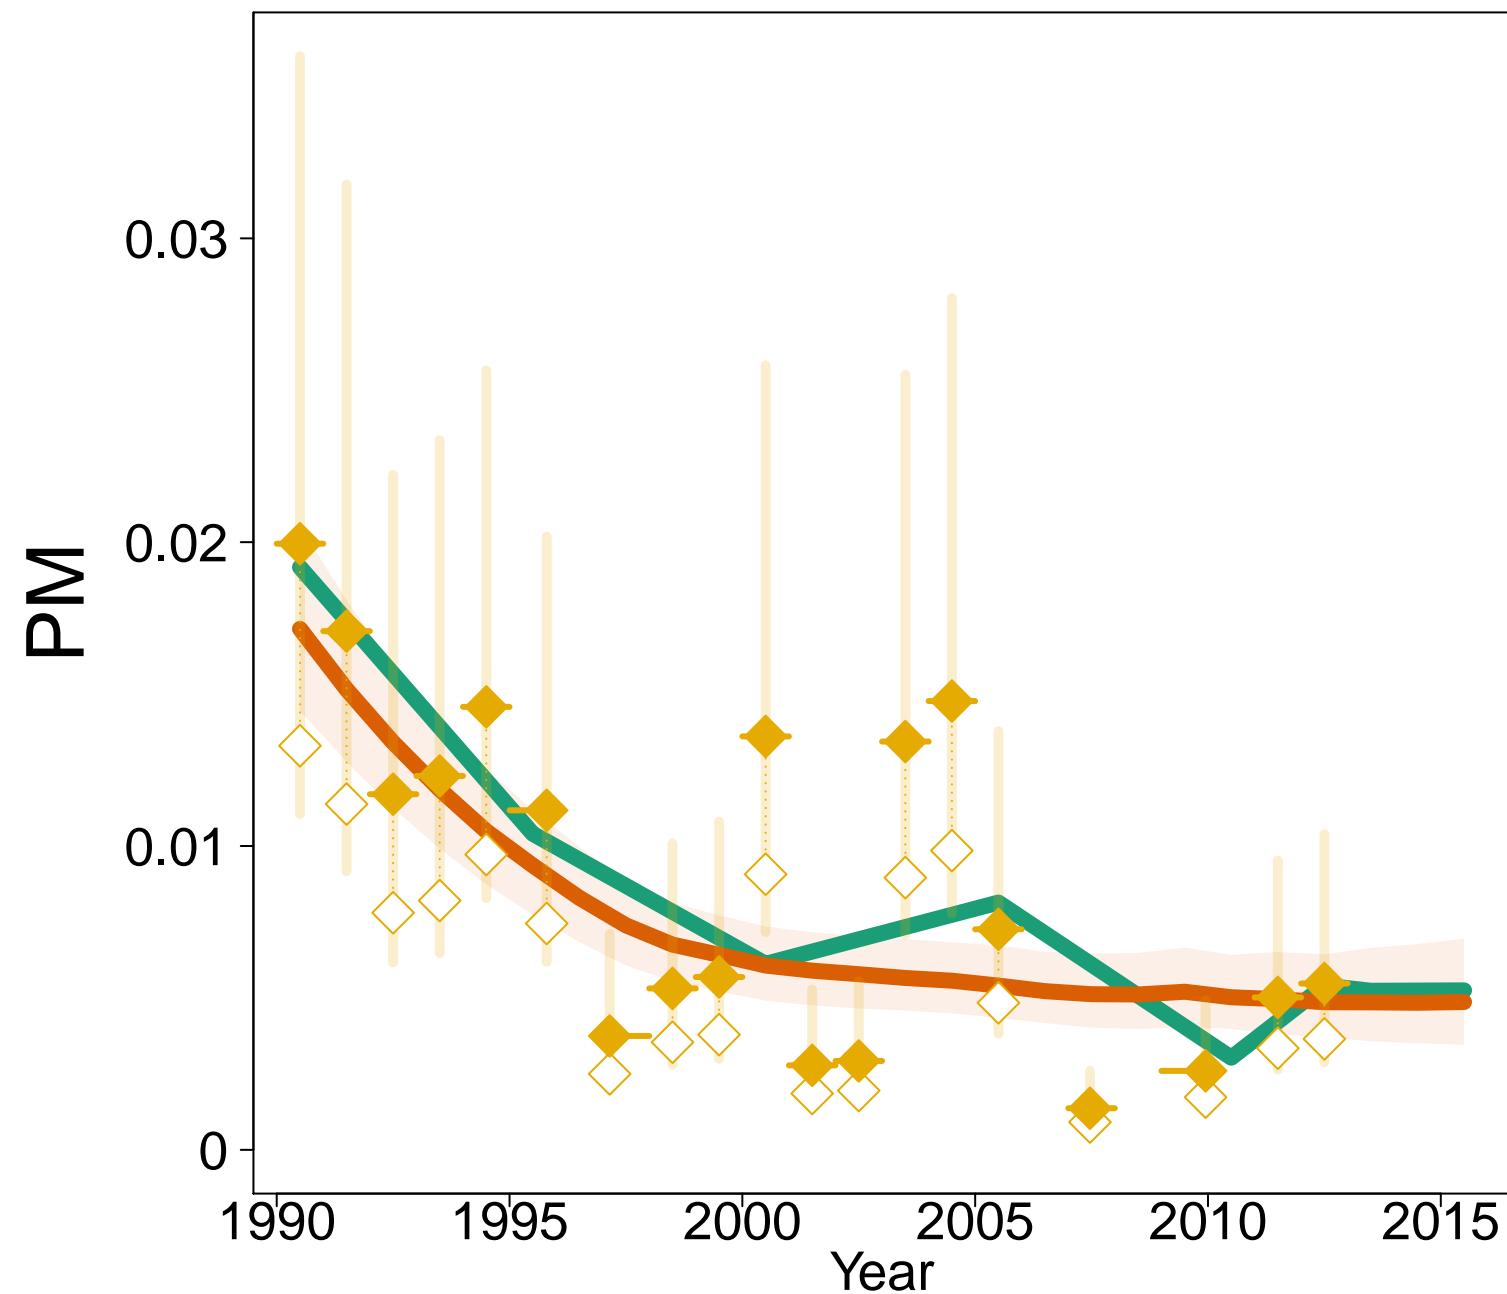

Estonia [EST; A]  
(Developed regions)

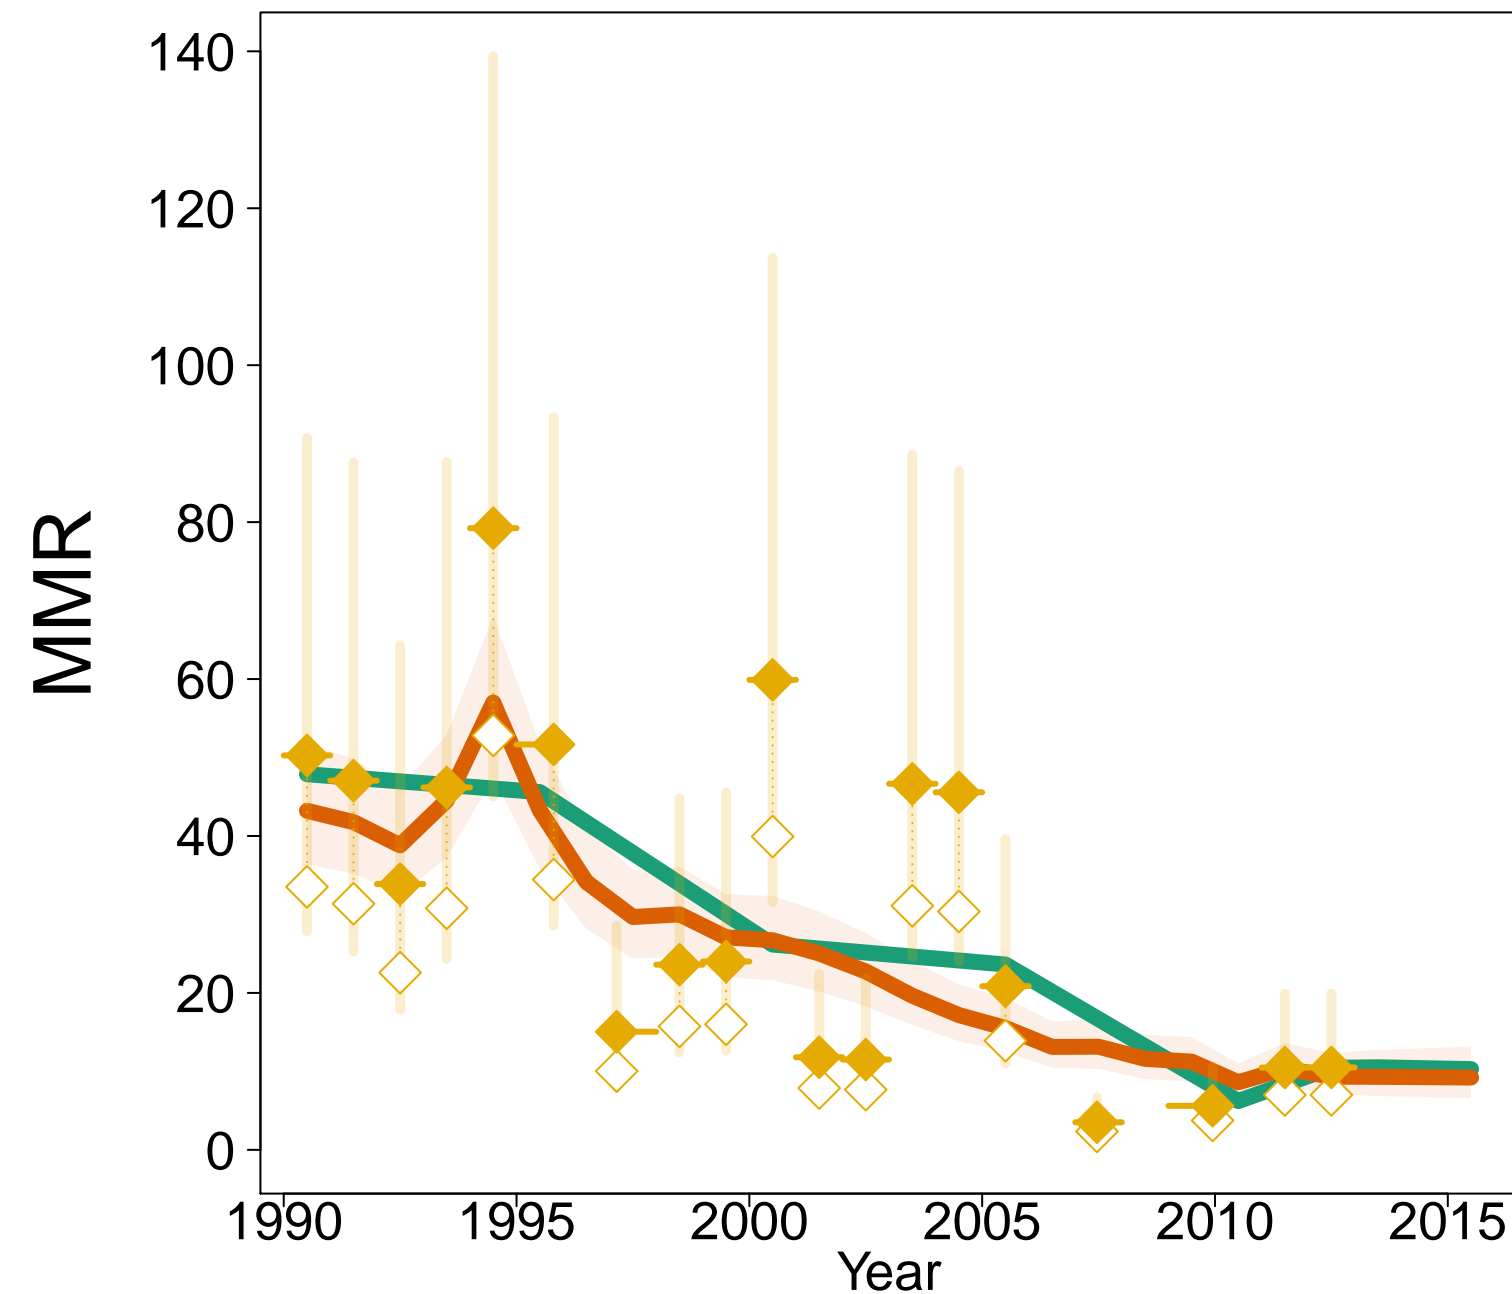

- Estimates –
- Bmat 2014
- MMEIG 2014
- Data –
- Observed Data
- Adjusted Data
- Data type –
- VR

Ethiopia [ETH; B]  
(Eastern Africa)

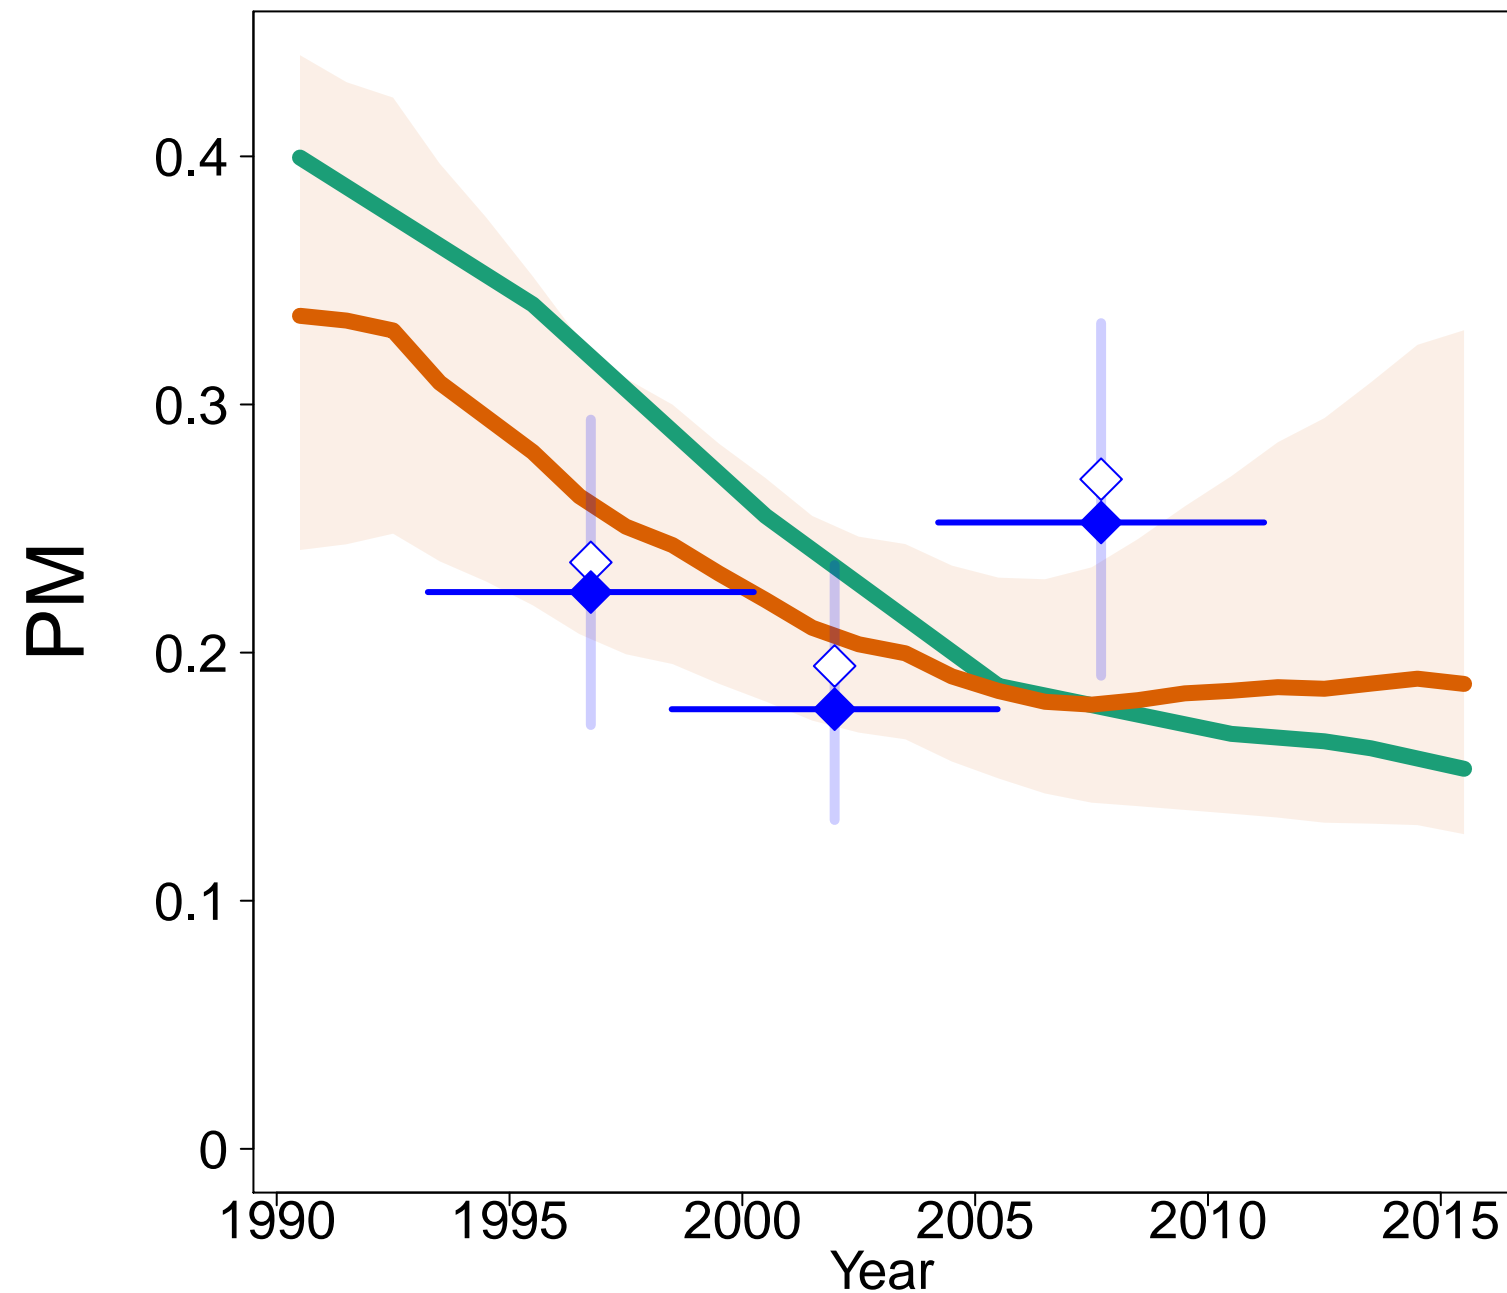

Ethiopia [ETH; B]  
(Eastern Africa)

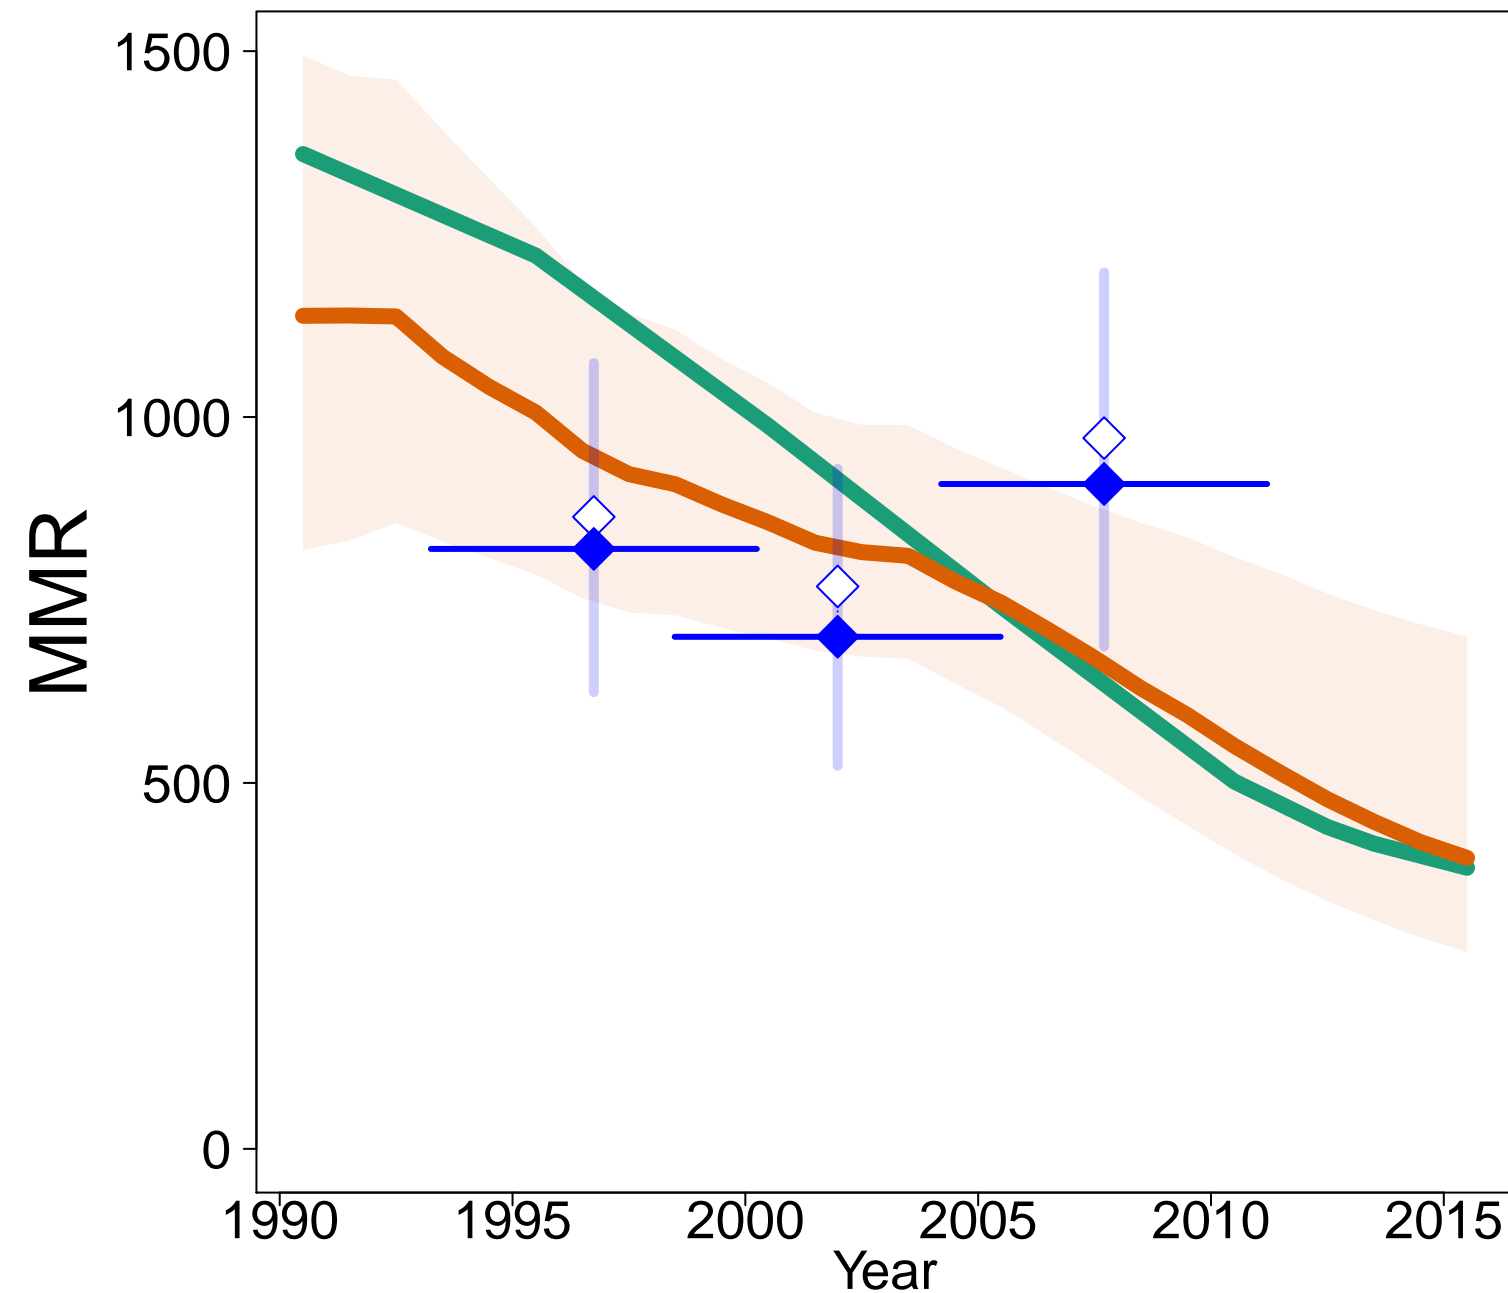

- Estimates –
- Bmat 2014
- MMEIG 2014
- Data –
- Observed Data
- Adjusted Data
- Data type –
- DHS

Fiji [FJI; B]  
(South-Eastern Asia / Oceania)

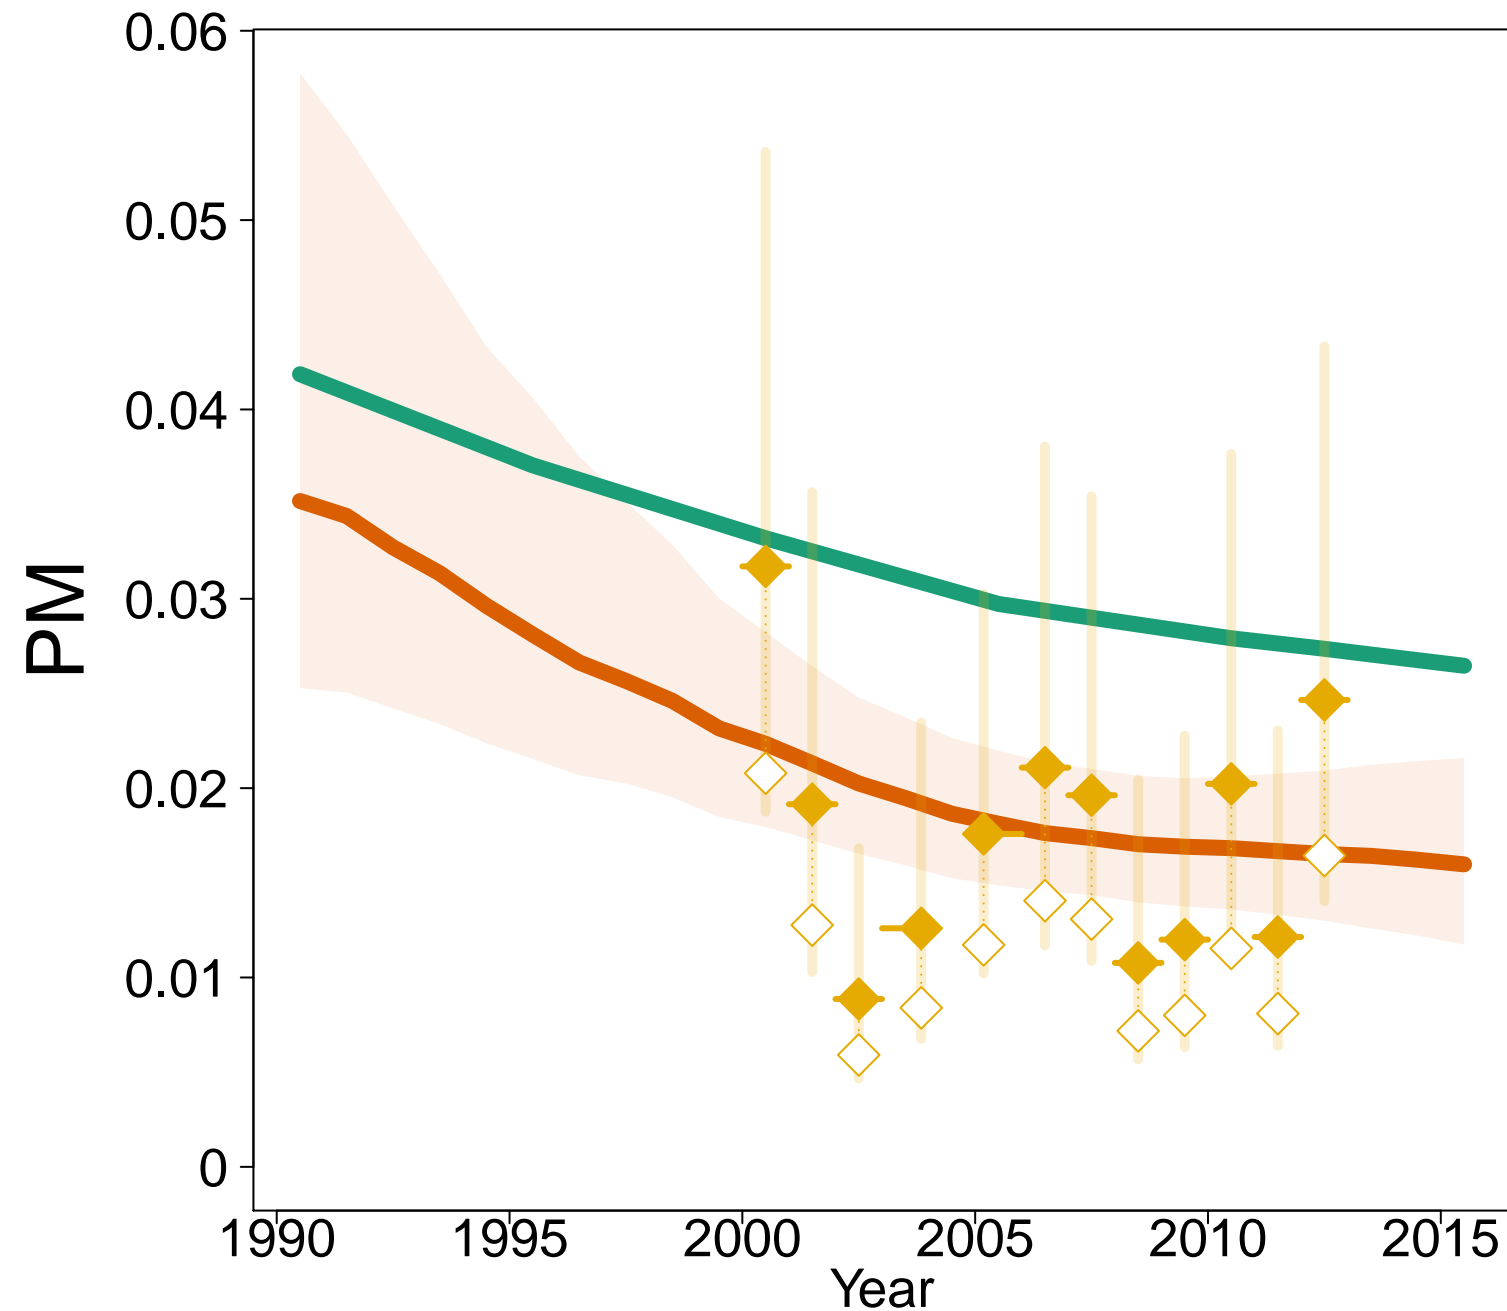

Fiji [FJI; B]  
(South-Eastern Asia / Oceania)

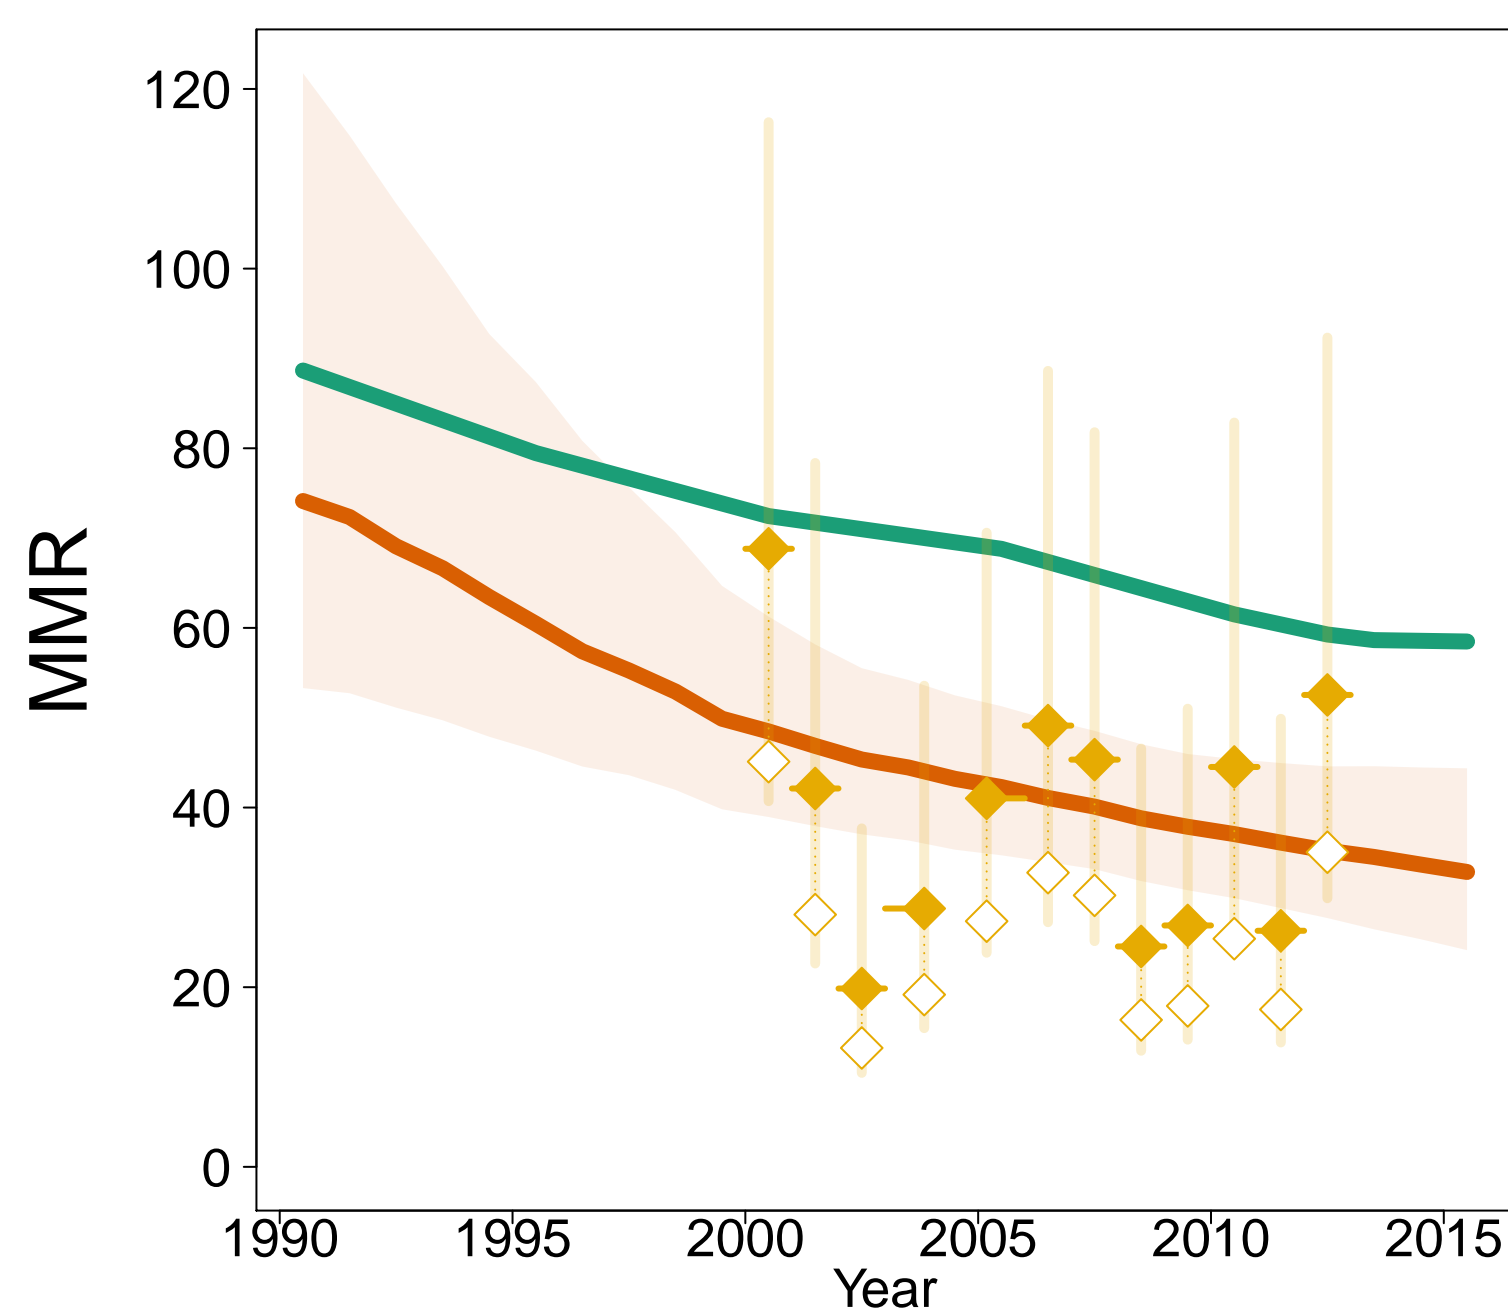

- Estimates –
- Bmat 2014
- MMEIG 2014
- Data –
- Observed Data
- Adjusted Data
- Data type –
- VR



Finland [FIN; A]  
(Developed regions)

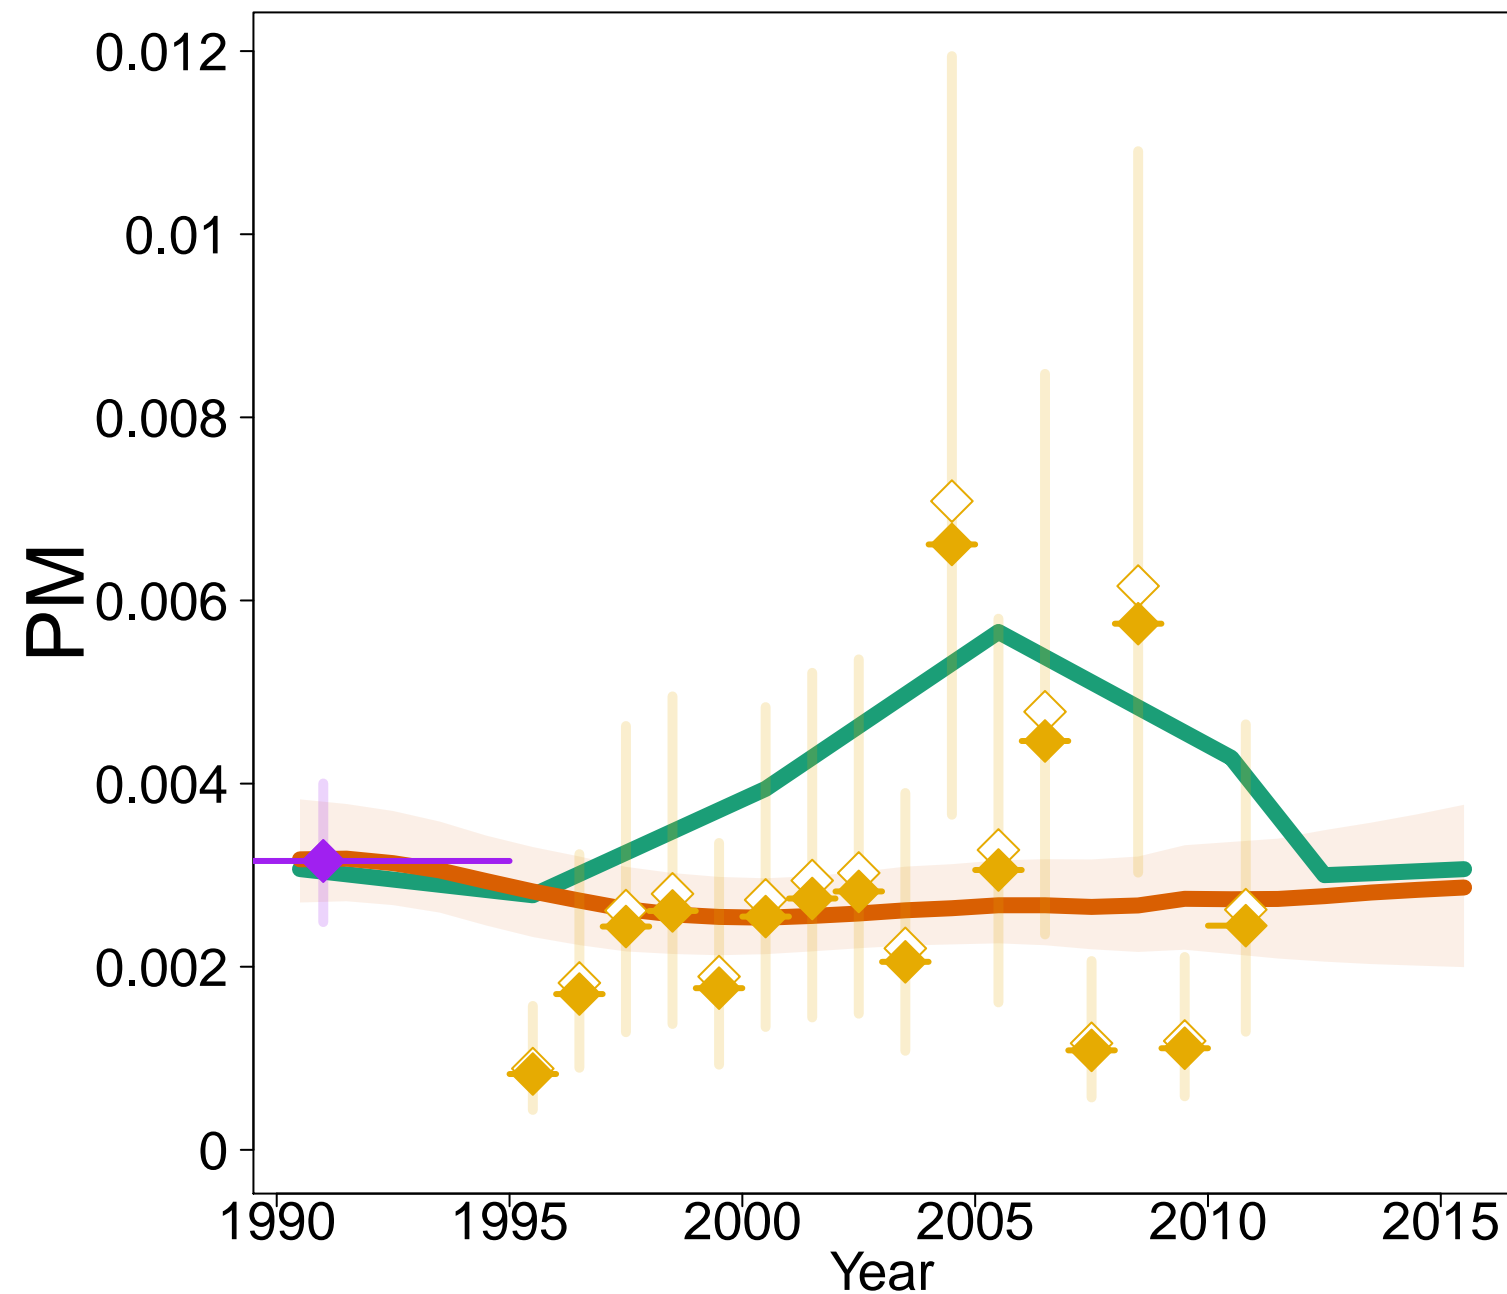

Finland [FIN; A]  
(Developed regions)

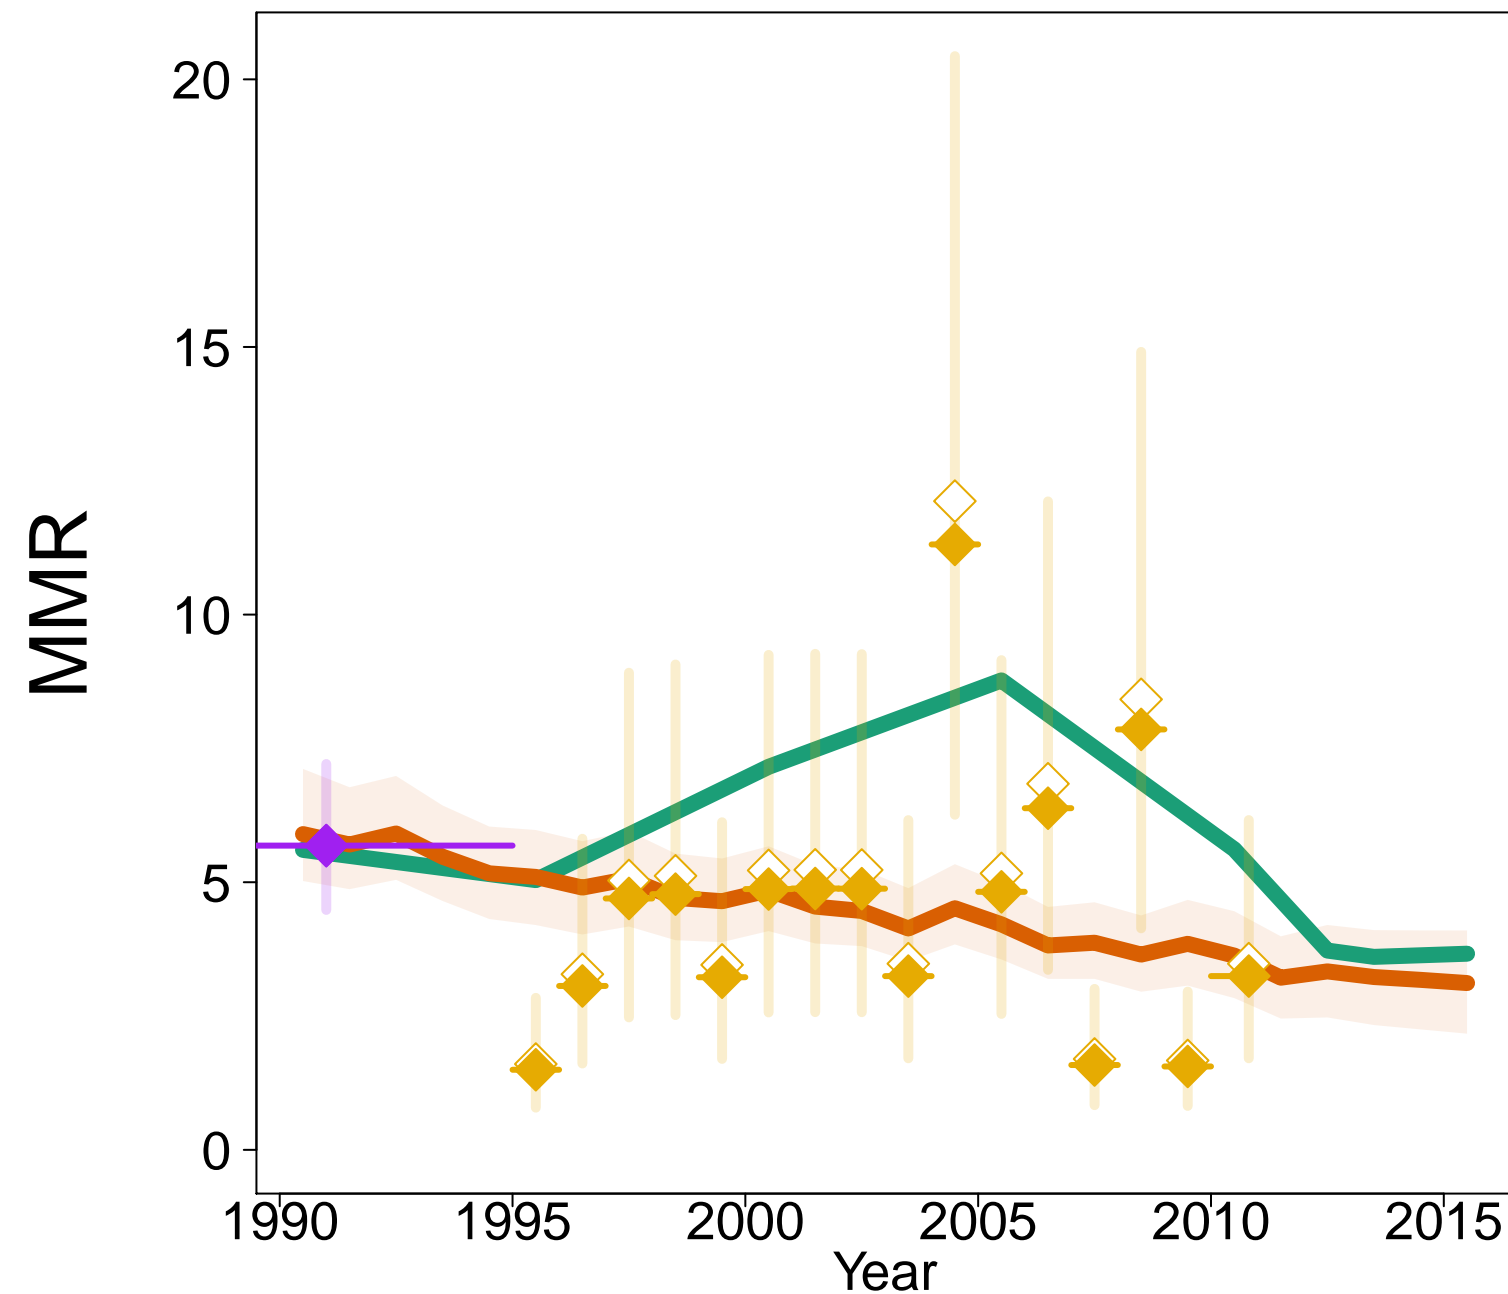

- Estimates –
- Bmat 2014
- MMEIG 2014
- Data –
- ◊ Observed Data
- ◆ Adjusted Data
- Data type –
- ◆ VR
- ◆ Spec. studies

France [FRA; A]  
(Developed regions)

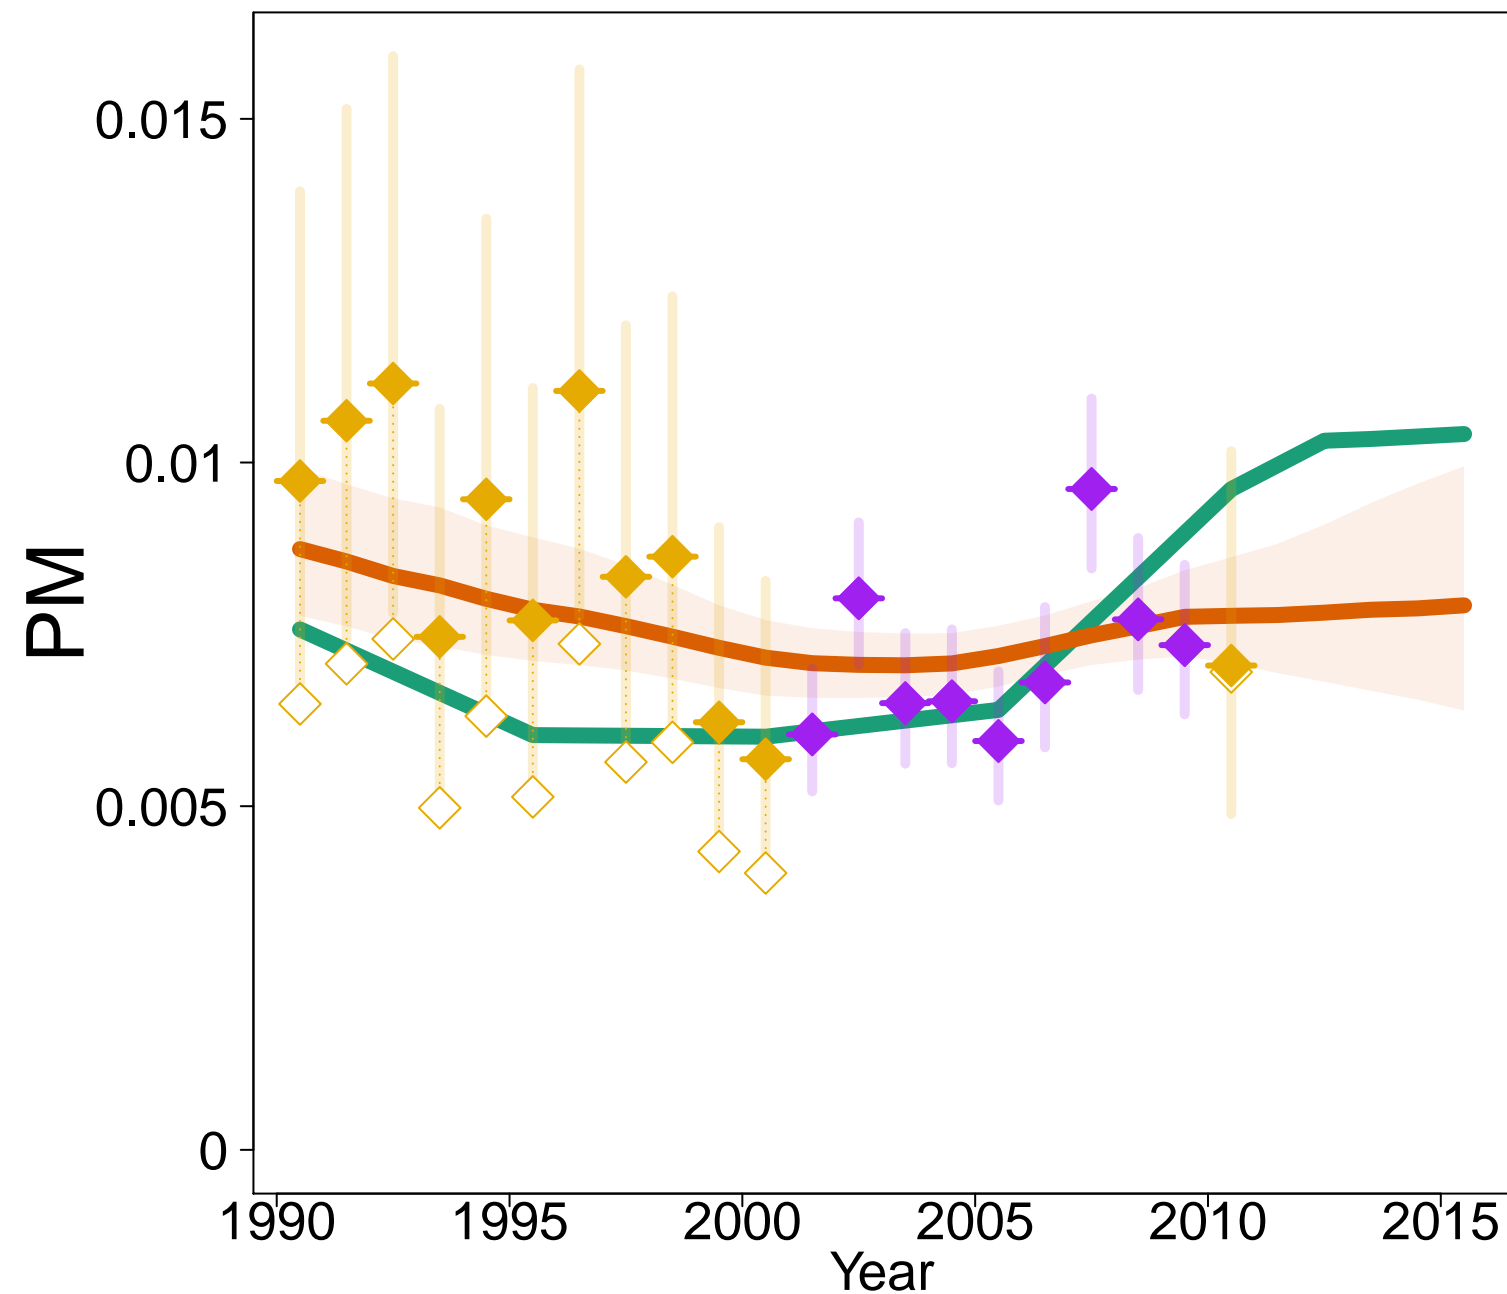

France [FRA; A]  
(Developed regions)

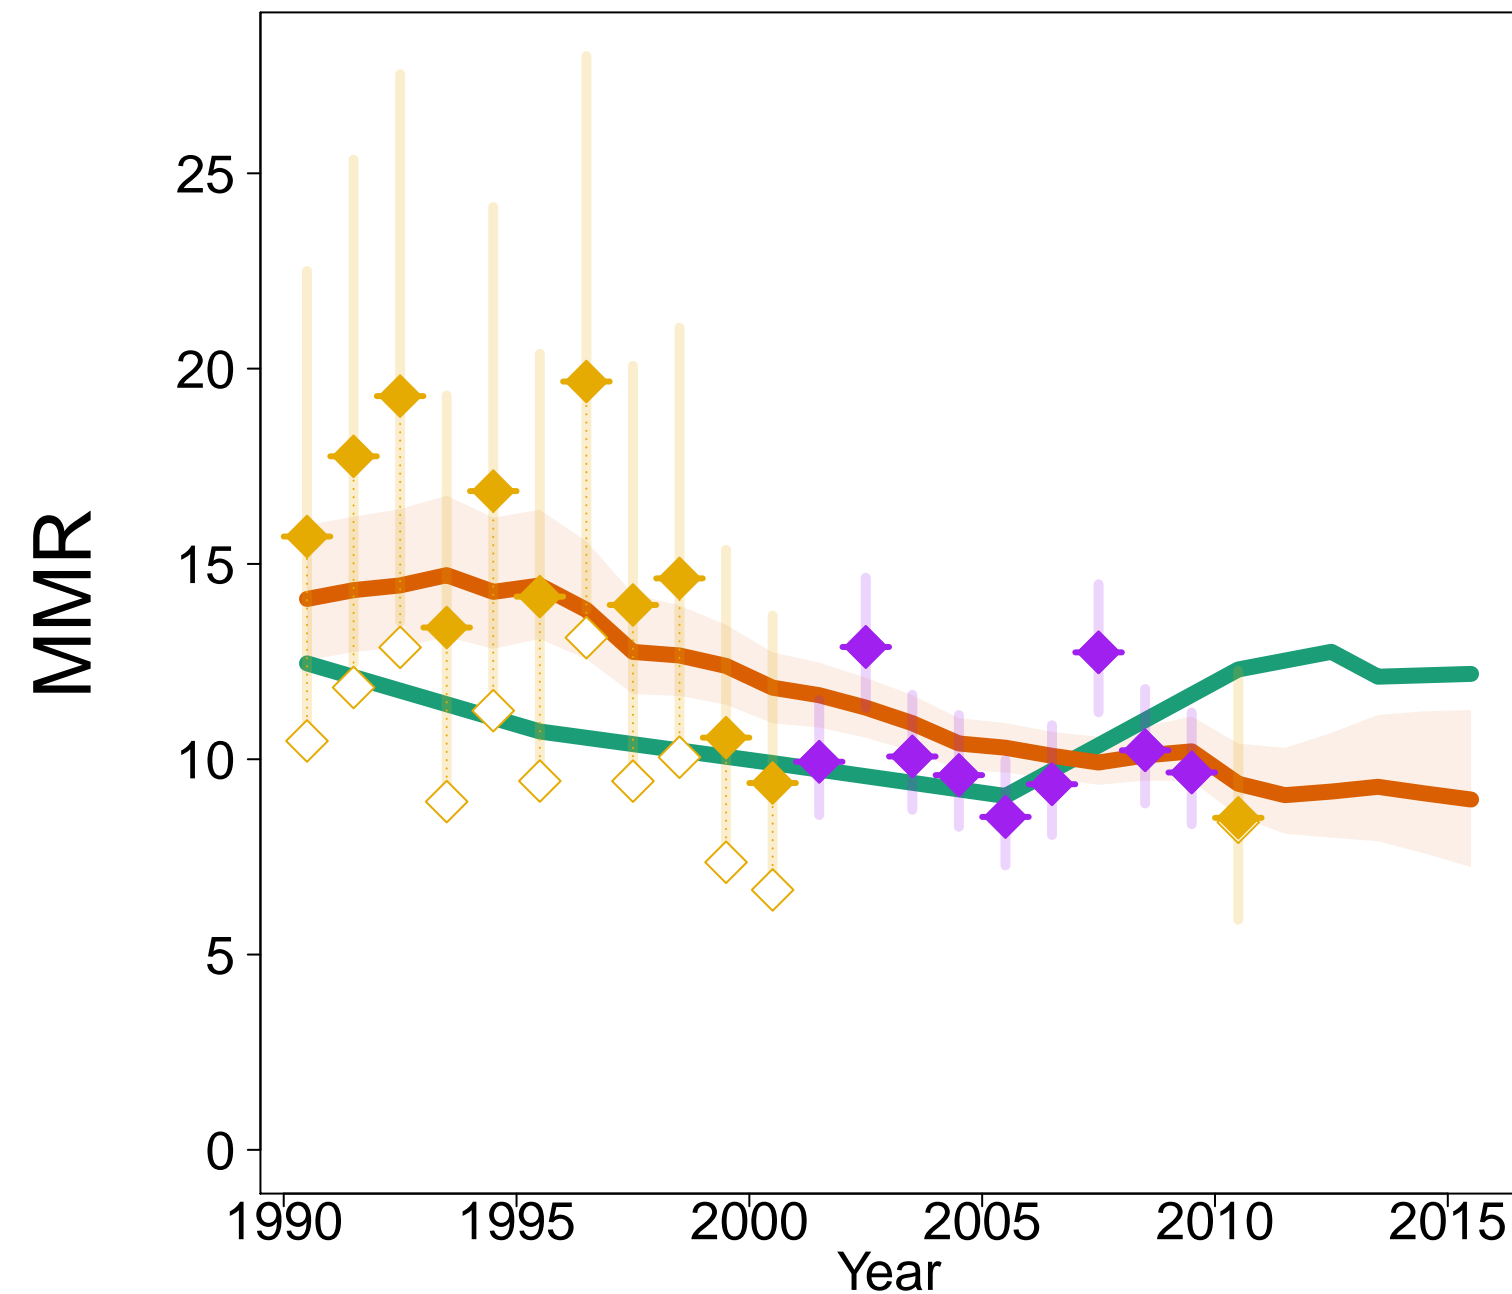

- Estimates –
- Bmat 2014
- MMEIG 2014
- Data –
- Observed Data
- Adjusted Data
- Data type –
- VR
- Spec. studies

Gabon [GAB; B]  
(Middle Africa)

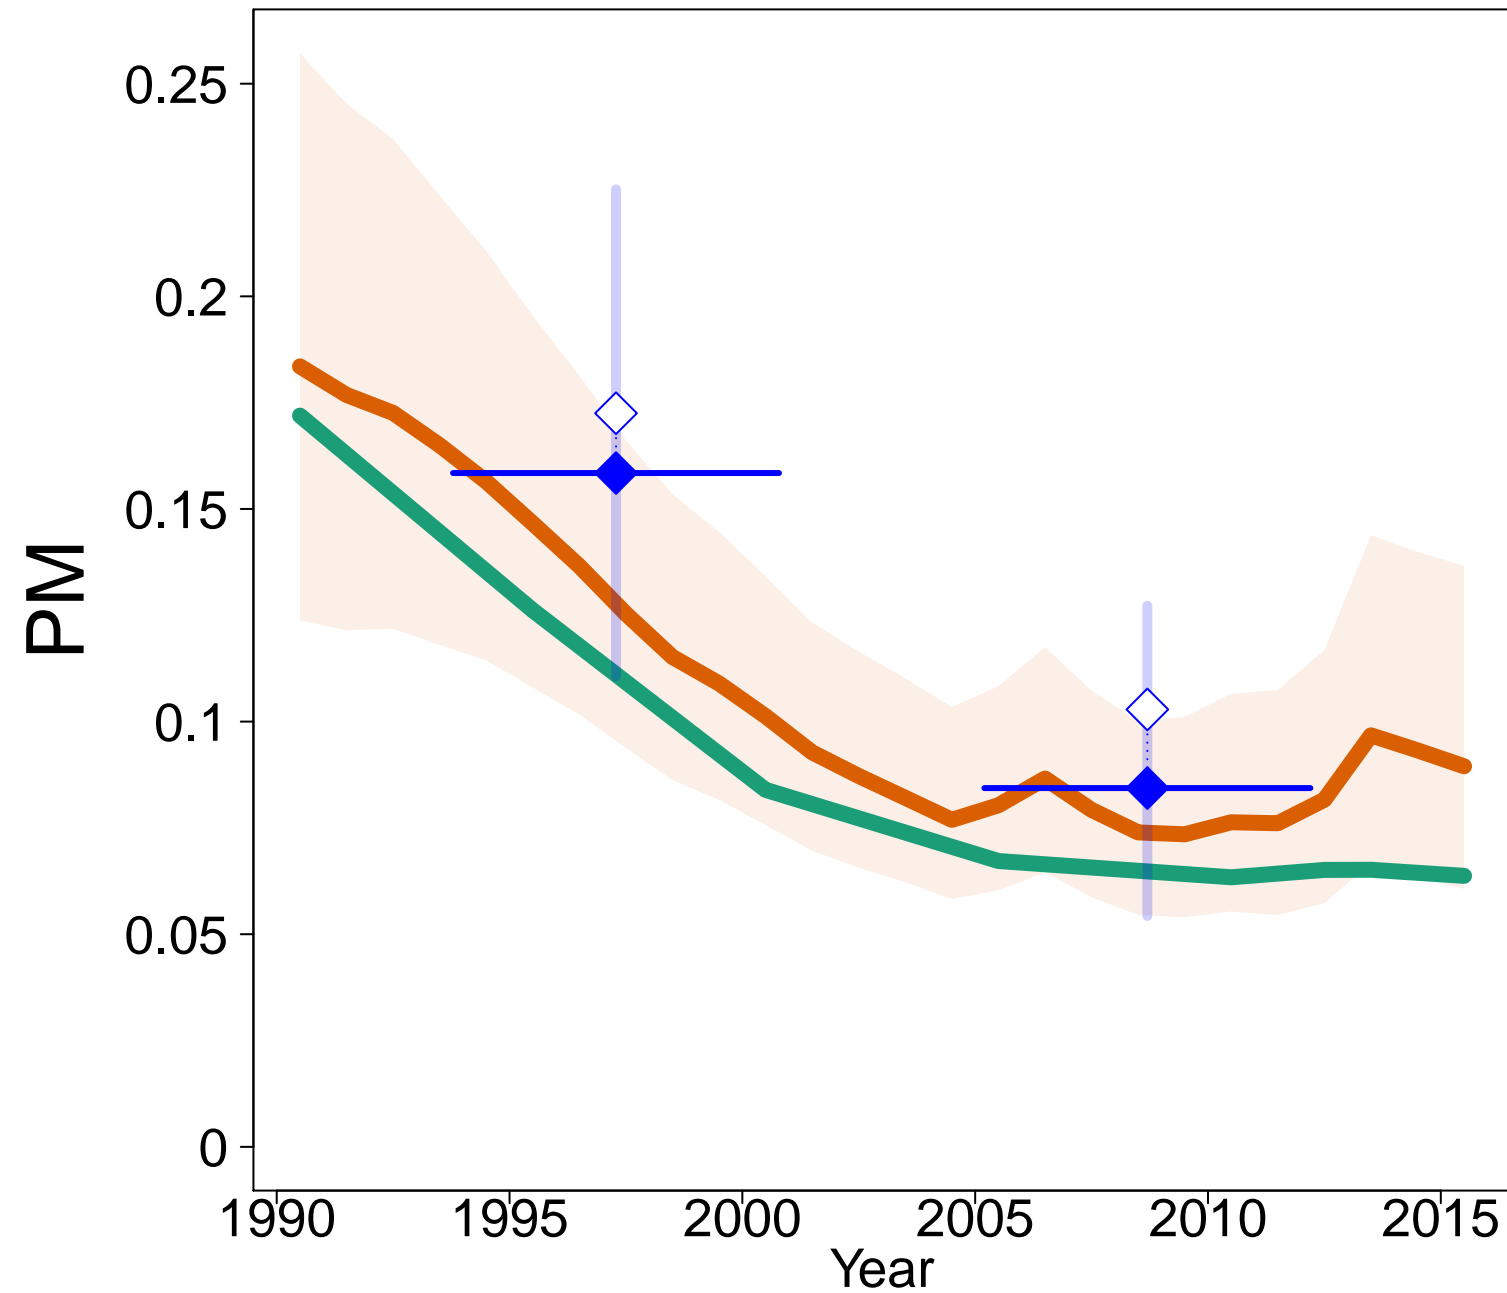

Gabon [GAB; B]  
(Middle Africa)

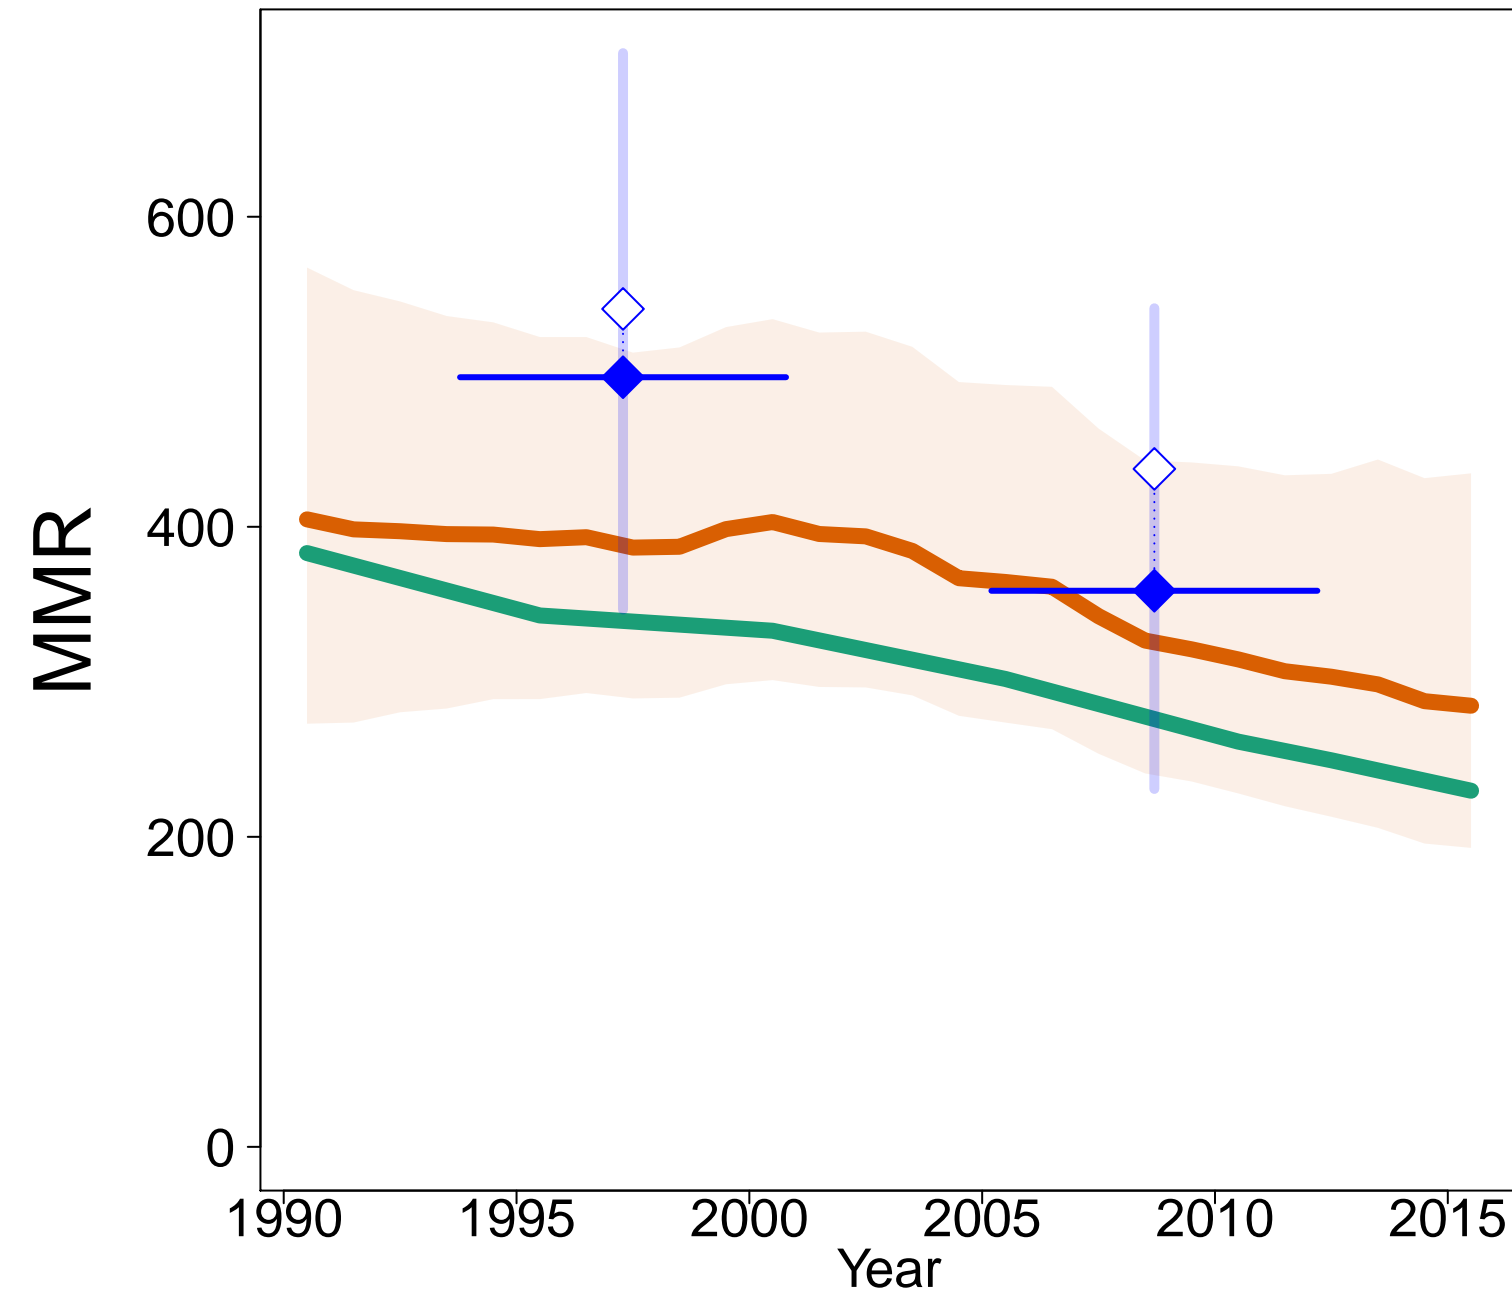

- Estimates –
- Bmat 2014
- MMEIG 2014
- Data –
- Observed Data
- Adjusted Data
- Data type –
- DHS

Gambia [GMB; C]  
(Western Africa)

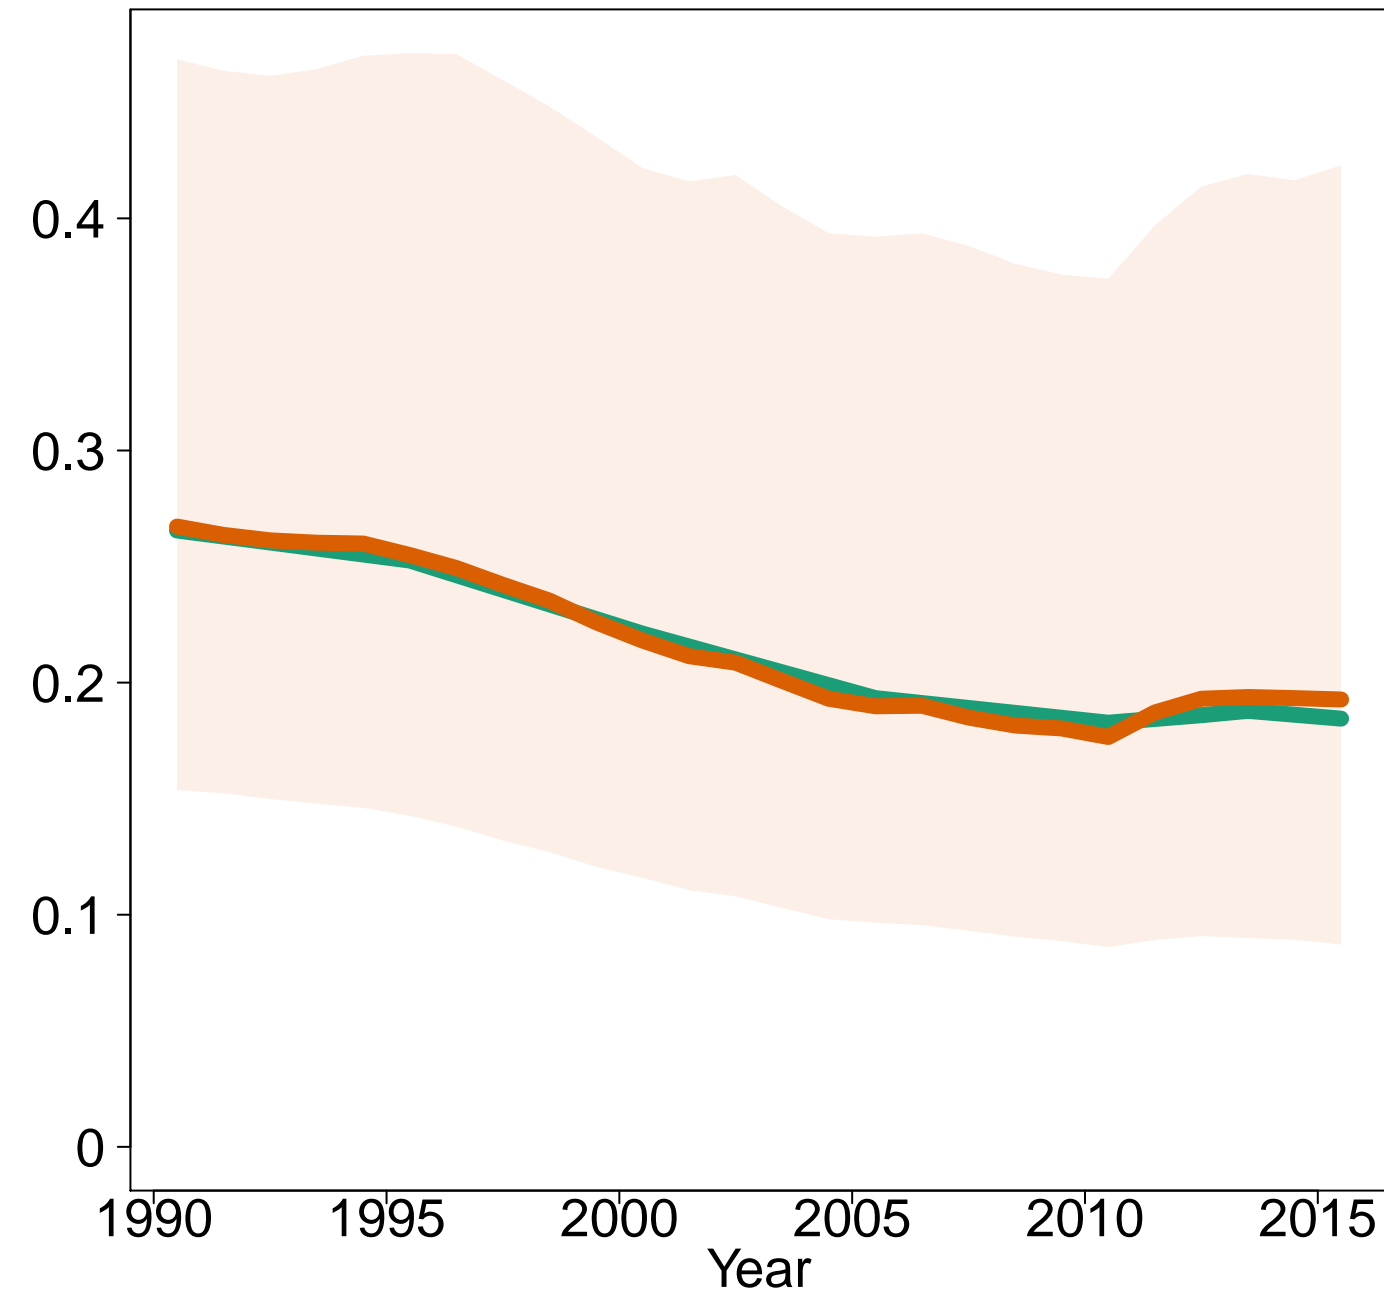

Gambia [GMB; C]  
(Western Africa)

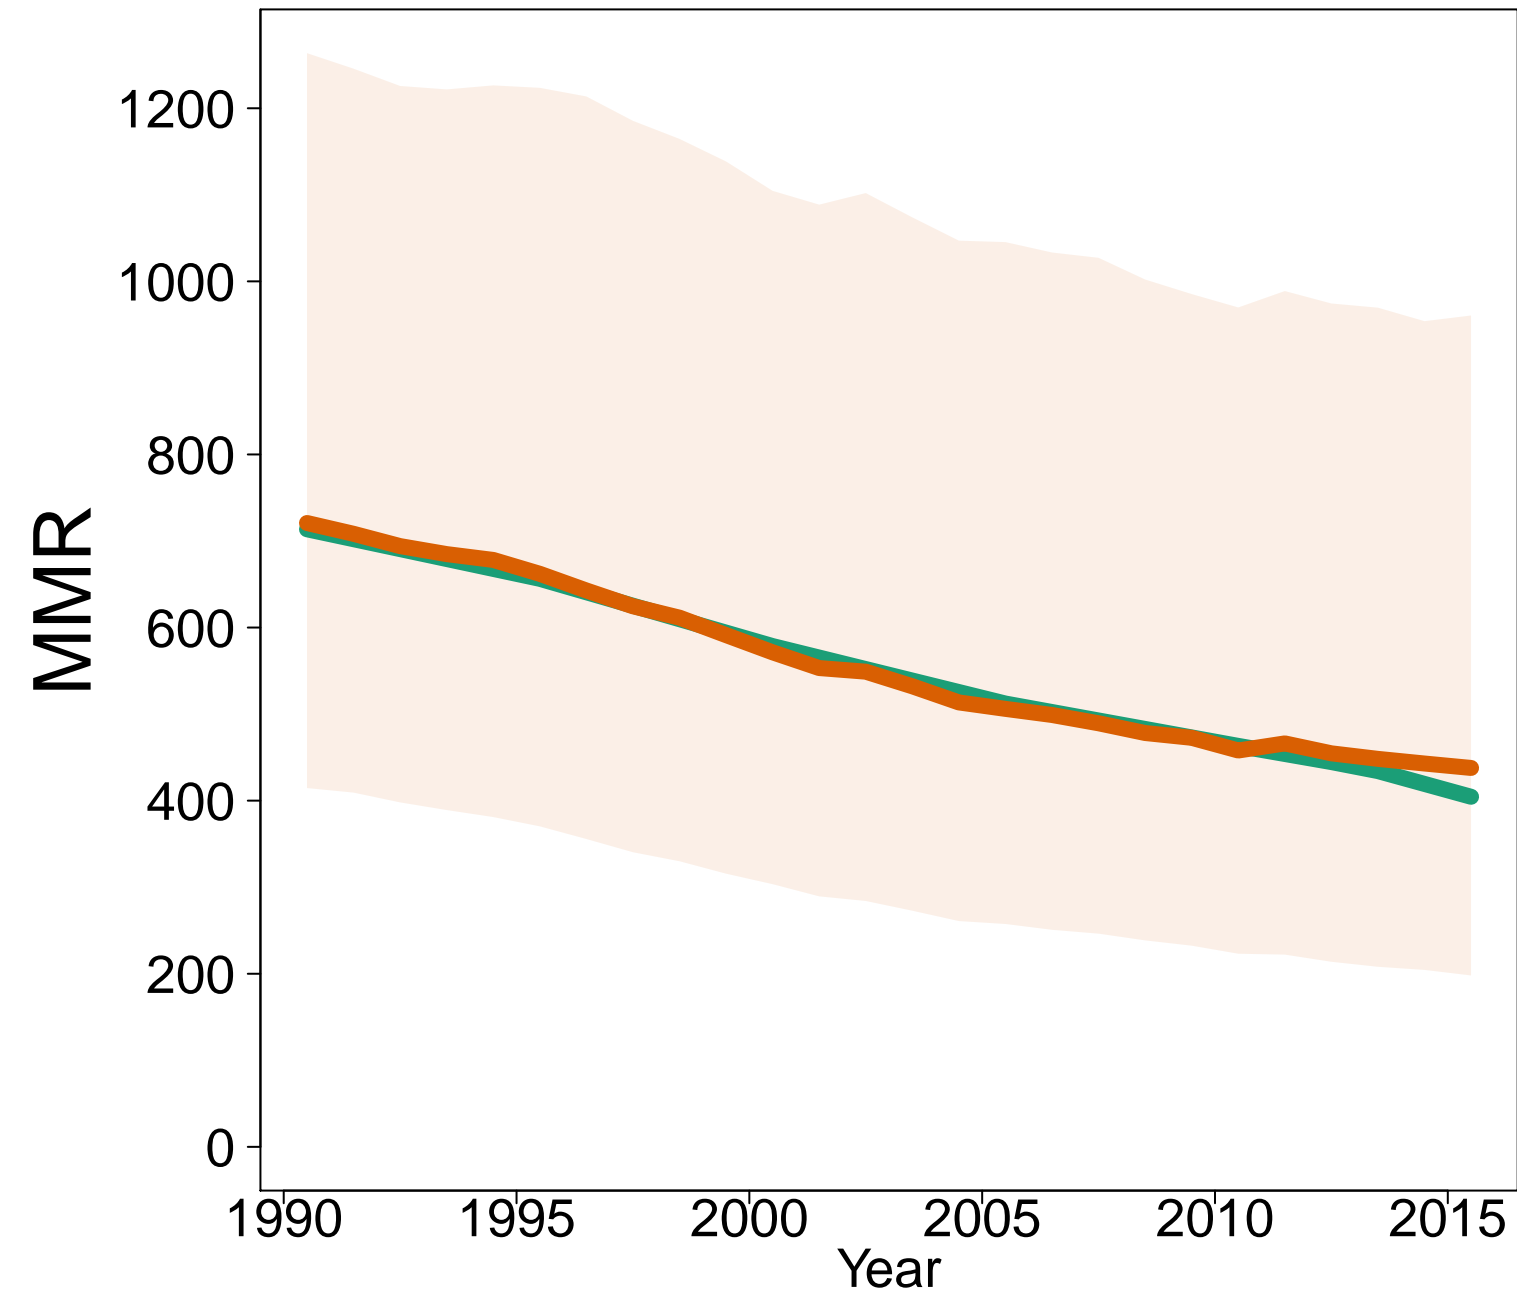

– Estimates –  
Bmat 2014  
MMEIG 2014  
– Data –

Georgia [GEO; B]  
(Western Asia)

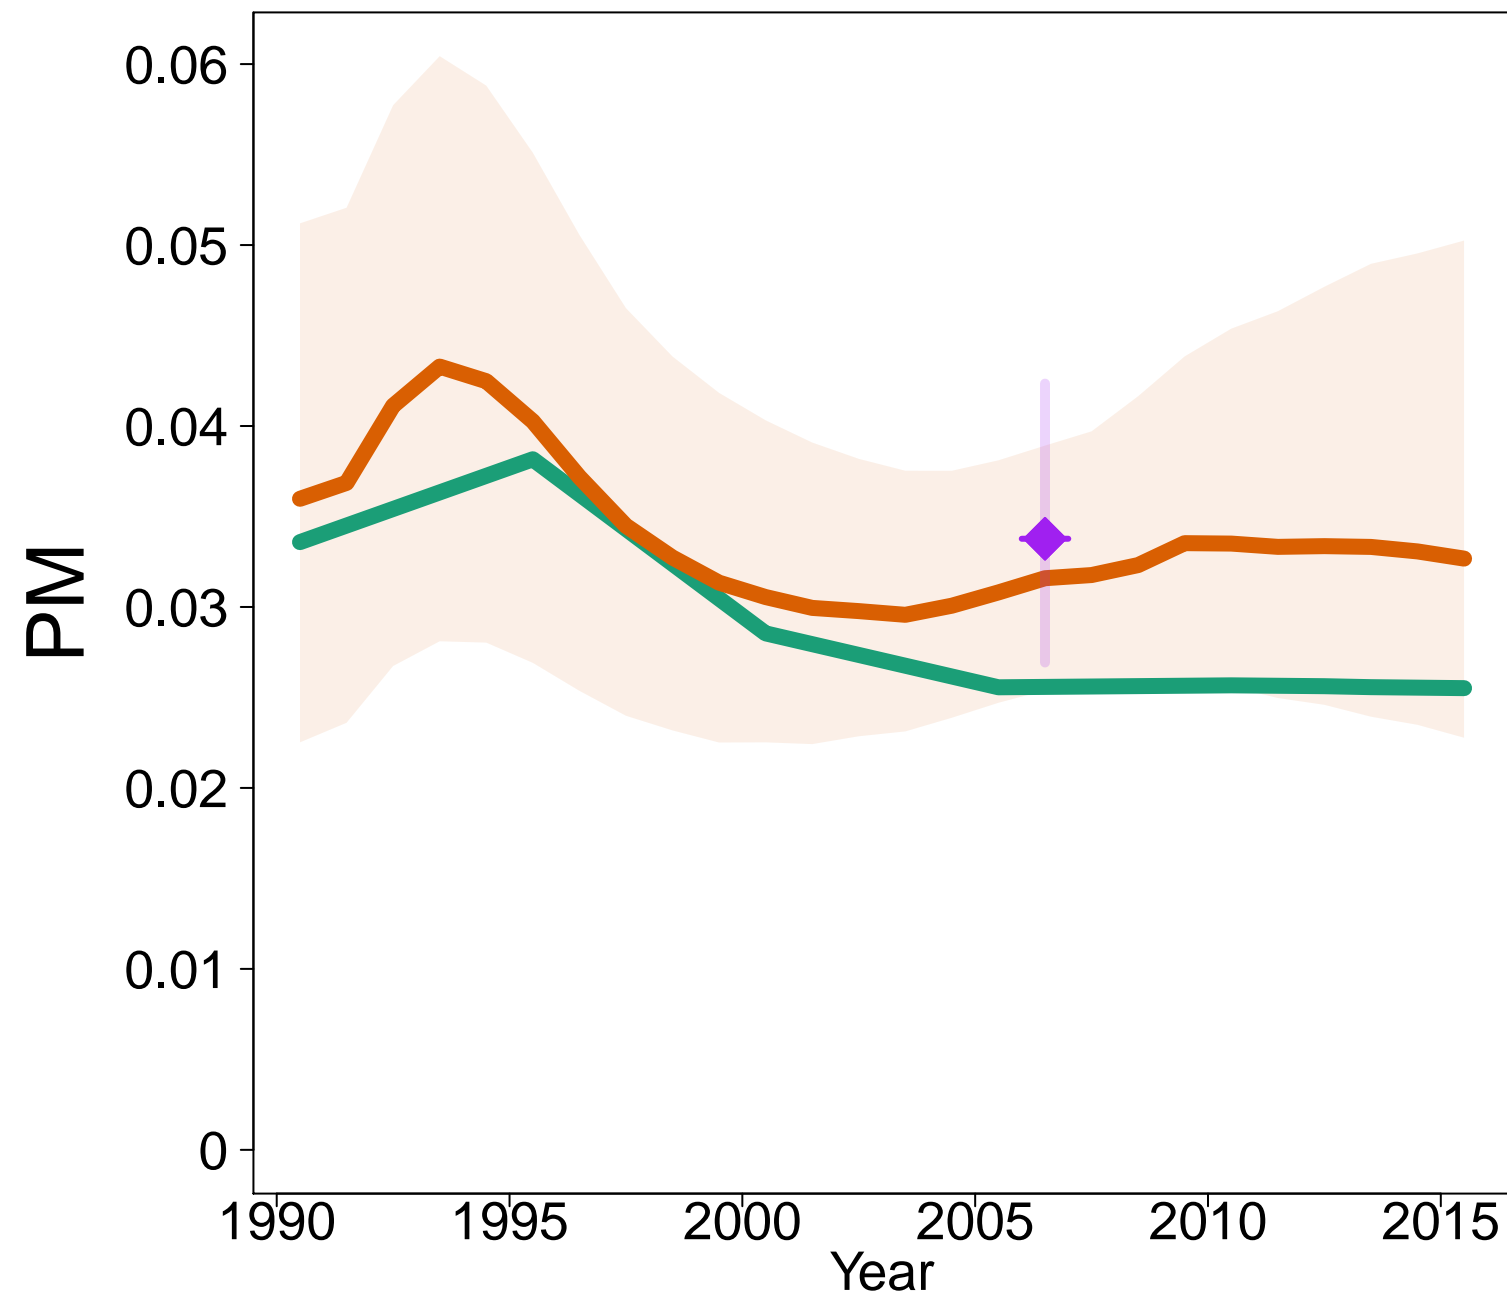

Georgia [GEO; B]  
(Western Asia)

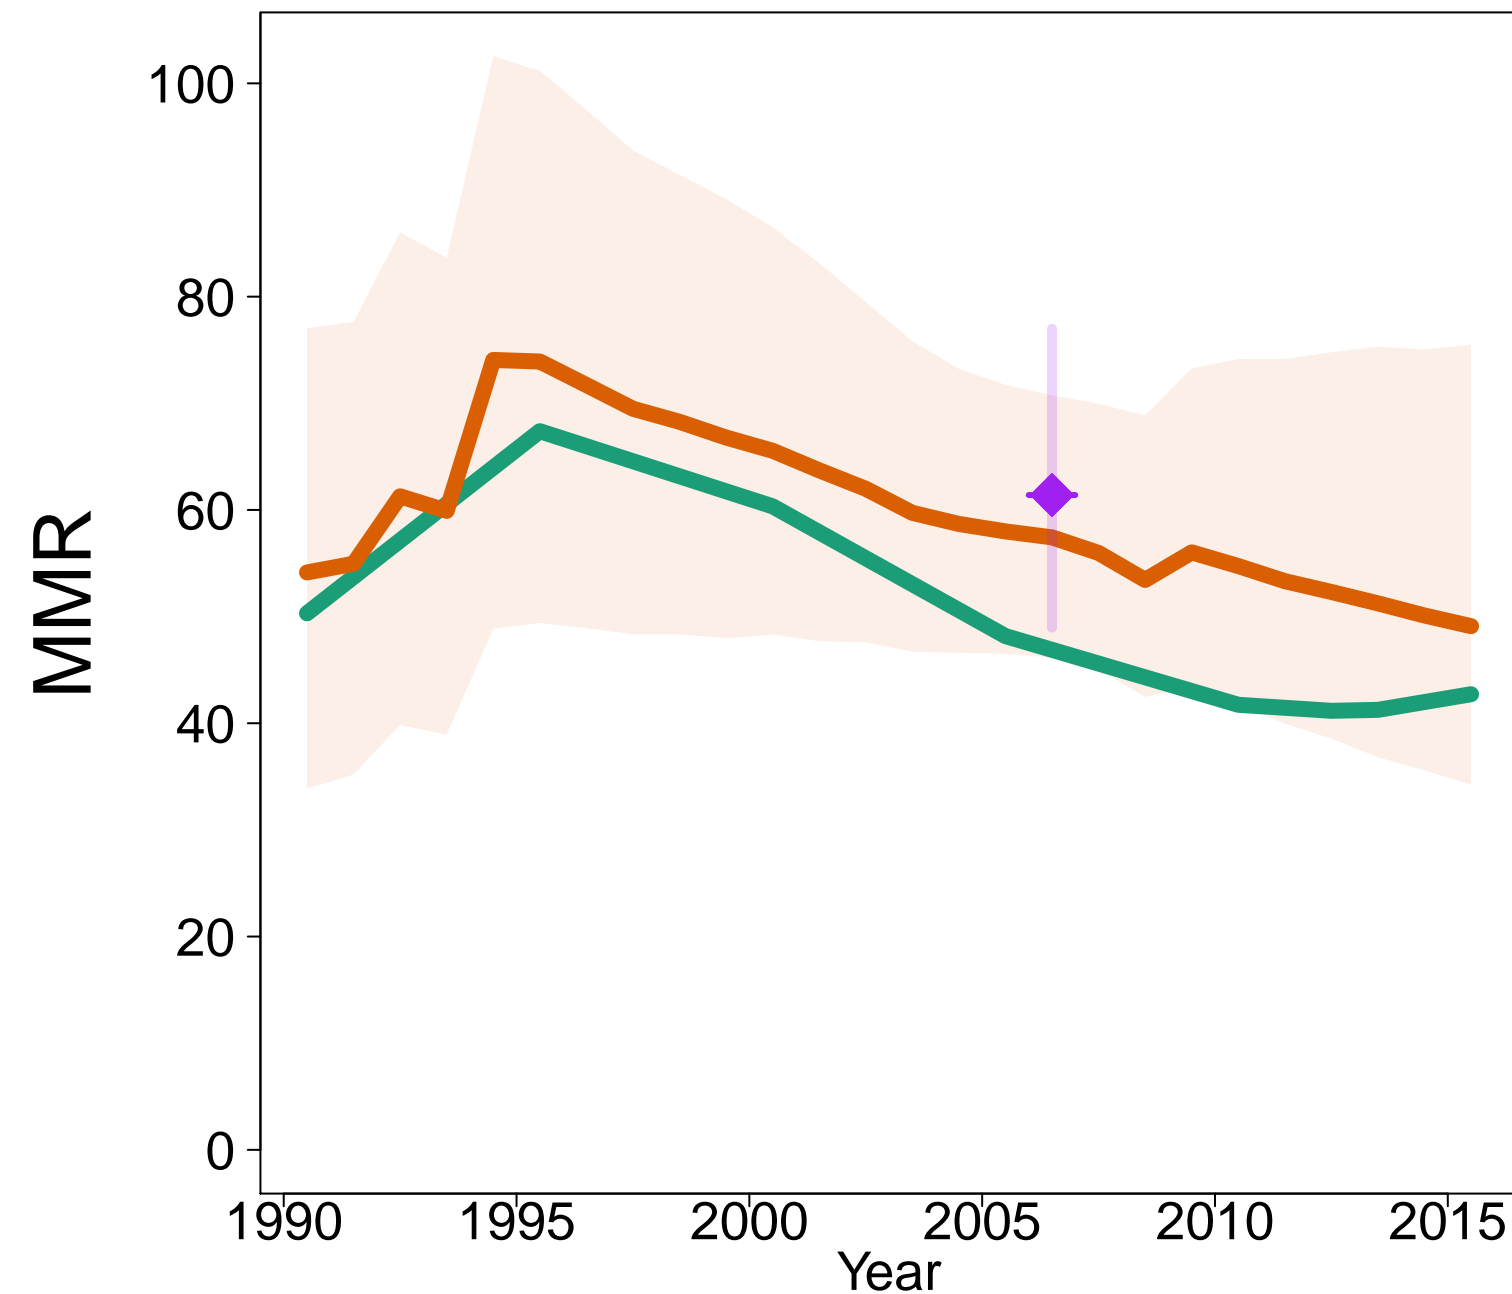

- Estimates –
- Bmat 2014
- MMEIG 2014
- Data –
- Observed Data
- Adjusted Data
- Data type –
- Spec. studies

Germany [DEU; A]  
(Developed regions)

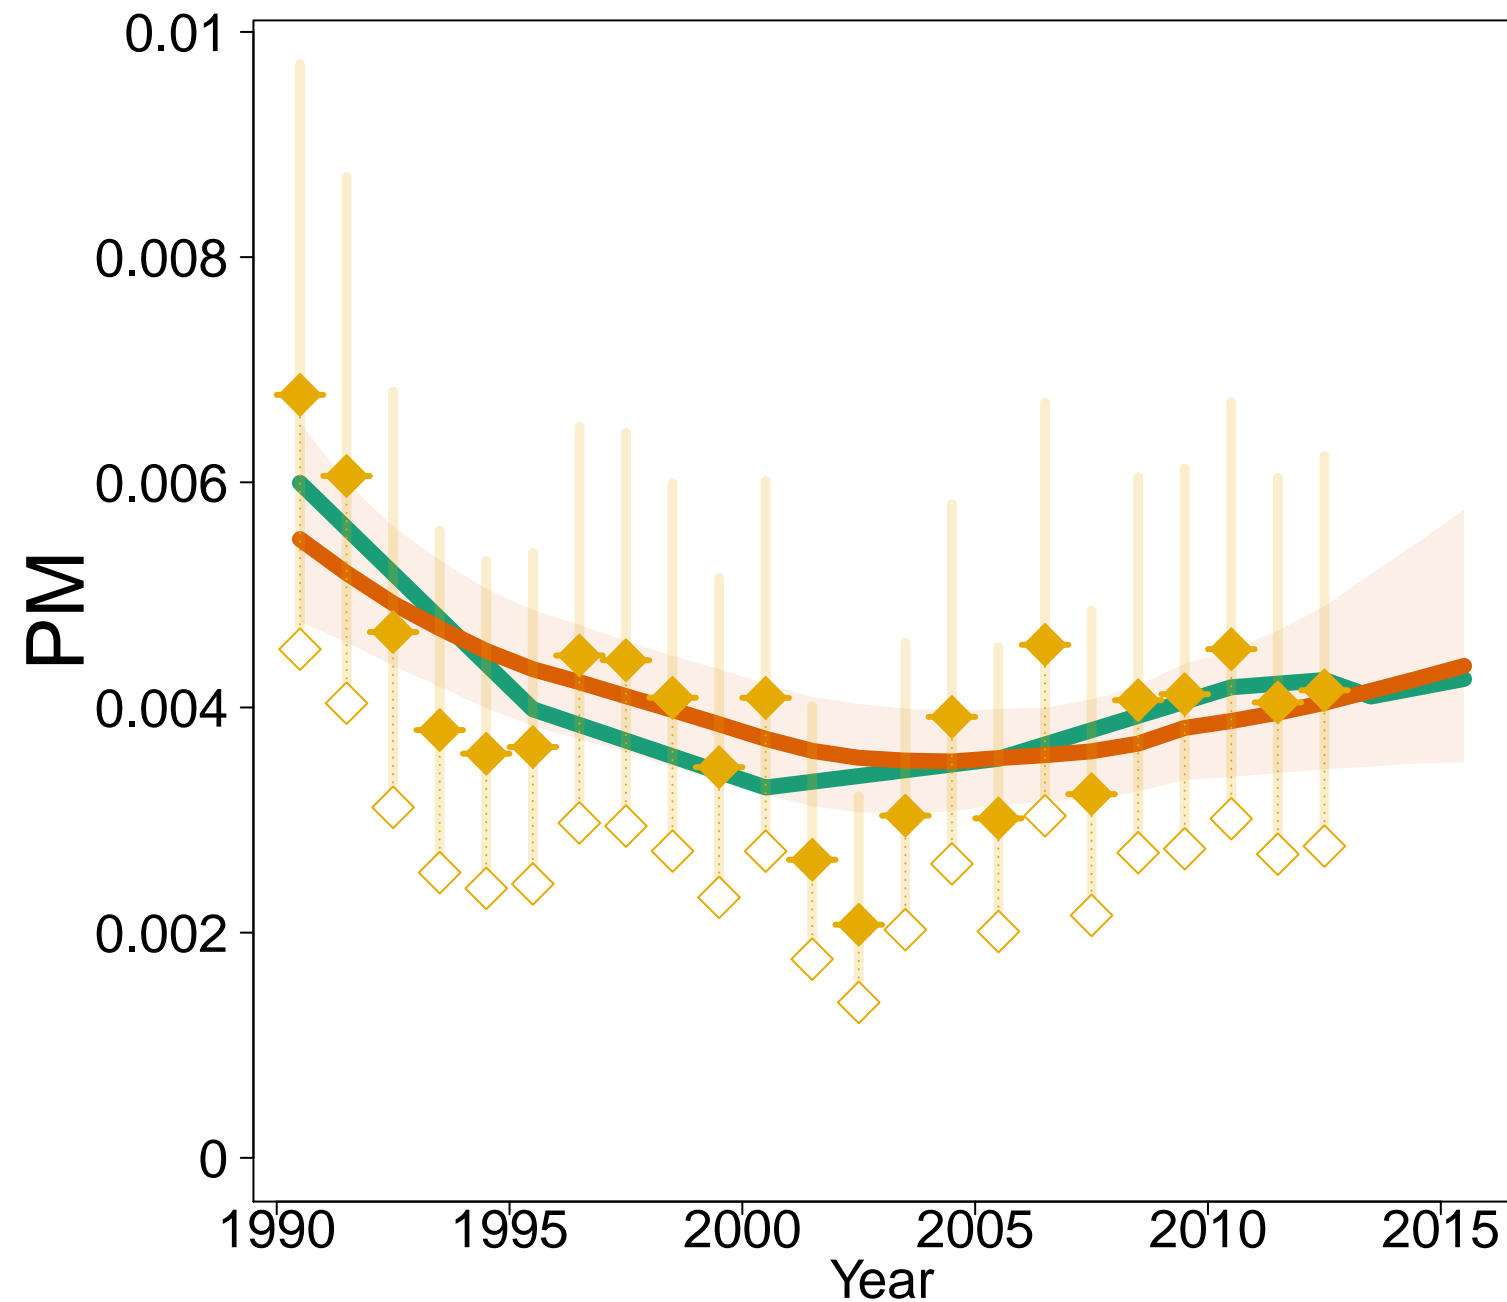

Germany [DEU; A]  
(Developed regions)

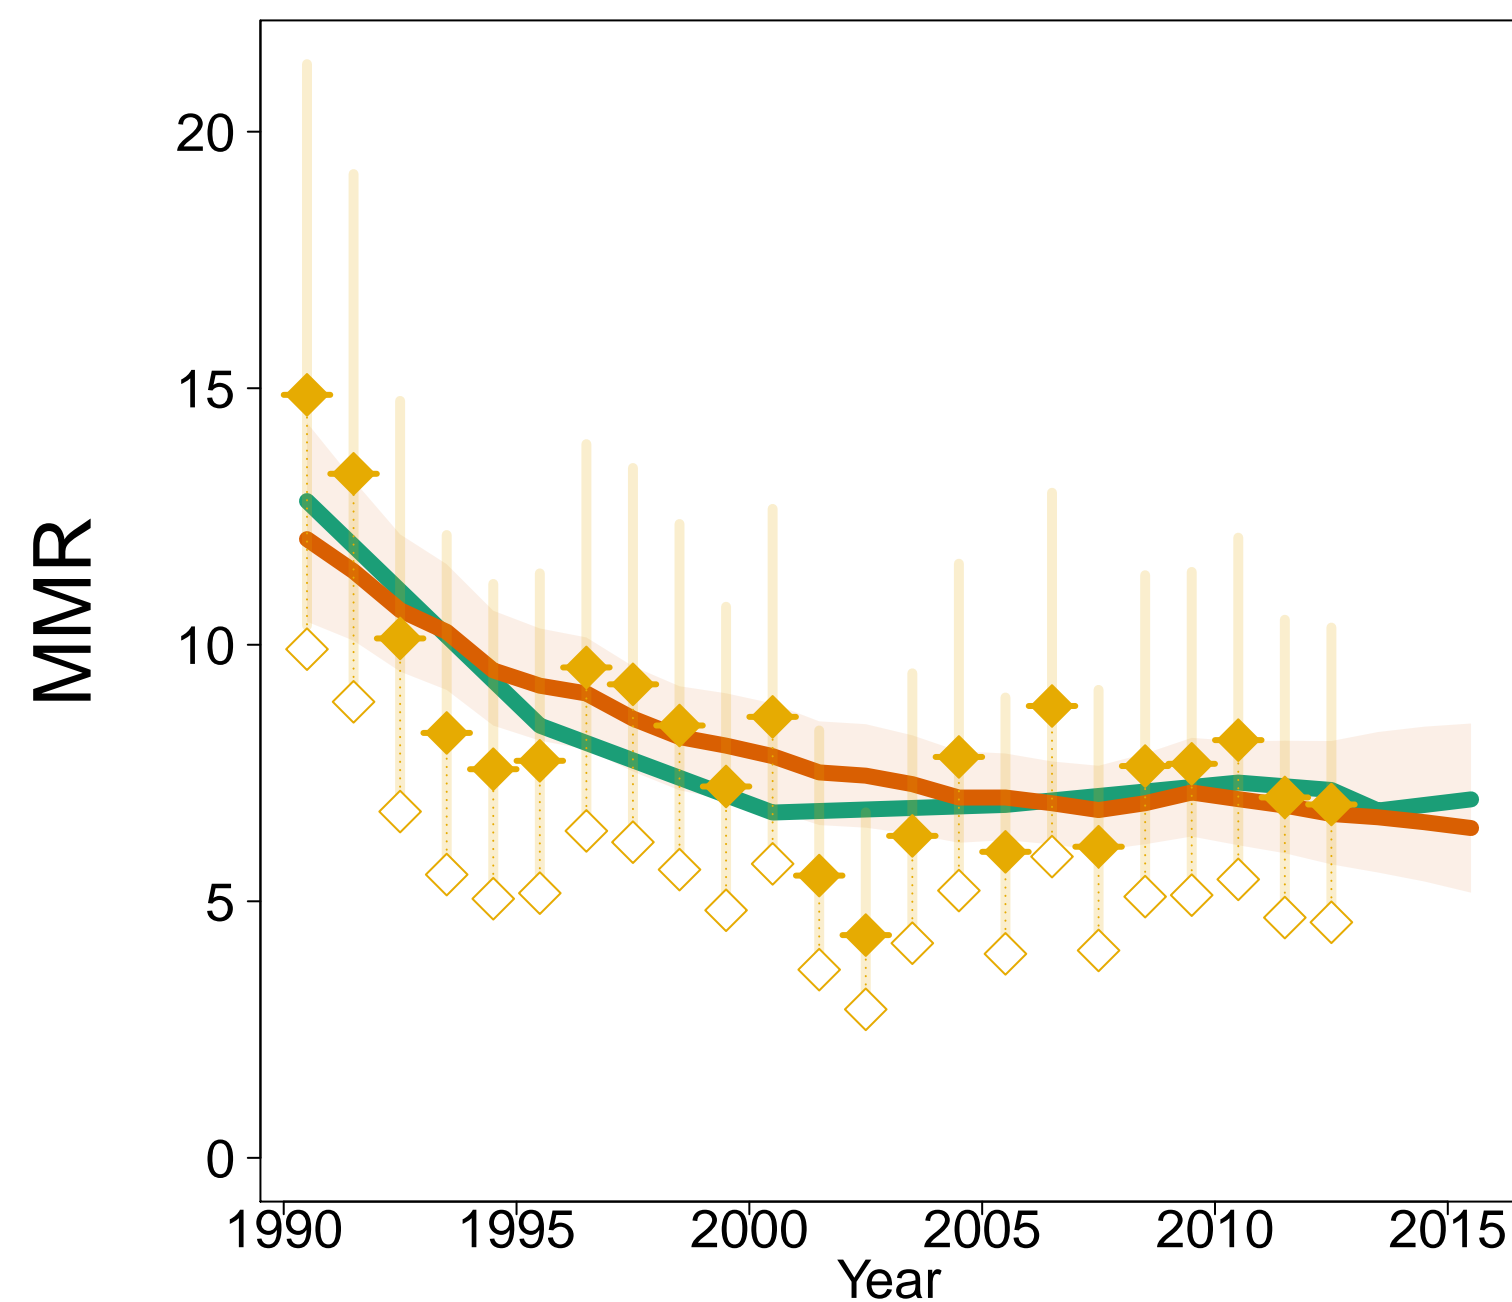

- Estimates –
- Bmat 2014
- MMEIG 2014
- Data –
- Observed Data
- Adjusted Data
- Data type –
- VR

Ghana [GHA; B]  
(Western Africa)

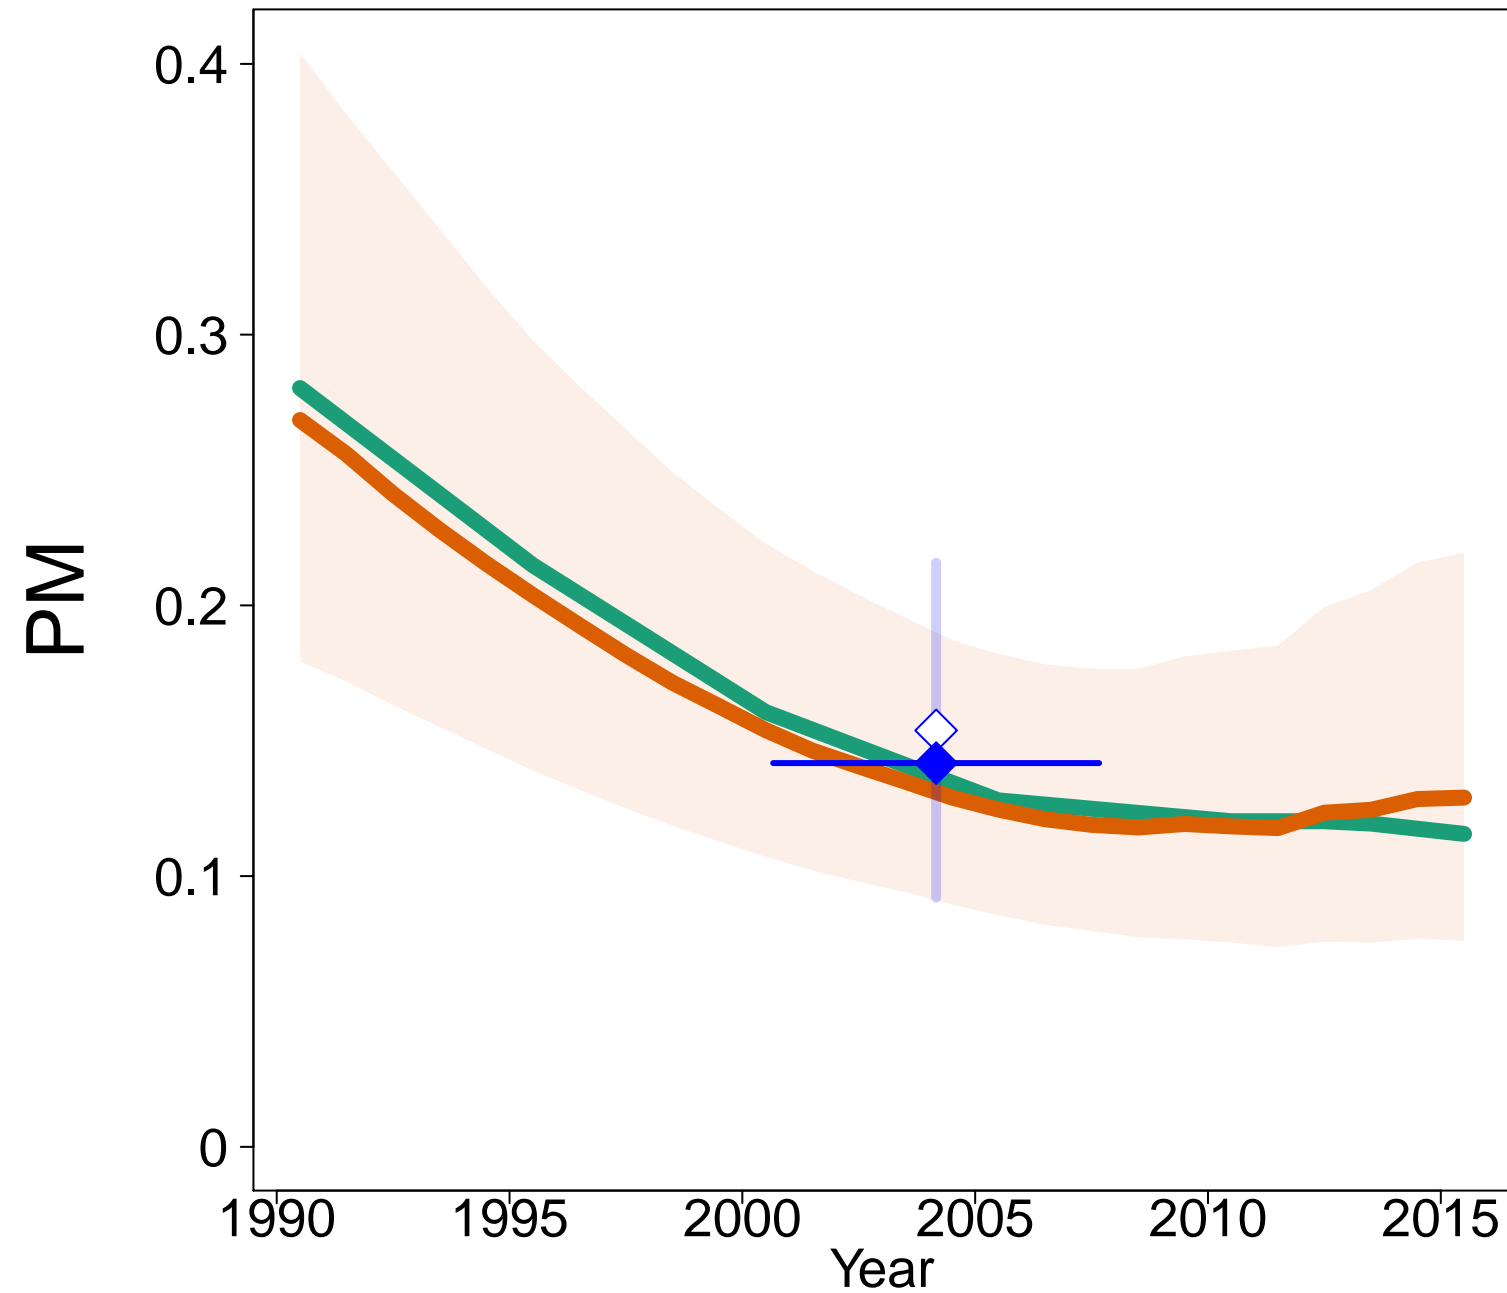

Ghana [GHA; B]  
(Western Africa)

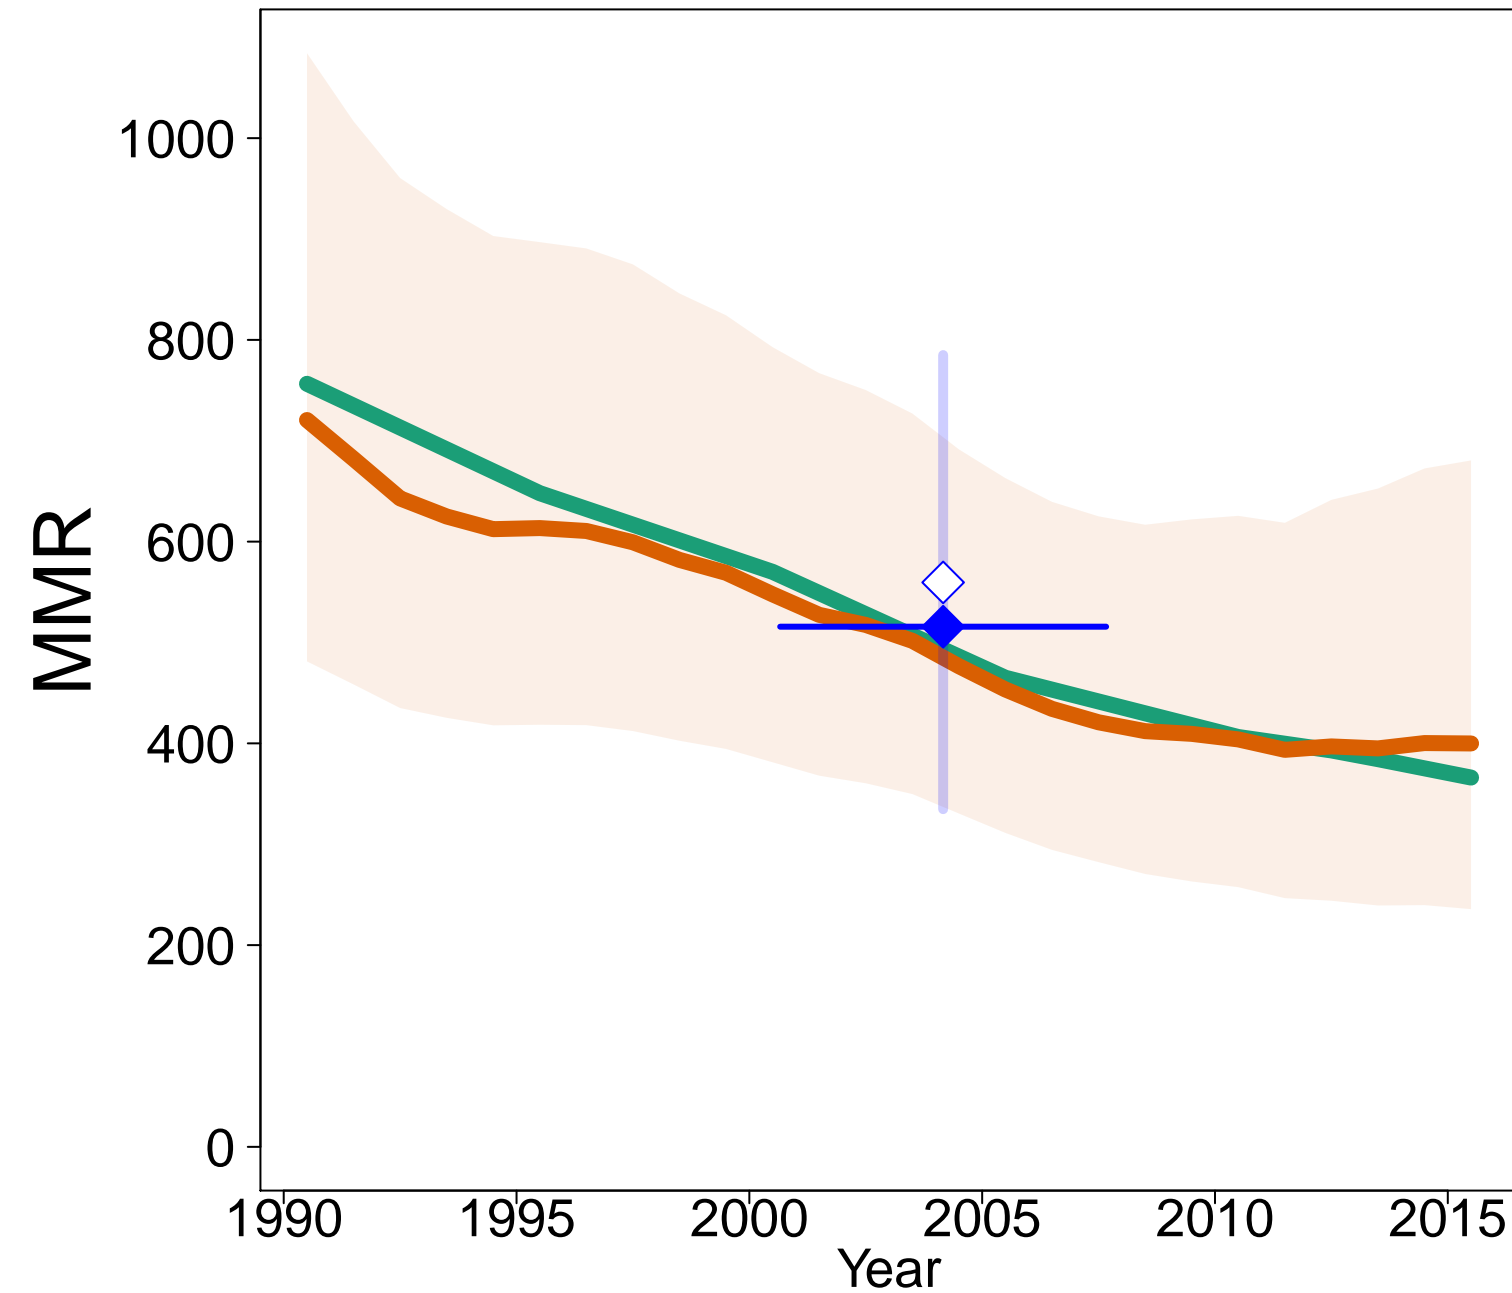

- Estimates –
- Bmat 2014
- MMEIG 2014
- Data –
- Observed Data
- Adjusted Data
- Data type –
- DHS

Greece [GRC; A]  
(Developed regions)

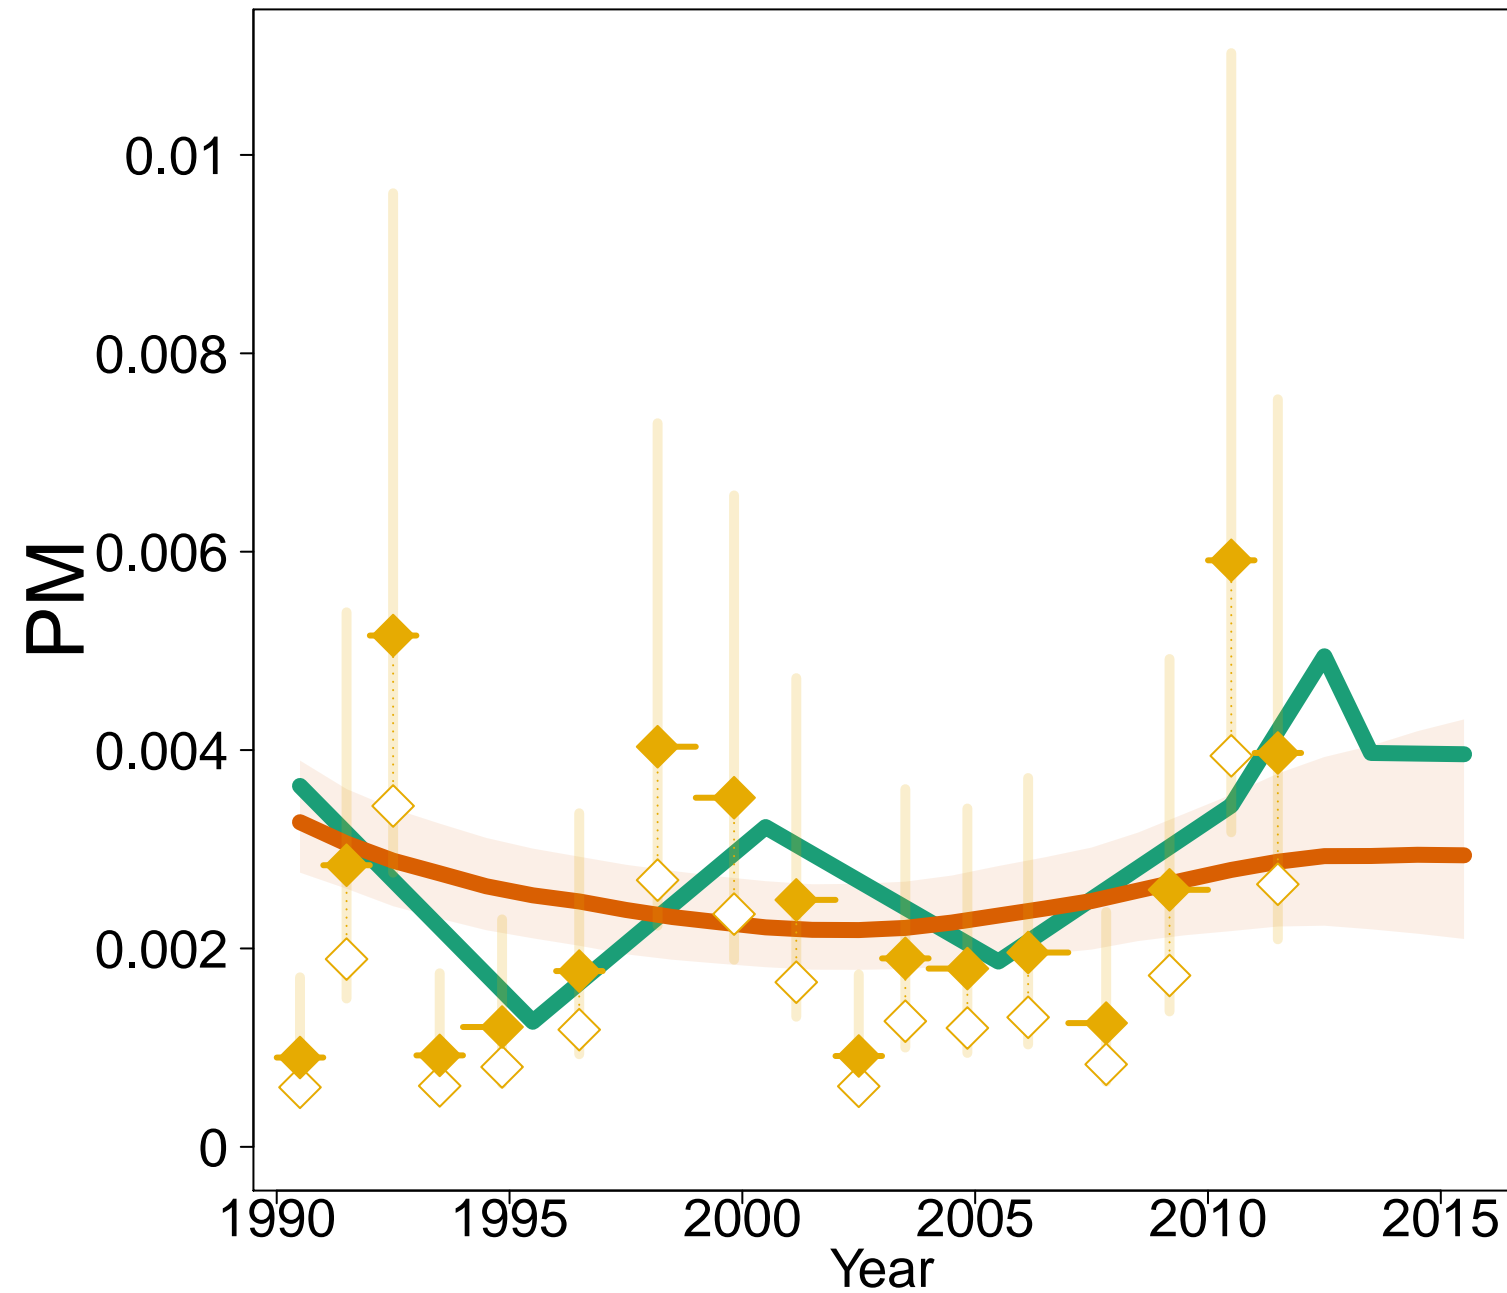

Greece [GRC; A]  
(Developed regions)

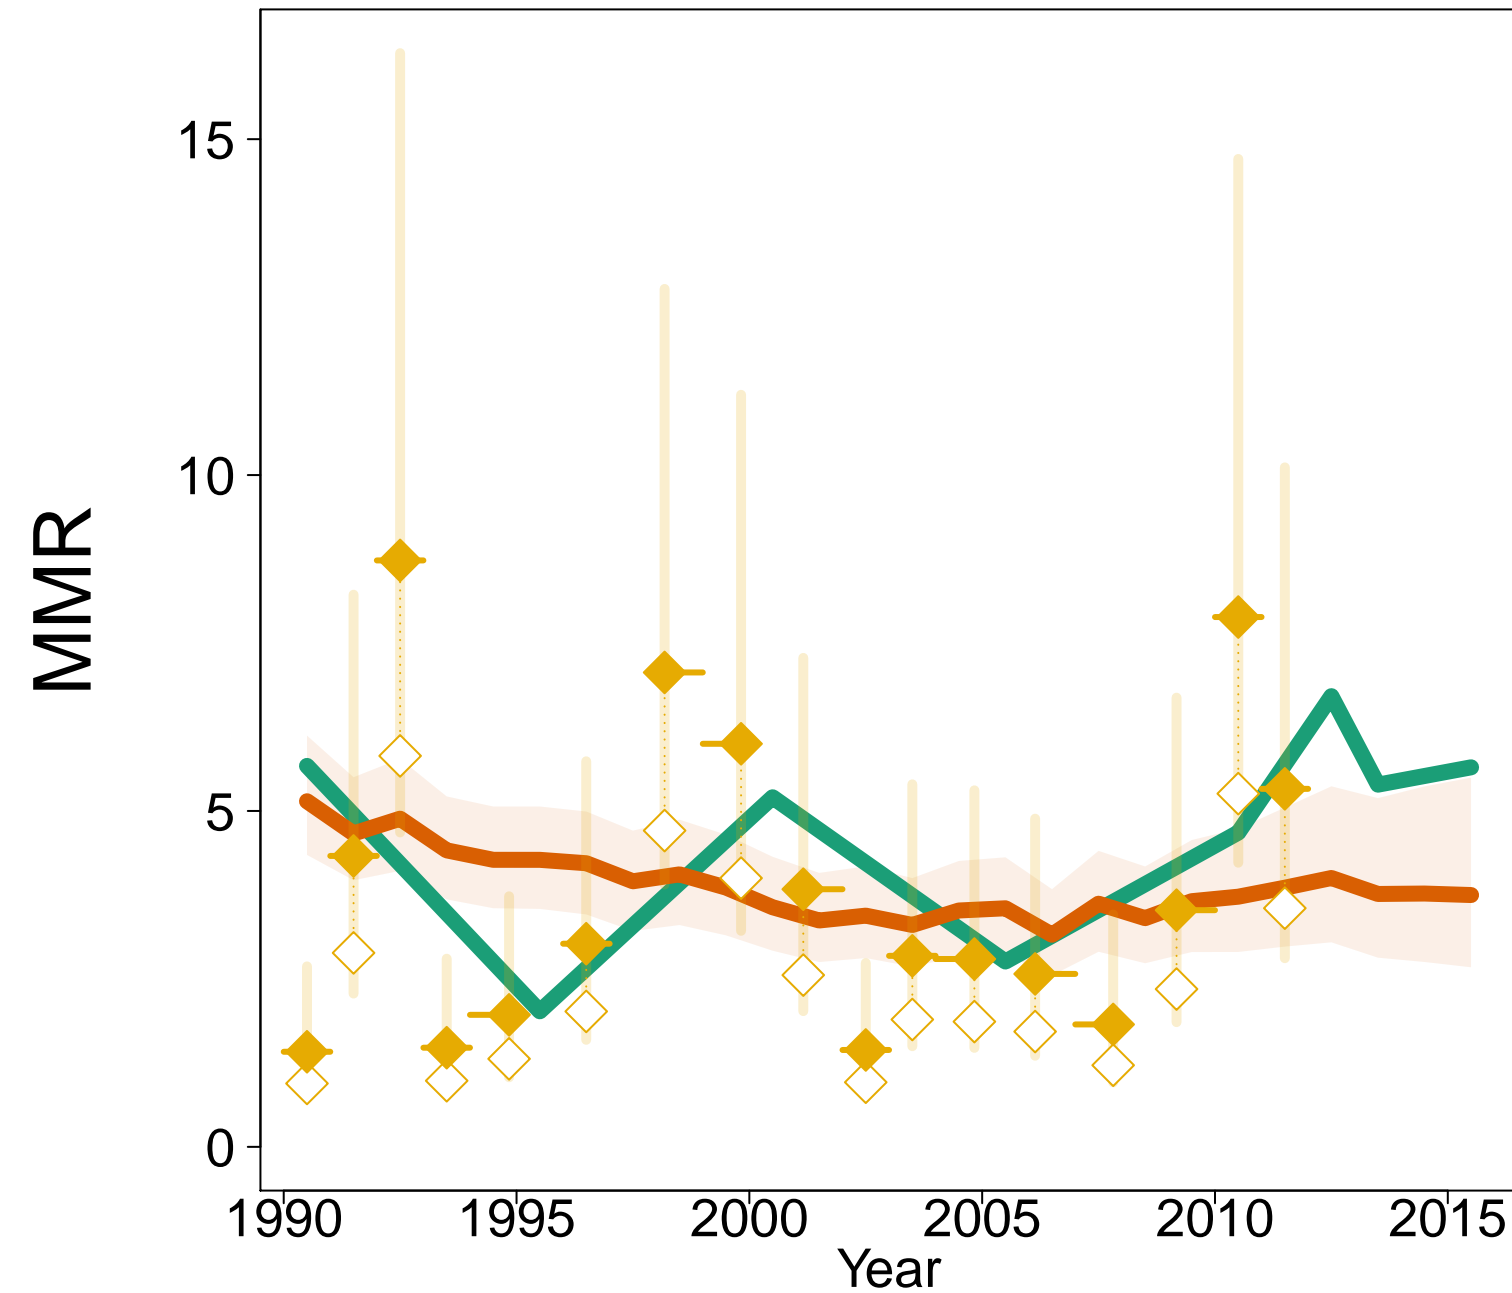

– Estimates –  
Bmat 2014  
MMEIG 2014  
– Data –  
Observed Data  
Adjusted Data  
– Data type –  
VR



Grenada [GRD; B]  
(Caribbean)

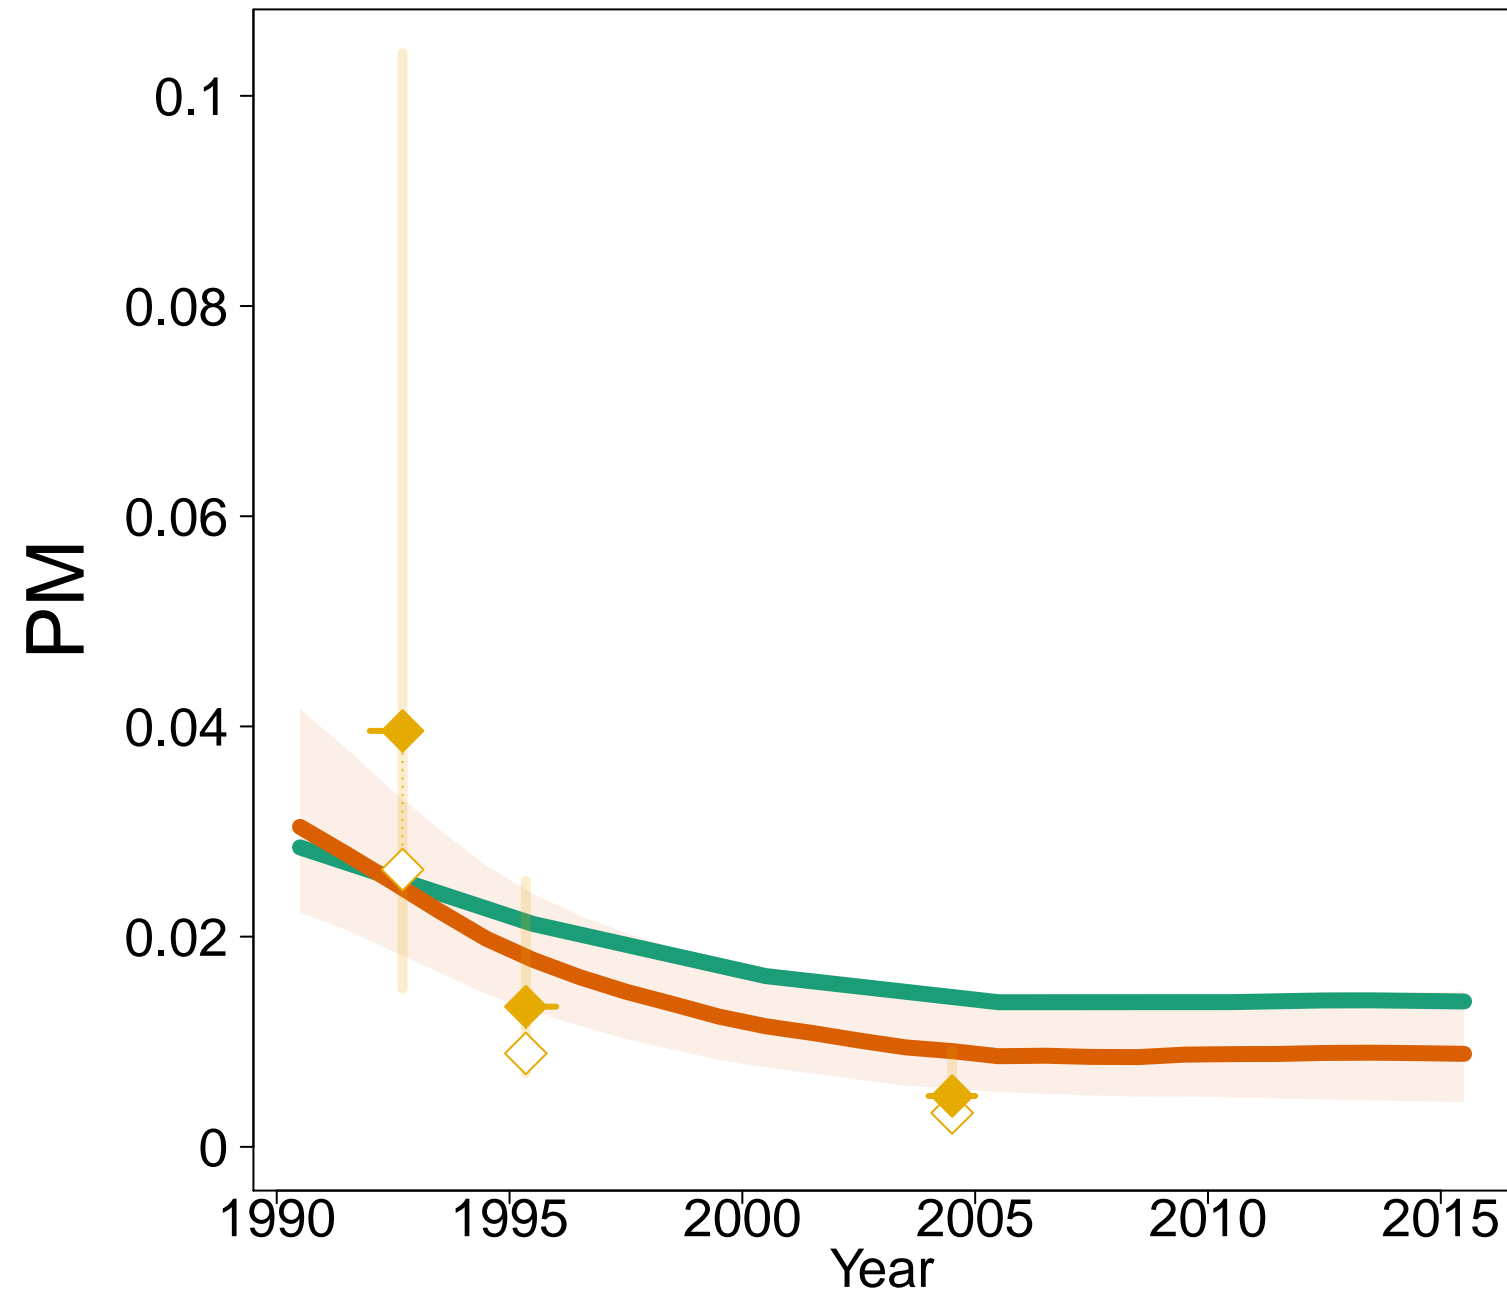

Grenada [GRD; B]  
(Caribbean)

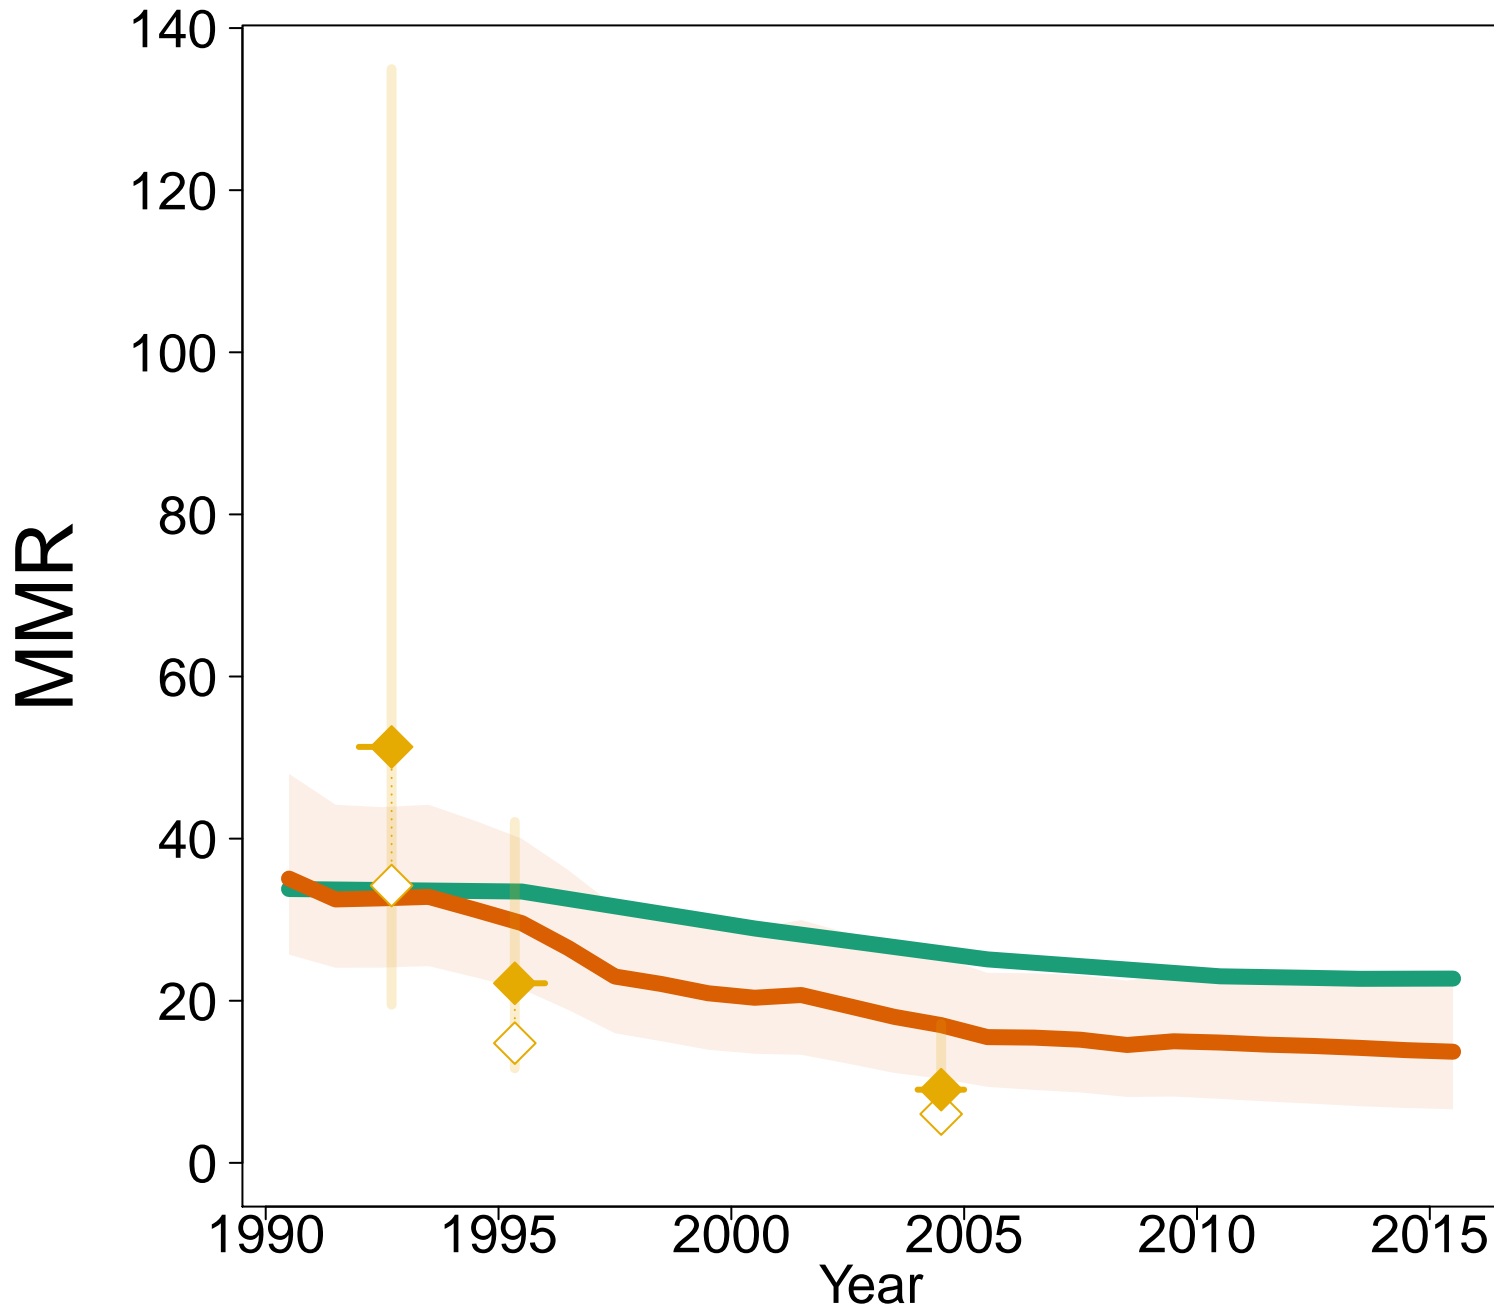

- Estimates –
- Bmat 2014
- MMEIG 2014
- Data –
- Observed Data
- Adjusted Data
- Data type –
- VR

Guatemala [GTM; A]  
(Central America)

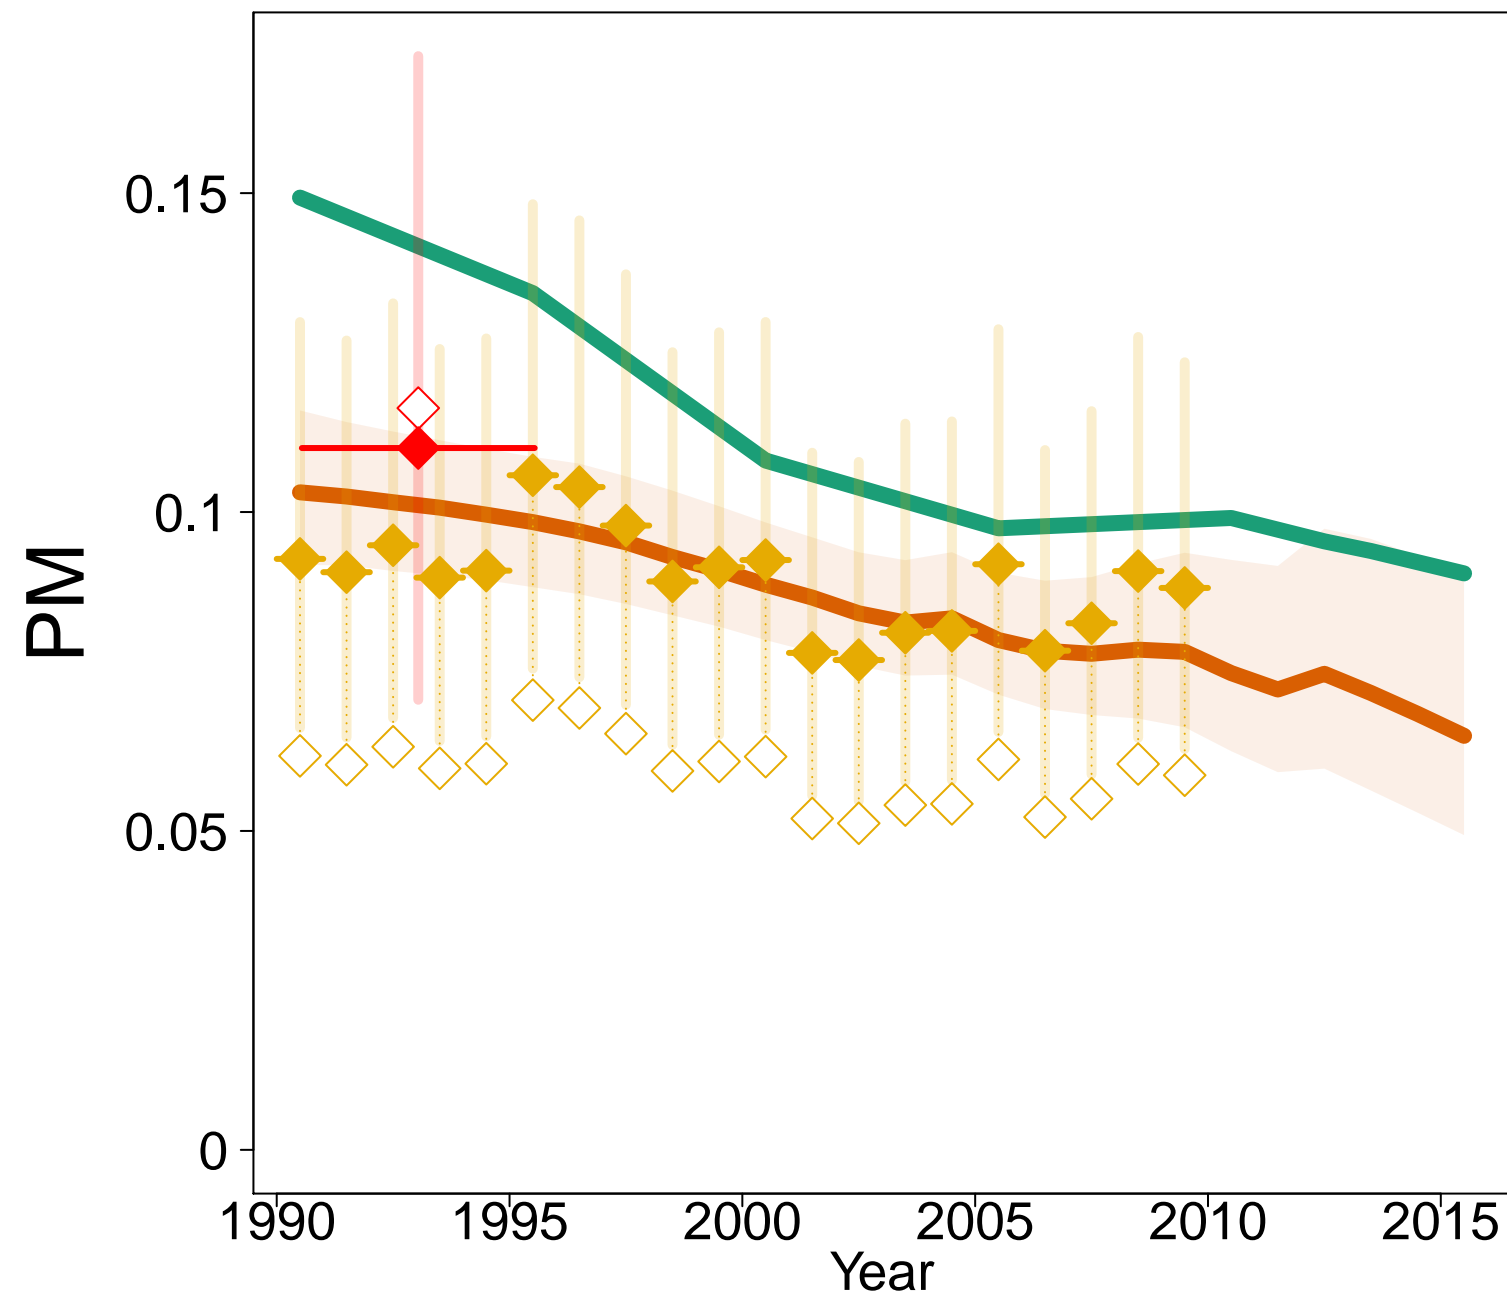

Guatemala [GTM; A]  
(Central America)

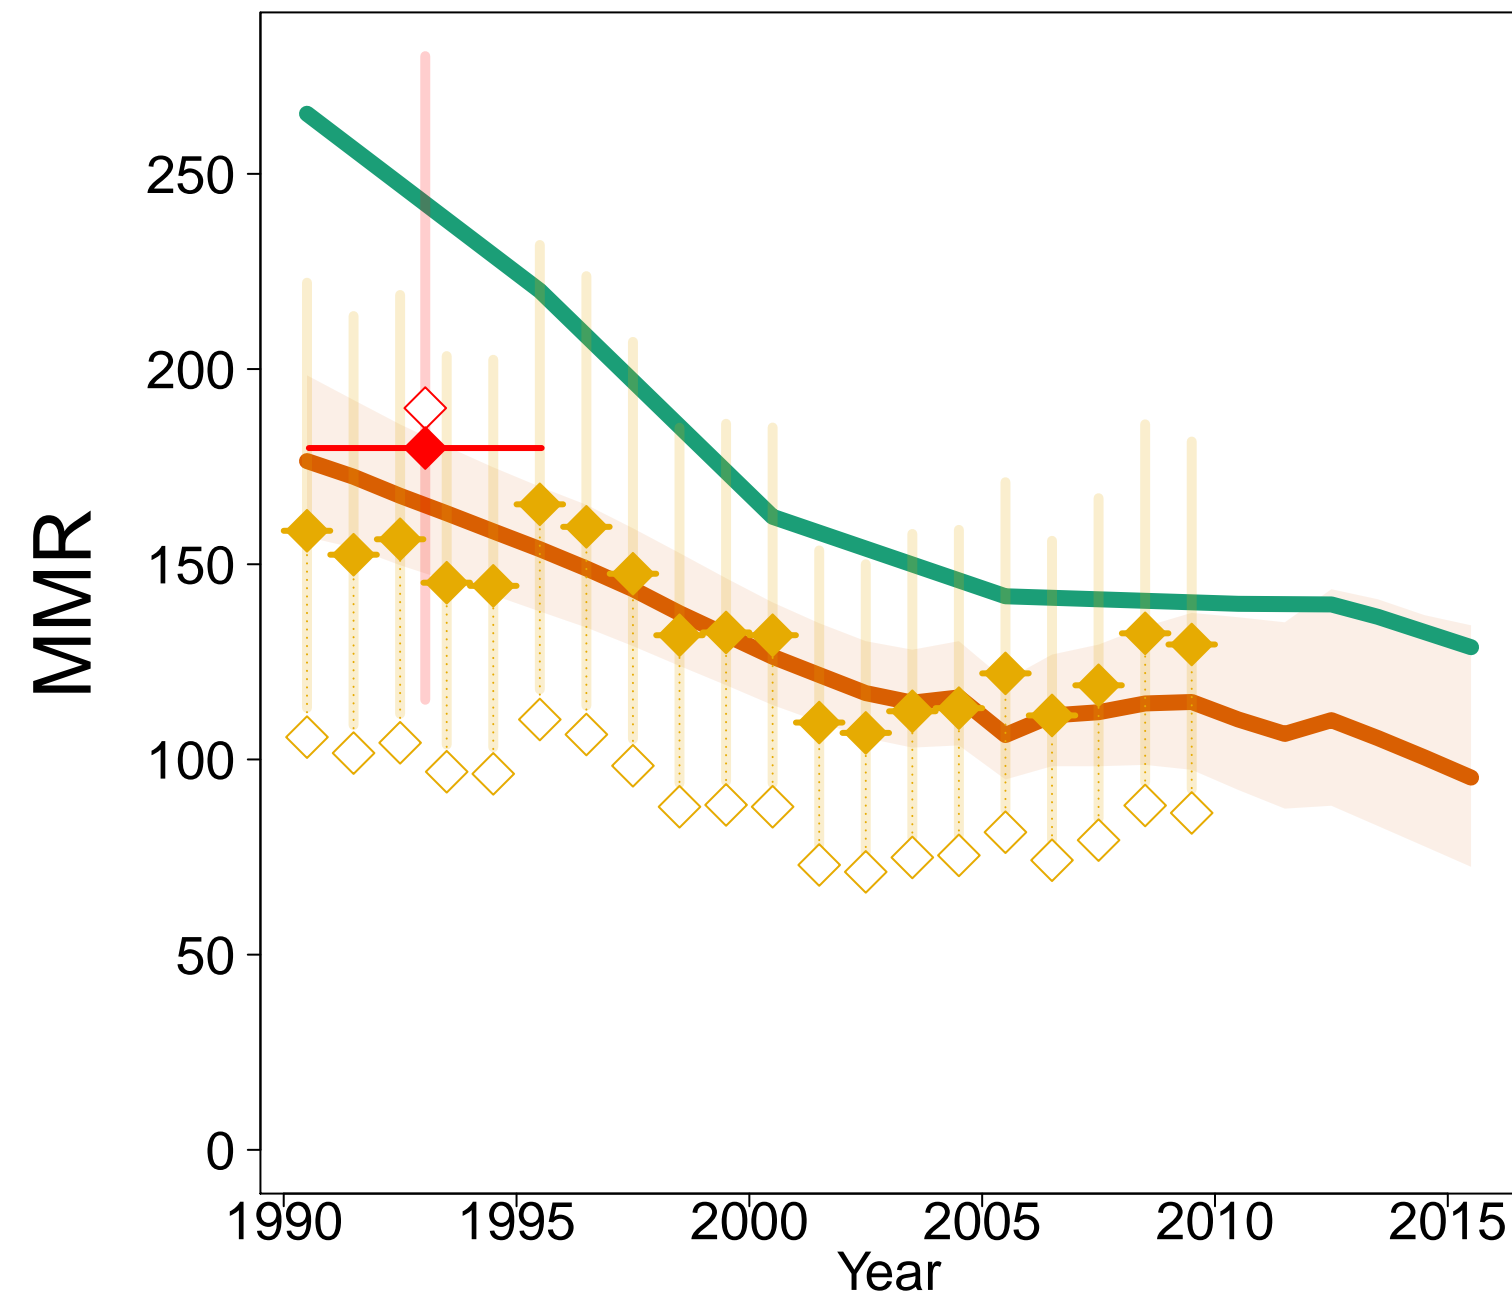

- Estimates –
- Bmat 2014
- MMEIG 2014
- Data –
- Observed Data
- Adjusted Data
- Data type –
- VR
- Misc. studies

Guinea [GIN; B]  
(Western Africa)

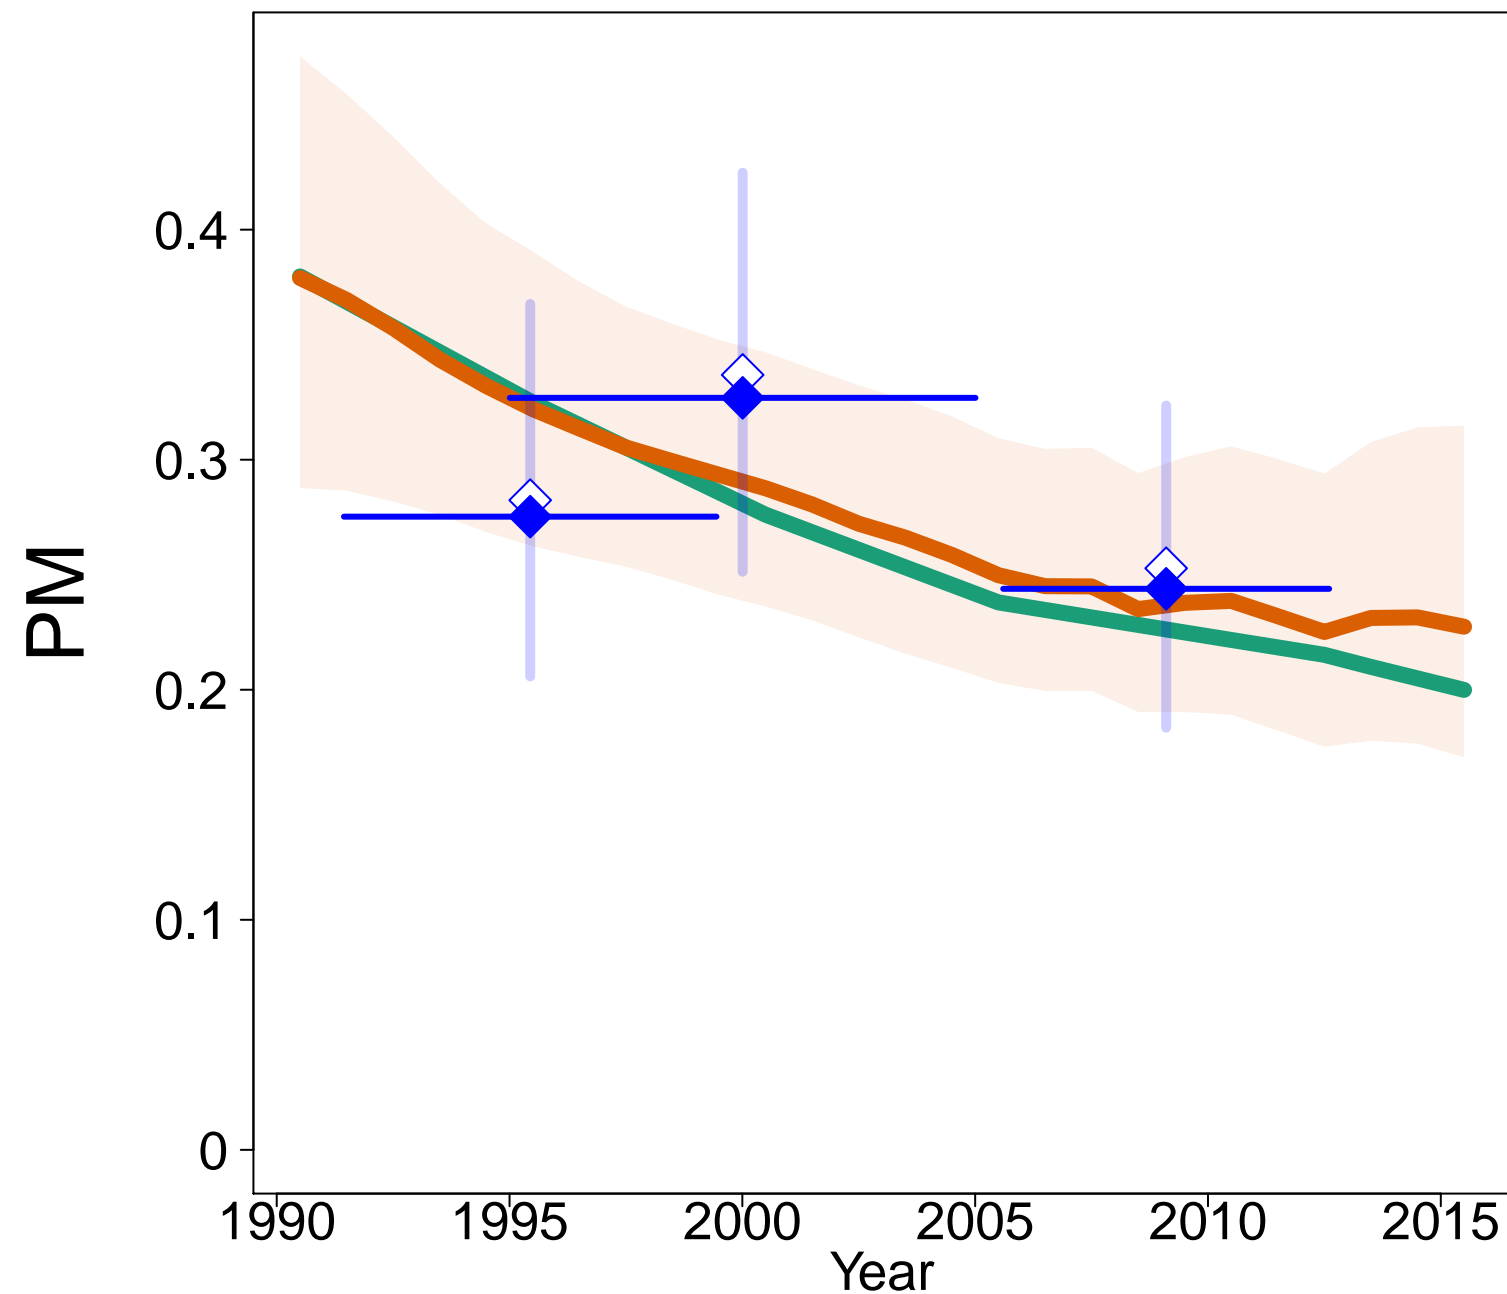

Guinea [GIN; B]  
(Western Africa)

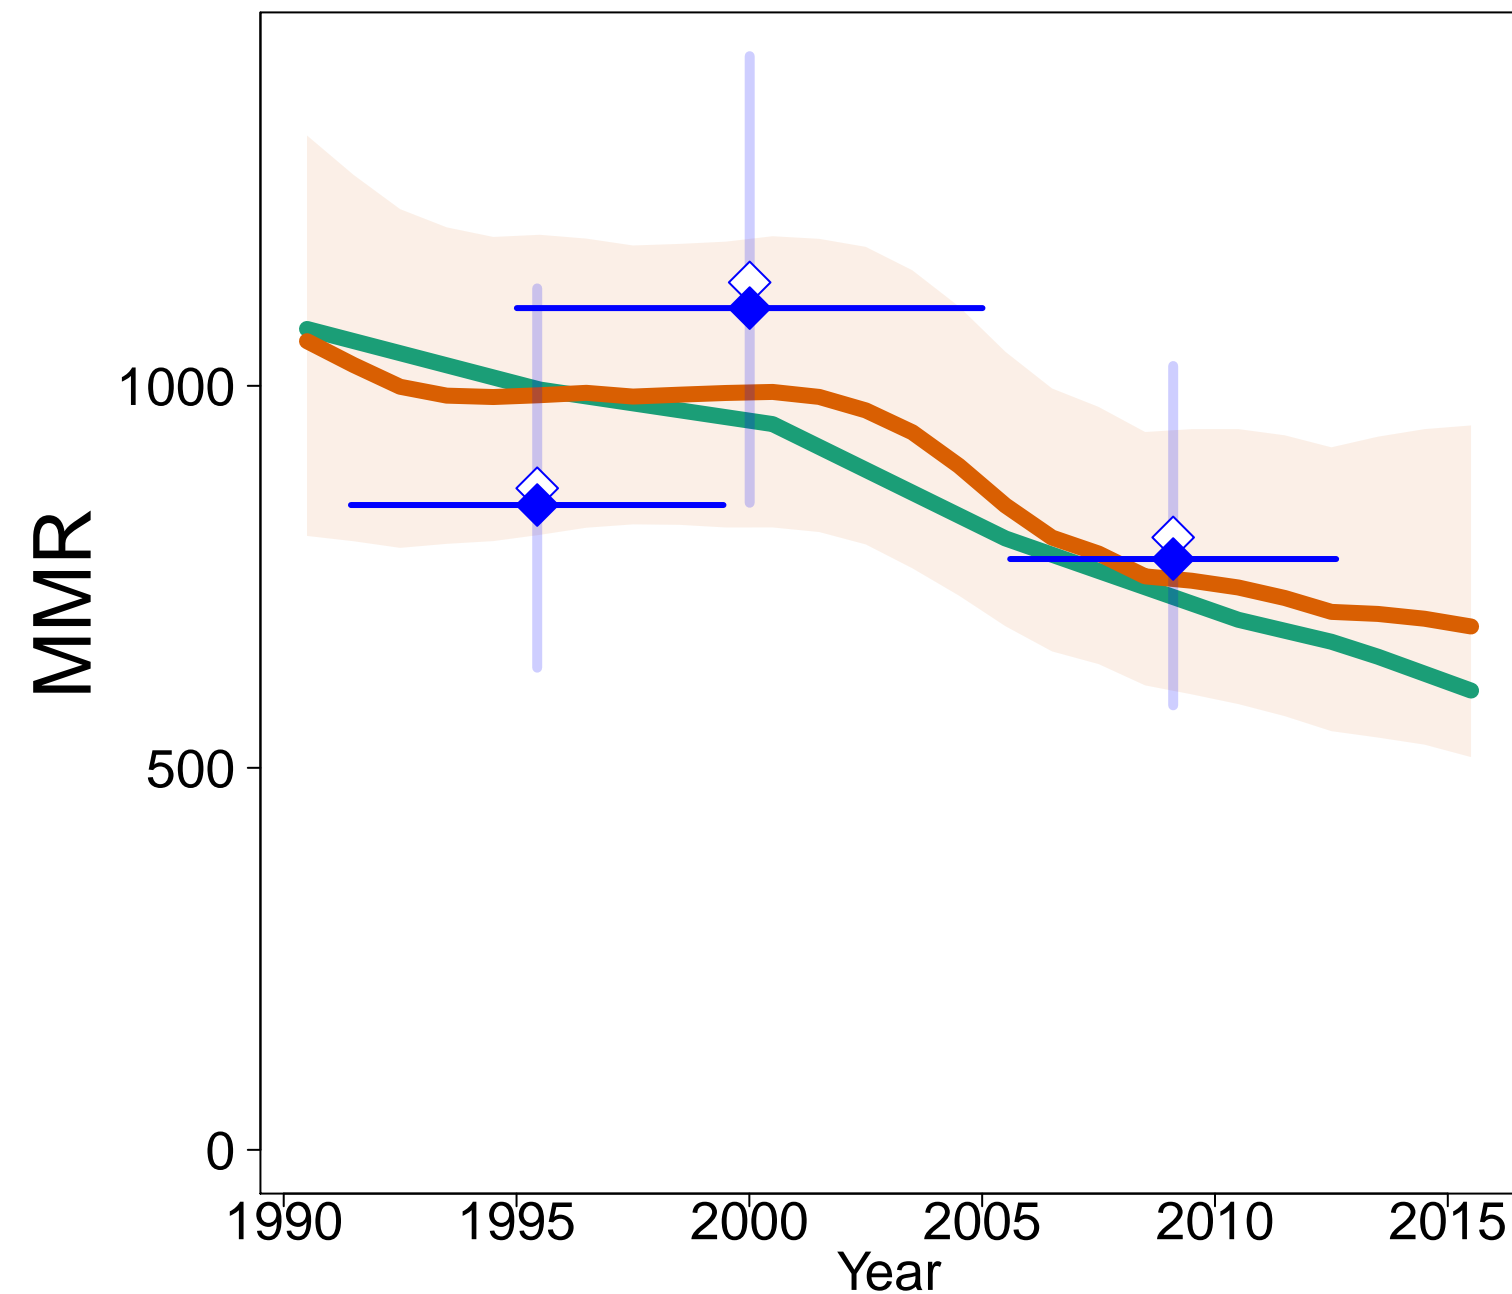

- Estimates –
- Bmat 2014
- MMEIG 2014
- Data –
- Observed Data
- Adjusted Data
- Data type –
- DHS

Guinea-Bissau [GNB; C]  
(Western Africa)

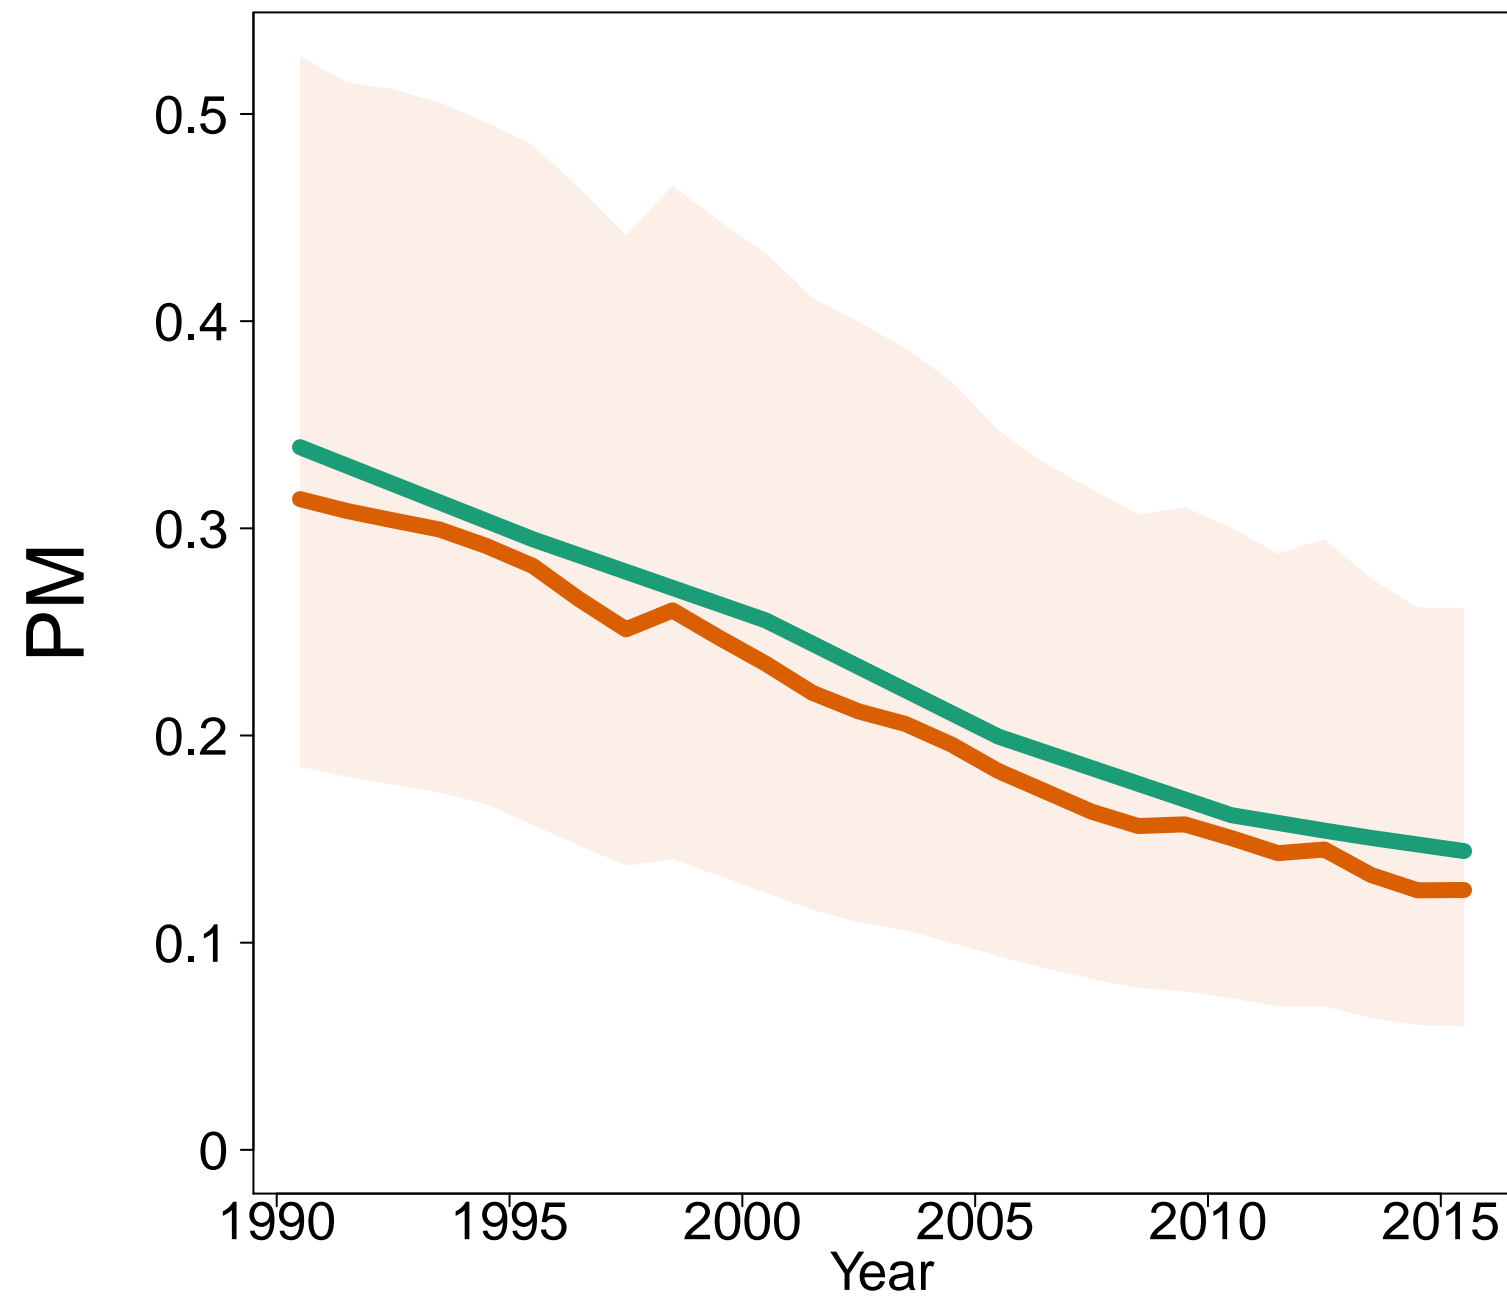

Guinea-Bissau [GNB; C]  
(Western Africa)

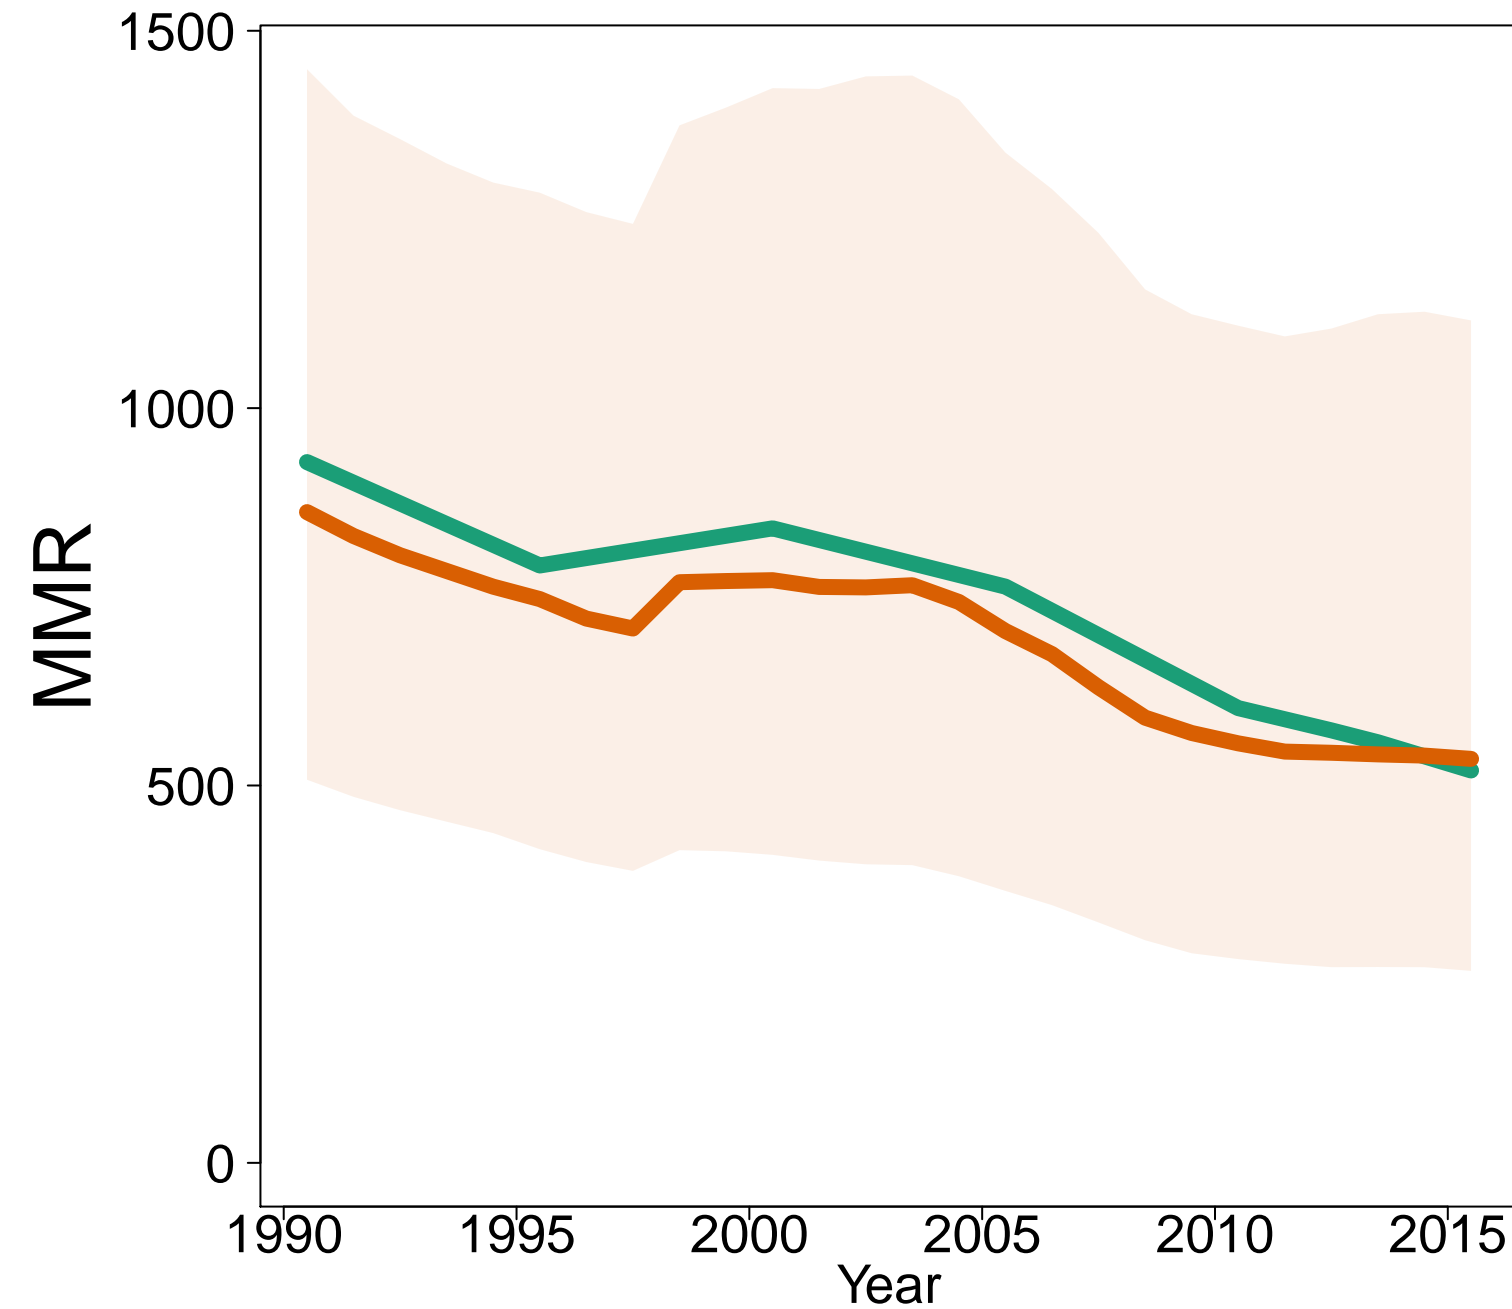

– Estimates –  
Bmat 2014  
MMEIG 2014  
– Data –

Guyana [GUY; B]  
(South America)

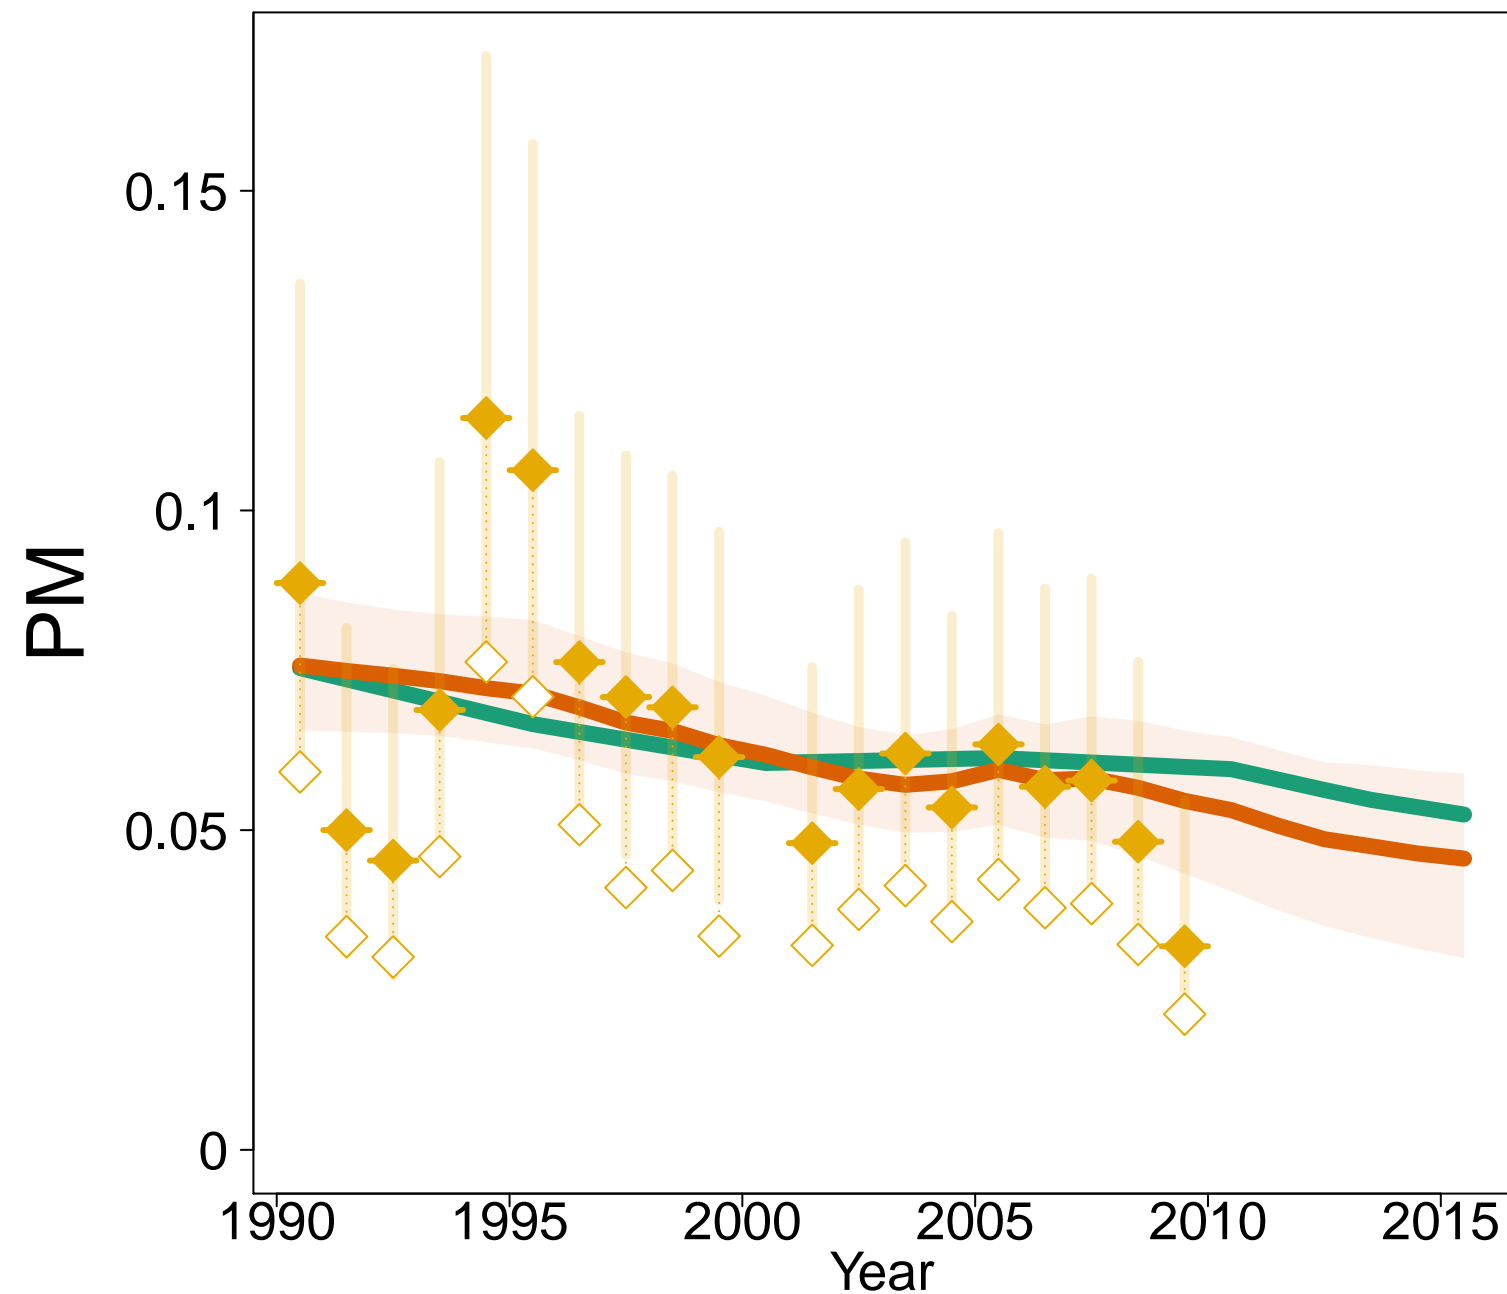

Guyana [GUY; B]  
(South America)

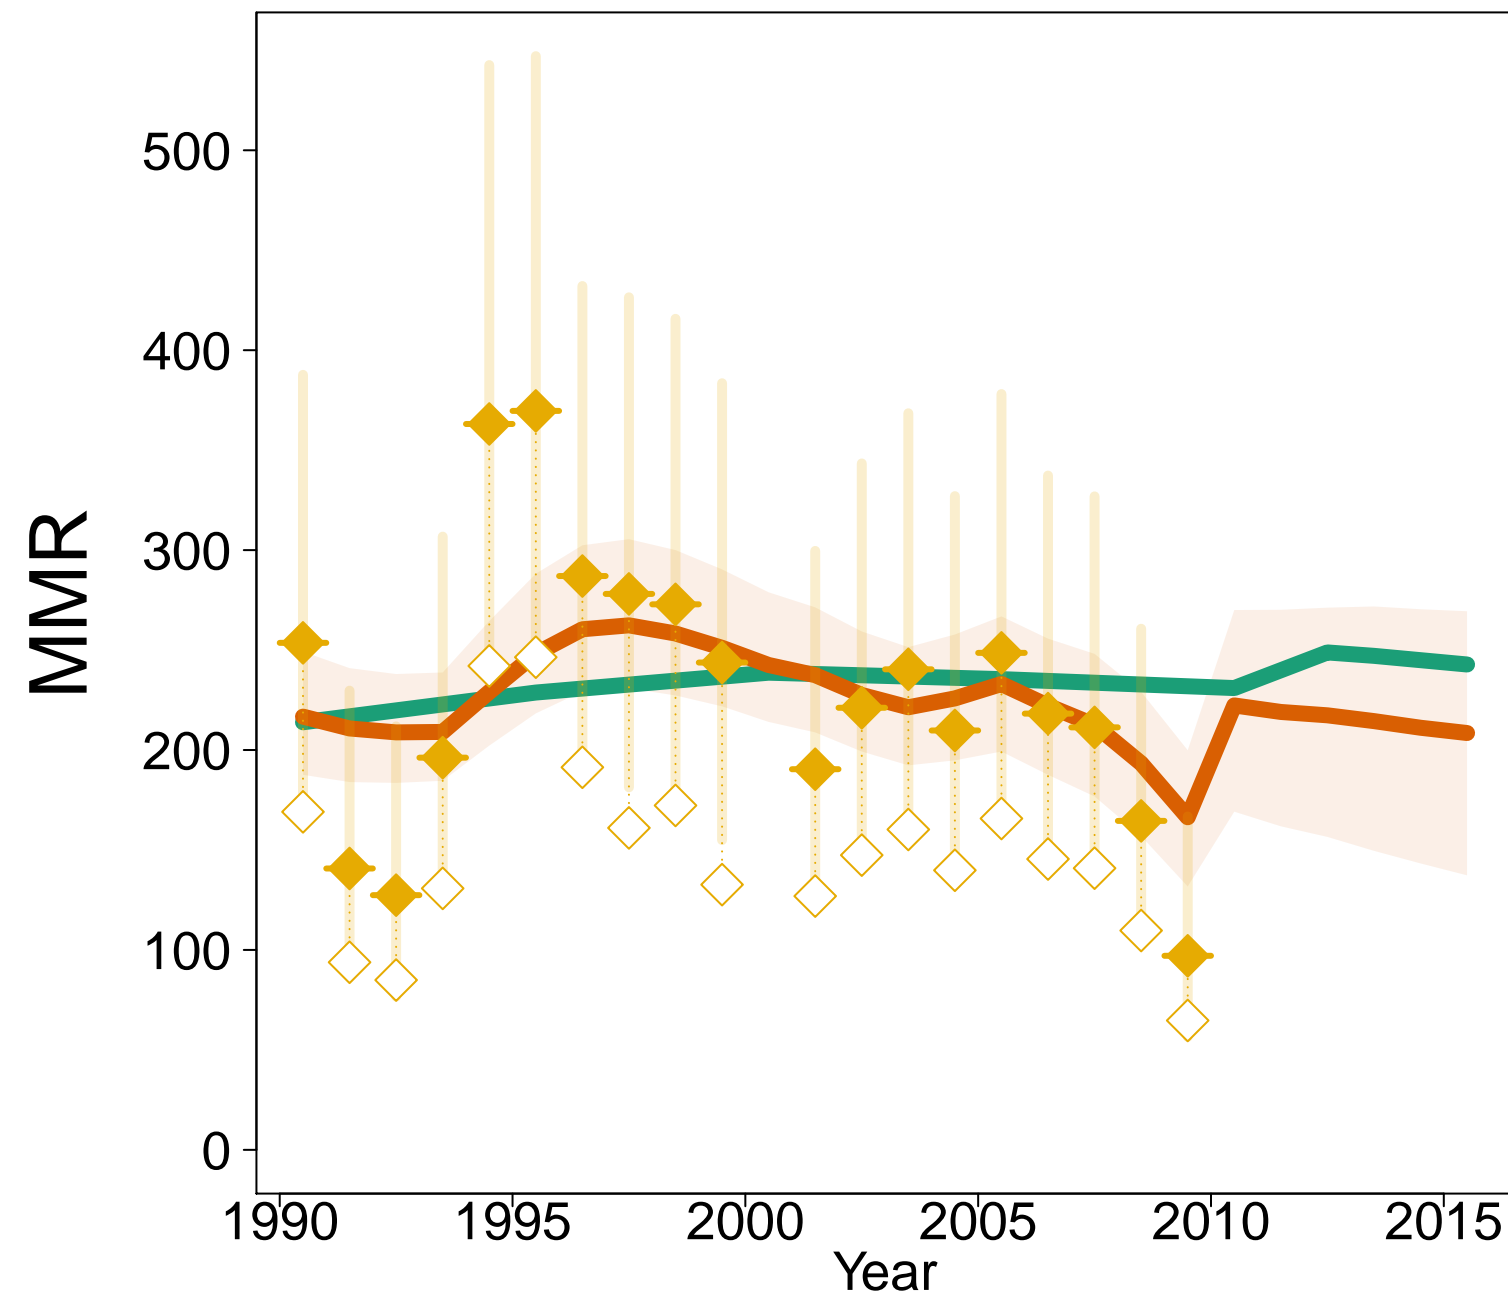

– Estimates –

Bmat 2014

MMEIG 2014

– Data –

Observed Data

Adjusted Data

– Data type –

VR

Haiti [HTI; B]  
(Caribbean)

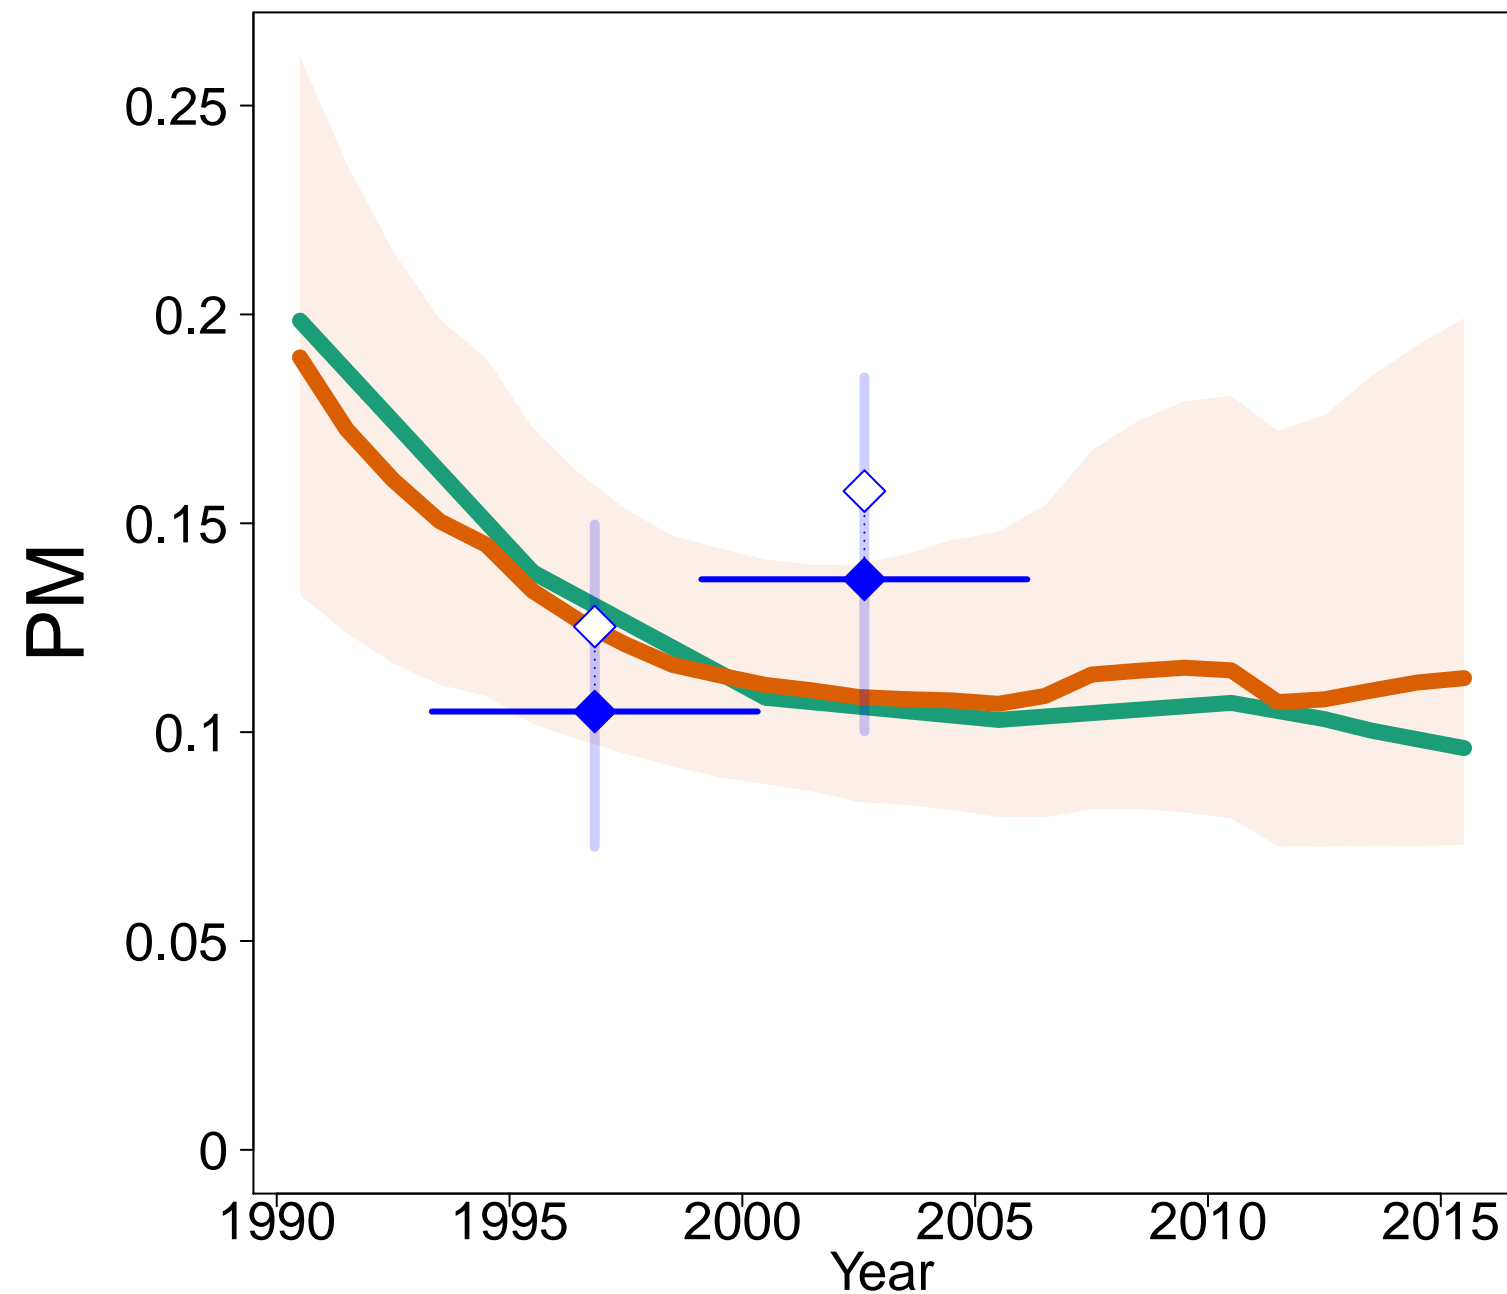

Haiti [HTI; B]  
(Caribbean)

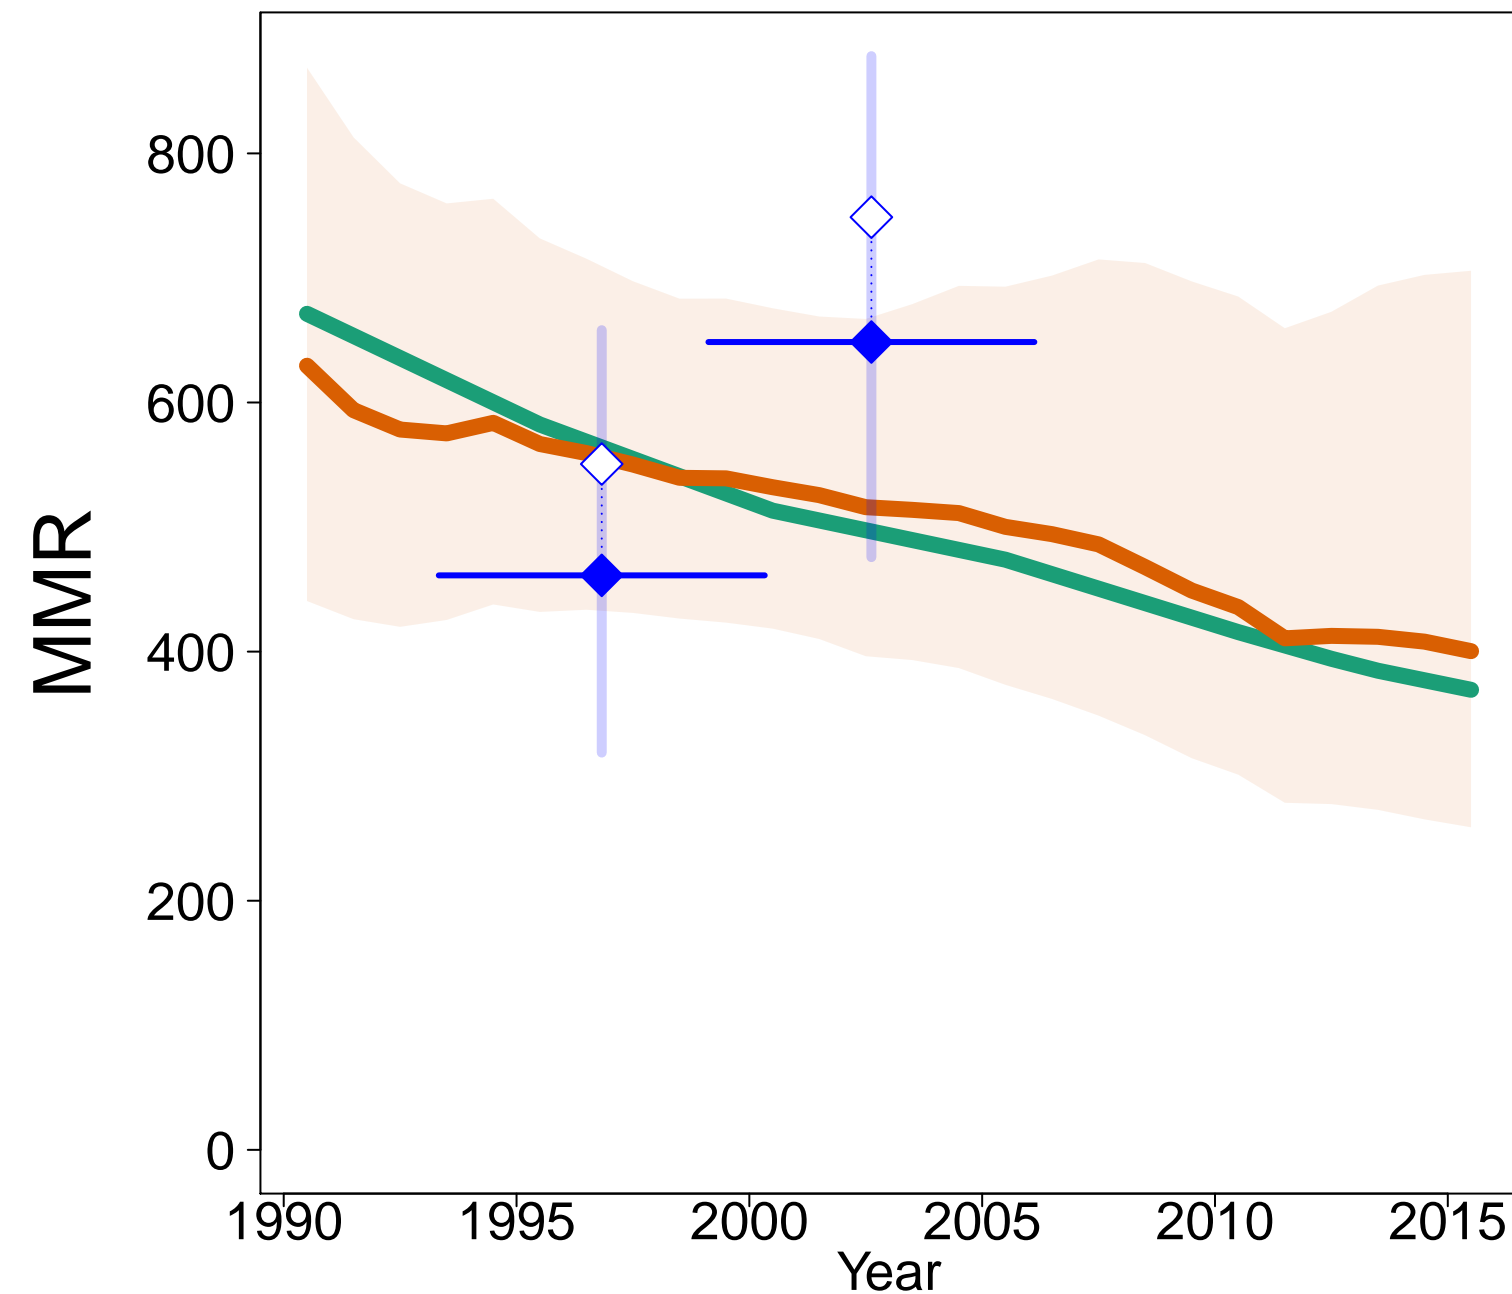

– Estimates –

Bmat 2014

MMEIG 2014

– Data –

Observed Data

Adjusted Data

– Data type –

DHS

Honduras [HND; B]  
(Central America)

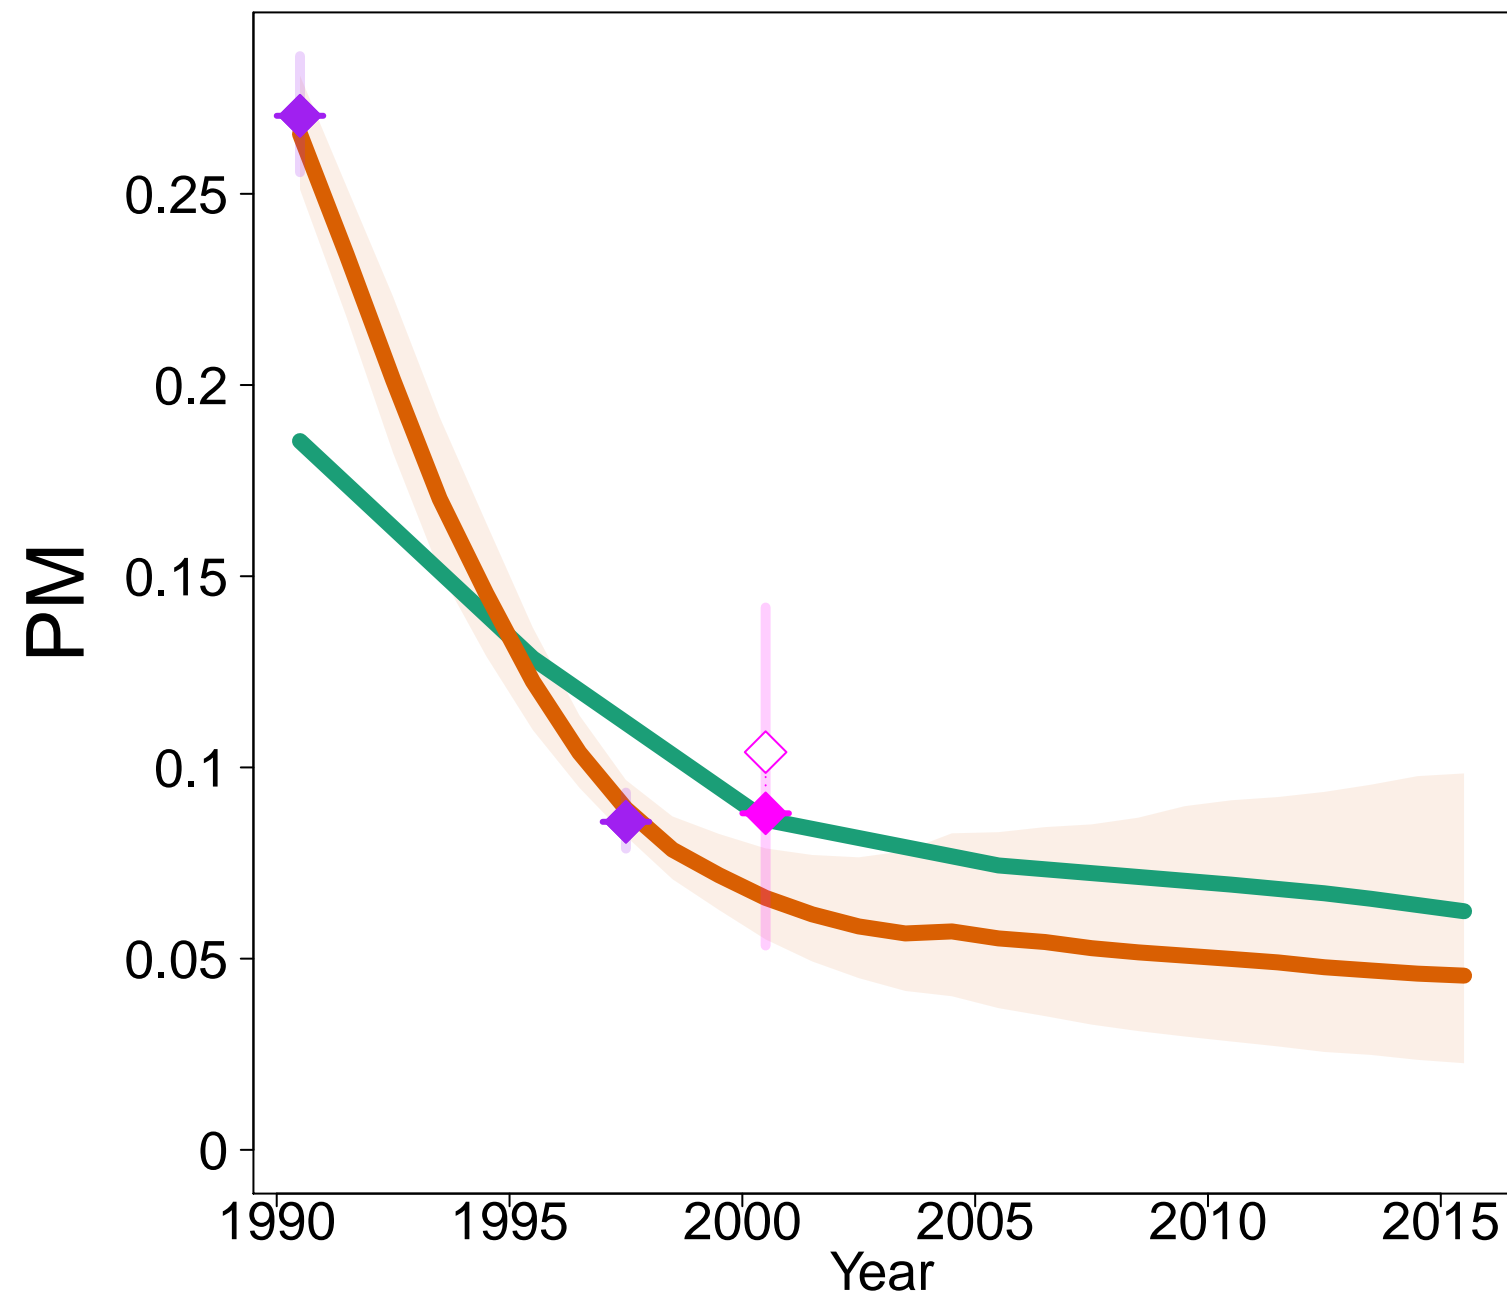

Honduras [HND; B]  
(Central America)

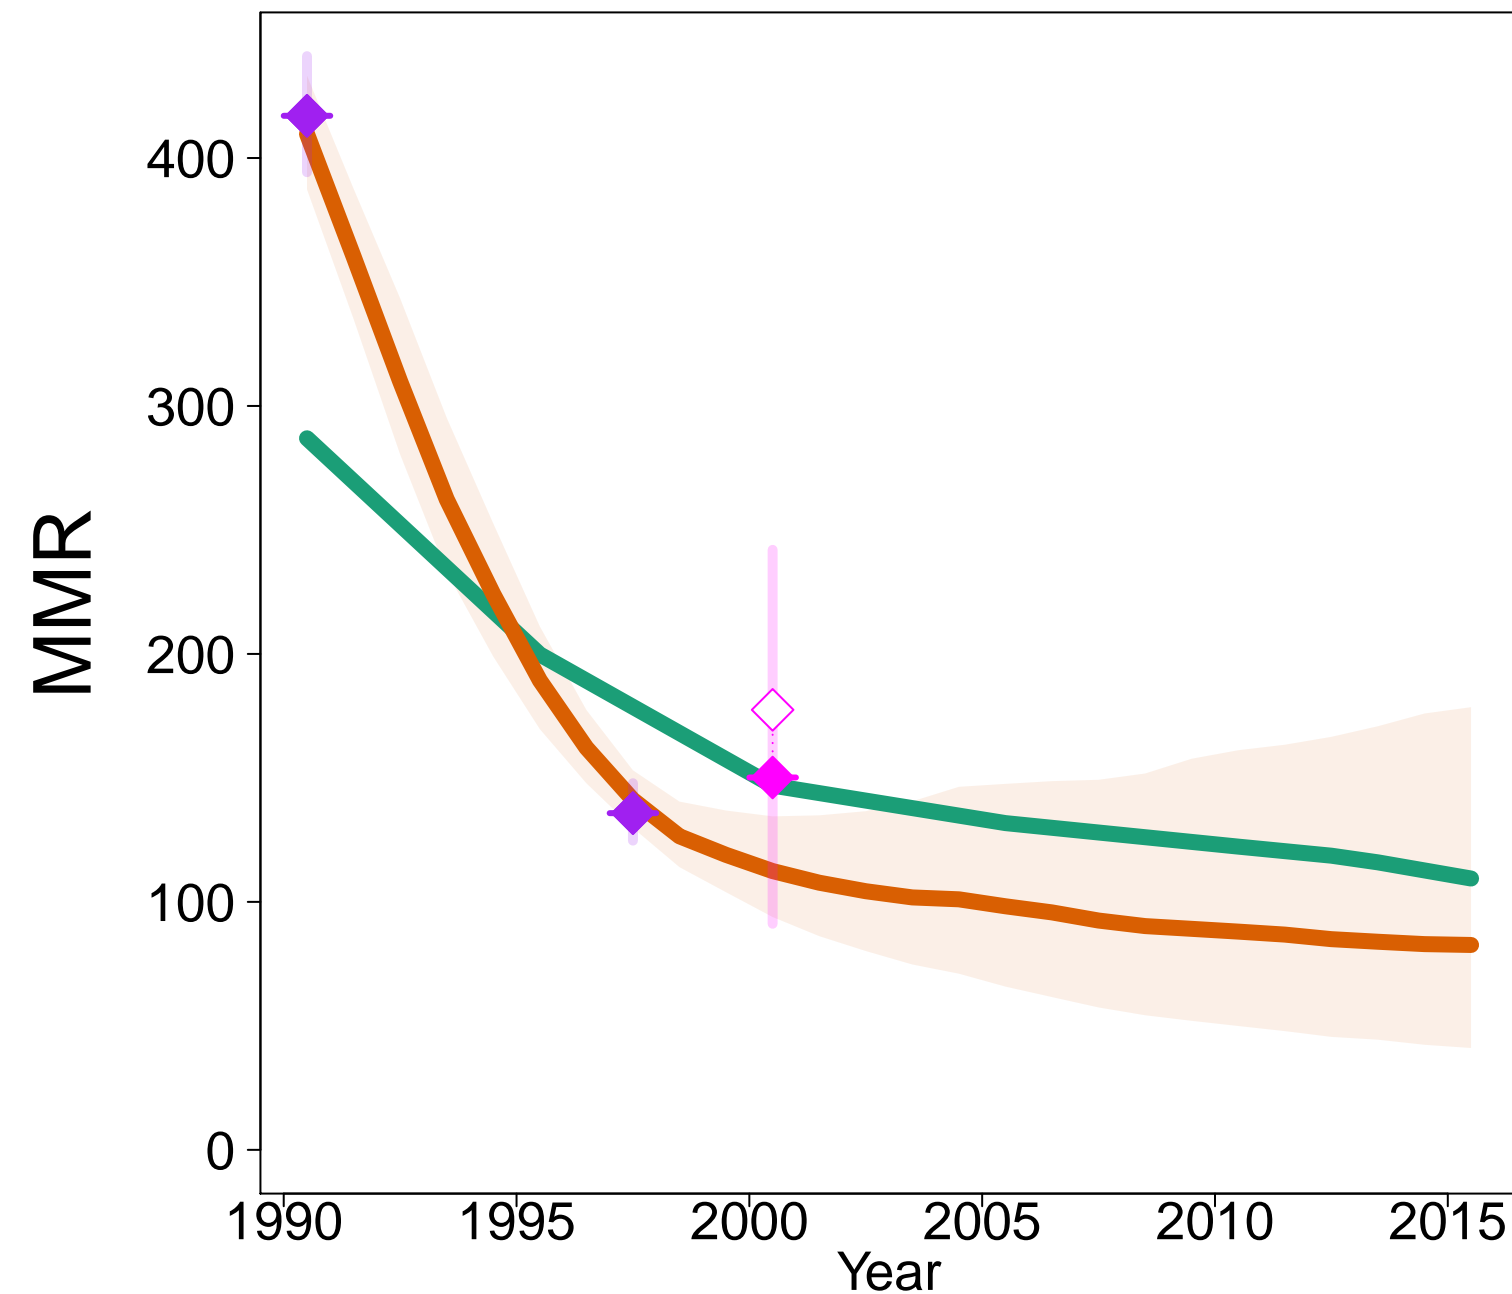

- Estimates –
- Bmat 2014
- MMEIG 2014
- Data –
- Observed Data
- Adjusted Data
- Data type –
- Spec. studies
- Census

Hungary [HUN; A]  
(Developed regions)

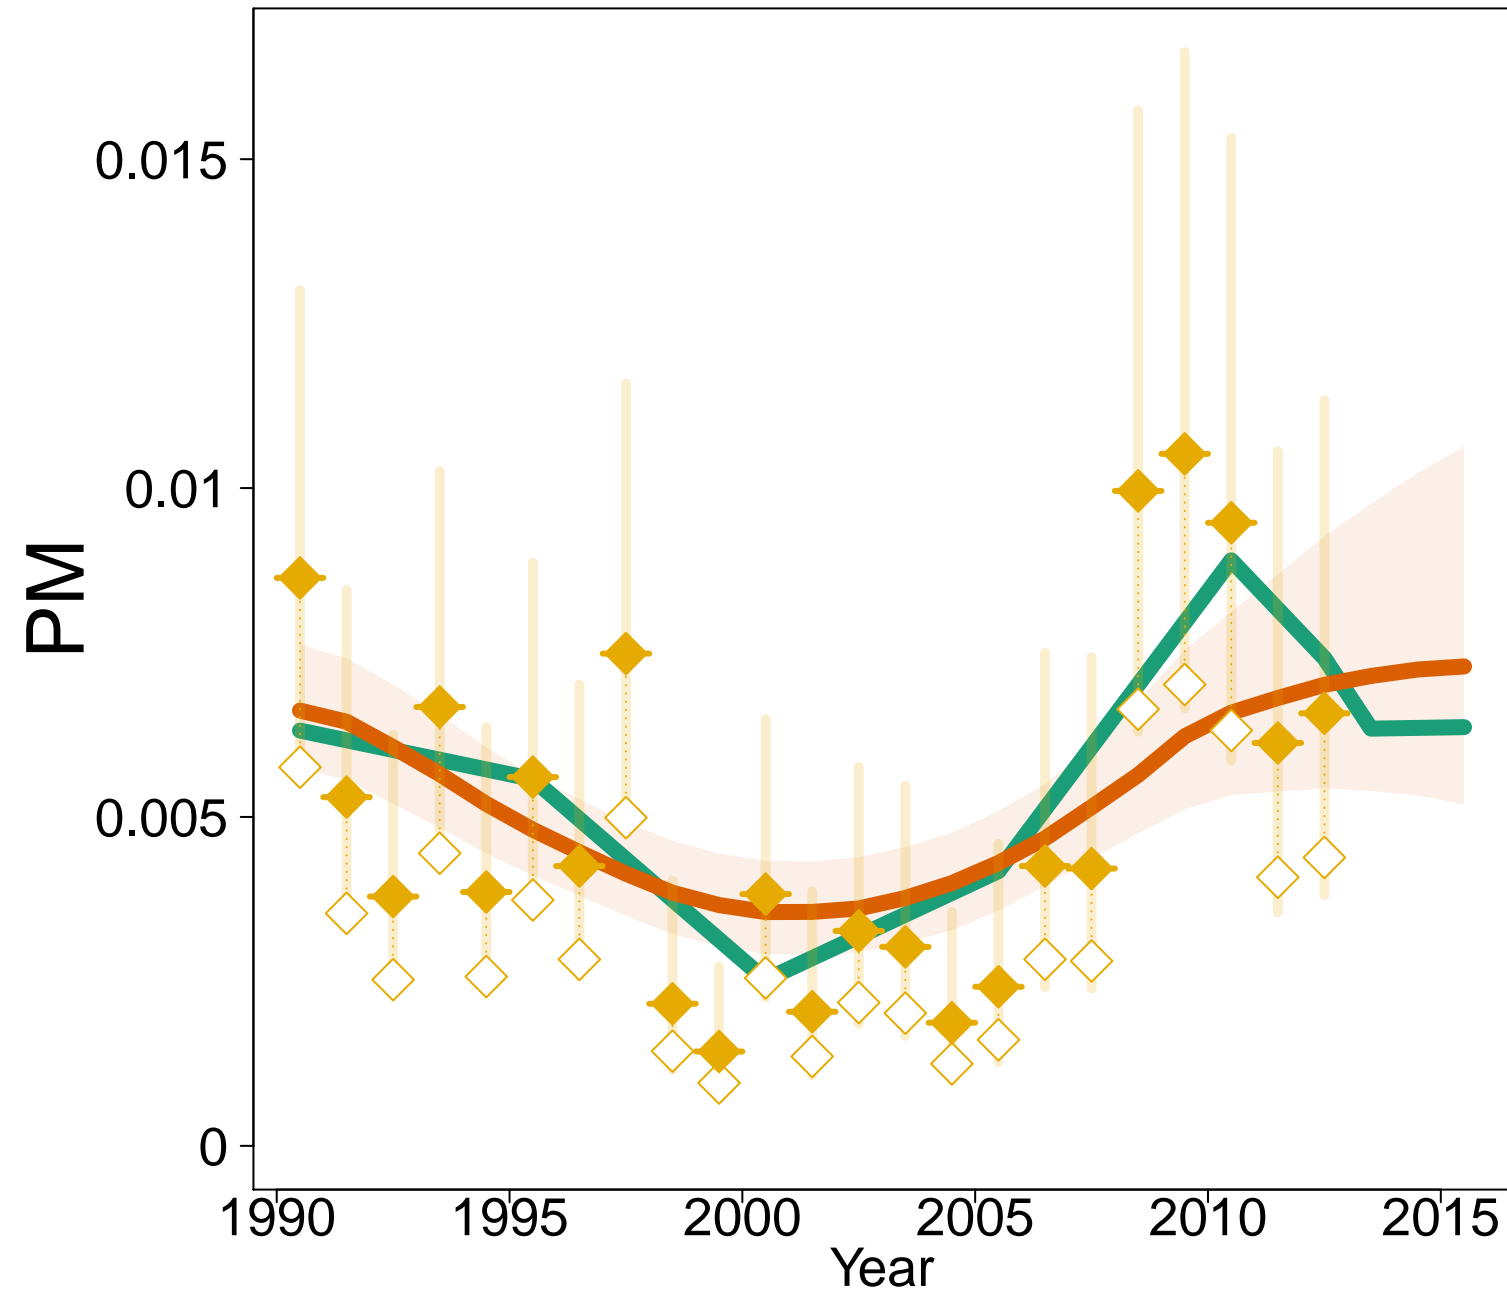

Hungary [HUN; A]  
(Developed regions)

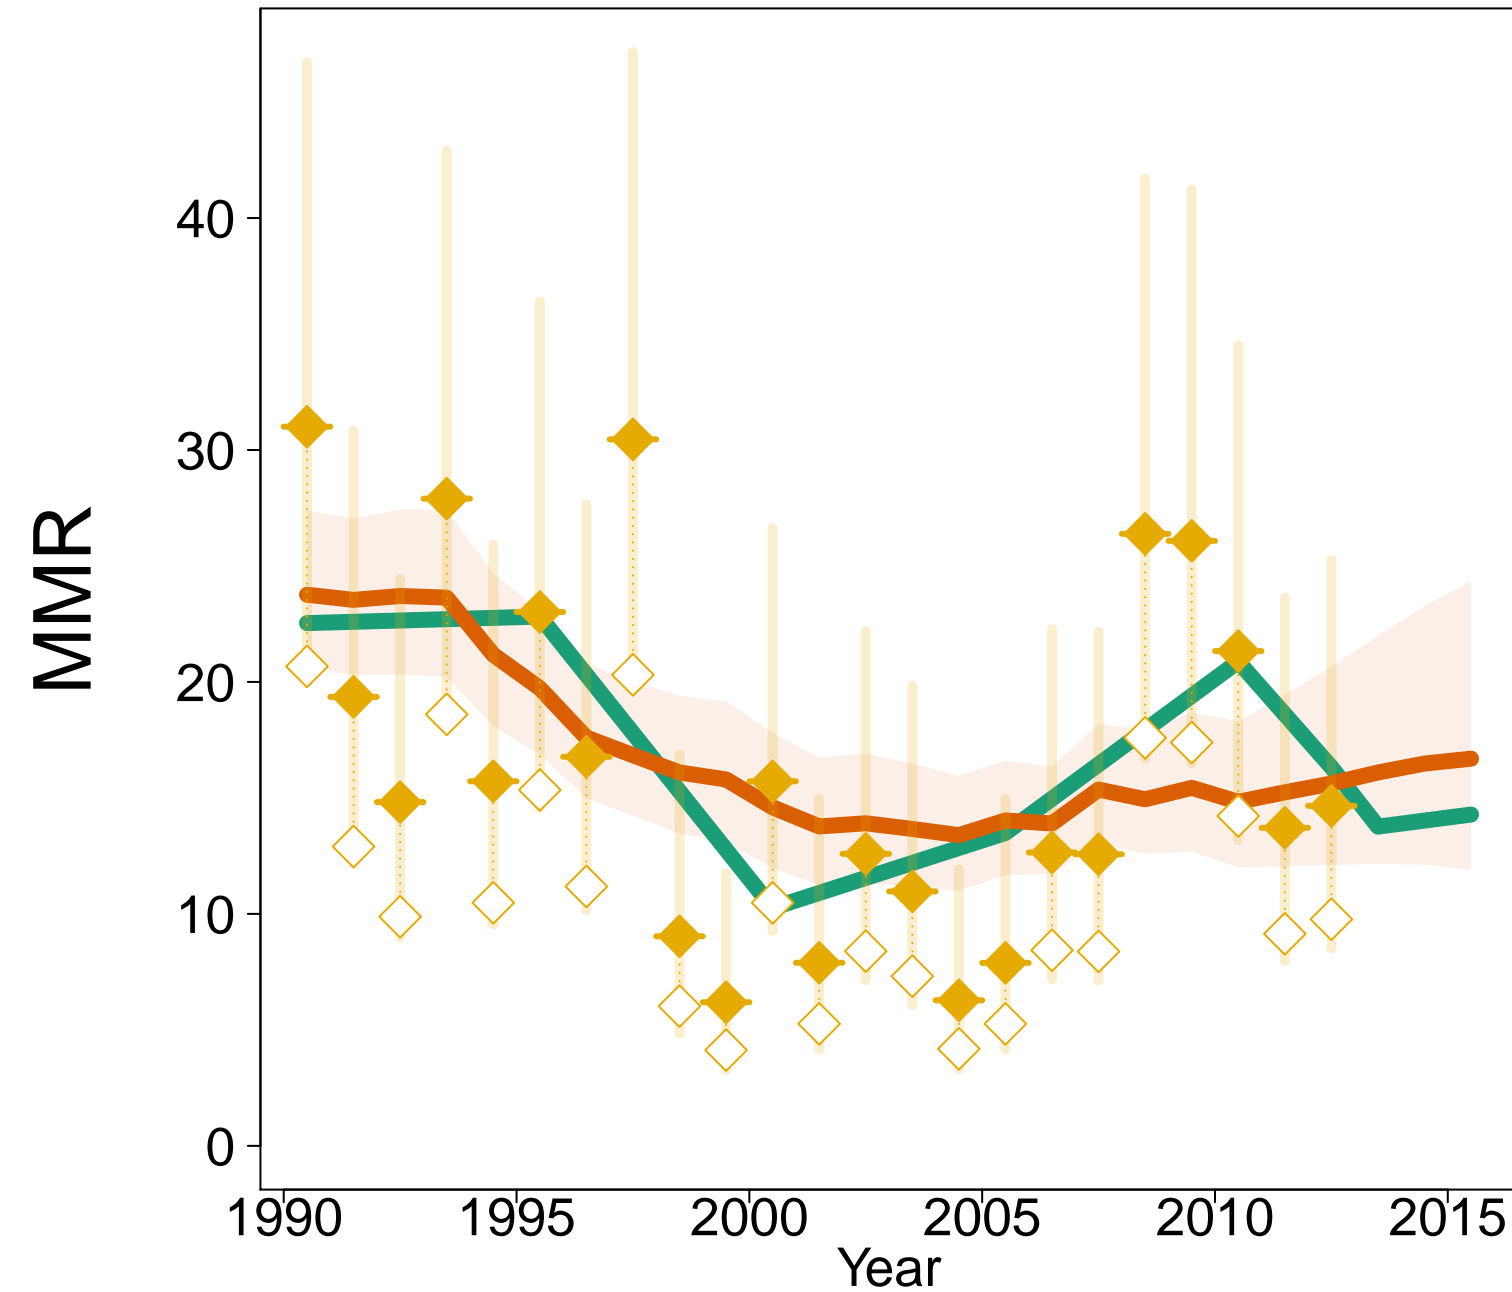

– Estimates –  
Bmat 2014  
MMEIG 2014  
– Data –  
Observed Data  
Adjusted Data  
– Data type –  
VR



Iceland [ISL; A]  
(Developed regions)

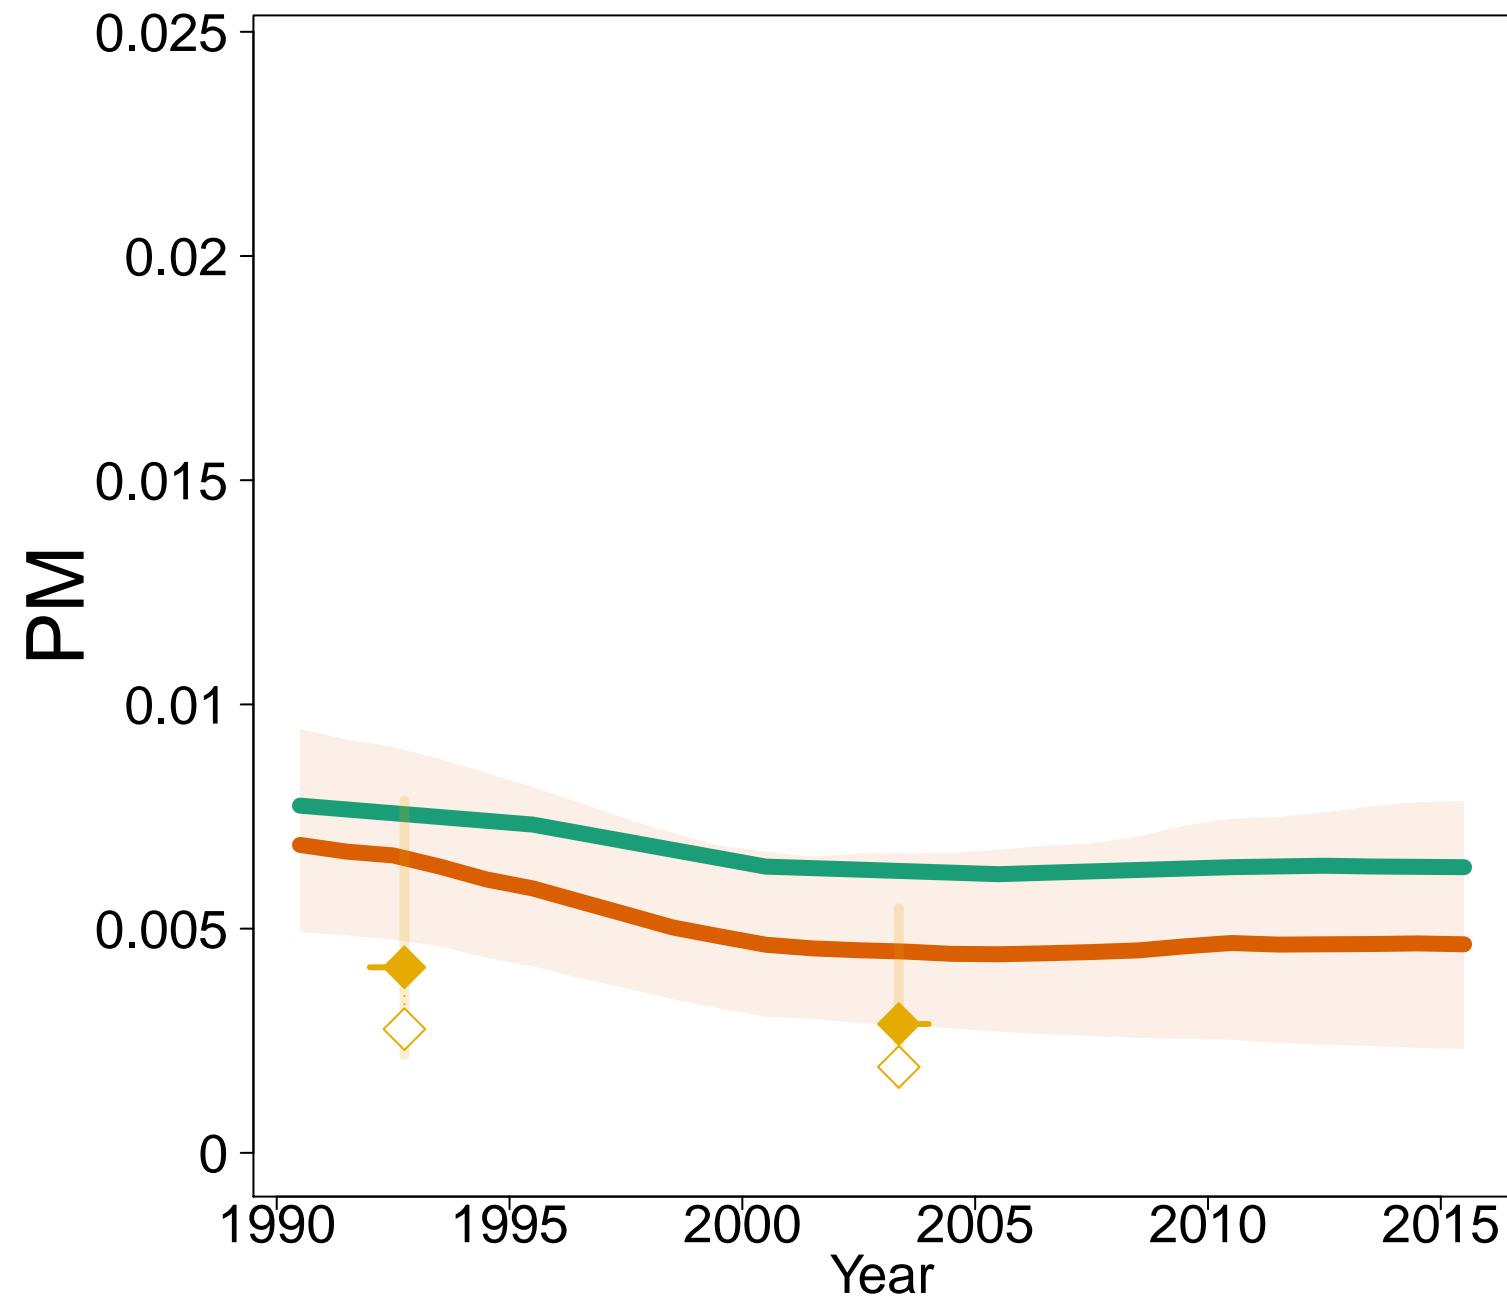

Iceland [ISL; A]  
(Developed regions)

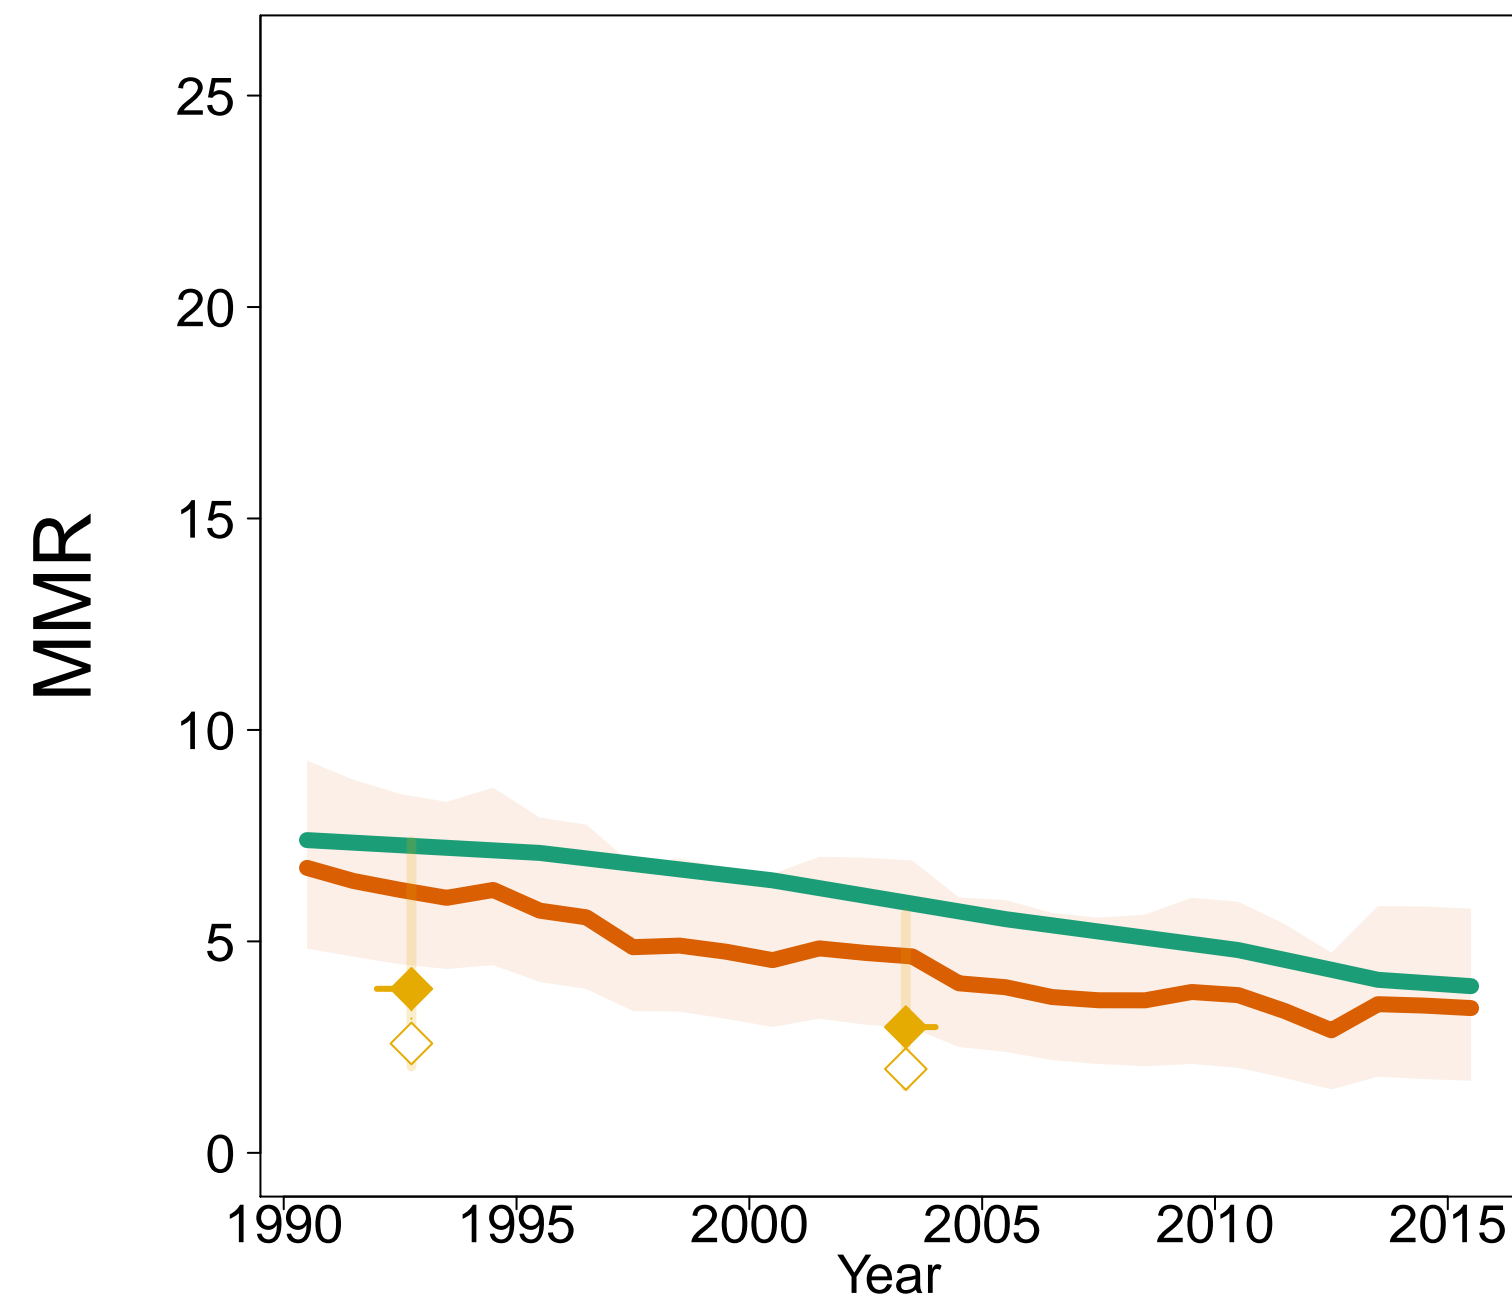

- Estimates –
- Bmat 2014
- MMEIG 2014
- Data –
- Observed Data
- Adjusted Data
- Data type –
- VR

India [IND; B]  
(Southern Asia)

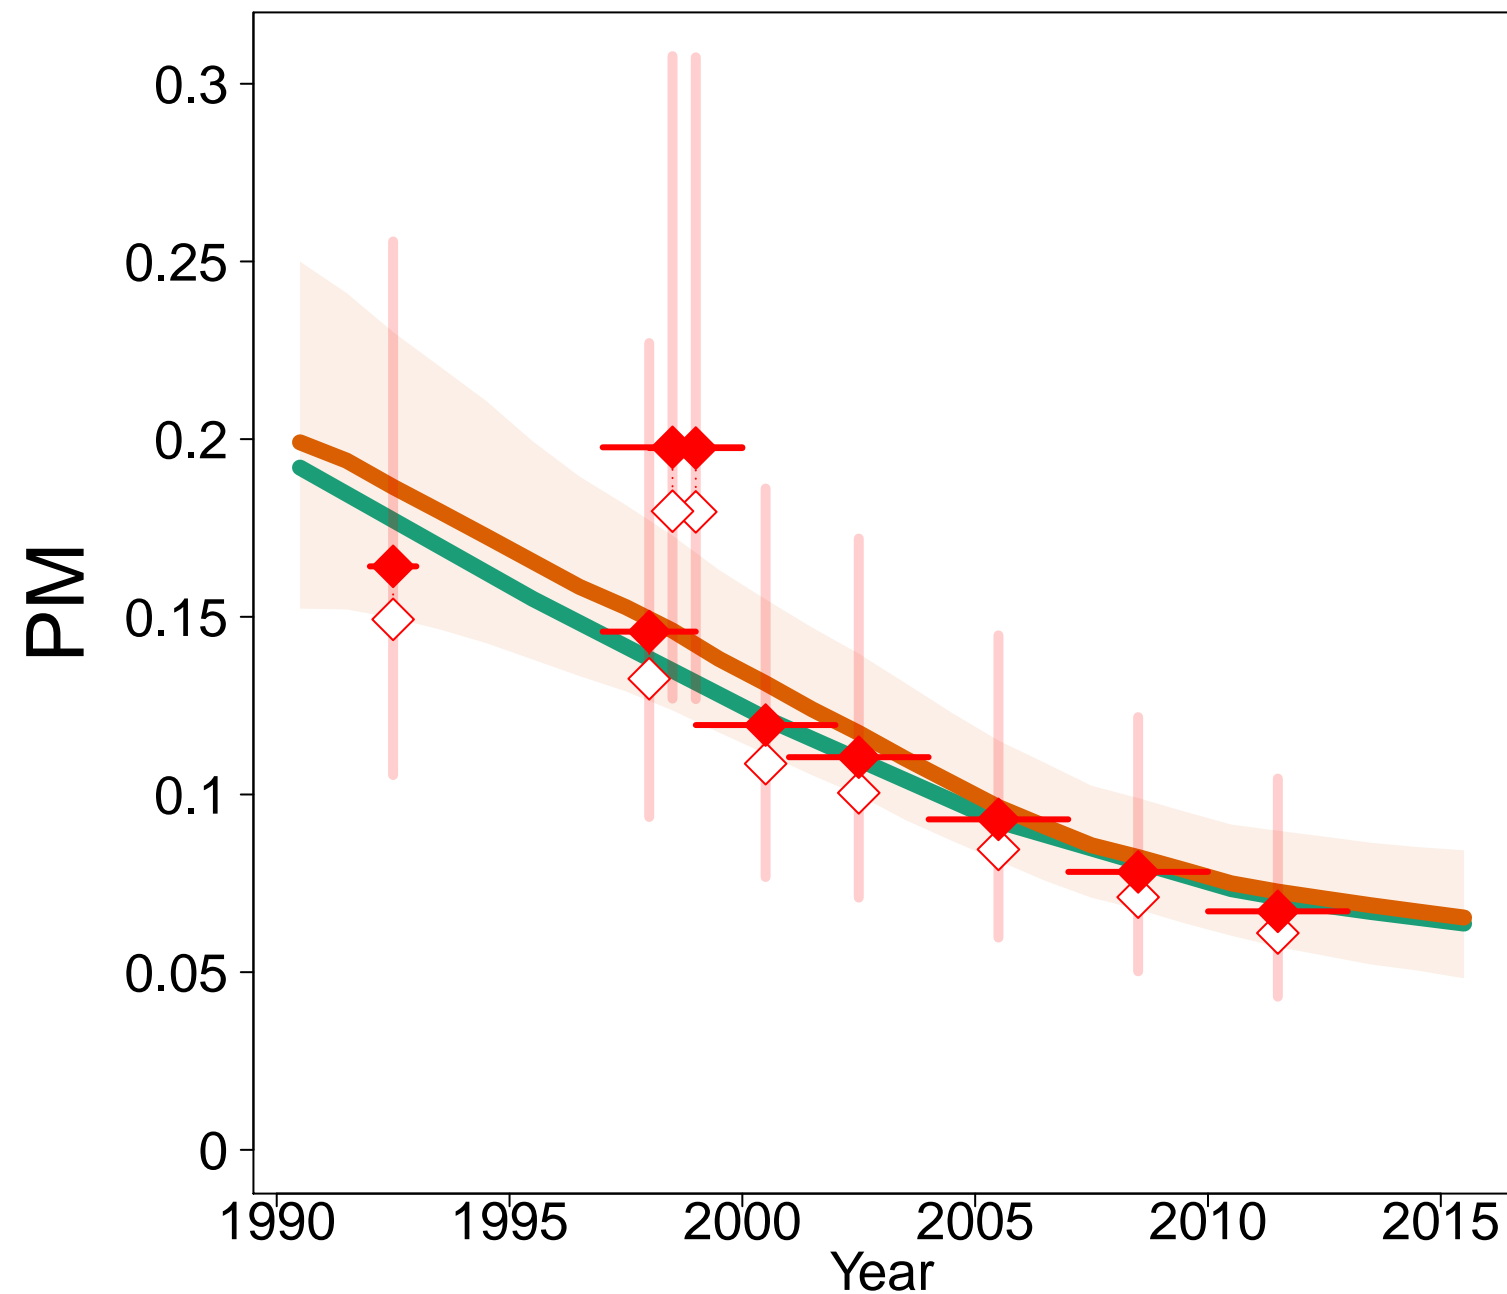

India [IND; B]  
(Southern Asia)

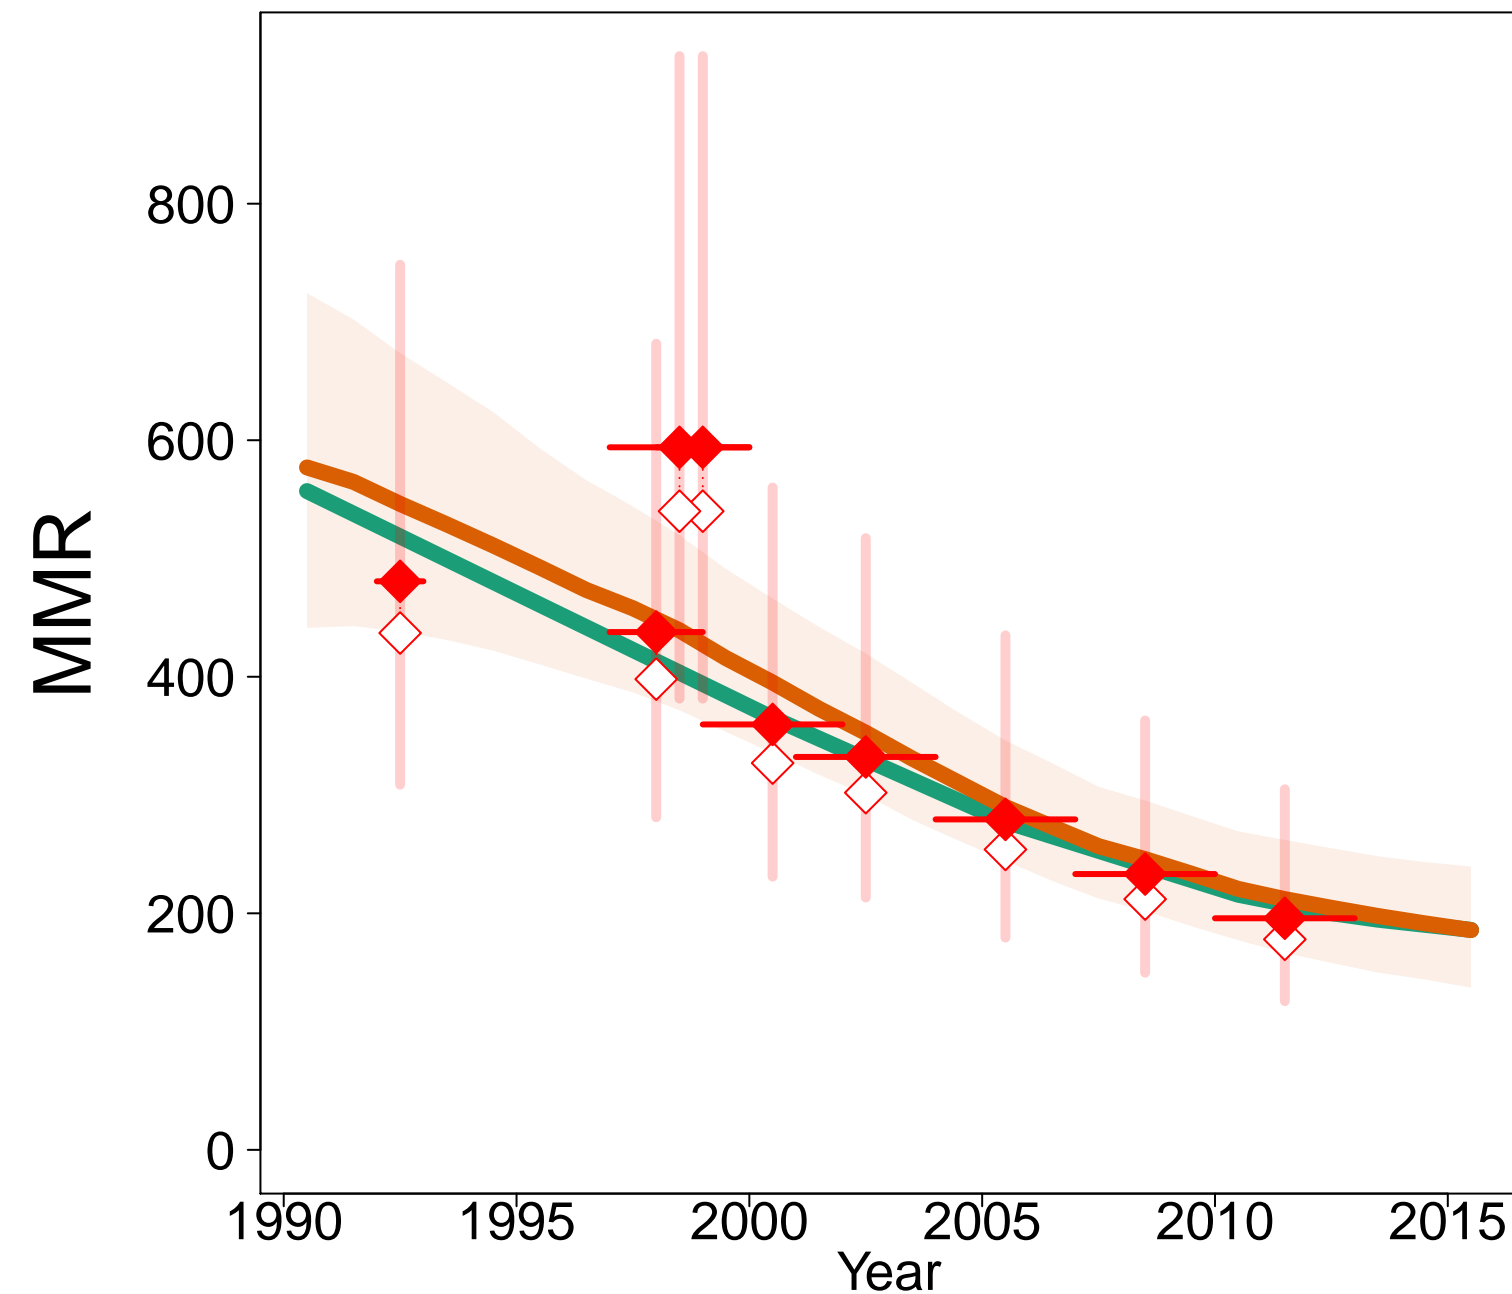

- Estimates –
- Bmat 2014
- MMEIG 2014
- Data –
- Observed Data
- Adjusted Data
- Data type –
- Misc. studies

Indonesia [IDN; B]  
(South-Eastern Asia / Oceania)

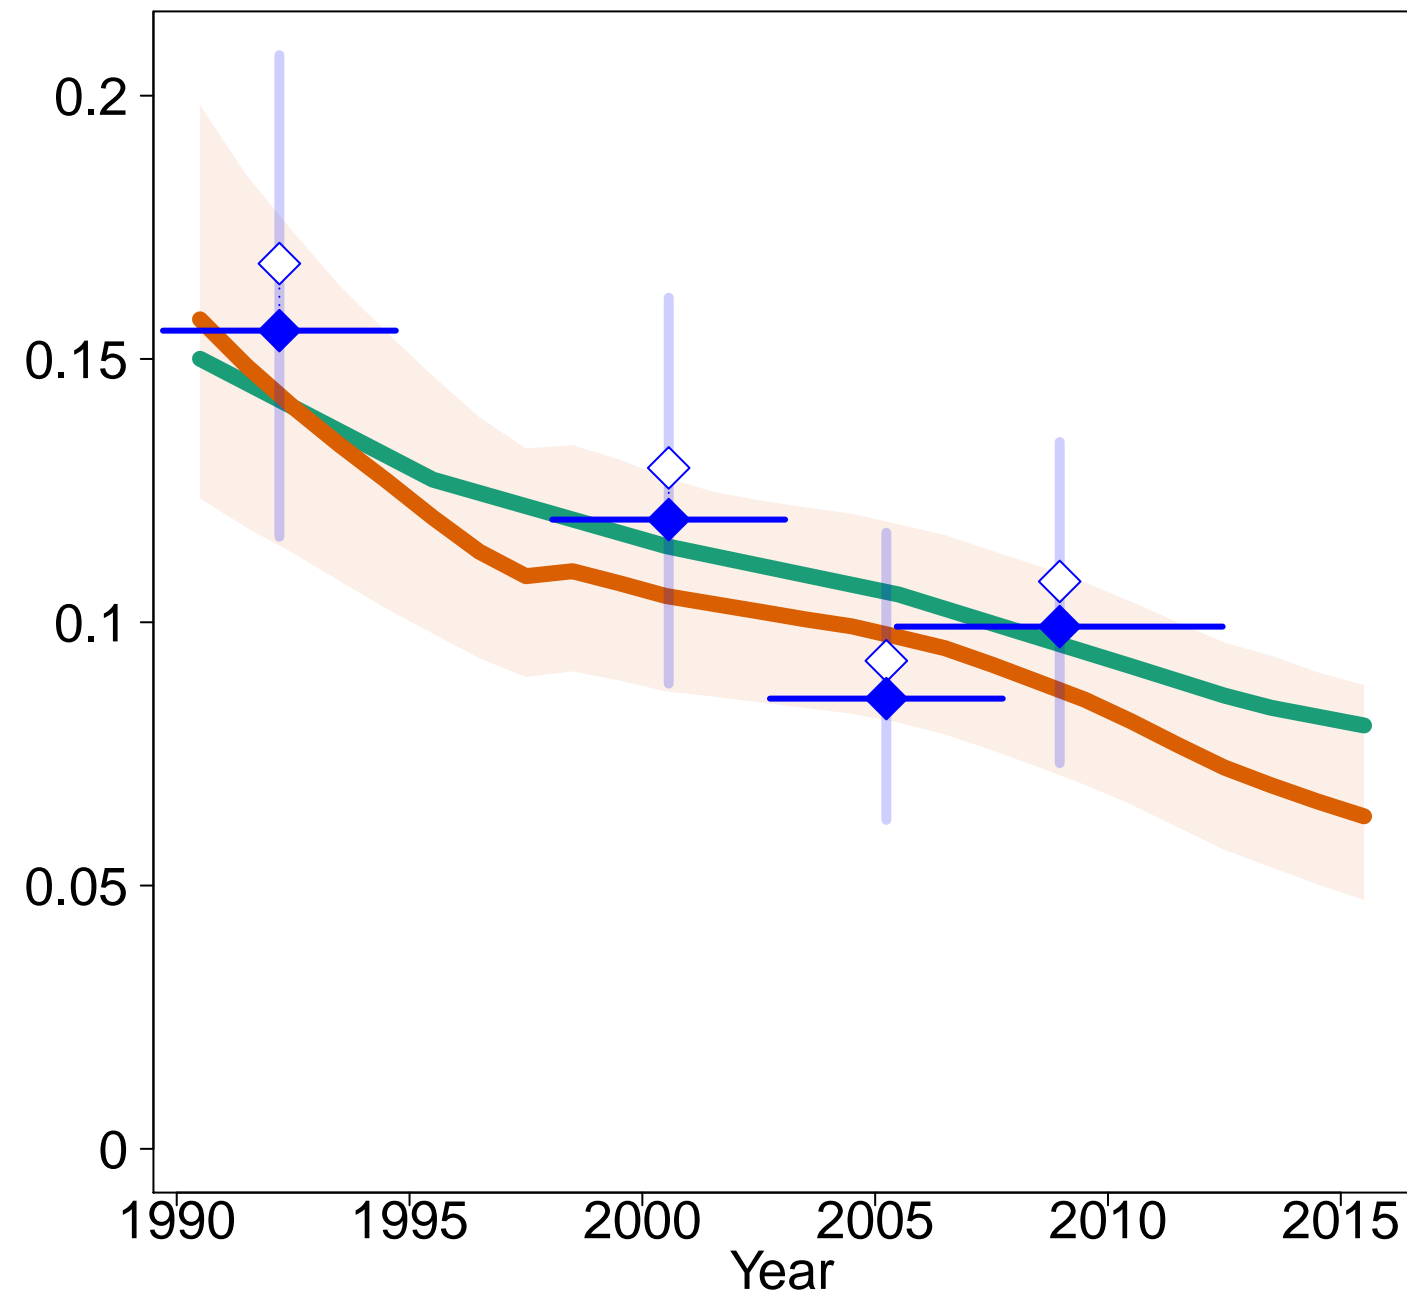

Indonesia [IDN; B]  
(South-Eastern Asia / Oceania)

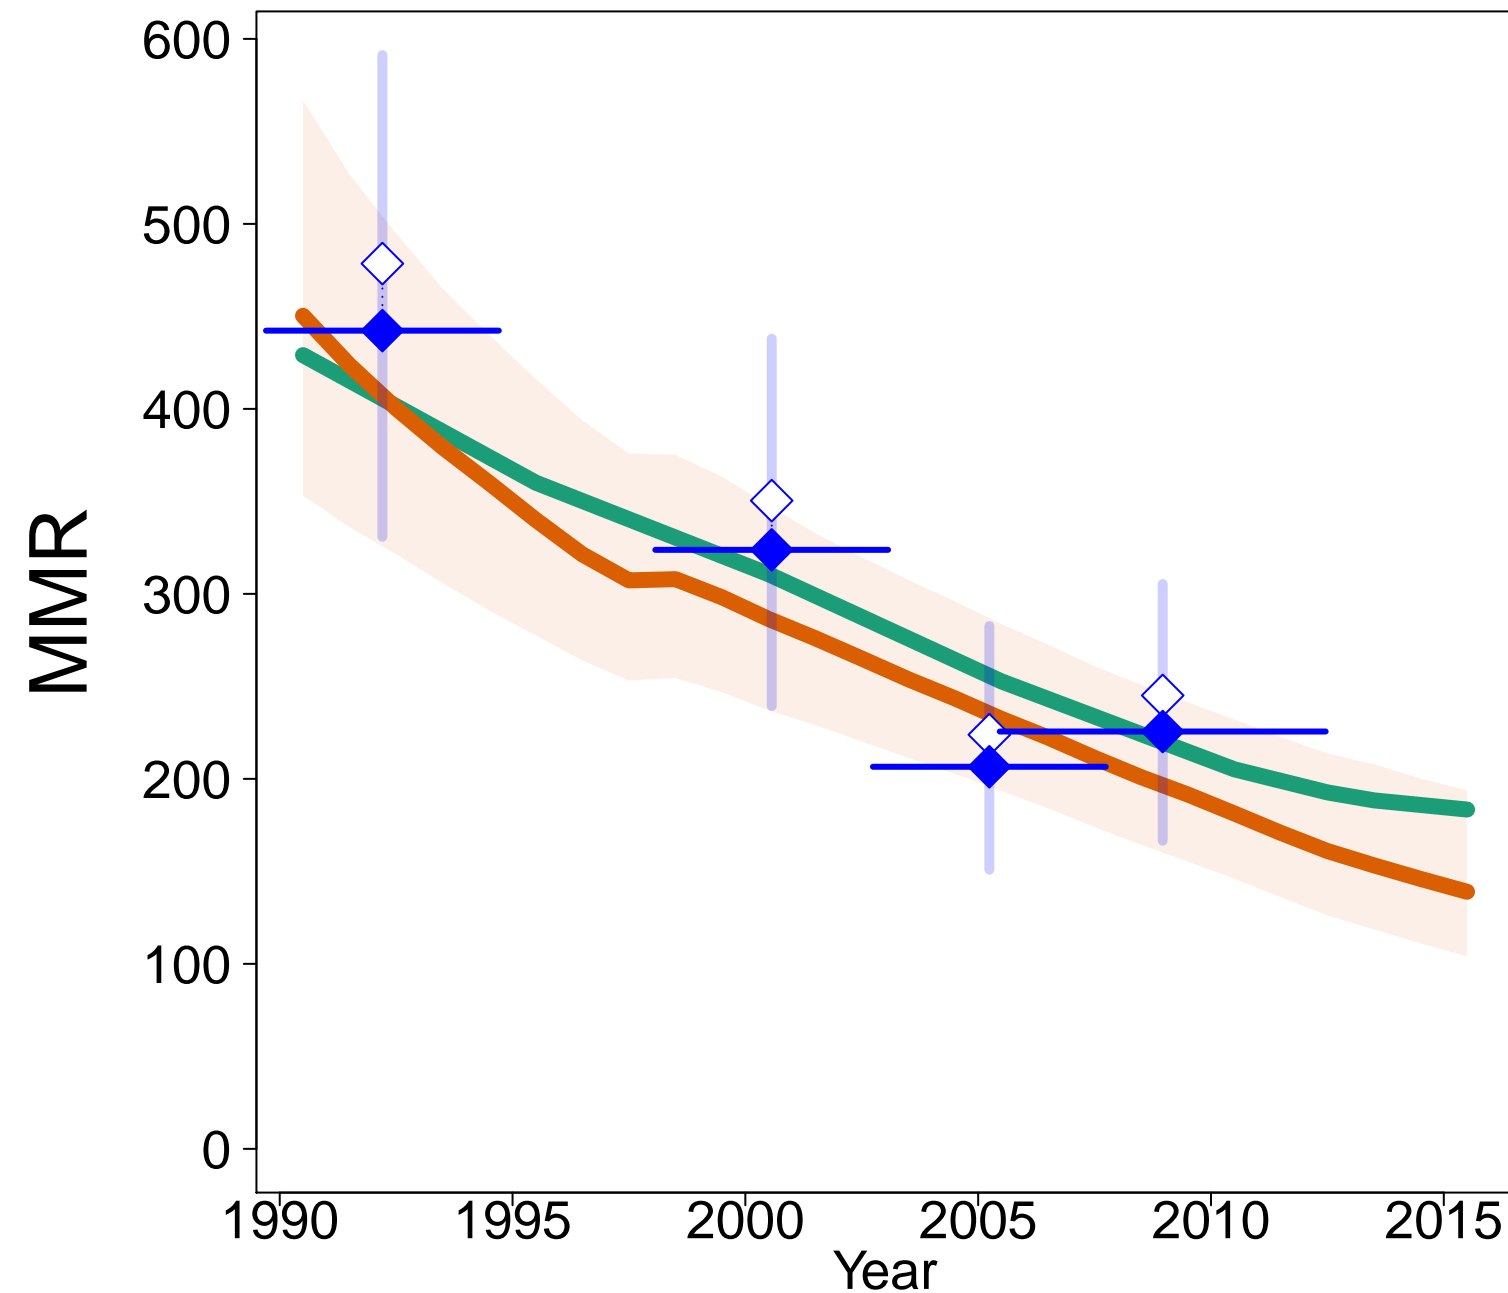

– Estimates –  
 Bmat 2014  
 MMEIG 2014  
 – Data –  
 Observed Data  
 Adjusted Data  
 – Data type –  
 DHS

Iran [IRN; B]  
(Southern Asia)

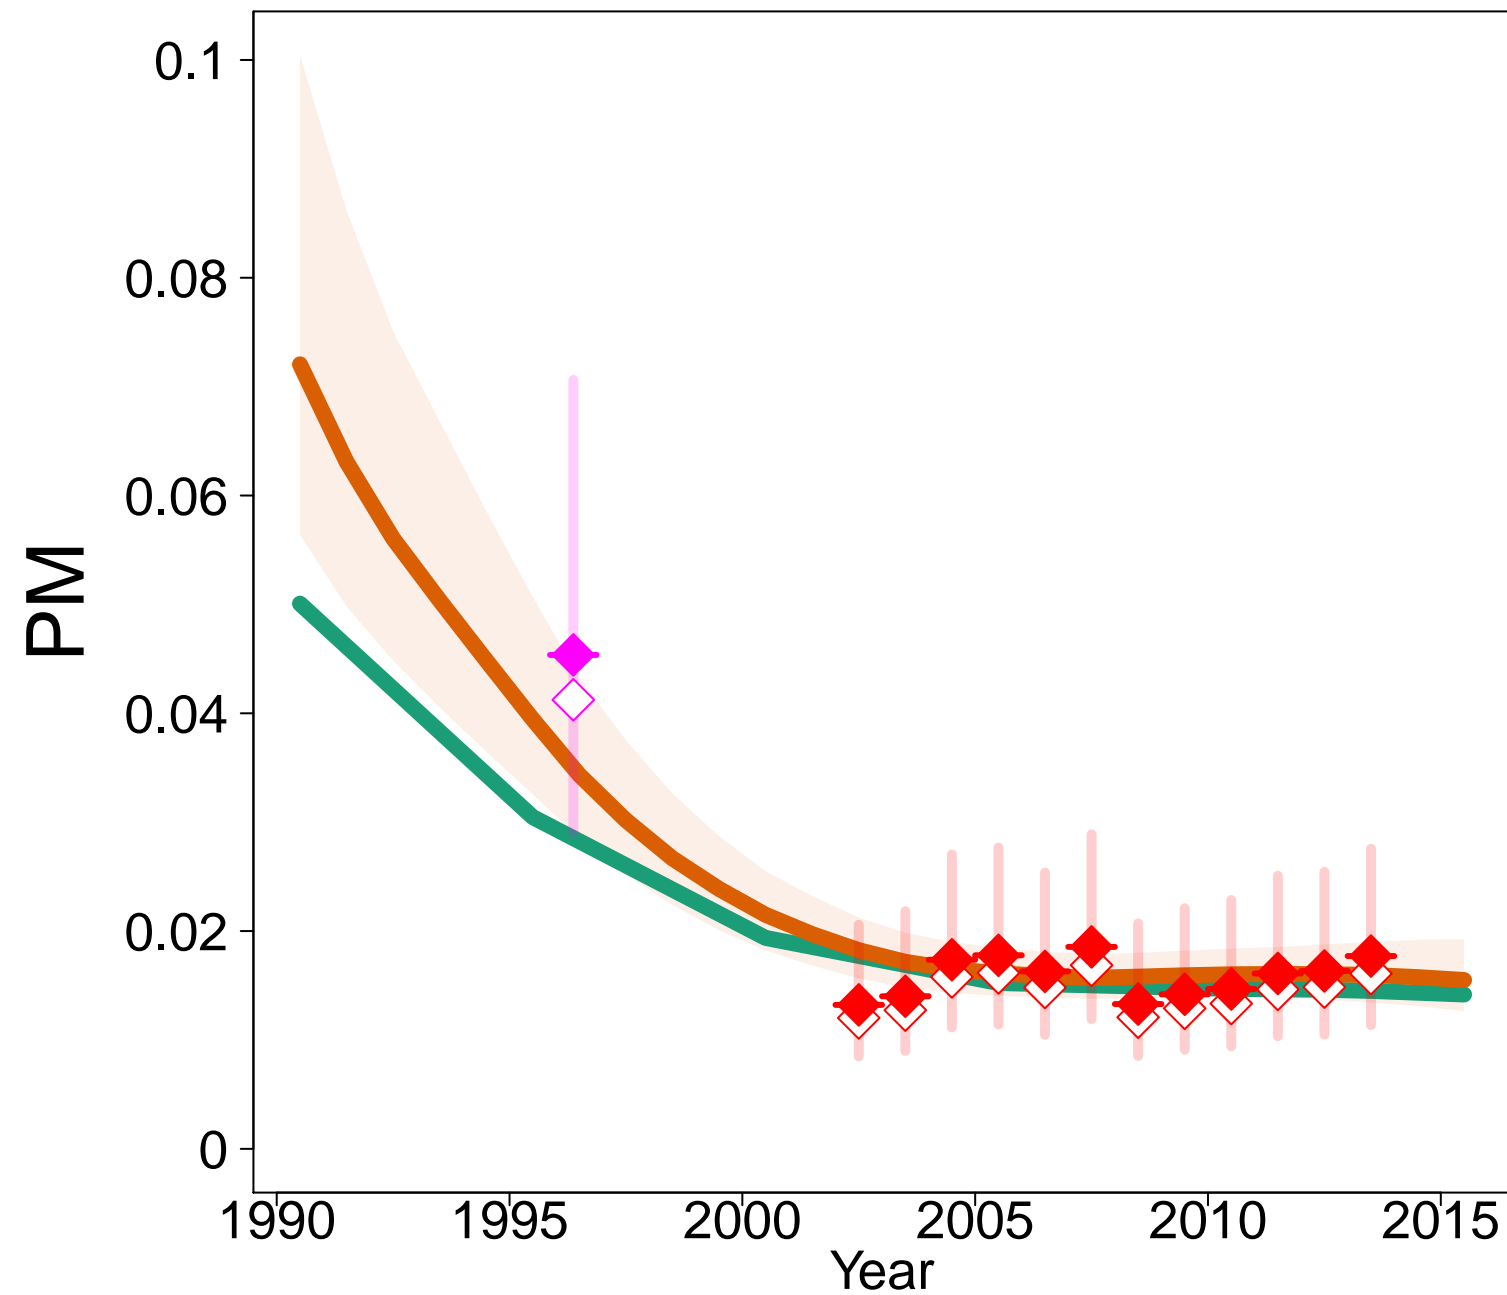

Iran [IRN; B]  
(Southern Asia)

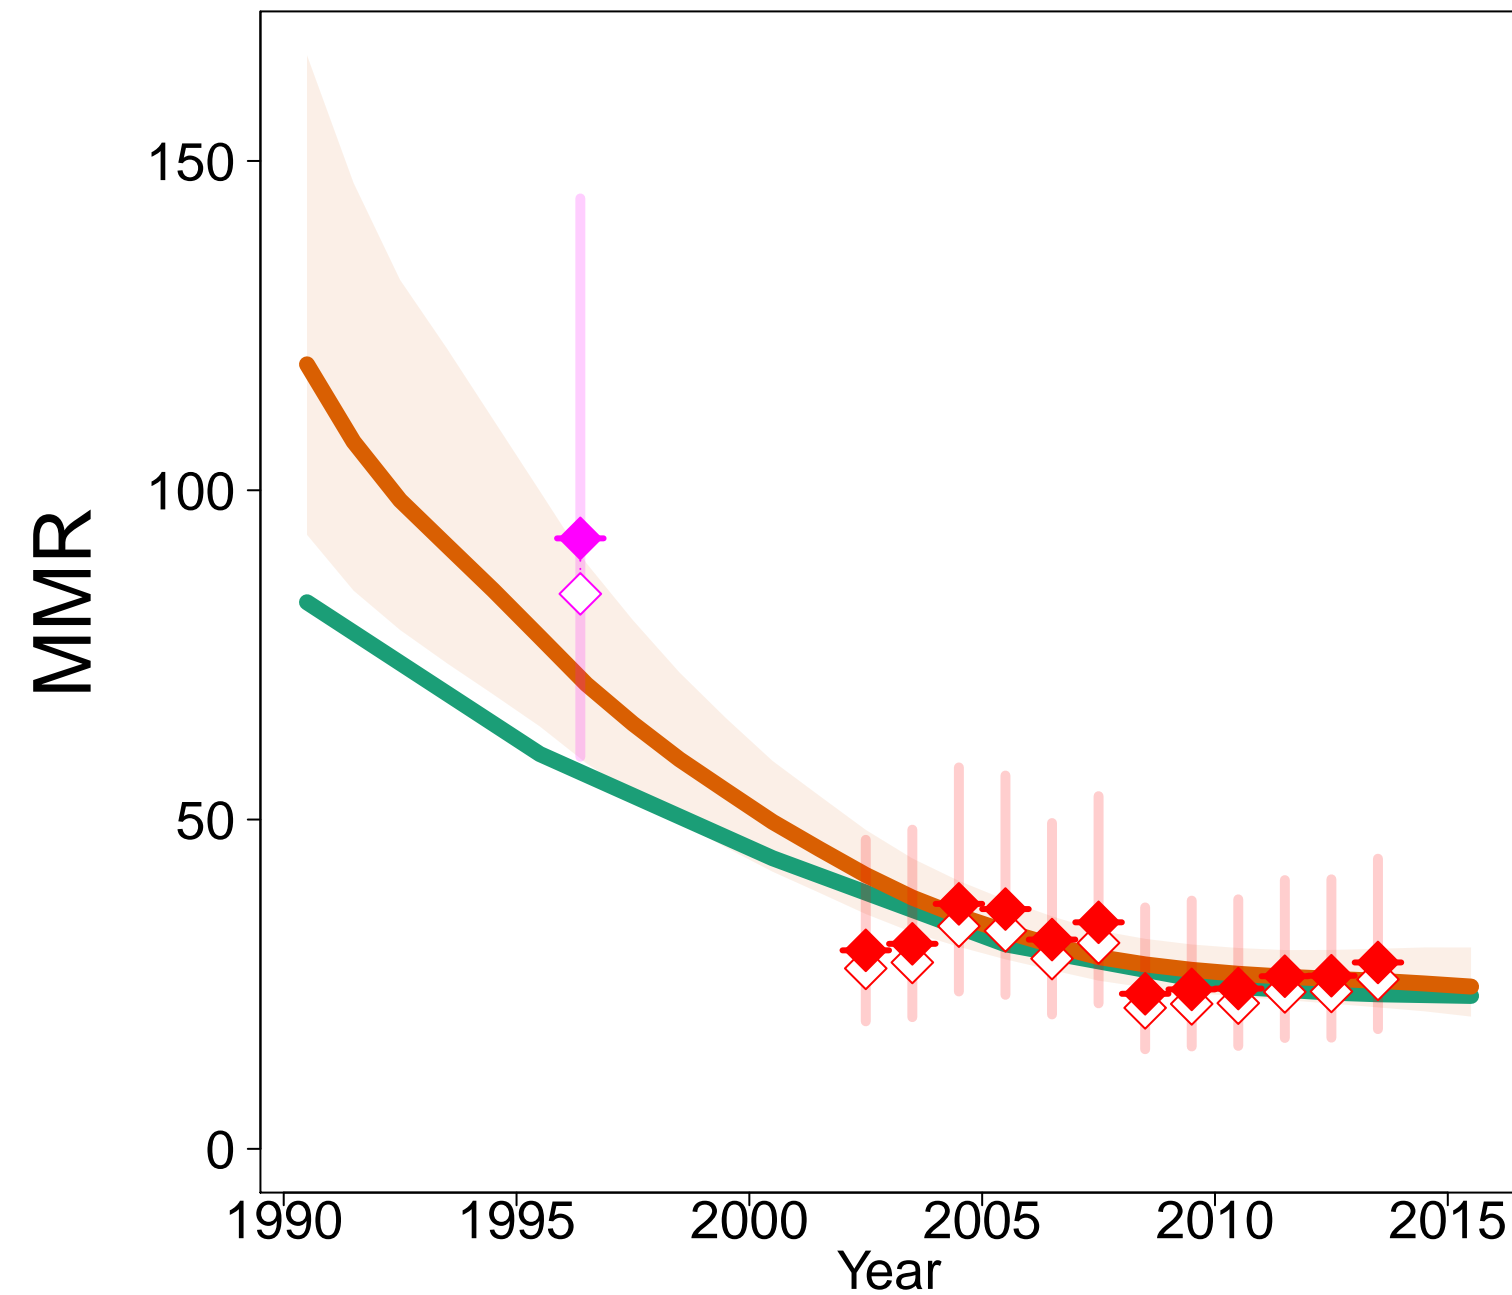

- Estimates –
- Bmat 2014
- MMEIG 2014
- Data –
- Observed Data
- Adjusted Data
- Data type –
- Census
- Misc. studies

Iraq [IRQ; B]  
(Western Asia)

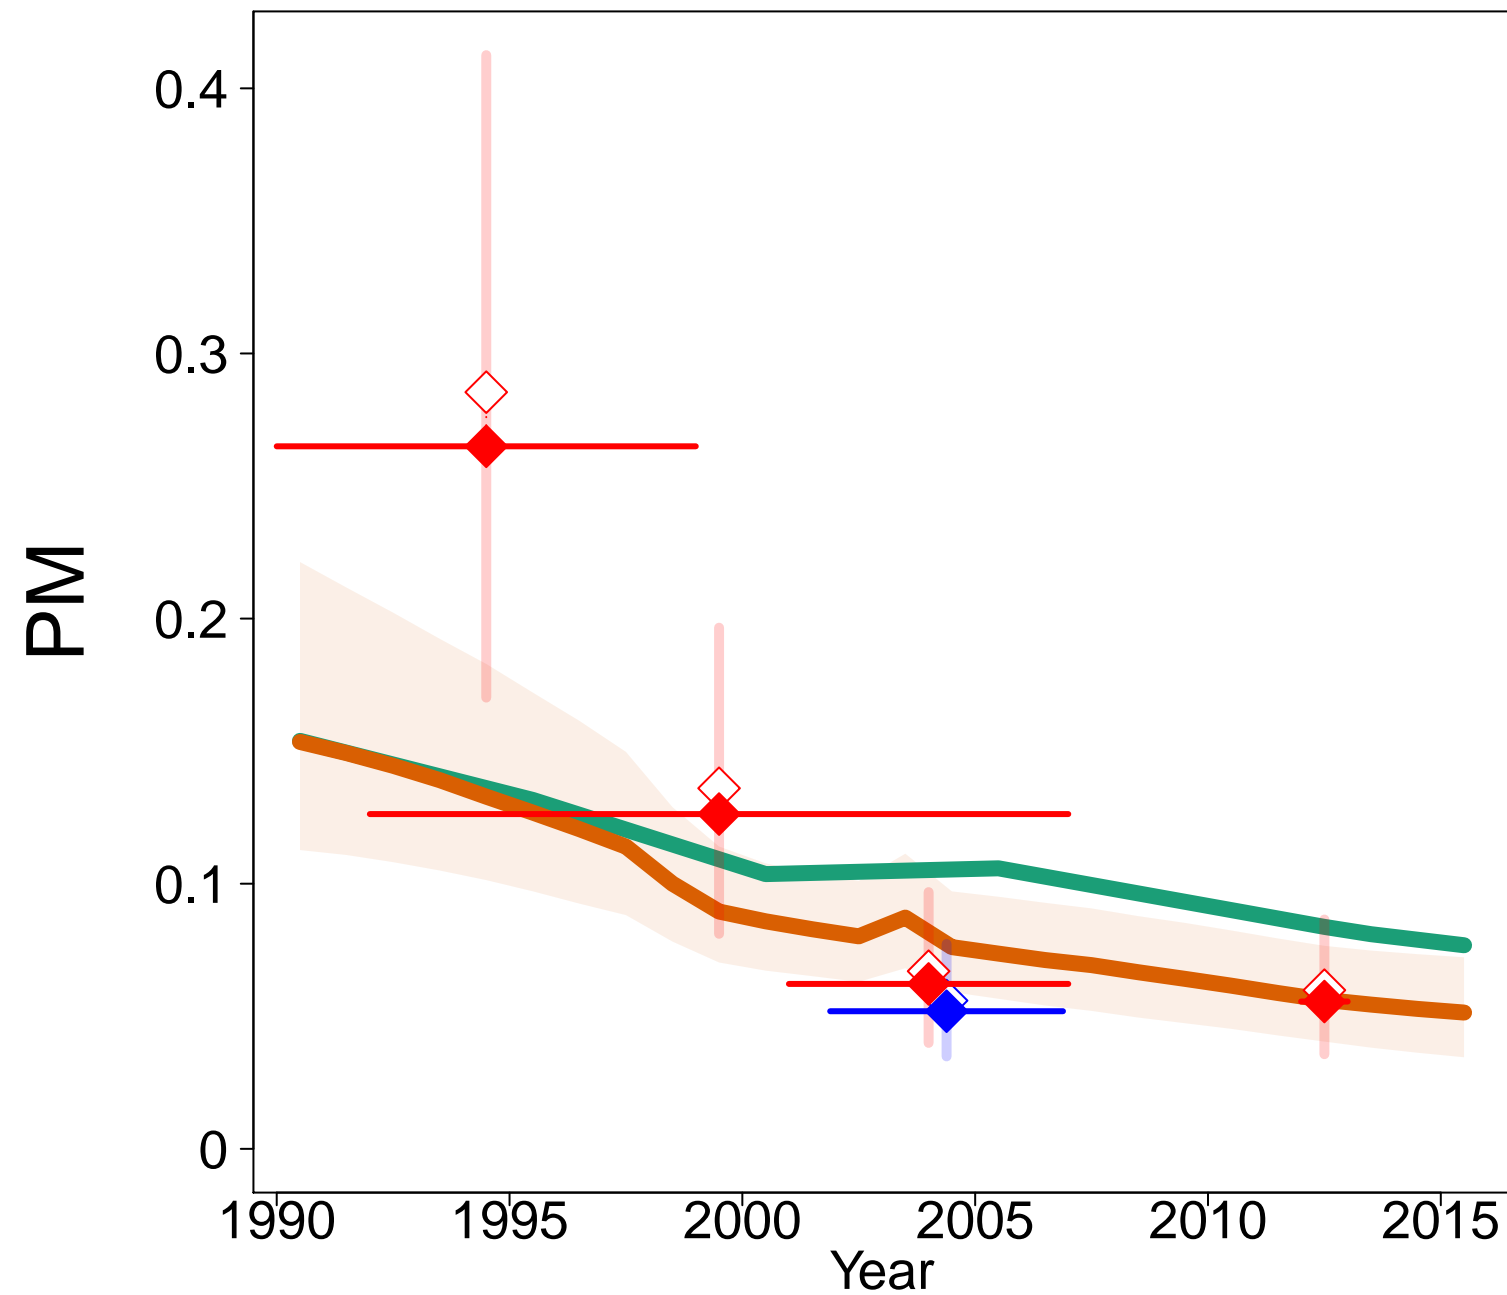

Iraq [IRQ; B]  
(Western Asia)

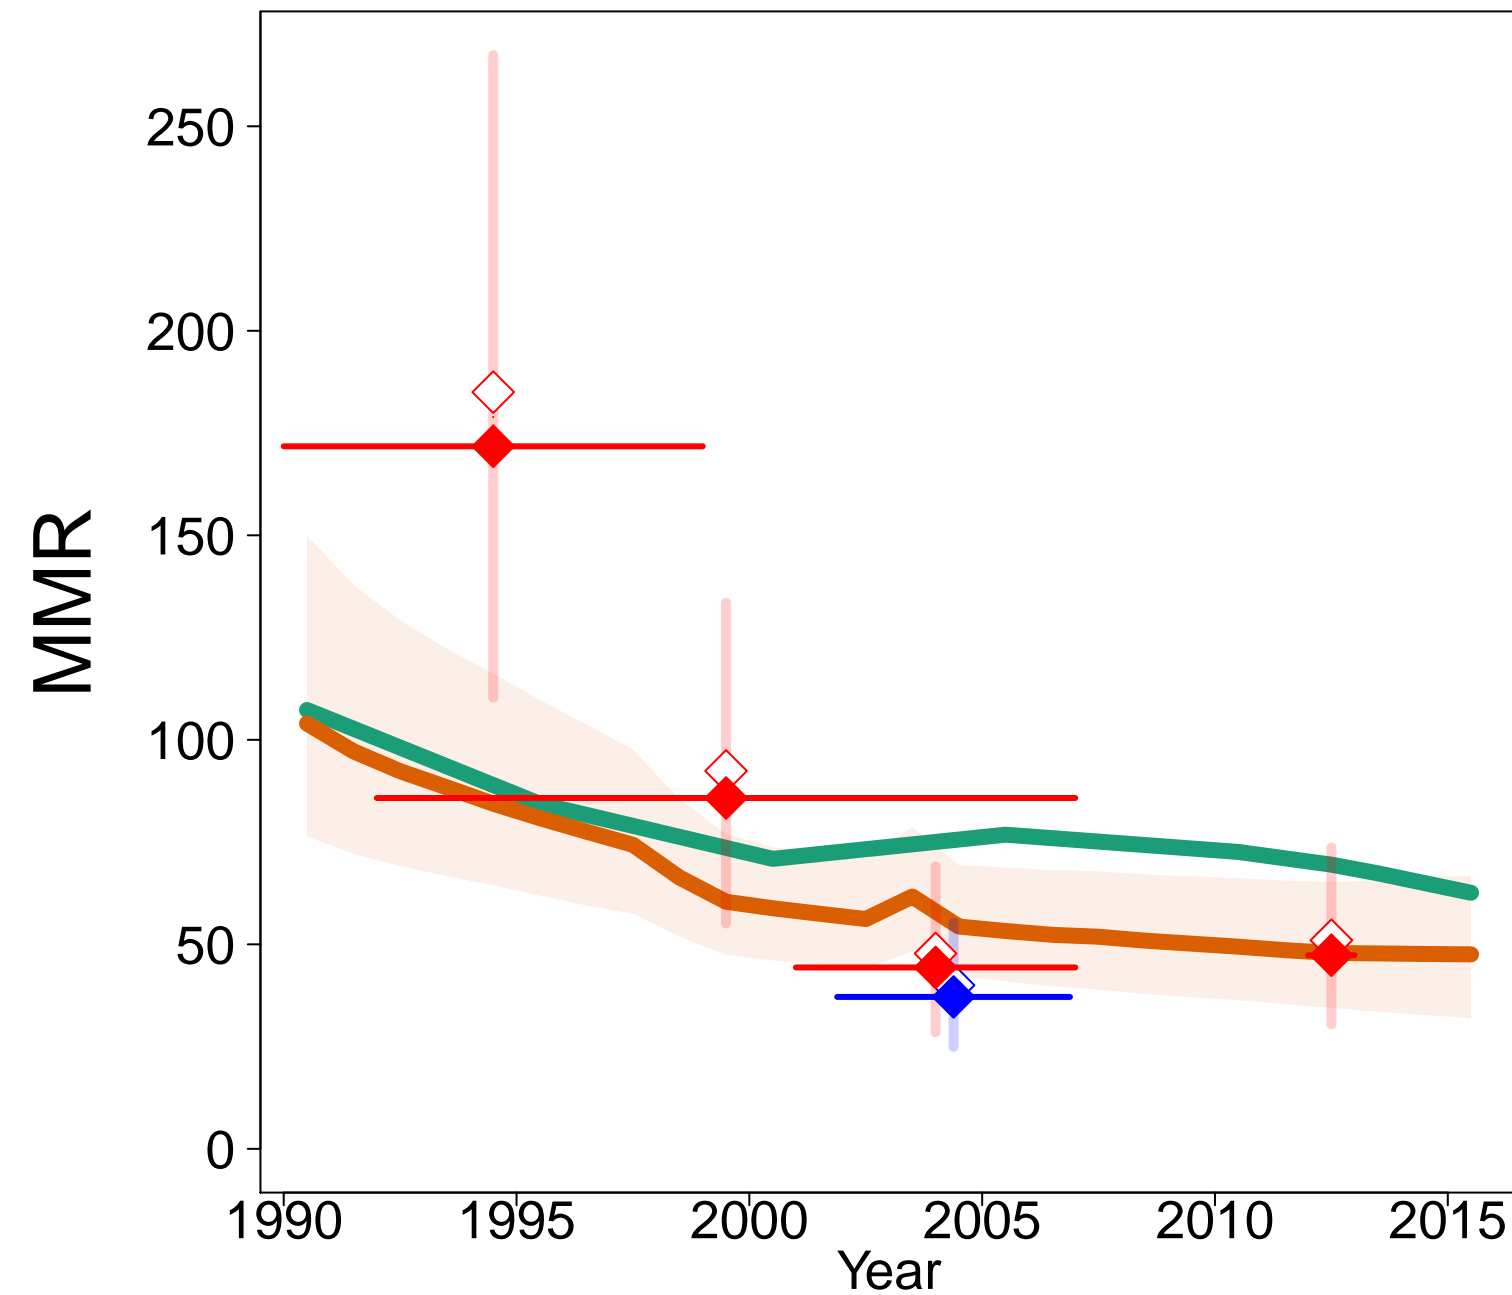

- Estimates –
- Bmat 2014
- MMEIG 2014
- Data –
- Observed Data
- Adjusted Data
- Data type –
- DHS
- Misc. studies

Ireland [IRL; A]  
(Developed regions)

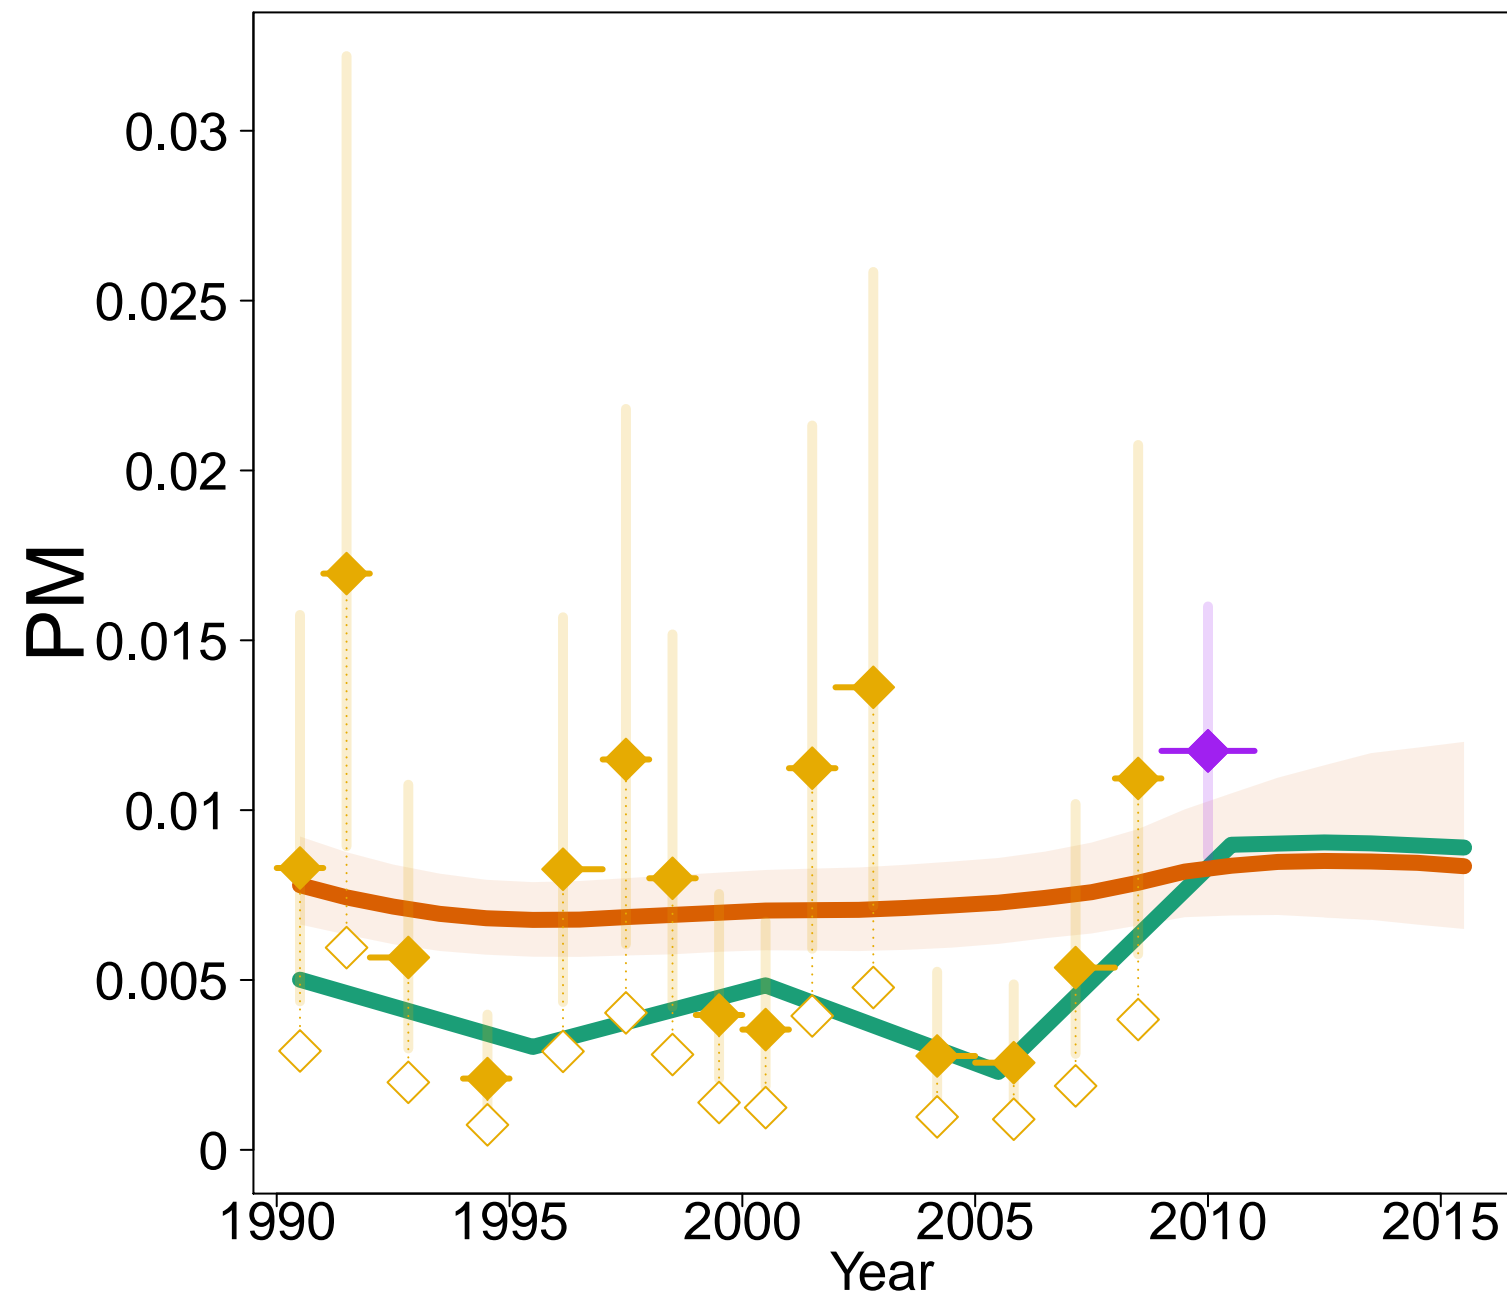

Ireland [IRL; A]  
(Developed regions)

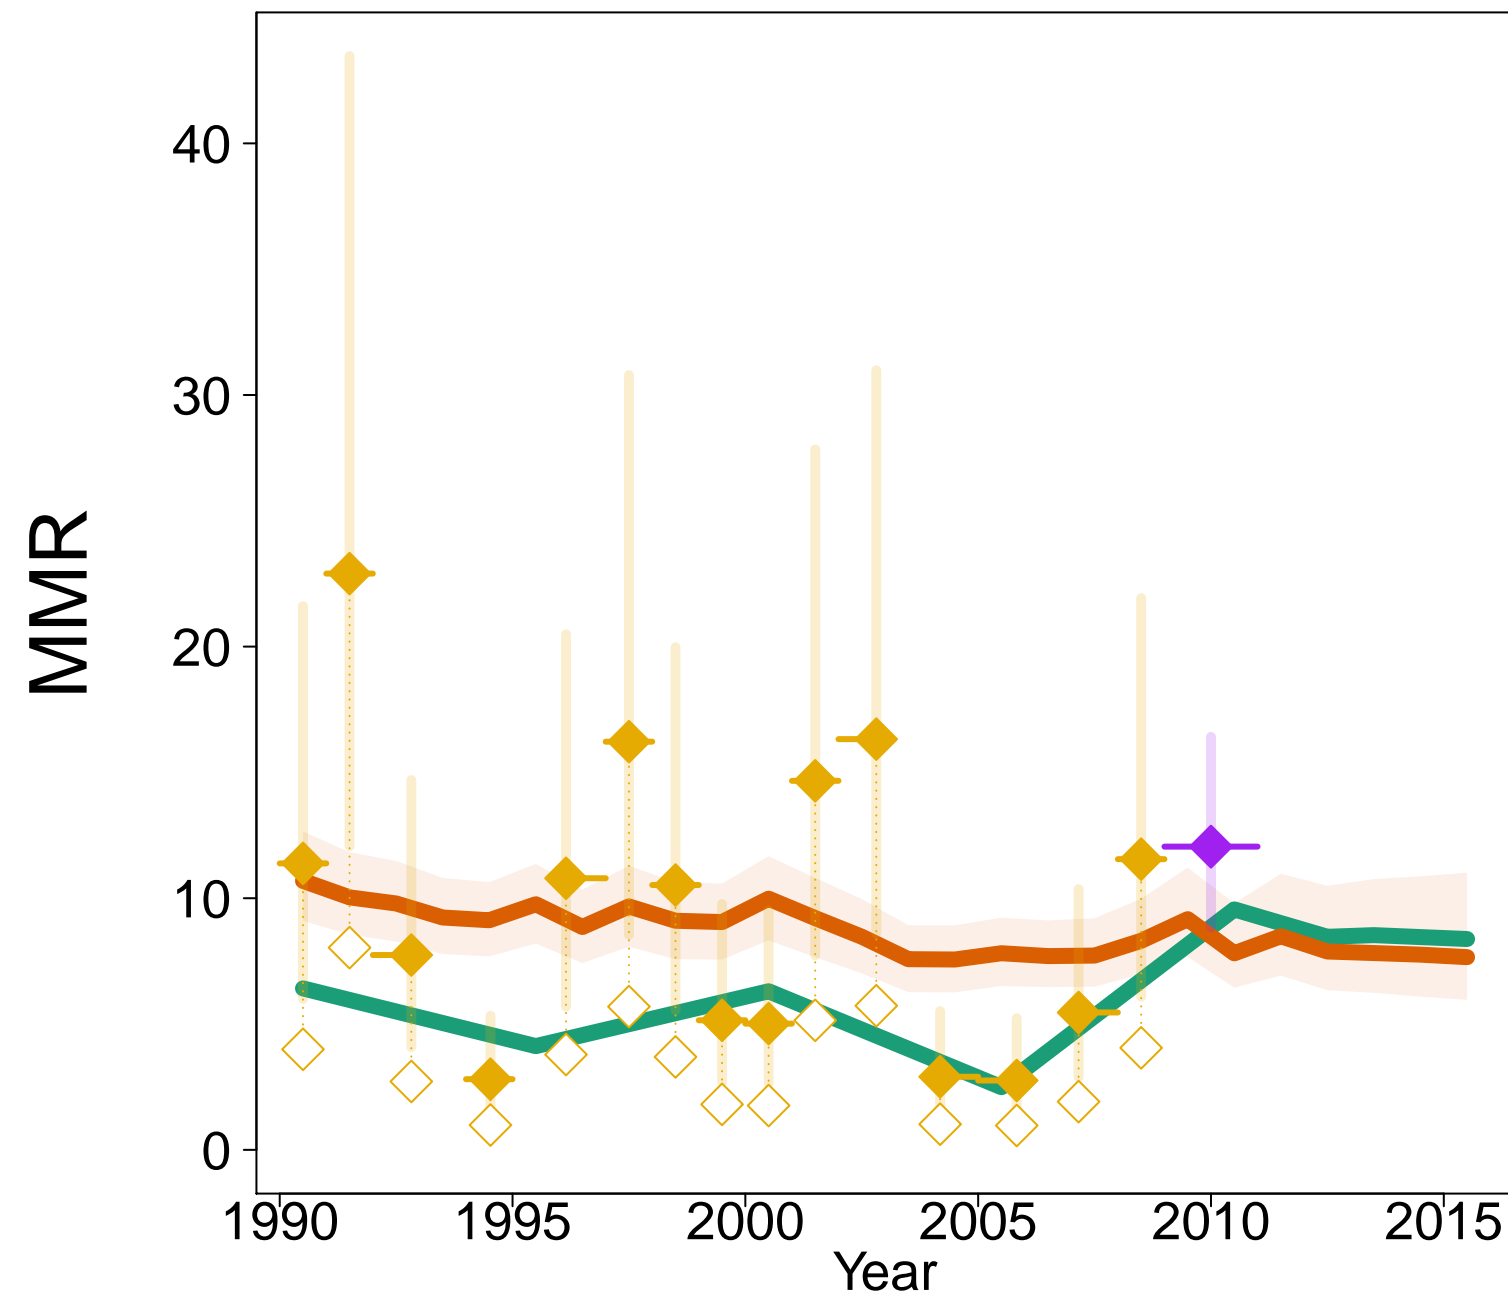

- Estimates –
- Bmat 2014
- MMEIG 2014
- Data –
- Observed Data
- Adjusted Data
- Data type –
- VR
- Spec. studies

Israel [ISR; A]  
(Western Asia)

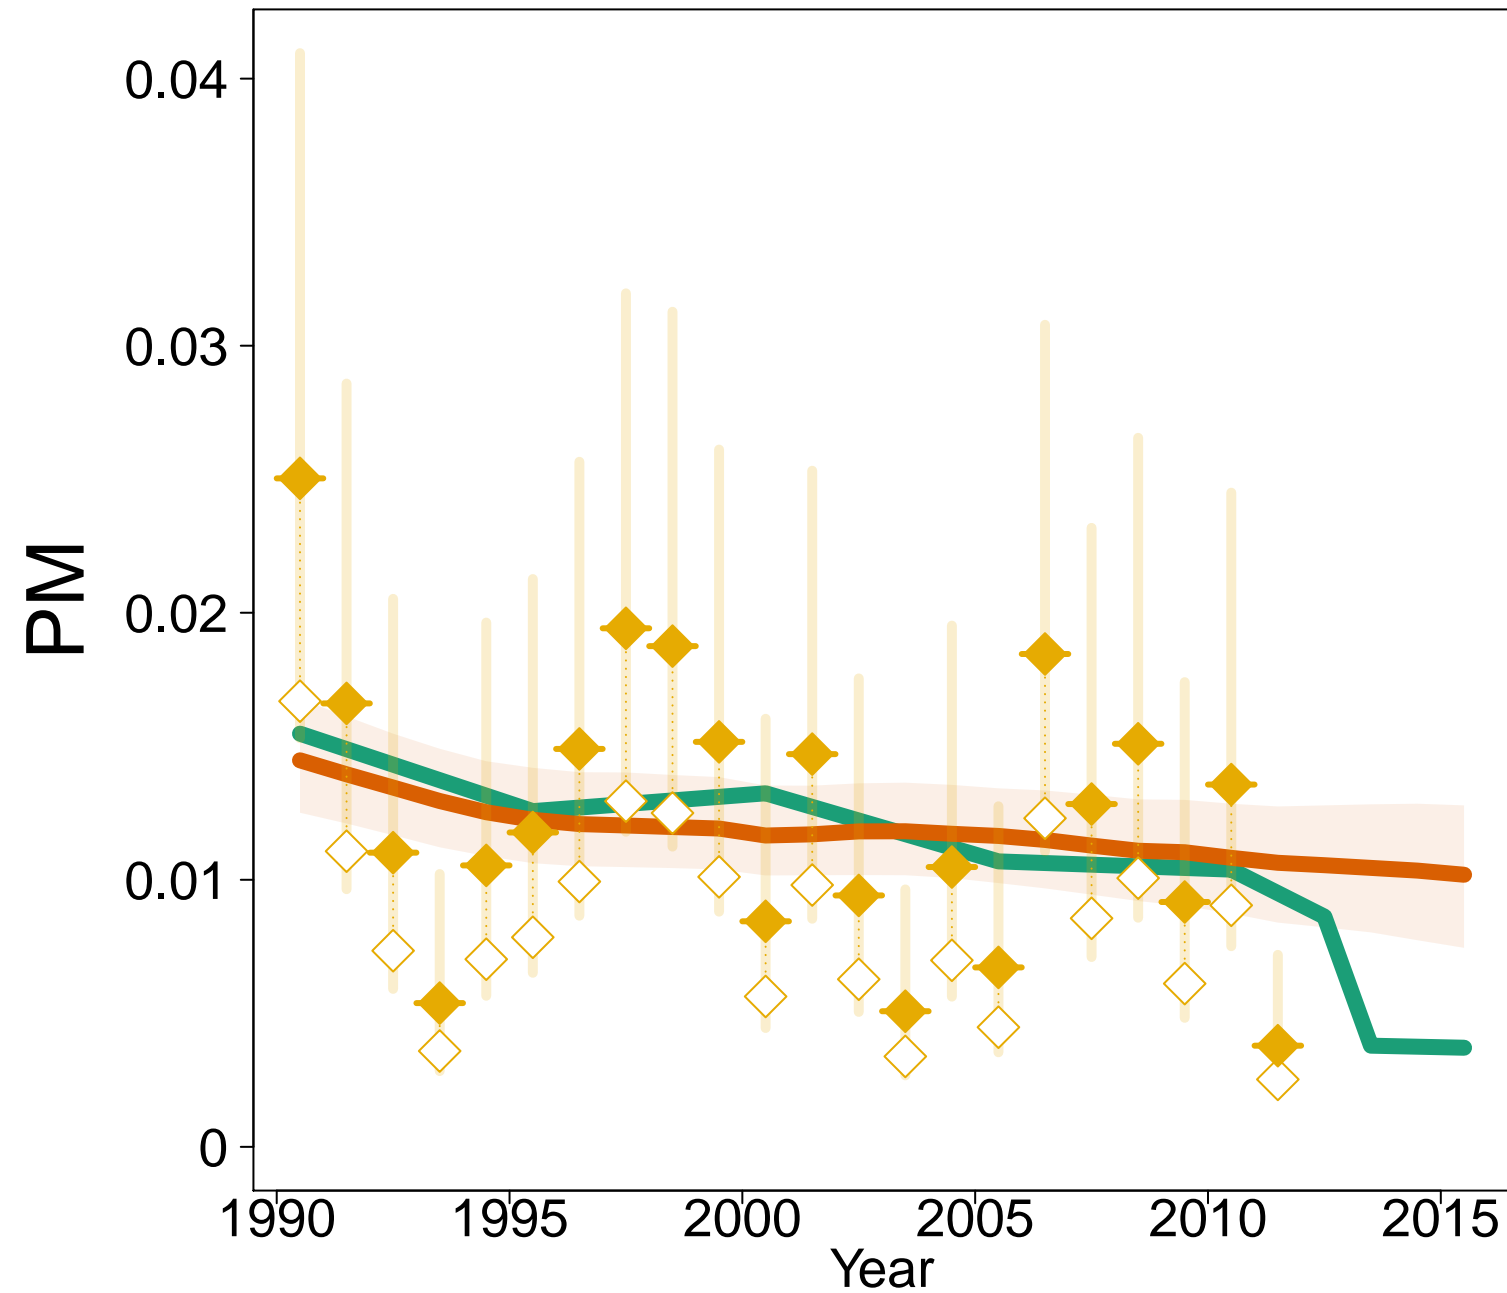

Israel [ISR; A]  
(Western Asia)

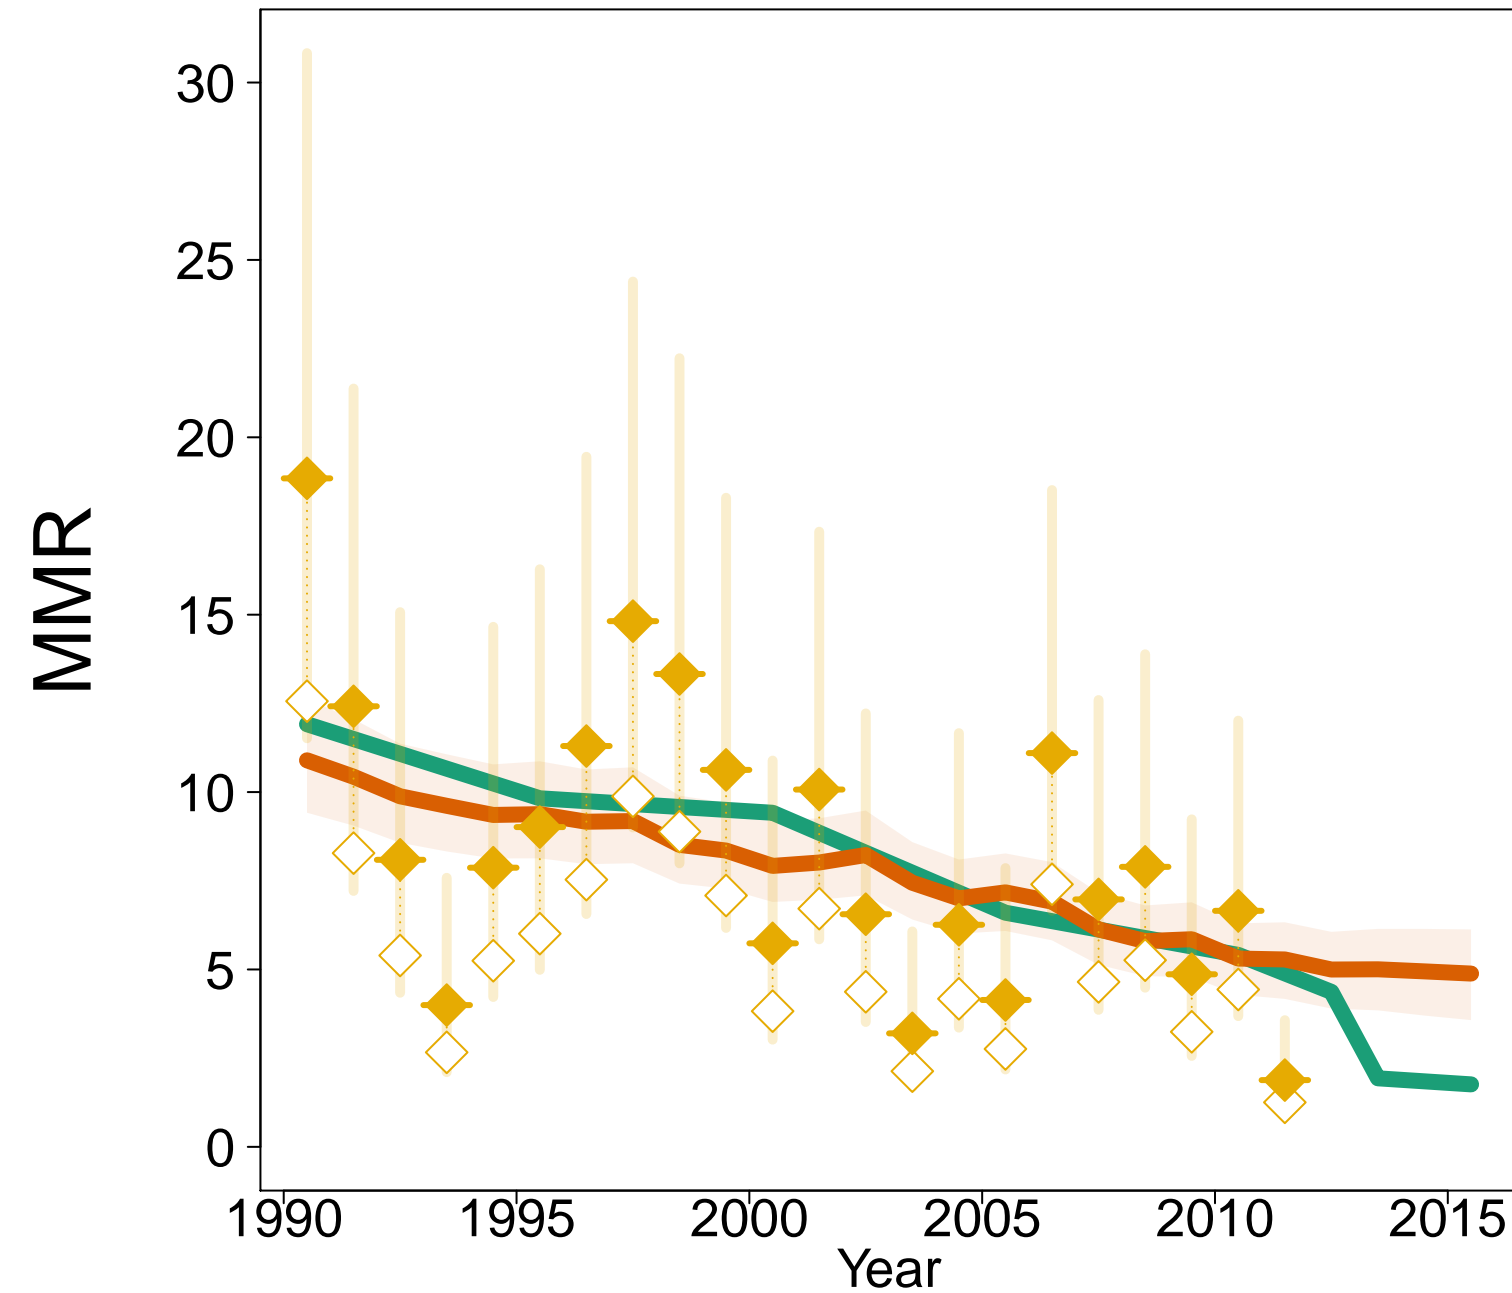

- Estimates –
- Bmat 2014
- MMEIG 2014
- Data –
- Observed Data
- Adjusted Data
- Data type –
- VR

Italy [ITA; A]  
(Developed regions)

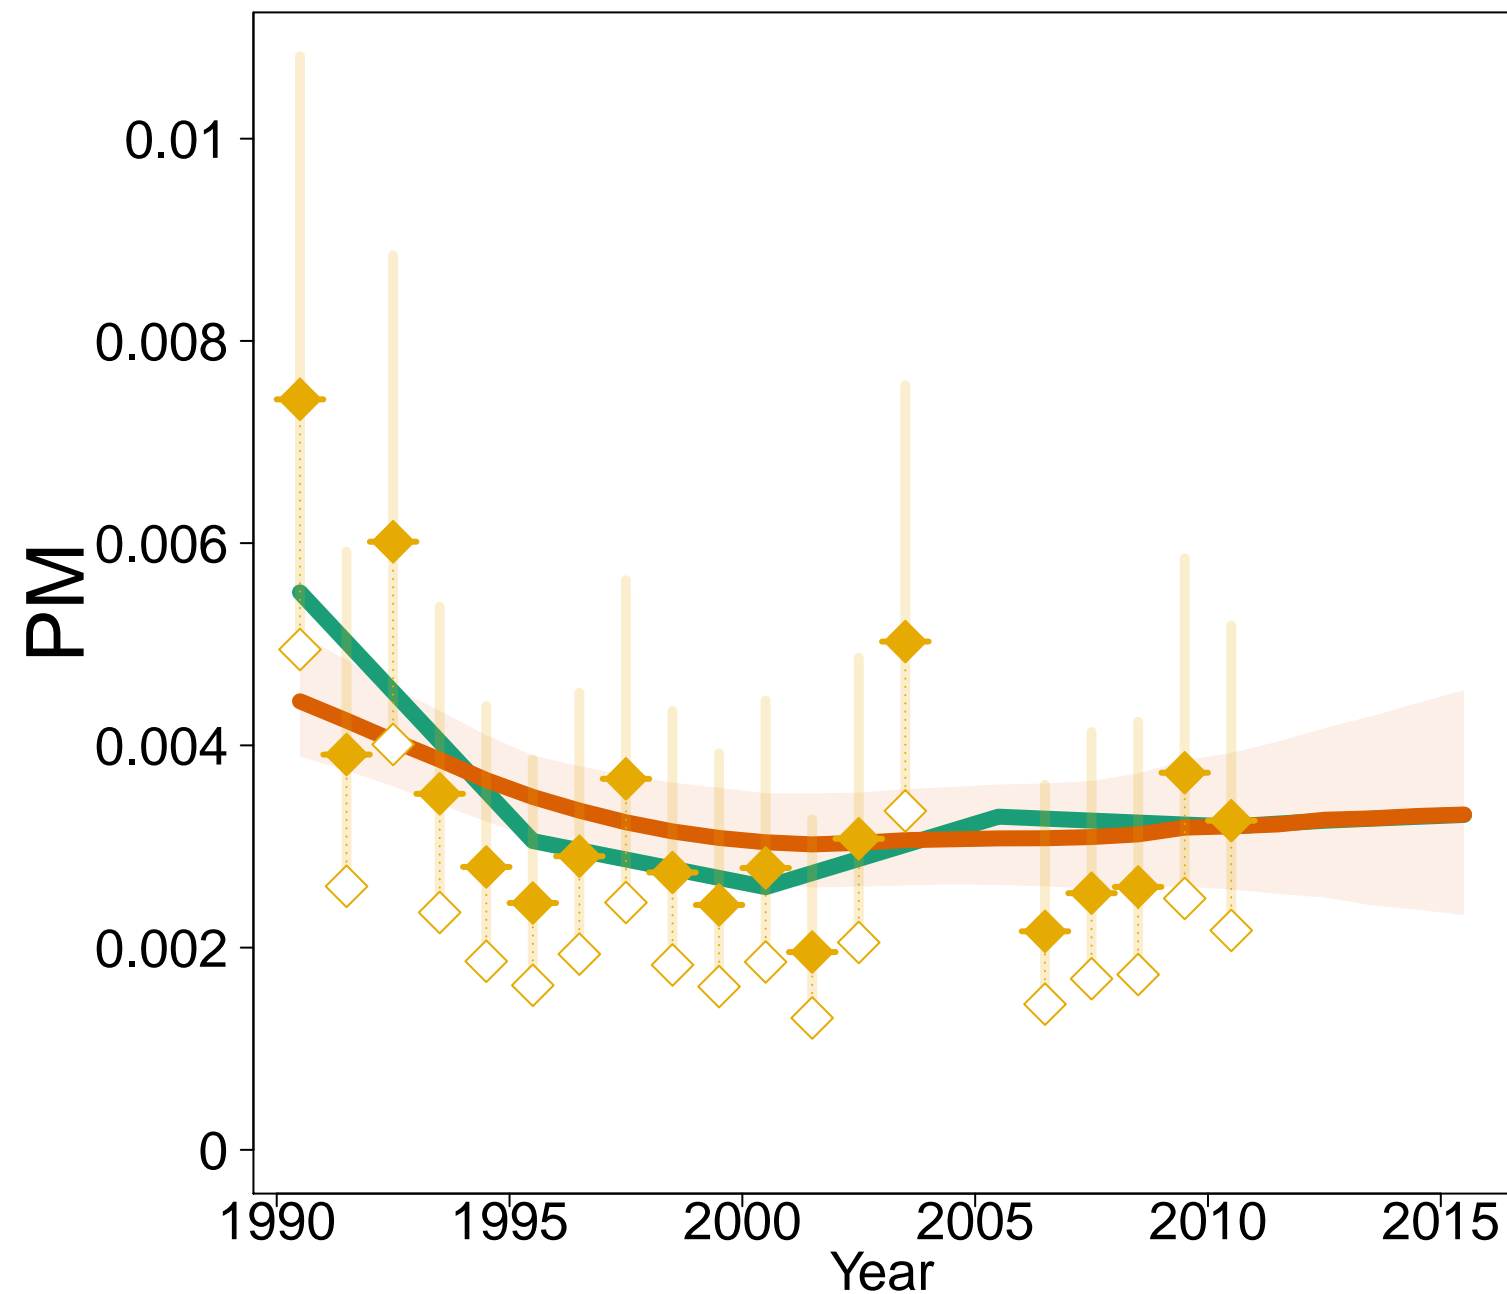

Italy [ITA; A]  
(Developed regions)

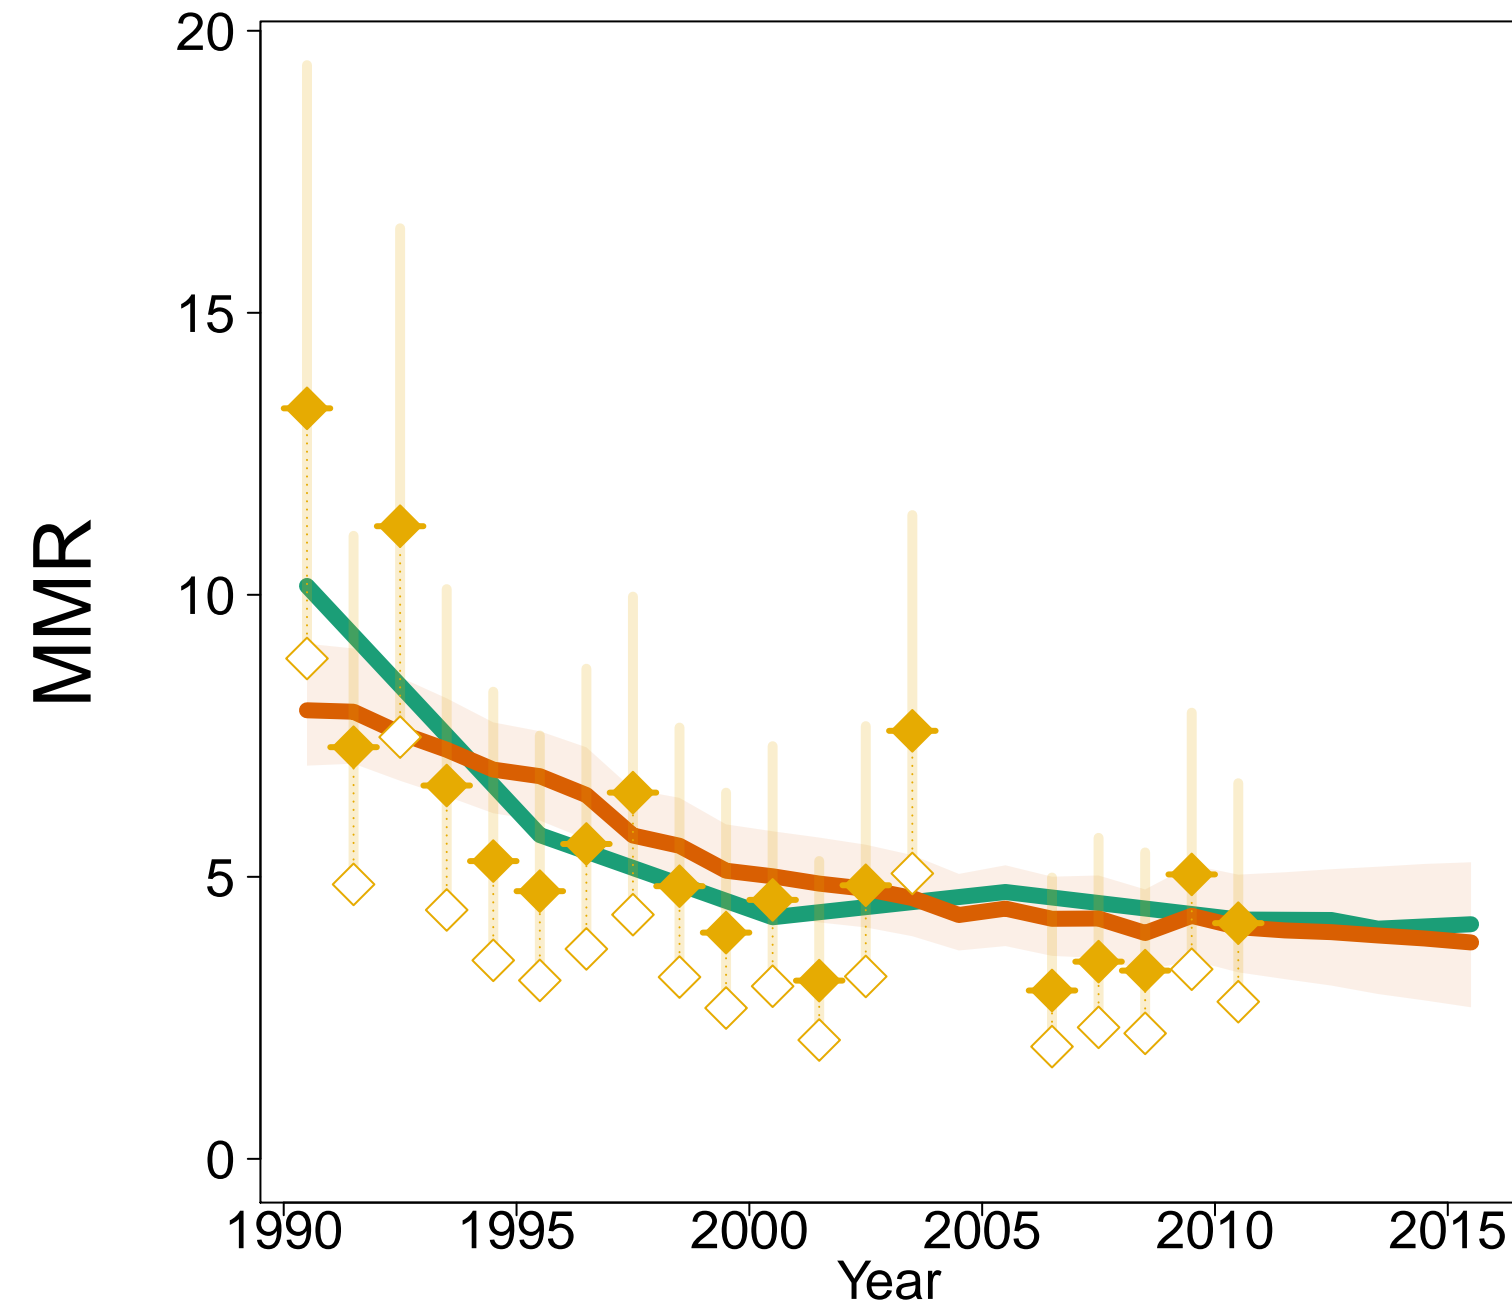

- Estimates –
- Bmat 2014
- MMEIG 2014
- Data –
- Observed Data
- Adjusted Data
- Data type –
- VR



Jamaica [JAM; B]  
(Caribbean)

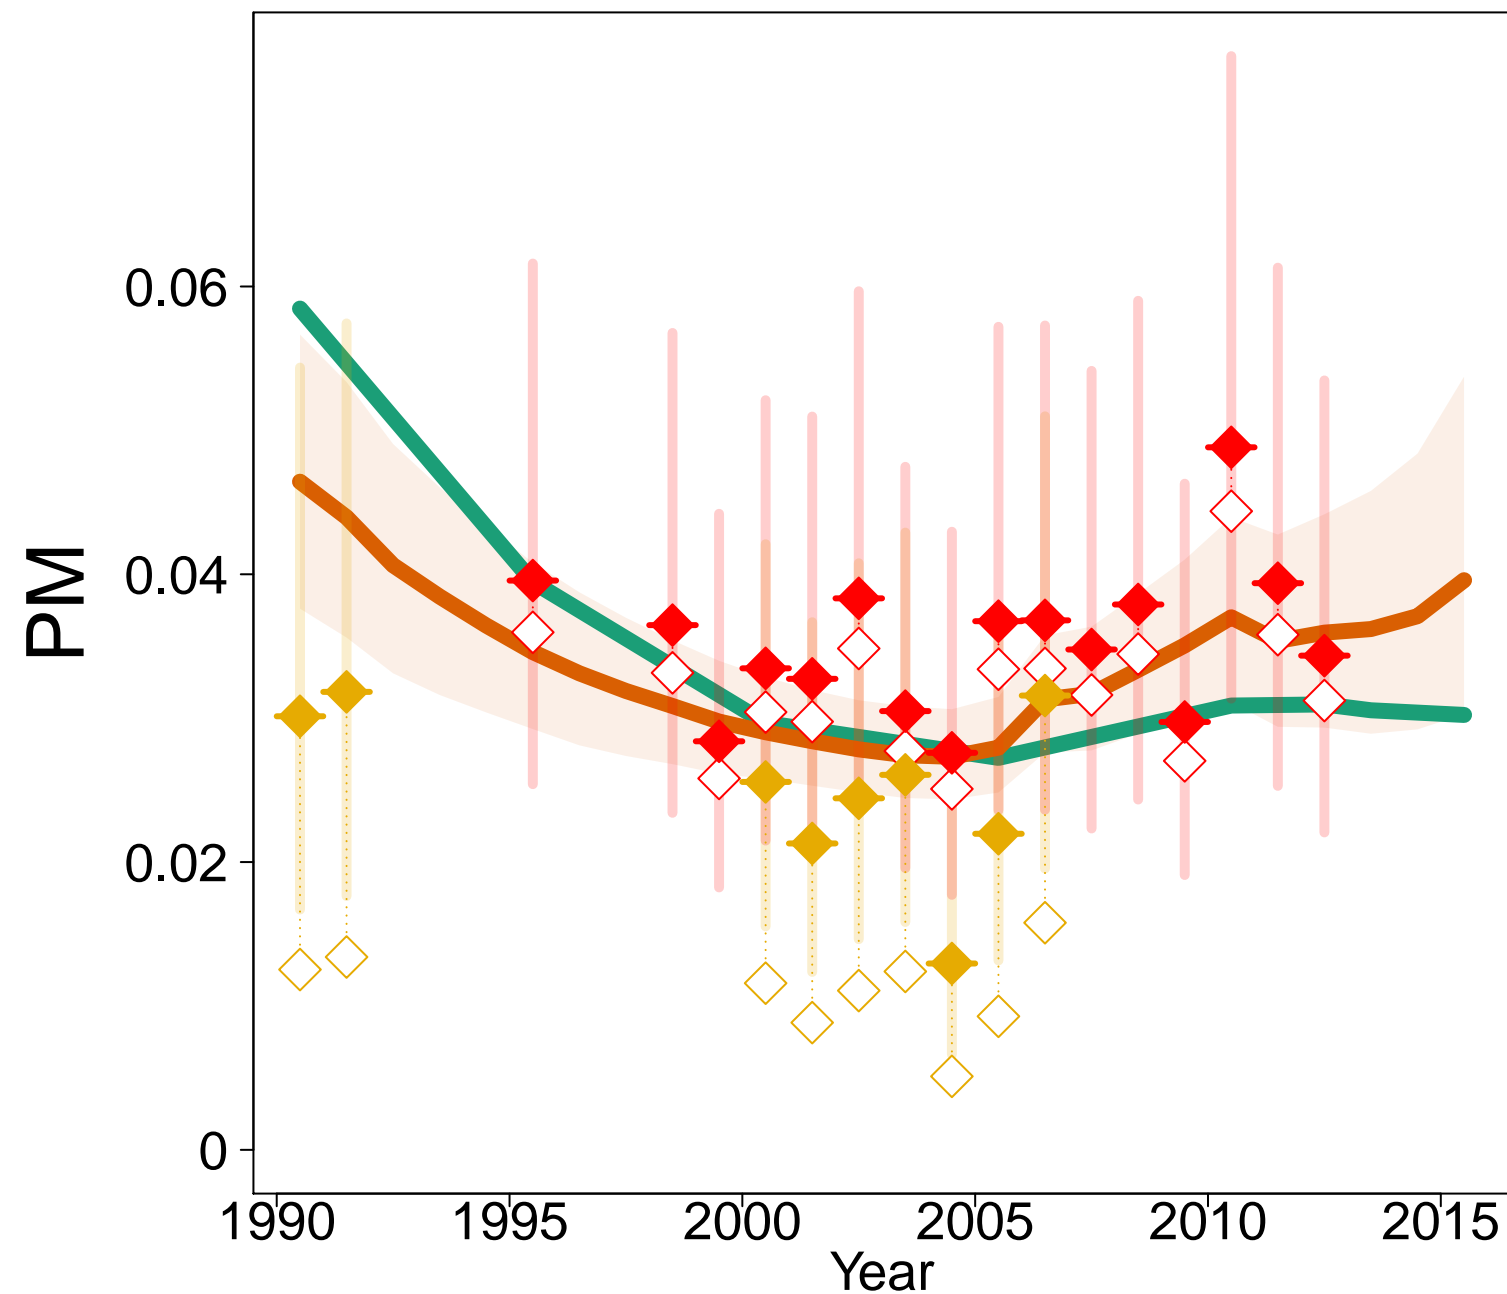

Jamaica [JAM; B]  
(Caribbean)

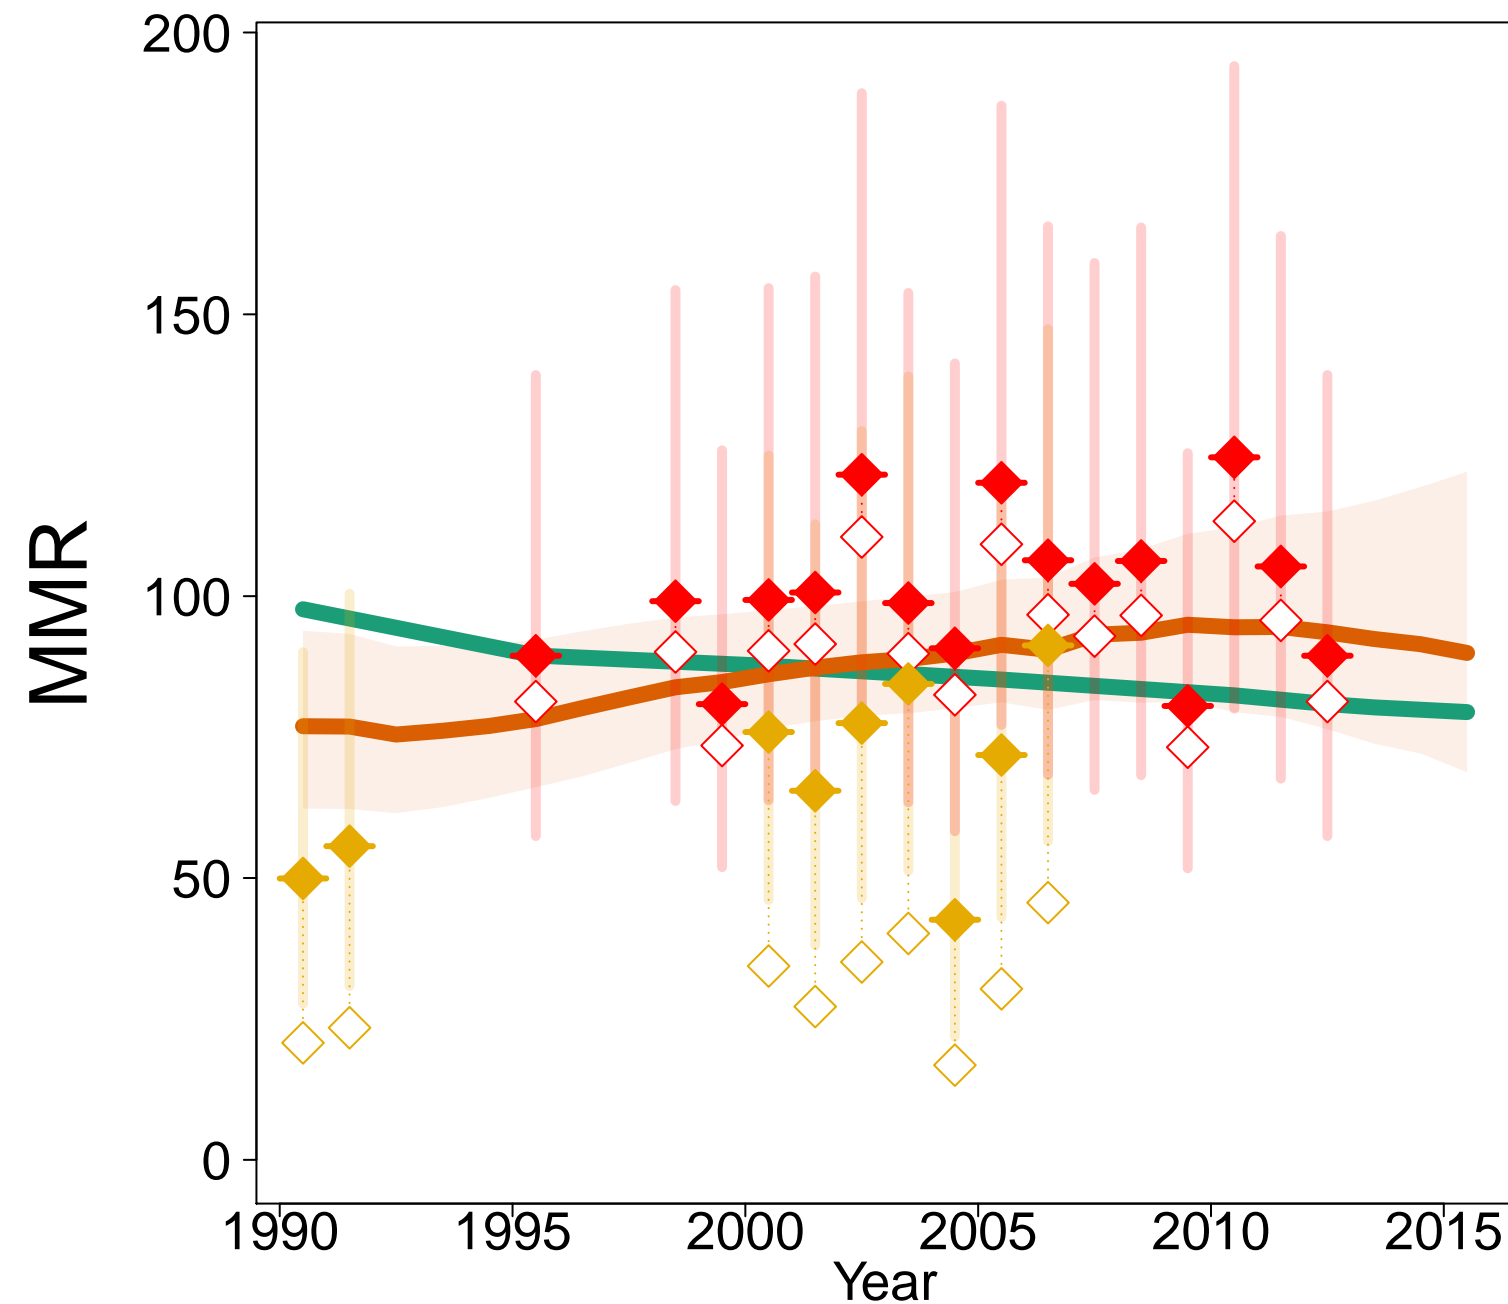

- Estimates –
- Bmat 2014
- MMEIG 2014
- Data –
- Observed Data
- Adjusted Data
- Data type –
- VR
- Misc. studies

Japan [JPN; A]  
(Developed regions)

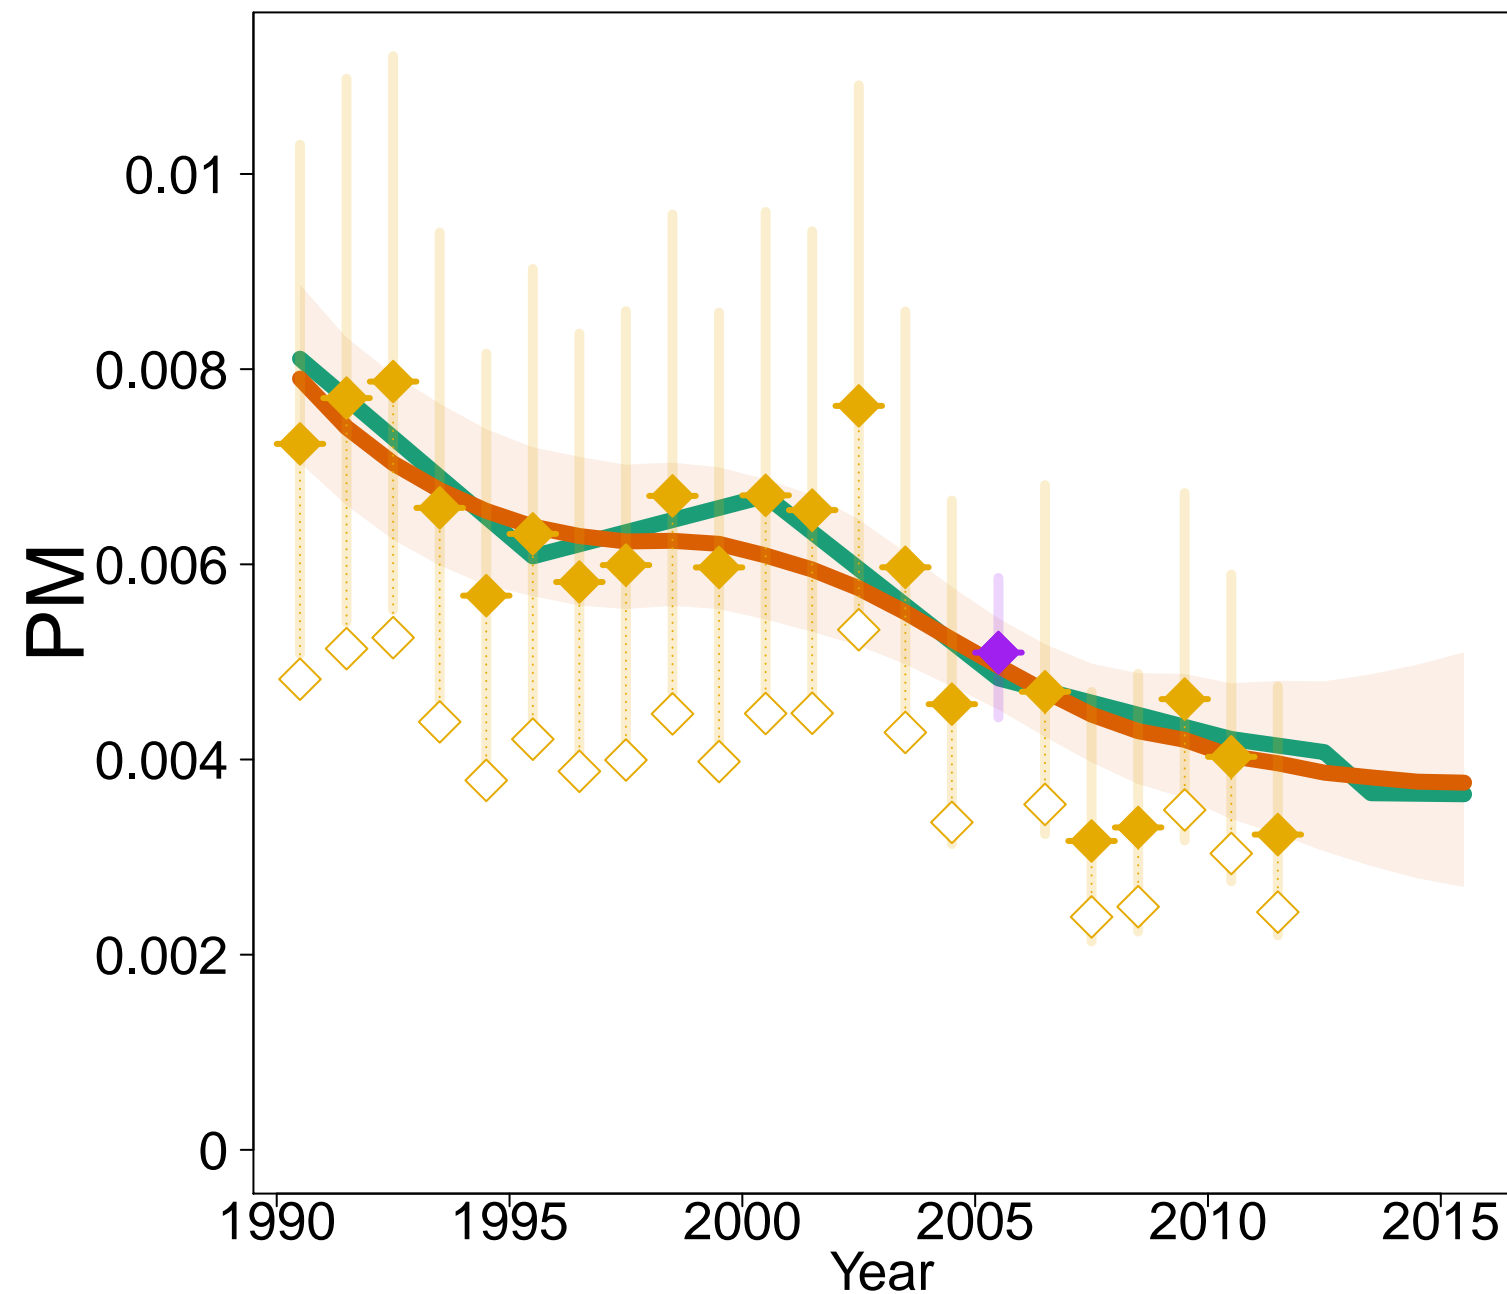

Japan [JPN; A]  
(Developed regions)

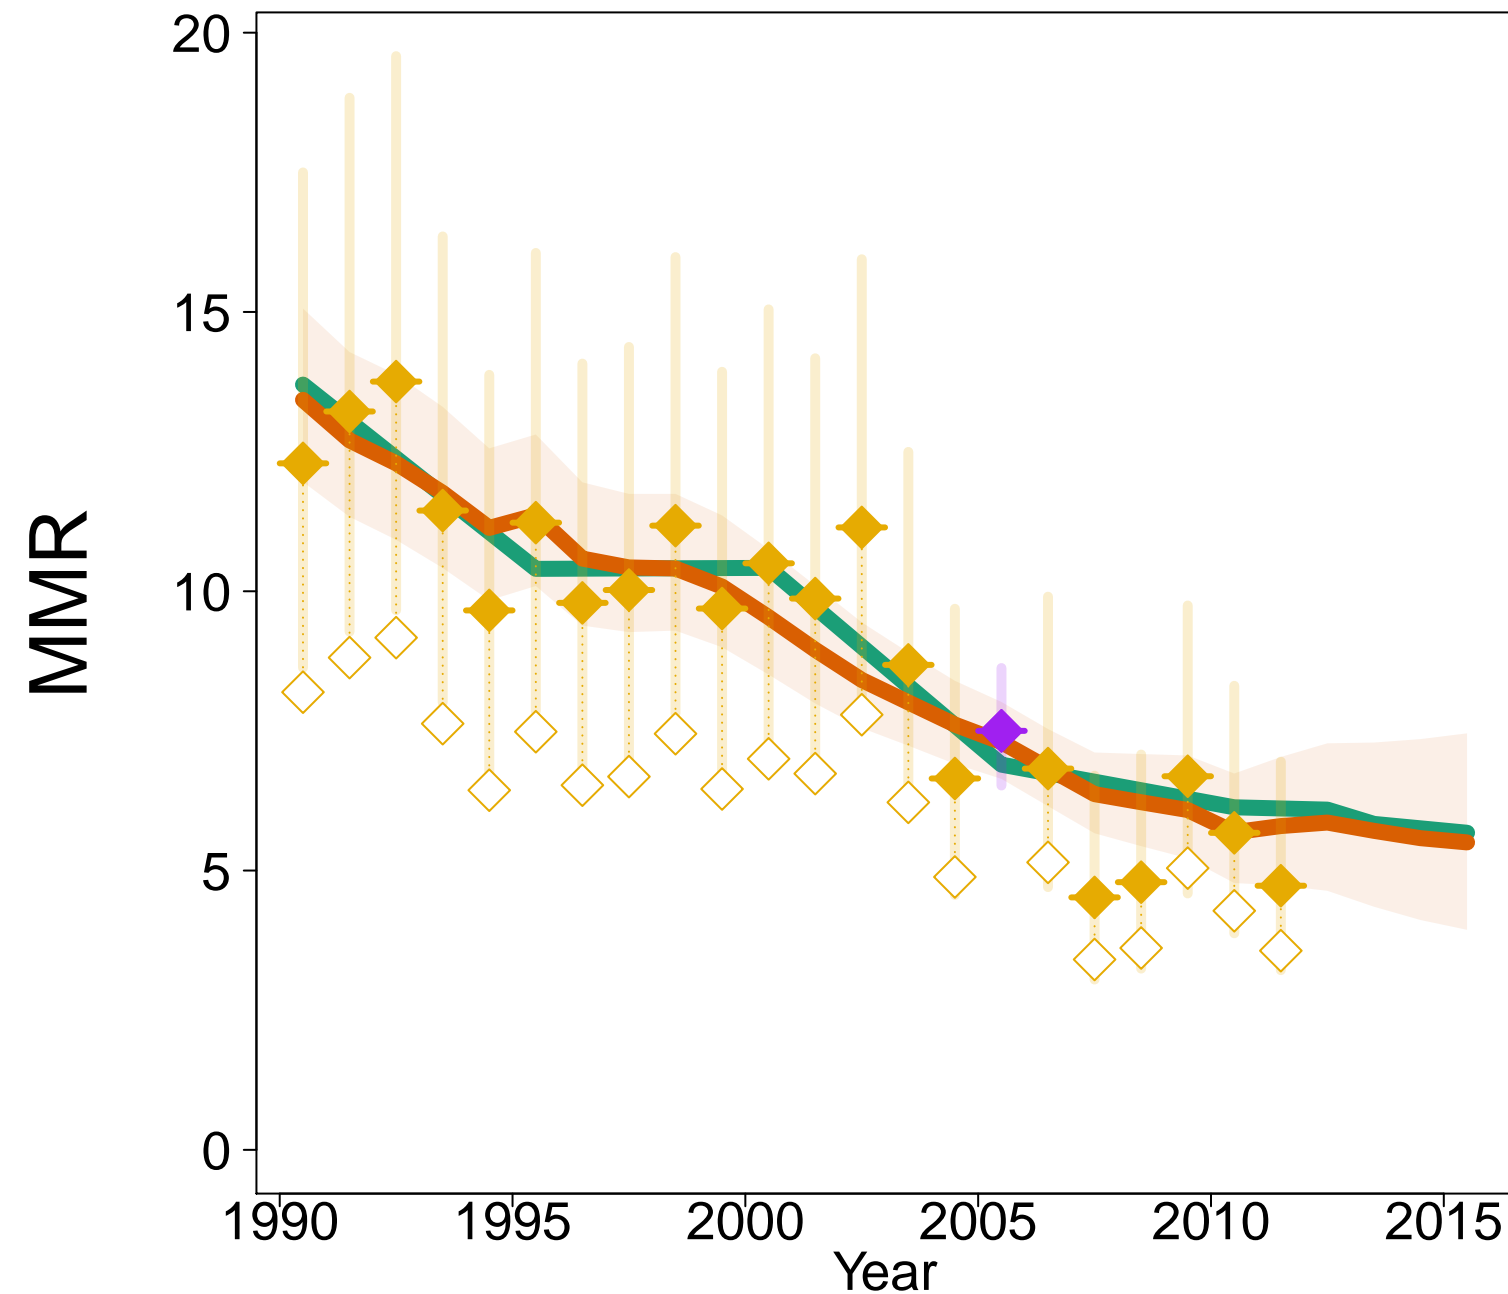

- Estimates –
- Bmat 2014
- MMEIG 2014
- Data –
- ◊ Observed Data
- ◆ Adjusted Data
- Data type –
- ◆ VR
- ◆ Spec. studies

Jordan [JOR; B]  
(Western Asia)

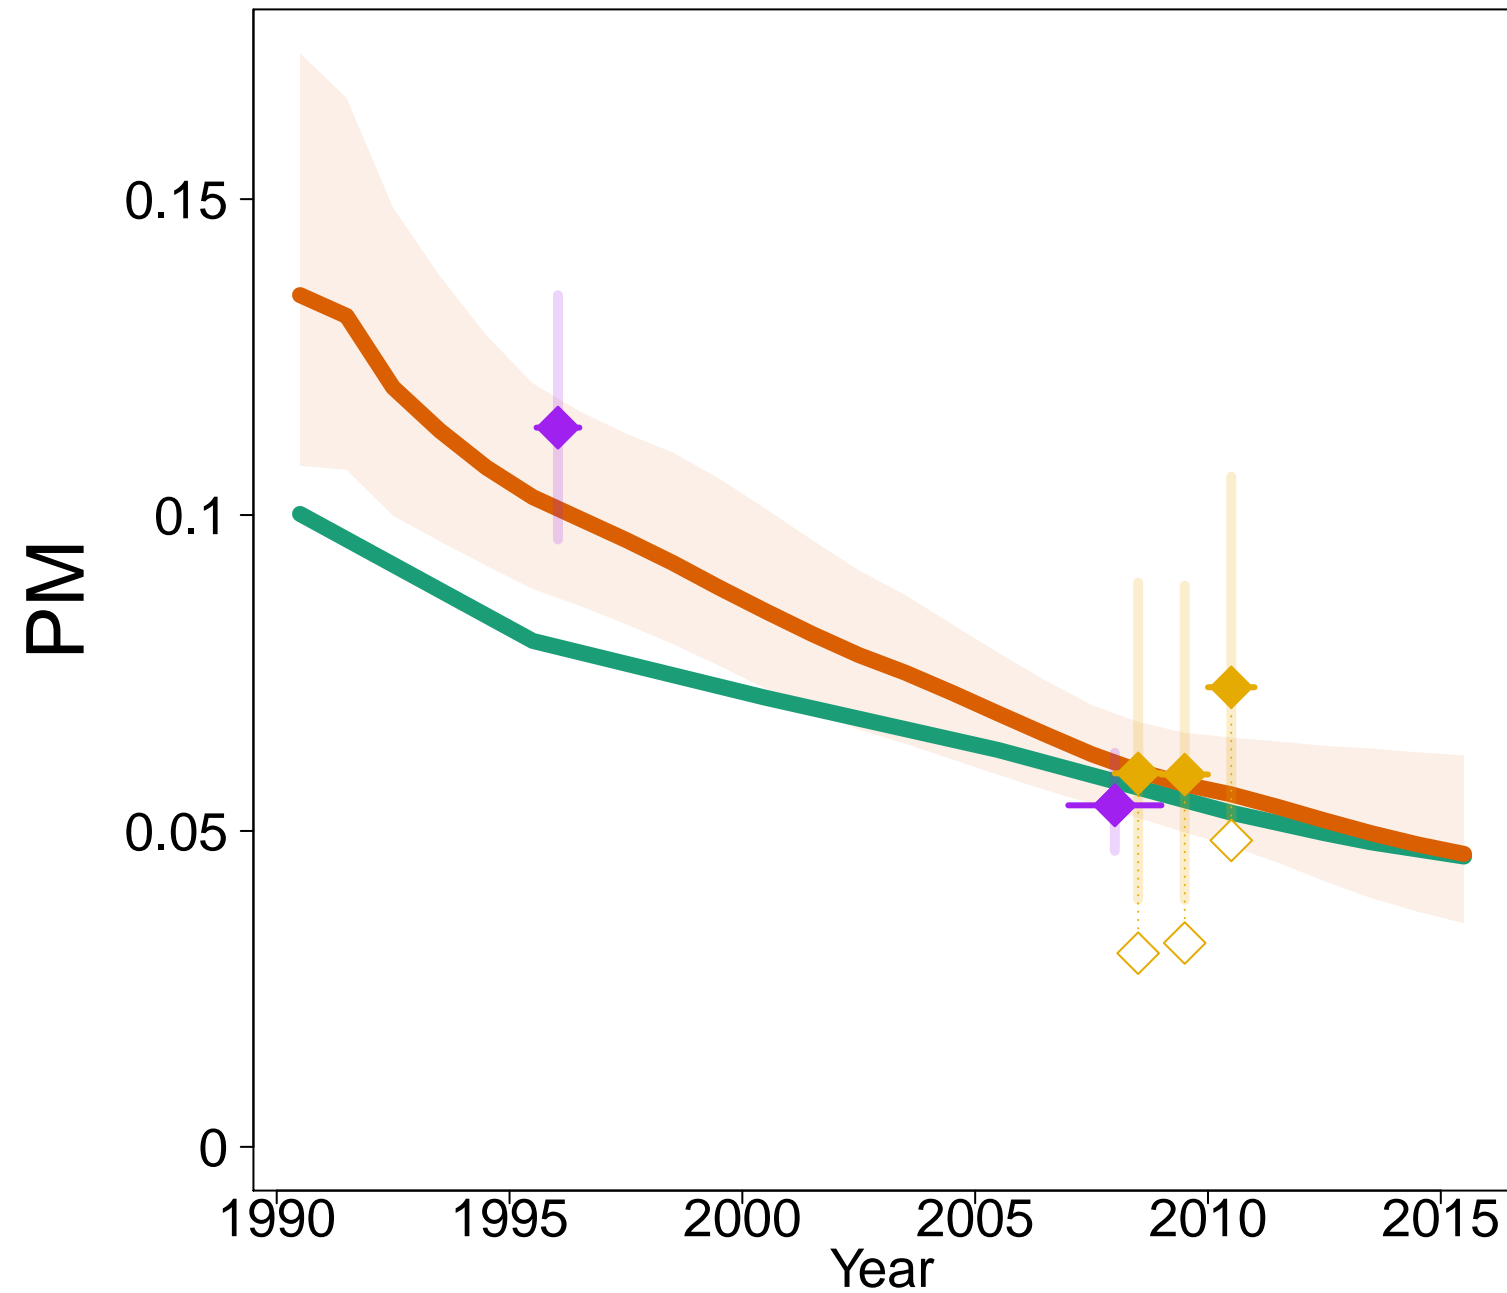

Jordan [JOR; B]  
(Western Asia)

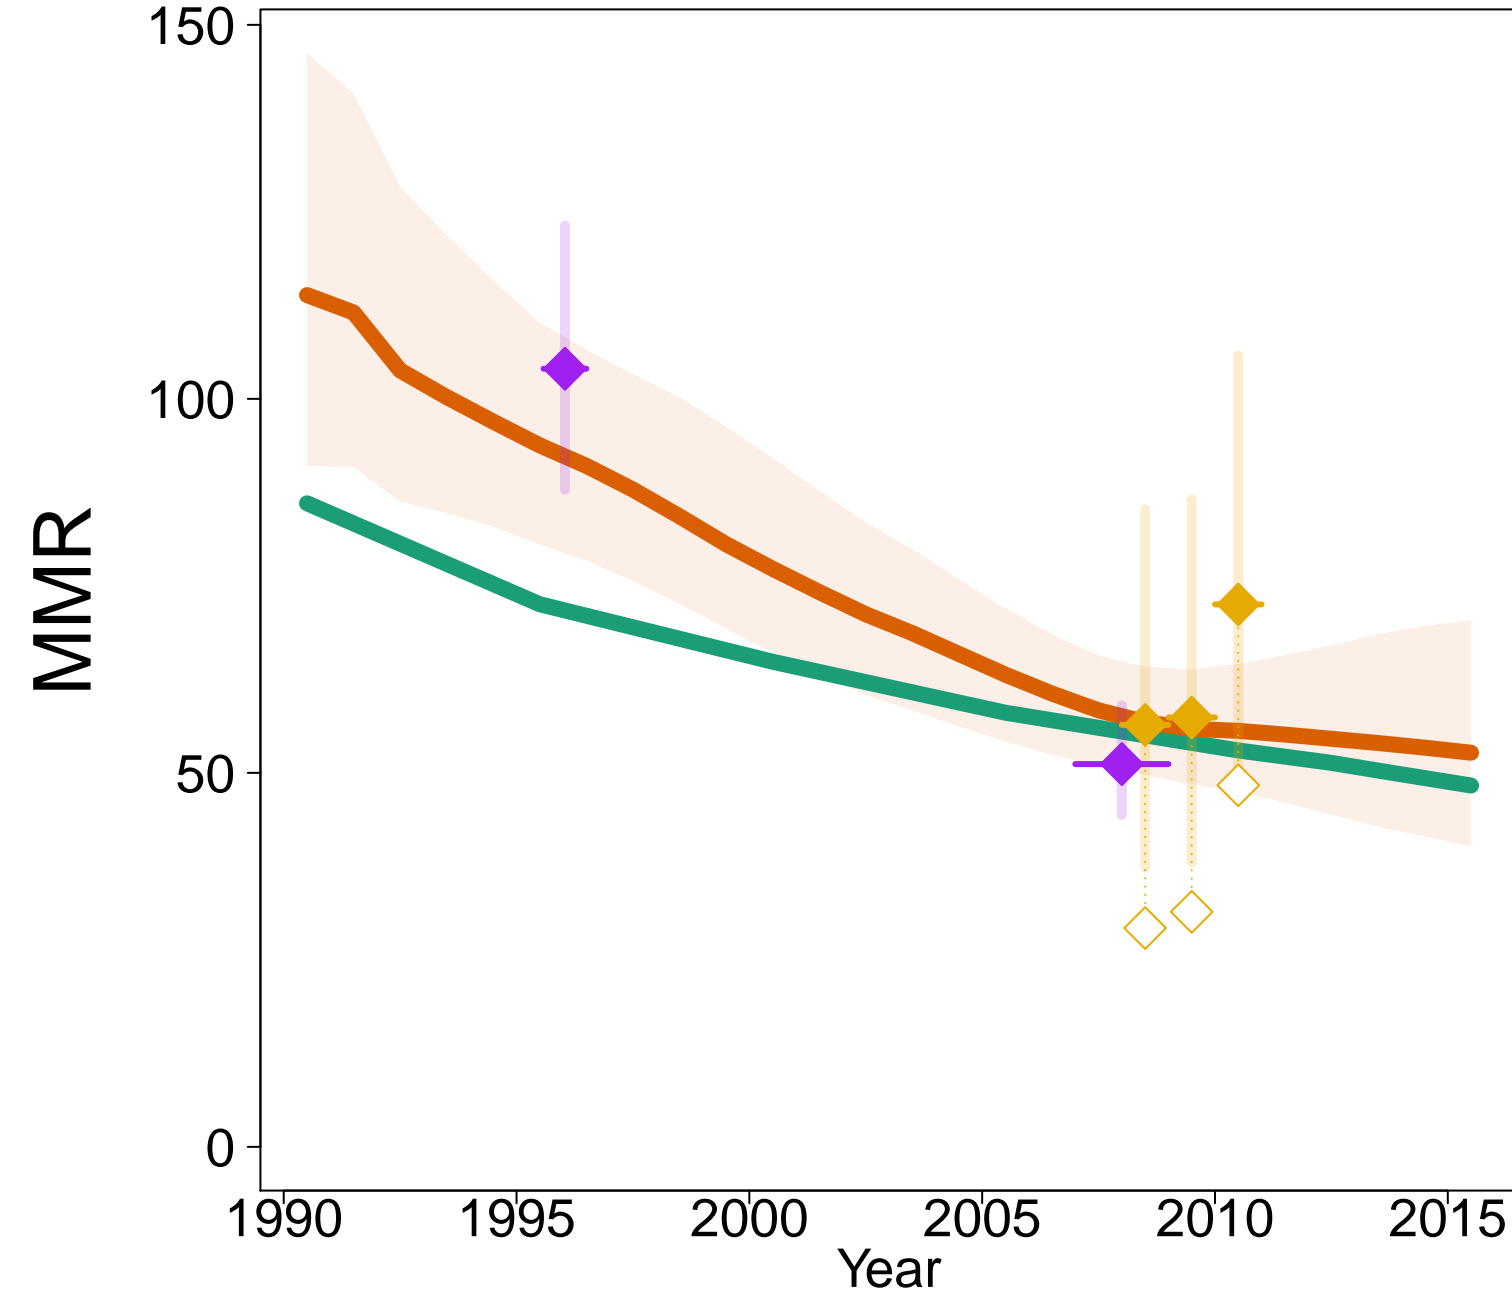

- Estimates –
- Bmat 2014
- MMEIG 2014
- Data –
- ◊ Observed Data
- ◼ Adjusted Data
- Data type –
- ◼ VR
- ◼ Spec. studies

Kazakhstan [KAZ; A]  
(Central Asia)

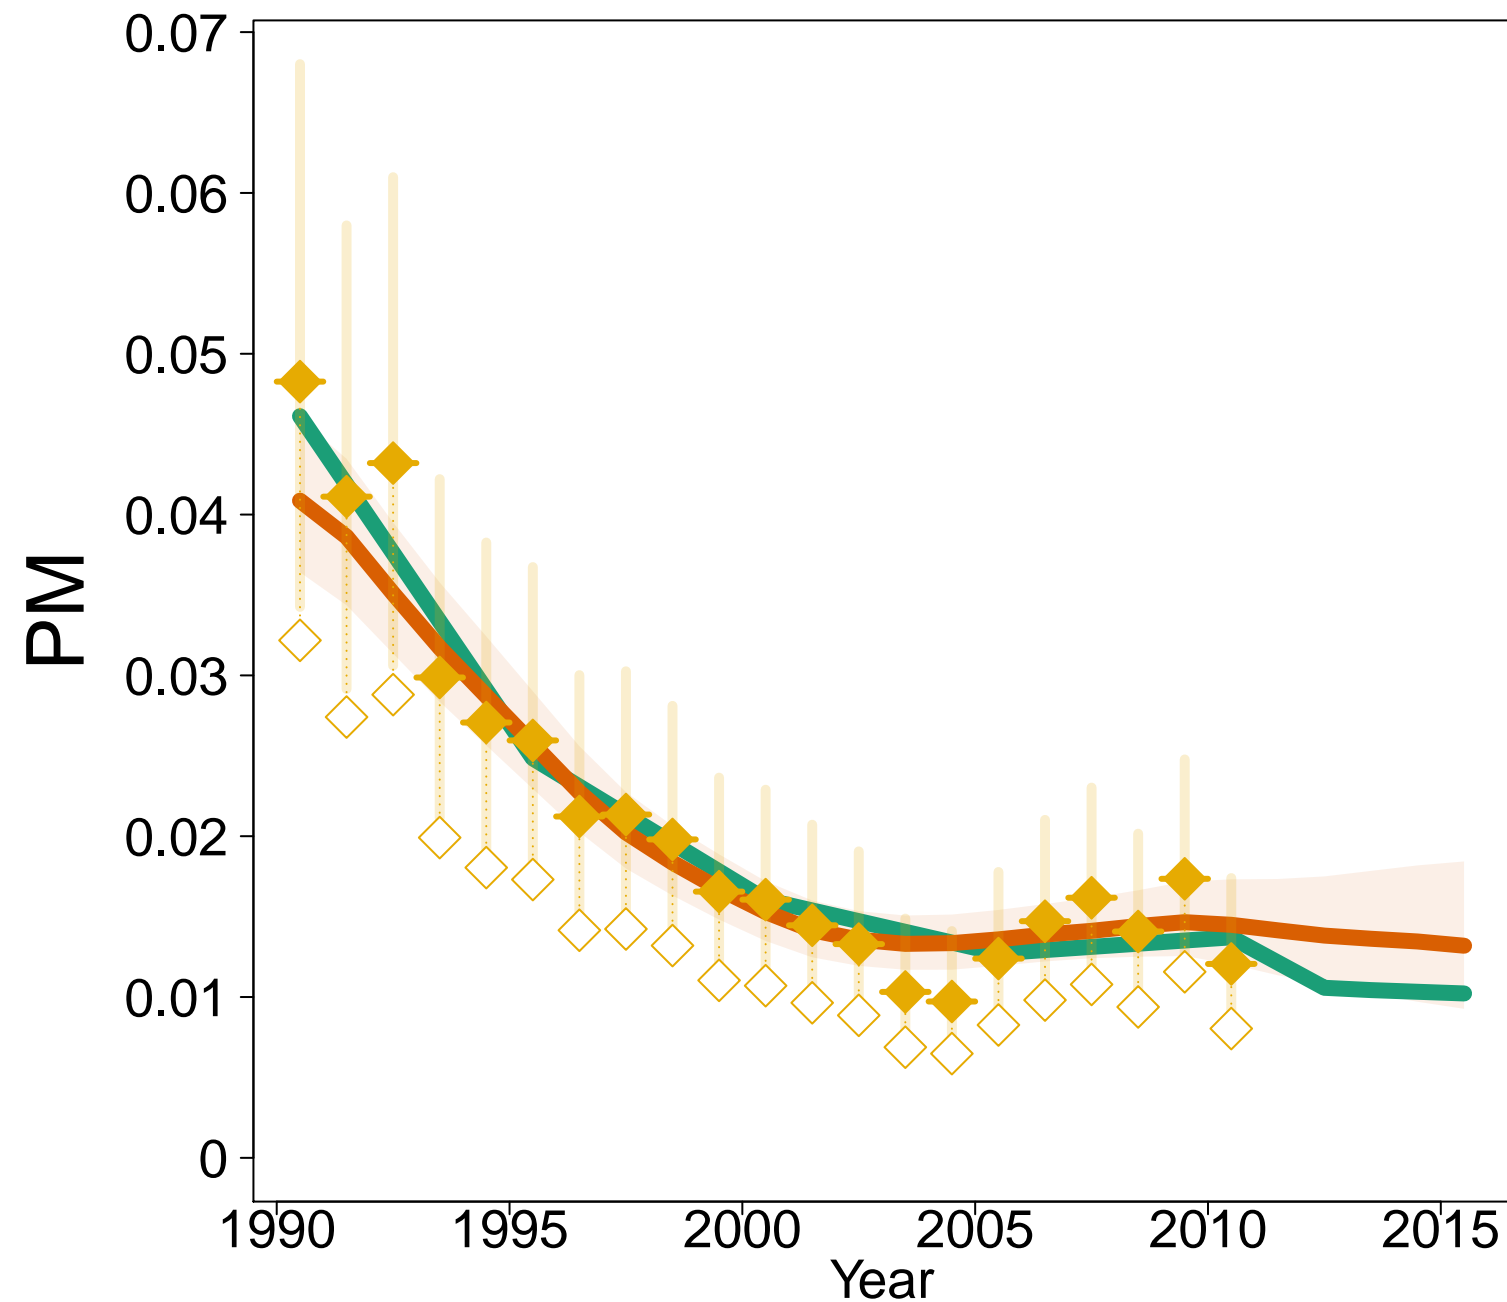

Kazakhstan [KAZ; A]  
(Central Asia)

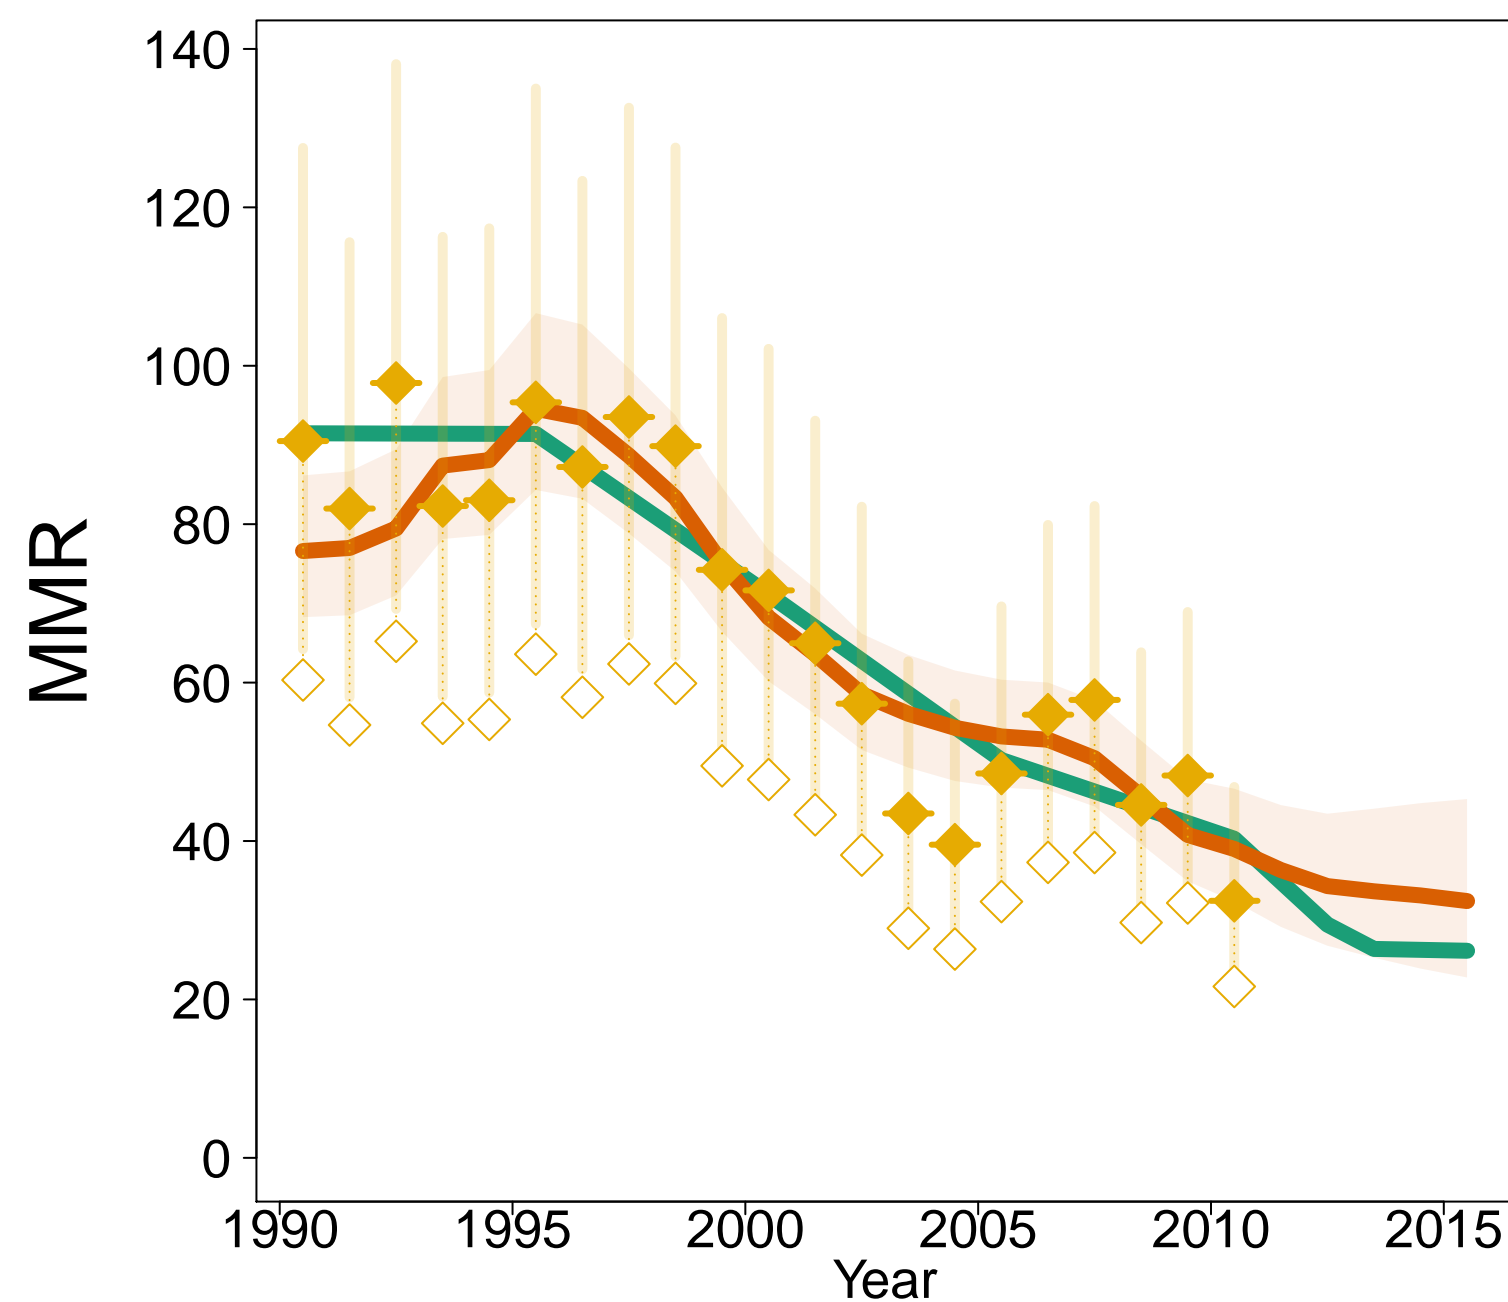

- Estimates –
- Bmat 2014
- MMEIG 2014
- Data –
- Observed Data
- Adjusted Data
- Data type –
- VR

Kenya [KEN; B]  
(Eastern Africa)

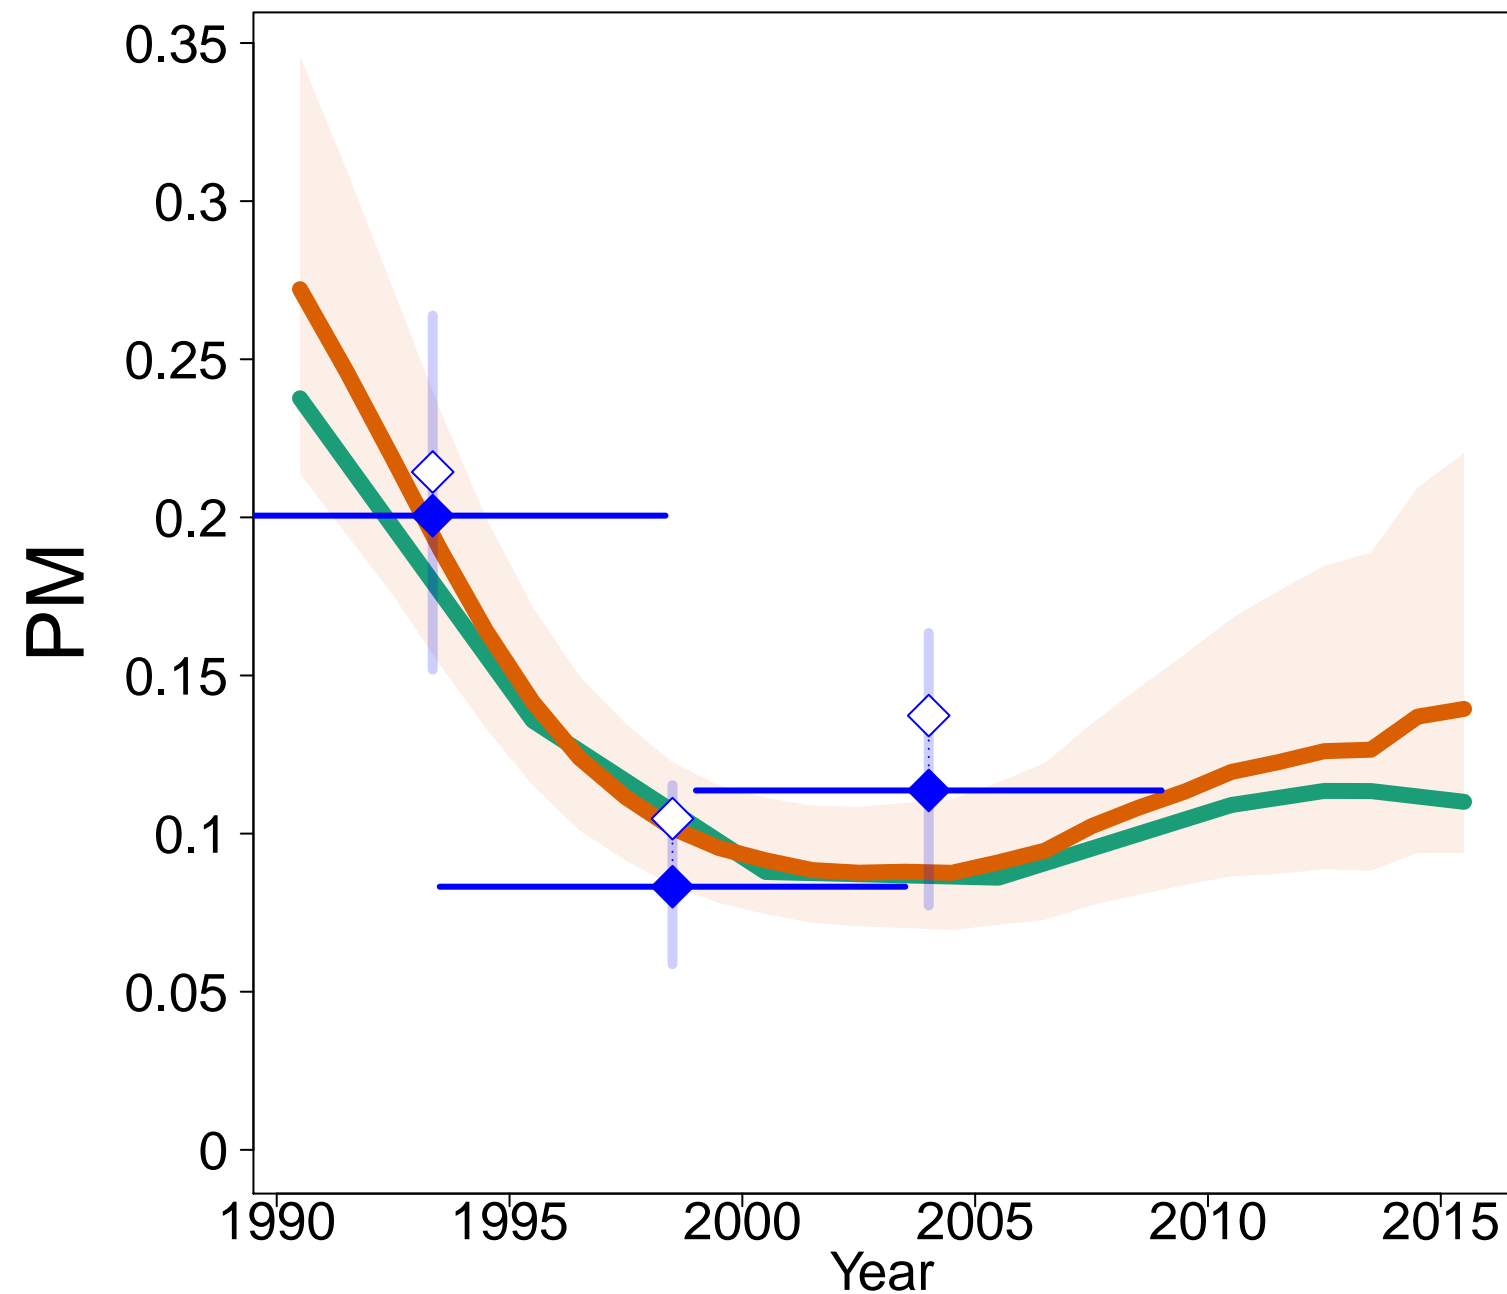

Kenya [KEN; B]  
(Eastern Africa)

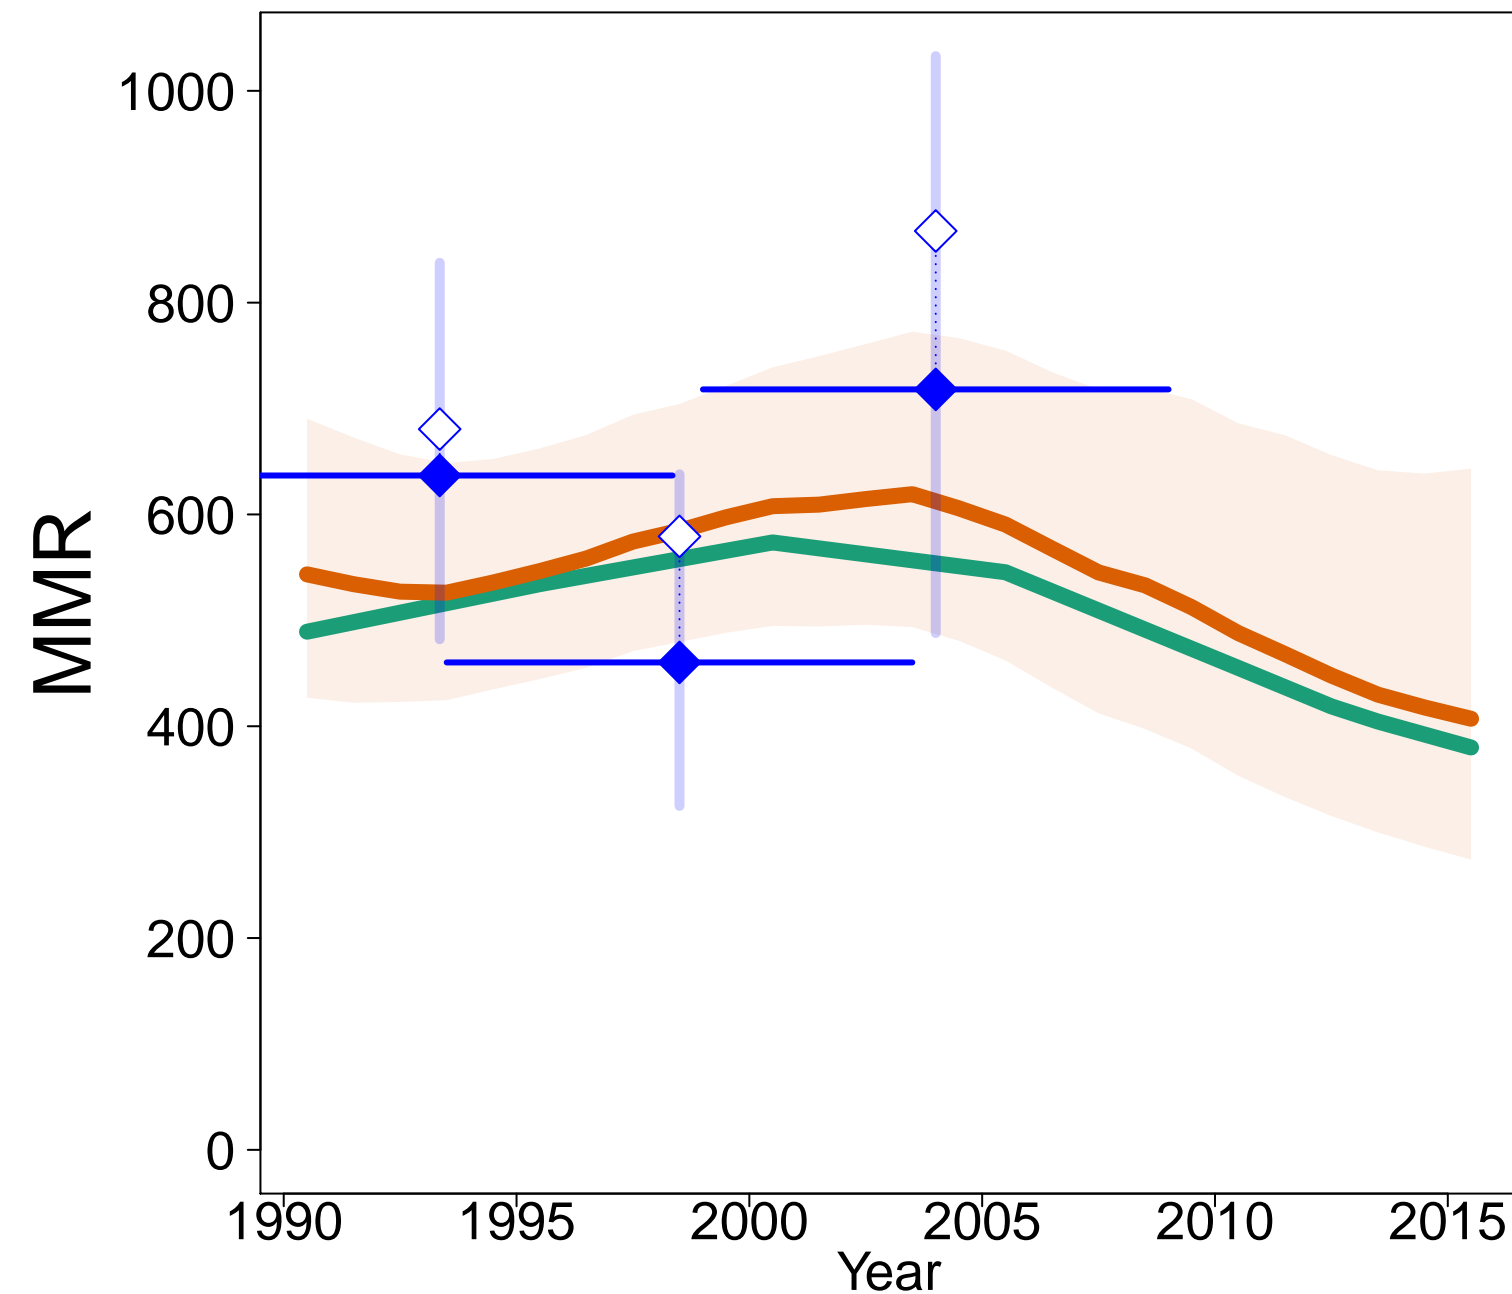

– Estimates –

Bmat 2014

MMEIG 2014

– Data –

Observed Data

Adjusted Data

– Data type –

DHS

Kiribati [KIR; C]  
(South-Eastern Asia / Oceania)

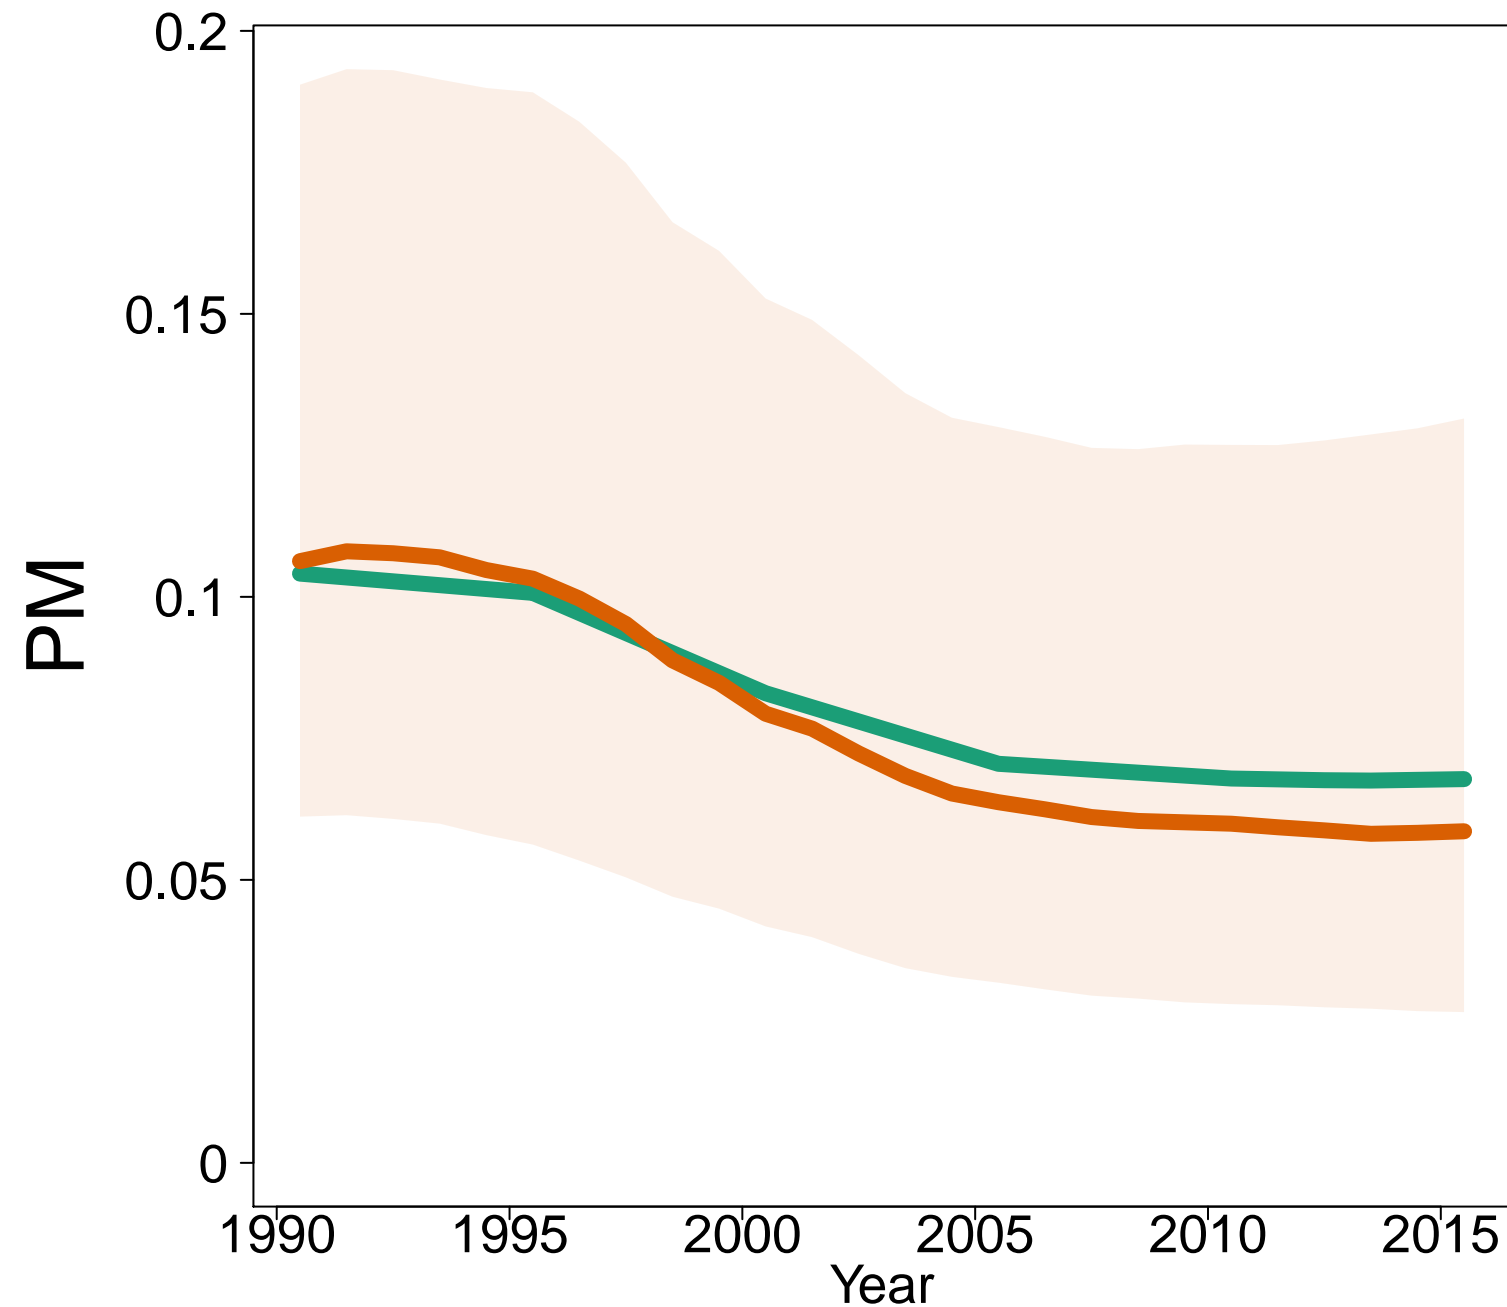

Kiribati [KIR; C]  
(South-Eastern Asia / Oceania)

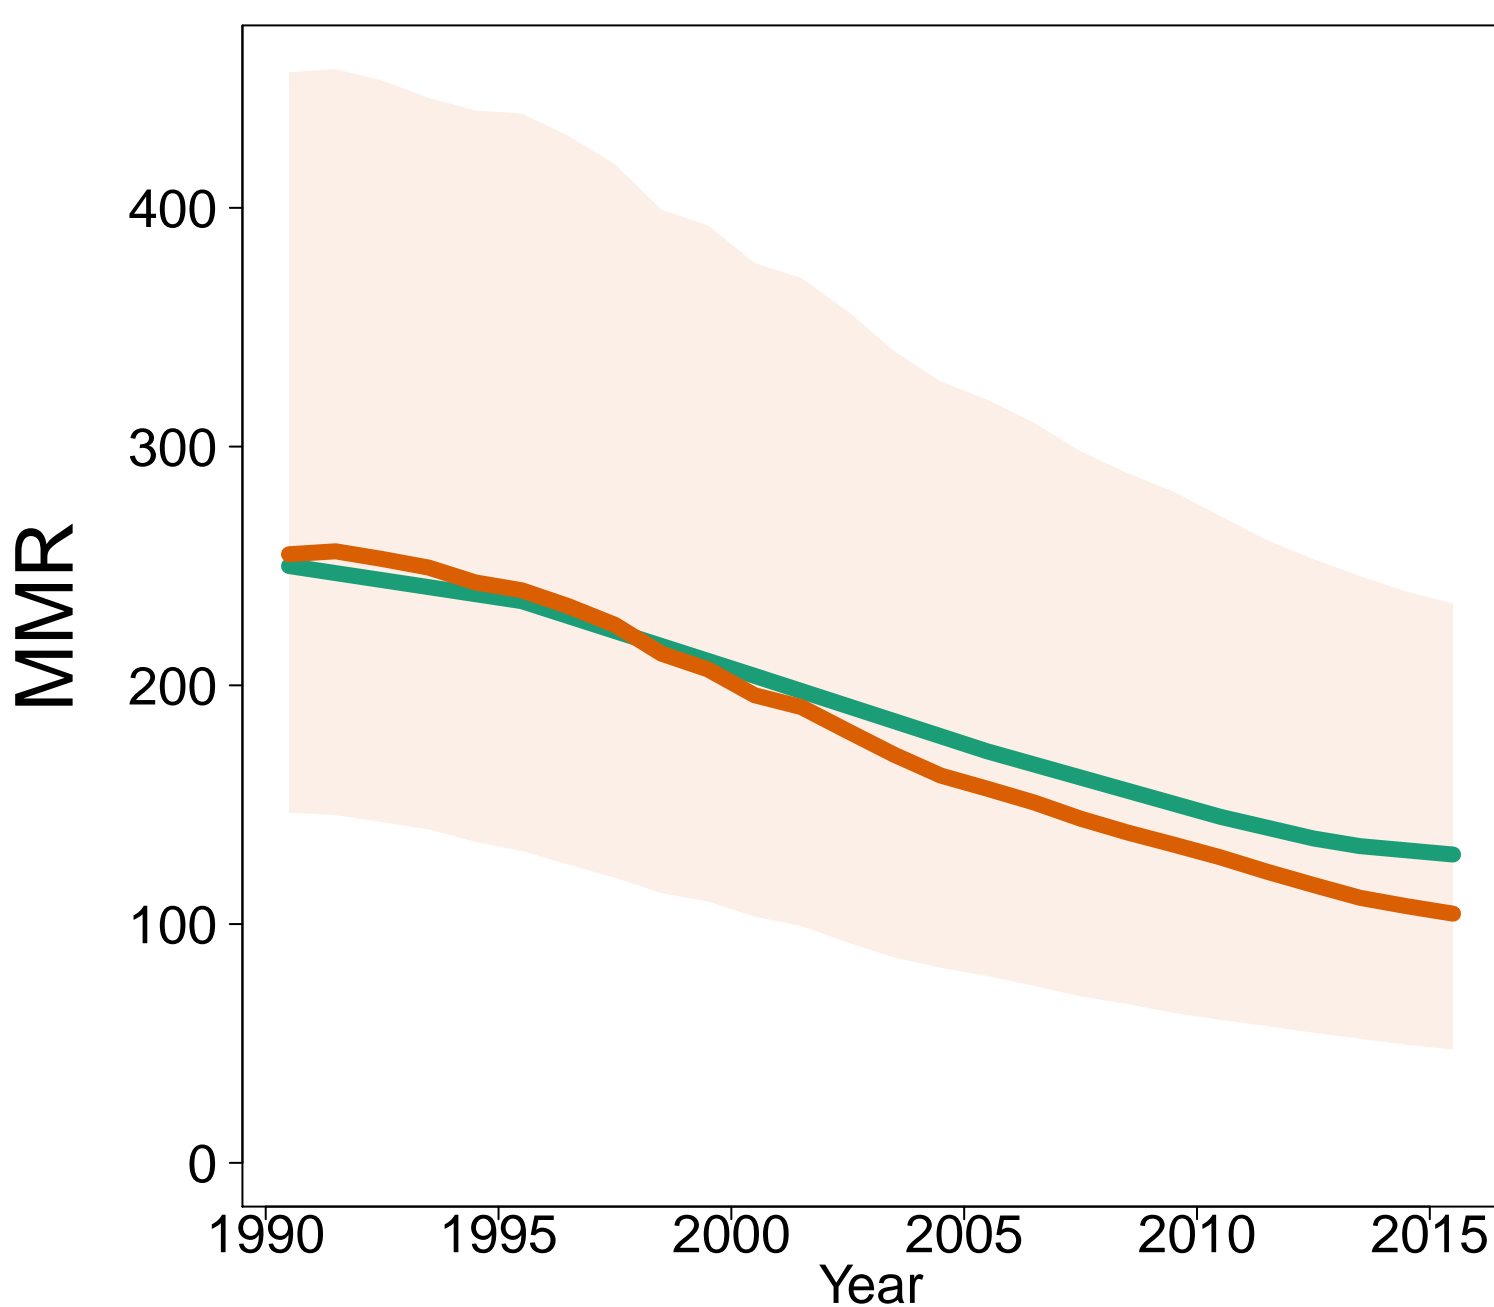

- Estimates –
- Bmat 2014
- MMEIG 2014
- Data –
- ◊ Observed Data
- ◆ Adjusted Data
- Data type –

Kuwait [KWT; A]  
(Western Asia)

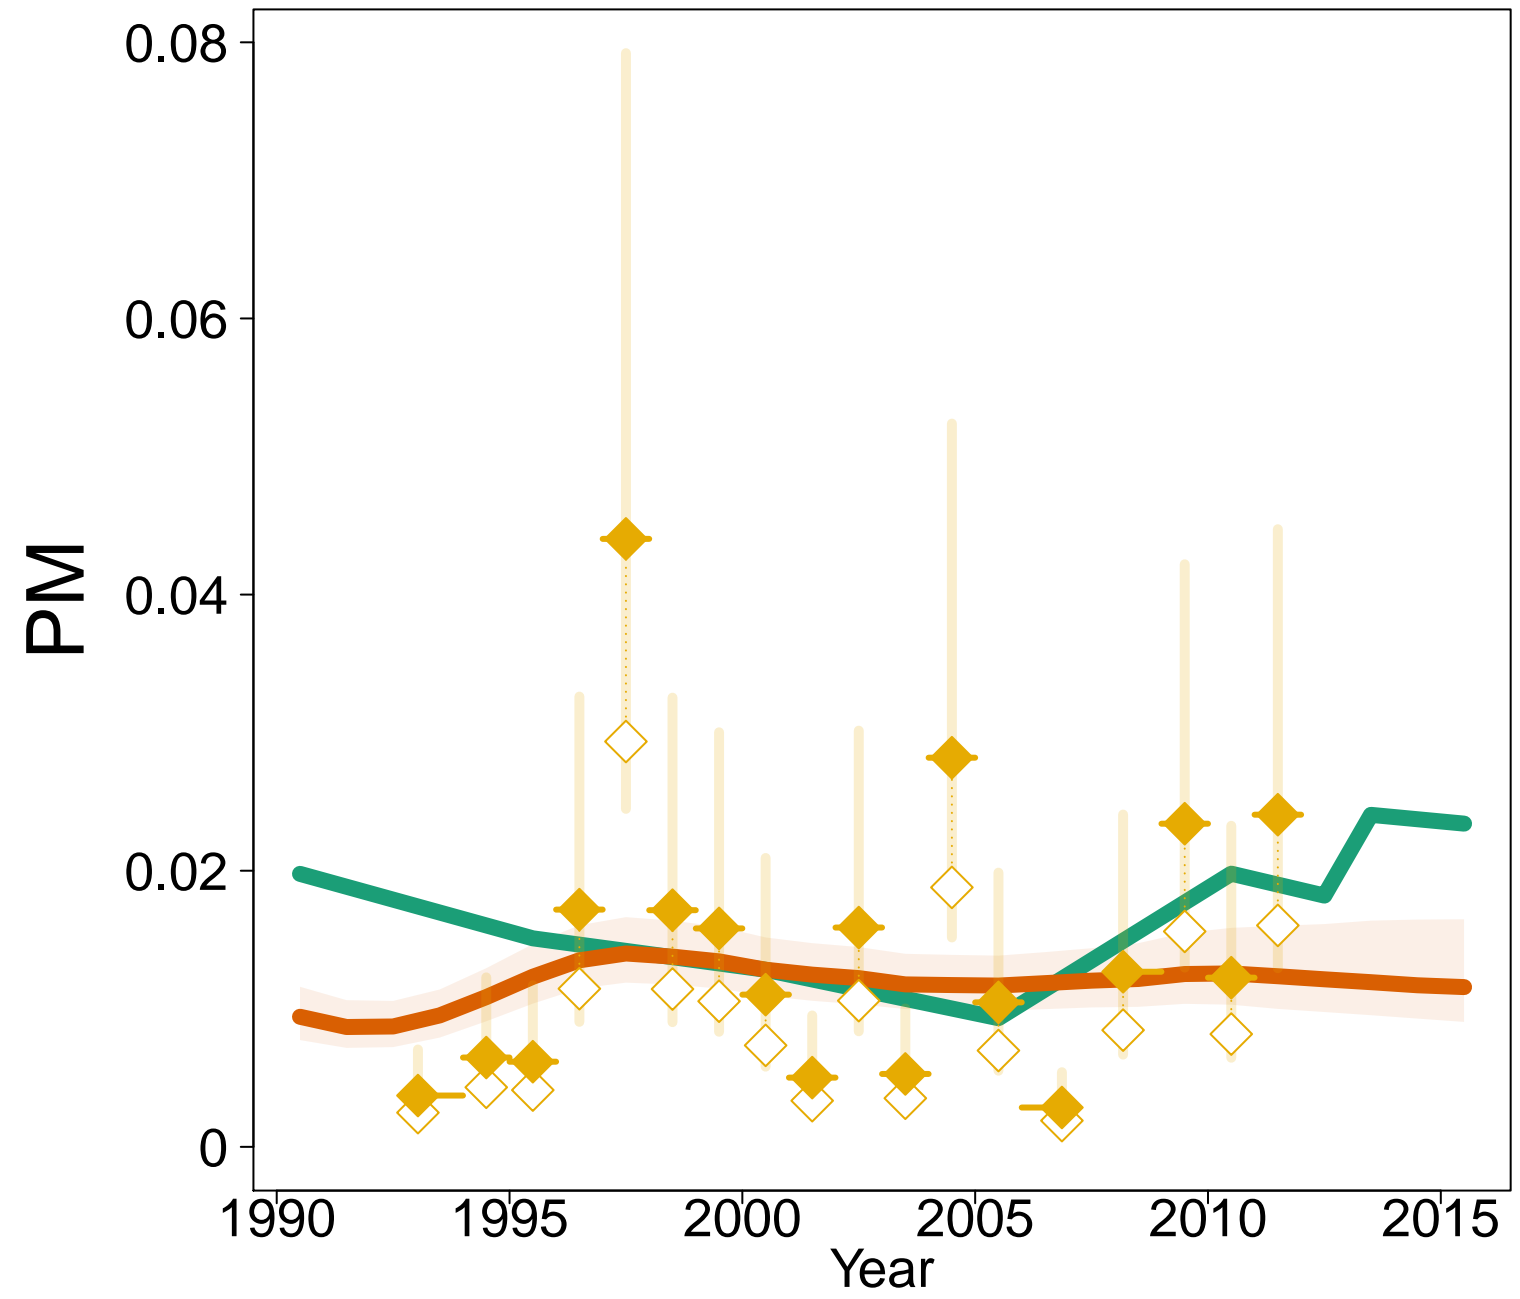

Kuwait [KWT; A]  
(Western Asia)

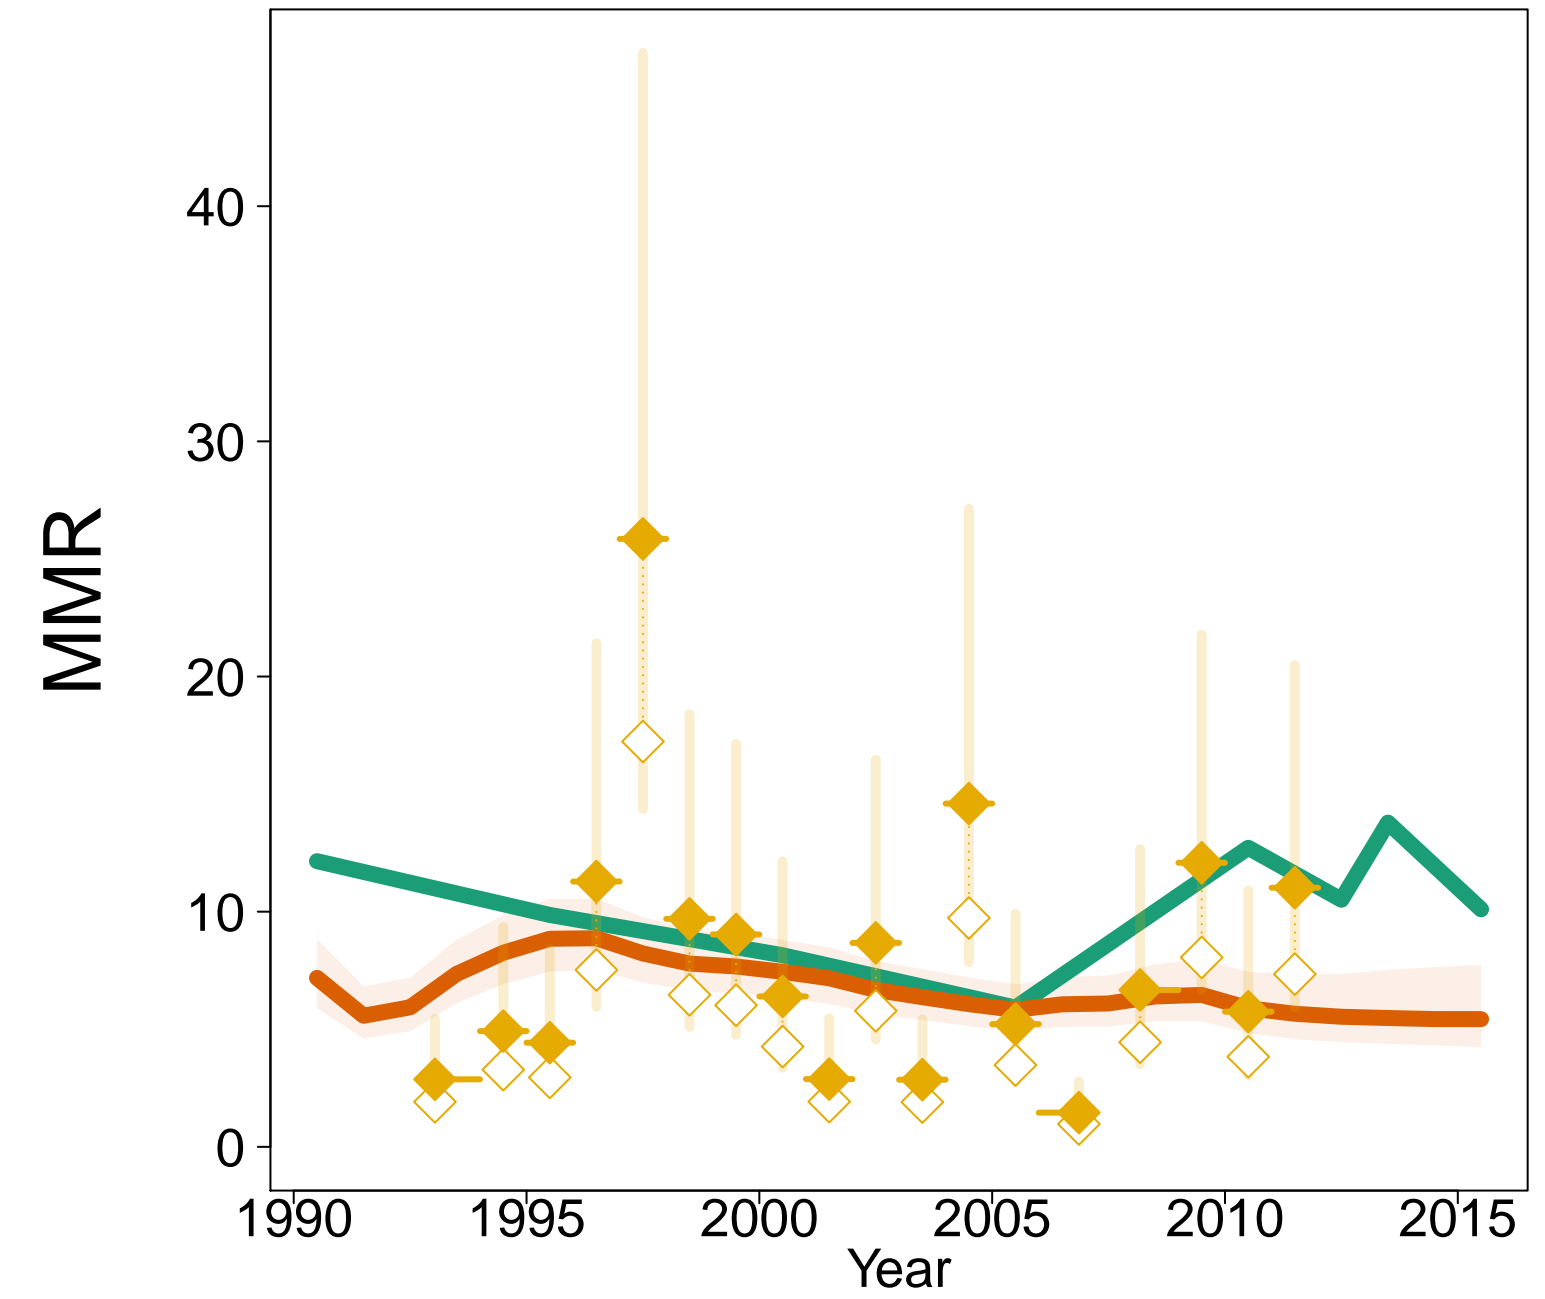

- Estimates –
- Bmat 2014
- MMEIG 2014
- Data –
- Observed Data
- Adjusted Data
- Data type –
- VR

Kyrgyzstan [KGZ; B]  
(Central Asia)

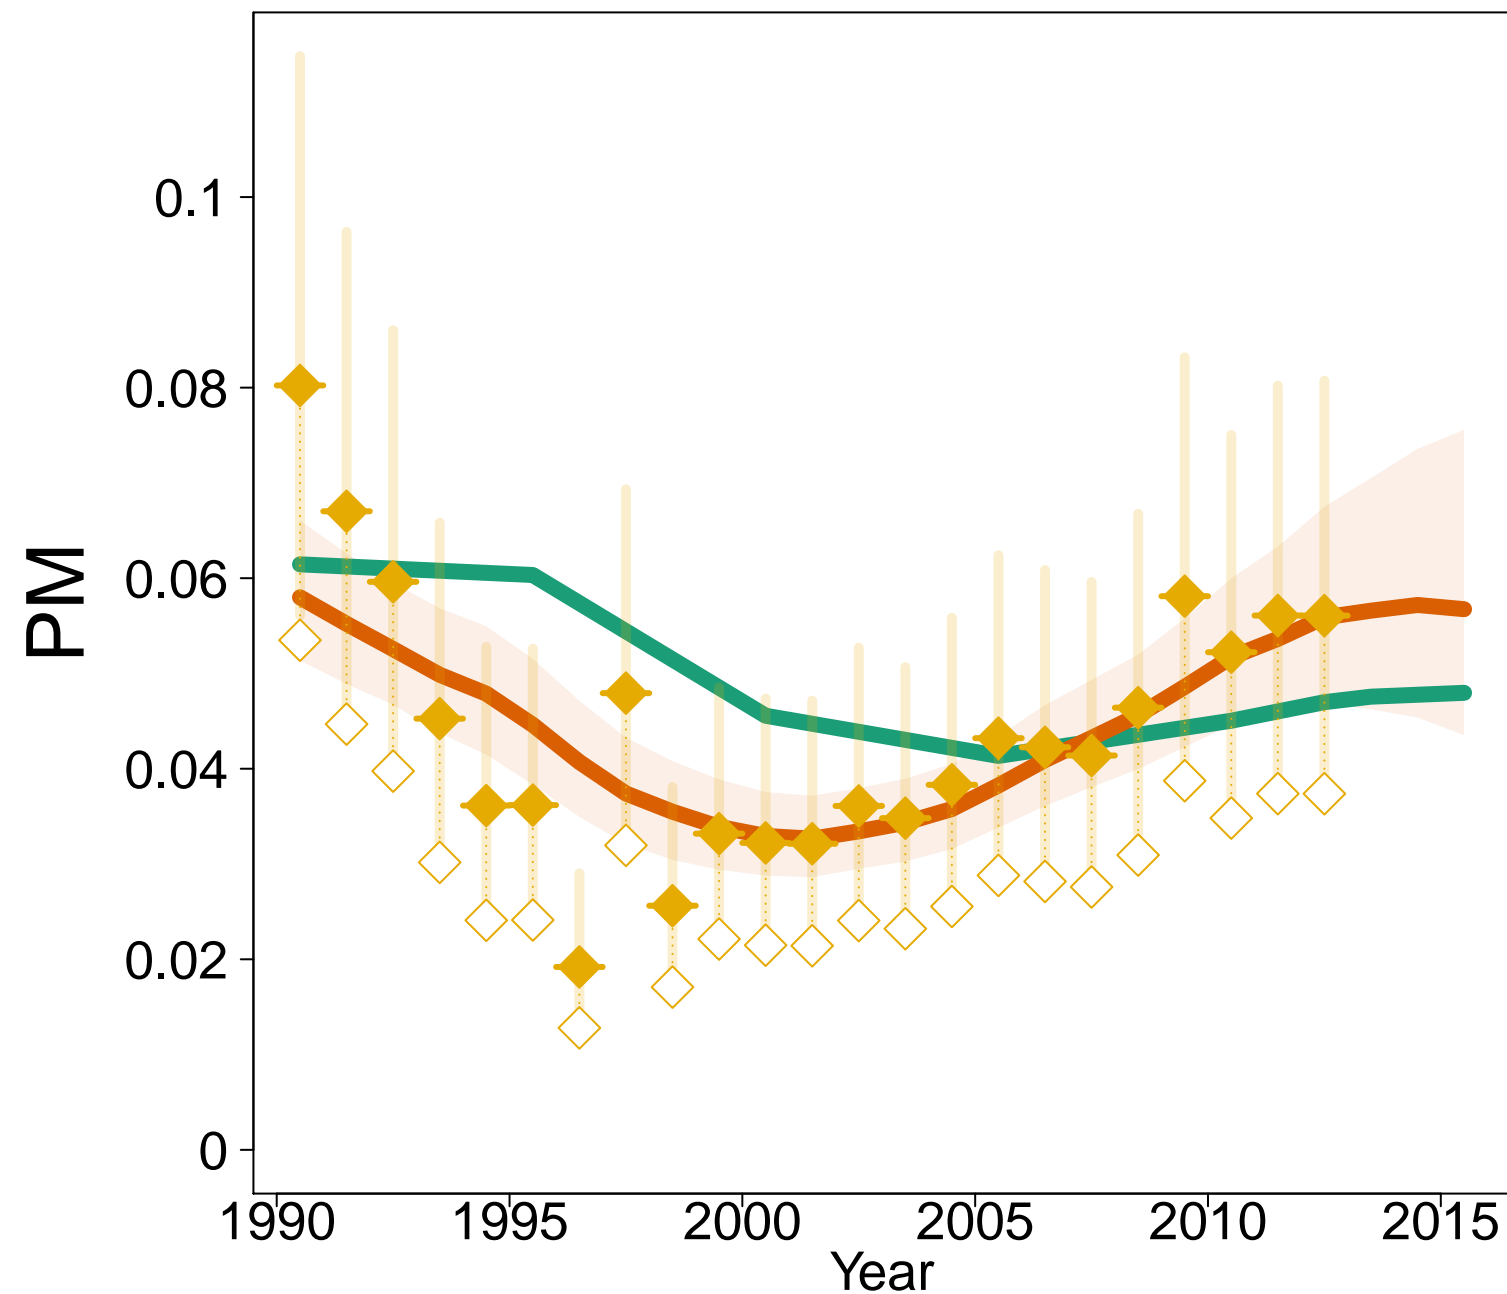

Kyrgyzstan [KGZ; B]  
(Central Asia)

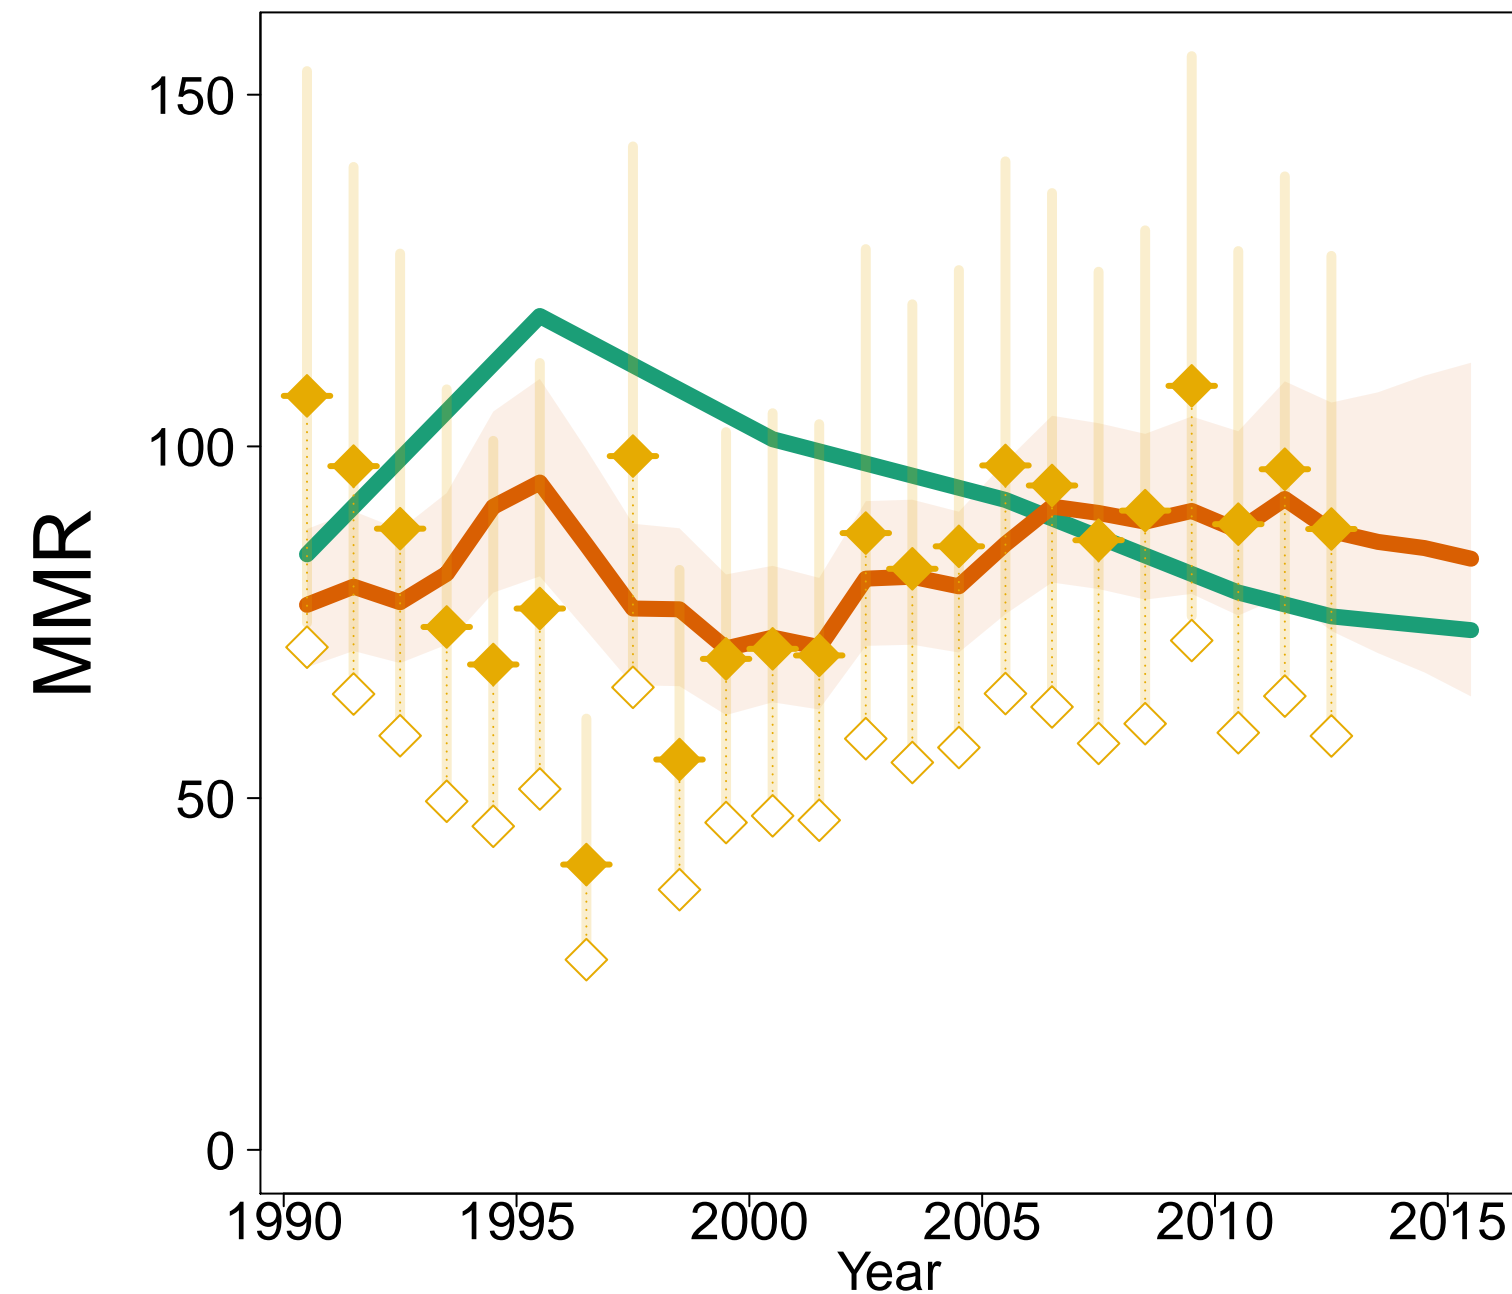

- Estimates –
- Bmat 2014
- MMEIG 2014
- Data –
- Observed Data
- Adjusted Data
- Data type –
- VR



Lao [LAO; B]  
(South-Eastern Asia / Oceania)

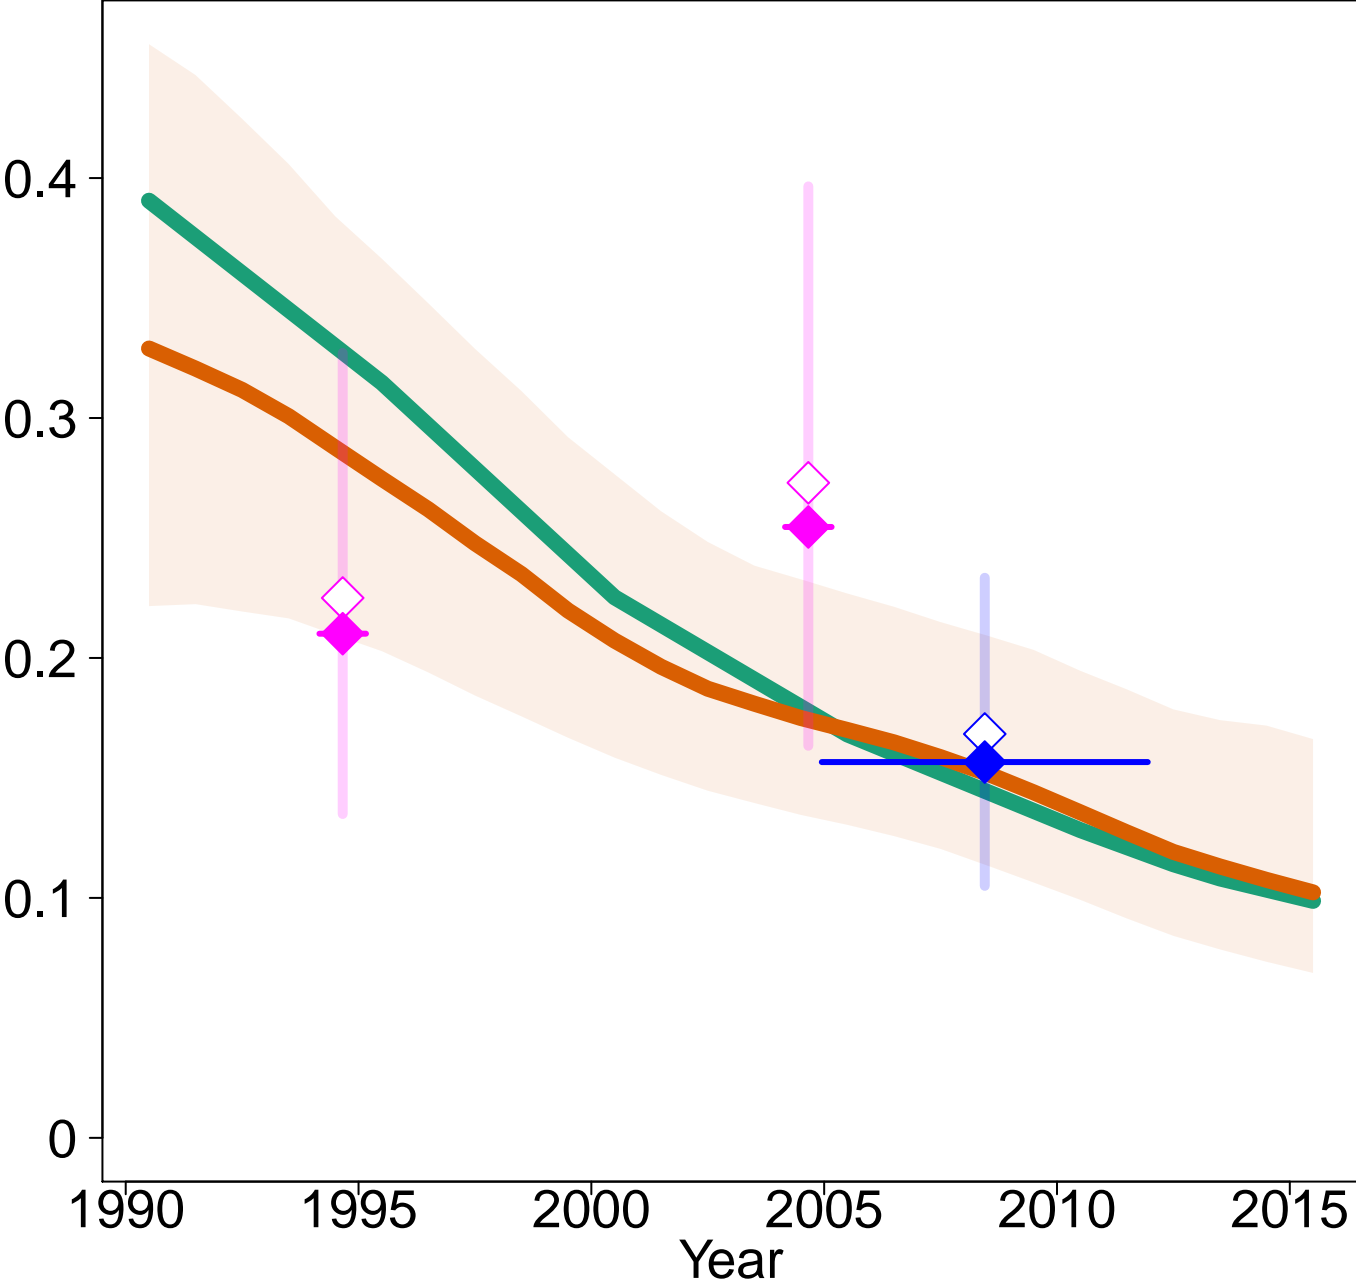

Lao [LAO; B]  
(South-Eastern Asia / Oceania)

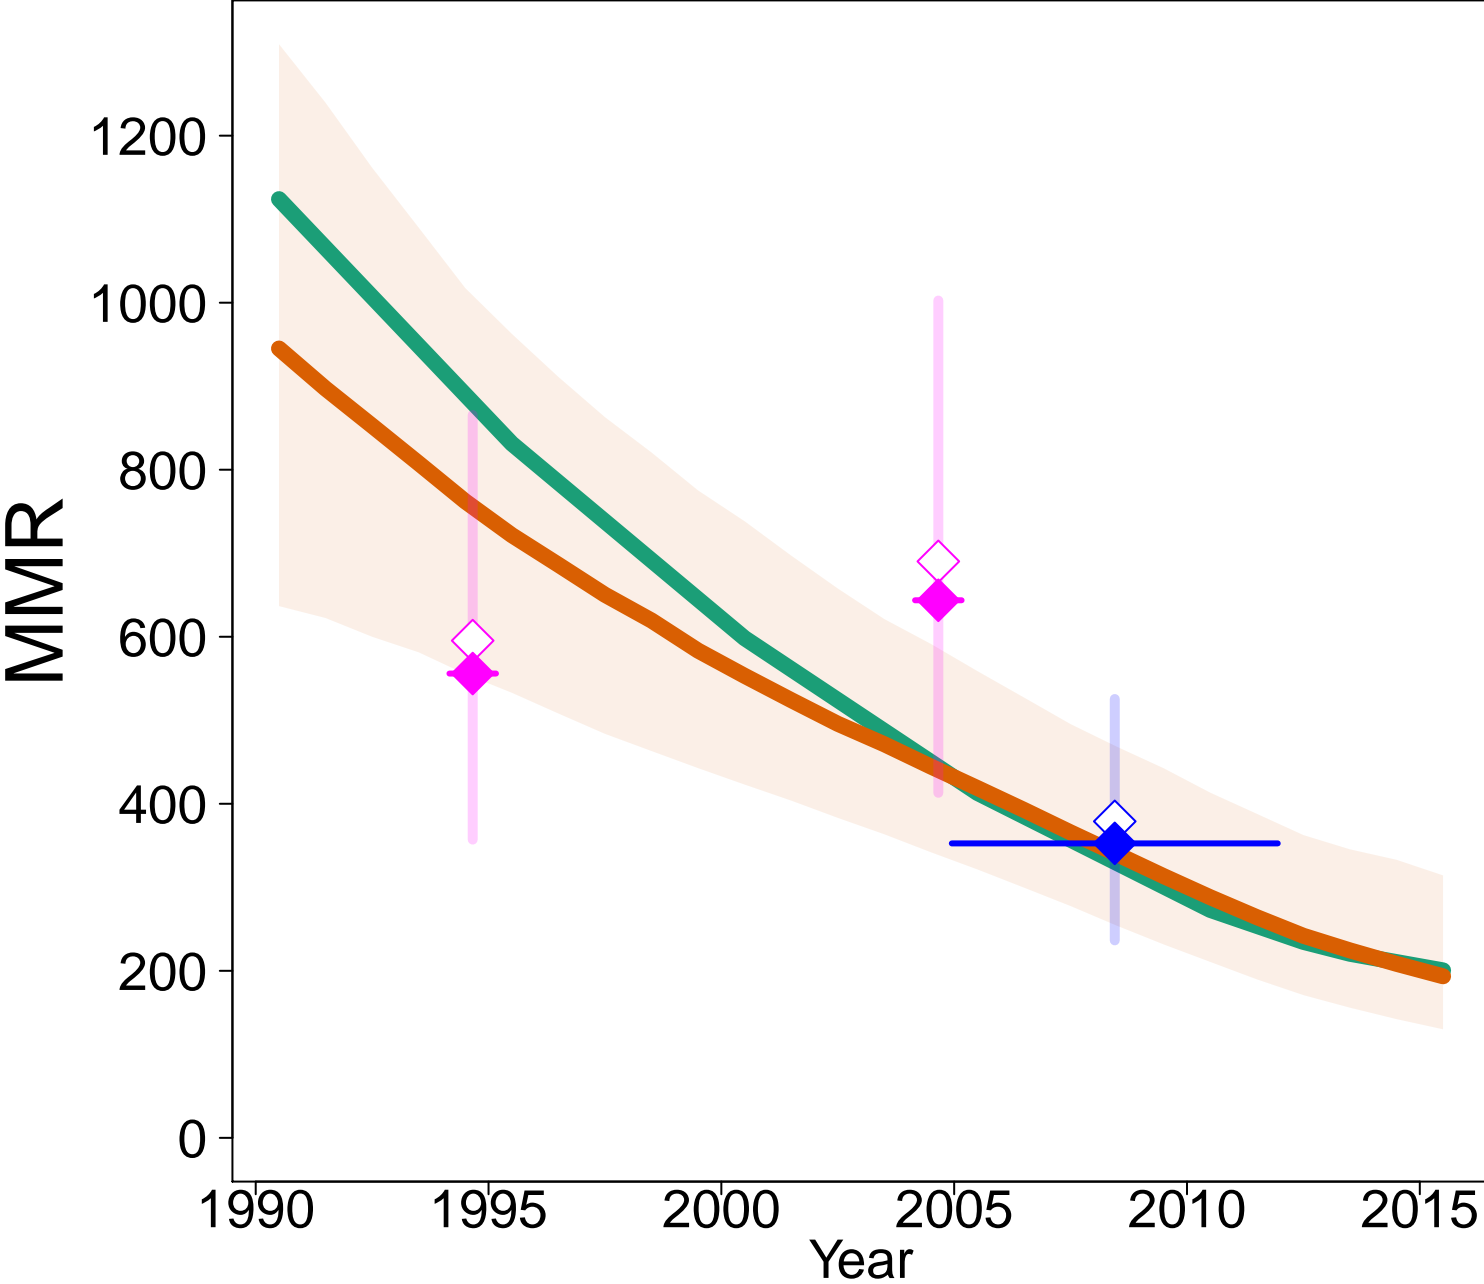

- Estimates –
- Bmat 2014
- MMEIG 2014
- Data –
- Observed Data
- Adjusted Data
- Data type –
- DHS
- Census

Latvia [LVA; A]  
(Developed regions)

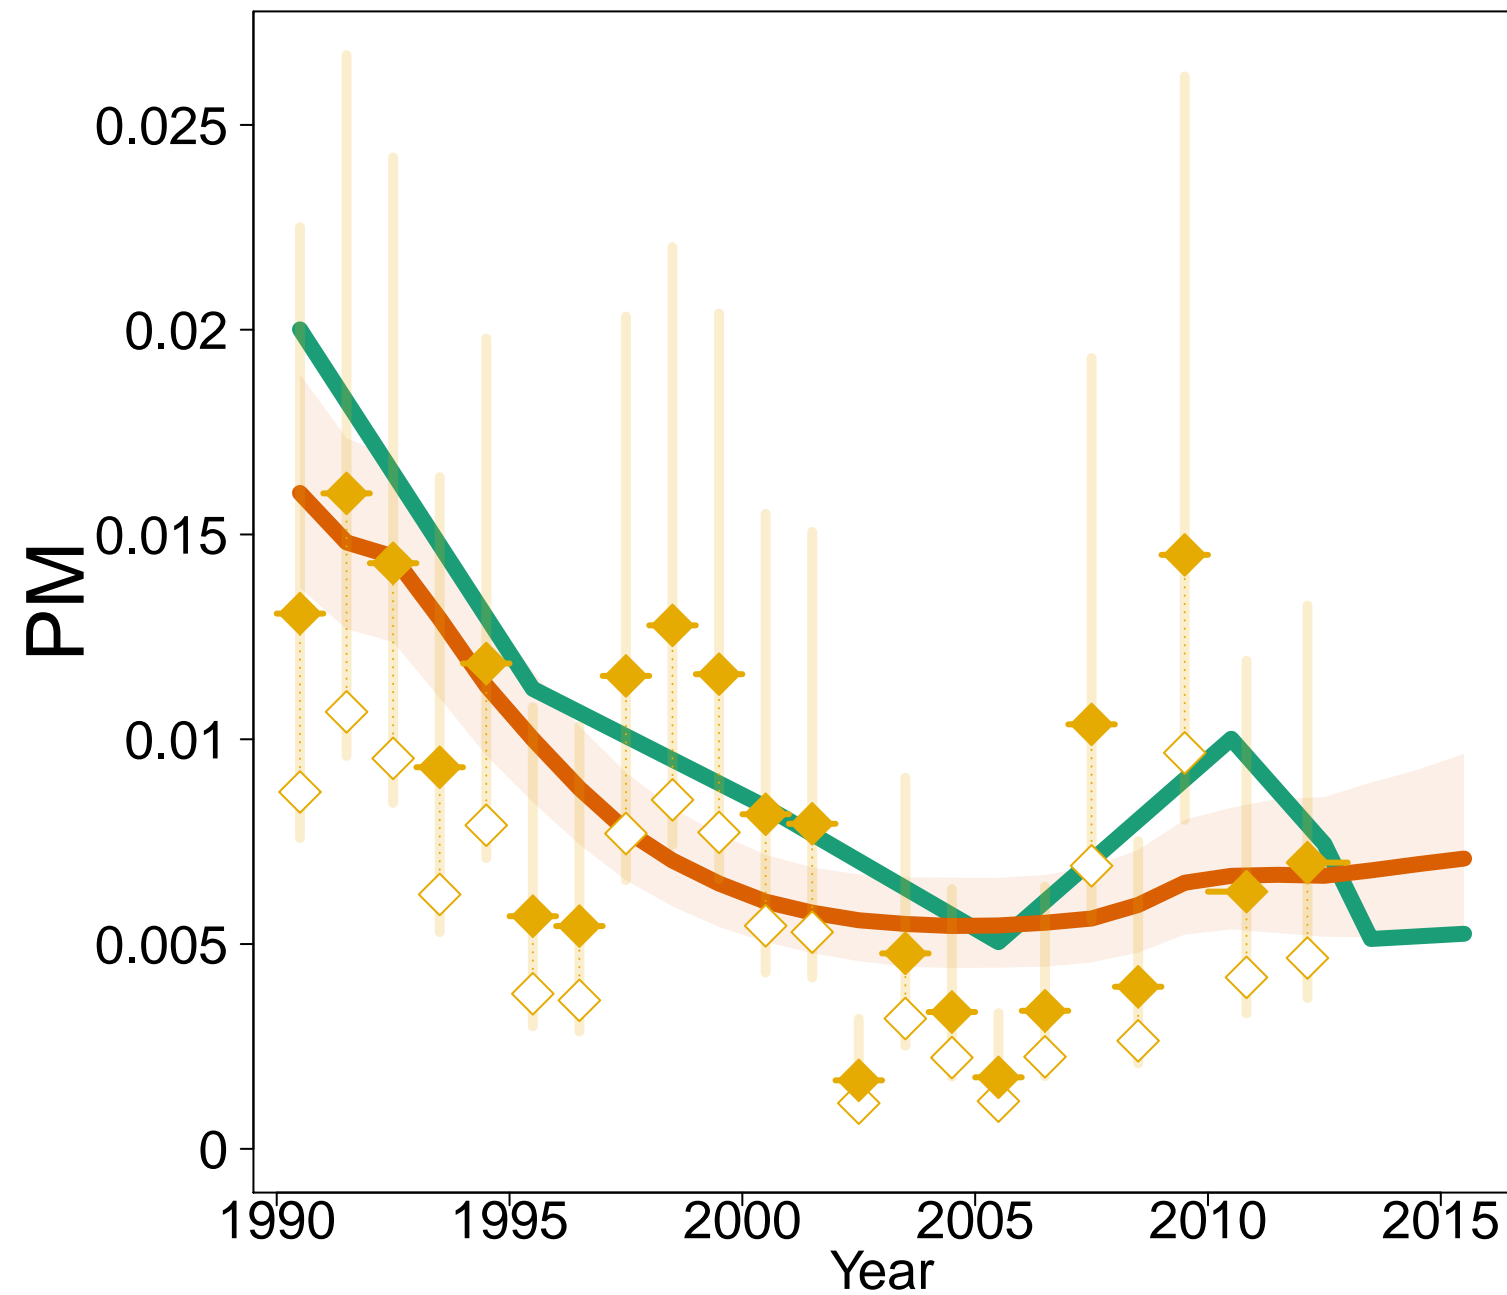

Latvia [LVA; A]  
(Developed regions)

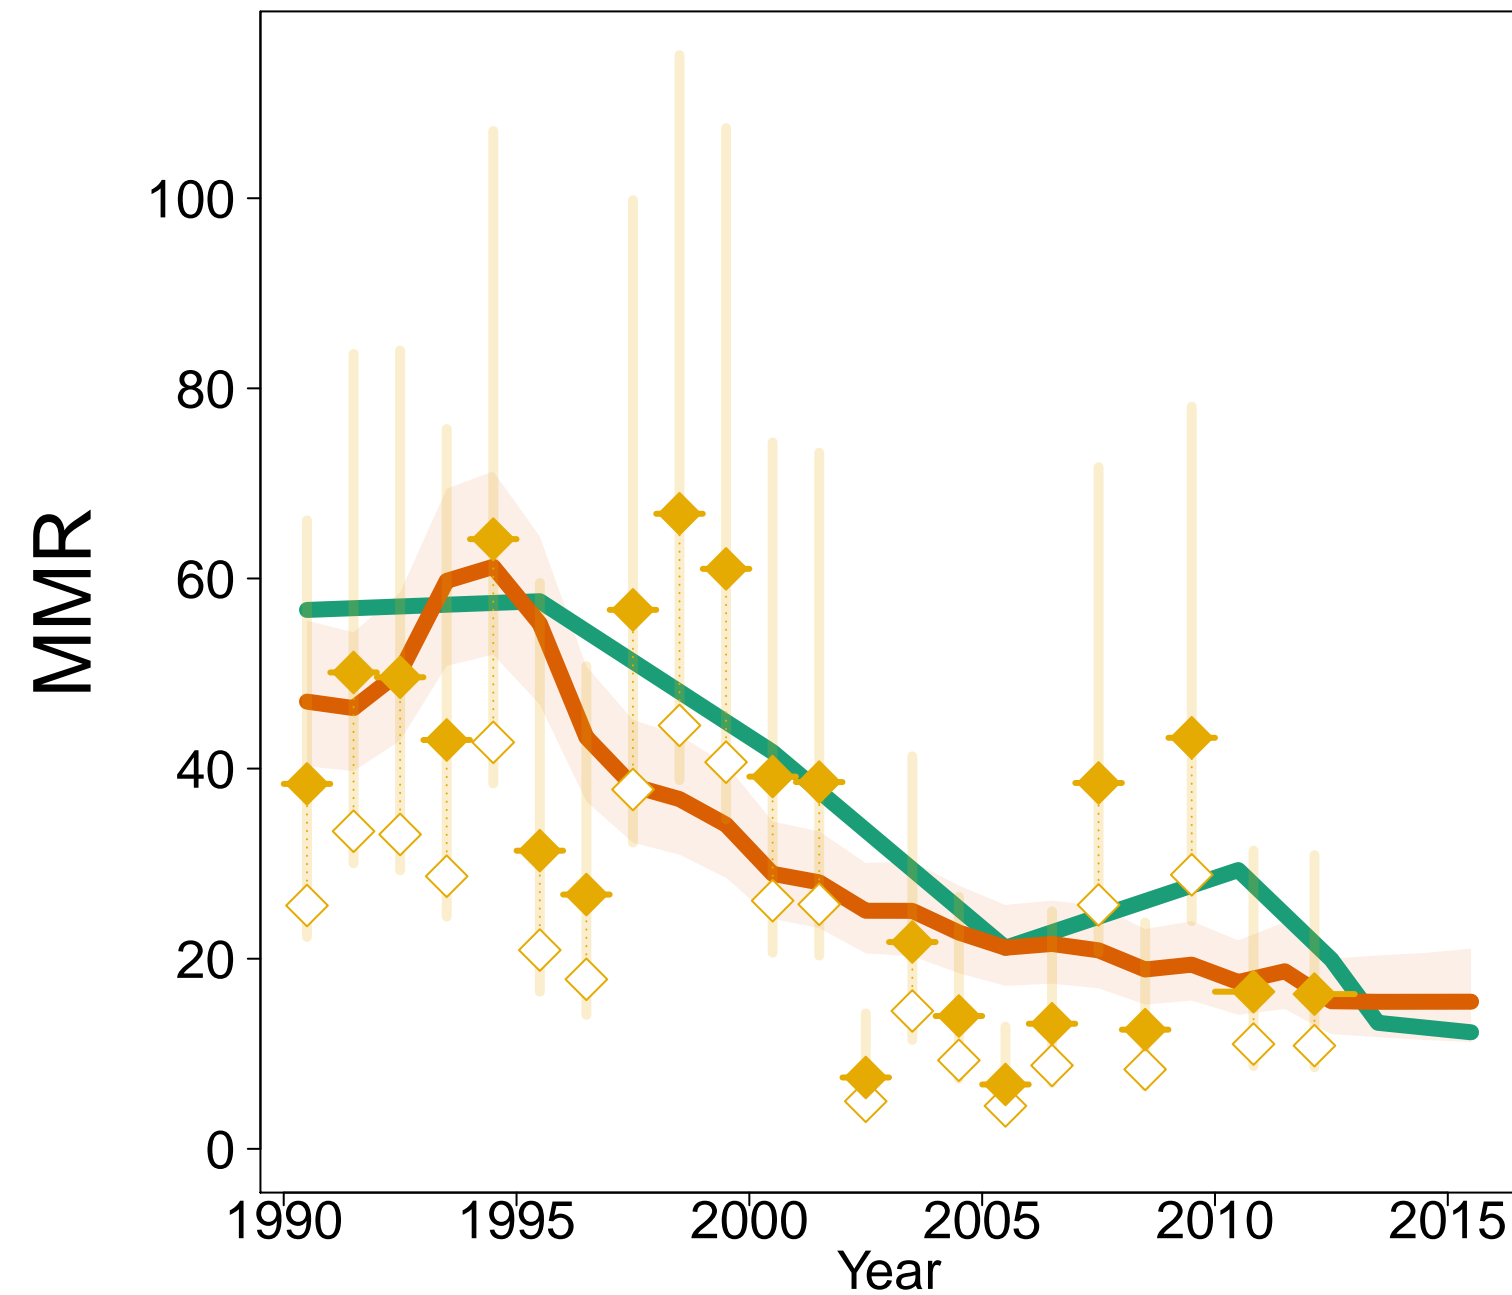

- Estimates –
- Bmat 2014
- MMEIG 2014
- Data –
- Observed Data
- Adjusted Data
- Data type –
- VR

Lebanon [LBN; B]  
(Western Asia)

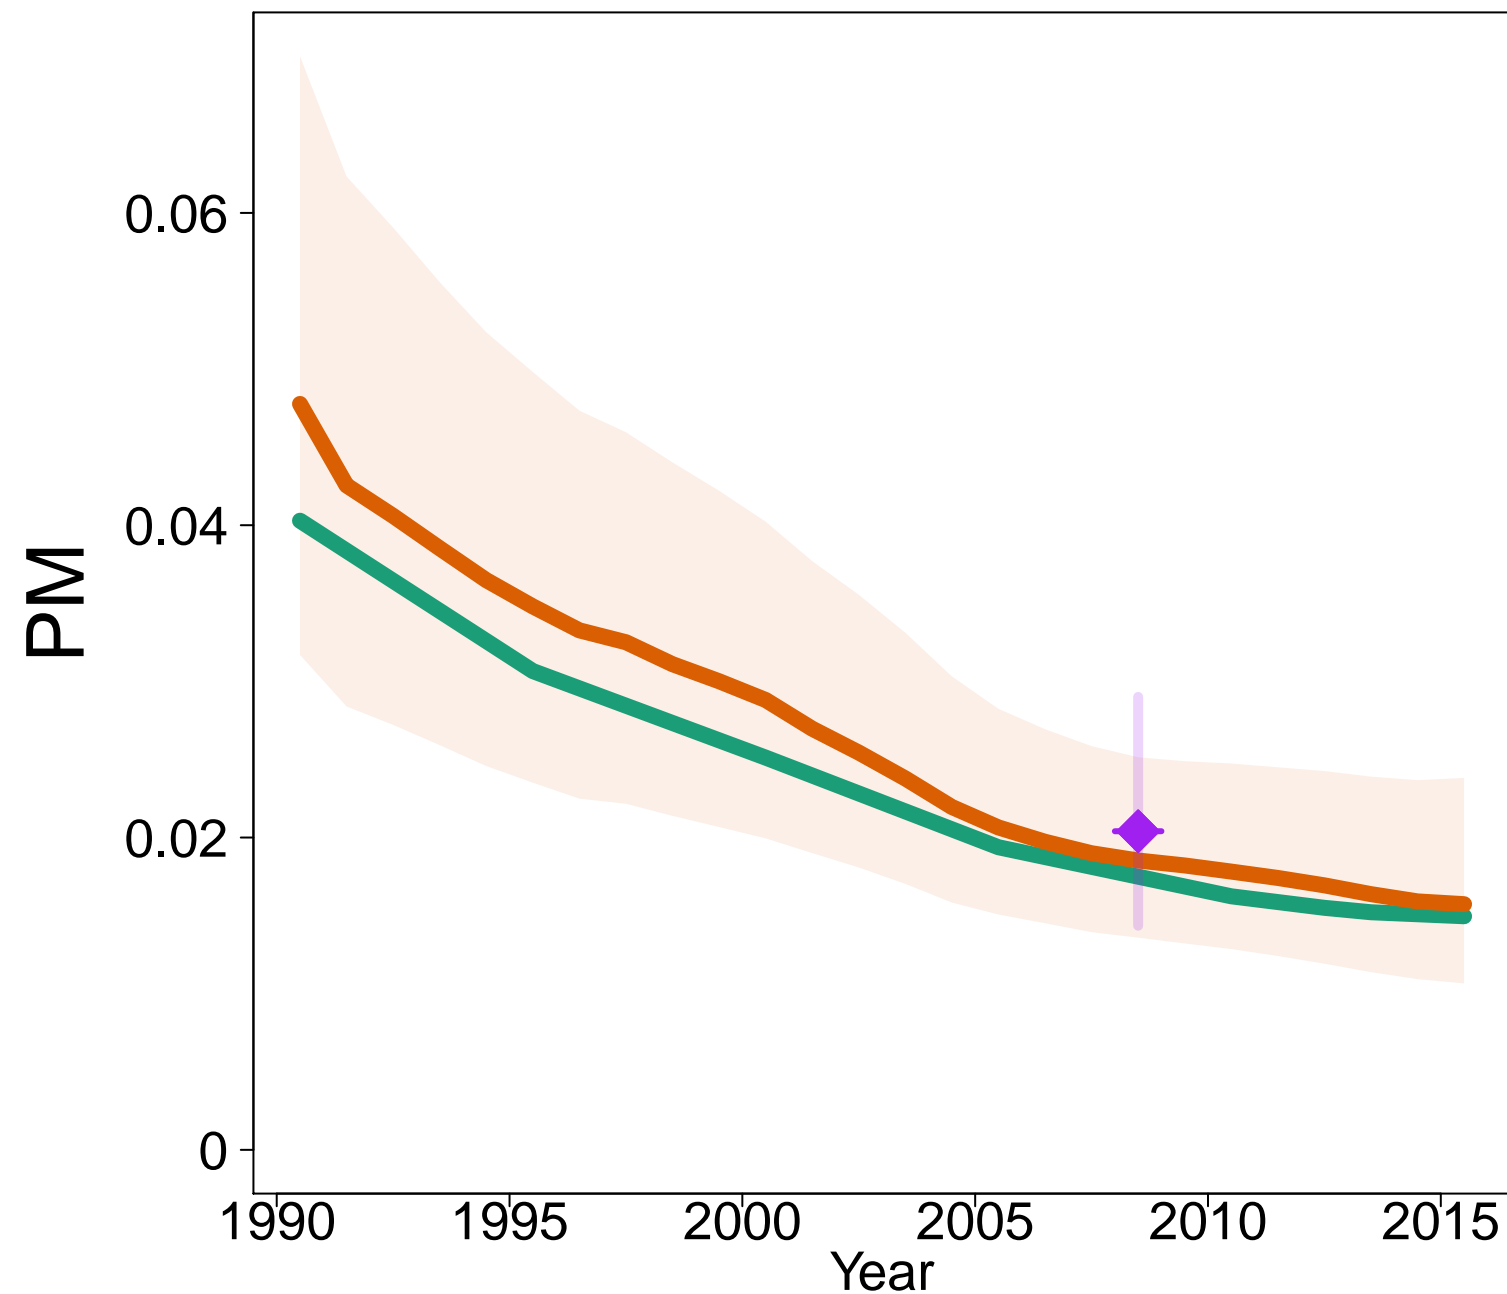

Lebanon [LBN; B]  
(Western Asia)

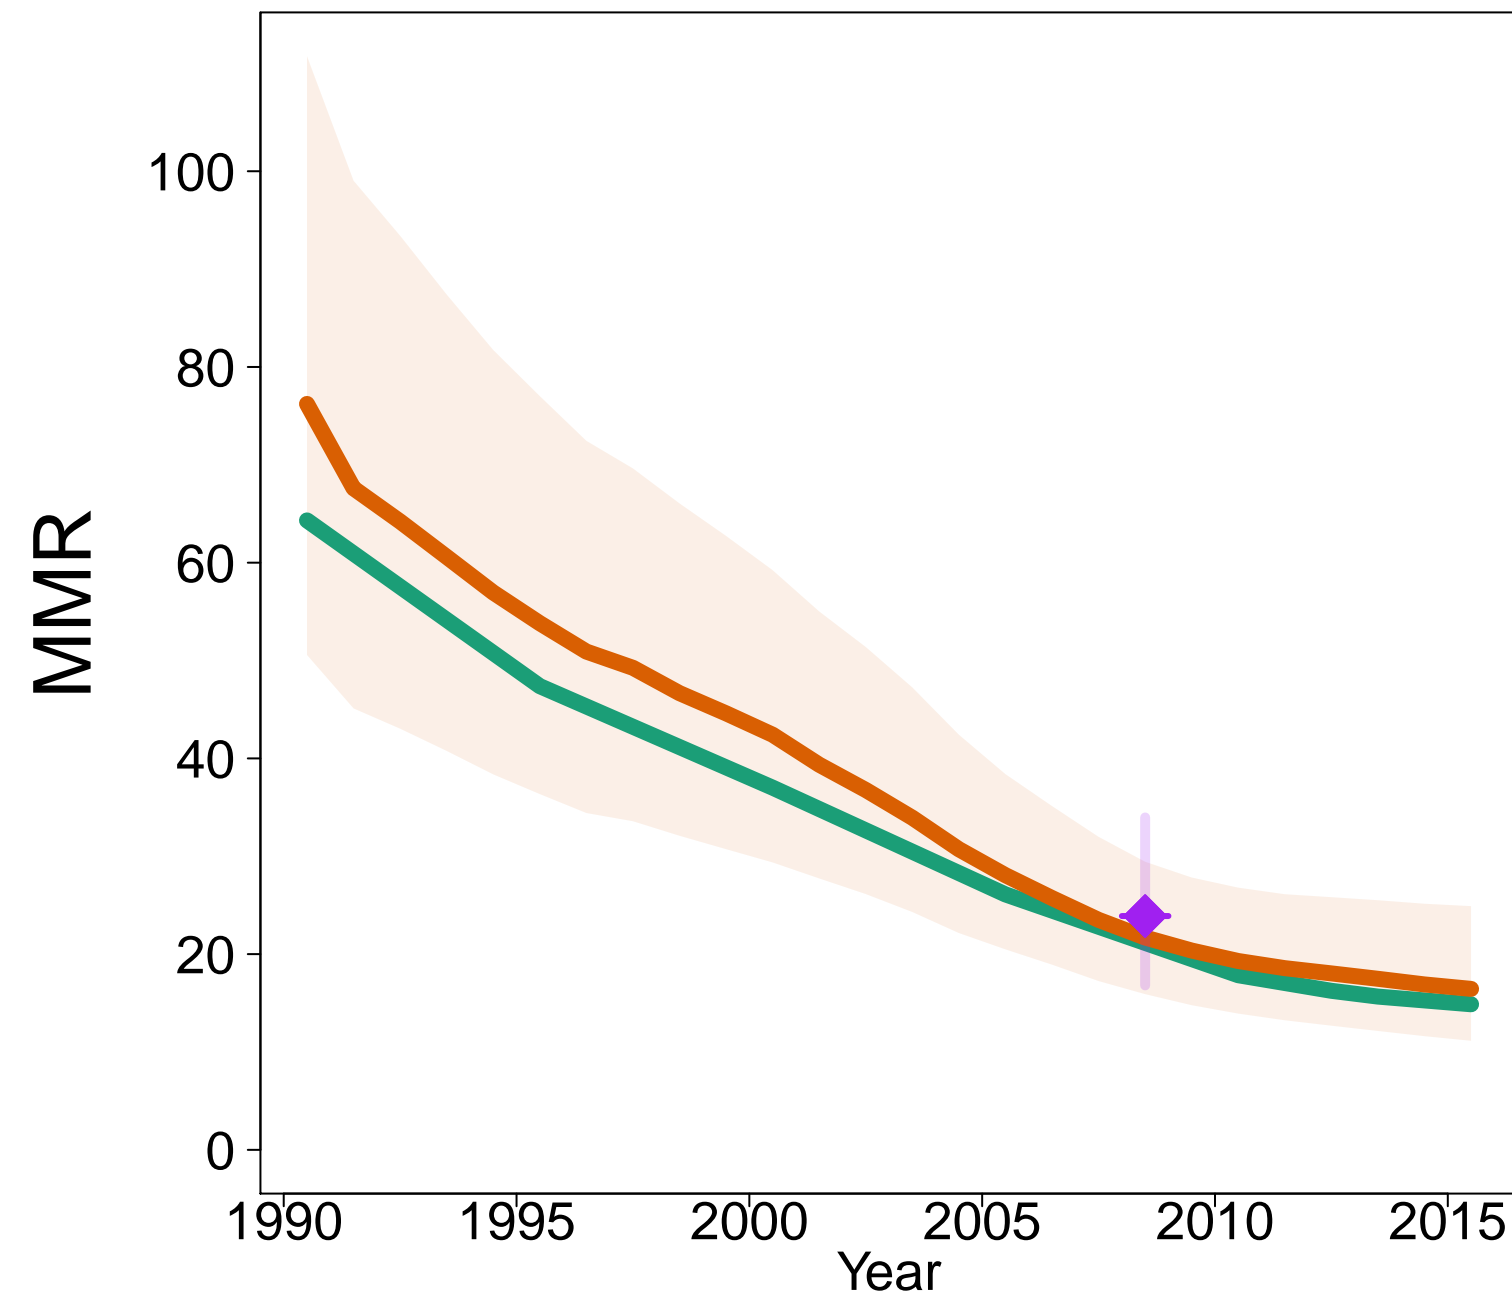

- Estimates –
- Bmat 2014
- MMEIG 2014
- Data –
- Observed Data
- Adjusted Data
- Data type –
- Spec. studies

Lesotho [LSO; B]  
(Southern Africa)

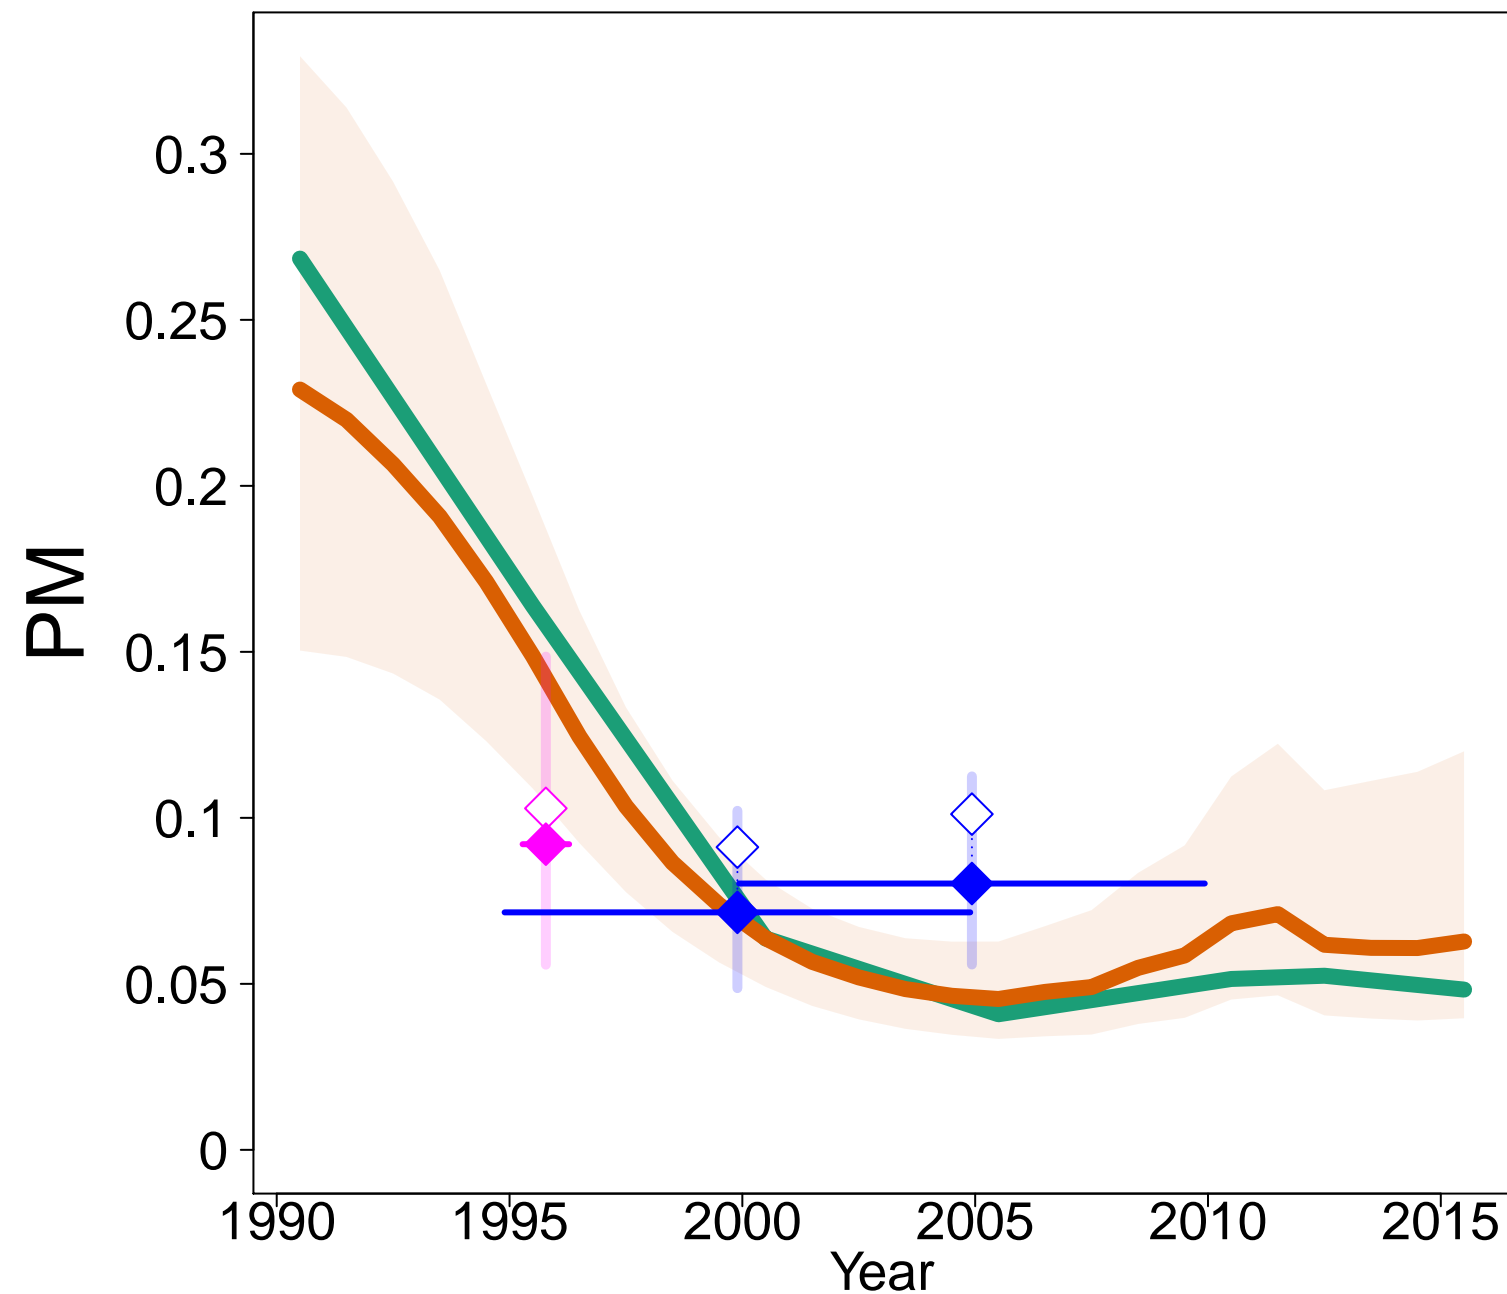

Lesotho [LSO; B]  
(Southern Africa)

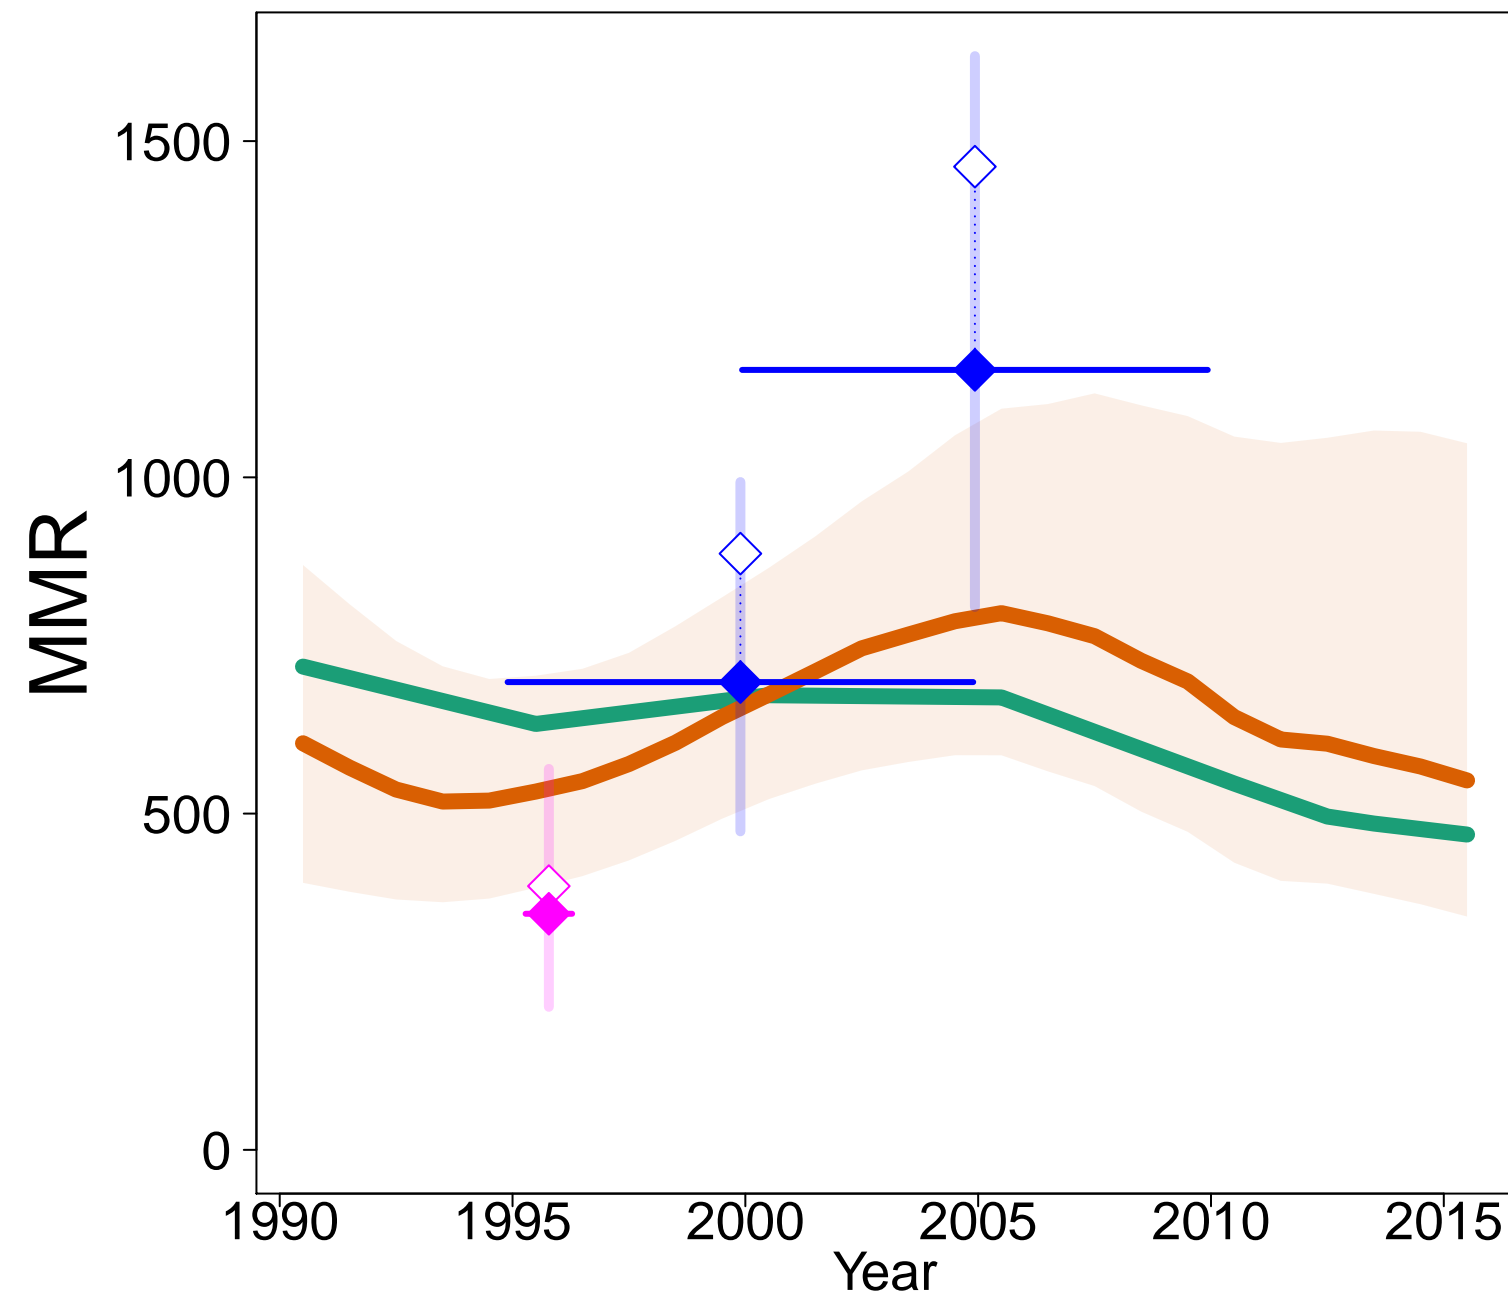

- Estimates –
- Bmat 2014
- MMEIG 2014
- Data –
- Observed Data
- Adjusted Data
- Data type –
- DHS
- Census

Liberia [LBR; B]  
(Western Africa)

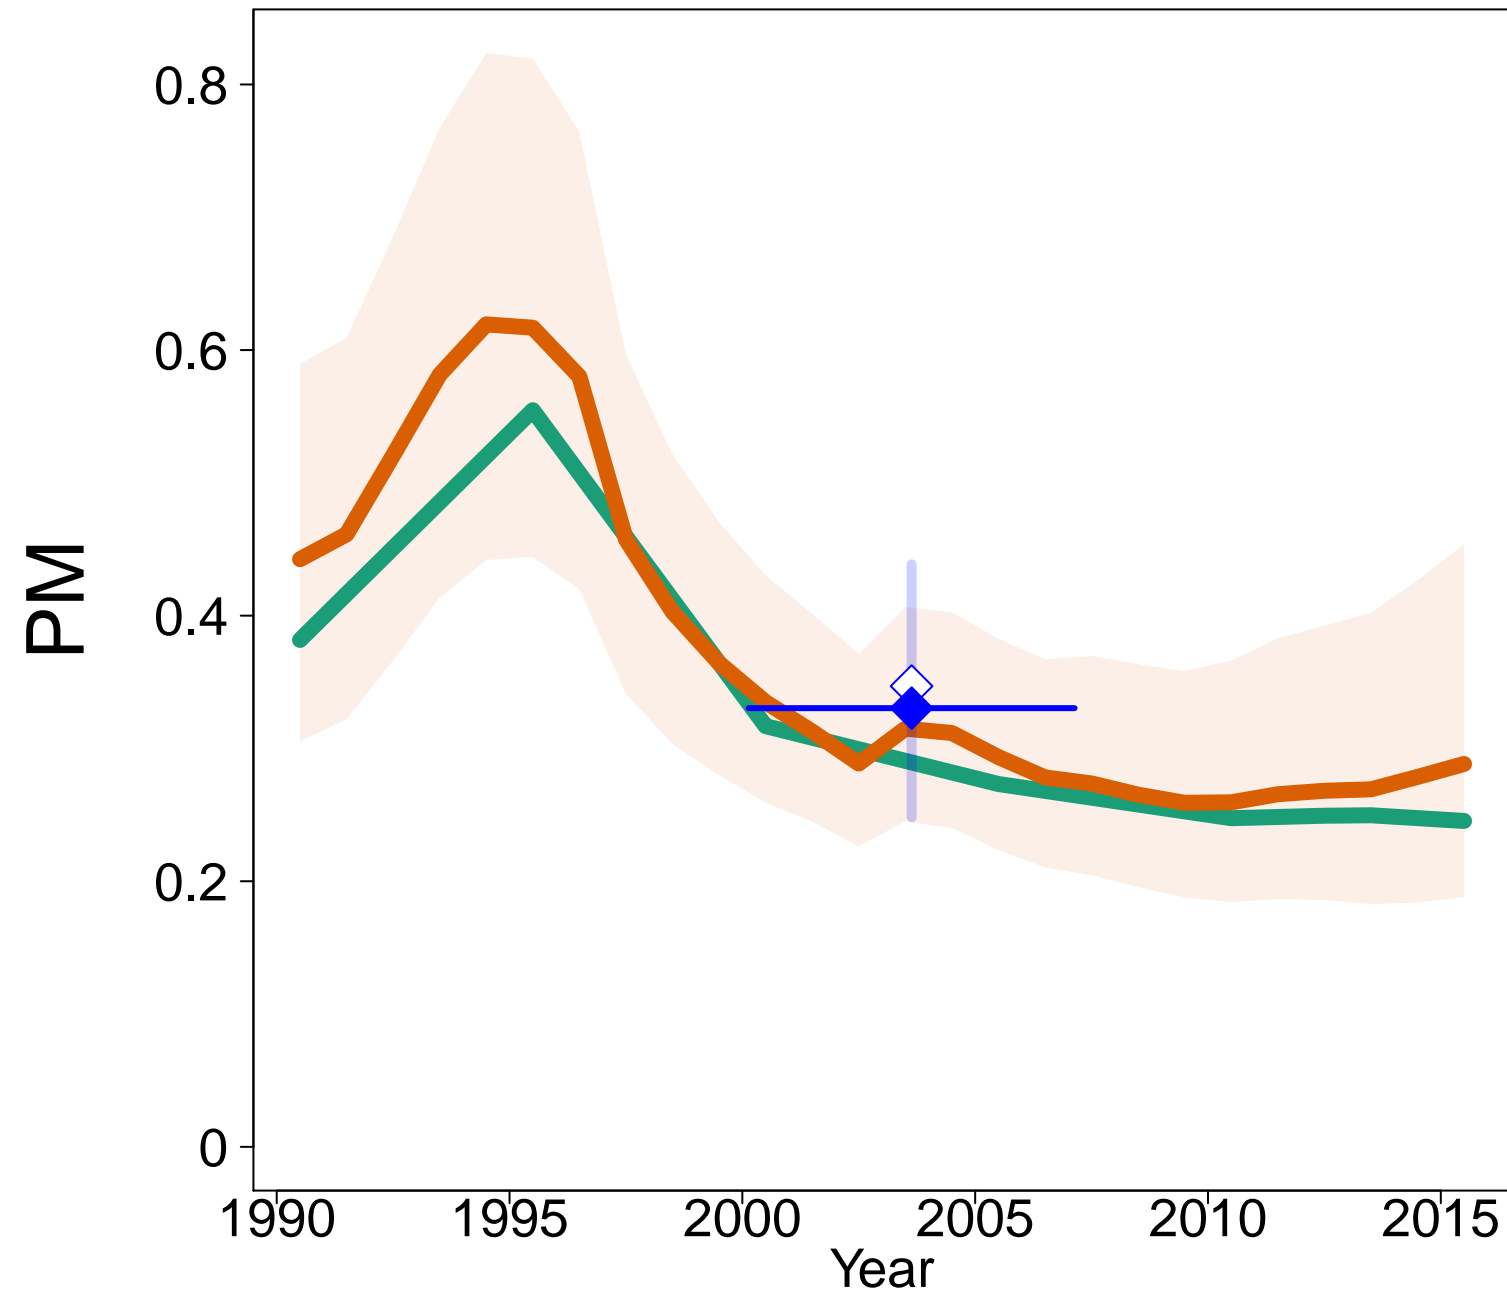

Liberia [LBR; B]  
(Western Africa)

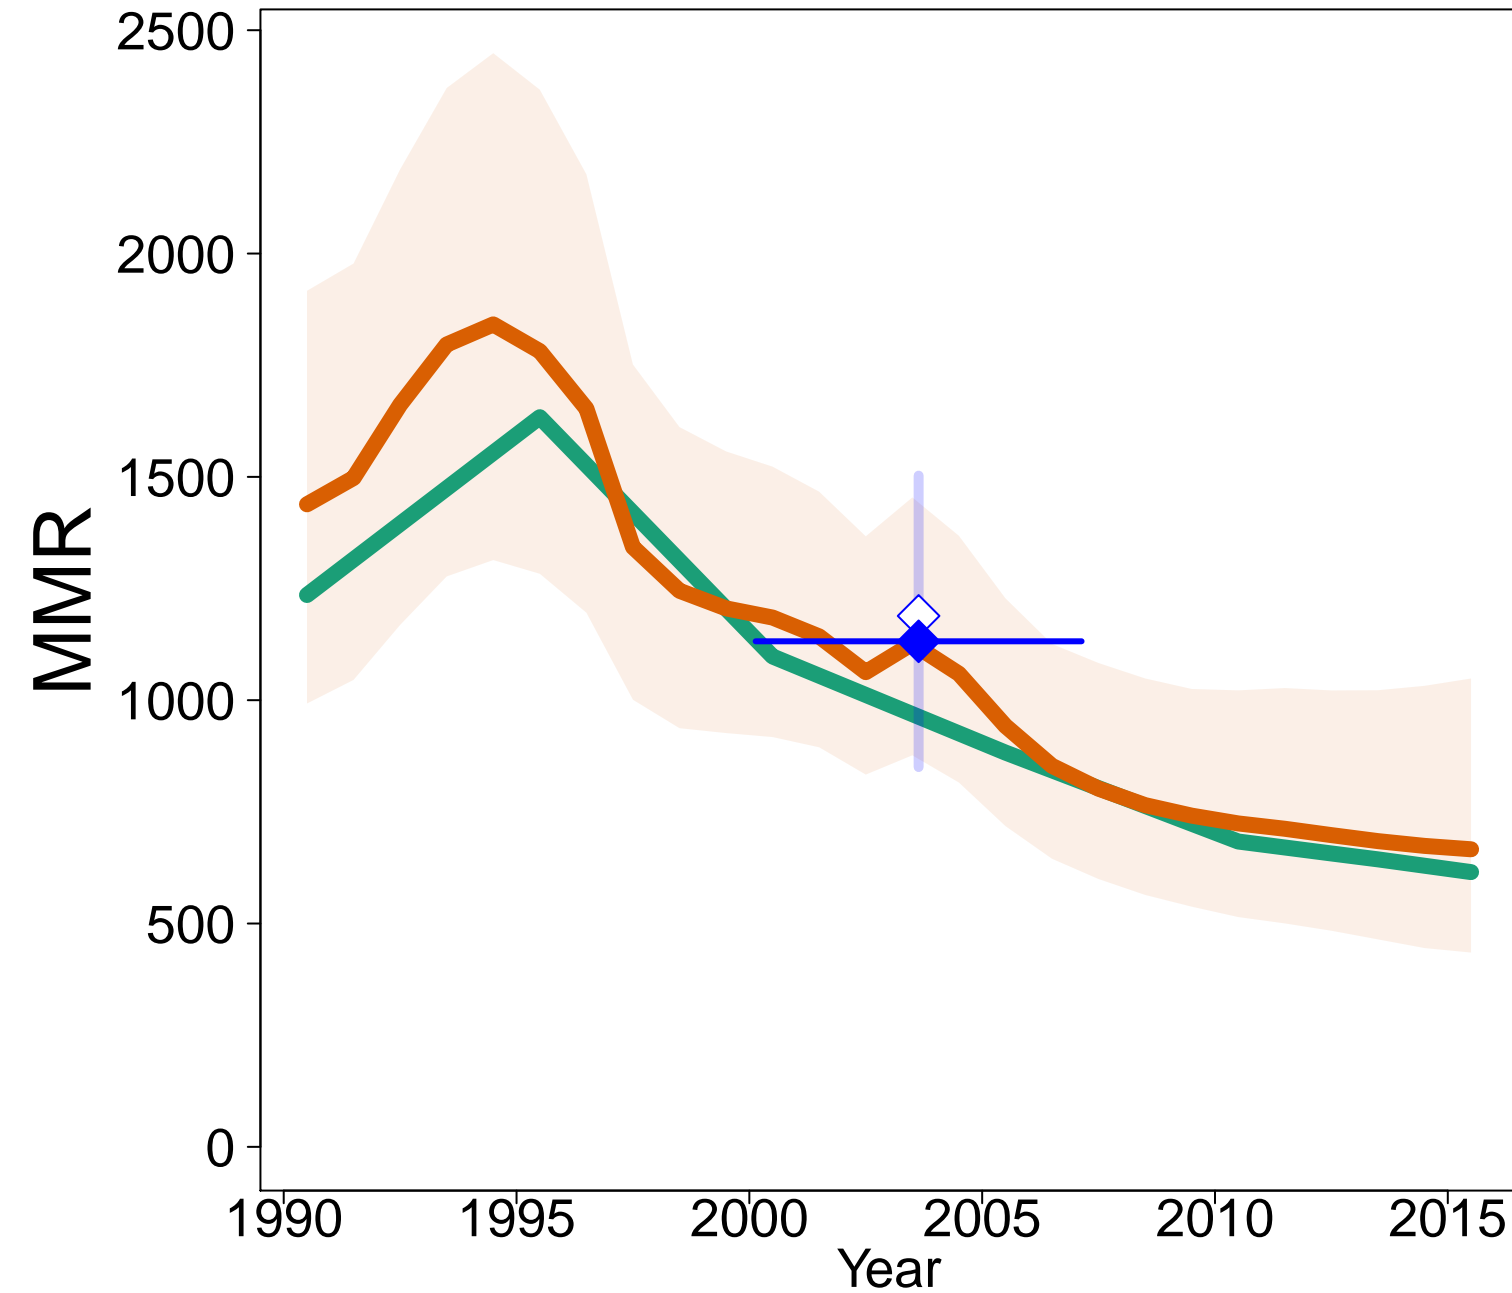

- Estimates –
- Bmat 2014
- MMEIG 2014
- Data –
- Observed Data
- Adjusted Data
- Data type –
- DHS

Libya [LBY; B]  
(Northern Africa)

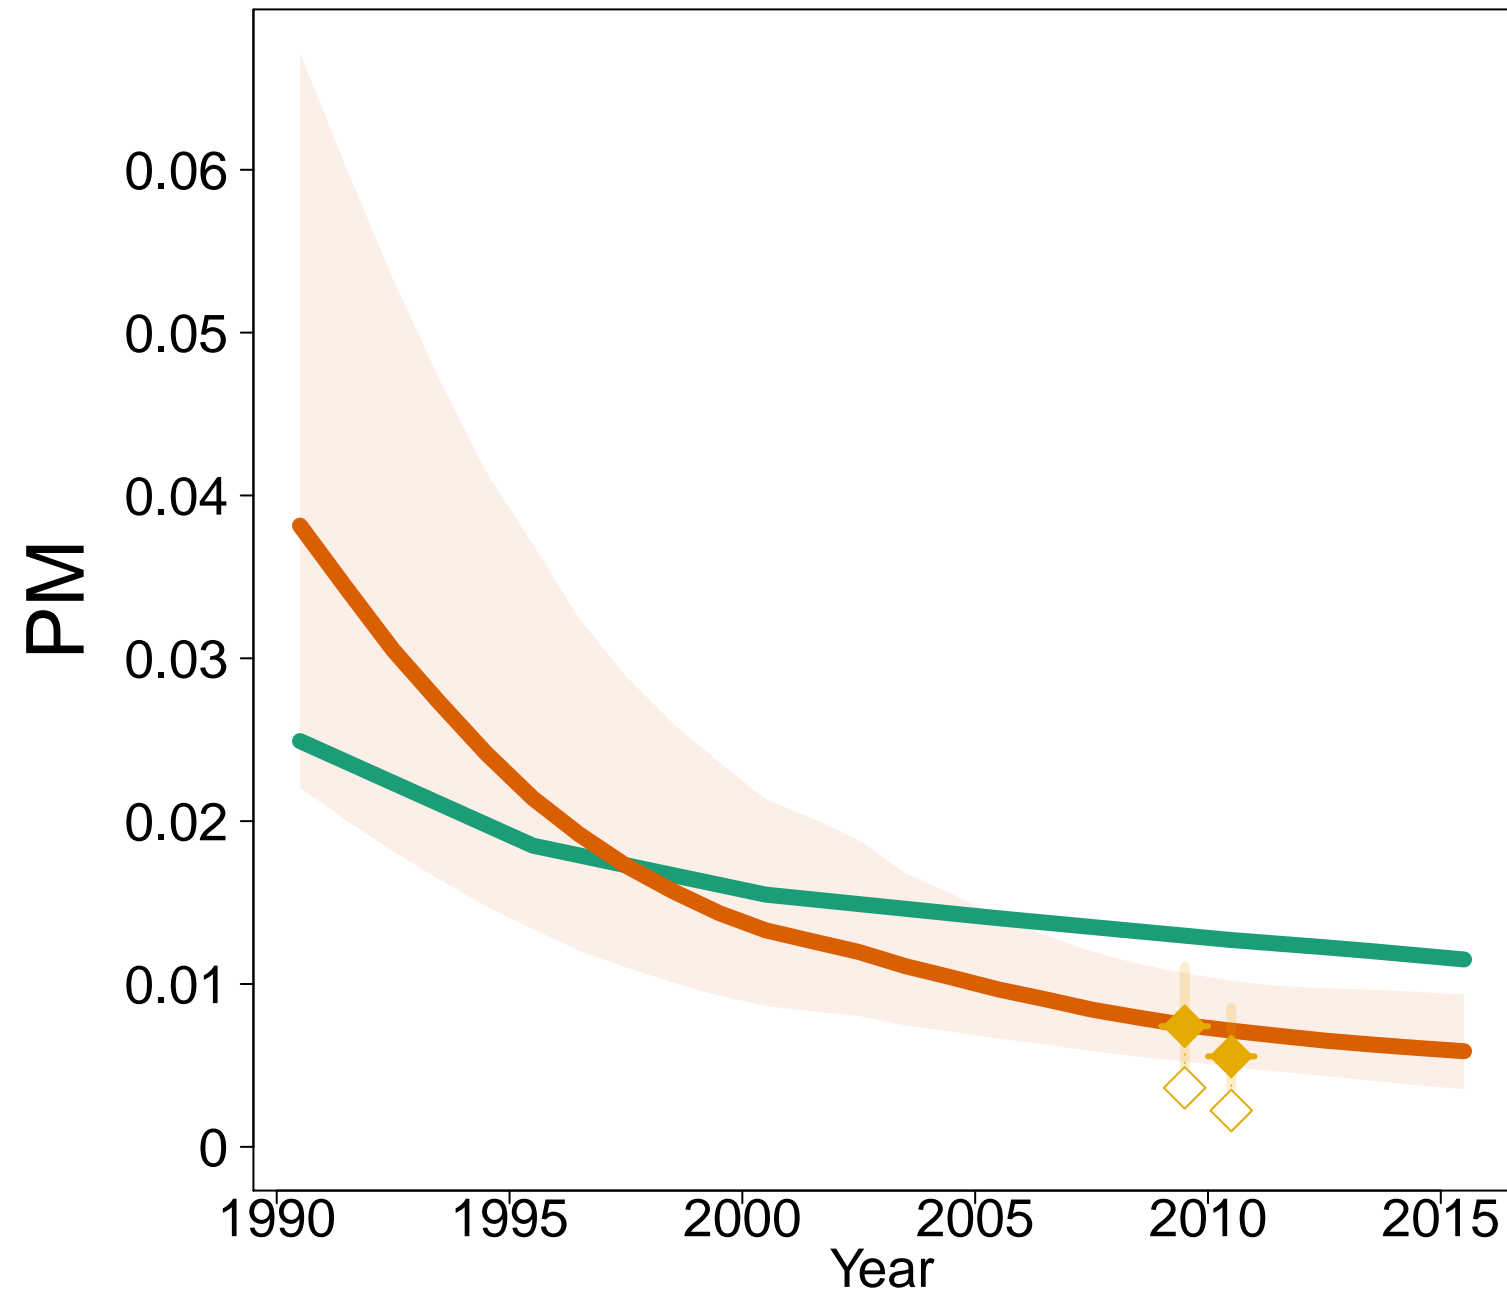

Libya [LBY; B]  
(Northern Africa)

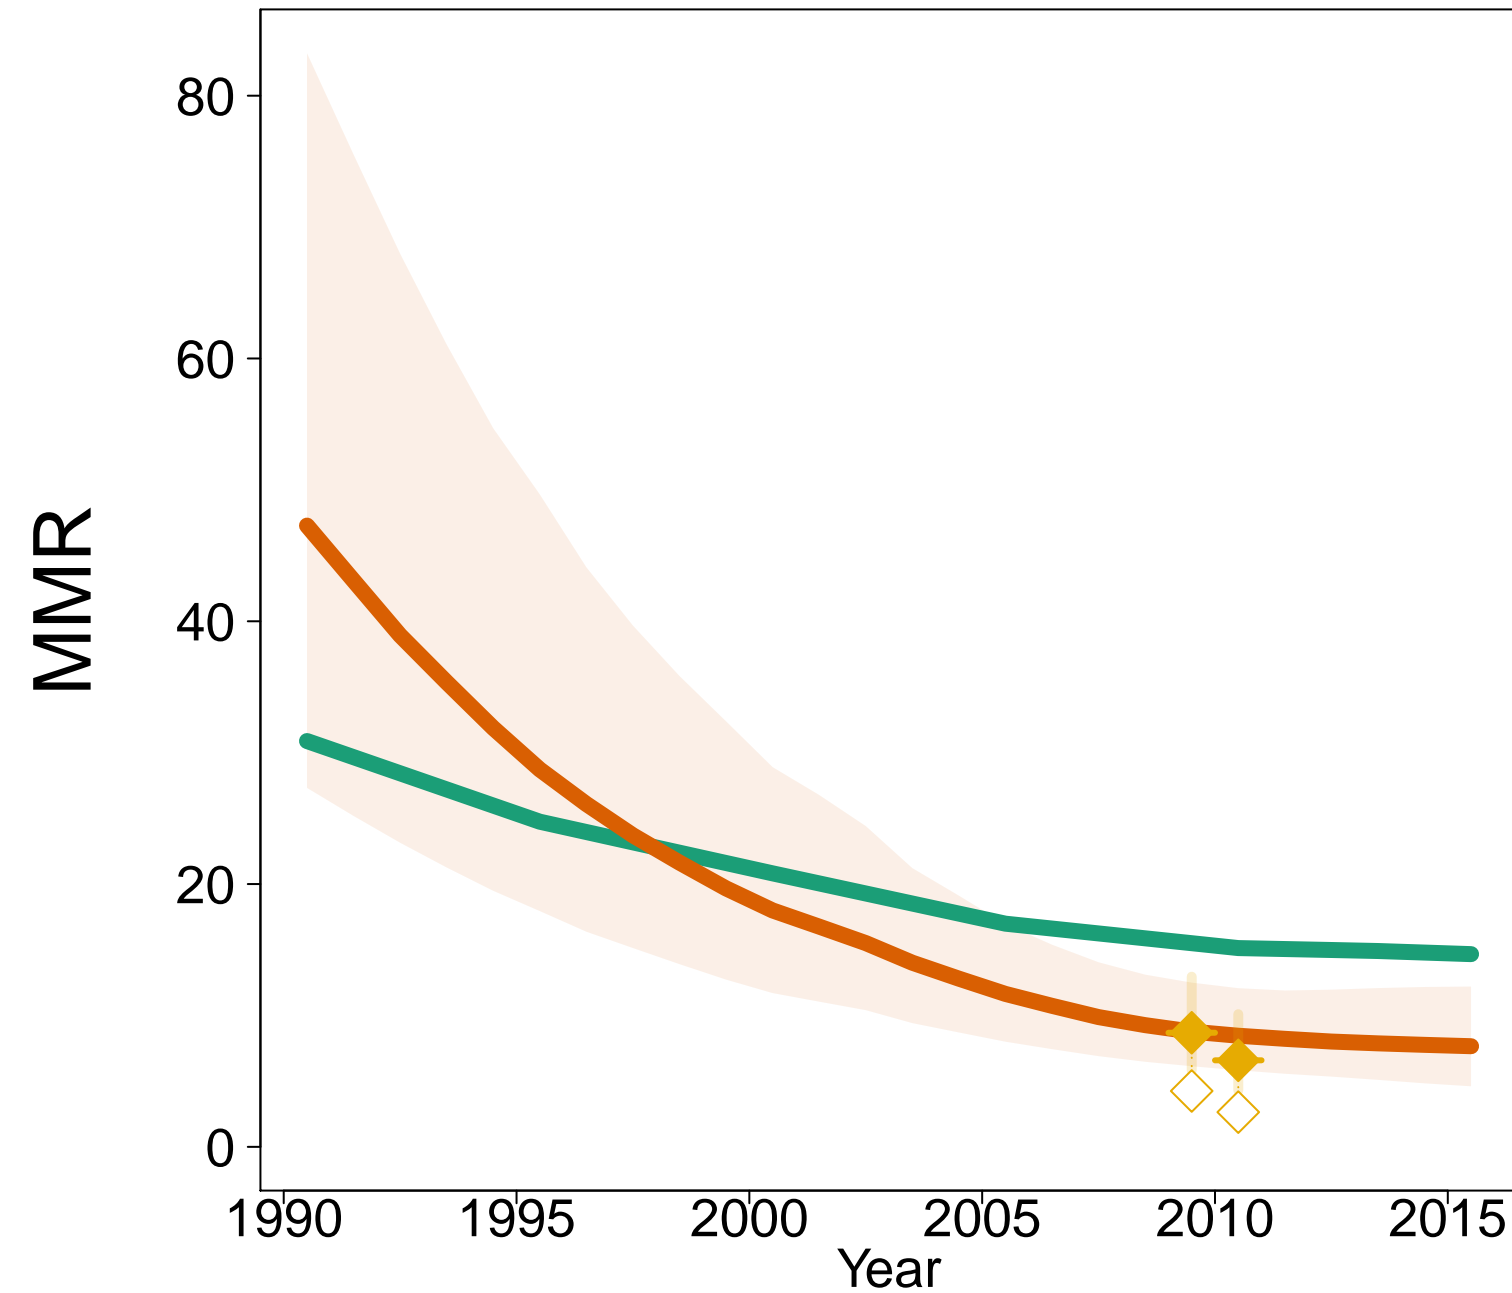

- Estimates –
- Bmat 2014
- MMEIG 2014
- Data –
- Observed Data
- Adjusted Data
- Data type –
- VR

Lithuania [LTU; A]  
(Developed regions)

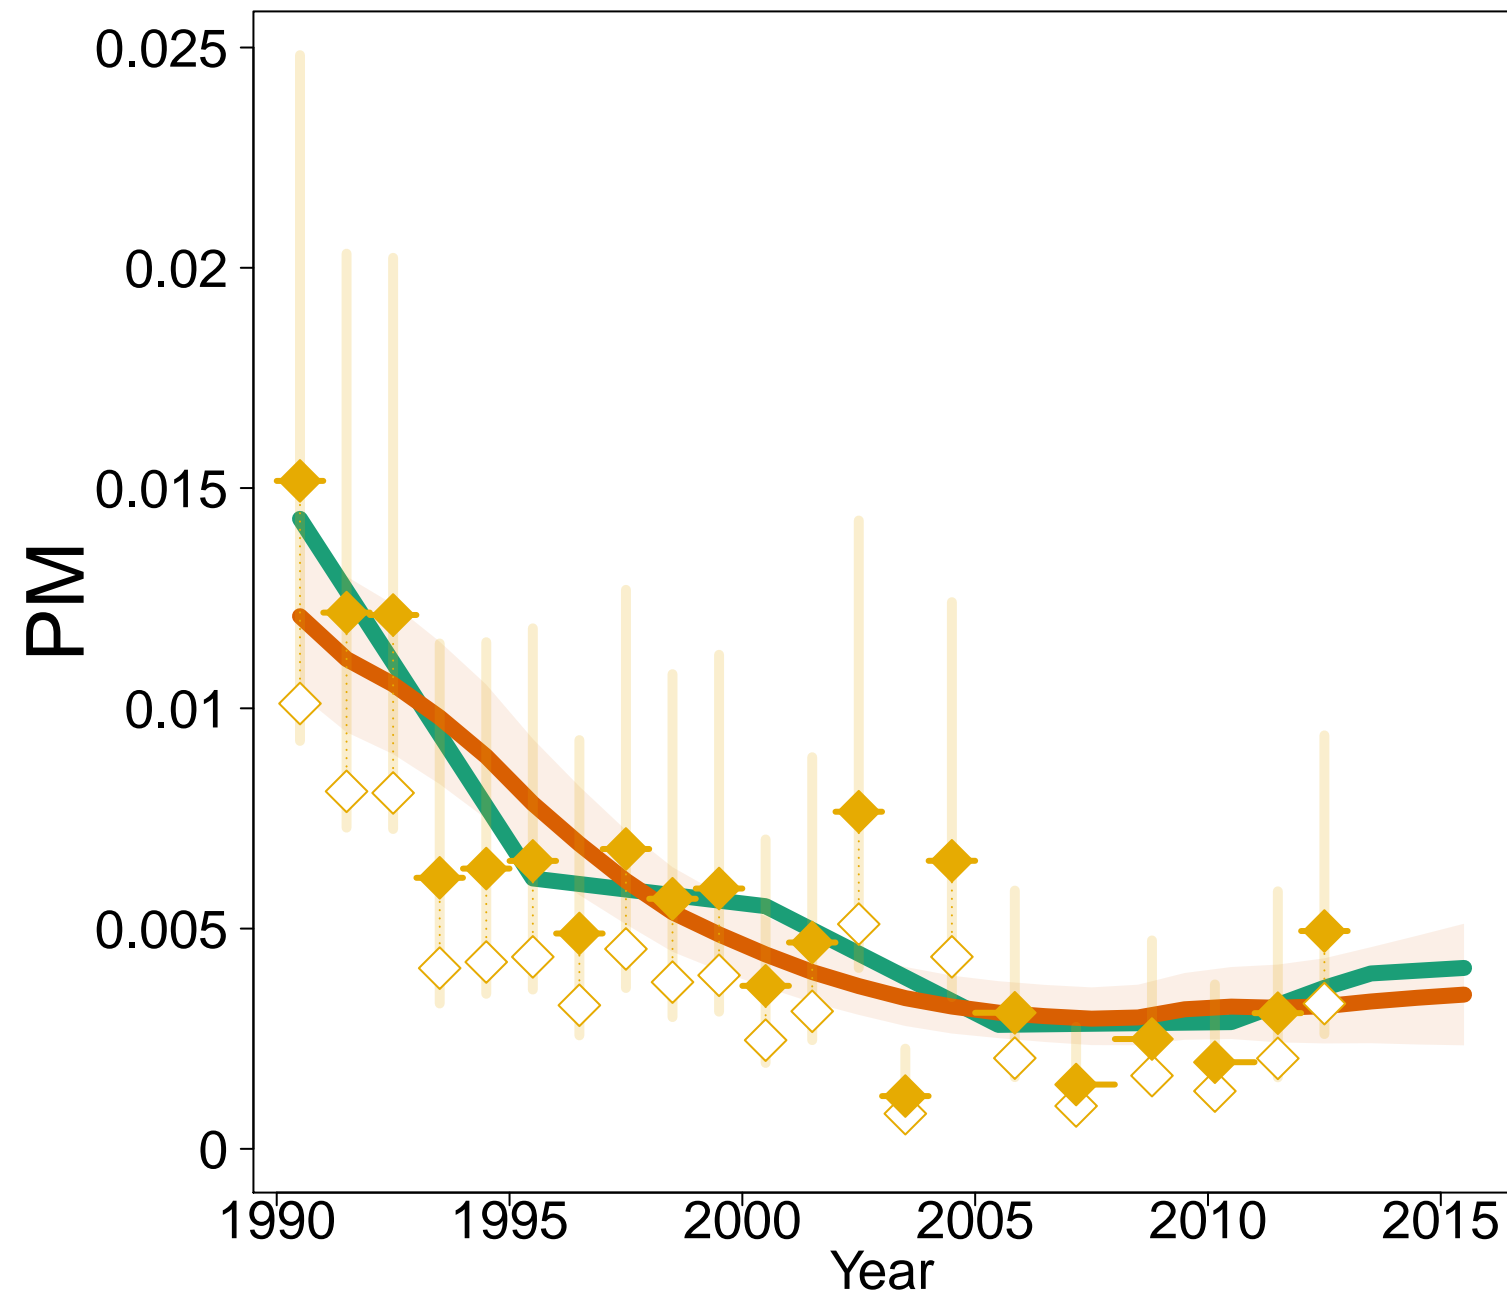

Lithuania [LTU; A]  
(Developed regions)

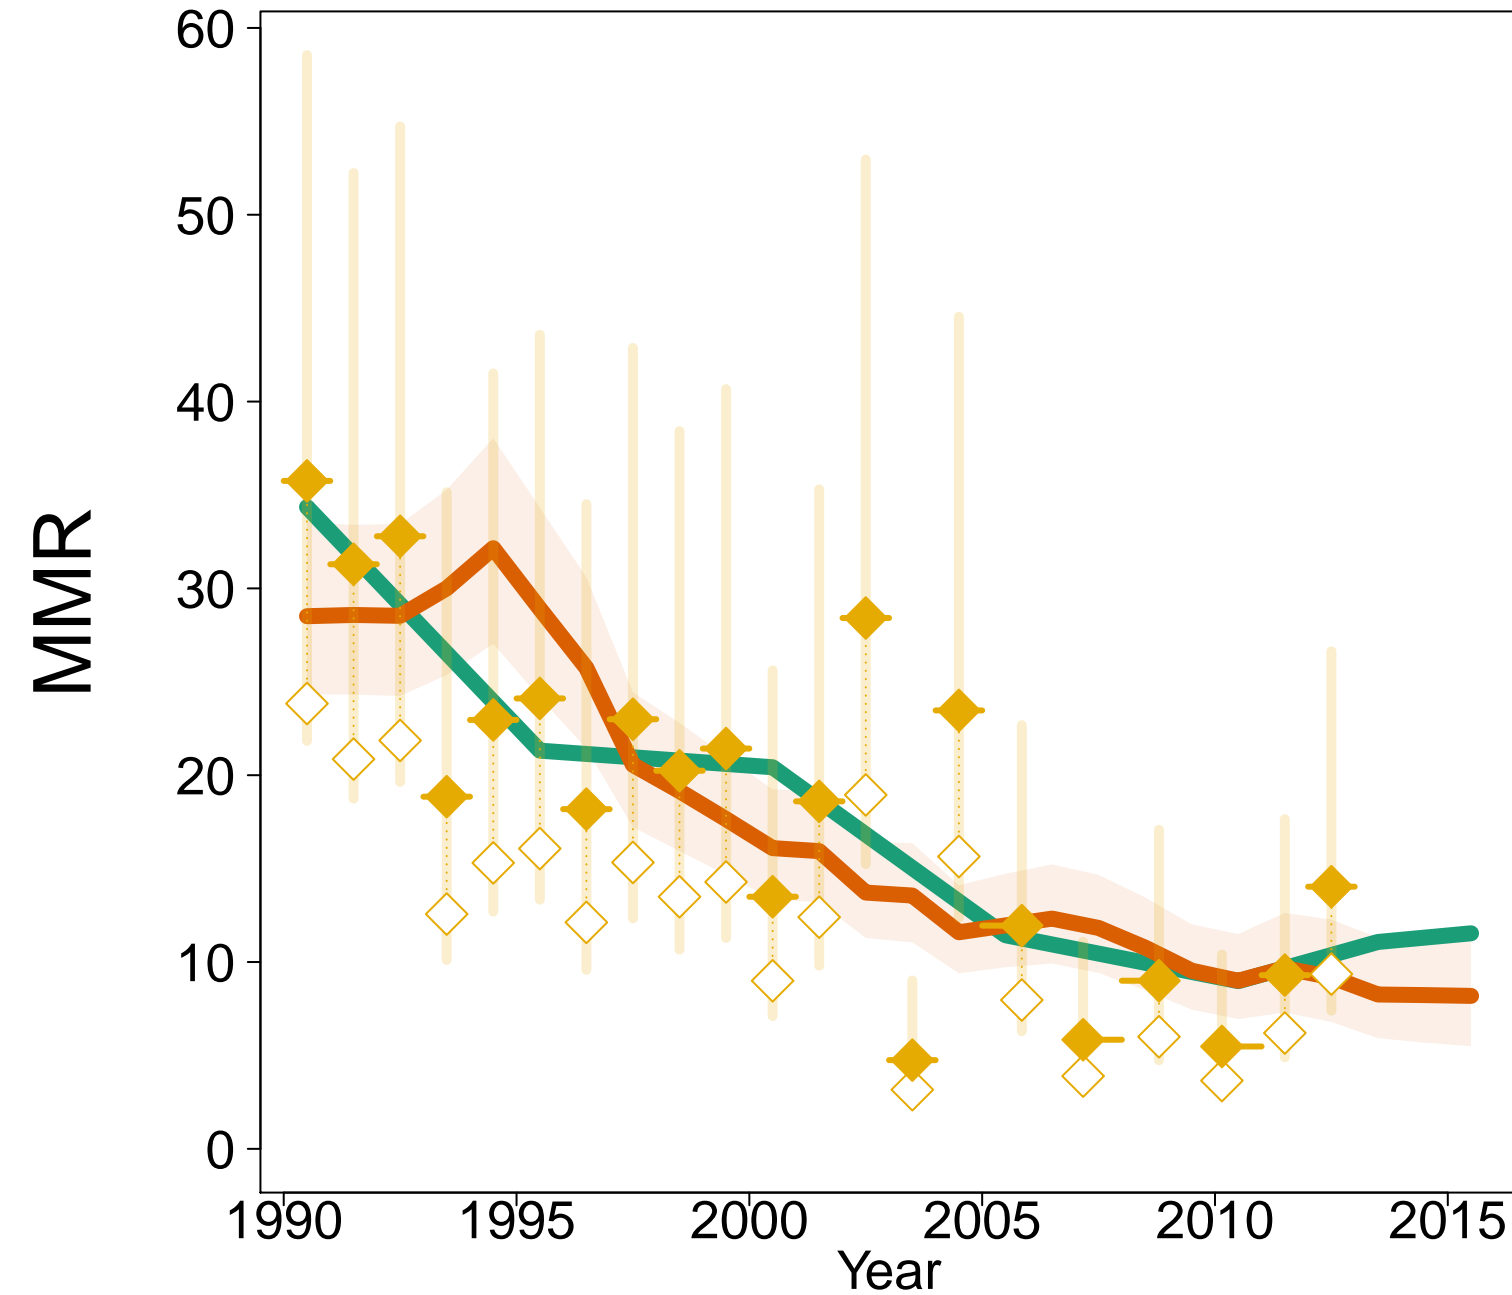

- Estimates –
- Bmat 2014
- MMEIG 2014
- Data –
- Observed Data
- Adjusted Data
- Data type –
- VR

Luxembourg [LUX; A]  
(Developed regions)

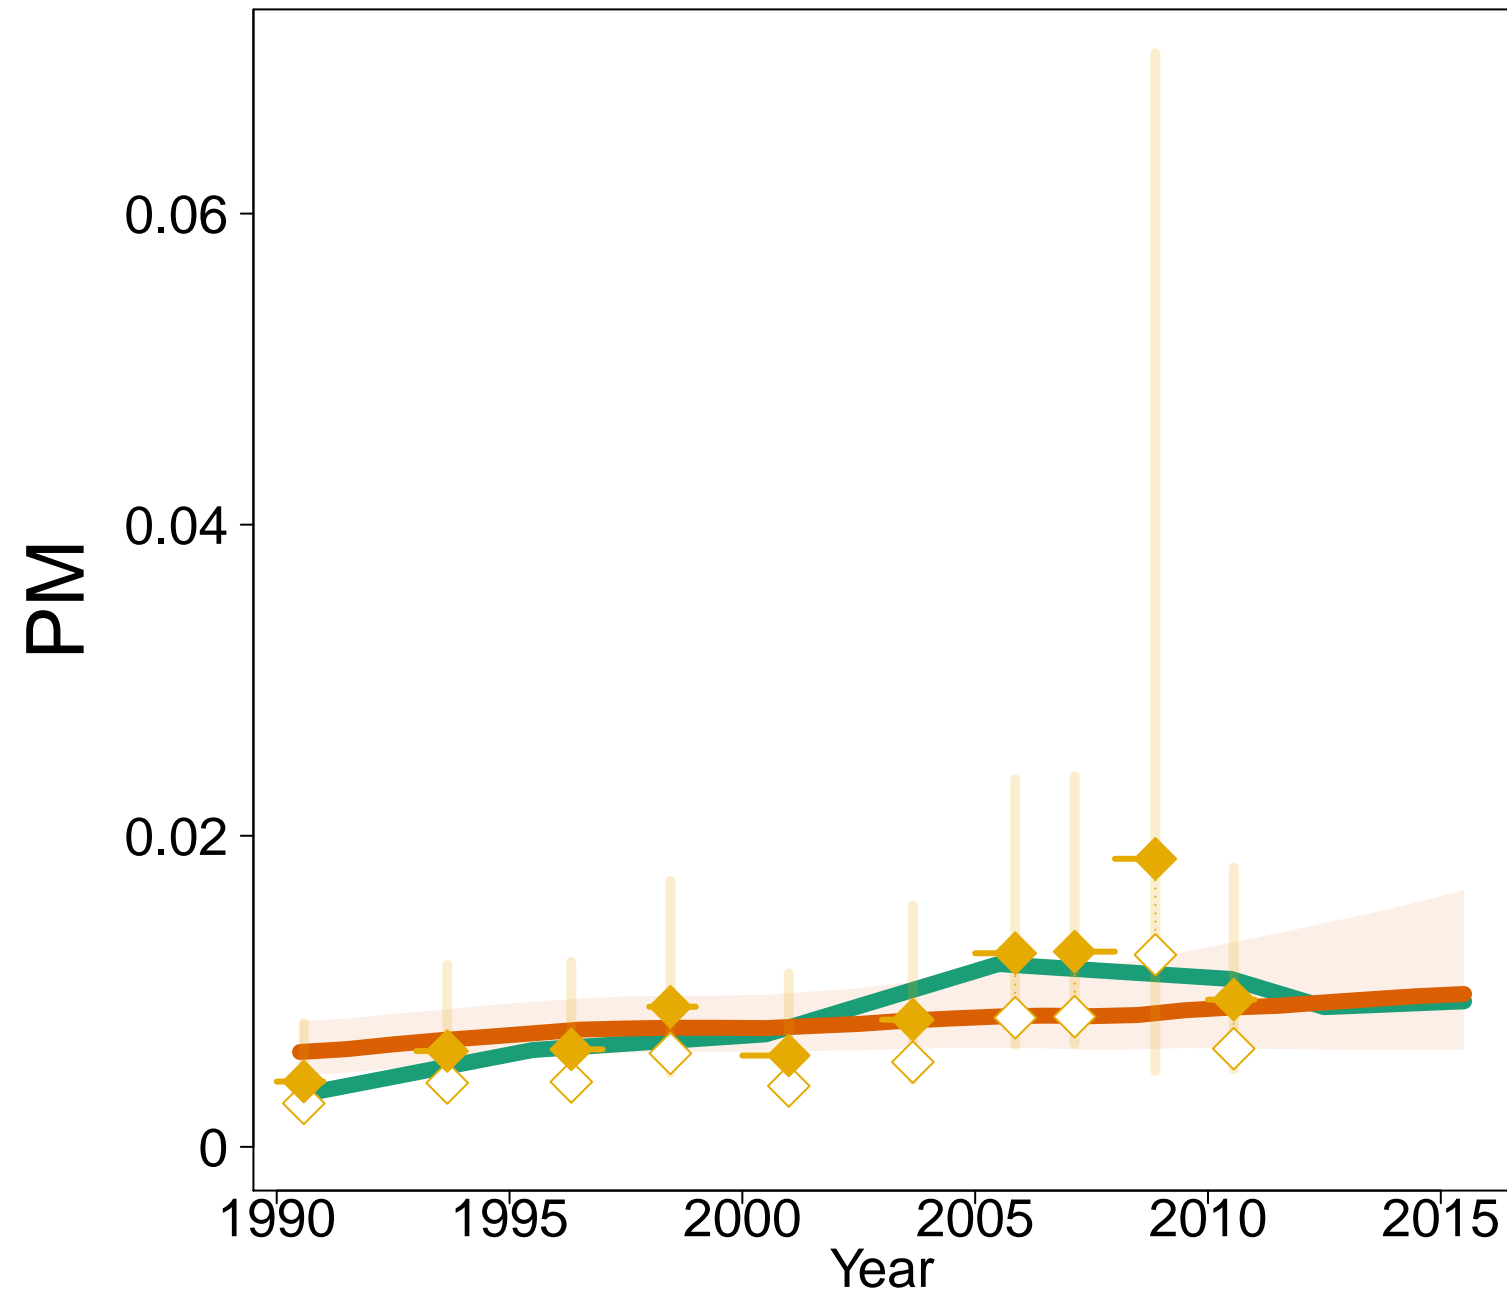

Luxembourg [LUX; A]  
(Developed regions)

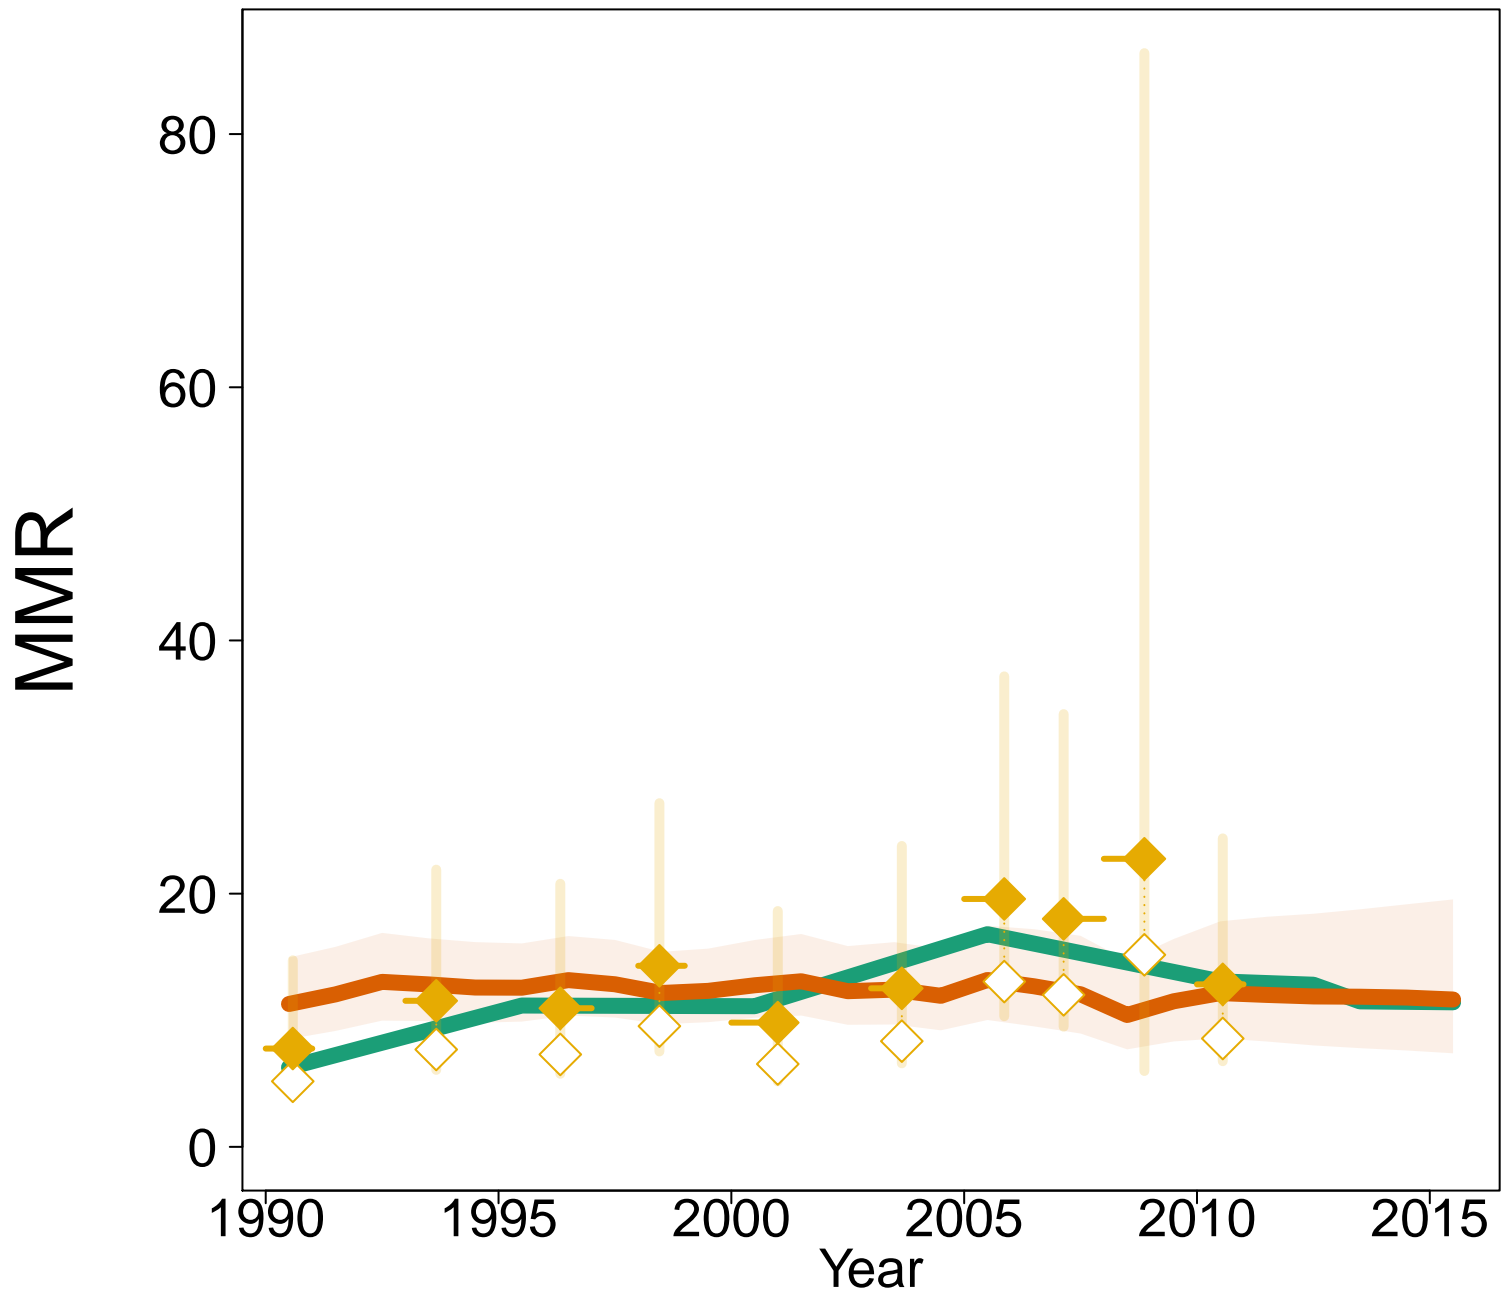

- Estimates –
- Bmat 2014
- MMEIG 2014
- Data –
- Observed Data
- Adjusted Data
- Data type –
- VR



Madagascar [MDG; B]  
(Eastern Africa)

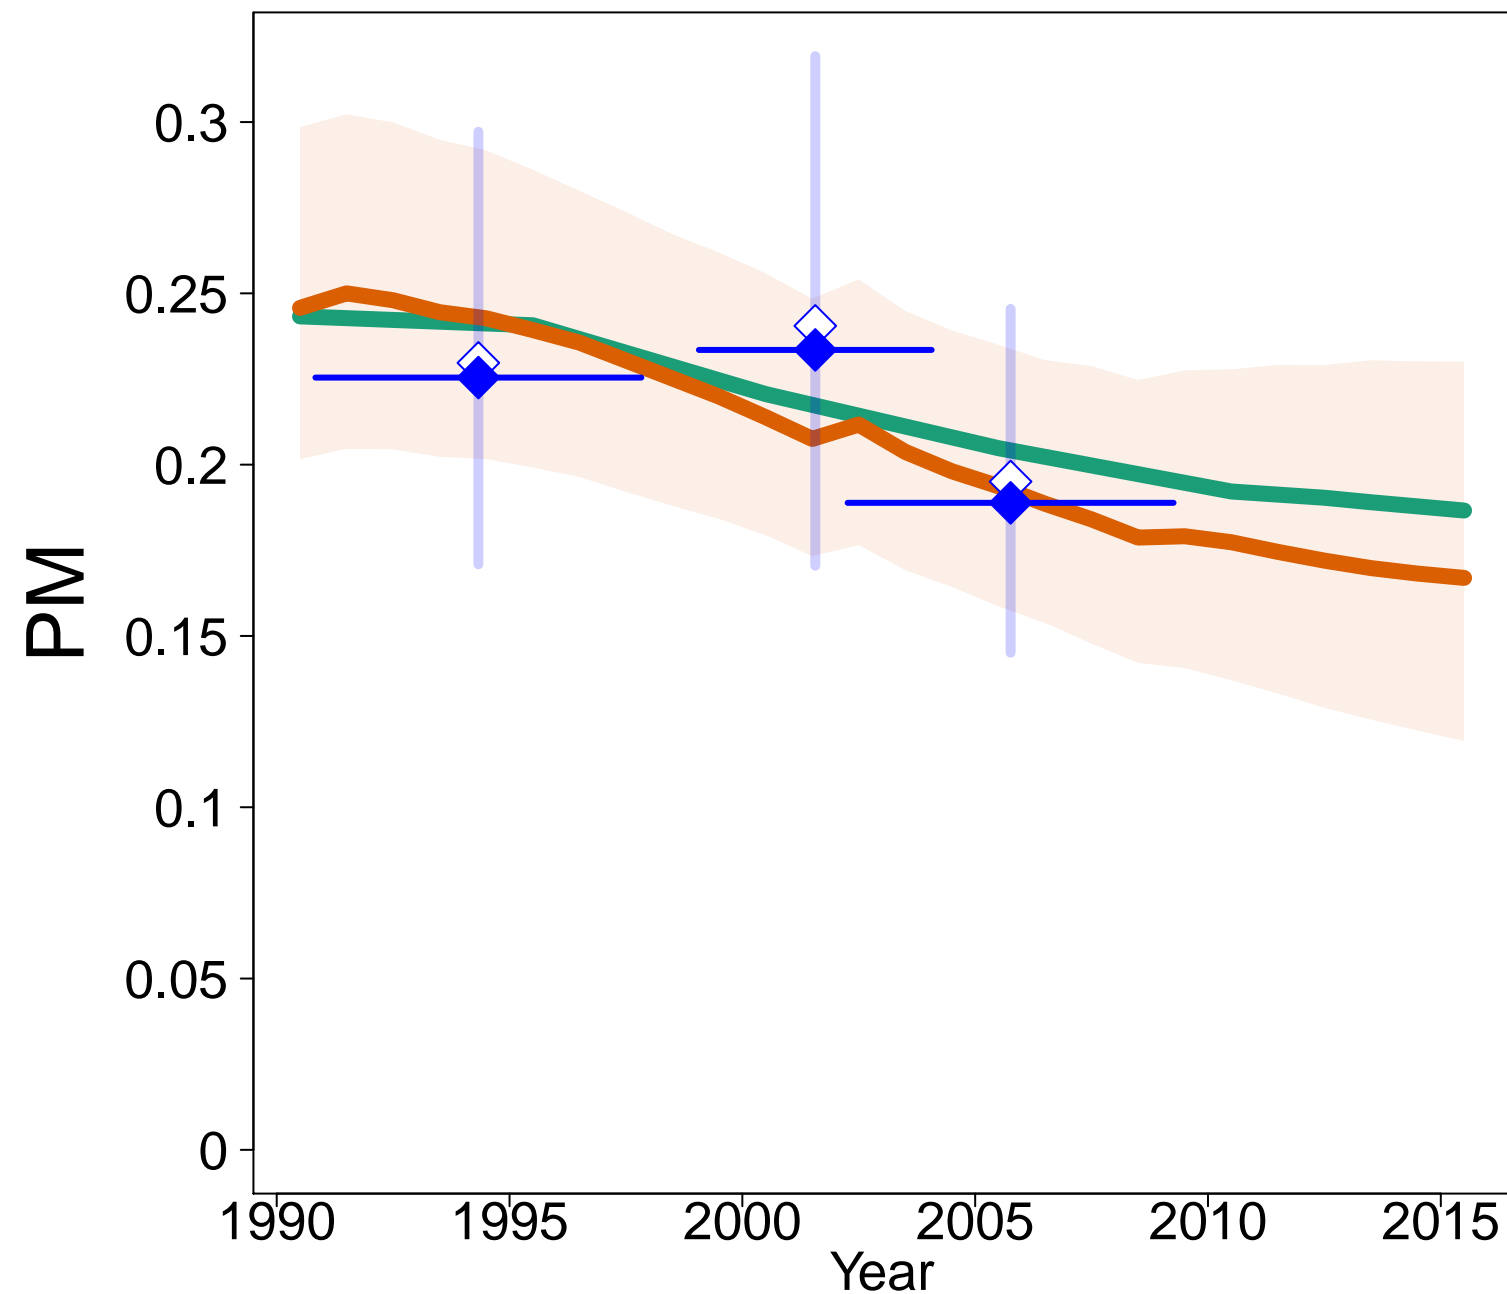

Madagascar [MDG; B]  
(Eastern Africa)

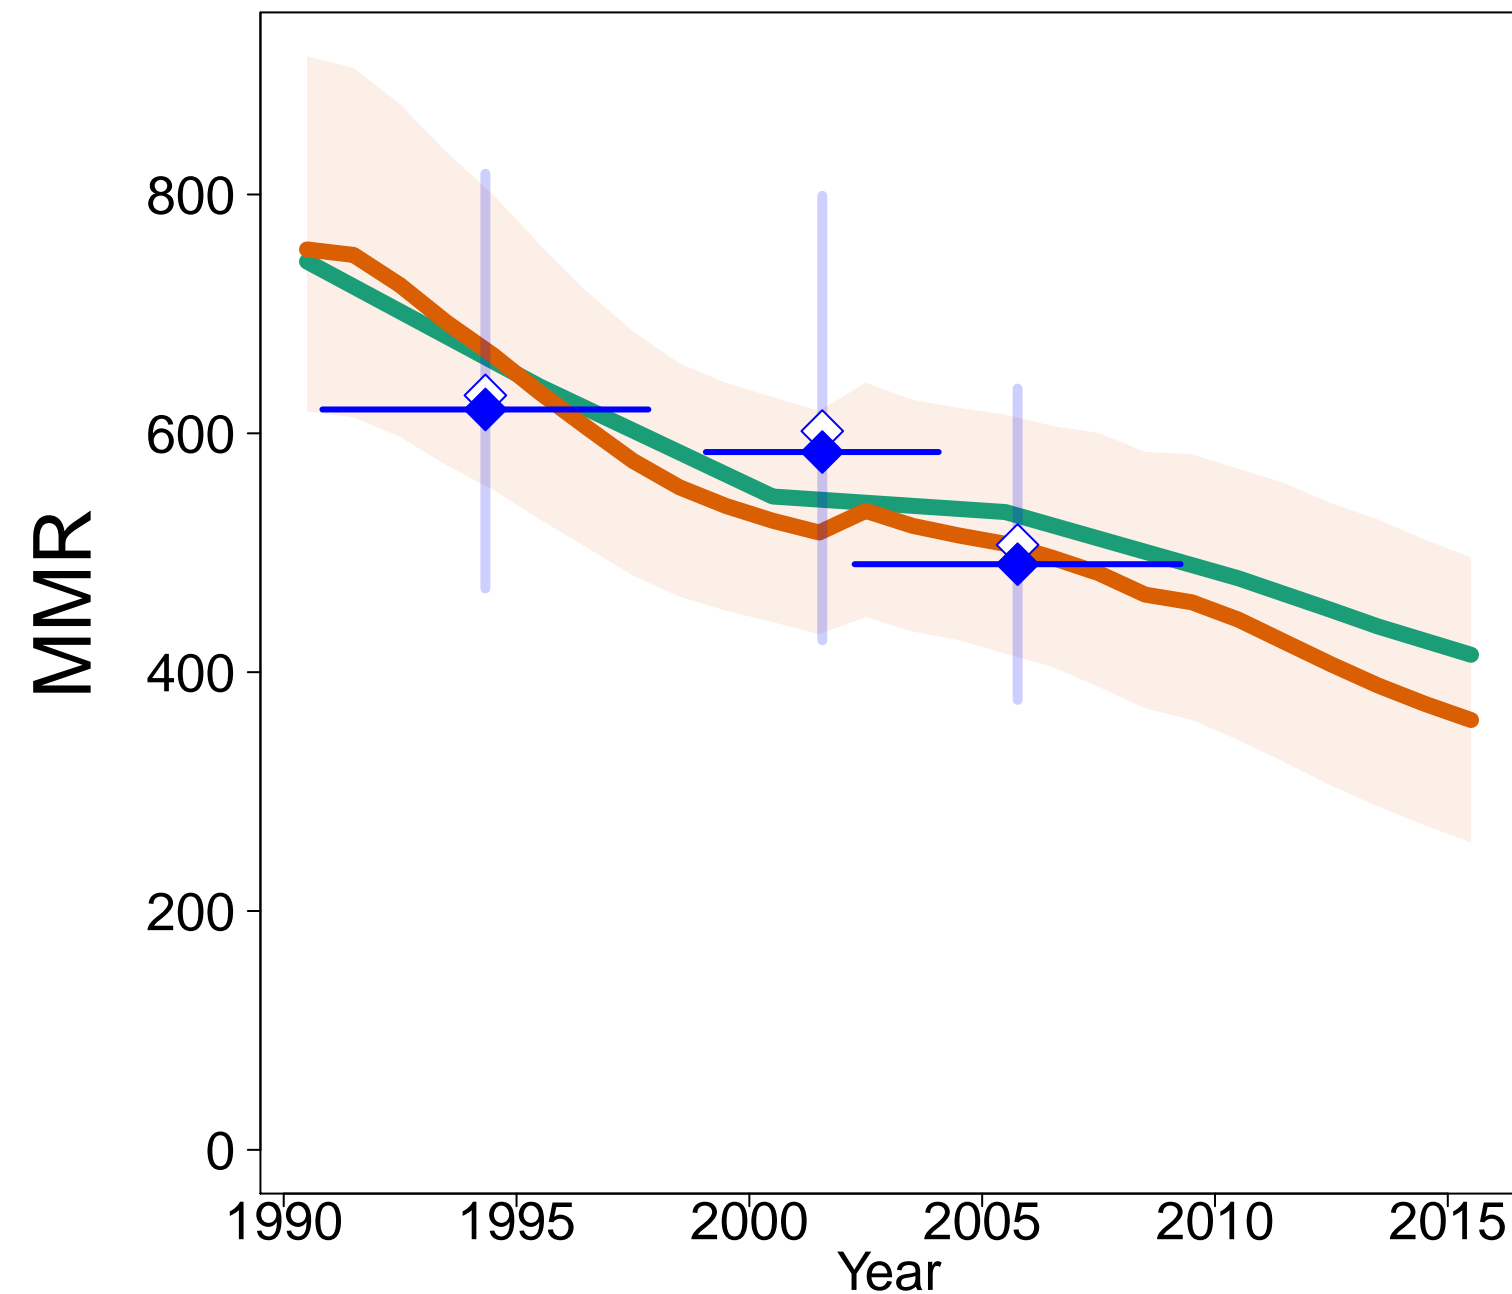

– Estimates –  
 Bmat 2014  
 MMEIG 2014  
 – Data –  
 Observed Data  
 Adjusted Data  
 – Data type –  
 DHS

Malawi [MWI; B]  
(Eastern Africa)

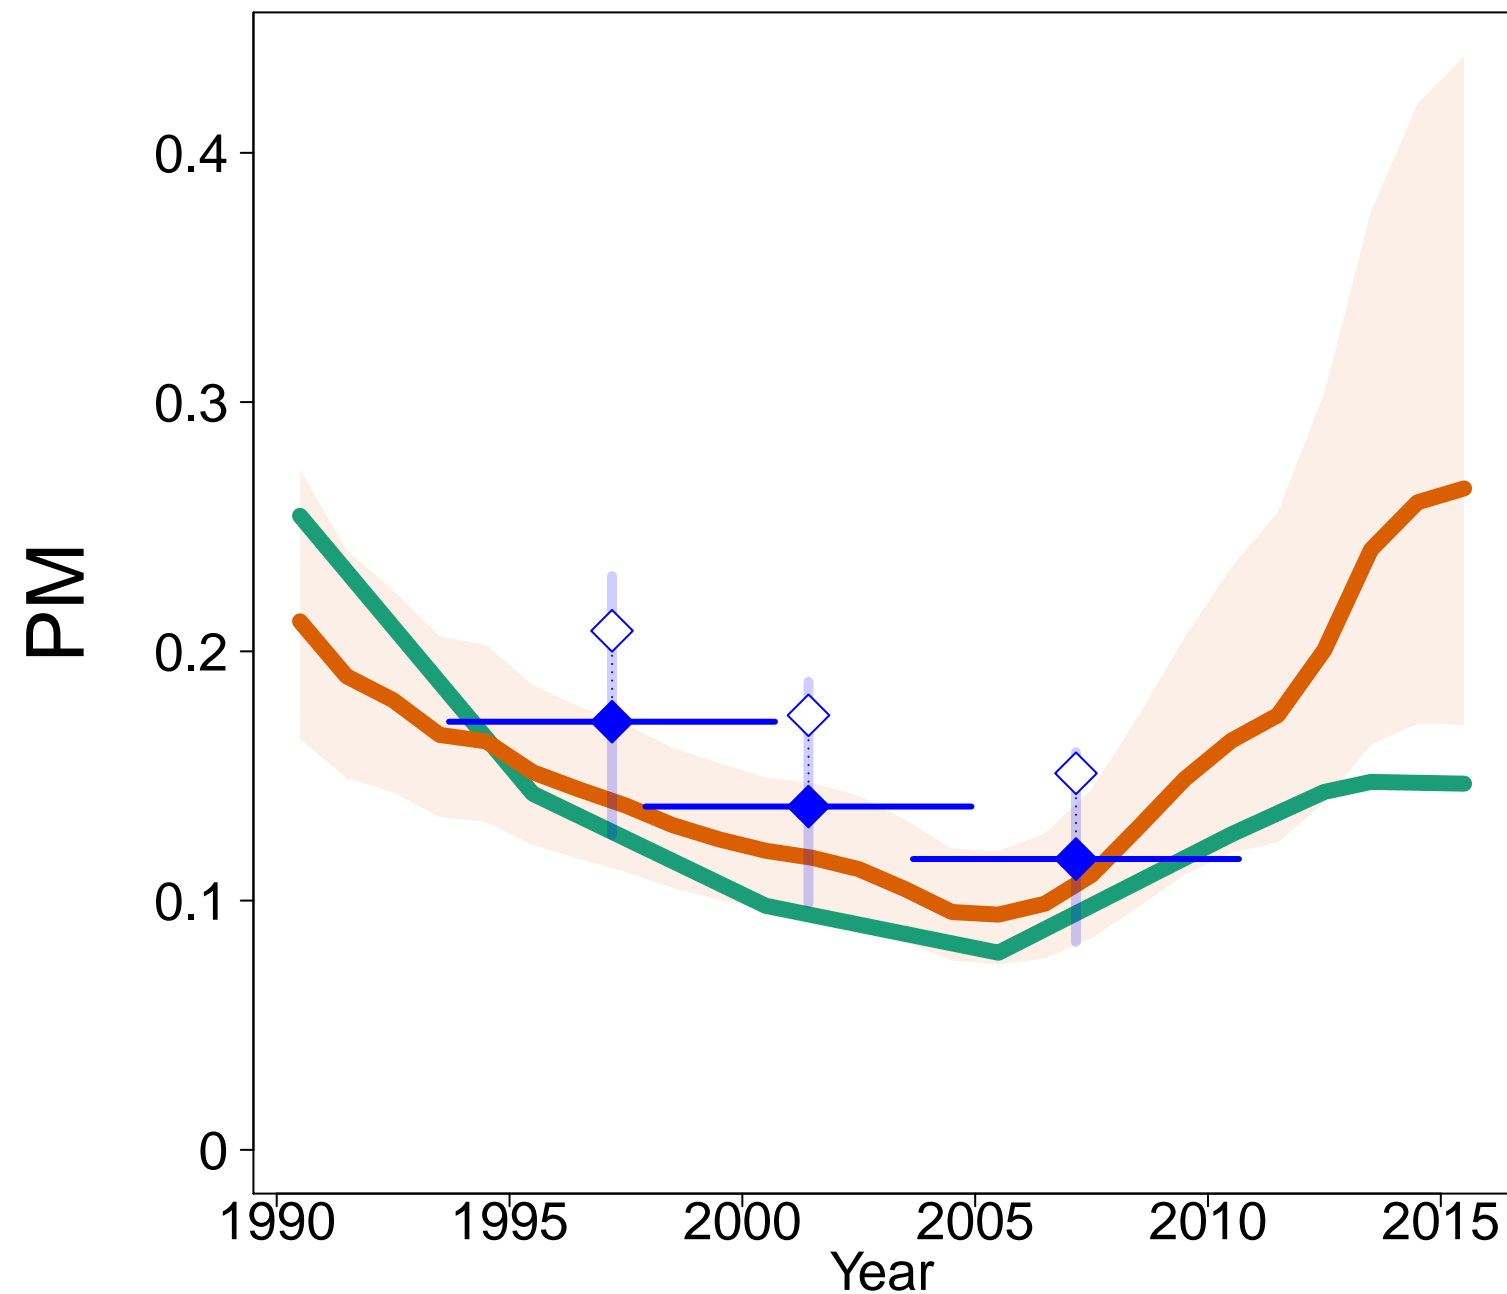

Malawi [MWI; B]  
(Eastern Africa)

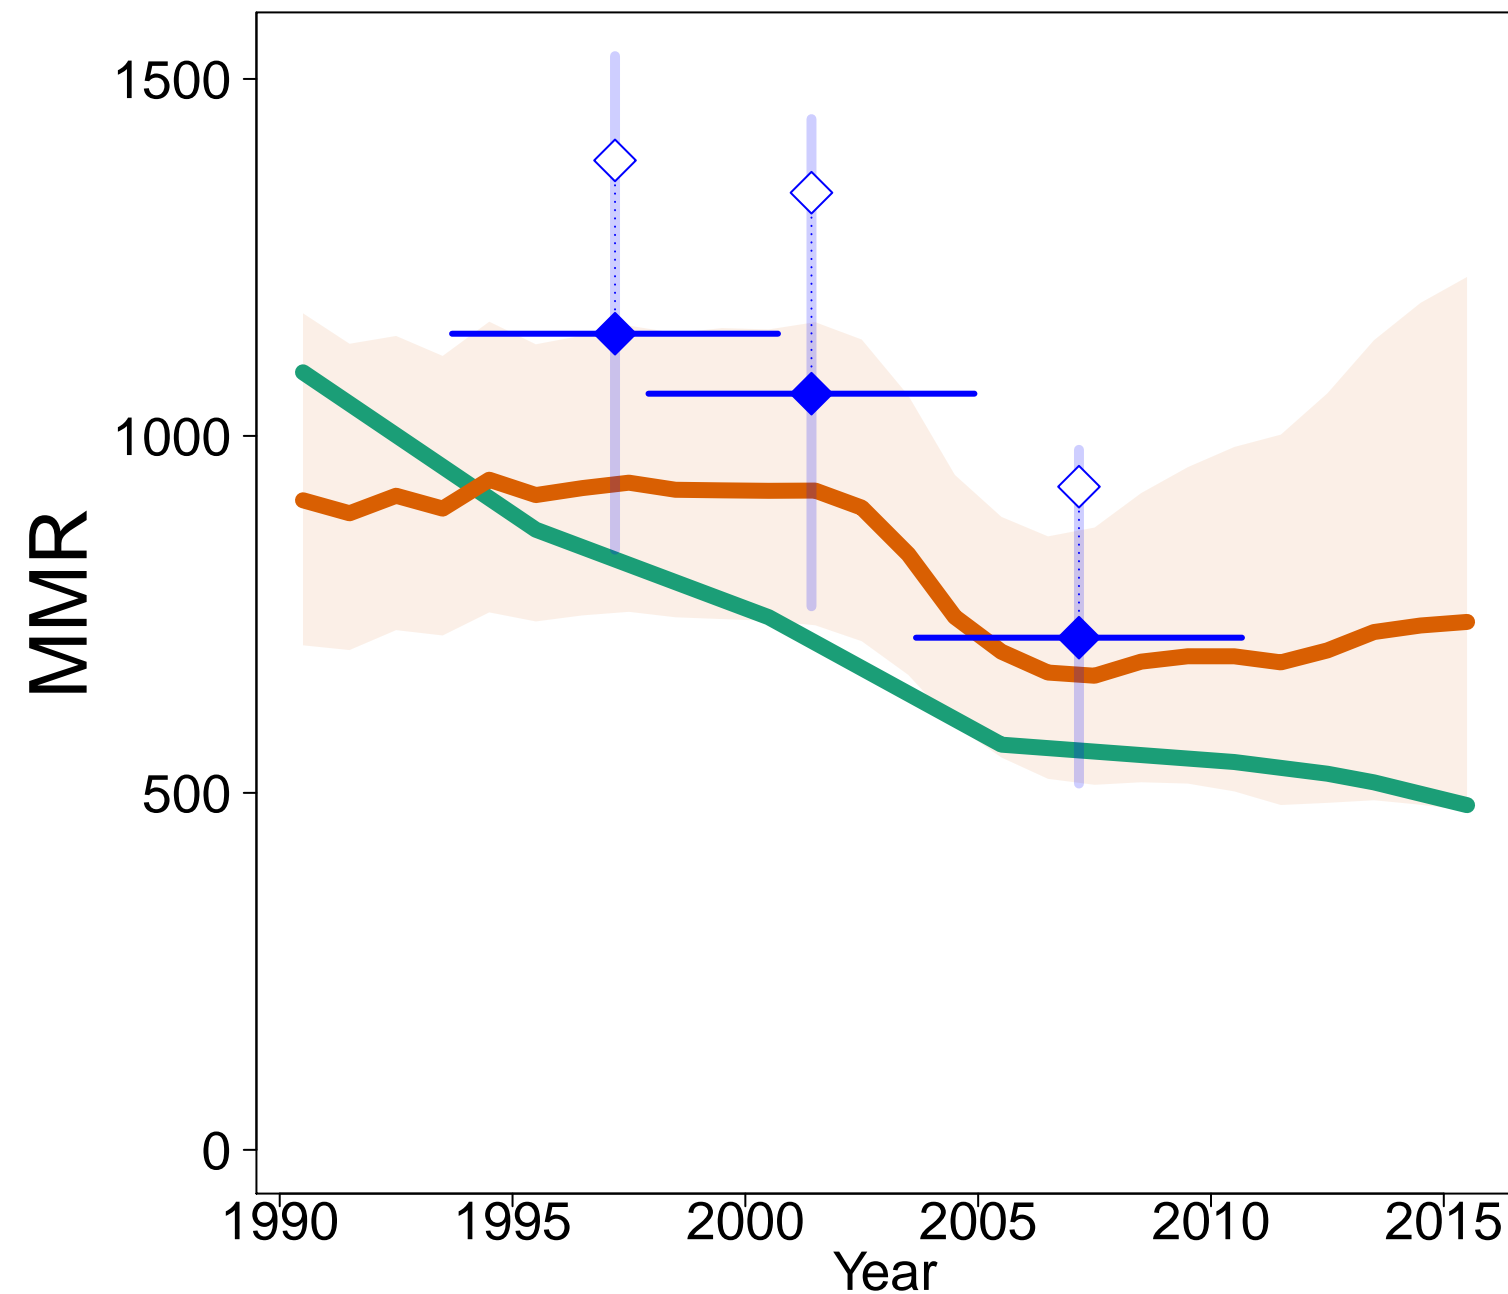

- Estimates –
- Bmat 2014
- MMEIG 2014
- Data –
- Observed Data
- Adjusted Data
- Data type –
- DHS

Malaysia [MYS; B]  
(South-Eastern Asia / Oceania)

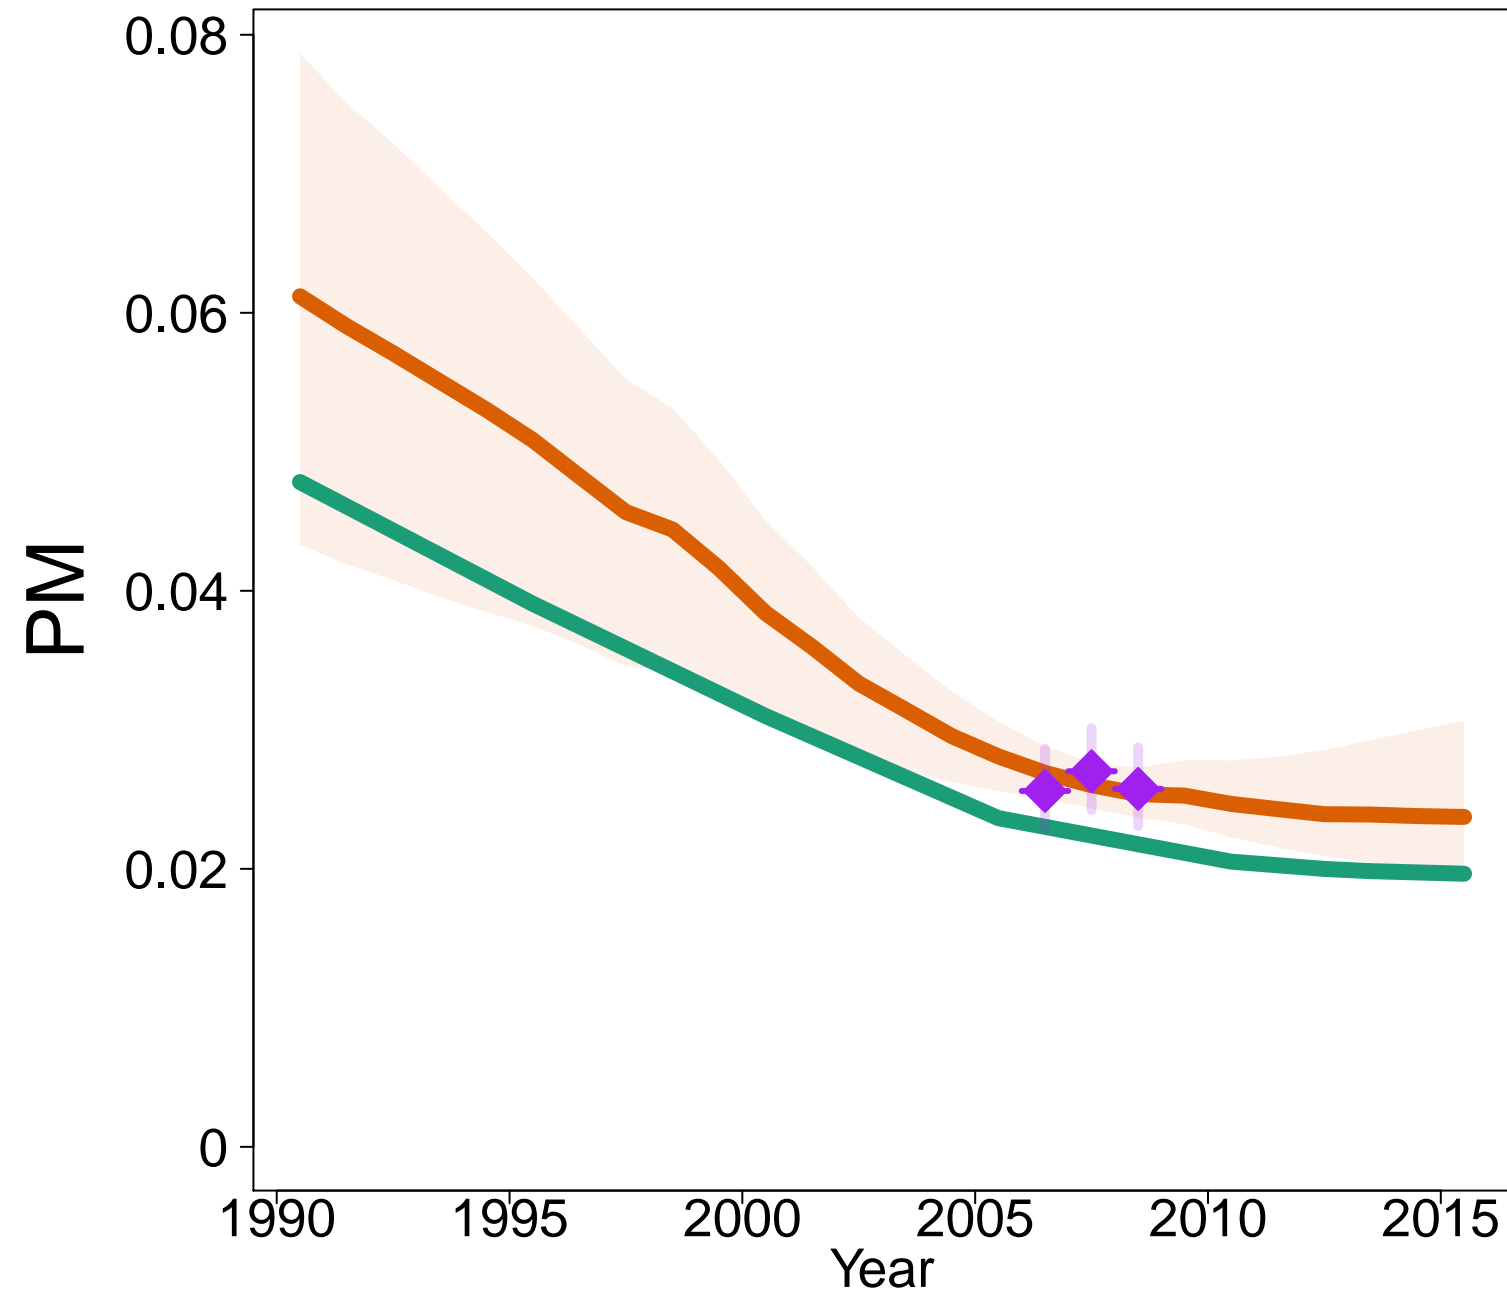

Malaysia [MYS; B]  
(South-Eastern Asia / Oceania)

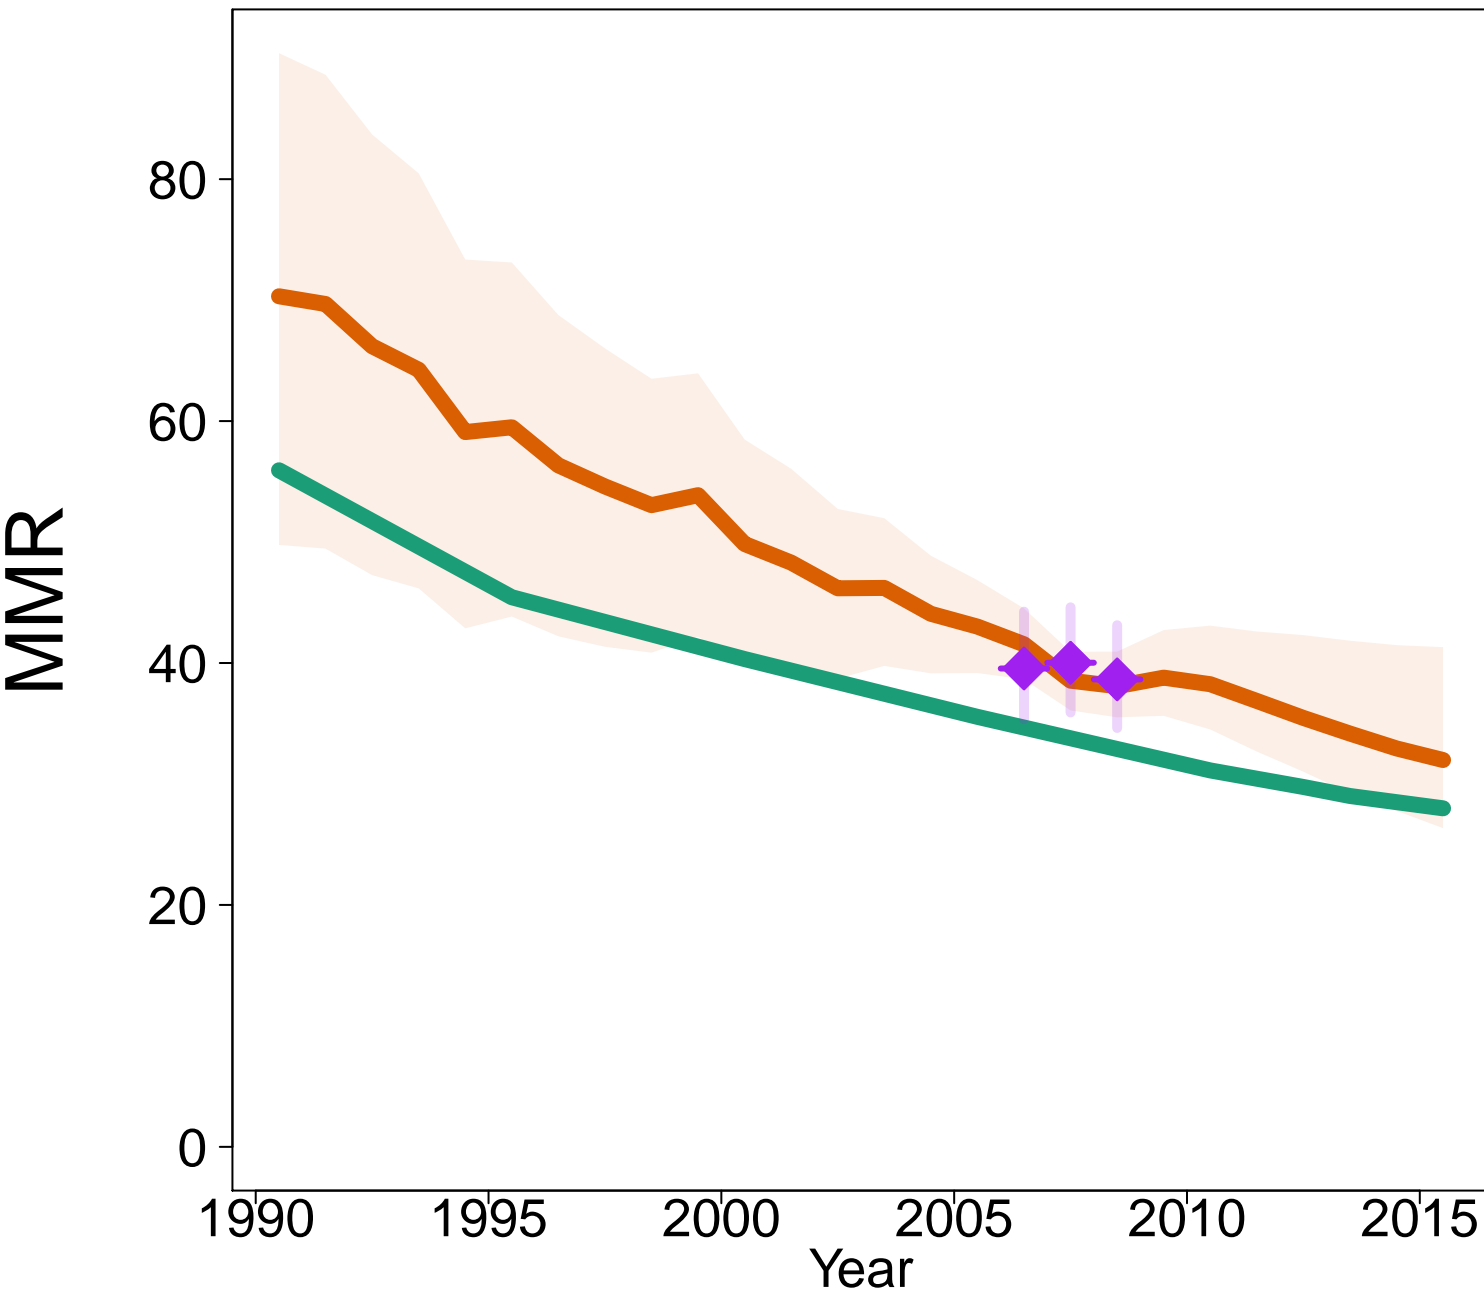

- Estimates –
- Bmat 2014
- MMEIG 2014
- Data –
- Observed Data
- Adjusted Data
- Data type –
- Spec. studies

Maldives [MDV; B]  
(Southern Asia)

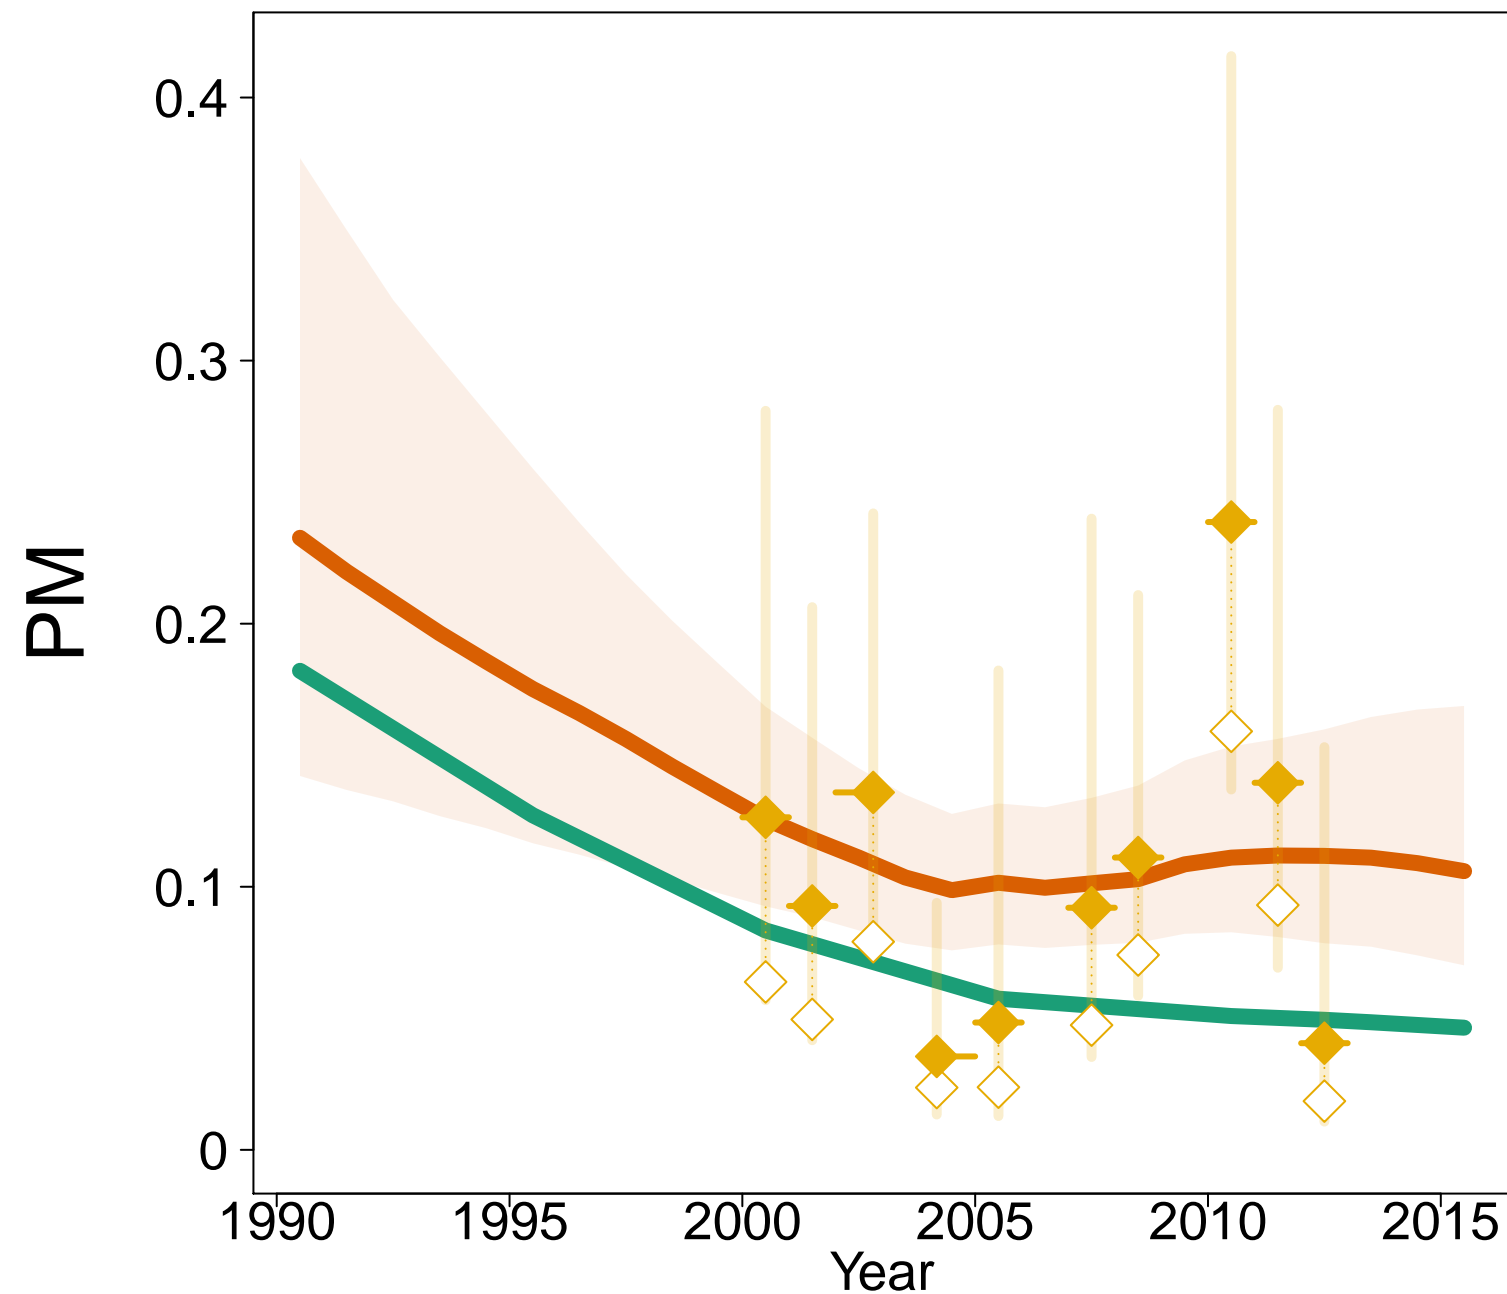

Maldives [MDV; B]  
(Southern Asia)

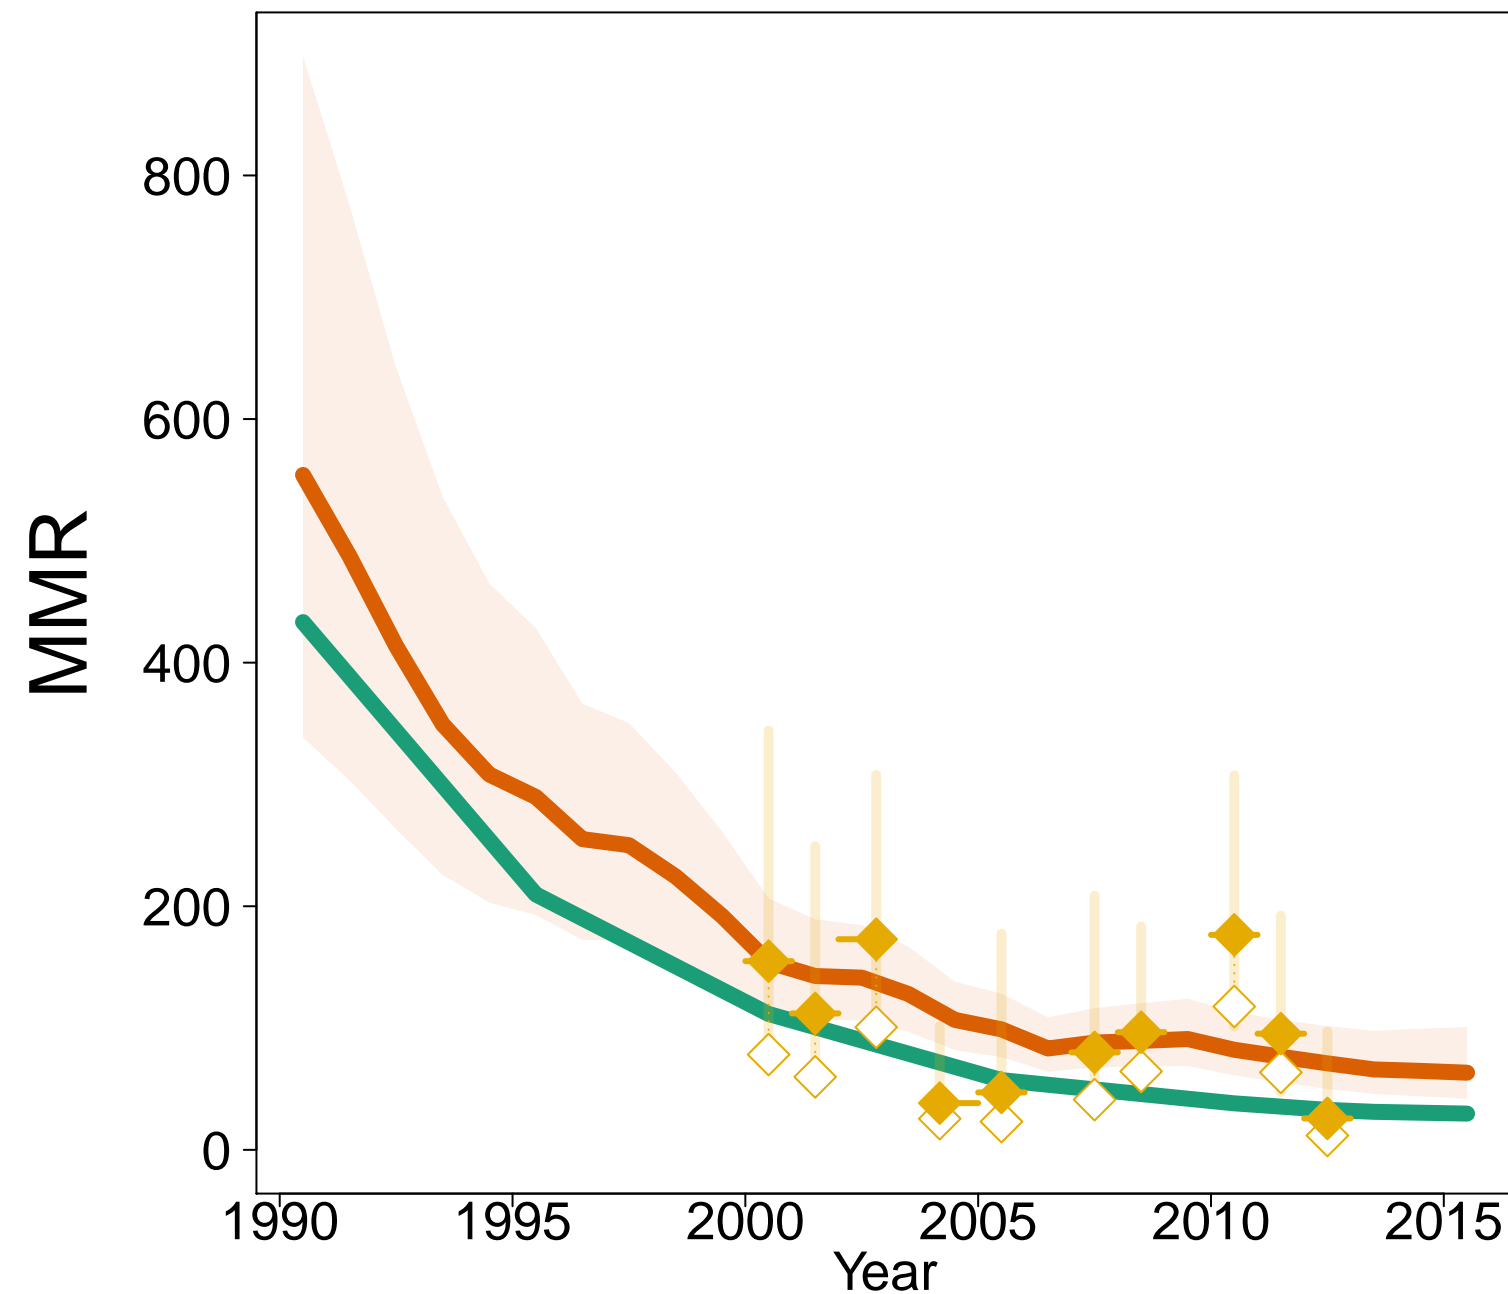

- Estimates –
- Bmat 2014
- MMEIG 2014
- Data –
- Observed Data
- Adjusted Data
- Data type –
- VR

Mali [MLI; B]  
(Western Africa)

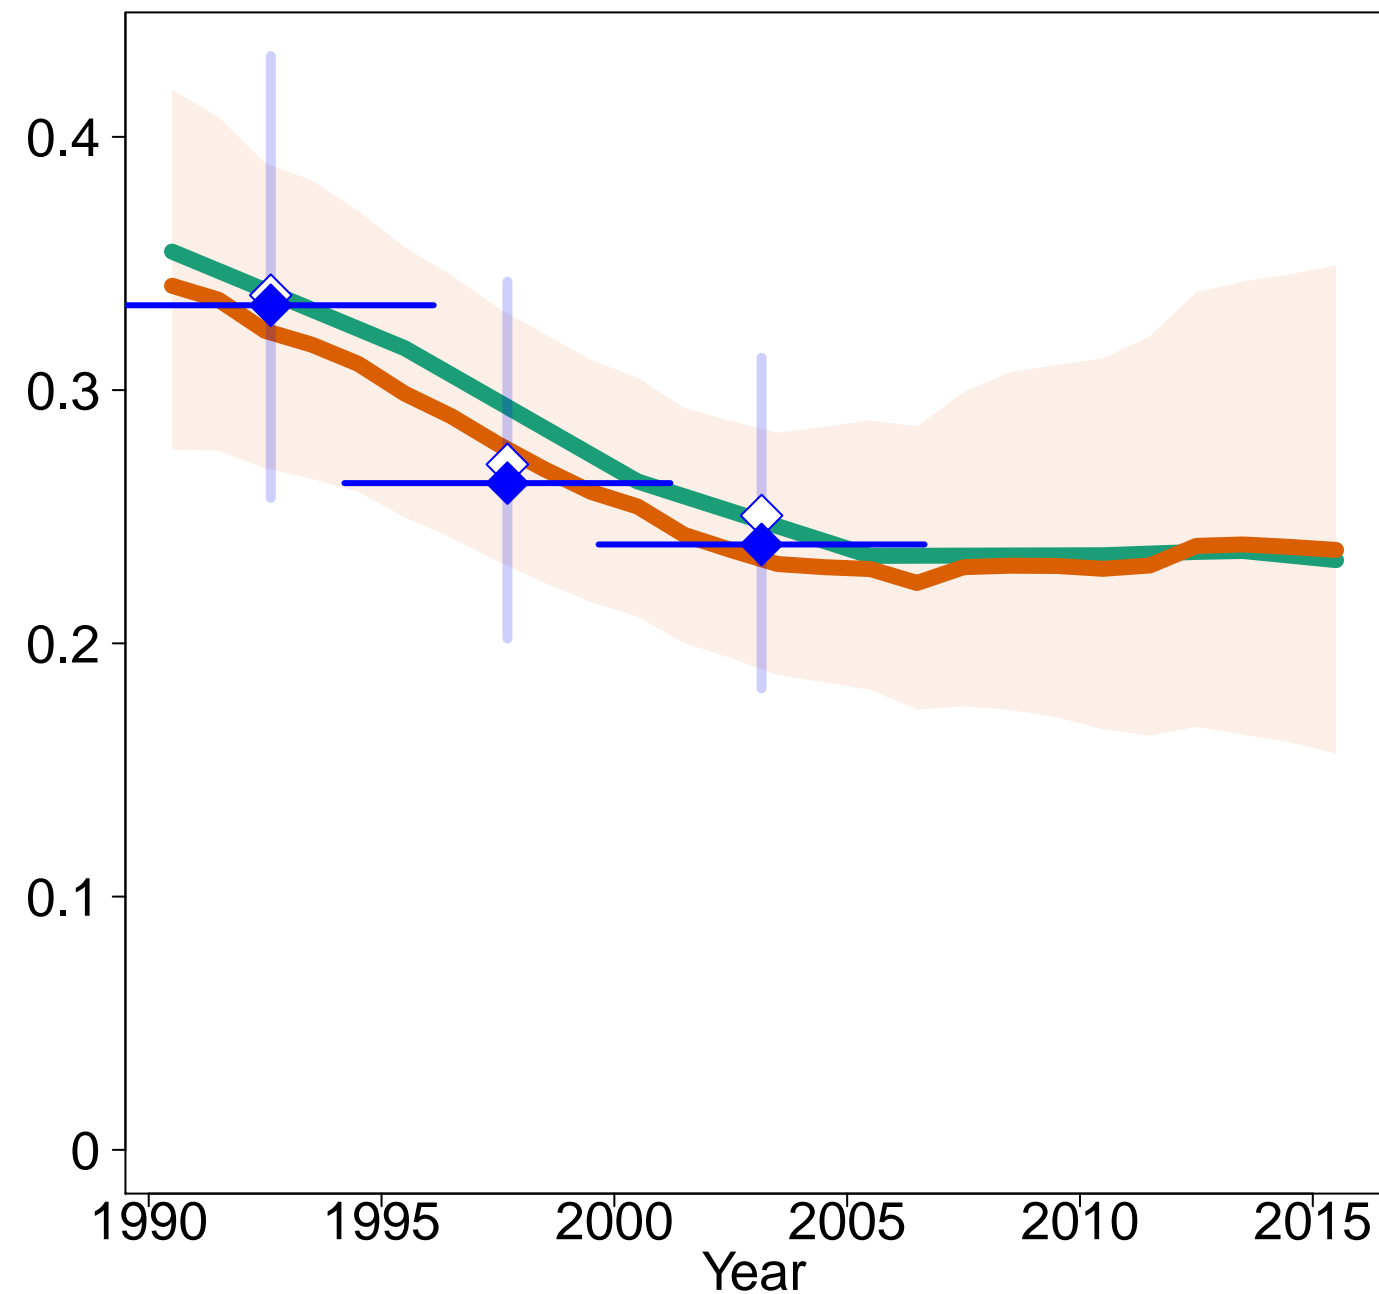

Mali [MLI; B]  
(Western Africa)

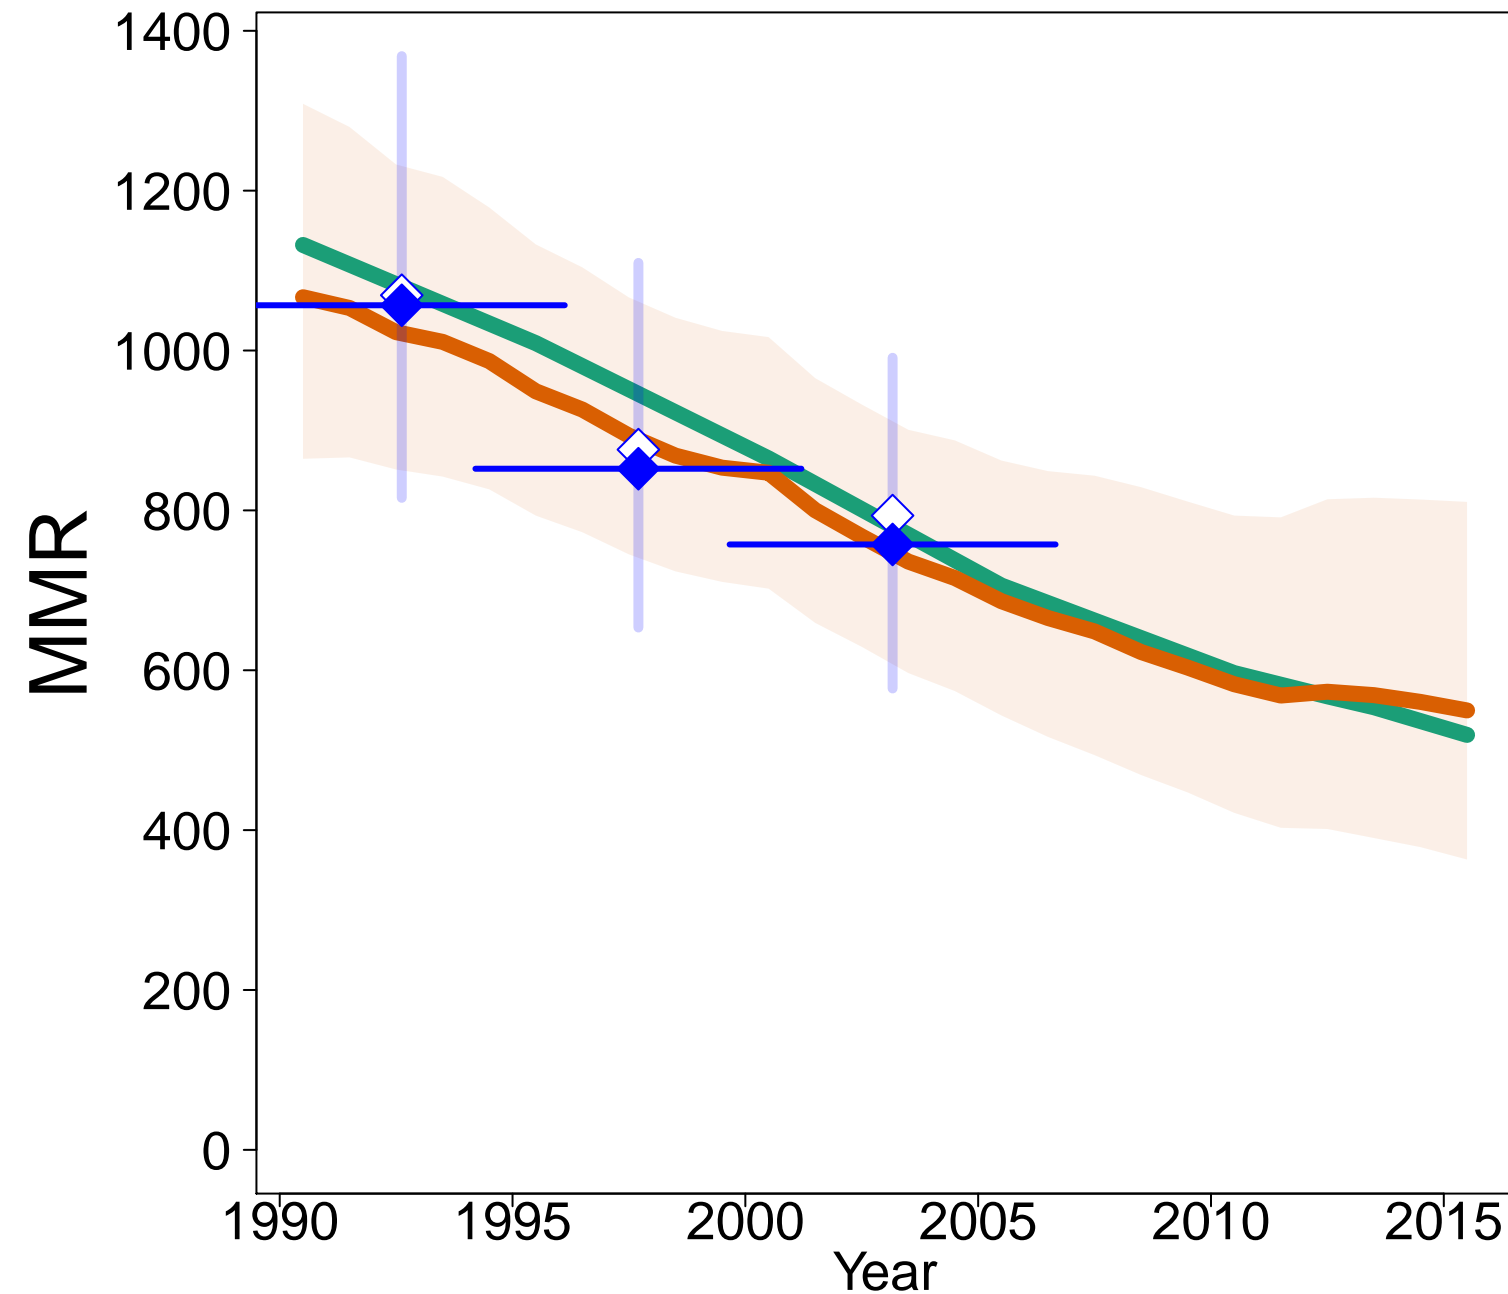

– Estimates –  
Bmat 2014  
MMEIG 2014  
– Data –  
Observed Data  
Adjusted Data  
– Data type –  
DHS

Malta [MLT; A]  
(Developed regions)

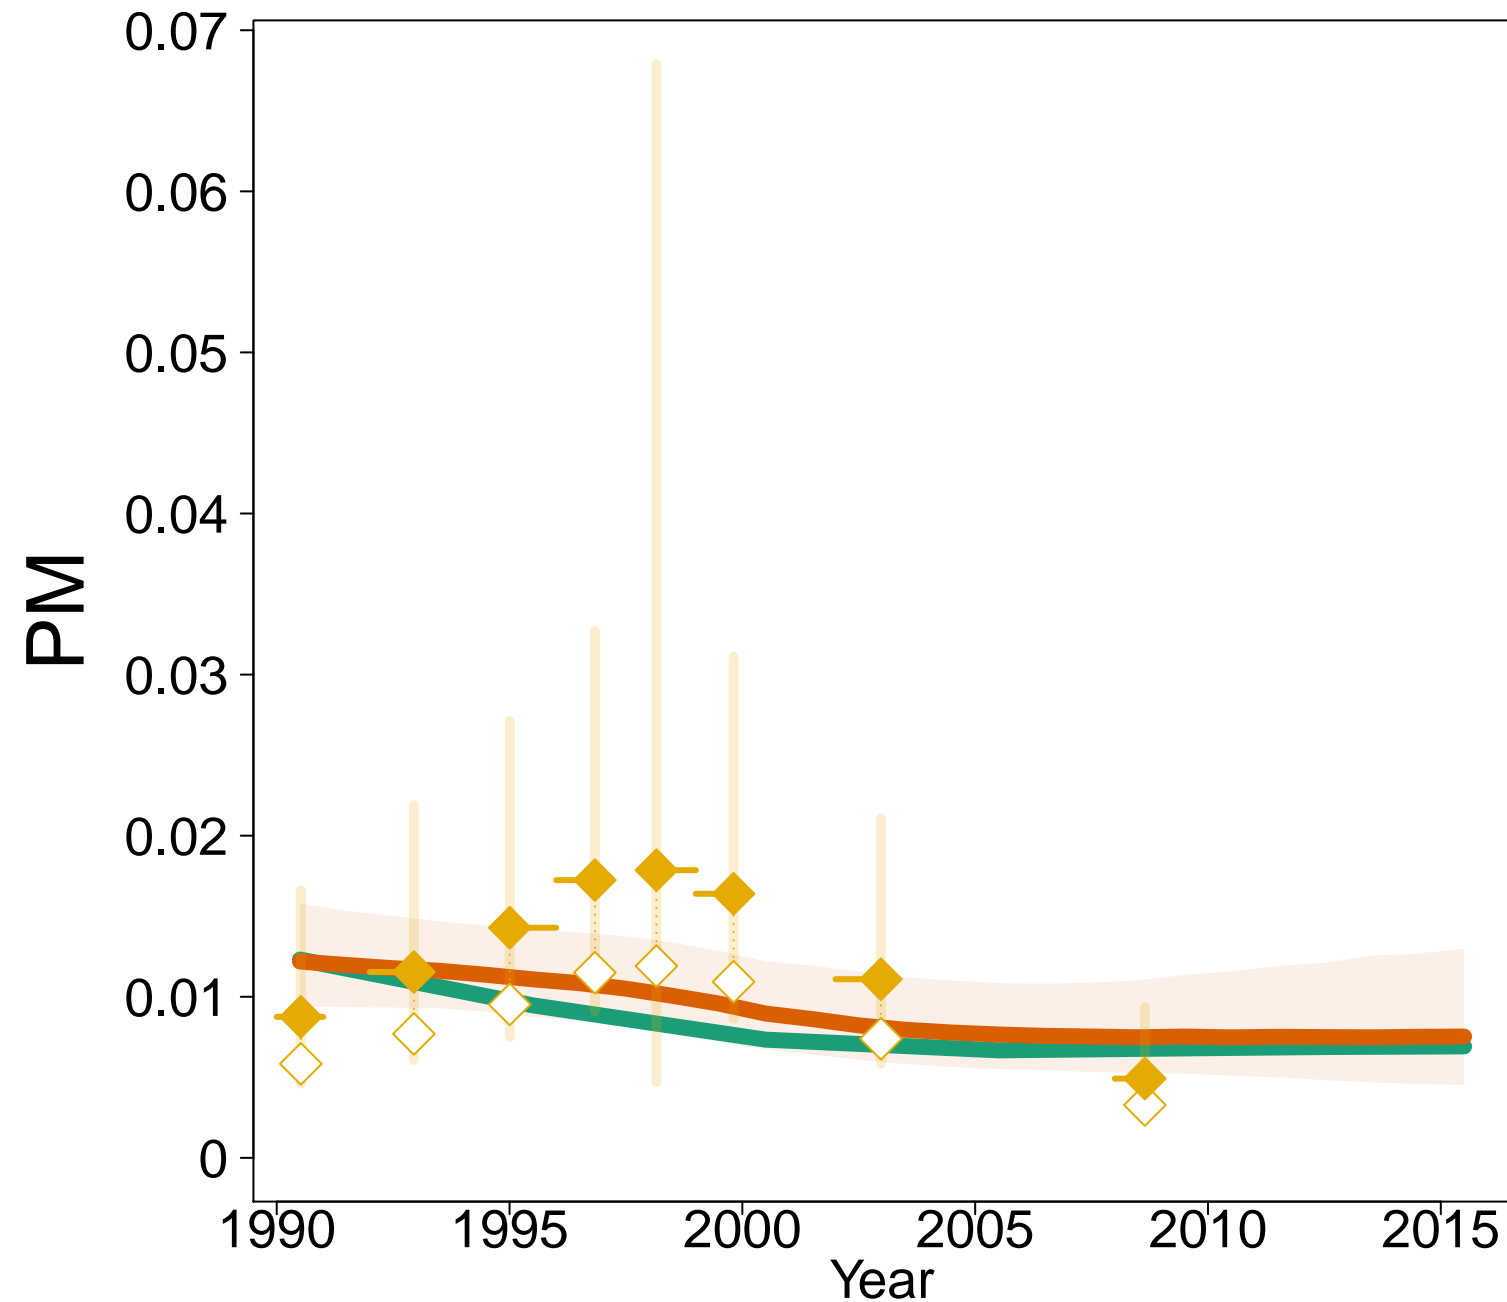

Malta [MLT; A]  
(Developed regions)

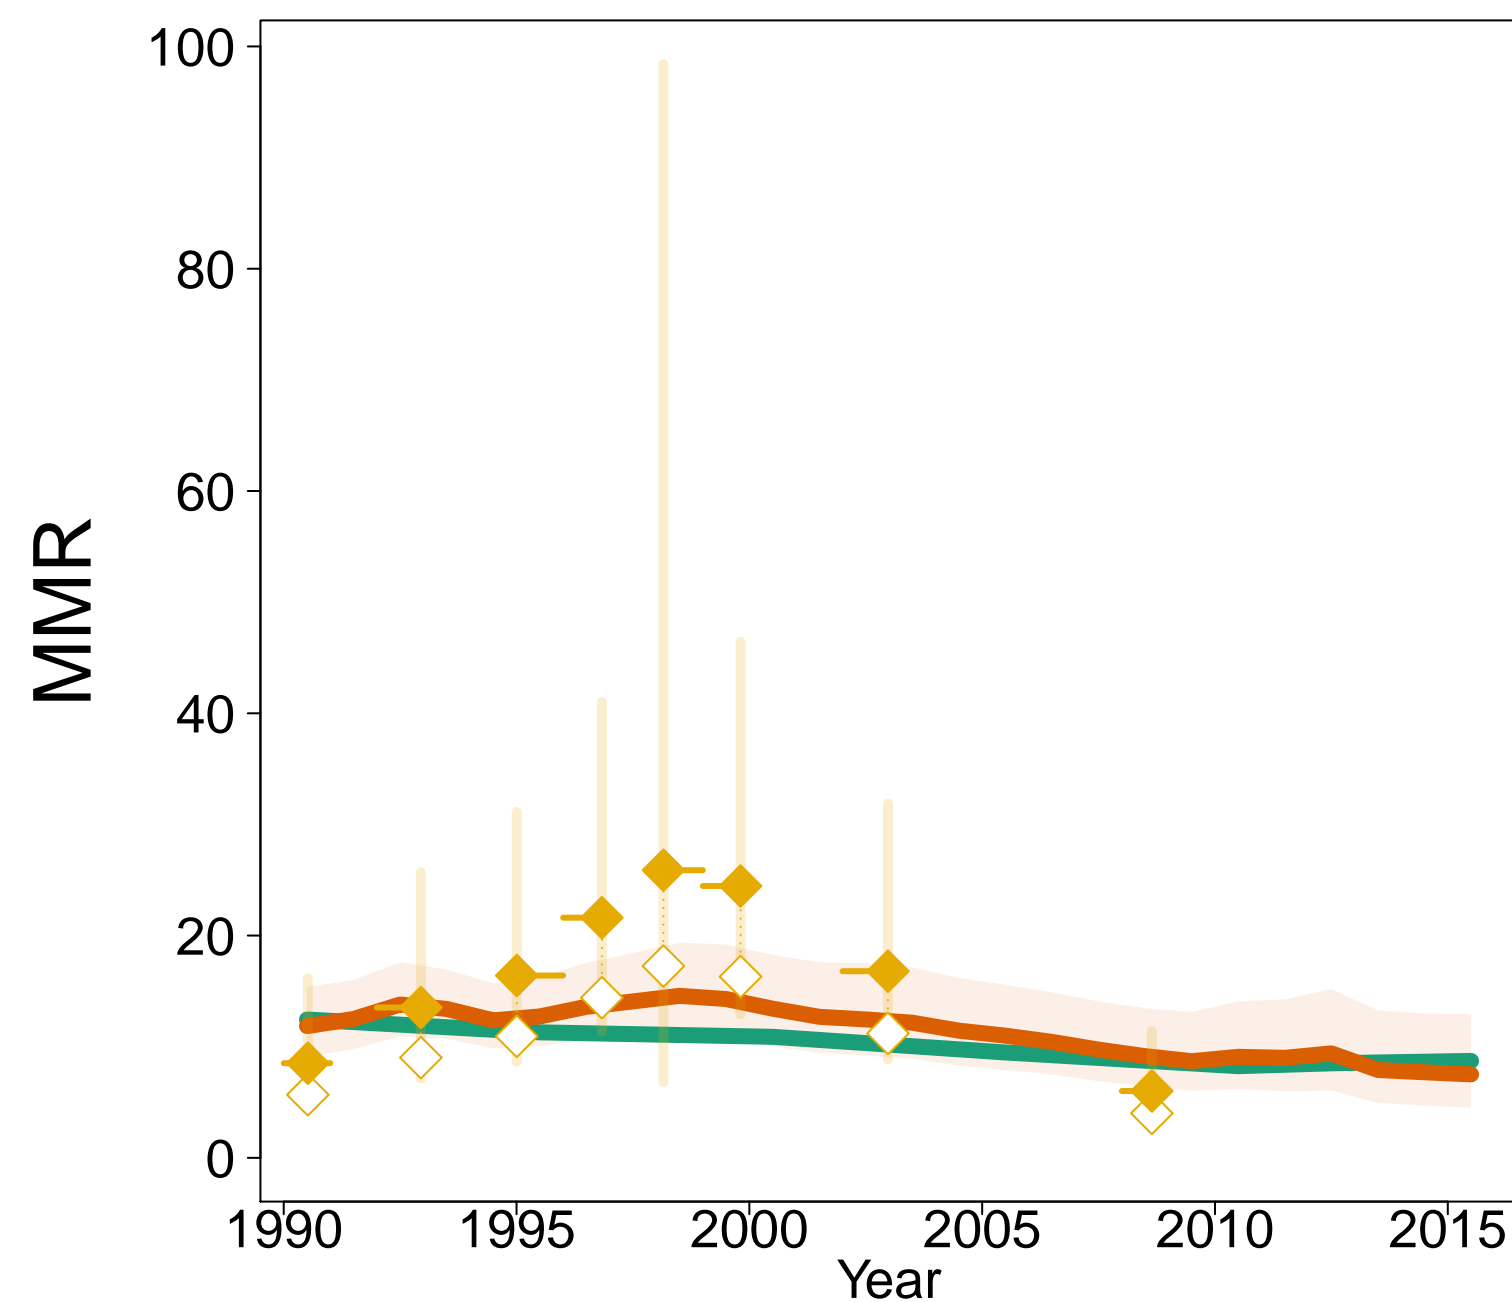

- Estimates –
- Bmat 2014
- MMEIG 2014
- Data –
- Observed Data
- Adjusted Data
- Data type –
- VR

Mauritania [MRT; B]  
(Western Africa)

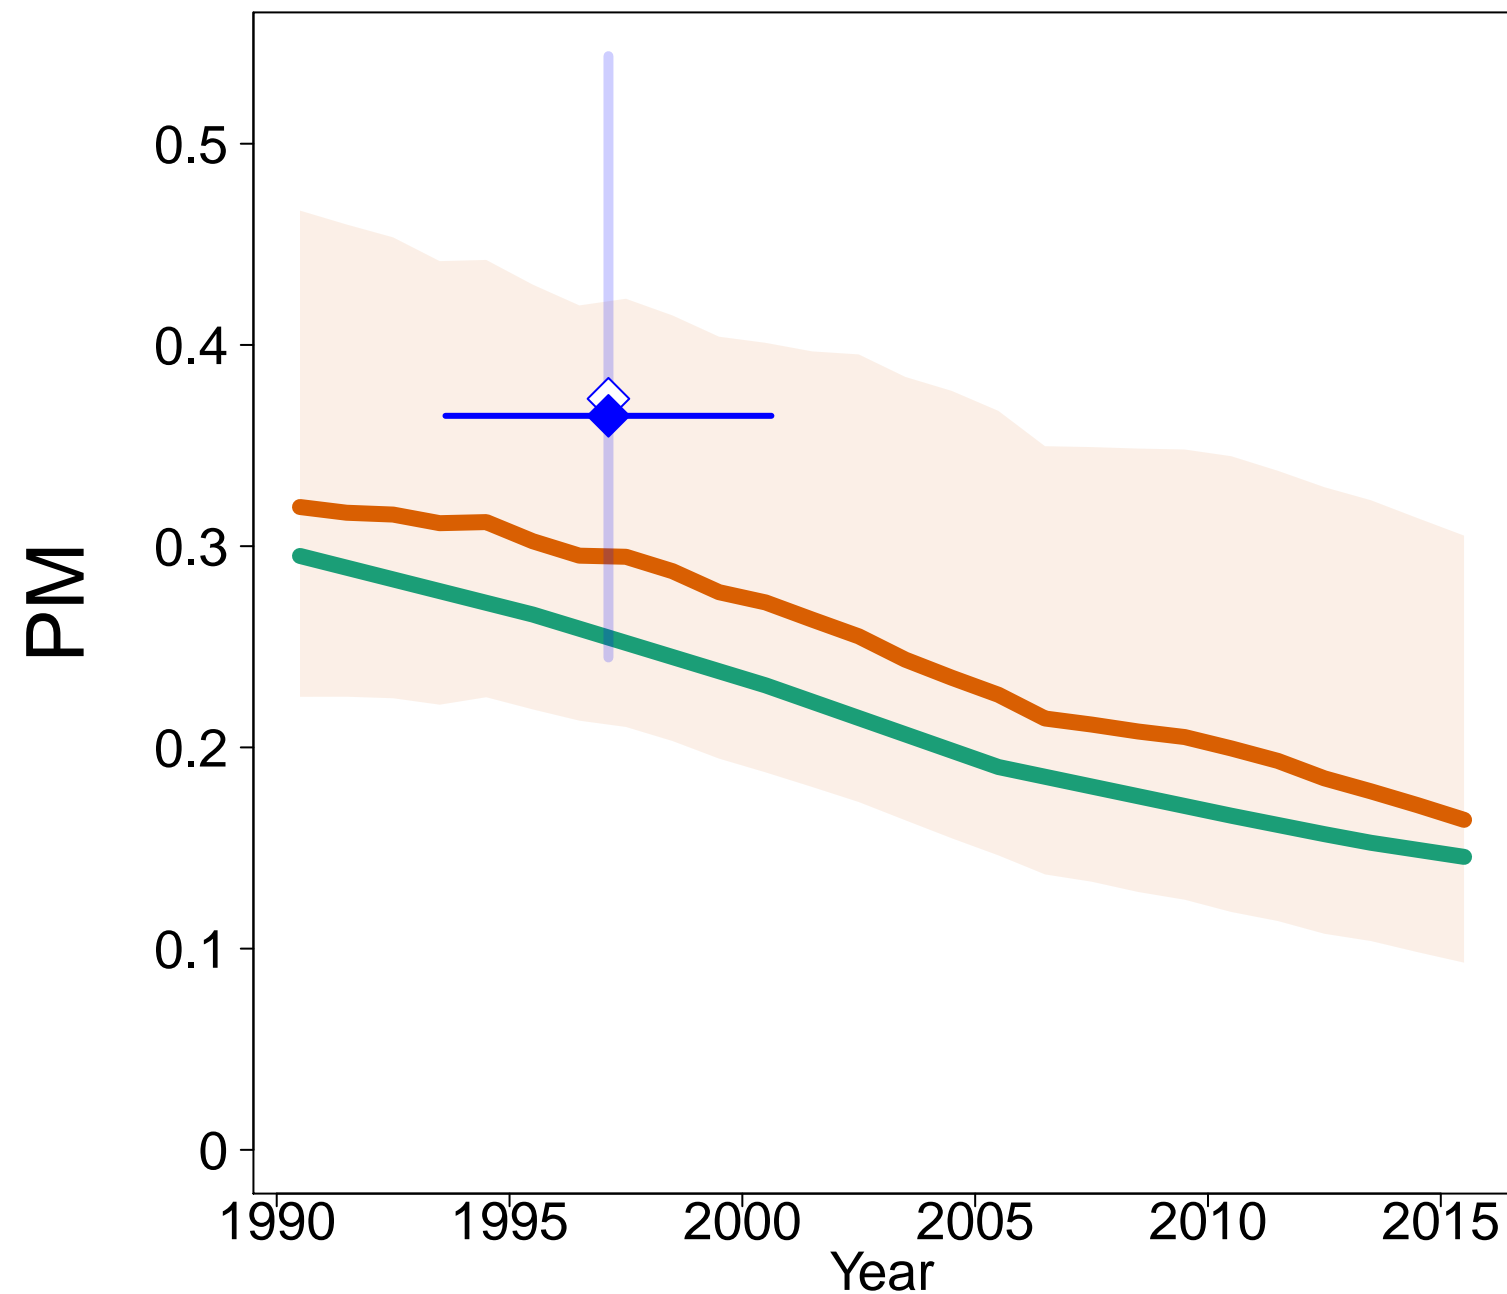

Mauritania [MRT; B]  
(Western Africa)

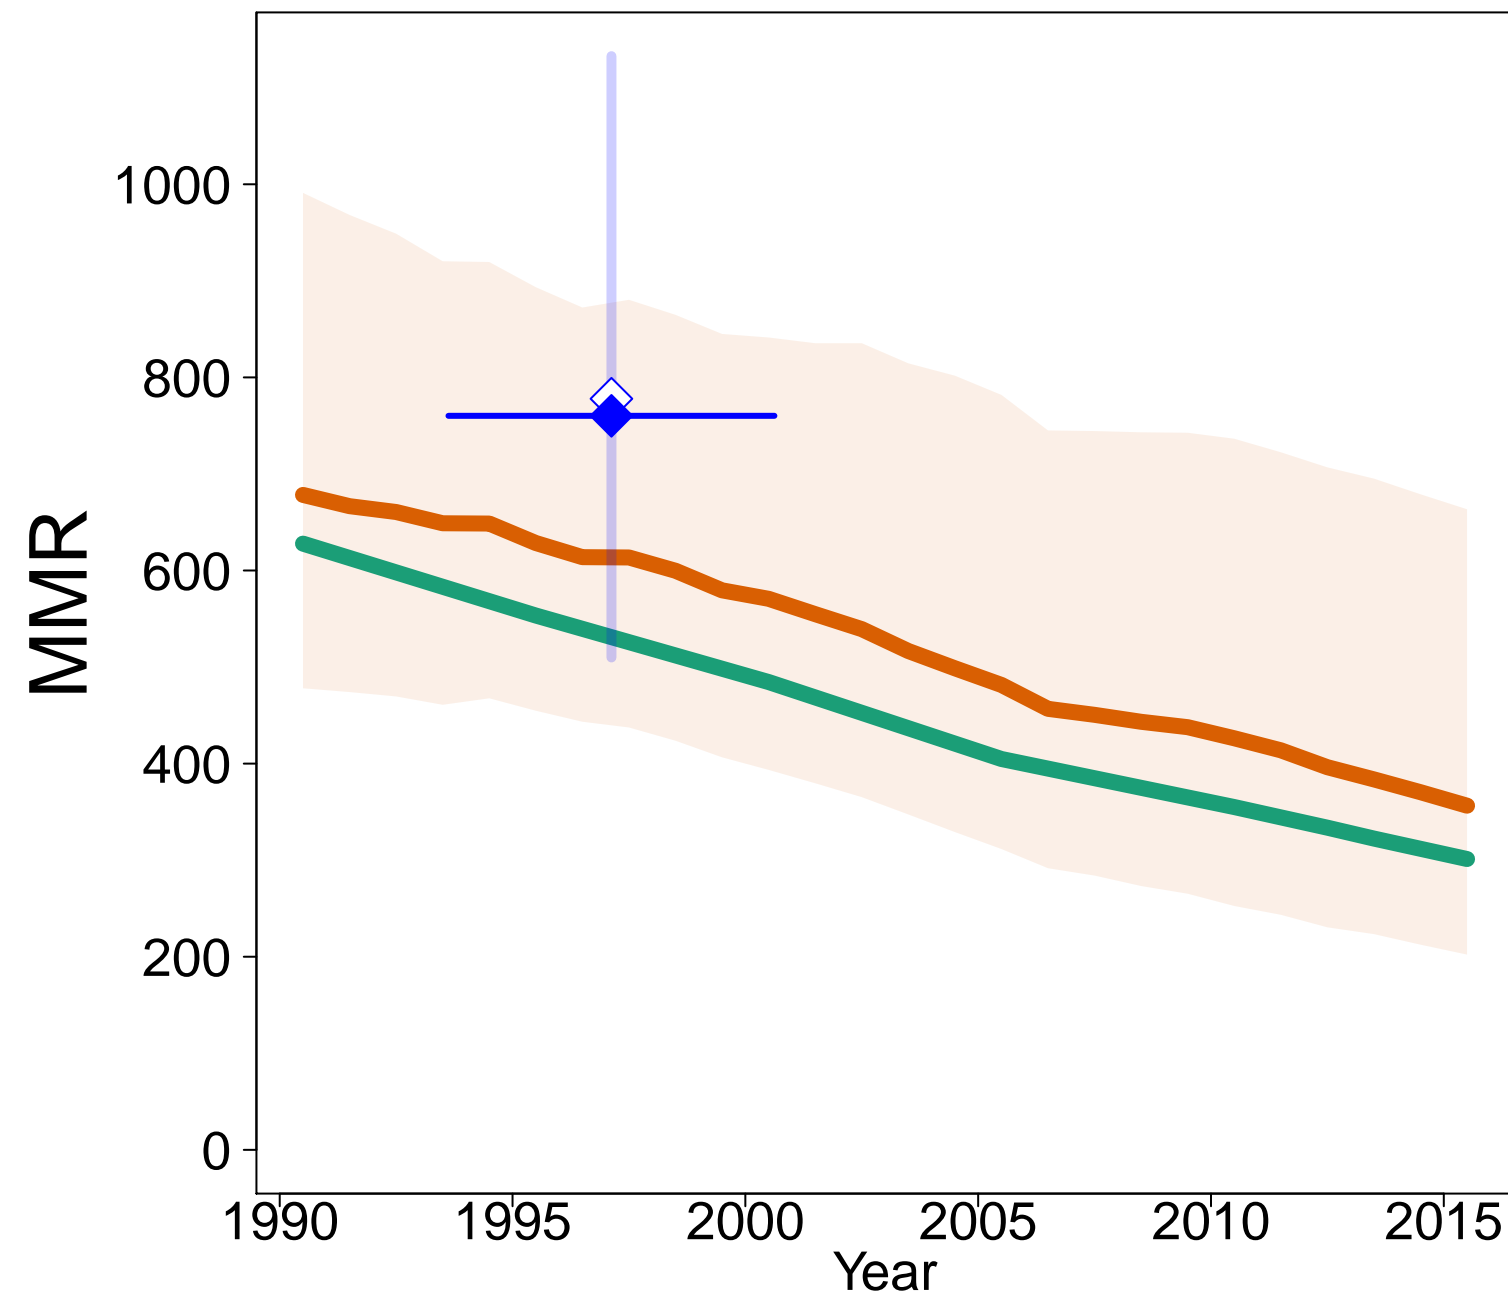

- Estimates –
- Bmat 2014
- MMEIG 2014
- Data –
- Observed Data
- Adjusted Data
- Data type –
- DHS

Mauritius [MUS; A]  
(Eastern Africa)

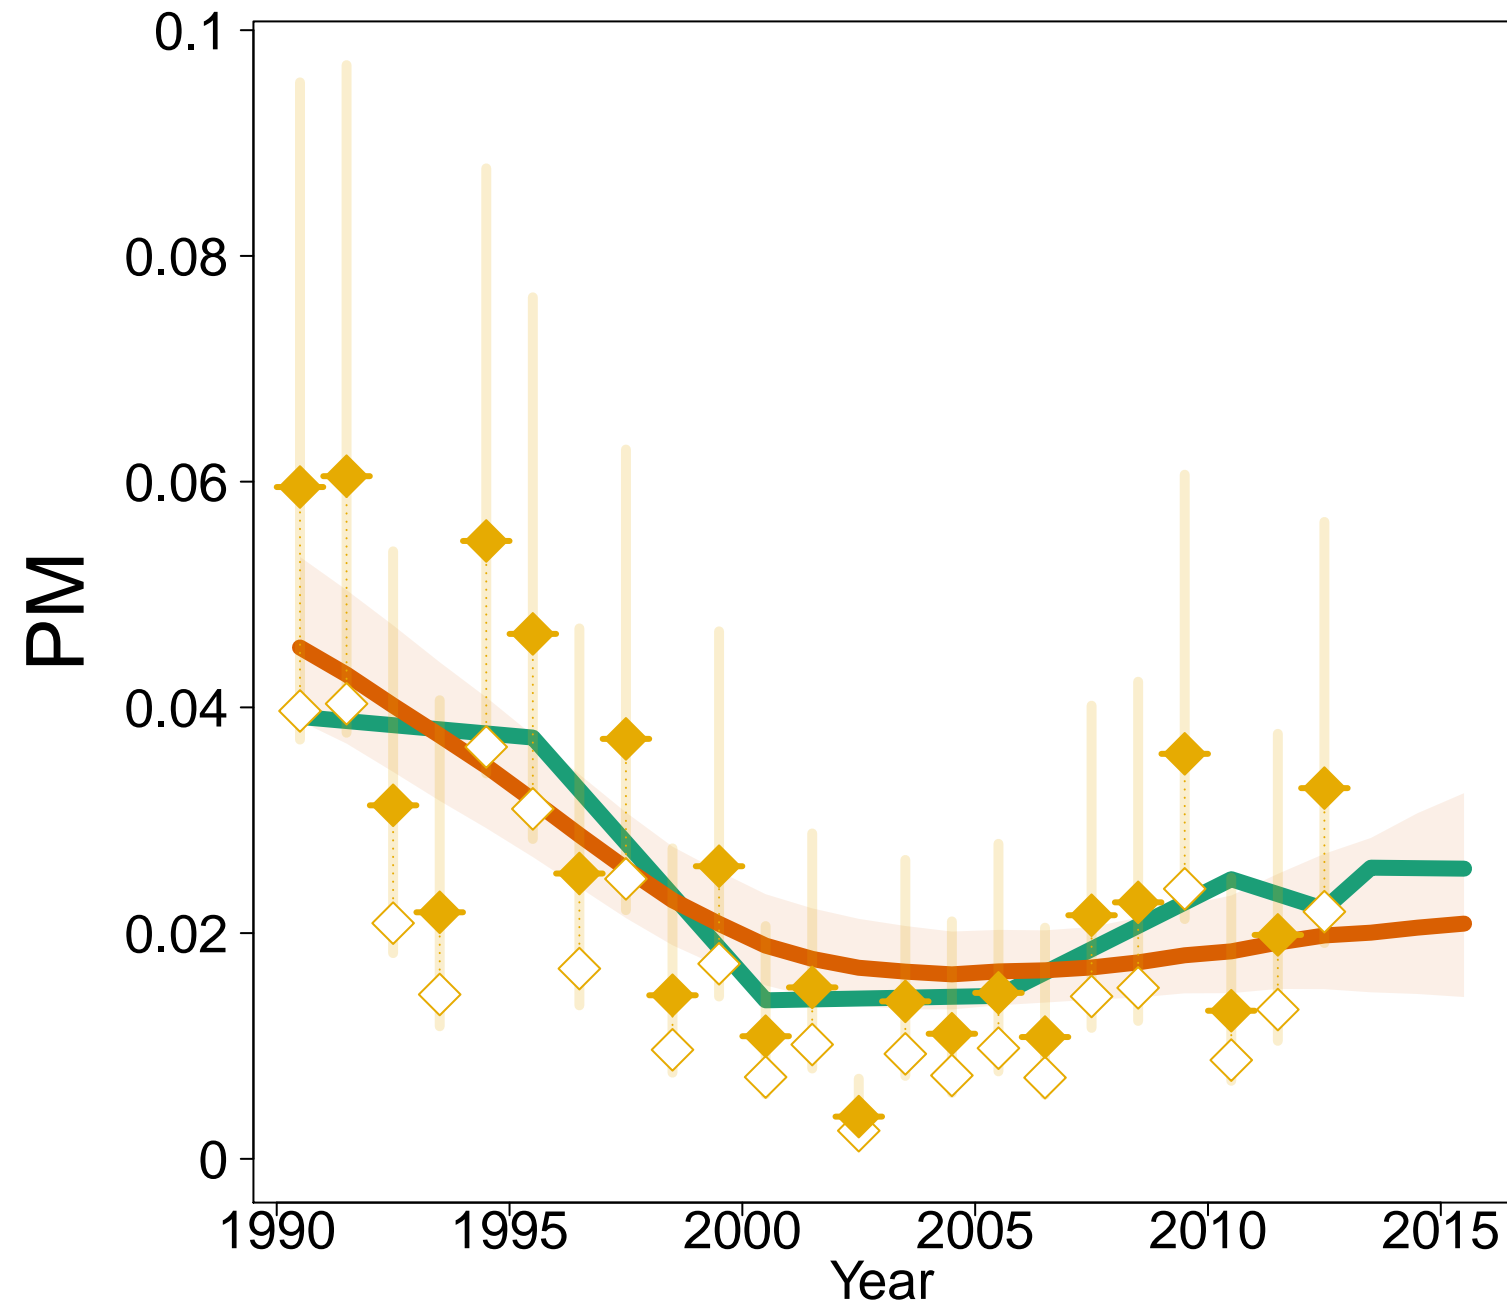

Mauritius [MUS; A]  
(Eastern Africa)

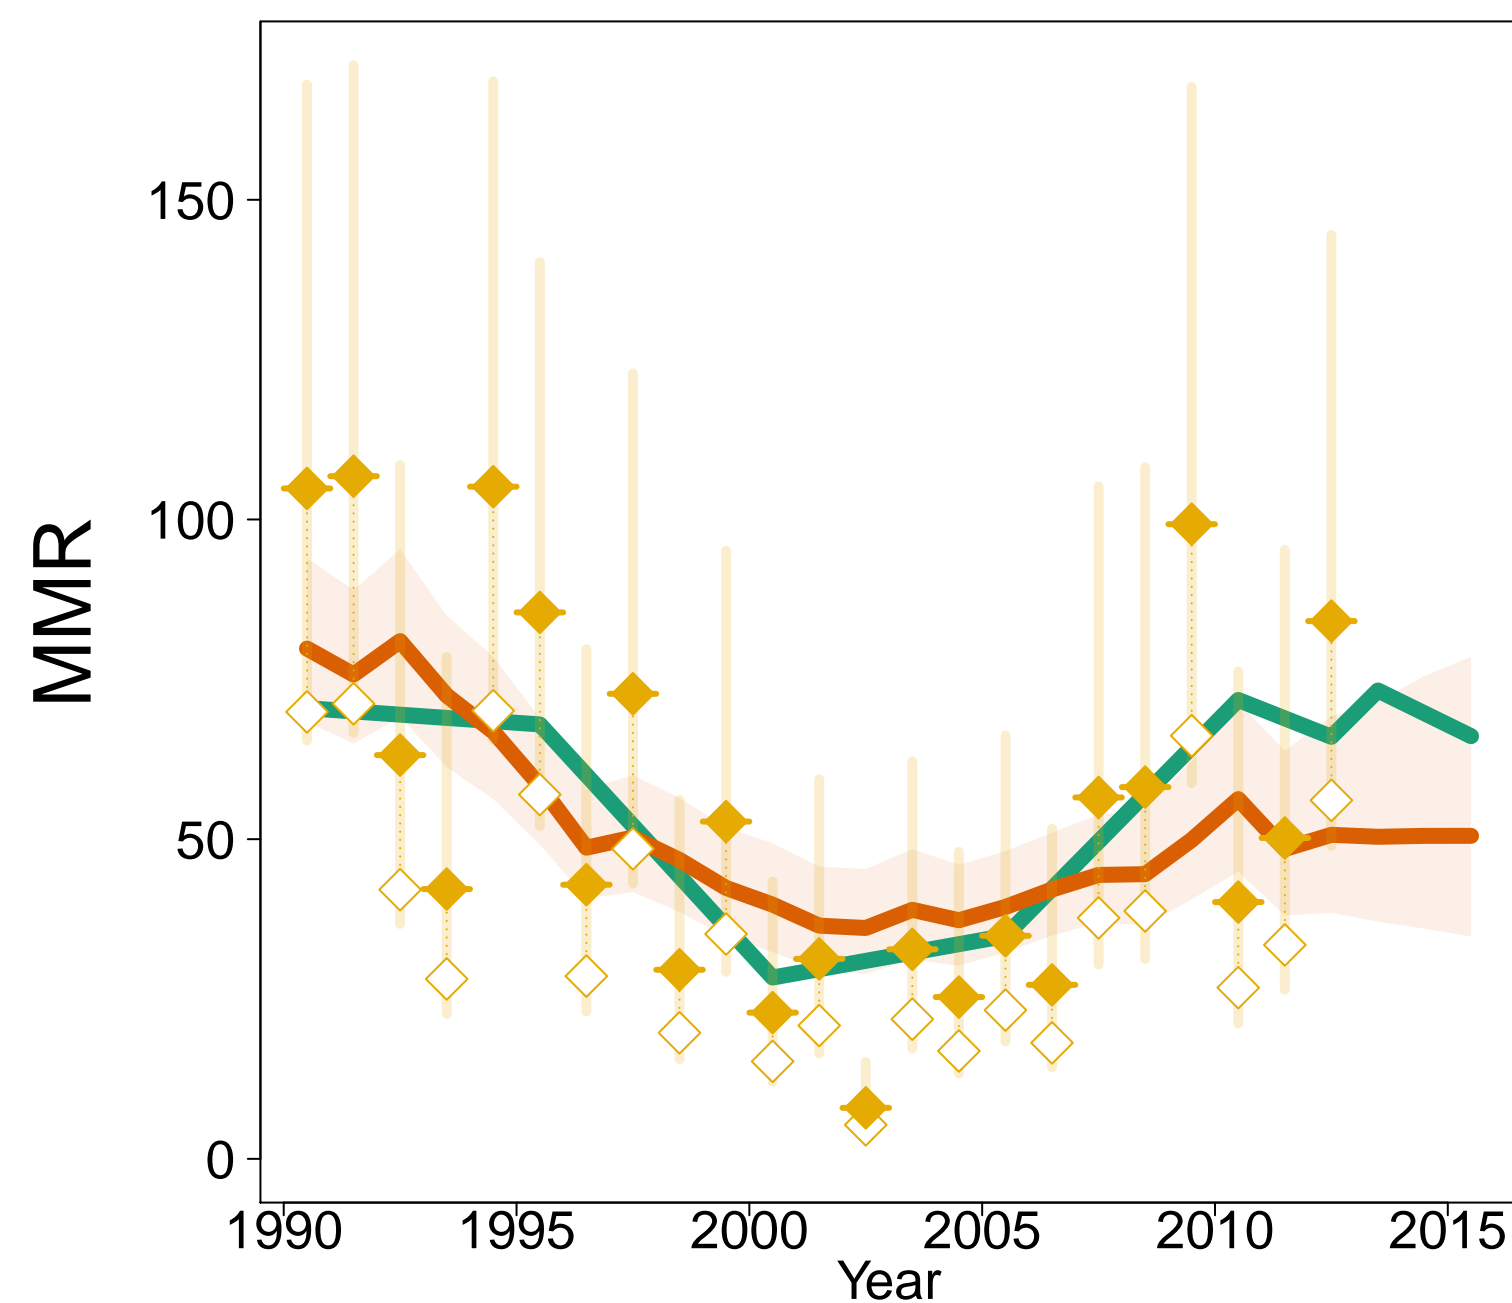



Mexico [MEX; A]  
(Central America)

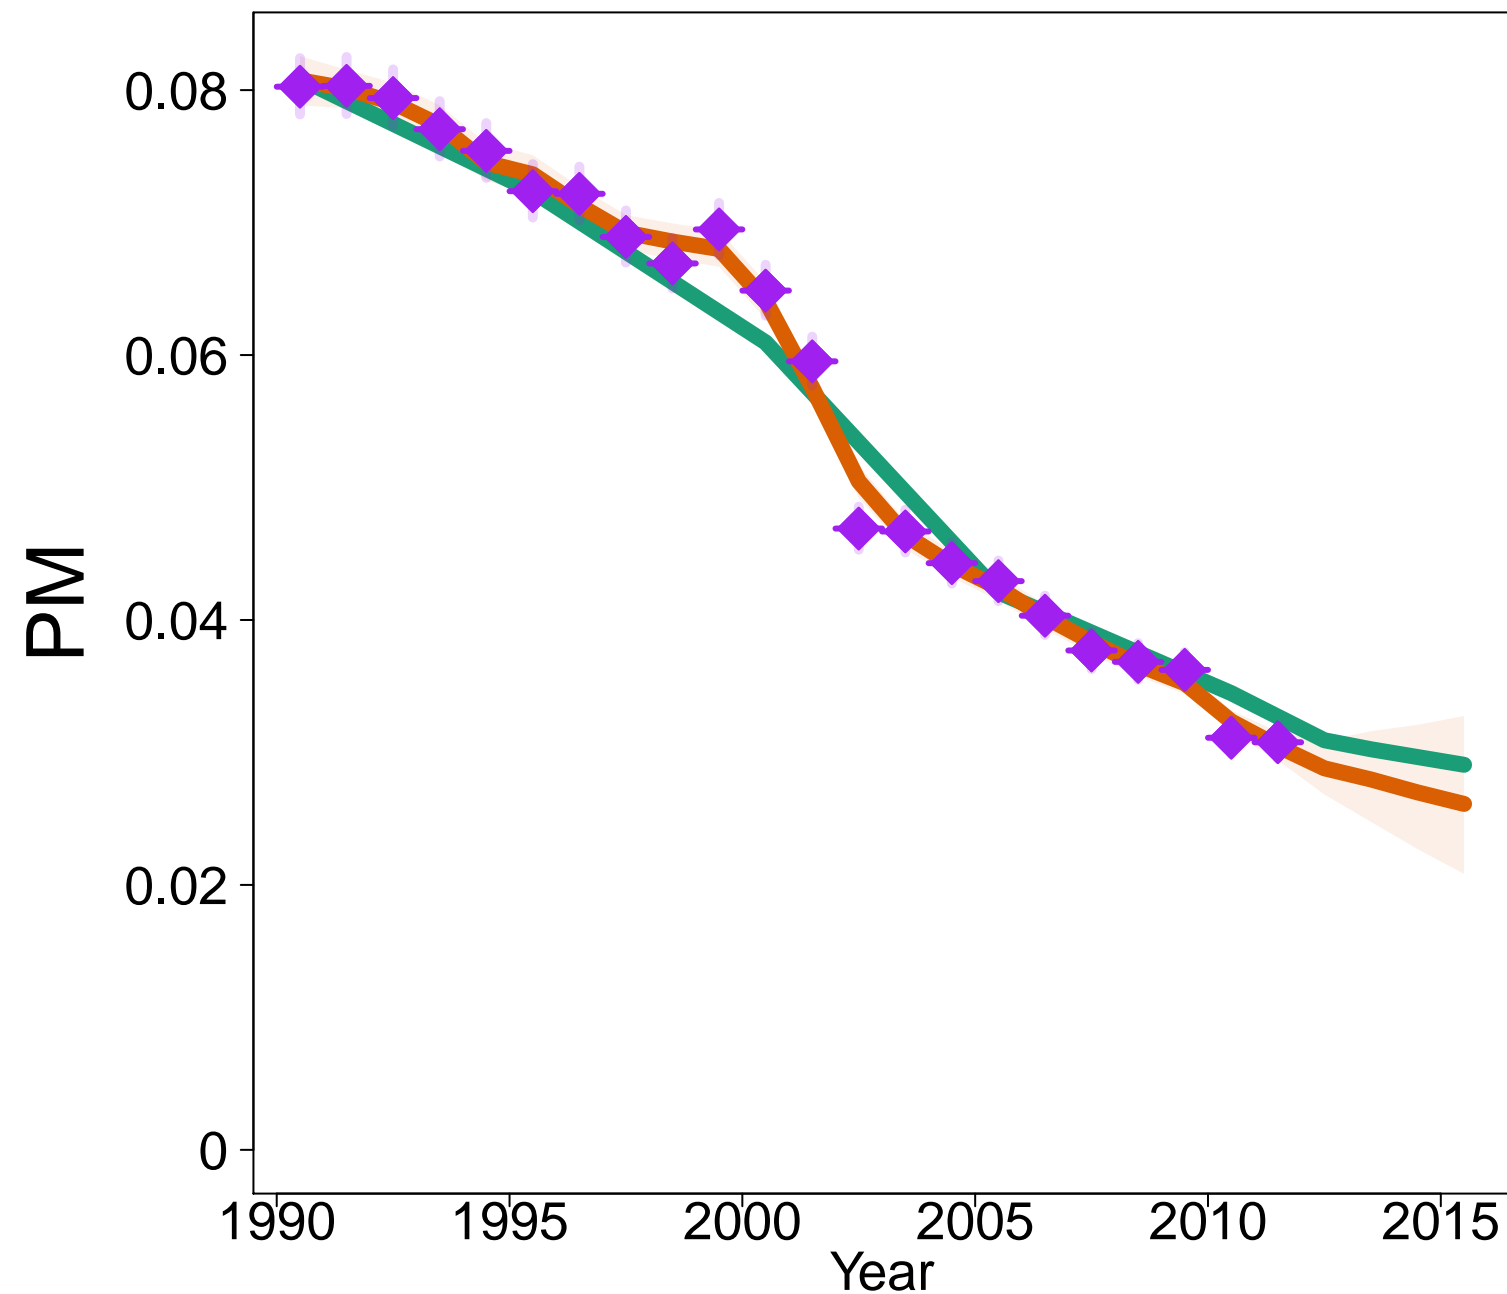

Mexico [MEX; A]  
(Central America)

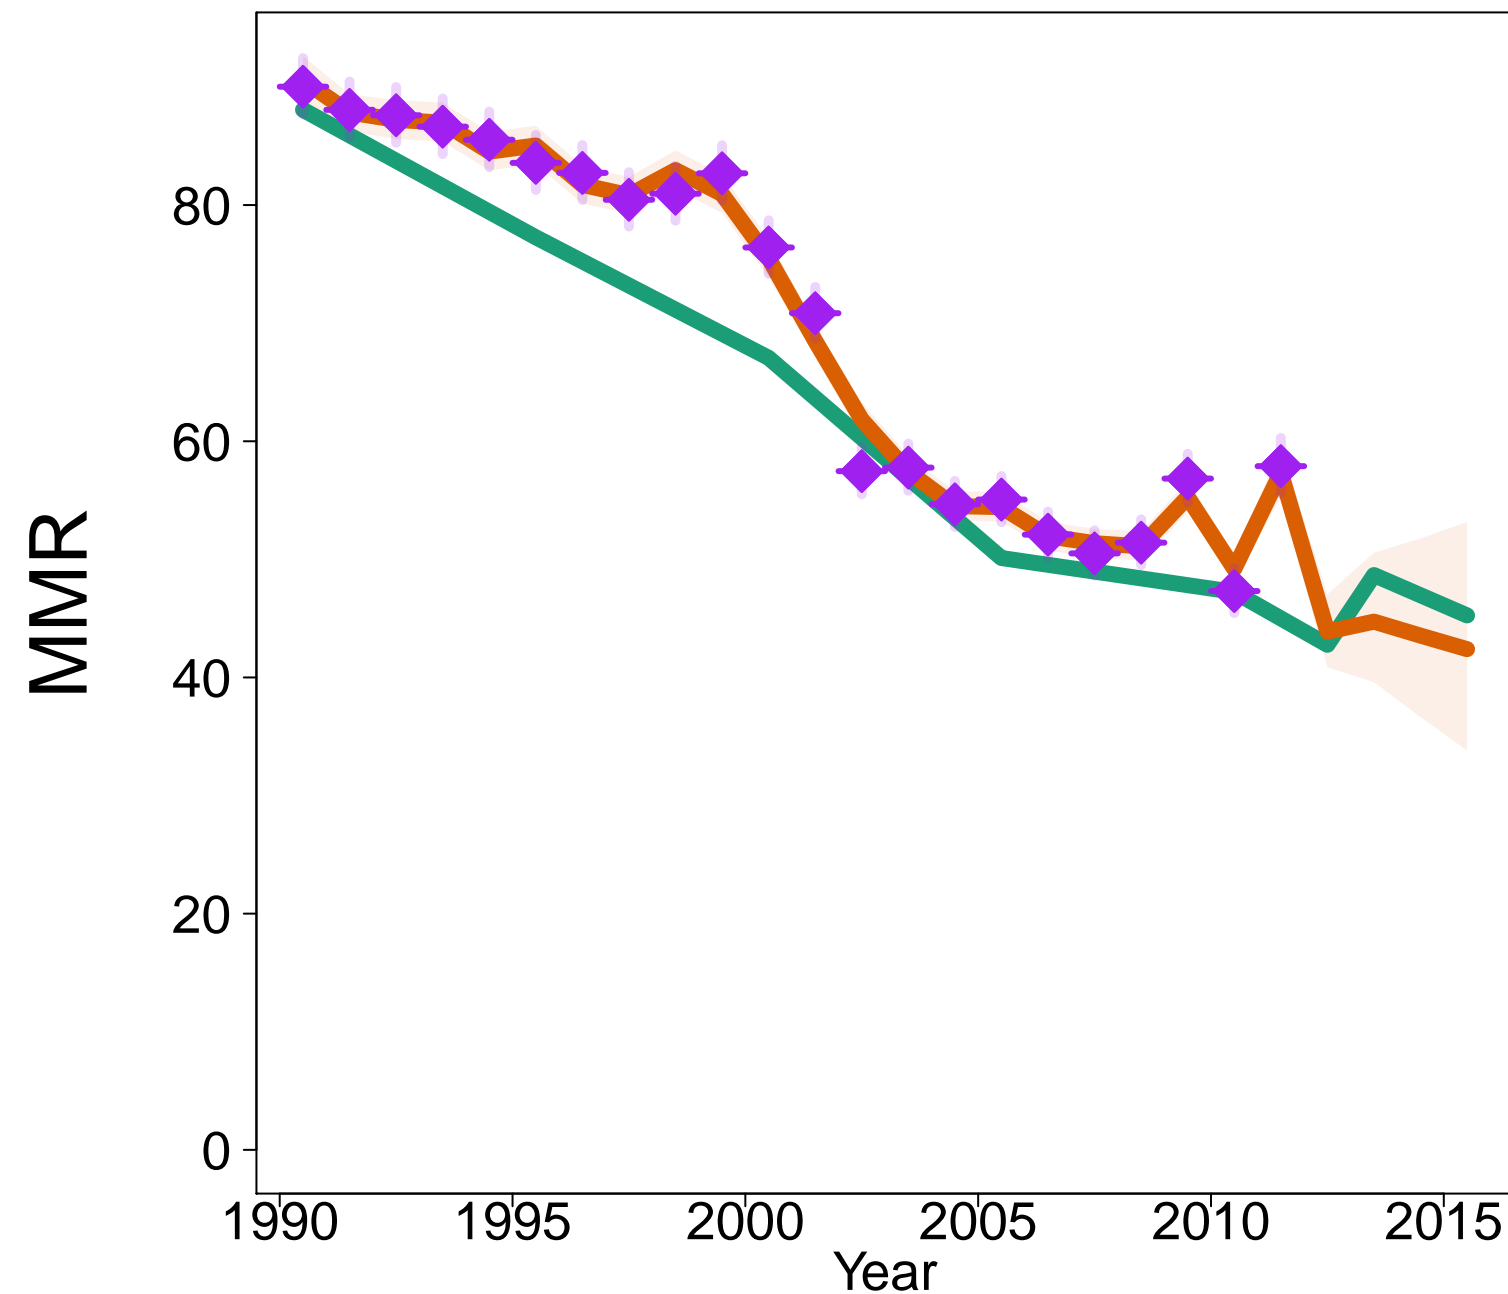

- Estimates –
- Bmat 2014
- MMEIG 2014
- Data –
- Observed Data
- Adjusted Data
- Data type –
- Spec. studies

Micronesia [FSM; C]  
(South-Eastern Asia / Oceania)

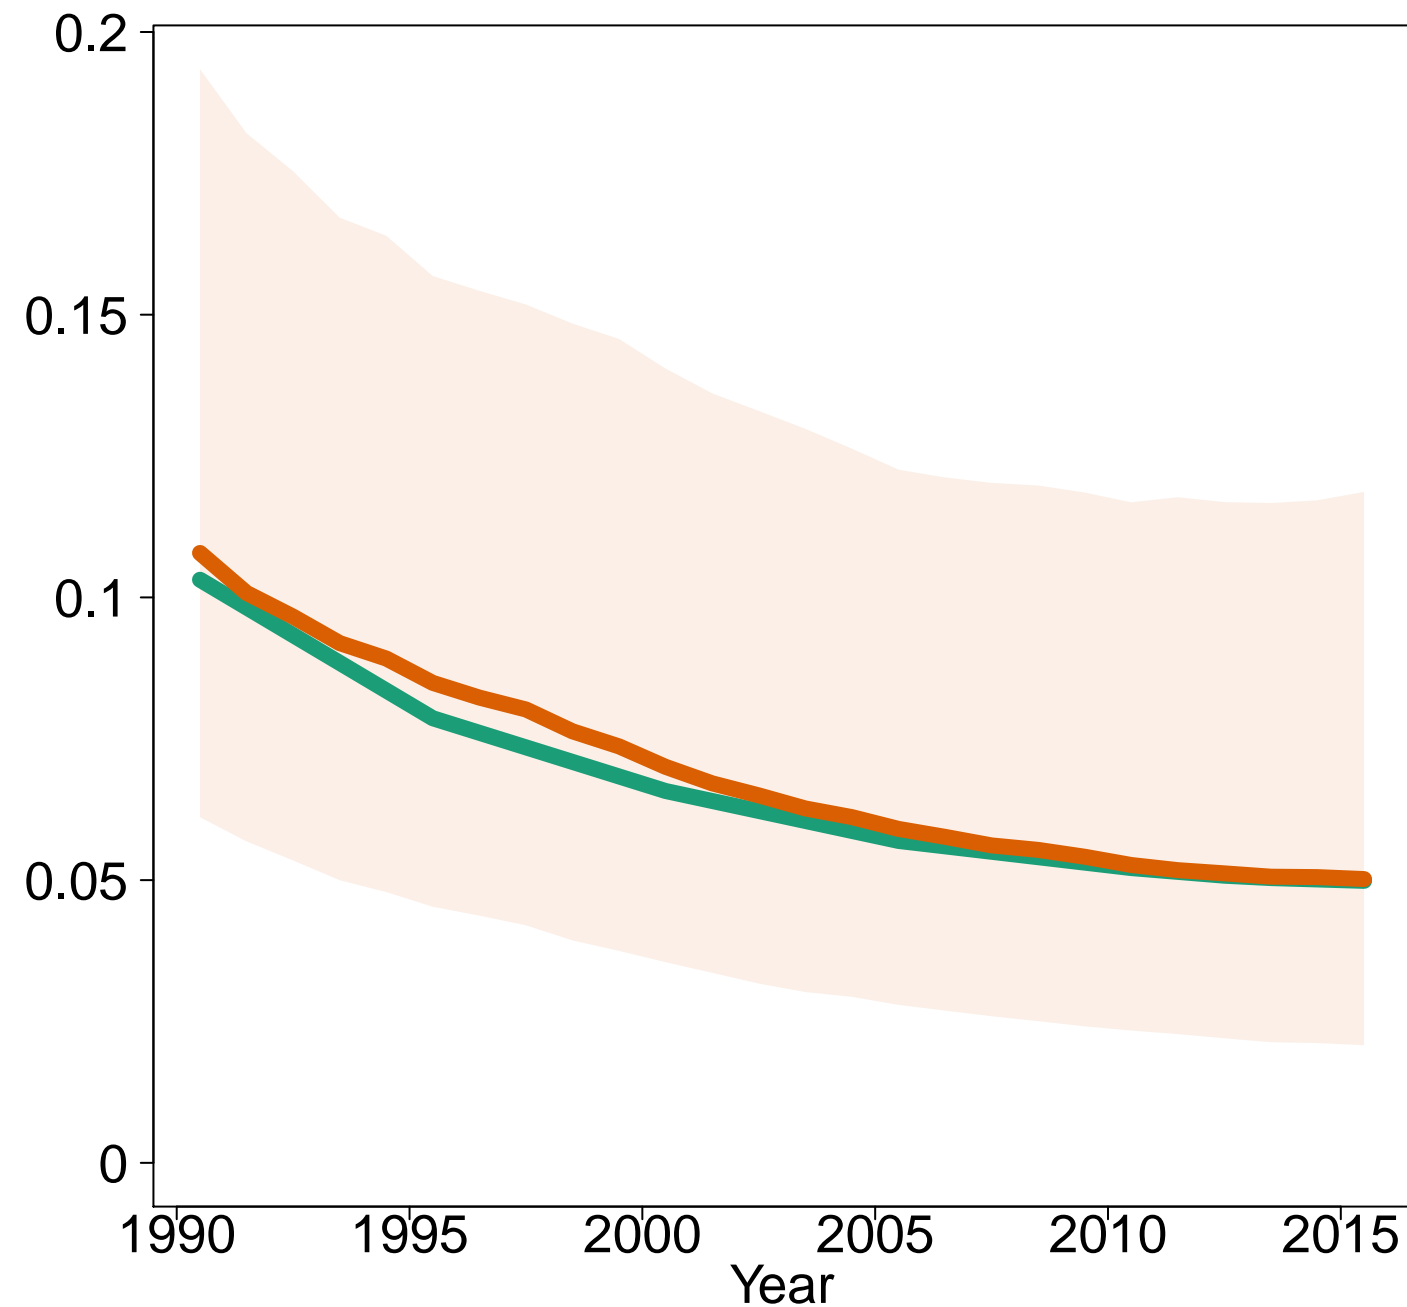

Micronesia [FSM; C]  
(South-Eastern Asia / Oceania)

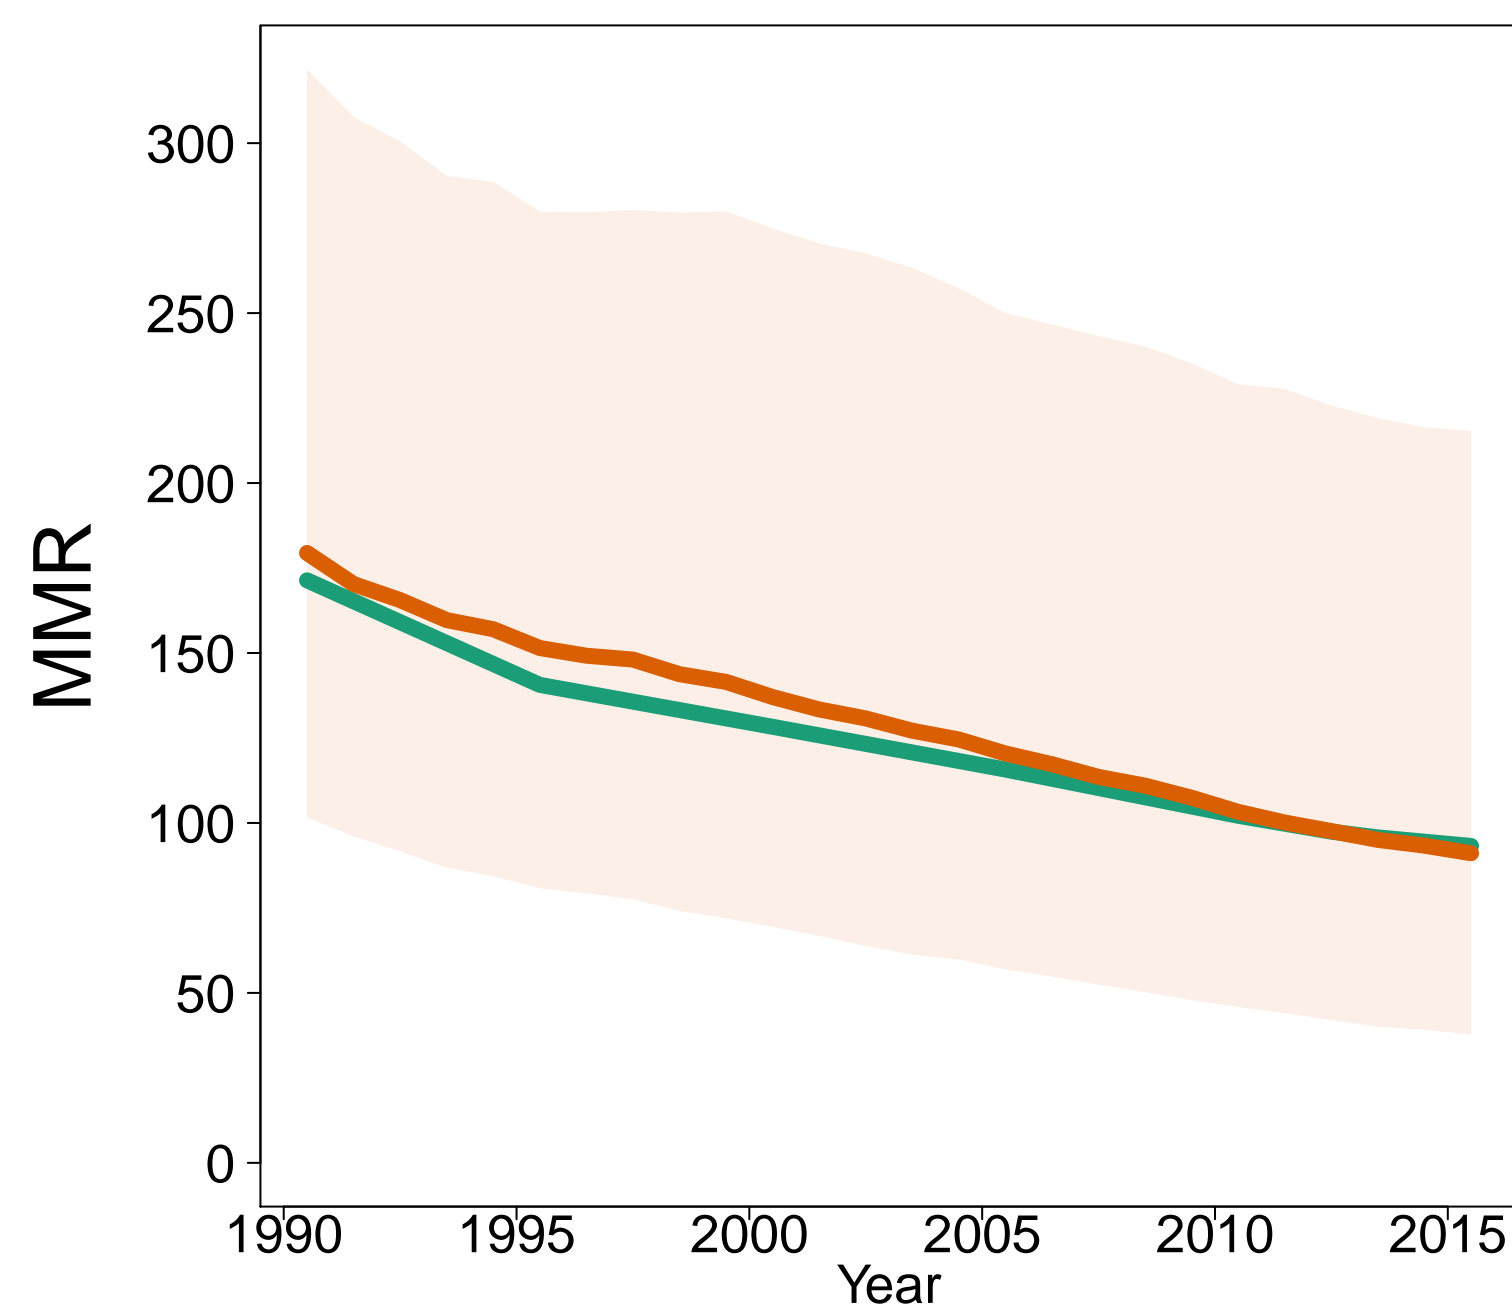

– Estimates –  
Bmat 2014  
MMEIG 2014  
– Data –

Mongolia [MNG; B]  
(Eastern Asia)

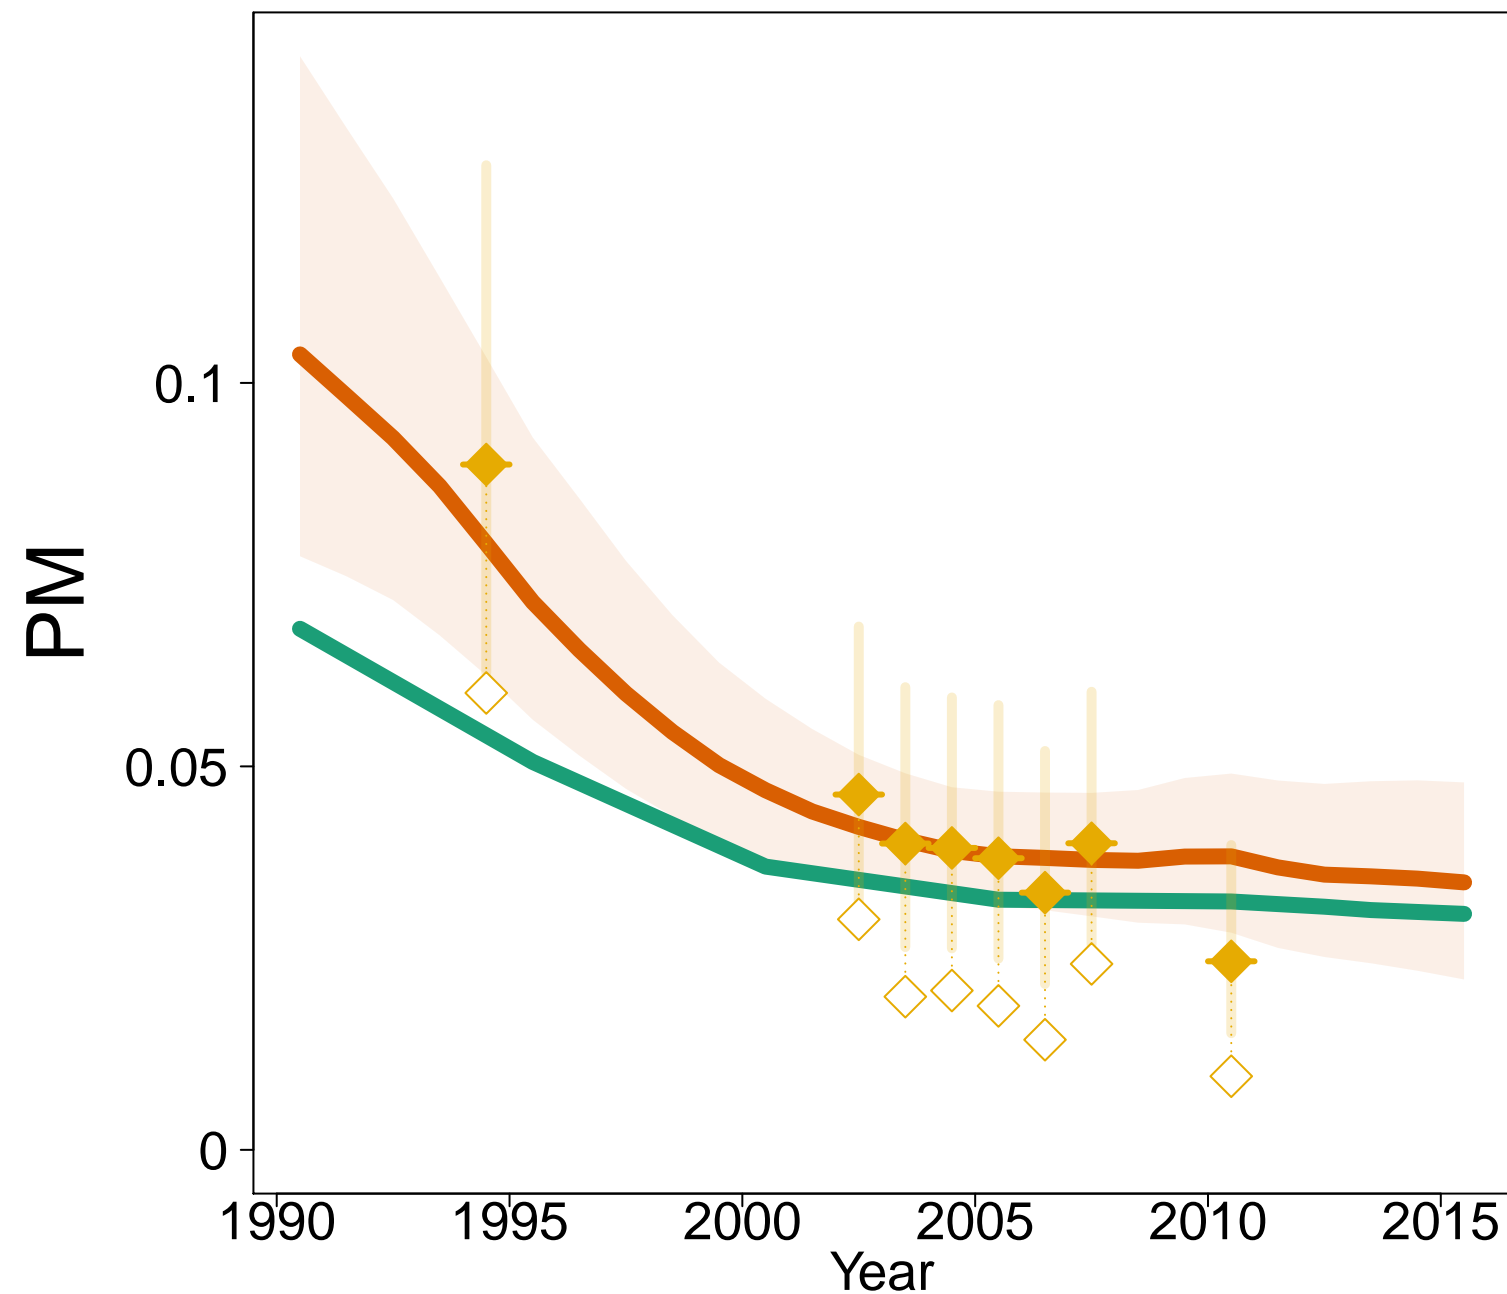

Mongolia [MNG; B]  
(Eastern Asia)

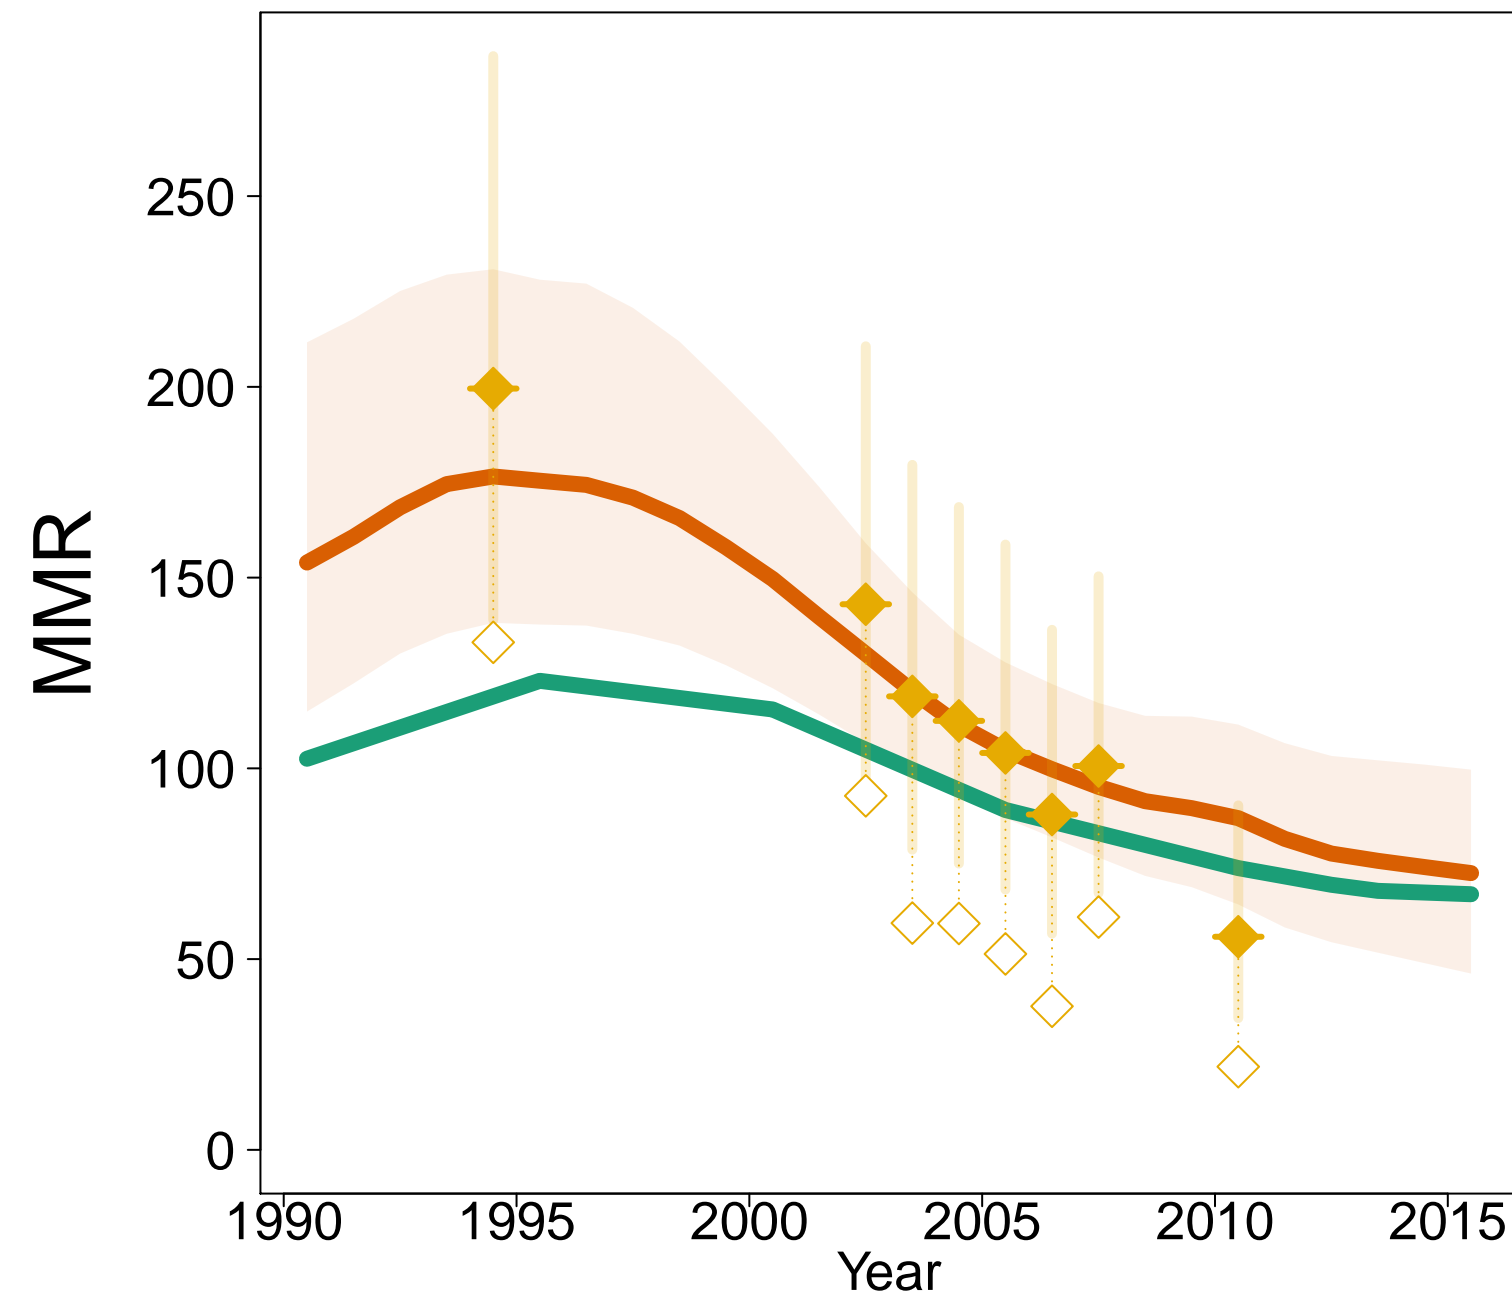

- Estimates –
- Bmat 2014
- MMEIG 2014
- Data –
- Observed Data
- Adjusted Data
- Data type –
- VR

Montenegro [MNE; B]  
(Transition countries of South-Eastern Europe)

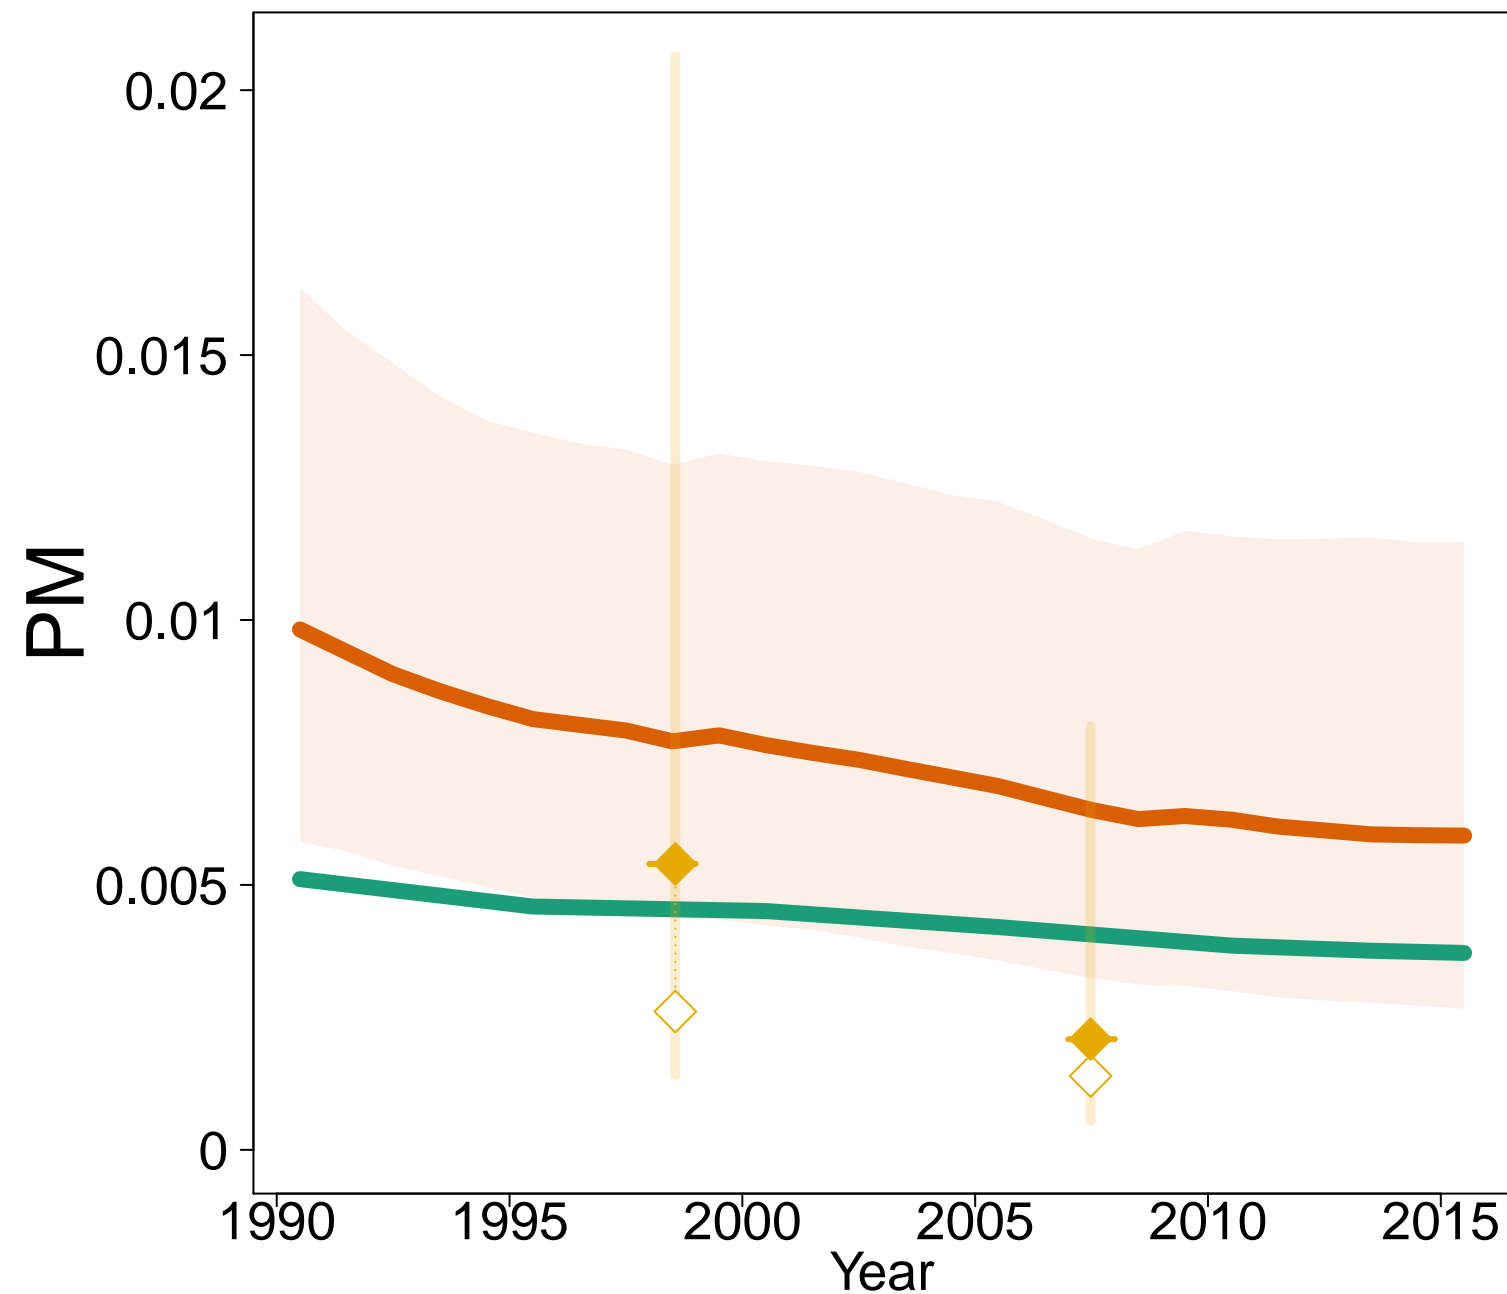

Montenegro [MNE; B]  
(Transition countries of South-Eastern Europe)

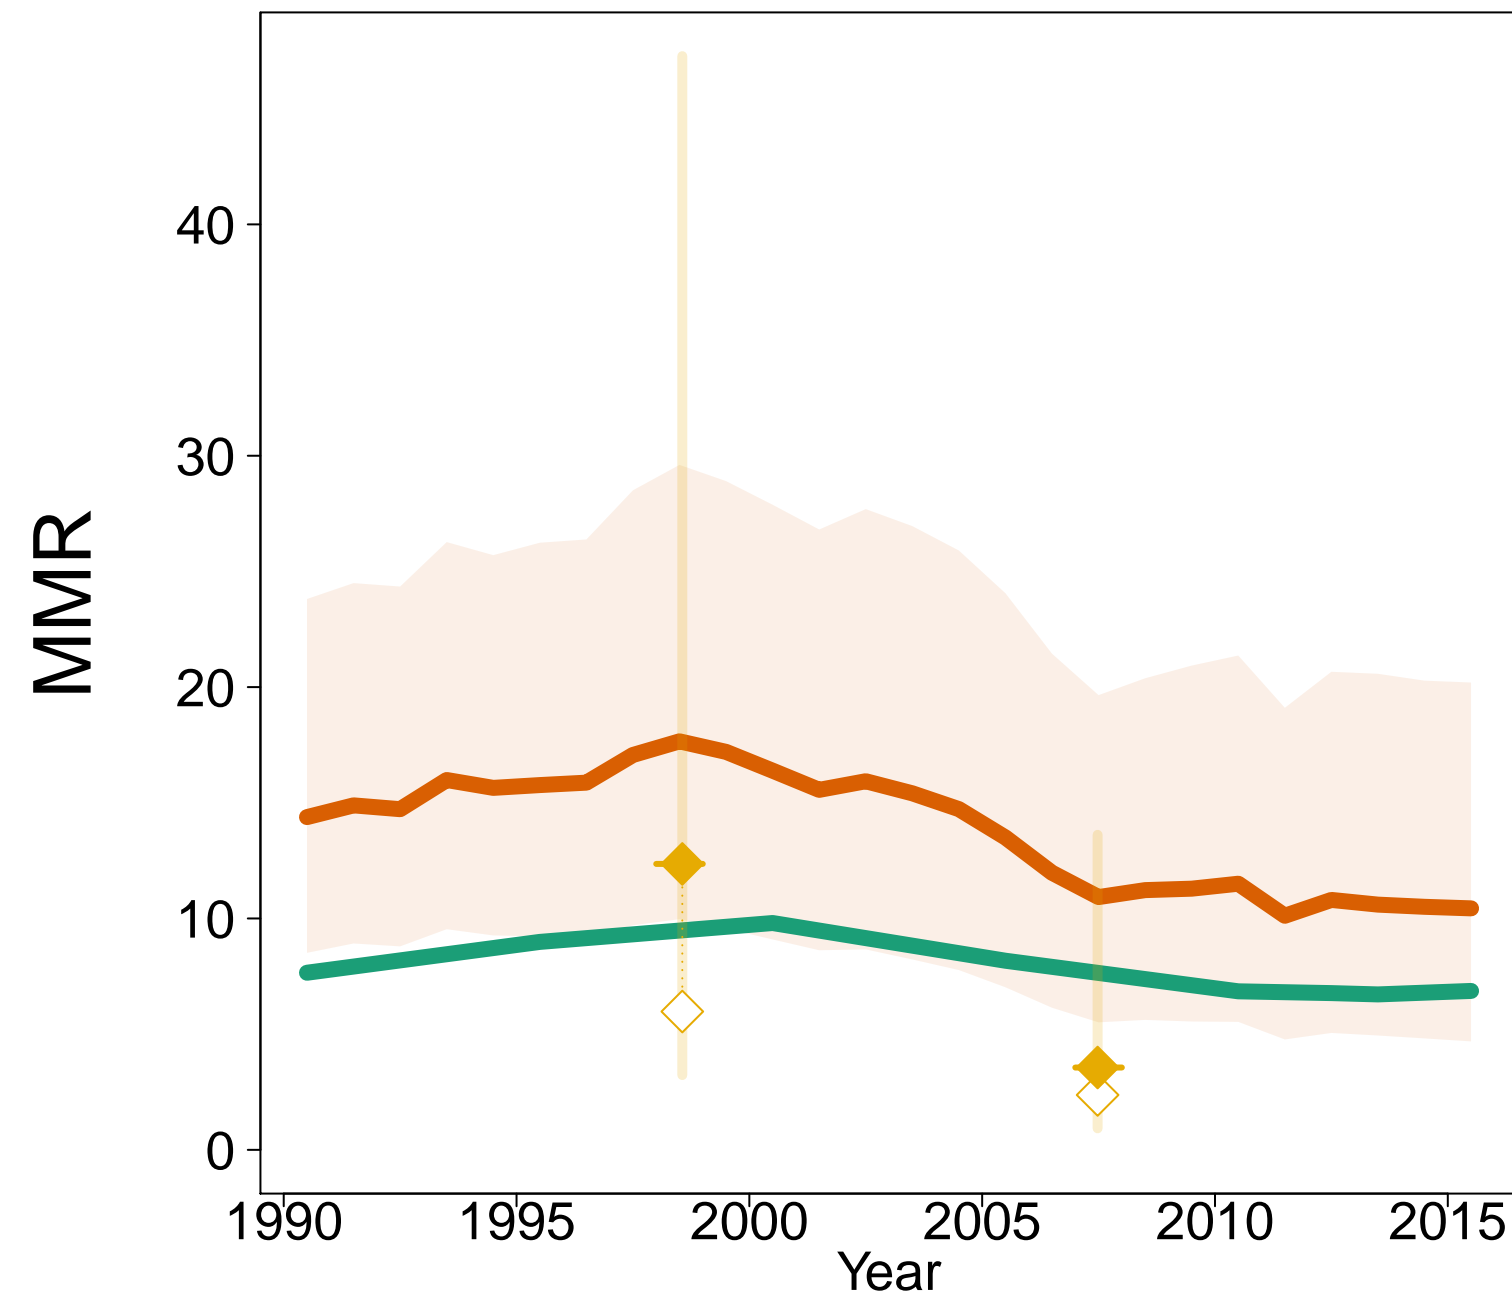

- Estimates –
- Bmat 2014
- MMEIG 2014
- Data –
- Observed Data
- Adjusted Data
- Data type –
- VR

Morocco [MAR; B]  
(Northern Africa)

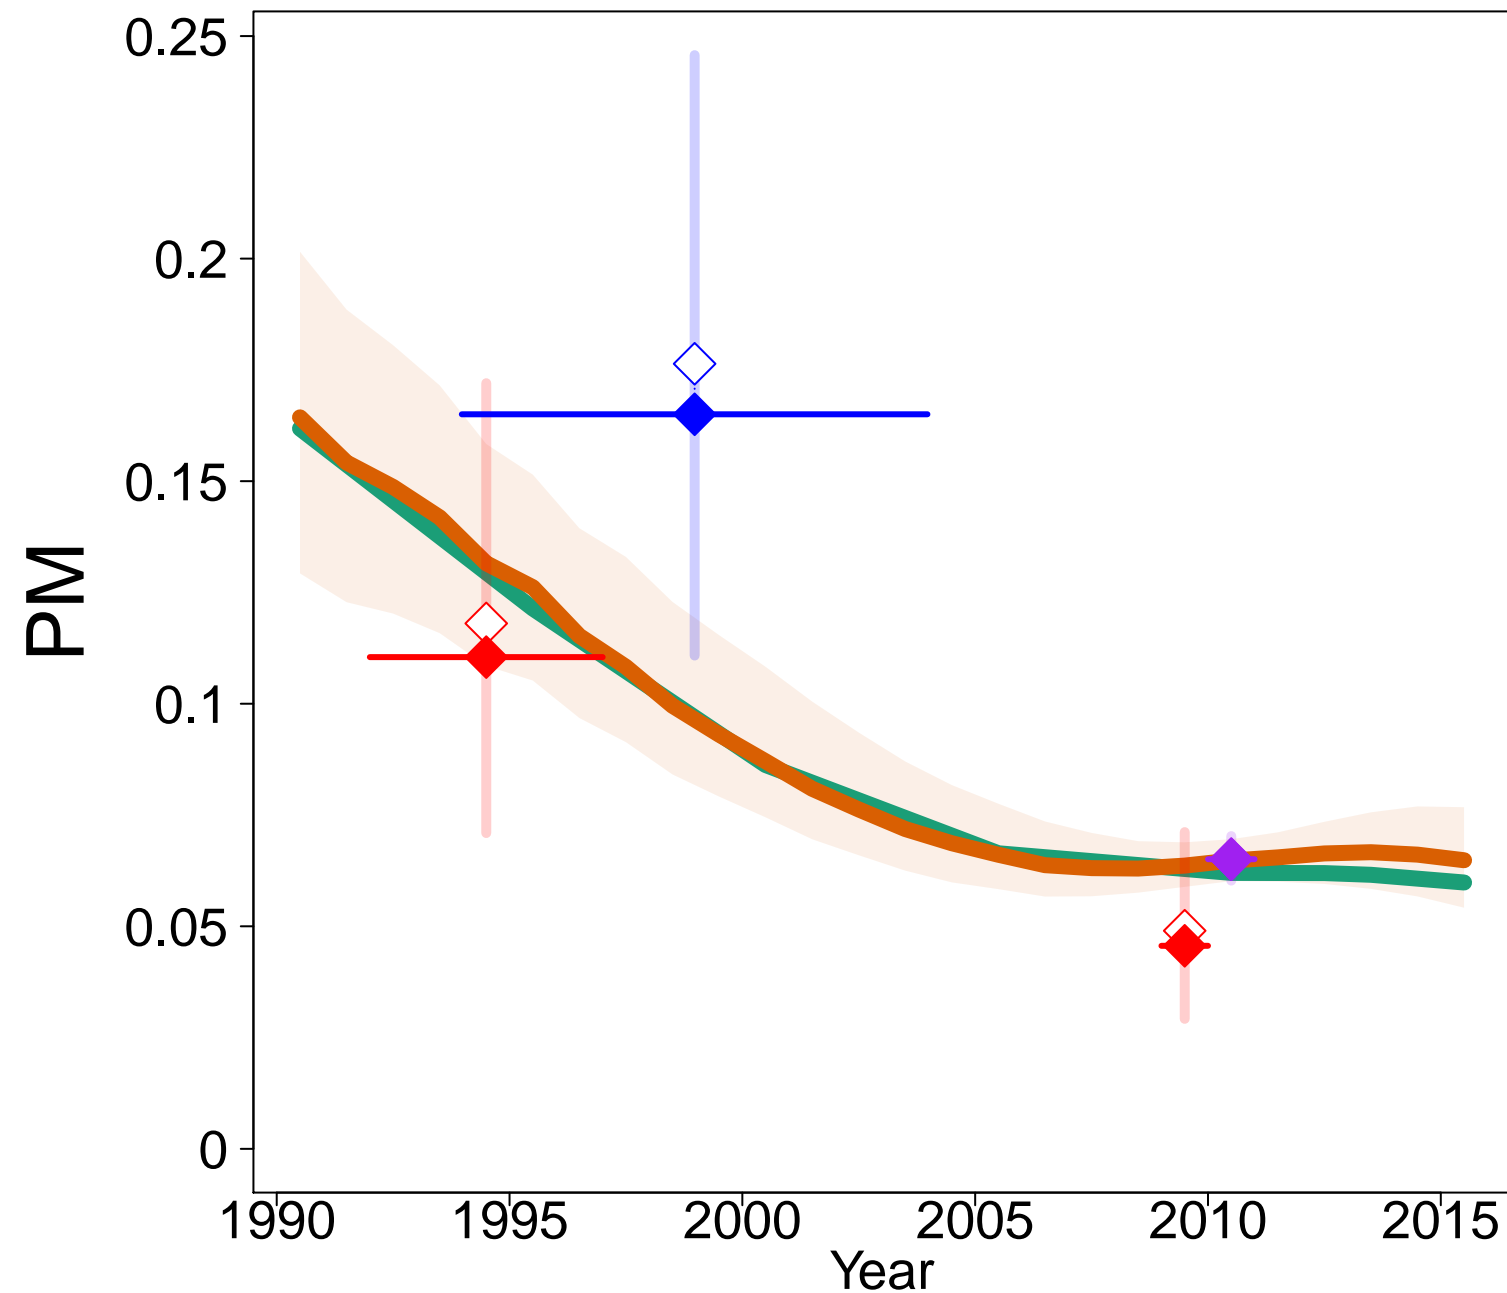

Morocco [MAR; B]  
(Northern Africa)

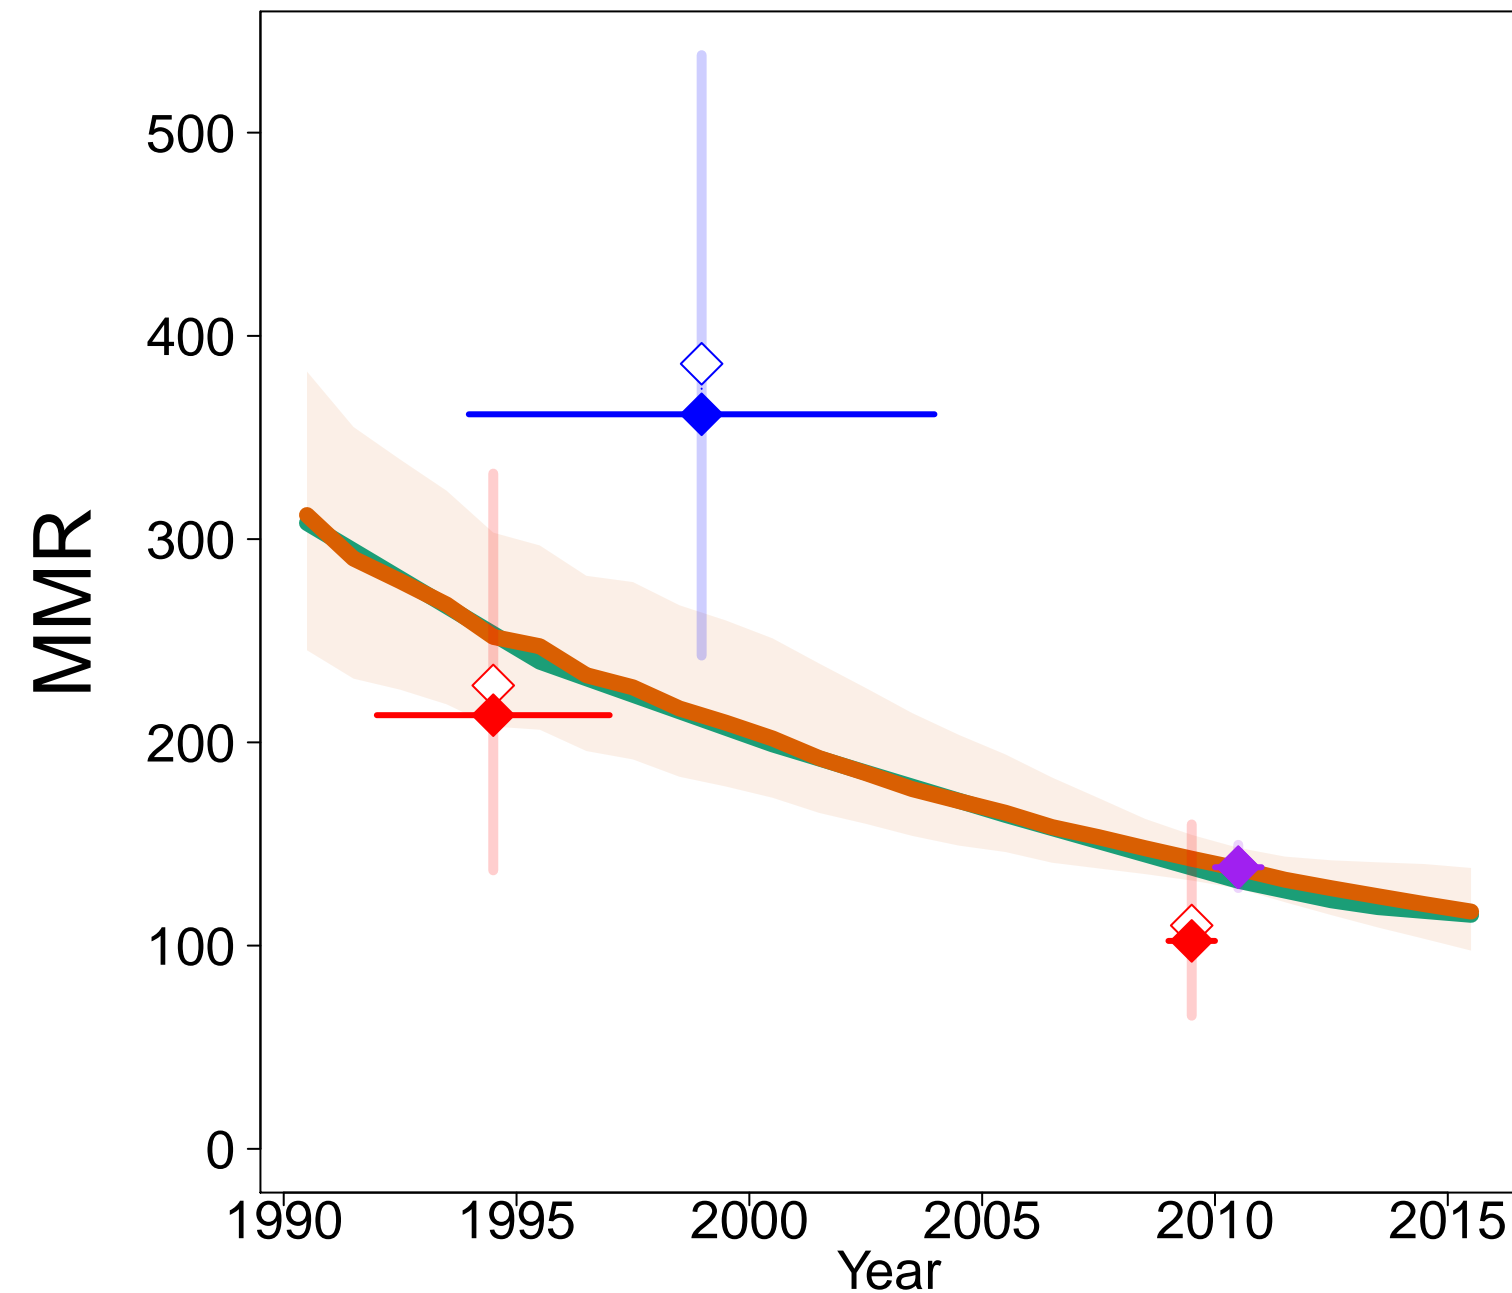

- Estimates –
- Bmat 2014
- MMEIG 2014
- Data –
- Observed Data
- Adjusted Data
- Data type –
- Spec. studies
- DHS
- Misc. studies

Mozambique [MOZ; B]  
(Eastern Africa)

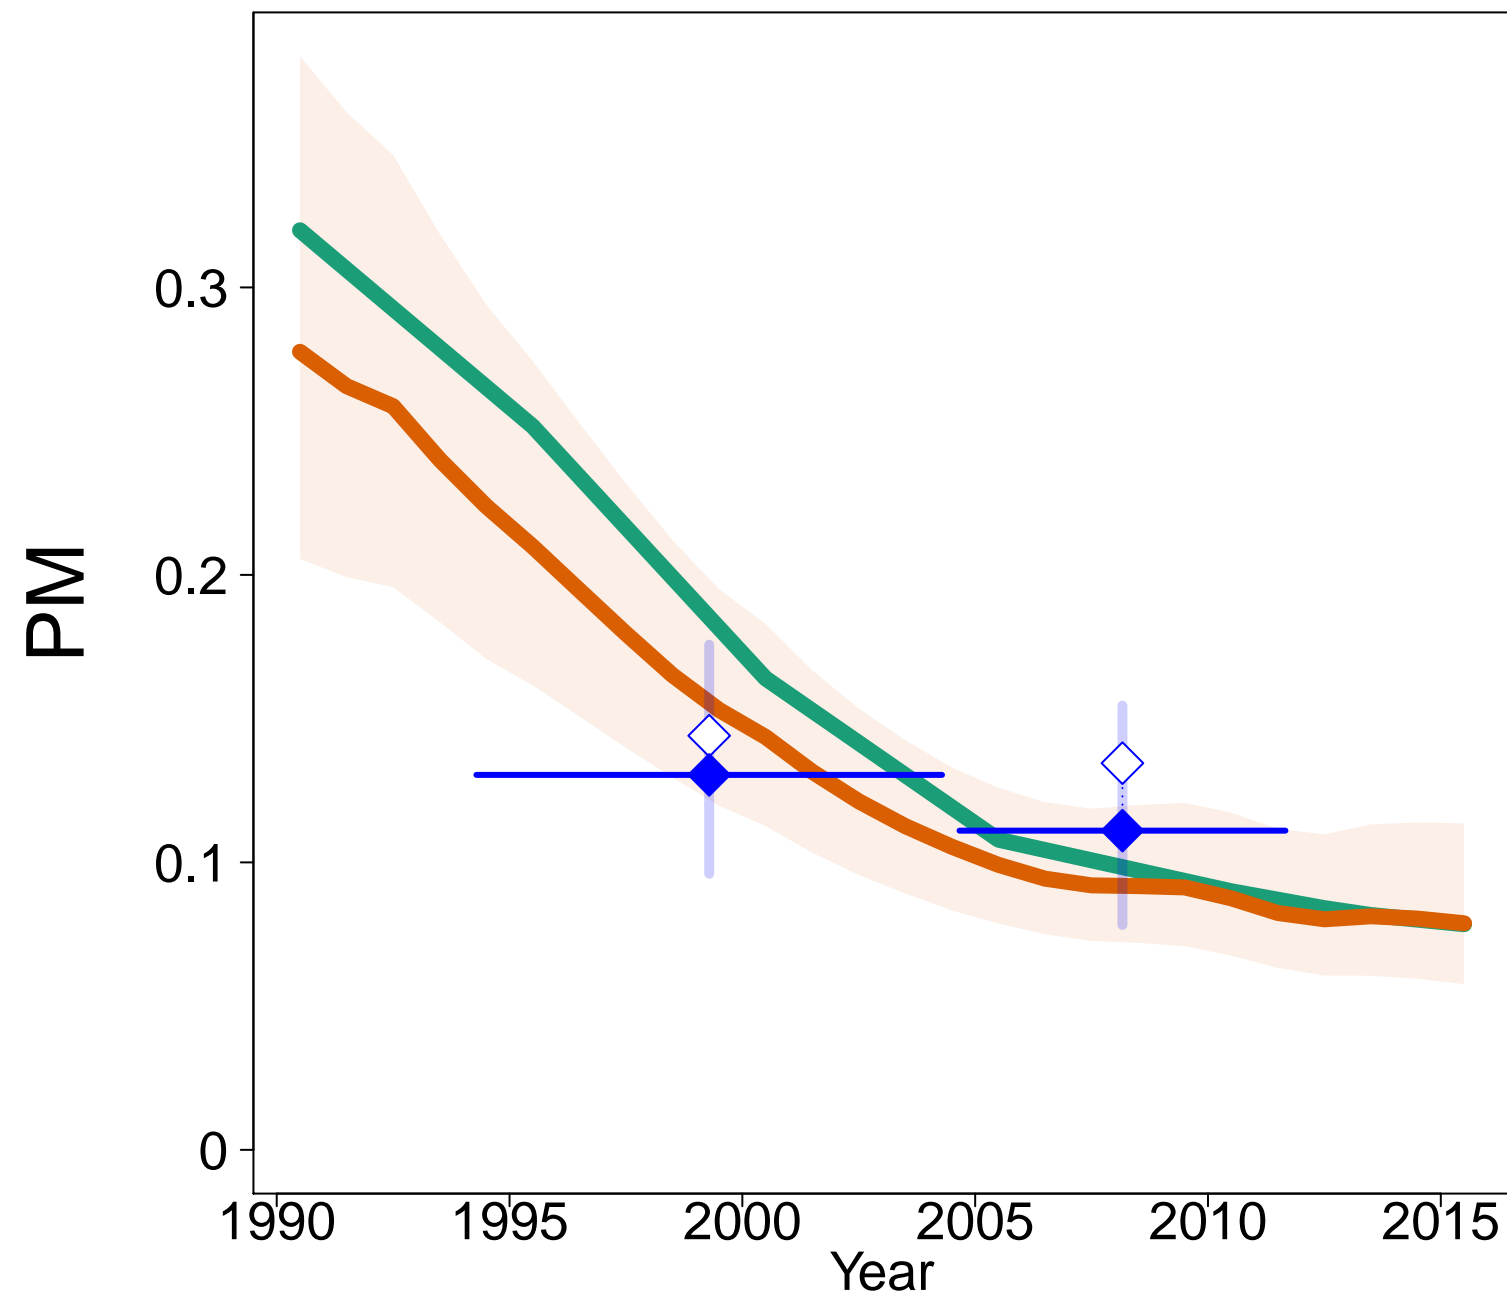

Mozambique [MOZ; B]  
(Eastern Africa)

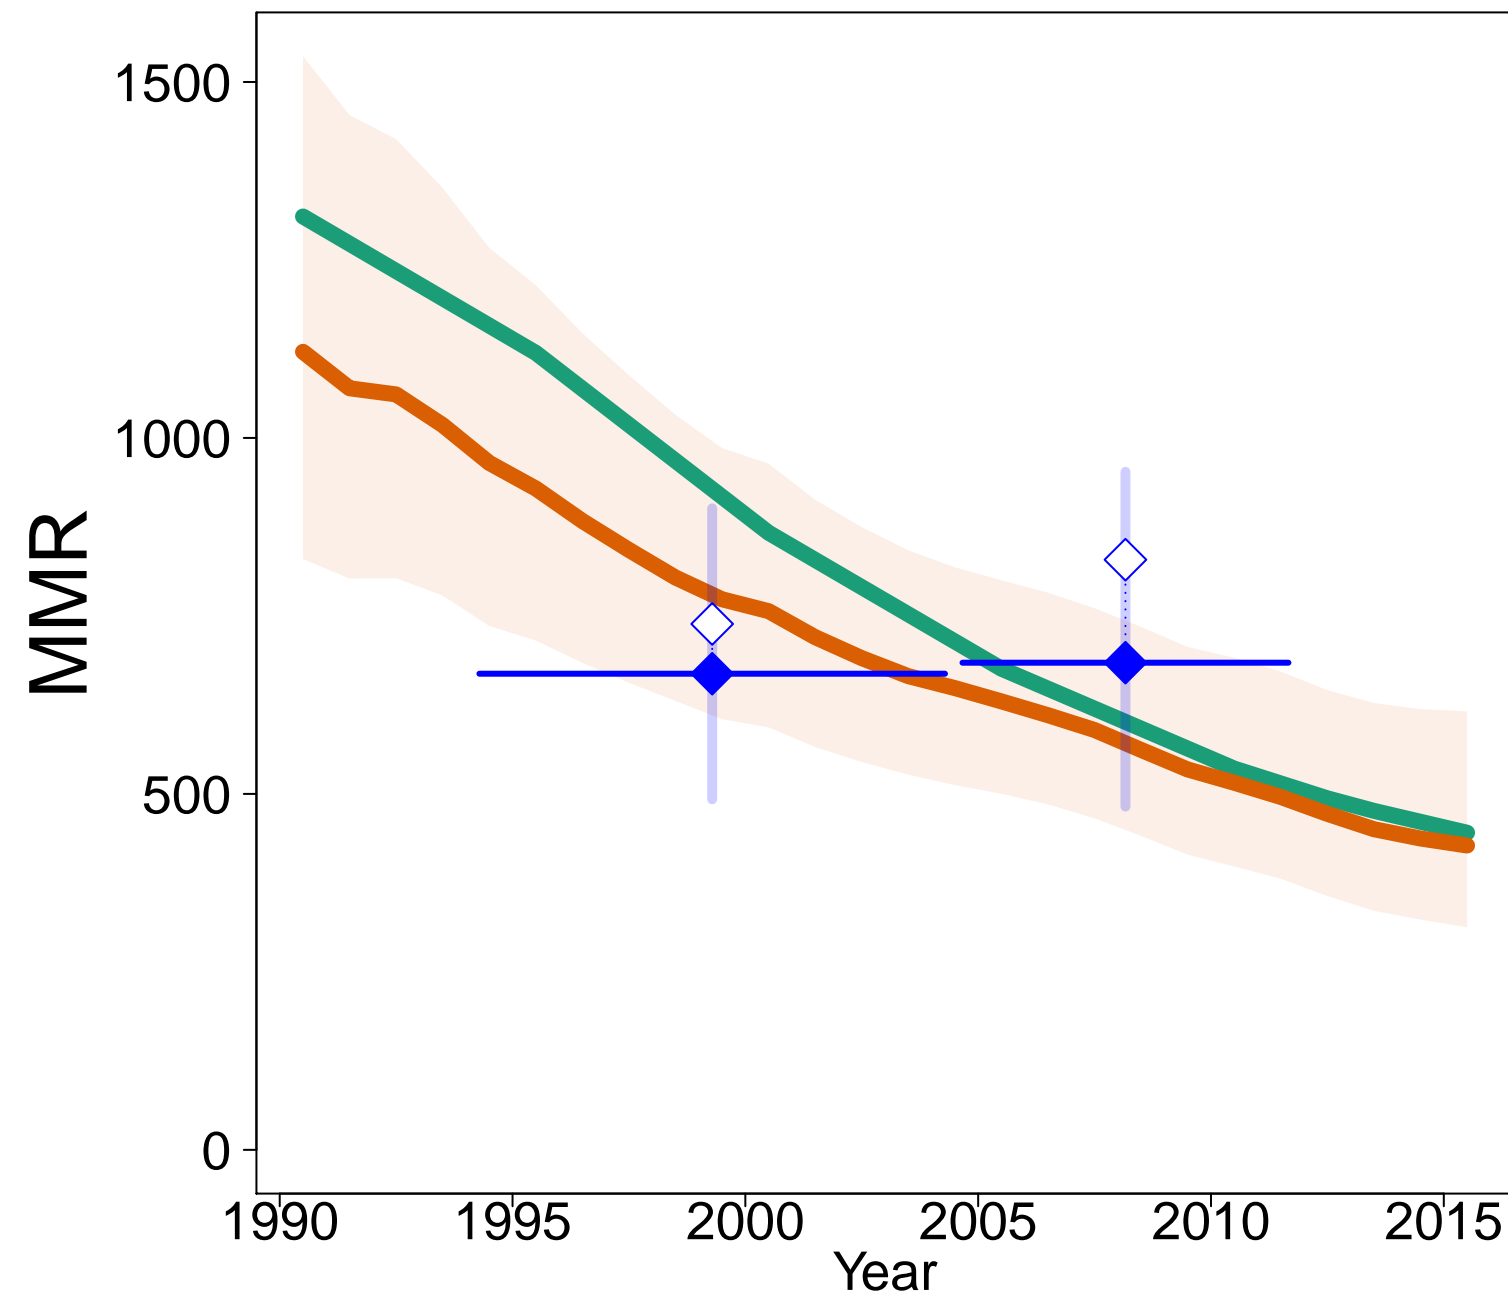

- Estimates –
- Bmat 2014
- MMEIG 2014
- Data –
- Observed Data
- Adjusted Data
- Data type –
- DHS

Myanmar [MMR; B]  
(South-Eastern Asia / Oceania)

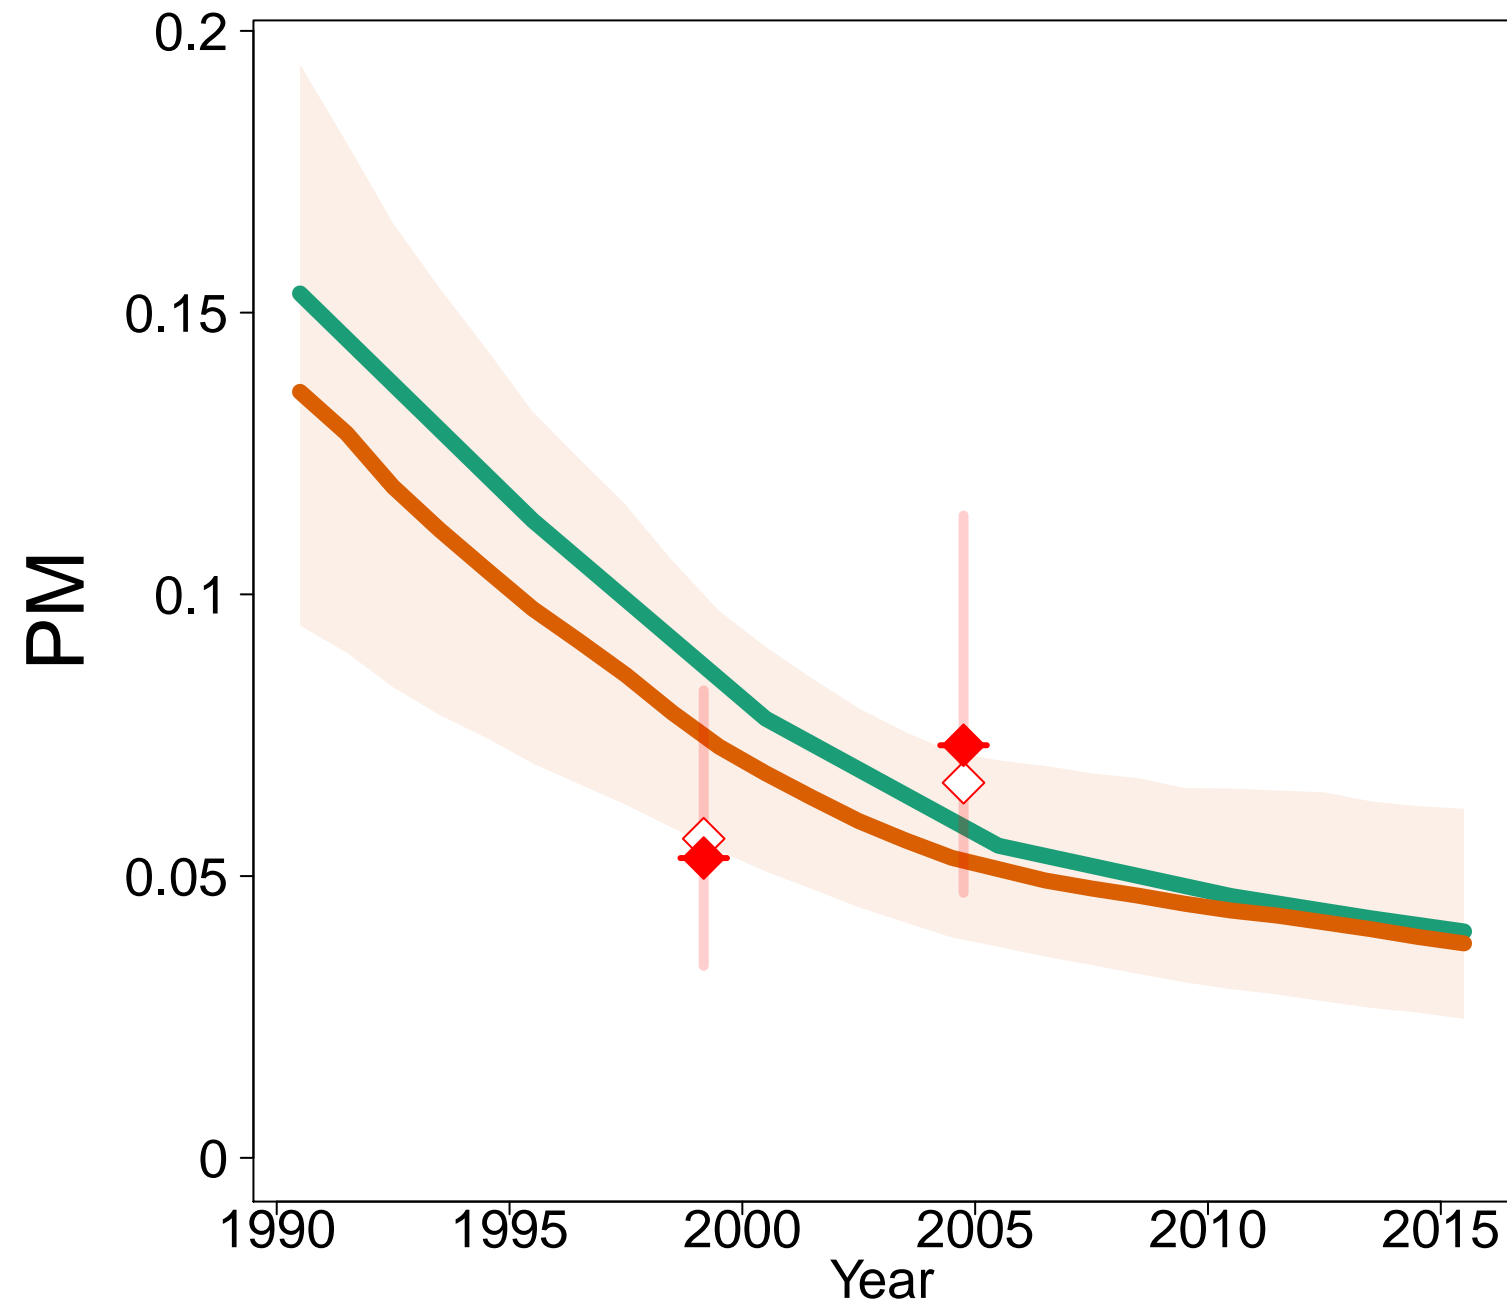

Myanmar [MMR; B]  
(South-Eastern Asia / Oceania)

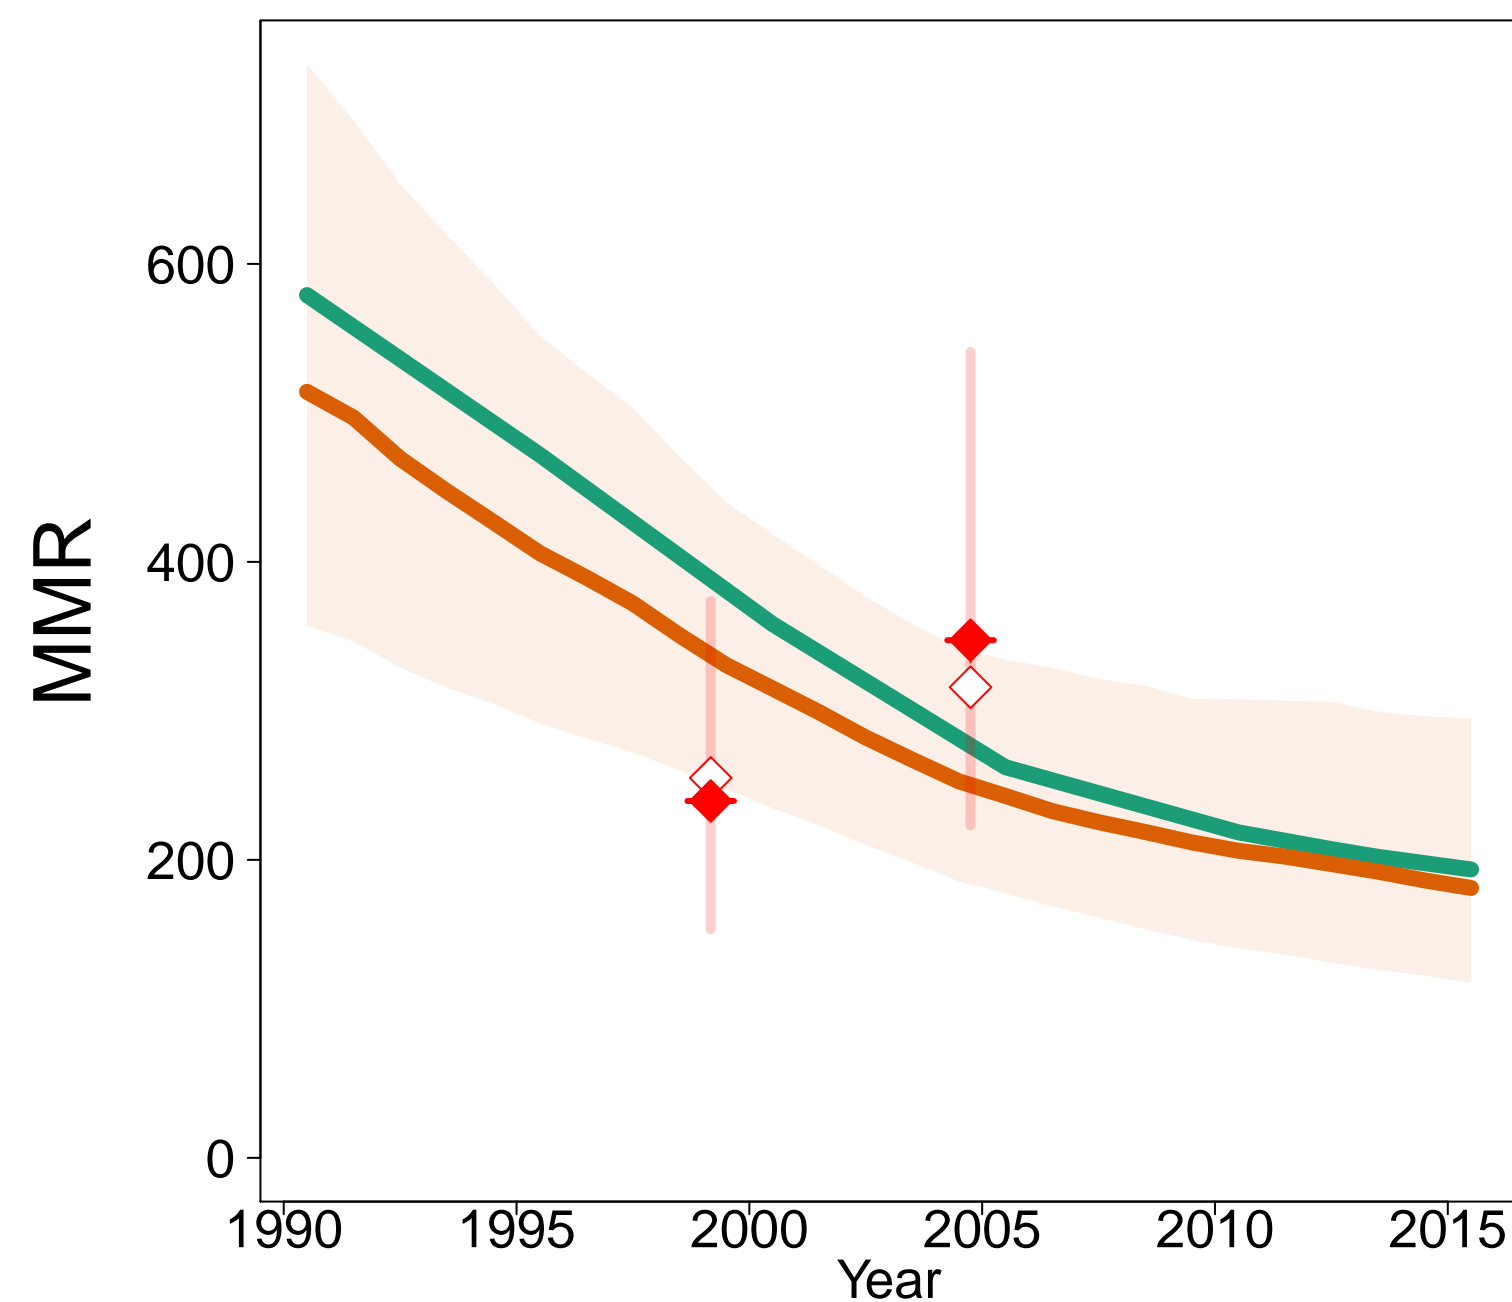

- Estimates –
- Bmat 2014
- MMEIG 2014
- Data –
- Observed Data
- Adjusted Data
- Data type –
- Misc. studies

Namibia [NAM; B]  
(Southern Africa)

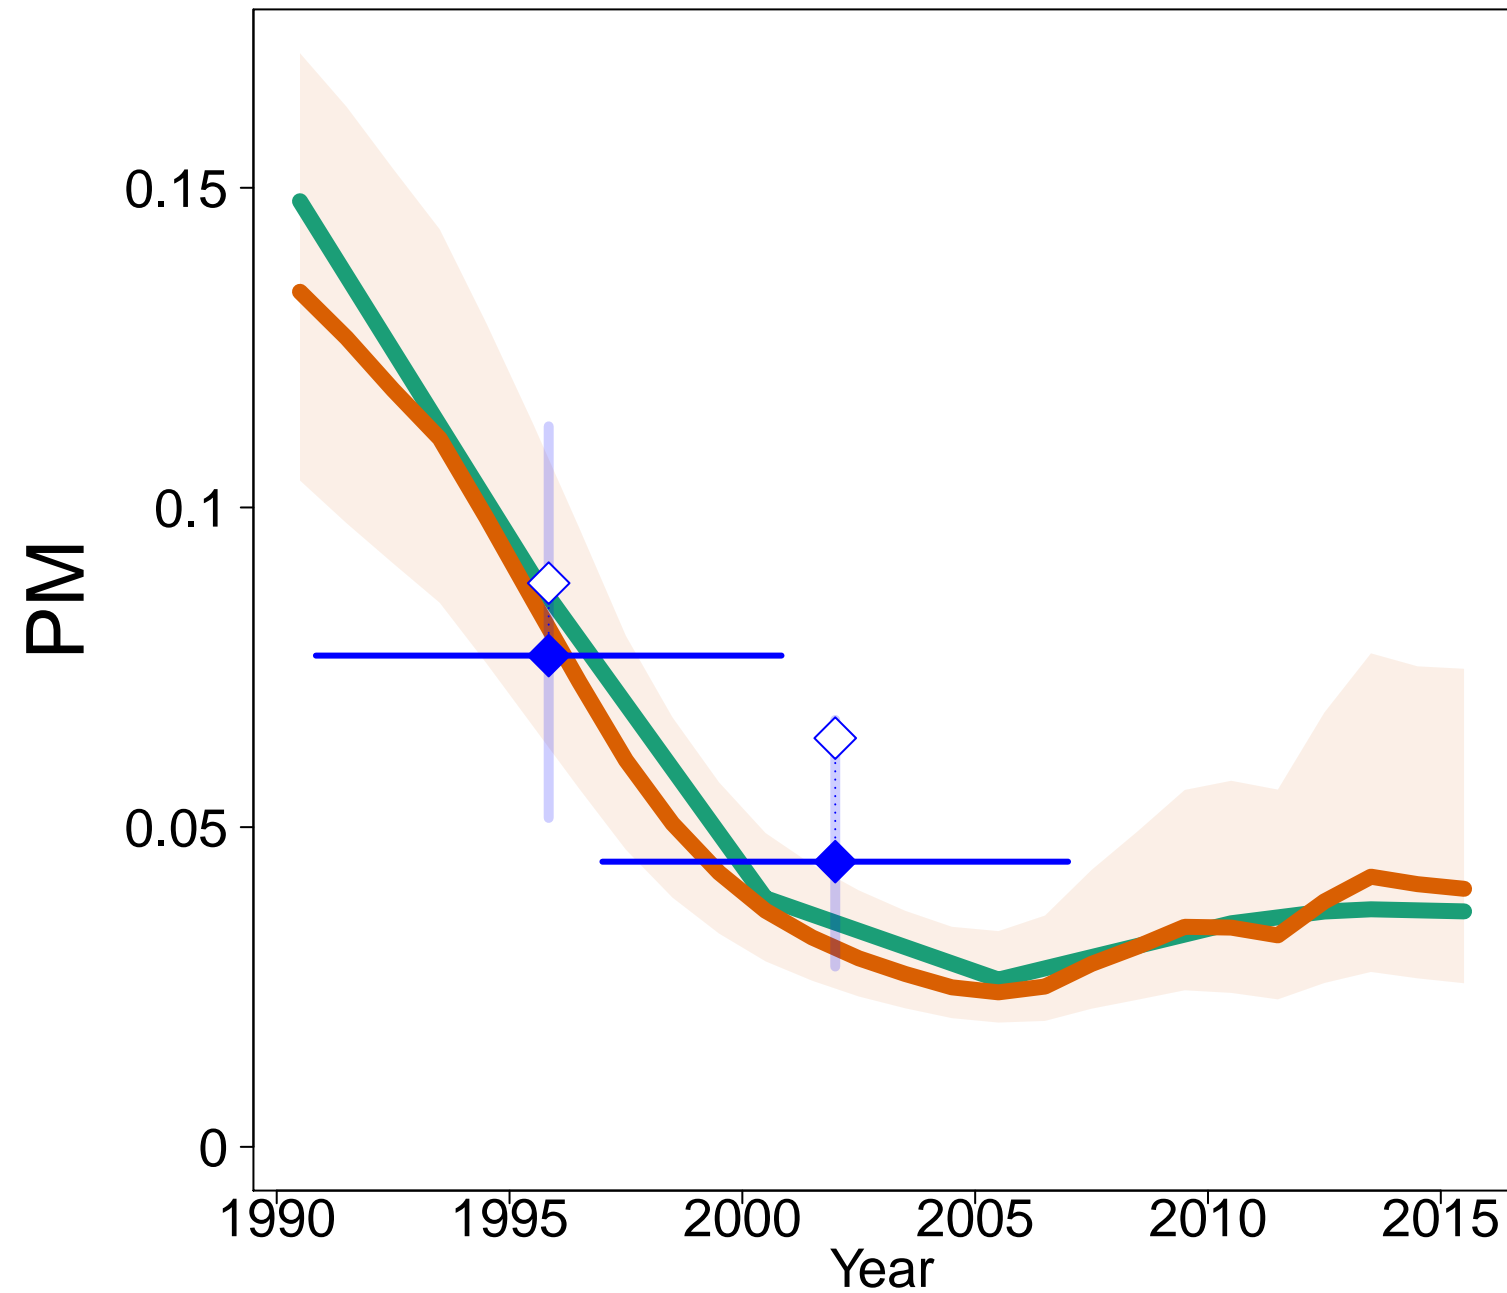

Namibia [NAM; B]  
(Southern Africa)

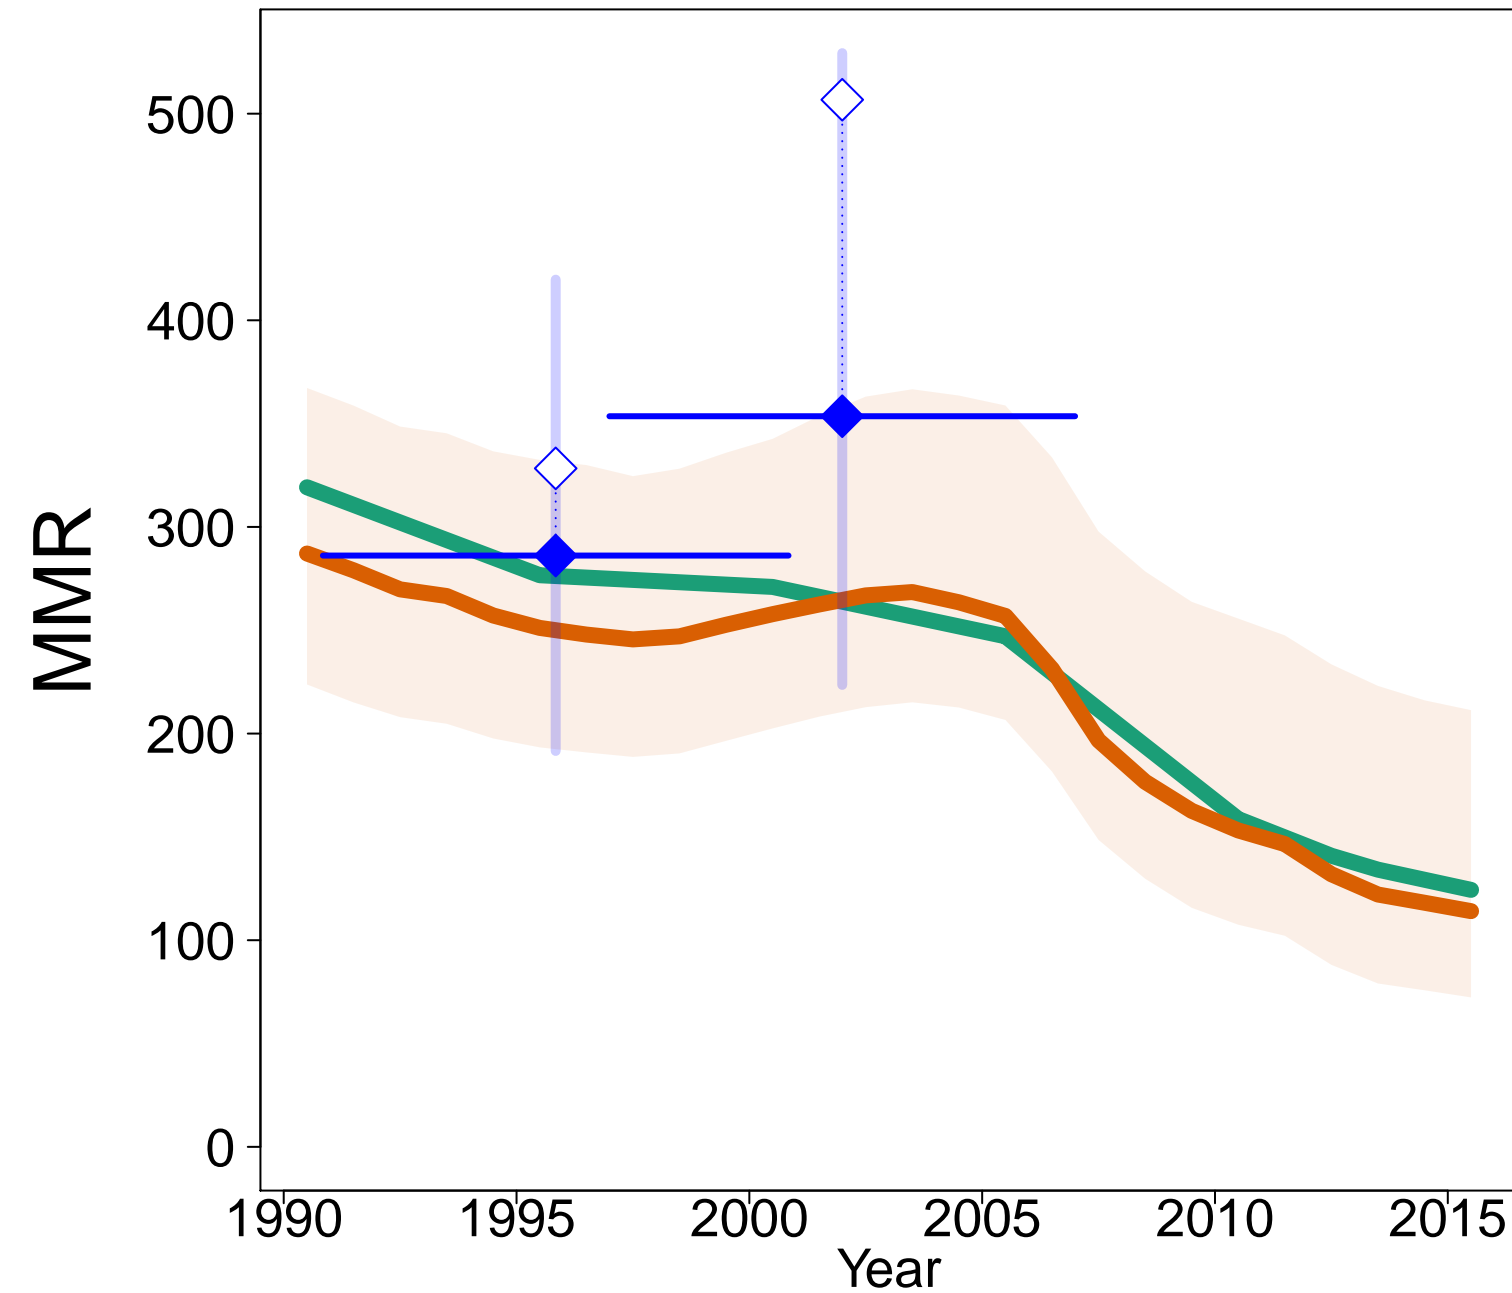

- Estimates –
- Bmat 2014
- MMEIG 2014
- Data –
- Observed Data
- Adjusted Data
- Data type –
- DHS



Nepal [NPL; B]  
(Southern Asia)

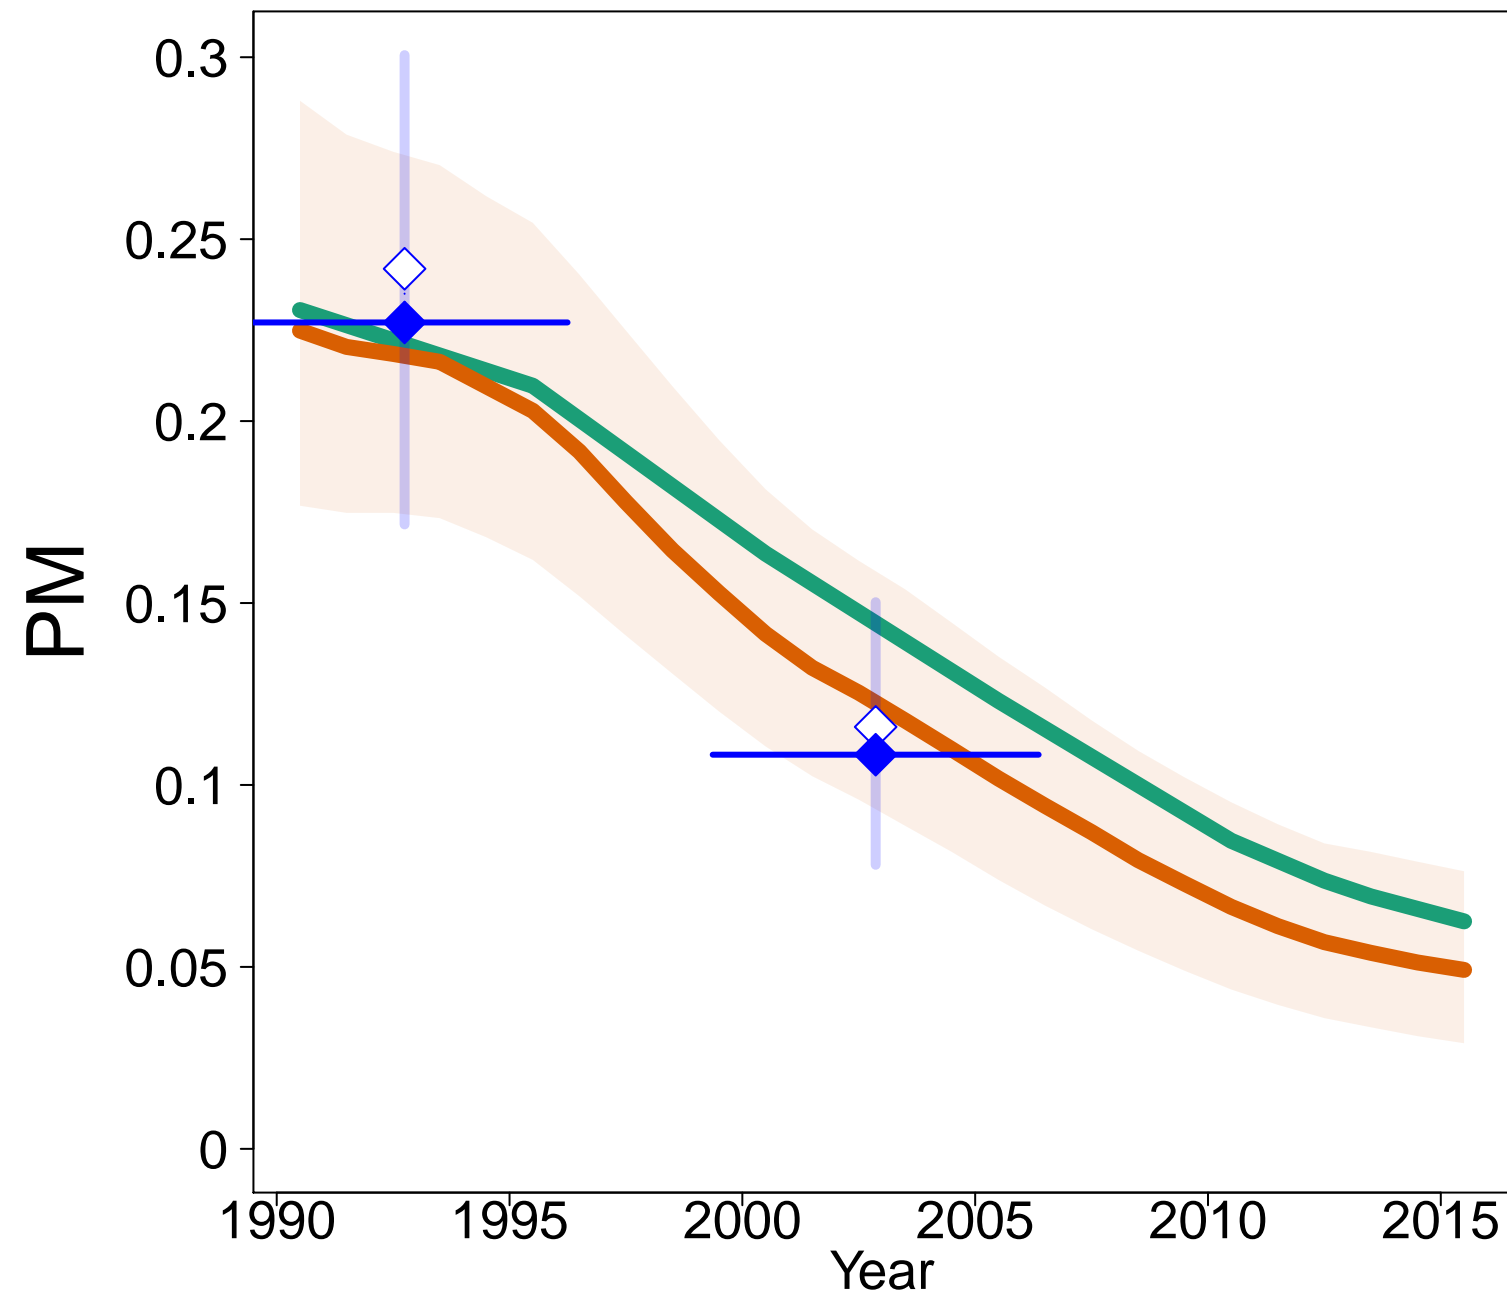

Nepal [NPL; B]  
(Southern Asia)

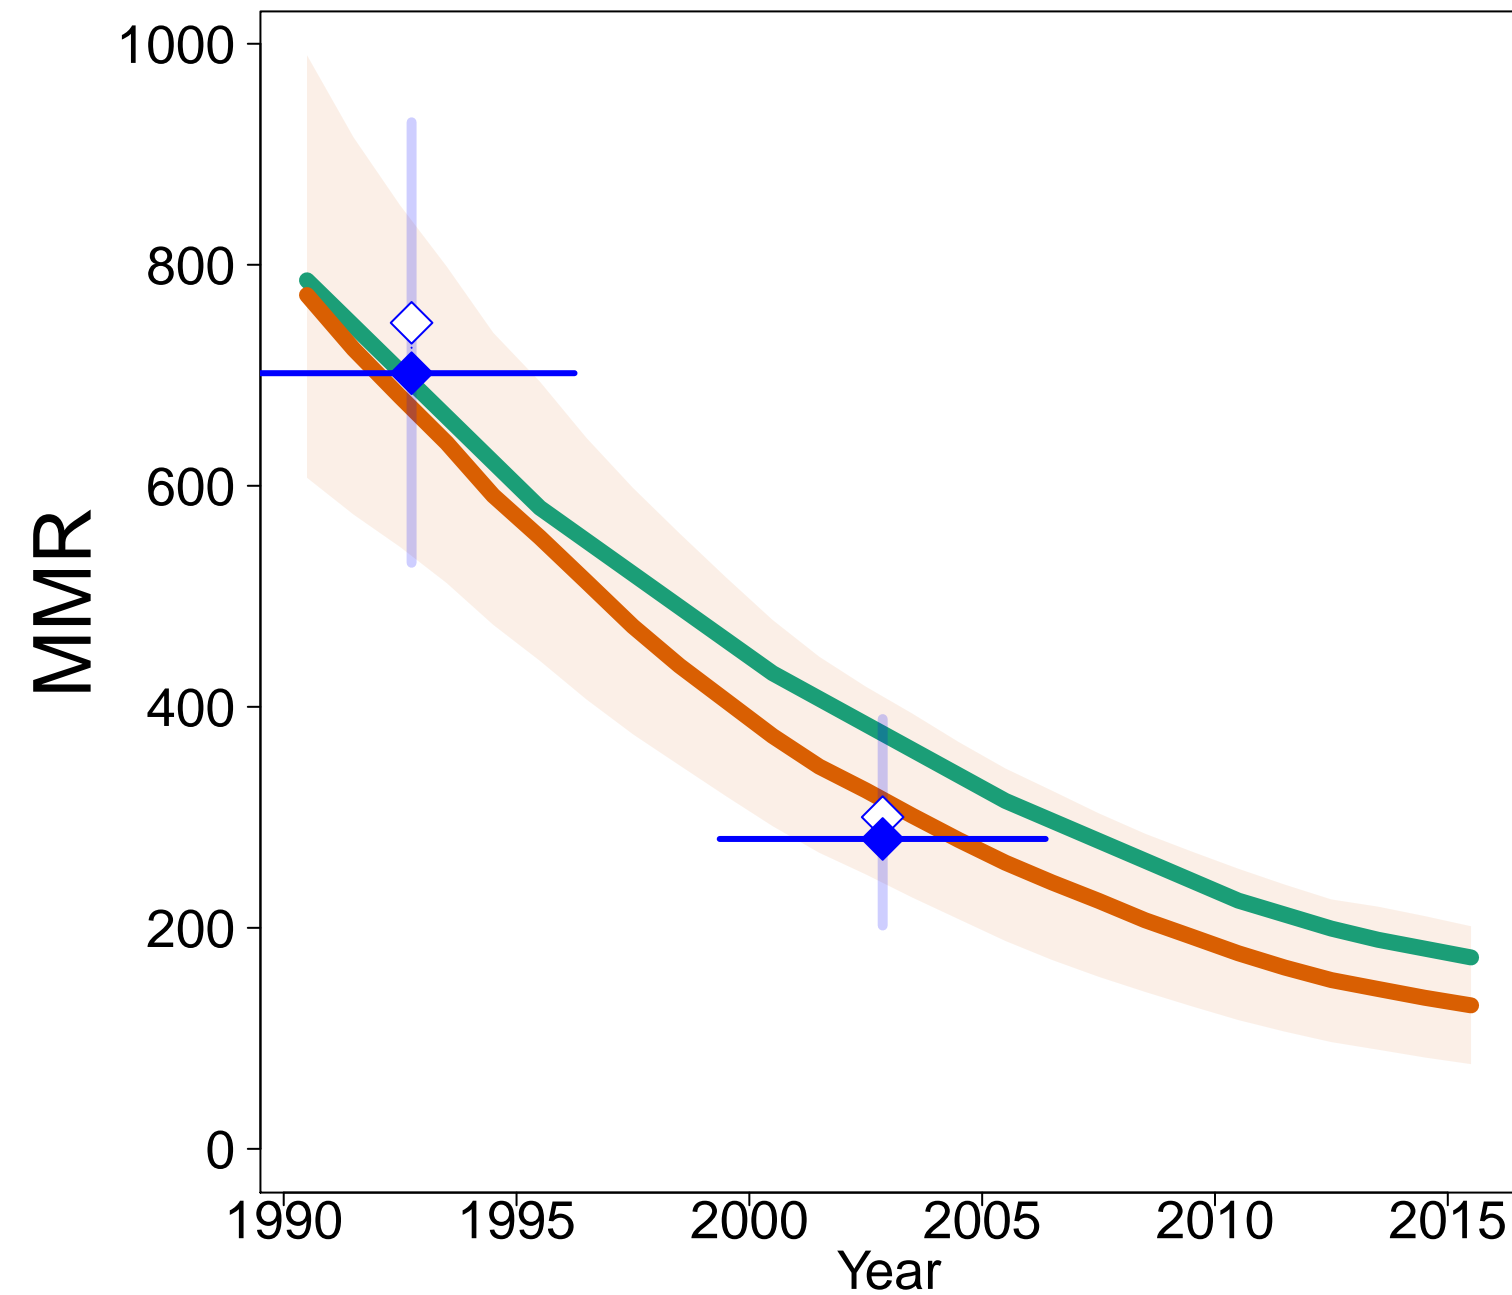

- Estimates –
- Bmat 2014
- MMEIG 2014
- Data –
- Observed Data
- Adjusted Data
- Data type –
- DHS

Netherlands [NLD; A]  
(Developed regions)

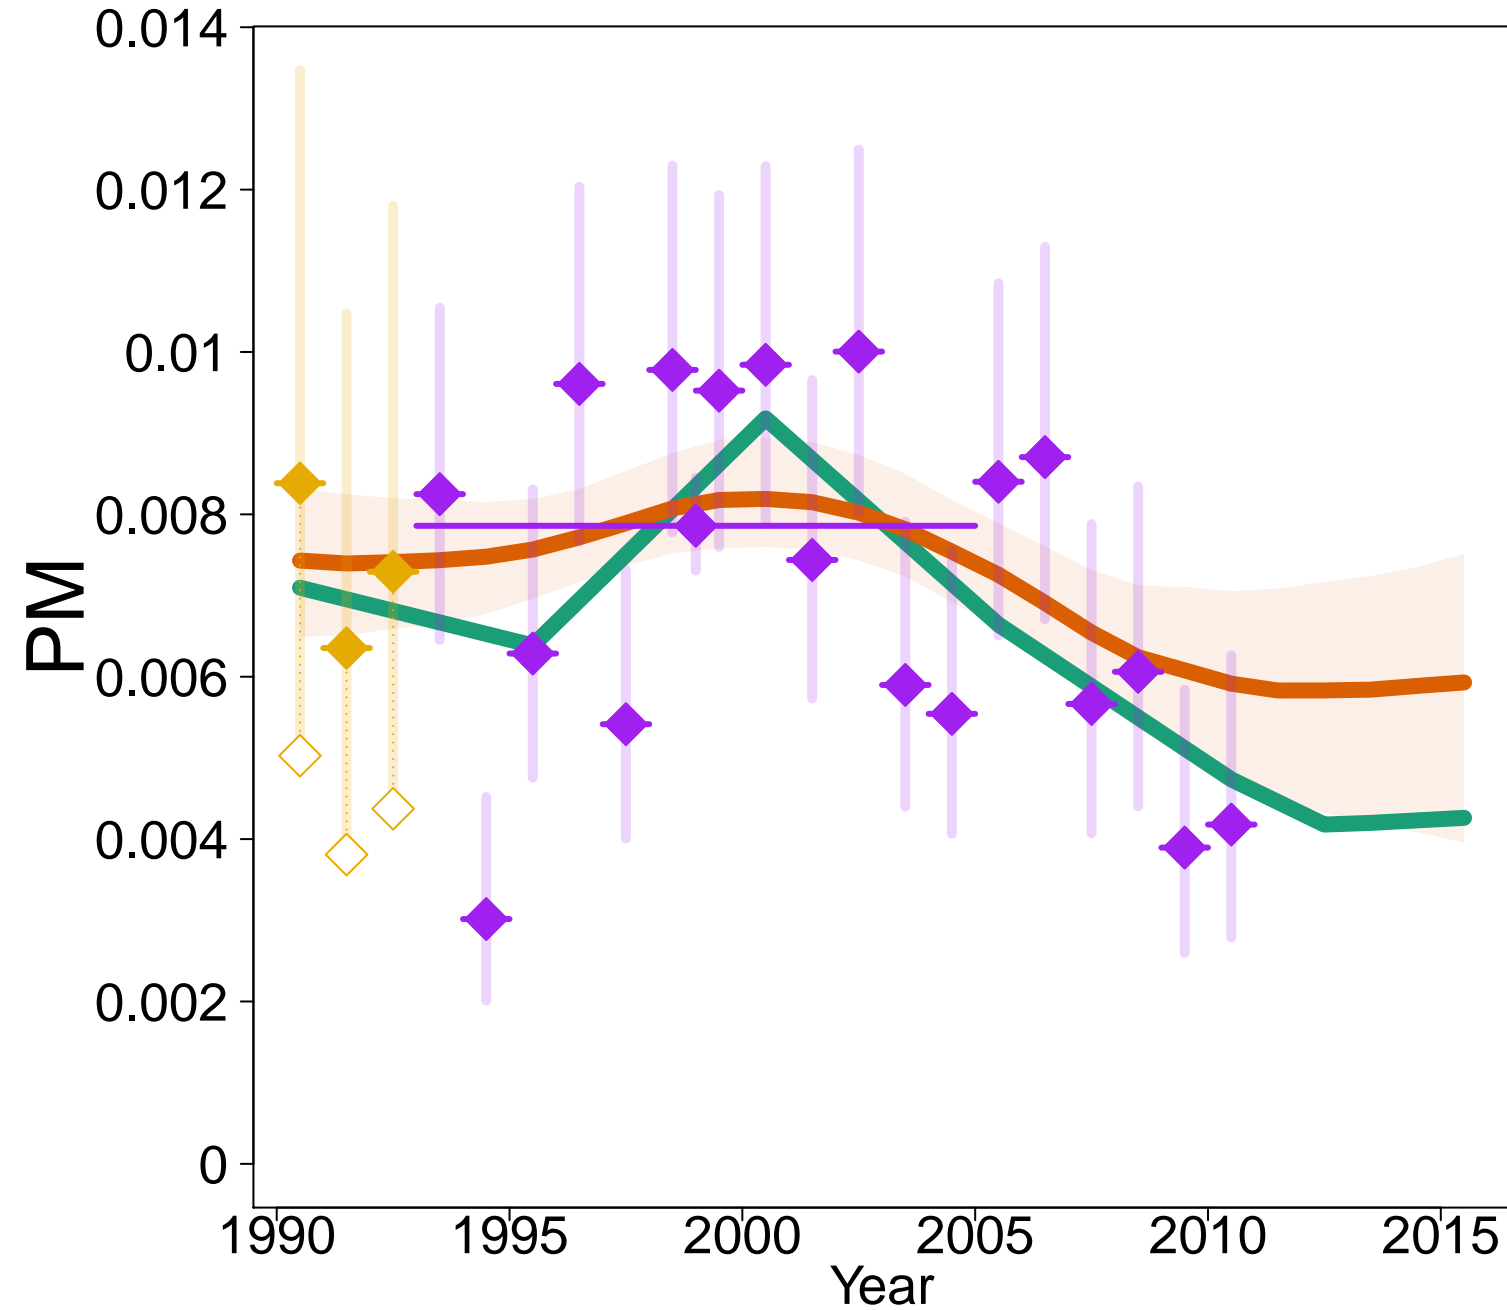

Netherlands [NLD; A]  
(Developed regions)

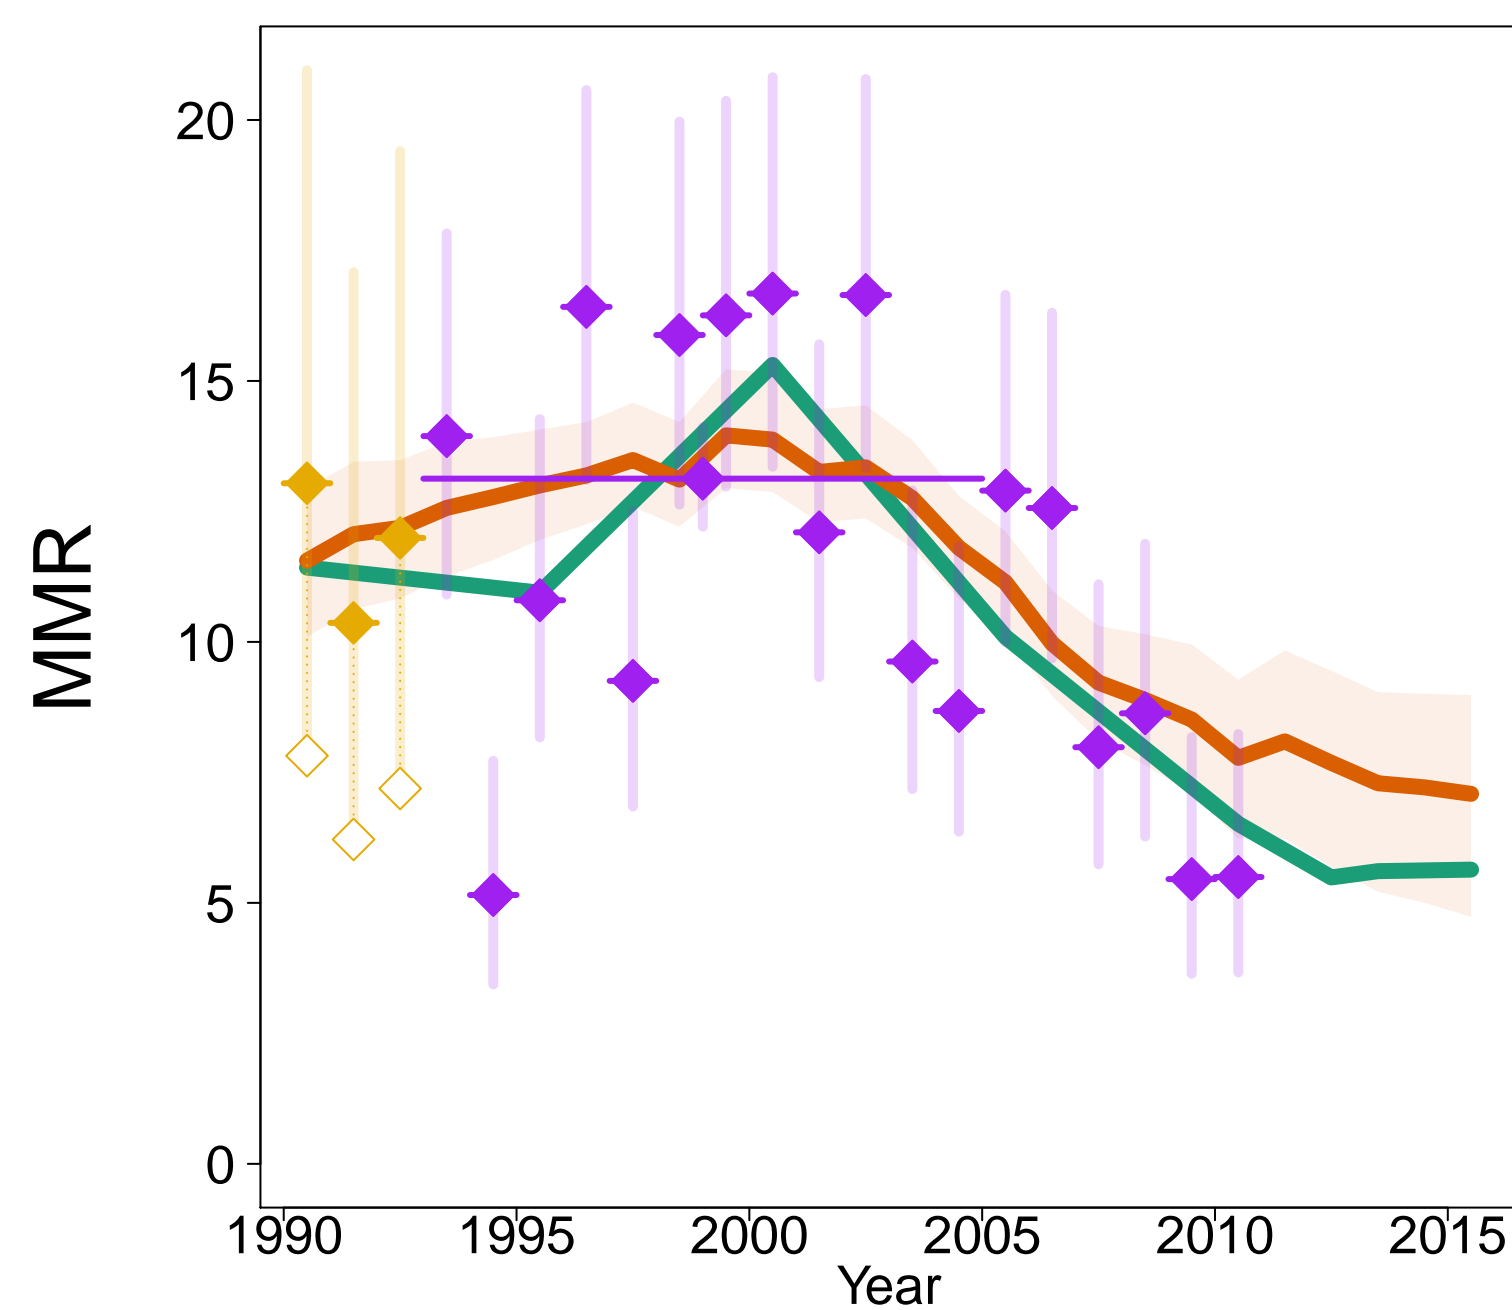

- Estimates –
- Bmat 2014
- MMEIG 2014
- Data –
- ◊ Observed Data
- ◆ Adjusted Data
- Data type –
- ◆ VR
- ◆ Spec. studies

New Zealand [NZL; A]  
(Developed regions)

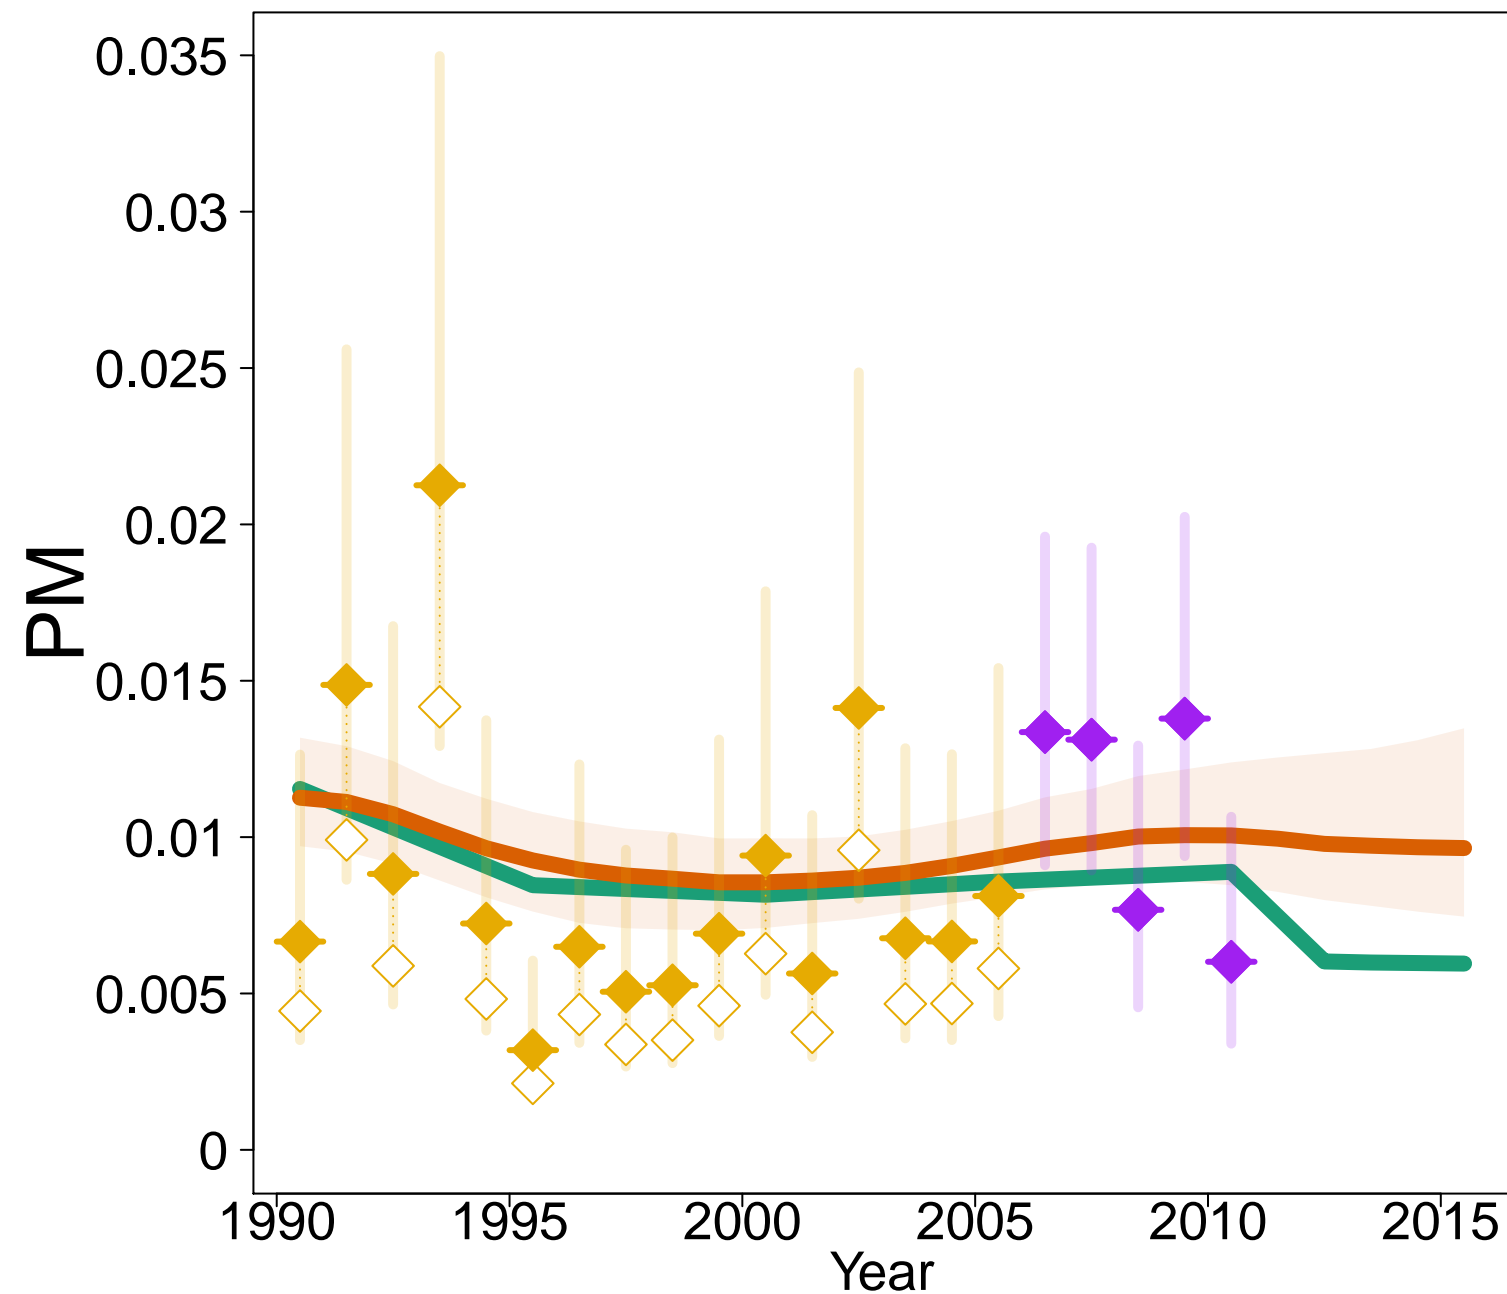

New Zealand [NZL; A]  
(Developed regions)

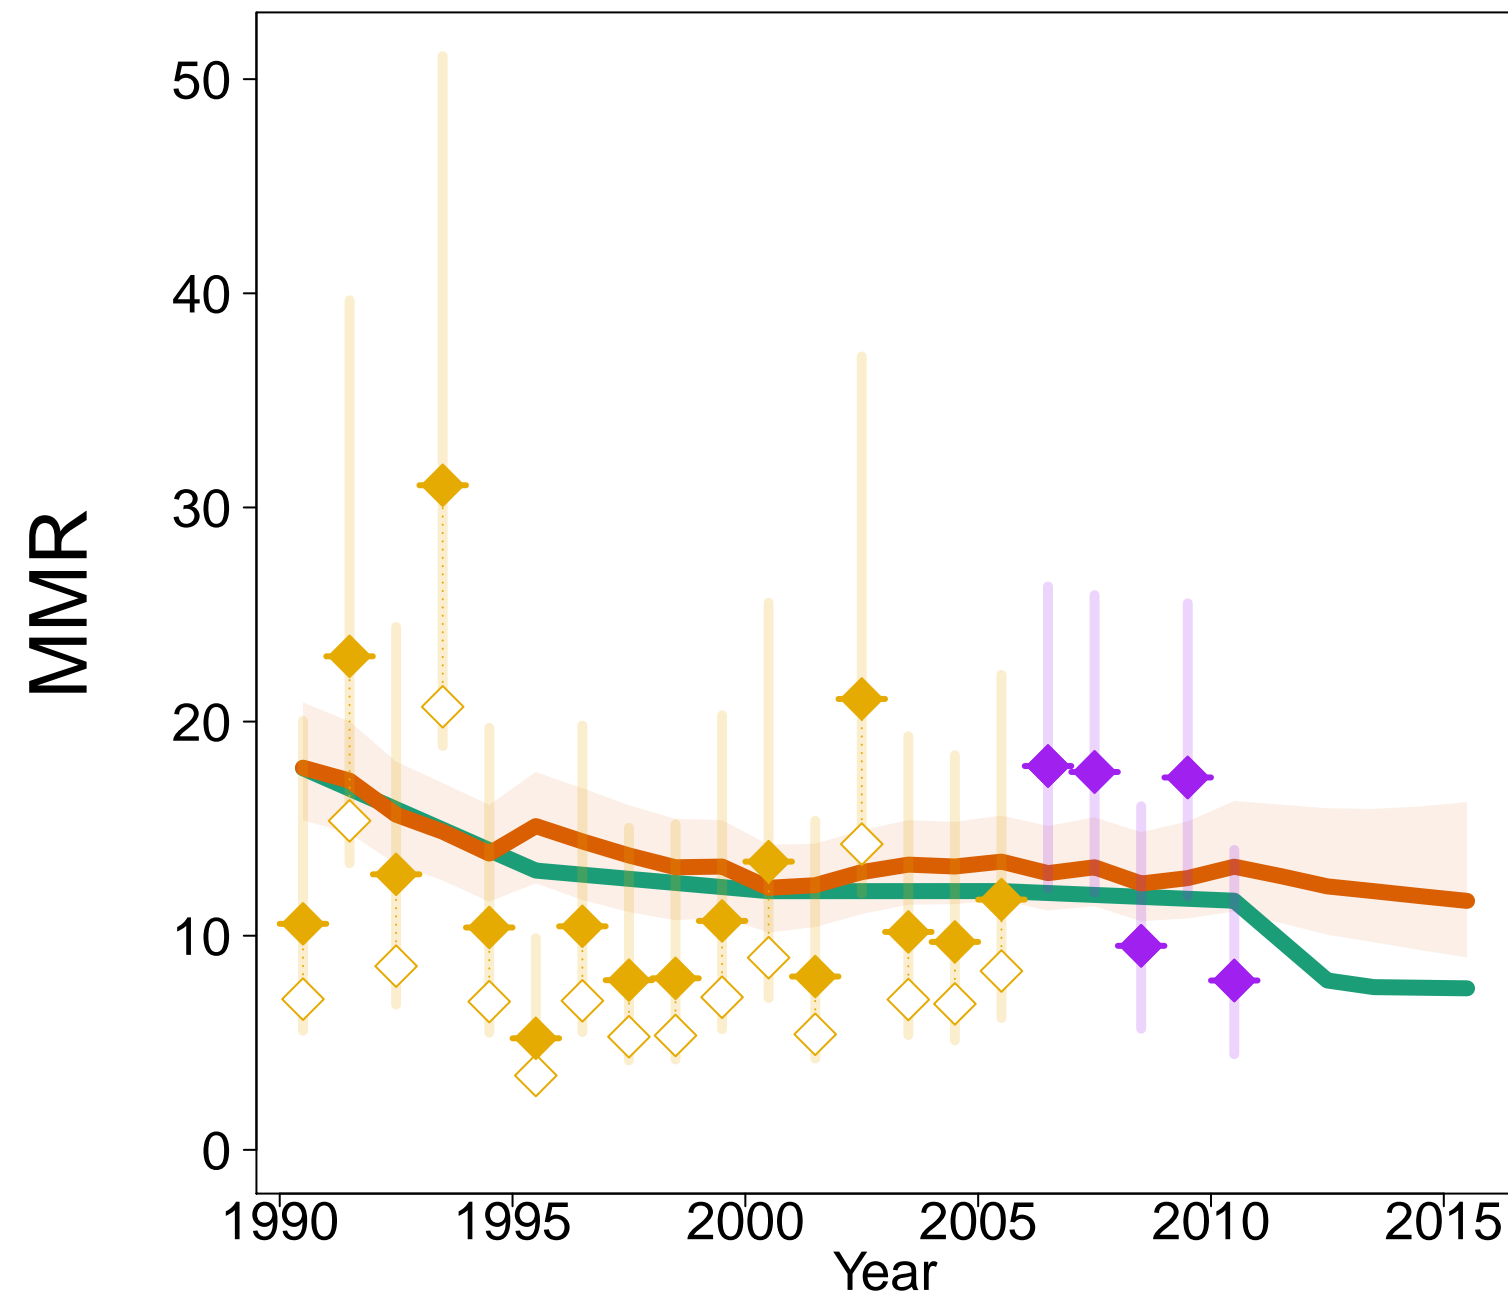

- Estimates –
- Bmat 2014
- MMEIG 2014
- Data –
- ◊ Observed Data
- ◆ Adjusted Data
- Data type –
- ◆ VR
- ◆ Spec. studies

Nicaragua [NIC; B]  
(Central America)

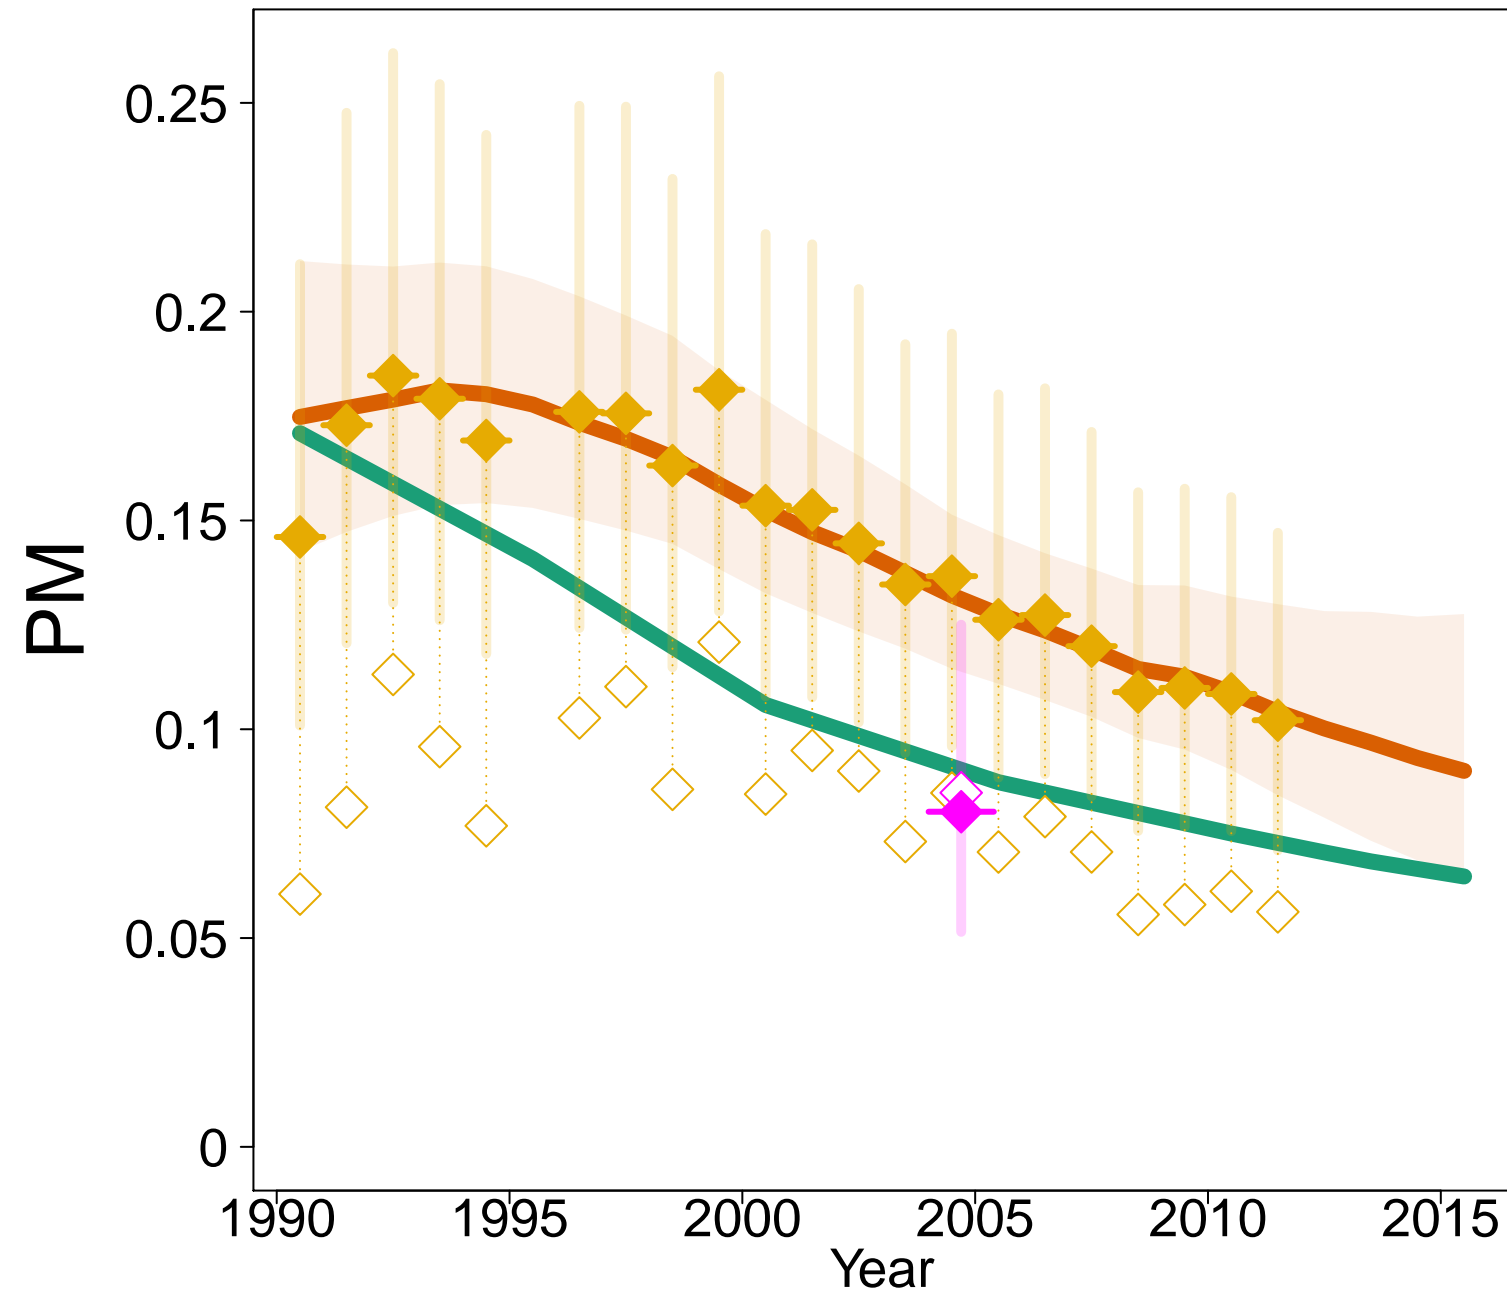

Nicaragua [NIC; B]  
(Central America)

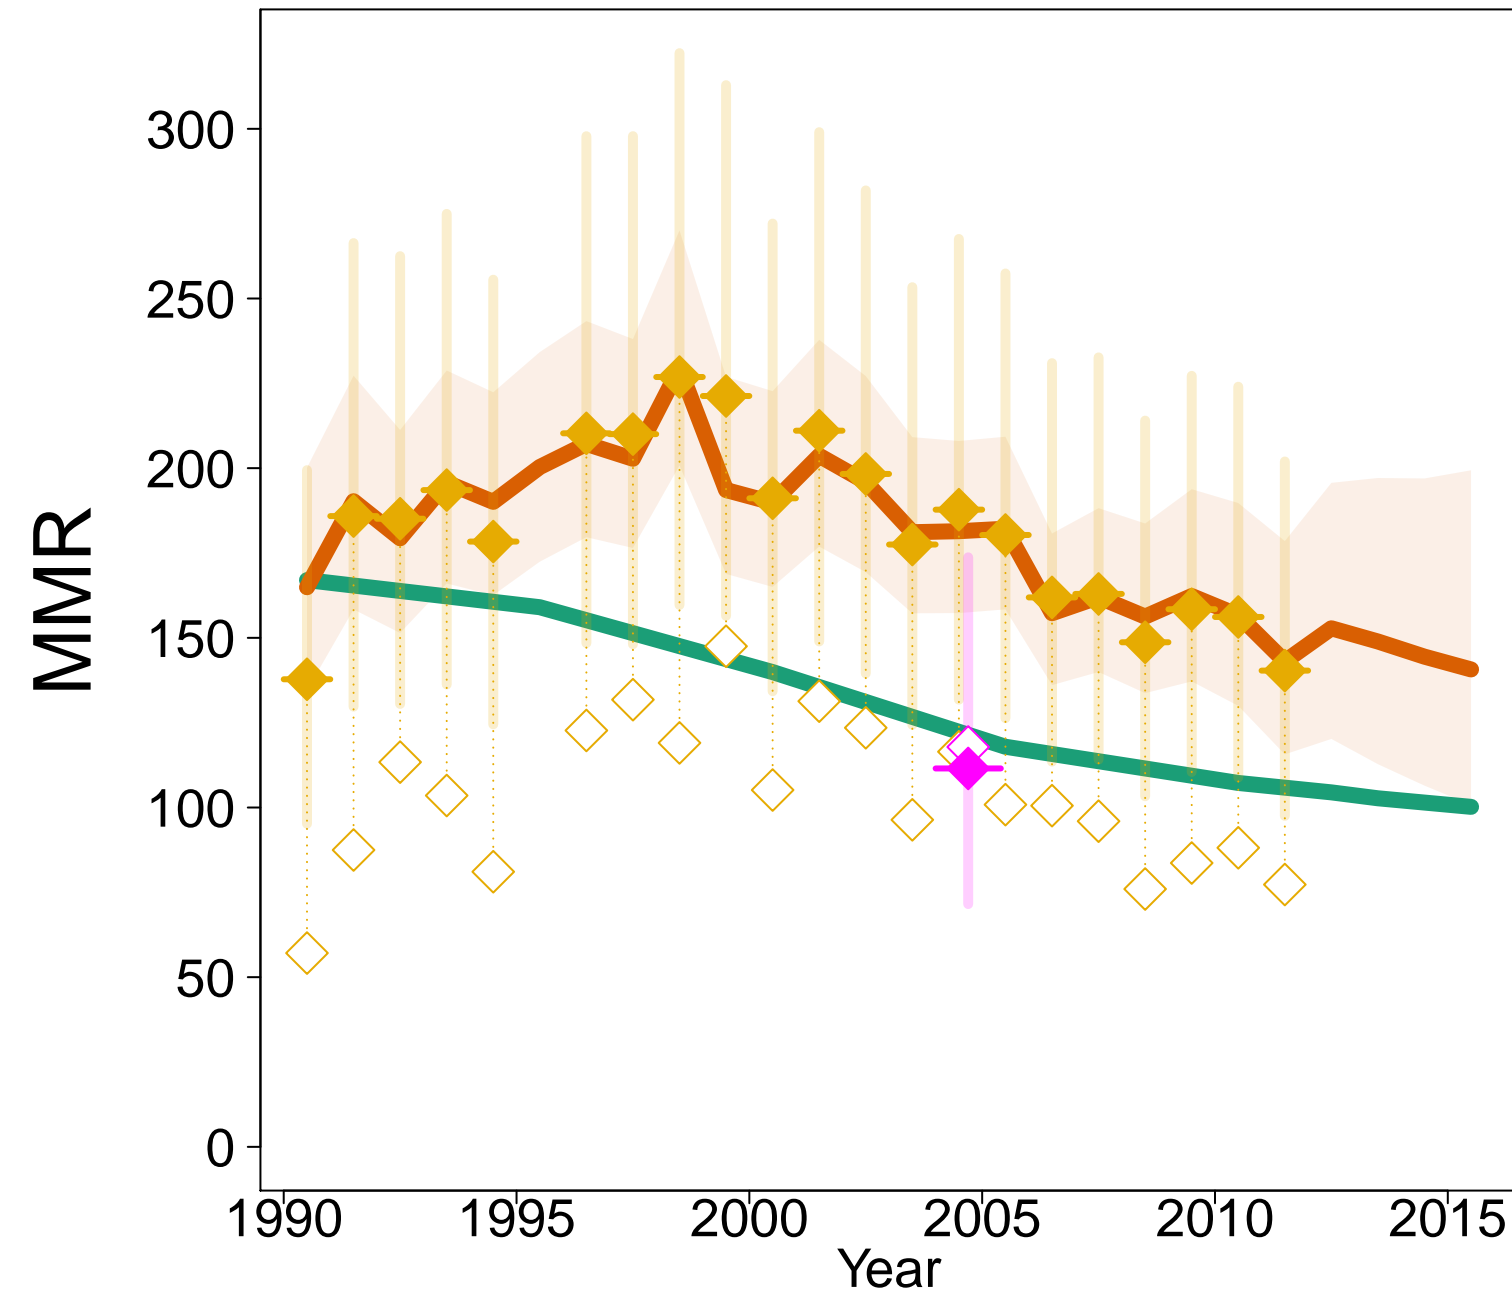

- Estimates –
- Bmat 2014
- MMEIG 2014
- Data –
- Observed Data
- Adjusted Data
- Data type –
- VR
- Census

Niger [NER; B]  
(Western Africa)

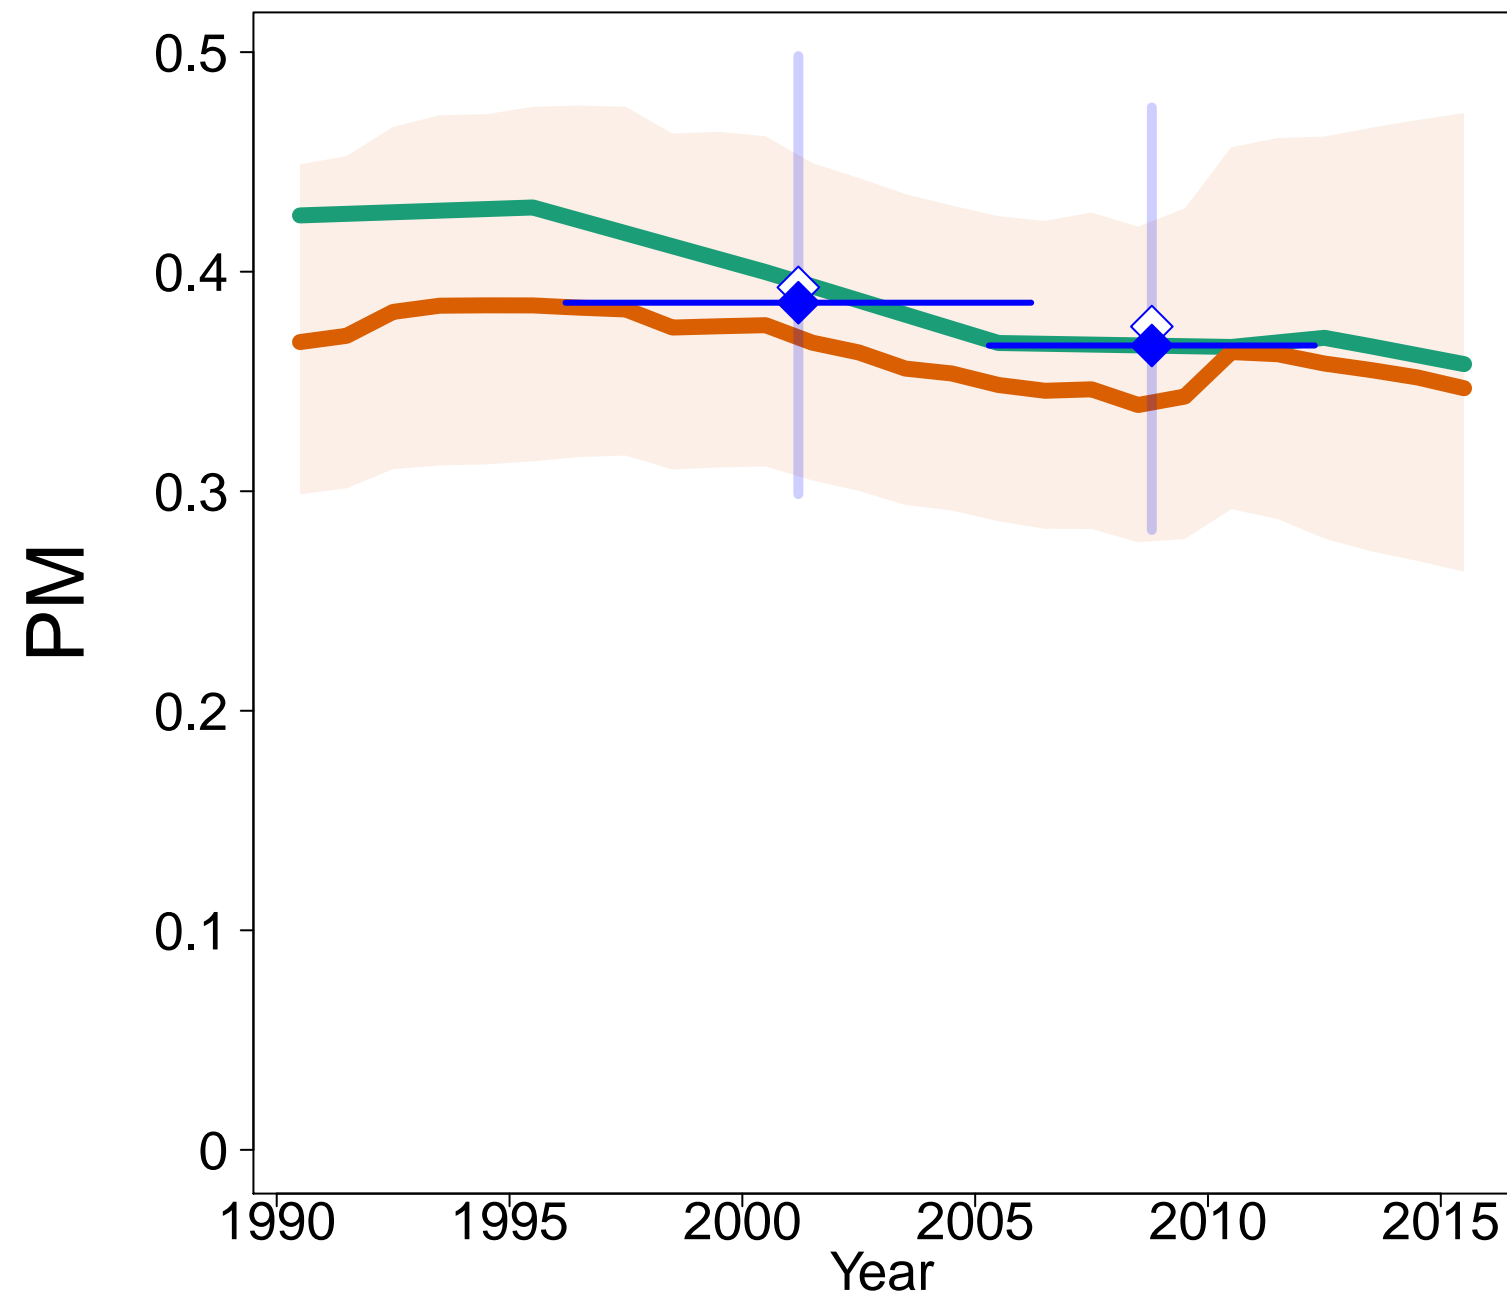

Niger [NER; B]  
(Western Africa)

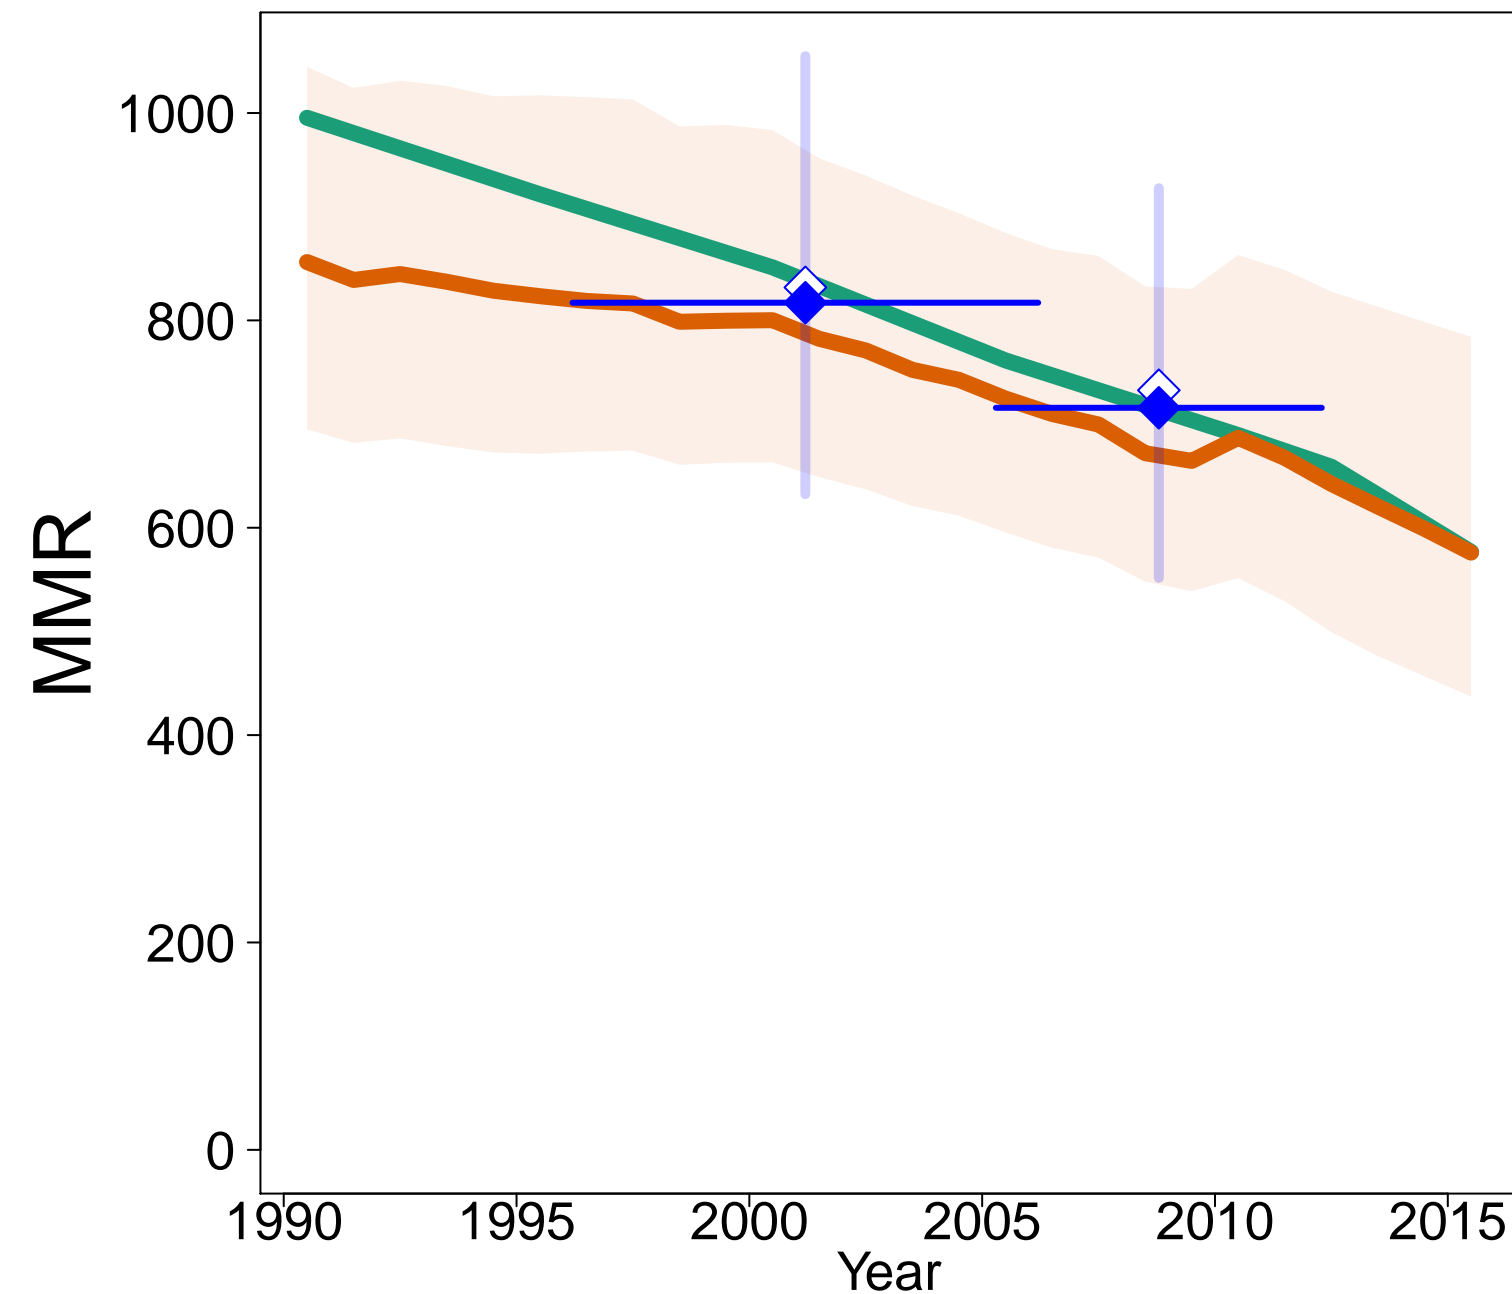

- Estimates –
- Bmat 2014
- MMEIG 2014
- Data –
- Observed Data
- Adjusted Data
- Data type –
- DHS

Nigeria [NGA; B]  
(Western Africa)

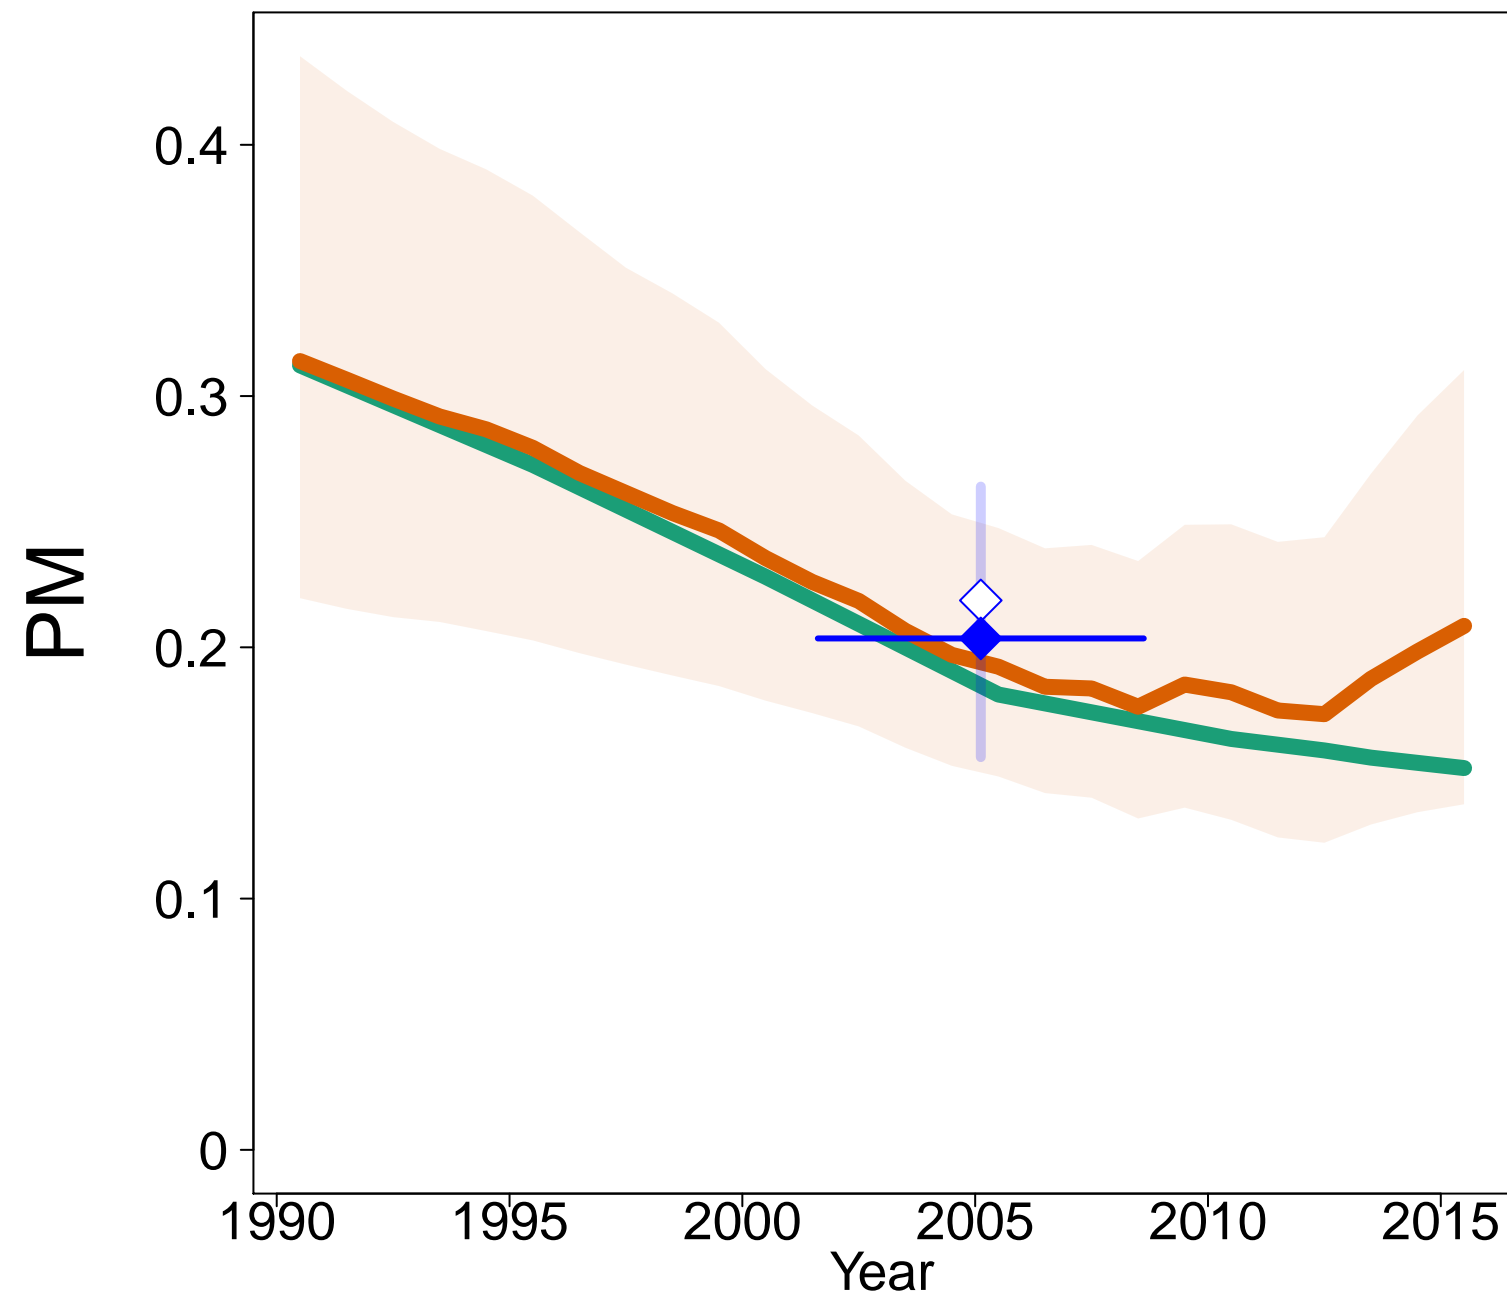

Nigeria [NGA; B]  
(Western Africa)

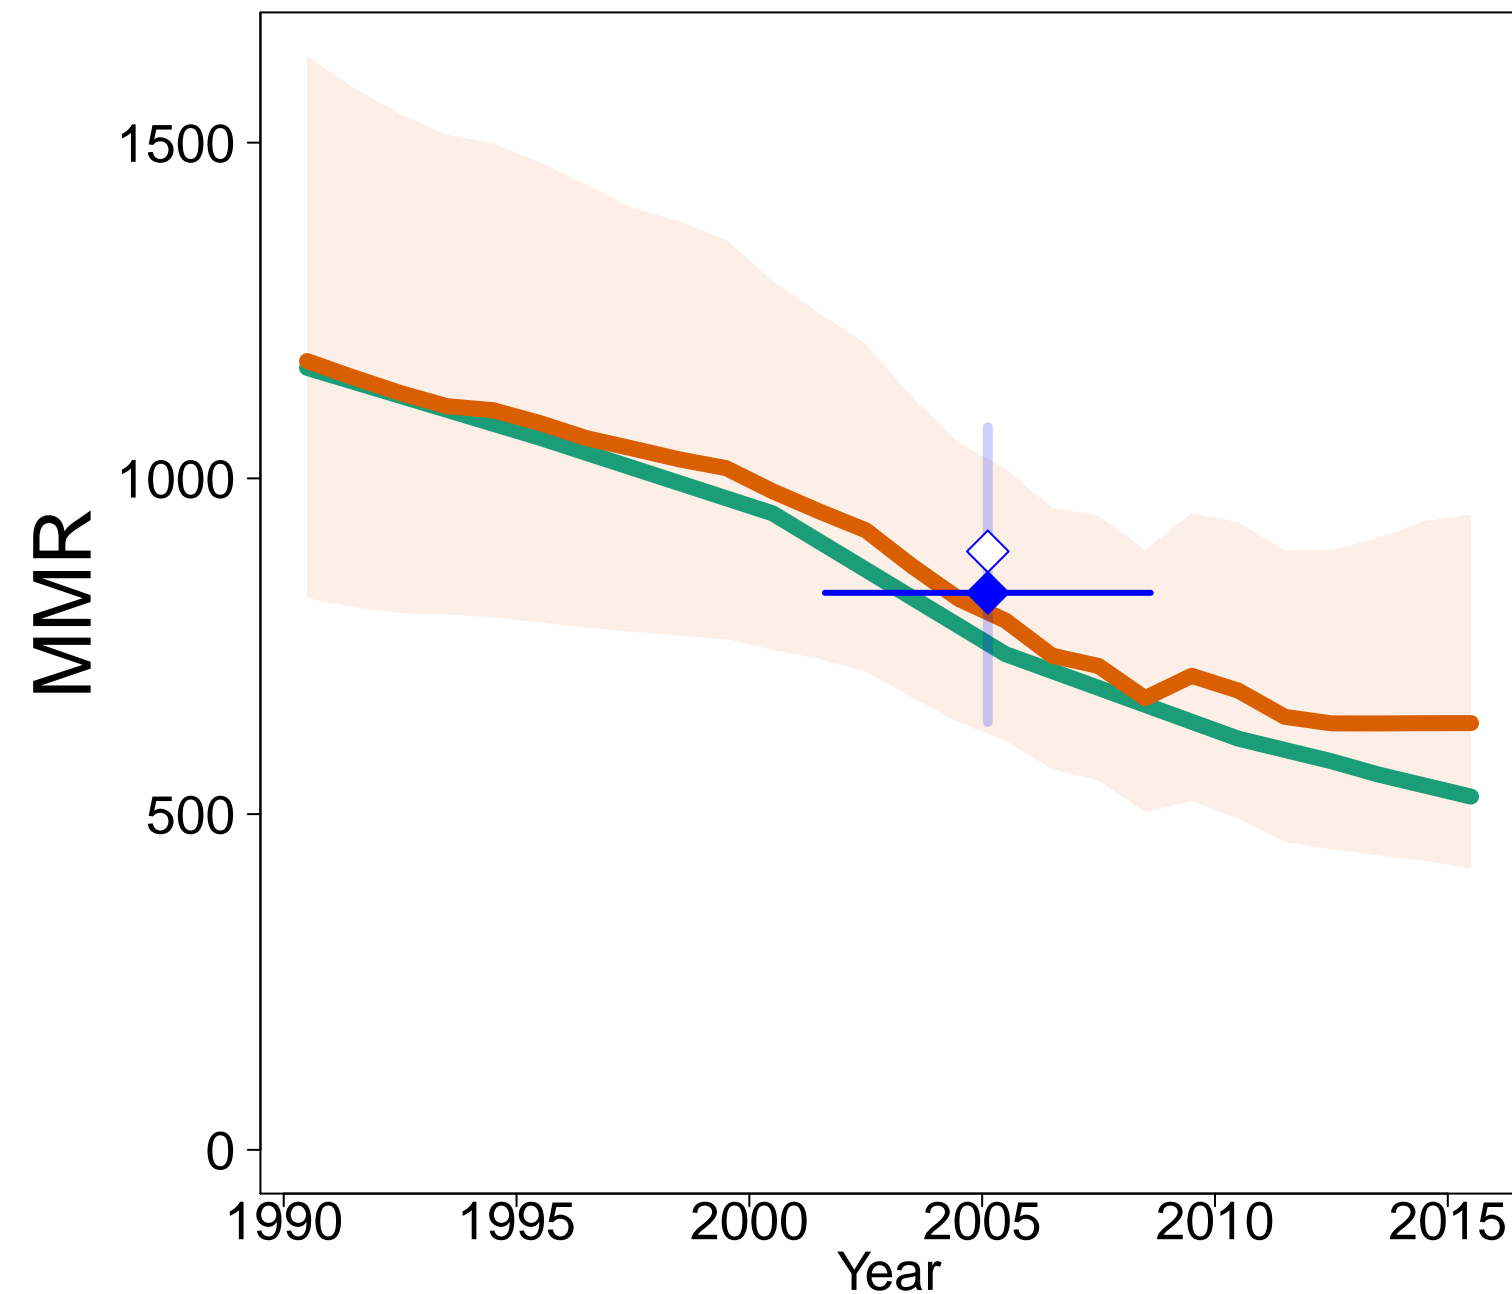

- Estimates –
- Bmat 2014
- MMEIG 2014
- Data –
- Observed Data
- Adjusted Data
- Data type –
- DHS

Norway [NOR; A]  
(Developed regions)

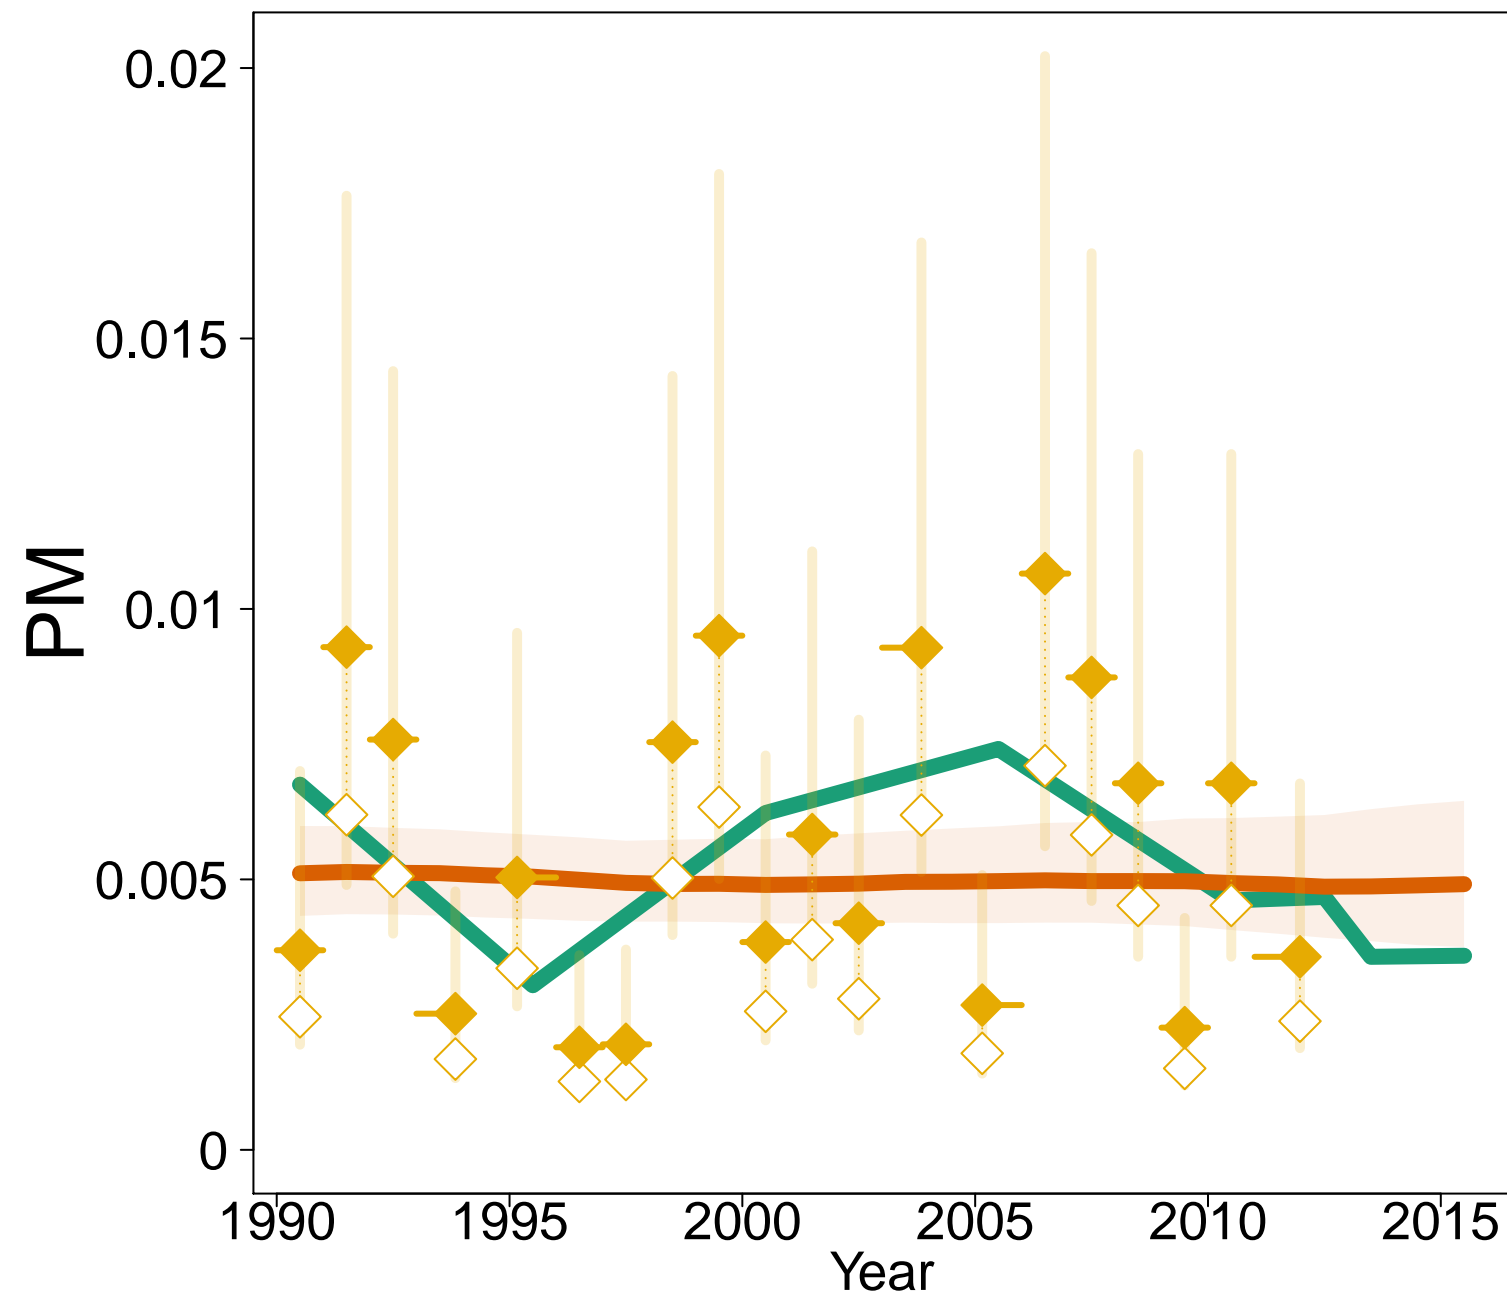

Norway [NOR; A]  
(Developed regions)

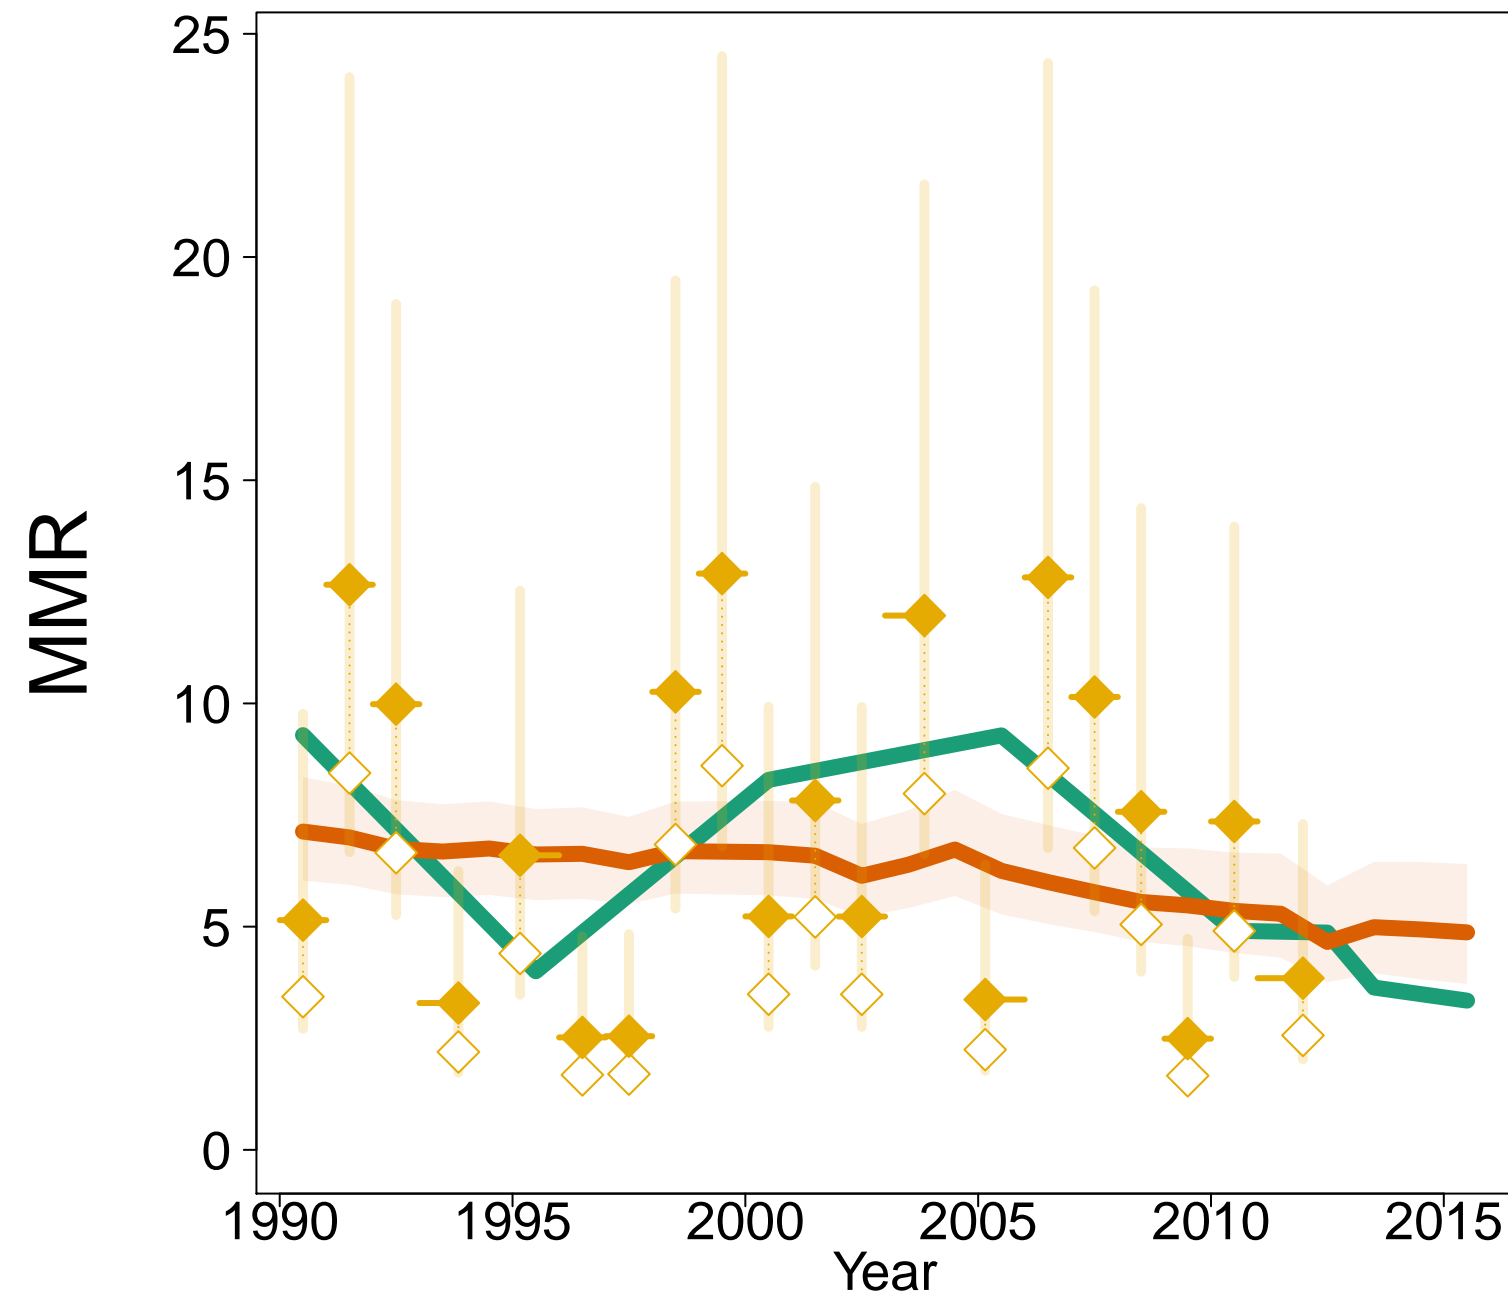

– Estimates –  
Bmat 2014  
MMEIG 2014  
– Data –  
Observed Data  
Adjusted Data  
– Data type –  
VR

Occupied Palestinian Territory [PSE; C]  
(Western Asia)

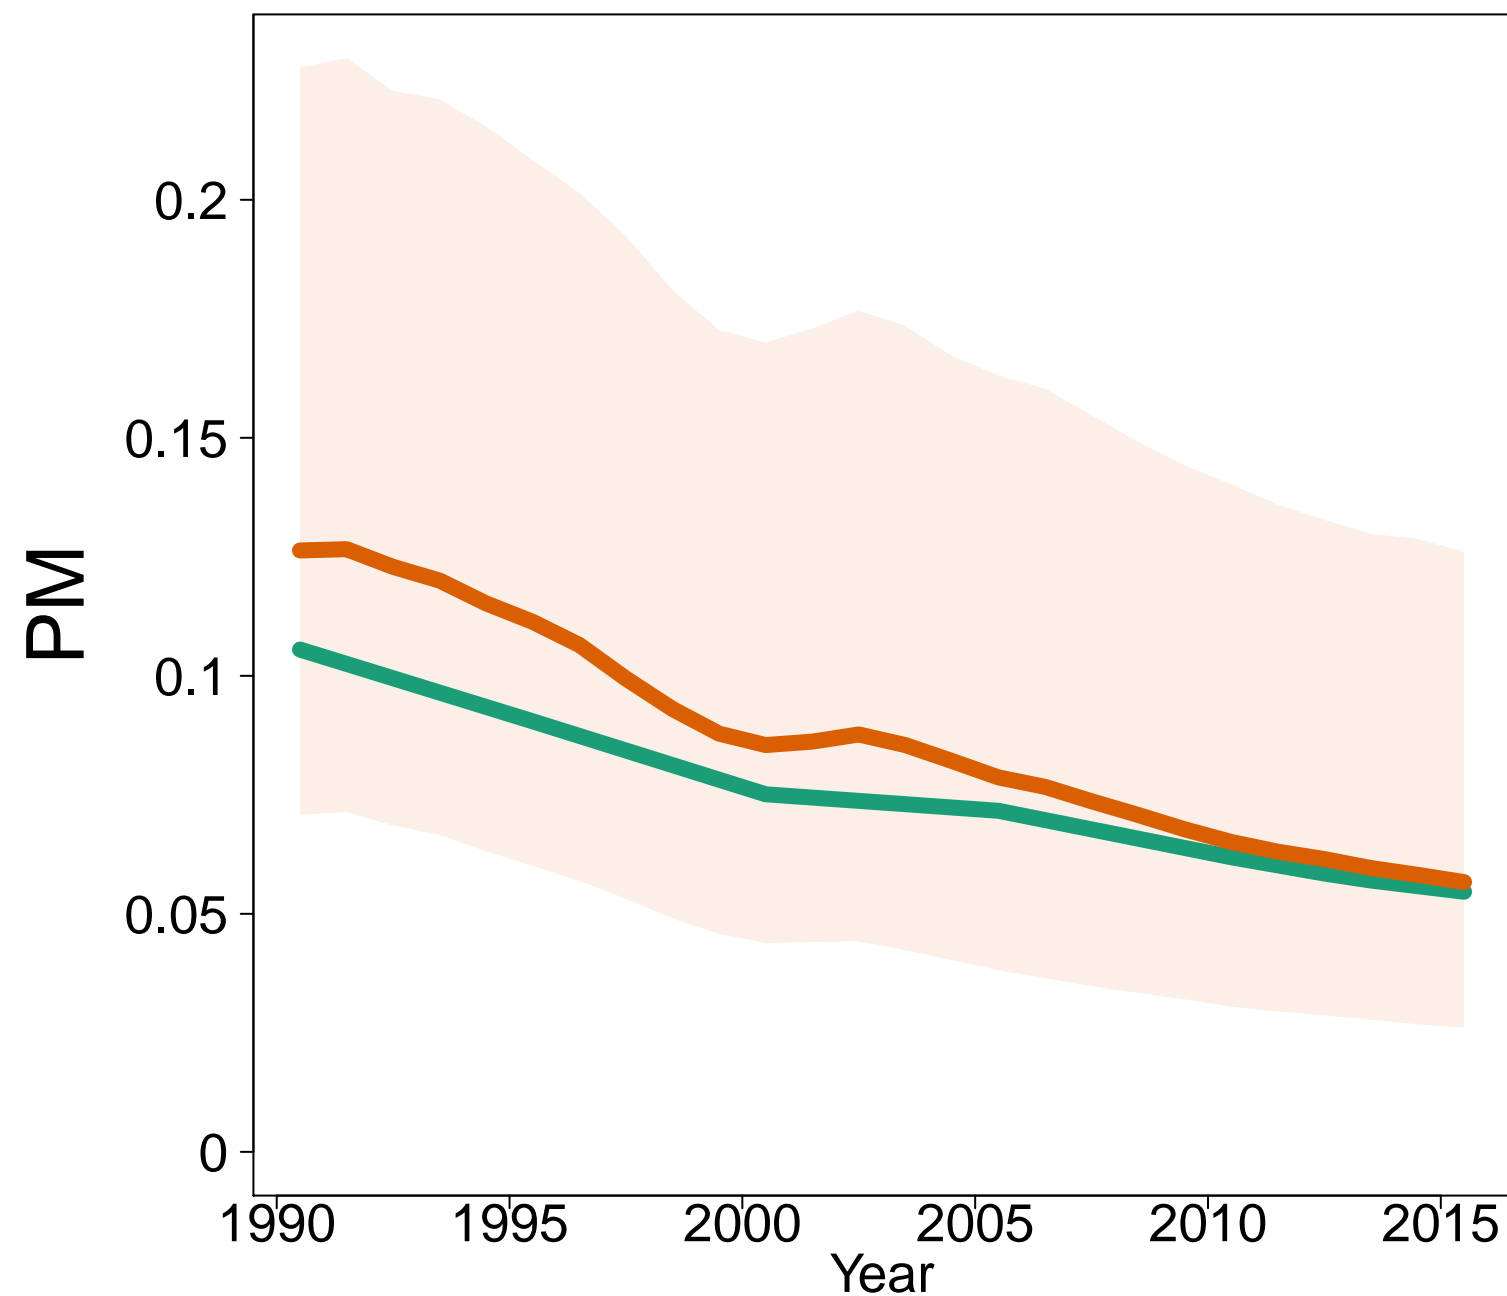

Occupied Palestinian Territory [PSE; C]  
(Western Asia)

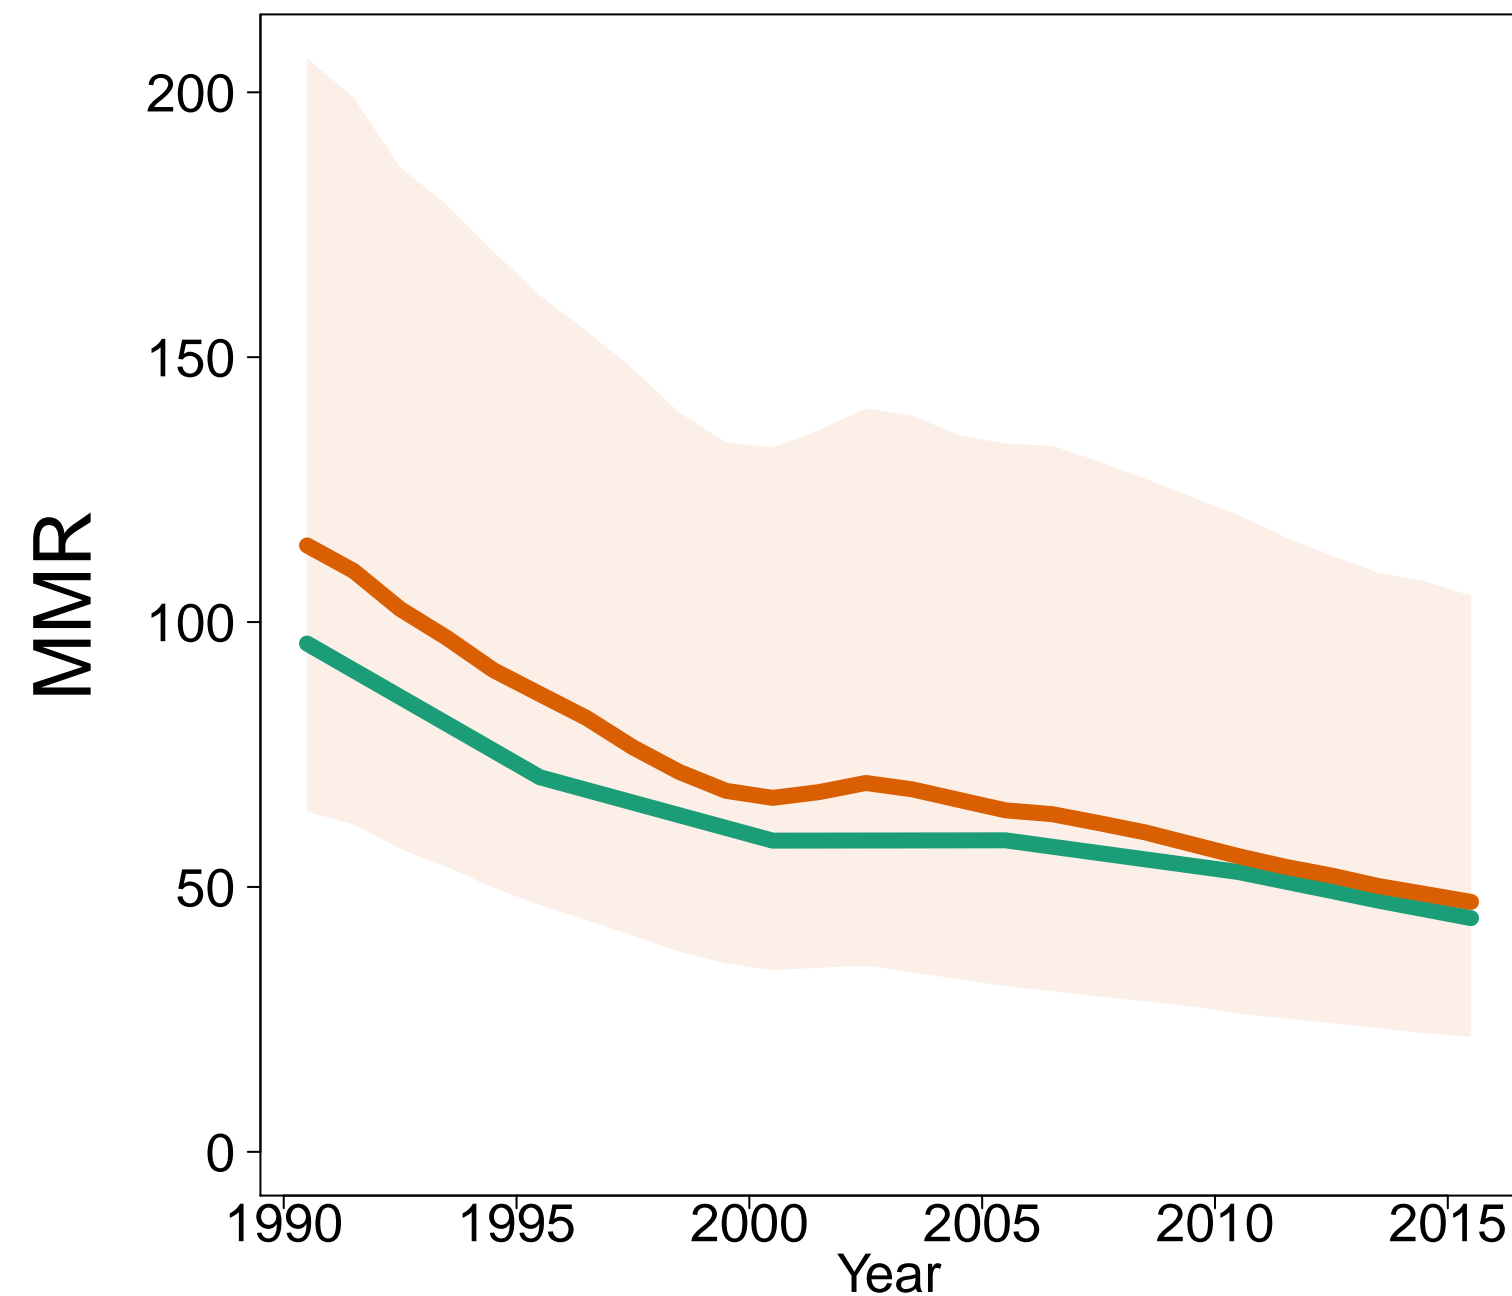

– Estimates –  
Bmat 2014  
MMEIG 2014  
– Data –



Oman [OMN; B]  
(Western Asia)

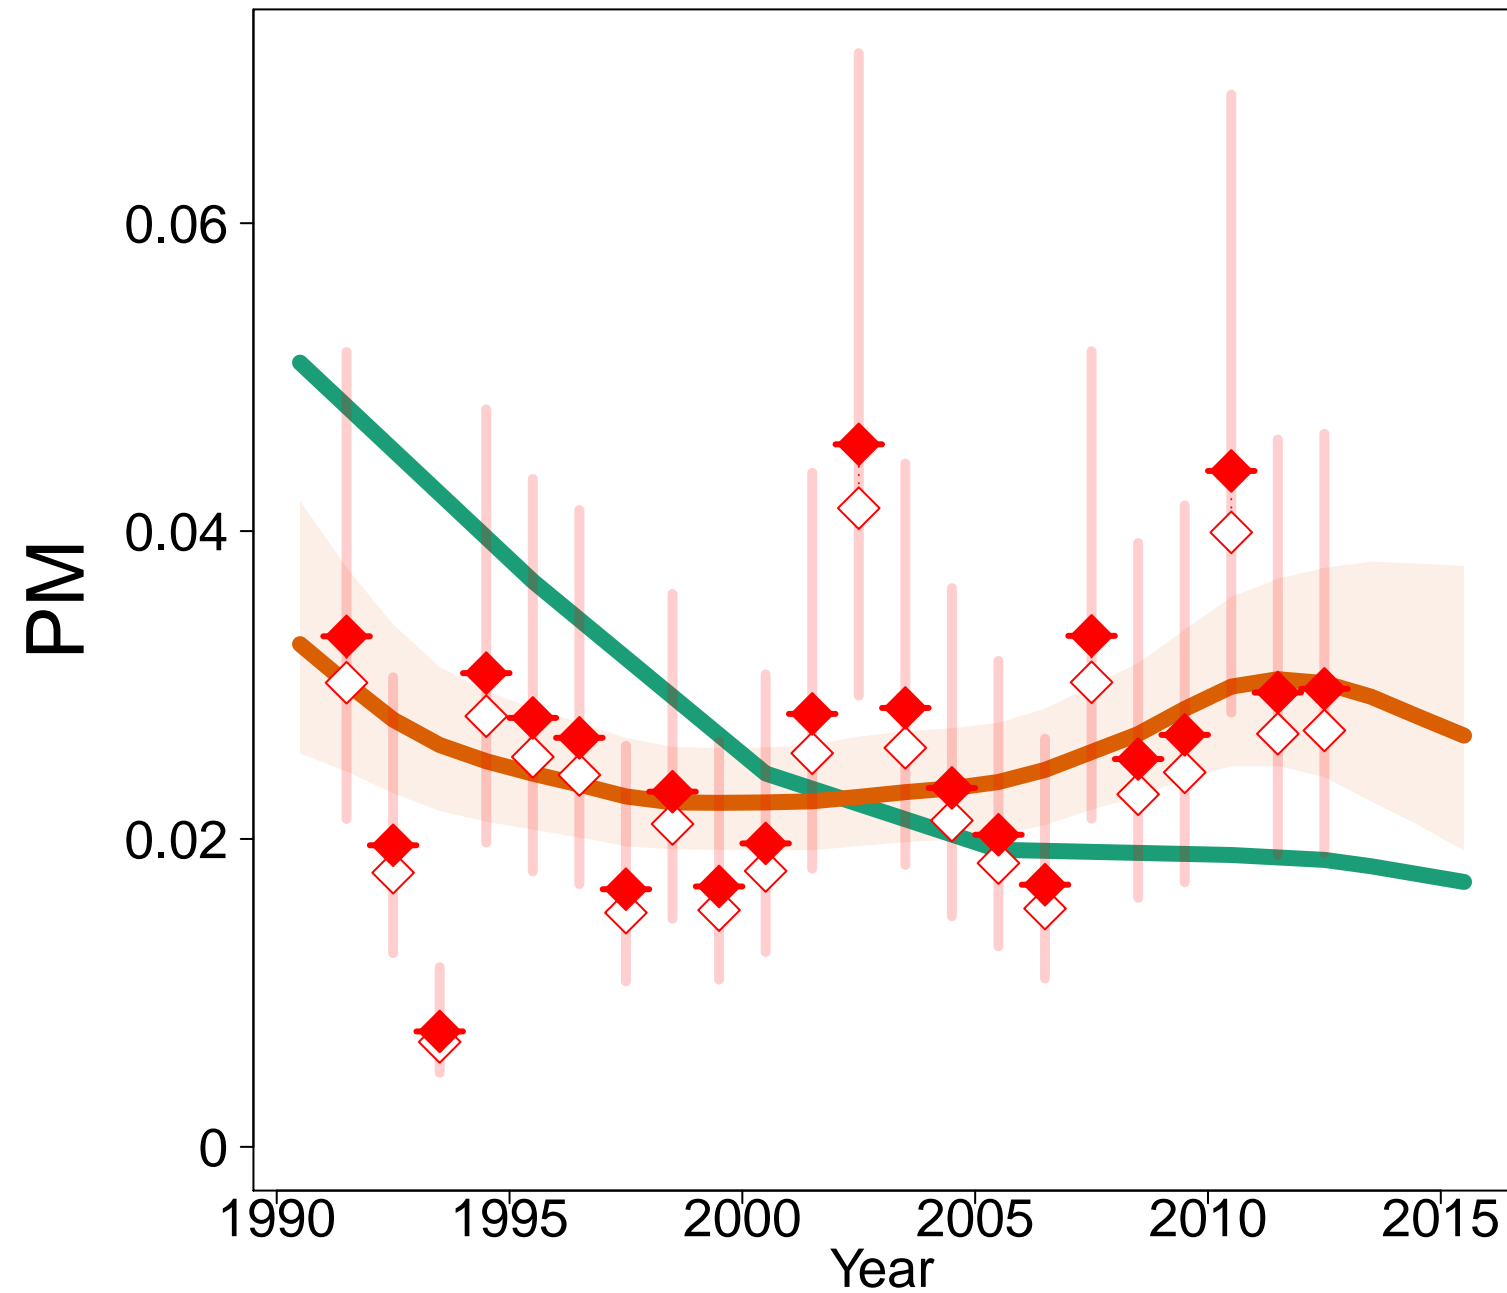

Oman [OMN; B]  
(Western Asia)

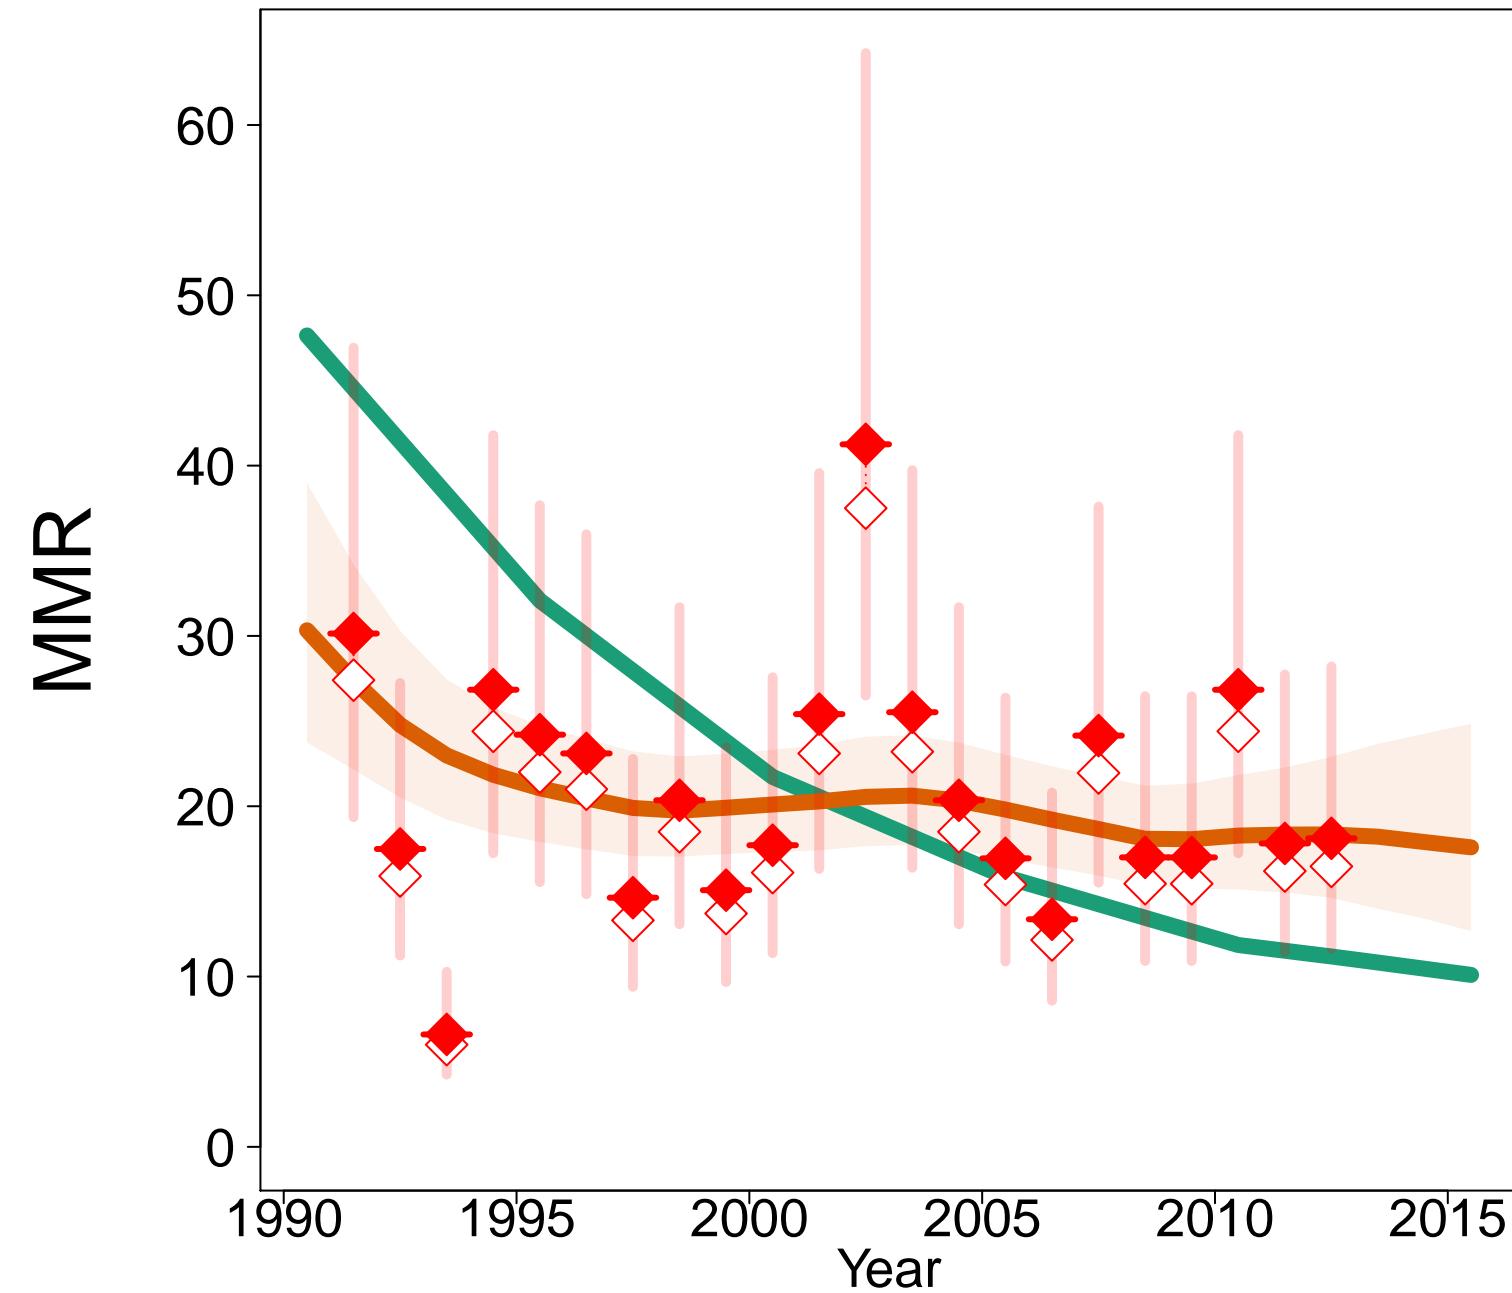

Pakistan [PAK; B]  
(Southern Asia)

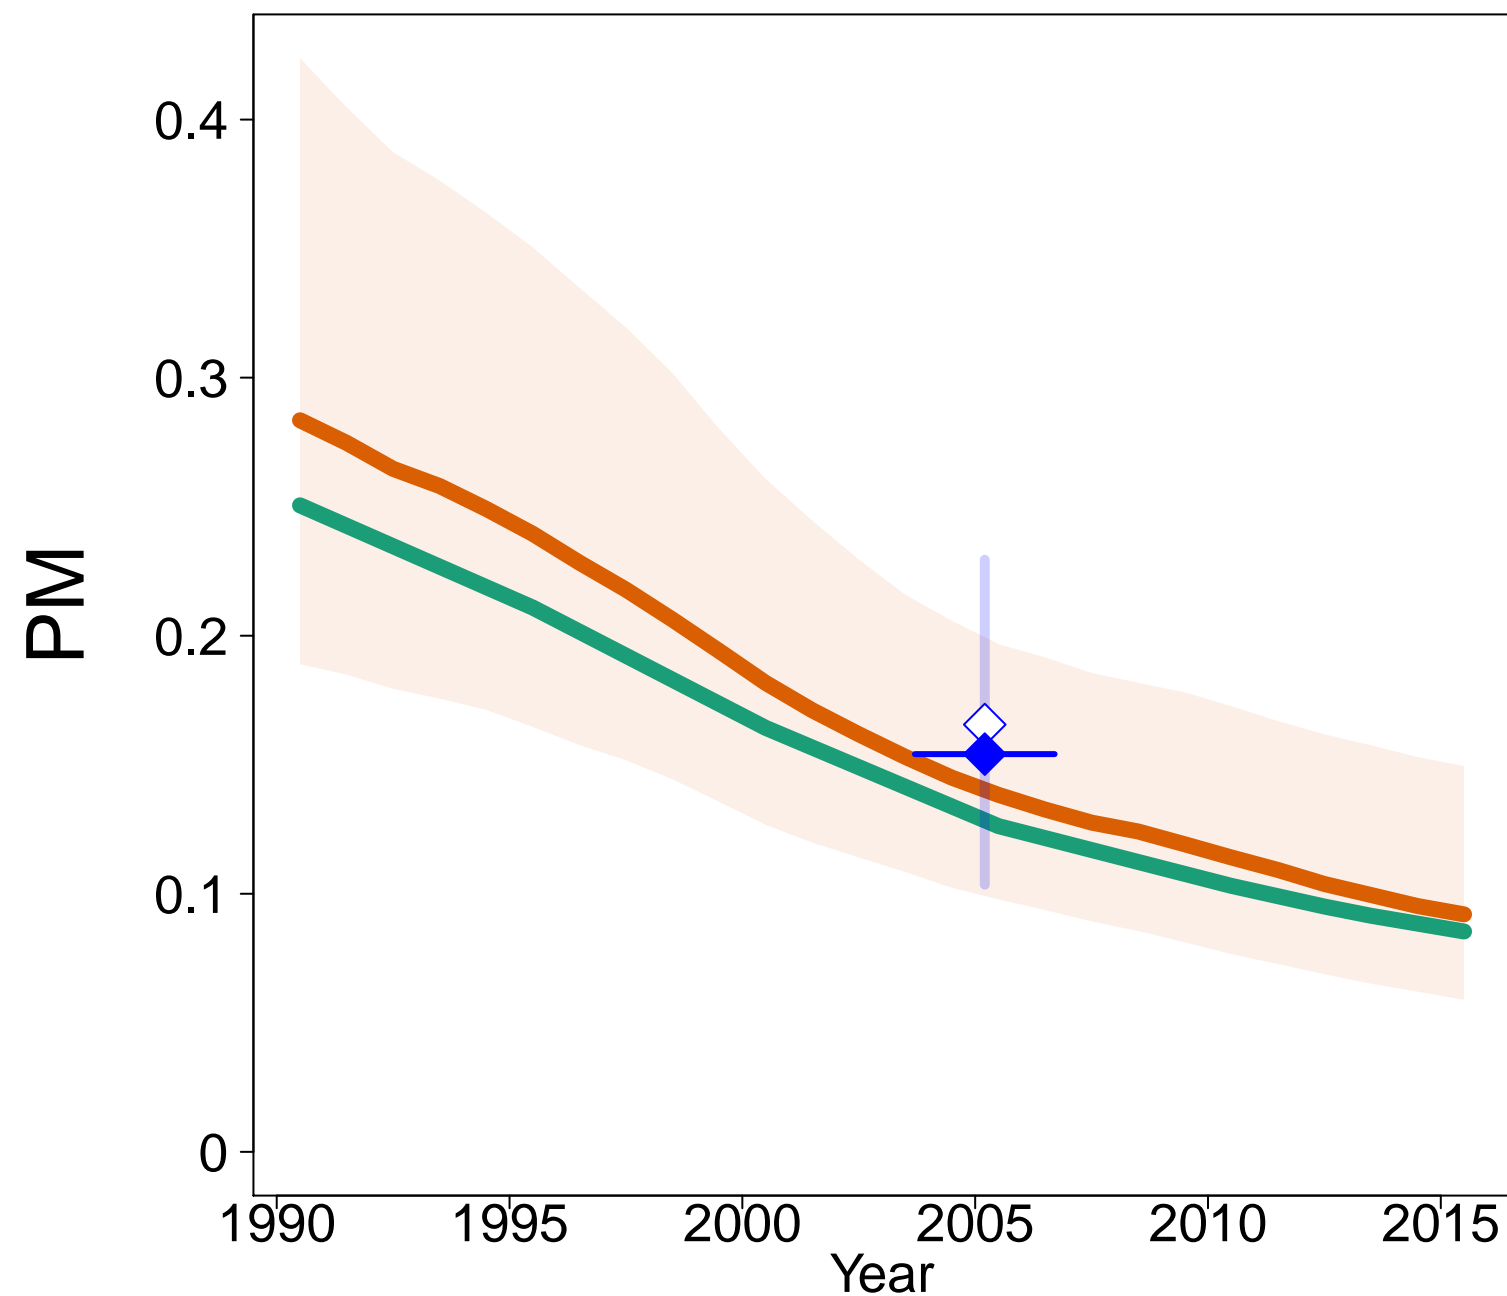

Pakistan [PAK; B]  
(Southern Asia)

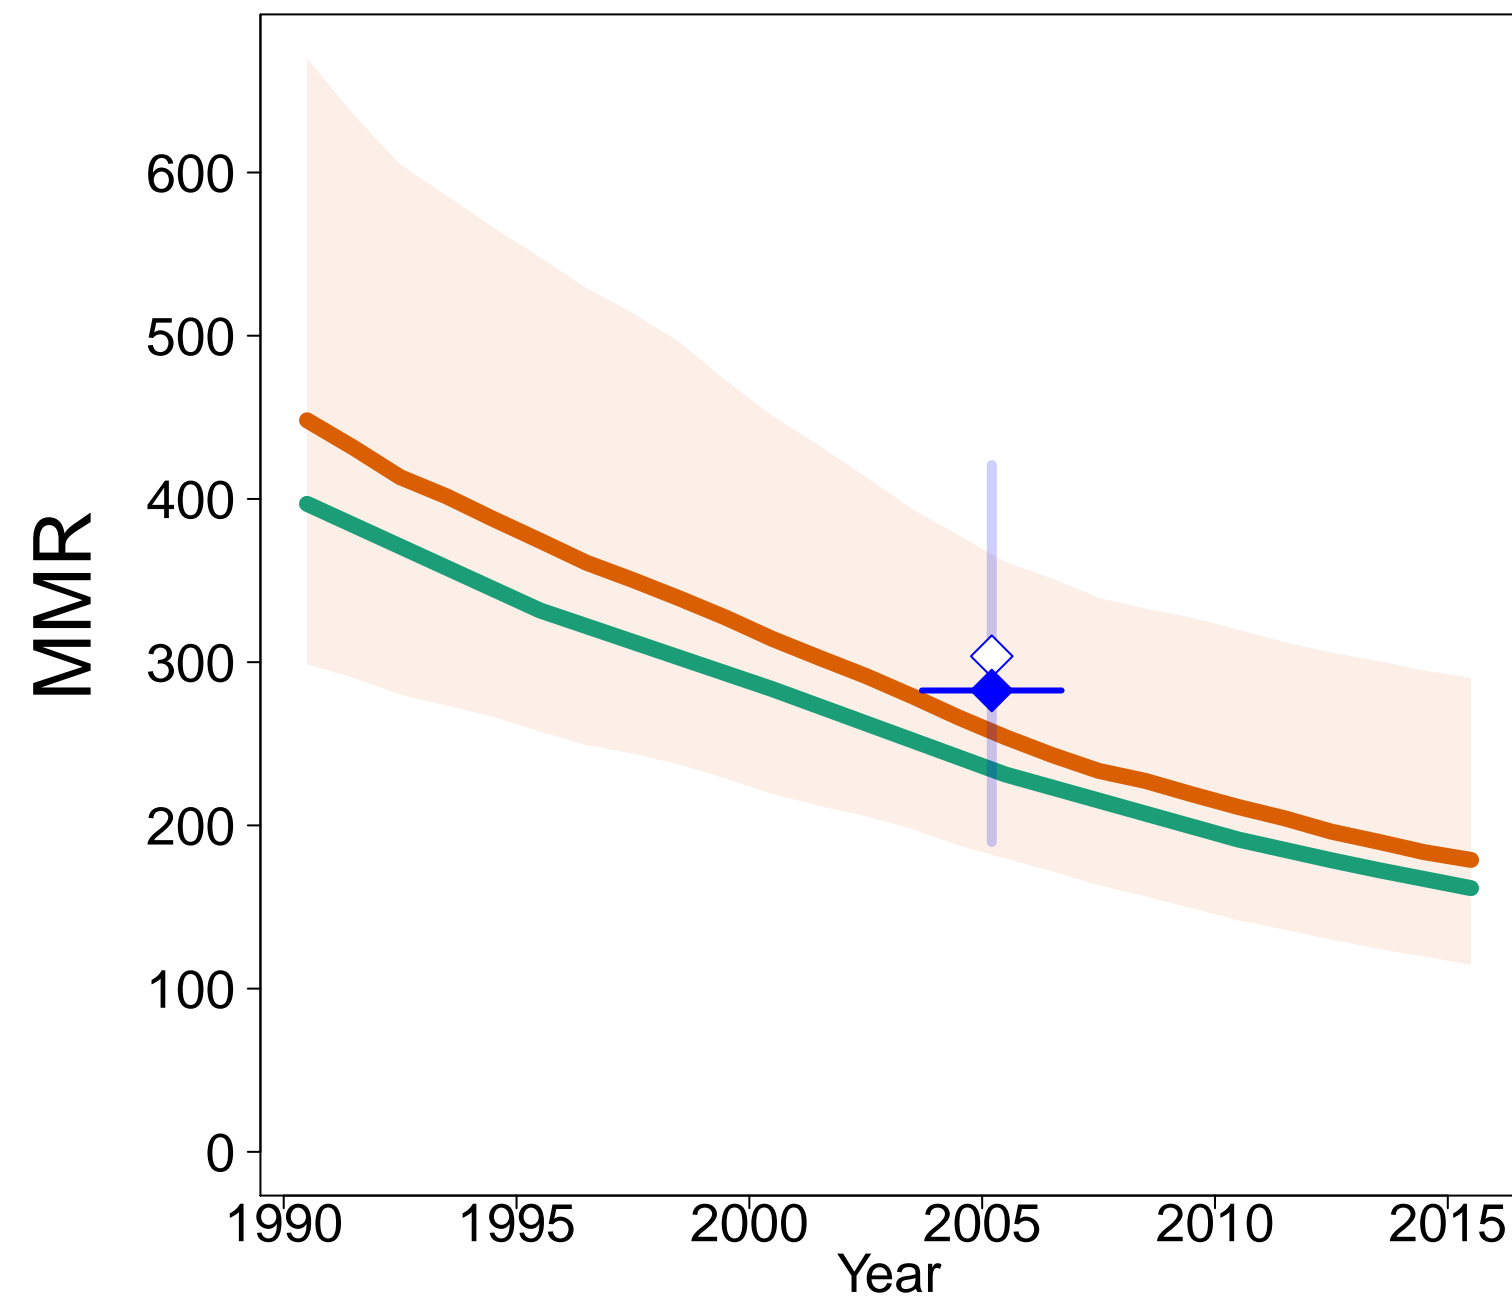

- Estimates –
- Bmat 2014
- MMEIG 2014
- Data –
- Observed Data
- Adjusted Data
- Data type –
- DHS

Panama [PAN; A]  
(Central America)

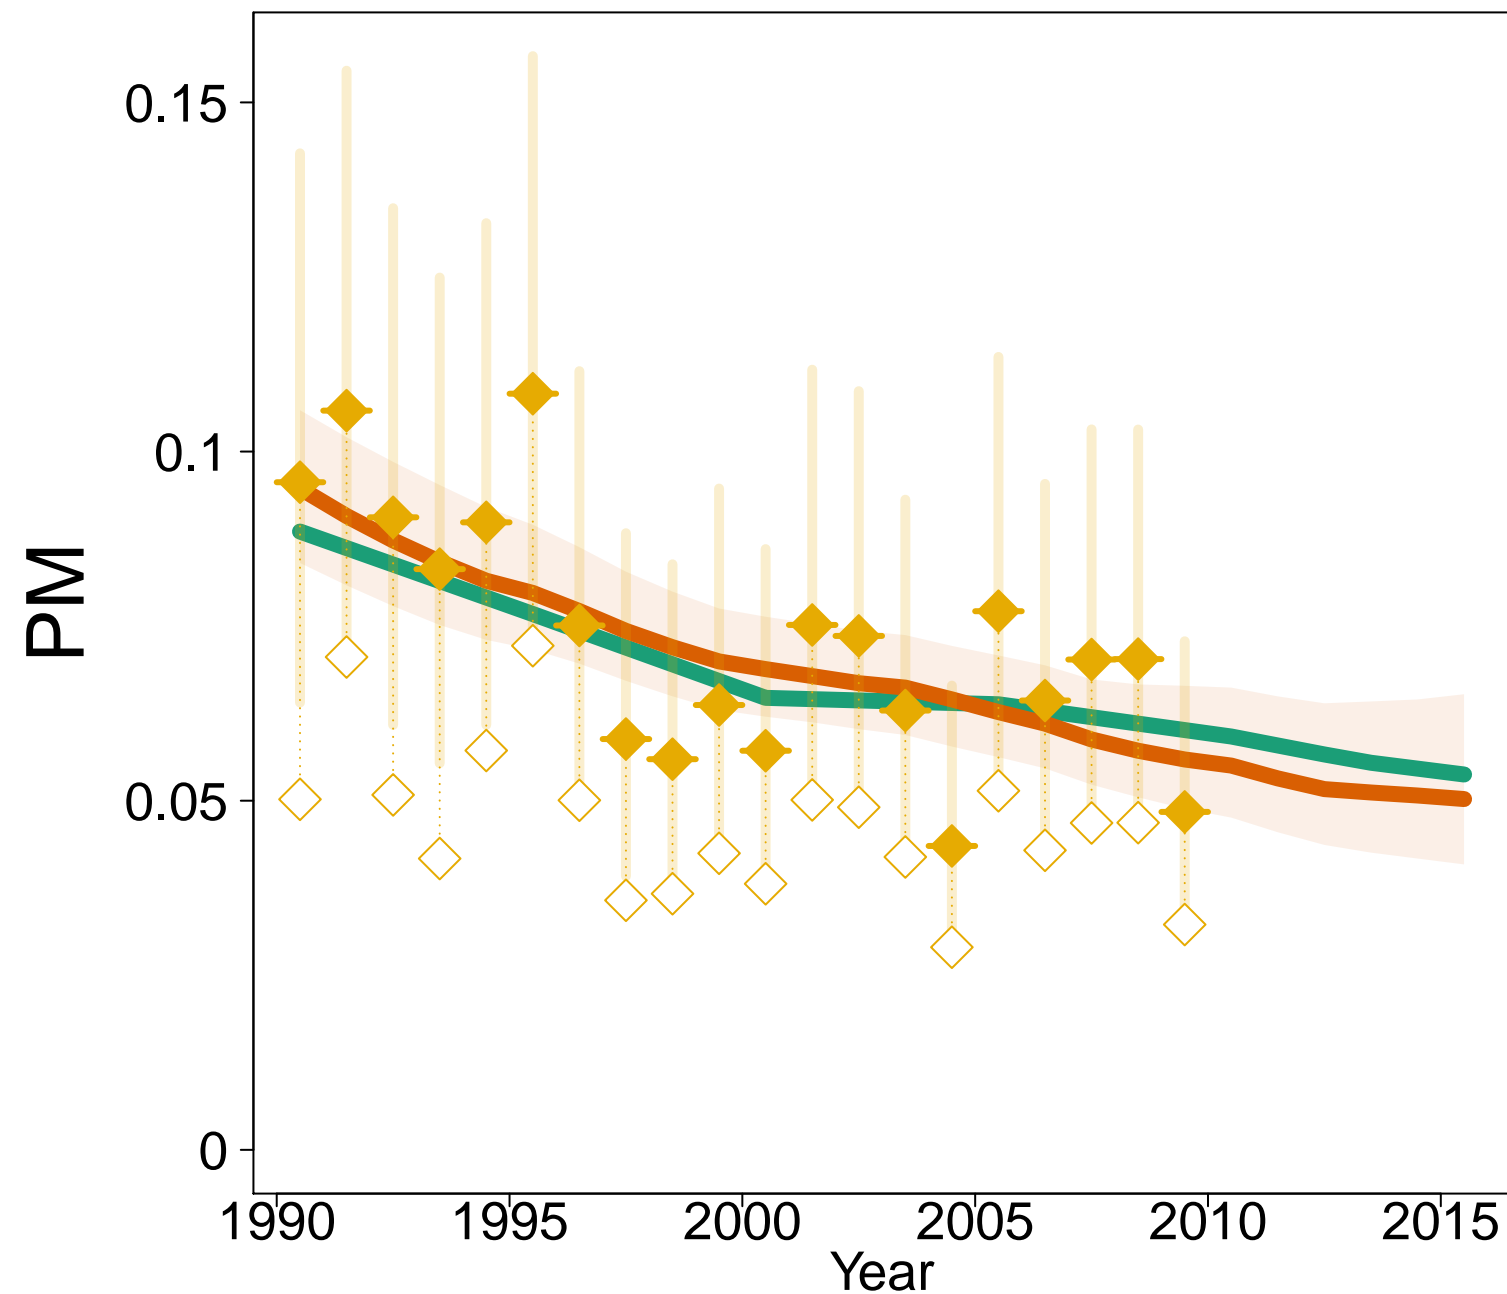

Panama [PAN; A]  
(Central America)

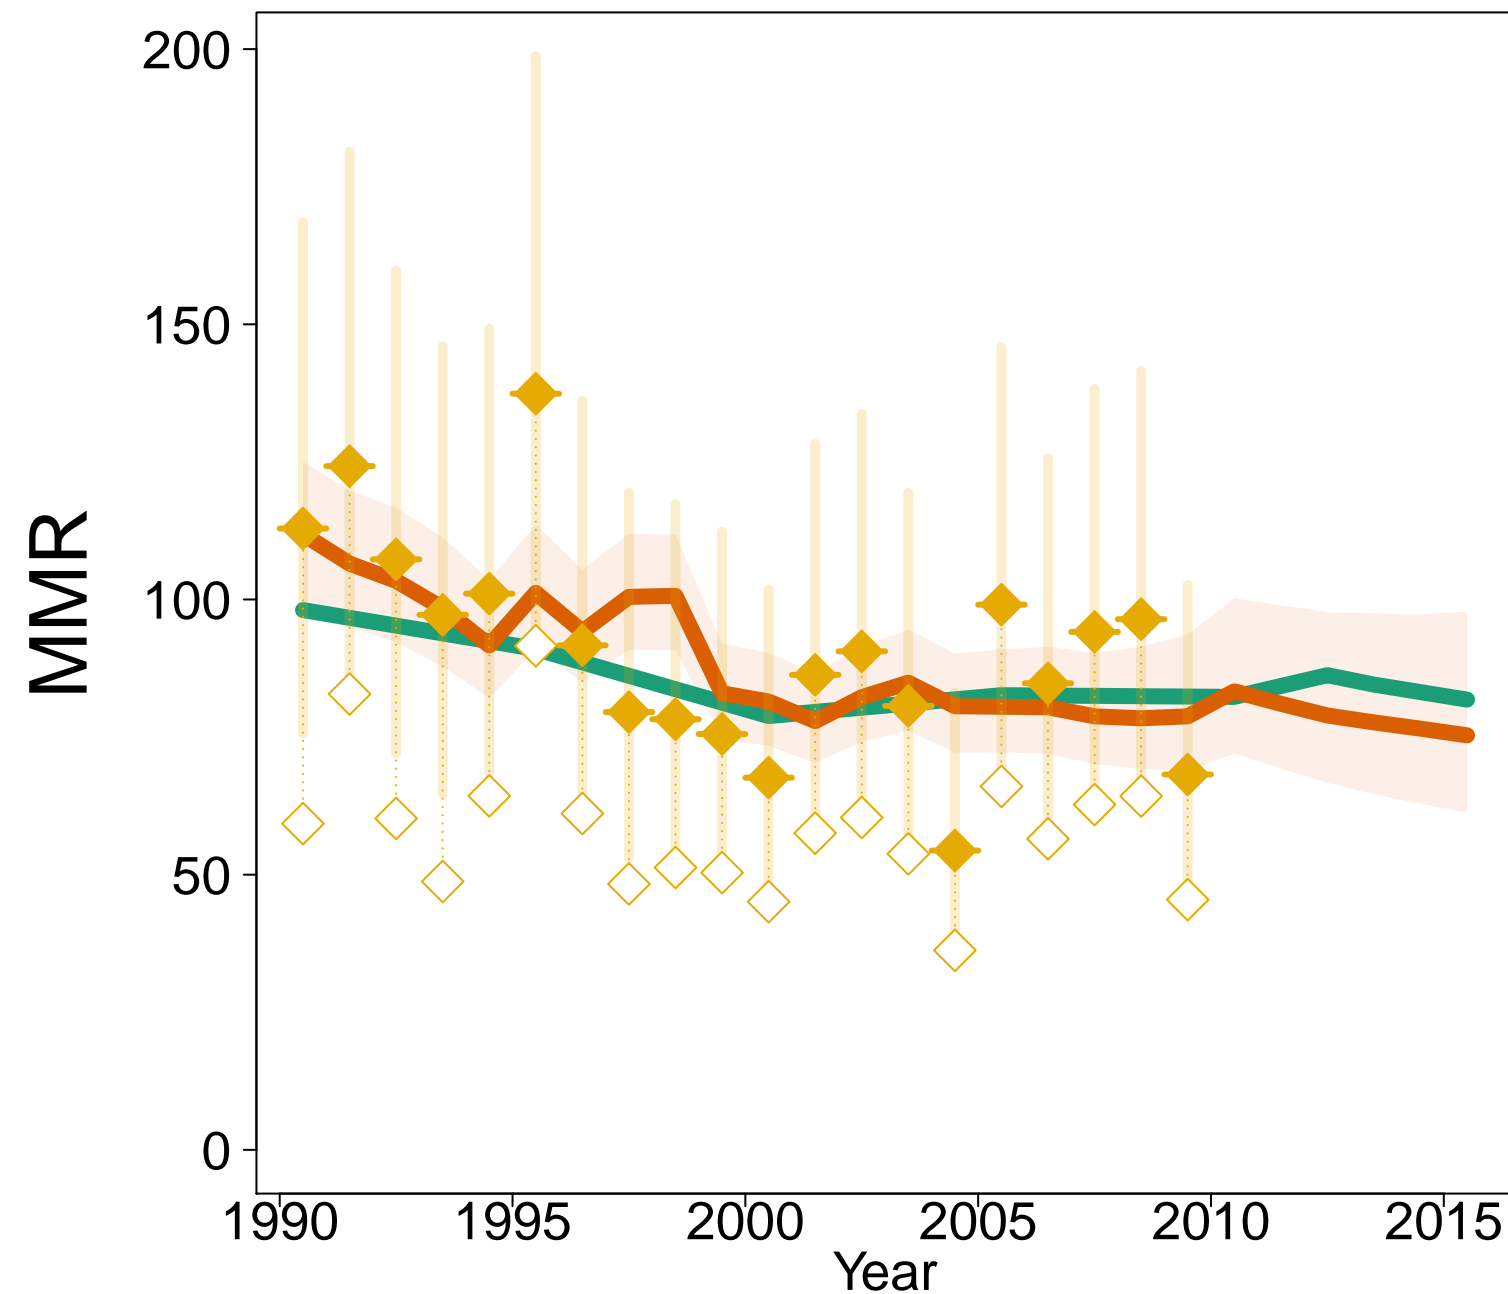

- Estimates –
- Bmat 2014
- MMEIG 2014
- Data –
- Observed Data
- Adjusted Data
- Data type –
- VR

Papua New Guinea [PNG; C]  
(South-Eastern Asia / Oceania)

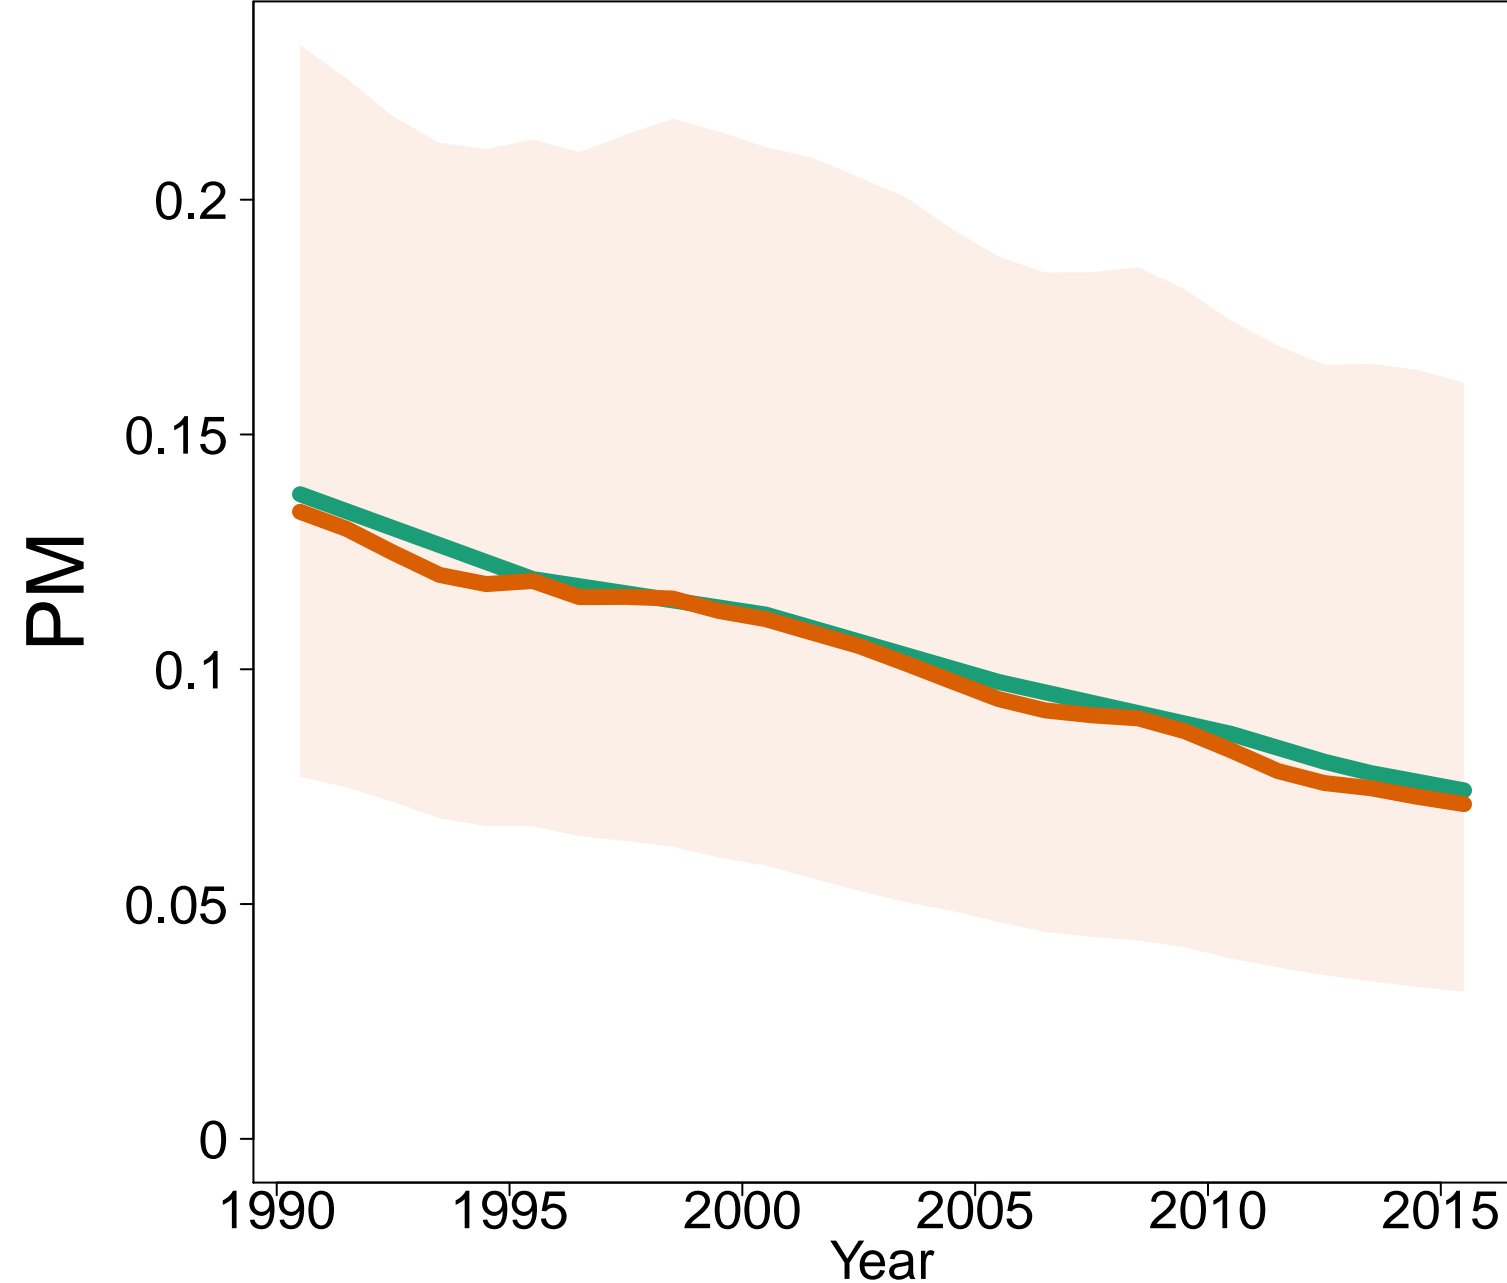

Papua New Guinea [PNG; C]  
(South-Eastern Asia / Oceania)

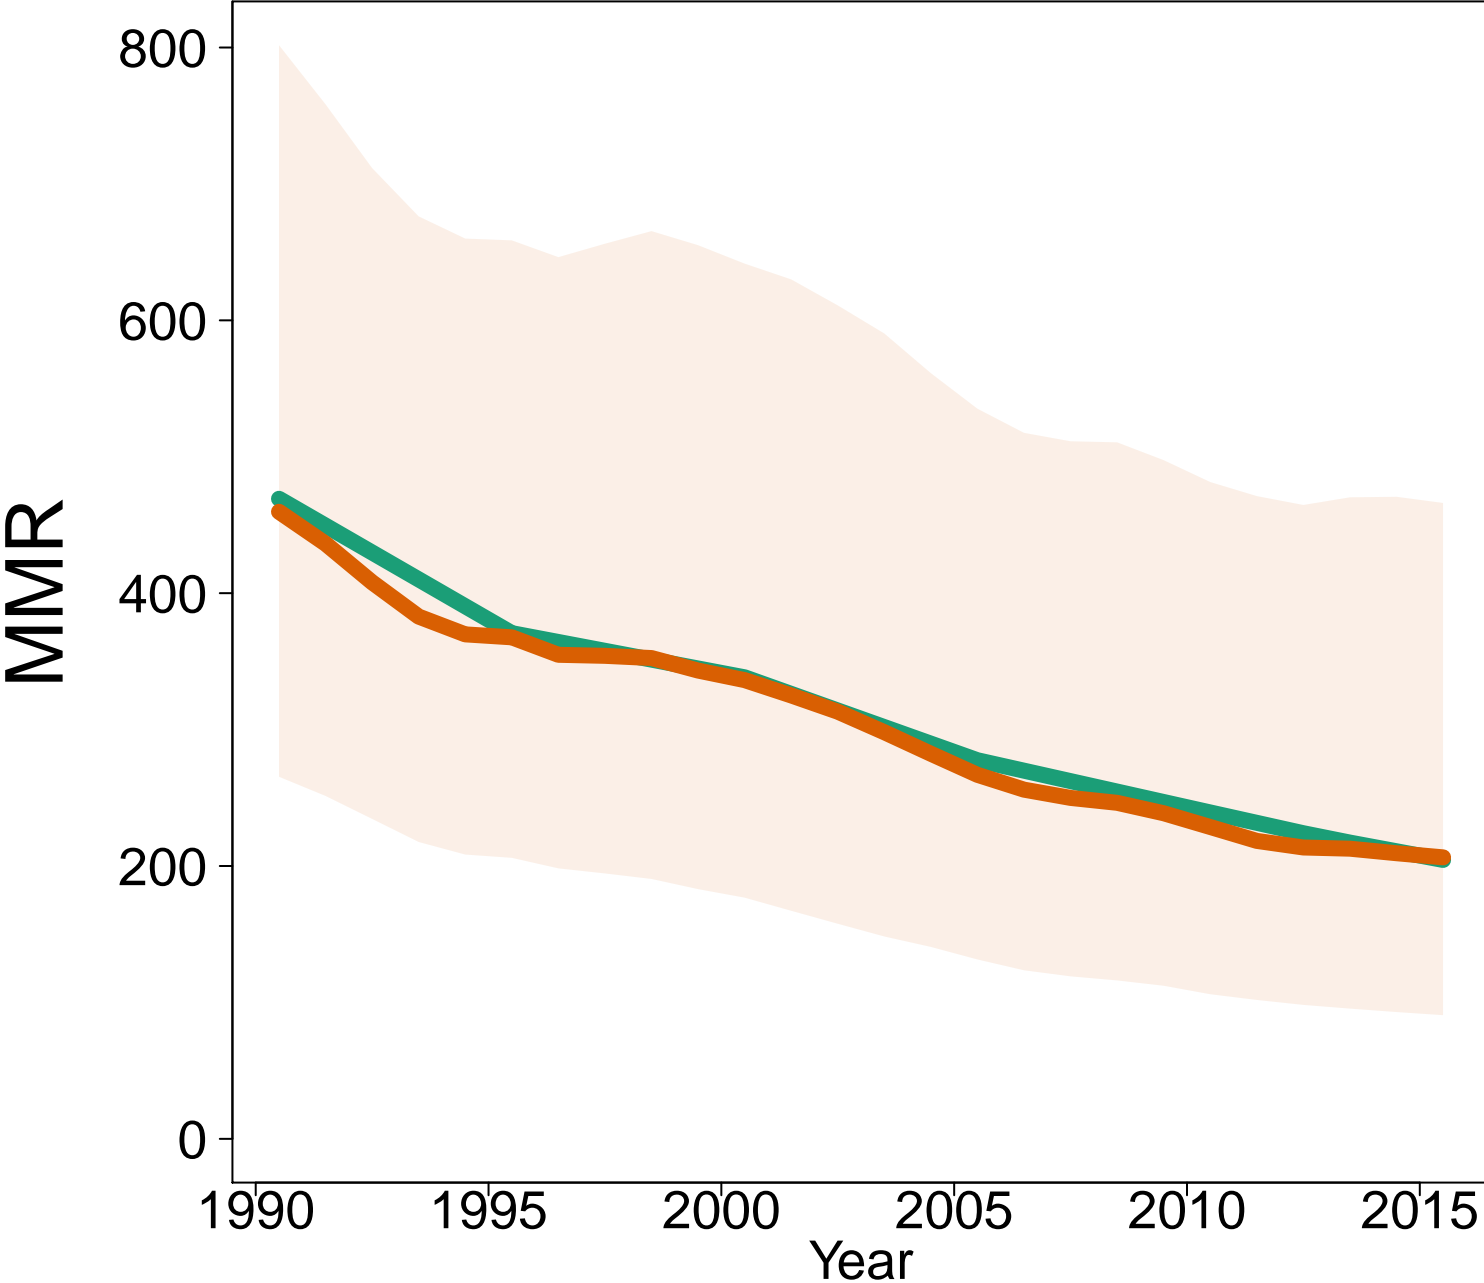

– Estimates –  
Bmat 2014  
MMEIG 2014  
– Data –

Paraguay [PRY; B]  
(South America)

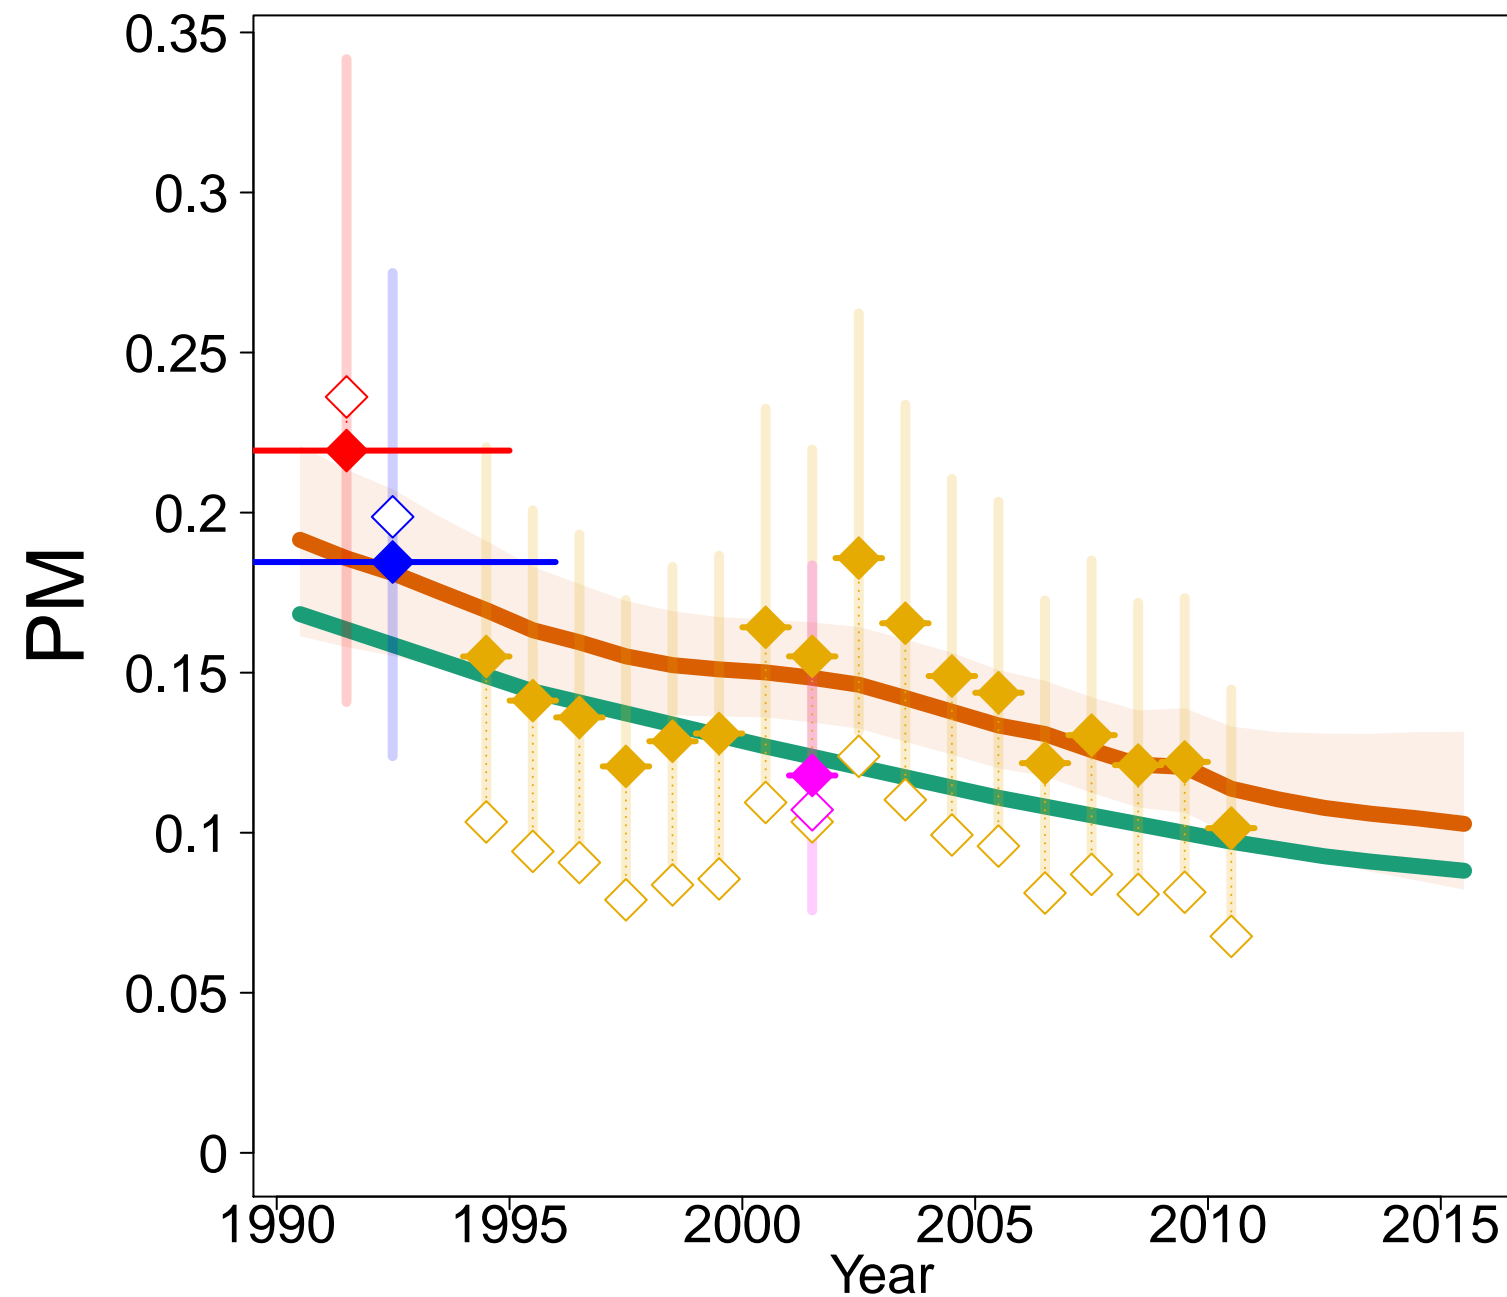

Paraguay [PRY; B]  
(South America)

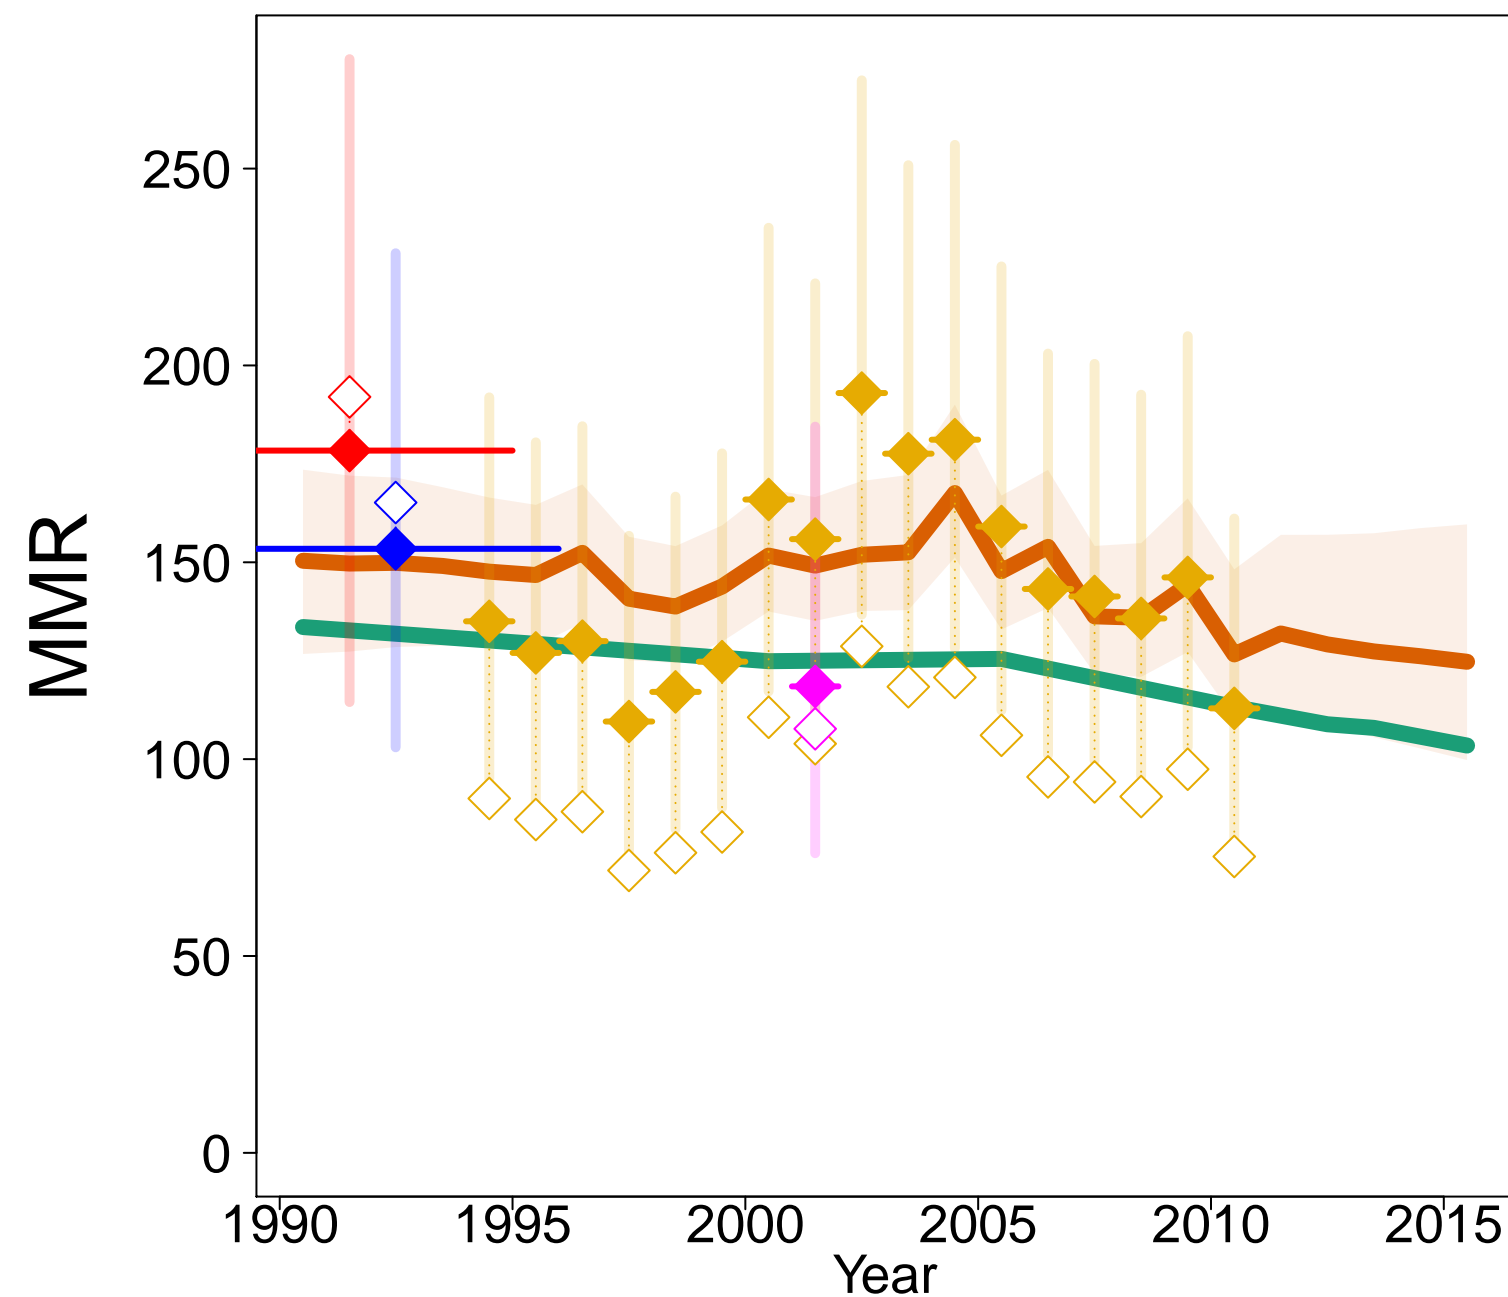

- Estimates –
- Bmat 2014
- MMEIG 2014
- Data –
- Observed Data
- Adjusted Data
- Data type –
- VR
- DHS
- Census
- Misc. studies

Peru [PER; B]  
(South America)

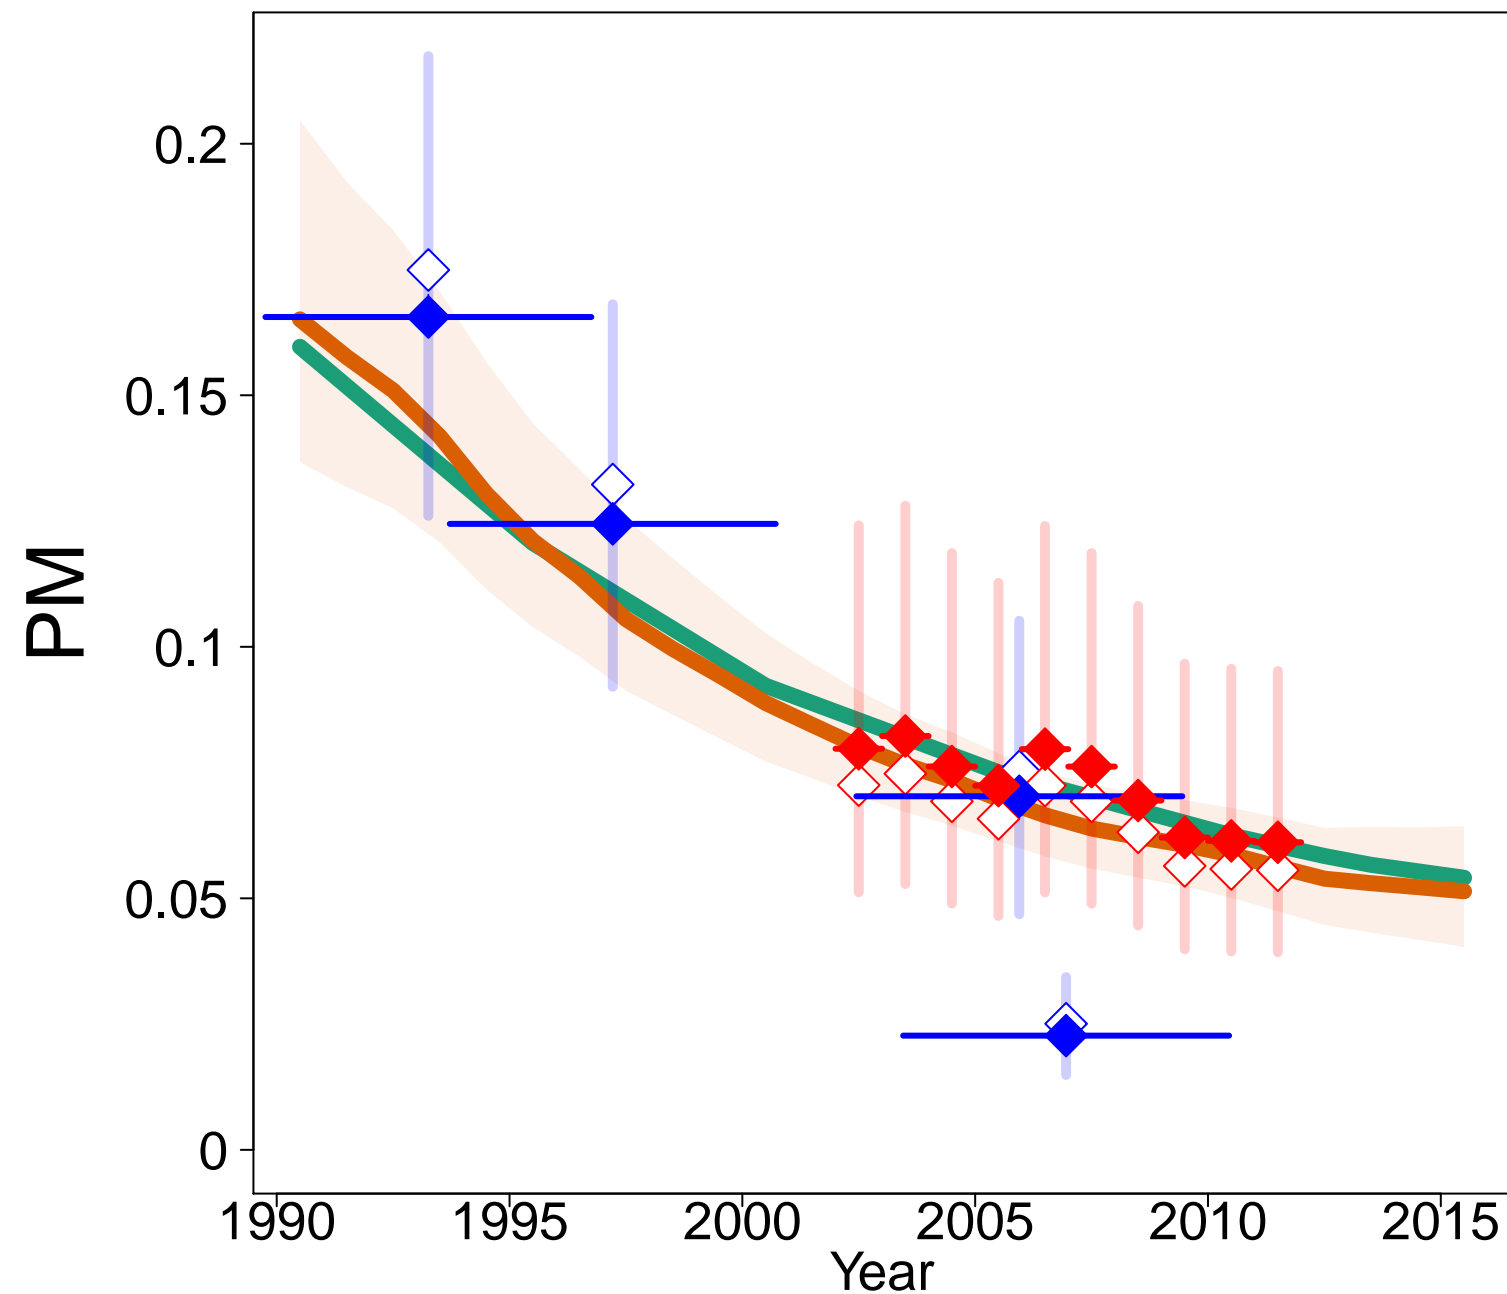

Peru [PER; B]  
(South America)

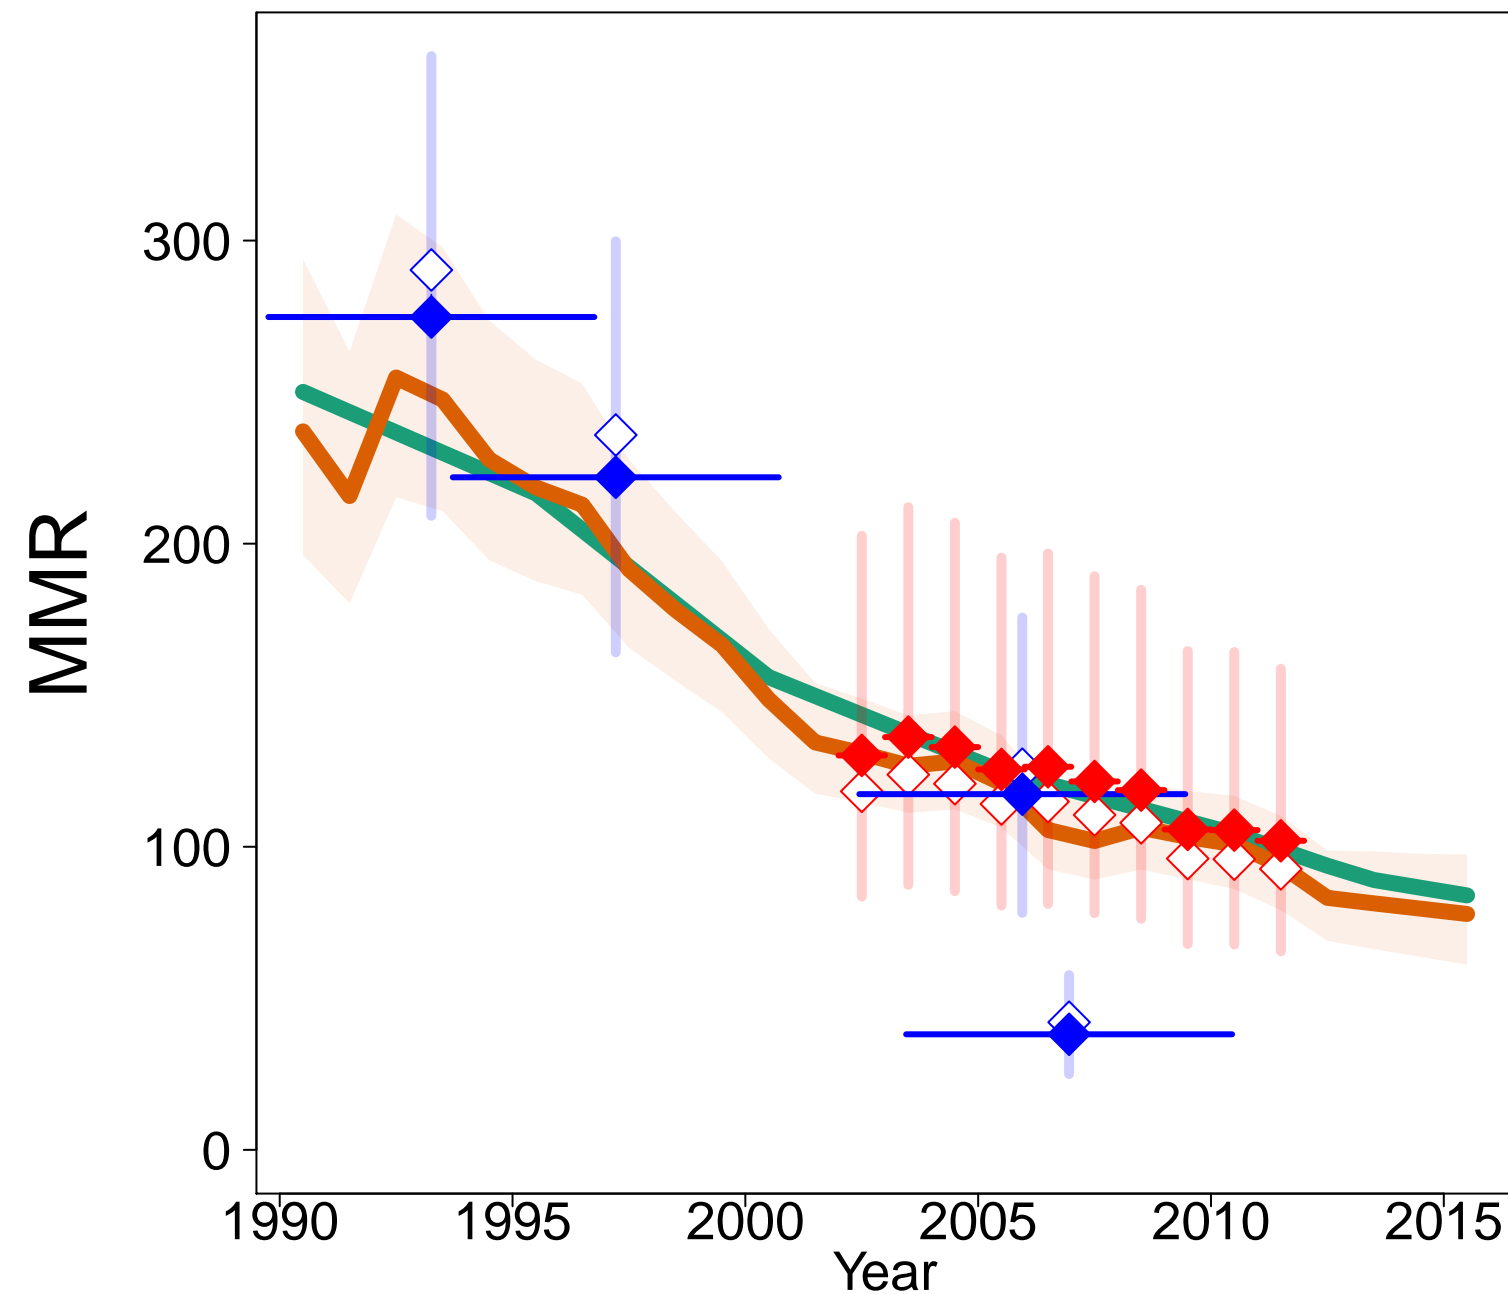

- Estimates –
- Bmat 2014
- MMEIG 2014
- Data –
- Observed Data
- Adjusted Data
- Data type –
- DHS
- Misc. studies

Philippines [PHL; A]  
(South-Eastern Asia / Oceania)

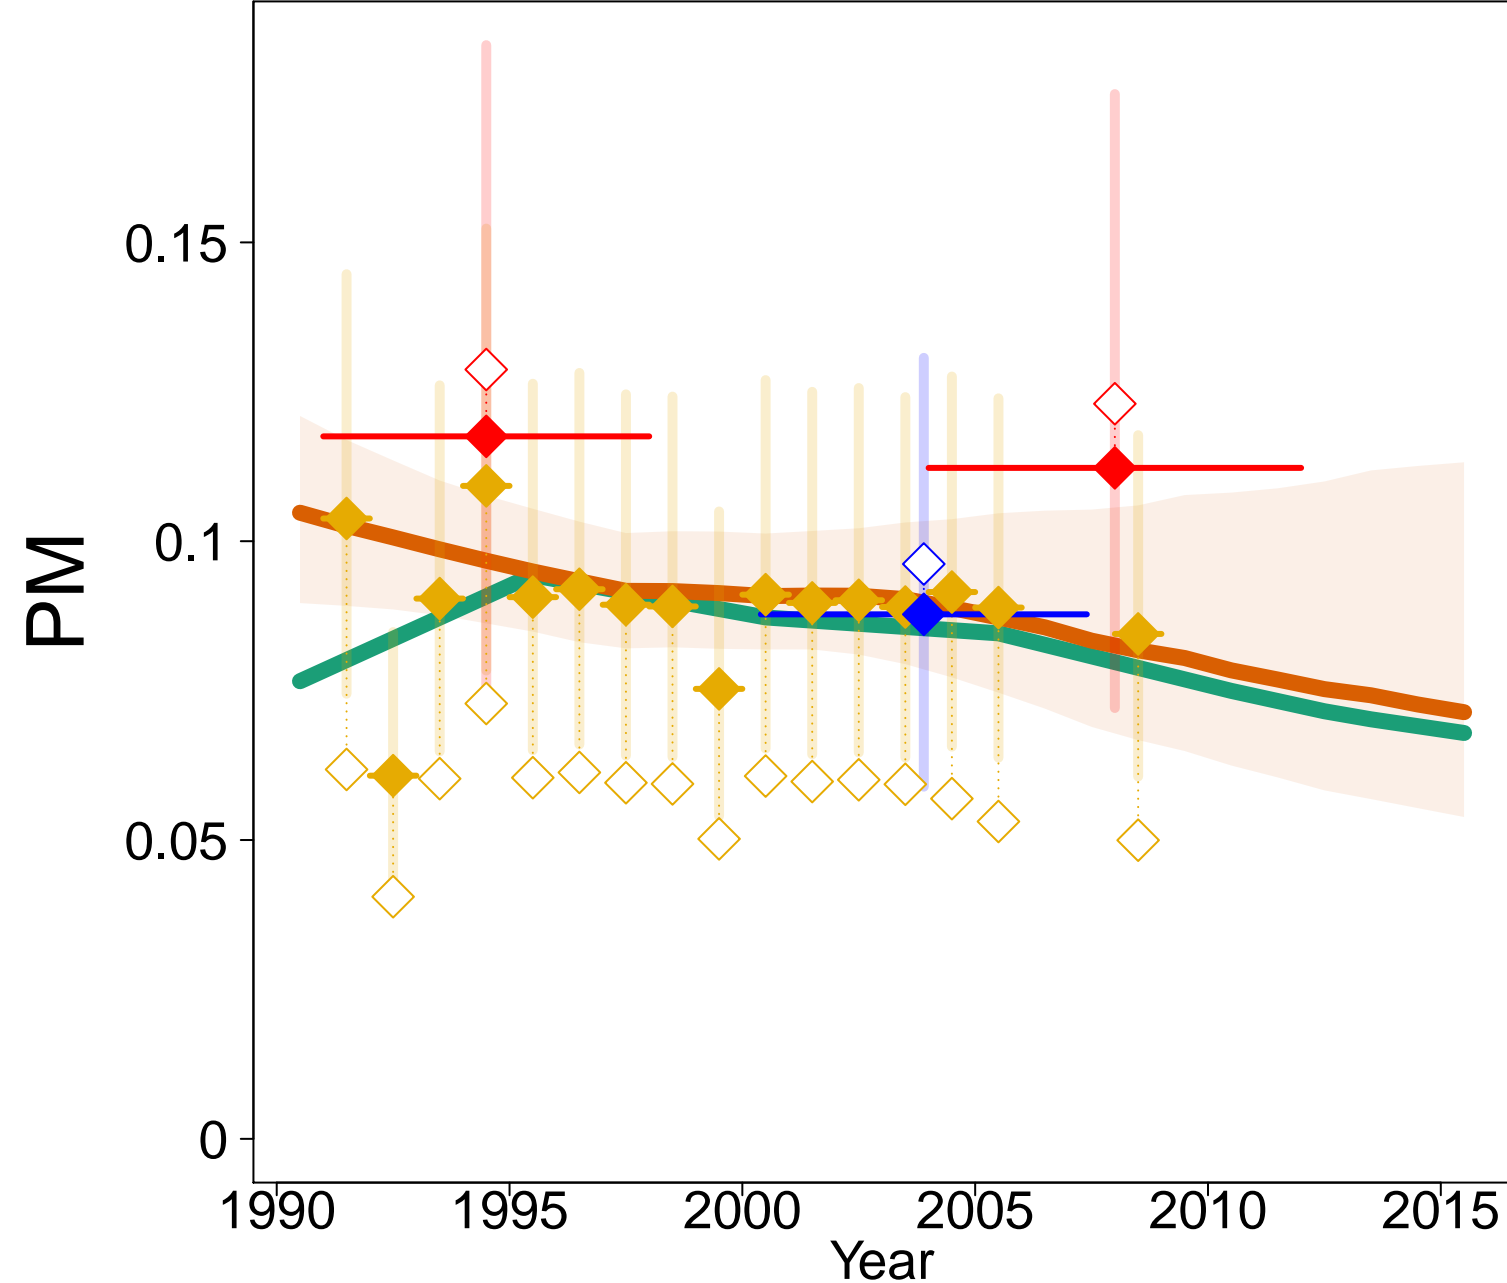

Philippines [PHL; A]  
(South-Eastern Asia / Oceania)

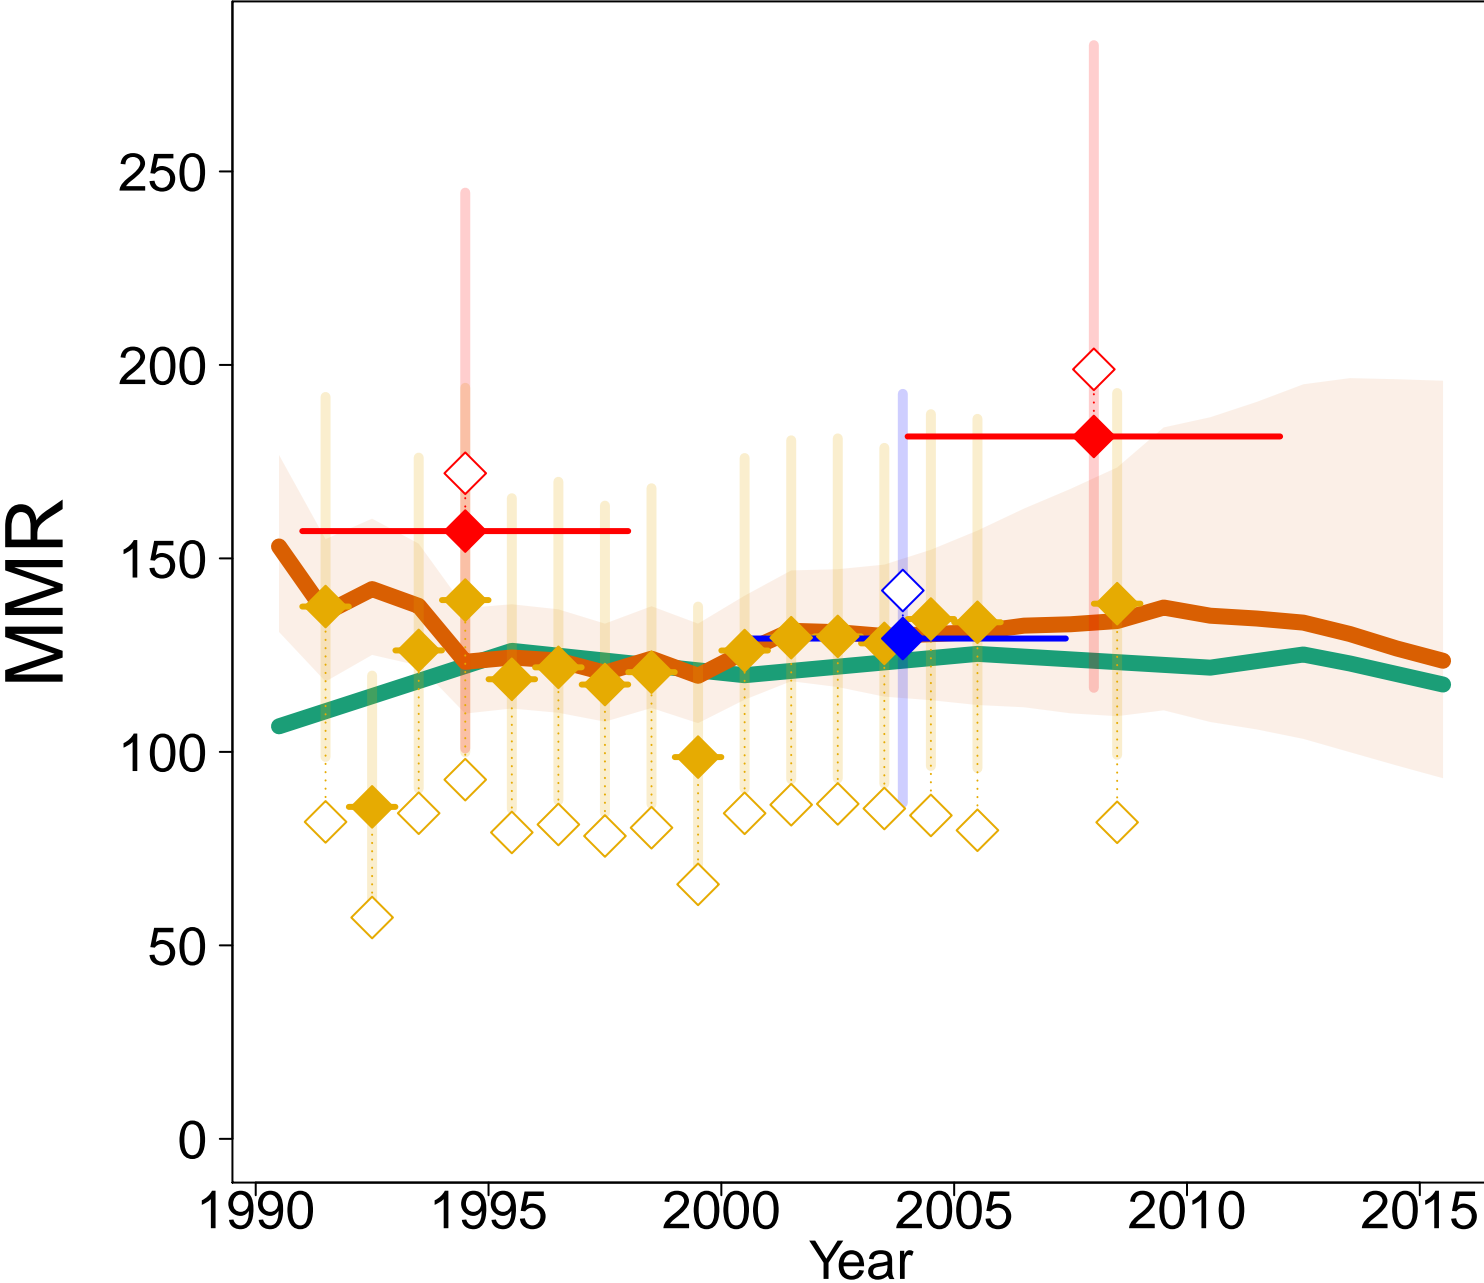

- Estimates –
- Bmat 2014
- MMEIG 2014
- Data –
- Observed Data
- Adjusted Data
- Data type –
- VR
- DHS
- Misc. studies

Poland [POL; A]  
(Developed regions)

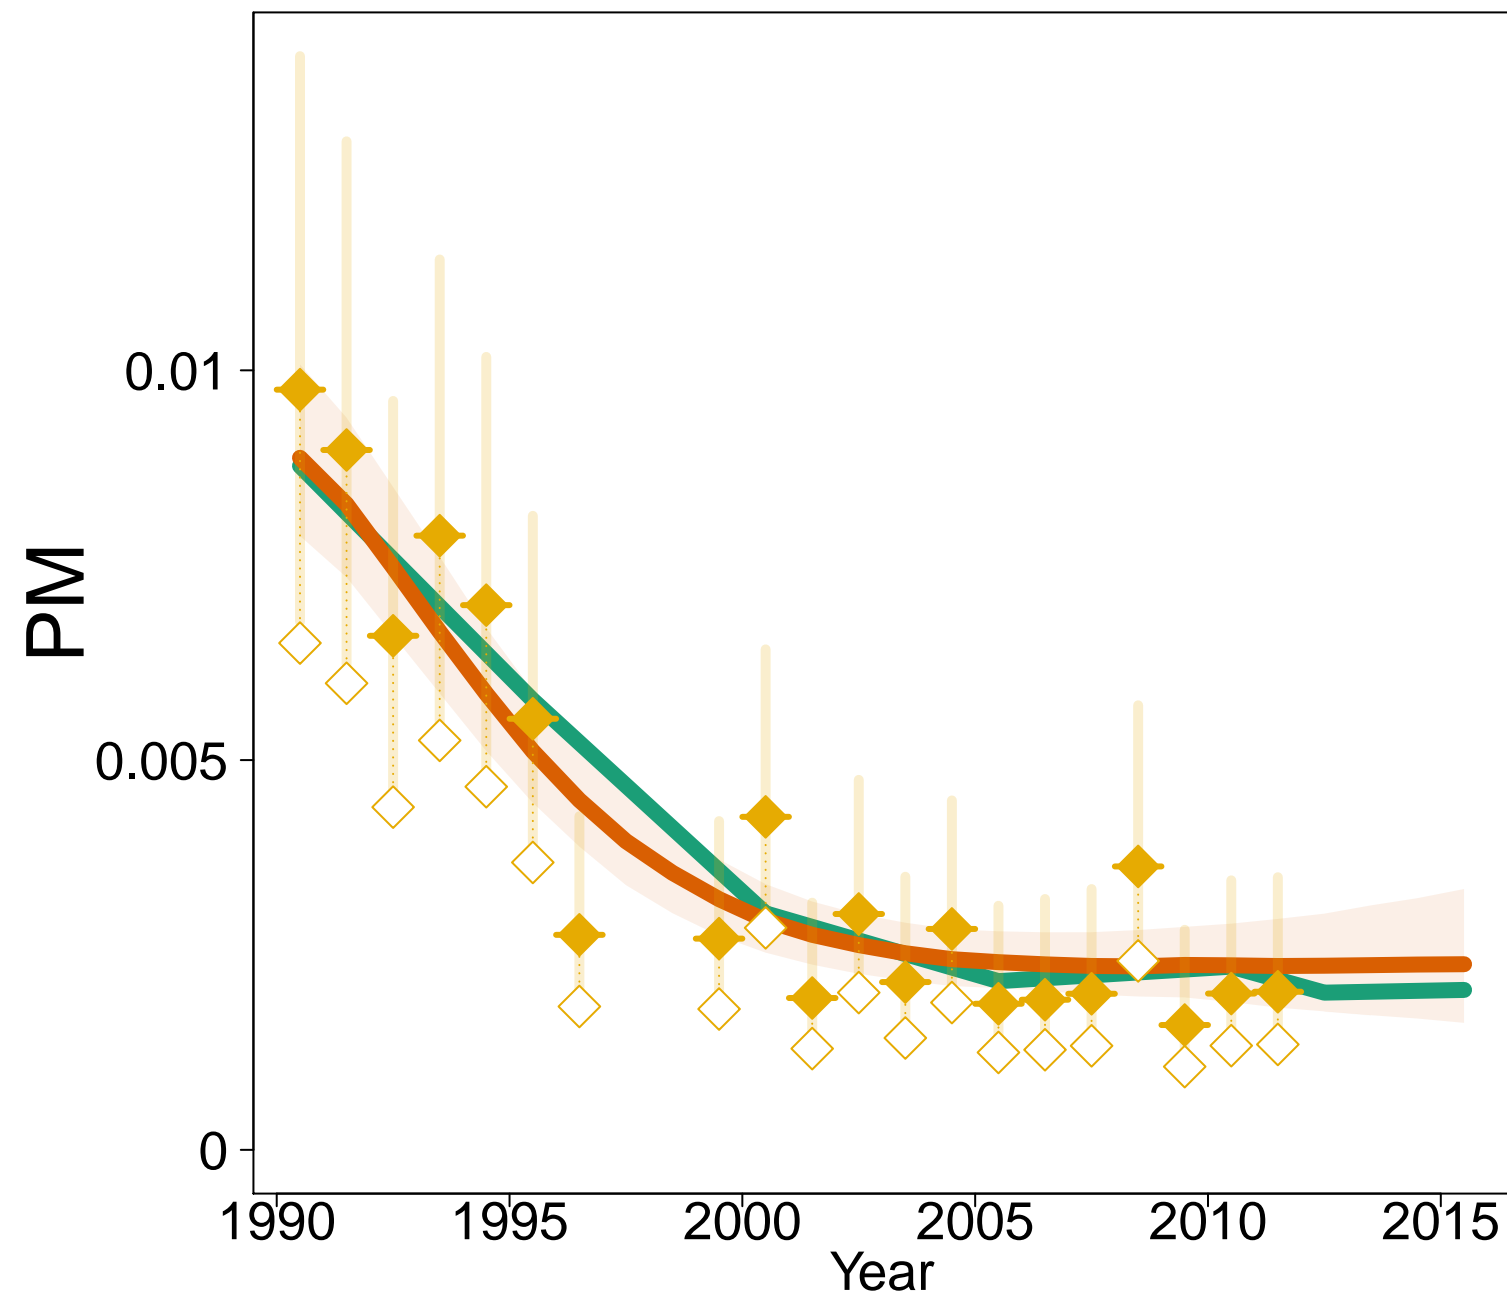

Poland [POL; A]  
(Developed regions)

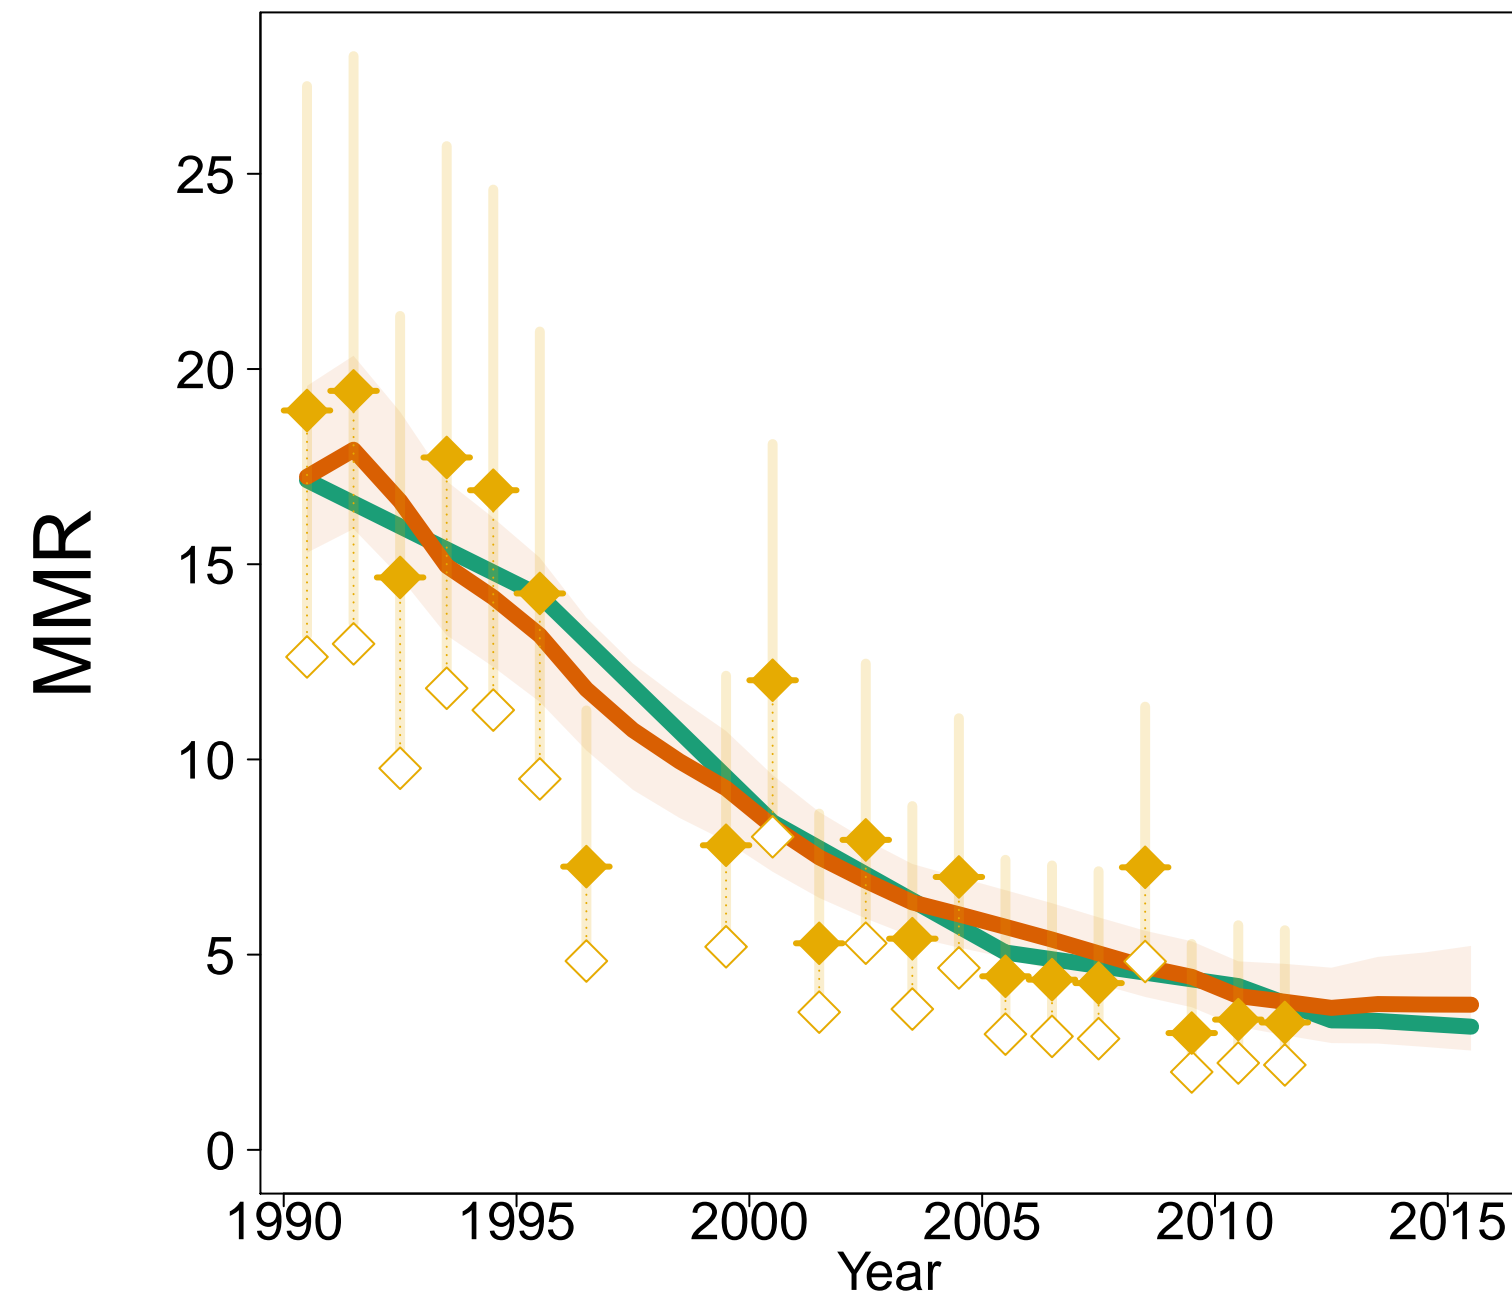

- Estimates –
- Bmat 2014
- MMEIG 2014
- Data –
- Observed Data
- Adjusted Data
- Data type –
- VR



Portugal [PRT; A]  
(Developed regions)

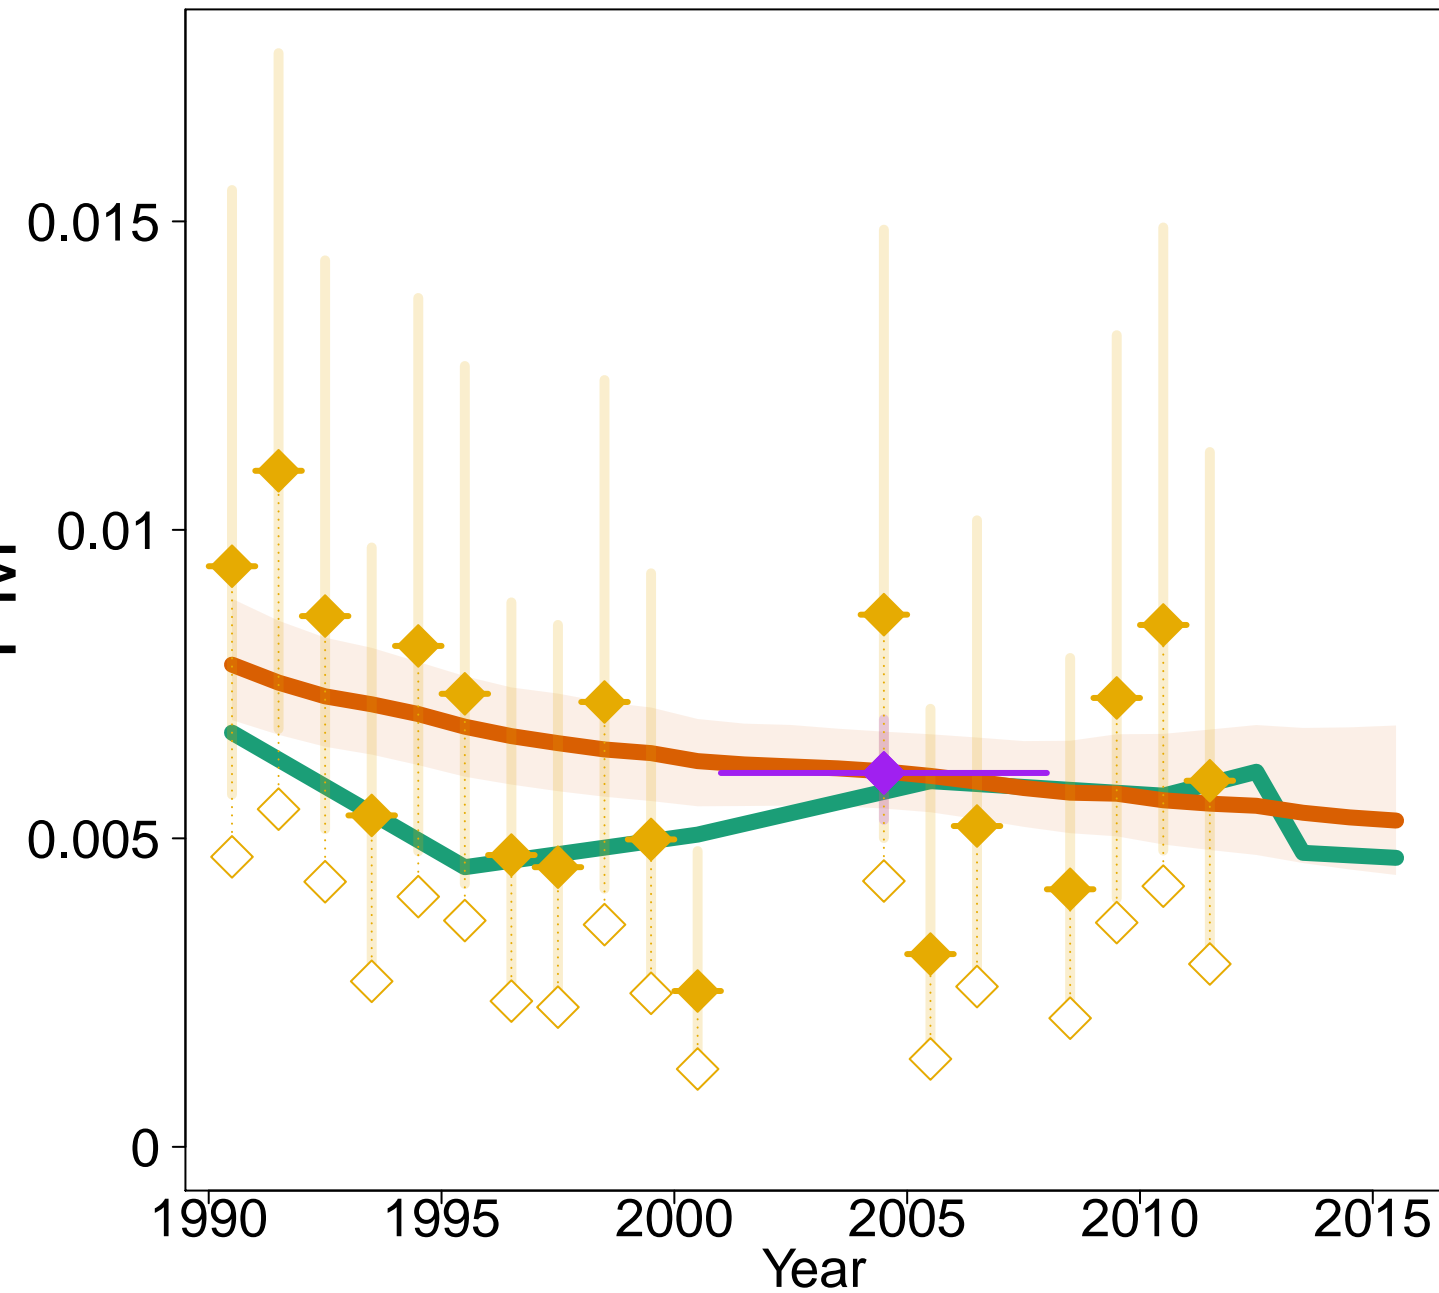

Portugal [PRT; A]  
(Developed regions)

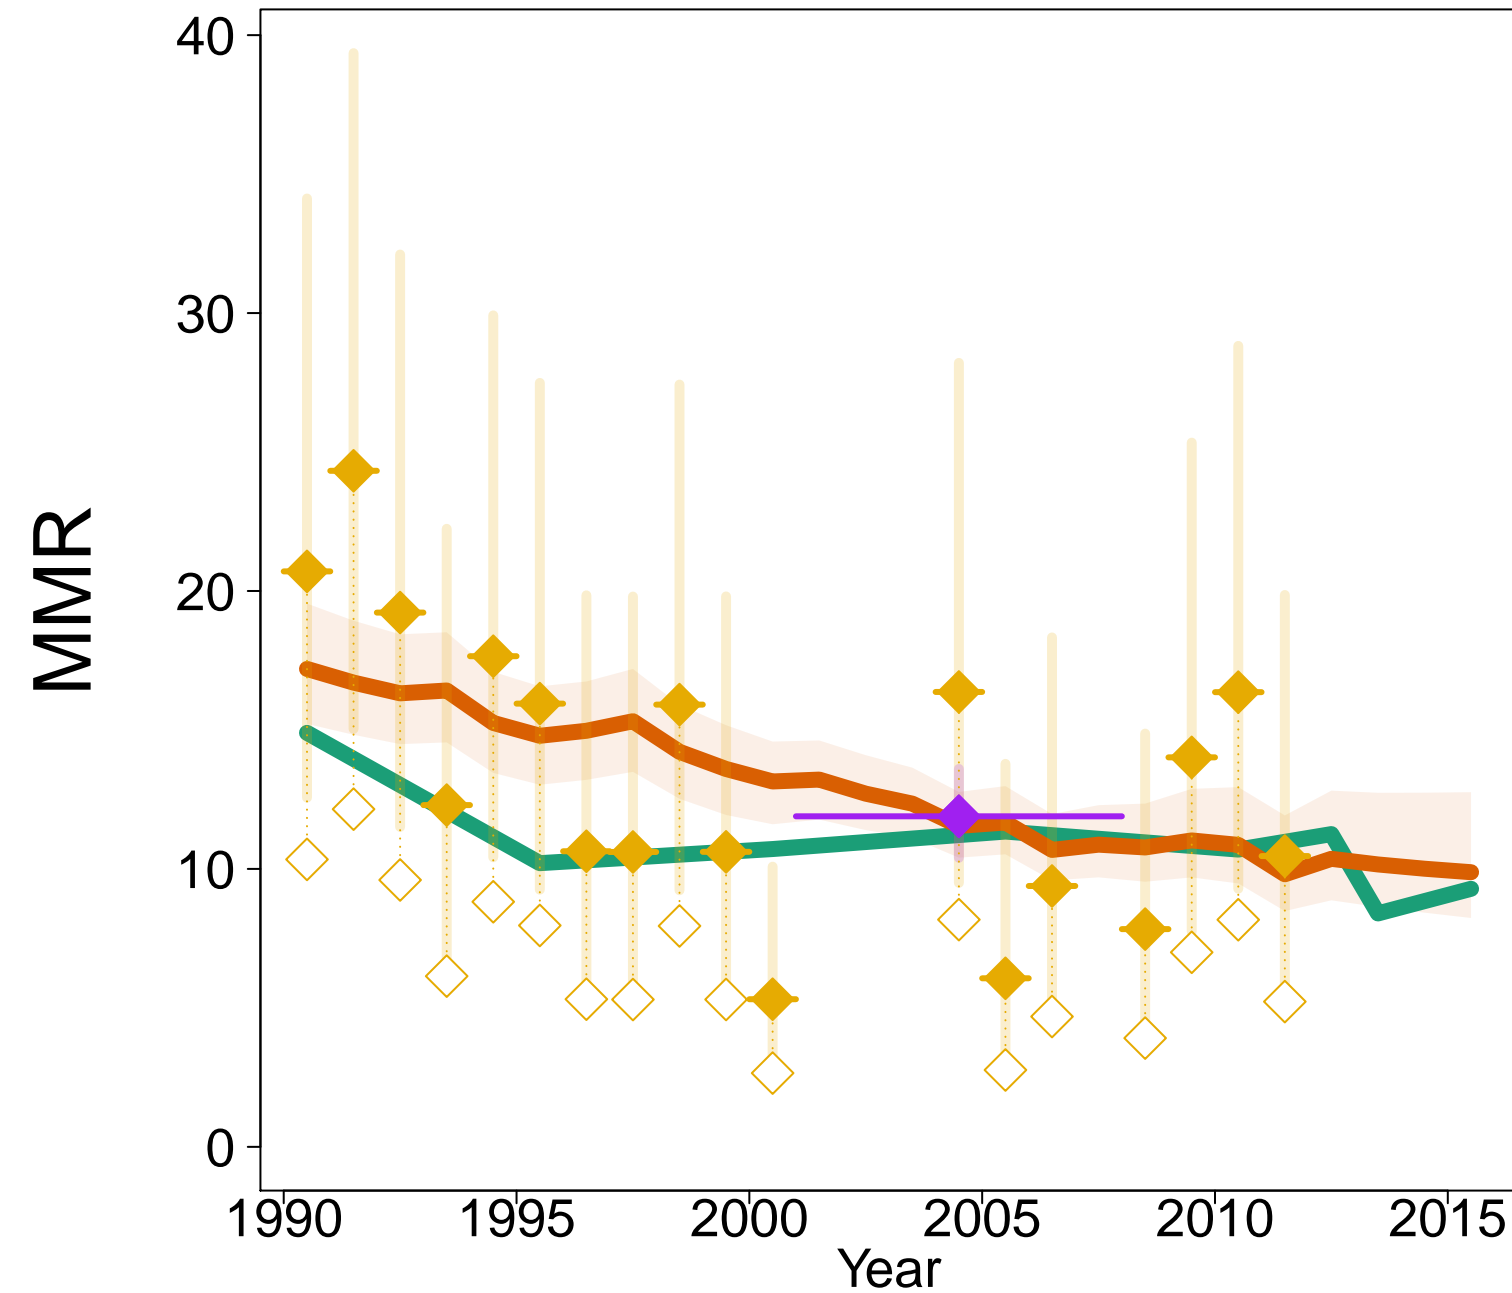

- Estimates –
- Bmat 2014
- MMEIG 2014
- Data –
- Observed Data
- Adjusted Data
- Data type –
- VR
- Spec. studies

Puerto Rico [PRI; B]  
(Caribbean)

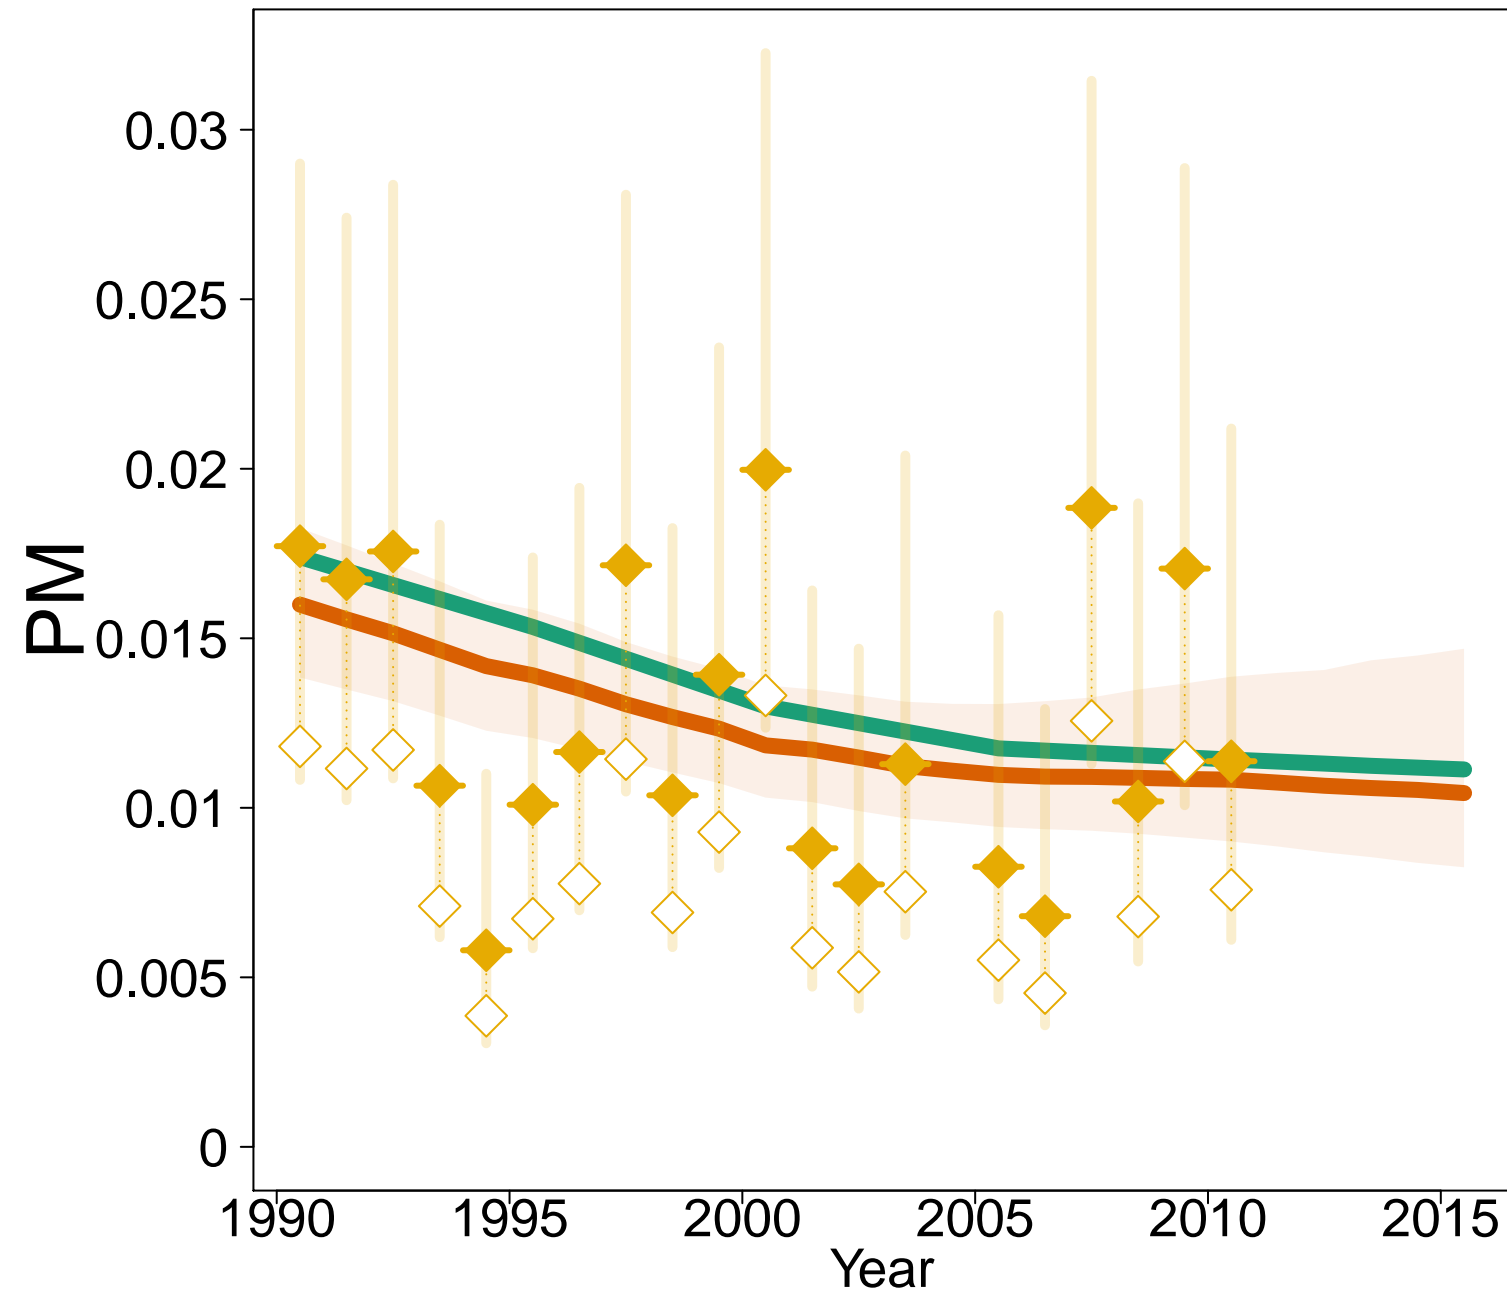

Puerto Rico [PRI; B]  
(Caribbean)

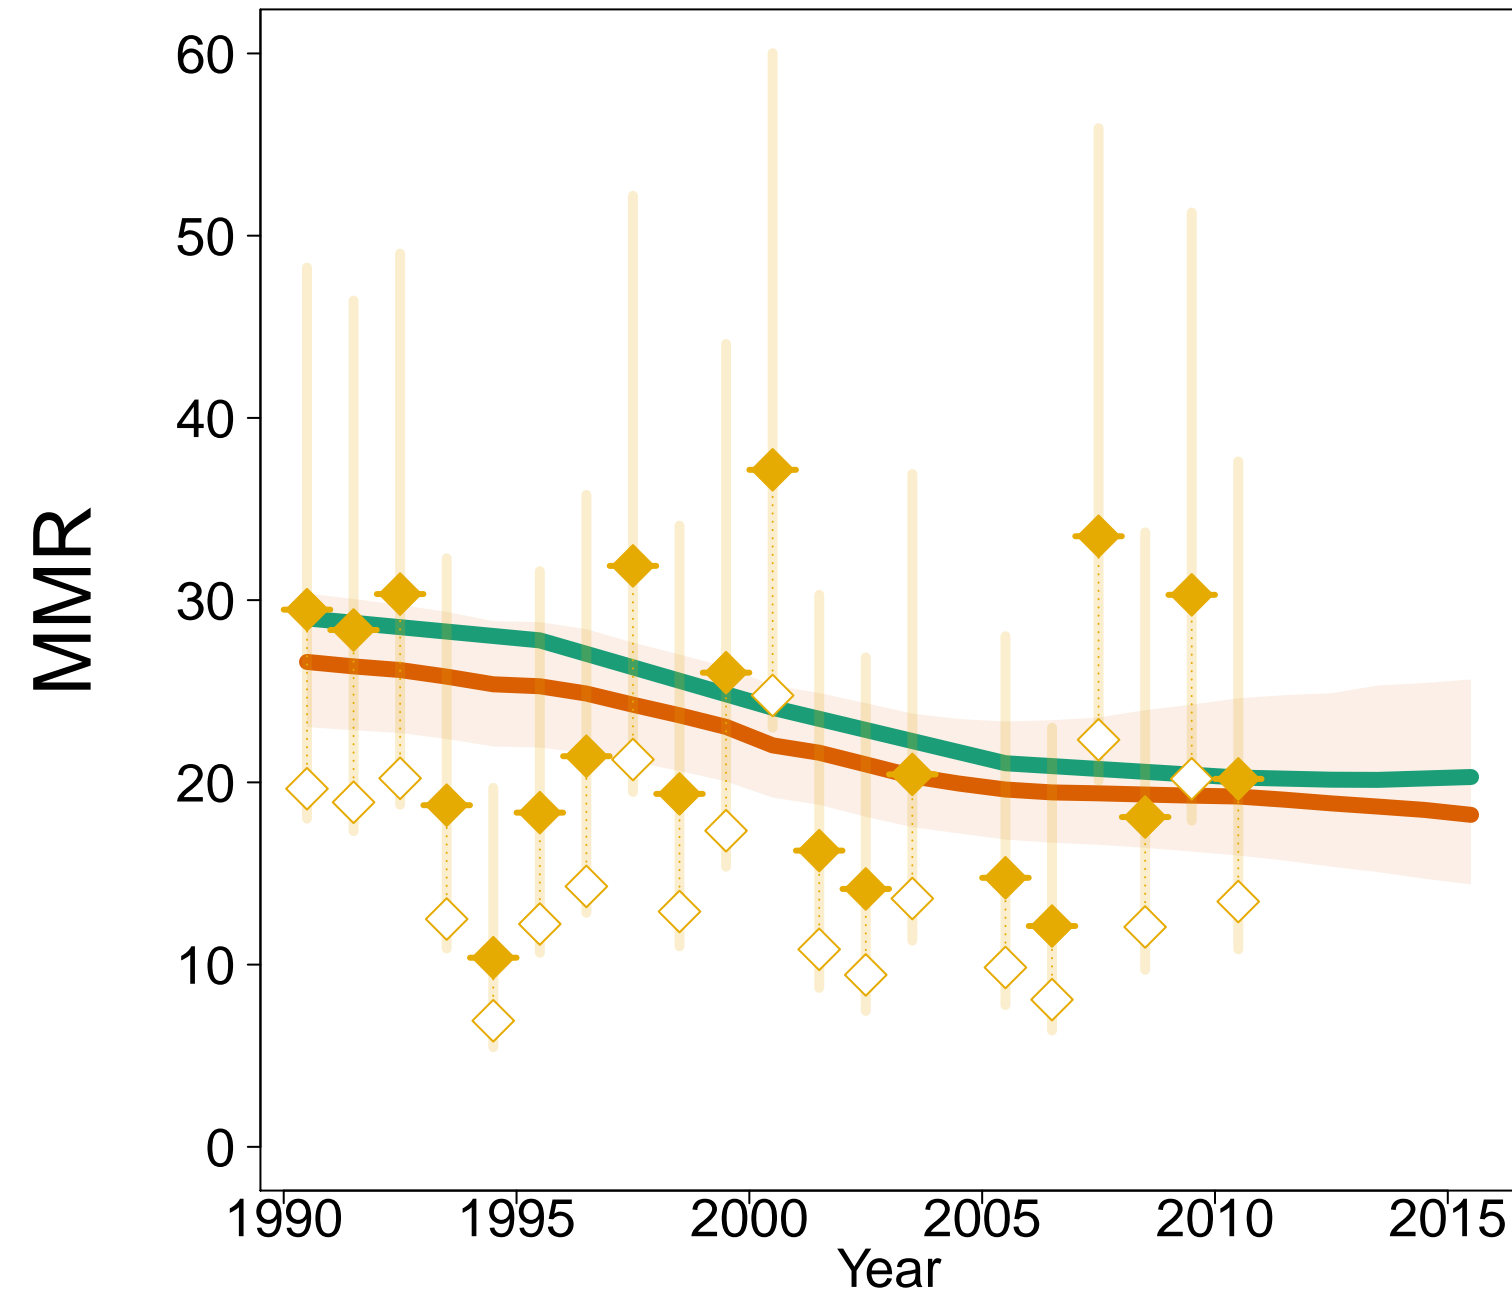

- Estimates –
- Bmat 2014
- MMEIG 2014
- Data –
- Observed Data
- Adjusted Data
- Data type –
- VR

Qatar [QAT; C]  
(Western Asia)

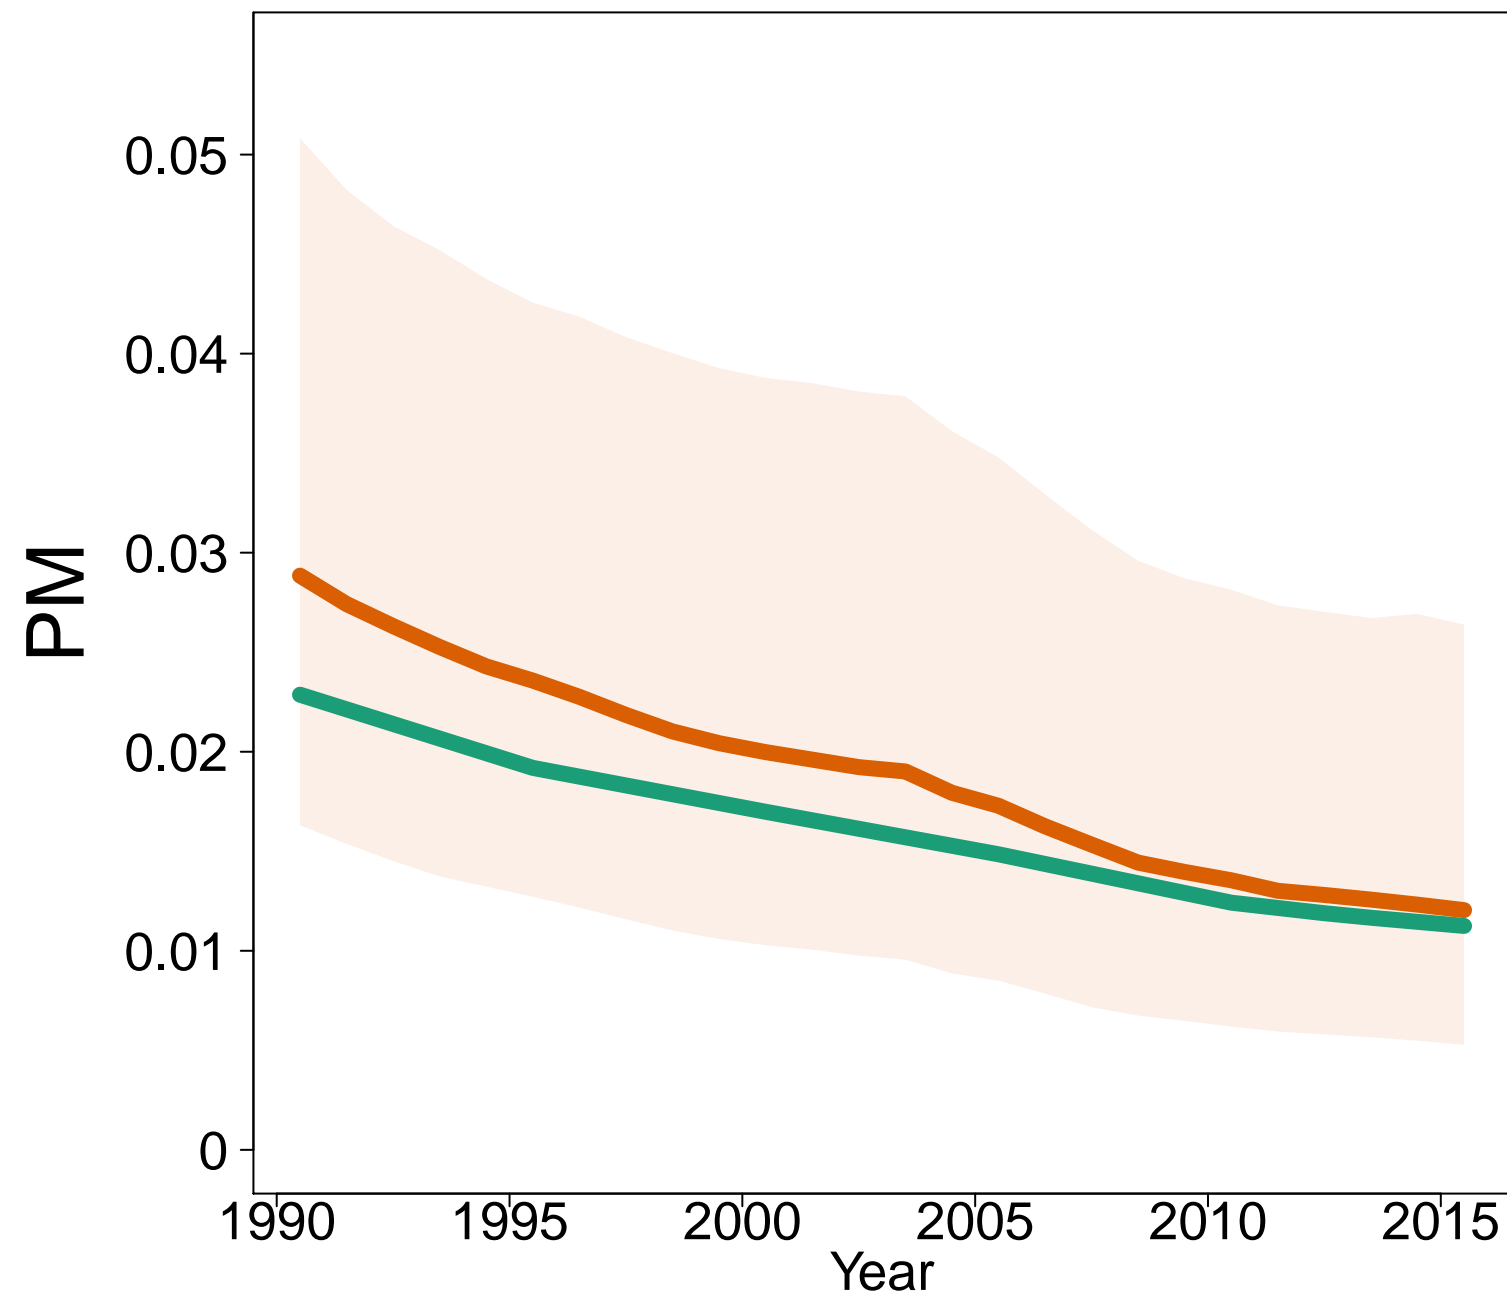

Qatar [QAT; C]  
(Western Asia)

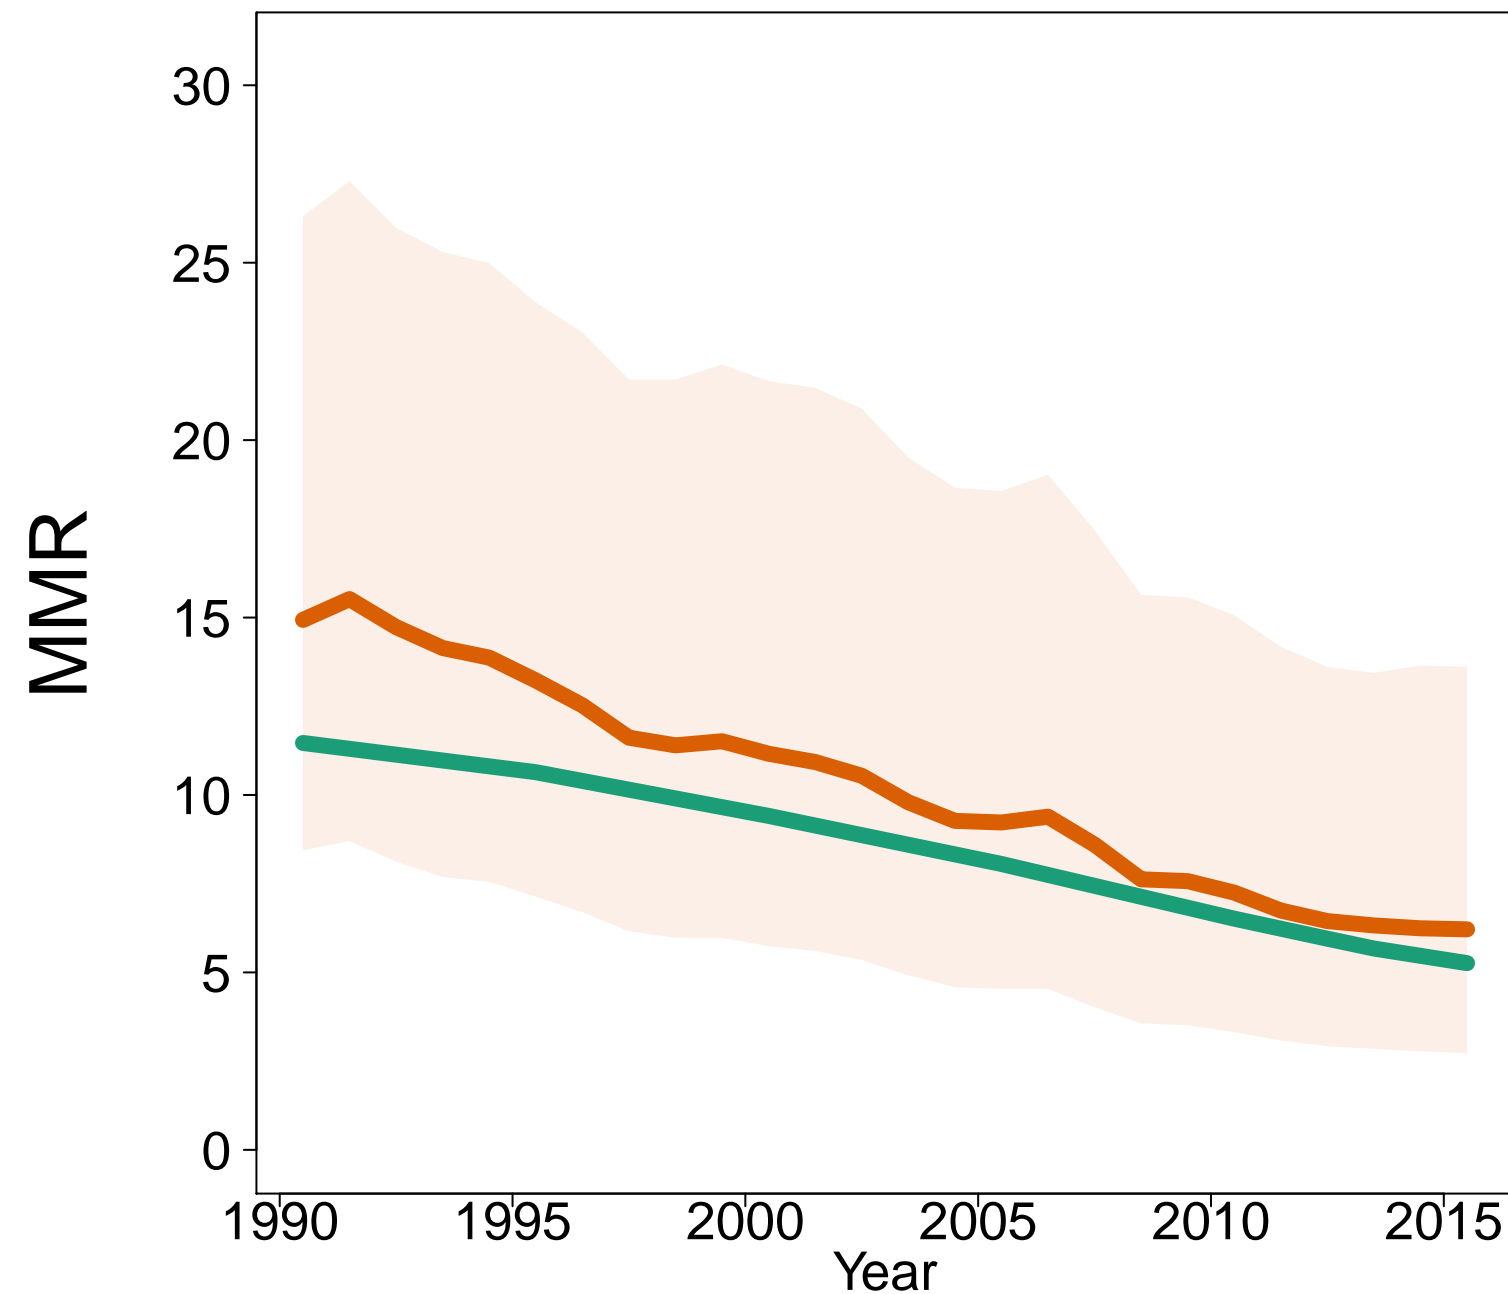

- Estimates –
- Bmat 2014
- MMEIG 2014
- Data –
- ◊ Observed Data
- ◆ Adjusted Data
- Data type –

Republic of Korea [KOR; A]  
(Eastern Asia)

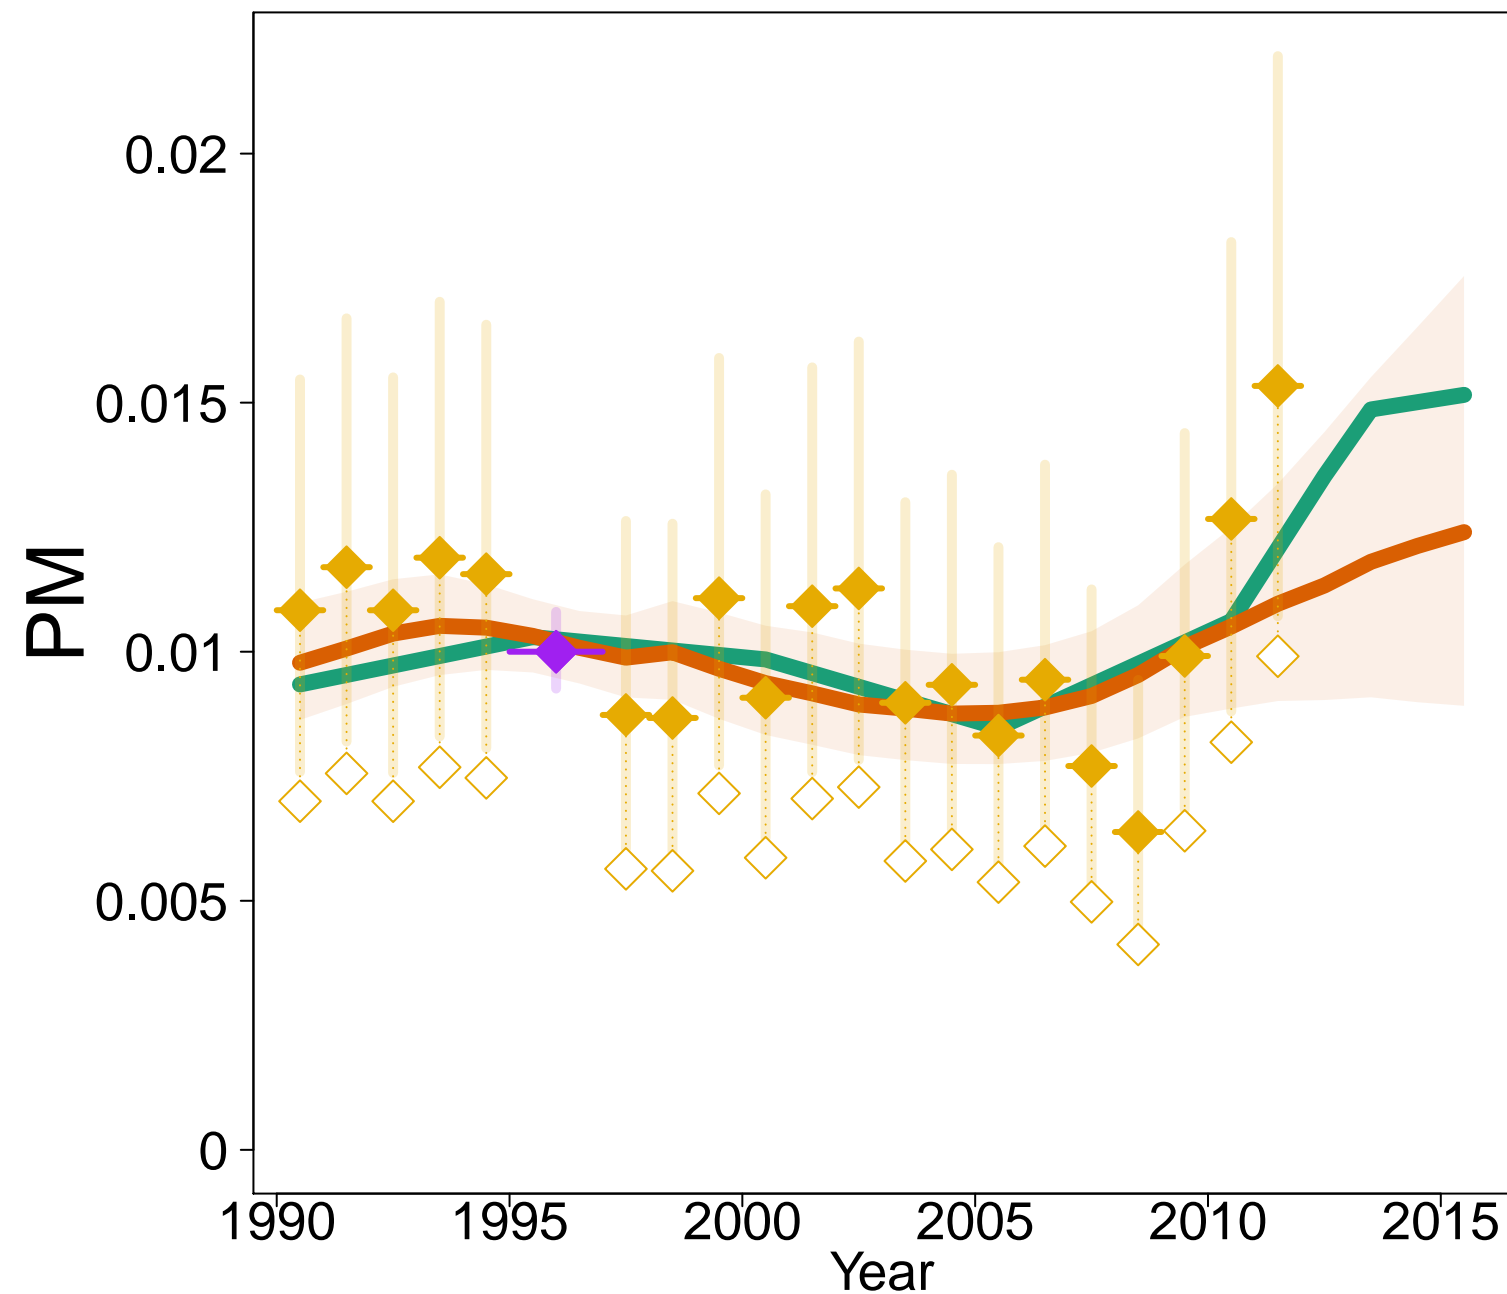

Republic of Korea [KOR; A]  
(Eastern Asia)

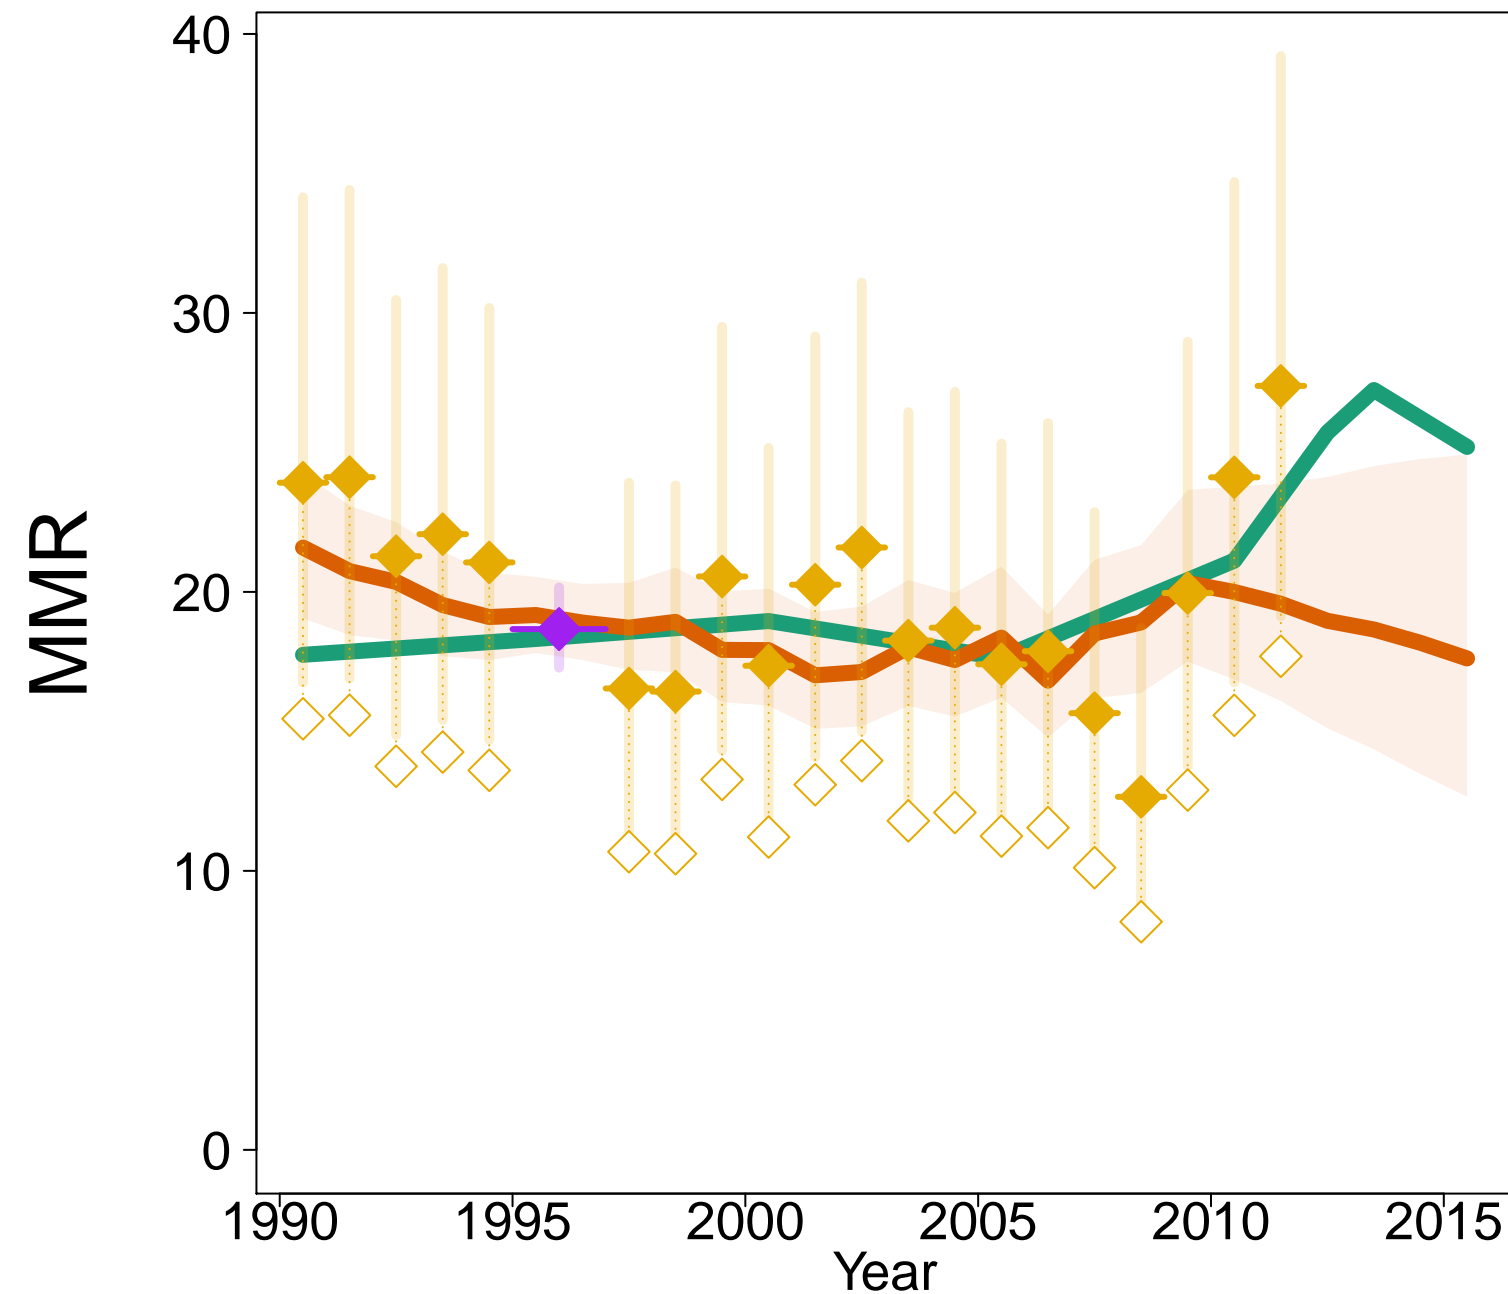

- Estimates –
- Bmat 2014
- MMEIG 2014
- Data –
- Observed Data
- Adjusted Data
- Data type –
- VR
- Spec. studies

Republic of Moldova [MDA; A]  
(Developed regions)

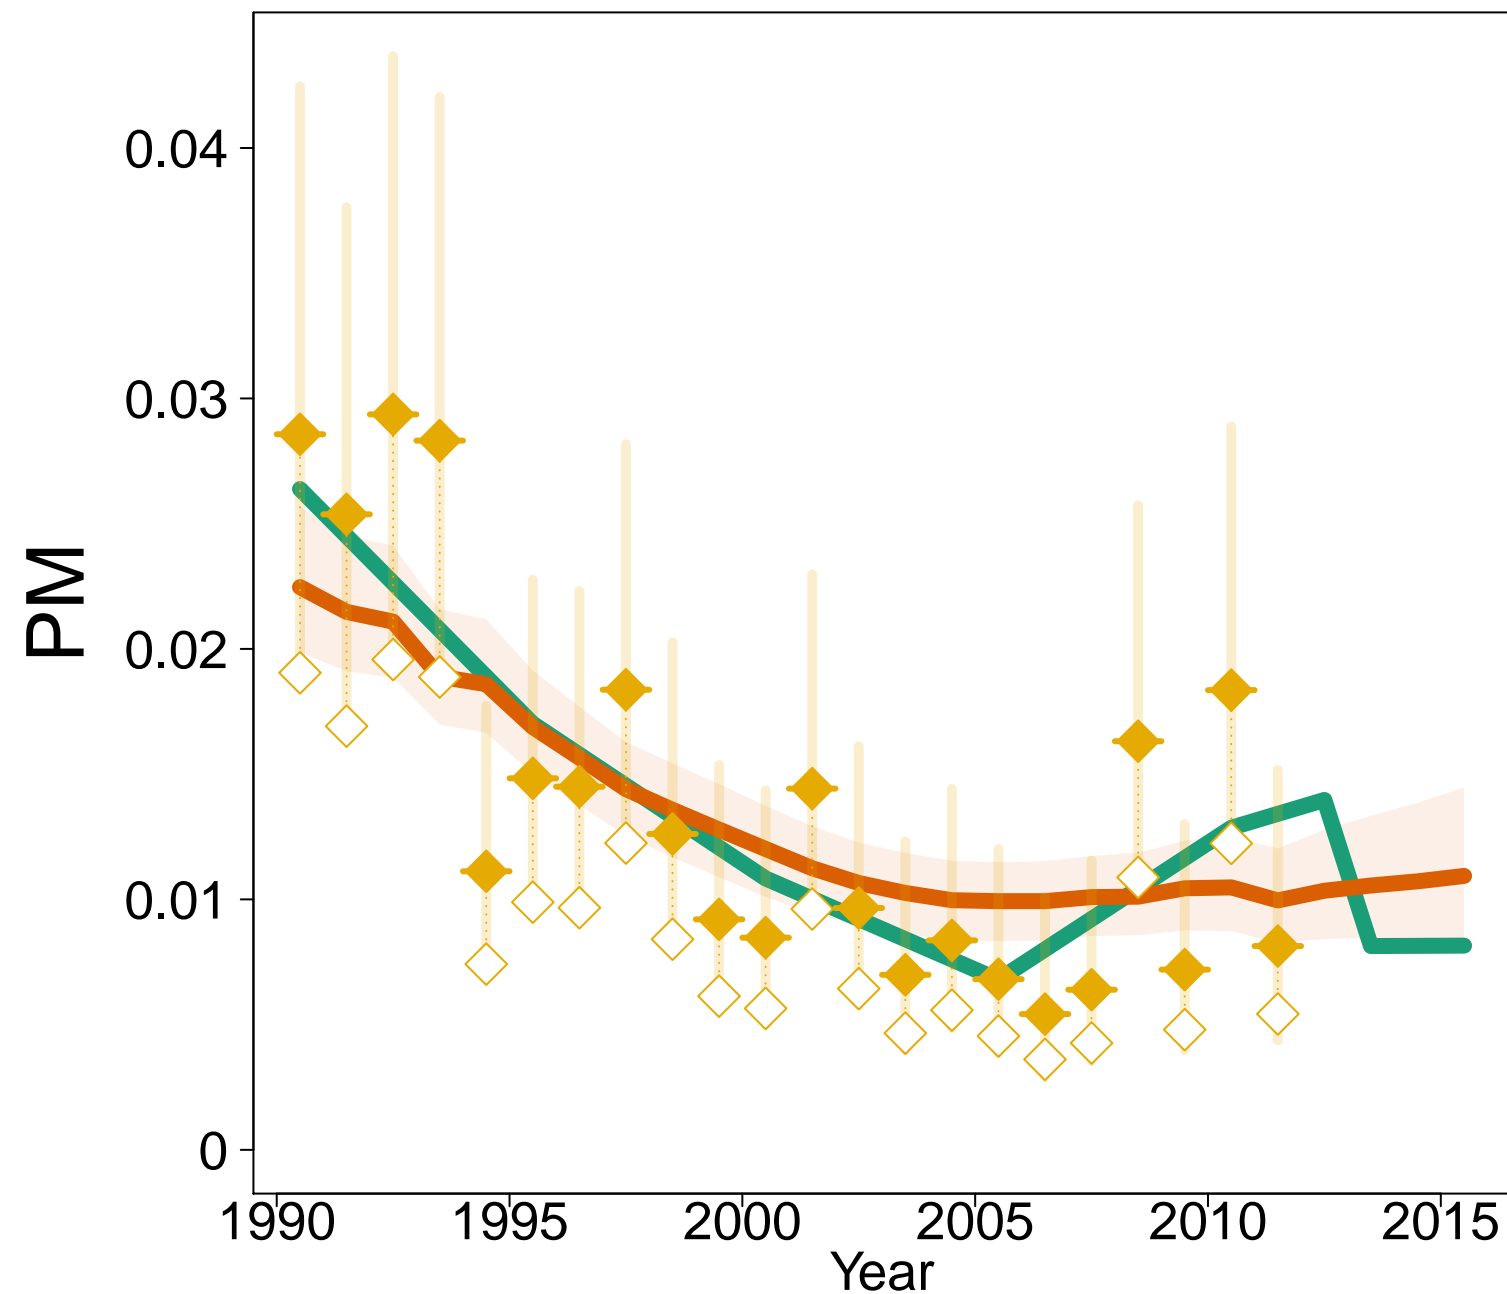

Republic of Moldova [MDA; A]  
(Developed regions)

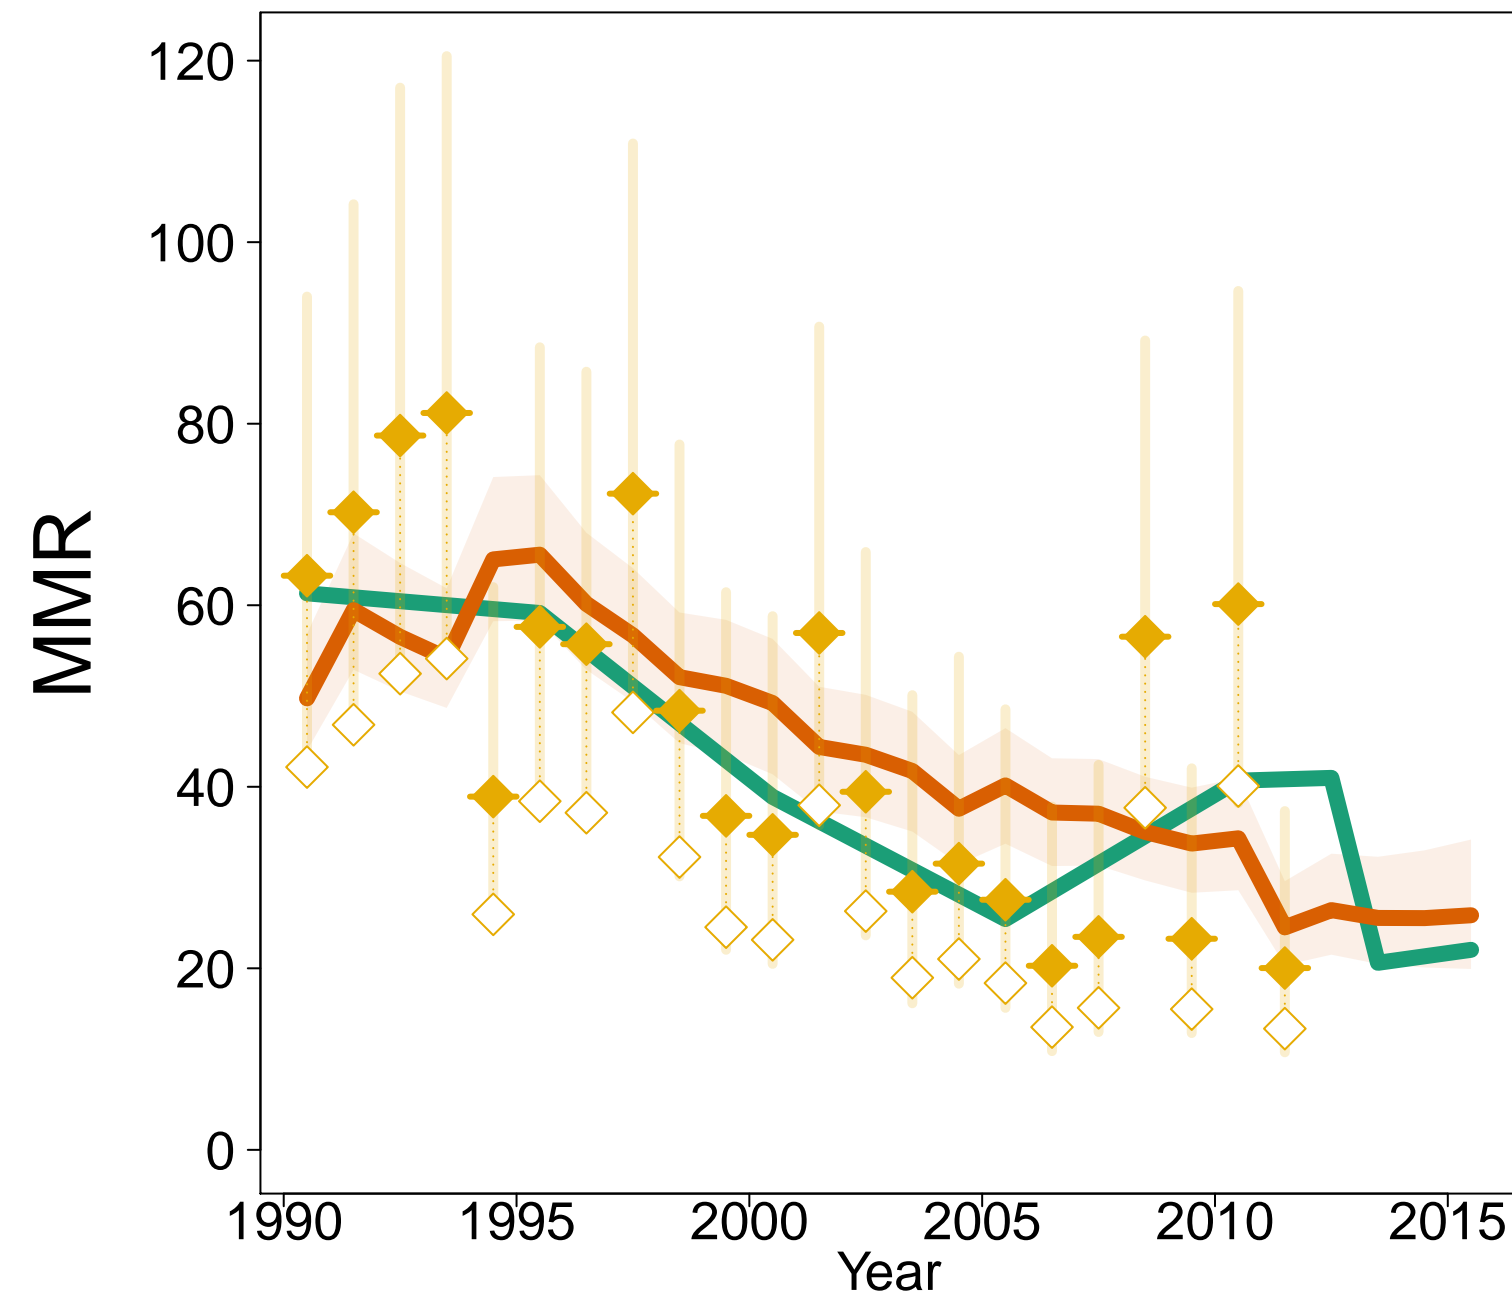

– Estimates –  
Bmat 2014  
MMEIG 2014  
– Data –  
Observed Data  
Adjusted Data  
– Data type –  
VR

Romania [ROU; A]  
(Developed regions)

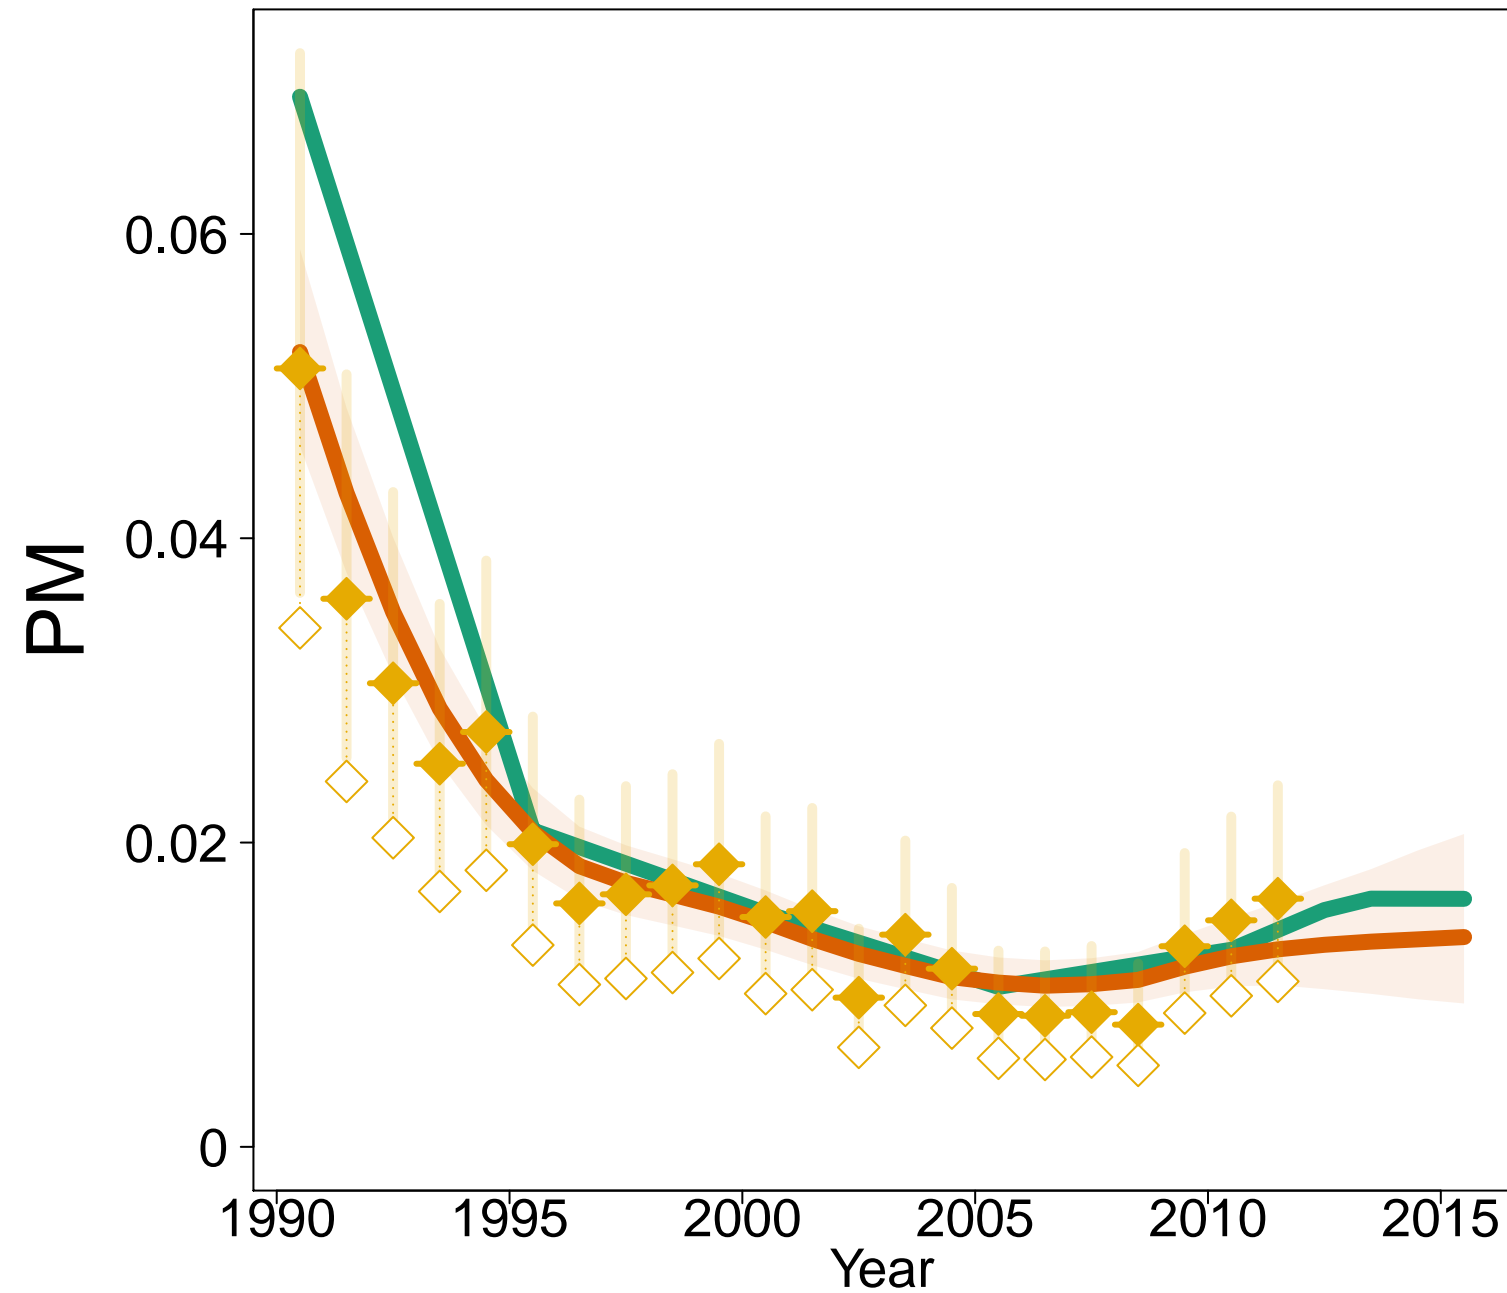

Romania [ROU; A]  
(Developed regions)

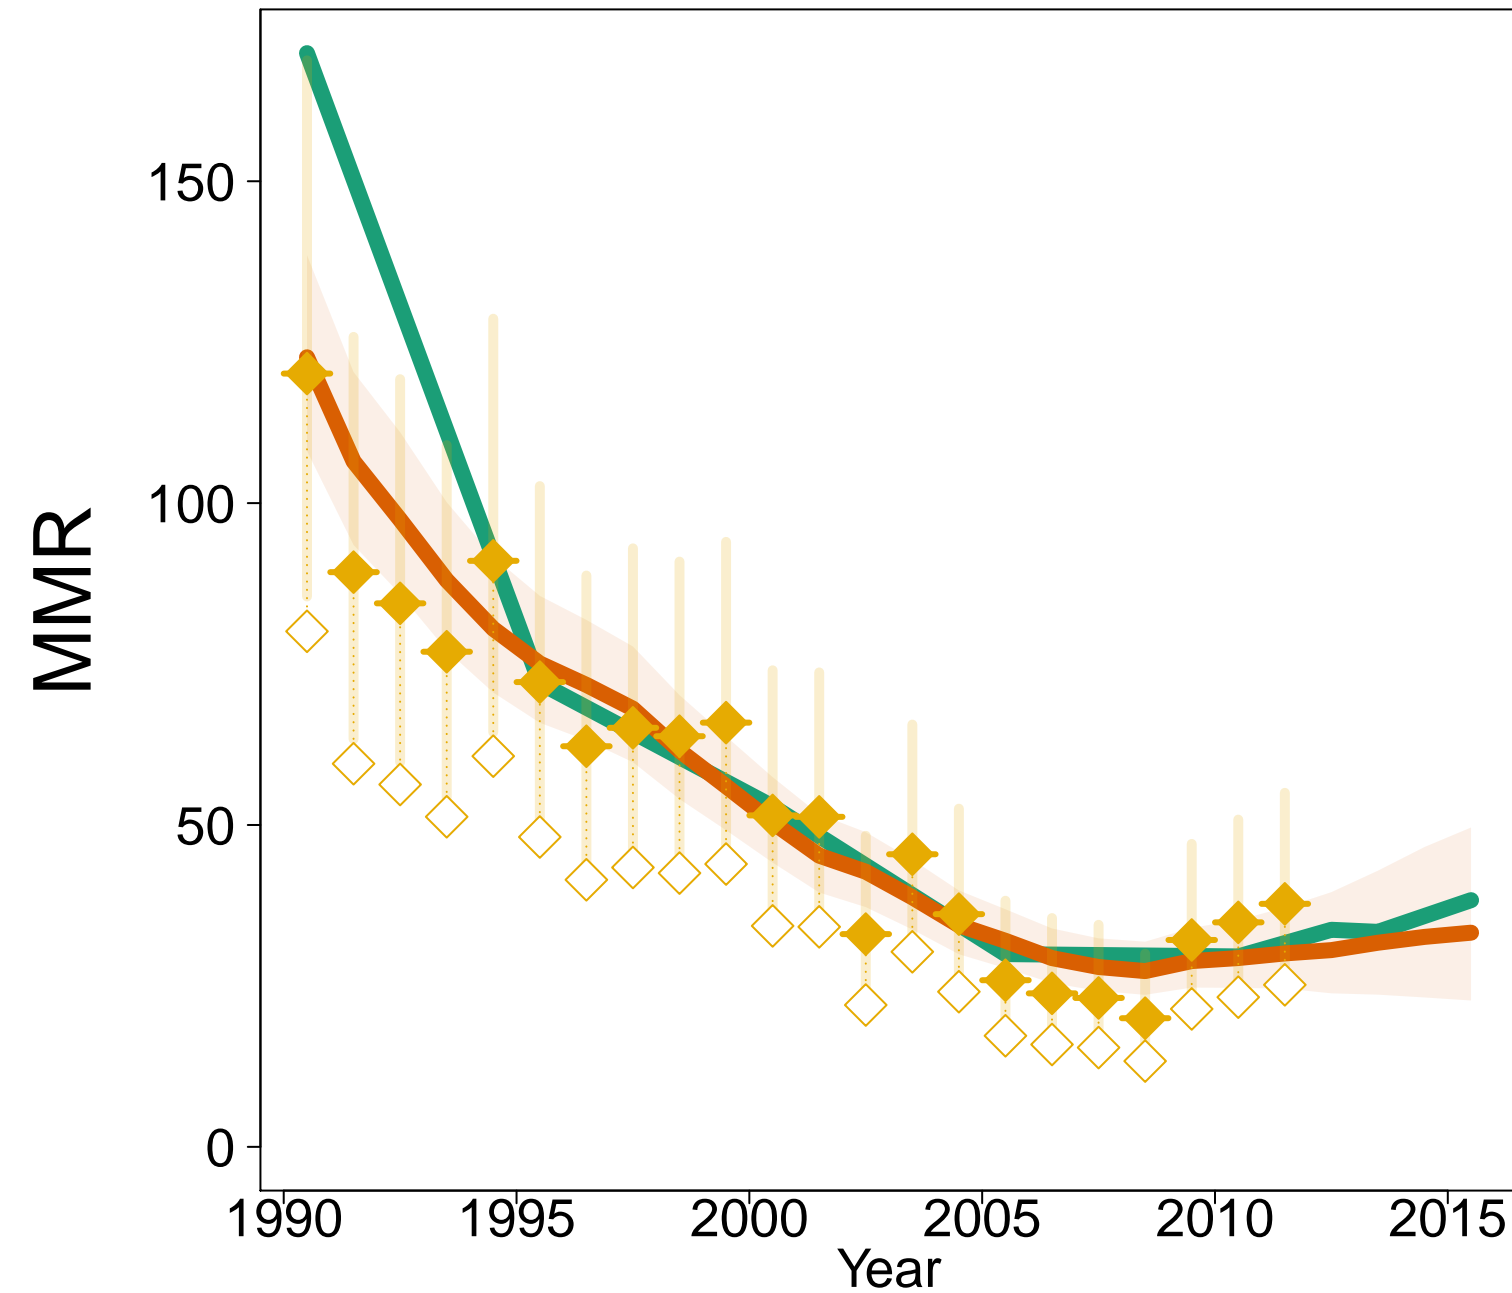

- Estimates –
- Bmat 2014
- MMEIG 2014
- Data –
- Observed Data
- Adjusted Data
- Data type –
- VR

Russian Federation [RUS; A]  
(Developed regions)

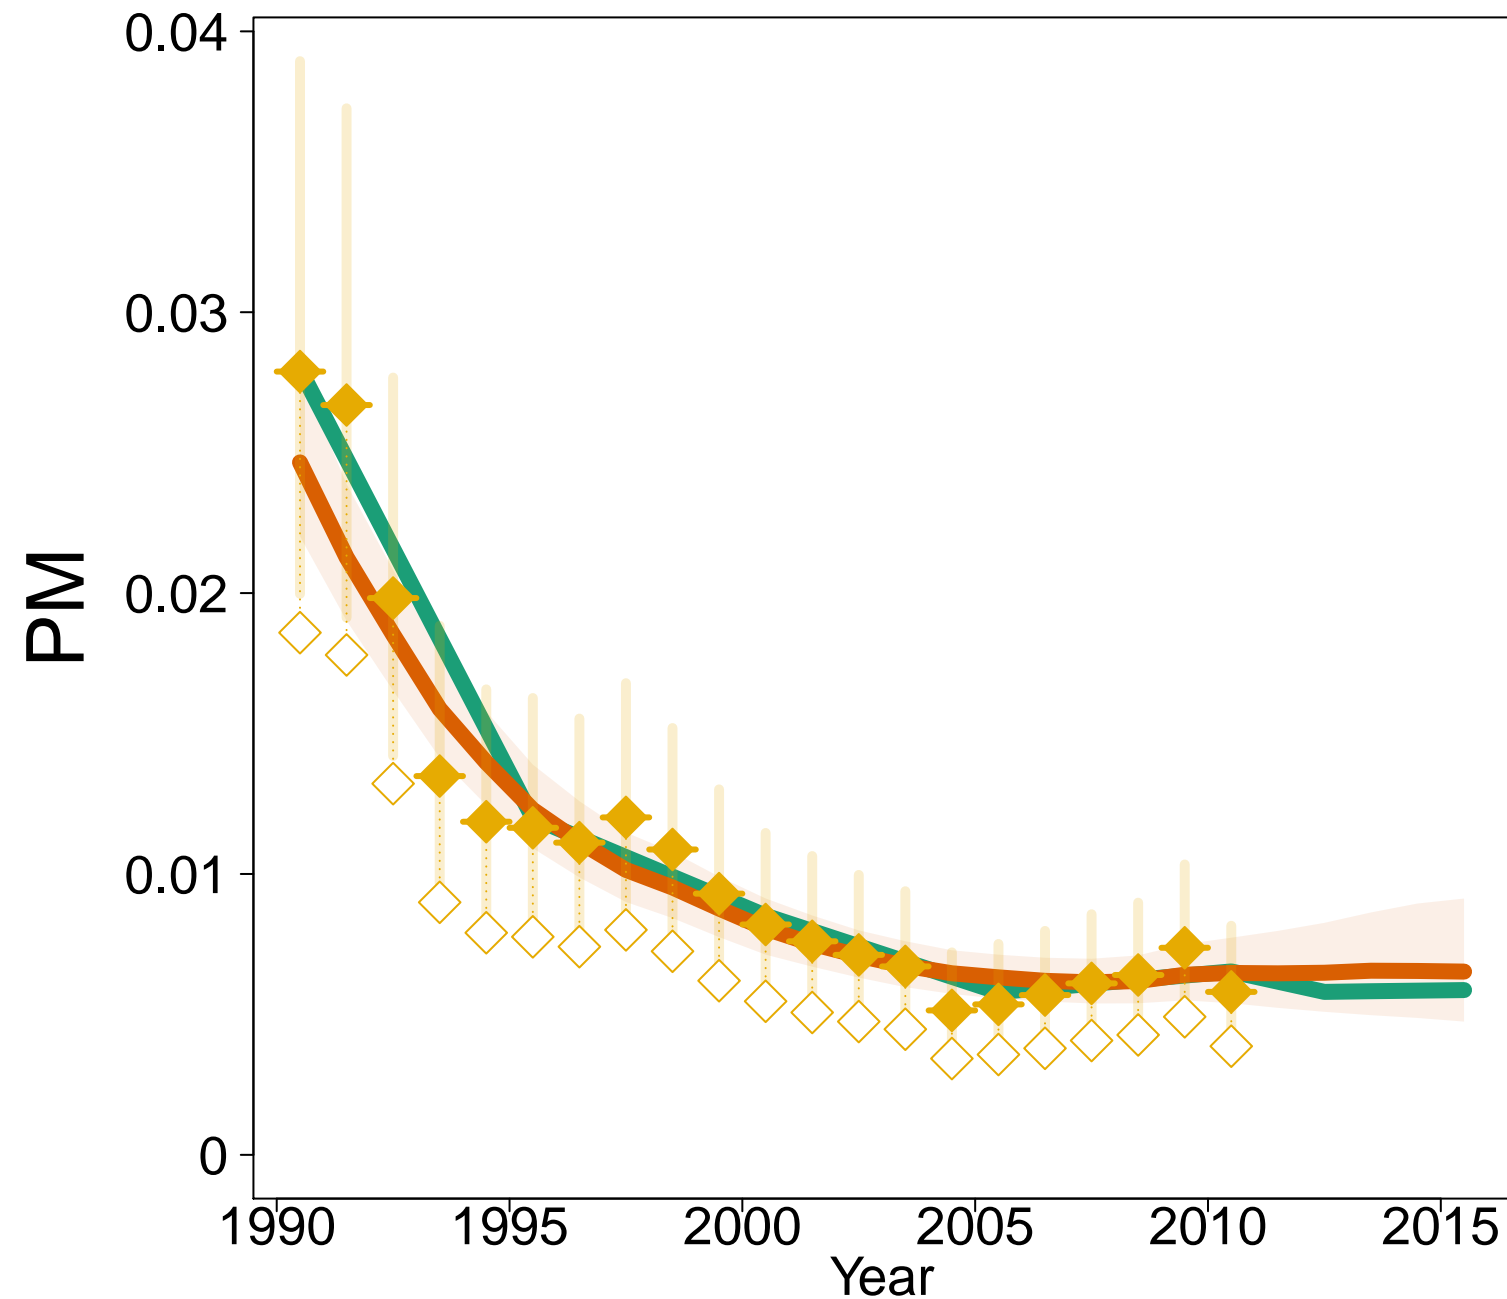

Russian Federation [RUS; A]  
(Developed regions)

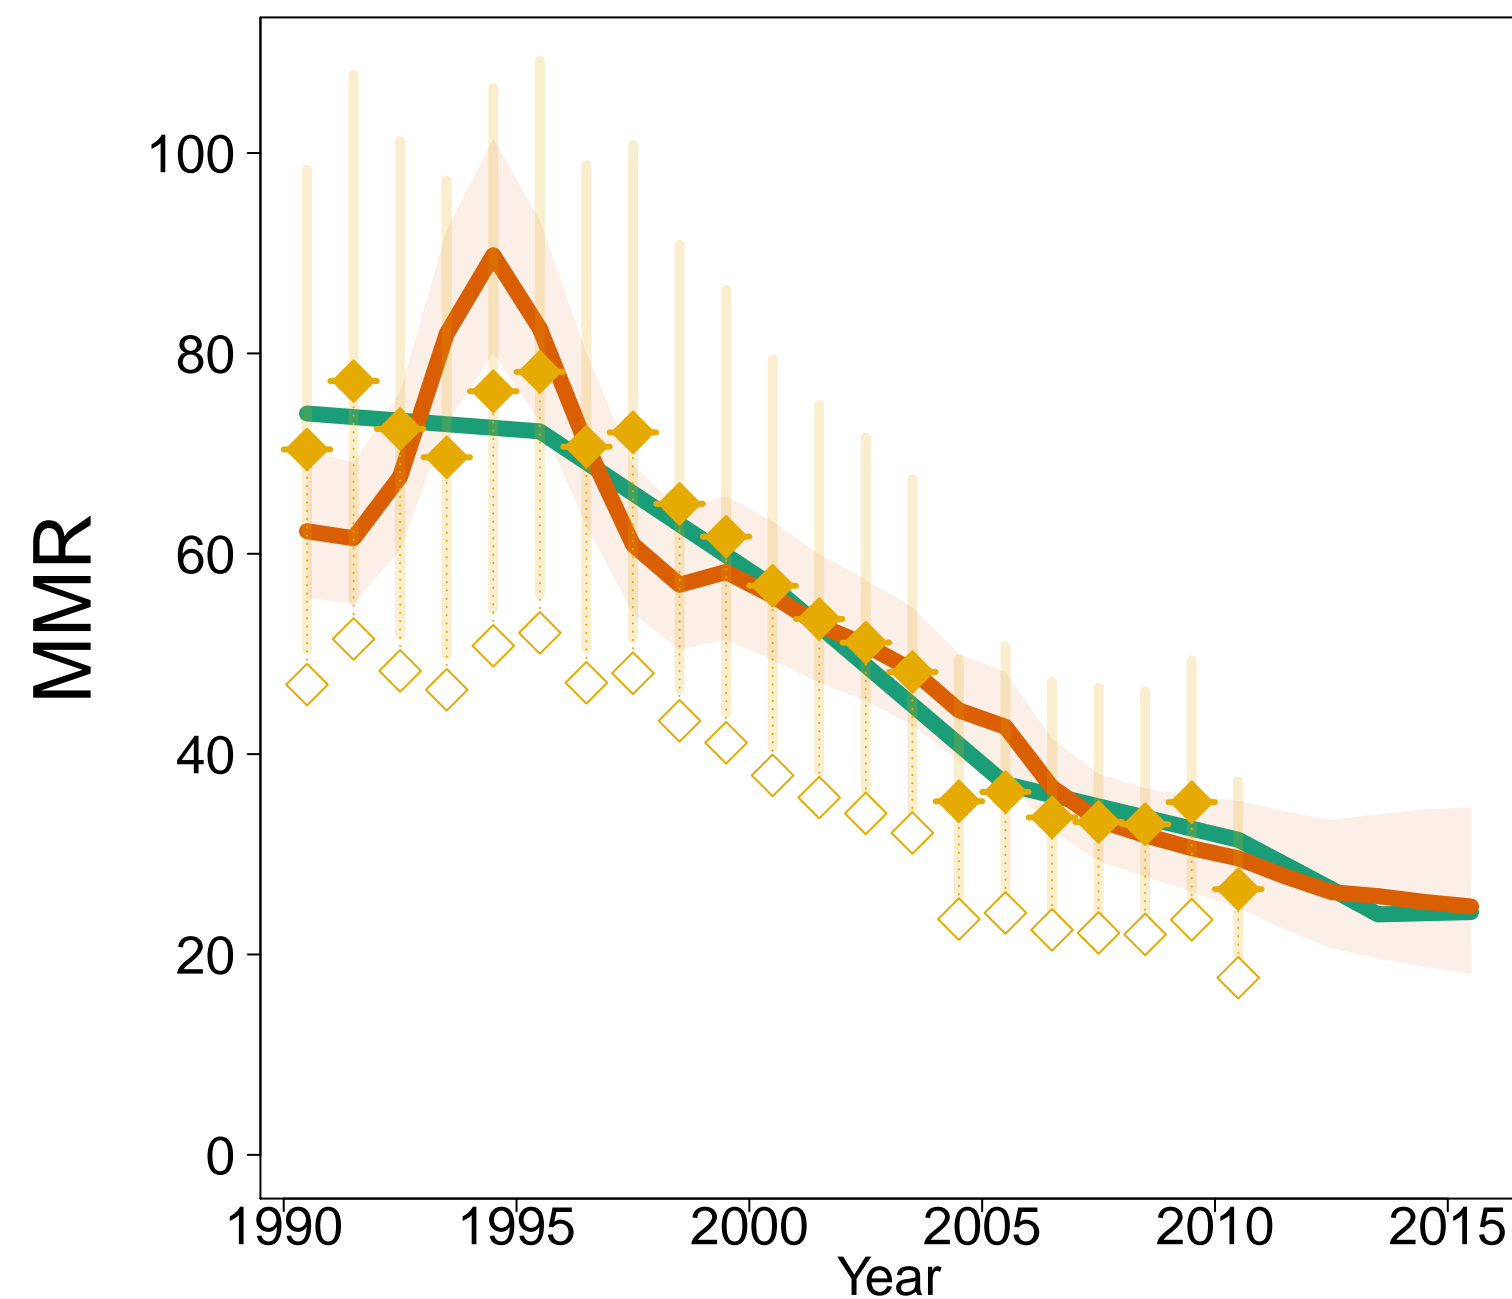

- Estimates –
- Bmat 2014
- MMEIG 2014
- Data –
- Observed Data
- Adjusted Data
- Data type –
- VR

Rwanda [RWA; B]  
(Eastern Africa)

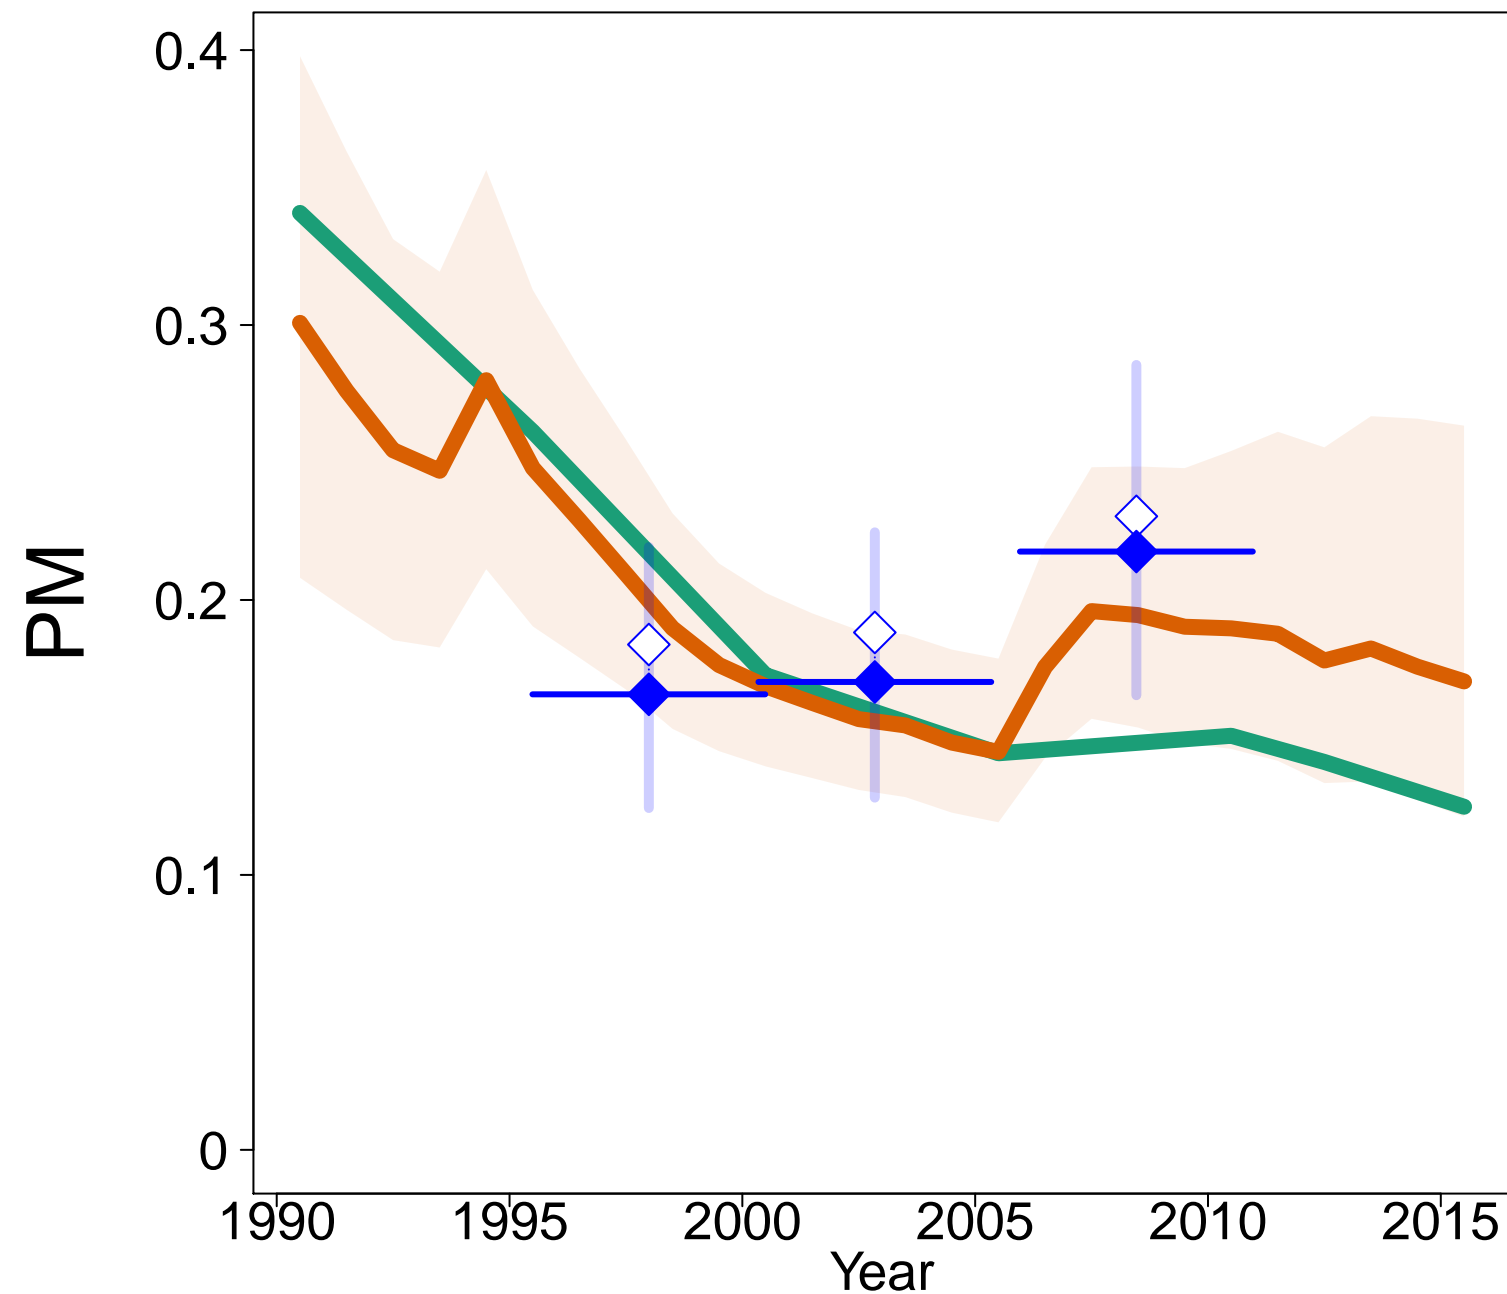

Rwanda [RWA; B]  
(Eastern Africa)

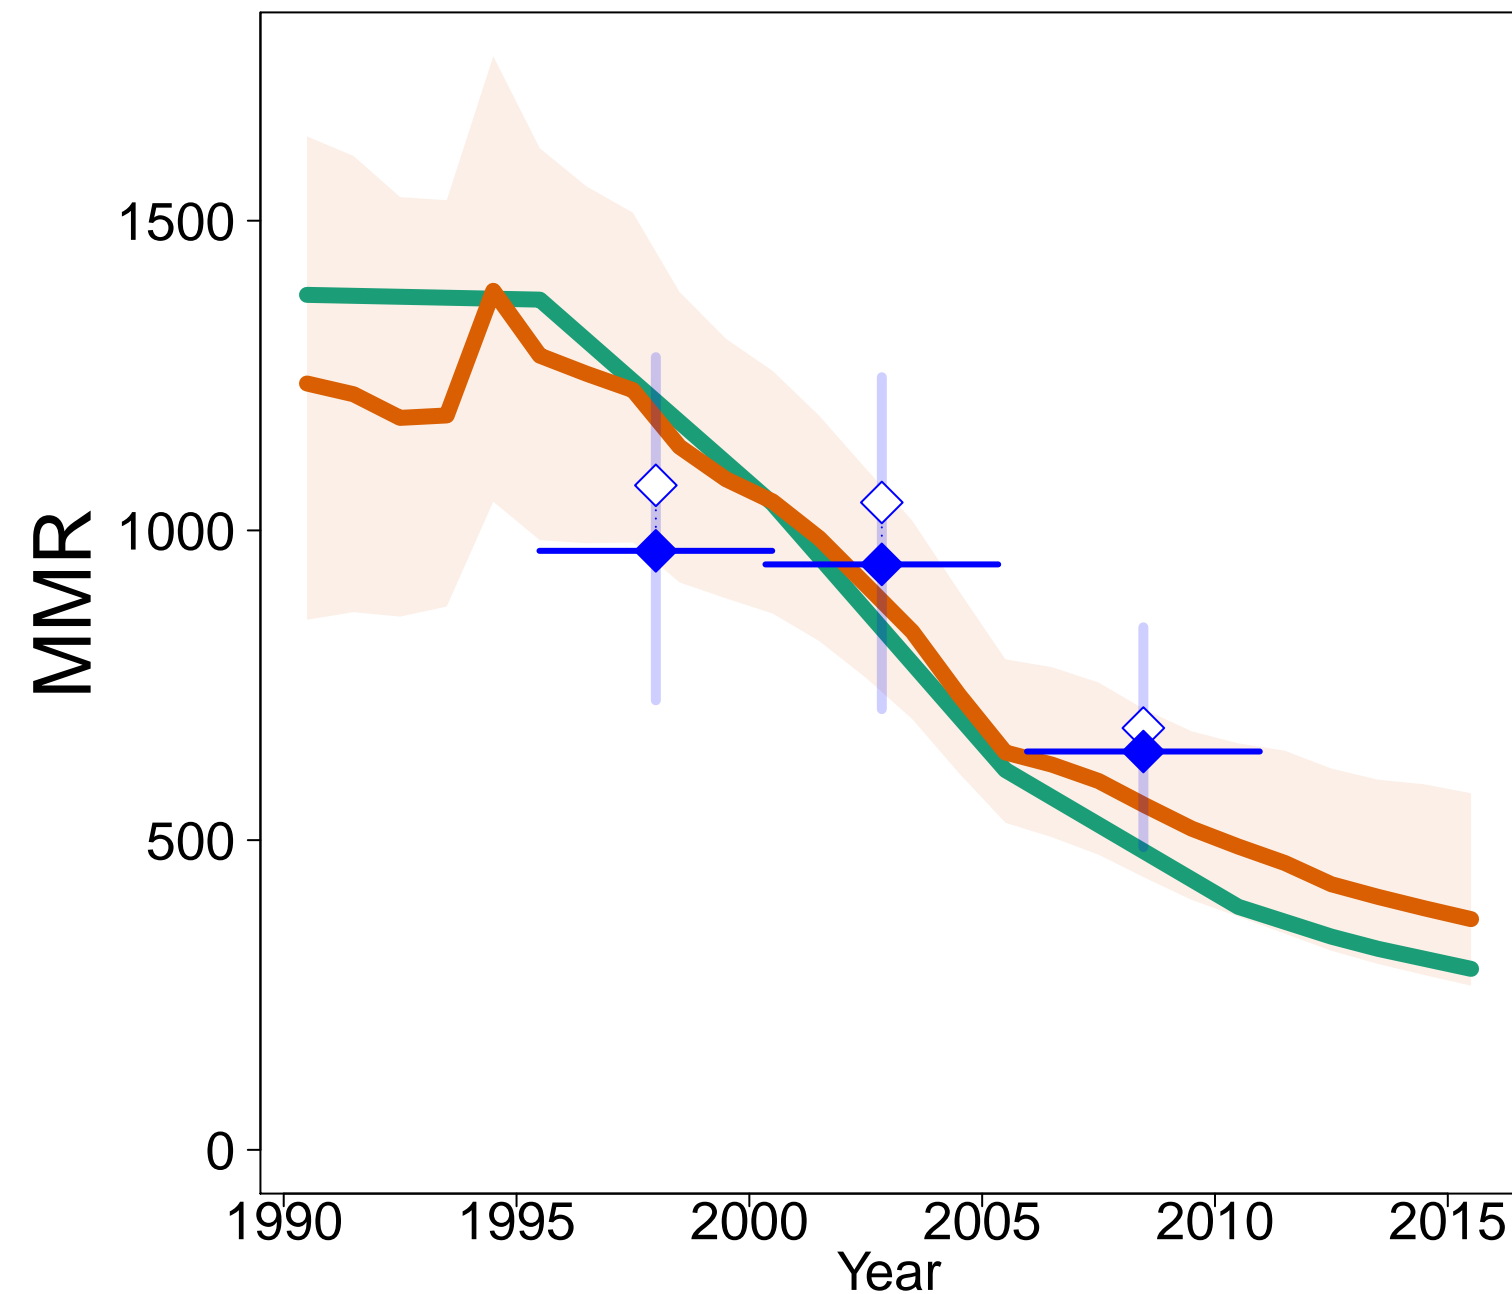

- Estimates –
- Bmat 2014
- MMEIG 2014
- Data –
- Observed Data
- Adjusted Data
- Data type –
- DHS



Saint Lucia [LCA; A]  
(Caribbean)

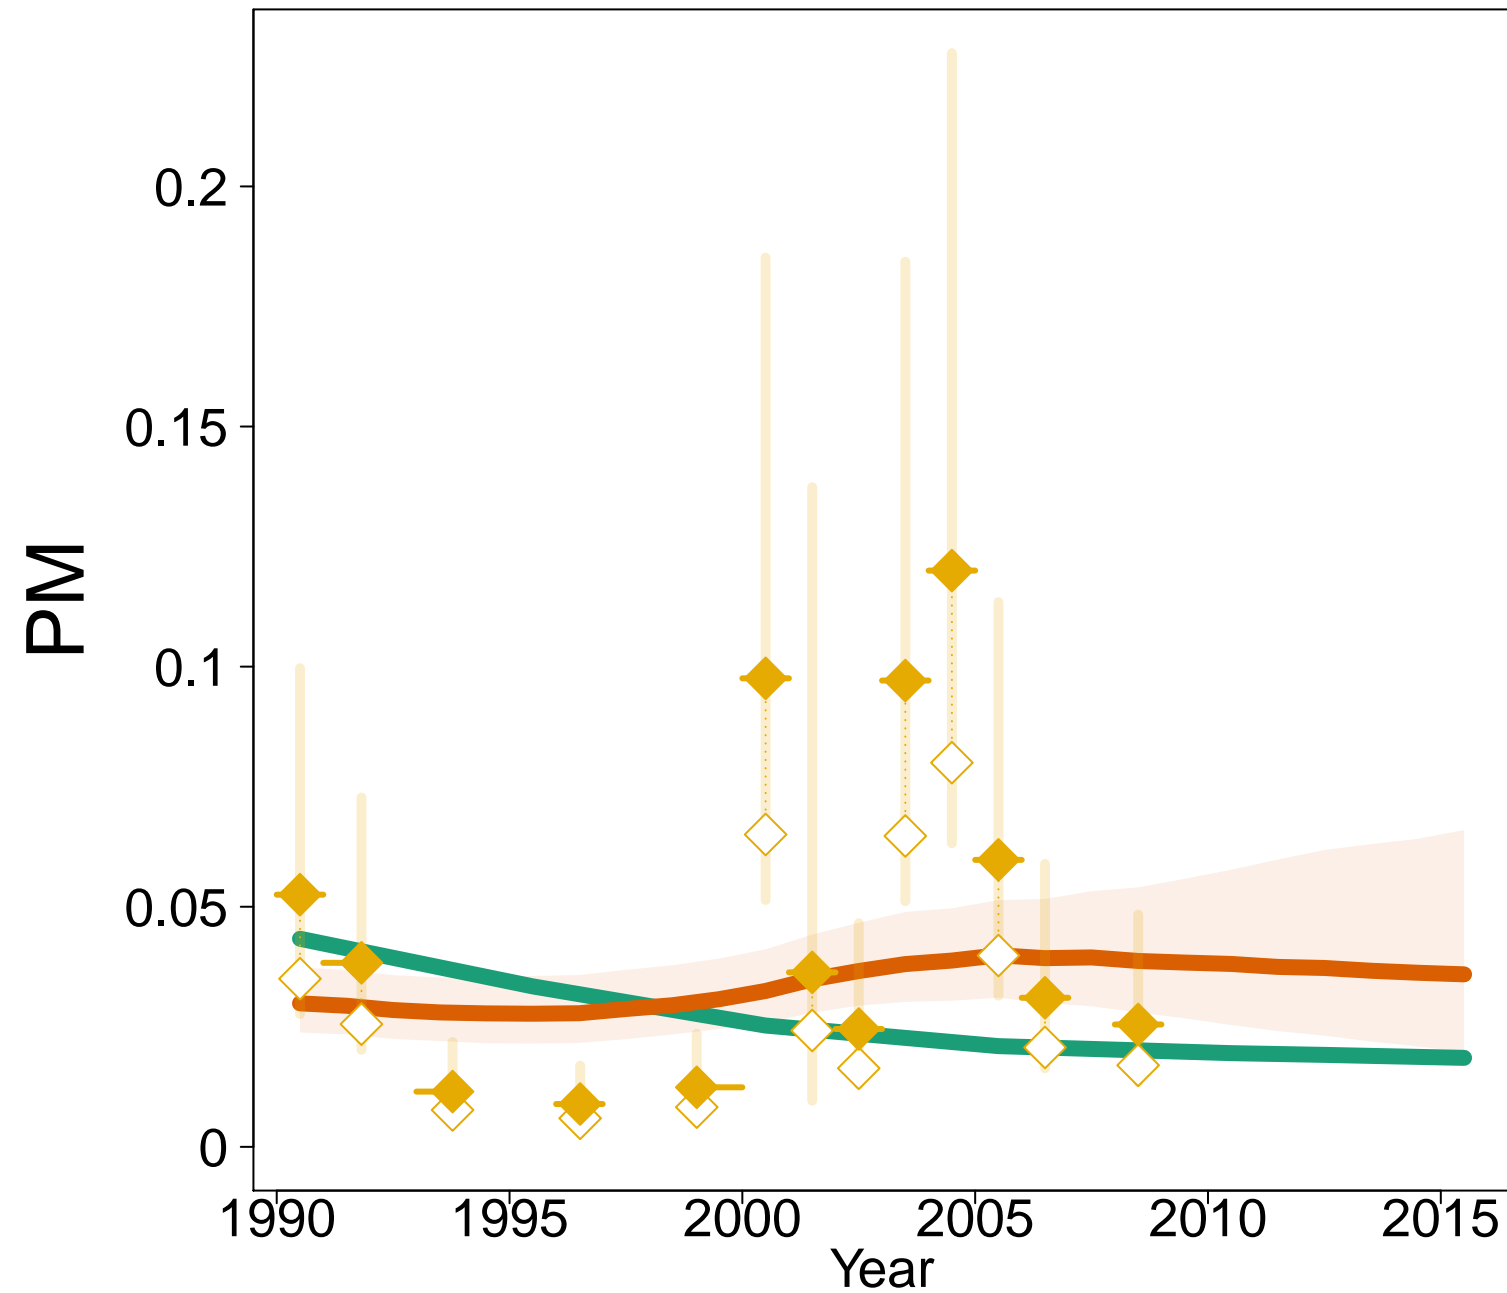

Saint Lucia [LCA; A]  
(Caribbean)

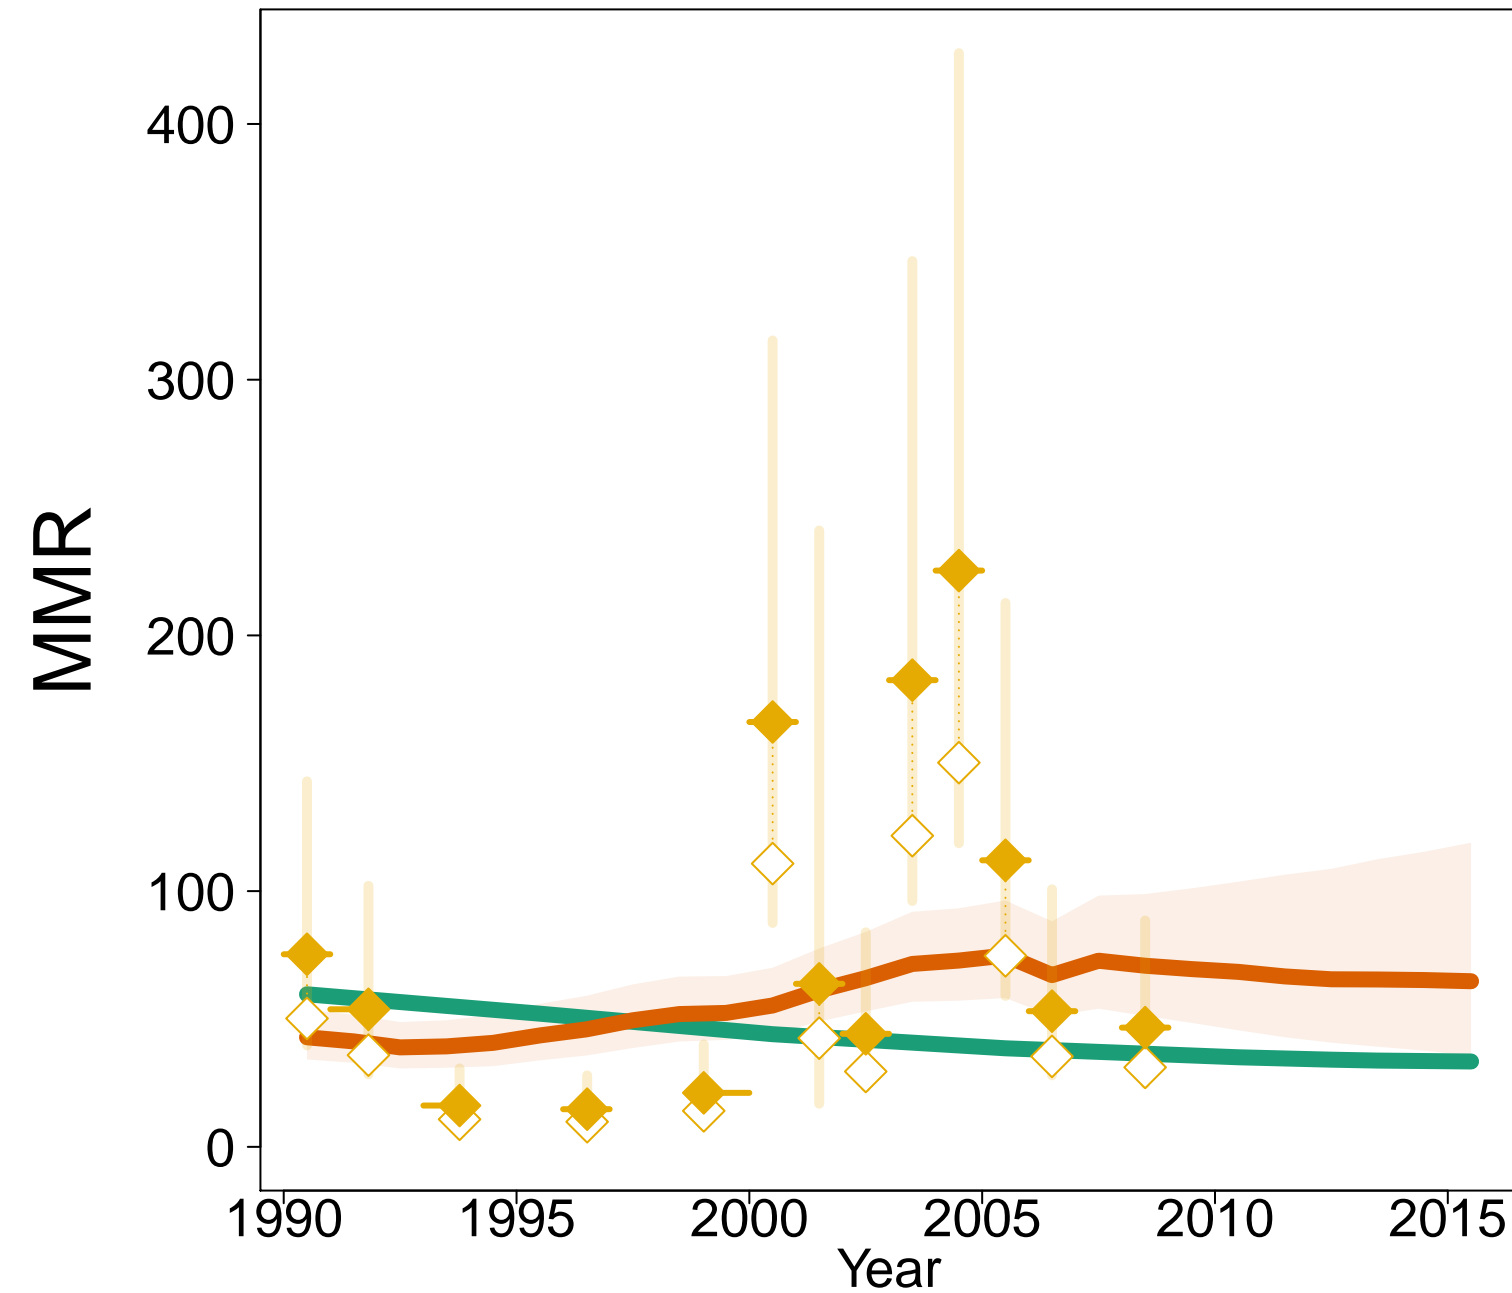

– Estimates –  
Bmat 2014  
MMEIG 2014  
– Data –  
Observed Data  
Adjusted Data  
– Data type –  
VR

Samoa [WSM; C]  
(South-Eastern Asia / Oceania)

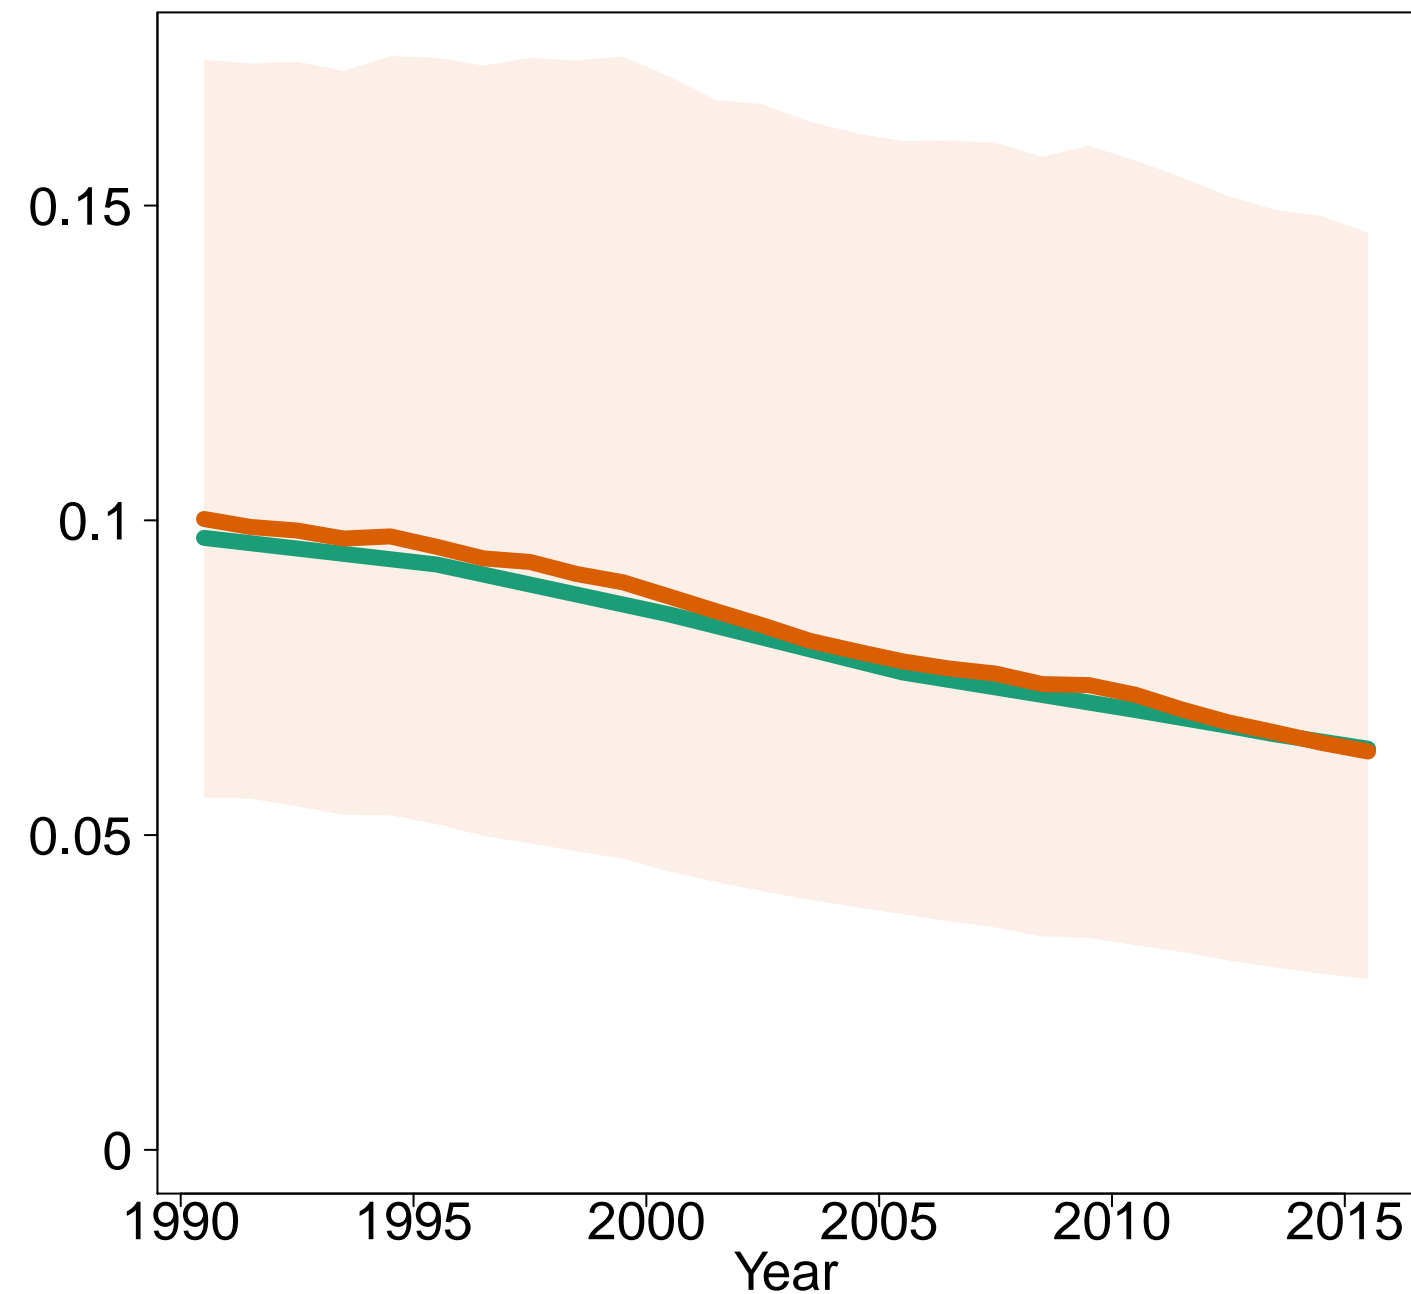

Samoa [WSM; C]  
(South-Eastern Asia / Oceania)

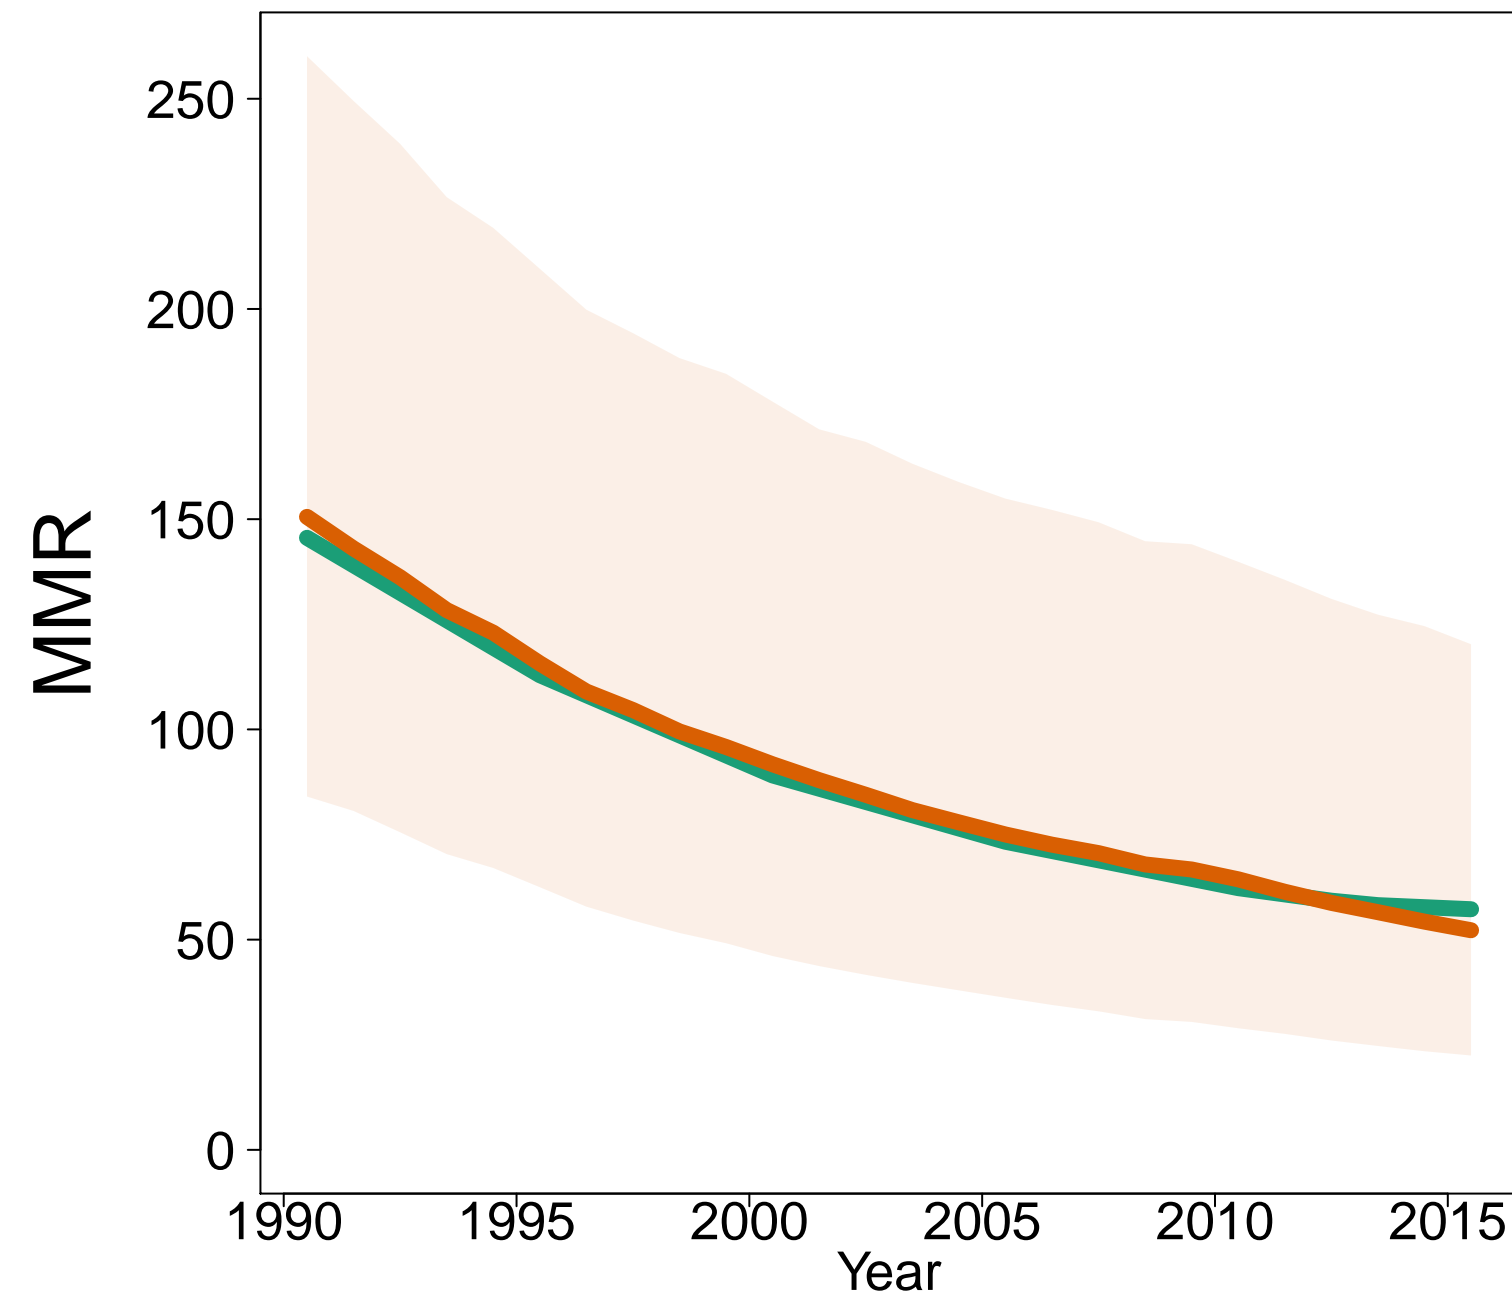

– Estimates –  
Bmat 2014  
MMEIG 2014  
– Data –

Sao Tome and Principe [STP; B]  
(Middle Africa)

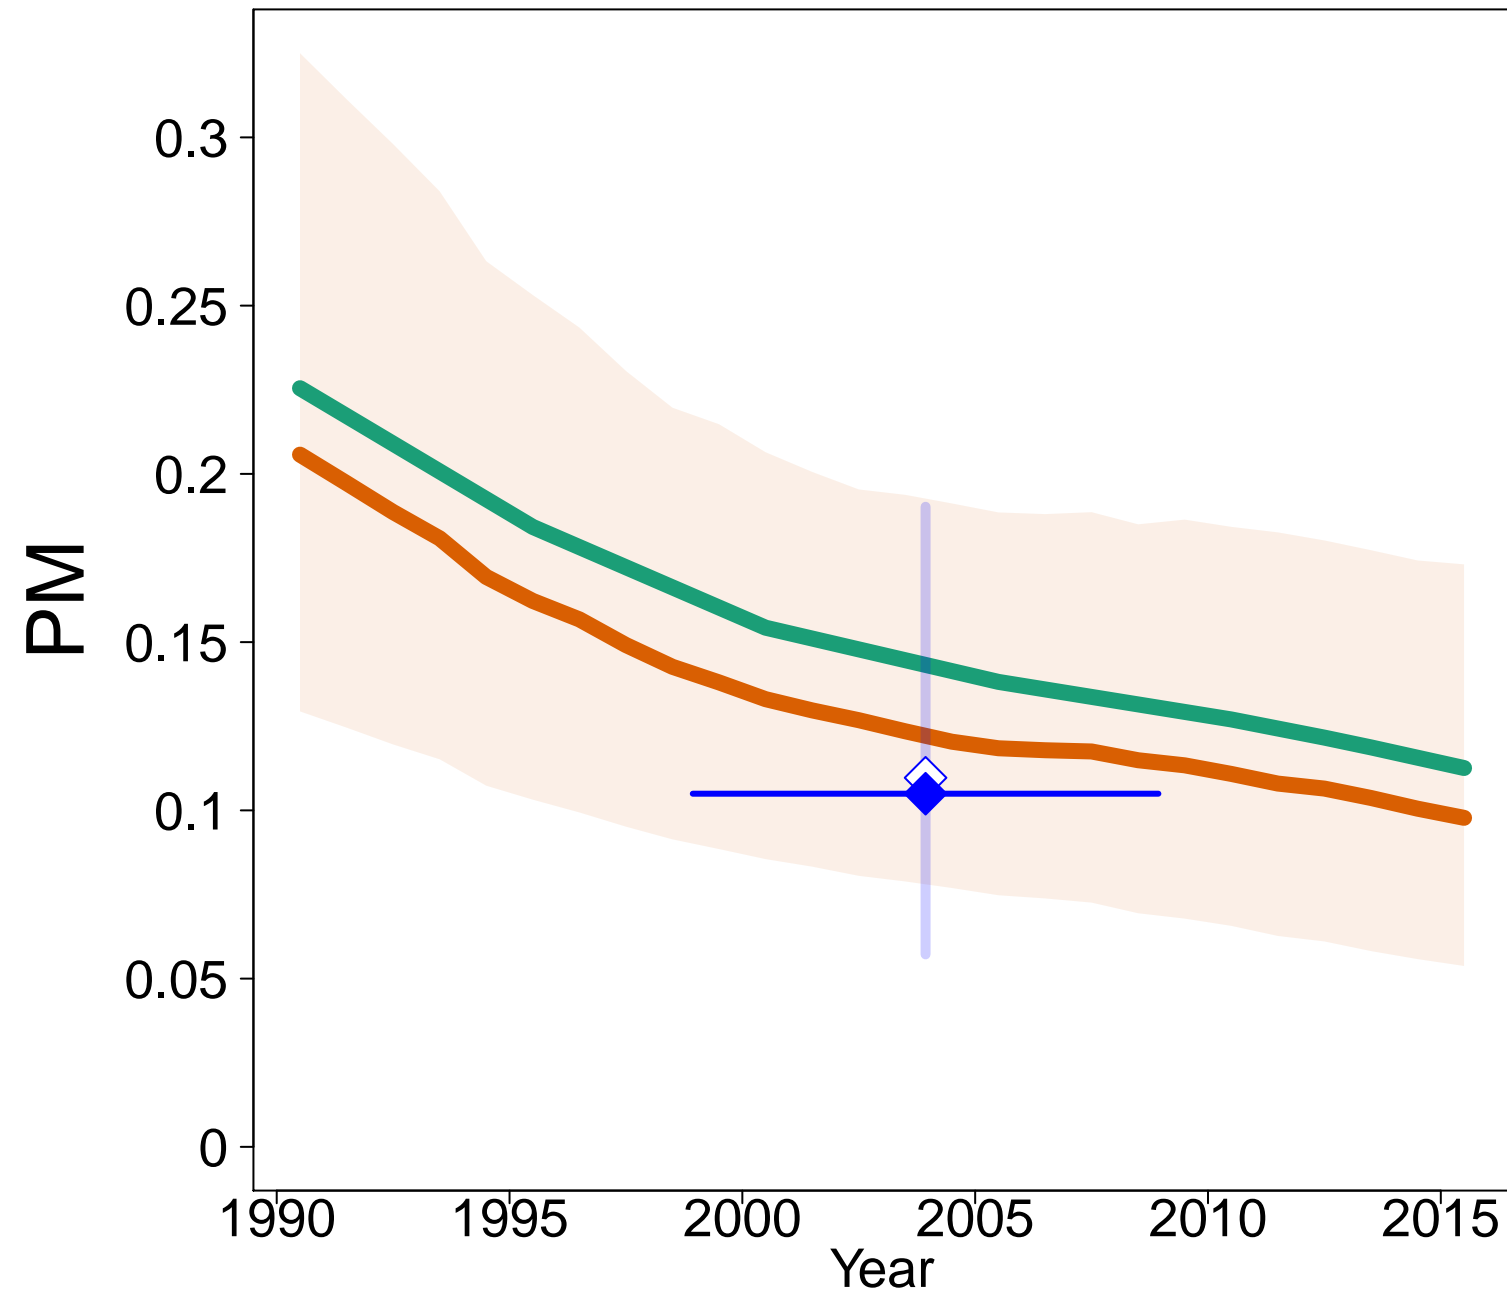

Sao Tome and Principe [STP; B]  
(Middle Africa)

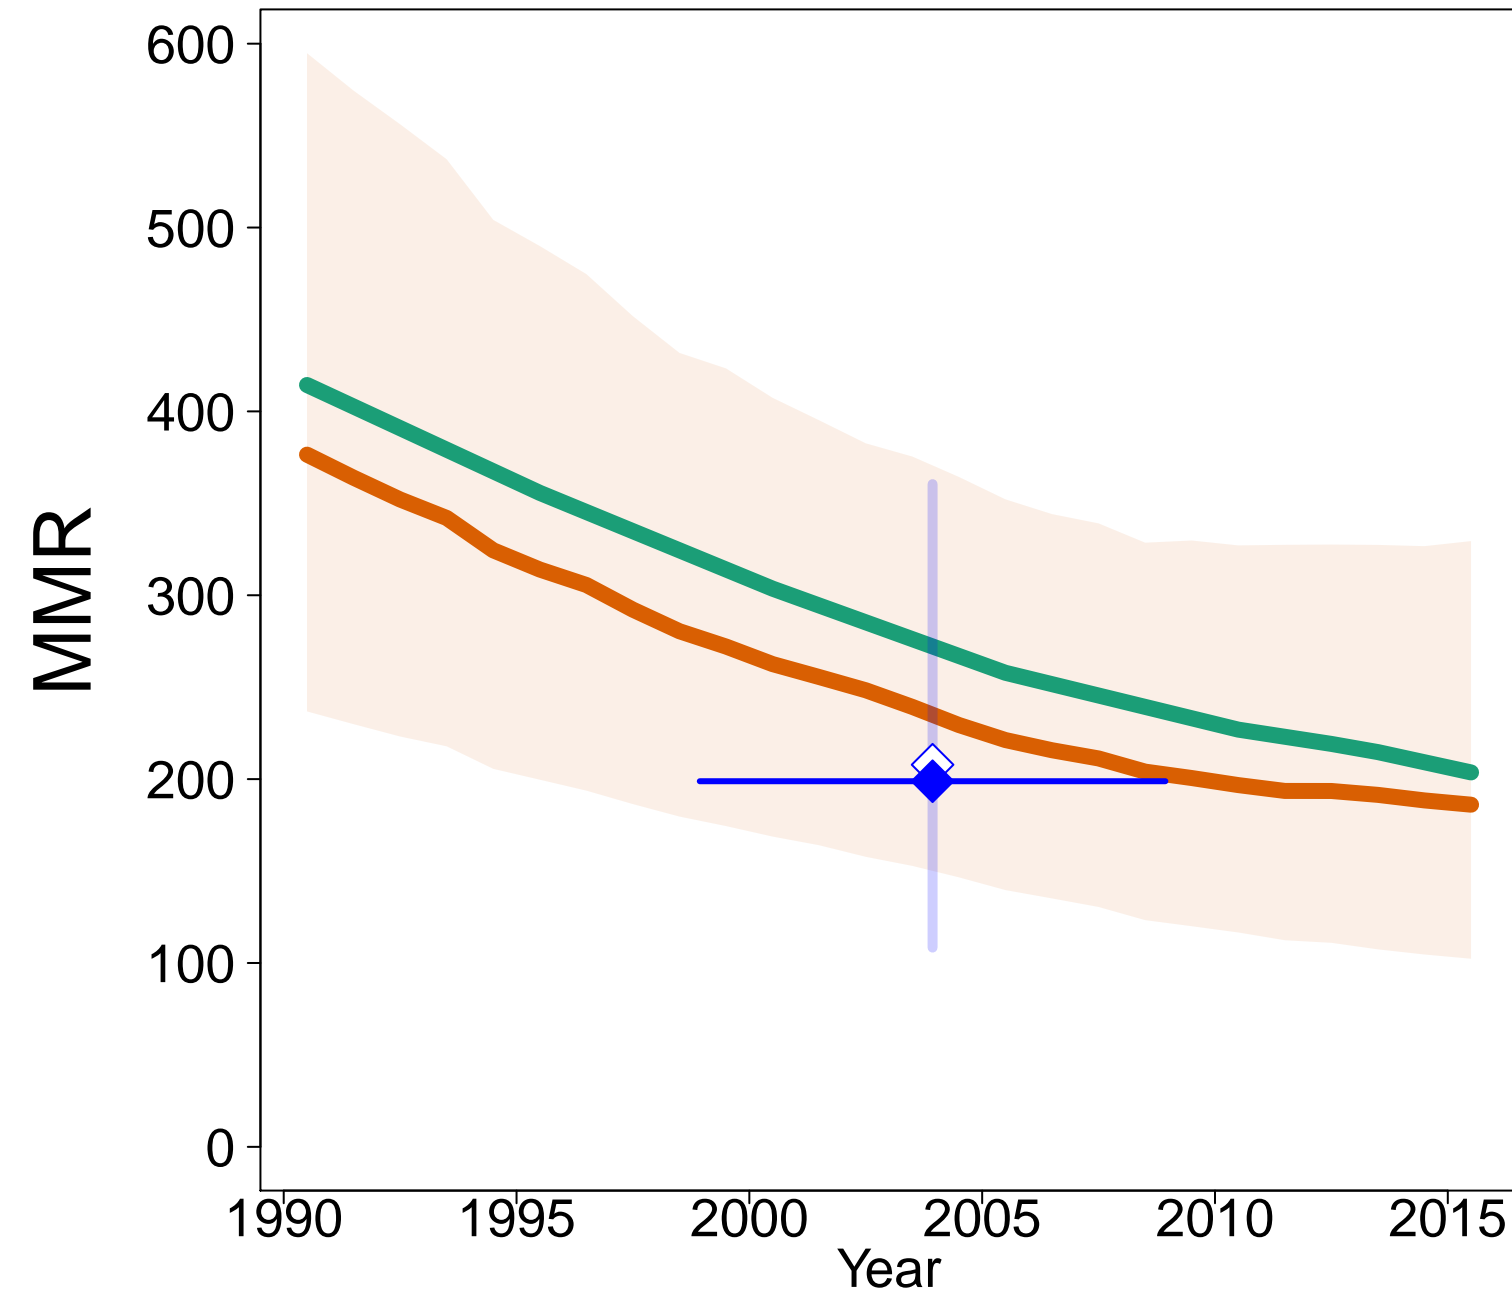

– Estimates –  
 Bmat 2014  
 MMEIG 2014  
 – Data –  
 Observed Data  
 Adjusted Data  
 – Data type –  
 DHS

Saudi Arabia [SAU; B]  
(Western Asia)

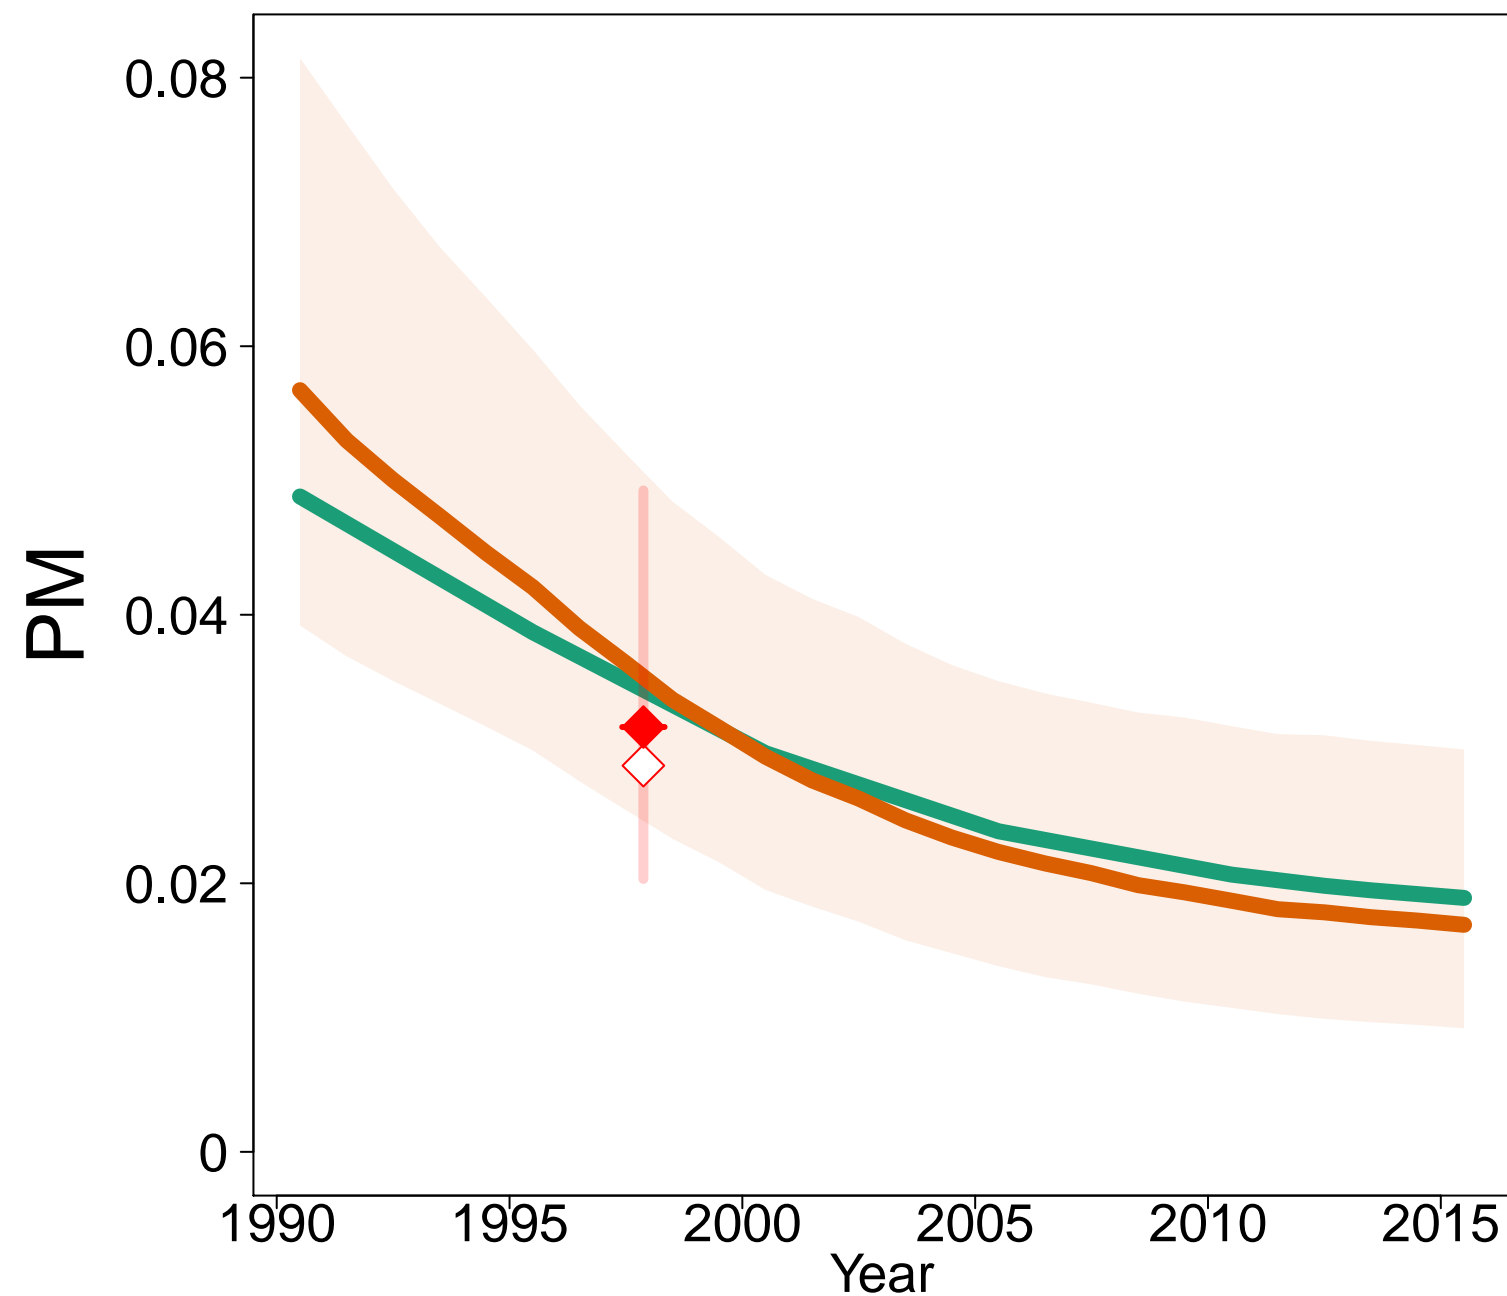

Saudi Arabia [SAU; B]  
(Western Asia)

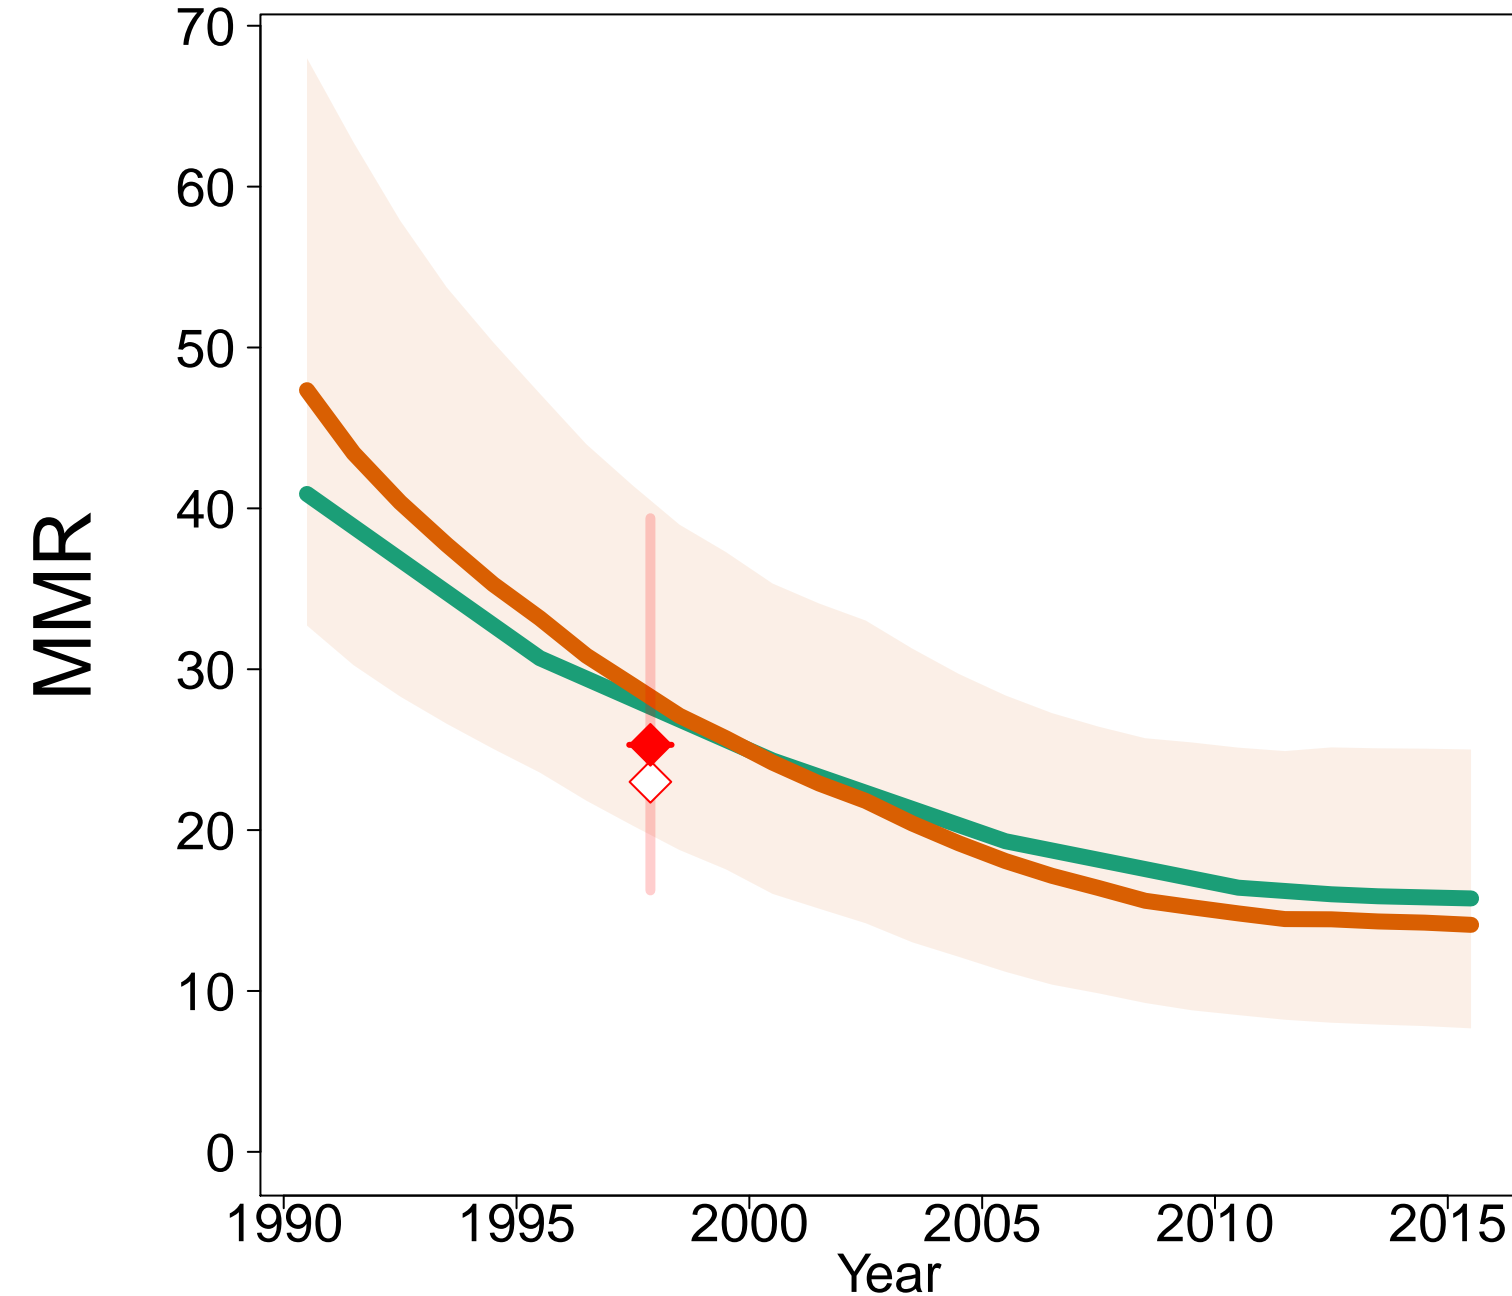

- Estimates –
- Bmat 2014
- MMEIG 2014
- Data –
- ◊ Observed Data
- ◆ Adjusted Data
- Data type –
- ◆ Misc. studies

Senegal [SEN; B]  
(Western Africa)

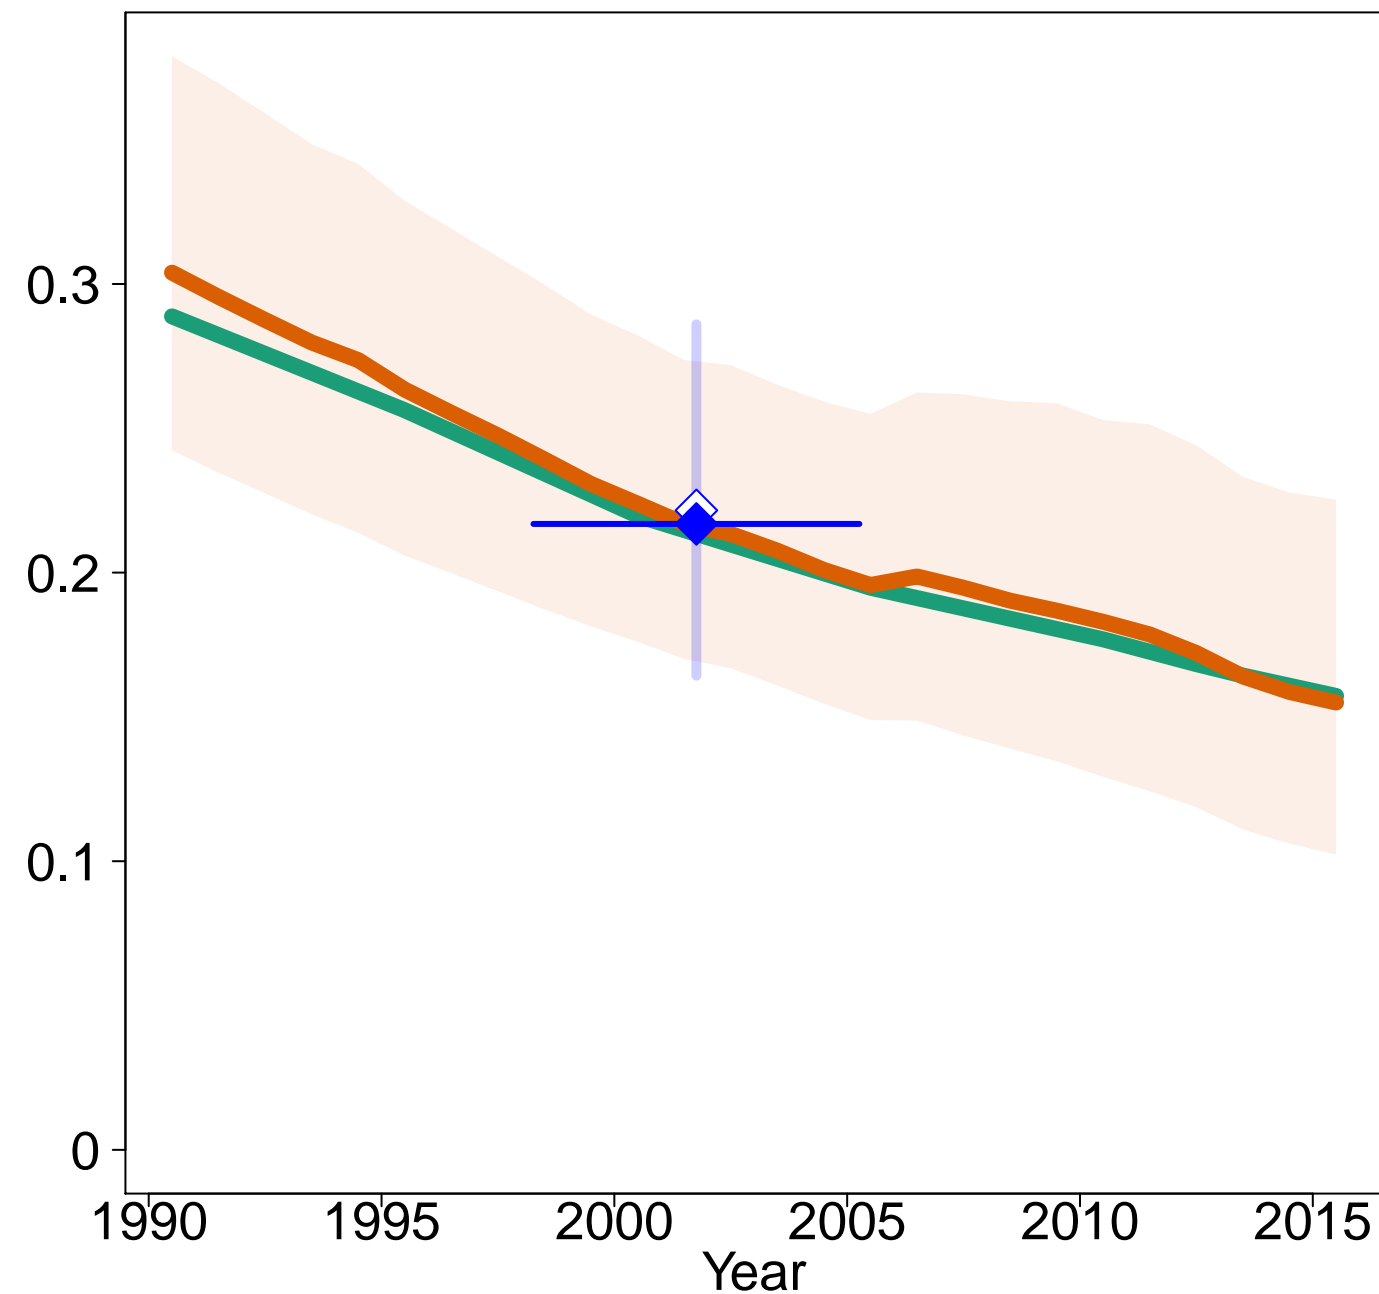

Senegal [SEN; B]  
(Western Africa)

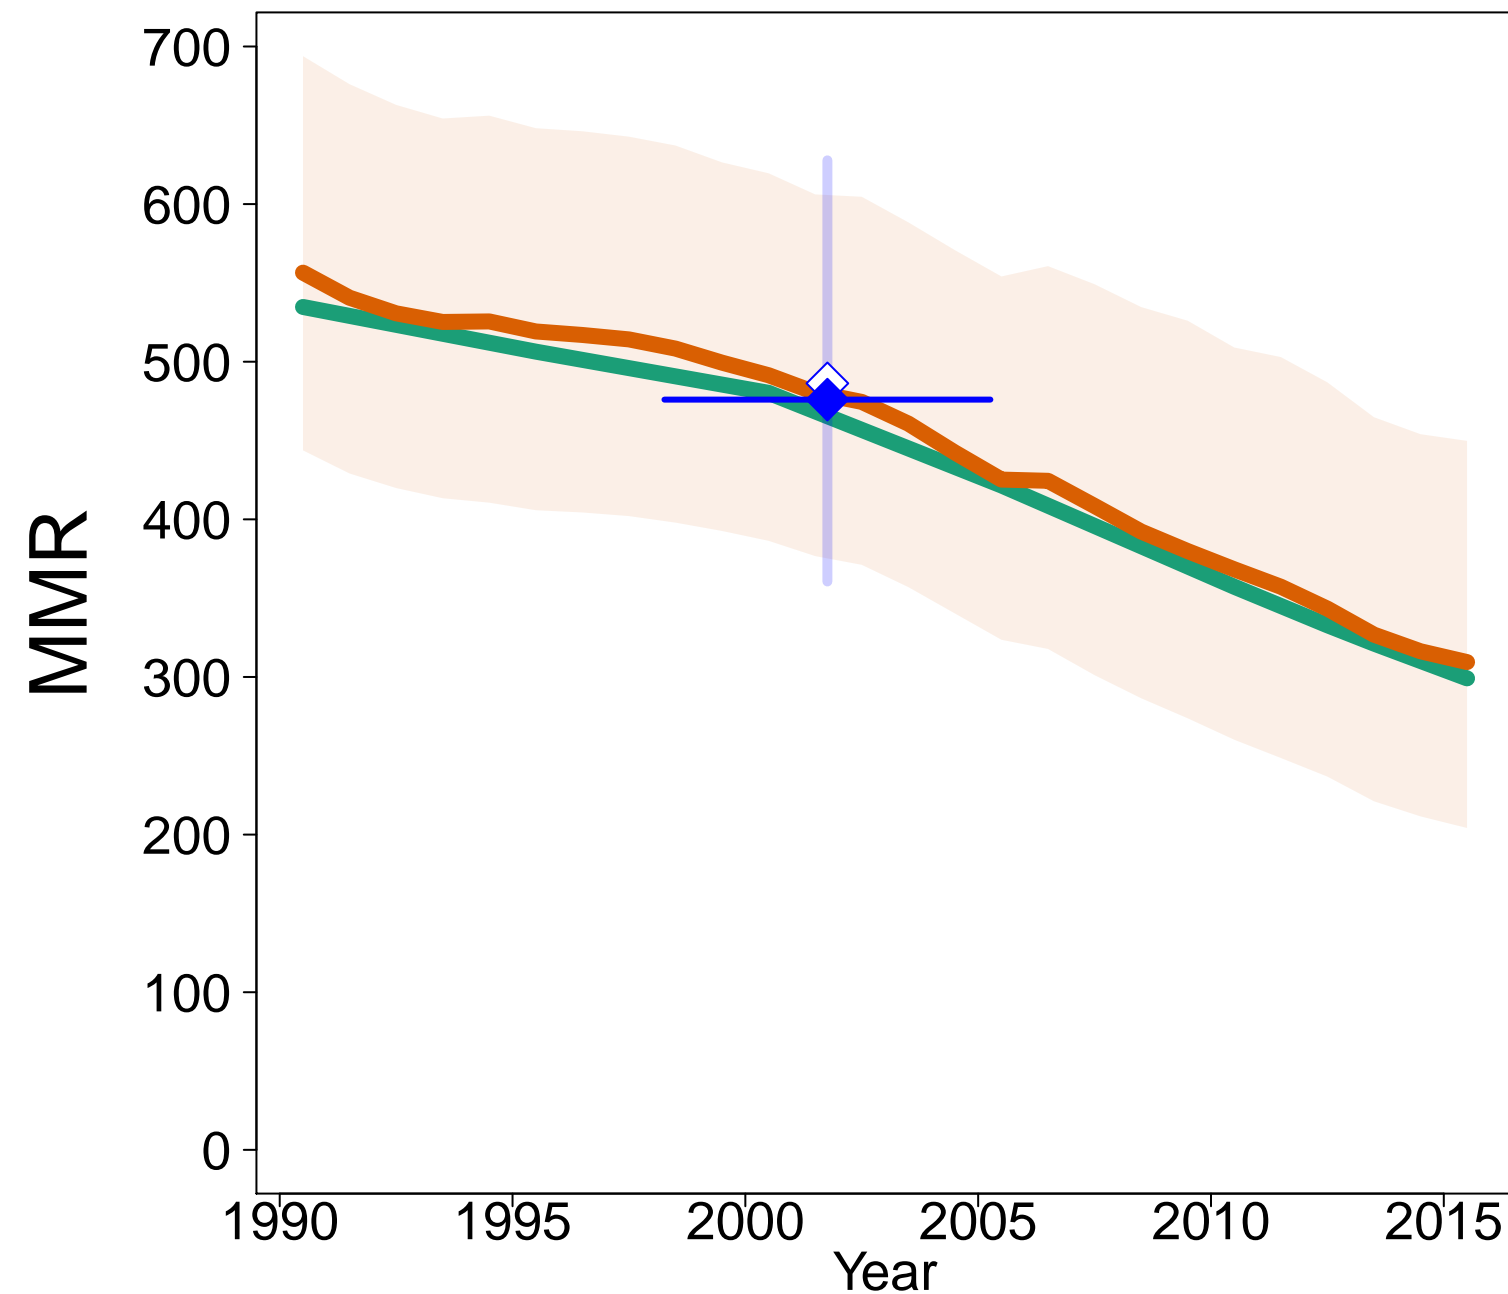

- Estimates –
- Bmat 2014
- MMEIG 2014
- Data –
- Observed Data
- Adjusted Data
- Data type –
- DHS

Serbia [SRB; A]  
(Transition countries of South-Eastern Europe)

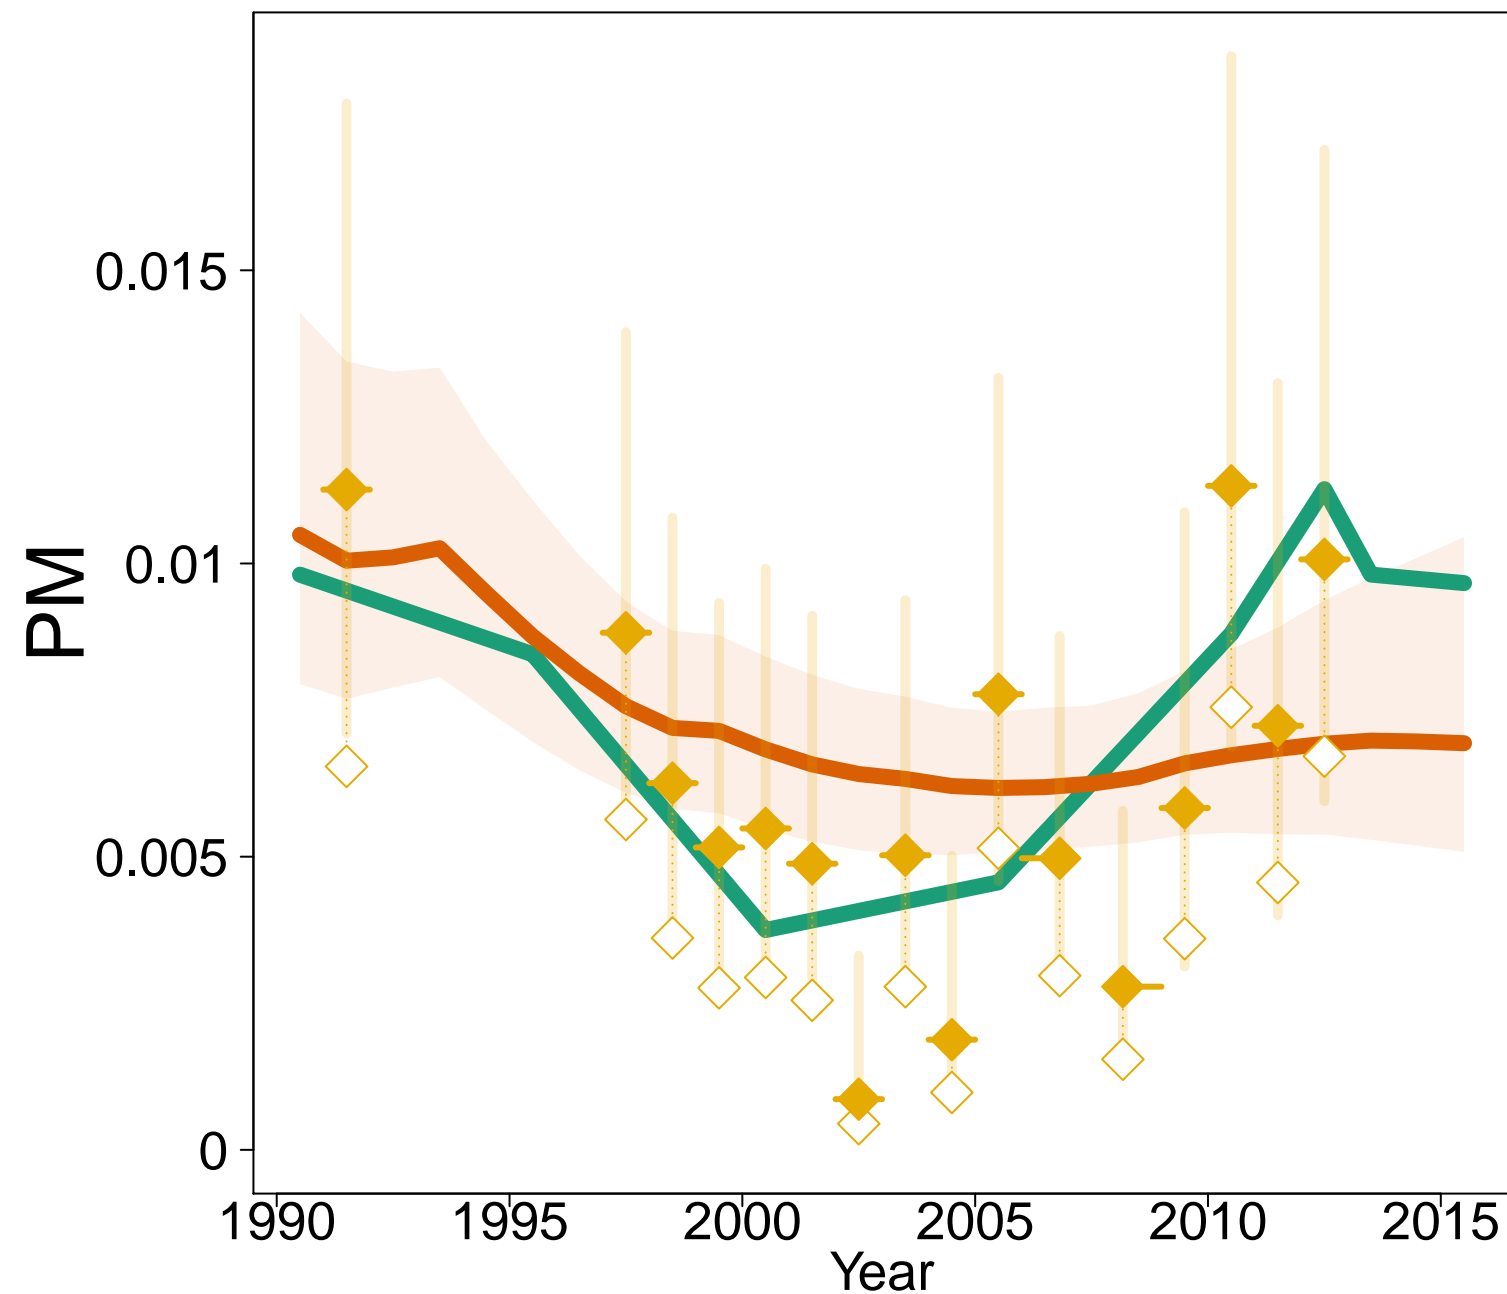

Serbia [SRB; A]  
(Transition countries of South-Eastern Europe)

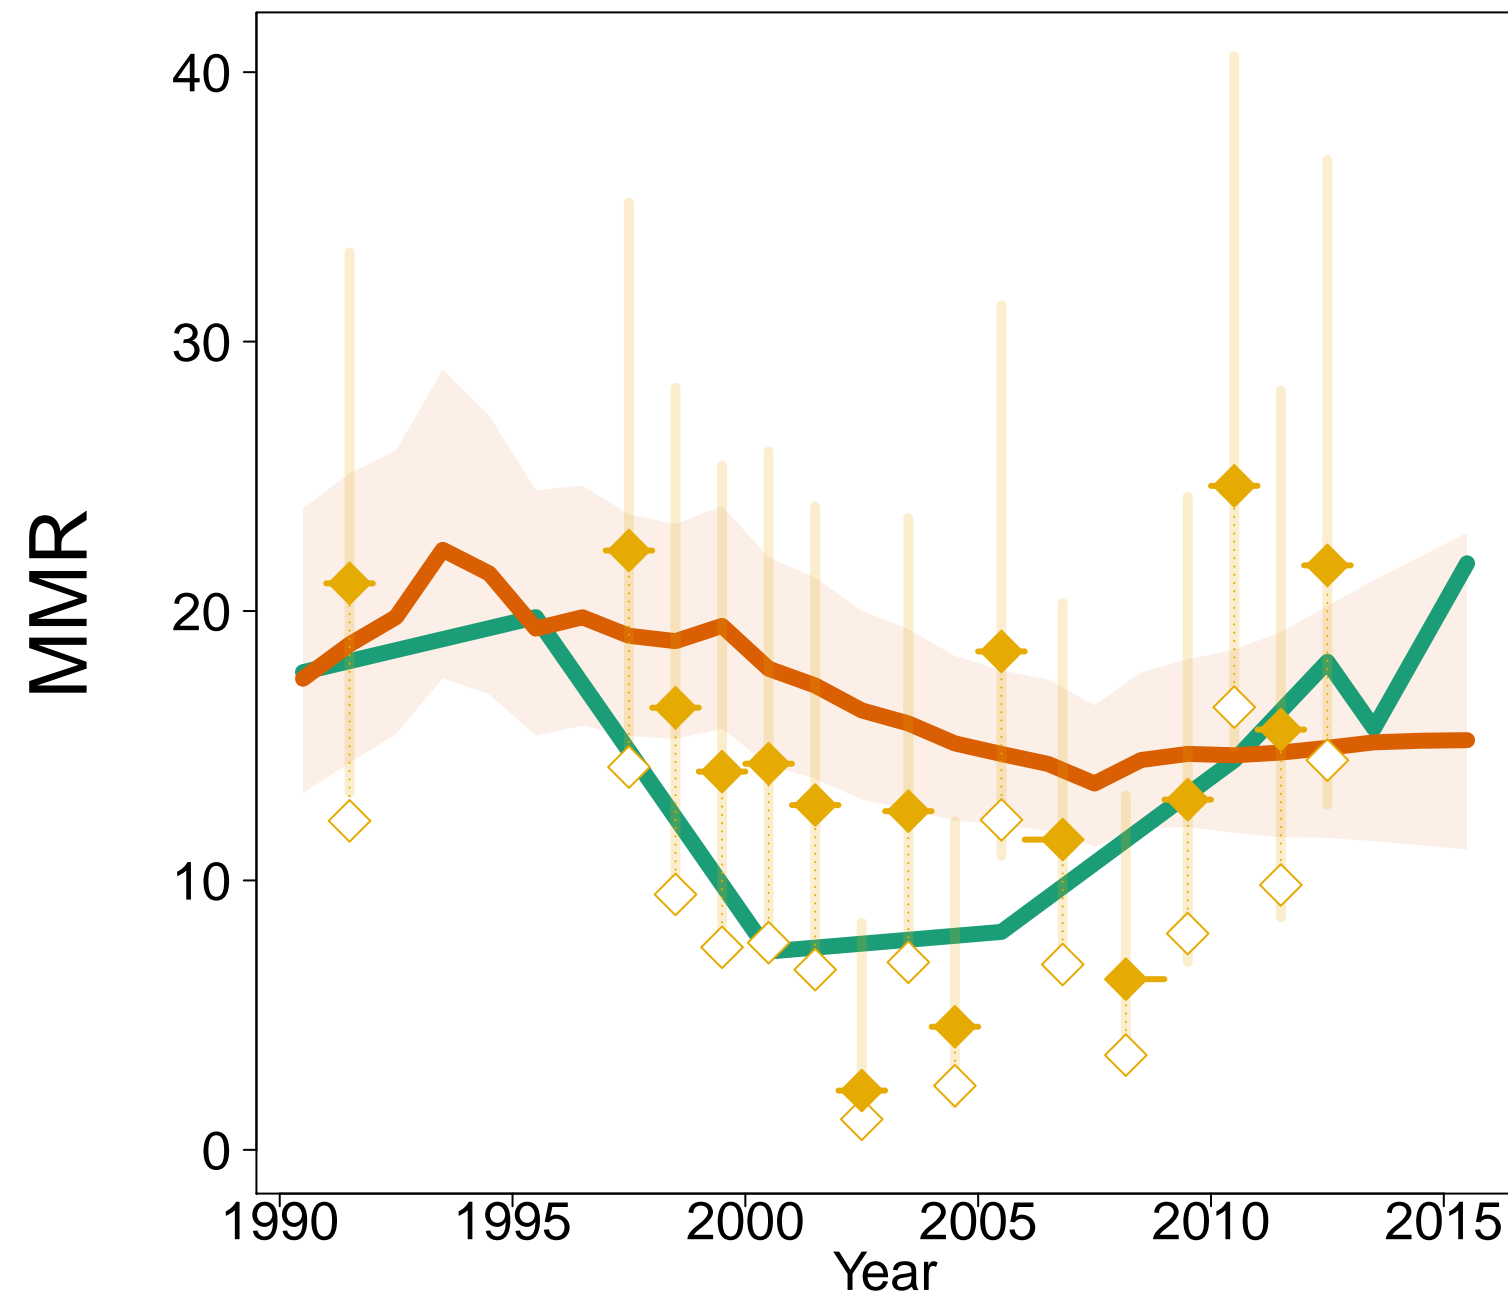

– Estimates –  
Bmat 2014  
MMEIG 2014  
– Data –  
Observed Data  
Adjusted Data  
– Data type –  
VR

Sierra Leone [SLE; B]  
(Western Africa)

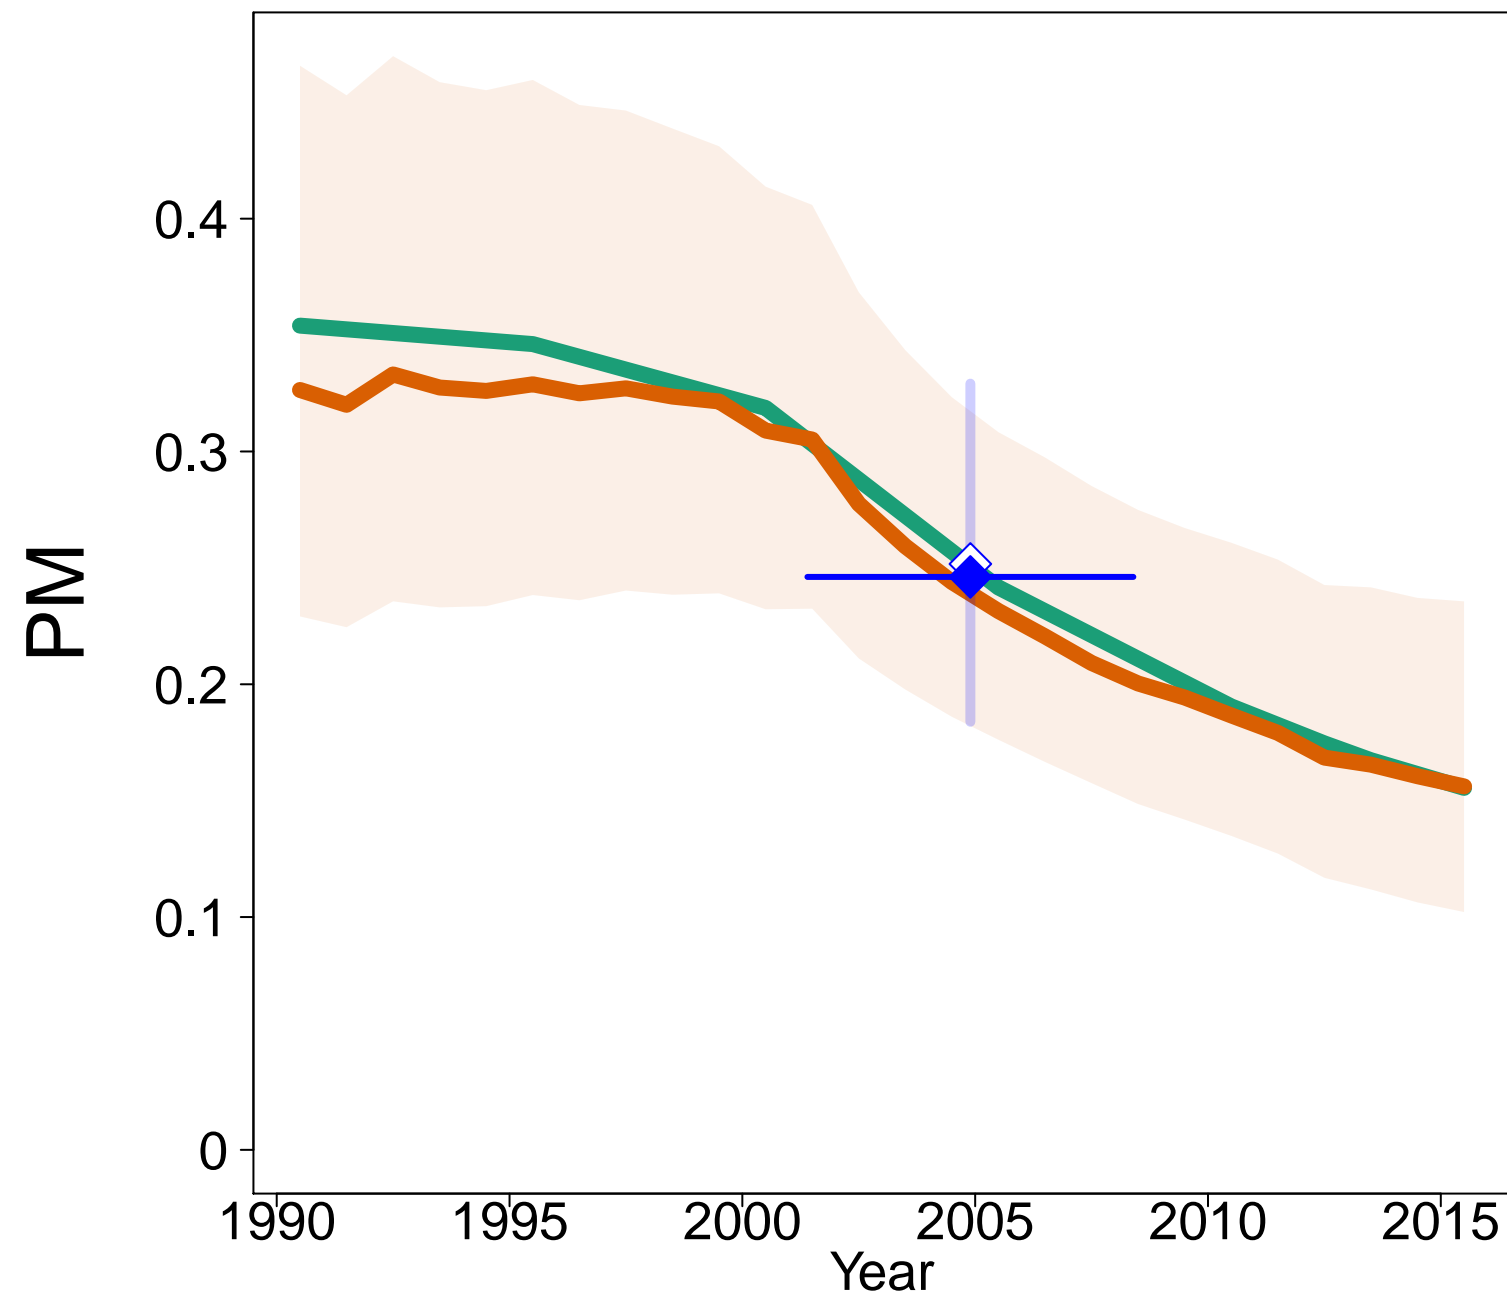

Sierra Leone [SLE; B]  
(Western Africa)

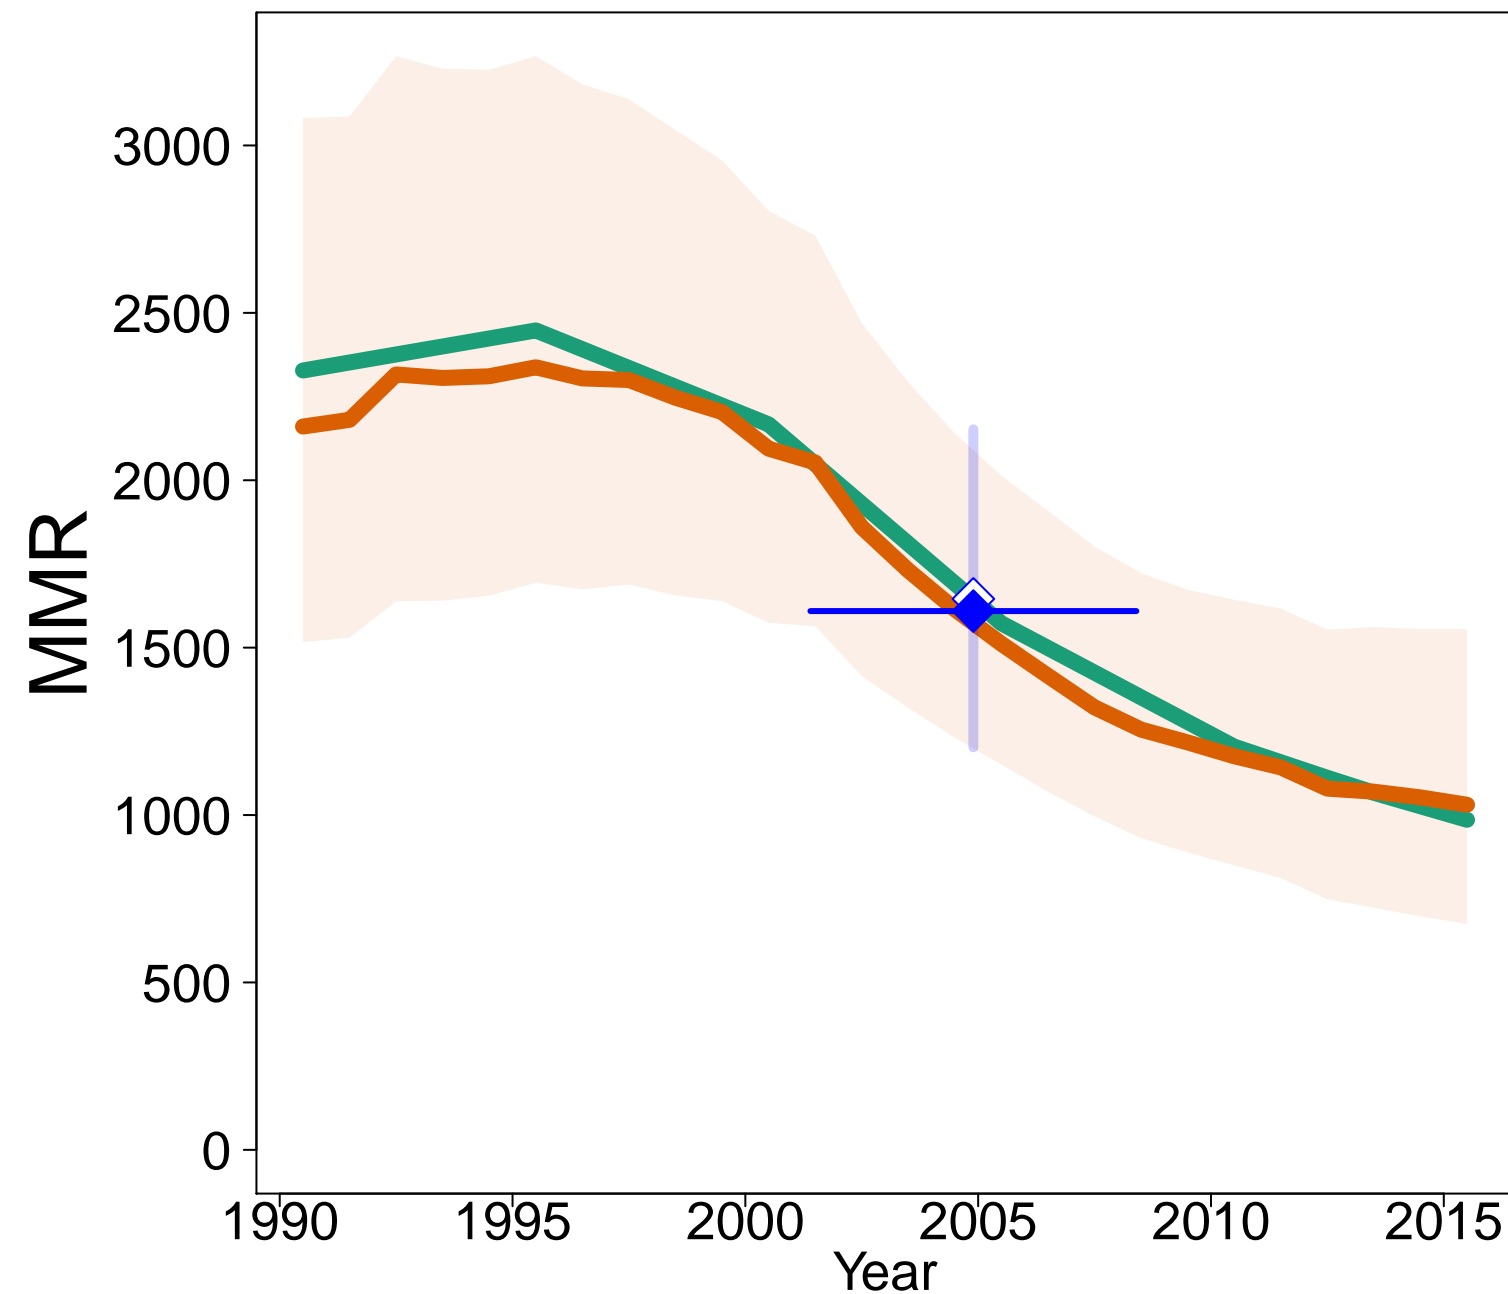

- Estimates –
- Bmat 2014
- MMEIG 2014
- Data –
- Observed Data
- Adjusted Data
- Data type –
- DHS

Singapore [SGP; A]  
(South-Eastern Asia / Oceania)

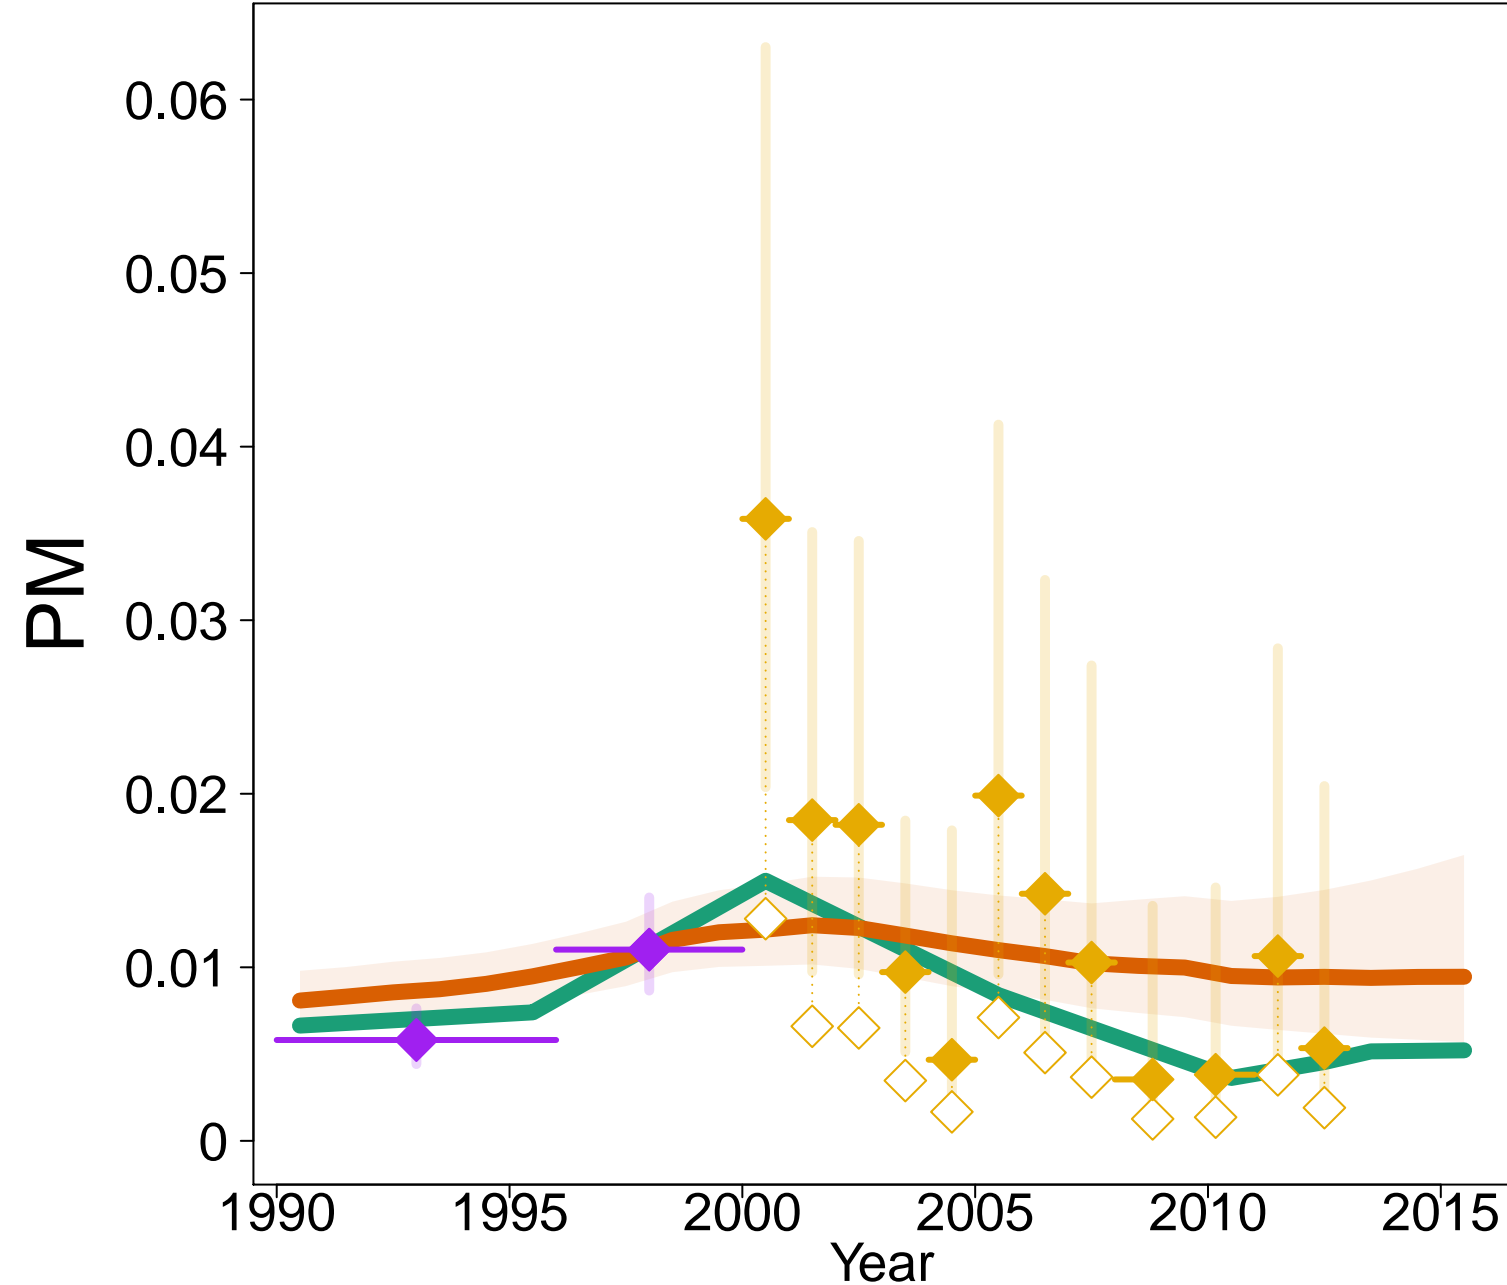

Singapore [SGP; A]  
(South-Eastern Asia / Oceania)

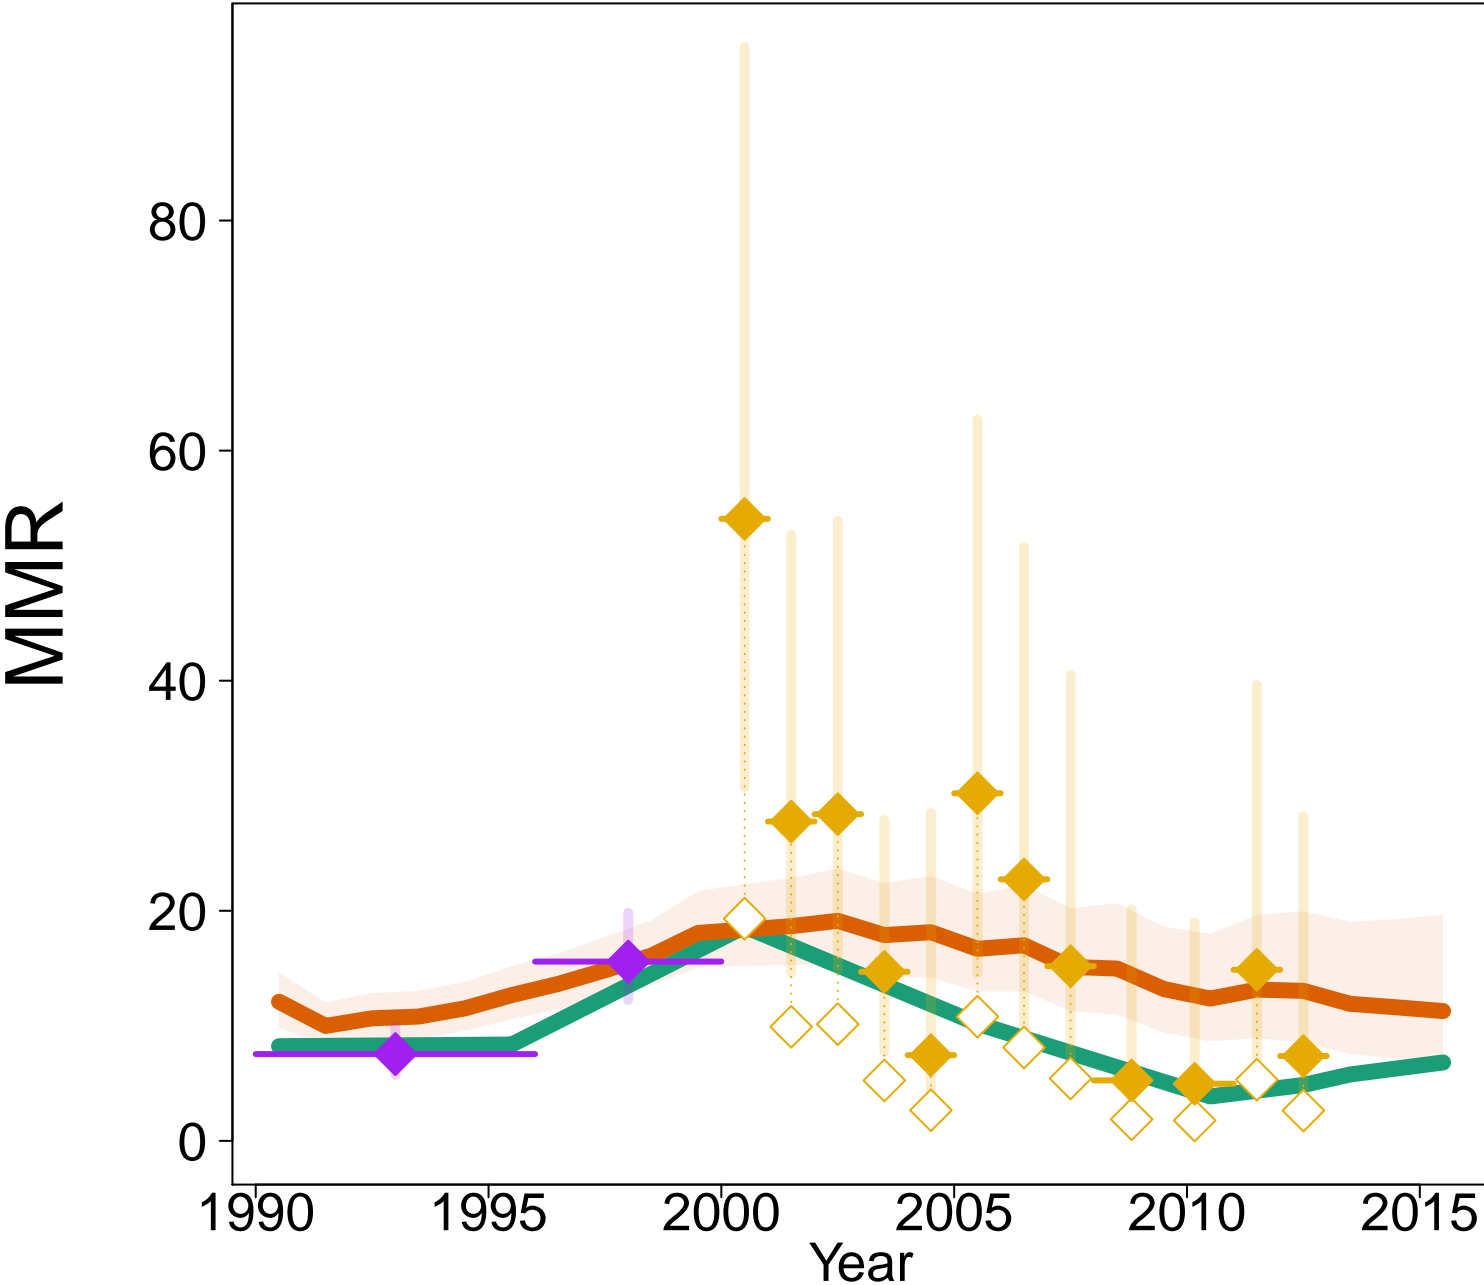

- Estimates –
- Bmat 2014
- MMEIG 2014
- Data –
- ◊ Observed Data
- ◆ Adjusted Data
- Data type –
- ◆ VR
- ◆ Spec. studies



Slovakia [SVK; A]  
(Developed regions)

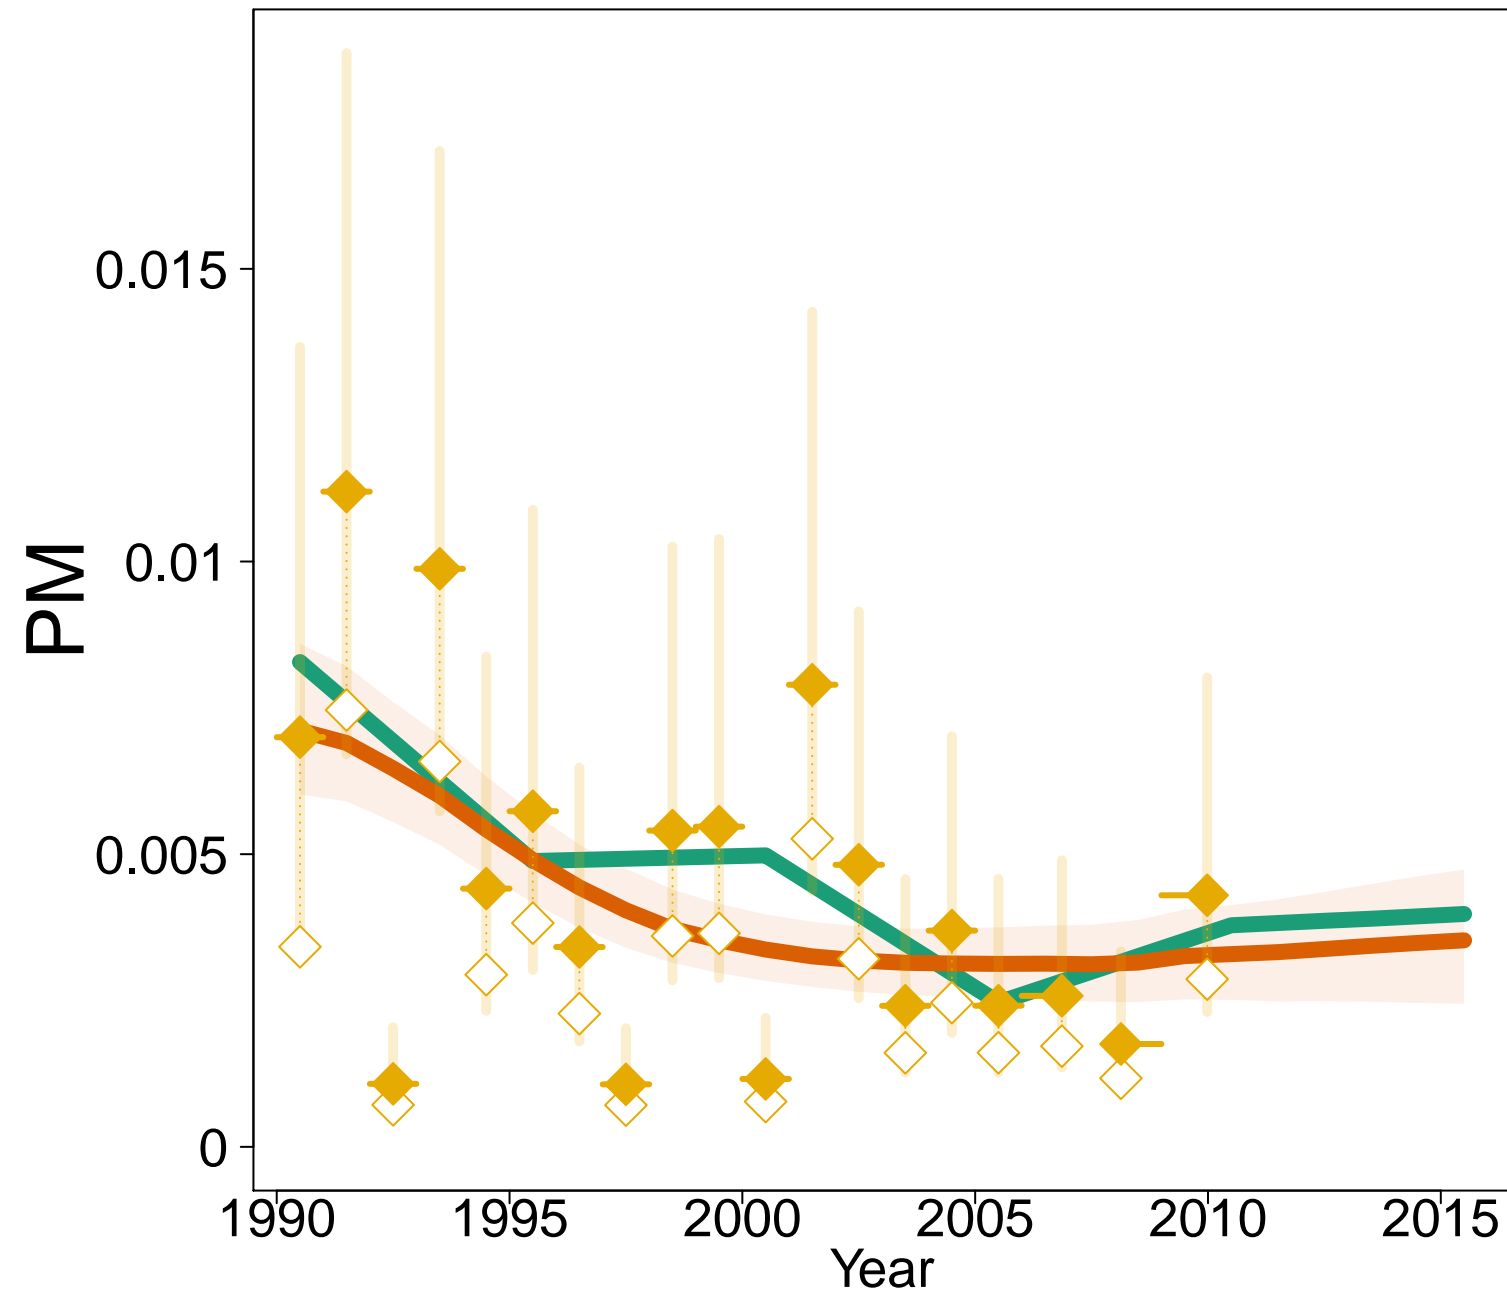

Slovakia [SVK; A]  
(Developed regions)

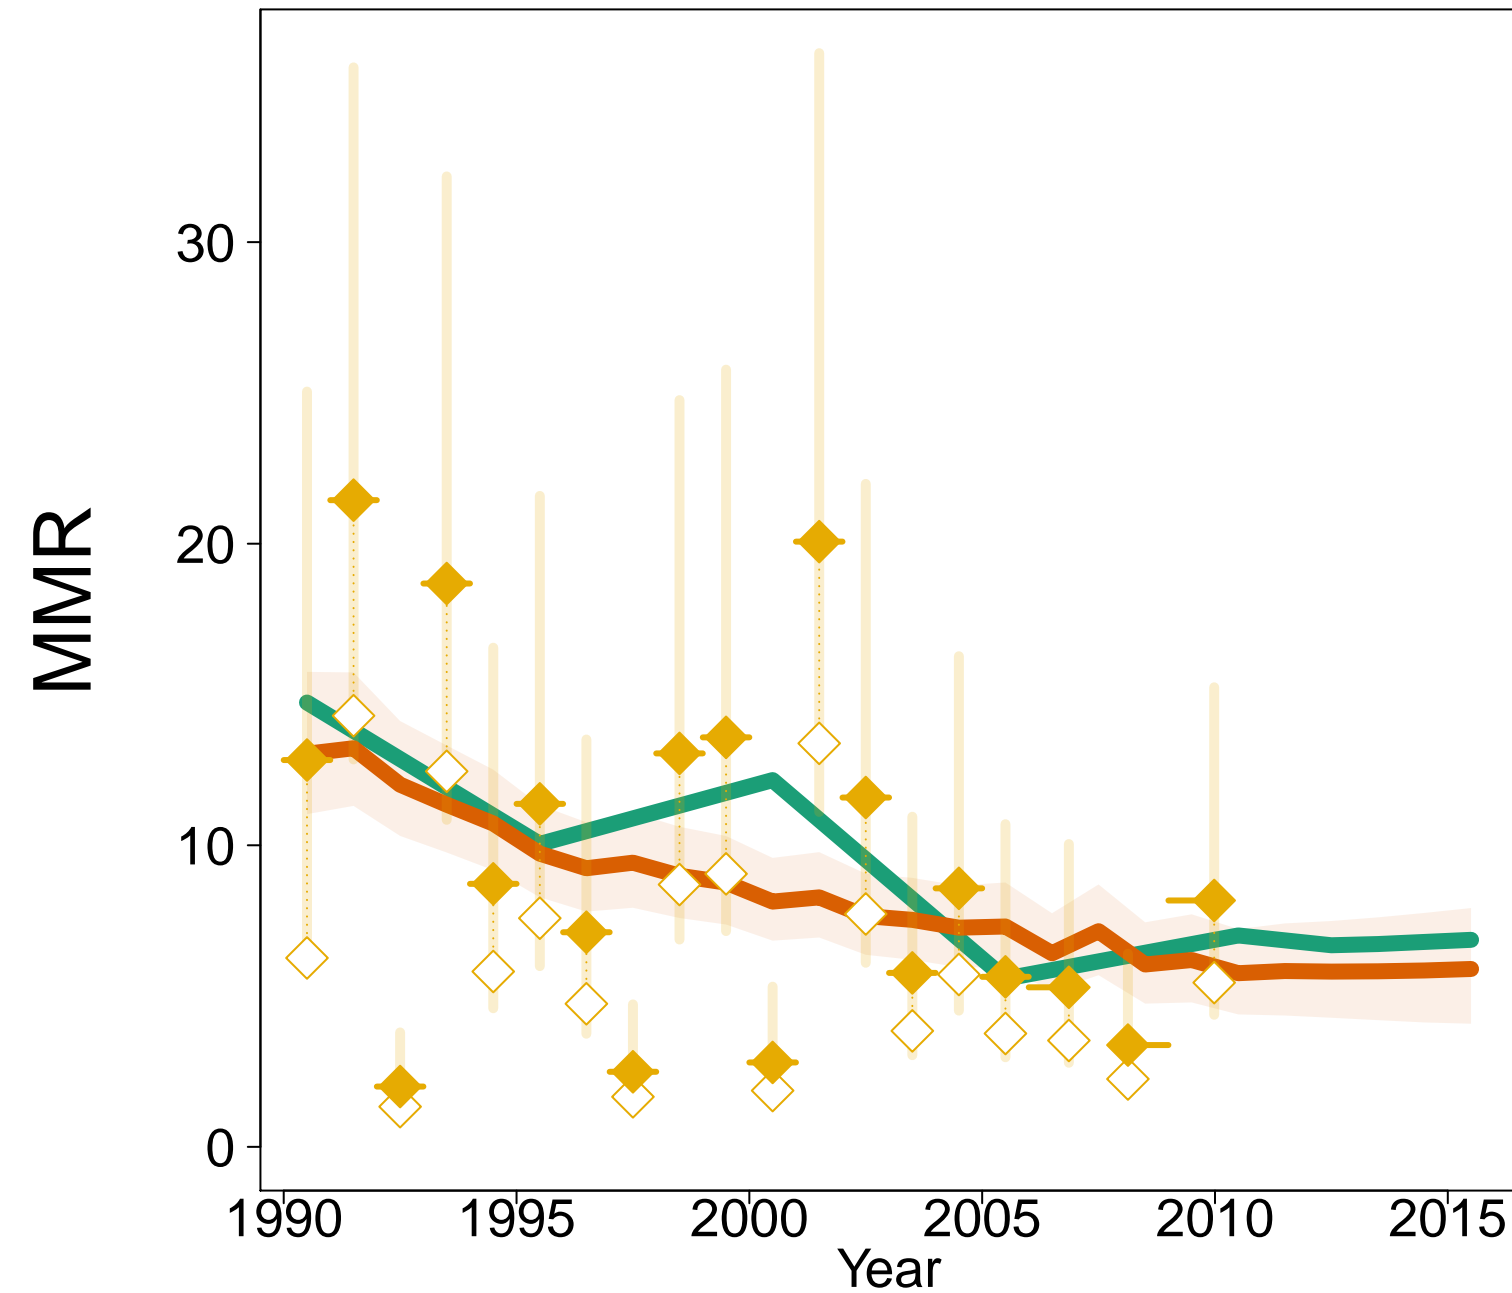

- Estimates –
- Bmat 2014
- MMEIG 2014
- Data –
- Observed Data
- Adjusted Data
- Data type –
- VR

Slovenia [SVN; A]  
(Developed regions)

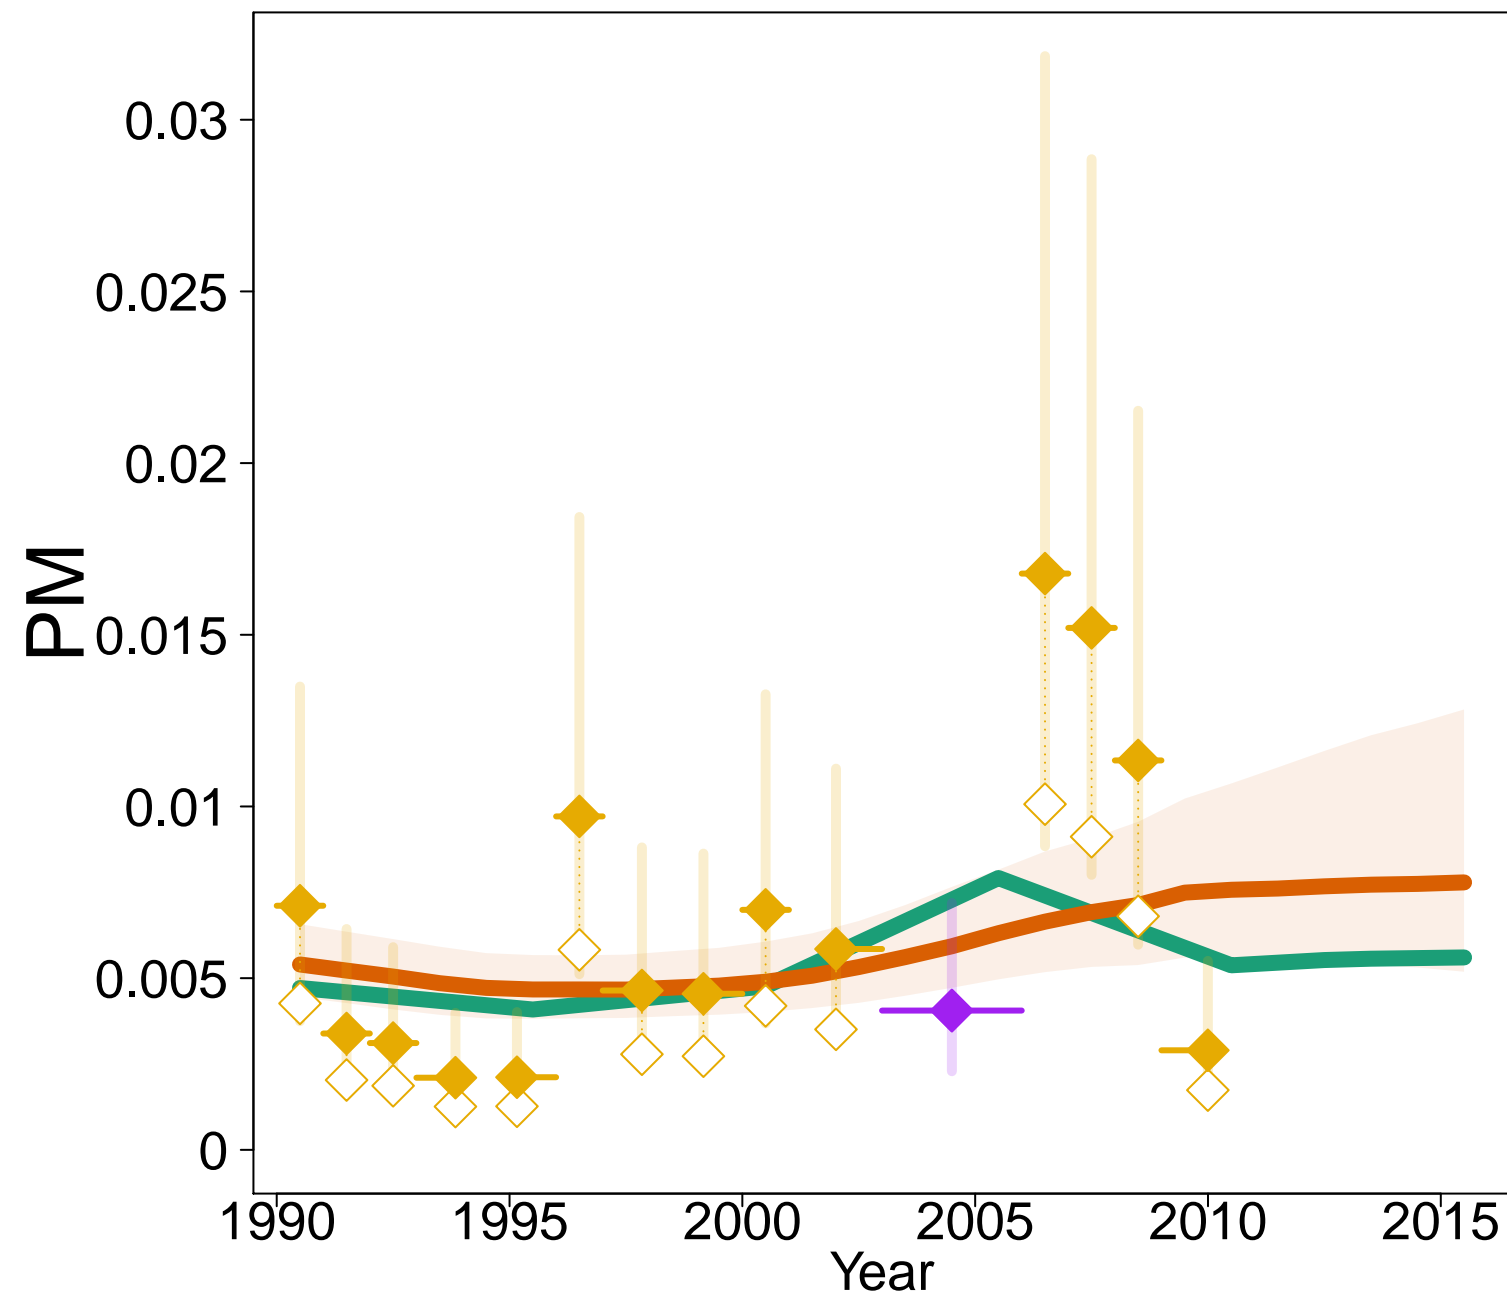

Slovenia [SVN; A]  
(Developed regions)

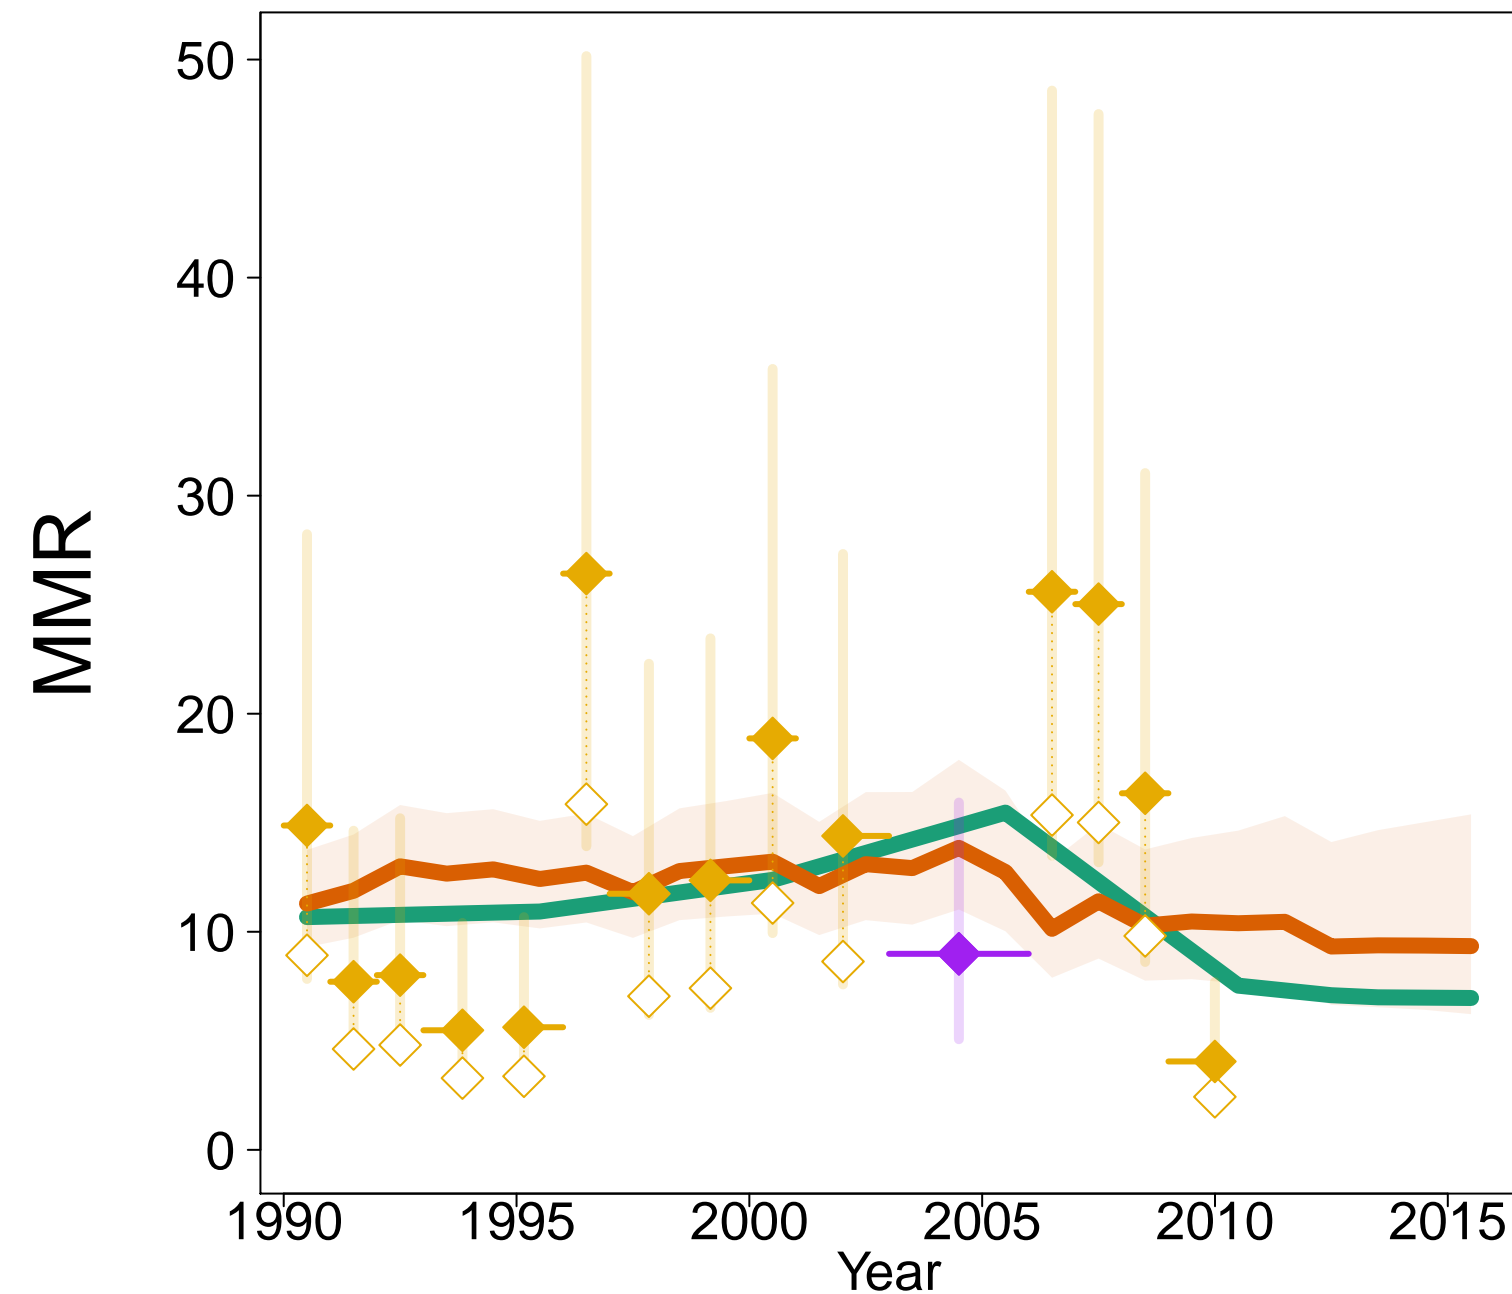

- Estimates –
- Bmat 2014
- MMEIG 2014
- Data –
- Observed Data
- Adjusted Data
- Data type –
- VR
- Spec. studies

Solomon Islands [SLB; C]  
(South-Eastern Asia / Oceania)

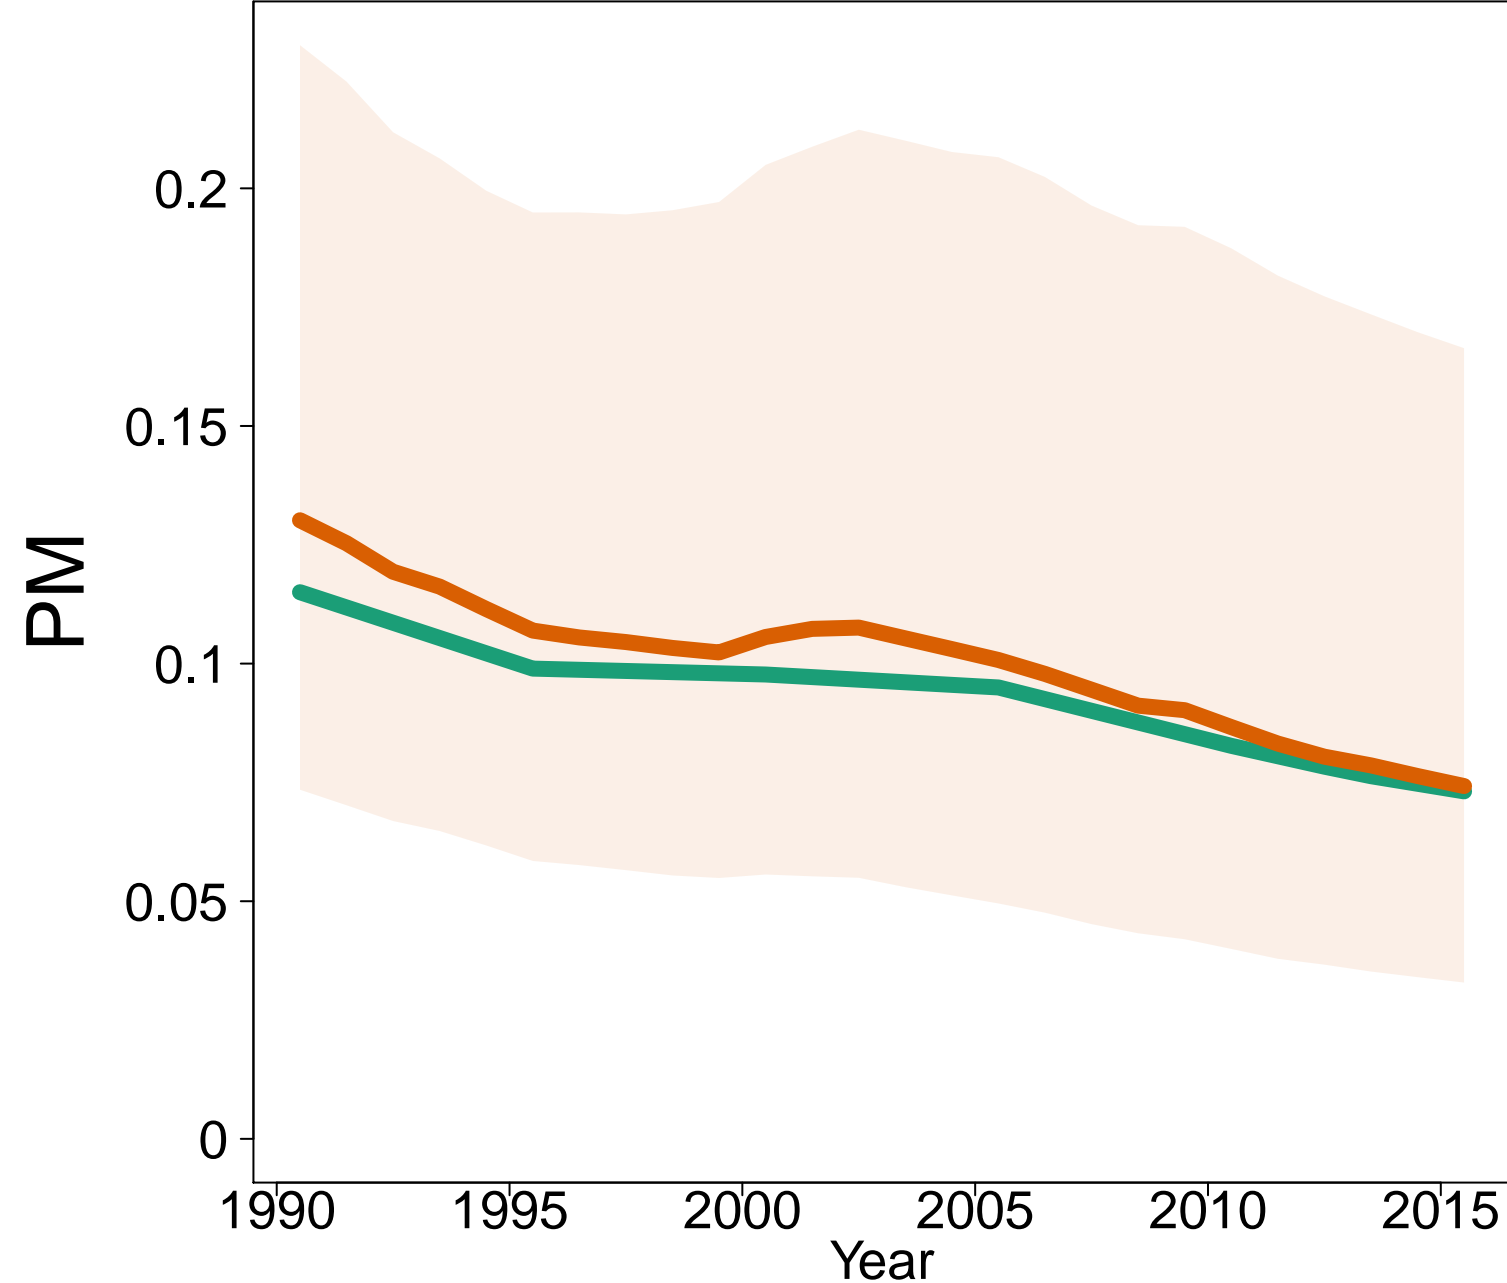

Solomon Islands [SLB; C]  
(South-Eastern Asia / Oceania)

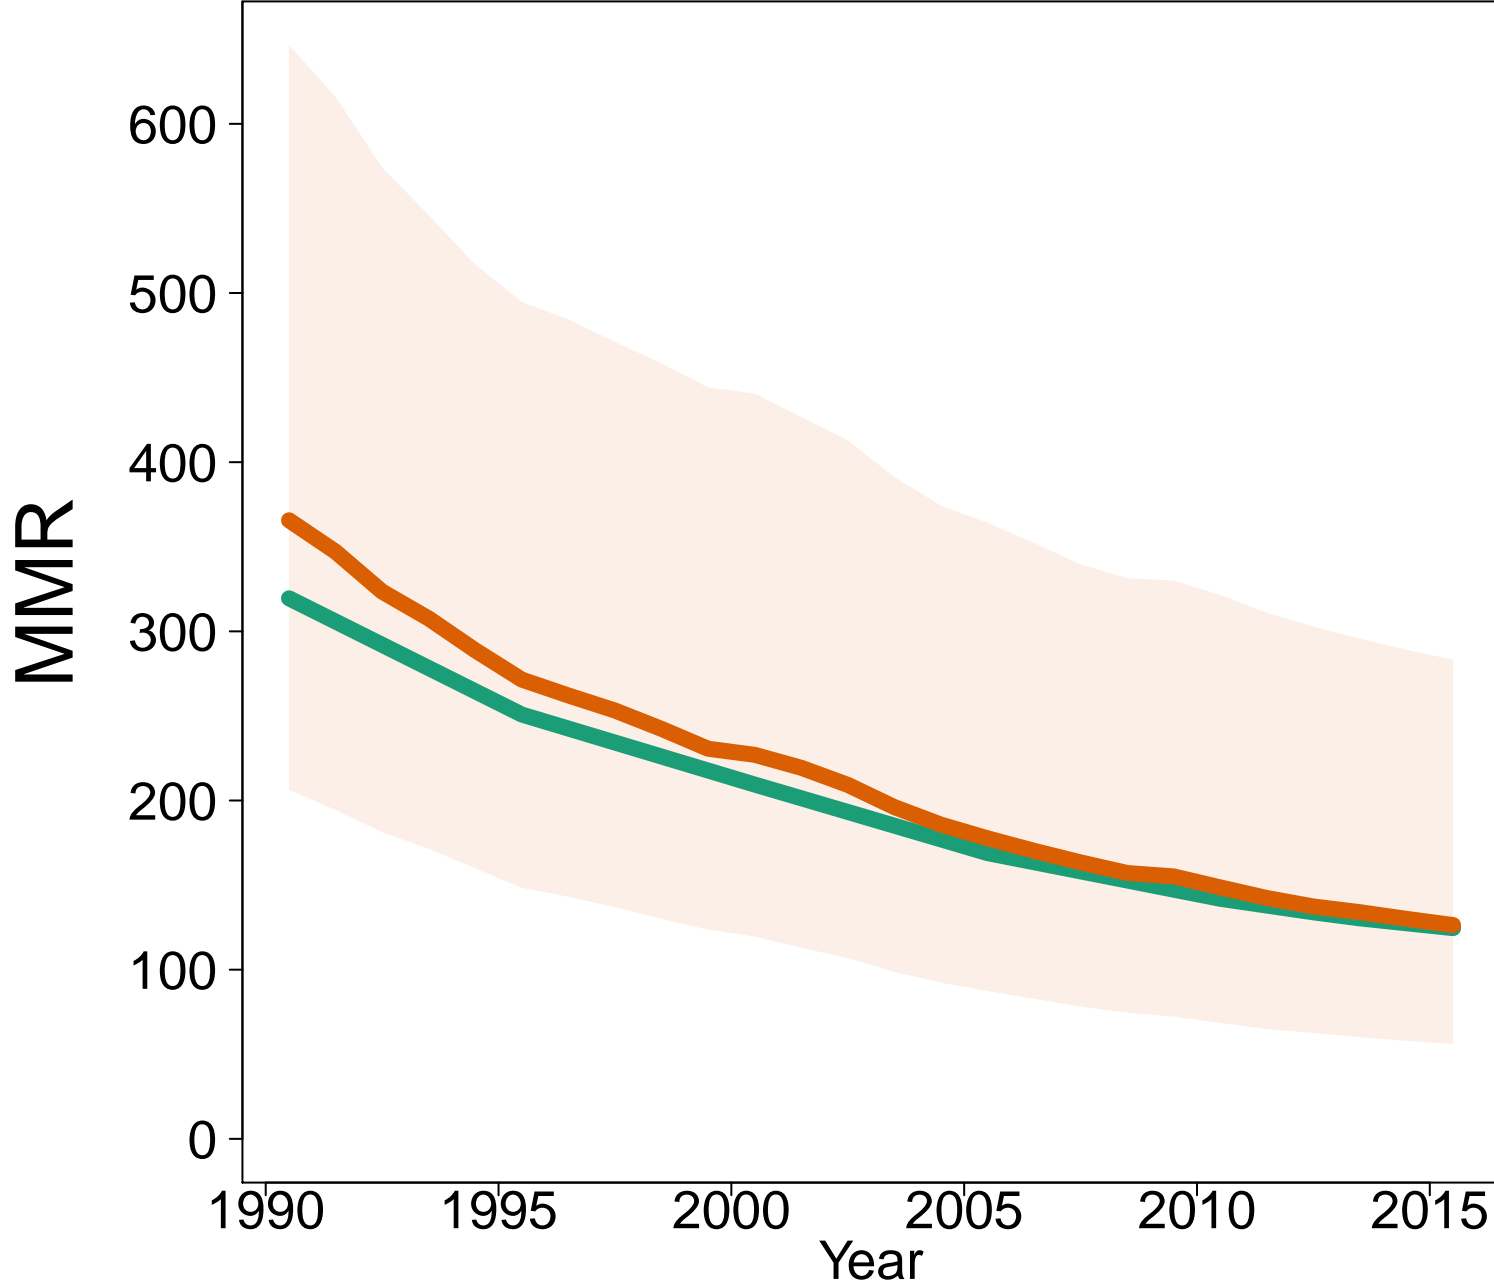

– Estimates –  
Bmat 2014  
MMEIG 2014  
– Data –

Somalia [SOM; C]  
(Eastern Africa)

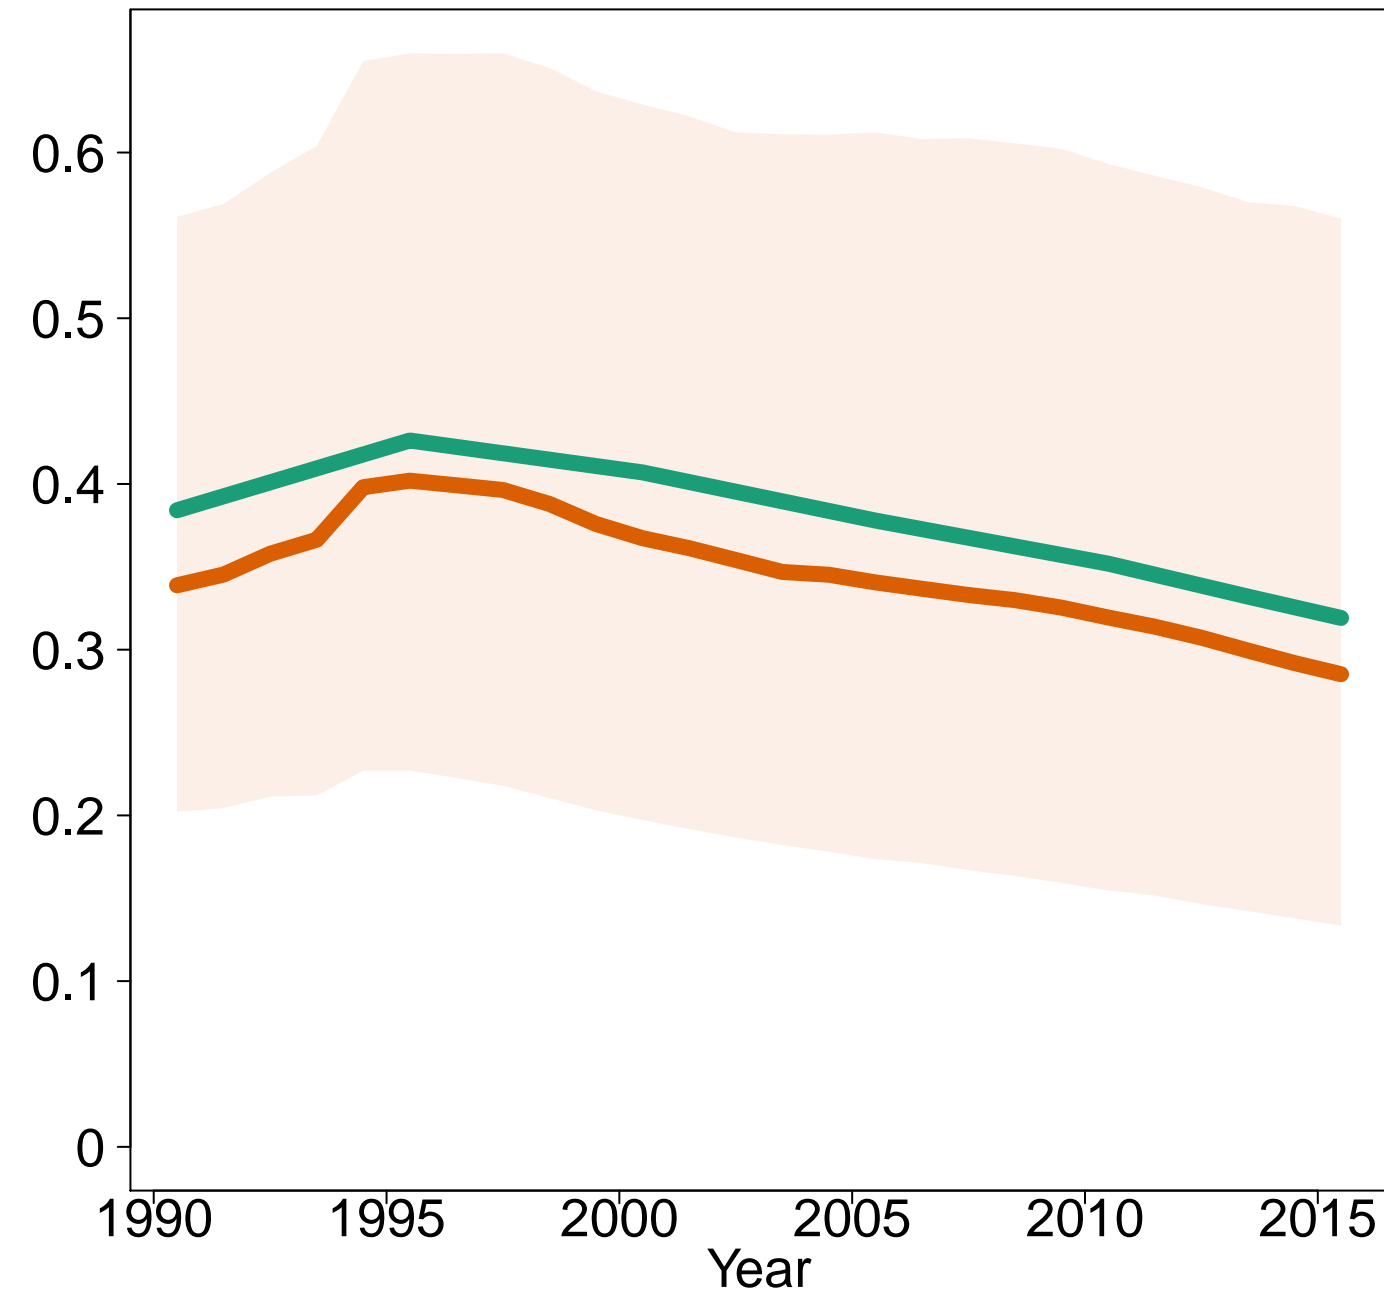

Somalia [SOM; C]  
(Eastern Africa)

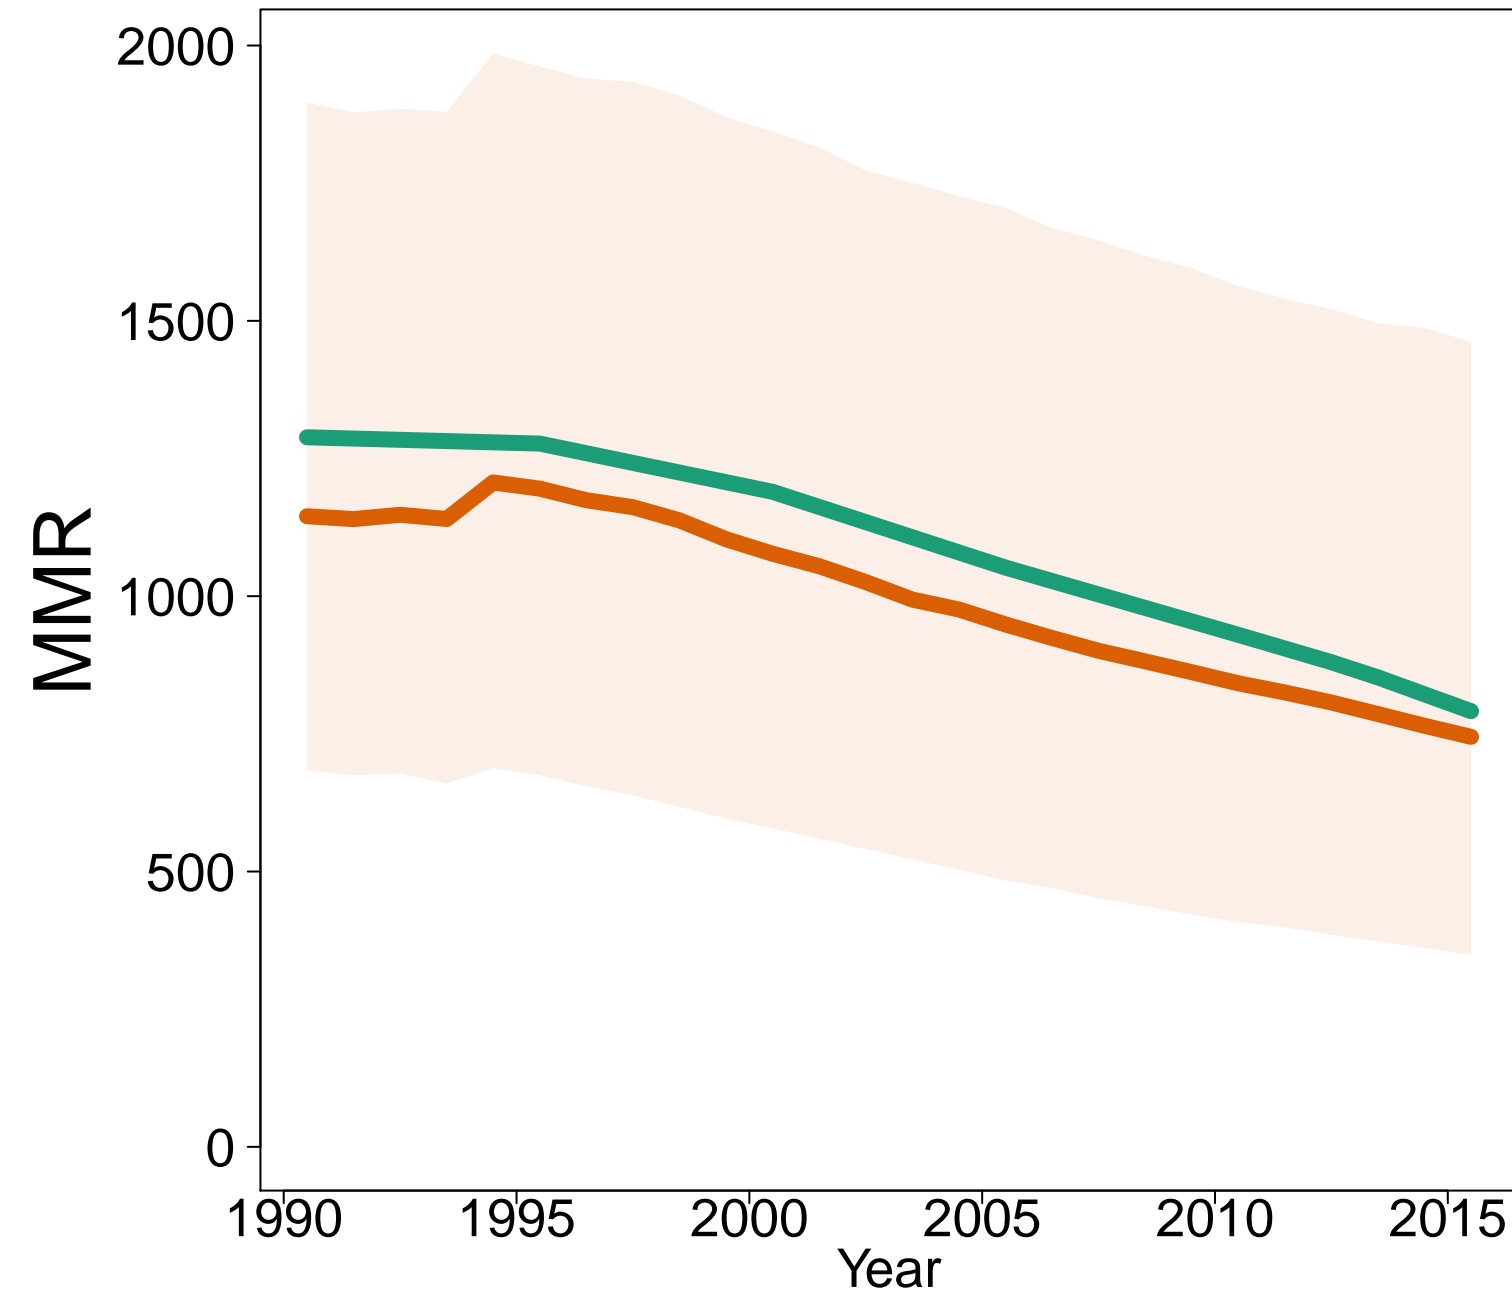

– Estimates –  
Bmat 2014  
MMEIG 2014  
– Data –

South Africa [ZAF; B]  
(Southern Africa)

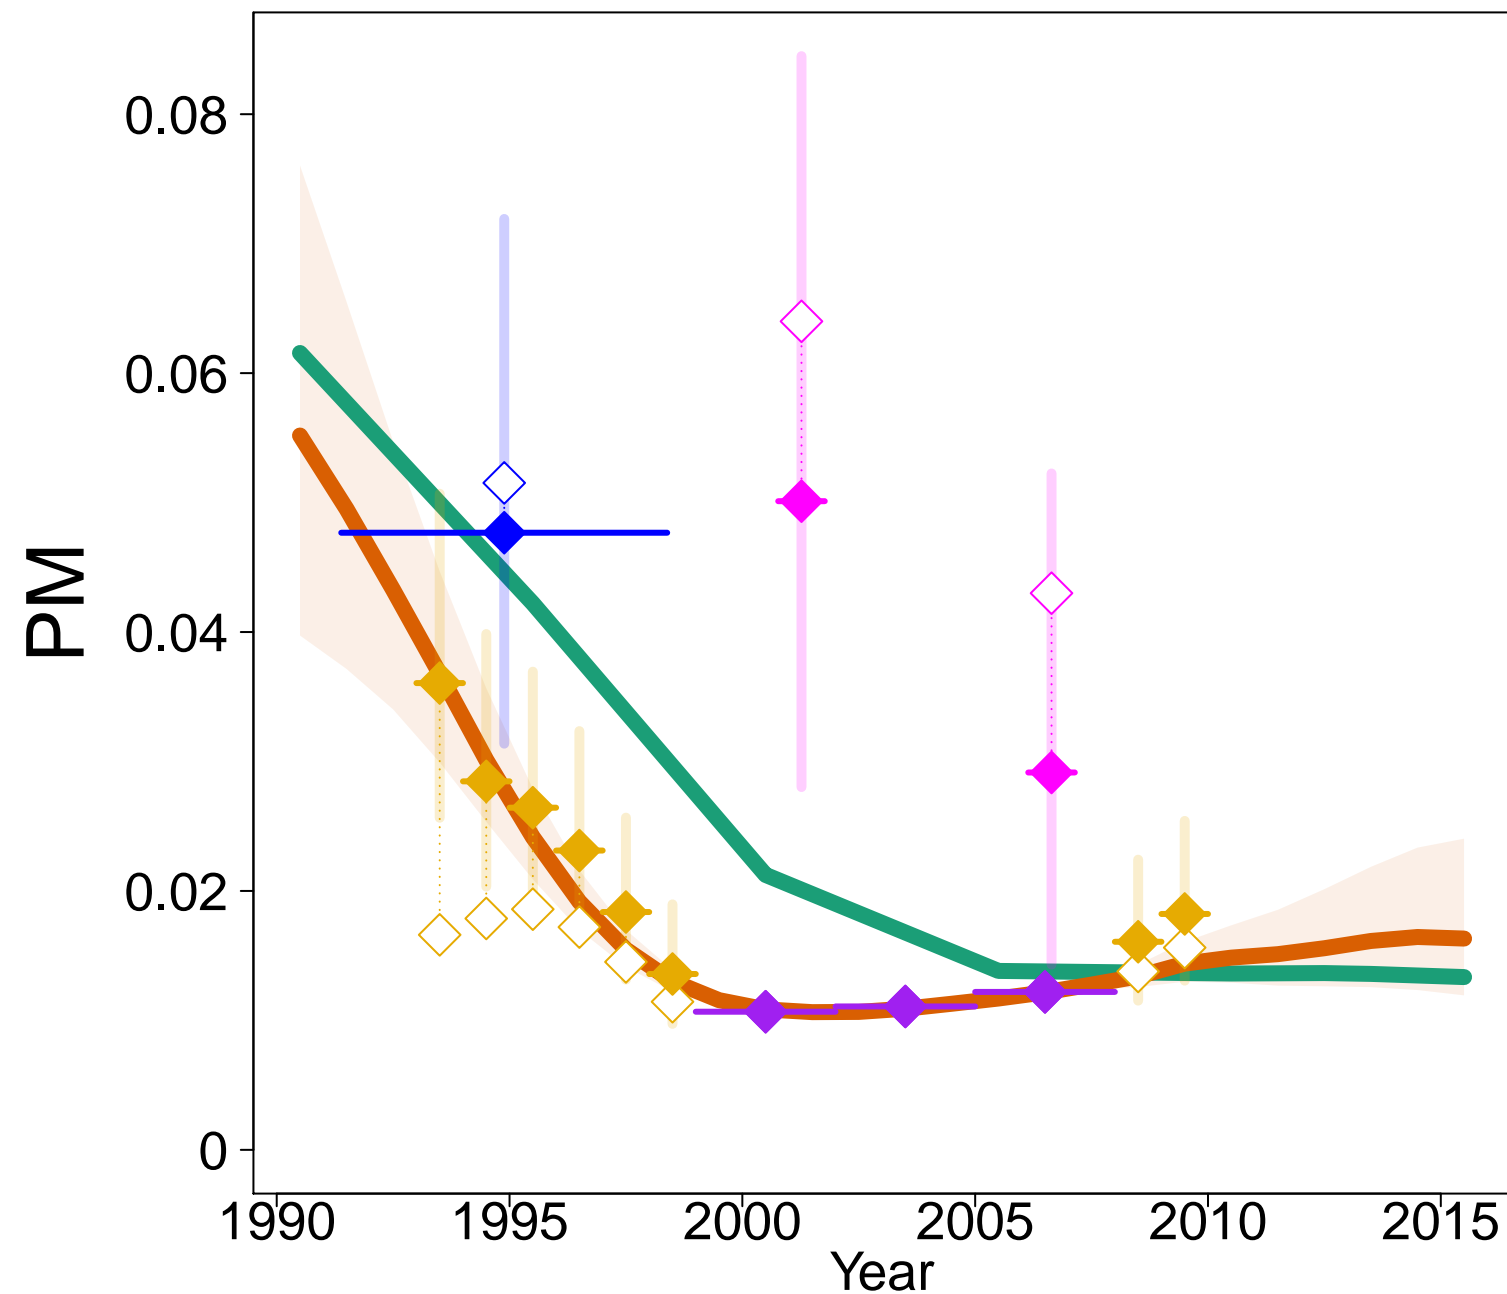

South Africa [ZAF; B]  
(Southern Africa)

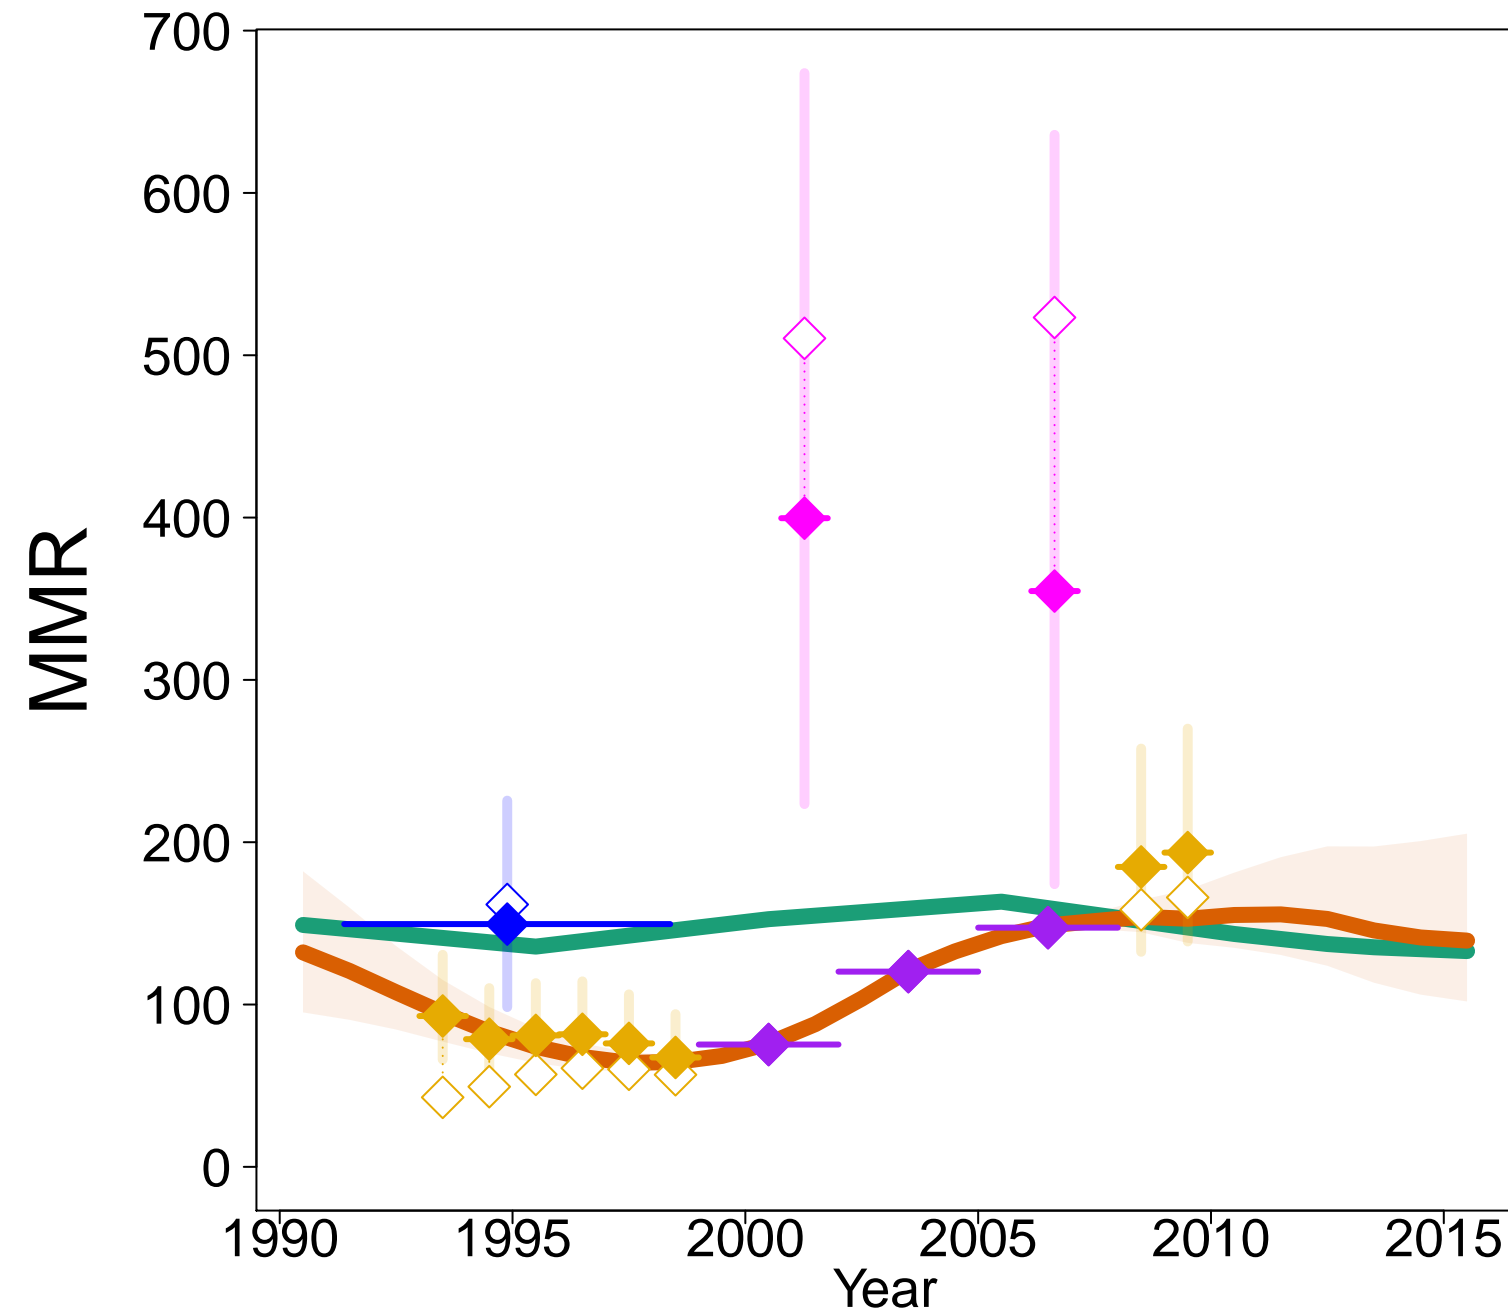

- Estimates –
- Bmat 2014
- MMEIG 2014
- Data –
- Observed Data
- Adjusted Data
- Data type –
- VR
- Spec. studies
- DHS
- Census

South Sudan [SSD; B]  
(Eastern Africa)

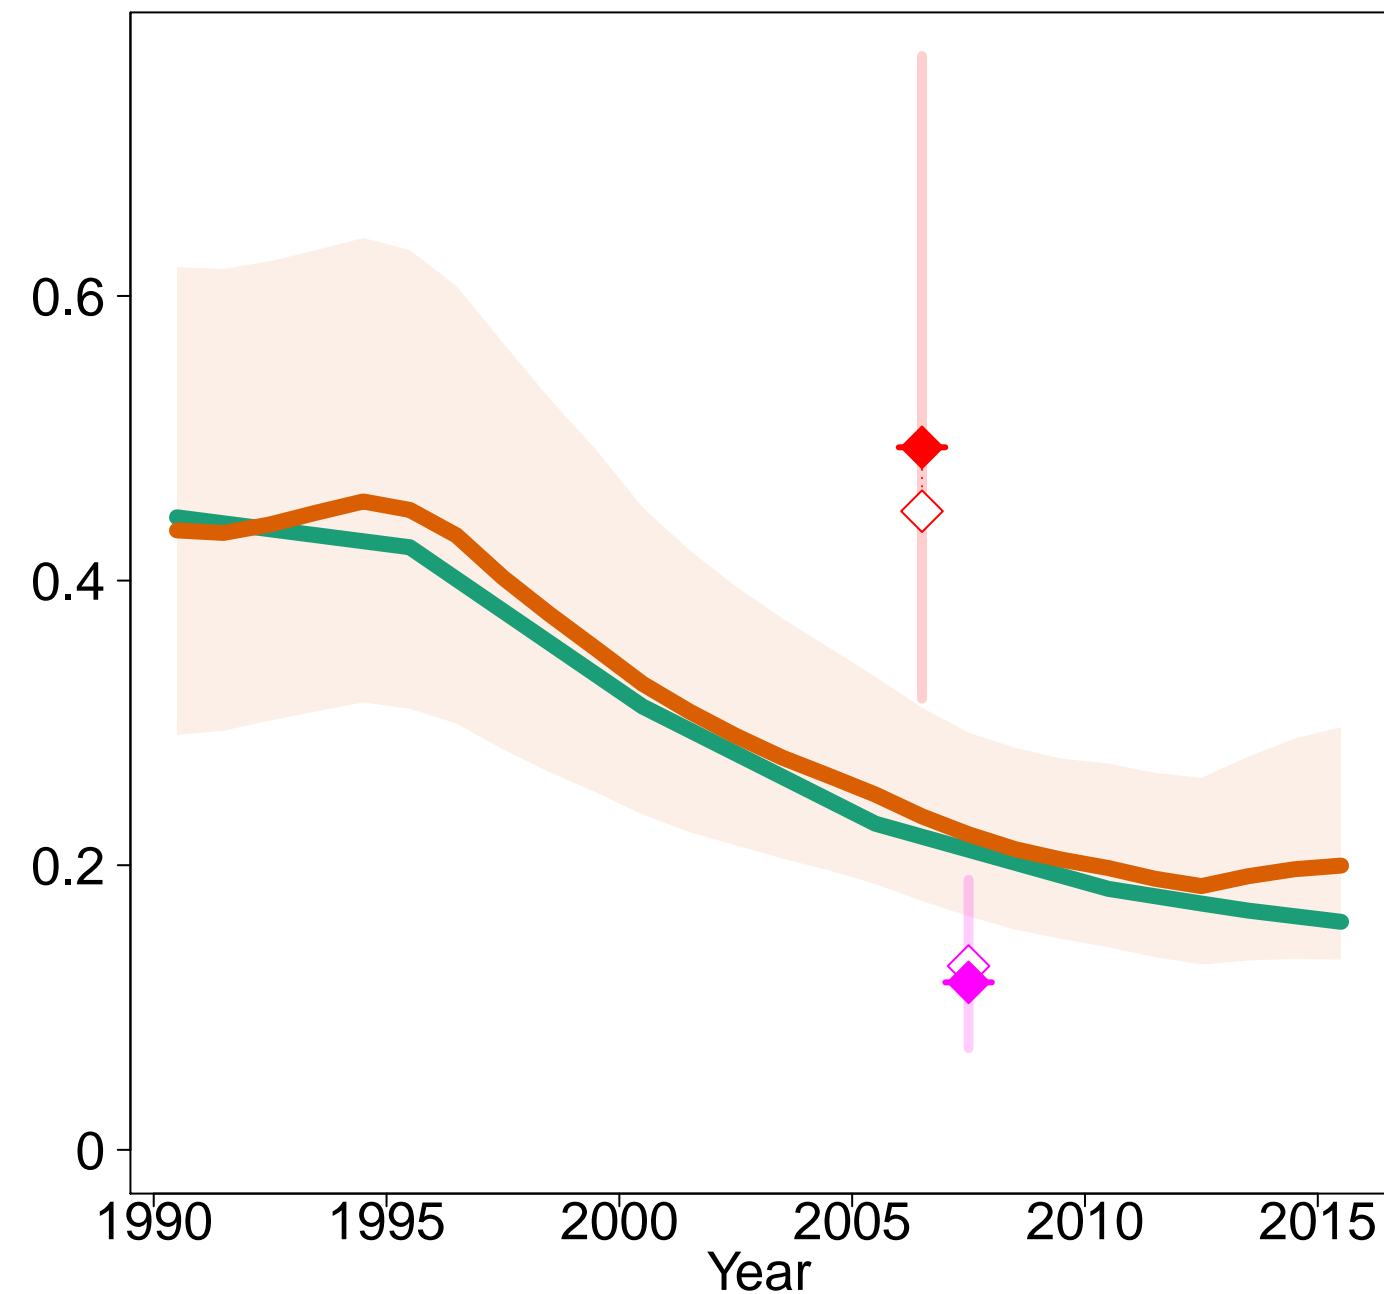

South Sudan [SSD; B]  
(Eastern Africa)

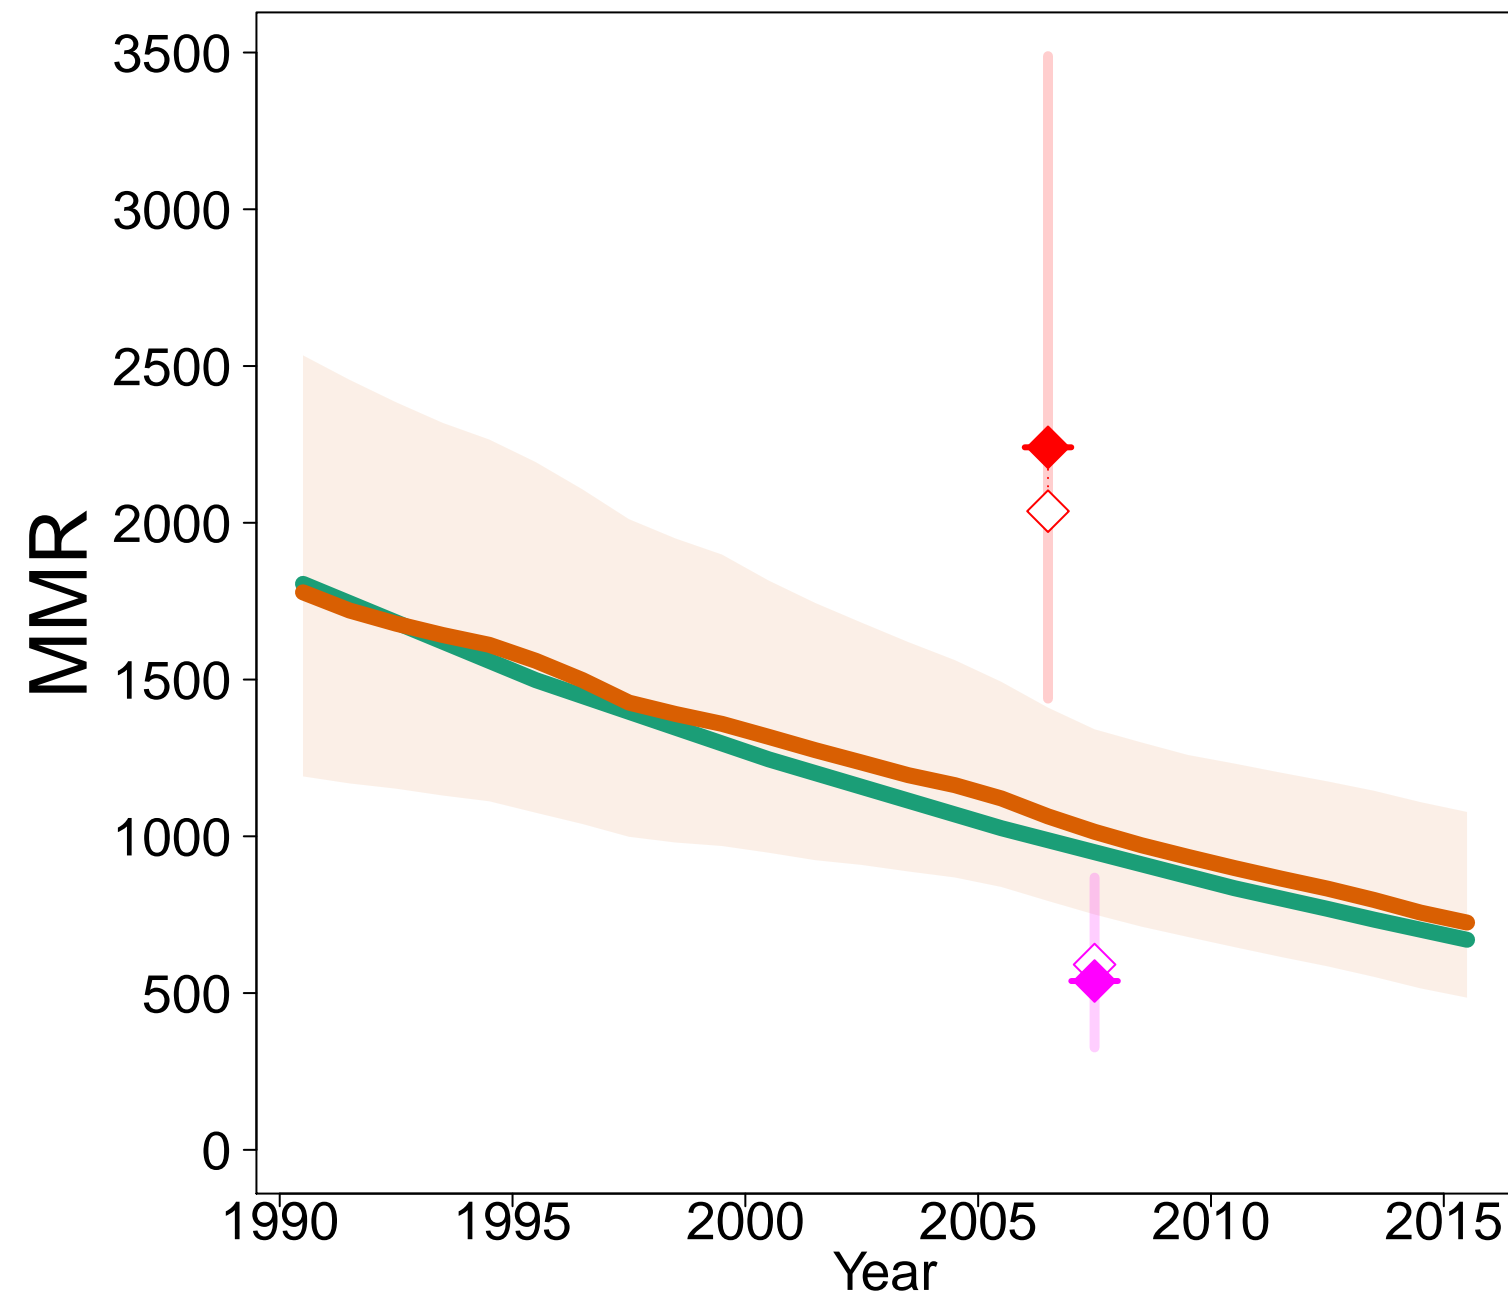

- Estimates –
- Bmat 2014
- MMEIG 2014
- Data –
- Observed Data
- Adjusted Data
- Data type –
- Census
- Misc. studies

Spain [ESP; A]  
(Developed regions)

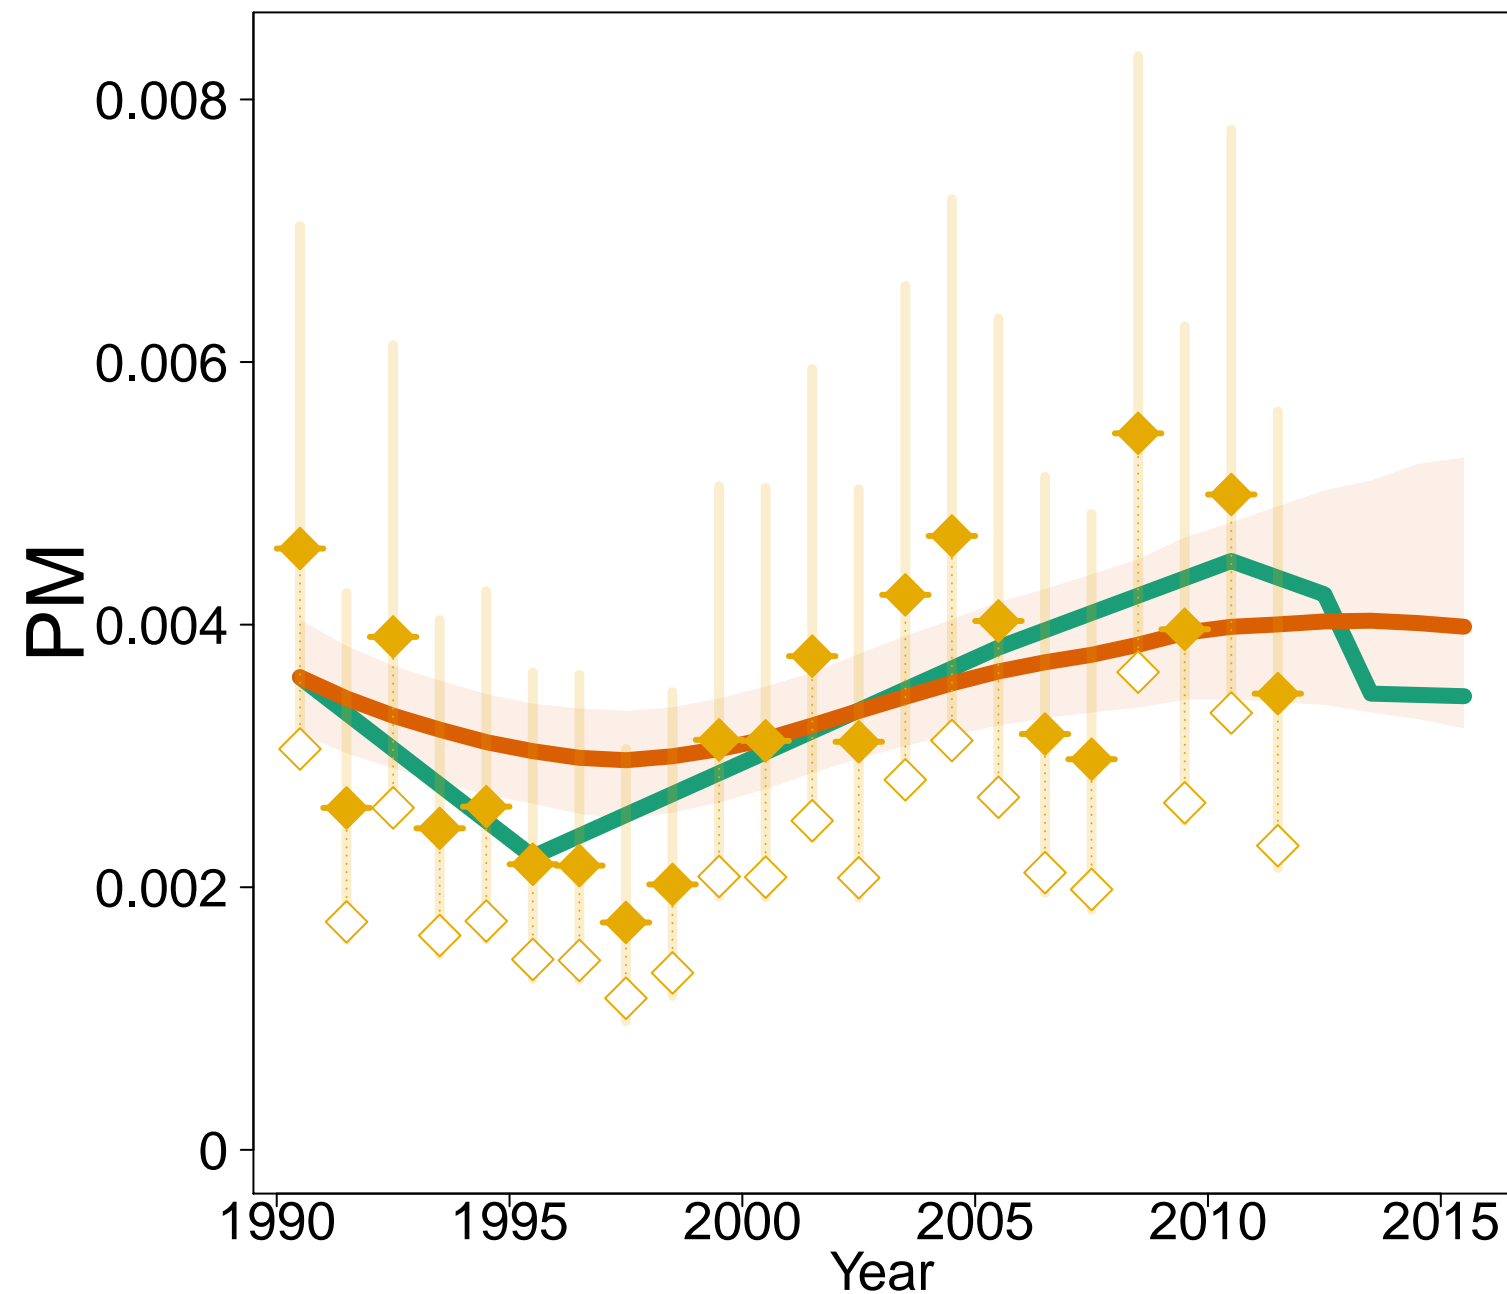

Spain [ESP; A]  
(Developed regions)

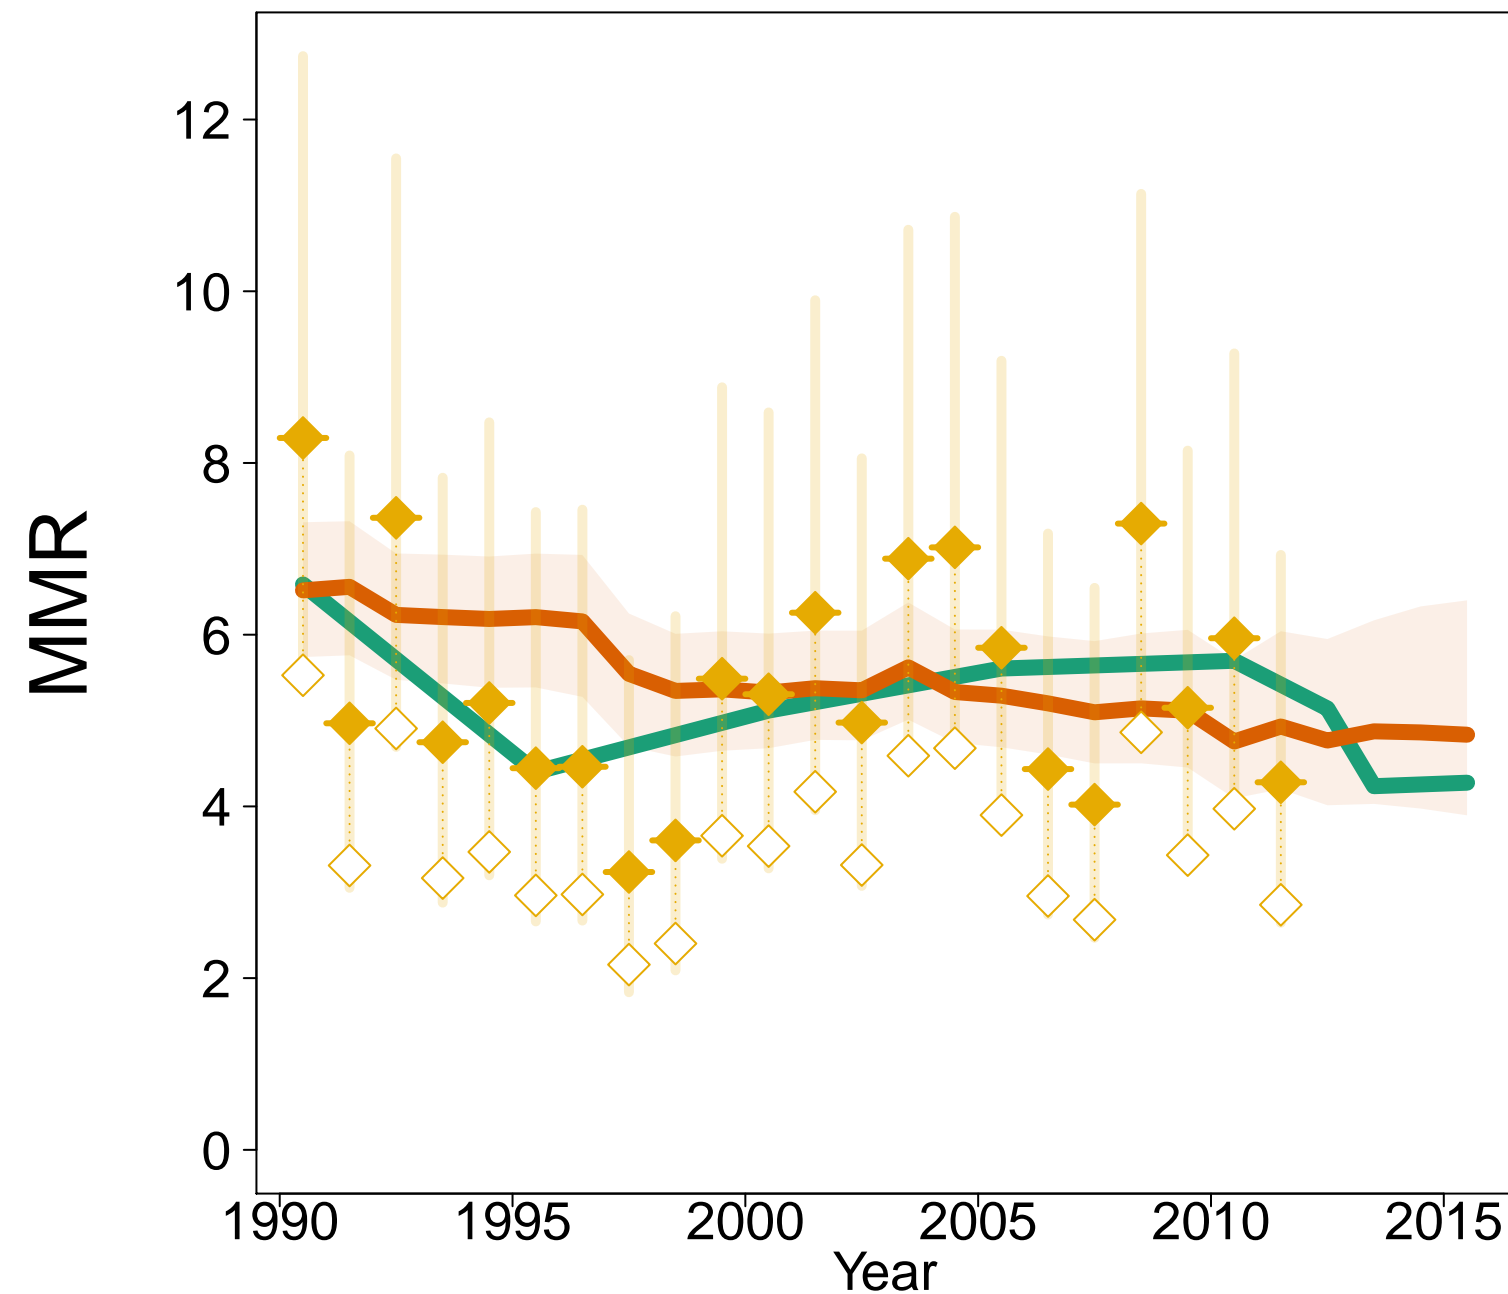

- Estimates –
- Bmat 2014
- MMEIG 2014
- Data –
- Observed Data
- Adjusted Data
- Data type –
- VR

Sri Lanka [LKA; B]  
(Southern Asia)

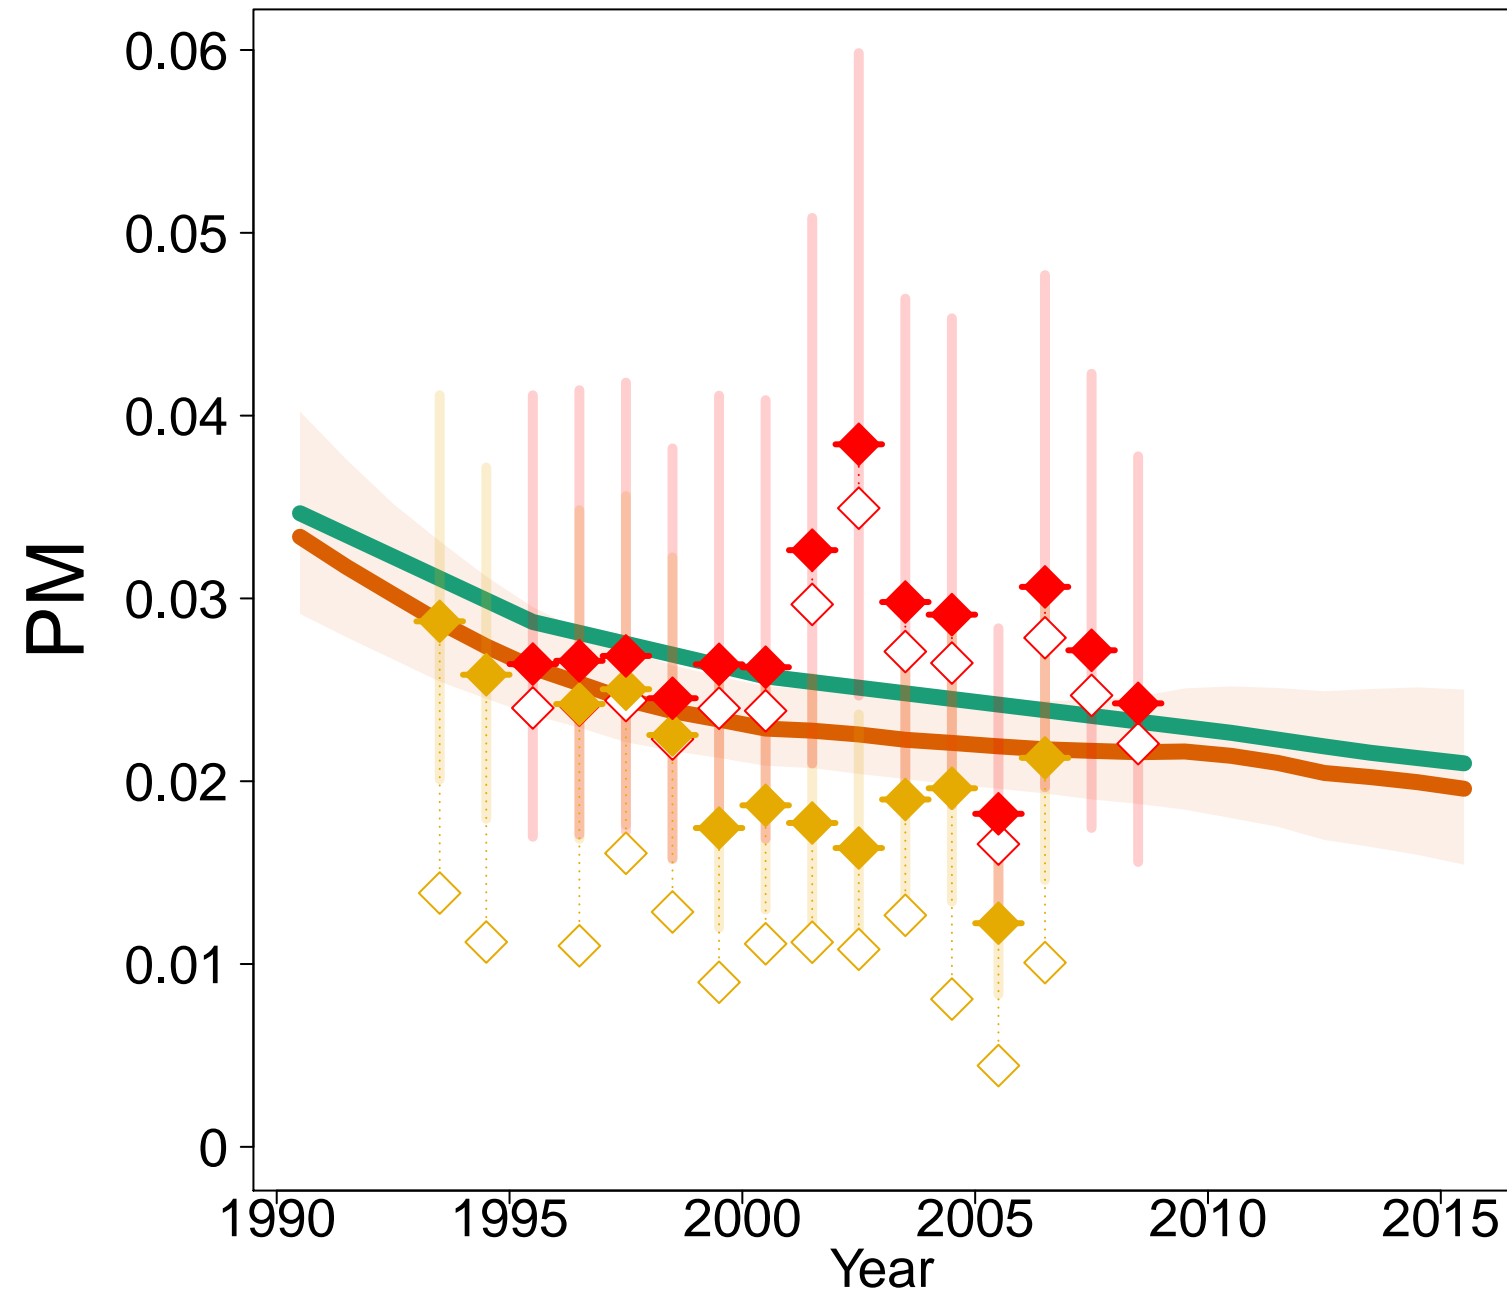

Sri Lanka [LKA; B]  
(Southern Asia)

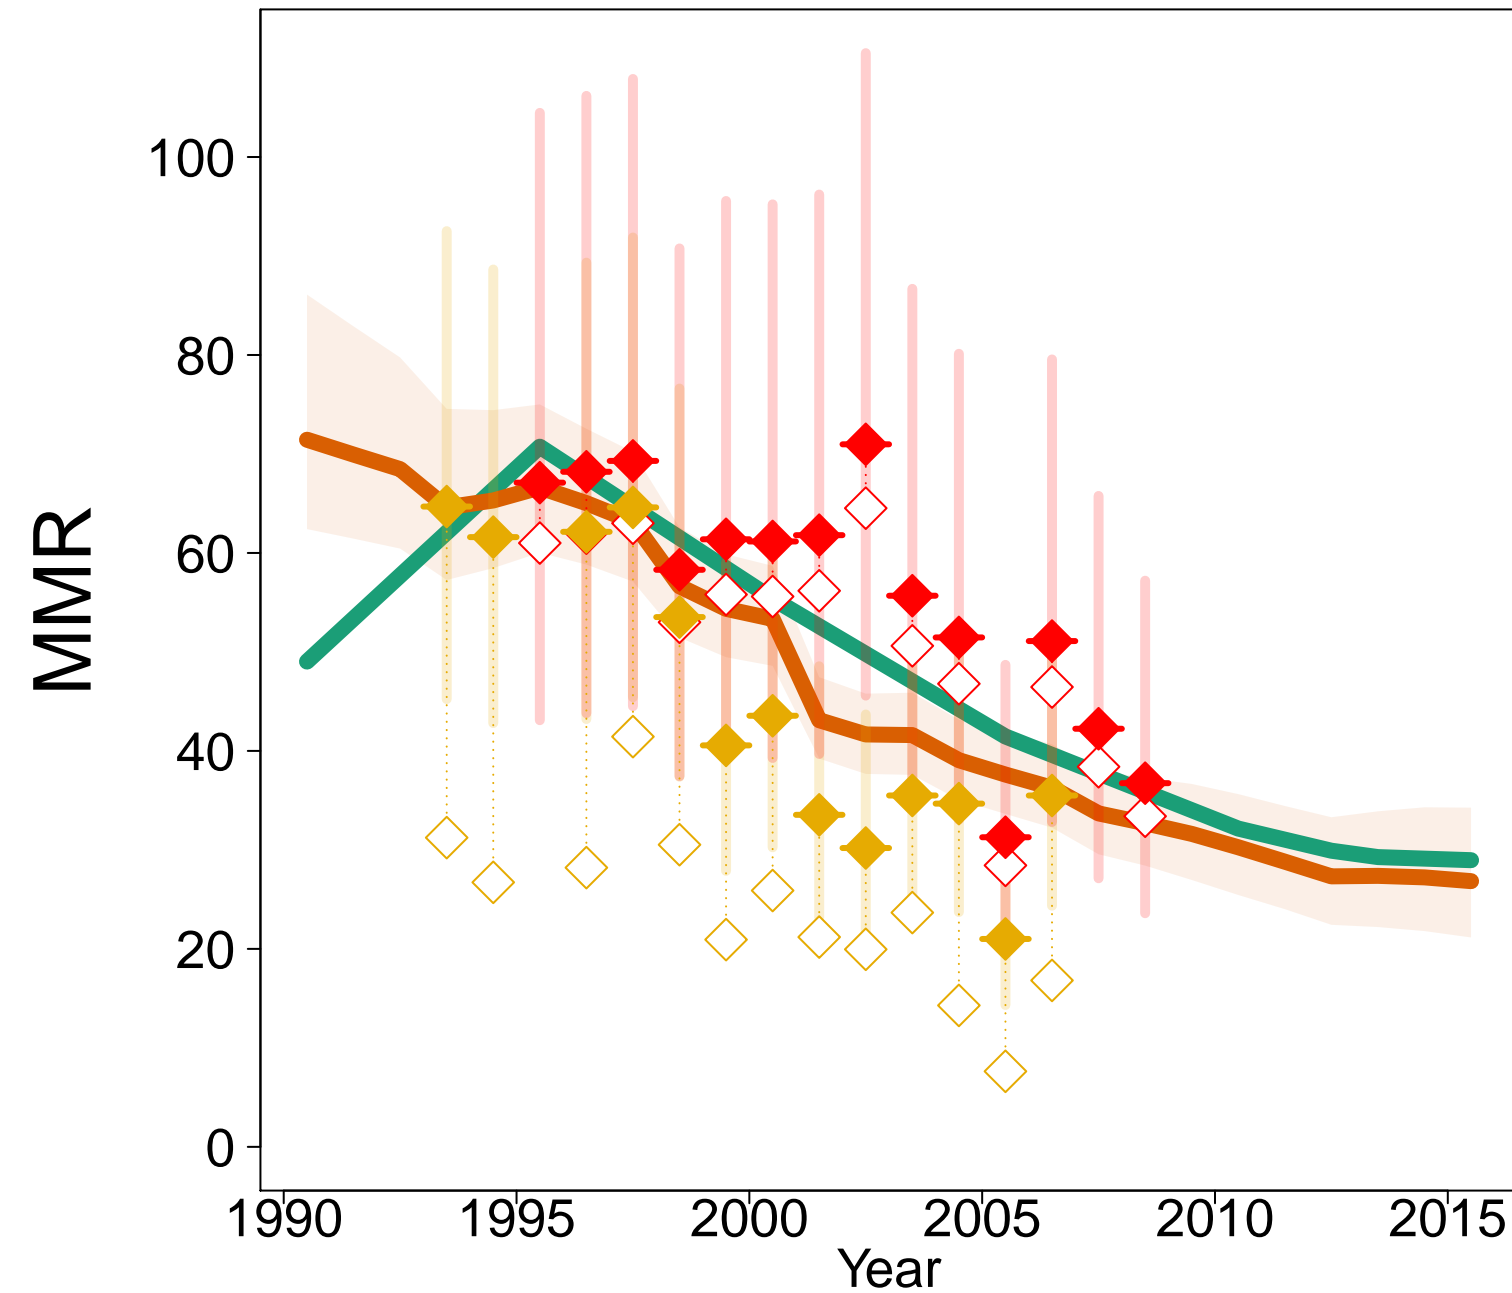

- Estimates –
- Bmat 2014
- MMEIG 2014
- Data –
- Observed Data
- Adjusted Data
- Data type –
- VR
- Misc. studies



St Vincent and the Grenadines [VCT; A]  
(Caribbean)

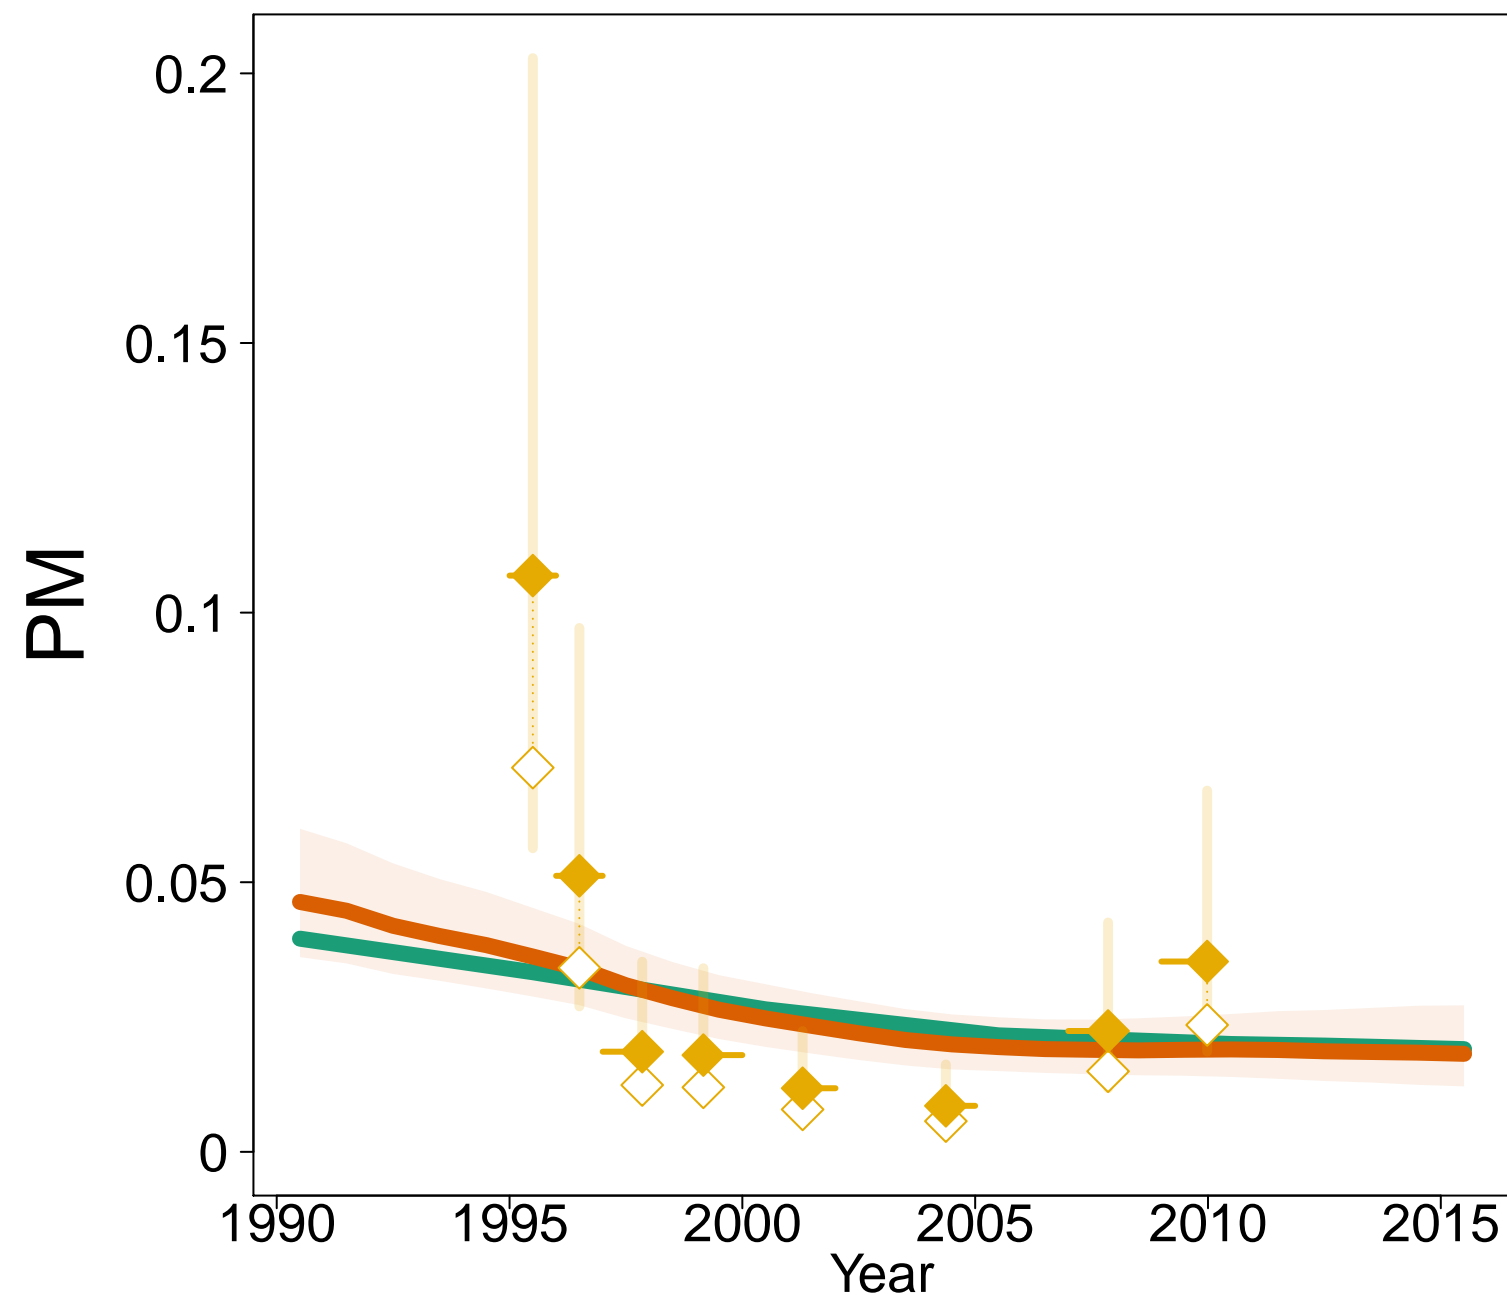

St Vincent and the Grenadines [VCT; A]  
(Caribbean)

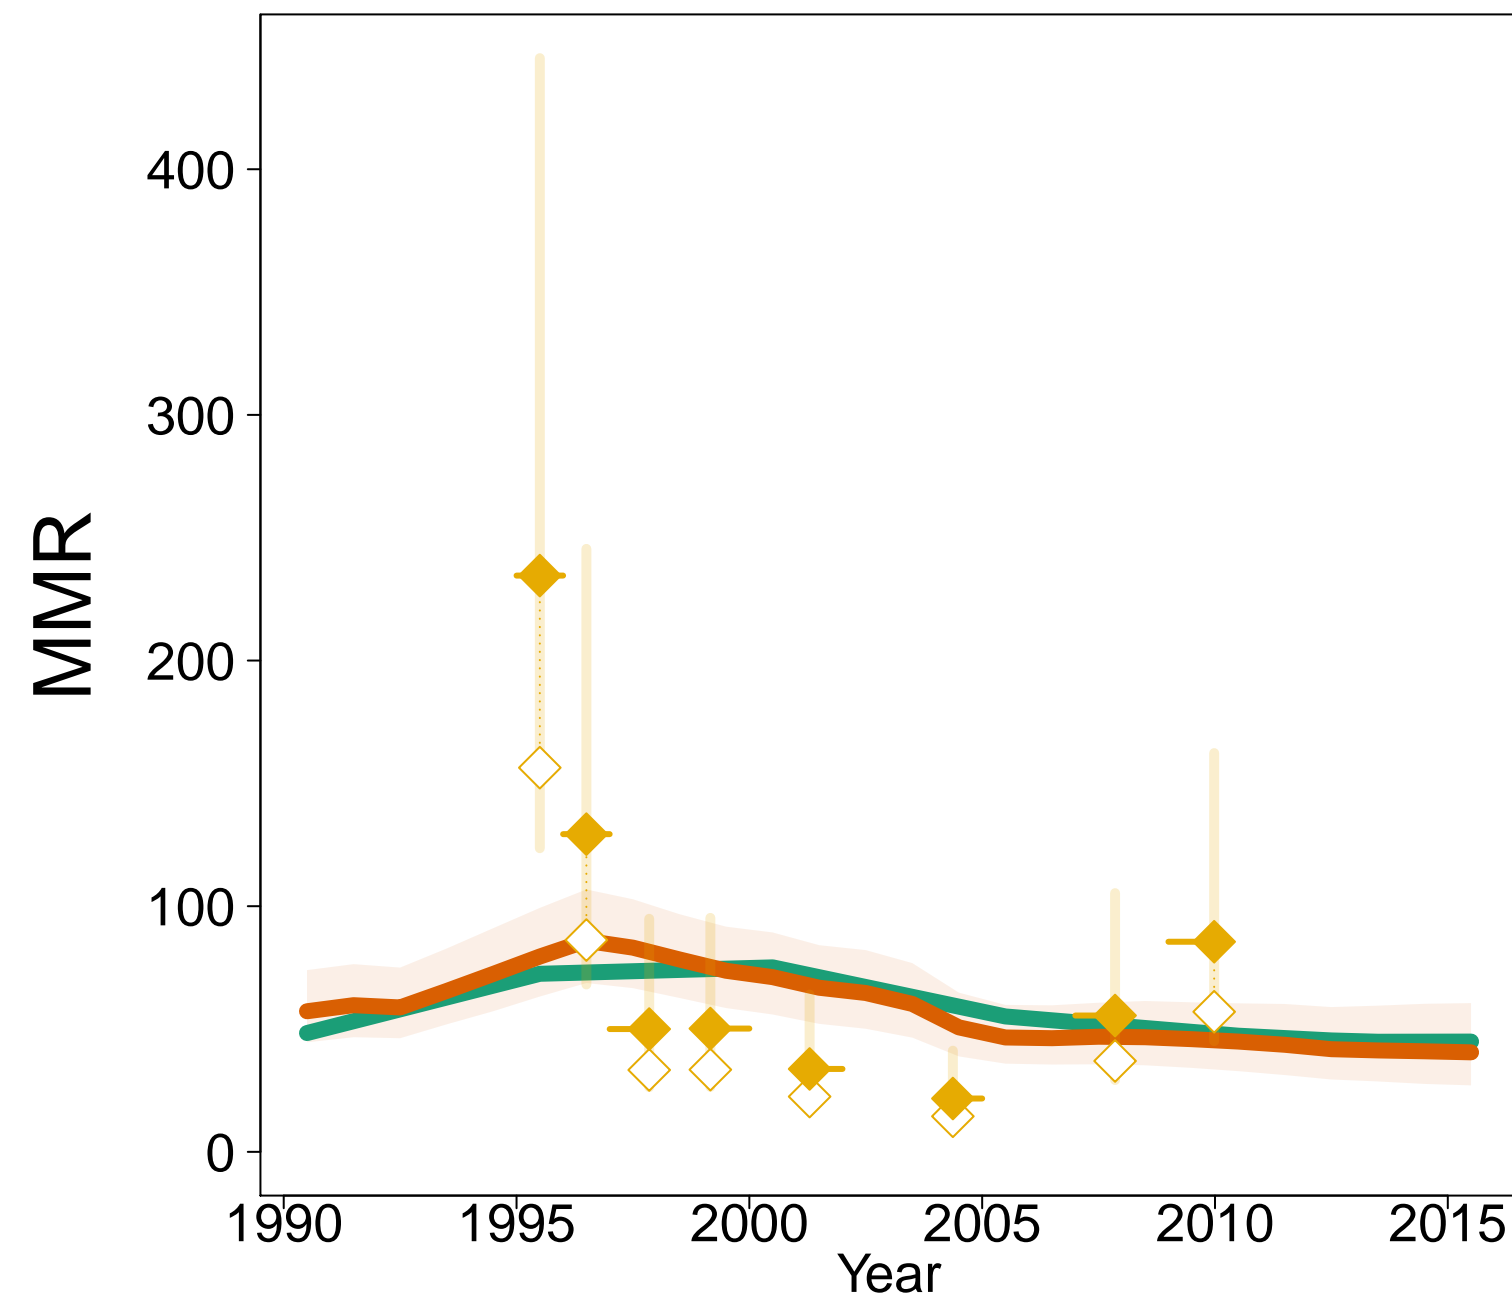

– Estimates –  
Bmat 2014  
MMEIG 2014  
– Data –  
Observed Data  
Adjusted Data  
– Data type –  
VR

Sudan [SDN; B]  
(Eastern Africa)

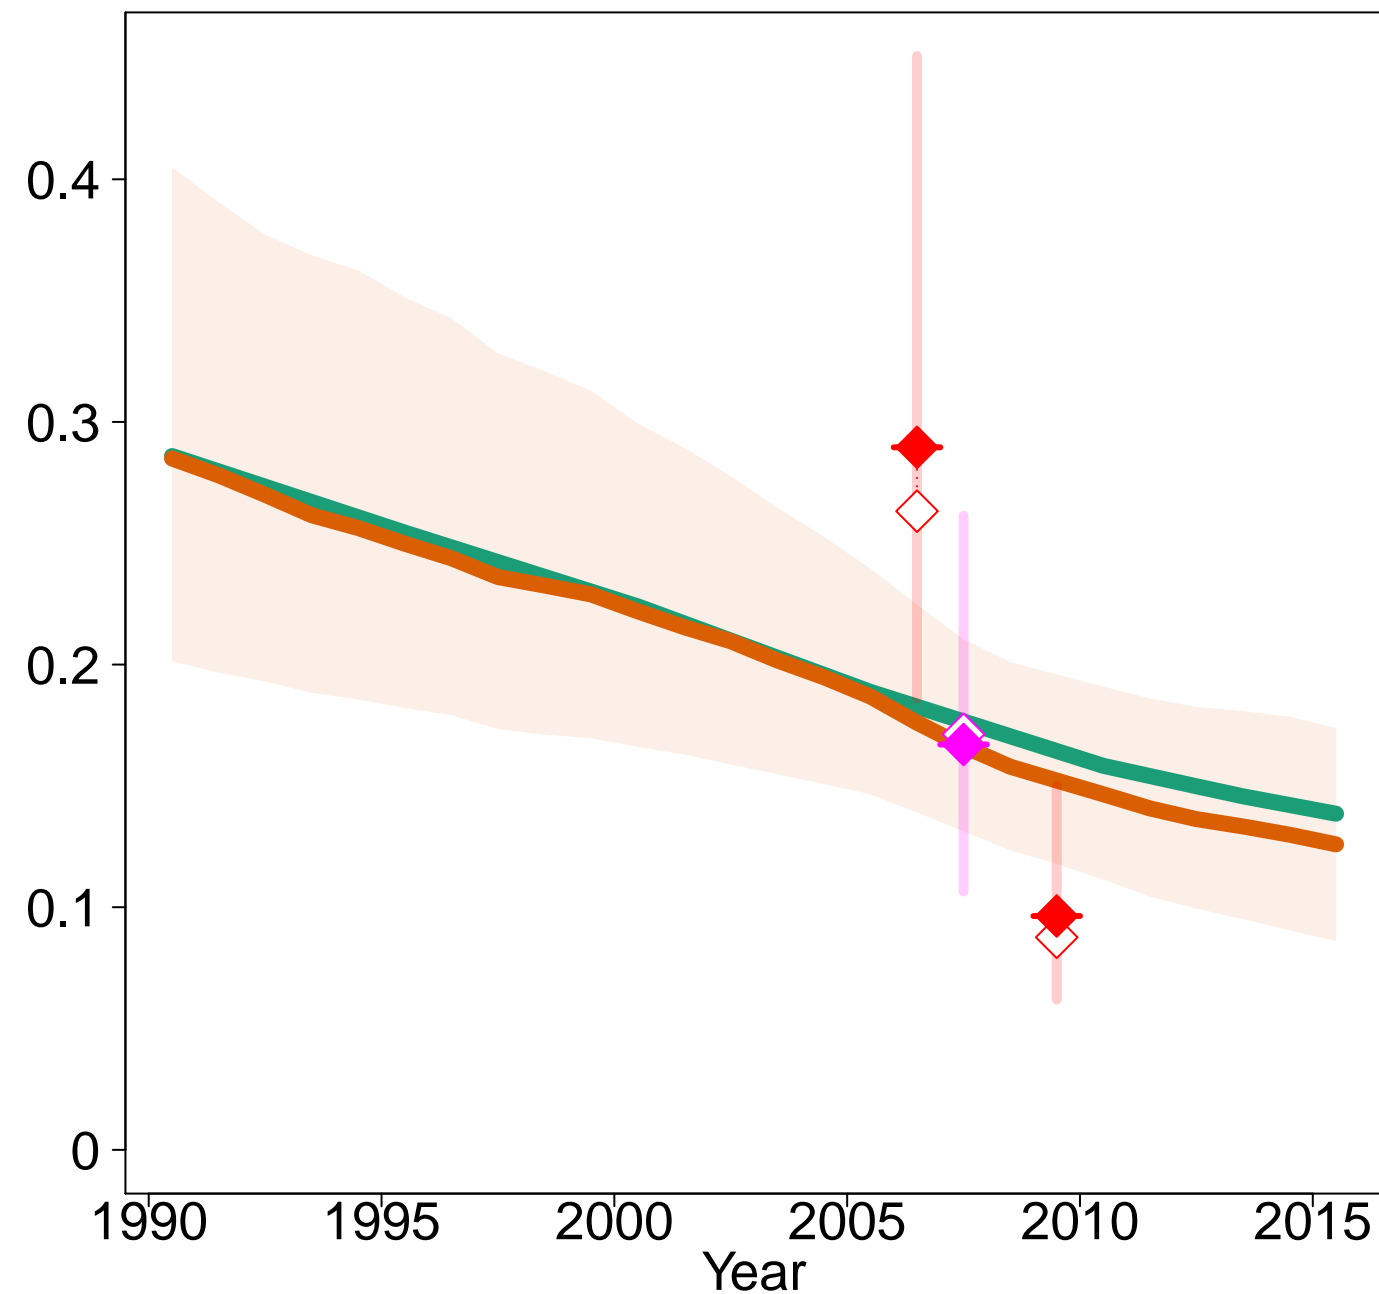

Sudan [SDN; B]  
(Eastern Africa)

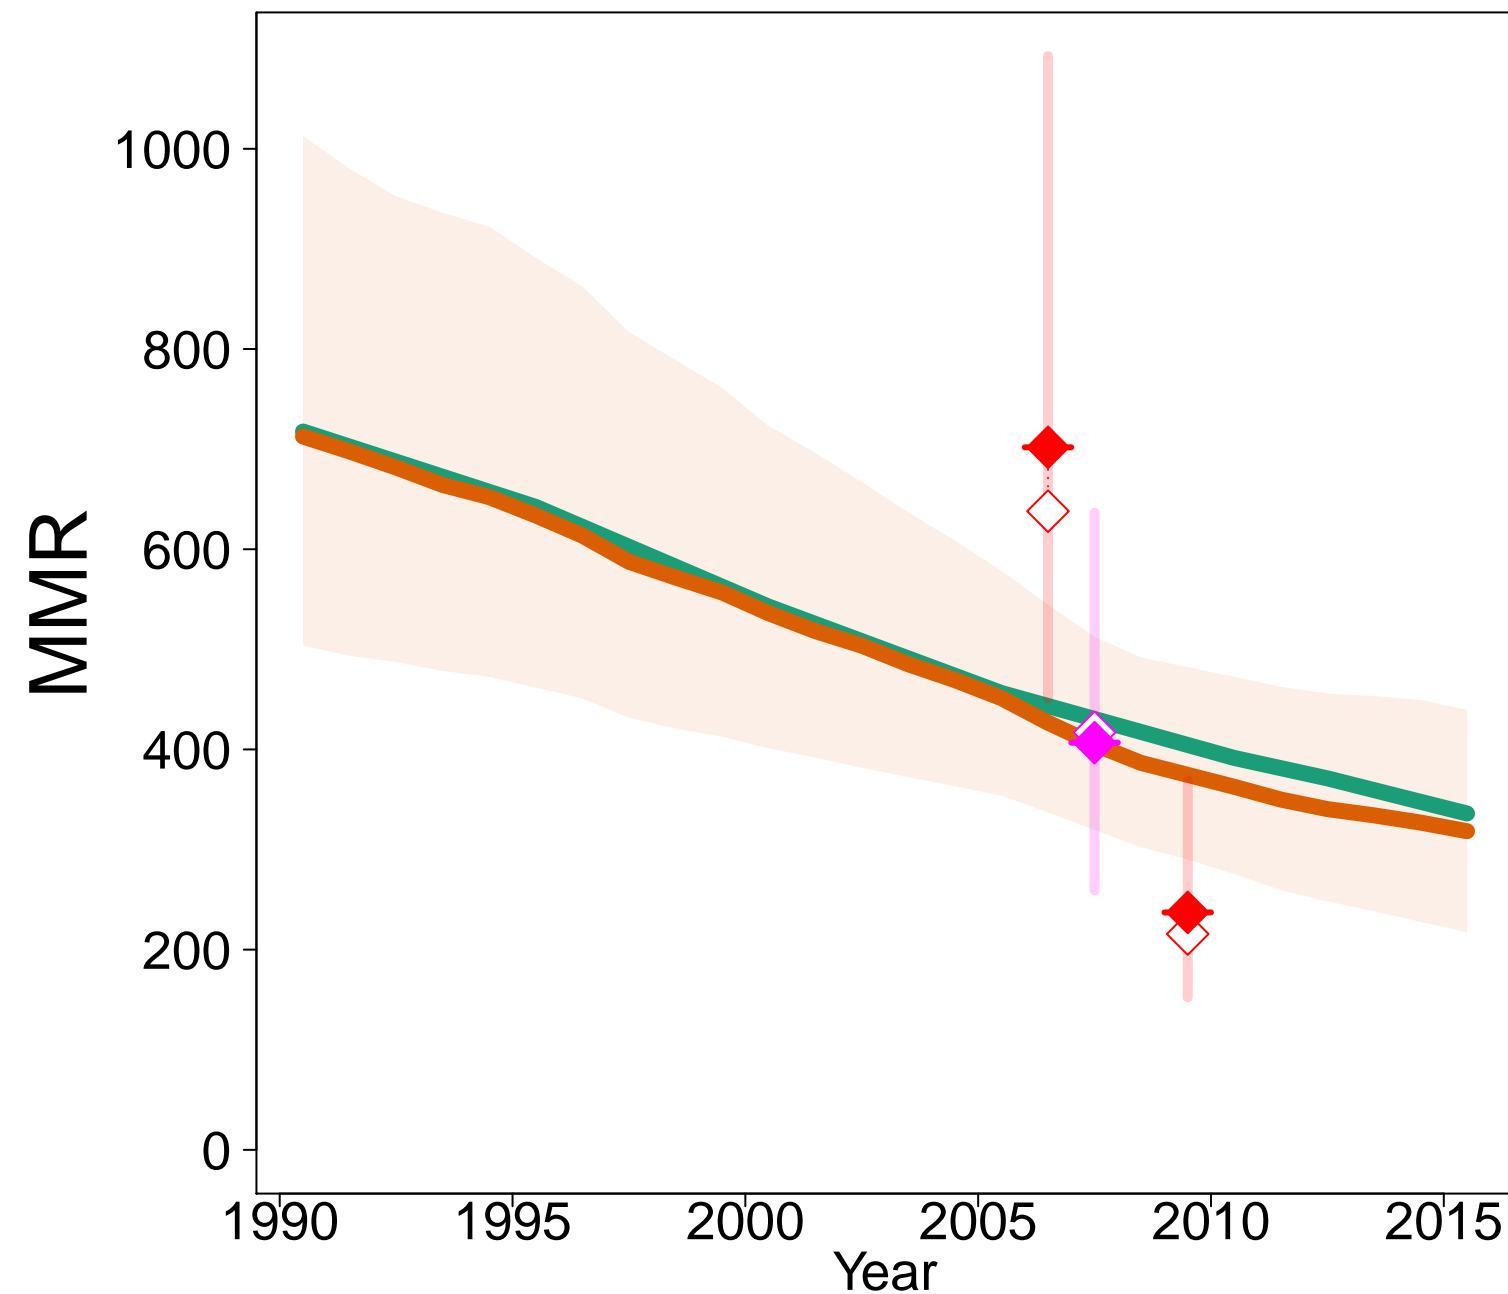

- Estimates –
- Bmat 2014
- MMEIG 2014
- Data –
- Observed Data
- Adjusted Data
- Data type –
- Census
- Misc. studies

Suriname [SUR; A]  
(South America)

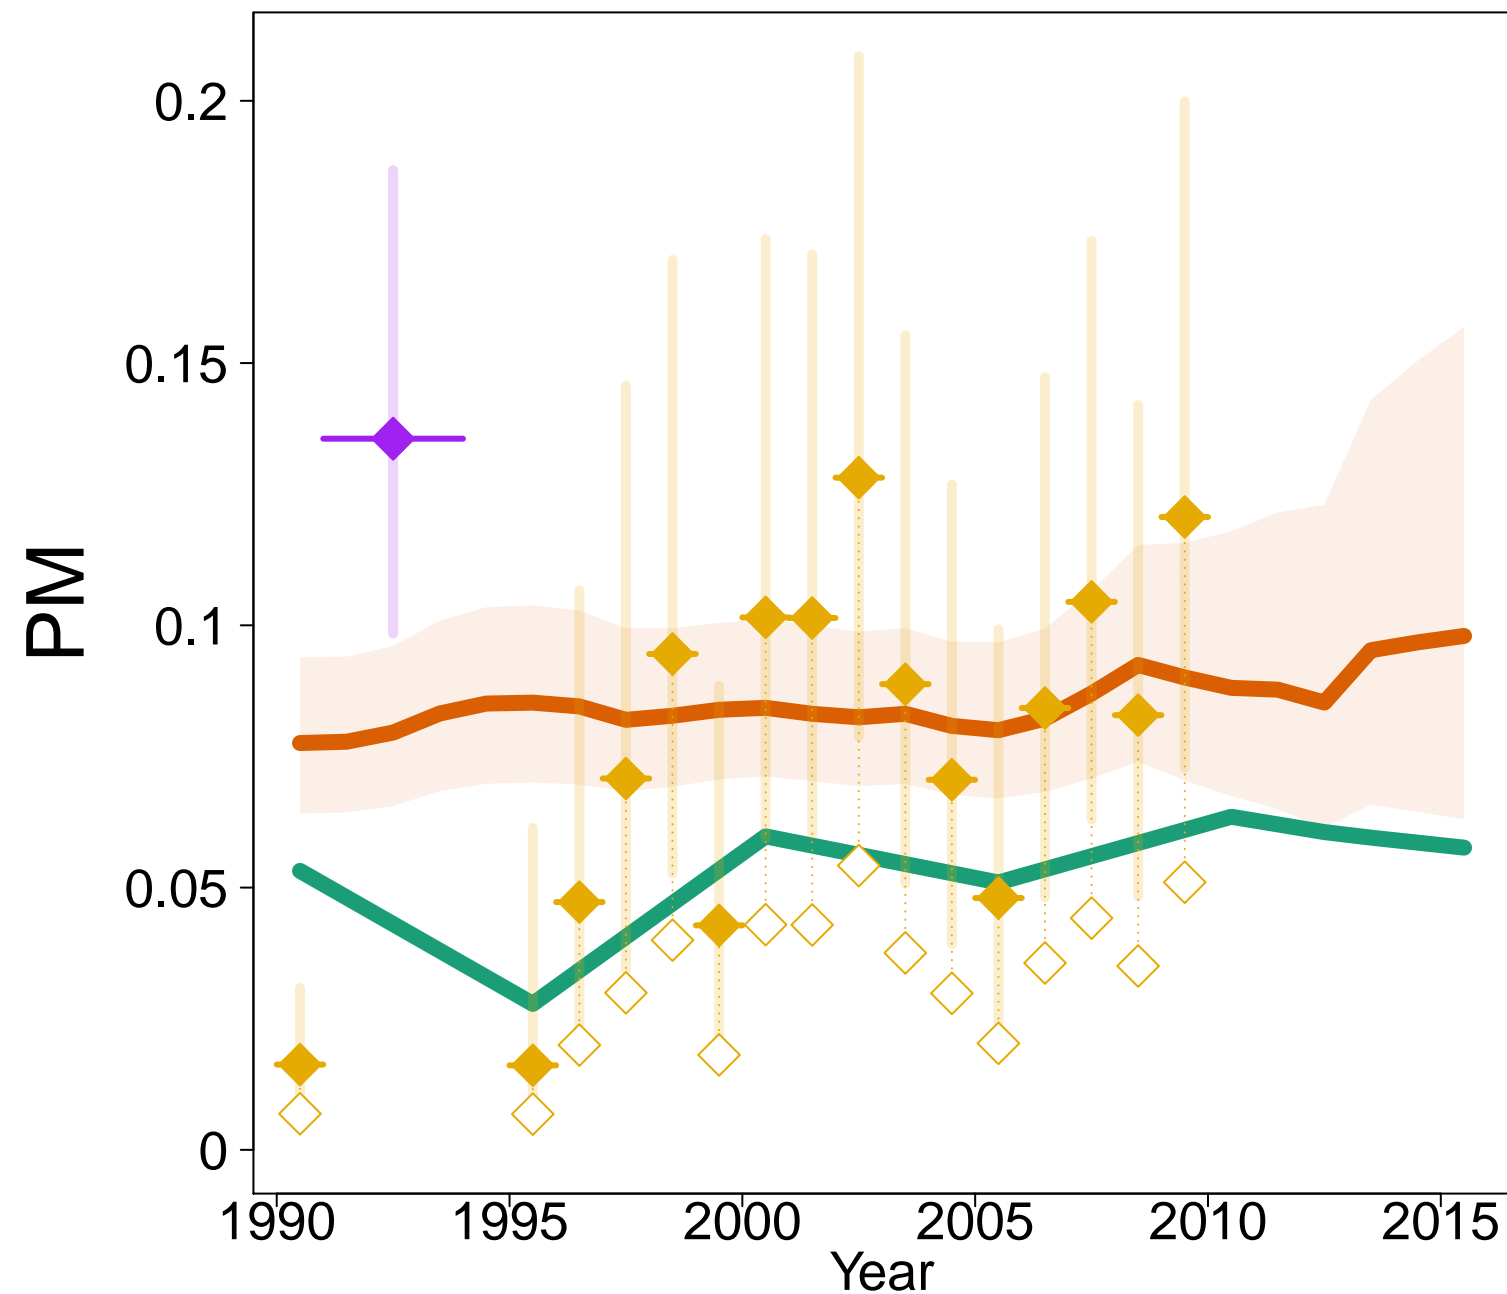

Suriname [SUR; A]  
(South America)

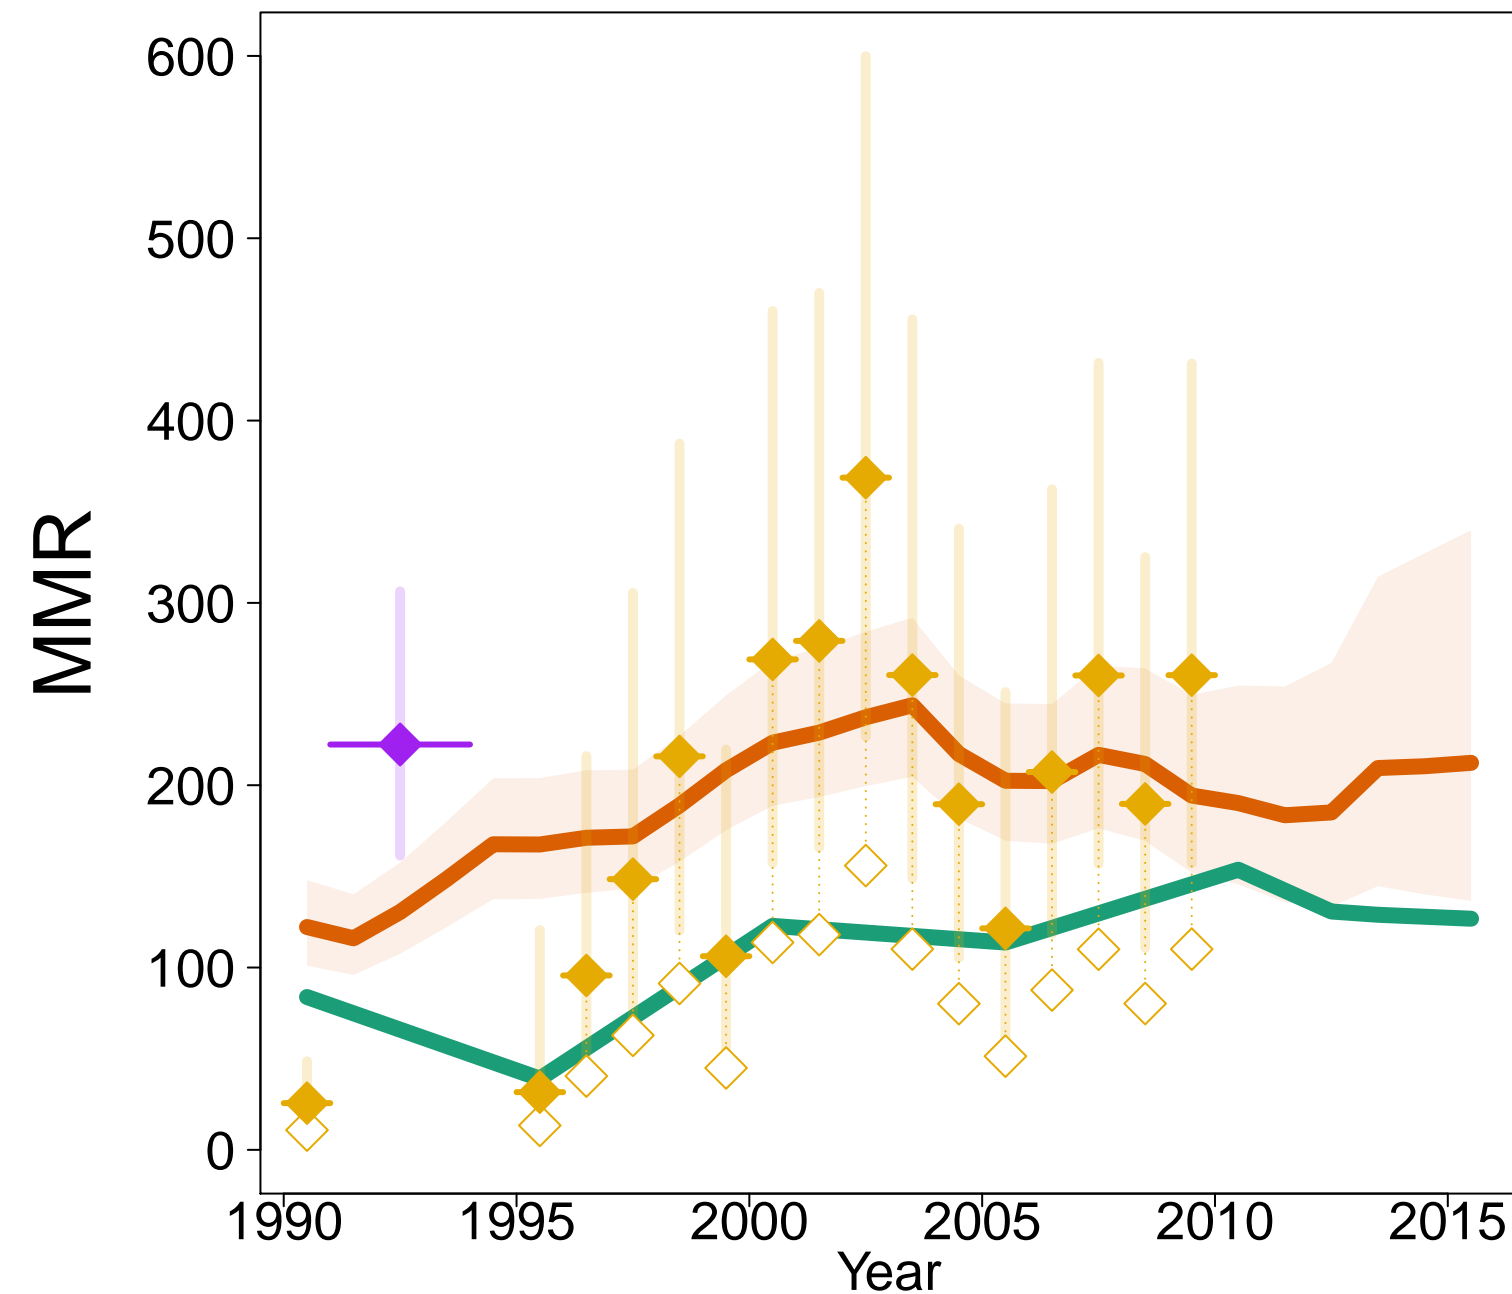

- Estimates –
- Bmat 2014
- MMEIG 2014
- Data –
- ◊ Observed Data
- ◆ Adjusted Data
- Data type –
- ◆ VR
- ◆ Spec. studies

Swaziland [SWZ; B]  
(Southern Africa)

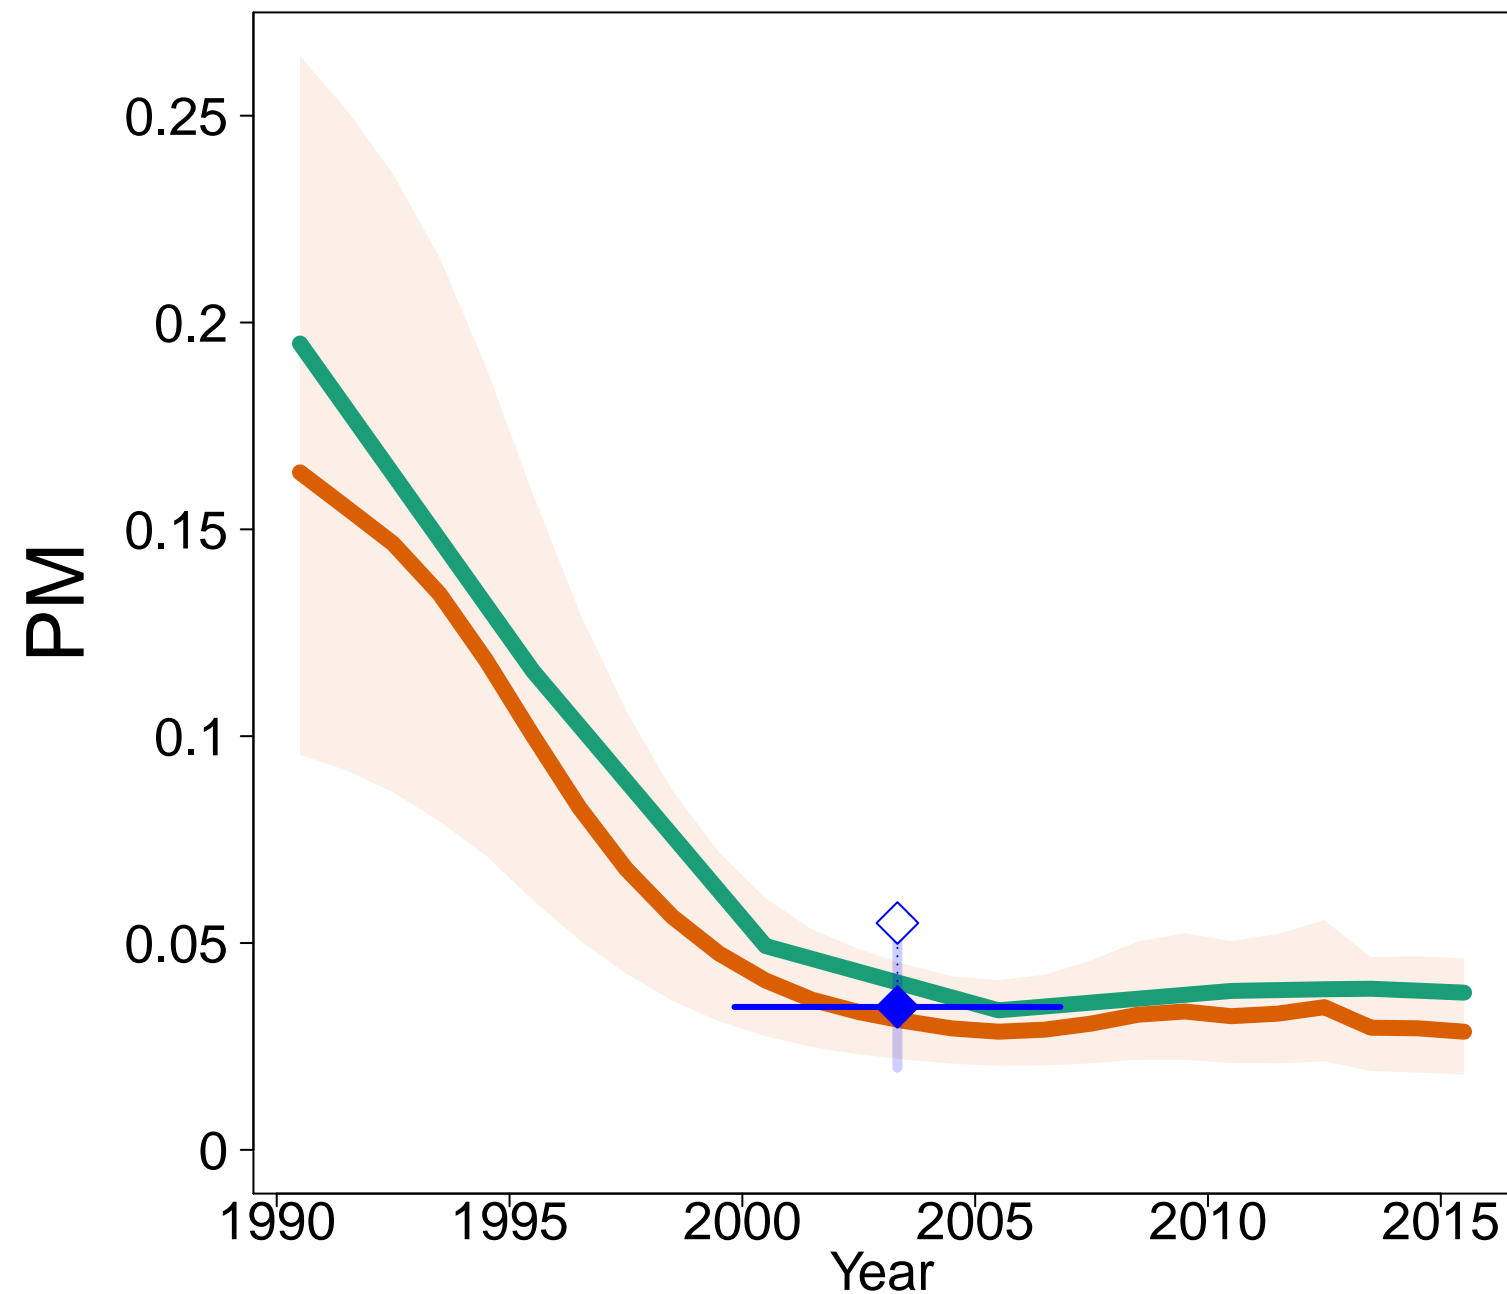

Swaziland [SWZ; B]  
(Southern Africa)

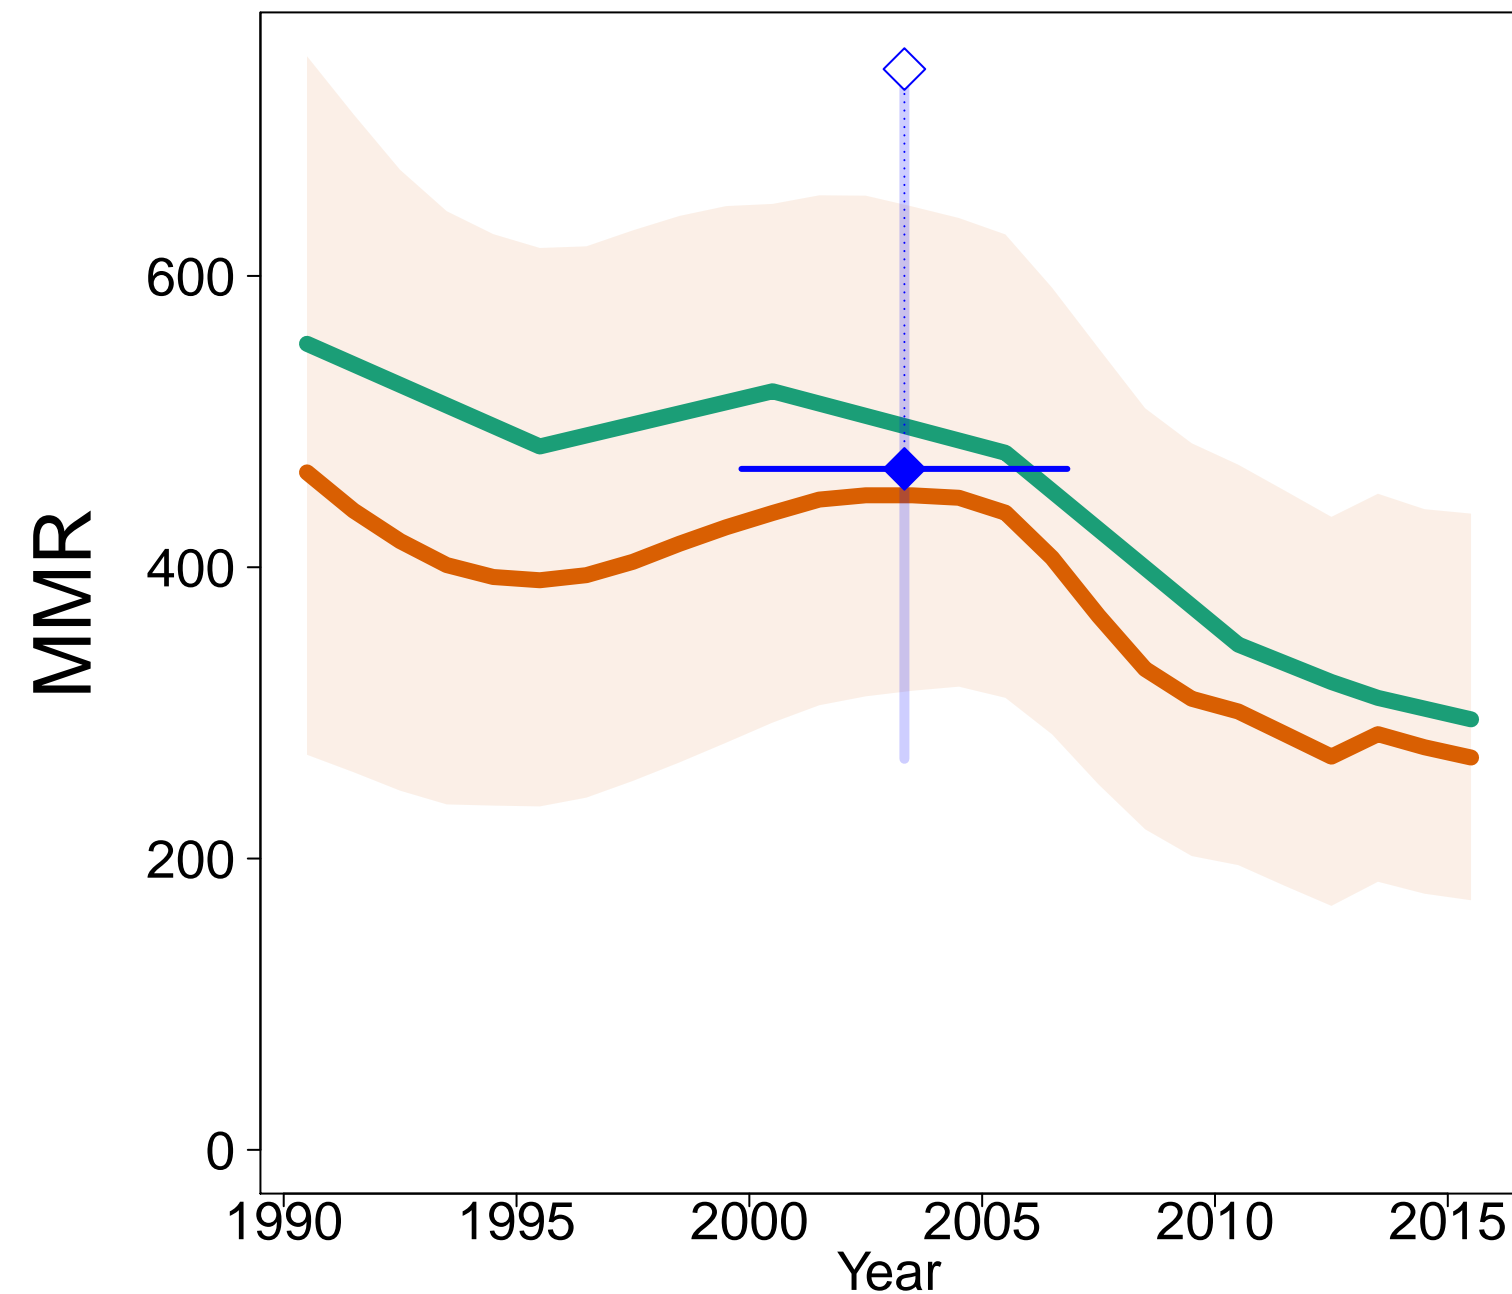

- Estimates –
- Bmat 2014
- MMEIG 2014
- Data –
- Observed Data
- Adjusted Data
- Data type –
- DHS

Sweden [SWE; A]  
(Developed regions)

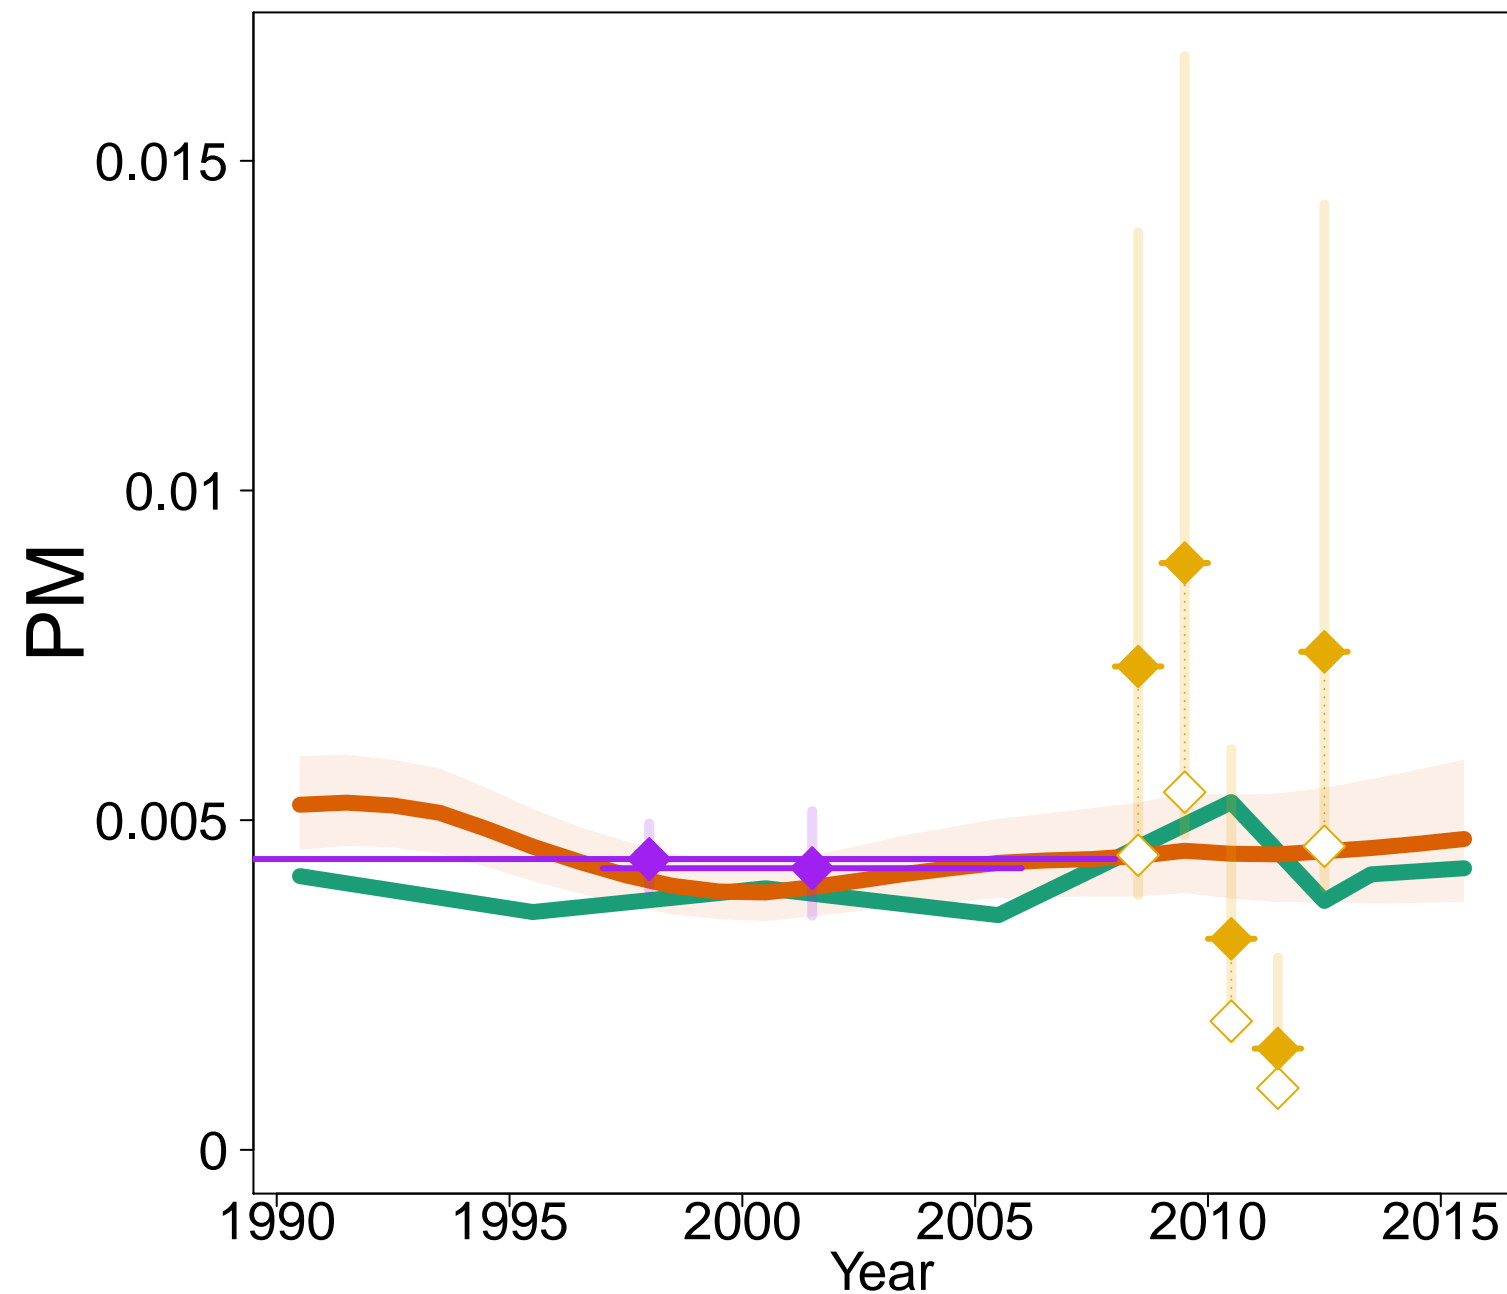

Sweden [SWE; A]  
(Developed regions)

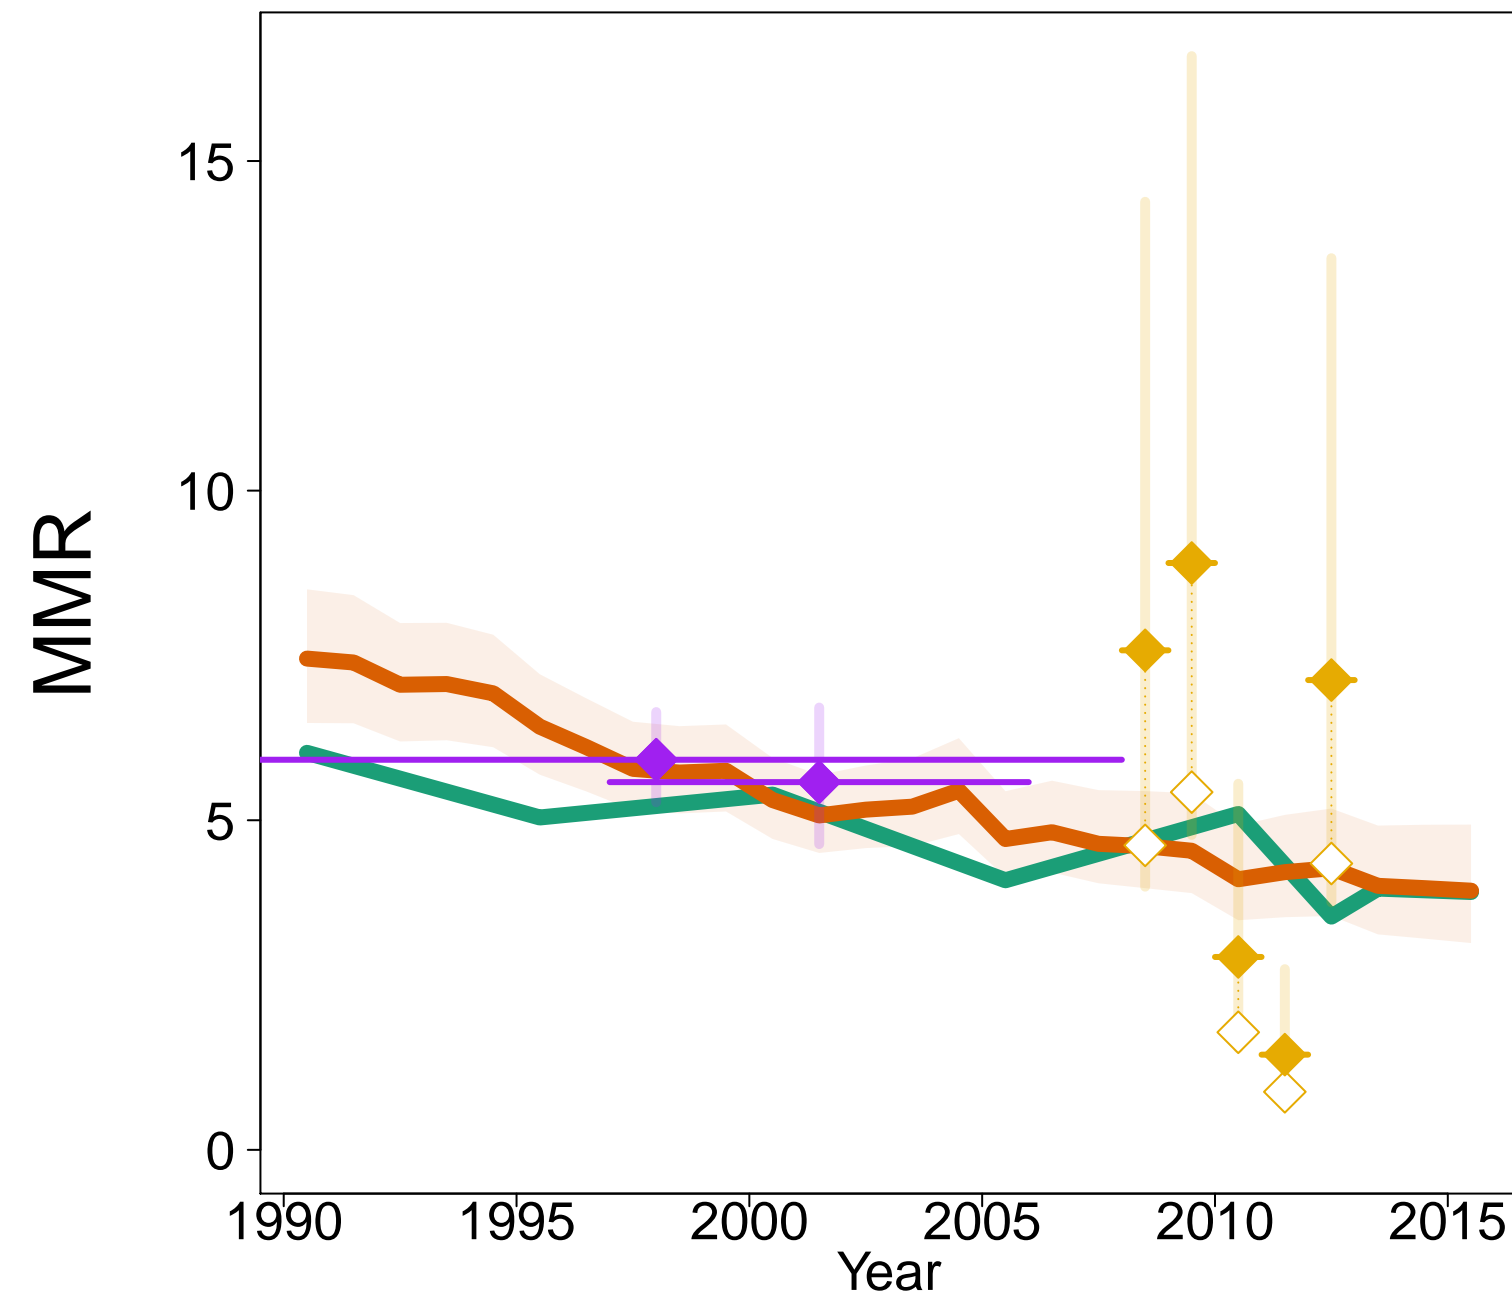

- Estimates –
- Bmat 2014
- MMEIG 2014
- Data –
- Observed Data
- Adjusted Data
- Data type –
- VR
- Spec. studies

Switzerland [CHE; A]  
(Developed regions)

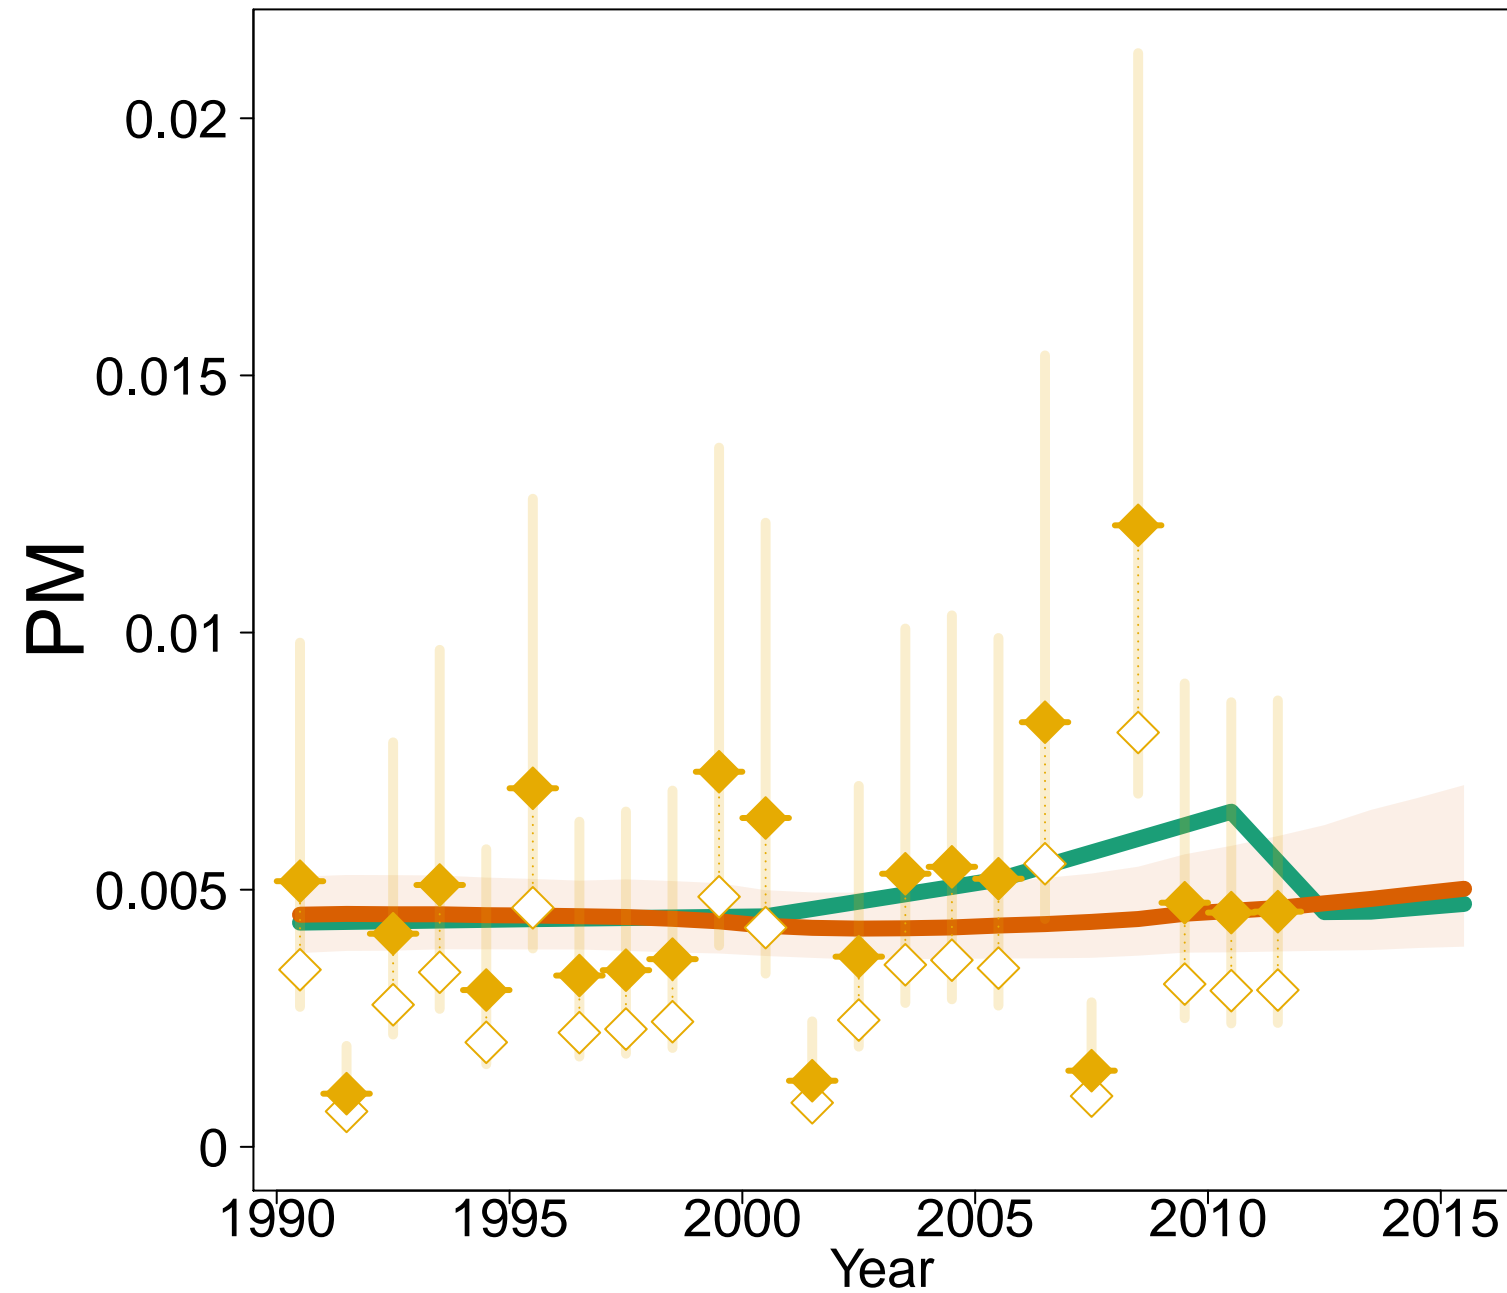

Switzerland [CHE; A]  
(Developed regions)

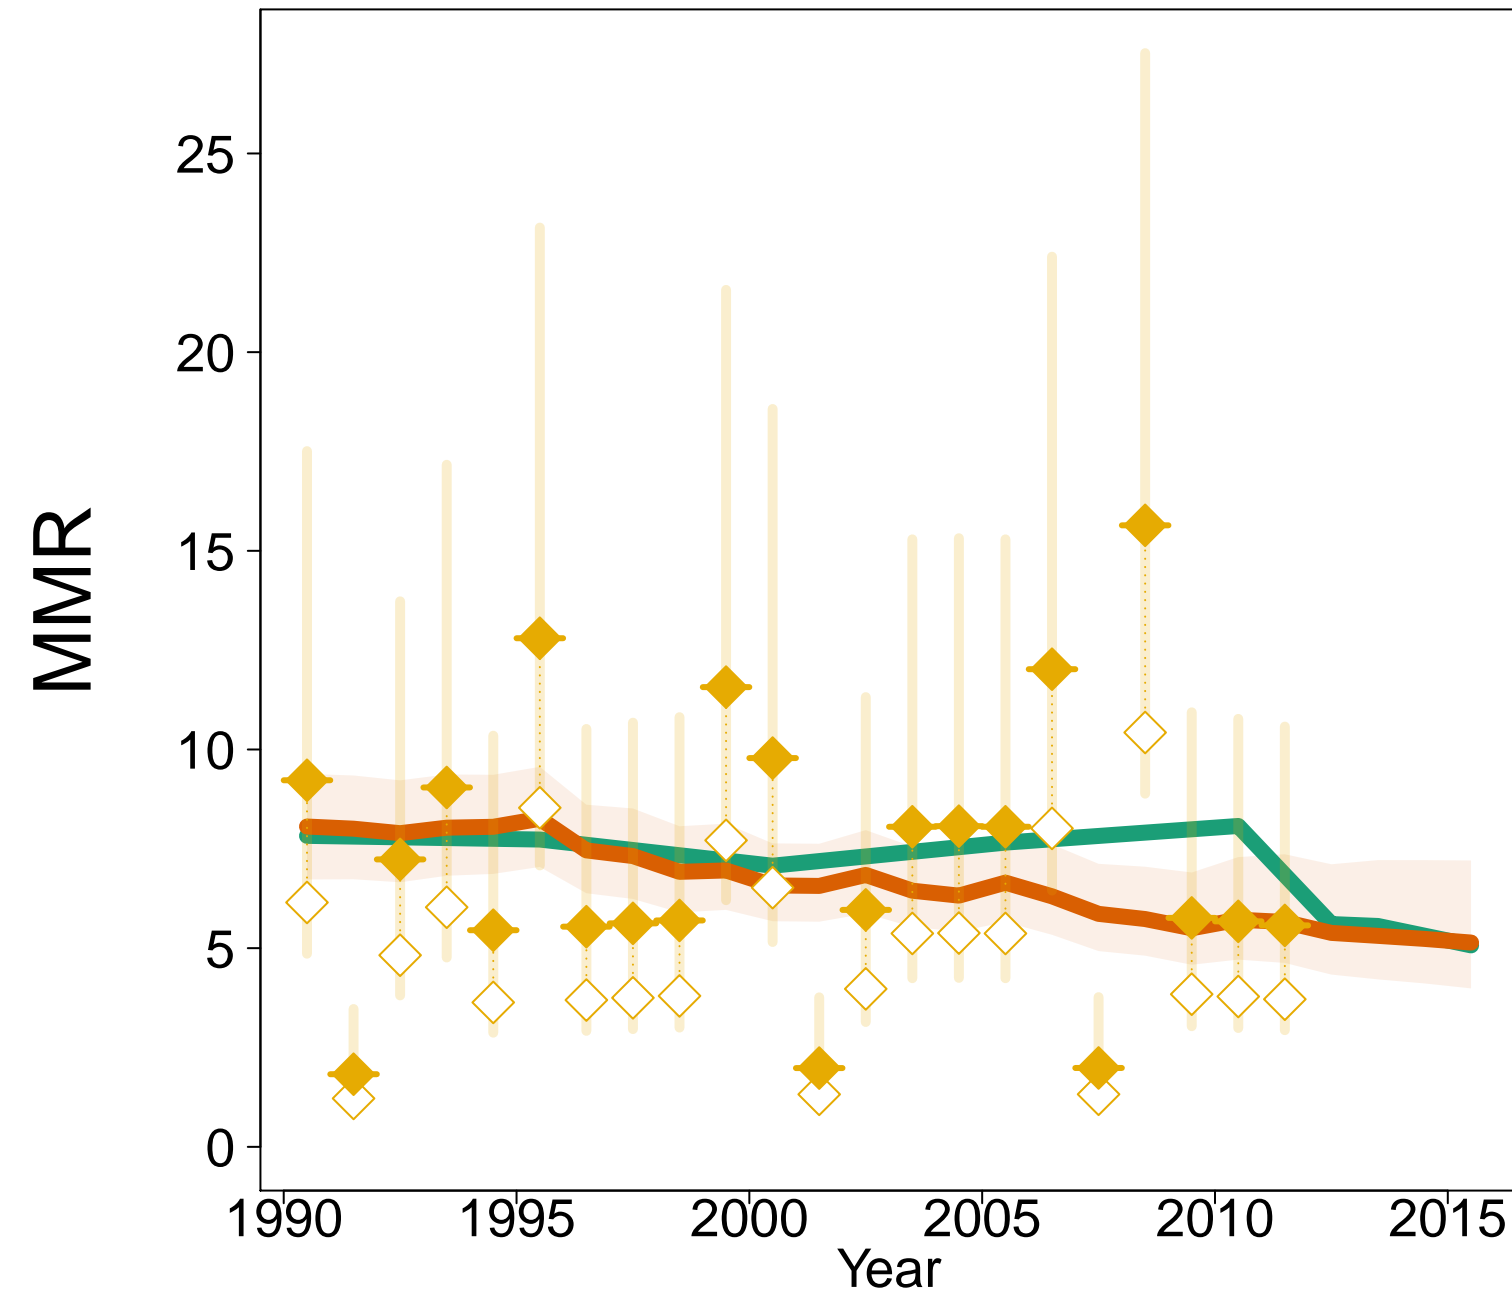

- Estimates –
- Bmat 2014
- MMEIG 2014
- Data –
- Observed Data
- Adjusted Data
- Data type –
- VR

Syrian Arab Republic [SYR; B]  
(Western Asia)

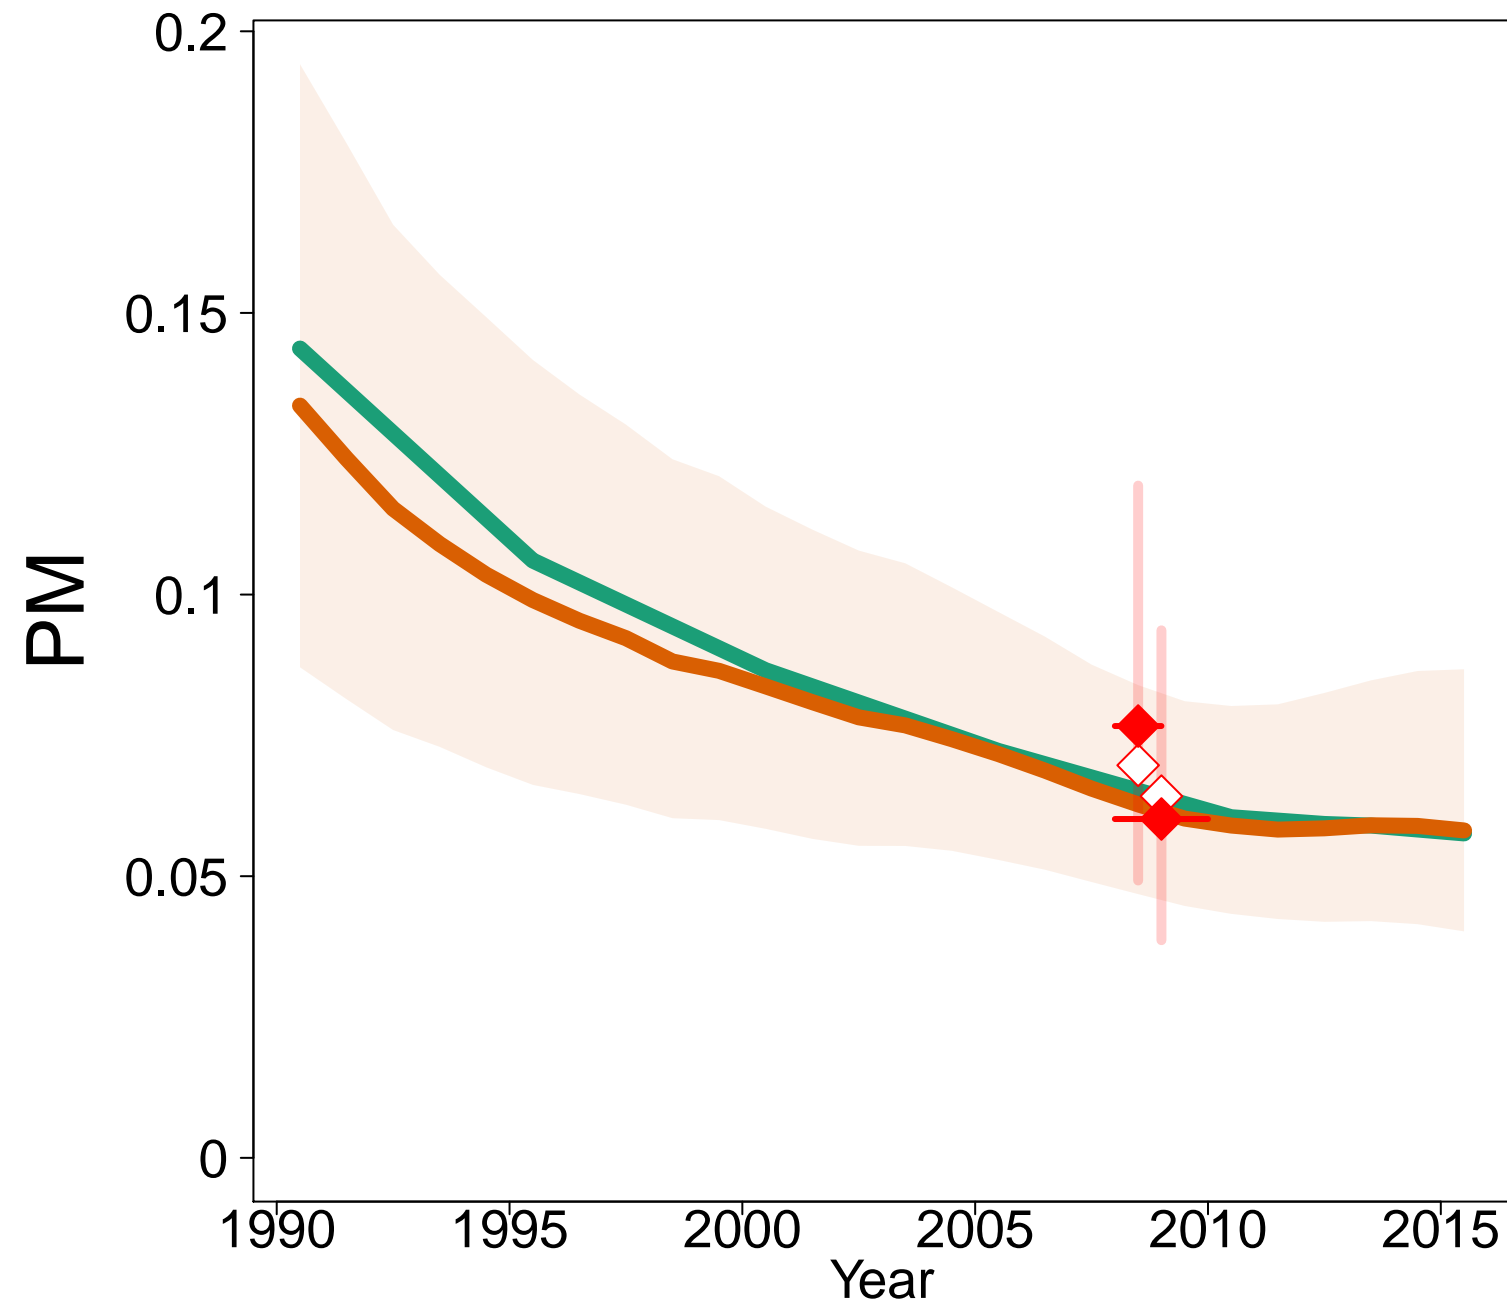

Syrian Arab Republic [SYR; B]  
(Western Asia)

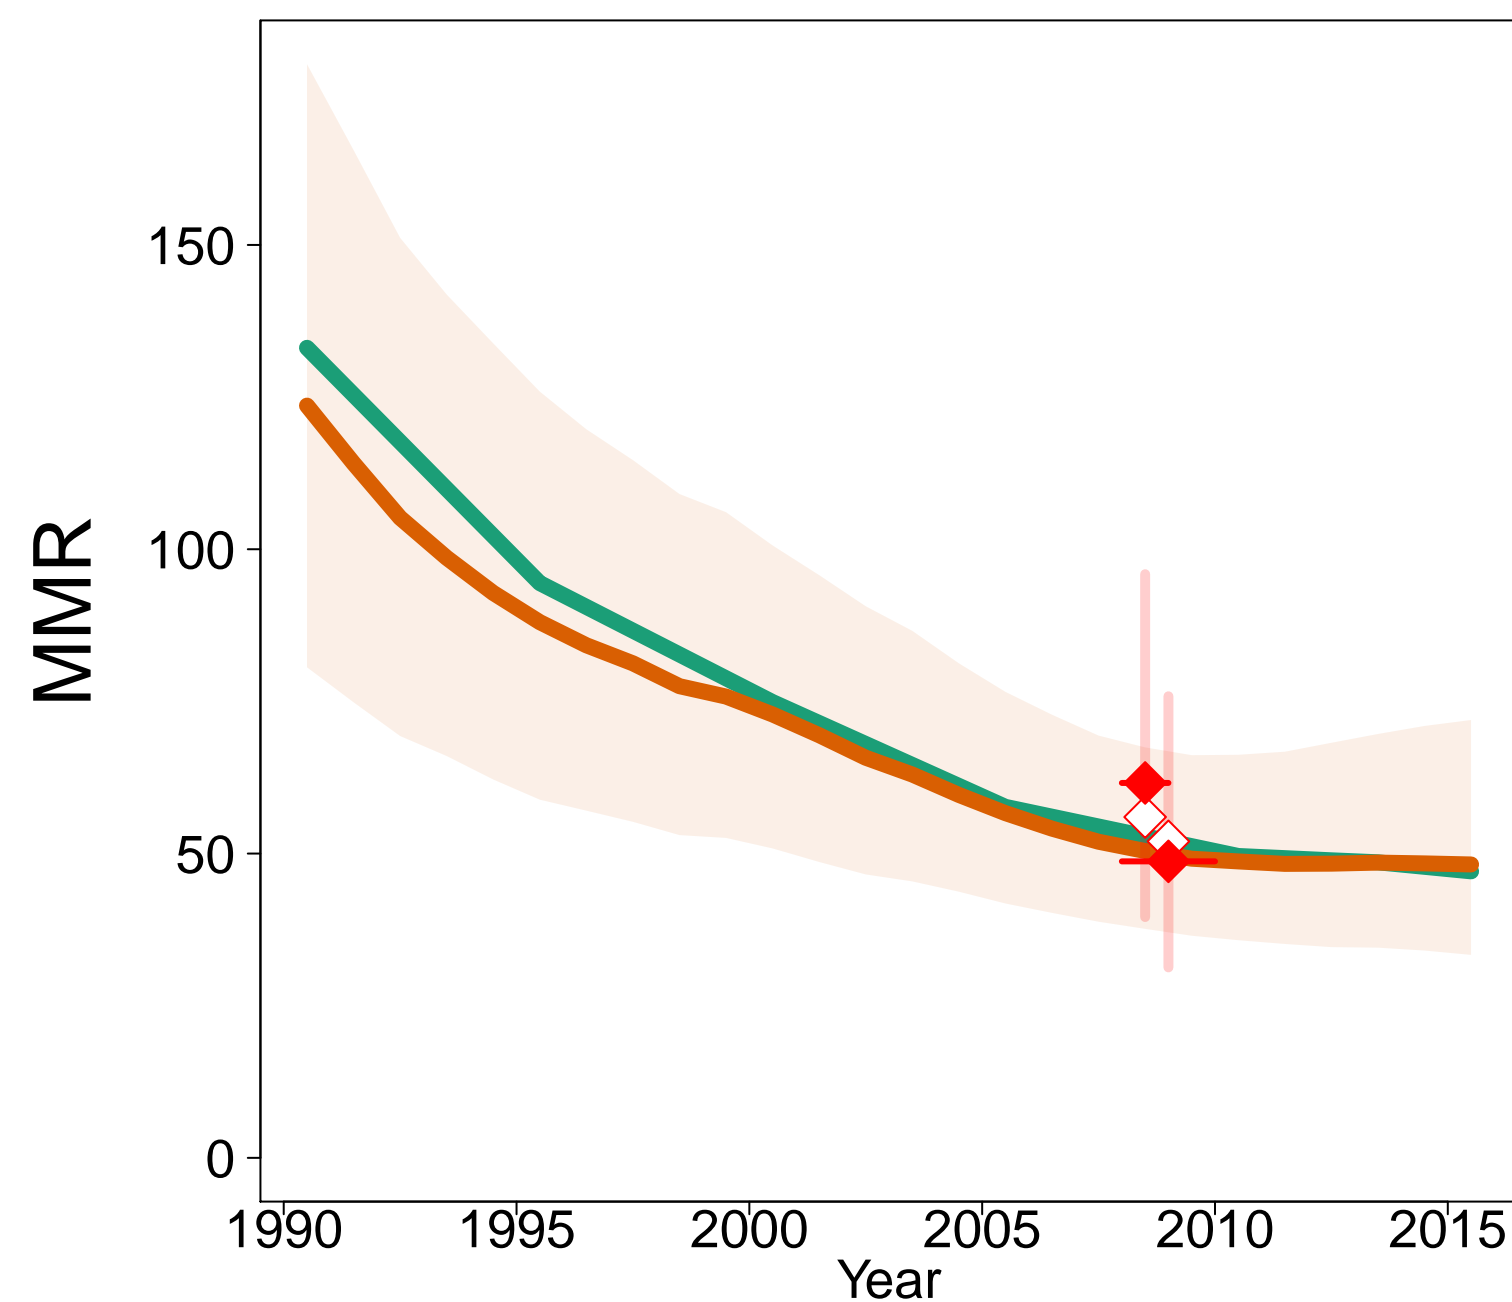

- Estimates –
- Bmat 2014
- MMEIG 2014
- Data –
- Observed Data
- Adjusted Data
- Data type –
- Misc. studies

Tajikistan [TJK; B]  
(Central Asia)

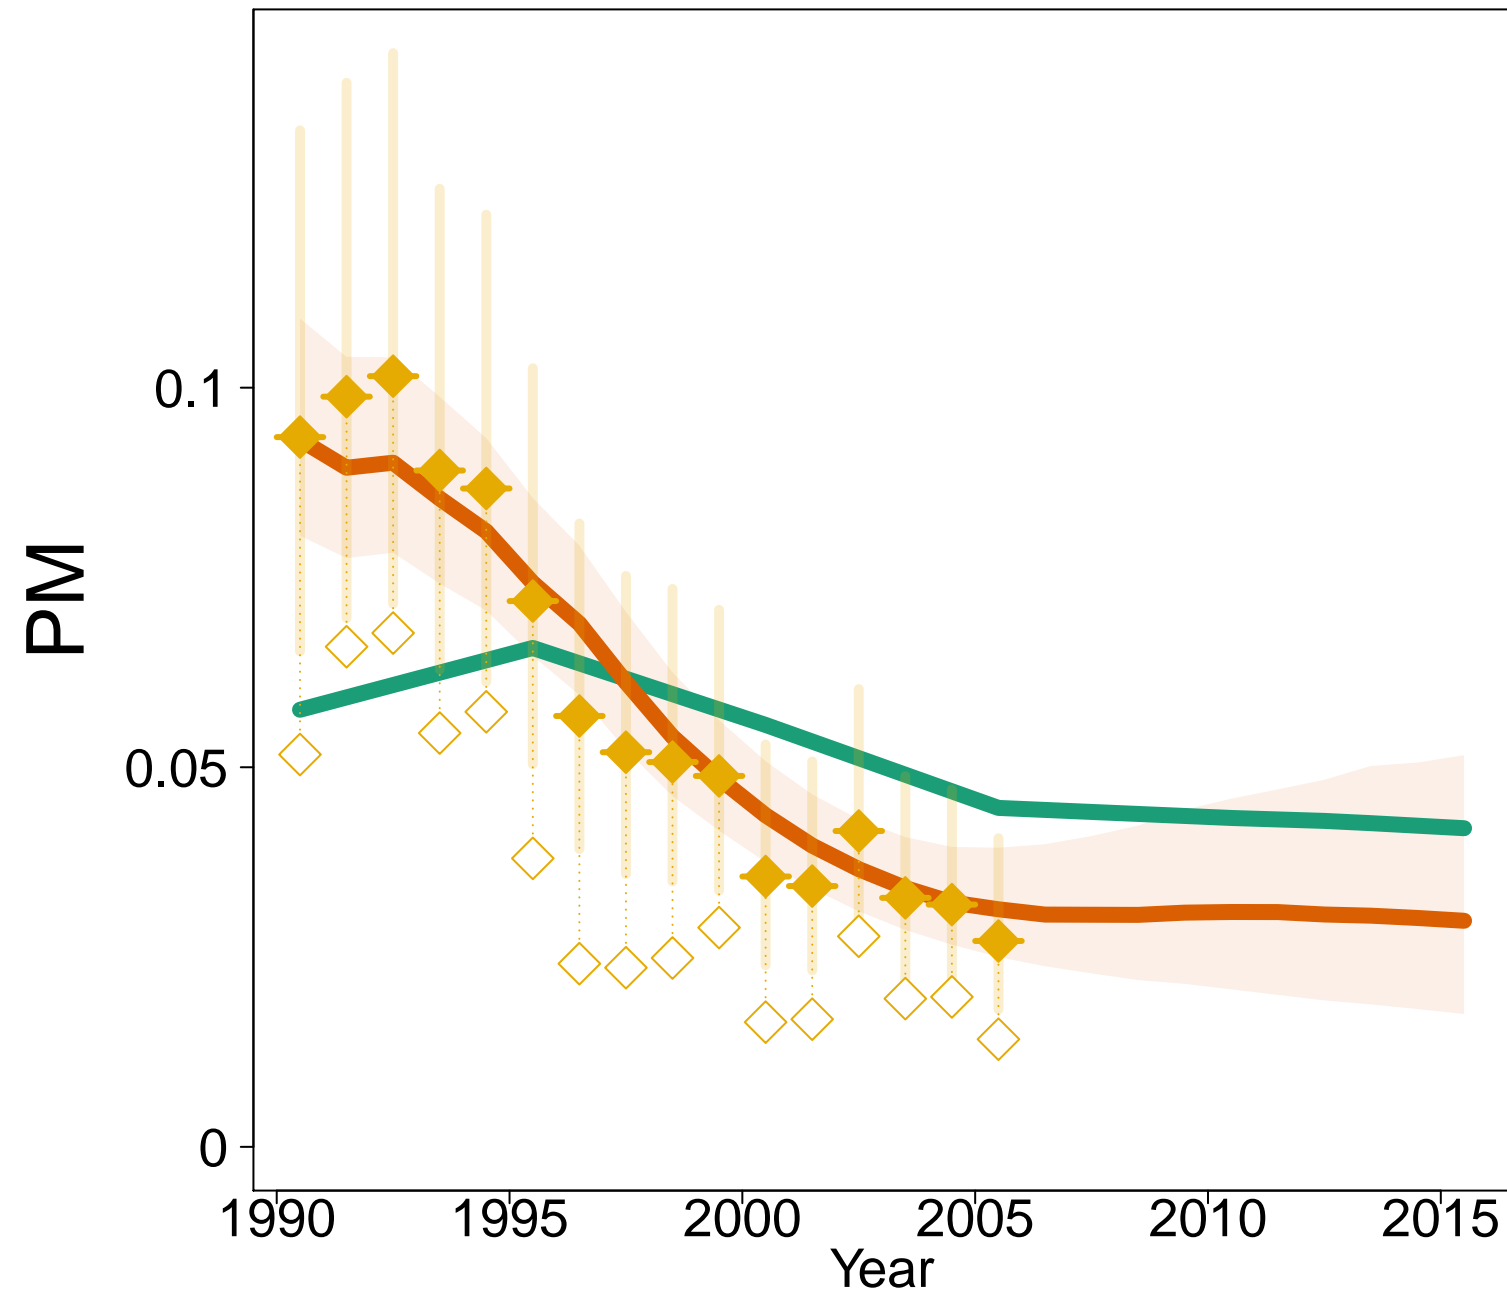

Tajikistan [TJK; B]  
(Central Asia)

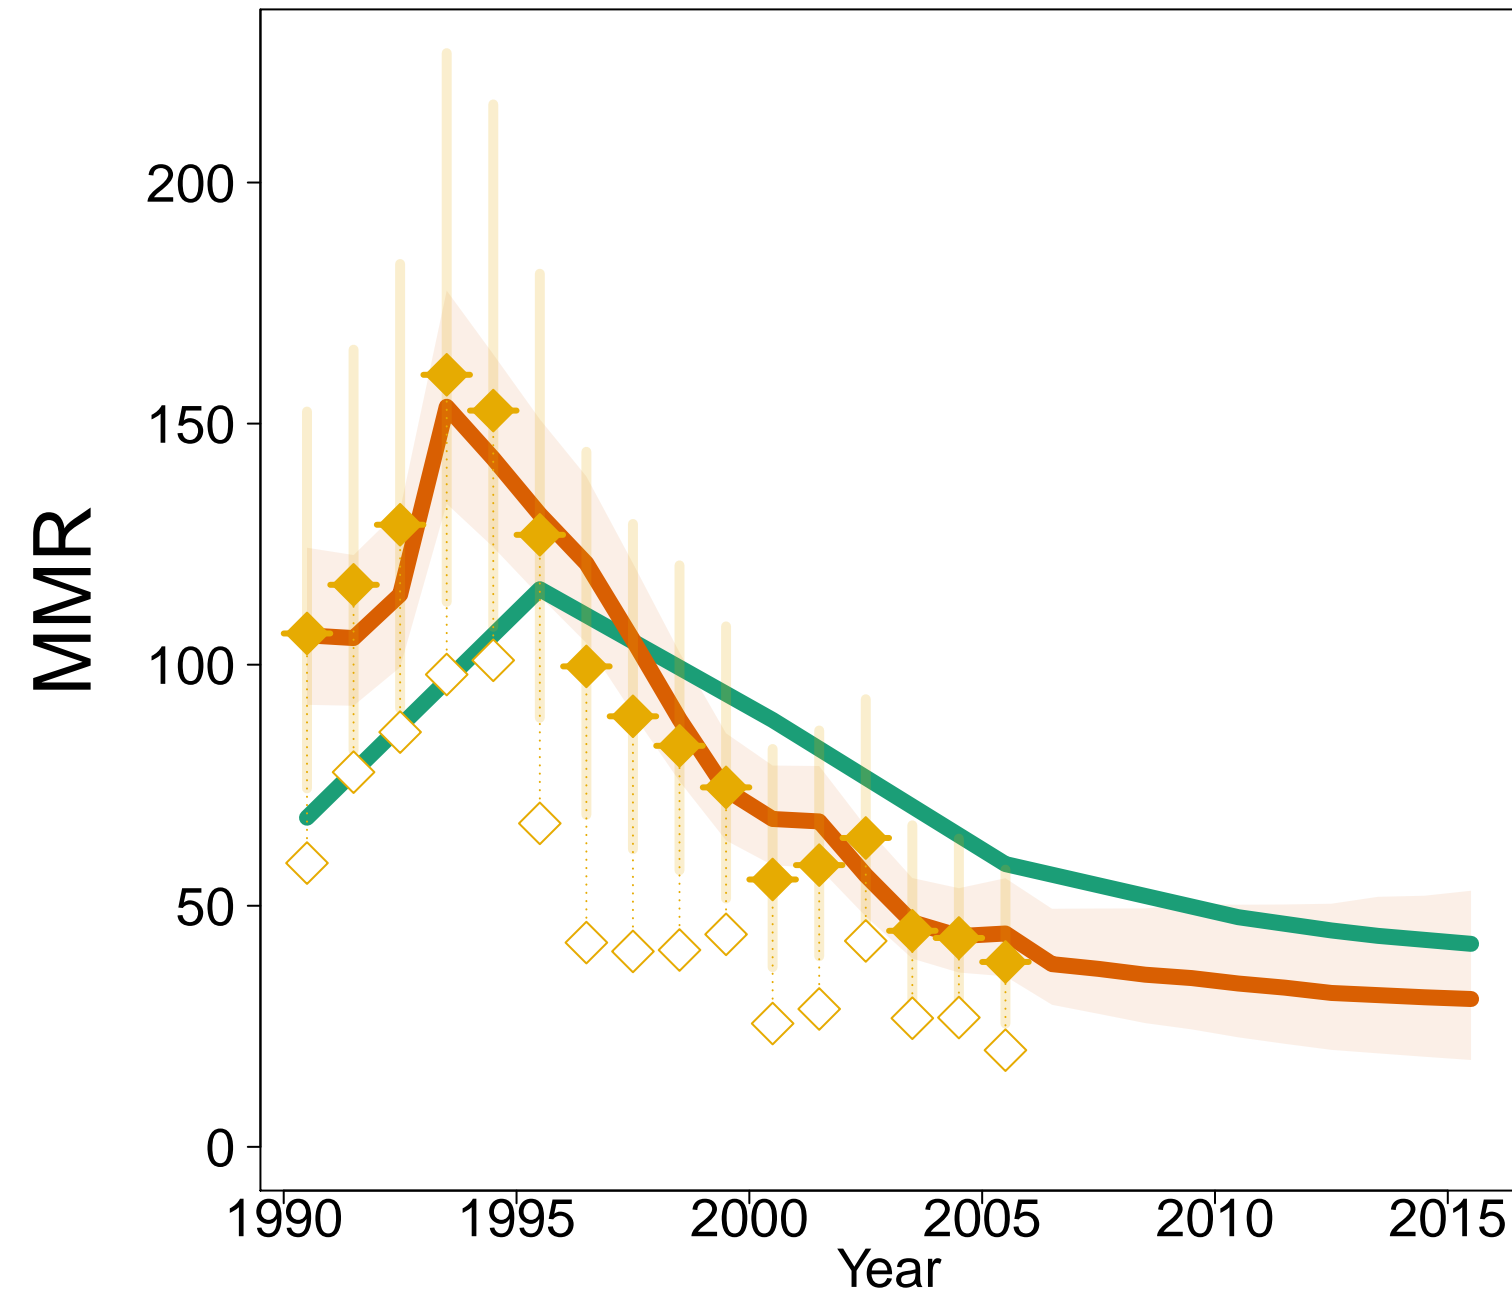

– Estimates –  
Bmat 2014  
MMEIG 2014  
– Data –  
Observed Data  
Adjusted Data  
– Data type –  
VR



Tanzania [TZA; B]  
(Eastern Africa)

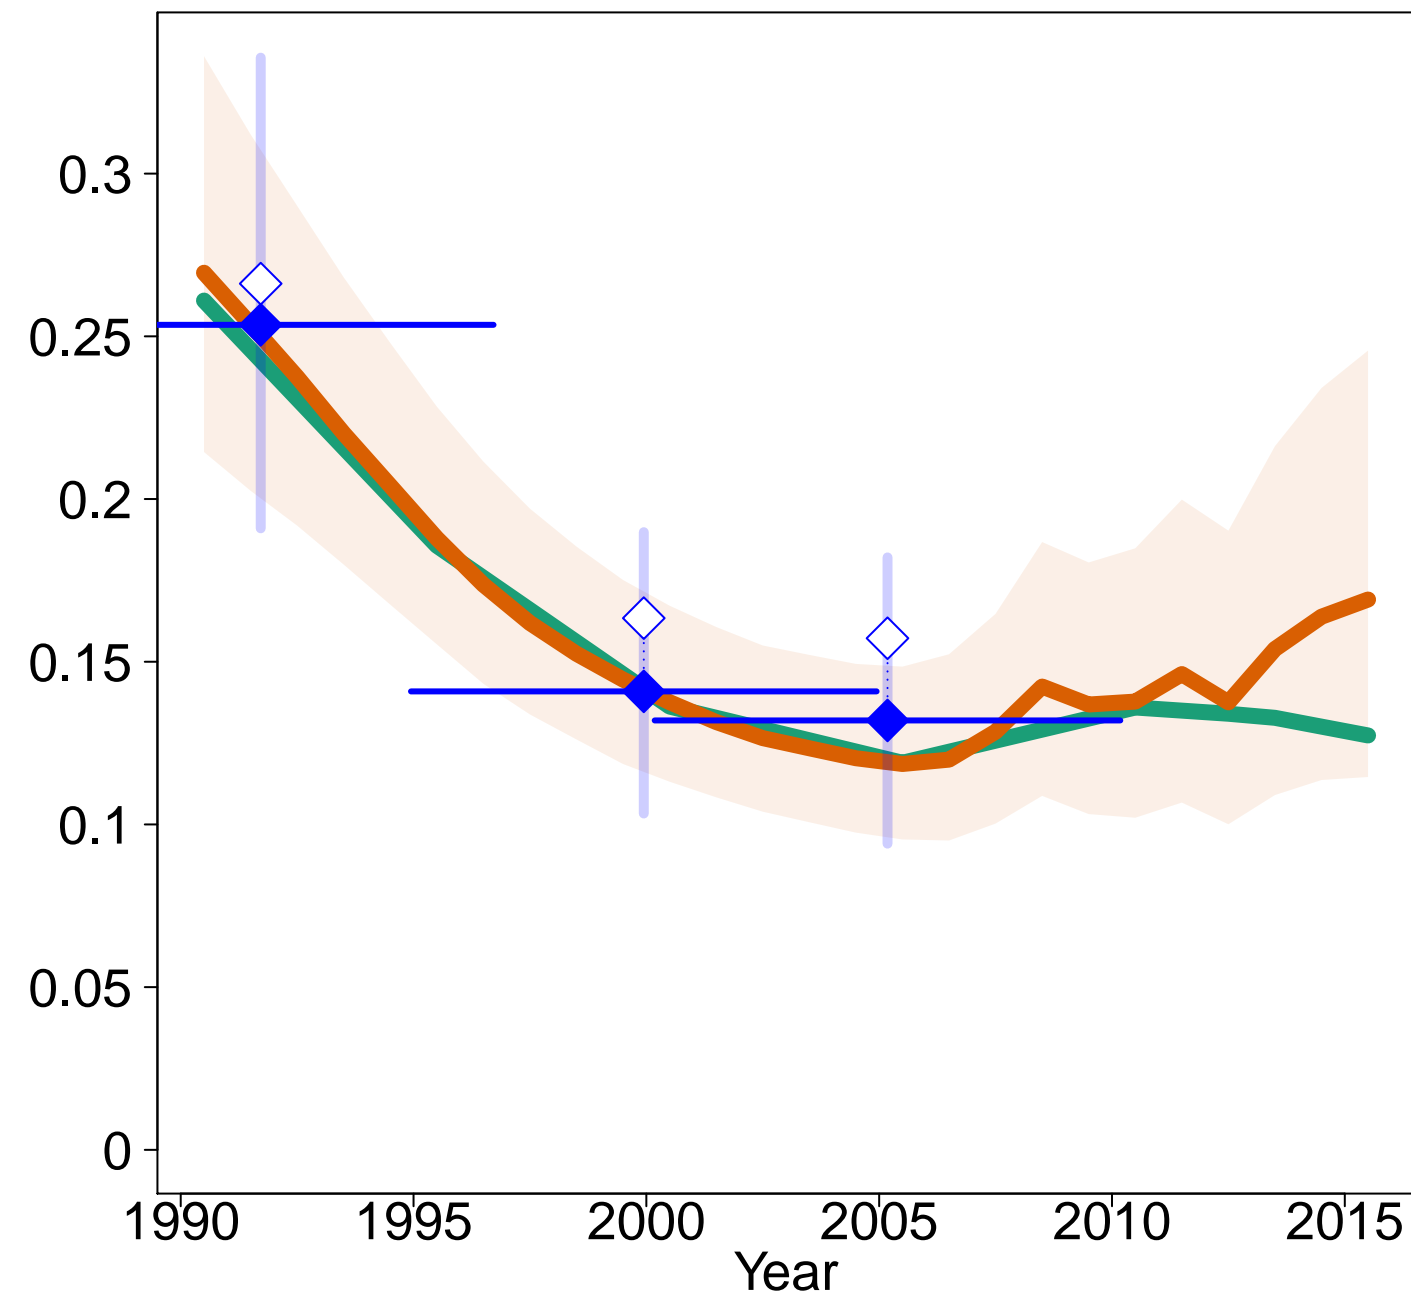

Tanzania [TZA; B]  
(Eastern Africa)

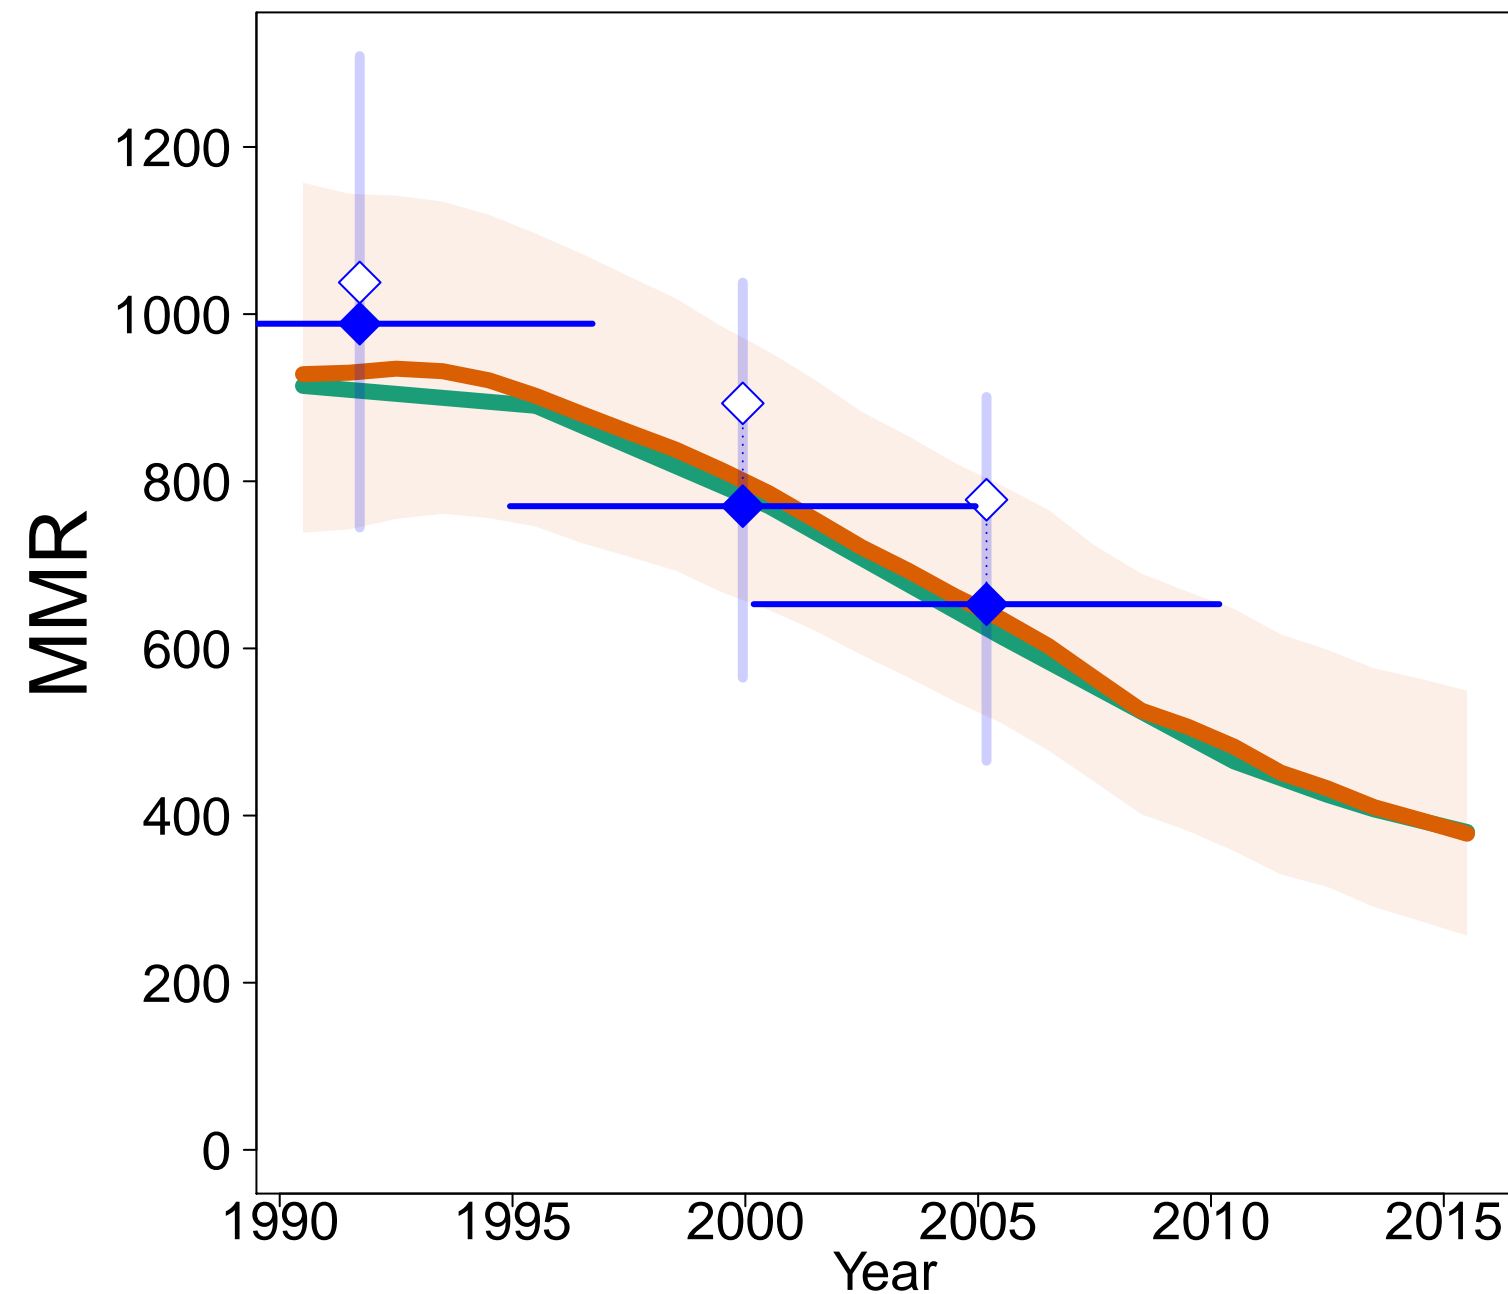

– Estimates –

Bmat 2014

MMEIG 2014

– Data –

Observed Data

Adjusted Data

– Data type –

DHS

TFYR Macedonia [MKD; A]  
(Transition countries of South-Eastern Europe)

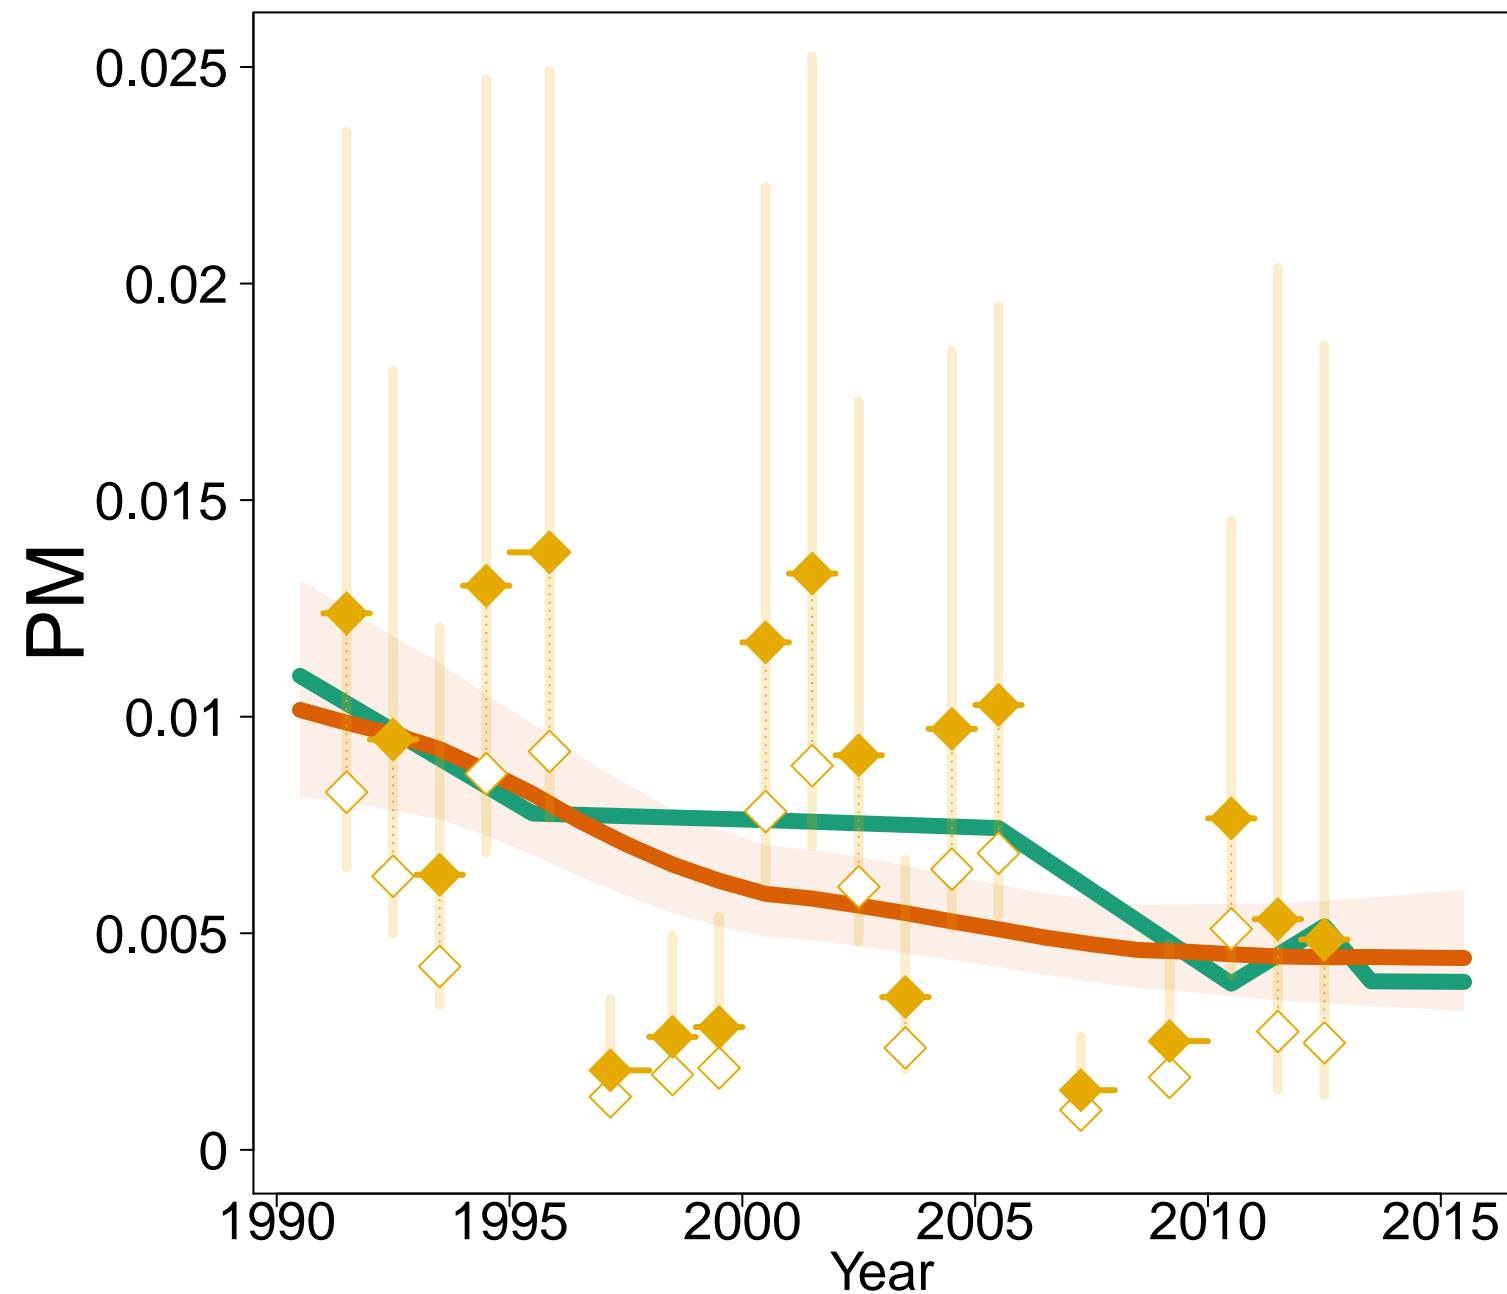

TFYR Macedonia [MKD; A]  
(Transition countries of South-Eastern Europe)

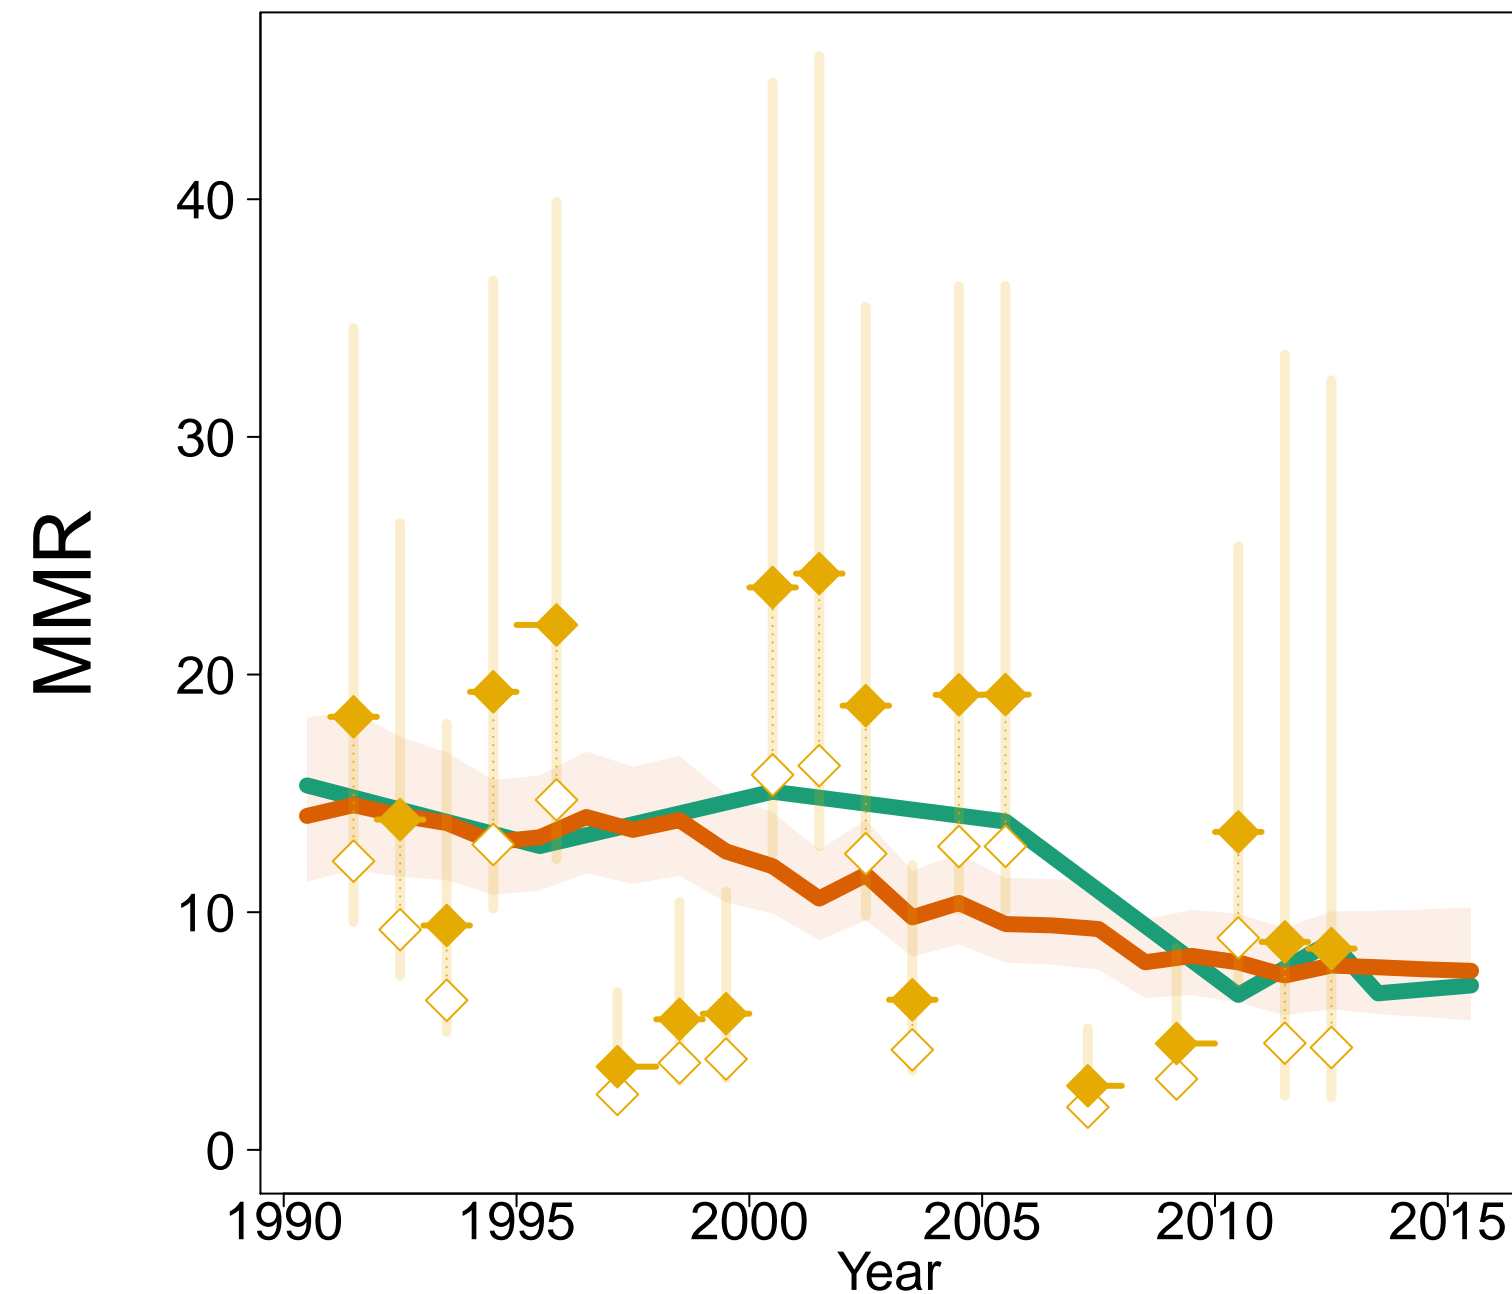

– Estimates –  
Bmat 2014  
MMEIG 2014  
– Data –  
Observed Data  
Adjusted Data  
– Data type –  
VR

Thailand [THA; B]  
(South-Eastern Asia / Oceania)

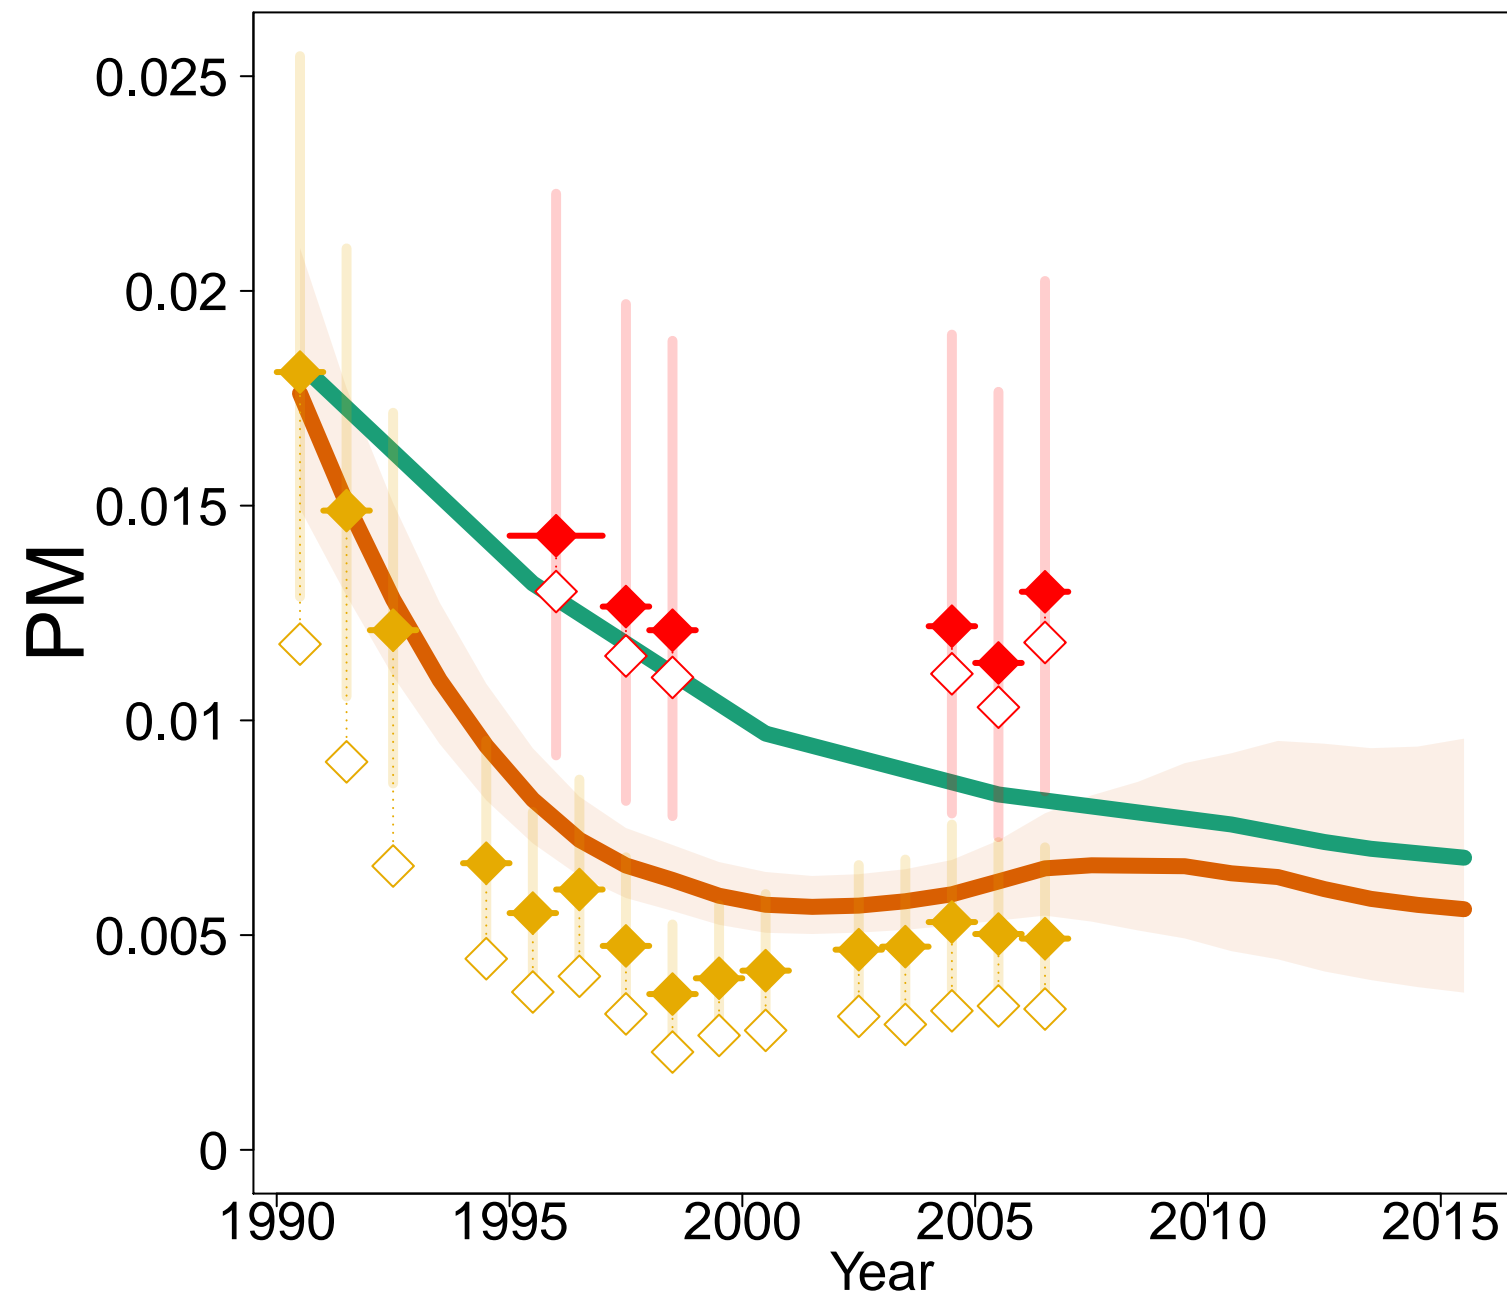

Thailand [THA; B]  
(South-Eastern Asia / Oceania)

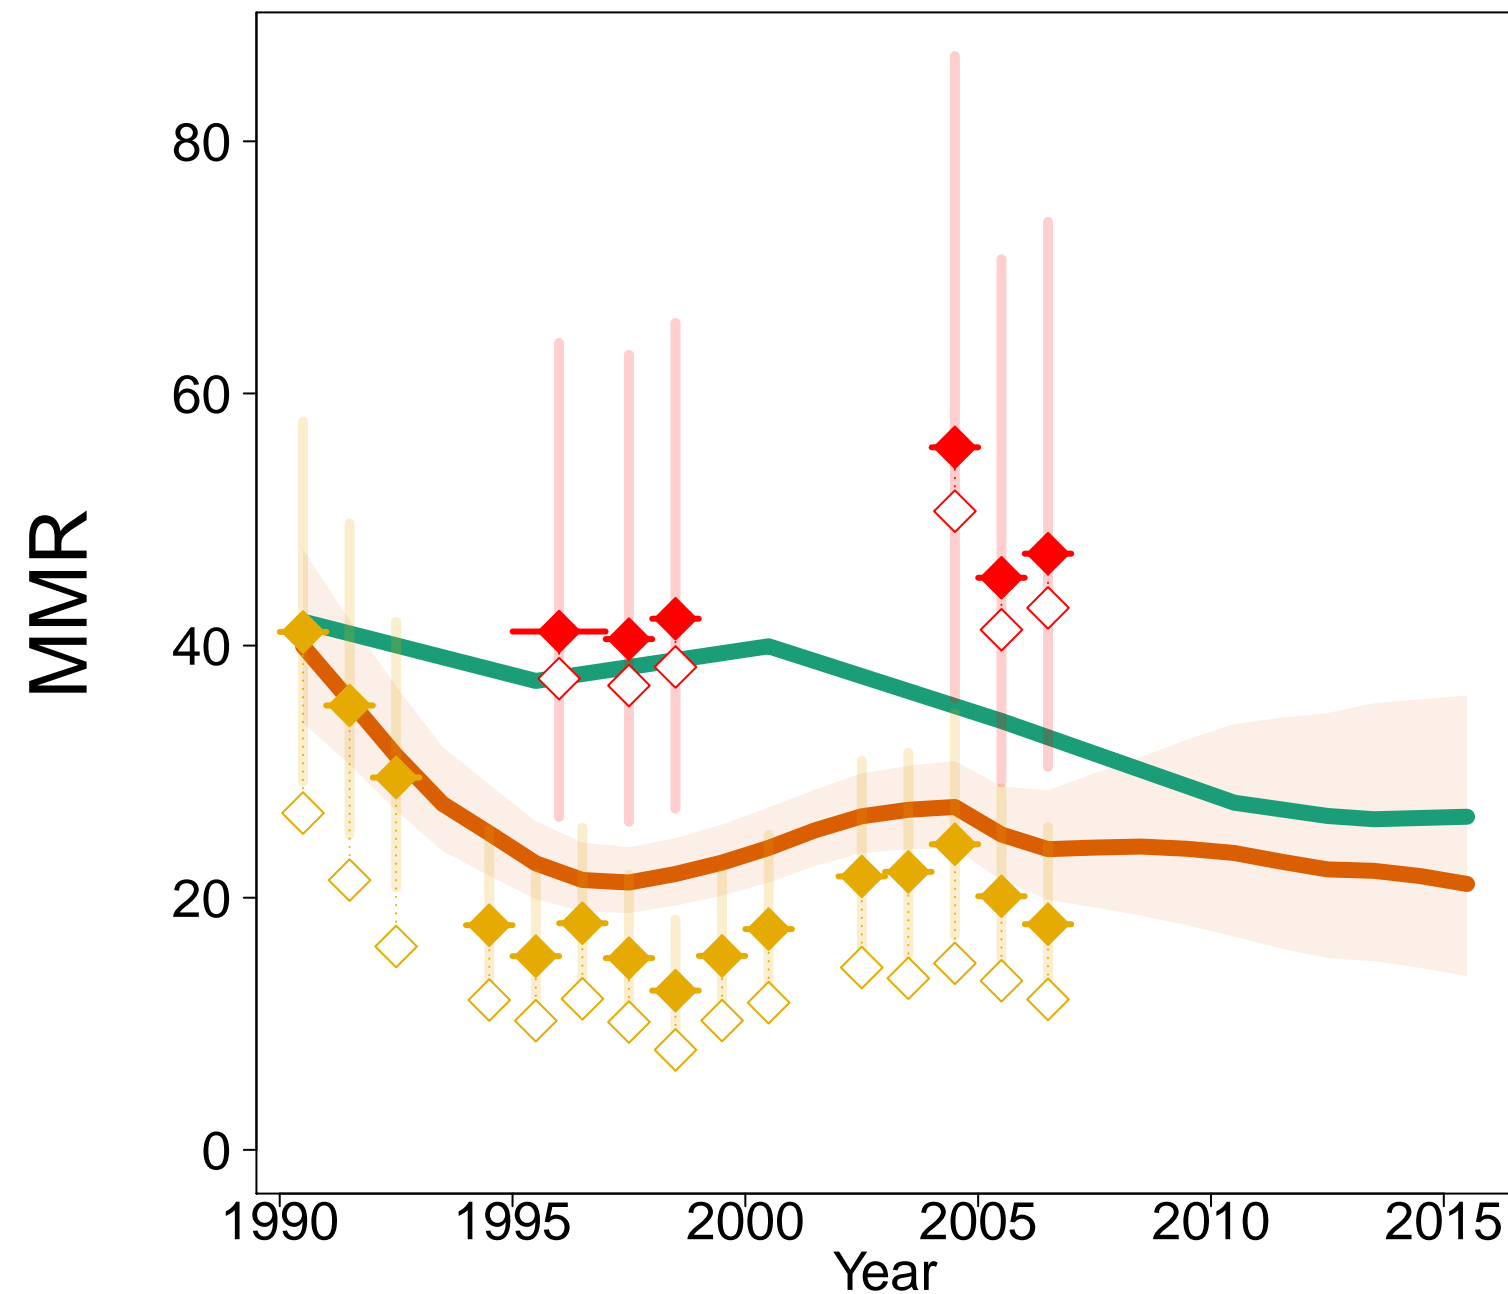

- Estimates –
- Bmat 2014
- MMEIG 2014
- Data –
- Observed Data
- Adjusted Data
- Data type –
- VR
- Misc. studies

Timor-Leste [TLS; B]  
(South-Eastern Asia / Oceania)

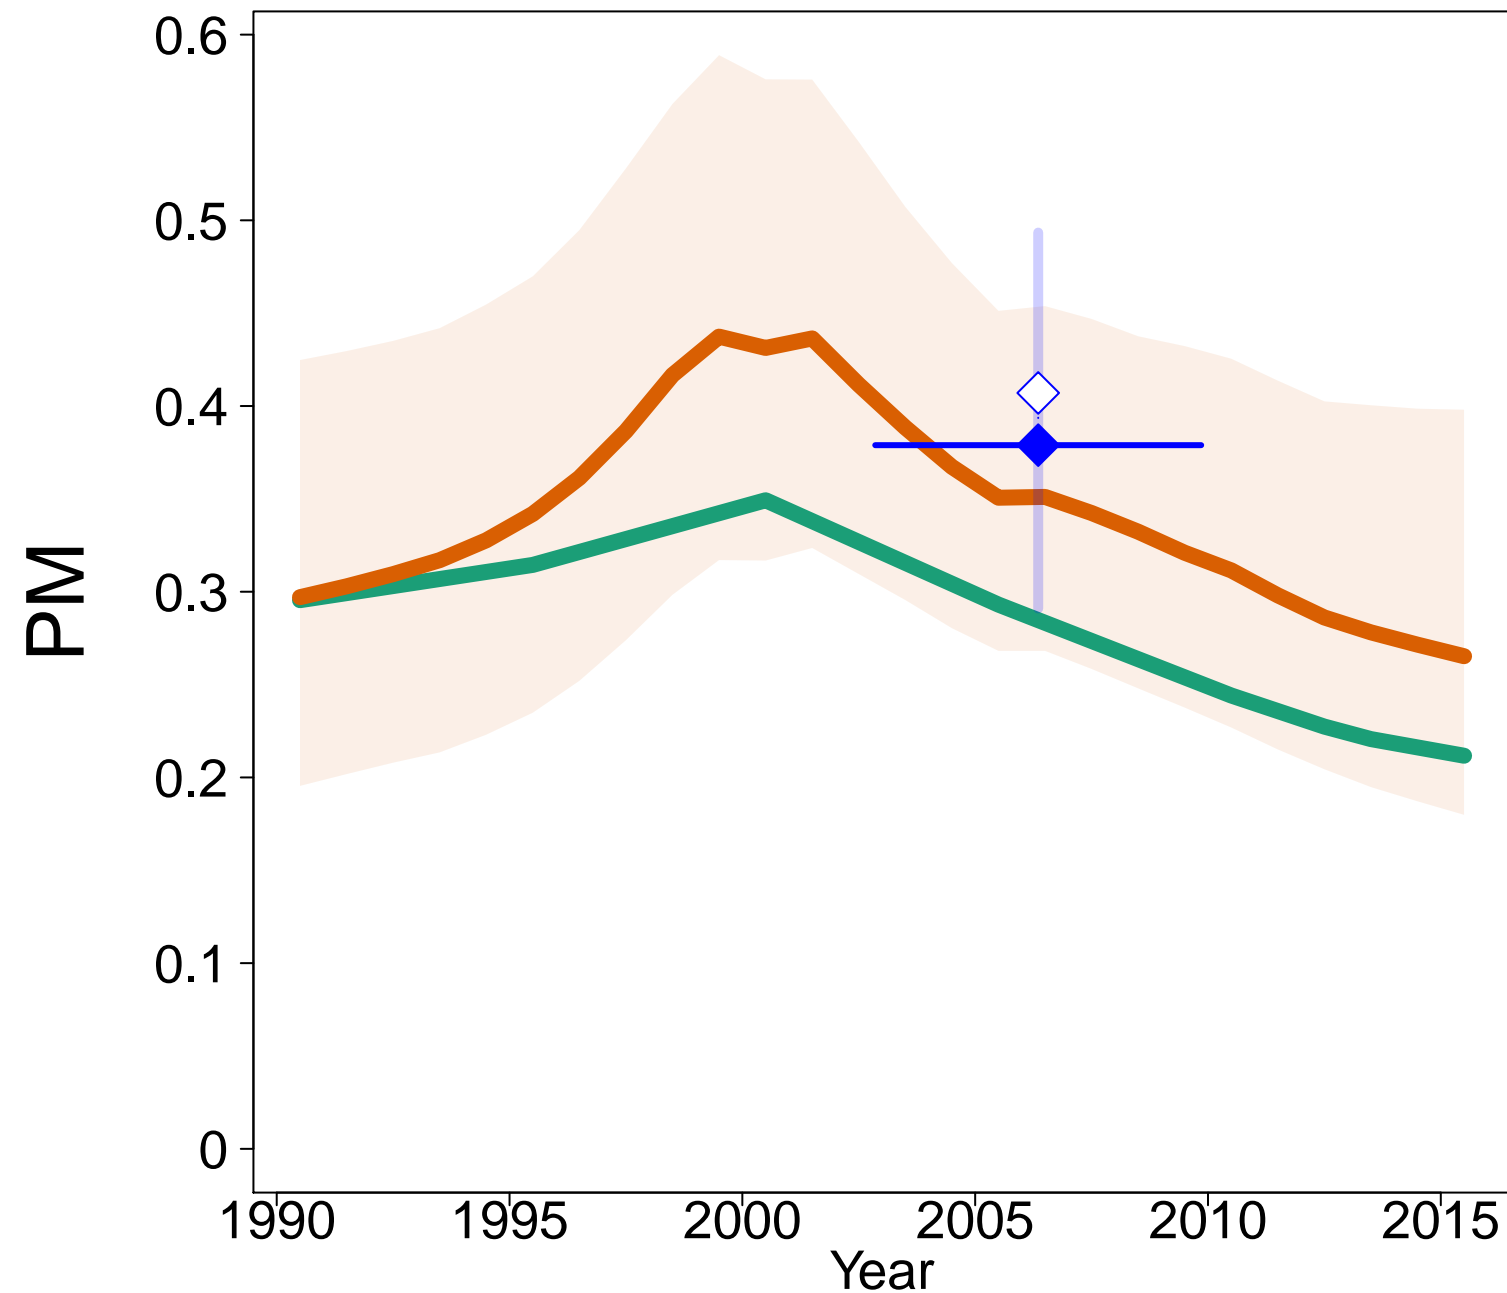

Timor-Leste [TLS; B]  
(South-Eastern Asia / Oceania)

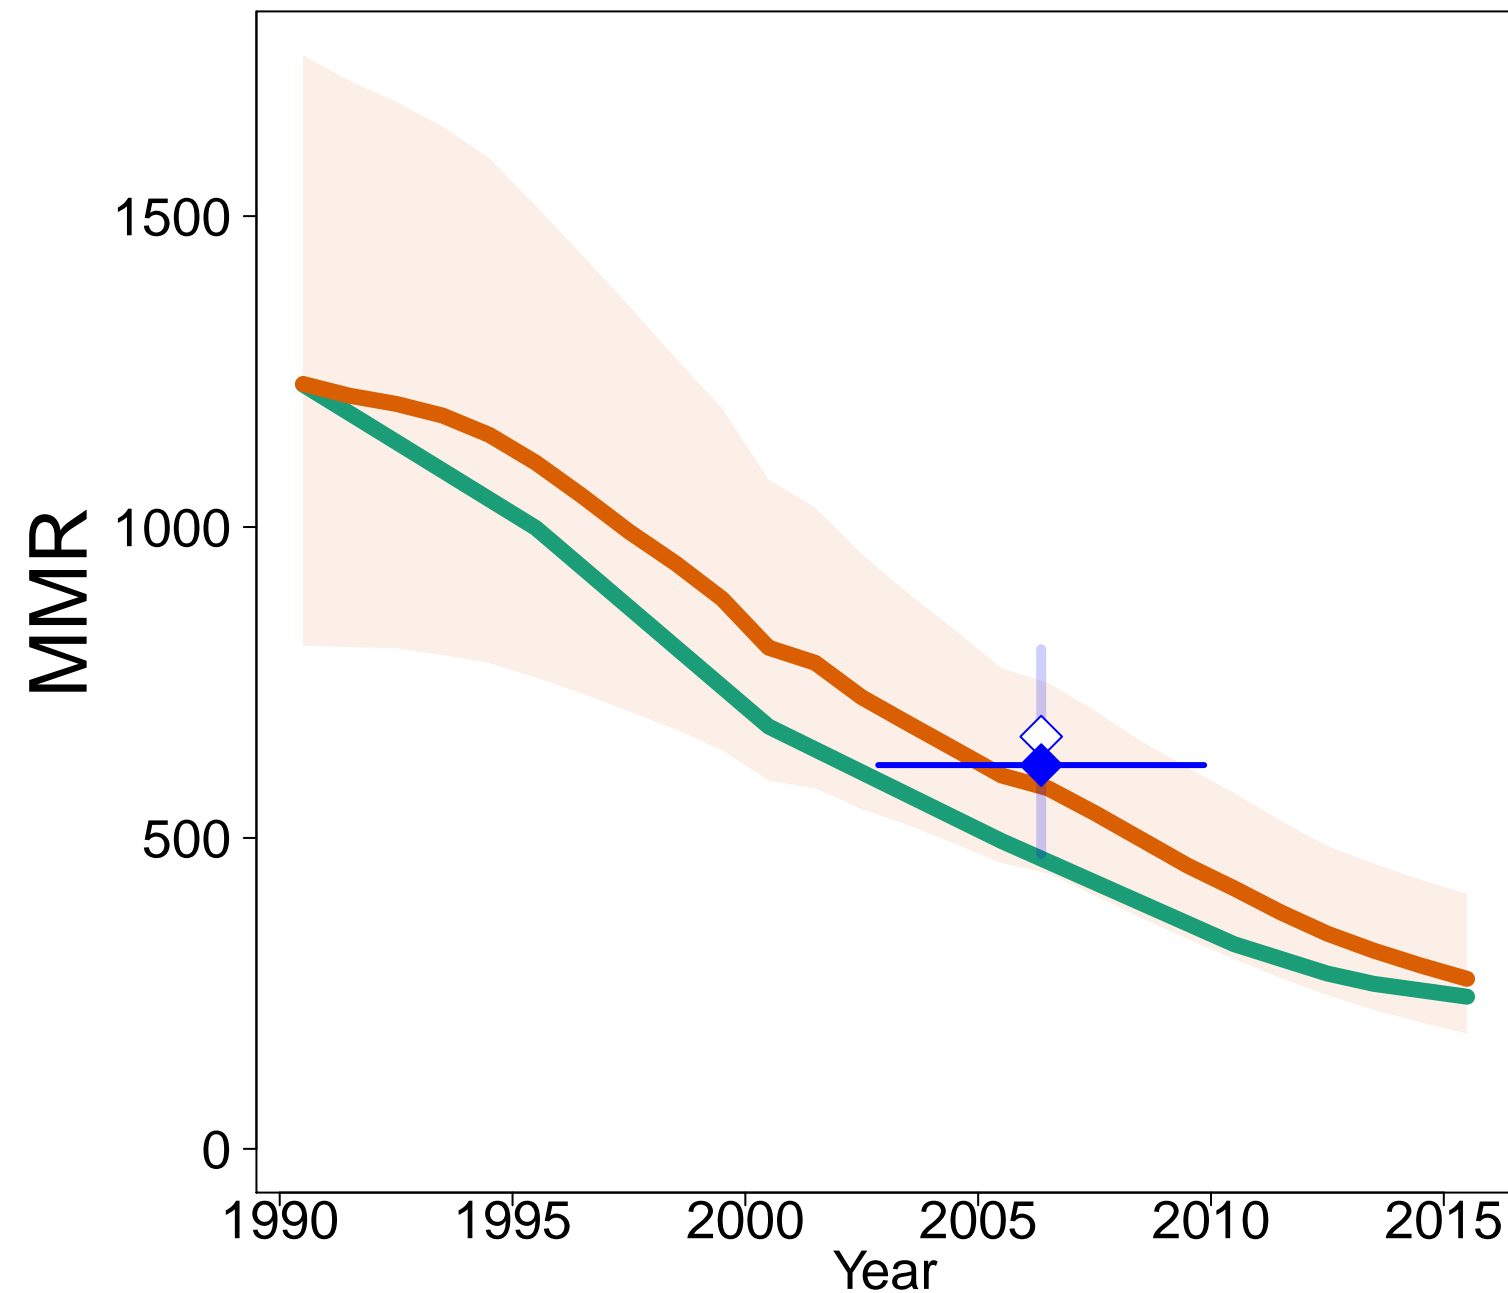

– Estimates –  
Bmat 2014  
MMEIG 2014  
– Data –  
Observed Data  
Adjusted Data  
– Data type –  
DHS

Togo [TGO; B]  
(Western Africa)

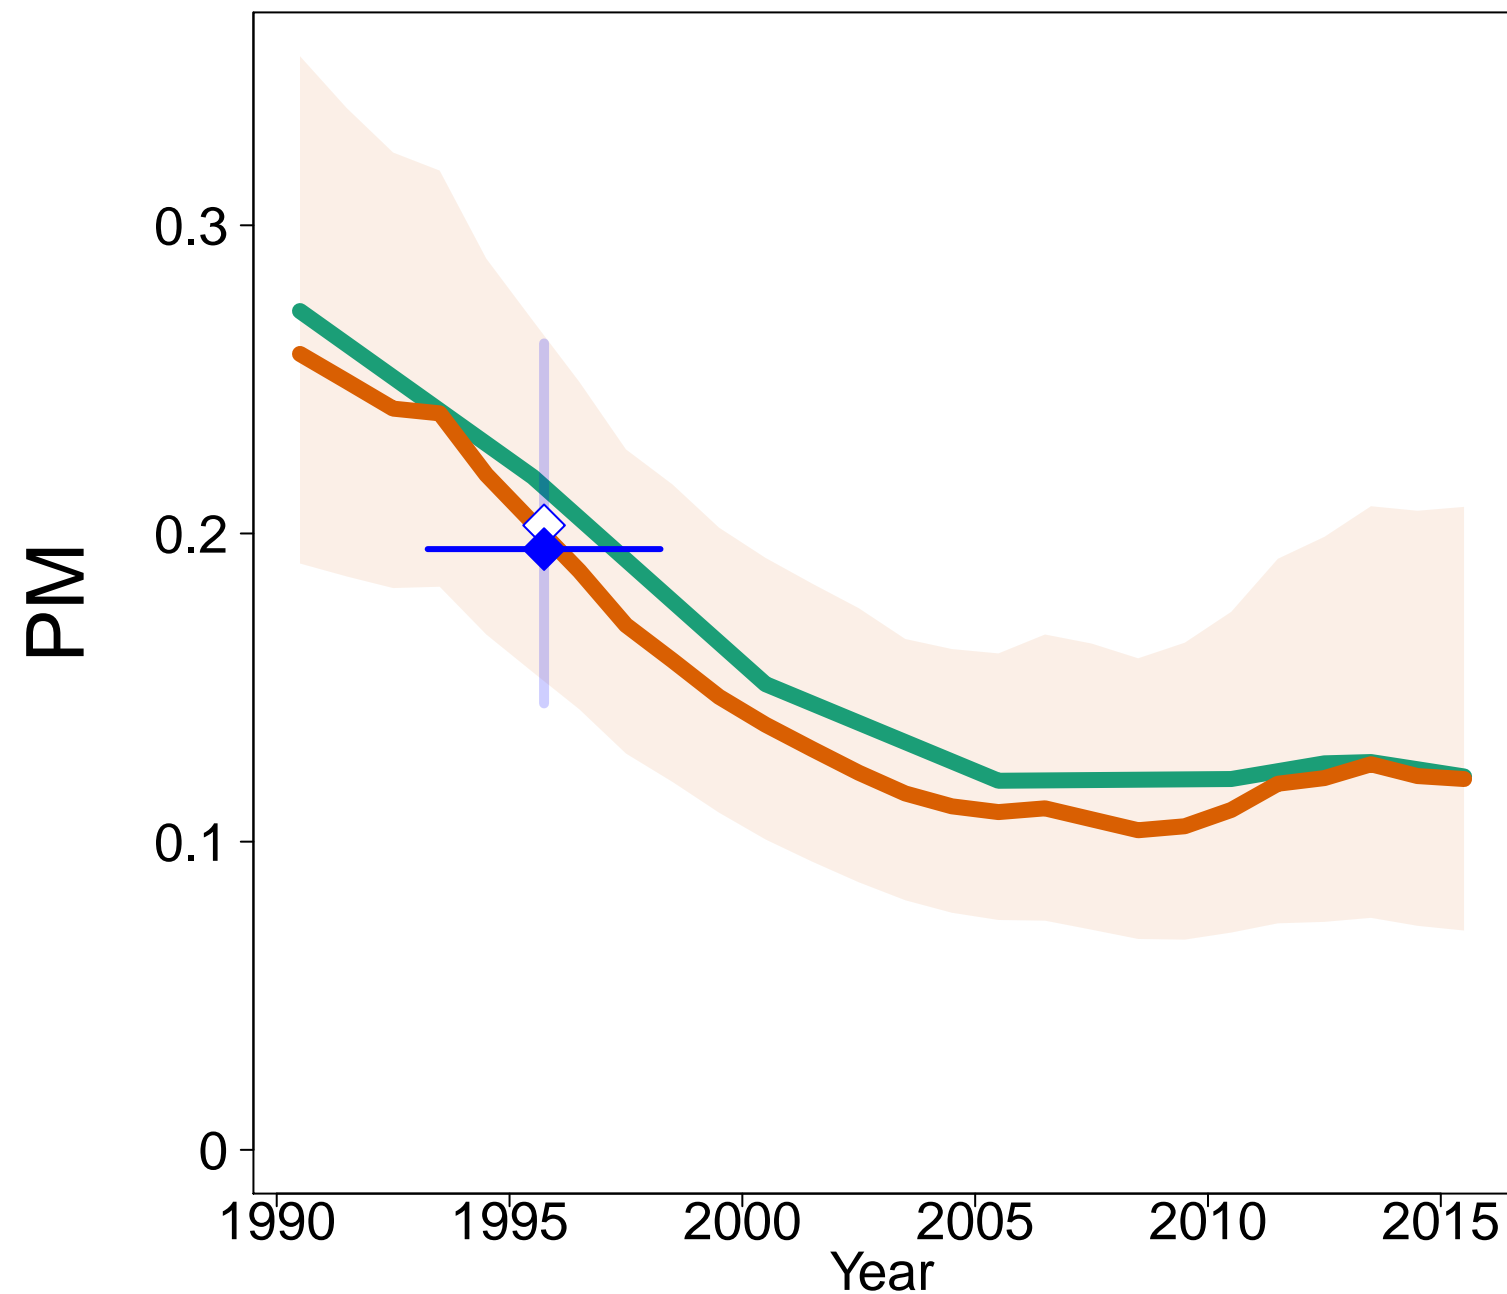

Togo [TGO; B]  
(Western Africa)

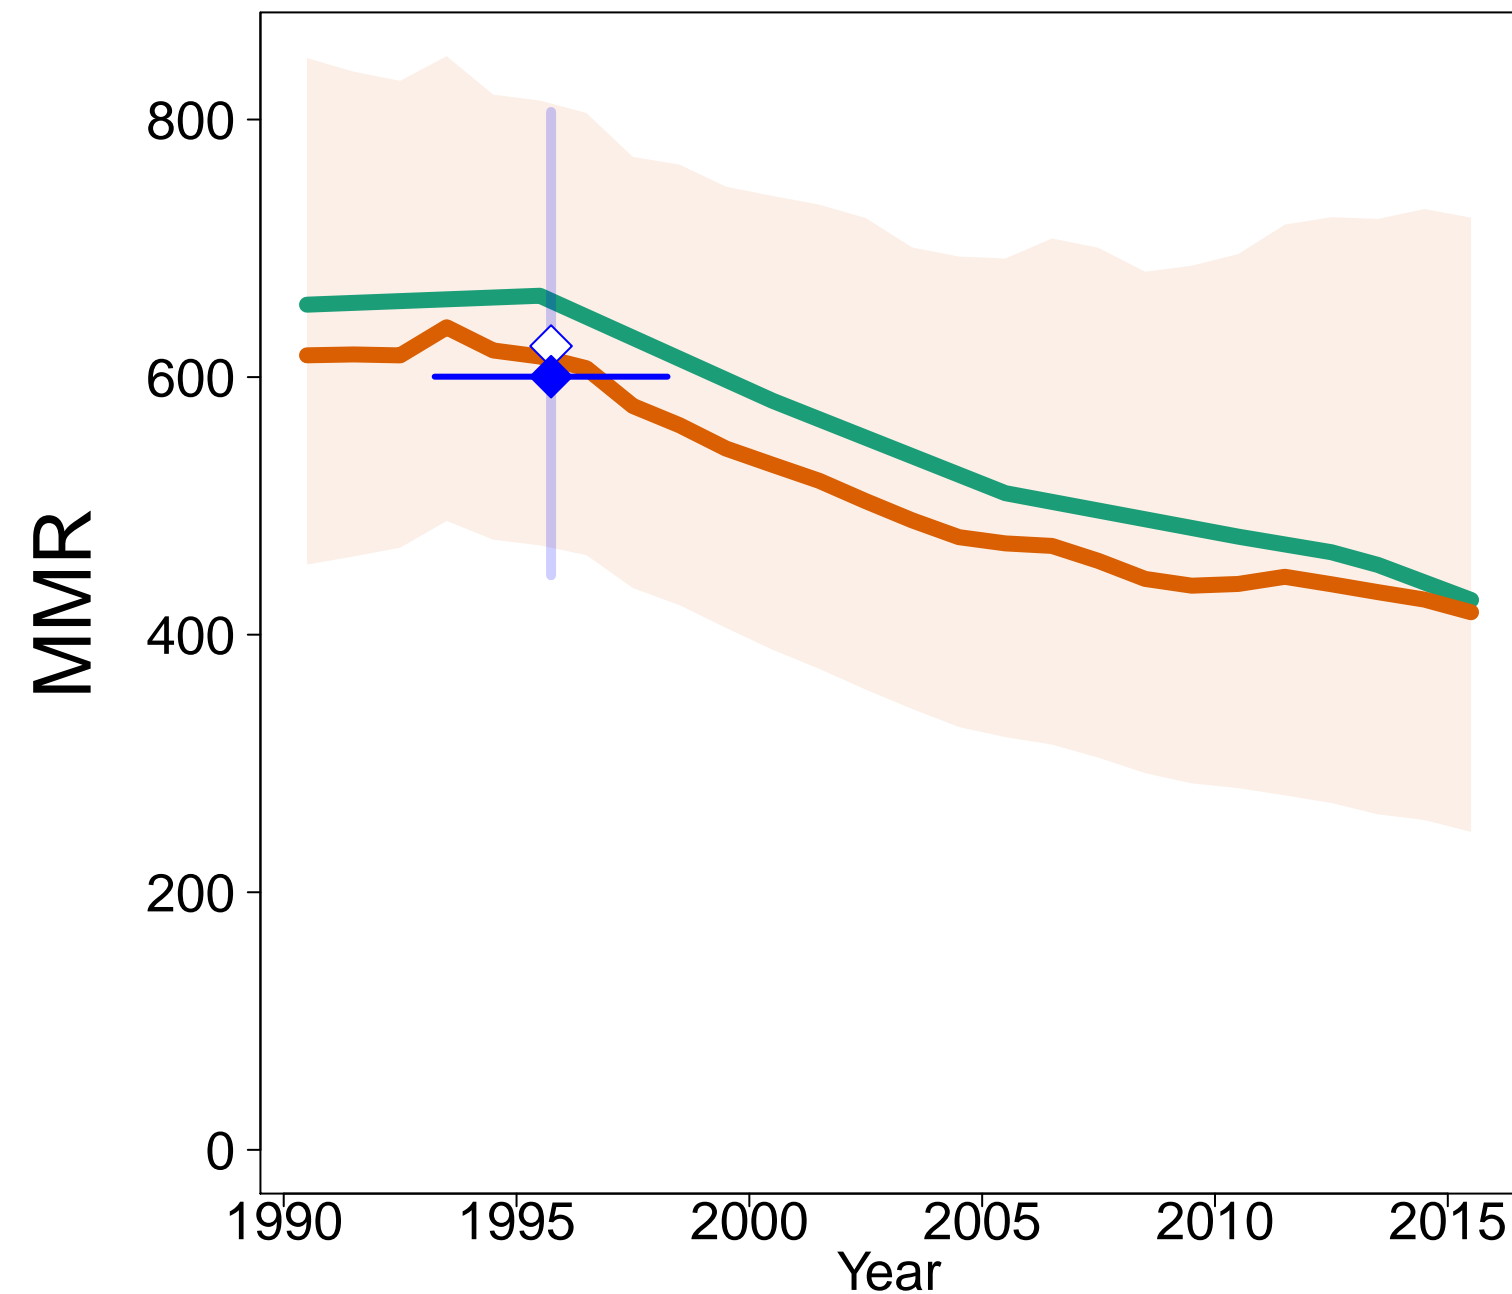

- Estimates –
- Bmat 2014
- MMEIG 2014
- Data –
- Observed Data
- Adjusted Data
- Data type –
- DHS

Tonga [TON; C]  
(South-Eastern Asia / Oceania)

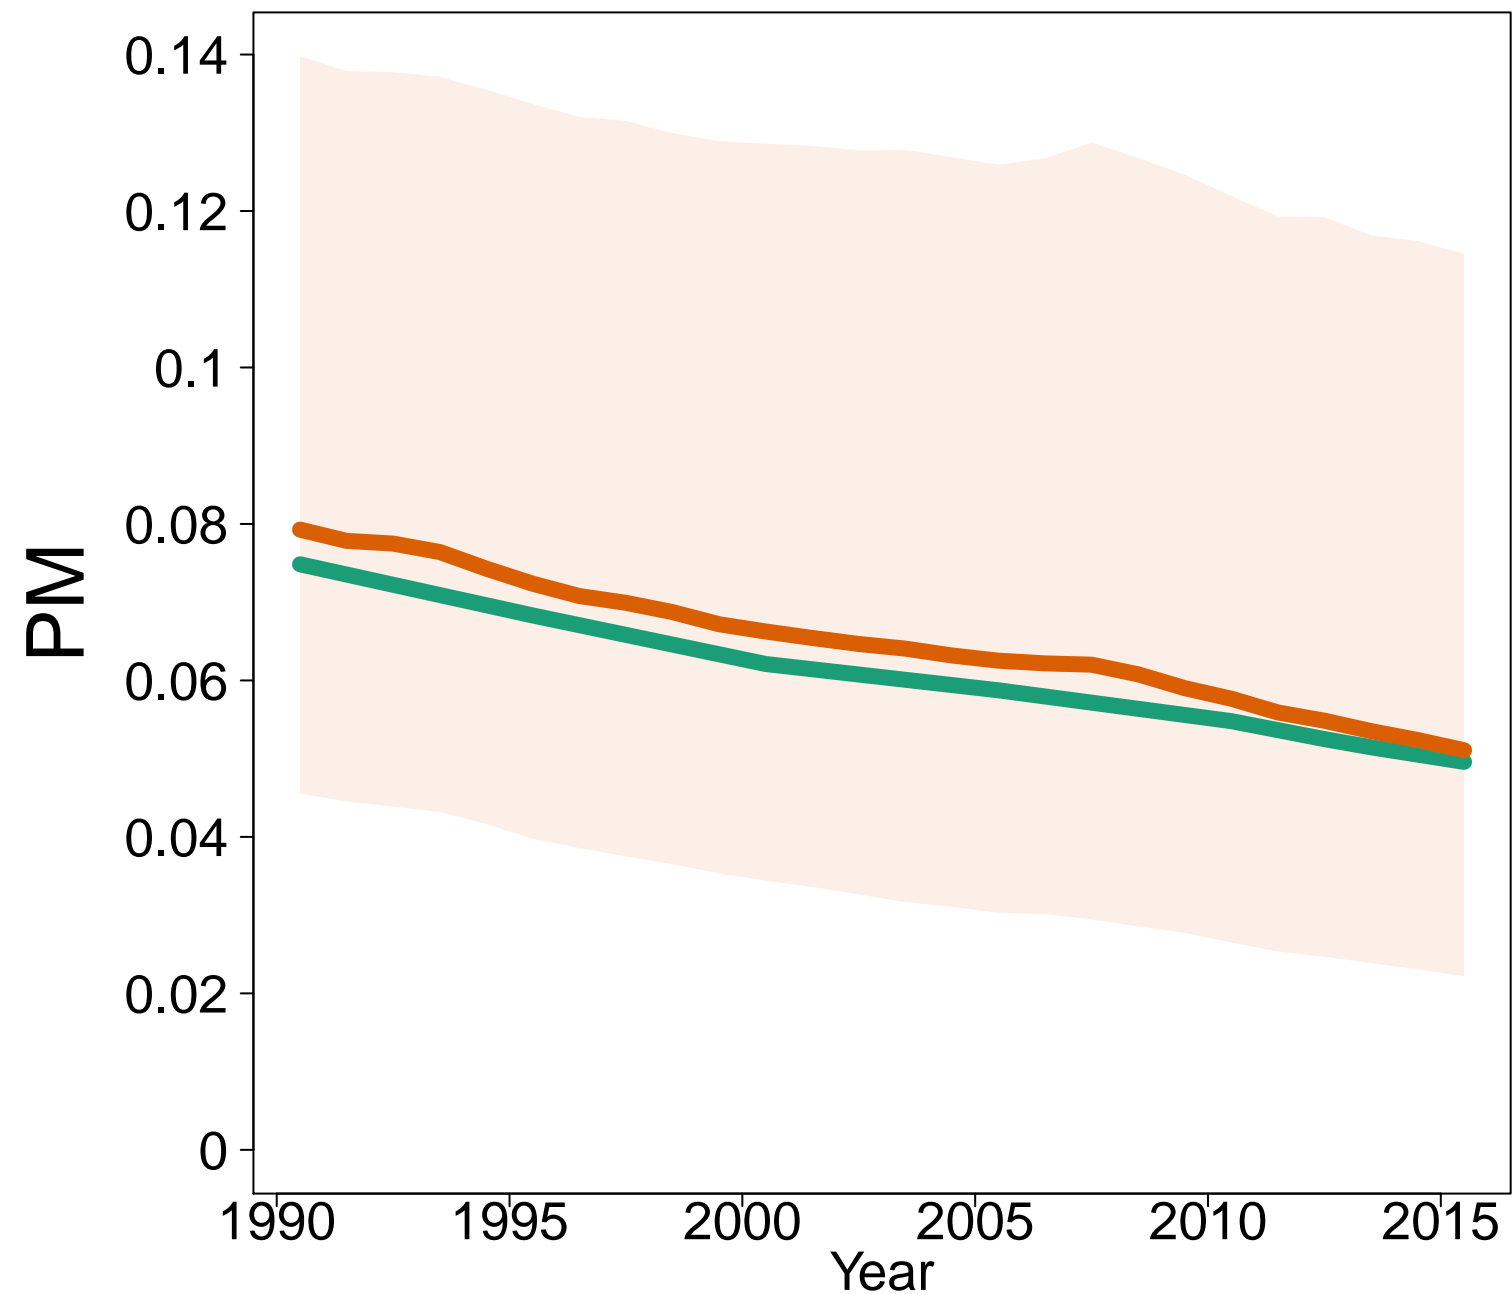

Tonga [TON; C]  
(South-Eastern Asia / Oceania)

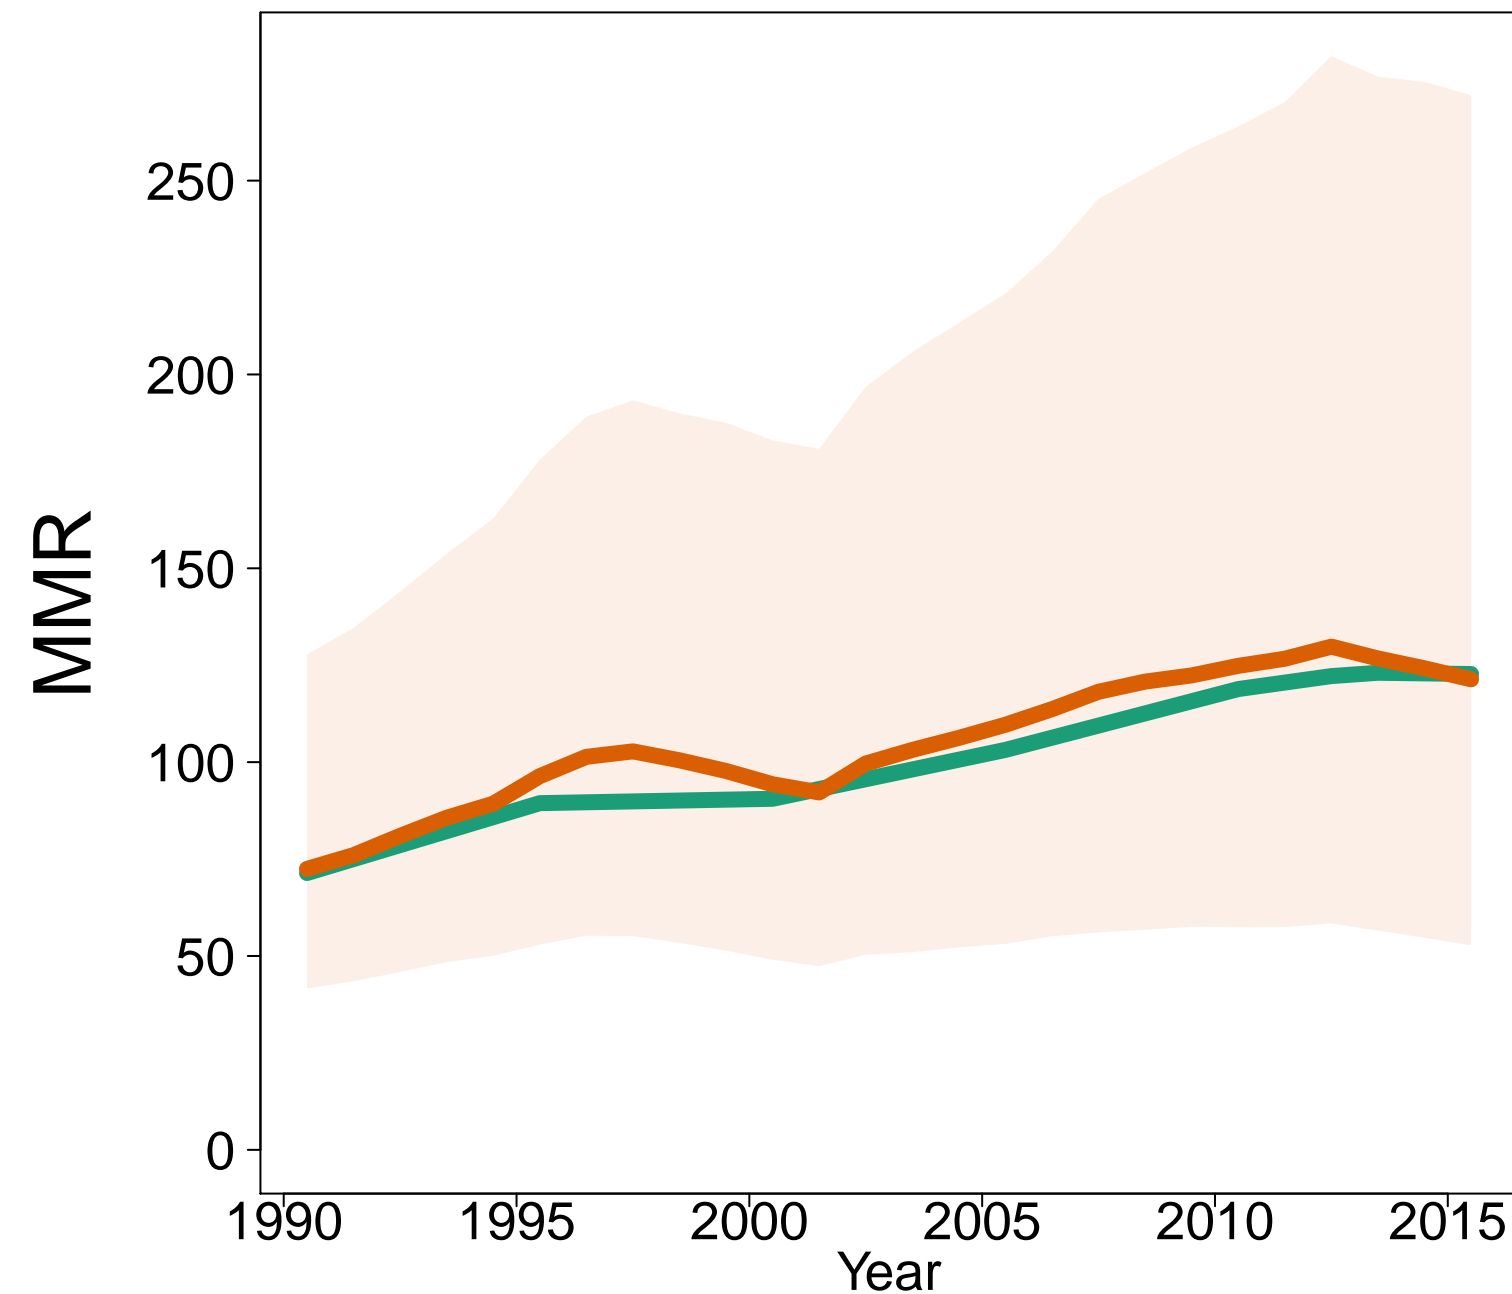

– Estimates –  
Bmat 2014  
MMEIG 2014  
– Data –

Trinidad and Tobago [TTO; A]  
(Caribbean)

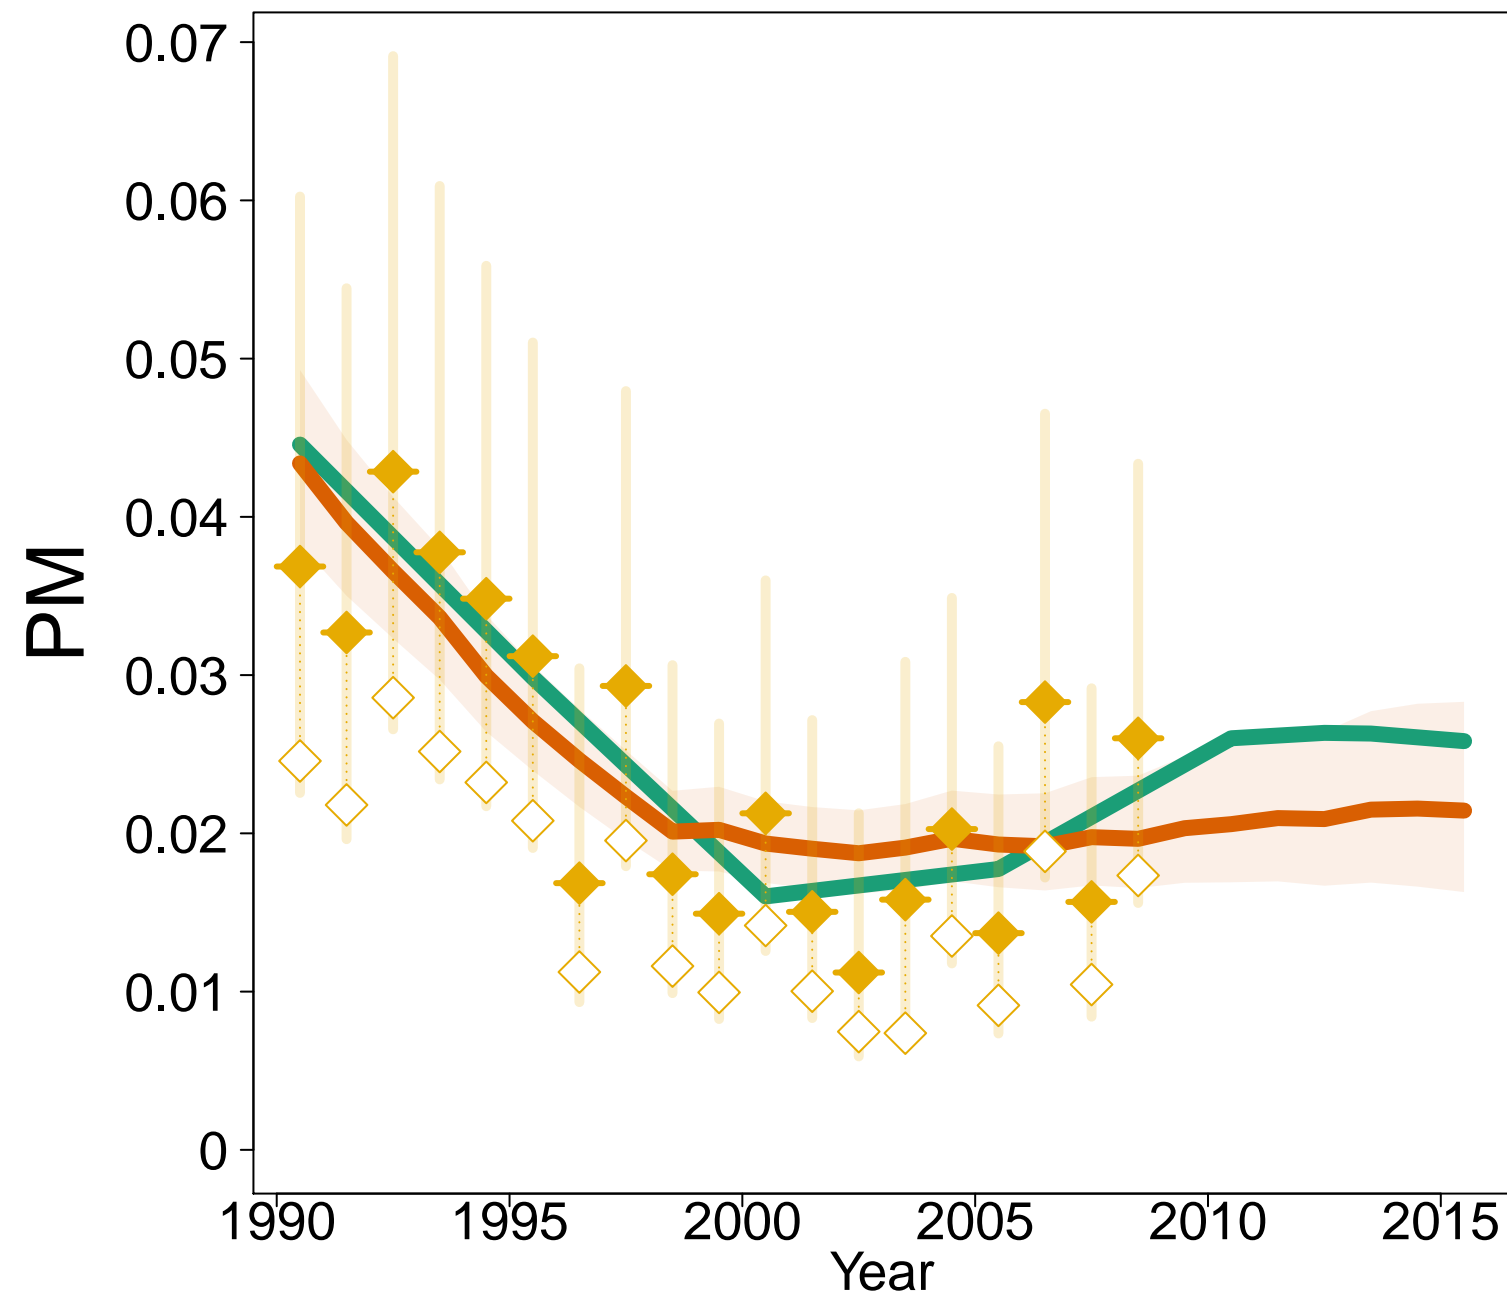

Trinidad and Tobago [TTO; A]  
(Caribbean)

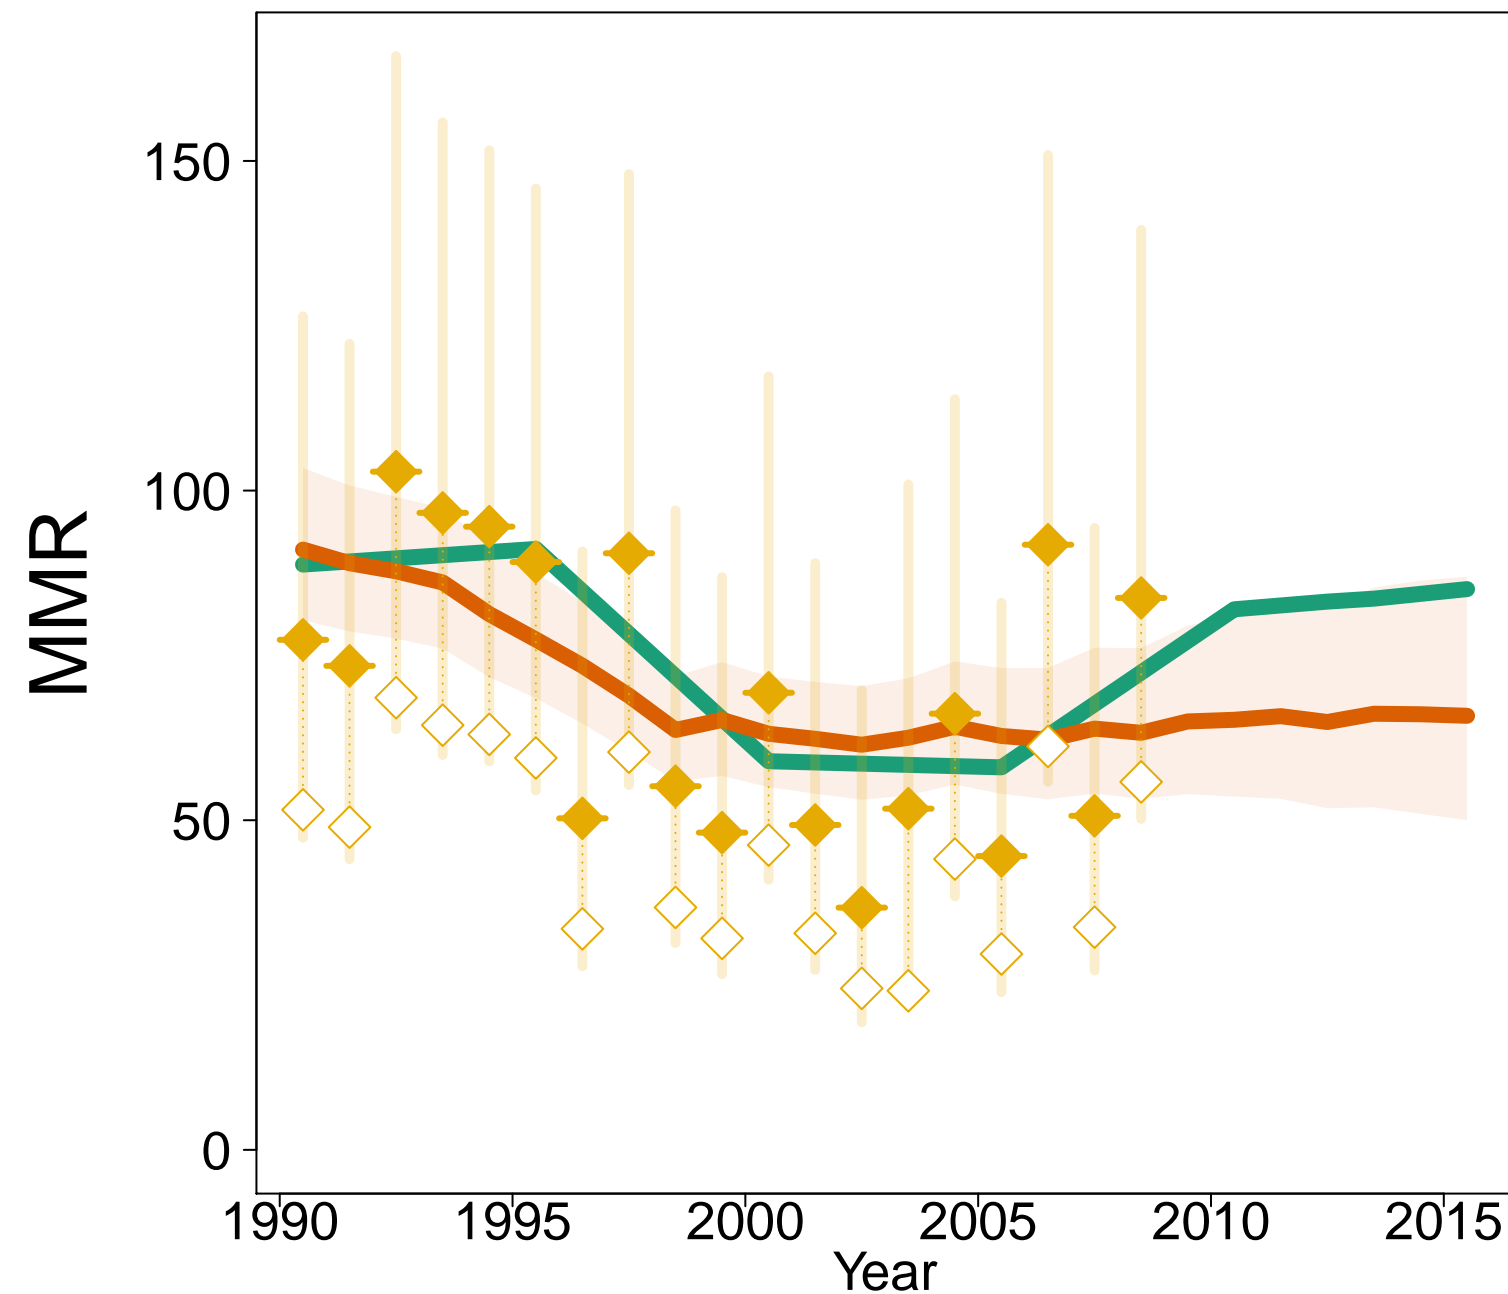

- Estimates –
- Bmat 2014
- MMEIG 2014
- Data –
- Observed Data
- Adjusted Data
- Data type –
- VR

Tunisia [TUN; B]  
(Northern Africa)

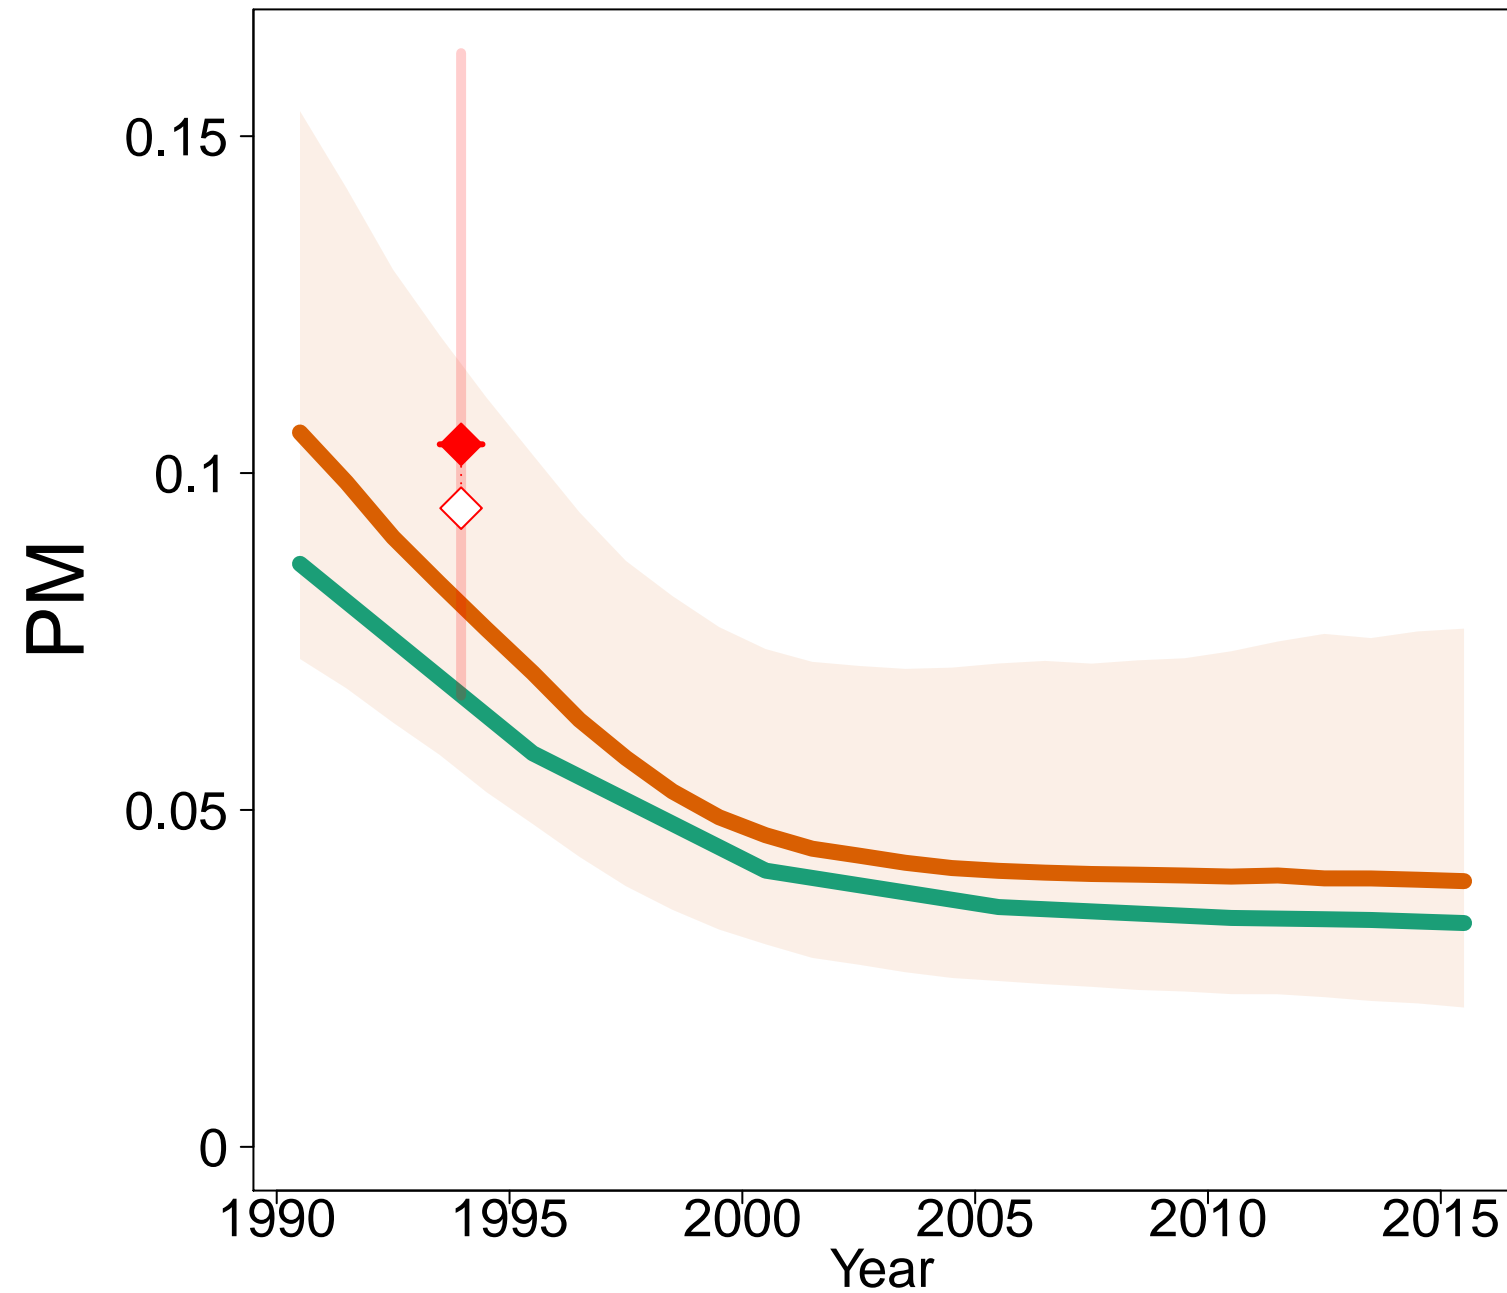

Tunisia [TUN; B]  
(Northern Africa)

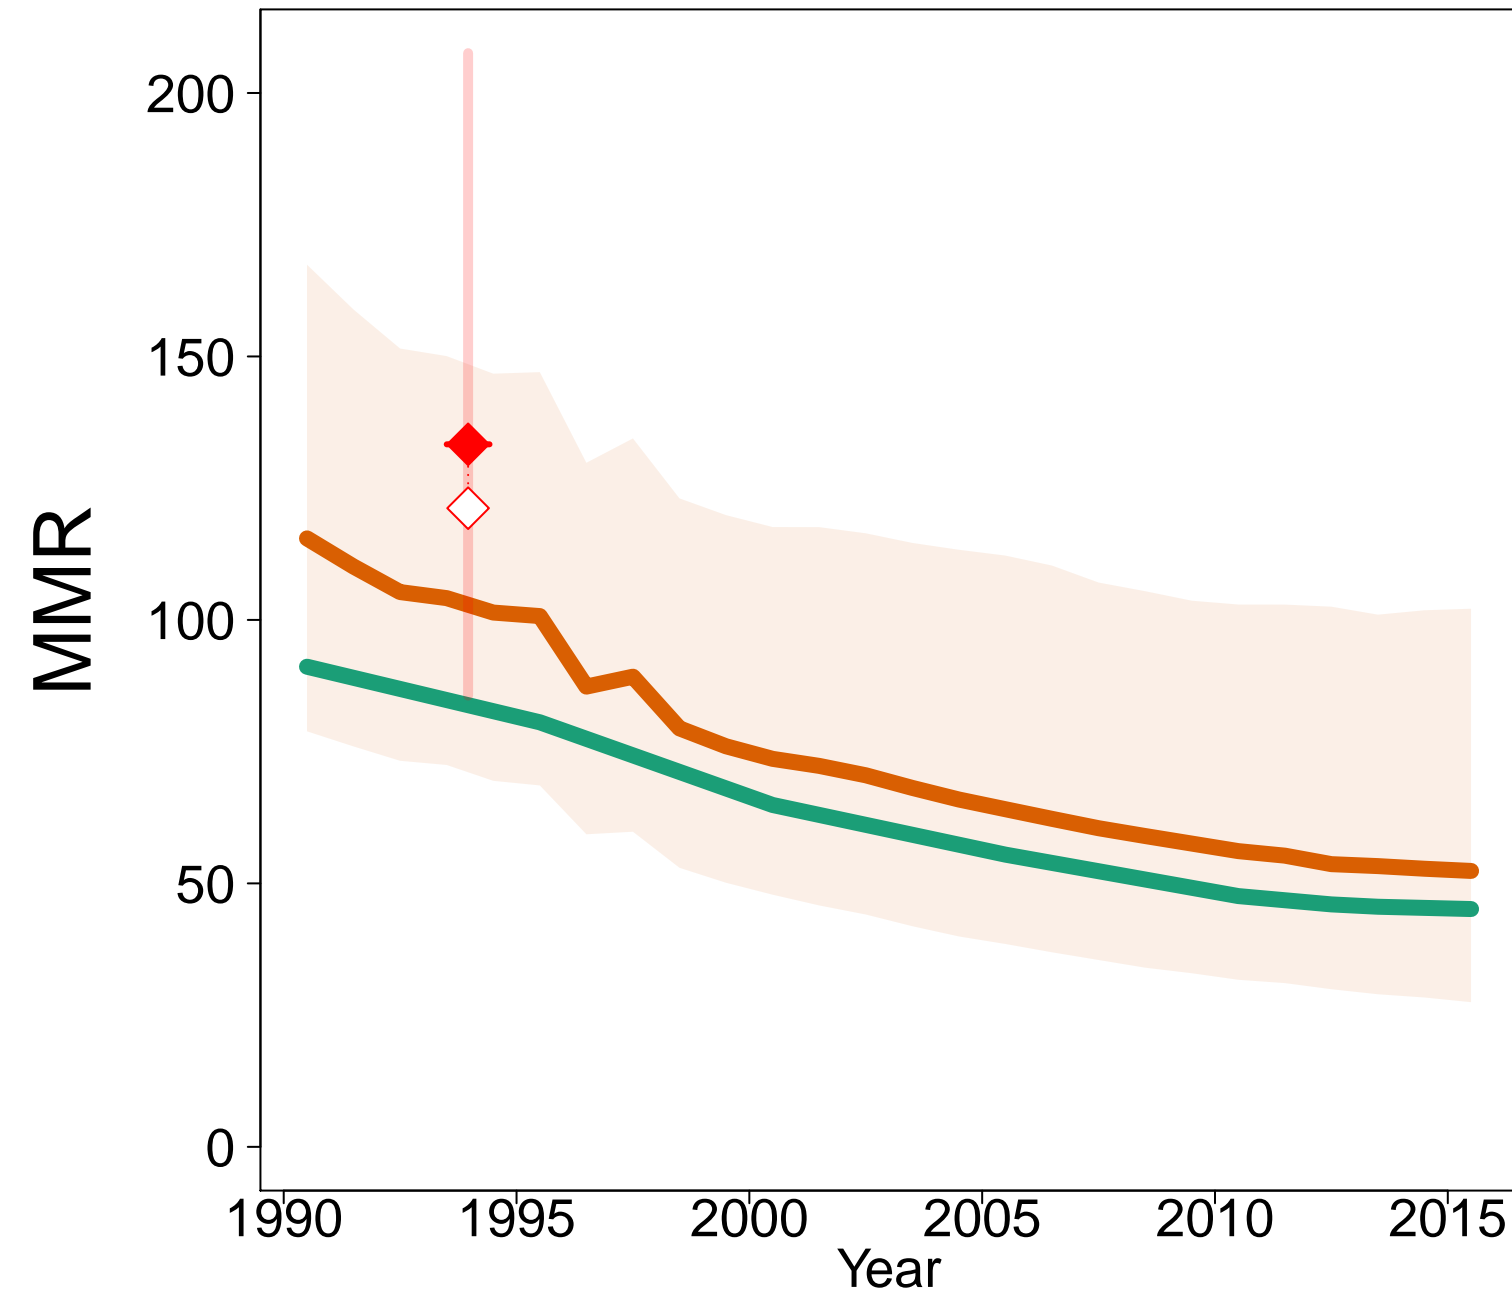

- Estimates –
- Bmat 2014
- MMEIG 2014
- Data –
- ◊ Observed Data
- ◆ Adjusted Data
- Data type –
- ◆ Misc. studies



Turkey [TUR; B]  
(Western Asia)

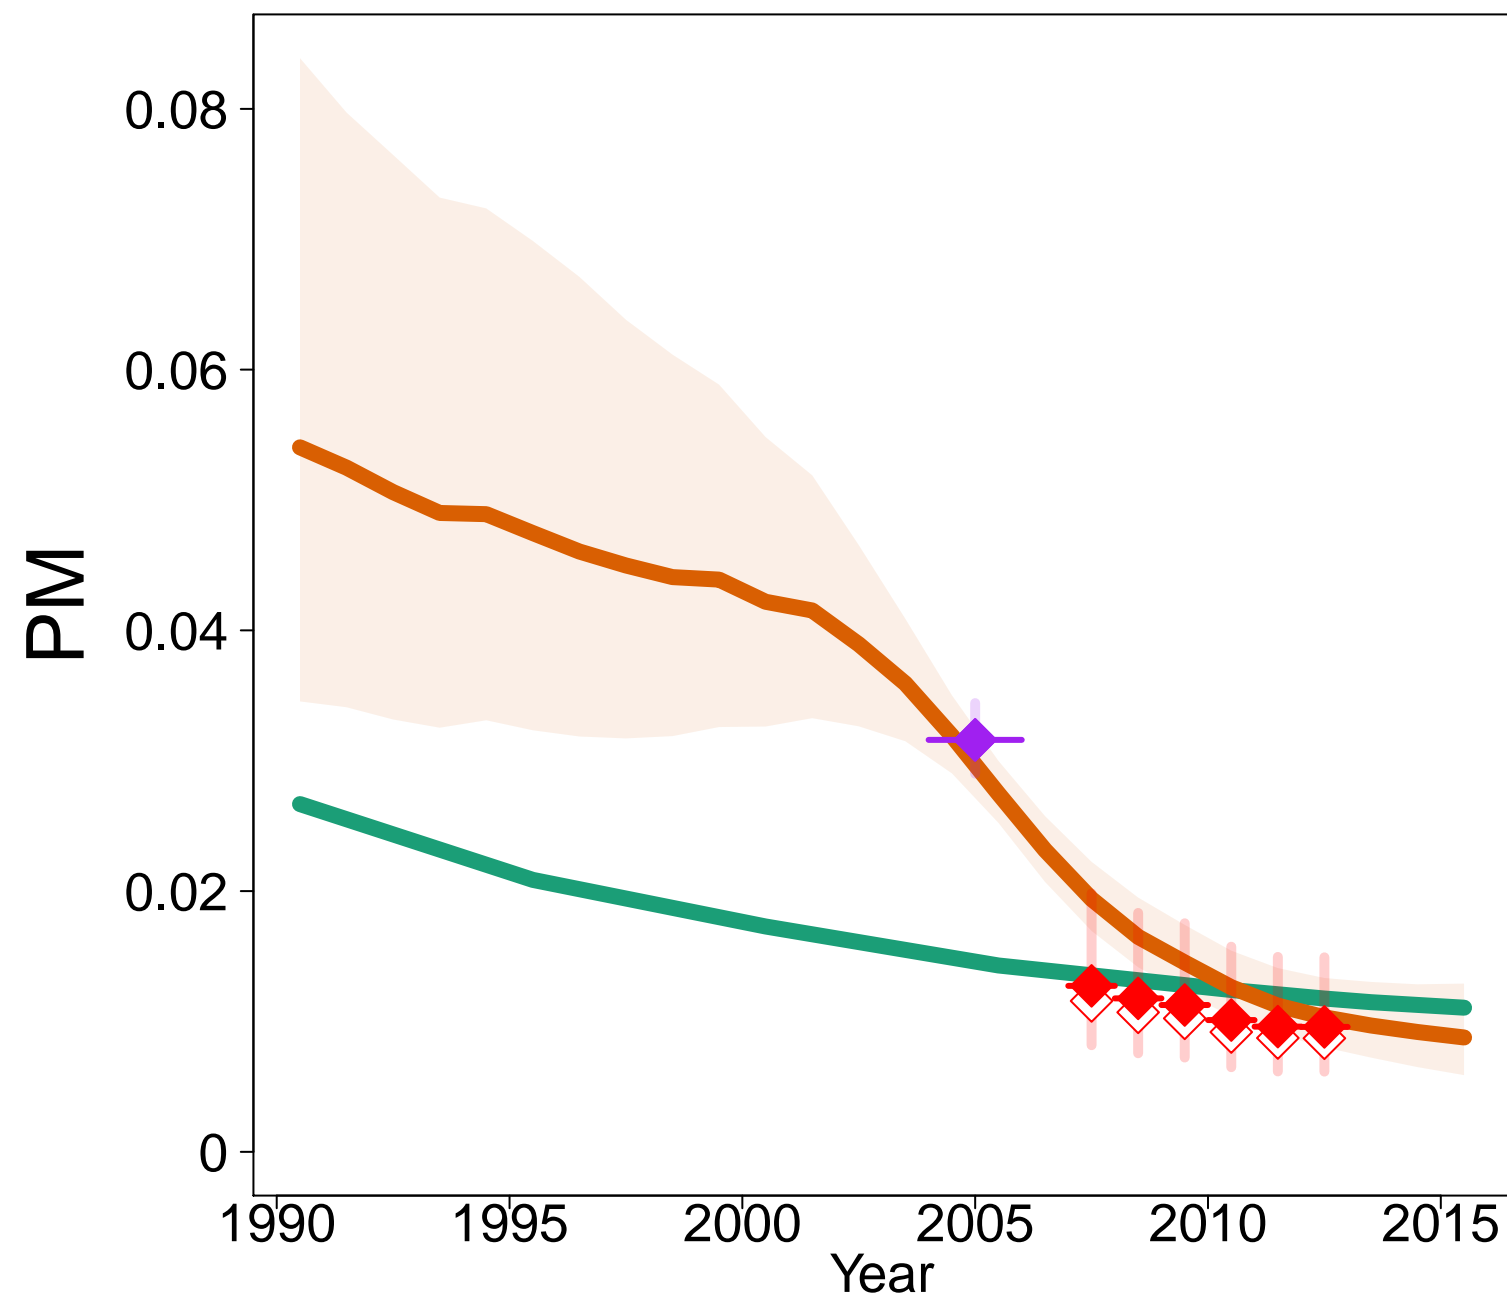

Turkey [TUR; B]  
(Western Asia)

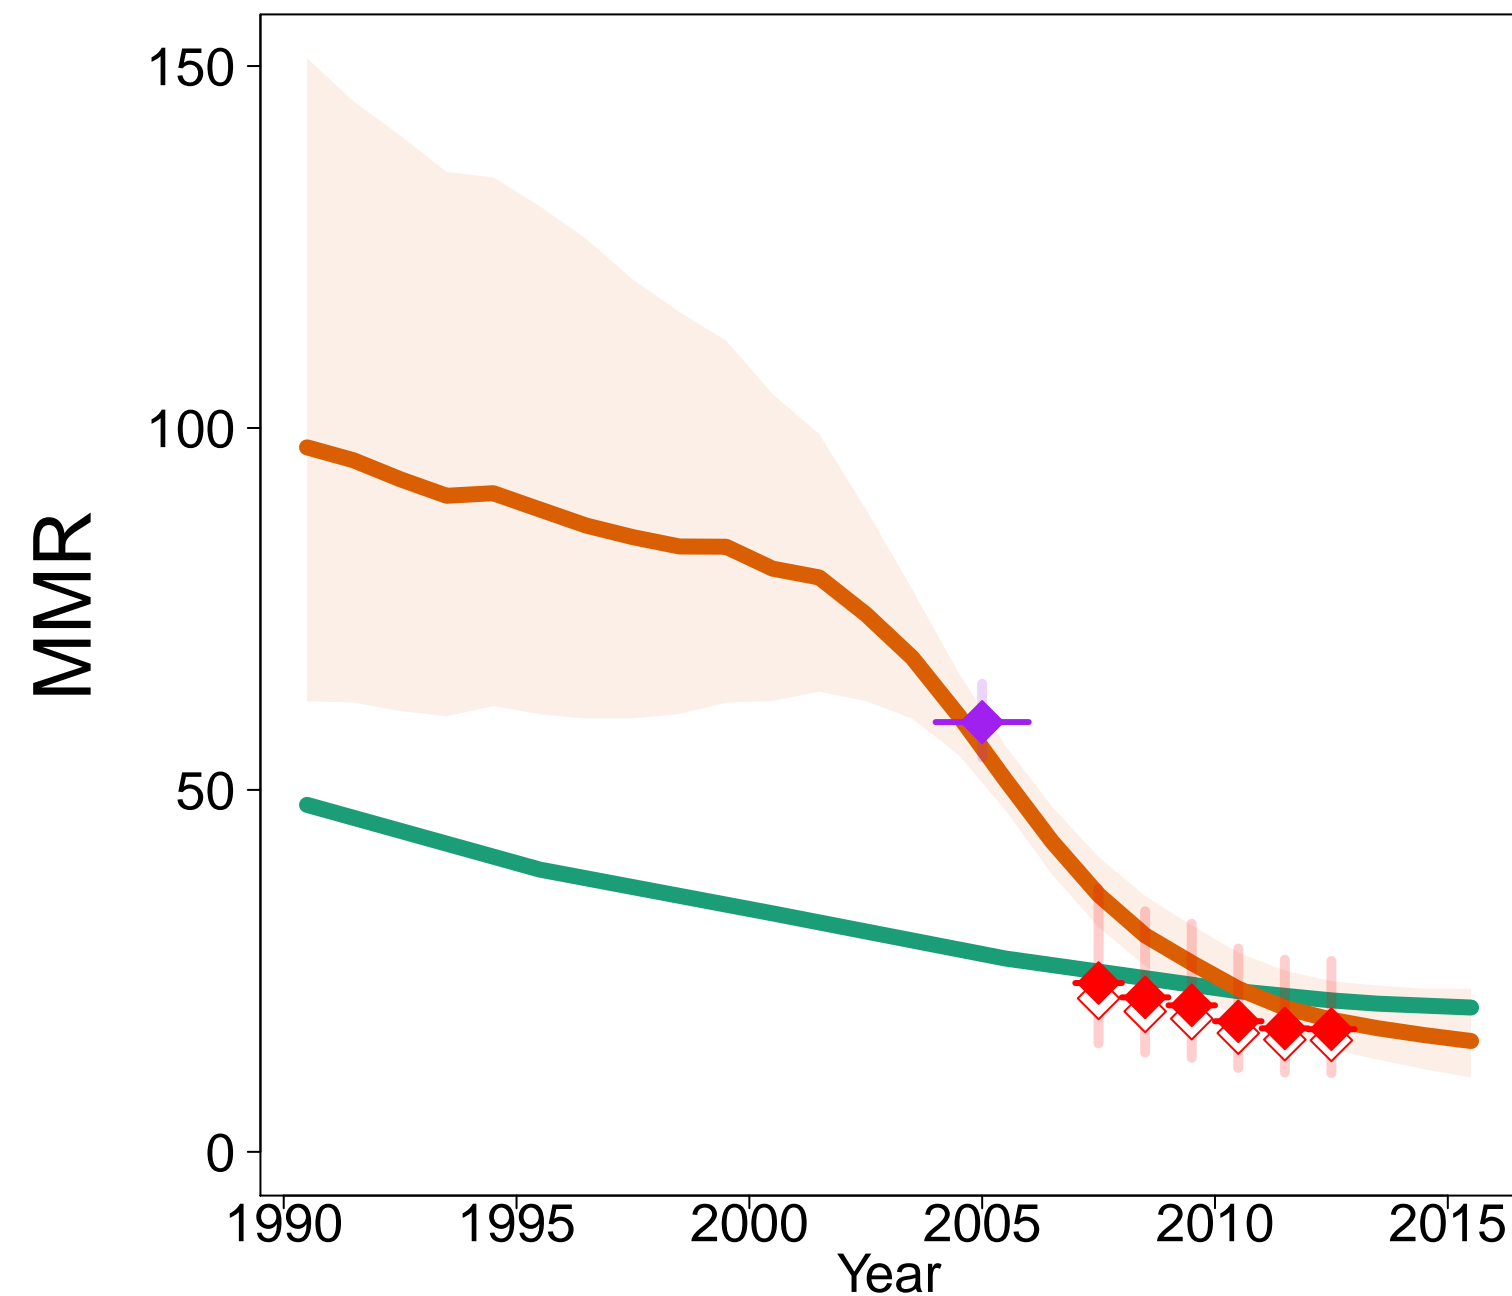

- Estimates –
- Bmat 2014
- MMEIG 2014
- Data –
- ◊ Observed Data
- ◆ Adjusted Data
- Data type –
- ◆ Spec. studies
- ◆ Misc. studies

Turkmenistan [TKM; C]  
(Central Asia)

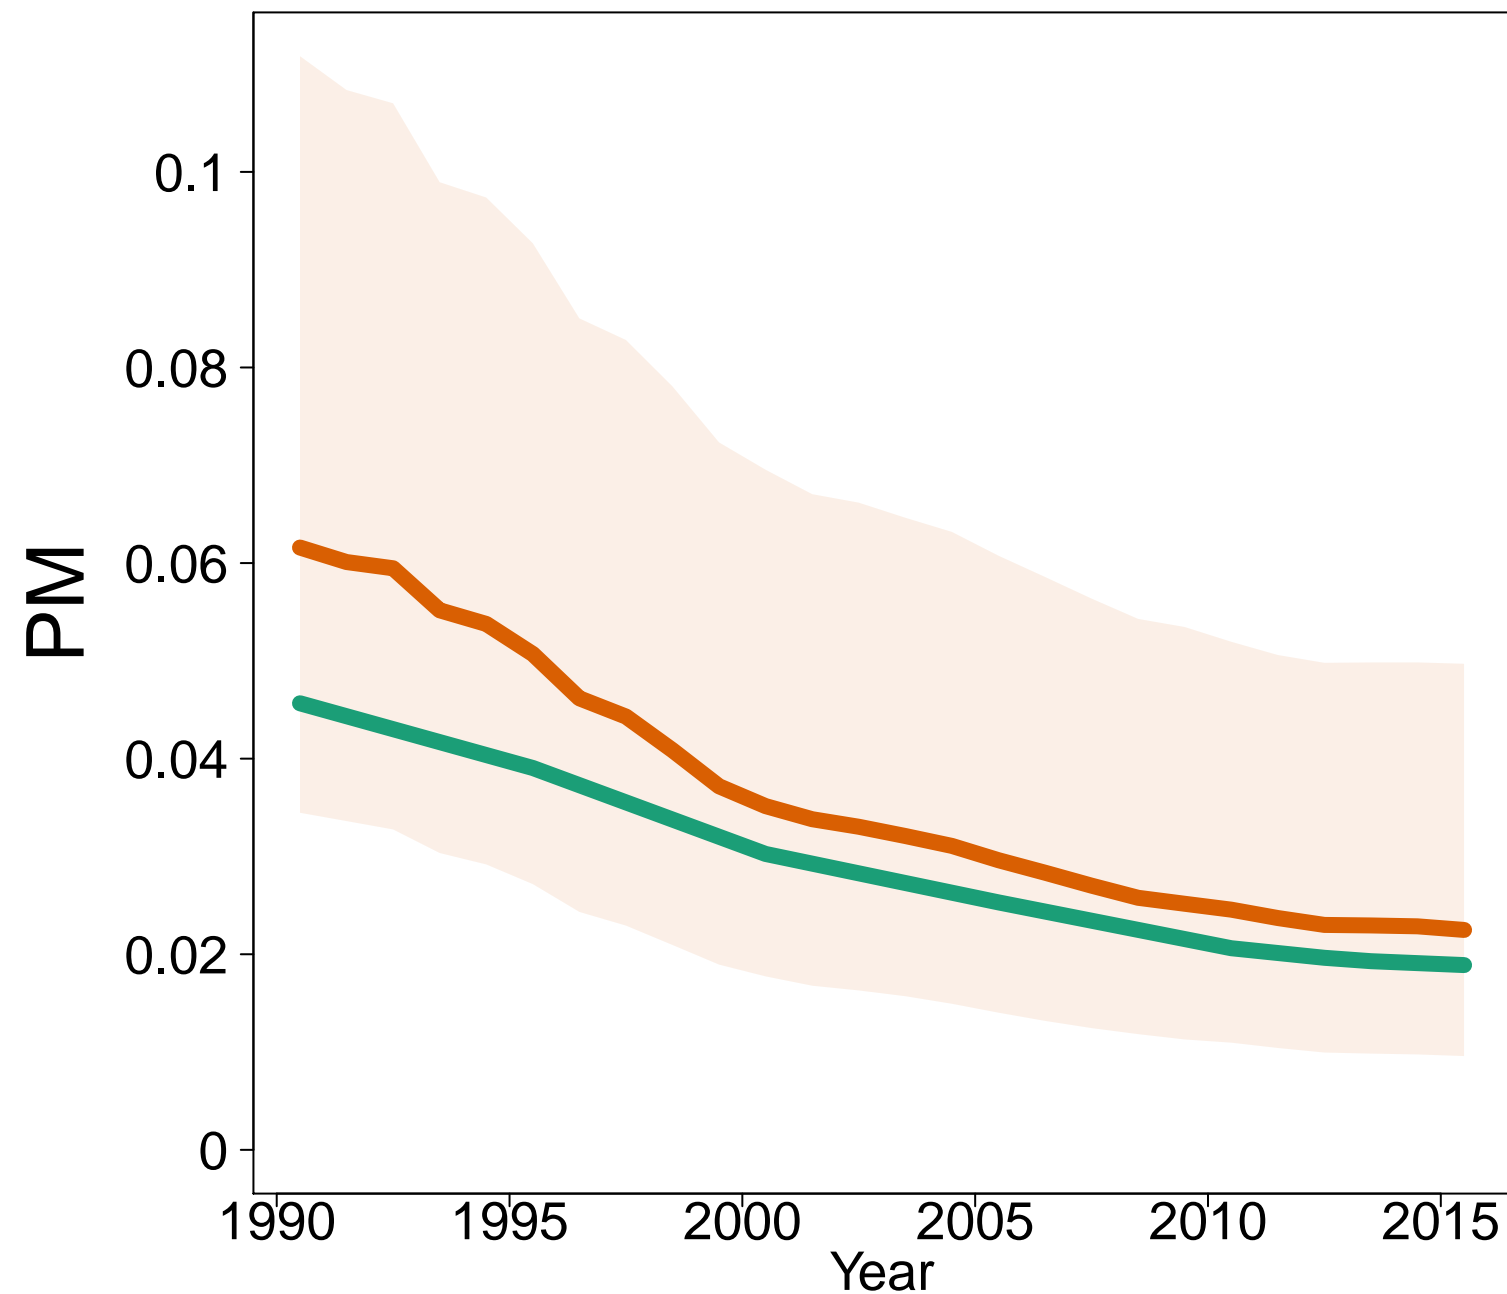

Turkmenistan [TKM; C]  
(Central Asia)

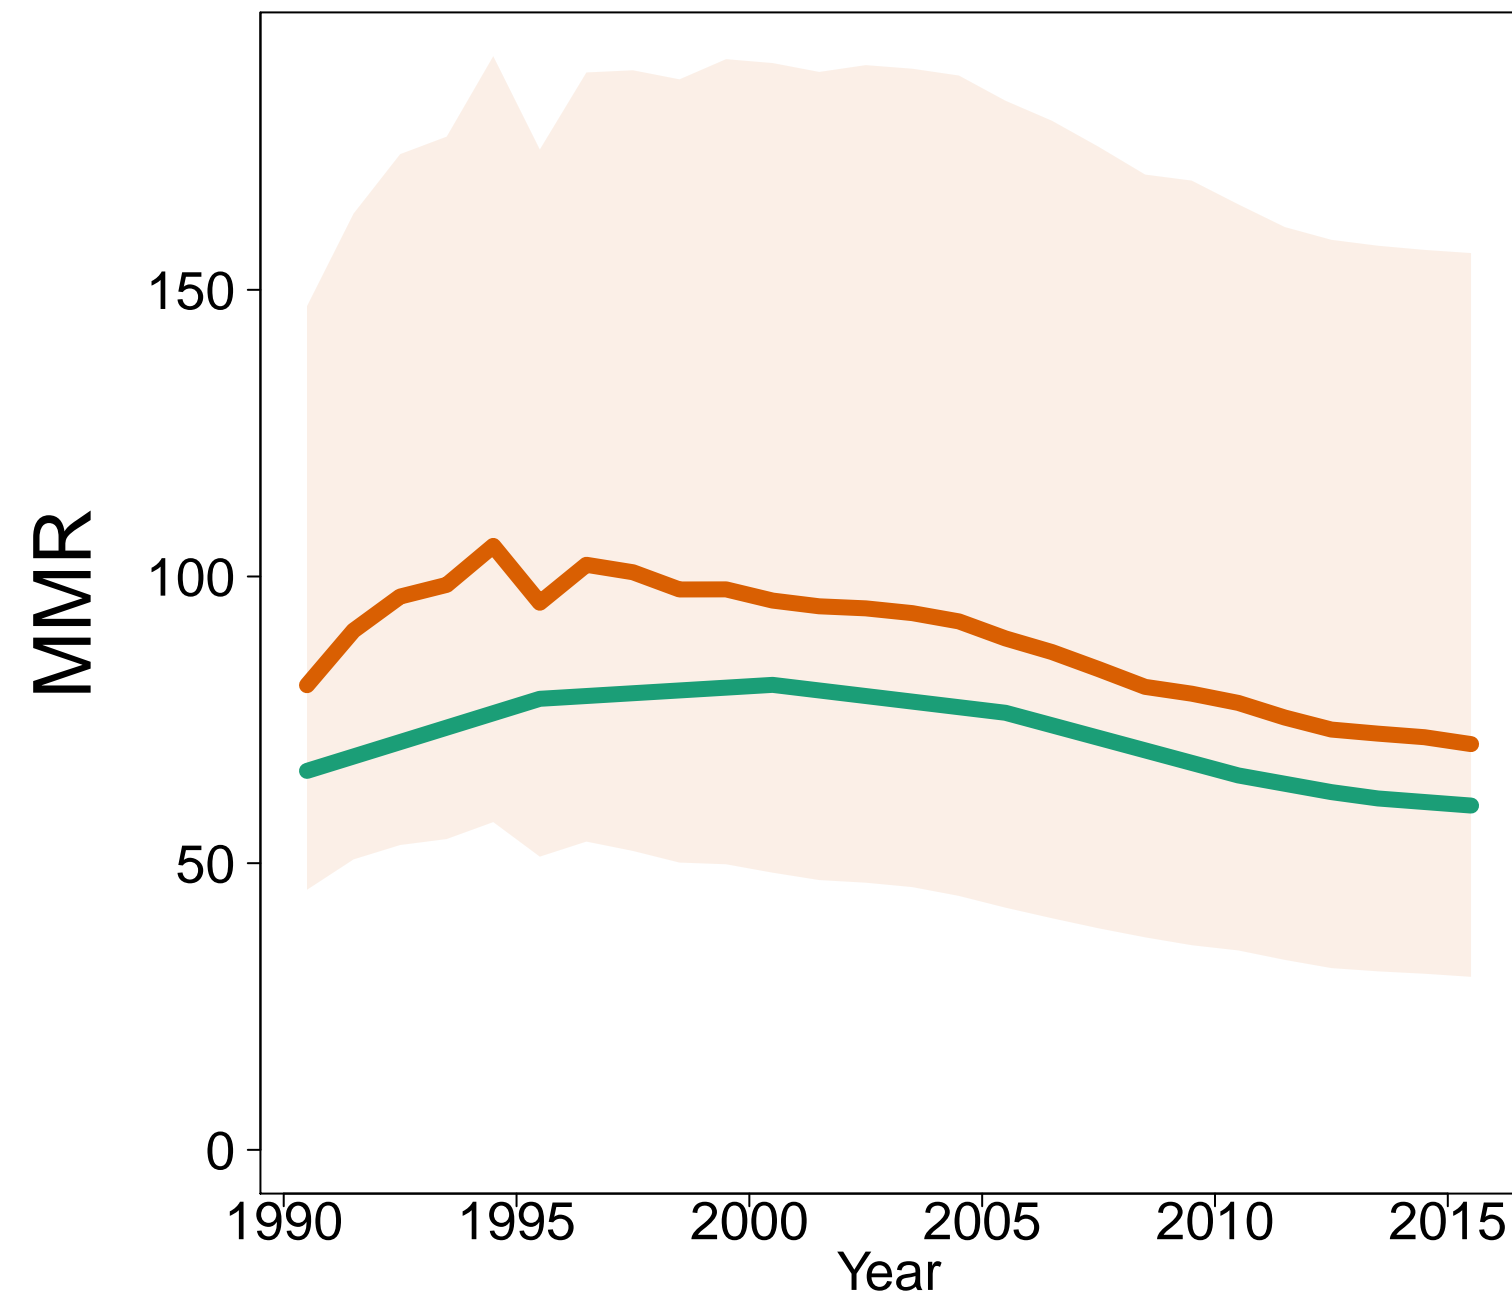

- Estimates –
- Bmat 2014
- MMEIG 2014
- Data –
- ◊ Observed Data
- ◆ Adjusted Data
- Data type –

Uganda [UGA; B]  
(Eastern Africa)

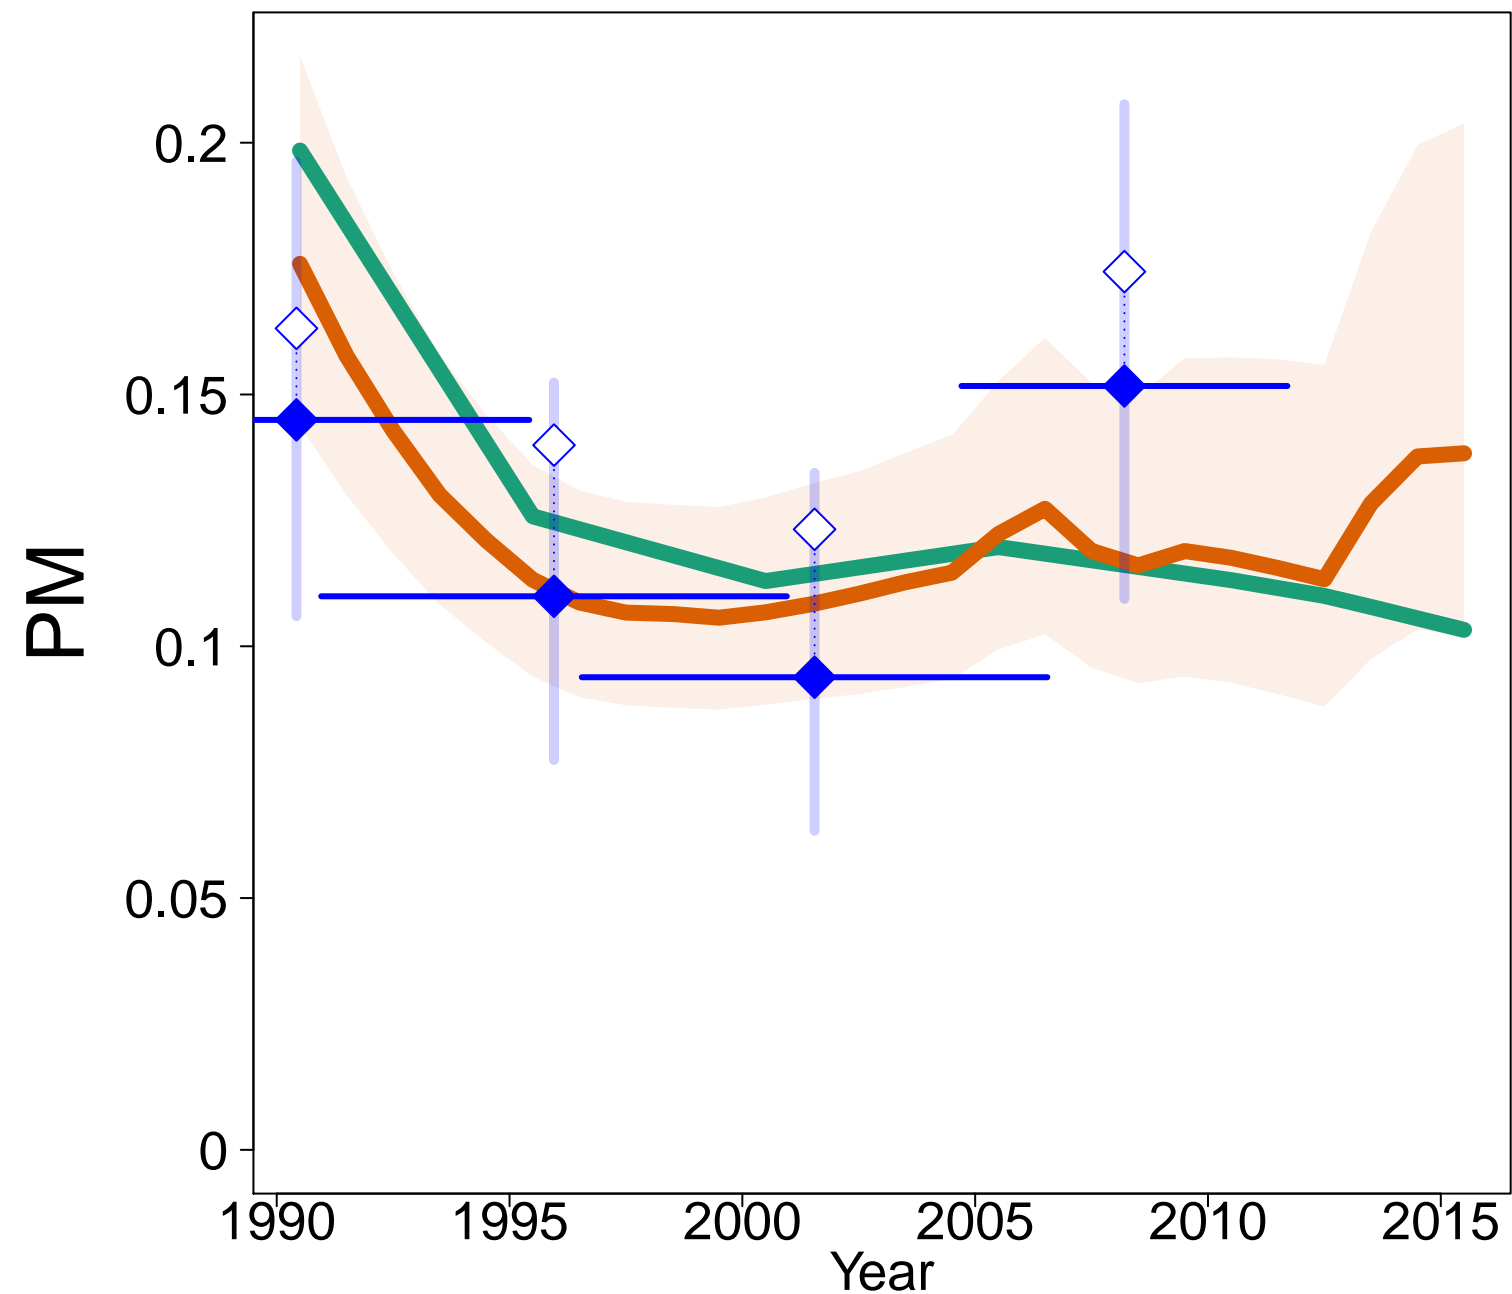

Uganda [UGA; B]  
(Eastern Africa)

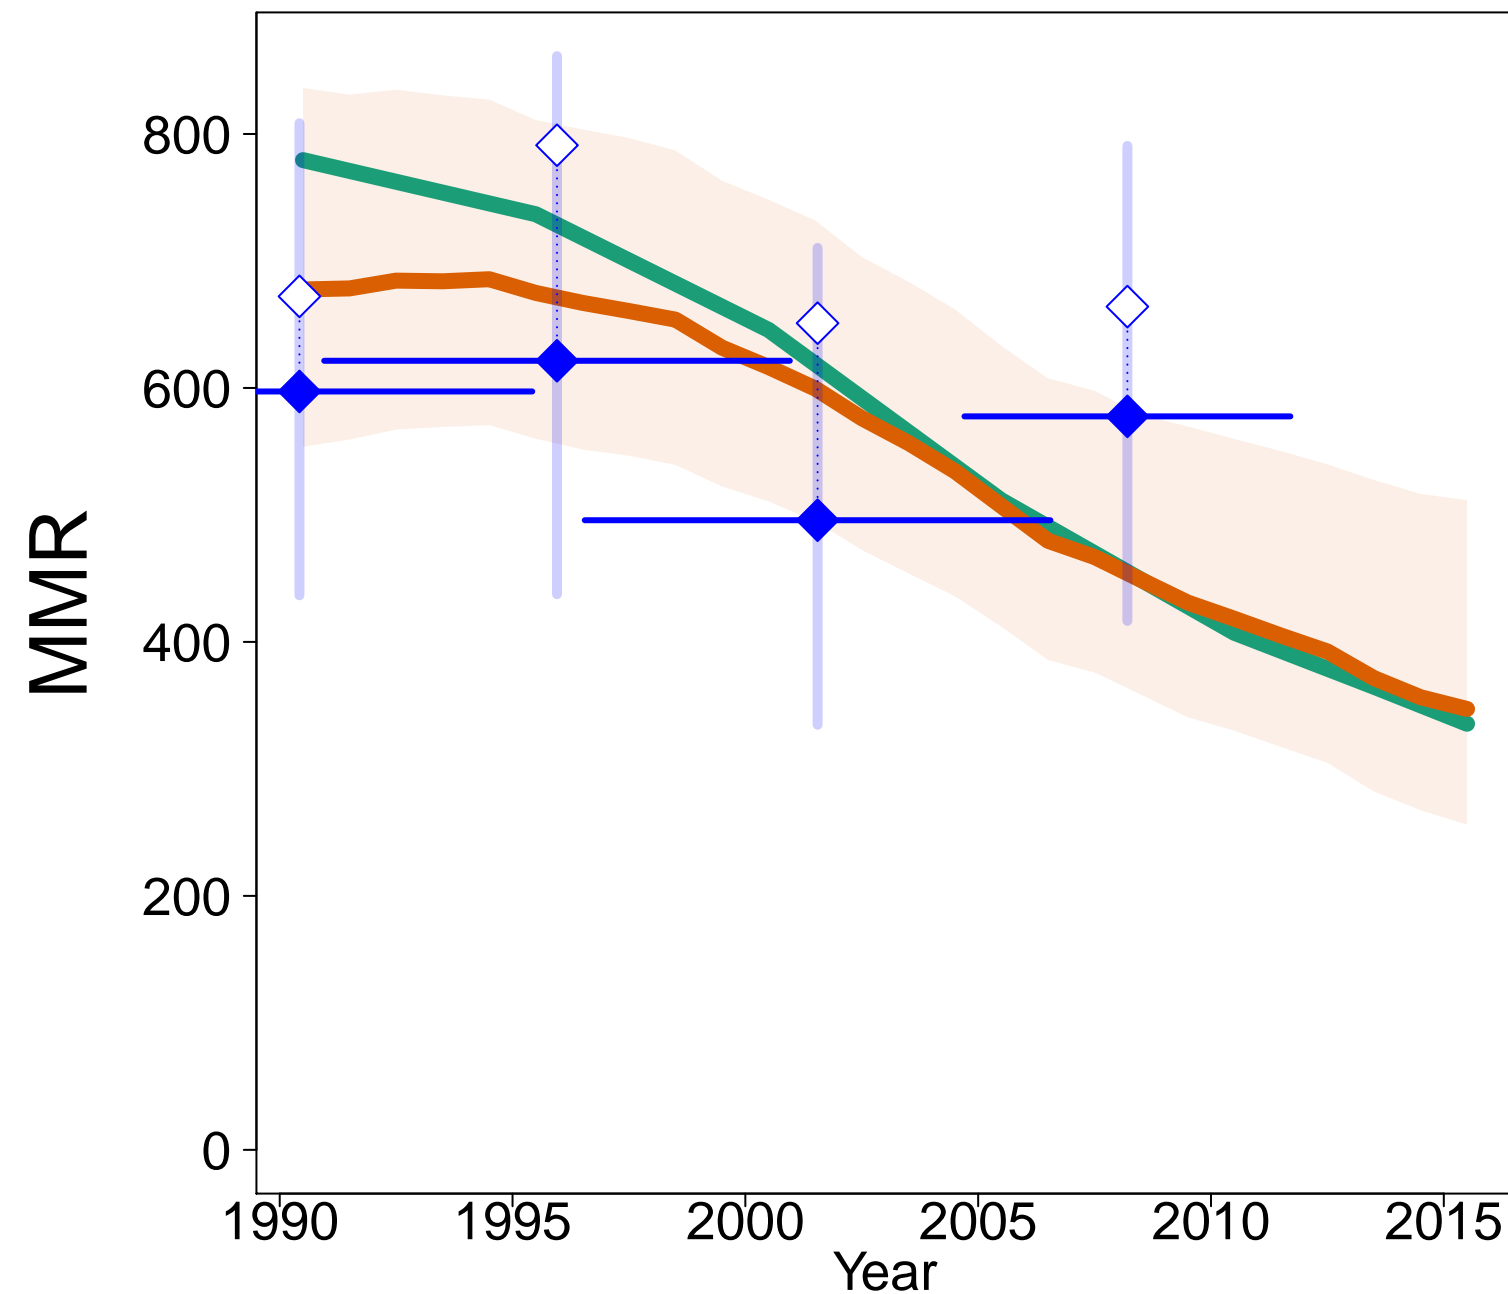

– Estimates –

Bmat 2014

MMEIG 2014

– Data –

Observed Data

Adjusted Data

– Data type –

DHS

Ukraine [UKR; A]  
(Developed regions)

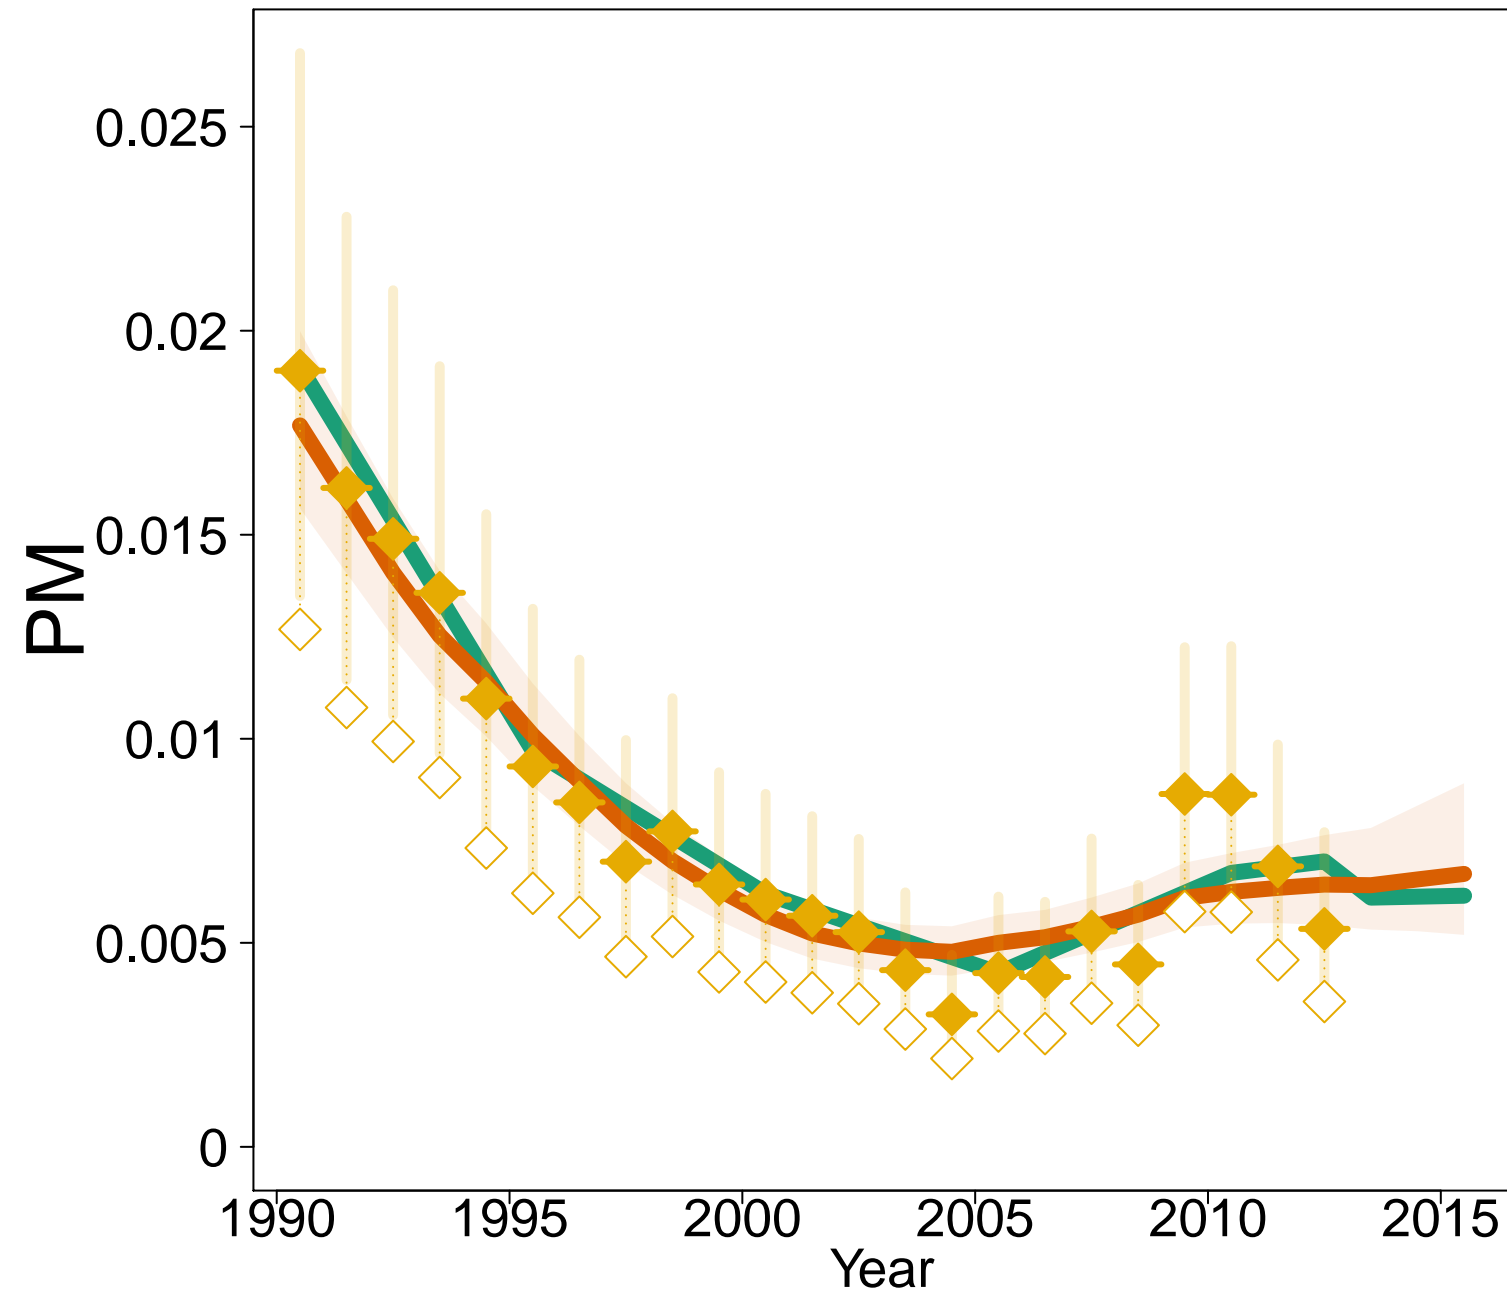

Ukraine [UKR; A]  
(Developed regions)

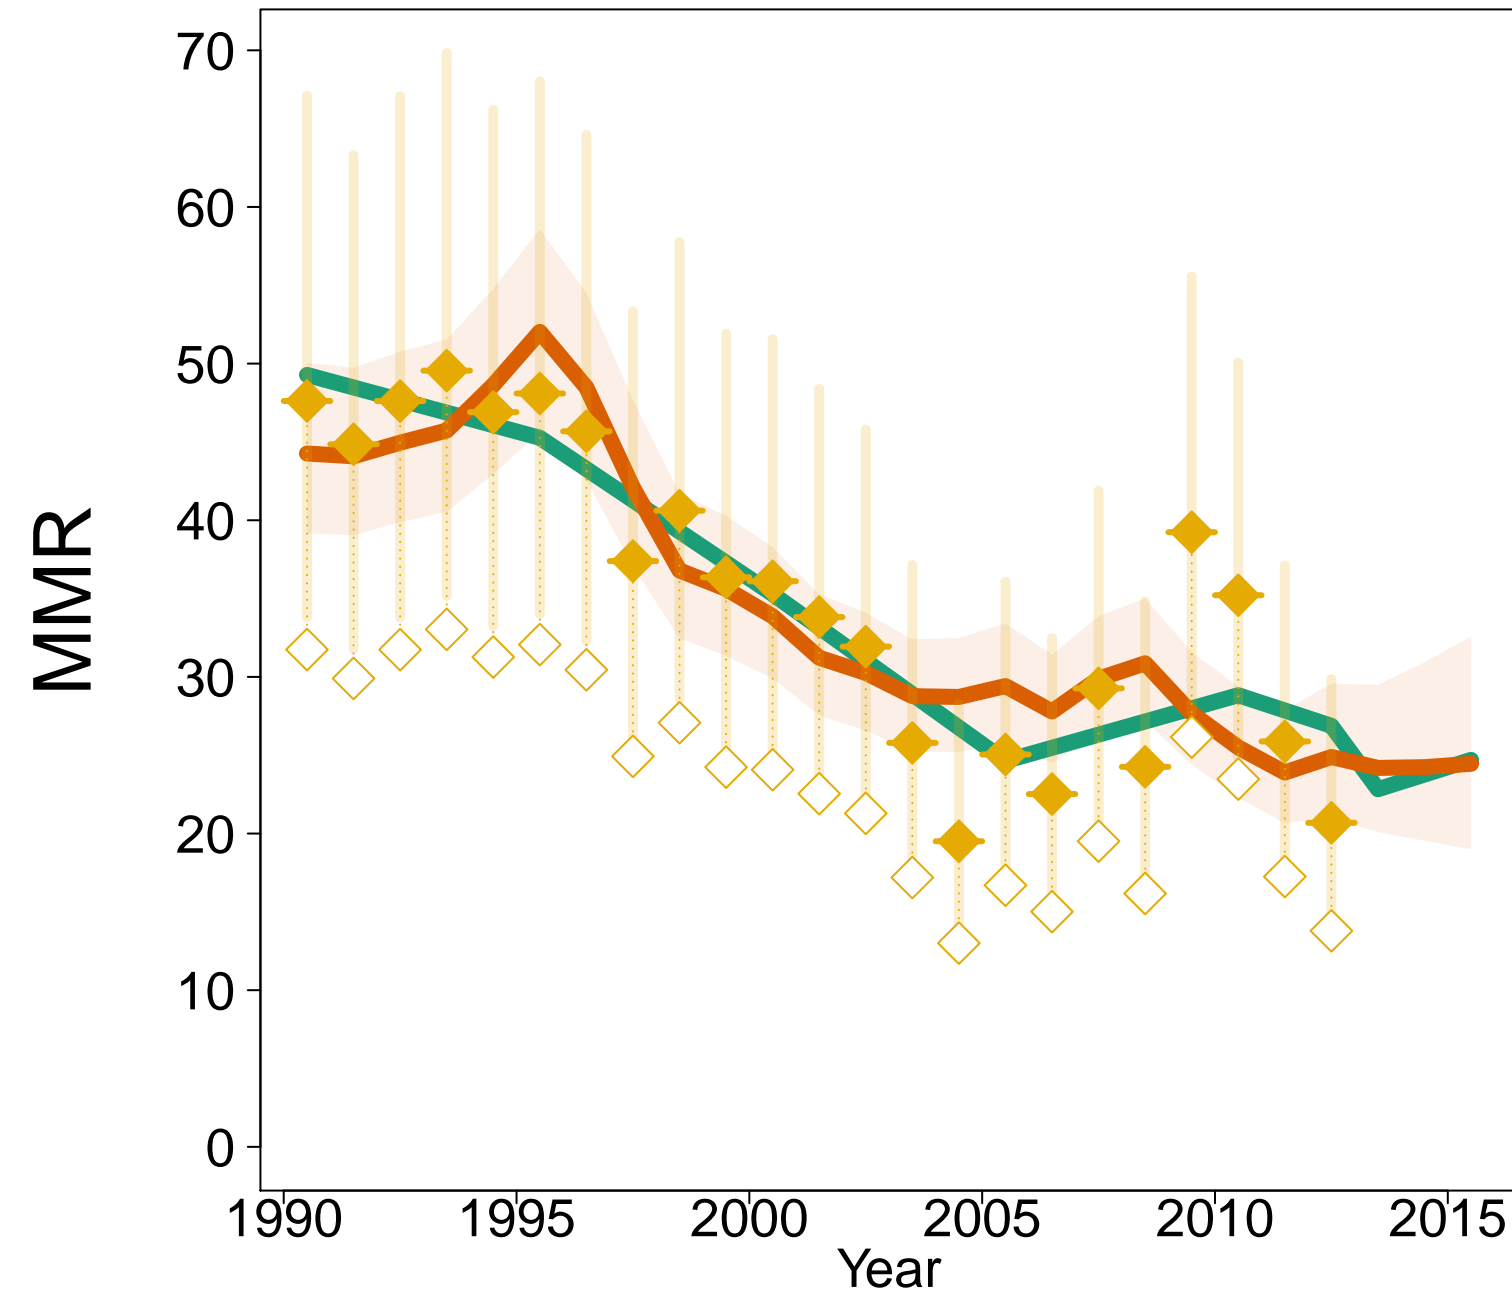

– Estimates –  
Bmat 2014  
MMEIG 2014  
– Data –  
Observed Data  
Adjusted Data  
– Data type –  
VR

United Arab Emirates [ARE; C]  
(Western Asia)

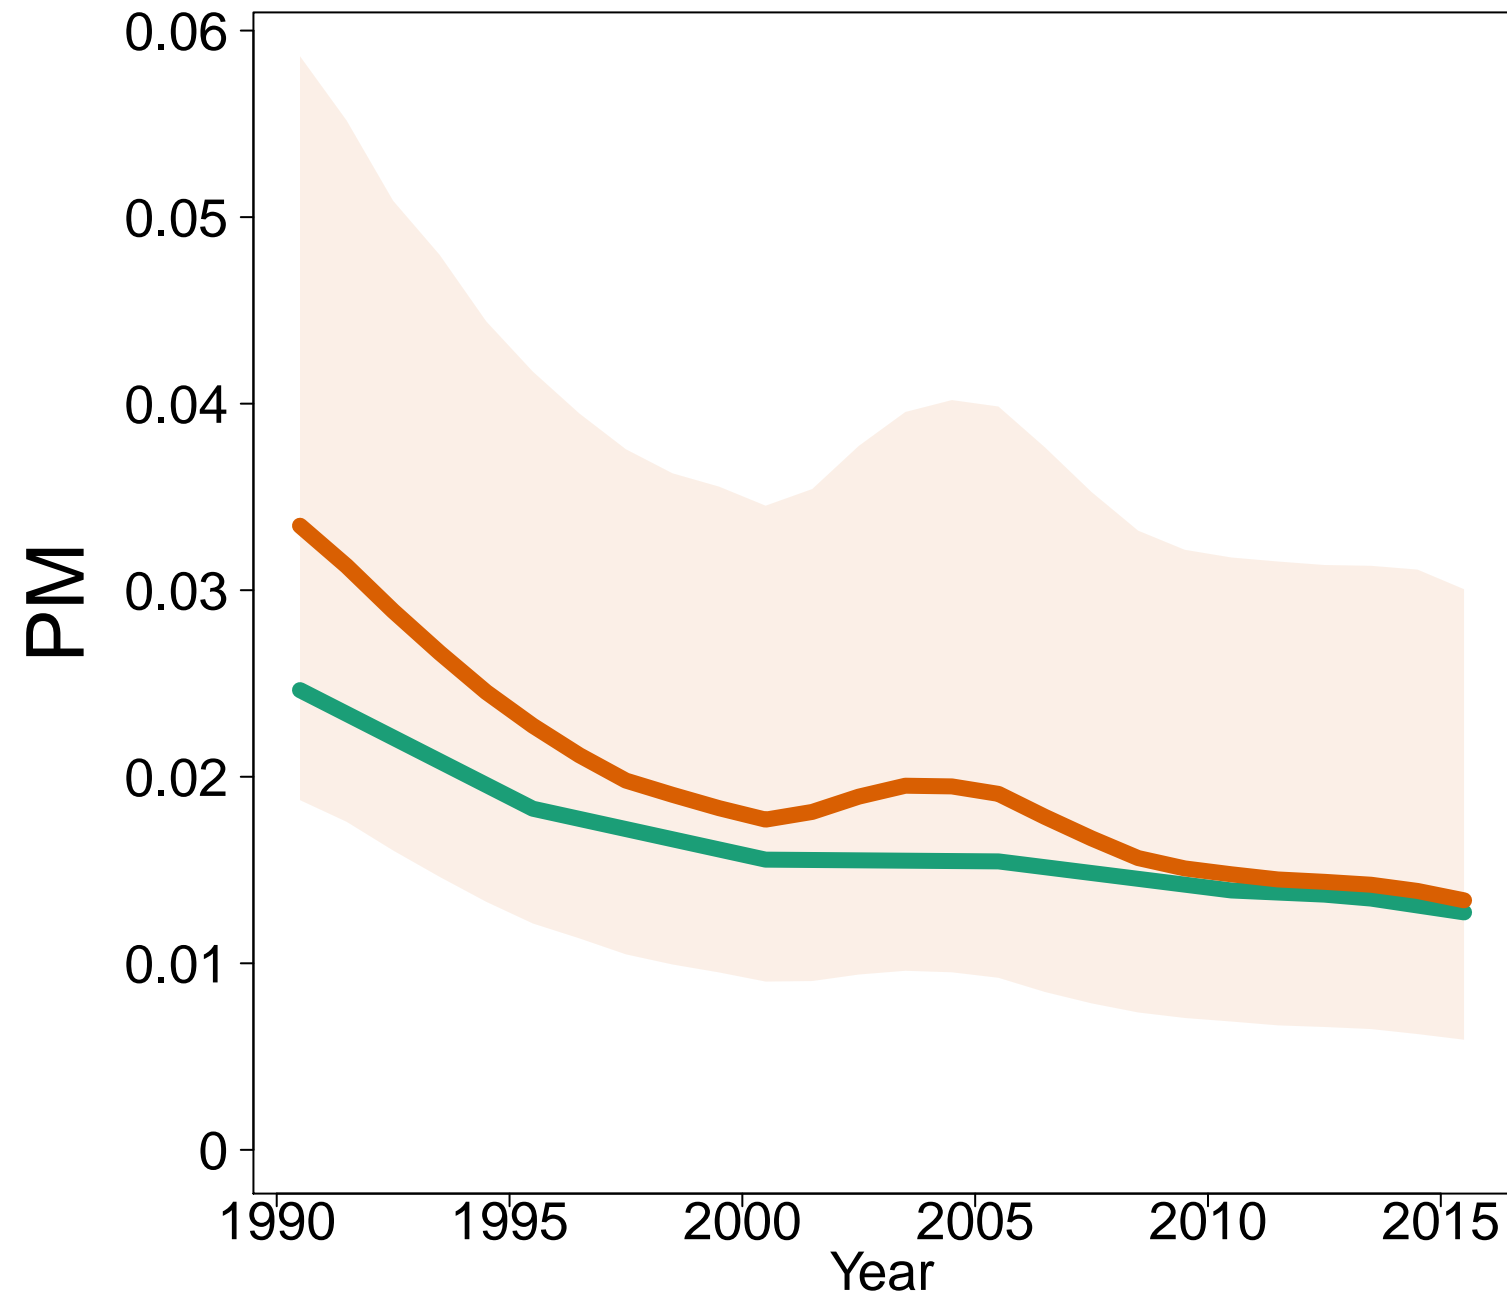

United Arab Emirates [ARE; C]  
(Western Asia)

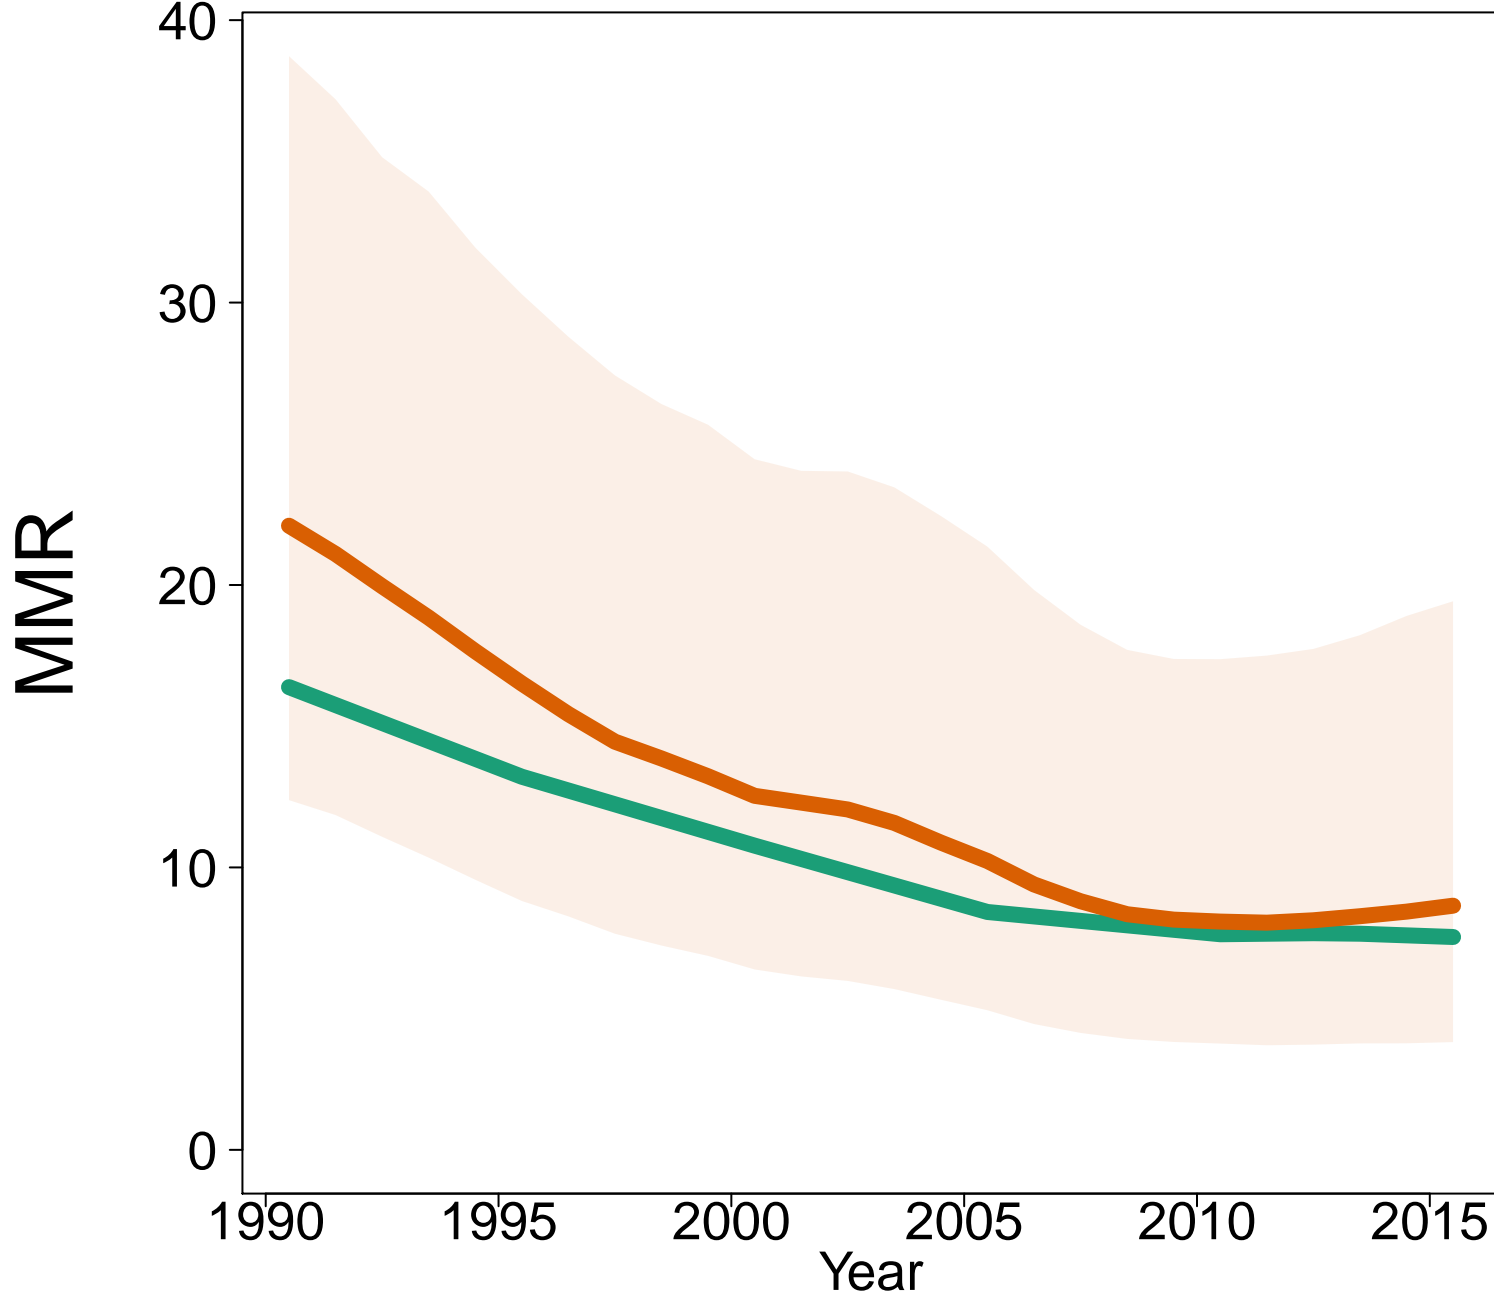

– Estimates –  
Bmat 2014  
MMEIG 2014  
– Data –  
Observed Data  
Adjusted Data  
– Data type –

United Kingdom [GBR; A]  
(Developed regions)

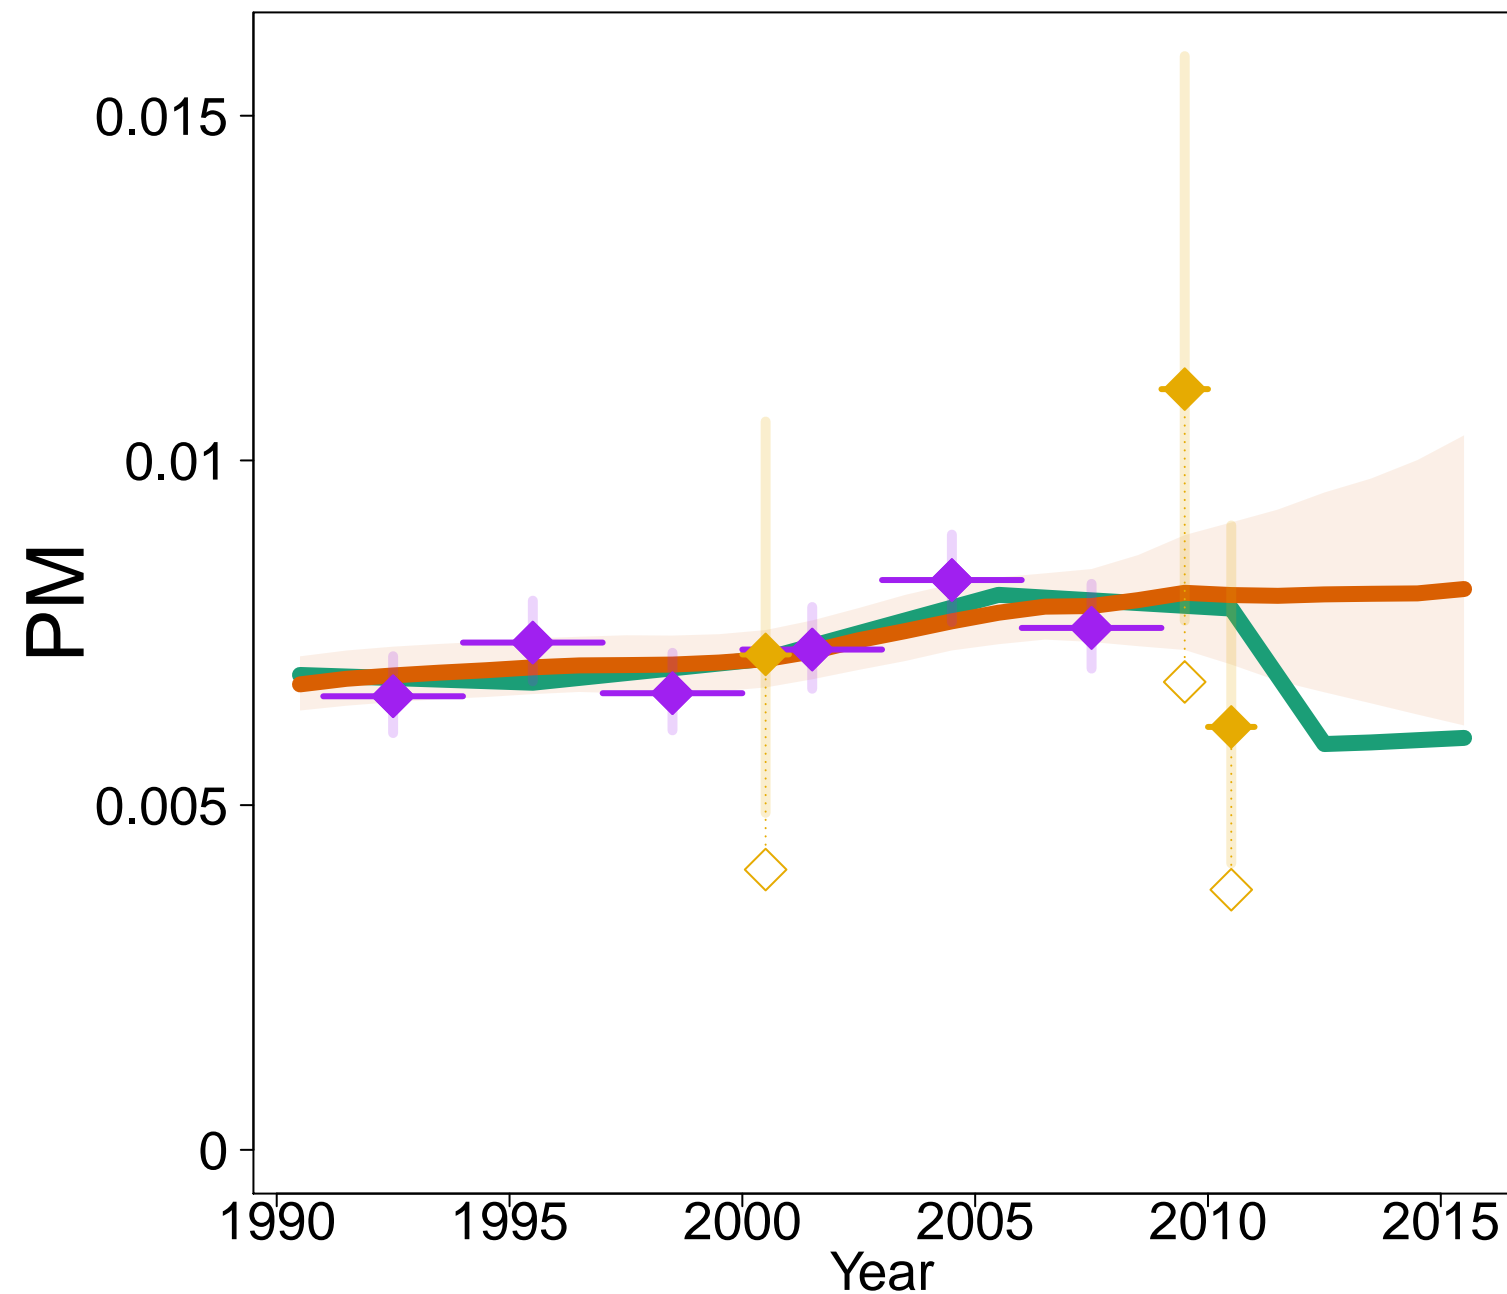

United Kingdom [GBR; A]  
(Developed regions)

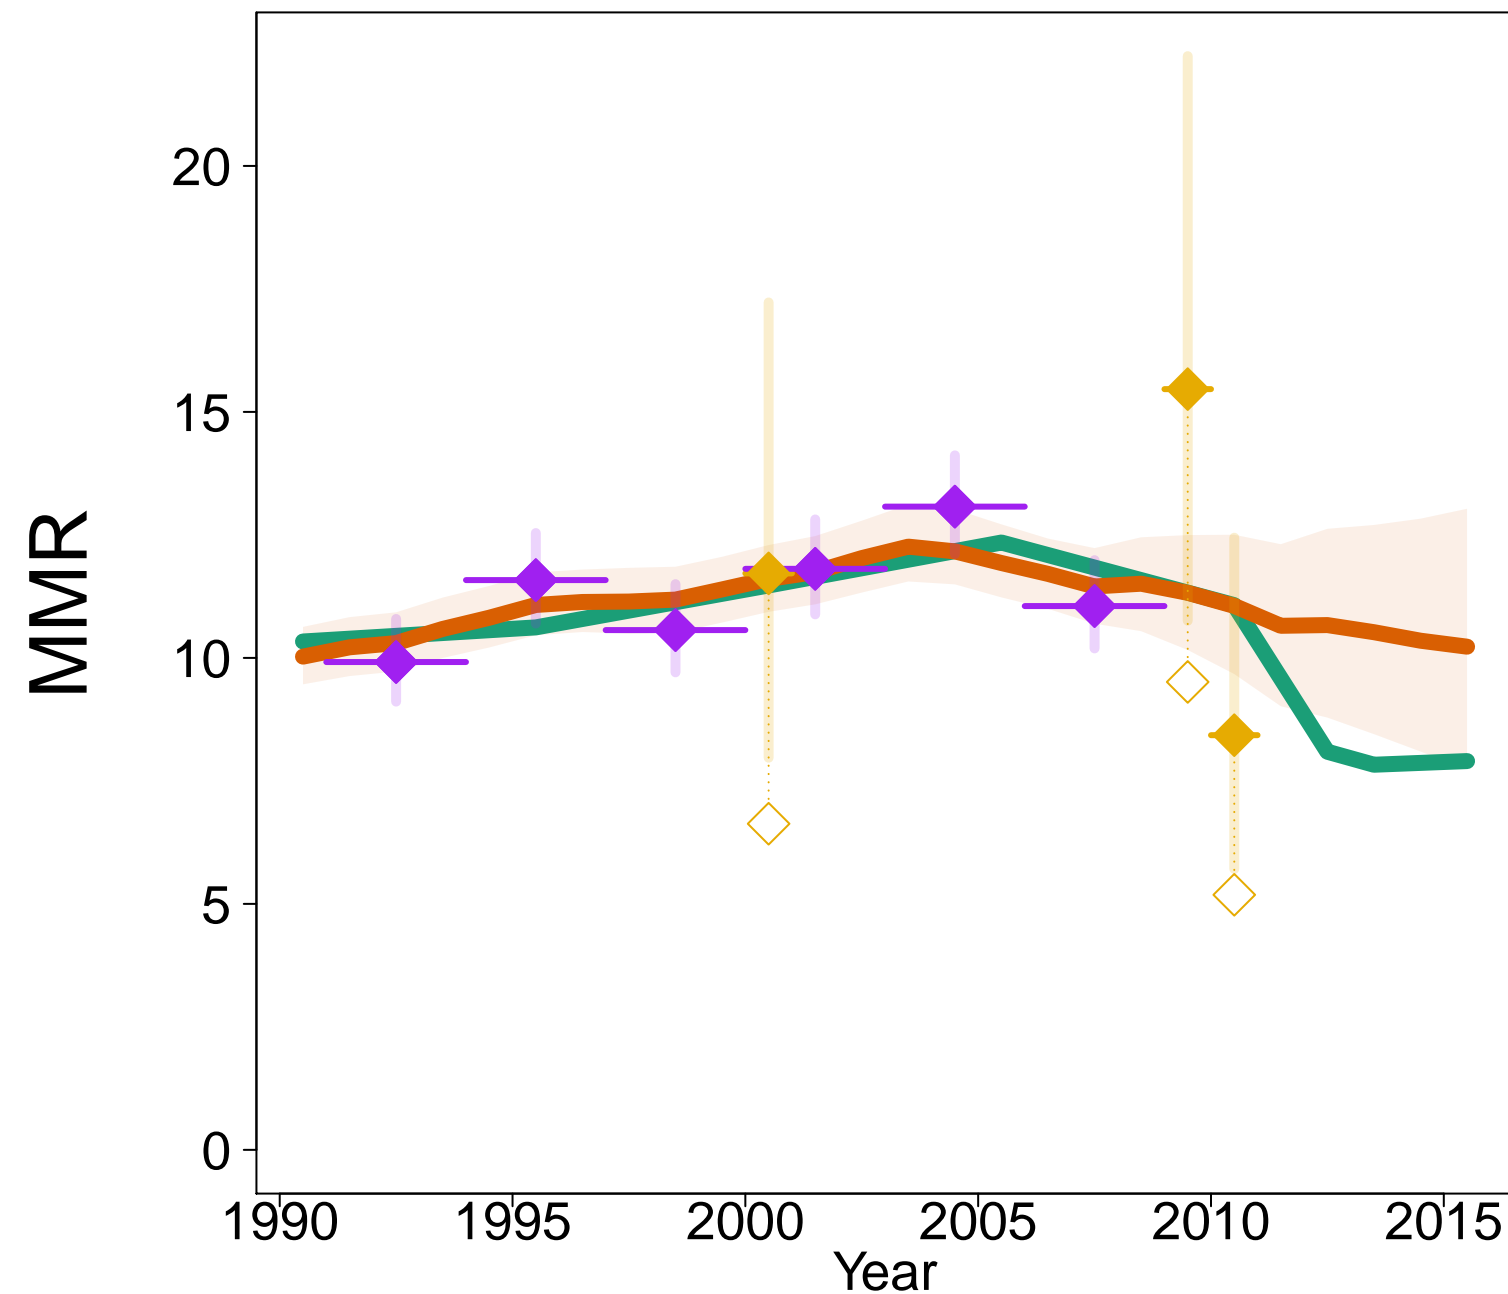

- Estimates –
- Bmat 2014
- MMEIG 2014
- Data –
- Observed Data
- Adjusted Data
- Data type –
- VR
- Spec. studies

United States of America [USA; A]  
(Developed regions)

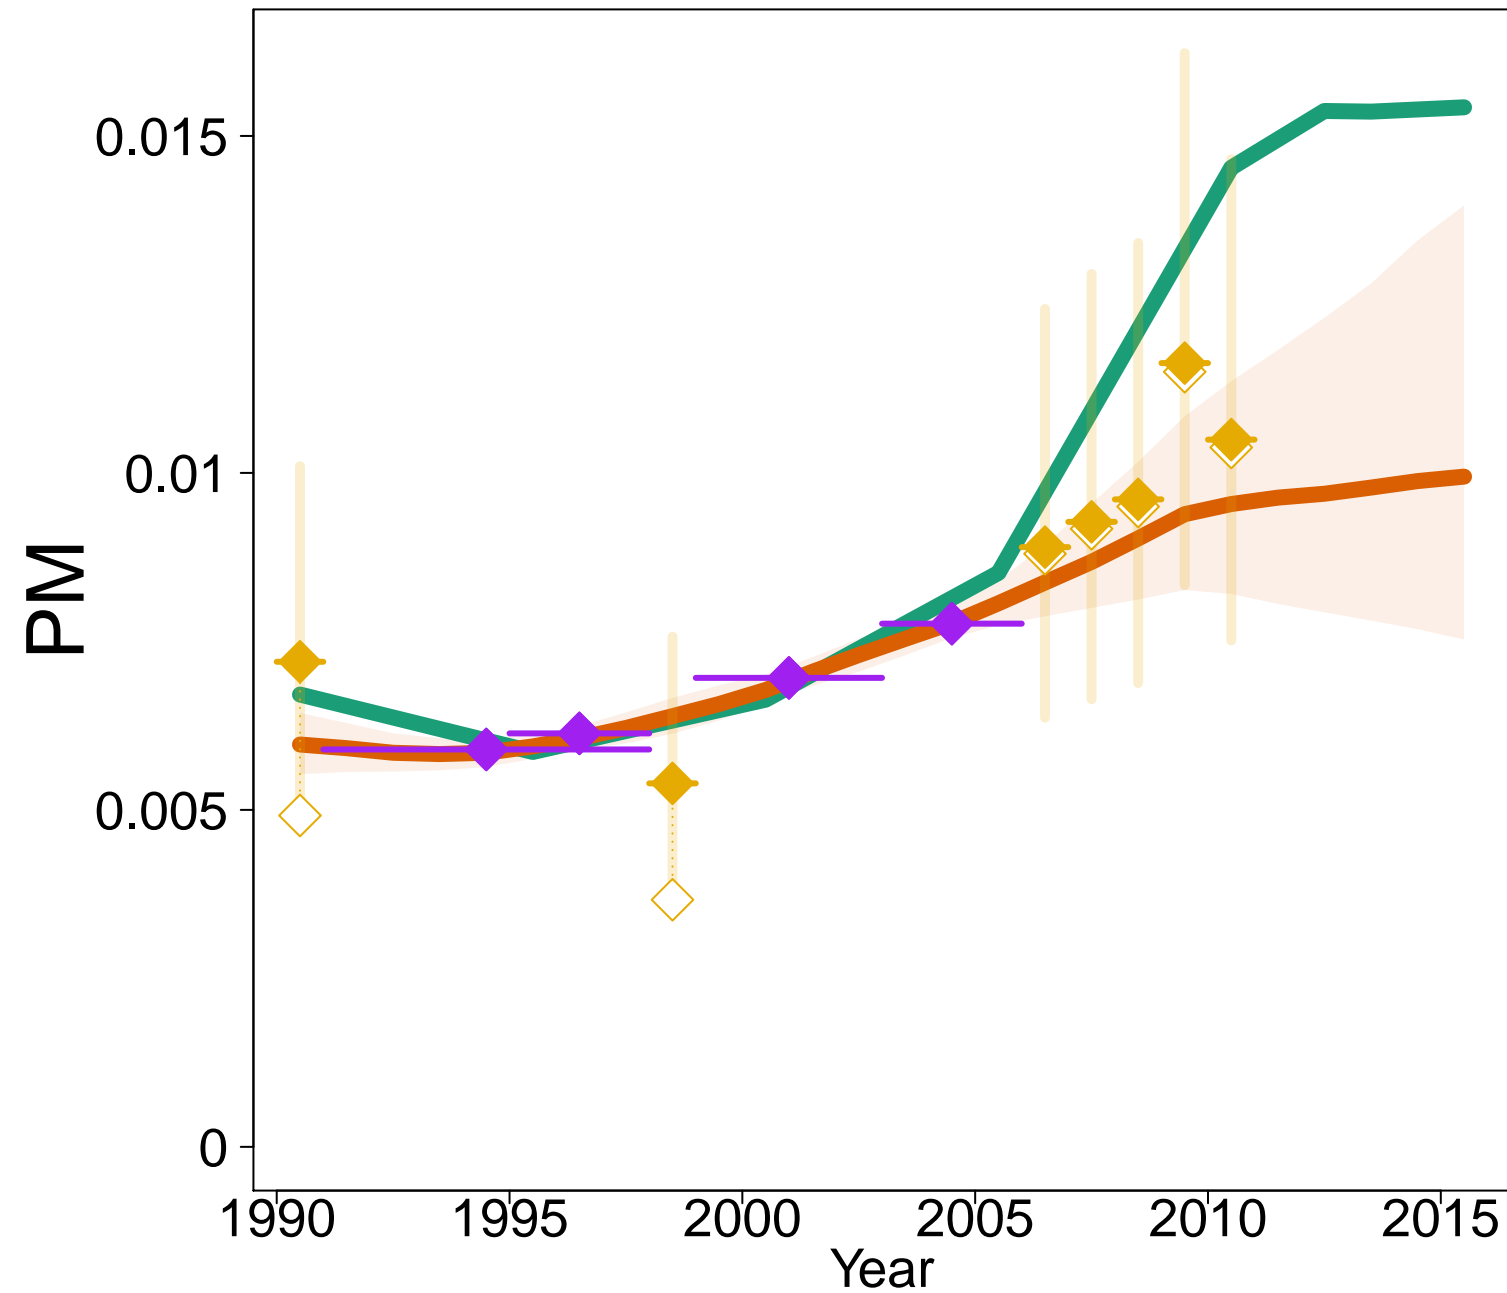

United States of America [USA; A]  
(Developed regions)

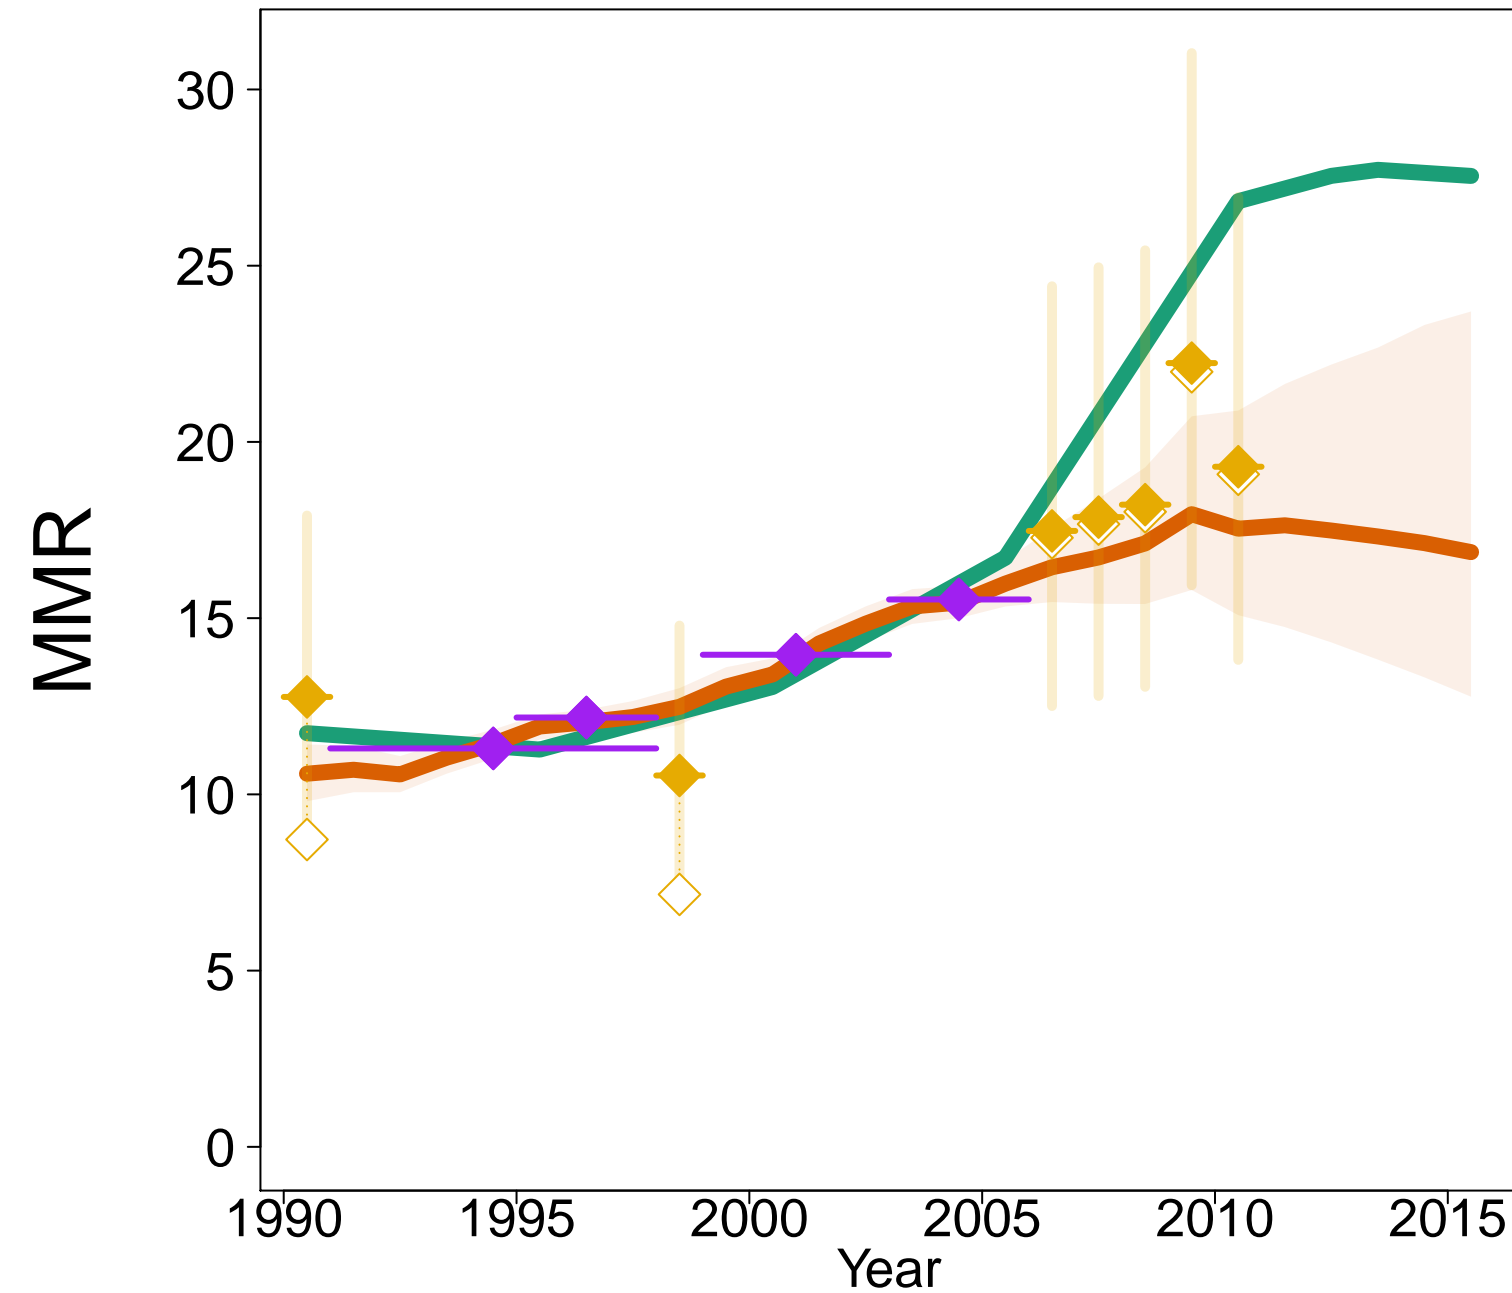

– Estimates –  
Bmat 2014  
MMEIG 2014  
– Data –  
Observed Data  
Adjusted Data  
– Data type –  
VR  
Spec. studies

Uruguay [URY; A]  
(South America)

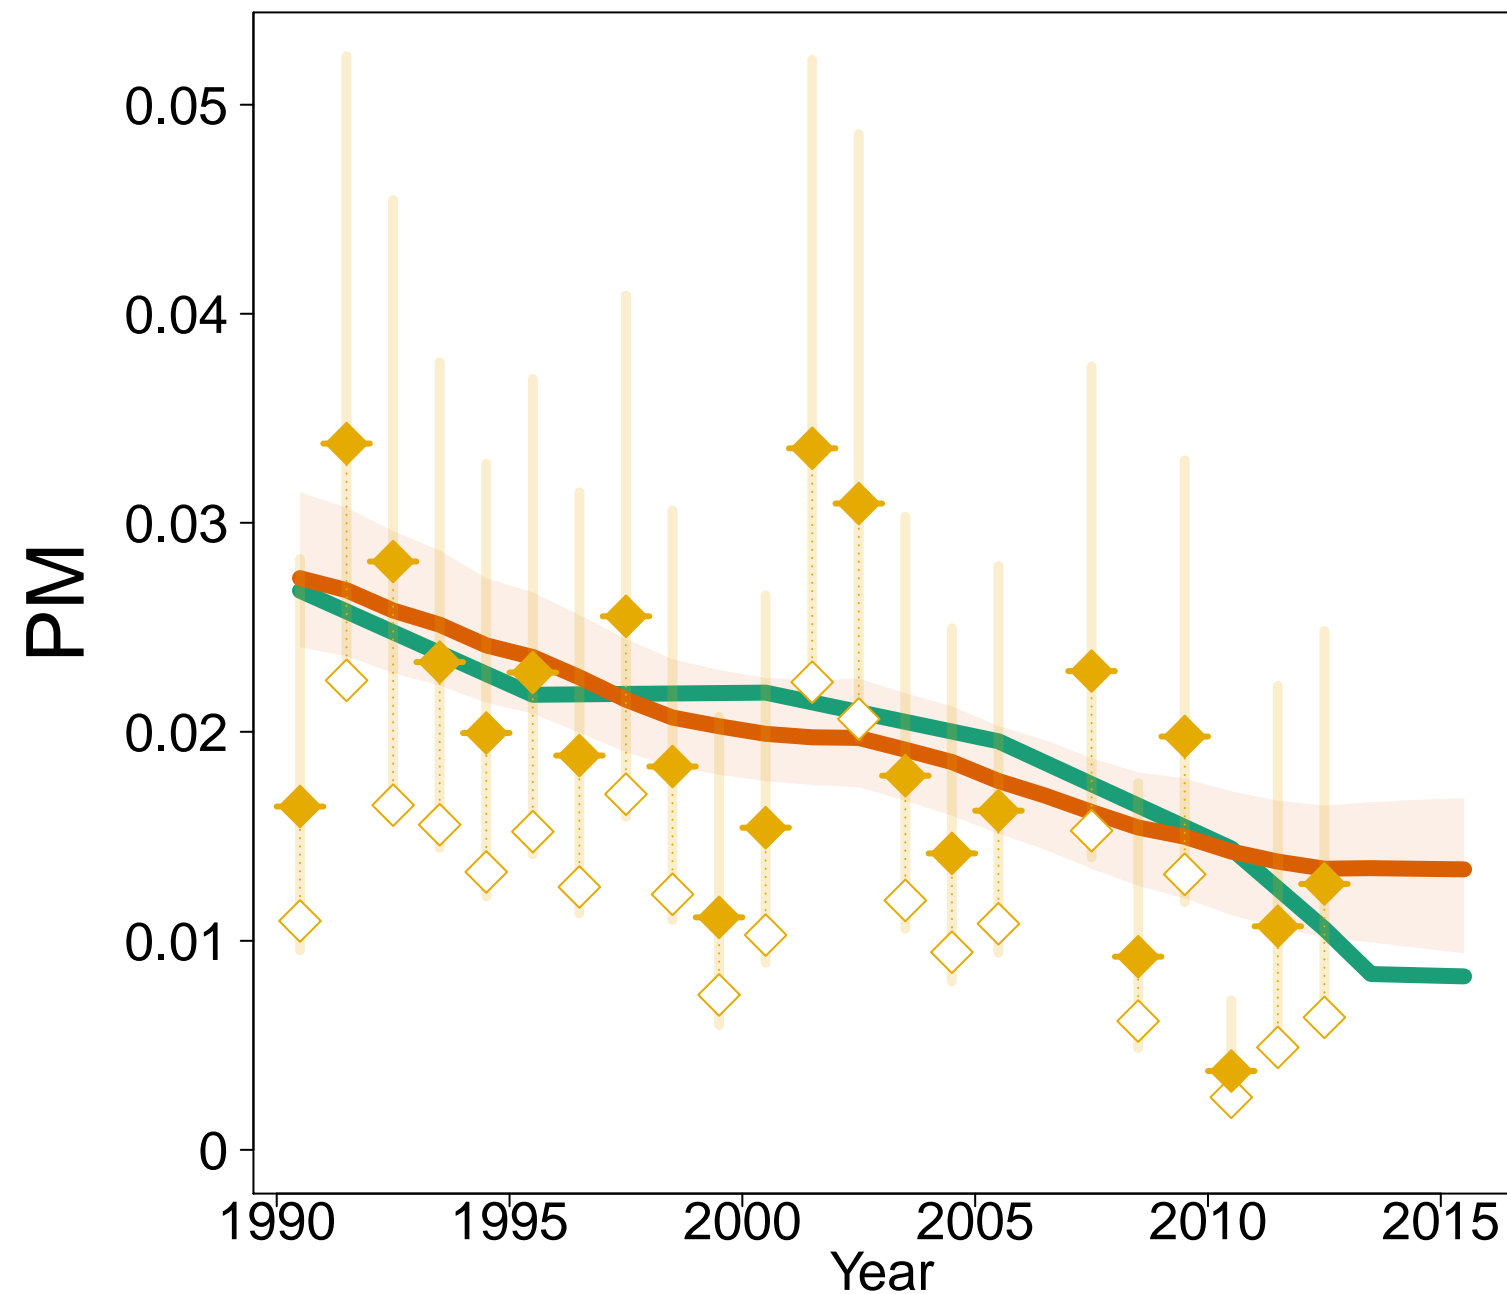

Uruguay [URY; A]  
(South America)

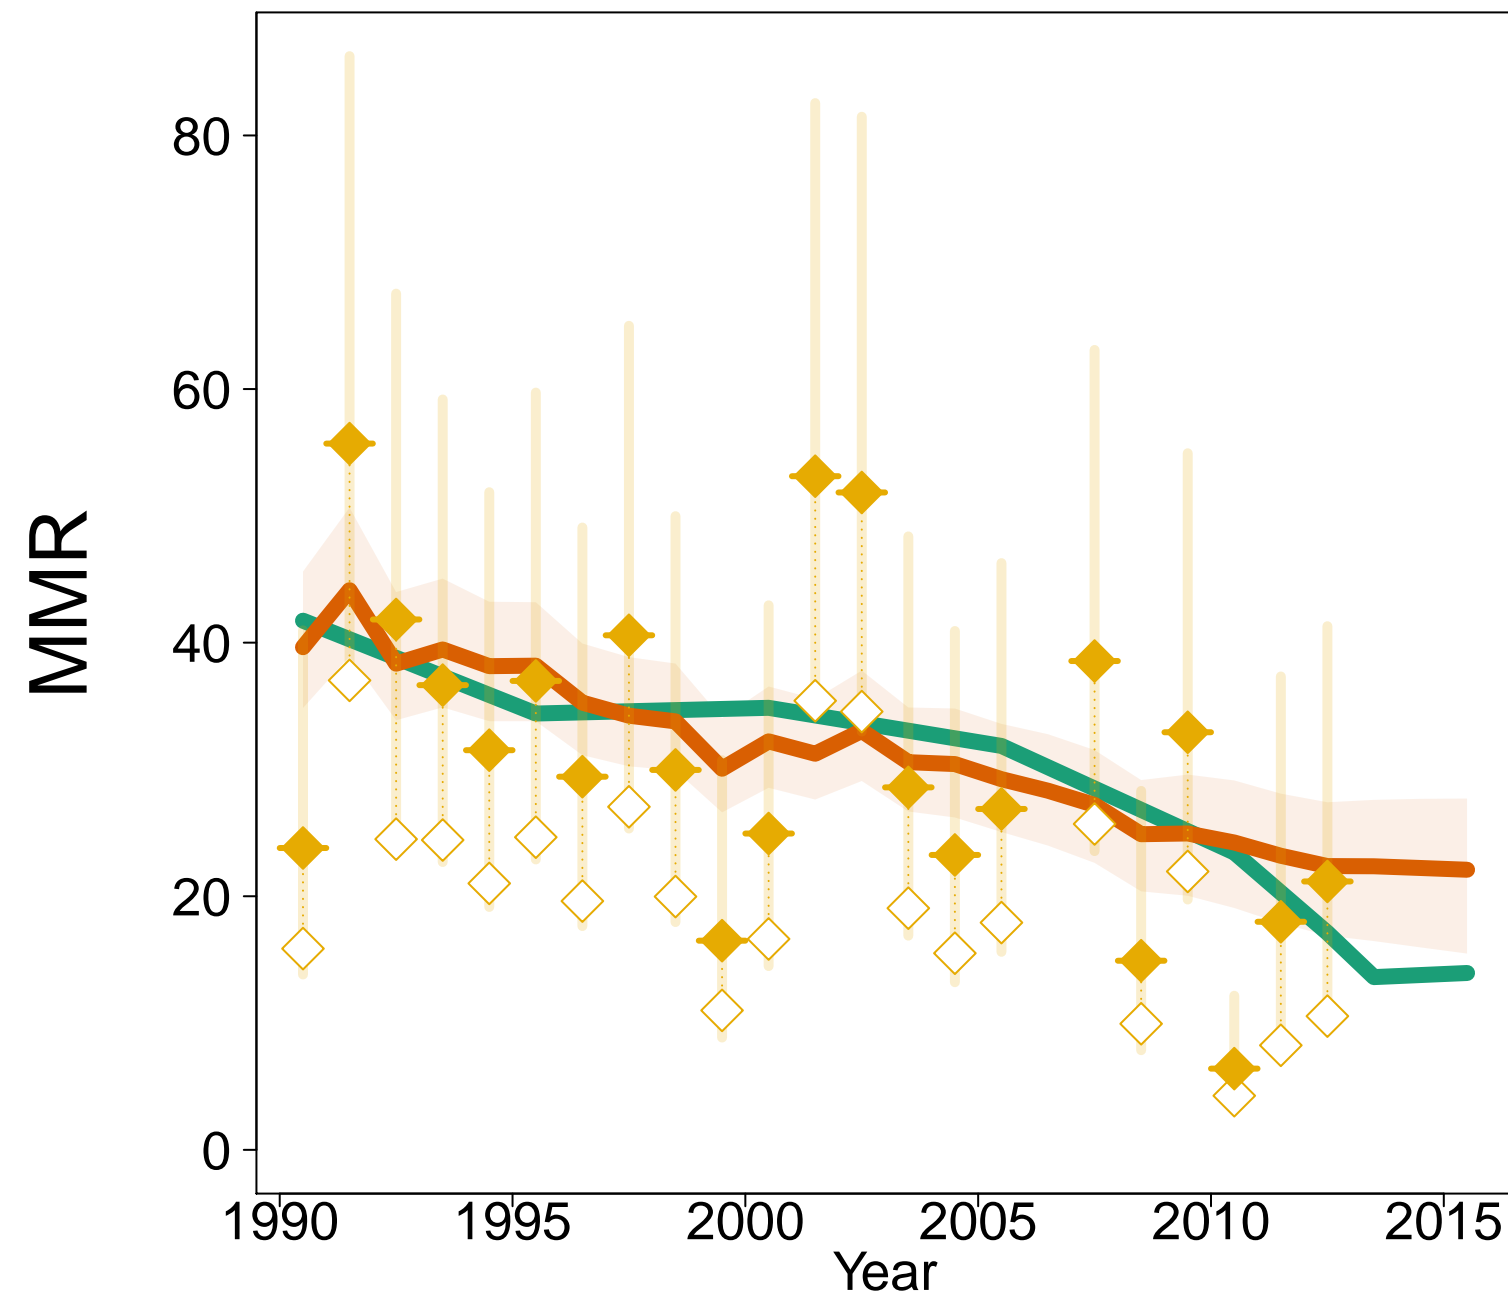

- Estimates –
- Bmat 2014
- MMEIG 2014
- Data –
- Observed Data
- Adjusted Data
- Data type –
- VR



Uzbekistan [UZB; A]  
(Central Asia)

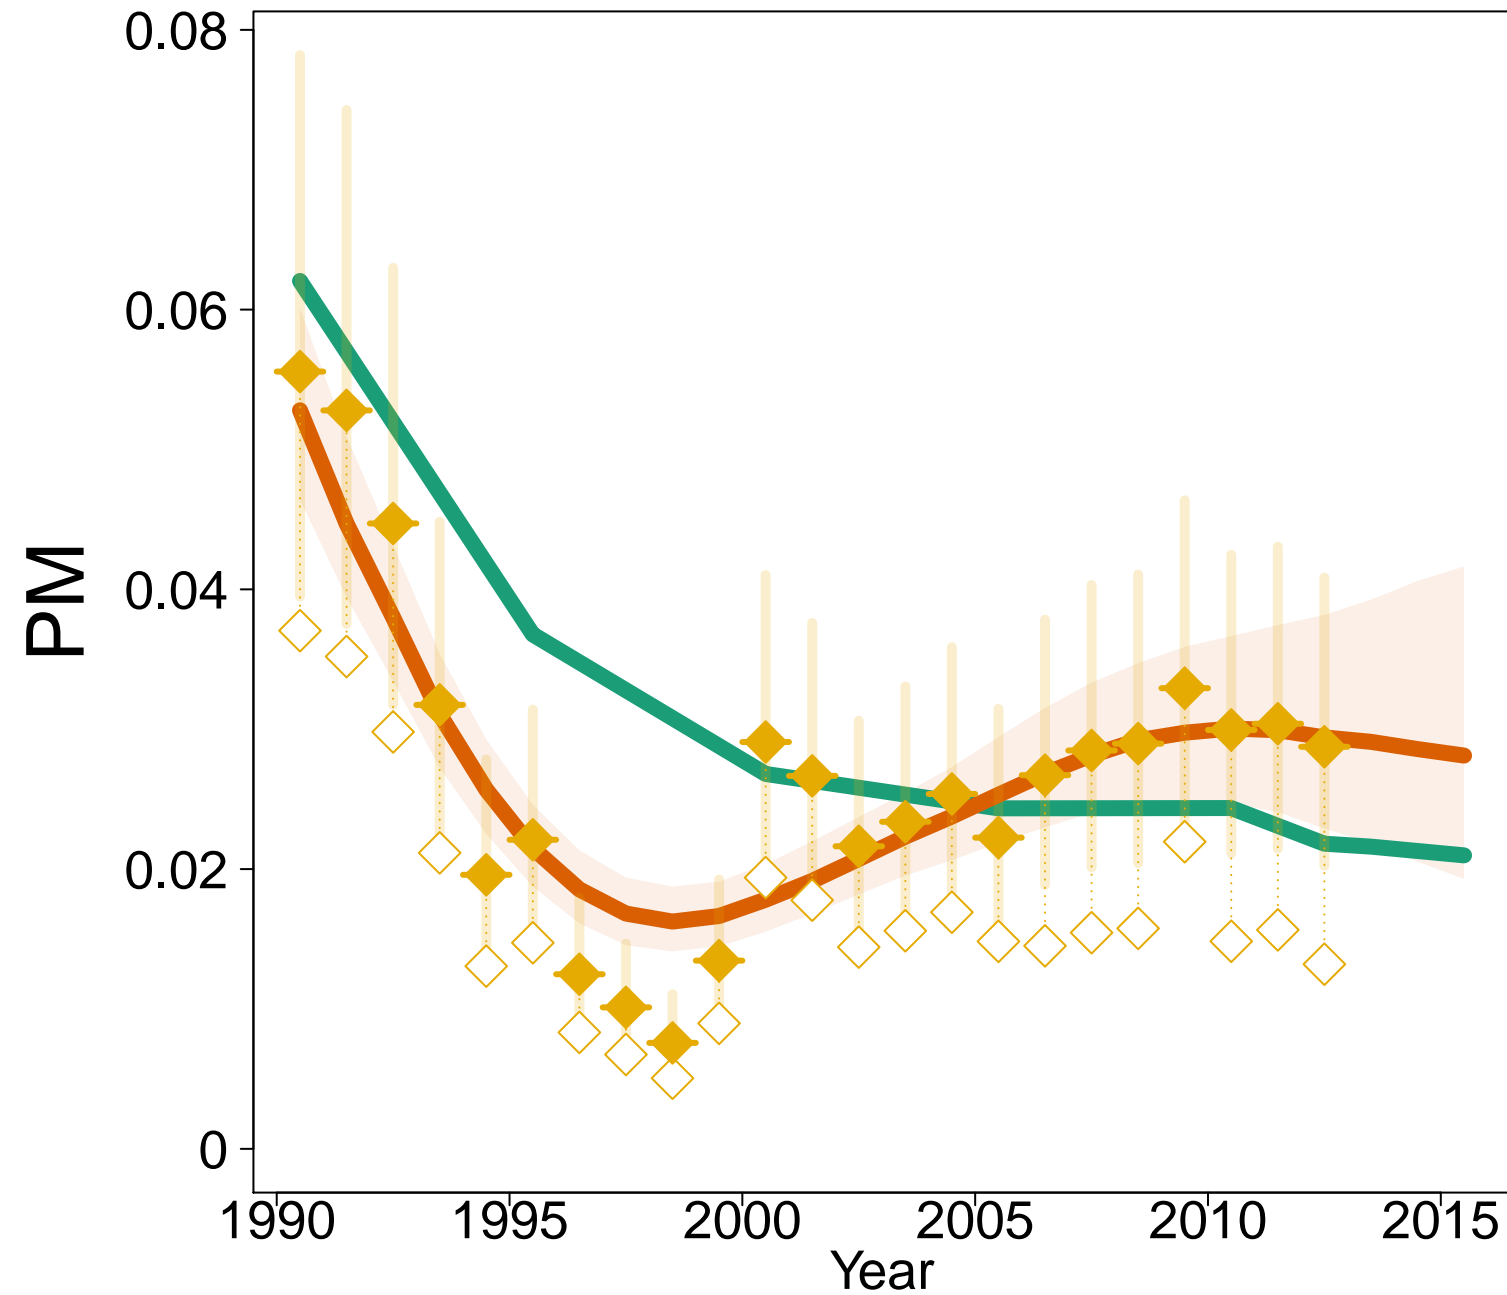

Uzbekistan [UZB; A]  
(Central Asia)

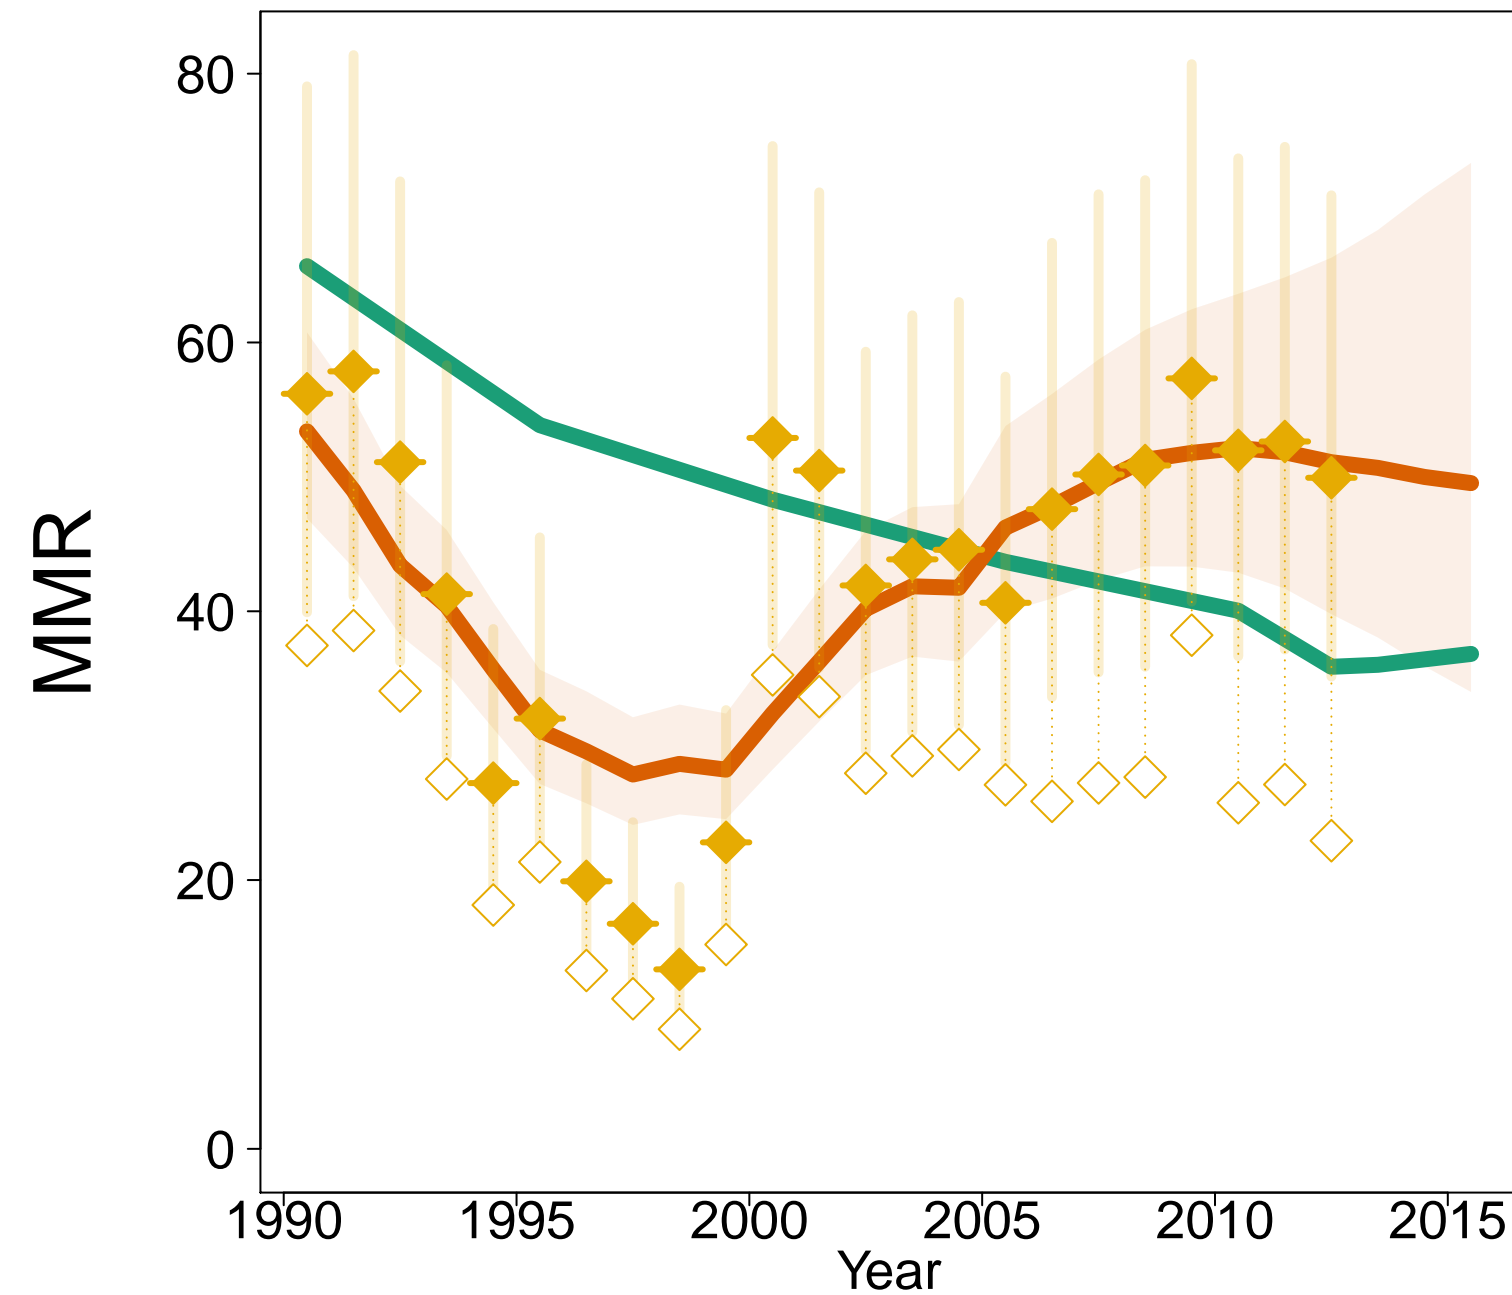

- Estimates –
- Bmat 2014
- MMEIG 2014
- Data –
- Observed Data
- Adjusted Data
- Data type –
- VR

Vanuatu [VUT; C]  
(South-Eastern Asia / Oceania)

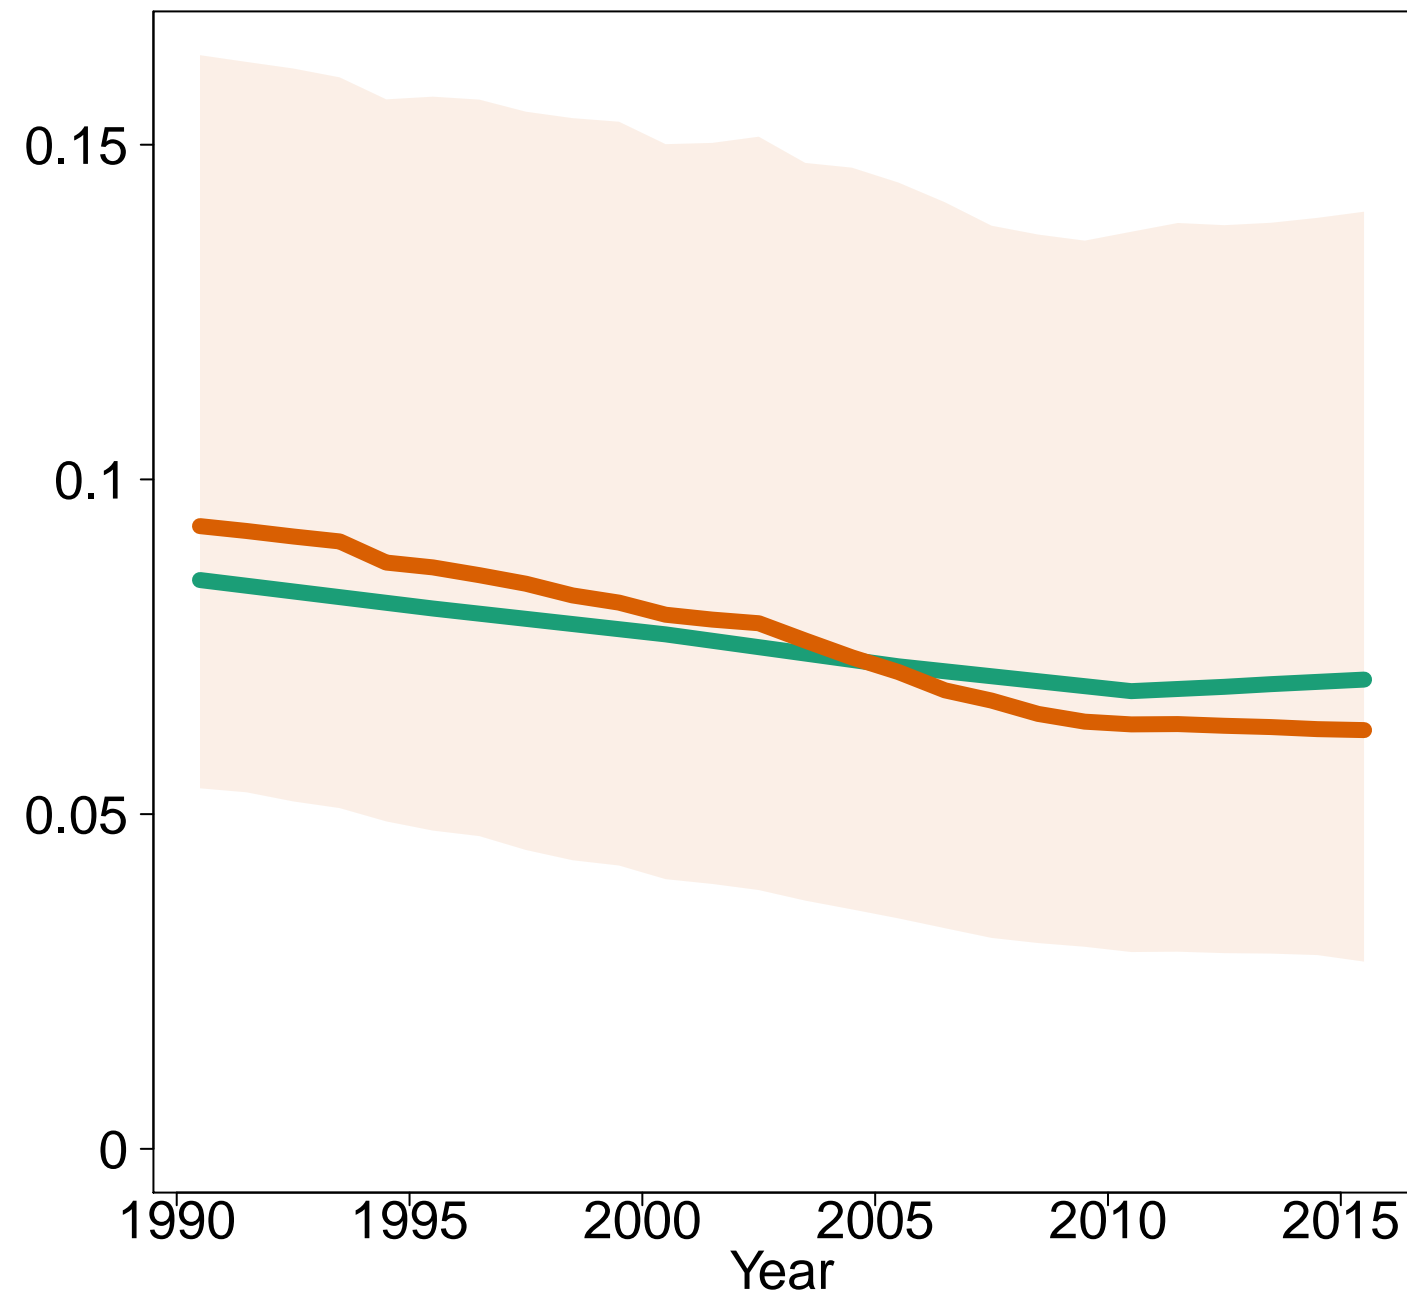

Vanuatu [VUT; C]  
(South-Eastern Asia / Oceania)

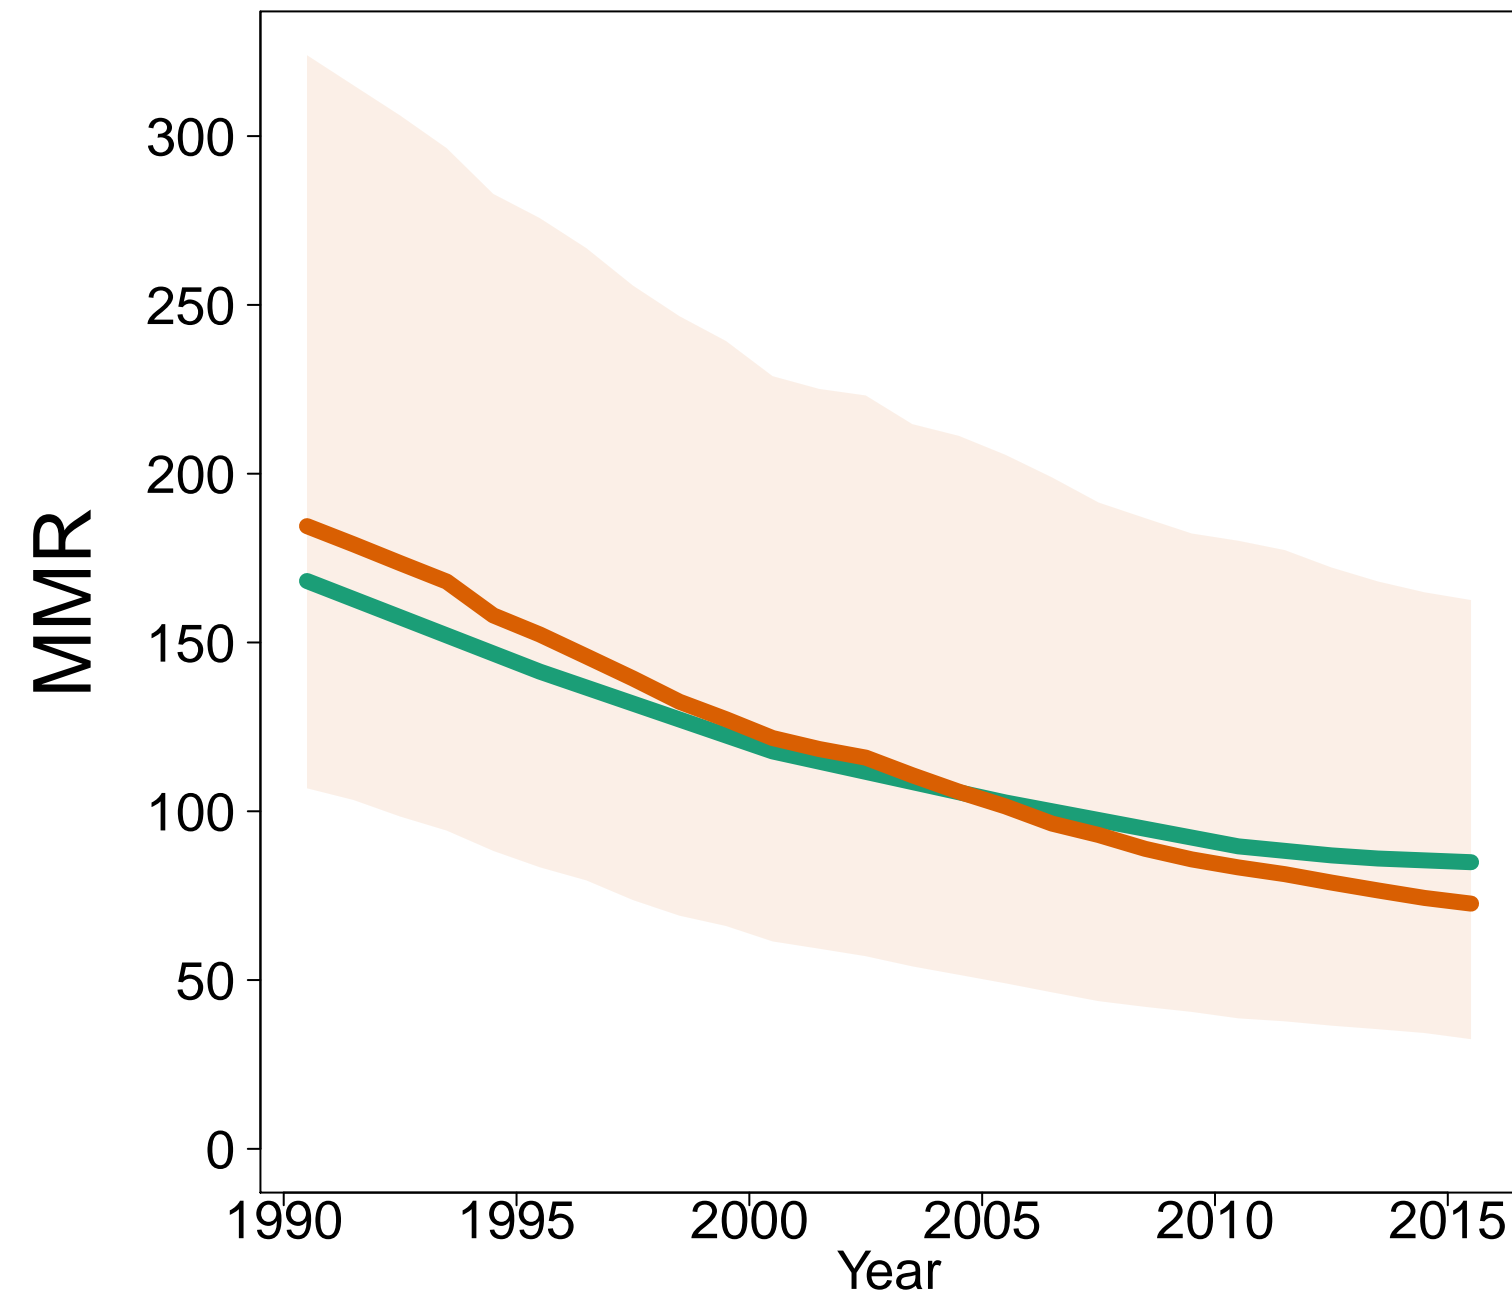

– Estimates –  
Bmat 2014  
MMEIG 2014  
– Data –

Venezuela [VEN; A]  
(South America)

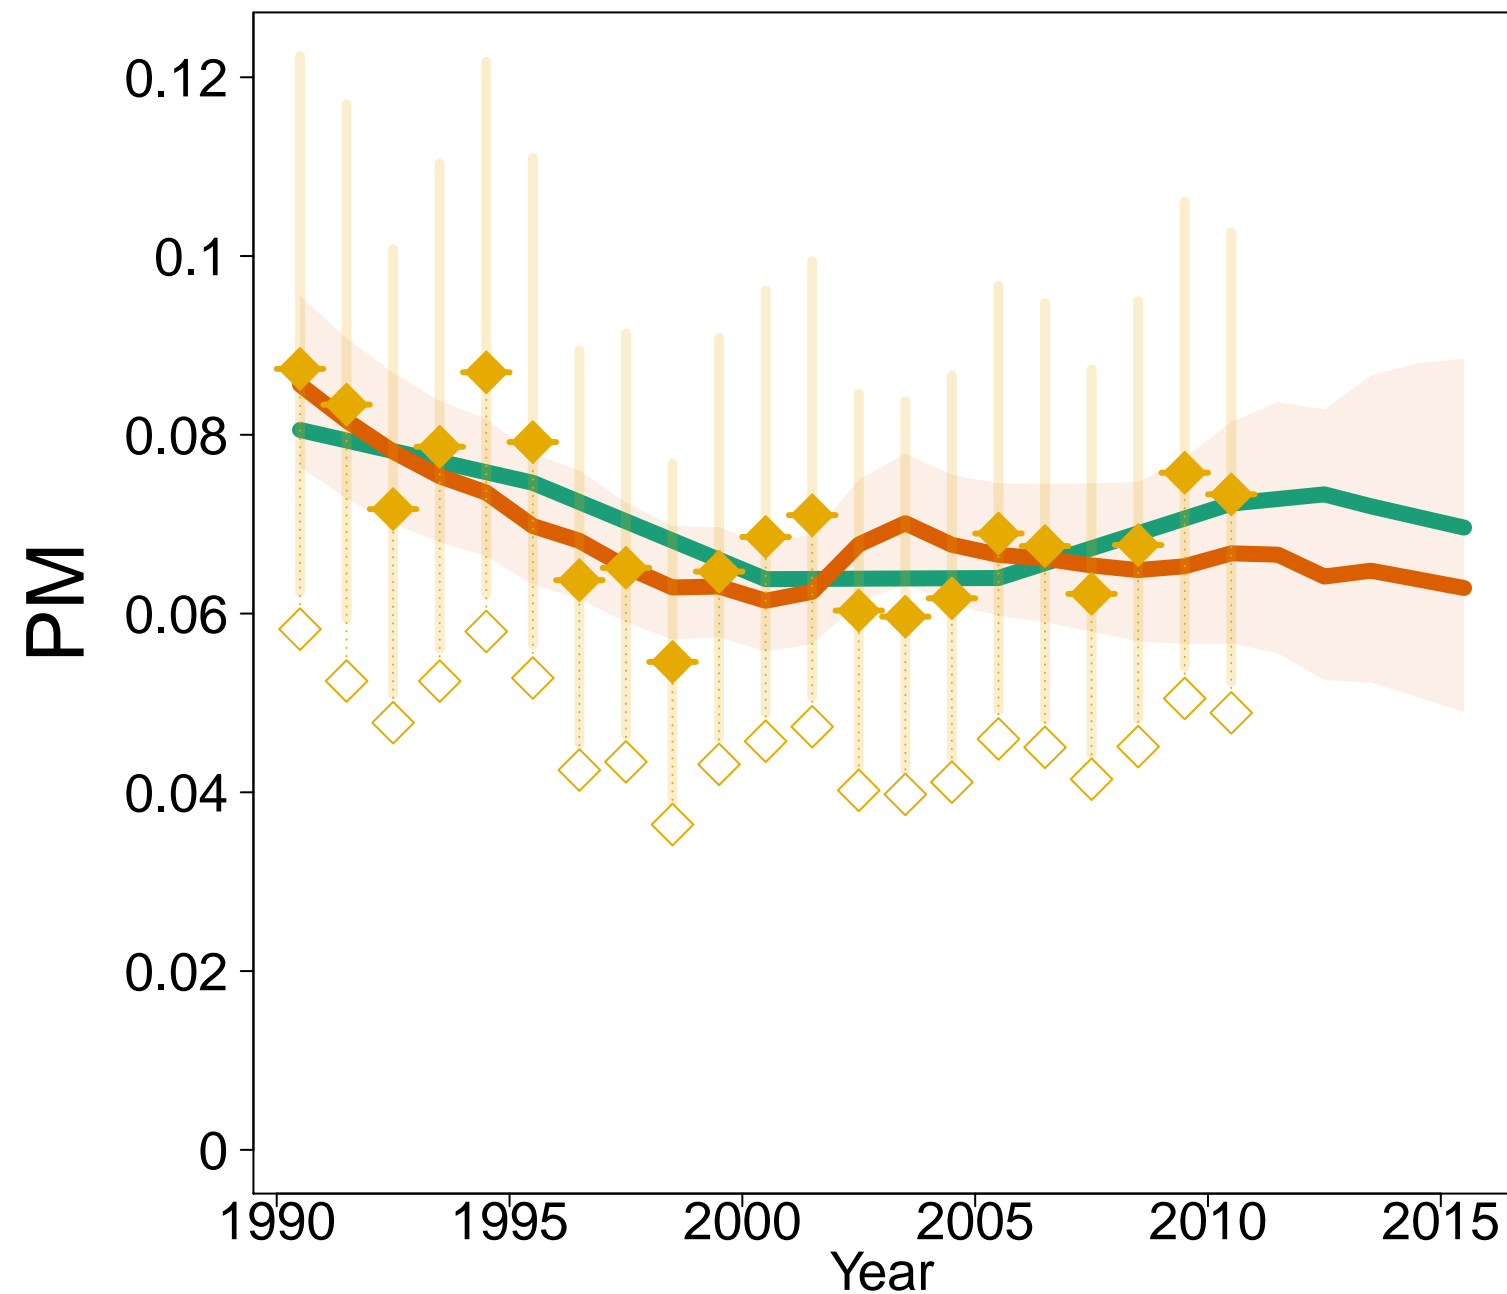

Venezuela [VEN; A]  
(South America)

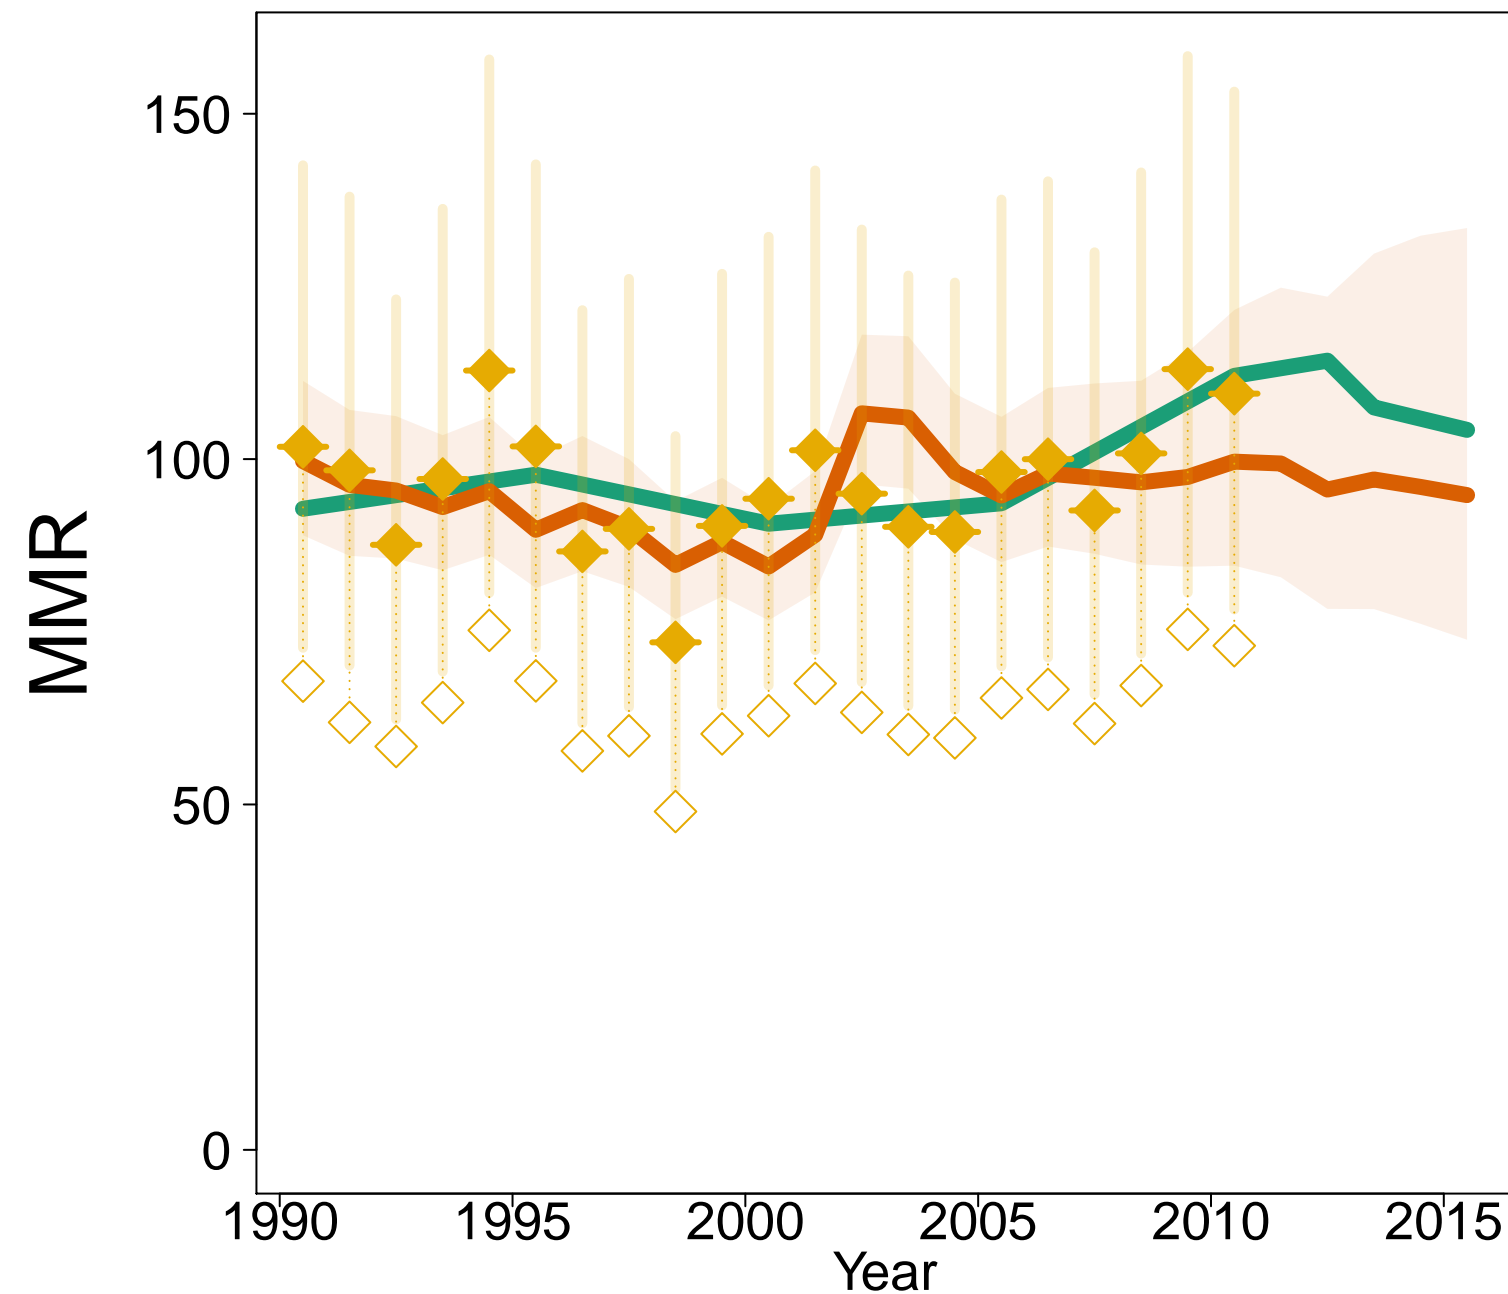

- Estimates –
- Bmat 2014
- MMEIG 2014
- Data –
- Observed Data
- Adjusted Data
- Data type –
- VR

Viet Nam [VNM; B]  
(South-Eastern Asia / Oceania)

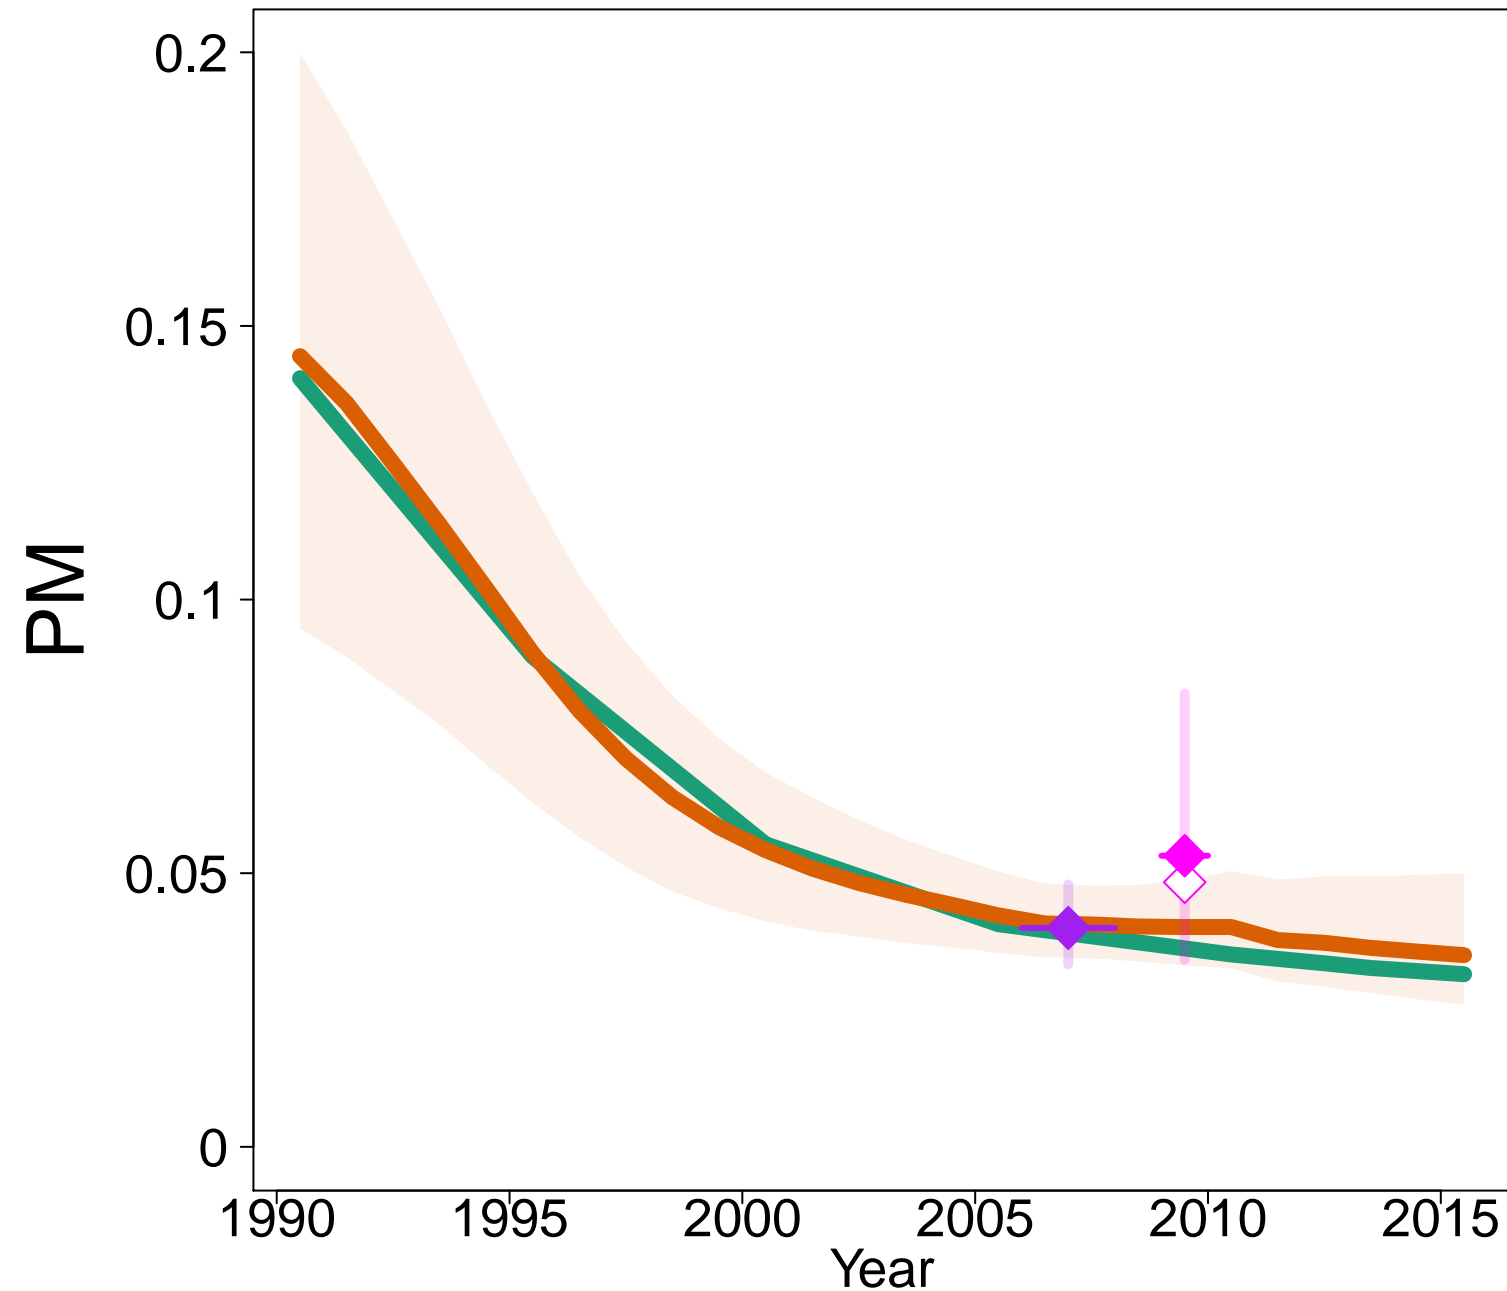

Viet Nam [VNM; B]  
(South-Eastern Asia / Oceania)

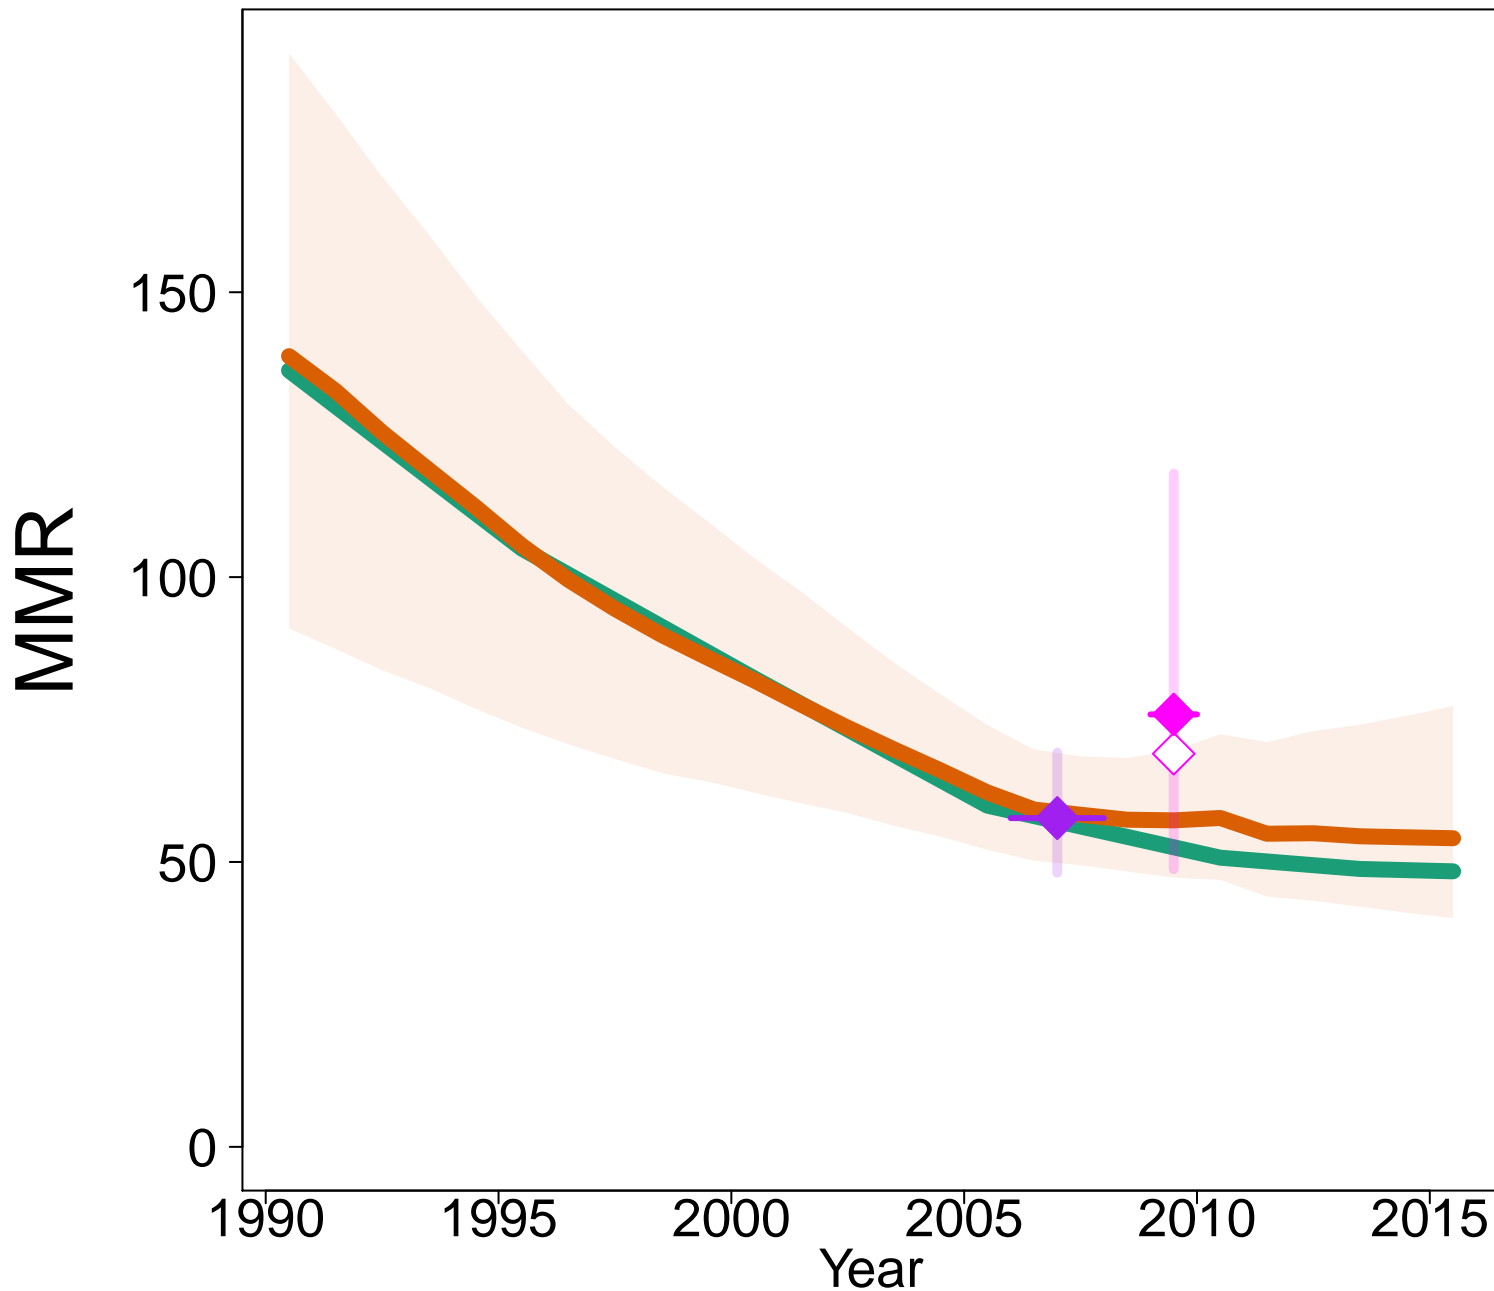

- Estimates –
- Bmat 2014
- MMEIG 2014
- Data –
- Observed Data
- Adjusted Data
- Data type –
- Spec. studies
- Census

Yemen [YEM; B]  
(Western Asia)

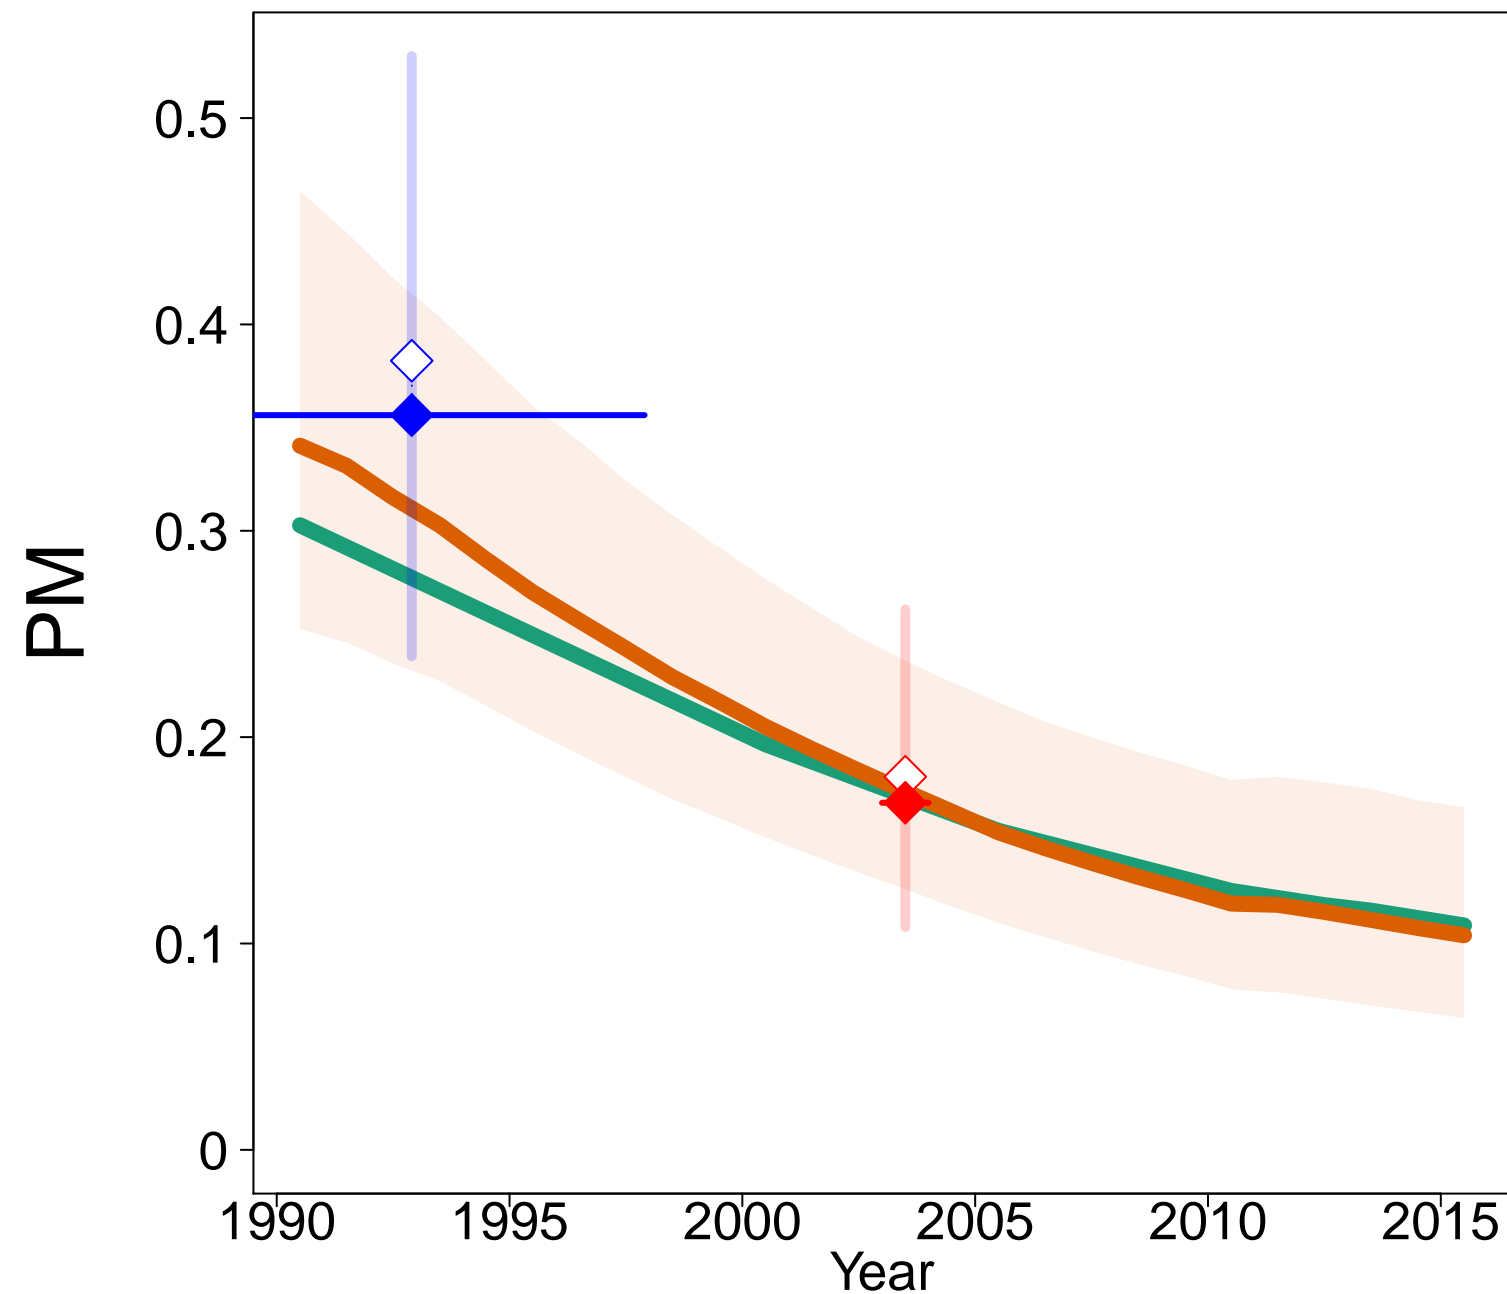

Yemen [YEM; B]  
(Western Asia)

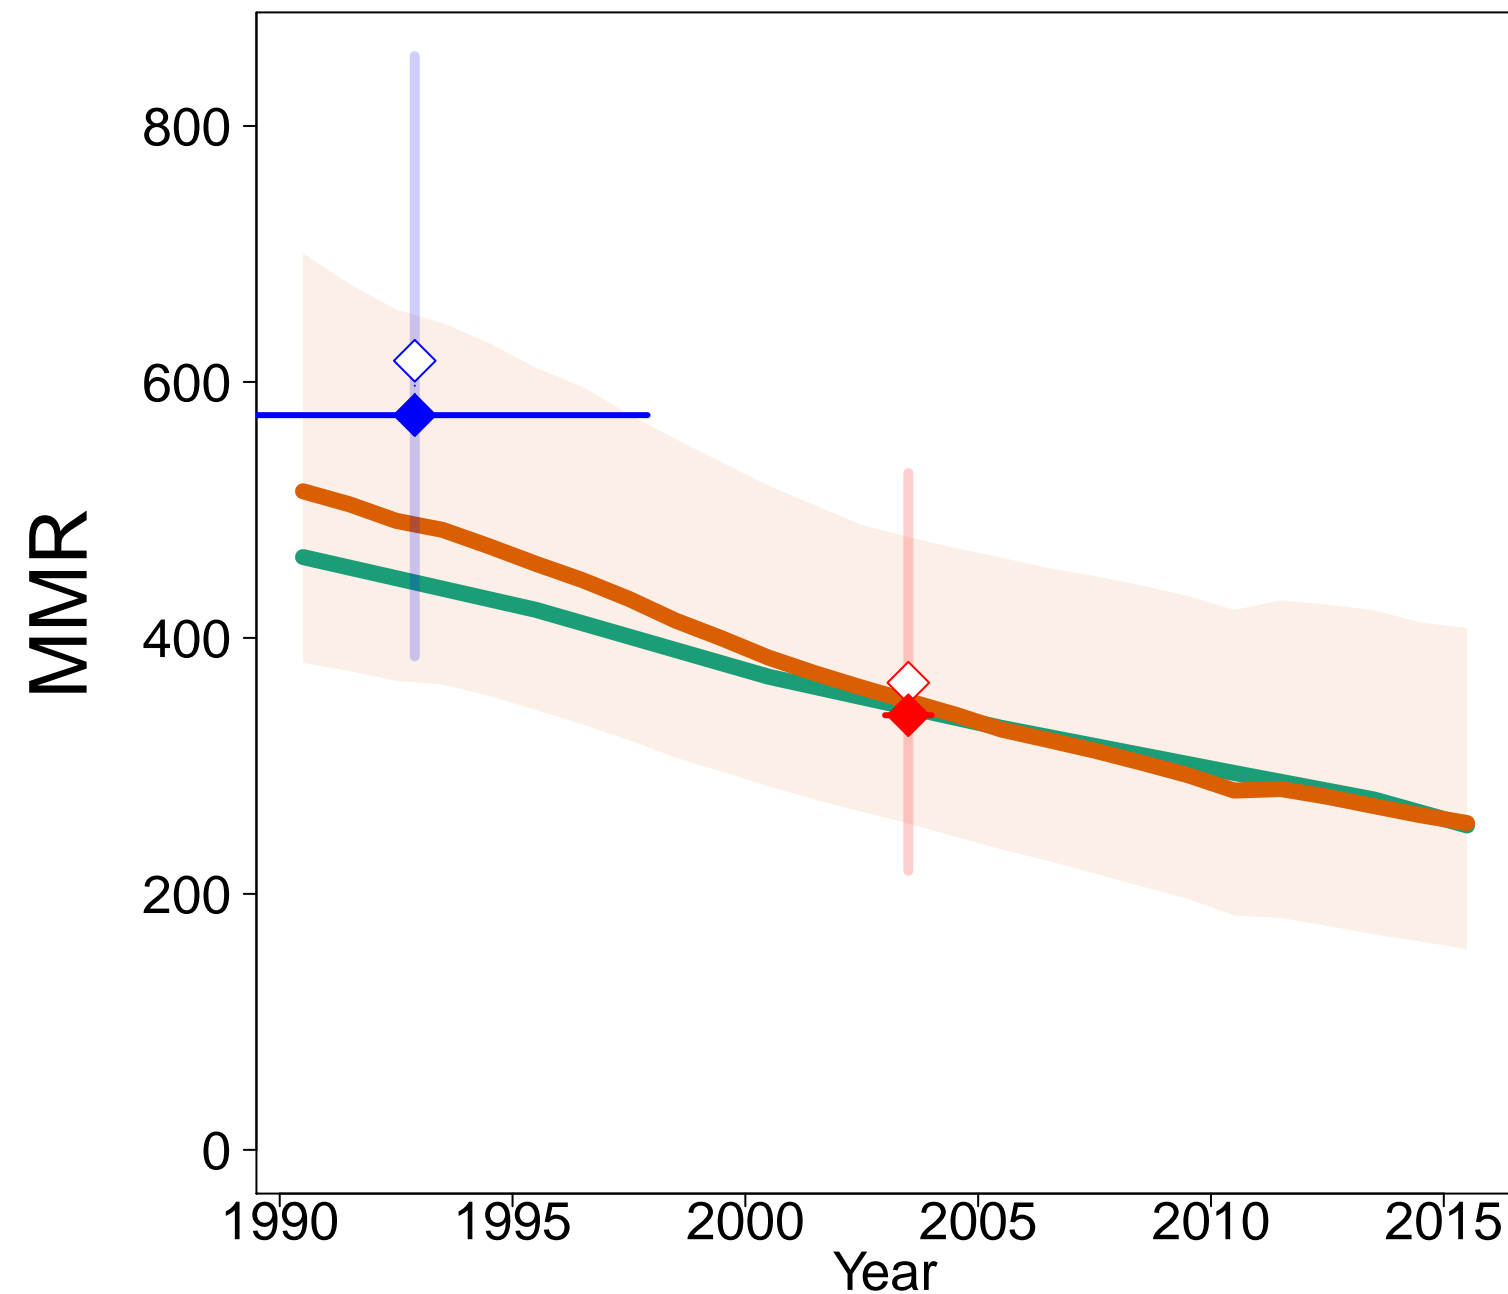

- Estimates –
- Bmat 2014
- MMEIG 2014
- Data –
- ◊ Observed Data
- ◆ Adjusted Data
- Data type –
- ◆ DHS
- ◆ Misc. studies

Zambia [ZMB; B]  
(Eastern Africa)

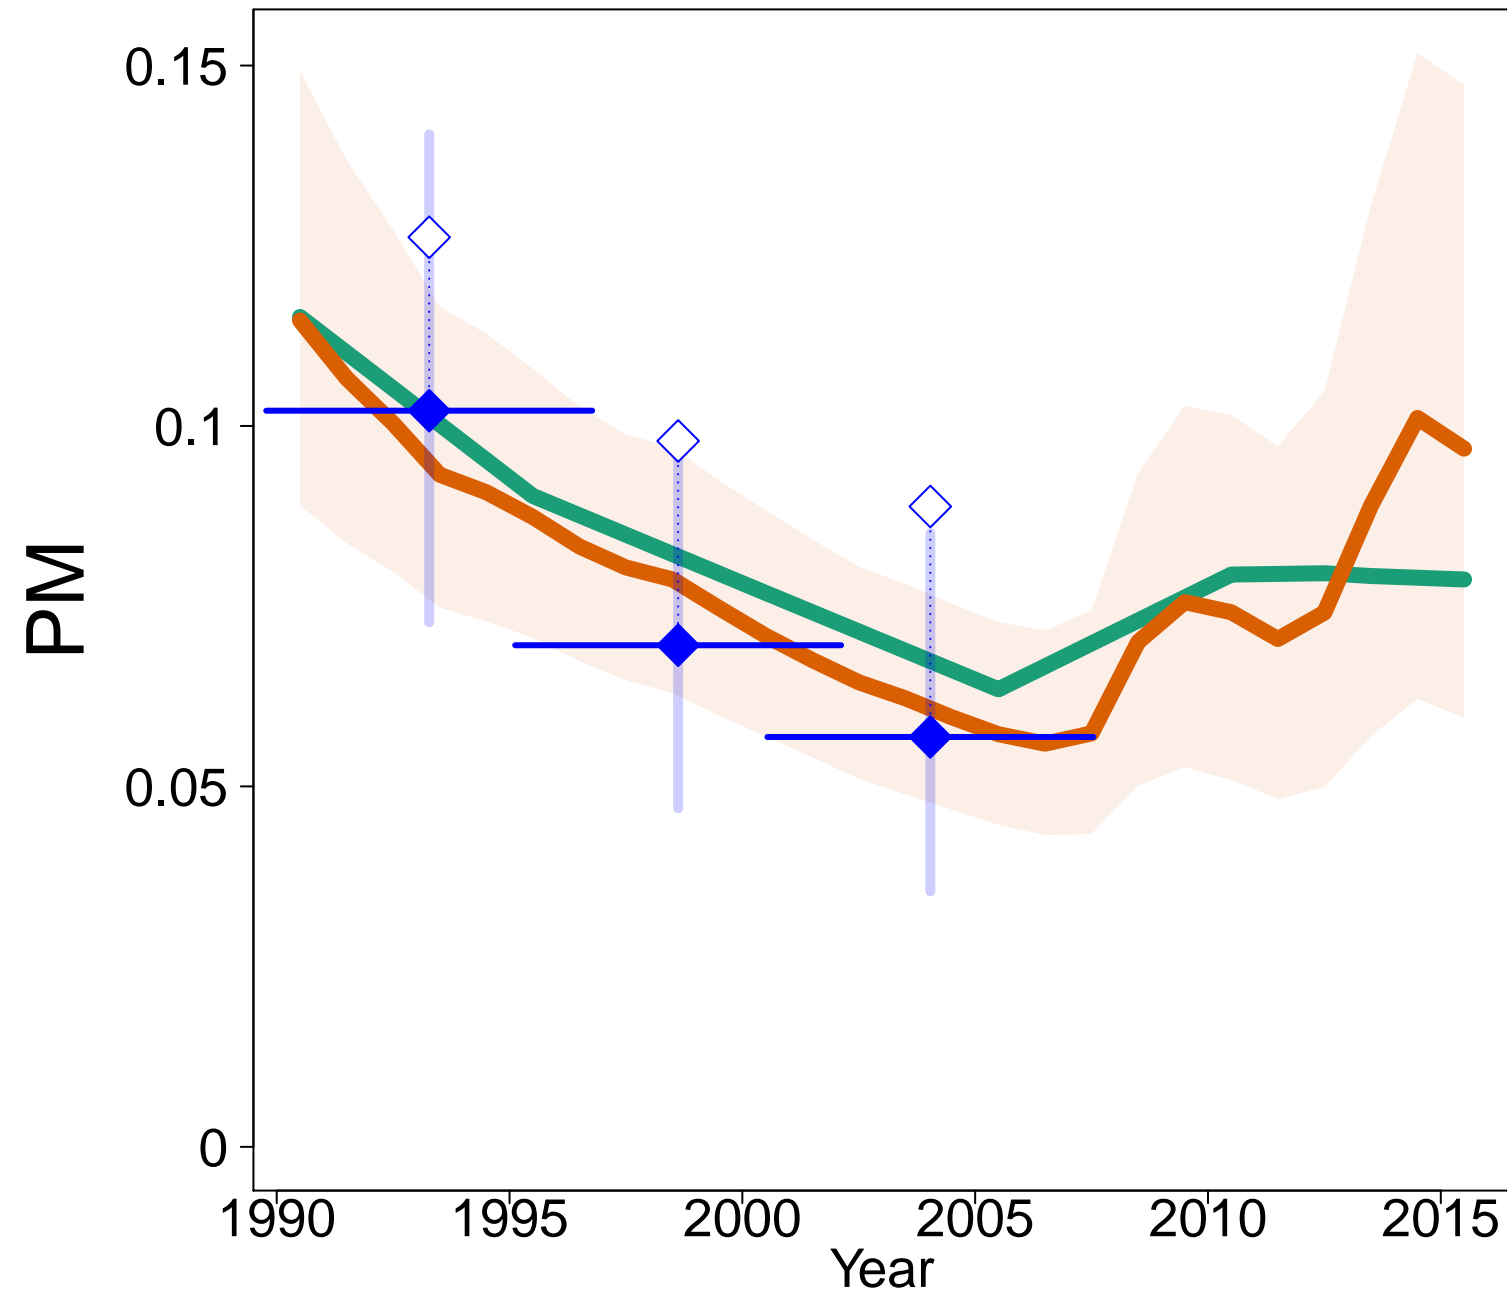

Zambia [ZMB; B]  
(Eastern Africa)

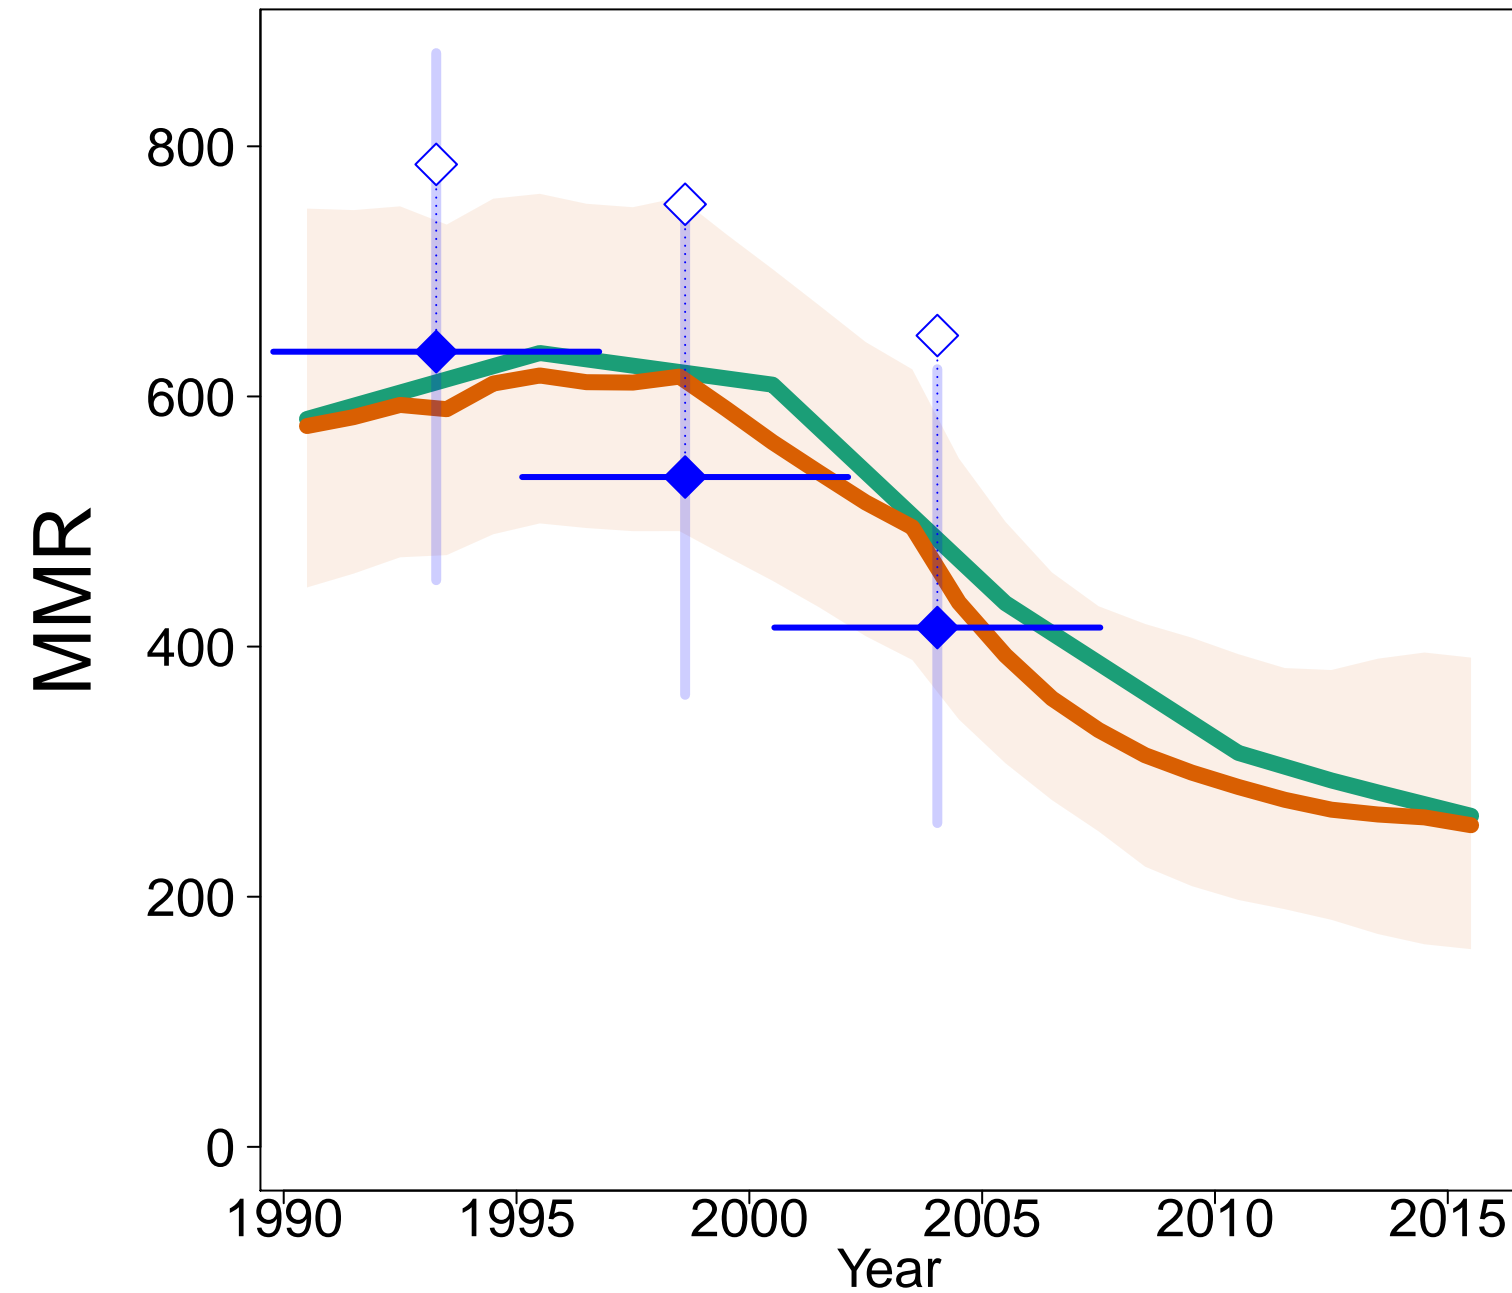

– Estimates –  
Bmat 2014  
MMEIG 2014  
– Data –  
Observed Data  
Adjusted Data  
– Data type –  
DHS

Zimbabwe [ZWE; B]  
(Eastern Africa)

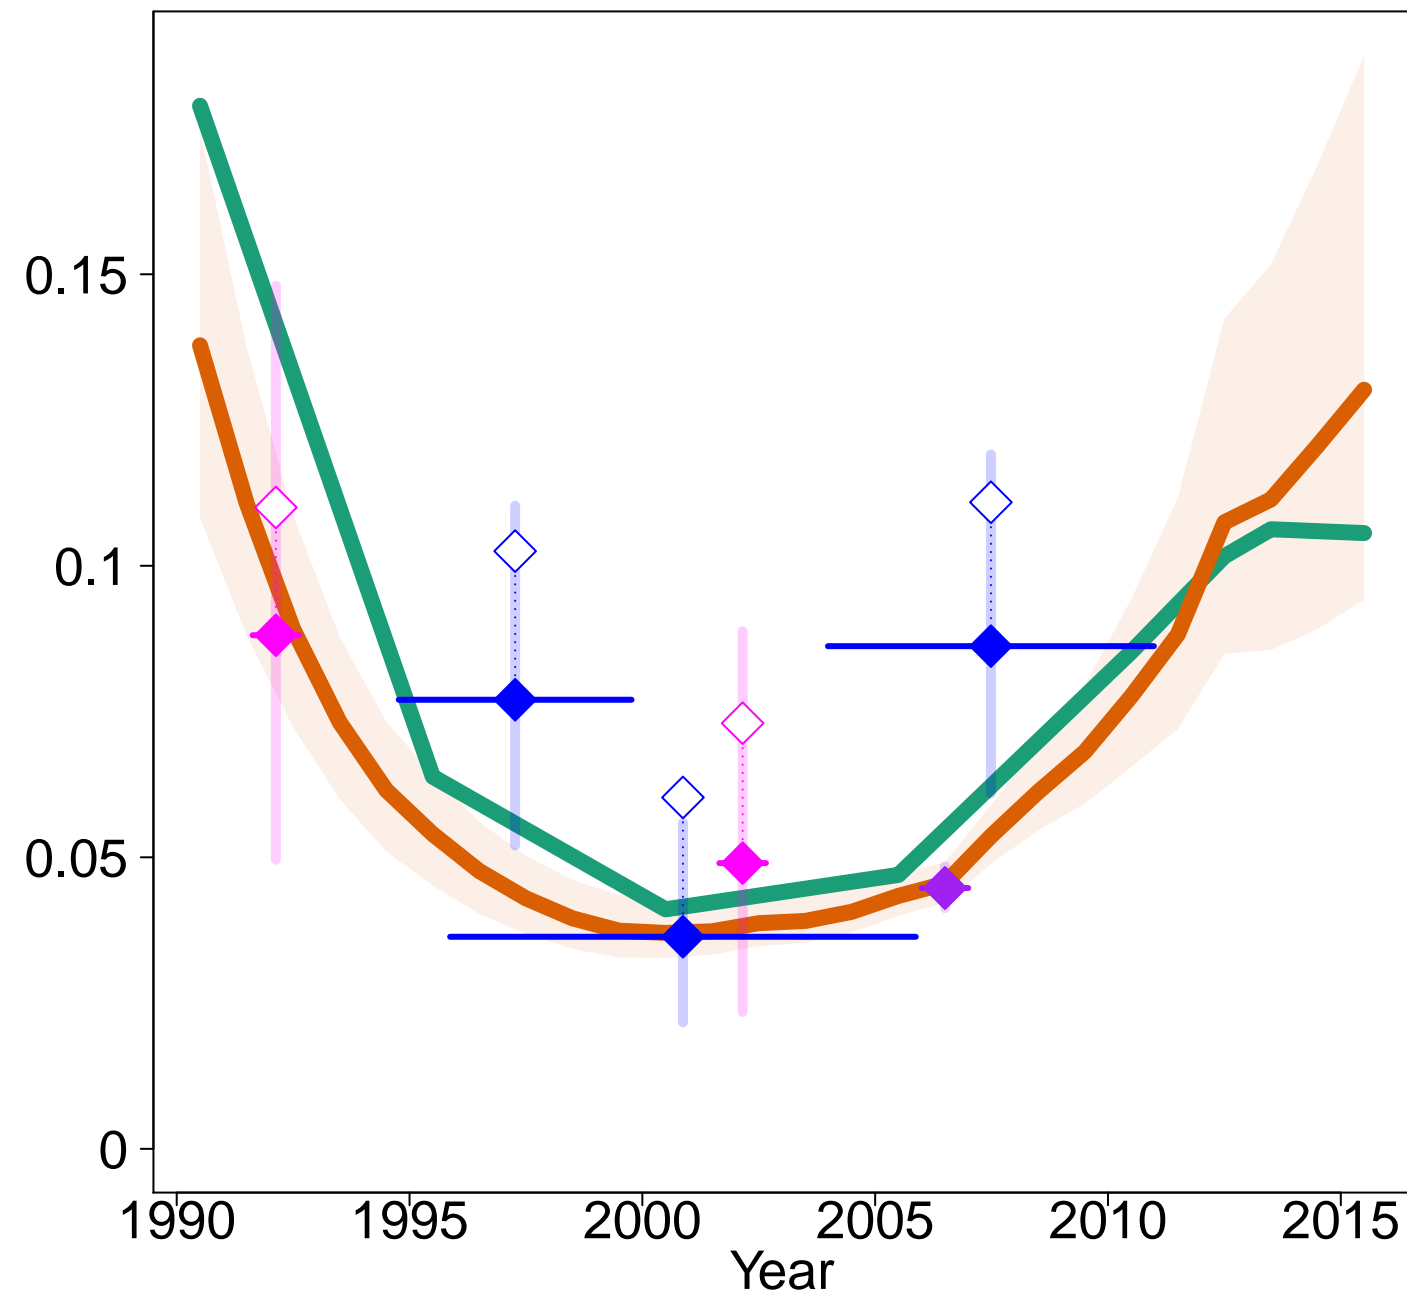

Zimbabwe [ZWE; B]  
(Eastern Africa)

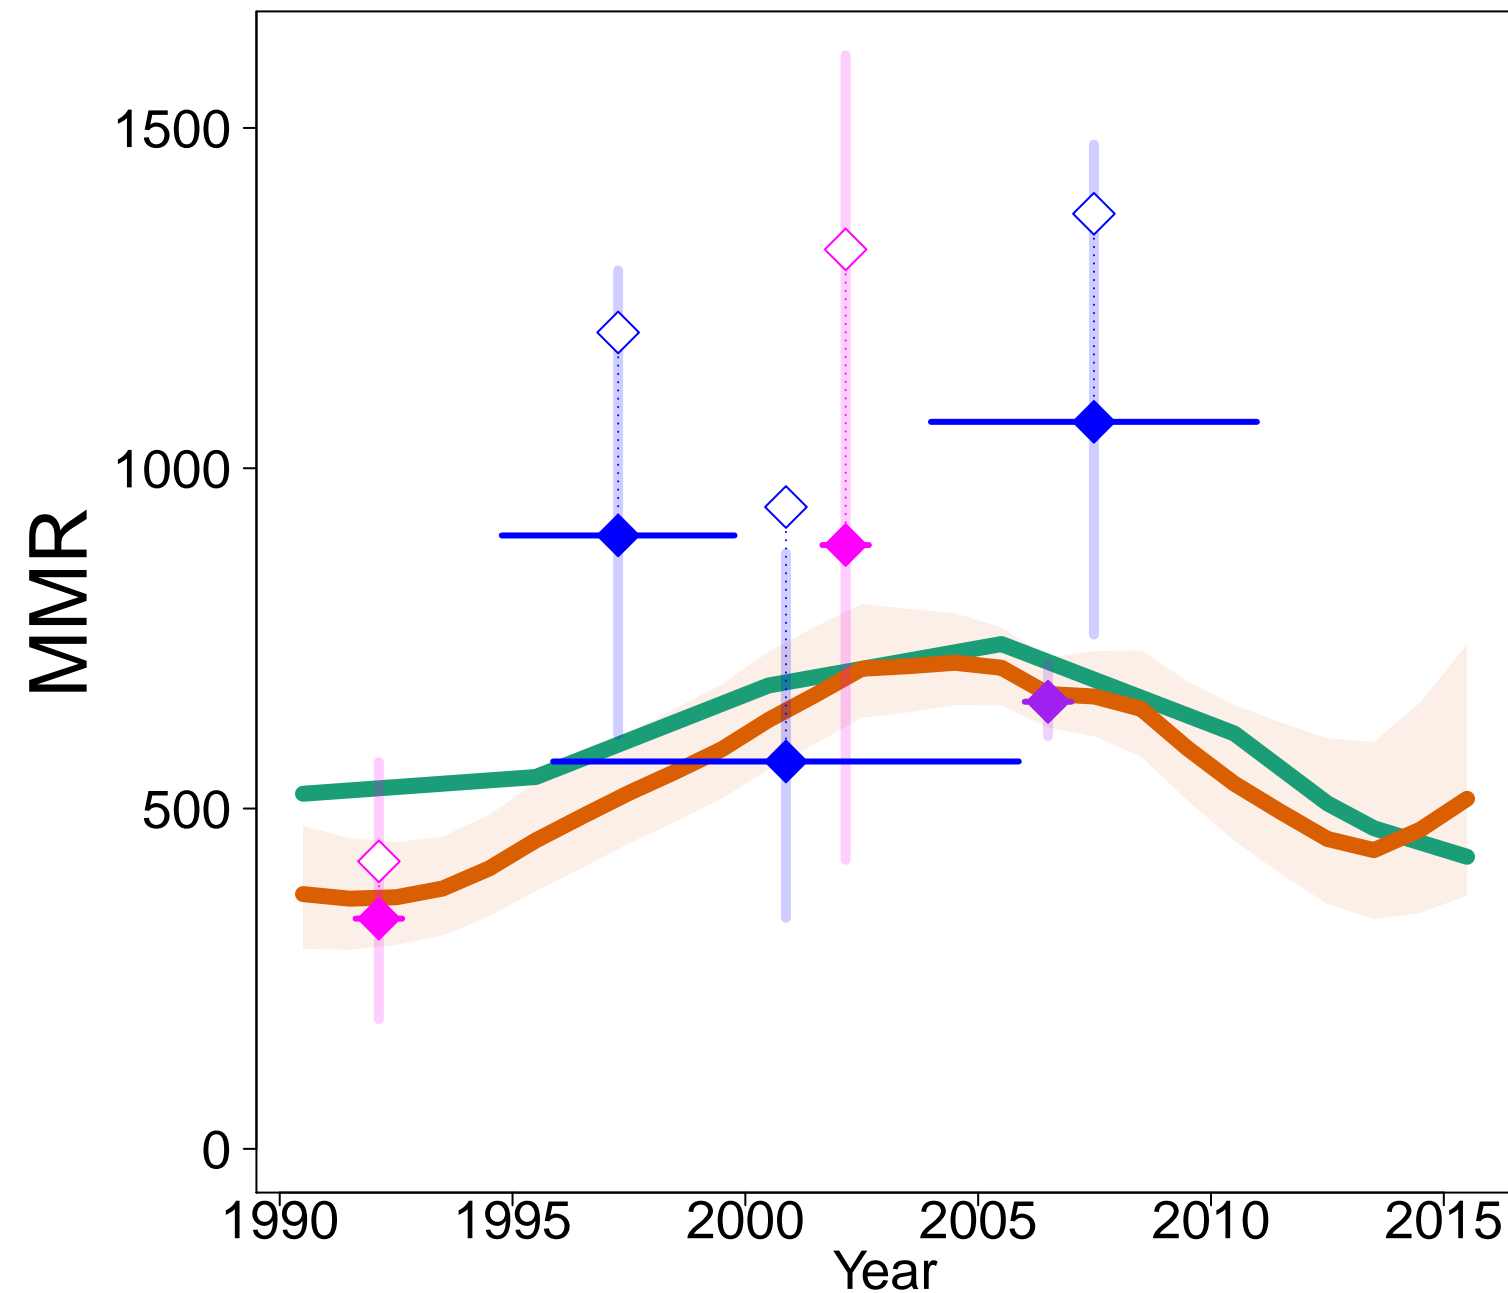

- Estimates –
- Bmat 2014
- MMEIG 2014
- Data –
- Observed Data
- Adjusted Data
- Data type –
- Spec. studies
- DHS
- Census
